# Supplementary material for: Fermi-surface diagnosis for topological superconductivity with $s$-wave-like pairing symmetries
Source: arXiv:2407.20231 ancillary file (2025-07-10)
Supplement: Supplementary file 1 [file SM2.pdf]

**Supplementary Materials II for “Fermi-surface  
diagnosis for  $s$ -wave-like topological  
superconductivity”**

**CONTENTS**

|                         |    |                         |     |
|-------------------------|----|-------------------------|-----|
| S1. Space group No. 1   | 7  | S28. Space group No. 28 | 49  |
| S2. Space group No. 2   | 8  | S29. Space group No. 29 | 52  |
| S3. Space group No. 3   | 8  | S30. Space group No. 30 | 55  |
| S4. Space group No. 4   | 10 | S31. Space group No. 31 | 58  |
| S5. Space group No. 5   | 11 | S32. Space group No. 32 | 60  |
| S6. Space group No. 6   | 12 | S33. Space group No. 33 | 63  |
| S7. Space group No. 7   | 14 | S34. Space group No. 34 | 65  |
| S8. Space group No. 8   | 16 | S35. Space group No. 35 | 68  |
| S9. Space group No. 9   | 17 | S36. Space group No. 36 | 70  |
| S10. Space group No. 10 | 18 | S37. Space group No. 37 | 71  |
| S11. Space group No. 11 | 19 | S38. Space group No. 38 | 73  |
| S12. Space group No. 12 | 20 | S39. Space group No. 39 | 75  |
| S13. Space group No. 13 | 21 | S40. Space group No. 40 | 76  |
| S14. Space group No. 14 | 22 | S41. Space group No. 41 | 78  |
| S15. Space group No. 15 | 24 | S42. Space group No. 42 | 80  |
| S16. Space group No. 16 | 25 | S43. Space group No. 43 | 82  |
| S17. Space group No. 17 | 28 | S44. Space group No. 44 | 84  |
| S18. Space group No. 18 | 30 | S45. Space group No. 45 | 85  |
| S19. Space group No. 19 | 32 | S46. Space group No. 46 | 87  |
| S20. Space group No. 20 | 35 | S47. Space group No. 47 | 88  |
| S21. Space group No. 21 | 36 | S48. Space group No. 48 | 89  |
| S22. Space group No. 22 | 38 | S49. Space group No. 49 | 92  |
| S23. Space group No. 23 | 40 | S50. Space group No. 50 | 94  |
| S24. Space group No. 24 | 42 | S51. Space group No. 51 | 96  |
| S25. Space group No. 25 | 43 | S52. Space group No. 52 | 97  |
| S26. Space group No. 26 | 45 | S53. Space group No. 53 | 99  |
| S27. Space group No. 27 | 47 | S54. Space group No. 54 | 101 |
|                         |    | S55. Space group No. 55 | 103 |
|                         |    | S56. Space group No. 56 | 105 |
|                         |    | S57. Space group No. 57 | 106 |
|                         |    | S58. Space group No. 58 | 109 |

|                         |     |                           |     |
|-------------------------|-----|---------------------------|-----|
| S59. Space group No. 59 | 111 | S90. Space group No. 90   | 151 |
| S60. Space group No. 60 | 112 | S91. Space group No. 91   | 154 |
| S61. Space group No. 61 | 115 | S92. Space group No. 92   | 156 |
| S62. Space group No. 62 | 118 | S93. Space group No. 93   | 158 |
| S63. Space group No. 63 | 119 | S94. Space group No. 94   | 161 |
| S64. Space group No. 64 | 121 | S95. Space group No. 95   | 163 |
| S65. Space group No. 65 | 122 | S96. Space group No. 96   | 165 |
| S66. Space group No. 66 | 123 | S97. Space group No. 97   | 167 |
| S67. Space group No. 67 | 124 | S98. Space group No. 98   | 169 |
| S68. Space group No. 68 | 125 | S99. Space group No. 99   | 170 |
| S69. Space group No. 69 | 127 | S100. Space group No. 100 | 172 |
| S70. Space group No. 70 | 127 | S101. Space group No. 101 | 175 |
| S71. Space group No. 71 | 129 | S102. Space group No. 102 | 176 |
| S72. Space group No. 72 | 130 | S103. Space group No. 103 | 179 |
| S73. Space group No. 73 | 131 | S104. Space group No. 104 | 181 |
| S74. Space group No. 74 | 132 | S105. Space group No. 105 | 183 |
| S75. Space group No. 75 | 133 | S106. Space group No. 106 | 185 |
| S76. Space group No. 76 | 135 | S107. Space group No. 107 | 187 |
| S77. Space group No. 77 | 136 | S108. Space group No. 108 | 188 |
| S78. Space group No. 78 | 138 | S109. Space group No. 109 | 190 |
| S79. Space group No. 79 | 139 | S110. Space group No. 110 | 191 |
| S80. Space group No. 80 | 140 | S111. Space group No. 111 | 193 |
| S81. Space group No. 81 | 141 | S112. Space group No. 112 | 195 |
| S82. Space group No. 82 | 142 | S113. Space group No. 113 | 197 |
| S83. Space group No. 83 | 143 | S114. Space group No. 114 | 199 |
| S84. Space group No. 84 | 144 | S115. Space group No. 115 | 200 |
| S85. Space group No. 85 | 145 | S116. Space group No. 116 | 202 |
| S86. Space group No. 86 | 146 | S117. Space group No. 117 | 204 |
| S87. Space group No. 87 | 147 | S118. Space group No. 118 | 205 |
| S88. Space group No. 88 | 148 | S119. Space group No. 119 | 208 |
| S89. Space group No. 89 | 149 | S120. Space group No. 120 | 209 |

|                           |     |                           |     |
|---------------------------|-----|---------------------------|-----|
| S121. Space group No. 121 | 210 | S152. Space group No. 152 | 249 |
| S122. Space group No. 122 | 212 | S153. Space group No. 153 | 251 |
| S123. Space group No. 123 | 214 | S154. Space group No. 154 | 252 |
| S124. Space group No. 124 | 215 | S155. Space group No. 155 | 254 |
| S125. Space group No. 125 | 217 | S156. Space group No. 156 | 255 |
| S126. Space group No. 126 | 218 | S157. Space group No. 157 | 256 |
| S127. Space group No. 127 | 220 | S158. Space group No. 158 | 258 |
| S128. Space group No. 128 | 221 | S159. Space group No. 159 | 260 |
| S129. Space group No. 129 | 223 | S160. Space group No. 160 | 261 |
| S130. Space group No. 130 | 224 | S161. Space group No. 161 | 263 |
| S131. Space group No. 131 | 226 | S162. Space group No. 162 | 264 |
| S132. Space group No. 132 | 227 | S163. Space group No. 163 | 265 |
| S133. Space group No. 133 | 228 | S164. Space group No. 164 | 266 |
| S134. Space group No. 134 | 230 | S165. Space group No. 165 | 266 |
| S135. Space group No. 135 | 232 | S166. Space group No. 166 | 268 |
| S136. Space group No. 136 | 233 | S167. Space group No. 167 | 268 |
| S137. Space group No. 137 | 234 | S168. Space group No. 168 | 269 |
| S138. Space group No. 138 | 236 | S169. Space group No. 169 | 271 |
| S139. Space group No. 139 | 237 | S170. Space group No. 170 | 272 |
| S140. Space group No. 140 | 238 | S171. Space group No. 171 | 273 |
| S141. Space group No. 141 | 239 | S172. Space group No. 172 | 274 |
| S142. Space group No. 142 | 240 | S173. Space group No. 173 | 276 |
| S143. Space group No. 143 | 241 | S174. Space group No. 174 | 278 |
| S144. Space group No. 144 | 242 | S175. Space group No. 175 | 279 |
| S145. Space group No. 145 | 243 | S176. Space group No. 176 | 280 |
| S146. Space group No. 146 | 243 | S177. Space group No. 177 | 281 |
| S147. Space group No. 147 | 244 | S178. Space group No. 178 | 283 |
| S148. Space group No. 148 | 245 | S179. Space group No. 179 | 286 |
| S149. Space group No. 149 | 245 | S180. Space group No. 180 | 288 |
| S150. Space group No. 150 | 247 | S181. Space group No. 181 | 290 |
| S151. Space group No. 151 | 248 | S182. Space group No. 182 | 293 |

|                           |     |                           |     |
|---------------------------|-----|---------------------------|-----|
| S183. Space group No. 183 | 295 | S214. Space group No. 214 | 338 |
| S184. Space group No. 184 | 297 | S215. Space group No. 215 | 340 |
| S185. Space group No. 185 | 299 | S216. Space group No. 216 | 341 |
| S186. Space group No. 186 | 301 | S217. Space group No. 217 | 342 |
| S187. Space group No. 187 | 303 | S218. Space group No. 218 | 343 |
| S188. Space group No. 188 | 304 | S219. Space group No. 219 | 344 |
| S189. Space group No. 189 | 306 | S220. Space group No. 220 | 346 |
| S190. Space group No. 190 | 308 | S221. Space group No. 221 | 347 |
| S191. Space group No. 191 | 310 | S222. Space group No. 222 | 348 |
| S192. Space group No. 192 | 311 | S223. Space group No. 223 | 349 |
| S193. Space group No. 193 | 313 | S224. Space group No. 224 | 350 |
| S194. Space group No. 194 | 314 | S225. Space group No. 225 | 351 |
| S195. Space group No. 195 | 315 | S226. Space group No. 226 | 352 |
| S196. Space group No. 196 | 317 | S227. Space group No. 227 | 353 |
| S197. Space group No. 197 | 318 | S228. Space group No. 228 | 353 |
| S198. Space group No. 198 | 319 | S229. Space group No. 229 | 354 |
| S199. Space group No. 199 | 320 | S230. Space group No. 230 | 355 |
| S200. Space group No. 200 | 321 | L1. Layer group No. 1     | 357 |
| S201. Space group No. 201 | 322 | L2. Layer group No. 2     | 357 |
| S202. Space group No. 202 | 323 | L3. Layer group No. 3     | 357 |
| S203. Space group No. 203 | 323 | L4. Layer group No. 4     | 358 |
| S204. Space group No. 204 | 324 | L5. Layer group No. 5     | 358 |
| S205. Space group No. 205 | 324 | L6. Layer group No. 6     | 359 |
| S206. Space group No. 206 | 325 | L7. Layer group No. 7     | 359 |
| S207. Space group No. 207 | 326 | L8. Layer group No. 8     | 360 |
| S208. Space group No. 208 | 328 | L9. Layer group No. 9     | 361 |
| S209. Space group No. 209 | 330 | L10. Layer group No. 10   | 361 |
| S210. Space group No. 210 | 332 | L11. Layer group No. 11   | 362 |
| S211. Space group No. 211 | 333 | L12. Layer group No. 12   | 362 |
| S212. Space group No. 212 | 335 | L13. Layer group No. 13   | 363 |
| S213. Space group No. 213 | 337 | L14. Layer group No. 14   | 364 |

|                         |     |                         |     |
|-------------------------|-----|-------------------------|-----|
| L15. Layer group No. 15 | 364 | L46. Layer group No. 46 | 383 |
| L16. Layer group No. 16 | 365 | L47. Layer group No. 47 | 384 |
| L17. Layer group No. 17 | 365 | L48. Layer group No. 48 | 385 |
| L18. Layer group No. 18 | 366 | L49. Layer group No. 49 | 385 |
| L19. Layer group No. 19 | 366 | L50. Layer group No. 50 | 385 |
| L20. Layer group No. 20 | 367 | L51. Layer group No. 51 | 386 |
| L21. Layer group No. 21 | 368 | L52. Layer group No. 52 | 386 |
| L22. Layer group No. 22 | 368 | L53. Layer group No. 53 | 386 |
| L23. Layer group No. 23 | 369 | L54. Layer group No. 54 | 387 |
| L24. Layer group No. 24 | 370 | L55. Layer group No. 55 | 387 |
| L25. Layer group No. 25 | 371 | L56. Layer group No. 56 | 388 |
| L26. Layer group No. 26 | 371 | L57. Layer group No. 57 | 389 |
| L27. Layer group No. 27 | 372 | L58. Layer group No. 58 | 389 |
| L28. Layer group No. 28 | 373 | L59. Layer group No. 59 | 390 |
| L29. Layer group No. 29 | 373 | L60. Layer group No. 60 | 390 |
| L30. Layer group No. 30 | 374 | L61. Layer group No. 61 | 391 |
| L31. Layer group No. 31 | 374 | L62. Layer group No. 62 | 391 |
| L32. Layer group No. 32 | 375 | L63. Layer group No. 63 | 392 |
| L33. Layer group No. 33 | 376 | L64. Layer group No. 64 | 392 |
| L34. Layer group No. 34 | 377 | L65. Layer group No. 65 | 393 |
| L35. Layer group No. 35 | 378 | L66. Layer group No. 66 | 393 |
| L36. Layer group No. 36 | 378 | L67. Layer group No. 67 | 393 |
| L37. Layer group No. 37 | 379 | L68. Layer group No. 68 | 394 |
| L38. Layer group No. 38 | 379 | L69. Layer group No. 69 | 394 |
| L39. Layer group No. 39 | 380 | L70. Layer group No. 70 | 395 |
| L40. Layer group No. 40 | 381 | L71. Layer group No. 71 | 395 |
| L41. Layer group No. 41 | 381 | L72. Layer group No. 72 | 396 |
| L42. Layer group No. 42 | 381 | L73. Layer group No. 73 | 396 |
| L43. Layer group No. 43 | 382 | L74. Layer group No. 74 | 396 |
| L44. Layer group No. 44 | 383 | L75. Layer group No. 75 | 397 |
| L45. Layer group No. 45 | 383 | L76. Layer group No. 76 | 397 |

|                         |     |
|-------------------------|-----|
| L77. Layer group No. 77 | 398 |
| L78. Layer group No. 78 | 398 |
| L79. Layer group No. 79 | 399 |
| L80. Layer group No. 80 | 399 |

# S1. SPACE GROUP NO. 1

| line segment                                               | character of irrep (generators only)                   |
|------------------------------------------------------------|--------------------------------------------------------|
| $a \left( \frac{t}{2}, 0, 0 \right)$                       | $a_1 \begin{Bmatrix} 1 & 0 & 0 & 0 \\ 1 \end{Bmatrix}$ |
| $b \left( \frac{1}{2}, \frac{t}{2}, 0 \right)$             | $b_1 \begin{Bmatrix} 1 & 0 & 0 & 0 \\ 1 \end{Bmatrix}$ |
| $c \left( \frac{1-t}{2}, \frac{1}{2}, 0 \right)$           | $c_1 \begin{Bmatrix} 1 & 0 & 0 & 0 \\ 1 \end{Bmatrix}$ |
| $d \left( \frac{t}{2}, 0, \frac{1}{2} \right)$             | $d_1 \begin{Bmatrix} 1 & 0 & 0 & 0 \\ 1 \end{Bmatrix}$ |
| $e \left( \frac{1}{2}, \frac{t}{2}, \frac{1}{2} \right)$   | $e_1 \begin{Bmatrix} 1 & 0 & 0 & 0 \\ 1 \end{Bmatrix}$ |
| $f \left( \frac{1-t}{2}, \frac{1}{2}, \frac{1}{2} \right)$ | $f_1 \begin{Bmatrix} 1 & 0 & 0 & 0 \\ 1 \end{Bmatrix}$ |
| $g \left( \frac{1}{2}, \frac{1}{2}, \frac{t}{2} \right)$   | $g_1 \begin{Bmatrix} 1 & 0 & 0 & 0 \\ 1 \end{Bmatrix}$ |

$$\mathcal{X}_1 = \sum_{m=1}^{n_{a_1}} \frac{1 - \text{sgn}(\delta_m^{a_1})}{2} + \sum_{m=1}^{n_{b_1}} \frac{1 - \text{sgn}(\delta_m^{b_1})}{2} + \sum_{m=1}^{n_{f_1}} \frac{1 - \text{sgn}(\delta_m^{f_1})}{2} + \sum_{m=1}^{n_{g_1}} \frac{1 - \text{sgn}(\delta_m^{g_1})}{2} \mod 2 \quad (\text{S1.1})$$

$$\mathcal{X}_2 = \sum_{m=1}^{n_{b_1}} \frac{1 - \text{sgn}(\delta_m^{b_1})}{2} + \sum_{m=1}^{n_{f_1}} \frac{1 - \text{sgn}(\delta_m^{f_1})}{2} + \sum_{m=1}^{n_{g_1}} \frac{1 - \text{sgn}(\delta_m^{g_1})}{2} \mod 2 \quad (\text{S1.2})$$

$$\mathcal{X}_3 = \sum_{m=1}^{n_{f_1}} \frac{1 - \text{sgn}(\delta_m^{f_1})}{2} + \sum_{m=1}^{n_{g_1}} \frac{1 - \text{sgn}(\delta_m^{g_1})}{2} \mod 2 \quad (\text{S1.3})$$

$$\mathcal{X}_4 = \sum_{m=1}^{n_{c_1}} \frac{1 - \text{sgn}(\delta_m^{c_1})}{2} + \sum_{m=1}^{n_{f_1}} \frac{1 - \text{sgn}(\delta_m^{f_1})}{2} + \sum_{m=1}^{n_{g_1}} \frac{1 - \text{sgn}(\delta_m^{g_1})}{2} \mod 2 \quad (\text{S1.4})$$

$$\mathcal{X}_5 = \sum_{m=1}^{n_{d_1}} \frac{1 - \text{sgn}(\delta_m^{d_1})}{2} + \sum_{m=1}^{n_{e_1}} \frac{1 - \text{sgn}(\delta_m^{e_1})}{2} + \sum_{m=1}^{n_{f_1}} \frac{1 - \text{sgn}(\delta_m^{f_1})}{2} \mod 2 \quad (\text{S1.5})$$

$$\mathcal{X}_6 = \sum_{m=1}^{n_{e_1}} \frac{1 - \text{sgn}(\delta_m^{e_1})}{2} + \sum_{m=1}^{n_{f_1}} \frac{1 - \text{sgn}(\delta_m^{f_1})}{2} \mod 2 \quad (\text{S1.6})$$

$$\mathcal{X}_7 = \sum_{m=1}^{n_{f_1}} \frac{1 - \text{sgn}(\delta_m^{f_1})}{2} \mod 2 \quad (\text{S1.7})$$

**S2. SPACE GROUP NO. 2**

| line segment                                               | character of irrep (generators only)                      |
|------------------------------------------------------------|-----------------------------------------------------------|
| $a \left( \frac{t}{2}, 0, 0 \right)$                       | $a_1 \begin{Bmatrix} \{1  0 & 0 & 0\} \\ 1 \end{Bmatrix}$ |
| $b \left( \frac{1}{2}, \frac{t}{2}, 0 \right)$             | $b_1 \begin{Bmatrix} \{1  0 & 0 & 0\} \\ 1 \end{Bmatrix}$ |
| $c \left( \frac{1-t}{2}, \frac{1}{2}, 0 \right)$           | $c_1 \begin{Bmatrix} \{1  0 & 0 & 0\} \\ 1 \end{Bmatrix}$ |
| $d \left( \frac{t}{2}, 0, \frac{1}{2} \right)$             | $d_1 \begin{Bmatrix} \{1  0 & 0 & 0\} \\ 1 \end{Bmatrix}$ |
| $e \left( \frac{1}{2}, \frac{t}{2}, \frac{1}{2} \right)$   | $e_1 \begin{Bmatrix} \{1  0 & 0 & 0\} \\ 1 \end{Bmatrix}$ |
| $f \left( \frac{1-t}{2}, \frac{1}{2}, \frac{1}{2} \right)$ | $f_1 \begin{Bmatrix} \{1  0 & 0 & 0\} \\ 1 \end{Bmatrix}$ |
| $g \left( \frac{1}{2}, \frac{1}{2}, \frac{t}{2} \right)$   | $g_1 \begin{Bmatrix} \{1  0 & 0 & 0\} \\ 1 \end{Bmatrix}$ |

**S3. SPACE GROUP NO. 3**

| line segment                                               | character of irrep (generators only)                                                                         |
|------------------------------------------------------------|--------------------------------------------------------------------------------------------------------------|
| $a \left( \frac{t}{2}, 0, 0 \right)$                       | $a_1 \begin{Bmatrix} \{1  0 & 0 & 0\} \\ 1 \end{Bmatrix}$                                                    |
| $b \left( \frac{1}{2}, \frac{t}{2}, 0 \right)$             | $b_1 \begin{Bmatrix} \{2_{010}  0 & 0 & 0\} \\ -i \end{Bmatrix}$<br>$b_2 \begin{Bmatrix} \\ i \end{Bmatrix}$ |
| $c \left( \frac{1-t}{2}, \frac{1}{2}, 0 \right)$           | $c_1 \begin{Bmatrix} \{1  0 & 0 & 0\} \\ 1 \end{Bmatrix}$                                                    |
| $d \left( \frac{t}{2}, 0, \frac{1}{2} \right)$             | $d_1 \begin{Bmatrix} \{1  0 & 0 & 0\} \\ 1 \end{Bmatrix}$                                                    |
| $e \left( \frac{1}{2}, \frac{t}{2}, \frac{1}{2} \right)$   | $e_1 \begin{Bmatrix} \{2_{010}  0 & 0 & 0\} \\ -i \end{Bmatrix}$<br>$e_2 \begin{Bmatrix} \\ i \end{Bmatrix}$ |
| $f \left( \frac{1-t}{2}, \frac{1}{2}, \frac{1}{2} \right)$ | $f_1 \begin{Bmatrix} \{1  0 & 0 & 0\} \\ 1 \end{Bmatrix}$                                                    |
| $g \left( 0, \frac{t}{2}, 0 \right)$                       | $g_1 \begin{Bmatrix} \{2_{010}  0 & 0 & 0\} \\ -i \end{Bmatrix}$<br>$g_2 \begin{Bmatrix} \\ i \end{Bmatrix}$ |
| $h \left( 0, \frac{t}{2}, \frac{1}{2} \right)$             | $h_1 \begin{Bmatrix} \{2_{010}  0 & 0 & 0\} \\ -i \end{Bmatrix}$<br>$h_2 \begin{Bmatrix} \\ i \end{Bmatrix}$ |
| $i \left( \frac{1}{2}, 0, \frac{t}{2} \right)$             | $i_1 \begin{Bmatrix} \{1  0 & 0 & 0\} \\ 1 \end{Bmatrix}$                                                    |
| $j \left( \frac{1}{2}, \frac{1}{2}, \frac{t}{2} \right)$   | $j_1 \begin{Bmatrix} \{1  0 & 0 & 0\} \\ 1 \end{Bmatrix}$                                                    |



$$\begin{aligned}
\mathcal{W}_1^{\text{gapless}} = & \sum_{m=1}^{n_{a_1}} \text{sgn}(v_m^{a_1}) \frac{1 - \text{sgn}(\delta_m^{a_1})}{2} + \sum_{m=1}^{n_{c_1}} \text{sgn}(v_m^{c_1}) \frac{1 - \text{sgn}(\delta_m^{c_1})}{2} + \sum_{m=1}^{n_{e_1}} \text{sgn}(v_m^{e_1}) \frac{1 - \text{sgn}(\delta_m^{e_1})}{2} \\
& + \sum_{m=1}^{n_{e_2}} \text{sgn}(v_m^{e_2}) \frac{1 - \text{sgn}(\delta_m^{e_2})}{2} - \sum_{m=1}^{n_{g_1}} \text{sgn}(v_m^{g_1}) \frac{1 - \text{sgn}(\delta_m^{g_1})}{2} - \sum_{m=1}^{n_{g_2}} \text{sgn}(v_m^{g_2}) \frac{1 - \text{sgn}(\delta_m^{g_2})}{2} \\
& + \sum_{m=1}^{n_{i_1}} \text{sgn}(v_m^{i_1}) \frac{1 - \text{sgn}(\delta_m^{i_1})}{2} - \sum_{m=1}^{n_{j_1}} \text{sgn}(v_m^{j_1}) \frac{1 - \text{sgn}(\delta_m^{j_1})}{2}
\end{aligned} \tag{S3.1}$$

$$\begin{aligned}
\mathcal{W}_2^{\text{gapless}} = & \sum_{m=1}^{n_{b_1}} \text{sgn}(v_m^{b_1}) \frac{1 - \text{sgn}(\delta_m^{b_1})}{2} + \sum_{m=1}^{n_{b_2}} \text{sgn}(v_m^{b_2}) \frac{1 - \text{sgn}(\delta_m^{b_2})}{2} - \sum_{m=1}^{n_{e_1}} \text{sgn}(v_m^{e_1}) \frac{1 - \text{sgn}(\delta_m^{e_1})}{2} \\
& - \sum_{m=1}^{n_{e_2}} \text{sgn}(v_m^{e_2}) \frac{1 - \text{sgn}(\delta_m^{e_2})}{2} - \sum_{m=1}^{n_{i_1}} \text{sgn}(v_m^{i_1}) \frac{1 - \text{sgn}(\delta_m^{i_1})}{2} + \sum_{m=1}^{n_{j_1}} \text{sgn}(v_m^{j_1}) \frac{1 - \text{sgn}(\delta_m^{j_1})}{2}
\end{aligned} \tag{S3.2}$$

$$\begin{aligned}
\mathcal{W}_3^{\text{gapless}} = & \sum_{m=1}^{n_{d_1}} \text{sgn}(v_m^{d_1}) \frac{1 - \text{sgn}(\delta_m^{d_1})}{2} + \sum_{m=1}^{n_{e_1}} \text{sgn}(v_m^{e_1}) \frac{1 - \text{sgn}(\delta_m^{e_1})}{2} + \sum_{m=1}^{n_{e_2}} \text{sgn}(v_m^{e_2}) \frac{1 - \text{sgn}(\delta_m^{e_2})}{2} \\
& + \sum_{m=1}^{n_{f_1}} \text{sgn}(v_m^{f_1}) \frac{1 - \text{sgn}(\delta_m^{f_1})}{2} - \sum_{m=1}^{n_{h_1}} \text{sgn}(v_m^{h_1}) \frac{1 - \text{sgn}(\delta_m^{h_1})}{2} - \sum_{m=1}^{n_{h_2}} \text{sgn}(v_m^{h_2}) \frac{1 - \text{sgn}(\delta_m^{h_2})}{2}
\end{aligned} \tag{S3.3}$$

$$\mathcal{W}_1^{\text{gapped}} = - \sum_{m=1}^{n_{g_1}} \text{sgn}(v_m^{g_1}) \frac{1 - \text{sgn}(\delta_m^{g_1})}{2} + \sum_{m=1}^{n_{g_2}} \text{sgn}(v_m^{g_2}) \frac{1 - \text{sgn}(\delta_m^{g_2})}{2} \tag{S3.4}$$

$$\mathcal{W}_2^{\text{gapped}} = - \sum_{m=1}^{n_{h_1}} \text{sgn}(v_m^{h_1}) \frac{1 - \text{sgn}(\delta_m^{h_1})}{2} + \sum_{m=1}^{n_{h_2}} \text{sgn}(v_m^{h_2}) \frac{1 - \text{sgn}(\delta_m^{h_2})}{2} \tag{S3.5}$$

$$\mathcal{W}_3^{\text{gapped}} = - \sum_{m=1}^{n_{e_1}} \text{sgn}(v_m^{e_1}) \frac{1 - \text{sgn}(\delta_m^{e_1})}{2} + \sum_{m=1}^{n_{e_2}} \text{sgn}(v_m^{e_2}) \frac{1 - \text{sgn}(\delta_m^{e_2})}{2} \tag{S3.6}$$

$$\begin{aligned}
\mathcal{W}_4^{\text{gapped}} = & 2 \sum_{m=1}^{n_{b_2}} \text{sgn}(v_m^{b_2}) \frac{1 - \text{sgn}(\delta_m^{b_2})}{2} - 2 \sum_{m=1}^{n_{e_1}} \text{sgn}(v_m^{e_1}) \frac{1 - \text{sgn}(\delta_m^{e_1})}{2} - \sum_{m=1}^{n_{i_1}} \text{sgn}(v_m^{i_1}) \frac{1 - \text{sgn}(\delta_m^{i_1})}{2} \\
& + \sum_{m=1}^{n_{j_1}} \text{sgn}(v_m^{j_1}) \frac{1 - \text{sgn}(\delta_m^{j_1})}{2}
\end{aligned} \tag{S3.7}$$

$$\mathcal{X}_1 = \sum_{m=1}^{n_{c_1}} \frac{1 - \text{sgn}(\delta_m^{c_1})}{2} \mod 2 \tag{S3.8}$$

$$\mathcal{X}_2 = \sum_{m=1}^{n_{c_1}} \frac{1 - \text{sgn}(\delta_m^{c_1})}{2} + \sum_{m=1}^{n_{f_1}} \frac{1 - \text{sgn}(\delta_m^{f_1})}{2} + \sum_{m=1}^{n_{i_1}} \frac{1 - \text{sgn}(\delta_m^{i_1})}{2} \mod 2 \quad (\text{S3.9})$$

$$\mathcal{X}_3 = \sum_{m=1}^{n_{c_1}} \frac{1 - \text{sgn}(\delta_m^{c_1})}{2} + \sum_{m=1}^{n_{i_1}} \frac{1 - \text{sgn}(\delta_m^{i_1})}{2} \mod 2 \quad (\text{S3.10})$$

#### S4. SPACE GROUP NO. 4

| line segment                                               | character of irrep (generators only)                                                                                                                                      |
|------------------------------------------------------------|---------------------------------------------------------------------------------------------------------------------------------------------------------------------------|
| $a \left( \frac{t}{2}, 0, 0 \right)$                       | $a_1 \begin{Bmatrix} 1 \\ 0 \\ 0 \\ 0 \end{Bmatrix}$                                                                                                                      |
| $b \left( \frac{1}{2}, \frac{t}{2}, 0 \right)$             | $b_1 \begin{Bmatrix} 2_{010} \\ 0 \\ 0 \\ \frac{1}{2} \end{Bmatrix}$<br>$b_2 \begin{Bmatrix} -ie^{-\frac{1}{2}i\pi t} \\ ie^{-\frac{1}{2}i\pi t} \\ 0 \\ 0 \end{Bmatrix}$ |
| $c \left( \frac{1-t}{2}, \frac{1}{2}, 0 \right)$           | $c_1 \begin{Bmatrix} 1 \\ 0 \\ 0 \\ 0 \end{Bmatrix}$                                                                                                                      |
| $d \left( \frac{t}{2}, 0, \frac{1}{2} \right)$             | $d_1 \begin{Bmatrix} 1 \\ 0 \\ 0 \\ 0 \end{Bmatrix}$                                                                                                                      |
| $e \left( \frac{1}{2}, \frac{t}{2}, \frac{1}{2} \right)$   | $e_1 \begin{Bmatrix} 2_{010} \\ 0 \\ 0 \\ \frac{1}{2} \end{Bmatrix}$<br>$e_2 \begin{Bmatrix} -ie^{-\frac{1}{2}i\pi t} \\ ie^{-\frac{1}{2}i\pi t} \\ 0 \\ 0 \end{Bmatrix}$ |
| $f \left( \frac{1-t}{2}, \frac{1}{2}, \frac{1}{2} \right)$ | $f_1 \begin{Bmatrix} 1 \\ 0 \\ 0 \\ 0 \end{Bmatrix}$                                                                                                                      |
| $g \left( 0, \frac{t}{2}, 0 \right)$                       | $g_1 \begin{Bmatrix} 2_{010} \\ 0 \\ 0 \\ \frac{1}{2} \end{Bmatrix}$<br>$g_2 \begin{Bmatrix} -ie^{-\frac{1}{2}i\pi t} \\ ie^{-\frac{1}{2}i\pi t} \\ 0 \\ 0 \end{Bmatrix}$ |
| $h \left( 0, \frac{t}{2}, \frac{1}{2} \right)$             | $h_1 \begin{Bmatrix} 2_{010} \\ 0 \\ 0 \\ \frac{1}{2} \end{Bmatrix}$<br>$h_2 \begin{Bmatrix} -ie^{-\frac{1}{2}i\pi t} \\ ie^{-\frac{1}{2}i\pi t} \\ 0 \\ 0 \end{Bmatrix}$ |
| $i \left( \frac{1}{2}, 0, \frac{t}{2} \right)$             | $i_1 \begin{Bmatrix} 1 \\ 0 \\ 0 \\ 0 \end{Bmatrix}$                                                                                                                      |
| $j \left( \frac{1}{2}, \frac{1}{2}, \frac{t}{2} \right)$   | $j_1 \begin{Bmatrix} 1 \\ 0 \\ 0 \\ 0 \end{Bmatrix}$                                                                                                                      |

$$\begin{aligned} \mathcal{W}_1^{\text{gapless}} = & \sum_{m=1}^{n_{a_1}} \text{sgn}(v_m^{a_1}) \frac{1 - \text{sgn}(\delta_m^{a_1})}{2} + 2 \sum_{m=1}^{n_{c_1}} \text{sgn}(v_m^{c_1}) \frac{1 - \text{sgn}(\delta_m^{c_1})}{2} + \sum_{m=1}^{n_{e_1}} \text{sgn}(v_m^{e_1}) \frac{1 - \text{sgn}(\delta_m^{e_1})}{2} \\ & + \sum_{m=1}^{n_{e_2}} \text{sgn}(v_m^{e_2}) \frac{1 - \text{sgn}(\delta_m^{e_2})}{2} - \sum_{m=1}^{n_{g_1}} \text{sgn}(v_m^{g_1}) \frac{1 - \text{sgn}(\delta_m^{g_1})}{2} - \sum_{m=1}^{n_{g_2}} \text{sgn}(v_m^{g_2}) \frac{1 - \text{sgn}(\delta_m^{g_2})}{2} \\ & + \sum_{m=1}^{n_{i_1}} \text{sgn}(v_m^{i_1}) \frac{1 - \text{sgn}(\delta_m^{i_1})}{2} - 2 \sum_{m=1}^{n_{j_1}} \text{sgn}(v_m^{j_1}) \frac{1 - \text{sgn}(\delta_m^{j_1})}{2} \end{aligned} \quad (\text{S4.1})$$

$$\begin{aligned} \mathcal{W}_2^{\text{gapless}} = & \sum_{m=1}^{n_{b_1}} \text{sgn}(v_m^{b_1}) \frac{1 - \text{sgn}(\delta_m^{b_1})}{2} + \sum_{m=1}^{n_{b_2}} \text{sgn}(v_m^{b_2}) \frac{1 - \text{sgn}(\delta_m^{b_2})}{2} - \sum_{m=1}^{n_{e_1}} \text{sgn}(v_m^{e_1}) \frac{1 - \text{sgn}(\delta_m^{e_1})}{2} \\ & - \sum_{m=1}^{n_{e_2}} \text{sgn}(v_m^{e_2}) \frac{1 - \text{sgn}(\delta_m^{e_2})}{2} - \sum_{m=1}^{n_{i_1}} \text{sgn}(v_m^{i_1}) \frac{1 - \text{sgn}(\delta_m^{i_1})}{2} + 2 \sum_{m=1}^{n_{j_1}} \text{sgn}(v_m^{j_1}) \frac{1 - \text{sgn}(\delta_m^{j_1})}{2} \end{aligned} \quad (\text{S4.2})$$

$$\begin{aligned} \mathcal{W}_3^{\text{gapless}} = & \sum_{m=1}^{n_{d_1}} \text{sgn}(v_m^{d_1}) \frac{1 - \text{sgn}(\delta_m^{d_1})}{2} + \sum_{m=1}^{n_{e_1}} \text{sgn}(v_m^{e_1}) \frac{1 - \text{sgn}(\delta_m^{e_1})}{2} + \sum_{m=1}^{n_{e_2}} \text{sgn}(v_m^{e_2}) \frac{1 - \text{sgn}(\delta_m^{e_2})}{2} \\ & + 2 \sum_{m=1}^{n_{f_1}} \text{sgn}(v_m^{f_1}) \frac{1 - \text{sgn}(\delta_m^{f_1})}{2} - \sum_{m=1}^{n_{h_1}} \text{sgn}(v_m^{h_1}) \frac{1 - \text{sgn}(\delta_m^{h_1})}{2} - \sum_{m=1}^{n_{h_2}} \text{sgn}(v_m^{h_2}) \frac{1 - \text{sgn}(\delta_m^{h_2})}{2} \end{aligned} \quad (\text{S4.3})$$

$$\mathcal{X}_1 = \sum_{m=1}^{n_{g_1}} \frac{1 - \text{sgn}(\delta_m^{g_1})}{2} + \sum_{m=1}^{n_{g_2}} \frac{1 - \text{sgn}(\delta_m^{g_2})}{2} \quad \text{mod } 2 \quad (\text{S4.4})$$

$$\begin{aligned} \mathcal{X}_2 = & 2 \sum_{m=1}^{n_{b_2}} \text{sgn}(v_m^{b_2}) \frac{1 - \text{sgn}(\delta_m^{b_2})}{2} + 2 \sum_{m=1}^{n_{c_1}} \text{sgn}(v_m^{c_1}) \frac{1 - \text{sgn}(\delta_m^{c_1})}{2} - \sum_{m=1}^{n_{e_1}} \text{sgn}(v_m^{e_1}) \frac{1 - \text{sgn}(\delta_m^{e_1})}{2} \\ & - \sum_{m=1}^{n_{e_2}} \text{sgn}(v_m^{e_2}) \frac{1 - \text{sgn}(\delta_m^{e_2})}{2} - \sum_{m=1}^{n_{g_1}} \text{sgn}(v_m^{g_1}) \frac{1 - \text{sgn}(\delta_m^{g_1})}{2} + \sum_{m=1}^{n_{g_2}} \text{sgn}(v_m^{g_2}) \frac{1 - \text{sgn}(\delta_m^{g_2})}{2} - \sum_{m=1}^{n_{i_1}} \text{sgn}(v_m^{i_1}) \frac{1 - \text{sgn}(\delta_m^{i_1})}{2} \\ & - 2 \sum_{m=1}^{n_{j_1}} \text{sgn}(v_m^{j_1}) \frac{1 - \text{sgn}(\delta_m^{j_1})}{2} \quad \text{mod } 4 \end{aligned} \quad (\text{S4.5})$$

$$\begin{aligned} \mathcal{X}_3 = & 2 \sum_{m=1}^{n_{c_1}} \text{sgn}(v_m^{c_1}) \frac{1 - \text{sgn}(\delta_m^{c_1})}{2} + \sum_{m=1}^{n_{e_1}} \text{sgn}(v_m^{e_1}) \frac{1 - \text{sgn}(\delta_m^{e_1})}{2} - \sum_{m=1}^{n_{e_2}} \text{sgn}(v_m^{e_2}) \frac{1 - \text{sgn}(\delta_m^{e_2})}{2} \\ & - \sum_{m=1}^{n_{g_1}} \text{sgn}(v_m^{g_1}) \frac{1 - \text{sgn}(\delta_m^{g_1})}{2} + \sum_{m=1}^{n_{g_2}} \text{sgn}(v_m^{g_2}) \frac{1 - \text{sgn}(\delta_m^{g_2})}{2} - 2 \sum_{m=1}^{n_{j_1}} \text{sgn}(v_m^{j_1}) \frac{1 - \text{sgn}(\delta_m^{j_1})}{2} \quad \text{mod } 4 \end{aligned} \quad (\text{S4.6})$$

$$\begin{aligned} \mathcal{X}_4 = & 2 \sum_{m=1}^{n_{c_1}} \text{sgn}(v_m^{c_1}) \frac{1 - \text{sgn}(\delta_m^{c_1})}{2} - 2 \sum_{m=1}^{n_{f_1}} \text{sgn}(v_m^{f_1}) \frac{1 - \text{sgn}(\delta_m^{f_1})}{2} - \sum_{m=1}^{n_{g_1}} \text{sgn}(v_m^{g_1}) \frac{1 - \text{sgn}(\delta_m^{g_1})}{2} + \sum_{m=1}^{n_{g_2}} \text{sgn}(v_m^{g_2}) \frac{1 - \text{sgn}(\delta_m^{g_2})}{2} \\ & - \sum_{m=1}^{n_{h_1}} \text{sgn}(v_m^{h_1}) \frac{1 - \text{sgn}(\delta_m^{h_1})}{2} + \sum_{m=1}^{n_{h_2}} \text{sgn}(v_m^{h_2}) \frac{1 - \text{sgn}(\delta_m^{h_2})}{2} - 2 \sum_{m=1}^{n_{j_1}} \text{sgn}(v_m^{j_1}) \frac{1 - \text{sgn}(\delta_m^{j_1})}{2} \quad \text{mod } 4 \end{aligned} \quad (\text{S4.7})$$

## S5. SPACE GROUP NO. 5

| line segment                                | character of irrep (generators only)                         |
|---------------------------------------------|--------------------------------------------------------------|
| $a \quad (0, t, 0)$                         | $\{2_{010}   0 \ 0 \ 0\}$<br>$a_1 \quad -i$<br>$a_2 \quad i$ |
| $b \quad (t, 0, 0)$                         | $\{1   0 \ 0 \ 0\}$<br>$b_1 \quad 1$                         |
| $c \quad (\frac{1-t}{2}, \frac{t+1}{2}, 0)$ | $\{1   0 \ 0 \ 0\}$<br>$c_1 \quad 1$                         |
| $d \quad (0, t, \frac{1}{2})$               | $\{2_{010}   0 \ 0 \ 0\}$<br>$d_1 \quad -i$<br>$d_2 \quad i$ |
| $e \quad (t, 0, \frac{1}{2})$               | $\{1   0 \ 0 \ 0\}$<br>$e_1 \quad 1$                         |

|                                                       |                                                                    |
|-------------------------------------------------------|--------------------------------------------------------------------|
| $f \quad (\frac{1-t}{2}, \frac{t+1}{2}, \frac{1}{2})$ | $f_1 \quad \begin{Bmatrix} 1 & 0 & 0 & 0 \\ & 1 & & \end{Bmatrix}$ |
| $g \quad (1, 0, \frac{t}{2})$                         | $g_1 \quad \begin{Bmatrix} 1 & 0 & 0 & 0 \\ & 1 & & \end{Bmatrix}$ |

$$\mathcal{W}_1^{\text{gapless}} = \sum_{m=1}^{n_{a_1}} \text{sgn}(v_m^{a_1}) \frac{1 - \text{sgn}(\delta_m^{a_1})}{2} + \sum_{m=1}^{n_{a_2}} \text{sgn}(v_m^{a_2}) \frac{1 - \text{sgn}(\delta_m^{a_2})}{2} - \sum_{m=1}^{n_{b_1}} \text{sgn}(v_m^{b_1}) \frac{1 - \text{sgn}(\delta_m^{b_1})}{2} \quad (\text{S5.1})$$

$$\mathcal{W}_2^{\text{gapless}} = \sum_{m=1}^{n_{d_1}} \text{sgn}(v_m^{d_1}) \frac{1 - \text{sgn}(\delta_m^{d_1})}{2} + \sum_{m=1}^{n_{d_2}} \text{sgn}(v_m^{d_2}) \frac{1 - \text{sgn}(\delta_m^{d_2})}{2} - \sum_{m=1}^{n_{e_1}} \text{sgn}(v_m^{e_1}) \frac{1 - \text{sgn}(\delta_m^{e_1})}{2} \quad (\text{S5.2})$$

$$\mathcal{W}_1^{\text{gapped}} = -2 \sum_{m=1}^{n_{d_2}} \text{sgn}(v_m^{d_2}) \frac{1 - \text{sgn}(\delta_m^{d_2})}{2} + \sum_{m=1}^{n_{e_1}} \text{sgn}(v_m^{e_1}) \frac{1 - \text{sgn}(\delta_m^{e_1})}{2} \quad (\text{S5.3})$$

$$\mathcal{W}_2^{\text{gapped}} = 2 \sum_{m=1}^{n_{a_2}} \text{sgn}(v_m^{a_2}) \frac{1 - \text{sgn}(\delta_m^{a_2})}{2} - \sum_{m=1}^{n_{b_1}} \text{sgn}(v_m^{b_1}) \frac{1 - \text{sgn}(\delta_m^{b_1})}{2} \quad (\text{S5.4})$$

$$\mathcal{X}_1 = \sum_{m=1}^{n_{c_1}} \frac{1 - \text{sgn}(\delta_m^{c_1})}{2} \quad \text{mod } 2 \quad (\text{S5.5})$$

$$\mathcal{X}_2 = \sum_{m=1}^{n_{f_1}} \frac{1 - \text{sgn}(\delta_m^{f_1})}{2} + \sum_{m=1}^{n_{g_1}} \frac{1 - \text{sgn}(\delta_m^{g_1})}{2} \quad \text{mod } 2 \quad (\text{S5.6})$$

$$\mathcal{X}_3 = \sum_{m=1}^{n_{g_1}} \frac{1 - \text{sgn}(\delta_m^{g_1})}{2} \quad \text{mod } 2 \quad (\text{S5.7})$$

## S6. SPACE GROUP NO. 6

| line segment                              | character of irrep (generators only)                                       |
|-------------------------------------------|----------------------------------------------------------------------------|
| $a \quad (\frac{t}{2}, 0, 0)$             | $\begin{Bmatrix} m_{010} & 0 & 0 & 0 \\ a_1 & -i \\ a_2 & i \end{Bmatrix}$ |
| $b \quad (\frac{1}{2}, \frac{t}{2}, 0)$   | $\begin{Bmatrix} 1 & 0 & 0 & 0 \\ b_1 & 1 \end{Bmatrix}$                   |
| $c \quad (\frac{1-t}{2}, \frac{1}{2}, 0)$ | $\begin{Bmatrix} m_{010} & 0 & 0 & 0 \\ c_1 & -i \\ c_2 & i \end{Bmatrix}$ |
| $d \quad (\frac{t}{2}, 0, \frac{1}{2})$   | $\begin{Bmatrix} m_{010} & 0 & 0 & 0 \\ d_1 & -i \\ d_2 & i \end{Bmatrix}$ |

|                                                     |                                                                            |
|-----------------------------------------------------|----------------------------------------------------------------------------|
| $e \quad (\frac{1}{2}, \frac{t}{2}, \frac{1}{2})$   | $\begin{matrix} \{1 0 & 0 & 0\} \\ e_1 & 1 \end{matrix}$                   |
| $f \quad (\frac{1-t}{2}, \frac{1}{2}, \frac{1}{2})$ | $\begin{matrix} \{m_{010} 0 & 0 & 0\} \\ f_1 & -i \\ f_2 & i \end{matrix}$ |
| $g \quad (0, \frac{t}{2}, 0)$                       | $\begin{matrix} \{1 0 & 0 & 0\} \\ g_1 & 1 \end{matrix}$                   |
| $h \quad (0, \frac{t}{2}, \frac{1}{2})$             | $\begin{matrix} \{1 0 & 0 & 0\} \\ h_1 & 1 \end{matrix}$                   |
| $i \quad (\frac{1}{2}, 0, \frac{t}{2})$             | $\begin{matrix} \{m_{010} 0 & 0 & 0\} \\ i_1 & -i \\ i_2 & i \end{matrix}$ |
| $j \quad (\frac{1}{2}, \frac{1}{2}, \frac{t}{2})$   | $\begin{matrix} \{m_{010} 0 & 0 & 0\} \\ j_1 & -i \\ j_2 & i \end{matrix}$ |

$$\begin{aligned}
\mathcal{W}_1^{\text{gapless}} = & \sum_{m=1}^{n_{a_1}} \text{sgn}(v_m^{a_1}) \frac{1 - \text{sgn}(\delta_m^{a_1})}{2} + \sum_{m=1}^{n_{a_2}} \text{sgn}(v_m^{a_2}) \frac{1 - \text{sgn}(\delta_m^{a_2})}{2} + 2 \sum_{m=1}^{n_{c_2}} \text{sgn}(v_m^{c_2}) \frac{1 - \text{sgn}(\delta_m^{c_2})}{2} \\
& + \sum_{m=1}^{n_{e_1}} \text{sgn}(v_m^{e_1}) \frac{1 - \text{sgn}(\delta_m^{e_1})}{2} + \sum_{m=1}^{n_{f_1}} \text{sgn}(v_m^{f_1}) \frac{1 - \text{sgn}(\delta_m^{f_1})}{2} - \sum_{m=1}^{n_{f_2}} \text{sgn}(v_m^{f_2}) \frac{1 - \text{sgn}(\delta_m^{f_2})}{2} \\
& - \sum_{m=1}^{n_{g_1}} \text{sgn}(v_m^{g_1}) \frac{1 - \text{sgn}(\delta_m^{g_1})}{2} + \sum_{m=1}^{n_{i_1}} \text{sgn}(v_m^{i_1}) \frac{1 - \text{sgn}(\delta_m^{i_1})}{2} + \sum_{m=1}^{n_{i_2}} \text{sgn}(v_m^{i_2}) \frac{1 - \text{sgn}(\delta_m^{i_2})}{2} \\
& - \sum_{m=1}^{n_{j_1}} \text{sgn}(v_m^{j_1}) \frac{1 - \text{sgn}(\delta_m^{j_1})}{2} - \sum_{m=1}^{n_{j_2}} \text{sgn}(v_m^{j_2}) \frac{1 - \text{sgn}(\delta_m^{j_2})}{2}
\end{aligned} \tag{S6.1}$$

$$\begin{aligned}
\mathcal{W}_2^{\text{gapless}} = & 2 \sum_{m=1}^{n_{a_2}} \text{sgn}(v_m^{a_2}) \frac{1 - \text{sgn}(\delta_m^{a_2})}{2} + 2 \sum_{m=1}^{n_{c_2}} \text{sgn}(v_m^{c_2}) \frac{1 - \text{sgn}(\delta_m^{c_2})}{2} - 2 \sum_{m=1}^{n_{d_2}} \text{sgn}(v_m^{d_2}) \frac{1 - \text{sgn}(\delta_m^{d_2})}{2} \\
& - 2 \sum_{m=1}^{n_{f_2}} \text{sgn}(v_m^{f_2}) \frac{1 - \text{sgn}(\delta_m^{f_2})}{2} - \sum_{m=1}^{n_{g_1}} \text{sgn}(v_m^{g_1}) \frac{1 - \text{sgn}(\delta_m^{g_1})}{2} + \sum_{m=1}^{n_{h_1}} \text{sgn}(v_m^{h_1}) \frac{1 - \text{sgn}(\delta_m^{h_1})}{2} \\
& + \sum_{m=1}^{n_{i_1}} \text{sgn}(v_m^{i_1}) \frac{1 - \text{sgn}(\delta_m^{i_1})}{2} + \sum_{m=1}^{n_{i_2}} \text{sgn}(v_m^{i_2}) \frac{1 - \text{sgn}(\delta_m^{i_2})}{2} - \sum_{m=1}^{n_{j_1}} \text{sgn}(v_m^{j_1}) \frac{1 - \text{sgn}(\delta_m^{j_1})}{2} - \sum_{m=1}^{n_{j_2}} \text{sgn}(v_m^{j_2}) \frac{1 - \text{sgn}(\delta_m^{j_2})}{2}
\end{aligned} \tag{S6.2}$$

$$\begin{aligned}
\mathcal{W}_3^{\text{gapless}} = & \sum_{m=1}^{n_{b_1}} \text{sgn}(v_m^{b_1}) \frac{1 - \text{sgn}(\delta_m^{b_1})}{2} - \sum_{m=1}^{n_{e_1}} \text{sgn}(v_m^{e_1}) \frac{1 - \text{sgn}(\delta_m^{e_1})}{2} - \sum_{m=1}^{n_{i_1}} \text{sgn}(v_m^{i_1}) \frac{1 - \text{sgn}(\delta_m^{i_1})}{2} \\
& - \sum_{m=1}^{n_{i_2}} \text{sgn}(v_m^{i_2}) \frac{1 - \text{sgn}(\delta_m^{i_2})}{2} + \sum_{m=1}^{n_{j_1}} \text{sgn}(v_m^{j_1}) \frac{1 - \text{sgn}(\delta_m^{j_1})}{2} + \sum_{m=1}^{n_{j_2}} \text{sgn}(v_m^{j_2}) \frac{1 - \text{sgn}(\delta_m^{j_2})}{2}
\end{aligned} \tag{S6.3}$$

$$\mathcal{W}_4^{\text{gapless}} = \sum_{m=1}^{n_{c_1}} \text{sgn}(v_m^{c_1}) \frac{1 - \text{sgn}(\delta_m^{c_1})}{2} - \sum_{m=1}^{n_{c_2}} \text{sgn}(v_m^{c_2}) \frac{1 - \text{sgn}(\delta_m^{c_2})}{2} - \sum_{m=1}^{n_{f_1}} \text{sgn}(v_m^{f_1}) \frac{1 - \text{sgn}(\delta_m^{f_1})}{2} + \sum_{m=1}^{n_{f_2}} \text{sgn}(v_m^{f_2}) \frac{1 - \text{sgn}(\delta_m^{f_2})}{2} \tag{S6.4}$$

$$\begin{aligned} \mathcal{W}_5^{\text{gapless}} = & \sum_{m=1}^{n_{d_1}} \text{sgn}(v_m^{d_1}) \frac{1 - \text{sgn}(\delta_m^{d_1})}{2} + \sum_{m=1}^{n_{d_2}} \text{sgn}(v_m^{d_2}) \frac{1 - \text{sgn}(\delta_m^{d_2})}{2} + \sum_{m=1}^{n_{e_1}} \text{sgn}(v_m^{e_1}) \frac{1 - \text{sgn}(\delta_m^{e_1})}{2} \\ & + \sum_{m=1}^{n_{f_1}} \text{sgn}(v_m^{f_1}) \frac{1 - \text{sgn}(\delta_m^{f_1})}{2} + \sum_{m=1}^{n_{f_2}} \text{sgn}(v_m^{f_2}) \frac{1 - \text{sgn}(\delta_m^{f_2})}{2} - \sum_{m=1}^{n_{h_1}} \text{sgn}(v_m^{h_1}) \frac{1 - \text{sgn}(\delta_m^{h_1})}{2} \end{aligned} \quad (\text{S6.5})$$

$$\begin{aligned} \mathcal{W}_1^{\text{gapped}} = & 2 \sum_{m=1}^{n_{d_2}} \text{sgn}(v_m^{d_2}) \frac{1 - \text{sgn}(\delta_m^{d_2})}{2} + \sum_{m=1}^{n_{e_1}} \text{sgn}(v_m^{e_1}) \frac{1 - \text{sgn}(\delta_m^{e_1})}{2} + 2 \sum_{m=1}^{n_{f_2}} \text{sgn}(v_m^{f_2}) \frac{1 - \text{sgn}(\delta_m^{f_2})}{2} \\ & - \sum_{m=1}^{n_{h_1}} \text{sgn}(v_m^{h_1}) \frac{1 - \text{sgn}(\delta_m^{h_1})}{2} \end{aligned} \quad (\text{S6.6})$$

$$\mathcal{W}_2^{\text{gapped}} = - \sum_{m=1}^{n_{i_1}} \text{sgn}(v_m^{i_1}) \frac{1 - \text{sgn}(\delta_m^{i_1})}{2} + \sum_{m=1}^{n_{i_2}} \text{sgn}(v_m^{i_2}) \frac{1 - \text{sgn}(\delta_m^{i_2})}{2} \quad (\text{S6.7})$$

$$\mathcal{W}_3^{\text{gapped}} = \sum_{m=1}^{n_{f_1}} \text{sgn}(v_m^{f_1}) \frac{1 - \text{sgn}(\delta_m^{f_1})}{2} - \sum_{m=1}^{n_{f_2}} \text{sgn}(v_m^{f_2}) \frac{1 - \text{sgn}(\delta_m^{f_2})}{2} \quad (\text{S6.8})$$

$$\begin{aligned} \mathcal{W}_4^{\text{gapped}} = & -2 \sum_{m=1}^{n_{a_2}} \text{sgn}(v_m^{a_2}) \frac{1 - \text{sgn}(\delta_m^{a_2})}{2} - 2 \sum_{m=1}^{n_{c_2}} \text{sgn}(v_m^{c_2}) \frac{1 - \text{sgn}(\delta_m^{c_2})}{2} + 2 \sum_{m=1}^{n_{d_2}} \text{sgn}(v_m^{d_2}) \frac{1 - \text{sgn}(\delta_m^{d_2})}{2} \\ & + 2 \sum_{m=1}^{n_{f_2}} \text{sgn}(v_m^{f_2}) \frac{1 - \text{sgn}(\delta_m^{f_2})}{2} + \sum_{m=1}^{n_{g_1}} \text{sgn}(v_m^{g_1}) \frac{1 - \text{sgn}(\delta_m^{g_1})}{2} - \sum_{m=1}^{n_{h_1}} \text{sgn}(v_m^{h_1}) \frac{1 - \text{sgn}(\delta_m^{h_1})}{2} \\ & - 2 \sum_{m=1}^{n_{i_2}} \text{sgn}(v_m^{i_2}) \frac{1 - \text{sgn}(\delta_m^{i_2})}{2} + 2 \sum_{m=1}^{n_{j_2}} \text{sgn}(v_m^{j_2}) \frac{1 - \text{sgn}(\delta_m^{j_2})}{2} \end{aligned} \quad (\text{S6.9})$$

$$\mathcal{X}_1 = \sum_{m=1}^{n_{e_1}} \frac{1 - \text{sgn}(\delta_m^{e_1})}{2} \quad \text{mod } 2 \quad (\text{S6.10})$$

## 57. SPACE GROUP NO. 7

| line segment                              | character of irrep (generators only)                                   |
|-------------------------------------------|------------------------------------------------------------------------|
| $a \quad (\frac{t}{2}, 0, 0)$             | $\{m_{010}   0 \ 0 \ \frac{1}{2}\}$<br>$a_1 \quad -i$<br>$a_2 \quad i$ |
| $b \quad (\frac{1}{2}, \frac{t}{2}, 0)$   | $\{1   0 \ 0 \ 0\}$<br>$b_1 \quad 1$                                   |
| $c \quad (\frac{1-t}{2}, \frac{1}{2}, 0)$ | $\{m_{010}   0 \ 0 \ \frac{1}{2}\}$<br>$c_1 \quad -i$<br>$c_2 \quad i$ |
| $d \quad (\frac{t}{2}, 0, \frac{1}{2})$   | $\{m_{010}   0 \ 0 \ \frac{1}{2}\}$<br>$d_1 \quad -1$<br>$d_2 \quad 1$ |

|                                                     |                                                                                                                                  |
|-----------------------------------------------------|----------------------------------------------------------------------------------------------------------------------------------|
| $e \quad (\frac{1}{2}, \frac{t}{2}, \frac{1}{2})$   | $\begin{matrix} \{1 0 & 0 & 0 & 0\} \\ e_1 & 1 \end{matrix}$                                                                     |
| $f \quad (\frac{1-t}{2}, \frac{1}{2}, \frac{1}{2})$ | $\begin{matrix} \{m_{010} 0 & 0 & \frac{1}{2}\} \\ f_1 & -1 \\ f_2 & 1 \end{matrix}$                                             |
| $g \quad (0, \frac{t}{2}, 0)$                       | $\begin{matrix} \{1 0 & 0 & 0 & 0\} \\ g_1 & 1 \end{matrix}$                                                                     |
| $h \quad (0, \frac{t}{2}, \frac{1}{2})$             | $\begin{matrix} \{1 0 & 0 & 0 & 0\} \\ h_1 & 1 \end{matrix}$                                                                     |
| $i \quad (\frac{1}{2}, 0, \frac{t}{2})$             | $\begin{matrix} \{m_{010} 0 & 0 & \frac{1}{2}\} \\ i_1 & -ie^{-\frac{1}{2}i\pi t} \\ i_2 & ie^{-\frac{1}{2}i\pi t} \end{matrix}$ |
| $j \quad (\frac{1}{2}, \frac{1}{2}, \frac{t}{2})$   | $\begin{matrix} \{m_{010} 0 & 0 & \frac{1}{2}\} \\ j_1 & -ie^{-\frac{1}{2}i\pi t} \\ j_2 & ie^{-\frac{1}{2}i\pi t} \end{matrix}$ |

$$\begin{aligned}
\mathcal{W}_1^{\text{gapless}} = & \sum_{m=1}^{n_{a_1}} \text{sgn}(v_m^{a_1}) \frac{1 - \text{sgn}(\delta_m^{a_1})}{2} + \sum_{m=1}^{n_{a_2}} \text{sgn}(v_m^{a_2}) \frac{1 - \text{sgn}(\delta_m^{a_2})}{2} + 2 \sum_{m=1}^{n_{c_2}} \text{sgn}(v_m^{c_2}) \frac{1 - \text{sgn}(\delta_m^{c_2})}{2} \\
& + 2 \sum_{m=1}^{n_{e_1}} \text{sgn}(v_m^{e_1}) \frac{1 - \text{sgn}(\delta_m^{e_1})}{2} - \sum_{m=1}^{n_{g_1}} \text{sgn}(v_m^{g_1}) \frac{1 - \text{sgn}(\delta_m^{g_1})}{2} + \sum_{m=1}^{n_{i_1}} \text{sgn}(v_m^{i_1}) \frac{1 - \text{sgn}(\delta_m^{i_1})}{2} \\
& + \sum_{m=1}^{n_{i_2}} \text{sgn}(v_m^{i_2}) \frac{1 - \text{sgn}(\delta_m^{i_2})}{2} - \sum_{m=1}^{n_{j_1}} \text{sgn}(v_m^{j_1}) \frac{1 - \text{sgn}(\delta_m^{j_1})}{2} - \sum_{m=1}^{n_{j_2}} \text{sgn}(v_m^{j_2}) \frac{1 - \text{sgn}(\delta_m^{j_2})}{2}
\end{aligned} \tag{S7.1}$$

$$\begin{aligned}
\mathcal{W}_2^{\text{gapless}} = & 2 \sum_{m=1}^{n_{a_2}} \text{sgn}(v_m^{a_2}) \frac{1 - \text{sgn}(\delta_m^{a_2})}{2} + 2 \sum_{m=1}^{n_{c_2}} \text{sgn}(v_m^{c_2}) \frac{1 - \text{sgn}(\delta_m^{c_2})}{2} \\
& + 2 \sum_{m=1}^{n_{e_1}} \text{sgn}(v_m^{e_1}) \frac{1 - \text{sgn}(\delta_m^{e_1})}{2} - \sum_{m=1}^{n_{g_1}} \text{sgn}(v_m^{g_1}) \frac{1 - \text{sgn}(\delta_m^{g_1})}{2} + \sum_{m=1}^{n_{i_1}} \text{sgn}(v_m^{i_1}) \frac{1 - \text{sgn}(\delta_m^{i_1})}{2} \\
& + \sum_{m=1}^{n_{i_2}} \text{sgn}(v_m^{i_2}) \frac{1 - \text{sgn}(\delta_m^{i_2})}{2} - \sum_{m=1}^{n_{j_1}} \text{sgn}(v_m^{j_1}) \frac{1 - \text{sgn}(\delta_m^{j_1})}{2} - \sum_{m=1}^{n_{j_2}} \text{sgn}(v_m^{j_2}) \frac{1 - \text{sgn}(\delta_m^{j_2})}{2}
\end{aligned} \tag{S7.2}$$

$$\begin{aligned}
\mathcal{W}_3^{\text{gapless}} = & \sum_{m=1}^{n_{b_1}} \text{sgn}(v_m^{b_1}) \frac{1 - \text{sgn}(\delta_m^{b_1})}{2} - 2 \sum_{m=1}^{n_{e_1}} \text{sgn}(v_m^{e_1}) \frac{1 - \text{sgn}(\delta_m^{e_1})}{2} - \sum_{m=1}^{n_{i_1}} \text{sgn}(v_m^{i_1}) \frac{1 - \text{sgn}(\delta_m^{i_1})}{2} \\
& - \sum_{m=1}^{n_{i_2}} \text{sgn}(v_m^{i_2}) \frac{1 - \text{sgn}(\delta_m^{i_2})}{2} + \sum_{m=1}^{n_{j_1}} \text{sgn}(v_m^{j_1}) \frac{1 - \text{sgn}(\delta_m^{j_1})}{2} + \sum_{m=1}^{n_{j_2}} \text{sgn}(v_m^{j_2}) \frac{1 - \text{sgn}(\delta_m^{j_2})}{2}
\end{aligned} \tag{S7.3}$$

$$\mathcal{W}_4^{\text{gapless}} = \sum_{m=1}^{n_{c_1}} \text{sgn}(v_m^{c_1}) \frac{1 - \text{sgn}(\delta_m^{c_1})}{2} - \sum_{m=1}^{n_{c_2}} \text{sgn}(v_m^{c_2}) \frac{1 - \text{sgn}(\delta_m^{c_2})}{2} \tag{S7.4}$$

$$\begin{aligned}
\mathcal{W}_5^{\text{gapless}} = & \sum_{m=1}^{n_{d_1}} \text{sgn}(v_m^{d_1}) \frac{1 - \text{sgn}(\delta_m^{d_1})}{2} + \sum_{m=1}^{n_{d_2}} \text{sgn}(v_m^{d_2}) \frac{1 - \text{sgn}(\delta_m^{d_2})}{2} + 2 \sum_{m=1}^{n_{e_1}} \text{sgn}(v_m^{e_1}) \frac{1 - \text{sgn}(\delta_m^{e_1})}{2} \\
& + \sum_{m=1}^{n_{f_1}} \text{sgn}(v_m^{f_1}) \frac{1 - \text{sgn}(\delta_m^{f_1})}{2} + \sum_{m=1}^{n_{f_2}} \text{sgn}(v_m^{f_2}) \frac{1 - \text{sgn}(\delta_m^{f_2})}{2} - 2 \sum_{m=1}^{n_{h_1}} \text{sgn}(v_m^{h_1}) \frac{1 - \text{sgn}(\delta_m^{h_1})}{2}
\end{aligned} \tag{S7.5}$$

$$\mathcal{X}_1 = \sum_{m=1}^{n_{d_2}} \frac{1 - \text{sgn}(\delta_m^{d_2})}{2} + \sum_{m=1}^{n_{g_1}} \frac{1 - \text{sgn}(\delta_m^{g_1})}{2} \mod 2 \quad (\text{S7.6})$$

$$\mathcal{X}_2 = \sum_{m=1}^{n_{d_2}} \frac{1 - \text{sgn}(\delta_m^{d_2})}{2} + \sum_{m=1}^{n_{f_1}} \frac{1 - \text{sgn}(\delta_m^{f_1})}{2} + \sum_{m=1}^{n_{f_2}} \frac{1 - \text{sgn}(\delta_m^{f_2})}{2} + \sum_{m=1}^{n_{i_1}} \frac{1 - \text{sgn}(\delta_m^{i_1})}{2} + \sum_{m=1}^{n_{i_2}} \frac{1 - \text{sgn}(\delta_m^{i_2})}{2} \mod 2 \quad (\text{S7.7})$$

$$\mathcal{X}_3 = \sum_{m=1}^{n_{f_1}} \frac{1 - \text{sgn}(\delta_m^{f_1})}{2} + \sum_{m=1}^{n_{g_1}} \frac{1 - \text{sgn}(\delta_m^{g_1})}{2} \mod 2 \quad (\text{S7.8})$$

$$\mathcal{X}_4 = \sum_{m=1}^{n_{f_1}} \frac{1 - \text{sgn}(\delta_m^{f_1})}{2} + \sum_{m=1}^{n_{i_1}} \frac{1 - \text{sgn}(\delta_m^{i_1})}{2} + \sum_{m=1}^{n_{i_2}} \frac{1 - \text{sgn}(\delta_m^{i_2})}{2} \mod 2 \quad (\text{S7.9})$$

$$\begin{aligned} \mathcal{X}_5 = & -2 \sum_{m=1}^{n_{a_2}} \text{sgn}(v_m^{a_2}) \frac{1 - \text{sgn}(\delta_m^{a_2})}{2} - 2 \sum_{m=1}^{n_{c_2}} \text{sgn}(v_m^{c_2}) \frac{1 - \text{sgn}(\delta_m^{c_2})}{2} - 2 \sum_{m=1}^{n_{f_1}} \text{sgn}(v_m^{f_1}) \frac{1 - \text{sgn}(\delta_m^{f_1})}{2} \\ & + \sum_{m=1}^{n_{g_1}} \text{sgn}(v_m^{g_1}) \frac{1 - \text{sgn}(\delta_m^{g_1})}{2} - 2 \sum_{m=1}^{n_{i_1}} \text{sgn}(v_m^{i_1}) \frac{1 - \text{sgn}(\delta_m^{i_1})}{2} + 2 \sum_{m=1}^{n_{j_2}} \text{sgn}(v_m^{j_2}) \frac{1 - \text{sgn}(\delta_m^{j_2})}{2} \mod 4 \end{aligned} \quad (\text{S7.10})$$

## S8. SPACE GROUP NO. 8

| line segment                                      | character of irrep (generators only)                                        |
|---------------------------------------------------|-----------------------------------------------------------------------------|
| $a \ (0, t, 0)$                                   | $\begin{matrix} \{1  0 & 0 & 0\} \\ a_1 & 1 \end{matrix}$                   |
| $b \ (t, 0, 0)$                                   | $\begin{matrix} \{m_{010}  0 & 0 & 0\} \\ b_1 & -i \\ b_2 & i \end{matrix}$ |
| $c \ (\frac{1-t}{2}, \frac{t+1}{2}, 0)$           | $\begin{matrix} \{1  0 & 0 & 0\} \\ c_1 & 1 \end{matrix}$                   |
| $d \ (0, t, \frac{1}{2})$                         | $\begin{matrix} \{1  0 & 0 & 0\} \\ d_1 & 1 \end{matrix}$                   |
| $e \ (t, 0, \frac{1}{2})$                         | $\begin{matrix} \{m_{010}  0 & 0 & 0\} \\ e_1 & -i \\ e_2 & i \end{matrix}$ |
| $f \ (\frac{1-t}{2}, \frac{t+1}{2}, \frac{1}{2})$ | $\begin{matrix} \{1  0 & 0 & 0\} \\ f_1 & 1 \end{matrix}$                   |
| $g \ (1, 0, \frac{t}{2})$                         | $\begin{matrix} \{m_{010}  0 & 0 & 0\} \\ g_1 & -i \\ g_2 & i \end{matrix}$ |

$$\mathcal{W}_1^{\text{gapless}} = \sum_{m=1}^{n_{a_1}} \text{sgn}(v_m^{a_1}) \frac{1 - \text{sgn}(\delta_m^{a_1})}{2} - 2 \sum_{m=1}^{n_{b_2}} \text{sgn}(v_m^{b_2}) \frac{1 - \text{sgn}(\delta_m^{b_2})}{2} - \sum_{m=1}^{n_{e_1}} \text{sgn}(v_m^{e_1}) \frac{1 - \text{sgn}(\delta_m^{e_1})}{2} + \sum_{m=1}^{n_{e_2}} \text{sgn}(v_m^{e_2}) \frac{1 - \text{sgn}(\delta_m^{e_2})}{2} \quad (\text{S8.1})$$



$$\mathcal{W}_2^{\text{gapless}} = \sum_{m=1}^{n_{b_1}} \text{sgn}(v_m^{b_1}) \frac{1 - \text{sgn}(\delta_m^{b_1})}{2} - \sum_{m=1}^{n_{b_2}} \text{sgn}(v_m^{b_2}) \frac{1 - \text{sgn}(\delta_m^{b_2})}{2} - \sum_{m=1}^{n_{e_1}} \text{sgn}(v_m^{e_1}) \frac{1 - \text{sgn}(\delta_m^{e_1})}{2} + \sum_{m=1}^{n_{e_2}} \text{sgn}(v_m^{e_2}) \frac{1 - \text{sgn}(\delta_m^{e_2})}{2} \quad (\text{S8.2})$$

$$\mathcal{W}_3^{\text{gapless}} = \sum_{m=1}^{n_{d_1}} \text{sgn}(v_m^{d_1}) \frac{1 - \text{sgn}(\delta_m^{d_1})}{2} - \sum_{m=1}^{n_{e_1}} \text{sgn}(v_m^{e_1}) \frac{1 - \text{sgn}(\delta_m^{e_1})}{2} - \sum_{m=1}^{n_{e_2}} \text{sgn}(v_m^{e_2}) \frac{1 - \text{sgn}(\delta_m^{e_2})}{2} \quad (\text{S8.3})$$

$$\mathcal{W}_1^{\text{gapped}} = \sum_{m=1}^{n_{e_1}} \text{sgn}(v_m^{e_1}) \frac{1 - \text{sgn}(\delta_m^{e_1})}{2} - \sum_{m=1}^{n_{e_2}} \text{sgn}(v_m^{e_2}) \frac{1 - \text{sgn}(\delta_m^{e_2})}{2} \quad (\text{S8.4})$$

$$\mathcal{W}_2^{\text{gapped}} = - \sum_{m=1}^{n_{g_1}} \text{sgn}(v_m^{g_1}) \frac{1 - \text{sgn}(\delta_m^{g_1})}{2} + \sum_{m=1}^{n_{g_2}} \text{sgn}(v_m^{g_2}) \frac{1 - \text{sgn}(\delta_m^{g_2})}{2} \quad (\text{S8.5})$$

$$\mathcal{X}_1 = \sum_{m=1}^{n_{c_1}} \frac{1 - \text{sgn}(\delta_m^{c_1})}{2} + \sum_{m=1}^{n_{f_1}} \frac{1 - \text{sgn}(\delta_m^{f_1})}{2} \quad \text{mod } 2 \quad (\text{S8.6})$$

$$\mathcal{X}_2 = \sum_{m=1}^{n_{c_1}} \frac{1 - \text{sgn}(\delta_m^{c_1})}{2} \quad \text{mod } 2 \quad (\text{S8.7})$$

### S9. SPACE GROUP NO. 9

| line segment                                      | character of irrep (generators only)                                                                                              |
|---------------------------------------------------|-----------------------------------------------------------------------------------------------------------------------------------|
| $a \ (0, t, 0)$                                   | $\begin{matrix} \{1  0 & 0 & 0\} \\ a_1 & 1 \end{matrix}$                                                                         |
| $b \ (t, 0, 0)$                                   | $\begin{matrix} \{m_{010}  0 & 0 & \frac{1}{2}\} \\ b_1 & -i \\ b_2 & i \end{matrix}$                                             |
| $c \ (\frac{1-t}{2}, \frac{t+1}{2}, 0)$           | $\begin{matrix} \{1  0 & 0 & 0\} \\ c_1 & 1 \end{matrix}$                                                                         |
| $d \ (0, t, \frac{1}{2})$                         | $\begin{matrix} \{1  0 & 0 & 0\} \\ d_1 & 1 \end{matrix}$                                                                         |
| $e \ (t, 0, \frac{1}{2})$                         | $\begin{matrix} \{m_{010}  0 & 0 & \frac{1}{2}\} \\ e_1 & -1 \\ e_2 & 1 \end{matrix}$                                             |
| $f \ (\frac{1-t}{2}, \frac{t+1}{2}, \frac{1}{2})$ | $\begin{matrix} \{1  0 & 0 & 0\} \\ f_1 & 1 \end{matrix}$                                                                         |
| $g \ (1, 0, \frac{t}{2})$                         | $\begin{matrix} \{m_{010}  0 & 0 & \frac{1}{2}\} \\ g_1 & -ie^{-\frac{1}{2}i\pi t} \\ g_2 & ie^{-\frac{1}{2}i\pi t} \end{matrix}$ |

$$\mathcal{W}_1^{\text{gapless}} = \sum_{m=1}^{n_{a_1}} \text{sgn}(v_m^{a_1}) \frac{1 - \text{sgn}(\delta_m^{a_1})}{2} - 2 \sum_{m=1}^{n_{b_2}} \text{sgn}(v_m^{b_2}) \frac{1 - \text{sgn}(\delta_m^{b_2})}{2} \quad (\text{S9.1})$$

$$\mathcal{W}_2^{\text{gapless}} = \sum_{m=1}^{n_{b_1}} \text{sgn}(v_m^{b_1}) \frac{1 - \text{sgn}(\delta_m^{b_1})}{2} - \sum_{m=1}^{n_{b_2}} \text{sgn}(v_m^{b_2}) \frac{1 - \text{sgn}(\delta_m^{b_2})}{2} \quad (\text{S9.2})$$

$$\mathcal{W}_3^{\text{gapless}} = 2 \sum_{m=1}^{n_{d_1}} \text{sgn}(v_m^{d_1}) \frac{1 - \text{sgn}(\delta_m^{d_1})}{2} - \sum_{m=1}^{n_{e_1}} \text{sgn}(v_m^{e_1}) \frac{1 - \text{sgn}(\delta_m^{e_1})}{2} - \sum_{m=1}^{n_{e_2}} \text{sgn}(v_m^{e_2}) \frac{1 - \text{sgn}(\delta_m^{e_2})}{2} \quad (\text{S9.3})$$

$$\mathcal{X}_1 = \sum_{m=1}^{n_{c_1}} \frac{1 - \text{sgn}(\delta_m^{c_1})}{2} + \sum_{m=1}^{n_{f_1}} \frac{1 - \text{sgn}(\delta_m^{f_1})}{2} + \sum_{m=1}^{n_{g_1}} \frac{1 - \text{sgn}(\delta_m^{g_1})}{2} + \sum_{m=1}^{n_{g_2}} \frac{1 - \text{sgn}(\delta_m^{g_2})}{2} \mod 2 \quad (\text{S9.4})$$

$$\mathcal{X}_2 = \sum_{m=1}^{n_{c_1}} \frac{1 - \text{sgn}(\delta_m^{c_1})}{2} + \sum_{m=1}^{n_{e_1}} \frac{1 - \text{sgn}(\delta_m^{e_1})}{2} \mod 2 \quad (\text{S9.5})$$

$$\mathcal{X}_3 = \sum_{m=1}^{n_{c_1}} \frac{1 - \text{sgn}(\delta_m^{c_1})}{2} + \sum_{m=1}^{n_{g_1}} \frac{1 - \text{sgn}(\delta_m^{g_1})}{2} + \sum_{m=1}^{n_{g_2}} \frac{1 - \text{sgn}(\delta_m^{g_2})}{2} \mod 2 \quad (\text{S9.6})$$

$$\mathcal{X}_4 = \sum_{m=1}^{n_{c_1}} \frac{1 - \text{sgn}(\delta_m^{c_1})}{2} \mod 2 \quad (\text{S9.7})$$

### S10. SPACE GROUP NO. 10

| line segment                                        | character of irrep (generators only)                         |
|-----------------------------------------------------|--------------------------------------------------------------|
| $a \quad (\frac{t}{2}, 0, 0)$                       | $\{m_{010}   0 \ 0 \ 0\}$<br>$a_1 \quad -i$<br>$a_2 \quad i$ |
| $b \quad (\frac{1}{2}, \frac{t}{2}, 0)$             | $\{2_{010}   0 \ 0 \ 0\}$<br>$b_1 \quad -i$<br>$b_2 \quad i$ |
| $c \quad (\frac{1-t}{2}, \frac{1}{2}, 0)$           | $\{m_{010}   0 \ 0 \ 0\}$<br>$c_1 \quad -i$<br>$c_2 \quad i$ |
| $d \quad (\frac{t}{2}, 0, \frac{1}{2})$             | $\{m_{010}   0 \ 0 \ 0\}$<br>$d_1 \quad -i$<br>$d_2 \quad i$ |
| $e \quad (\frac{1}{2}, \frac{t}{2}, \frac{1}{2})$   | $\{2_{010}   0 \ 0 \ 0\}$<br>$e_1 \quad -i$<br>$e_2 \quad i$ |
| $f \quad (\frac{1-t}{2}, \frac{1}{2}, \frac{1}{2})$ | $\{m_{010}   0 \ 0 \ 0\}$<br>$f_1 \quad -i$<br>$f_2 \quad i$ |
| $g \quad (0, \frac{t}{2}, 0)$                       | $\{2_{010}   0 \ 0 \ 0\}$<br>$g_1 \quad -i$<br>$g_2 \quad i$ |
| $h \quad (0, \frac{t}{2}, \frac{1}{2})$             | $\{2_{010}   0 \ 0 \ 0\}$<br>$h_1 \quad -i$<br>$h_2 \quad i$ |

|                                                   |                                                               |
|---------------------------------------------------|---------------------------------------------------------------|
| $i \quad (\frac{1}{2}, 0, \frac{t}{2})$           | $\{m_{010}   0 \ 0 \ 0 \}$<br>$i_1 \quad -i$<br>$i_2 \quad i$ |
| $j \quad (\frac{1}{2}, \frac{1}{2}, \frac{t}{2})$ | $\{m_{010}   0 \ 0 \ 0 \}$<br>$j_1 \quad -i$<br>$j_2 \quad i$ |

$$\begin{aligned} \mathcal{W}_1^{\text{gapless}} = & \sum_{m=1}^{n_{a_1}} \text{sgn}(v_m^{a_1}) \frac{1 - \text{sgn}(\delta_m^{a_1})}{2} + \sum_{m=1}^{n_{c_1}} \text{sgn}(v_m^{c_1}) \frac{1 - \text{sgn}(\delta_m^{c_1})}{2} + \sum_{m=1}^{n_{e_1}} \text{sgn}(v_m^{e_1}) \frac{1 - \text{sgn}(\delta_m^{e_1})}{2} \\ & - \sum_{m=1}^{n_{g_1}} \text{sgn}(v_m^{g_1}) \frac{1 - \text{sgn}(\delta_m^{g_1})}{2} + \sum_{m=1}^{n_{i_1}} \text{sgn}(v_m^{i_1}) \frac{1 - \text{sgn}(\delta_m^{i_1})}{2} - \sum_{m=1}^{n_{j_1}} \text{sgn}(v_m^{j_1}) \frac{1 - \text{sgn}(\delta_m^{j_1})}{2} \end{aligned} \quad (\text{S10.1})$$

$$\mathcal{W}_2^{\text{gapless}} = \sum_{m=1}^{n_{b_1}} \text{sgn}(v_m^{b_1}) \frac{1 - \text{sgn}(\delta_m^{b_1})}{2} - \sum_{m=1}^{n_{e_1}} \text{sgn}(v_m^{e_1}) \frac{1 - \text{sgn}(\delta_m^{e_1})}{2} - \sum_{m=1}^{n_{i_1}} \text{sgn}(v_m^{i_1}) \frac{1 - \text{sgn}(\delta_m^{i_1})}{2} + \sum_{m=1}^{n_{j_1}} \text{sgn}(v_m^{j_1}) \frac{1 - \text{sgn}(\delta_m^{j_1})}{2} \quad (\text{S10.2})$$

$$\mathcal{W}_3^{\text{gapless}} = \sum_{m=1}^{n_{d_1}} \text{sgn}(v_m^{d_1}) \frac{1 - \text{sgn}(\delta_m^{d_1})}{2} + \sum_{m=1}^{n_{e_1}} \text{sgn}(v_m^{e_1}) \frac{1 - \text{sgn}(\delta_m^{e_1})}{2} + \sum_{m=1}^{n_{f_1}} \text{sgn}(v_m^{f_1}) \frac{1 - \text{sgn}(\delta_m^{f_1})}{2} - \sum_{m=1}^{n_{h_1}} \text{sgn}(v_m^{h_1}) \frac{1 - \text{sgn}(\delta_m^{h_1})}{2} \quad (\text{S10.3})$$

### S11. SPACE GROUP NO. 11

| line segment                                        | character of irrep (generators only)                                                                                |
|-----------------------------------------------------|---------------------------------------------------------------------------------------------------------------------|
| $a \quad (\frac{t}{2}, 0, 0)$                       | $\{m_{010}   0 \ \frac{1}{2} \ 0 \}$<br>$a_1 \quad -i$<br>$a_2 \quad i$                                             |
| $b \quad (\frac{1}{2}, \frac{t}{2}, 0)$             | $\{2_{010}   0 \ \frac{1}{2} \ 0 \}$<br>$b_1 \quad -ie^{-\frac{1}{2}i\pi t}$<br>$b_2 \quad ie^{-\frac{1}{2}i\pi t}$ |
| $c \quad (\frac{1-t}{2}, \frac{1}{2}, 0)$           | $\{m_{010}   0 \ \frac{1}{2} \ 0 \}$<br>$c_1 \quad i$<br>$c_2 \quad -i$                                             |
| $d \quad (\frac{t}{2}, 0, \frac{1}{2})$             | $\{m_{010}   0 \ \frac{1}{2} \ 0 \}$<br>$d_1 \quad -i$<br>$d_2 \quad i$                                             |
| $e \quad (\frac{1}{2}, \frac{t}{2}, \frac{1}{2})$   | $\{2_{010}   0 \ \frac{1}{2} \ 0 \}$<br>$e_1 \quad -ie^{-\frac{1}{2}i\pi t}$<br>$e_2 \quad ie^{-\frac{1}{2}i\pi t}$ |
| $f \quad (\frac{1-t}{2}, \frac{1}{2}, \frac{1}{2})$ | $\{m_{010}   0 \ \frac{1}{2} \ 0 \}$<br>$f_1 \quad i$<br>$f_2 \quad -i$                                             |
| $g \quad (0, \frac{t}{2}, 0)$                       | $\{2_{010}   0 \ \frac{1}{2} \ 0 \}$<br>$g_1 \quad -ie^{-\frac{1}{2}i\pi t}$<br>$g_2 \quad ie^{-\frac{1}{2}i\pi t}$ |
| $h \quad (0, \frac{t}{2}, \frac{1}{2})$             | $\{2_{010}   0 \ \frac{1}{2} \ 0 \}$<br>$h_1 \quad -ie^{-\frac{1}{2}i\pi t}$<br>$h_2 \quad ie^{-\frac{1}{2}i\pi t}$ |

|                                                   |                                                                                 |
|---------------------------------------------------|---------------------------------------------------------------------------------|
| $i \quad (\frac{1}{2}, 0, \frac{t}{2})$           | $\{m_{010}   0 \quad \frac{1}{2} \quad 0 \}$<br>$i_1 \quad -i$<br>$i_2 \quad i$ |
| $j \quad (\frac{1}{2}, \frac{1}{2}, \frac{t}{2})$ | $\{m_{010}   0 \quad \frac{1}{2} \quad 0 \}$<br>$j_1 \quad i$<br>$j_2 \quad -i$ |

$$\begin{aligned}
\mathcal{W}_1^{\text{gapless}} = & \sum_{m=1}^{n_{a_1}} \text{sgn}(v_m^{a_1}) \frac{1 - \text{sgn}(\delta_m^{a_1})}{2} + 2 \sum_{m=1}^{n_{c_2}} \text{sgn}(v_m^{c_2}) \frac{1 - \text{sgn}(\delta_m^{c_2})}{2} + \sum_{m=1}^{n_{e_1}} \text{sgn}(v_m^{e_1}) \frac{1 - \text{sgn}(\delta_m^{e_1})}{2} \\
& + \sum_{m=1}^{n_{f_1}} \text{sgn}(v_m^{f_1}) \frac{1 - \text{sgn}(\delta_m^{f_1})}{2} - \sum_{m=1}^{n_{f_2}} \text{sgn}(v_m^{f_2}) \frac{1 - \text{sgn}(\delta_m^{f_2})}{2} - \sum_{m=1}^{n_{g_1}} \text{sgn}(v_m^{g_1}) \frac{1 - \text{sgn}(\delta_m^{g_1})}{2} \\
& + \sum_{m=1}^{n_{i_1}} \text{sgn}(v_m^{i_1}) \frac{1 - \text{sgn}(\delta_m^{i_1})}{2} - \sum_{m=1}^{n_{j_1}} \text{sgn}(v_m^{j_1}) \frac{1 - \text{sgn}(\delta_m^{j_1})}{2} - \sum_{m=1}^{n_{j_2}} \text{sgn}(v_m^{j_2}) \frac{1 - \text{sgn}(\delta_m^{j_2})}{2}
\end{aligned} \tag{S11.1}$$

$$\begin{aligned}
\mathcal{W}_2^{\text{gapless}} = & \sum_{m=1}^{n_{b_1}} \text{sgn}(v_m^{b_1}) \frac{1 - \text{sgn}(\delta_m^{b_1})}{2} - \sum_{m=1}^{n_{e_1}} \text{sgn}(v_m^{e_1}) \frac{1 - \text{sgn}(\delta_m^{e_1})}{2} - \sum_{m=1}^{n_{i_1}} \text{sgn}(v_m^{i_1}) \frac{1 - \text{sgn}(\delta_m^{i_1})}{2} \\
& + \sum_{m=1}^{n_{j_1}} \text{sgn}(v_m^{j_1}) \frac{1 - \text{sgn}(\delta_m^{j_1})}{2} + \sum_{m=1}^{n_{j_2}} \text{sgn}(v_m^{j_2}) \frac{1 - \text{sgn}(\delta_m^{j_2})}{2}
\end{aligned} \tag{S11.2}$$

$$\begin{aligned}
\mathcal{W}_3^{\text{gapless}} = & \sum_{m=1}^{n_{c_1}} \text{sgn}(v_m^{c_1}) \frac{1 - \text{sgn}(\delta_m^{c_1})}{2} - \sum_{m=1}^{n_{c_2}} \text{sgn}(v_m^{c_2}) \frac{1 - \text{sgn}(\delta_m^{c_2})}{2} - \sum_{m=1}^{n_{f_1}} \text{sgn}(v_m^{f_1}) \frac{1 - \text{sgn}(\delta_m^{f_1})}{2} + \sum_{m=1}^{n_{f_2}} \text{sgn}(v_m^{f_2}) \frac{1 - \text{sgn}(\delta_m^{f_2})}{2}
\end{aligned} \tag{S11.3}$$

$$\begin{aligned}
\mathcal{W}_4^{\text{gapless}} = & \sum_{m=1}^{n_{d_1}} \text{sgn}(v_m^{d_1}) \frac{1 - \text{sgn}(\delta_m^{d_1})}{2} + \sum_{m=1}^{n_{e_1}} \text{sgn}(v_m^{e_1}) \frac{1 - \text{sgn}(\delta_m^{e_1})}{2} + \sum_{m=1}^{n_{f_1}} \text{sgn}(v_m^{f_1}) \frac{1 - \text{sgn}(\delta_m^{f_1})}{2} \\
& + \sum_{m=1}^{n_{f_2}} \text{sgn}(v_m^{f_2}) \frac{1 - \text{sgn}(\delta_m^{f_2})}{2} - \sum_{m=1}^{n_{h_1}} \text{sgn}(v_m^{h_1}) \frac{1 - \text{sgn}(\delta_m^{h_1})}{2}
\end{aligned} \tag{S11.4}$$

$$\mathcal{W}_1^{\text{gapped}} = - \sum_{m=1}^{n_{f_1}} \text{sgn}(v_m^{f_1}) \frac{1 - \text{sgn}(\delta_m^{f_1})}{2} + \sum_{m=1}^{n_{f_2}} \text{sgn}(v_m^{f_2}) \frac{1 - \text{sgn}(\delta_m^{f_2})}{2} \tag{S11.5}$$

$$\mathcal{W}_2^{\text{gapped}} = - \sum_{m=1}^{n_{j_1}} \text{sgn}(v_m^{j_1}) \frac{1 - \text{sgn}(\delta_m^{j_1})}{2} + \sum_{m=1}^{n_{j_2}} \text{sgn}(v_m^{j_2}) \frac{1 - \text{sgn}(\delta_m^{j_2})}{2} \tag{S11.6}$$

## S12. SPACE GROUP NO. 12

| line segment | character of irrep (generators only) |
|--------------|--------------------------------------|
|--------------|--------------------------------------|

|                                                   |                                                               |
|---------------------------------------------------|---------------------------------------------------------------|
| $a \ (0, t, 0)$                                   | $\{2_{010}   0 \ 0 \ 0 \}$<br>$a_1 \quad -i$<br>$a_2 \quad i$ |
| $b \ (t, 0, 0)$                                   | $\{m_{010}   0 \ 0 \ 0 \}$<br>$b_1 \quad -i$<br>$b_2 \quad i$ |
| $c \ (\frac{1-t}{2}, \frac{t+1}{2}, 0)$           | $\{1   0 \ 0 \ 0 \}$<br>$c_1 \quad 1$                         |
| $d \ (0, t, \frac{1}{2})$                         | $\{2_{010}   0 \ 0 \ 0 \}$<br>$d_1 \quad -i$<br>$d_2 \quad i$ |
| $e \ (t, 0, \frac{1}{2})$                         | $\{m_{010}   0 \ 0 \ 0 \}$<br>$e_1 \quad -i$<br>$e_2 \quad i$ |
| $f \ (\frac{1-t}{2}, \frac{t+1}{2}, \frac{1}{2})$ | $\{1   0 \ 0 \ 0 \}$<br>$f_1 \quad 1$                         |
| $g \ (1, 0, \frac{t}{2})$                         | $\{m_{010}   0 \ 0 \ 0 \}$<br>$g_1 \quad -i$<br>$g_2 \quad i$ |

$$\mathcal{W}_1^{\text{gapless}} = \sum_{m=1}^{n_{a_1}} \text{sgn}(v_m^{a_1}) \frac{1 - \text{sgn}(\delta_m^{a_1})}{2} - \sum_{m=1}^{n_{b_1}} \text{sgn}(v_m^{b_1}) \frac{1 - \text{sgn}(\delta_m^{b_1})}{2} \quad (\text{S12.1})$$

$$\mathcal{W}_2^{\text{gapless}} = \sum_{m=1}^{n_{d_1}} \text{sgn}(v_m^{d_1}) \frac{1 - \text{sgn}(\delta_m^{d_1})}{2} - \sum_{m=1}^{n_{e_1}} \text{sgn}(v_m^{e_1}) \frac{1 - \text{sgn}(\delta_m^{e_1})}{2} \quad (\text{S12.2})$$

### S13. SPACE GROUP NO. 13

| line segment                                    | character of irrep (generators only)                                    |
|-------------------------------------------------|-------------------------------------------------------------------------|
| $a \ (\frac{t}{2}, 0, 0)$                       | $\{m_{010}   0 \ 0 \ \frac{1}{2} \}$<br>$a_1 \quad -i$<br>$a_2 \quad i$ |
| $b \ (\frac{1}{2}, \frac{t}{2}, 0)$             | $\{2_{010}   0 \ 0 \ \frac{1}{2} \}$<br>$b_1 \quad -i$<br>$b_2 \quad i$ |
| $c \ (\frac{1-t}{2}, \frac{1}{2}, 0)$           | $\{m_{010}   0 \ 0 \ \frac{1}{2} \}$<br>$c_1 \quad -i$<br>$c_2 \quad i$ |
| $d \ (\frac{t}{2}, 0, \frac{1}{2})$             | $\{m_{010}   0 \ 0 \ \frac{1}{2} \}$<br>$d_1 \quad -1$<br>$d_2 \quad 1$ |
| $e \ (\frac{1}{2}, \frac{t}{2}, \frac{1}{2})$   | $\{2_{010}   0 \ 0 \ \frac{1}{2} \}$<br>$e_1 \quad i$<br>$e_2 \quad -i$ |
| $f \ (\frac{1-t}{2}, \frac{1}{2}, \frac{1}{2})$ | $\{m_{010}   0 \ 0 \ \frac{1}{2} \}$<br>$f_1 \quad -1$<br>$f_2 \quad 1$ |
| $g \ (0, \frac{t}{2}, 0)$                       | $\{2_{010}   0 \ 0 \ \frac{1}{2} \}$<br>$g_1 \quad -i$<br>$g_2 \quad i$ |
| $h \ (0, \frac{t}{2}, \frac{1}{2})$             | $\{2_{010}   0 \ 0 \ \frac{1}{2} \}$<br>$h_1 \quad i$<br>$h_2 \quad -i$ |

|                                                   |                                                                                                                    |
|---------------------------------------------------|--------------------------------------------------------------------------------------------------------------------|
| $i \quad (\frac{1}{2}, 0, \frac{t}{2})$           | $\{m_{010}   0 \ 0 \ \frac{1}{2}\}$<br>$i_1 \quad -ie^{-\frac{1}{2}i\pi t}$<br>$i_2 \quad ie^{-\frac{1}{2}i\pi t}$ |
| $j \quad (\frac{1}{2}, \frac{1}{2}, \frac{t}{2})$ | $\{m_{010}   0 \ 0 \ \frac{1}{2}\}$<br>$j_1 \quad -ie^{-\frac{1}{2}i\pi t}$<br>$j_2 \quad ie^{-\frac{1}{2}i\pi t}$ |

$$\begin{aligned} \mathcal{W}_1^{\text{gapless}} = & \sum_{m=1}^{n_{a_1}} \text{sgn}(v_m^{a_1}) \frac{1 - \text{sgn}(\delta_m^{a_1})}{2} + \sum_{m=1}^{n_{c_1}} \text{sgn}(v_m^{c_1}) \frac{1 - \text{sgn}(\delta_m^{c_1})}{2} + \sum_{m=1}^{n_{e_1}} \text{sgn}(v_m^{e_1}) \frac{1 - \text{sgn}(\delta_m^{e_1})}{2} + \sum_{m=1}^{n_{e_2}} \text{sgn}(v_m^{e_2}) \frac{1 - \text{sgn}(\delta_m^{e_2})}{2} \\ & - \sum_{m=1}^{n_{g_1}} \text{sgn}(v_m^{g_1}) \frac{1 - \text{sgn}(\delta_m^{g_1})}{2} + \sum_{m=1}^{n_{i_1}} \text{sgn}(v_m^{i_1}) \frac{1 - \text{sgn}(\delta_m^{i_1})}{2} - \sum_{m=1}^{n_{j_1}} \text{sgn}(v_m^{j_1}) \frac{1 - \text{sgn}(\delta_m^{j_1})}{2} \end{aligned} \quad (\text{S13.1})$$

$$\begin{aligned} \mathcal{W}_2^{\text{gapless}} = & \sum_{m=1}^{n_{b_1}} \text{sgn}(v_m^{b_1}) \frac{1 - \text{sgn}(\delta_m^{b_1})}{2} - \sum_{m=1}^{n_{e_1}} \text{sgn}(v_m^{e_1}) \frac{1 - \text{sgn}(\delta_m^{e_1})}{2} - \sum_{m=1}^{n_{e_2}} \text{sgn}(v_m^{e_2}) \frac{1 - \text{sgn}(\delta_m^{e_2})}{2} \\ & - \sum_{m=1}^{n_{i_1}} \text{sgn}(v_m^{i_1}) \frac{1 - \text{sgn}(\delta_m^{i_1})}{2} + \sum_{m=1}^{n_{j_1}} \text{sgn}(v_m^{j_1}) \frac{1 - \text{sgn}(\delta_m^{j_1})}{2} \end{aligned} \quad (\text{S13.2})$$

$$\begin{aligned} \mathcal{W}_3^{\text{gapless}} = & \sum_{m=1}^{n_{d_1}} \text{sgn}(v_m^{d_1}) \frac{1 - \text{sgn}(\delta_m^{d_1})}{2} + \sum_{m=1}^{n_{e_1}} \text{sgn}(v_m^{e_1}) \frac{1 - \text{sgn}(\delta_m^{e_1})}{2} + \sum_{m=1}^{n_{e_2}} \text{sgn}(v_m^{e_2}) \frac{1 - \text{sgn}(\delta_m^{e_2})}{2} \\ & + \sum_{m=1}^{n_{f_1}} \text{sgn}(v_m^{f_1}) \frac{1 - \text{sgn}(\delta_m^{f_1})}{2} - \sum_{m=1}^{n_{h_1}} \text{sgn}(v_m^{h_1}) \frac{1 - \text{sgn}(\delta_m^{h_1})}{2} - \sum_{m=1}^{n_{h_2}} \text{sgn}(v_m^{h_2}) \frac{1 - \text{sgn}(\delta_m^{h_2})}{2} \end{aligned} \quad (\text{S13.3})$$

$$\mathcal{W}_1^{\text{gapped}} = - \sum_{m=1}^{n_{h_1}} \text{sgn}(v_m^{h_1}) \frac{1 - \text{sgn}(\delta_m^{h_1})}{2} + \sum_{m=1}^{n_{h_2}} \text{sgn}(v_m^{h_2}) \frac{1 - \text{sgn}(\delta_m^{h_2})}{2} \quad (\text{S13.4})$$

$$\mathcal{W}_2^{\text{gapped}} = - \sum_{m=1}^{n_{e_1}} \text{sgn}(v_m^{e_1}) \frac{1 - \text{sgn}(\delta_m^{e_1})}{2} + \sum_{m=1}^{n_{e_2}} \text{sgn}(v_m^{e_2}) \frac{1 - \text{sgn}(\delta_m^{e_2})}{2} \quad (\text{S13.5})$$

$$\mathcal{X}_1 = \sum_{m=1}^{n_{f_1}} \frac{1 - \text{sgn}(\delta_m^{f_1})}{2} \mod 2 \quad (\text{S13.6})$$

#### S14. SPACE GROUP NO. 14

|              |                                      |
|--------------|--------------------------------------|
| line segment | character of irrep (generators only) |
|--------------|--------------------------------------|

|                                                     |                                                                                                                                          |
|-----------------------------------------------------|------------------------------------------------------------------------------------------------------------------------------------------|
| $a \quad (\frac{t}{2}, 0, 0)$                       | $\{m_{010}   0 \quad \frac{1}{2} \quad \frac{1}{2}\}$<br>$a_1 \quad -i$<br>$a_2 \quad i$                                                 |
| $b \quad (\frac{1}{2}, \frac{t}{2}, 0)$             | $\{2_{010}   0 \quad \frac{1}{2} \quad \frac{1}{2}\}$<br>$b_1 \quad -ie^{-\frac{1}{2}i\pi t}$<br>$b_2 \quad ie^{-\frac{1}{2}i\pi t}$     |
| $c \quad (\frac{1-t}{2}, \frac{1}{2}, 0)$           | $\{m_{010}   0 \quad \frac{1}{2} \quad \frac{1}{2}\}$<br>$c_1 \quad i$<br>$c_2 \quad -i$                                                 |
| $d \quad (\frac{t}{2}, 0, \frac{1}{2})$             | $\{m_{010}   0 \quad \frac{1}{2} \quad \frac{1}{2}\}$<br>$d_1 \quad -1$<br>$d_2 \quad 1$                                                 |
| $e \quad (\frac{1}{2}, \frac{t}{2}, \frac{1}{2})$   | $\{2_{010}   0 \quad \frac{1}{2} \quad \frac{1}{2}\}$<br>$e_1 \quad -e^{-\frac{1}{2}i\pi(t+1)}$<br>$e_2 \quad e^{-\frac{1}{2}i\pi(t+1)}$ |
| $f \quad (\frac{1-t}{2}, \frac{1}{2}, \frac{1}{2})$ | $\{m_{010}   0 \quad \frac{1}{2} \quad \frac{1}{2}\}$<br>$f_1 \quad 1$<br>$f_2 \quad -1$                                                 |
| $g \quad (0, \frac{t}{2}, 0)$                       | $\{2_{010}   0 \quad \frac{1}{2} \quad \frac{1}{2}\}$<br>$g_1 \quad -ie^{-\frac{1}{2}i\pi t}$<br>$g_2 \quad ie^{-\frac{1}{2}i\pi t}$     |
| $h \quad (0, \frac{t}{2}, \frac{1}{2})$             | $\{2_{010}   0 \quad \frac{1}{2} \quad \frac{1}{2}\}$<br>$h_1 \quad -e^{-\frac{1}{2}i\pi(t+1)}$<br>$h_2 \quad e^{-\frac{1}{2}i\pi(t+1)}$ |
| $i \quad (\frac{1}{2}, 0, \frac{t}{2})$             | $\{m_{010}   0 \quad \frac{1}{2} \quad \frac{1}{2}\}$<br>$i_1 \quad -ie^{-\frac{1}{2}i\pi t}$<br>$i_2 \quad ie^{-\frac{1}{2}i\pi t}$     |
| $j \quad (\frac{1}{2}, \frac{1}{2}, \frac{t}{2})$   | $\{m_{010}   0 \quad \frac{1}{2} \quad \frac{1}{2}\}$<br>$j_1 \quad -e^{-\frac{1}{2}i\pi(t+1)}$<br>$j_2 \quad e^{-\frac{1}{2}i\pi(t+1)}$ |

$$\begin{aligned}
\mathcal{W}_1^{\text{gapless}} = & \sum_{m=1}^{n_{a_1}} \text{sgn}(v_m^{a_1}) \frac{1 - \text{sgn}(\delta_m^{a_1})}{2} + 2 \sum_{m=1}^{n_{c_2}} \text{sgn}(v_m^{c_2}) \frac{1 - \text{sgn}(\delta_m^{c_2})}{2} + \sum_{m=1}^{n_{e_1}} \text{sgn}(v_m^{e_1}) \frac{1 - \text{sgn}(\delta_m^{e_1})}{2} + \sum_{m=1}^{n_{e_2}} \text{sgn}(v_m^{e_2}) \frac{1 - \text{sgn}(\delta_m^{e_2})}{2} \\
& - \sum_{m=1}^{n_{g_1}} \text{sgn}(v_m^{g_1}) \frac{1 - \text{sgn}(\delta_m^{g_1})}{2} + \sum_{m=1}^{n_{i_1}} \text{sgn}(v_m^{i_1}) \frac{1 - \text{sgn}(\delta_m^{i_1})}{2} - \sum_{m=1}^{n_{j_1}} \text{sgn}(v_m^{j_1}) \frac{1 - \text{sgn}(\delta_m^{j_1})}{2} - \sum_{m=1}^{n_{j_2}} \text{sgn}(v_m^{j_2}) \frac{1 - \text{sgn}(\delta_m^{j_2})}{2}
\end{aligned} \tag{S14.1}$$

$$\begin{aligned}
\mathcal{W}_2^{\text{gapless}} = & \sum_{m=1}^{n_{b_1}} \text{sgn}(v_m^{b_1}) \frac{1 - \text{sgn}(\delta_m^{b_1})}{2} - \sum_{m=1}^{n_{e_1}} \text{sgn}(v_m^{e_1}) \frac{1 - \text{sgn}(\delta_m^{e_1})}{2} - \sum_{m=1}^{n_{e_2}} \text{sgn}(v_m^{e_2}) \frac{1 - \text{sgn}(\delta_m^{e_2})}{2} \\
& - \sum_{m=1}^{n_{i_1}} \text{sgn}(v_m^{i_1}) \frac{1 - \text{sgn}(\delta_m^{i_1})}{2} + \sum_{m=1}^{n_{j_1}} \text{sgn}(v_m^{j_1}) \frac{1 - \text{sgn}(\delta_m^{j_1})}{2} + \sum_{m=1}^{n_{j_2}} \text{sgn}(v_m^{j_2}) \frac{1 - \text{sgn}(\delta_m^{j_2})}{2}
\end{aligned} \tag{S14.2}$$

$$\mathcal{W}_3^{\text{gapless}} = \sum_{m=1}^{n_{c_1}} \text{sgn}(v_m^{c_1}) \frac{1 - \text{sgn}(\delta_m^{c_1})}{2} - \sum_{m=1}^{n_{c_2}} \text{sgn}(v_m^{c_2}) \frac{1 - \text{sgn}(\delta_m^{c_2})}{2} \tag{S14.3}$$

$$\begin{aligned}
\mathcal{W}_4^{\text{gapless}} = & \sum_{m=1}^{n_{d_1}} \text{sgn}(v_m^{d_1}) \frac{1 - \text{sgn}(\delta_m^{d_1})}{2} + \sum_{m=1}^{n_{e_1}} \text{sgn}(v_m^{e_1}) \frac{1 - \text{sgn}(\delta_m^{e_1})}{2} + \sum_{m=1}^{n_{e_2}} \text{sgn}(v_m^{e_2}) \frac{1 - \text{sgn}(\delta_m^{e_2})}{2} + \sum_{m=1}^{n_{f_1}} \text{sgn}(v_m^{f_1}) \frac{1 - \text{sgn}(\delta_m^{f_1})}{2} \\
& + \sum_{m=1}^{n_{f_2}} \text{sgn}(v_m^{f_2}) \frac{1 - \text{sgn}(\delta_m^{f_2})}{2} - \sum_{m=1}^{n_{h_1}} \text{sgn}(v_m^{h_1}) \frac{1 - \text{sgn}(\delta_m^{h_1})}{2} - \sum_{m=1}^{n_{h_2}} \text{sgn}(v_m^{h_2}) \frac{1 - \text{sgn}(\delta_m^{h_2})}{2}
\end{aligned} \tag{S14.4}$$

$$\begin{aligned}
\mathcal{X}_1 = & \sum_{m=1}^{n_{e_1}} \frac{1 - \text{sgn}(\delta_m^{e_1})}{2} + \sum_{m=1}^{n_{e_2}} \frac{1 - \text{sgn}(\delta_m^{e_2})}{2} + \sum_{m=1}^{n_{f_1}} \frac{1 - \text{sgn}(\delta_m^{f_1})}{2} + \sum_{m=1}^{n_{f_2}} \frac{1 - \text{sgn}(\delta_m^{f_2})}{2} \\
& + \sum_{m=1}^{n_{h_1}} \frac{1 - \text{sgn}(\delta_m^{h_1})}{2} + \sum_{m=1}^{n_{h_2}} \frac{1 - \text{sgn}(\delta_m^{h_2})}{2} \pmod{2}
\end{aligned} \tag{S14.5}$$

$$\mathcal{X}_2 = \sum_{m=1}^{n_{e_1}} \frac{1 - \text{sgn}(\delta_m^{e_1})}{2} + \sum_{m=1}^{n_{e_2}} \frac{1 - \text{sgn}(\delta_m^{e_2})}{2} + \sum_{m=1}^{n_{j_1}} \frac{1 - \text{sgn}(\delta_m^{j_1})}{2} + \sum_{m=1}^{n_{j_2}} \frac{1 - \text{sgn}(\delta_m^{j_2})}{2} \pmod{2} \tag{S14.6}$$

### S15. SPACE GROUP NO. 15

| line segment                                      | character of irrep (generators only)                                                                               |
|---------------------------------------------------|--------------------------------------------------------------------------------------------------------------------|
| $a \ (0, t, 0)$                                   | $\{2_{010}   0 \ 0 \ \frac{1}{2}\}$<br>$a_1 \quad -i$<br>$a_2 \quad i$                                             |
| $b \ (t, 0, 0)$                                   | $\{m_{010}   0 \ 0 \ \frac{1}{2}\}$<br>$b_1 \quad -i$<br>$b_2 \quad i$                                             |
| $c \ (\frac{1-t}{2}, \frac{t+1}{2}, 0)$           | $\{1   0 \ 0 \ 0\}$<br>$c_1 \quad 1$                                                                               |
| $d \ (0, t, \frac{1}{2})$                         | $\{2_{010}   0 \ 0 \ \frac{1}{2}\}$<br>$d_1 \quad i$<br>$d_2 \quad -i$                                             |
| $e \ (t, 0, \frac{1}{2})$                         | $\{m_{010}   0 \ 0 \ \frac{1}{2}\}$<br>$e_1 \quad -1$<br>$e_2 \quad 1$                                             |
| $f \ (\frac{1-t}{2}, \frac{t+1}{2}, \frac{1}{2})$ | $\{1   0 \ 0 \ 0\}$<br>$f_1 \quad 1$                                                                               |
| $g \ (1, 0, \frac{t}{2})$                         | $\{m_{010}   0 \ 0 \ \frac{1}{2}\}$<br>$g_1 \quad -ie^{-\frac{1}{2}i\pi t}$<br>$g_2 \quad ie^{-\frac{1}{2}i\pi t}$ |

$$\mathcal{W}_1^{\text{gapless}} = \sum_{m=1}^{n_{a_1}} \text{sgn}(v_m^{a_1}) \frac{1 - \text{sgn}(\delta_m^{a_1})}{2} - \sum_{m=1}^{n_{b_1}} \text{sgn}(v_m^{b_1}) \frac{1 - \text{sgn}(\delta_m^{b_1})}{2} \tag{S15.1}$$

$$\mathcal{W}_2^{\text{gapless}} = \sum_{m=1}^{n_{d_1}} \text{sgn}(v_m^{d_1}) \frac{1 - \text{sgn}(\delta_m^{d_1})}{2} + \sum_{m=1}^{n_{d_2}} \text{sgn}(v_m^{d_2}) \frac{1 - \text{sgn}(\delta_m^{d_2})}{2} - \sum_{m=1}^{n_{e_1}} \text{sgn}(v_m^{e_1}) \frac{1 - \text{sgn}(\delta_m^{e_1})}{2} \tag{S15.2}$$

$$\mathcal{W}_1^{\text{gapped}} = 2 \sum_{m=1}^{n_{d_2}} \text{sgn}(v_m^{d_2}) \frac{1 - \text{sgn}(\delta_m^{d_2})}{2} - \sum_{m=1}^{n_{e_1}} \text{sgn}(v_m^{e_1}) \frac{1 - \text{sgn}(\delta_m^{e_1})}{2} \tag{S15.3}$$



## S16. SPACE GROUP NO. 16

| line segment                                        | character of irrep (generators only)                                          |
|-----------------------------------------------------|-------------------------------------------------------------------------------|
| $a \quad (\frac{t}{2}, 0, 0)$                       | $\begin{matrix} \{2_{100}   0 & 0 & 0 \} \\ a_1 & -i \\ a_2 & i \end{matrix}$ |
| $b \quad (0, \frac{t}{2}, 0)$                       | $\begin{matrix} \{2_{010}   0 & 0 & 0 \} \\ b_1 & -i \\ b_2 & i \end{matrix}$ |
| $c \quad (\frac{1}{2}, \frac{t}{2}, 0)$             | $\begin{matrix} \{2_{010}   0 & 0 & 0 \} \\ c_1 & -i \\ c_2 & i \end{matrix}$ |
| $d \quad (\frac{1-t}{2}, \frac{1}{2}, 0)$           | $\begin{matrix} \{2_{100}   0 & 0 & 0 \} \\ d_1 & -i \\ d_2 & i \end{matrix}$ |
| $e \quad (\frac{t}{2}, 0, \frac{1}{2})$             | $\begin{matrix} \{2_{100}   0 & 0 & 0 \} \\ e_1 & -i \\ e_2 & i \end{matrix}$ |
| $f \quad (0, \frac{t}{2}, \frac{1}{2})$             | $\begin{matrix} \{2_{010}   0 & 0 & 0 \} \\ f_1 & -i \\ f_2 & i \end{matrix}$ |
| $g \quad (\frac{1}{2}, \frac{t}{2}, \frac{1}{2})$   | $\begin{matrix} \{2_{010}   0 & 0 & 0 \} \\ g_1 & -i \\ g_2 & i \end{matrix}$ |
| $h \quad (\frac{1-t}{2}, \frac{1}{2}, \frac{1}{2})$ | $\begin{matrix} \{2_{100}   0 & 0 & 0 \} \\ h_1 & -i \\ h_2 & i \end{matrix}$ |
| $i \quad (0, 0, \frac{t}{2})$                       | $\begin{matrix} \{2_{001}   0 & 0 & 0 \} \\ i_1 & -i \\ i_2 & i \end{matrix}$ |
| $j \quad (\frac{1}{2}, 0, \frac{t}{2})$             | $\begin{matrix} \{2_{001}   0 & 0 & 0 \} \\ j_1 & -i \\ j_2 & i \end{matrix}$ |
| $k \quad (\frac{1}{2}, \frac{1}{2}, \frac{t}{2})$   | $\begin{matrix} \{2_{001}   0 & 0 & 0 \} \\ k_1 & -i \\ k_2 & i \end{matrix}$ |
| $l \quad (0, \frac{1}{2}, \frac{t}{2})$             | $\begin{matrix} \{2_{001}   0 & 0 & 0 \} \\ l_1 & -i \\ l_2 & i \end{matrix}$ |

$$\begin{aligned}
\mathcal{W}_1^{\text{gapless}} = & \sum_{m=1}^{n_{a_1}} \text{sgn}(v_m^{a_1}) \frac{1 - \text{sgn}(\delta_m^{a_1})}{2} + \sum_{m=1}^{n_{a_2}} \text{sgn}(v_m^{a_2}) \frac{1 - \text{sgn}(\delta_m^{a_2})}{2} - \sum_{m=1}^{n_{f_1}} \text{sgn}(v_m^{f_1}) \frac{1 - \text{sgn}(\delta_m^{f_1})}{2} \\
& - \sum_{m=1}^{n_{f_2}} \text{sgn}(v_m^{f_2}) \frac{1 - \text{sgn}(\delta_m^{f_2})}{2} + \sum_{m=1}^{n_{g_1}} \text{sgn}(v_m^{g_1}) \frac{1 - \text{sgn}(\delta_m^{g_1})}{2} + \sum_{m=1}^{n_{g_2}} \text{sgn}(v_m^{g_2}) \frac{1 - \text{sgn}(\delta_m^{g_2})}{2} \\
& + \sum_{m=1}^{n_{h_1}} \text{sgn}(v_m^{h_1}) \frac{1 - \text{sgn}(\delta_m^{h_1})}{2} + \sum_{m=1}^{n_{h_2}} \text{sgn}(v_m^{h_2}) \frac{1 - \text{sgn}(\delta_m^{h_2})}{2} - \sum_{m=1}^{n_{i_1}} \text{sgn}(v_m^{i_1}) \frac{1 - \text{sgn}(\delta_m^{i_1})}{2} \\
& - \sum_{m=1}^{n_{i_2}} \text{sgn}(v_m^{i_2}) \frac{1 - \text{sgn}(\delta_m^{i_2})}{2} + \sum_{m=1}^{n_{j_1}} \text{sgn}(v_m^{j_1}) \frac{1 - \text{sgn}(\delta_m^{j_1})}{2} + \sum_{m=1}^{n_{j_2}} \text{sgn}(v_m^{j_2}) \frac{1 - \text{sgn}(\delta_m^{j_2})}{2}
\end{aligned} \tag{S16.1}$$

$$\begin{aligned}
\mathcal{W}_2^{\text{gapless}} = & \sum_{m=1}^{n_{b_1}} \text{sgn}(v_m^{b_1}) \frac{1 - \text{sgn}(\delta_m^{b_1})}{2} + \sum_{m=1}^{n_{b_2}} \text{sgn}(v_m^{b_2}) \frac{1 - \text{sgn}(\delta_m^{b_2})}{2} - \sum_{m=1}^{n_{f_1}} \text{sgn}(v_m^{f_1}) \frac{1 - \text{sgn}(\delta_m^{f_1})}{2} - \sum_{m=1}^{n_{f_2}} \text{sgn}(v_m^{f_2}) \frac{1 - \text{sgn}(\delta_m^{f_2})}{2} \\
& - \sum_{m=1}^{n_{i_1}} \text{sgn}(v_m^{i_1}) \frac{1 - \text{sgn}(\delta_m^{i_1})}{2} - \sum_{m=1}^{n_{i_2}} \text{sgn}(v_m^{i_2}) \frac{1 - \text{sgn}(\delta_m^{i_2})}{2} + \sum_{m=1}^{n_{l_1}} \text{sgn}(v_m^{l_1}) \frac{1 - \text{sgn}(\delta_m^{l_1})}{2} + \sum_{m=1}^{n_{l_2}} \text{sgn}(v_m^{l_2}) \frac{1 - \text{sgn}(\delta_m^{l_2})}{2}
\end{aligned} \tag{S16.2}$$

$$\begin{aligned}
\mathcal{W}_3^{\text{gapless}} = & \sum_{m=1}^{n_{c_1}} \text{sgn}(v_m^{c_1}) \frac{1 - \text{sgn}(\delta_m^{c_1})}{2} + \sum_{m=1}^{n_{c_2}} \text{sgn}(v_m^{c_2}) \frac{1 - \text{sgn}(\delta_m^{c_2})}{2} - \sum_{m=1}^{n_{g_1}} \text{sgn}(v_m^{g_1}) \frac{1 - \text{sgn}(\delta_m^{g_1})}{2} \\
& - \sum_{m=1}^{n_{g_2}} \text{sgn}(v_m^{g_2}) \frac{1 - \text{sgn}(\delta_m^{g_2})}{2} - \sum_{m=1}^{n_{j_1}} \text{sgn}(v_m^{j_1}) \frac{1 - \text{sgn}(\delta_m^{j_1})}{2} - \sum_{m=1}^{n_{j_2}} \text{sgn}(v_m^{j_2}) \frac{1 - \text{sgn}(\delta_m^{j_2})}{2} \\
& + \sum_{m=1}^{n_{k_1}} \text{sgn}(v_m^{k_1}) \frac{1 - \text{sgn}(\delta_m^{k_1})}{2} + \sum_{m=1}^{n_{k_2}} \text{sgn}(v_m^{k_2}) \frac{1 - \text{sgn}(\delta_m^{k_2})}{2}
\end{aligned} \tag{S16.3}$$

$$\begin{aligned}
\mathcal{W}_4^{\text{gapless}} = & \sum_{m=1}^{n_{d_1}} \text{sgn}(v_m^{d_1}) \frac{1 - \text{sgn}(\delta_m^{d_1})}{2} + \sum_{m=1}^{n_{d_2}} \text{sgn}(v_m^{d_2}) \frac{1 - \text{sgn}(\delta_m^{d_2})}{2} - \sum_{m=1}^{n_{h_1}} \text{sgn}(v_m^{h_1}) \frac{1 - \text{sgn}(\delta_m^{h_1})}{2} \\
& - \sum_{m=1}^{n_{h_2}} \text{sgn}(v_m^{h_2}) \frac{1 - \text{sgn}(\delta_m^{h_2})}{2} - \sum_{m=1}^{n_{k_1}} \text{sgn}(v_m^{k_1}) \frac{1 - \text{sgn}(\delta_m^{k_1})}{2} \\
& - \sum_{m=1}^{n_{k_2}} \text{sgn}(v_m^{k_2}) \frac{1 - \text{sgn}(\delta_m^{k_2})}{2} + \sum_{m=1}^{n_{l_1}} \text{sgn}(v_m^{l_1}) \frac{1 - \text{sgn}(\delta_m^{l_1})}{2} + \sum_{m=1}^{n_{l_2}} \text{sgn}(v_m^{l_2}) \frac{1 - \text{sgn}(\delta_m^{l_2})}{2}
\end{aligned} \tag{S16.4}$$

$$\begin{aligned}
\mathcal{W}_5^{\text{gapless}} = & \sum_{m=1}^{n_{e_1}} \text{sgn}(v_m^{e_1}) \frac{1 - \text{sgn}(\delta_m^{e_1})}{2} + \sum_{m=1}^{n_{e_2}} \text{sgn}(v_m^{e_2}) \frac{1 - \text{sgn}(\delta_m^{e_2})}{2} - \sum_{m=1}^{n_{f_1}} \text{sgn}(v_m^{f_1}) \frac{1 - \text{sgn}(\delta_m^{f_1})}{2} \\
& - \sum_{m=1}^{n_{f_2}} \text{sgn}(v_m^{f_2}) \frac{1 - \text{sgn}(\delta_m^{f_2})}{2} + \sum_{m=1}^{n_{g_1}} \text{sgn}(v_m^{g_1}) \frac{1 - \text{sgn}(\delta_m^{g_1})}{2} + \sum_{m=1}^{n_{g_2}} \text{sgn}(v_m^{g_2}) \frac{1 - \text{sgn}(\delta_m^{g_2})}{2} \\
& + \sum_{m=1}^{n_{h_1}} \text{sgn}(v_m^{h_1}) \frac{1 - \text{sgn}(\delta_m^{h_1})}{2} + \sum_{m=1}^{n_{h_2}} \text{sgn}(v_m^{h_2}) \frac{1 - \text{sgn}(\delta_m^{h_2})}{2}
\end{aligned} \tag{S16.5}$$

$$\mathcal{W}_1^{\text{gapped}} = - \sum_{m=1}^{n_{f_1}} \text{sgn}(v_m^{f_1}) \frac{1 - \text{sgn}(\delta_m^{f_1})}{2} + \sum_{m=1}^{n_{f_2}} \text{sgn}(v_m^{f_2}) \frac{1 - \text{sgn}(\delta_m^{f_2})}{2} \tag{S16.6}$$

$$\mathcal{W}_2^{\text{gapped}} = - \sum_{m=1}^{n_{g_1}} \text{sgn}(v_m^{g_1}) \frac{1 - \text{sgn}(\delta_m^{g_1})}{2} + \sum_{m=1}^{n_{g_2}} \text{sgn}(v_m^{g_2}) \frac{1 - \text{sgn}(\delta_m^{g_2})}{2} \tag{S16.7}$$

$$\mathcal{W}_3^{\text{gapped}} = \sum_{m=1}^{n_{e_2}} \text{sgn}(v_m^{e_2}) \frac{1 - \text{sgn}(\delta_m^{e_2})}{2} - \sum_{m=1}^{n_{f_1}} \text{sgn}(v_m^{f_1}) \frac{1 - \text{sgn}(\delta_m^{f_1})}{2} + \sum_{m=1}^{n_{g_1}} \text{sgn}(v_m^{g_1}) \frac{1 - \text{sgn}(\delta_m^{g_1})}{2} + \sum_{m=1}^{n_{h_1}} \text{sgn}(v_m^{h_1}) \frac{1 - \text{sgn}(\delta_m^{h_1})}{2} \tag{S16.8}$$



## S17. SPACE GROUP NO. 17

| line segment                                             | character of irrep (generators only)                                                                                               |
|----------------------------------------------------------|------------------------------------------------------------------------------------------------------------------------------------|
| $a \left(\frac{t}{2}, 0, 0\right)$                       | $\begin{matrix} \{2_{100}   0 & 0 & 0\} \\ a_1 & -i \\ a_2 & i \end{matrix}$                                                       |
| $b \left(0, \frac{t}{2}, 0\right)$                       | $\begin{matrix} \{2_{010}   0 & 0 & \frac{1}{2}\} \\ b_1 & -i \\ b_2 & i \end{matrix}$                                             |
| $c \left(\frac{1}{2}, \frac{t}{2}, 0\right)$             | $\begin{matrix} \{2_{010}   0 & 0 & \frac{1}{2}\} \\ c_1 & -i \\ c_2 & i \end{matrix}$                                             |
| $d \left(\frac{1-t}{2}, \frac{1}{2}, 0\right)$           | $\begin{matrix} \{2_{100}   0 & 0 & 0\} \\ d_1 & -i \\ d_2 & i \end{matrix}$                                                       |
| $e \left(\frac{t}{2}, 0, \frac{1}{2}\right)$             | $\begin{matrix} \{2_{100}   0 & 0 & 0\} \\ e_1 & -i \\ e_2 & i \end{matrix}$                                                       |
| $f \left(0, \frac{t}{2}, \frac{1}{2}\right)$             | $\begin{matrix} \{2_{010}   0 & 0 & \frac{1}{2}\} \\ f_1 & i \\ f_2 & -i \end{matrix}$                                             |
| $g \left(\frac{1}{2}, \frac{t}{2}, \frac{1}{2}\right)$   | $\begin{matrix} \{2_{010}   0 & 0 & \frac{1}{2}\} \\ g_1 & i \\ g_2 & -i \end{matrix}$                                             |
| $h \left(\frac{1-t}{2}, \frac{1}{2}, \frac{1}{2}\right)$ | $\begin{matrix} \{2_{100}   0 & 0 & 0\} \\ h_1 & -i \\ h_2 & i \end{matrix}$                                                       |
| $i \left(0, 0, \frac{t}{2}\right)$                       | $\begin{matrix} \{2_{001}   0 & 0 & \frac{1}{2}\} \\ i_1 & -ie^{-\frac{1}{2}i\pi t} \\ i_2 & ie^{-\frac{1}{2}i\pi t} \end{matrix}$ |
| $j \left(\frac{1}{2}, 0, \frac{t}{2}\right)$             | $\begin{matrix} \{2_{001}   0 & 0 & \frac{1}{2}\} \\ j_1 & -ie^{-\frac{1}{2}i\pi t} \\ j_2 & ie^{-\frac{1}{2}i\pi t} \end{matrix}$ |
| $k \left(\frac{1}{2}, \frac{1}{2}, \frac{t}{2}\right)$   | $\begin{matrix} \{2_{001}   0 & 0 & \frac{1}{2}\} \\ k_1 & -ie^{-\frac{1}{2}i\pi t} \\ k_2 & ie^{-\frac{1}{2}i\pi t} \end{matrix}$ |
| $l \left(0, \frac{1}{2}, \frac{t}{2}\right)$             | $\begin{matrix} \{2_{001}   0 & 0 & \frac{1}{2}\} \\ l_1 & -ie^{-\frac{1}{2}i\pi t} \\ l_2 & ie^{-\frac{1}{2}i\pi t} \end{matrix}$ |

$$\begin{aligned}
\mathcal{W}_1^{\text{gapless}} = & \sum_{m=1}^{n_{a_1}} \text{sgn}(v_m^{a_1}) \frac{1 - \text{sgn}(\delta_m^{a_1})}{2} + \sum_{m=1}^{n_{a_2}} \text{sgn}(v_m^{a_2}) \frac{1 - \text{sgn}(\delta_m^{a_2})}{2} - 2 \sum_{m=1}^{n_{f_1}} \text{sgn}(v_m^{f_1}) \frac{1 - \text{sgn}(\delta_m^{f_1})}{2} \\
& + 2 \sum_{m=1}^{n_{g_1}} \text{sgn}(v_m^{g_1}) \frac{1 - \text{sgn}(\delta_m^{g_1})}{2} + 2 \sum_{m=1}^{n_{h_1}} \text{sgn}(v_m^{h_1}) \frac{1 - \text{sgn}(\delta_m^{h_1})}{2} - \sum_{m=1}^{n_{i_1}} \text{sgn}(v_m^{i_1}) \frac{1 - \text{sgn}(\delta_m^{i_1})}{2} \\
& - \sum_{m=1}^{n_{i_2}} \text{sgn}(v_m^{i_2}) \frac{1 - \text{sgn}(\delta_m^{i_2})}{2} + \sum_{m=1}^{n_{j_1}} \text{sgn}(v_m^{j_1}) \frac{1 - \text{sgn}(\delta_m^{j_1})}{2} + \sum_{m=1}^{n_{j_2}} \text{sgn}(v_m^{j_2}) \frac{1 - \text{sgn}(\delta_m^{j_2})}{2}
\end{aligned} \tag{S17.1}$$

$$\begin{aligned}
\mathcal{W}_2^{\text{gapless}} = & \sum_{m=1}^{n_{b_1}} \text{sgn}(v_m^{b_1}) \frac{1 - \text{sgn}(\delta_m^{b_1})}{2} + \sum_{m=1}^{n_{b_2}} \text{sgn}(v_m^{b_2}) \frac{1 - \text{sgn}(\delta_m^{b_2})}{2} - 2 \sum_{m=1}^{n_{f_1}} \text{sgn}(v_m^{f_1}) \frac{1 - \text{sgn}(\delta_m^{f_1})}{2} \\
& - \sum_{m=1}^{n_{i_1}} \text{sgn}(v_m^{i_1}) \frac{1 - \text{sgn}(\delta_m^{i_1})}{2} - \sum_{m=1}^{n_{i_2}} \text{sgn}(v_m^{i_2}) \frac{1 - \text{sgn}(\delta_m^{i_2})}{2} + \sum_{m=1}^{n_{l_1}} \text{sgn}(v_m^{l_1}) \frac{1 - \text{sgn}(\delta_m^{l_1})}{2} + \sum_{m=1}^{n_{l_2}} \text{sgn}(v_m^{l_2}) \frac{1 - \text{sgn}(\delta_m^{l_2})}{2}
\end{aligned} \tag{S17.2}$$

$$\begin{aligned}
\mathcal{W}_3^{\text{gapless}} = & \sum_{m=1}^{n_{c_1}} \text{sgn}(v_m^{c_1}) \frac{1 - \text{sgn}(\delta_m^{c_1})}{2} + \sum_{m=1}^{n_{c_2}} \text{sgn}(v_m^{c_2}) \frac{1 - \text{sgn}(\delta_m^{c_2})}{2} - 2 \sum_{m=1}^{n_{g_1}} \text{sgn}(v_m^{g_1}) \frac{1 - \text{sgn}(\delta_m^{g_1})}{2} - \sum_{m=1}^{n_{j_1}} \text{sgn}(v_m^{j_1}) \frac{1 - \text{sgn}(\delta_m^{j_1})}{2} \\
& - \sum_{m=1}^{n_{j_2}} \text{sgn}(v_m^{j_2}) \frac{1 - \text{sgn}(\delta_m^{j_2})}{2} + \sum_{m=1}^{n_{k_1}} \text{sgn}(v_m^{k_1}) \frac{1 - \text{sgn}(\delta_m^{k_1})}{2} + \sum_{m=1}^{n_{k_2}} \text{sgn}(v_m^{k_2}) \frac{1 - \text{sgn}(\delta_m^{k_2})}{2}
\end{aligned} \tag{S17.3}$$

$$\begin{aligned}
\mathcal{W}_4^{\text{gapless}} = & \sum_{m=1}^{n_{d_1}} \text{sgn}(v_m^{d_1}) \frac{1 - \text{sgn}(\delta_m^{d_1})}{2} + \sum_{m=1}^{n_{d_2}} \text{sgn}(v_m^{d_2}) \frac{1 - \text{sgn}(\delta_m^{d_2})}{2} - 2 \sum_{m=1}^{n_{h_1}} \text{sgn}(v_m^{h_1}) \frac{1 - \text{sgn}(\delta_m^{h_1})}{2} \\
& - \sum_{m=1}^{n_{k_1}} \text{sgn}(v_m^{k_1}) \frac{1 - \text{sgn}(\delta_m^{k_1})}{2} - \sum_{m=1}^{n_{k_2}} \text{sgn}(v_m^{k_2}) \frac{1 - \text{sgn}(\delta_m^{k_2})}{2} + \sum_{m=1}^{n_{l_1}} \text{sgn}(v_m^{l_1}) \frac{1 - \text{sgn}(\delta_m^{l_1})}{2} \\
& + \sum_{m=1}^{n_{l_2}} \text{sgn}(v_m^{l_2}) \frac{1 - \text{sgn}(\delta_m^{l_2})}{2}
\end{aligned} \tag{S17.4}$$

$$\mathcal{W}_5^{\text{gapless}} = \sum_{m=1}^{n_{e_1}} \text{sgn}(v_m^{e_1}) \frac{1 - \text{sgn}(\delta_m^{e_1})}{2} - \sum_{m=1}^{n_{f_1}} \text{sgn}(v_m^{f_1}) \frac{1 - \text{sgn}(\delta_m^{f_1})}{2} + \sum_{m=1}^{n_{g_1}} \text{sgn}(v_m^{g_1}) \frac{1 - \text{sgn}(\delta_m^{g_1})}{2} + \sum_{m=1}^{n_{h_1}} \text{sgn}(v_m^{h_1}) \frac{1 - \text{sgn}(\delta_m^{h_1})}{2} \tag{S17.5}$$

$$\mathcal{W}_1^{\text{gapped}} = \sum_{m=1}^{n_{a_2}} \text{sgn}(v_m^{a_2}) \frac{1 - \text{sgn}(\delta_m^{a_2})}{2} - \sum_{m=1}^{n_{b_2}} \text{sgn}(v_m^{b_2}) \frac{1 - \text{sgn}(\delta_m^{b_2})}{2} + \sum_{m=1}^{n_{c_2}} \text{sgn}(v_m^{c_2}) \frac{1 - \text{sgn}(\delta_m^{c_2})}{2} + \sum_{m=1}^{n_{d_2}} \text{sgn}(v_m^{d_2}) \frac{1 - \text{sgn}(\delta_m^{d_2})}{2} \tag{S17.6}$$

$$\begin{aligned}
\mathcal{W}_2^{\text{gapped}} = & 2 \sum_{m=1}^{n_{c_2}} \text{sgn}(v_m^{c_2}) \frac{1 - \text{sgn}(\delta_m^{c_2})}{2} - 2 \sum_{m=1}^{n_{g_1}} \text{sgn}(v_m^{g_1}) \frac{1 - \text{sgn}(\delta_m^{g_1})}{2} - \sum_{m=1}^{n_{j_1}} \text{sgn}(v_m^{j_1}) \frac{1 - \text{sgn}(\delta_m^{j_1})}{2} \\
& - \sum_{m=1}^{n_{j_2}} \text{sgn}(v_m^{j_2}) \frac{1 - \text{sgn}(\delta_m^{j_2})}{2} + \sum_{m=1}^{n_{k_1}} \text{sgn}(v_m^{k_1}) \frac{1 - \text{sgn}(\delta_m^{k_1})}{2} + \sum_{m=1}^{n_{k_2}} \text{sgn}(v_m^{k_2}) \frac{1 - \text{sgn}(\delta_m^{k_2})}{2}
\end{aligned} \tag{S17.7}$$

$$\begin{aligned}
\mathcal{W}_3^{\text{gapped}} = & -2 \sum_{m=1}^{n_{b_2}} \text{sgn}(v_m^{b_2}) \frac{1 - \text{sgn}(\delta_m^{b_2})}{2} + 2 \sum_{m=1}^{n_{c_2}} \text{sgn}(v_m^{c_2}) \frac{1 - \text{sgn}(\delta_m^{c_2})}{2} + 2 \sum_{m=1}^{n_{d_2}} \text{sgn}(v_m^{d_2}) \frac{1 - \text{sgn}(\delta_m^{d_2})}{2} \\
& + 2 \sum_{m=1}^{n_{f_1}} \text{sgn}(v_m^{f_1}) \frac{1 - \text{sgn}(\delta_m^{f_1})}{2} - 2 \sum_{m=1}^{n_{g_1}} \text{sgn}(v_m^{g_1}) \frac{1 - \text{sgn}(\delta_m^{g_1})}{2} - 2 \sum_{m=1}^{n_{h_1}} \text{sgn}(v_m^{h_1}) \frac{1 - \text{sgn}(\delta_m^{h_1})}{2} \\
& + \sum_{m=1}^{n_{i_1}} \text{sgn}(v_m^{i_1}) \frac{1 - \text{sgn}(\delta_m^{i_1})}{2} + \sum_{m=1}^{n_{i_2}} \text{sgn}(v_m^{i_2}) \frac{1 - \text{sgn}(\delta_m^{i_2})}{2} - \sum_{m=1}^{n_{j_1}} \text{sgn}(v_m^{j_1}) \frac{1 - \text{sgn}(\delta_m^{j_1})}{2} - \sum_{m=1}^{n_{j_2}} \text{sgn}(v_m^{j_2}) \frac{1 - \text{sgn}(\delta_m^{j_2})}{2}
\end{aligned} \tag{S17.8}$$

$$\begin{aligned}
\mathcal{W}_4^{\text{gapped}} = & 2 \sum_{m=1}^{n_{c_2}} \text{sgn}(v_m^{c_2}) \frac{1 - \text{sgn}(\delta_m^{c_2})}{2} + 2 \sum_{m=1}^{n_{d_2}} \text{sgn}(v_m^{d_2}) \frac{1 - \text{sgn}(\delta_m^{d_2})}{2} - 2 \sum_{m=1}^{n_{g_1}} \text{sgn}(v_m^{g_1}) \frac{1 - \text{sgn}(\delta_m^{g_1})}{2} \\
& - 2 \sum_{m=1}^{n_{h_1}} \text{sgn}(v_m^{h_1}) \frac{1 - \text{sgn}(\delta_m^{h_1})}{2} - \sum_{m=1}^{n_{j_1}} \text{sgn}(v_m^{j_1}) \frac{1 - \text{sgn}(\delta_m^{j_1})}{2} \\
& - \sum_{m=1}^{n_{j_2}} \text{sgn}(v_m^{j_2}) \frac{1 - \text{sgn}(\delta_m^{j_2})}{2} + \sum_{m=1}^{n_{l_1}} \text{sgn}(v_m^{l_1}) \frac{1 - \text{sgn}(\delta_m^{l_1})}{2} + \sum_{m=1}^{n_{l_2}} \text{sgn}(v_m^{l_2}) \frac{1 - \text{sgn}(\delta_m^{l_2})}{2}
\end{aligned} \tag{S17.9}$$

$$\mathcal{X}_1 = \sum_{m=1}^{n_{b_2}} \frac{1 - \text{sgn}(\delta_m^{b_2})}{2} + \sum_{m=1}^{n_{c_2}} \frac{1 - \text{sgn}(\delta_m^{c_2})}{2} + \sum_{m=1}^{n_{d_2}} \frac{1 - \text{sgn}(\delta_m^{d_2})}{2} + \sum_{m=1}^{n_{i_2}} \frac{1 - \text{sgn}(\delta_m^{i_2})}{2} + \sum_{m=1}^{n_{j_2}} \frac{1 - \text{sgn}(\delta_m^{j_2})}{2} \pmod{2} \tag{S17.10}$$

$$\mathcal{X}_2 = \sum_{m=1}^{n_{b_2}} \frac{1 - \text{sgn}(\delta_m^{b_2})}{2} + \sum_{m=1}^{n_{i_2}} \frac{1 - \text{sgn}(\delta_m^{i_2})}{2} + \sum_{m=1}^{n_{j_1}} \frac{1 - \text{sgn}(\delta_m^{j_1})}{2} + \sum_{m=1}^{n_{j_2}} \frac{1 - \text{sgn}(\delta_m^{j_2})}{2} + \sum_{m=1}^{n_{l_1}} \frac{1 - \text{sgn}(\delta_m^{l_1})}{2} \pmod{2} \tag{S17.11}$$

$$\begin{aligned}
\mathcal{X}_3 = & \sum_{m=1}^{n_{b_2}} \frac{1 - \text{sgn}(\delta_m^{b_2})}{2} + \sum_{m=1}^{n_{d_2}} \frac{1 - \text{sgn}(\delta_m^{d_2})}{2} + \sum_{m=1}^{n_{i_2}} \frac{1 - \text{sgn}(\delta_m^{i_2})}{2} + \sum_{m=1}^{n_{j_1}} \frac{1 - \text{sgn}(\delta_m^{j_1})}{2} \\
& + \sum_{m=1}^{n_{j_2}} \frac{1 - \text{sgn}(\delta_m^{j_2})}{2} + \sum_{m=1}^{n_{k_1}} \frac{1 - \text{sgn}(\delta_m^{k_1})}{2} \pmod{2}
\end{aligned} \tag{S17.12}$$

$$\mathcal{X}_4 = \sum_{m=1}^{n_{b_2}} \frac{1 - \text{sgn}(\delta_m^{b_2})}{2} + \sum_{m=1}^{n_{i_2}} \frac{1 - \text{sgn}(\delta_m^{i_2})}{2} + \sum_{m=1}^{n_{l_1}} \frac{1 - \text{sgn}(\delta_m^{l_1})}{2} \pmod{2} \tag{S17.13}$$

### S18. SPACE GROUP NO. 18

| line segment                              | character of irrep (generators only)                                                                                         |
|-------------------------------------------|------------------------------------------------------------------------------------------------------------------------------|
| $a \quad (\frac{t}{2}, 0, 0)$             | $\{2_{100}   \frac{1}{2} \frac{1}{2} 0\}$<br>$a_1 \quad -ie^{-\frac{1}{2}i\pi t}$<br>$a_2 \quad ie^{-\frac{1}{2}i\pi t}$     |
| $b \quad (0, \frac{t}{2}, 0)$             | $\{2_{010}   \frac{1}{2} \frac{1}{2} 0\}$<br>$b_1 \quad -ie^{-\frac{1}{2}i\pi t}$<br>$b_2 \quad ie^{-\frac{1}{2}i\pi t}$     |
| $c \quad (\frac{1}{2}, \frac{t}{2}, 0)$   | $\{2_{010}   \frac{1}{2} \frac{1}{2} 0\}$<br>$c_1 \quad -e^{-\frac{1}{2}i\pi(t+1)}$<br>$c_2 \quad e^{-\frac{1}{2}i\pi(t+1)}$ |
| $d \quad (\frac{1-t}{2}, \frac{1}{2}, 0)$ | $\{2_{100}   \frac{1}{2} \frac{1}{2} 0\}$<br>$d_1 \quad -e^{-\frac{1}{2}i\pi(2-t)}$<br>$d_2 \quad e^{-\frac{1}{2}i\pi(2-t)}$ |
| $e \quad (\frac{t}{2}, 0, \frac{1}{2})$   | $\{2_{100}   \frac{1}{2} \frac{1}{2} 0\}$<br>$e_1 \quad -ie^{-\frac{1}{2}i\pi t}$<br>$e_2 \quad ie^{-\frac{1}{2}i\pi t}$     |
| $f \quad (0, \frac{t}{2}, \frac{1}{2})$   | $\{2_{010}   \frac{1}{2} \frac{1}{2} 0\}$<br>$f_1 \quad -ie^{-\frac{1}{2}i\pi t}$<br>$f_2 \quad ie^{-\frac{1}{2}i\pi t}$     |

|                                                     |                                                                                                                                              |
|-----------------------------------------------------|----------------------------------------------------------------------------------------------------------------------------------------------|
| $g \quad (\frac{1}{2}, \frac{t}{2}, \frac{1}{2})$   | $\begin{matrix} \{2_{010}   \frac{1}{2} \frac{1}{2} 0\} \\ g_1 & -e^{-\frac{1}{2}i\pi(t+1)} \\ g_2 & e^{-\frac{1}{2}i\pi(t+1)} \end{matrix}$ |
| $h \quad (\frac{1-t}{2}, \frac{1}{2}, \frac{1}{2})$ | $\begin{matrix} \{2_{100}   \frac{1}{2} \frac{1}{2} 0\} \\ h_1 & -e^{-\frac{1}{2}i\pi(2-t)} \\ h_2 & e^{-\frac{1}{2}i\pi(2-t)} \end{matrix}$ |
| $i \quad (0, 0, \frac{t}{2})$                       | $\begin{matrix} \{2_{001}   0 \ 0 \ 0\} \\ i_1 & -i \\ i_2 & i \end{matrix}$                                                                 |
| $j \quad (\frac{1}{2}, 0, \frac{t}{2})$             | $\begin{matrix} \{2_{001}   0 \ 0 \ 0\} \\ j_1 & -i \\ j_2 & i \end{matrix}$                                                                 |
| $k \quad (\frac{1}{2}, \frac{1}{2}, \frac{t}{2})$   | $\begin{matrix} \{2_{001}   0 \ 0 \ 0\} \\ k_1 & -i \\ k_2 & i \end{matrix}$                                                                 |
| $l \quad (0, \frac{1}{2}, \frac{t}{2})$             | $\begin{matrix} \{2_{001}   0 \ 0 \ 0\} \\ l_1 & -i \\ l_2 & i \end{matrix}$                                                                 |

$$\begin{aligned}
\mathcal{W}_1^{\text{gapless}} = & \sum_{m=1}^{n_{a_1}} \text{sgn}(v_m^{a_1}) \frac{1 - \text{sgn}(\delta_m^{a_1})}{2} + \sum_{m=1}^{n_{a_2}} \text{sgn}(v_m^{a_2}) \frac{1 - \text{sgn}(\delta_m^{a_2})}{2} - \sum_{m=1}^{n_{f_1}} \text{sgn}(v_m^{f_1}) \frac{1 - \text{sgn}(\delta_m^{f_1})}{2} \\
& - \sum_{m=1}^{n_{f_2}} \text{sgn}(v_m^{f_2}) \frac{1 - \text{sgn}(\delta_m^{f_2})}{2} + 2 \sum_{m=1}^{n_{g_1}} \text{sgn}(v_m^{g_1}) \frac{1 - \text{sgn}(\delta_m^{g_1})}{2} + 2 \sum_{m=1}^{n_{h_1}} \text{sgn}(v_m^{h_1}) \frac{1 - \text{sgn}(\delta_m^{h_1})}{2} \\
& - \sum_{m=1}^{n_{i_1}} \text{sgn}(v_m^{i_1}) \frac{1 - \text{sgn}(\delta_m^{i_1})}{2} - \sum_{m=1}^{n_{i_2}} \text{sgn}(v_m^{i_2}) \frac{1 - \text{sgn}(\delta_m^{i_2})}{2} + 2 \sum_{m=1}^{n_{j_1}} \text{sgn}(v_m^{j_1}) \frac{1 - \text{sgn}(\delta_m^{j_1})}{2}
\end{aligned} \tag{S18.1}$$

$$\begin{aligned}
\mathcal{W}_2^{\text{gapless}} = & \sum_{m=1}^{n_{b_1}} \text{sgn}(v_m^{b_1}) \frac{1 - \text{sgn}(\delta_m^{b_1})}{2} + \sum_{m=1}^{n_{b_2}} \text{sgn}(v_m^{b_2}) \frac{1 - \text{sgn}(\delta_m^{b_2})}{2} - \sum_{m=1}^{n_{f_1}} \text{sgn}(v_m^{f_1}) \frac{1 - \text{sgn}(\delta_m^{f_1})}{2} - \sum_{m=1}^{n_{f_2}} \text{sgn}(v_m^{f_2}) \frac{1 - \text{sgn}(\delta_m^{f_2})}{2} \\
& - \sum_{m=1}^{n_{i_1}} \text{sgn}(v_m^{i_1}) \frac{1 - \text{sgn}(\delta_m^{i_1})}{2} - \sum_{m=1}^{n_{i_2}} \text{sgn}(v_m^{i_2}) \frac{1 - \text{sgn}(\delta_m^{i_2})}{2} + 2 \sum_{m=1}^{n_{l_1}} \text{sgn}(v_m^{l_1}) \frac{1 - \text{sgn}(\delta_m^{l_1})}{2}
\end{aligned} \tag{S18.2}$$

$$\begin{aligned}
\mathcal{W}_3^{\text{gapless}} = & \sum_{m=1}^{n_{c_1}} \text{sgn}(v_m^{c_1}) \frac{1 - \text{sgn}(\delta_m^{c_1})}{2} - \sum_{m=1}^{n_{g_1}} \text{sgn}(v_m^{g_1}) \frac{1 - \text{sgn}(\delta_m^{g_1})}{2} - \sum_{m=1}^{n_{j_1}} \text{sgn}(v_m^{j_1}) \frac{1 - \text{sgn}(\delta_m^{j_1})}{2} \\
& + \sum_{m=1}^{n_{k_1}} \text{sgn}(v_m^{k_1}) \frac{1 - \text{sgn}(\delta_m^{k_1})}{2} + \sum_{m=1}^{n_{k_2}} \text{sgn}(v_m^{k_2}) \frac{1 - \text{sgn}(\delta_m^{k_2})}{2}
\end{aligned} \tag{S18.3}$$

$$\begin{aligned}
\mathcal{W}_4^{\text{gapless}} = & \sum_{m=1}^{n_{d_1}} \text{sgn}(v_m^{d_1}) \frac{1 - \text{sgn}(\delta_m^{d_1})}{2} - \sum_{m=1}^{n_{h_1}} \text{sgn}(v_m^{h_1}) \frac{1 - \text{sgn}(\delta_m^{h_1})}{2} - \sum_{m=1}^{n_{k_1}} \text{sgn}(v_m^{k_1}) \frac{1 - \text{sgn}(\delta_m^{k_1})}{2} \\
& - \sum_{m=1}^{n_{k_2}} \text{sgn}(v_m^{k_2}) \frac{1 - \text{sgn}(\delta_m^{k_2})}{2} + \sum_{m=1}^{n_{l_1}} \text{sgn}(v_m^{l_1}) \frac{1 - \text{sgn}(\delta_m^{l_1})}{2}
\end{aligned} \tag{S18.4}$$

$$\begin{aligned} \mathcal{W}_5^{\text{gapless}} = & \sum_{m=1}^{n_{e_1}} \text{sgn}(v_m^{e_1}) \frac{1 - \text{sgn}(\delta_m^{e_1})}{2} + \sum_{m=1}^{n_{e_2}} \text{sgn}(v_m^{e_2}) \frac{1 - \text{sgn}(\delta_m^{e_2})}{2} - \sum_{m=1}^{n_{f_1}} \text{sgn}(v_m^{f_1}) \frac{1 - \text{sgn}(\delta_m^{f_1})}{2} \\ & - \sum_{m=1}^{n_{f_2}} \text{sgn}(v_m^{f_2}) \frac{1 - \text{sgn}(\delta_m^{f_2})}{2} + 2 \sum_{m=1}^{n_{g_1}} \text{sgn}(v_m^{g_1}) \frac{1 - \text{sgn}(\delta_m^{g_1})}{2} + 2 \sum_{m=1}^{n_{h_1}} \text{sgn}(v_m^{h_1}) \frac{1 - \text{sgn}(\delta_m^{h_1})}{2} \end{aligned} \quad (\text{S18.5})$$

$$\mathcal{W}_1^{\text{gapped}} = - \sum_{m=1}^{n_{k_1}} \text{sgn}(v_m^{k_1}) \frac{1 - \text{sgn}(\delta_m^{k_1})}{2} + \sum_{m=1}^{n_{k_2}} \text{sgn}(v_m^{k_2}) \frac{1 - \text{sgn}(\delta_m^{k_2})}{2} \quad (\text{S18.6})$$

$$\mathcal{W}_2^{\text{gapped}} = - \sum_{m=1}^{n_{i_1}} \text{sgn}(v_m^{i_1}) \frac{1 - \text{sgn}(\delta_m^{i_1})}{2} + \sum_{m=1}^{n_{i_2}} \text{sgn}(v_m^{i_2}) \frac{1 - \text{sgn}(\delta_m^{i_2})}{2} \quad (\text{S18.7})$$

$$\mathcal{X}_1 = \sum_{m=1}^{n_{a_2}} \frac{1 - \text{sgn}(\delta_m^{a_2})}{2} + \sum_{m=1}^{n_{b_2}} \frac{1 - \text{sgn}(\delta_m^{b_2})}{2} \quad \text{mod } 2 \quad (\text{S18.8})$$

$$\mathcal{X}_2 = \sum_{m=1}^{n_{b_2}} \frac{1 - \text{sgn}(\delta_m^{b_2})}{2} + \sum_{m=1}^{n_{e_2}} \frac{1 - \text{sgn}(\delta_m^{e_2})}{2} + \sum_{m=1}^{n_{i_1}} \frac{1 - \text{sgn}(\delta_m^{i_1})}{2} \quad \text{mod } 2 \quad (\text{S18.9})$$

$$\mathcal{X}_3 = \sum_{m=1}^{n_{b_2}} \frac{1 - \text{sgn}(\delta_m^{b_2})}{2} + \sum_{m=1}^{n_{f_2}} \frac{1 - \text{sgn}(\delta_m^{f_2})}{2} + \sum_{m=1}^{n_{i_1}} \frac{1 - \text{sgn}(\delta_m^{i_1})}{2} \quad \text{mod } 2 \quad (\text{S18.10})$$

$$\begin{aligned} \mathcal{X}_4 = & 2 \sum_{m=1}^{n_{b_2}} \text{sgn}(v_m^{b_2}) \frac{1 - \text{sgn}(\delta_m^{b_2})}{2} + \sum_{m=1}^{n_{f_1}} \text{sgn}(v_m^{f_1}) \frac{1 - \text{sgn}(\delta_m^{f_1})}{2} - 3 \sum_{m=1}^{n_{f_2}} \text{sgn}(v_m^{f_2}) \frac{1 - \text{sgn}(\delta_m^{f_2})}{2} \\ & - 2 \sum_{m=1}^{n_{h_1}} \text{sgn}(v_m^{h_1}) \frac{1 - \text{sgn}(\delta_m^{h_1})}{2} - 2 \sum_{m=1}^{n_{i_1}} \text{sgn}(v_m^{i_1}) \frac{1 - \text{sgn}(\delta_m^{i_1})}{2} \quad \text{mod } 4 \end{aligned} \quad (\text{S18.11})$$

### S19. SPACE GROUP NO. 19

| line segment                            | character of irrep (generators only)      |
|-----------------------------------------|-------------------------------------------|
| $a \quad (\frac{t}{2}, 0, 0)$           | $\{2_{100}   \frac{1}{2} \frac{1}{2} 0\}$ |
|                                         | $a_1 \quad -ie^{-\frac{1}{2}i\pi t}$      |
|                                         | $a_2 \quad ie^{-\frac{1}{2}i\pi t}$       |
| $b \quad (0, \frac{t}{2}, 0)$           | $\{2_{010}   0 \frac{1}{2} \frac{1}{2}\}$ |
|                                         | $b_1 \quad -ie^{-\frac{1}{2}i\pi t}$      |
|                                         | $b_2 \quad ie^{-\frac{1}{2}i\pi t}$       |
| $c \quad (\frac{1}{2}, \frac{t}{2}, 0)$ | $\{2_{010}   0 \frac{1}{2} \frac{1}{2}\}$ |
|                                         | $c_1 \quad -ie^{-\frac{1}{2}i\pi t}$      |
|                                         | $c_2 \quad ie^{-\frac{1}{2}i\pi t}$       |



|                                                     |                                                                                                                                                      |
|-----------------------------------------------------|------------------------------------------------------------------------------------------------------------------------------------------------------|
| $d \quad (\frac{1-t}{2}, \frac{1}{2}, 0)$           | $d_1 \quad \begin{cases} \{2_{100}   \frac{1}{2} \frac{1}{2} 0\} \\ -e^{-\frac{1}{2}i\pi(2-t)} \end{cases}$<br>$d_2 \quad e^{-\frac{1}{2}i\pi(2-t)}$ |
| $e \quad (\frac{t}{2}, 0, \frac{1}{2})$             | $e_1 \quad \begin{cases} \{2_{100}   \frac{1}{2} \frac{1}{2} 0\} \\ -ie^{-\frac{1}{2}i\pi t} \end{cases}$<br>$e_2 \quad ie^{-\frac{1}{2}i\pi t}$     |
| $f \quad (0, \frac{t}{2}, \frac{1}{2})$             | $f_1 \quad \begin{cases} \{2_{010}   0 \frac{1}{2} \frac{1}{2}\} \\ -e^{-\frac{1}{2}i\pi(t+1)} \end{cases}$<br>$f_2 \quad e^{-\frac{1}{2}i\pi(t+1)}$ |
| $g \quad (\frac{1}{2}, \frac{t}{2}, \frac{1}{2})$   | $g_1 \quad \begin{cases} \{2_{010}   0 \frac{1}{2} \frac{1}{2}\} \\ -e^{-\frac{1}{2}i\pi(t+1)} \end{cases}$<br>$g_2 \quad e^{-\frac{1}{2}i\pi(t+1)}$ |
| $h \quad (\frac{1-t}{2}, \frac{1}{2}, \frac{1}{2})$ | $h_1 \quad \begin{cases} \{2_{100}   \frac{1}{2} \frac{1}{2} 0\} \\ -e^{-\frac{1}{2}i\pi(2-t)} \end{cases}$<br>$h_2 \quad e^{-\frac{1}{2}i\pi(2-t)}$ |
| $i \quad (0, 0, \frac{t}{2})$                       | $i_1 \quad \begin{cases} \{2_{001}   \frac{1}{2} 0 \frac{1}{2}\} \\ -ie^{-\frac{1}{2}i\pi t} \end{cases}$<br>$i_2 \quad ie^{-\frac{1}{2}i\pi t}$     |
| $j \quad (\frac{1}{2}, 0, \frac{t}{2})$             | $j_1 \quad \begin{cases} \{2_{001}   \frac{1}{2} 0 \frac{1}{2}\} \\ -e^{-\frac{1}{2}i\pi(t+1)} \end{cases}$<br>$j_2 \quad e^{-\frac{1}{2}i\pi(t+1)}$ |
| $k \quad (\frac{1}{2}, \frac{1}{2}, \frac{t}{2})$   | $k_1 \quad \begin{cases} \{2_{001}   \frac{1}{2} 0 \frac{1}{2}\} \\ -e^{-\frac{1}{2}i\pi(t+1)} \end{cases}$<br>$k_2 \quad e^{-\frac{1}{2}i\pi(t+1)}$ |
| $l \quad (0, \frac{1}{2}, \frac{t}{2})$             | $l_1 \quad \begin{cases} \{2_{001}   \frac{1}{2} 0 \frac{1}{2}\} \\ -ie^{-\frac{1}{2}i\pi t} \end{cases}$<br>$l_2 \quad ie^{-\frac{1}{2}i\pi t}$     |

$$\begin{aligned}
\mathcal{W}_1^{\text{gapless}} = & \sum_{m=1}^{n_{a_1}} \text{sgn}(v_m^{a_1}) \frac{1 - \text{sgn}(\delta_m^{a_1})}{2} + \sum_{m=1}^{n_{a_2}} \text{sgn}(v_m^{a_2}) \frac{1 - \text{sgn}(\delta_m^{a_2})}{2} - 2 \sum_{m=1}^{n_{f_1}} \text{sgn}(v_m^{f_1}) \frac{1 - \text{sgn}(\delta_m^{f_1})}{2} \\
& + 2 \sum_{m=1}^{n_{g_1}} \text{sgn}(v_m^{g_1}) \frac{1 - \text{sgn}(\delta_m^{g_1})}{2} + 2 \sum_{m=1}^{n_{g_2}} \text{sgn}(v_m^{g_2}) \frac{1 - \text{sgn}(\delta_m^{g_2})}{2} + 2 \sum_{m=1}^{n_{h_1}} \text{sgn}(v_m^{h_1}) \frac{1 - \text{sgn}(\delta_m^{h_1})}{2} \\
& + 2 \sum_{m=1}^{n_{h_2}} \text{sgn}(v_m^{h_2}) \frac{1 - \text{sgn}(\delta_m^{h_2})}{2} - \sum_{m=1}^{n_{i_1}} \text{sgn}(v_m^{i_1}) \frac{1 - \text{sgn}(\delta_m^{i_1})}{2} - \sum_{m=1}^{n_{i_2}} \text{sgn}(v_m^{i_2}) \frac{1 - \text{sgn}(\delta_m^{i_2})}{2} \\
& + 2 \sum_{m=1}^{n_{j_1}} \text{sgn}(v_m^{j_1}) \frac{1 - \text{sgn}(\delta_m^{j_1})}{2}
\end{aligned} \tag{S19.1}$$

$$\begin{aligned}
\mathcal{W}_2^{\text{gapless}} = & \sum_{m=1}^{n_{b_1}} \text{sgn}(v_m^{b_1}) \frac{1 - \text{sgn}(\delta_m^{b_1})}{2} + \sum_{m=1}^{n_{b_2}} \text{sgn}(v_m^{b_2}) \frac{1 - \text{sgn}(\delta_m^{b_2})}{2} - 2 \sum_{m=1}^{n_{f_1}} \text{sgn}(v_m^{f_1}) \frac{1 - \text{sgn}(\delta_m^{f_1})}{2} \\
& - \sum_{m=1}^{n_{i_1}} \text{sgn}(v_m^{i_1}) \frac{1 - \text{sgn}(\delta_m^{i_1})}{2} - \sum_{m=1}^{n_{i_2}} \text{sgn}(v_m^{i_2}) \frac{1 - \text{sgn}(\delta_m^{i_2})}{2} + 2 \sum_{m=1}^{n_{l_1}} \text{sgn}(v_m^{l_1}) \frac{1 - \text{sgn}(\delta_m^{l_1})}{2}
\end{aligned} \tag{S19.2}$$

$$\begin{aligned}
\mathcal{W}_3^{\text{gapless}} = & \sum_{m=1}^{n_{c_1}} \text{sgn}(v_m^{c_1}) \frac{1 - \text{sgn}(\delta_m^{c_1})}{2} - \sum_{m=1}^{n_{g_1}} \text{sgn}(v_m^{g_1}) \frac{1 - \text{sgn}(\delta_m^{g_1})}{2} - \sum_{m=1}^{n_{g_2}} \text{sgn}(v_m^{g_2}) \frac{1 - \text{sgn}(\delta_m^{g_2})}{2} \\
& - \sum_{m=1}^{n_{j_1}} \text{sgn}(v_m^{j_1}) \frac{1 - \text{sgn}(\delta_m^{j_1})}{2} + \sum_{m=1}^{n_{k_1}} \text{sgn}(v_m^{k_1}) \frac{1 - \text{sgn}(\delta_m^{k_1})}{2} + \sum_{m=1}^{n_{k_2}} \text{sgn}(v_m^{k_2}) \frac{1 - \text{sgn}(\delta_m^{k_2})}{2}
\end{aligned} \tag{S19.3}$$

$$\begin{aligned} \mathcal{W}_4^{\text{gapless}} = & \sum_{m=1}^{n_{d_1}} \text{sgn}(v_m^{d_1}) \frac{1 - \text{sgn}(\delta_m^{d_1})}{2} - \sum_{m=1}^{n_{h_1}} \text{sgn}(v_m^{h_1}) \frac{1 - \text{sgn}(\delta_m^{h_1})}{2} - \sum_{m=1}^{n_{h_2}} \text{sgn}(v_m^{h_2}) \frac{1 - \text{sgn}(\delta_m^{h_2})}{2} \\ & - \sum_{m=1}^{n_{k_1}} \text{sgn}(v_m^{k_1}) \frac{1 - \text{sgn}(\delta_m^{k_1})}{2} - \sum_{m=1}^{n_{k_2}} \text{sgn}(v_m^{k_2}) \frac{1 - \text{sgn}(\delta_m^{k_2})}{2} + \sum_{m=1}^{n_{l_1}} \text{sgn}(v_m^{l_1}) \frac{1 - \text{sgn}(\delta_m^{l_1})}{2} \end{aligned} \quad (\text{S19.4})$$

$$\begin{aligned} \mathcal{W}_5^{\text{gapless}} = & \sum_{m=1}^{n_{e_1}} \text{sgn}(v_m^{e_1}) \frac{1 - \text{sgn}(\delta_m^{e_1})}{2} - \sum_{m=1}^{n_{f_1}} \text{sgn}(v_m^{f_1}) \frac{1 - \text{sgn}(\delta_m^{f_1})}{2} + \sum_{m=1}^{n_{g_1}} \text{sgn}(v_m^{g_1}) \frac{1 - \text{sgn}(\delta_m^{g_1})}{2} \\ & + \sum_{m=1}^{n_{g_2}} \text{sgn}(v_m^{g_2}) \frac{1 - \text{sgn}(\delta_m^{g_2})}{2} + \sum_{m=1}^{n_{h_1}} \text{sgn}(v_m^{h_1}) \frac{1 - \text{sgn}(\delta_m^{h_1})}{2} + \sum_{m=1}^{n_{h_2}} \text{sgn}(v_m^{h_2}) \frac{1 - \text{sgn}(\delta_m^{h_2})}{2} \end{aligned} \quad (\text{S19.5})$$

$$\begin{aligned} \mathcal{X}_1 = & \sum_{m=1}^{n_{b_2}} \frac{1 - \text{sgn}(\delta_m^{b_2})}{2} + \sum_{m=1}^{n_{g_1}} \frac{1 - \text{sgn}(\delta_m^{g_1})}{2} + \sum_{m=1}^{n_{g_2}} \frac{1 - \text{sgn}(\delta_m^{g_2})}{2} + \sum_{m=1}^{n_{i_2}} \frac{1 - \text{sgn}(\delta_m^{i_2})}{2} \\ & + \sum_{m=1}^{n_{k_1}} \frac{1 - \text{sgn}(\delta_m^{k_1})}{2} + \sum_{m=1}^{n_{k_2}} \frac{1 - \text{sgn}(\delta_m^{k_2})}{2} \pmod{2} \end{aligned} \quad (\text{S19.6})$$

$$\begin{aligned} \mathcal{X}_2 = & \sum_{m=1}^{n_{a_2}} \frac{1 - \text{sgn}(\delta_m^{a_2})}{2} + \sum_{m=1}^{n_{g_1}} \frac{1 - \text{sgn}(\delta_m^{g_1})}{2} + \sum_{m=1}^{n_{g_2}} \frac{1 - \text{sgn}(\delta_m^{g_2})}{2} + \sum_{m=1}^{n_{i_2}} \frac{1 - \text{sgn}(\delta_m^{i_2})}{2} \\ & + \sum_{m=1}^{n_{k_1}} \frac{1 - \text{sgn}(\delta_m^{k_1})}{2} + \sum_{m=1}^{n_{k_2}} \frac{1 - \text{sgn}(\delta_m^{k_2})}{2} \pmod{2} \end{aligned} \quad (\text{S19.7})$$

$$\begin{aligned} \mathcal{X}_3 = & \sum_{m=1}^{n_{h_1}} \frac{1 - \text{sgn}(\delta_m^{h_1})}{2} + \sum_{m=1}^{n_{h_2}} \frac{1 - \text{sgn}(\delta_m^{h_2})}{2} + \sum_{m=1}^{n_{i_1}} \frac{1 - \text{sgn}(\delta_m^{i_1})}{2} + \sum_{m=1}^{n_{i_2}} \frac{1 - \text{sgn}(\delta_m^{i_2})}{2} \\ & + \sum_{m=1}^{n_{k_1}} \frac{1 - \text{sgn}(\delta_m^{k_1})}{2} + \sum_{m=1}^{n_{k_2}} \frac{1 - \text{sgn}(\delta_m^{k_2})}{2} \pmod{2} \end{aligned} \quad (\text{S19.8})$$

$$\begin{aligned} \mathcal{X}_4 = & \sum_{m=1}^{n_{g_1}} \frac{1 - \text{sgn}(\delta_m^{g_1})}{2} + \sum_{m=1}^{n_{g_2}} \frac{1 - \text{sgn}(\delta_m^{g_2})}{2} + \sum_{m=1}^{n_{i_1}} \frac{1 - \text{sgn}(\delta_m^{i_1})}{2} + \sum_{m=1}^{n_{i_2}} \frac{1 - \text{sgn}(\delta_m^{i_2})}{2} \\ & + \sum_{m=1}^{n_{k_1}} \frac{1 - \text{sgn}(\delta_m^{k_1})}{2} + \sum_{m=1}^{n_{k_2}} \frac{1 - \text{sgn}(\delta_m^{k_2})}{2} \pmod{2} \end{aligned} \quad (\text{S19.9})$$

$$\begin{aligned} \mathcal{X}_5 = & -2 \sum_{m=1}^{n_{f_1}} \text{sgn}(v_m^{f_1}) \frac{1 - \text{sgn}(\delta_m^{f_1})}{2} + 2 \sum_{m=1}^{n_{g_1}} \text{sgn}(v_m^{g_1}) \frac{1 - \text{sgn}(\delta_m^{g_1})}{2} - 2 \sum_{m=1}^{n_{g_2}} \text{sgn}(v_m^{g_2}) \frac{1 - \text{sgn}(\delta_m^{g_2})}{2} - \sum_{m=1}^{n_{i_1}} \text{sgn}(v_m^{i_1}) \frac{1 - \text{sgn}(\delta_m^{i_1})}{2} \\ & + \sum_{m=1}^{n_{i_2}} \text{sgn}(v_m^{i_2}) \frac{1 - \text{sgn}(\delta_m^{i_2})}{2} + 2 \sum_{m=1}^{n_{k_1}} \text{sgn}(v_m^{k_1}) \frac{1 - \text{sgn}(\delta_m^{k_1})}{2} - 2 \sum_{m=1}^{n_{k_2}} \text{sgn}(v_m^{k_2}) \frac{1 - \text{sgn}(\delta_m^{k_2})}{2} \pmod{4} \end{aligned} \quad (\text{S19.10})$$

## S20. SPACE GROUP NO. 20

| line segment                                      | character of irrep (generators only)                                                                                               |
|---------------------------------------------------|------------------------------------------------------------------------------------------------------------------------------------|
| $a \ (t, 0, 0)$                                   | $\begin{matrix} \{2_{100}   0 & 0 & 0\} \\ a_1 & -i \\ a_2 & i \end{matrix}$                                                       |
| $b \ (0, t, 0)$                                   | $\begin{matrix} \{2_{010}   0 & 0 & \frac{1}{2}\} \\ b_1 & -i \\ b_2 & i \end{matrix}$                                             |
| $c \ (\frac{t}{2}, 1 - \frac{t}{2}, 0)$           | $\begin{matrix} \{1   0 & 0 & 0\} \\ c_1 & 1 \end{matrix}$                                                                         |
| $d \ (t, 0, \frac{1}{2})$                         | $\begin{matrix} \{2_{100}   0 & 0 & 0\} \\ d_1 & -i \\ d_2 & i \end{matrix}$                                                       |
| $e \ (0, t, \frac{1}{2})$                         | $\begin{matrix} \{2_{010}   0 & 0 & \frac{1}{2}\} \\ e_1 & i \\ e_2 & -i \end{matrix}$                                             |
| $f \ (\frac{t}{2}, 1 - \frac{t}{2}, \frac{1}{2})$ | $\begin{matrix} \{1   0 & 0 & 0\} \\ f_1 & 1 \end{matrix}$                                                                         |
| $g \ (0, 0, \frac{t}{2})$                         | $\begin{matrix} \{2_{001}   0 & 0 & \frac{1}{2}\} \\ g_1 & -ie^{-\frac{1}{2}i\pi t} \\ g_2 & ie^{-\frac{1}{2}i\pi t} \end{matrix}$ |
| $h \ (1, 0, \frac{t}{2})$                         | $\begin{matrix} \{2_{001}   0 & 0 & \frac{1}{2}\} \\ h_1 & -ie^{-\frac{1}{2}i\pi t} \\ h_2 & ie^{-\frac{1}{2}i\pi t} \end{matrix}$ |
| $i \ (\frac{1}{2}, \frac{1}{2}, \frac{t}{2})$     | $\begin{matrix} \{2_{001}   0 & 0 & \frac{1}{2}\} \\ i_1 & -ie^{-\frac{1}{2}i\pi t} \\ i_2 & ie^{-\frac{1}{2}i\pi t} \end{matrix}$ |

$$\begin{aligned}
\mathcal{W}_1^{\text{gapless}} = & \sum_{m=1}^{n_{a_1}} \text{sgn}(v_m^{a_1}) \frac{1 - \text{sgn}(\delta_m^{a_1})}{2} + \sum_{m=1}^{n_{a_2}} \text{sgn}(v_m^{a_2}) \frac{1 - \text{sgn}(\delta_m^{a_2})}{2} - 2 \sum_{m=1}^{n_{e_1}} \text{sgn}(v_m^{e_1}) \frac{1 - \text{sgn}(\delta_m^{e_1})}{2} \\
& - \sum_{m=1}^{n_{g_1}} \text{sgn}(v_m^{g_1}) \frac{1 - \text{sgn}(\delta_m^{g_1})}{2} - \sum_{m=1}^{n_{g_2}} \text{sgn}(v_m^{g_2}) \frac{1 - \text{sgn}(\delta_m^{g_2})}{2} + \sum_{m=1}^{n_{h_1}} \text{sgn}(v_m^{h_1}) \frac{1 - \text{sgn}(\delta_m^{h_1})}{2} \\
& + \sum_{m=1}^{n_{h_2}} \text{sgn}(v_m^{h_2}) \frac{1 - \text{sgn}(\delta_m^{h_2})}{2}
\end{aligned} \tag{S20.1}$$

$$\begin{aligned}
\mathcal{W}_2^{\text{gapless}} = & \sum_{m=1}^{n_{b_1}} \text{sgn}(v_m^{b_1}) \frac{1 - \text{sgn}(\delta_m^{b_1})}{2} + \sum_{m=1}^{n_{b_2}} \text{sgn}(v_m^{b_2}) \frac{1 - \text{sgn}(\delta_m^{b_2})}{2} - 2 \sum_{m=1}^{n_{e_1}} \text{sgn}(v_m^{e_1}) \frac{1 - \text{sgn}(\delta_m^{e_1})}{2} - \sum_{m=1}^{n_{g_1}} \text{sgn}(v_m^{g_1}) \frac{1 - \text{sgn}(\delta_m^{g_1})}{2} \\
& - \sum_{m=1}^{n_{g_2}} \text{sgn}(v_m^{g_2}) \frac{1 - \text{sgn}(\delta_m^{g_2})}{2} + \sum_{m=1}^{n_{h_1}} \text{sgn}(v_m^{h_1}) \frac{1 - \text{sgn}(\delta_m^{h_1})}{2} + \sum_{m=1}^{n_{h_2}} \text{sgn}(v_m^{h_2}) \frac{1 - \text{sgn}(\delta_m^{h_2})}{2}
\end{aligned} \tag{S20.2}$$

$$\begin{aligned}
\mathcal{W}_3^{\text{gapless}} = & \sum_{m=1}^{n_{c_1}} \text{sgn}(v_m^{c_1}) \frac{1 - \text{sgn}(\delta_m^{c_1})}{2} - 2 \sum_{m=1}^{n_{f_1}} \text{sgn}(v_m^{f_1}) \frac{1 - \text{sgn}(\delta_m^{f_1})}{2} - \sum_{m=1}^{n_{h_1}} \text{sgn}(v_m^{h_1}) \frac{1 - \text{sgn}(\delta_m^{h_1})}{2} \\
& - \sum_{m=1}^{n_{h_2}} \text{sgn}(v_m^{h_2}) \frac{1 - \text{sgn}(\delta_m^{h_2})}{2} + \sum_{m=1}^{n_{i_1}} \text{sgn}(v_m^{i_1}) \frac{1 - \text{sgn}(\delta_m^{i_1})}{2} + \sum_{m=1}^{n_{i_2}} \text{sgn}(v_m^{i_2}) \frac{1 - \text{sgn}(\delta_m^{i_2})}{2}
\end{aligned} \tag{S20.3}$$

$$\mathcal{W}_4^{\text{gapless}} = \sum_{m=1}^{n_{d_1}} \text{sgn}(v_m^{d_1}) \frac{1 - \text{sgn}(\delta_m^{d_1})}{2} - \sum_{m=1}^{n_{e_1}} \text{sgn}(v_m^{e_1}) \frac{1 - \text{sgn}(\delta_m^{e_1})}{2} \quad (\text{S20.4})$$

$$\begin{aligned} \mathcal{W}_1^{\text{gapped}} = & -2 \sum_{m=1}^{n_{a_2}} \text{sgn}(v_m^{a_2}) \frac{1 - \text{sgn}(\delta_m^{a_2})}{2} + 2 \sum_{m=1}^{n_{e_1}} \text{sgn}(v_m^{e_1}) \frac{1 - \text{sgn}(\delta_m^{e_1})}{2} + \sum_{m=1}^{n_{g_1}} \text{sgn}(v_m^{g_1}) \frac{1 - \text{sgn}(\delta_m^{g_1})}{2} \\ & + \sum_{m=1}^{n_{g_2}} \text{sgn}(v_m^{g_2}) \frac{1 - \text{sgn}(\delta_m^{g_2})}{2} - \sum_{m=1}^{n_{h_1}} \text{sgn}(v_m^{h_1}) \frac{1 - \text{sgn}(\delta_m^{h_1})}{2} - \sum_{m=1}^{n_{h_2}} \text{sgn}(v_m^{h_2}) \frac{1 - \text{sgn}(\delta_m^{h_2})}{2} \end{aligned} \quad (\text{S20.5})$$

$$\mathcal{W}_2^{\text{gapped}} = - \sum_{m=1}^{n_{a_2}} \text{sgn}(v_m^{a_2}) \frac{1 - \text{sgn}(\delta_m^{a_2})}{2} + \sum_{m=1}^{n_{b_2}} \text{sgn}(v_m^{b_2}) \frac{1 - \text{sgn}(\delta_m^{b_2})}{2} \quad (\text{S20.6})$$

$$\mathcal{X}_1 = \sum_{m=1}^{n_{a_2}} \frac{1 - \text{sgn}(\delta_m^{a_2})}{2} + \sum_{m=1}^{n_{g_2}} \frac{1 - \text{sgn}(\delta_m^{g_2})}{2} + \sum_{m=1}^{n_{h_1}} \frac{1 - \text{sgn}(\delta_m^{h_1})}{2} + \sum_{m=1}^{n_{i_1}} \frac{1 - \text{sgn}(\delta_m^{i_1})}{2} + \sum_{m=1}^{n_{i_2}} \frac{1 - \text{sgn}(\delta_m^{i_2})}{2} \mod 2 \quad (\text{S20.7})$$

$$\mathcal{X}_2 = \sum_{m=1}^{n_{a_2}} \frac{1 - \text{sgn}(\delta_m^{a_2})}{2} + \sum_{m=1}^{n_{g_2}} \frac{1 - \text{sgn}(\delta_m^{g_2})}{2} + \sum_{m=1}^{n_{h_1}} \frac{1 - \text{sgn}(\delta_m^{h_1})}{2} \mod 2 \quad (\text{S20.8})$$

$$\begin{aligned} \mathcal{X}_3 = & -2 \sum_{m=1}^{n_{f_1}} \text{sgn}(v_m^{f_1}) \frac{1 - \text{sgn}(\delta_m^{f_1})}{2} - \sum_{m=1}^{n_{h_1}} \text{sgn}(v_m^{h_1}) \frac{1 - \text{sgn}(\delta_m^{h_1})}{2} + \sum_{m=1}^{n_{h_2}} \text{sgn}(v_m^{h_2}) \frac{1 - \text{sgn}(\delta_m^{h_2})}{2} - \sum_{m=1}^{n_{i_1}} \text{sgn}(v_m^{i_1}) \frac{1 - \text{sgn}(\delta_m^{i_1})}{2} \\ & + \sum_{m=1}^{n_{i_2}} \text{sgn}(v_m^{i_2}) \frac{1 - \text{sgn}(\delta_m^{i_2})}{2} \mod 4 \end{aligned} \quad (\text{S20.9})$$

## S21. SPACE GROUP NO. 21

| line segment                                      | character of irrep (generators only)                         |
|---------------------------------------------------|--------------------------------------------------------------|
| $a \ (t, 0, 0)$                                   | $\{2_{100}   0 \ 0 \ 0\}$<br>$a_1 \quad -i$<br>$a_2 \quad i$ |
| $b \ (0, t, 0)$                                   | $\{2_{010}   0 \ 0 \ 0\}$<br>$b_1 \quad -i$<br>$b_2 \quad i$ |
| $c \ (\frac{t}{2}, 1 - \frac{t}{2}, 0)$           | $\{1   0 \ 0 \ 0\}$<br>$c_1 \quad 1$                         |
| $d \ (t, 0, \frac{1}{2})$                         | $\{2_{100}   0 \ 0 \ 0\}$<br>$d_1 \quad -i$<br>$d_2 \quad i$ |
| $e \ (0, t, \frac{1}{2})$                         | $\{2_{010}   0 \ 0 \ 0\}$<br>$e_1 \quad -i$<br>$e_2 \quad i$ |
| $f \ (\frac{t}{2}, 1 - \frac{t}{2}, \frac{1}{2})$ | $\{1   0 \ 0 \ 0\}$<br>$f_1 \quad 1$                         |

|                                                   |                                                                                    |
|---------------------------------------------------|------------------------------------------------------------------------------------|
| $g \quad (0, 0, \frac{t}{2})$                     | $\{2_{001}   \begin{smallmatrix} 0 & 0 & 0 \\ -i & & \\ & i & \end{smallmatrix}\}$ |
| $h \quad (1, 0, \frac{t}{2})$                     | $\{2_{001}   \begin{smallmatrix} 0 & 0 & 0 \\ -i & & \\ & i & \end{smallmatrix}\}$ |
| $i \quad (\frac{1}{2}, \frac{1}{2}, \frac{t}{2})$ | $\{2_{001}   \begin{smallmatrix} 0 & 0 & 0 \\ -i & & \\ & i & \end{smallmatrix}\}$ |

$$\begin{aligned}
\mathcal{W}_1^{\text{gapless}} = & \sum_{m=1}^{n_{a1}} \text{sgn}(v_m^{a1}) \frac{1 - \text{sgn}(\delta_m^{a1})}{2} + \sum_{m=1}^{n_{a2}} \text{sgn}(v_m^{a2}) \frac{1 - \text{sgn}(\delta_m^{a2})}{2} - \sum_{m=1}^{n_{e1}} \text{sgn}(v_m^{e1}) \frac{1 - \text{sgn}(\delta_m^{e1})}{2} \\
& - \sum_{m=1}^{n_{e2}} \text{sgn}(v_m^{e2}) \frac{1 - \text{sgn}(\delta_m^{e2})}{2} - \sum_{m=1}^{n_{g1}} \text{sgn}(v_m^{g1}) \frac{1 - \text{sgn}(\delta_m^{g1})}{2} - \sum_{m=1}^{n_{g2}} \text{sgn}(v_m^{g2}) \frac{1 - \text{sgn}(\delta_m^{g2})}{2} \\
& + \sum_{m=1}^{n_{h1}} \text{sgn}(v_m^{h1}) \frac{1 - \text{sgn}(\delta_m^{h1})}{2} + \sum_{m=1}^{n_{h2}} \text{sgn}(v_m^{h2}) \frac{1 - \text{sgn}(\delta_m^{h2})}{2}
\end{aligned} \tag{S21.1}$$

$$\begin{aligned}
\mathcal{W}_2^{\text{gapless}} = & \sum_{m=1}^{n_{b1}} \text{sgn}(v_m^{b1}) \frac{1 - \text{sgn}(\delta_m^{b1})}{2} + \sum_{m=1}^{n_{b2}} \text{sgn}(v_m^{b2}) \frac{1 - \text{sgn}(\delta_m^{b2})}{2} - \sum_{m=1}^{n_{e1}} \text{sgn}(v_m^{e1}) \frac{1 - \text{sgn}(\delta_m^{e1})}{2} \\
& - \sum_{m=1}^{n_{e2}} \text{sgn}(v_m^{e2}) \frac{1 - \text{sgn}(\delta_m^{e2})}{2} - \sum_{m=1}^{n_{g1}} \text{sgn}(v_m^{g1}) \frac{1 - \text{sgn}(\delta_m^{g1})}{2} - \sum_{m=1}^{n_{g2}} \text{sgn}(v_m^{g2}) \frac{1 - \text{sgn}(\delta_m^{g2})}{2} \\
& + \sum_{m=1}^{n_{h1}} \text{sgn}(v_m^{h1}) \frac{1 - \text{sgn}(\delta_m^{h1})}{2} + \sum_{m=1}^{n_{h2}} \text{sgn}(v_m^{h2}) \frac{1 - \text{sgn}(\delta_m^{h2})}{2}
\end{aligned} \tag{S21.2}$$

$$\begin{aligned}
\mathcal{W}_3^{\text{gapless}} = & \sum_{m=1}^{n_{c1}} \text{sgn}(v_m^{c1}) \frac{1 - \text{sgn}(\delta_m^{c1})}{2} - \sum_{m=1}^{n_{f1}} \text{sgn}(v_m^{f1}) \frac{1 - \text{sgn}(\delta_m^{f1})}{2} - \sum_{m=1}^{n_{h1}} \text{sgn}(v_m^{h1}) \frac{1 - \text{sgn}(\delta_m^{h1})}{2} \\
& - \sum_{m=1}^{n_{h2}} \text{sgn}(v_m^{h2}) \frac{1 - \text{sgn}(\delta_m^{h2})}{2} + \sum_{m=1}^{n_{i1}} \text{sgn}(v_m^{i1}) \frac{1 - \text{sgn}(\delta_m^{i1})}{2} + \sum_{m=1}^{n_{i2}} \text{sgn}(v_m^{i2}) \frac{1 - \text{sgn}(\delta_m^{i2})}{2}
\end{aligned} \tag{S21.3}$$

$$\begin{aligned}
\mathcal{W}_4^{\text{gapless}} = & \sum_{m=1}^{n_{d1}} \text{sgn}(v_m^{d1}) \frac{1 - \text{sgn}(\delta_m^{d1})}{2} + \sum_{m=1}^{n_{d2}} \text{sgn}(v_m^{d2}) \frac{1 - \text{sgn}(\delta_m^{d2})}{2} - \sum_{m=1}^{n_{e1}} \text{sgn}(v_m^{e1}) \frac{1 - \text{sgn}(\delta_m^{e1})}{2} - \sum_{m=1}^{n_{e2}} \text{sgn}(v_m^{e2}) \frac{1 - \text{sgn}(\delta_m^{e2})}{2}
\end{aligned} \tag{S21.4}$$

$$\mathcal{W}_1^{\text{gapped}} = - \sum_{m=1}^{n_{e1}} \text{sgn}(v_m^{e1}) \frac{1 - \text{sgn}(\delta_m^{e1})}{2} + \sum_{m=1}^{n_{e2}} \text{sgn}(v_m^{e2}) \frac{1 - \text{sgn}(\delta_m^{e2})}{2} \tag{S21.5}$$

$$\mathcal{W}_2^{\text{gapped}} = - \sum_{m=1}^{n_{a2}} \text{sgn}(v_m^{a2}) \frac{1 - \text{sgn}(\delta_m^{a2})}{2} + \sum_{m=1}^{n_{b2}} \text{sgn}(v_m^{b2}) \frac{1 - \text{sgn}(\delta_m^{b2})}{2} \tag{S21.6}$$

$$\mathcal{W}_3^{\text{gapped}} = - \sum_{m=1}^{n_{g1}} \text{sgn}(v_m^{g1}) \frac{1 - \text{sgn}(\delta_m^{g1})}{2} + \sum_{m=1}^{n_{g2}} \text{sgn}(v_m^{g2}) \frac{1 - \text{sgn}(\delta_m^{g2})}{2} \quad (\text{S21.7})$$

$$\mathcal{W}_4^{\text{gapped}} = \sum_{m=1}^{n_{a2}} \text{sgn}(v_m^{a2}) \frac{1 - \text{sgn}(\delta_m^{a2})}{2} - \sum_{m=1}^{n_{e1}} \text{sgn}(v_m^{e1}) \frac{1 - \text{sgn}(\delta_m^{e1})}{2} - \sum_{m=1}^{n_{g1}} \text{sgn}(v_m^{g1}) \frac{1 - \text{sgn}(\delta_m^{g1})}{2} + \sum_{m=1}^{n_{h1}} \text{sgn}(v_m^{h1}) \frac{1 - \text{sgn}(\delta_m^{h1})}{2} \quad (\text{S21.8})$$

$$\mathcal{W}_5^{\text{gapped}} = \sum_{m=1}^{n_{a2}} \text{sgn}(v_m^{a2}) \frac{1 - \text{sgn}(\delta_m^{a2})}{2} - \sum_{m=1}^{n_{e1}} \text{sgn}(v_m^{e1}) \frac{1 - \text{sgn}(\delta_m^{e1})}{2} - \sum_{m=1}^{n_{g1}} \text{sgn}(v_m^{g1}) \frac{1 - \text{sgn}(\delta_m^{g1})}{2} + \sum_{m=1}^{n_{h2}} \text{sgn}(v_m^{h2}) \frac{1 - \text{sgn}(\delta_m^{h2})}{2} \quad (\text{S21.9})$$

$$\mathcal{W}_6^{\text{gapped}} = \sum_{m=1}^{n_{d2}} \text{sgn}(v_m^{d2}) \frac{1 - \text{sgn}(\delta_m^{d2})}{2} - \sum_{m=1}^{n_{e1}} \text{sgn}(v_m^{e1}) \frac{1 - \text{sgn}(\delta_m^{e1})}{2} \quad (\text{S21.10})$$

$$\mathcal{W}_7^{\text{gapped}} = - \sum_{m=1}^{n_{i1}} \text{sgn}(v_m^{i1}) \frac{1 - \text{sgn}(\delta_m^{i1})}{2} + \sum_{m=1}^{n_{i2}} \text{sgn}(v_m^{i2}) \frac{1 - \text{sgn}(\delta_m^{i2})}{2} \quad (\text{S21.11})$$

$$\mathcal{X}_1 = \sum_{m=1}^{n_{f1}} \frac{1 - \text{sgn}(\delta_m^{f1})}{2} \mod 2 \quad (\text{S21.12})$$

## S22. SPACE GROUP NO. 22

| line segment                                        | character of irrep (generators only)                         |
|-----------------------------------------------------|--------------------------------------------------------------|
| $a \ (t, 0, 0)$                                     | $\{2_{100}   0 \ 0 \ 0\}$<br>$a_1 \quad -i$<br>$a_2 \quad i$ |
| $b \ (1, t, 0)$                                     | $\{2_{010}   0 \ 0 \ 0\}$<br>$b_1 \quad -i$<br>$b_2 \quad i$ |
| $c \ (0, 0, 1 - t)$                                 | $\{2_{001}   0 \ 0 \ 0\}$<br>$c_1 \quad -i$<br>$c_2 \quad i$ |
| $d \ (1 - t, 1, 0)$                                 | $\{2_{100}   0 \ 0 \ 0\}$<br>$d_1 \quad -i$<br>$d_2 \quad i$ |
| $e \ (0, t, 0)$                                     | $\{2_{010}   0 \ 0 \ 0\}$<br>$e_1 \quad -i$<br>$e_2 \quad i$ |
| $f \ (0, 1, 1 - t)$                                 | $\{2_{001}   0 \ 0 \ 0\}$<br>$f_1 \quad -i$<br>$f_2 \quad i$ |
| $g \ (1 - t, 0, t)$                                 | $\{1   0 \ 0 \ 0\}$<br>$g_1 \quad 1$                         |
| $h \ (\frac{t+1}{2}, \frac{1-t}{2}, \frac{1-t}{2})$ | $\{1   0 \ 0 \ 0\}$<br>$h_1 \quad 1$                         |

---


$$\begin{aligned} \mathcal{W}_1^{\text{gapless}} = & \sum_{m=1}^{n_{a_1}} \text{sgn}(v_m^{a_1}) \frac{1 - \text{sgn}(\delta_m^{a_1})}{2} + \sum_{m=1}^{n_{a_2}} \text{sgn}(v_m^{a_2}) \frac{1 - \text{sgn}(\delta_m^{a_2})}{2} - \sum_{m=1}^{n_{e_1}} \text{sgn}(v_m^{e_1}) \frac{1 - \text{sgn}(\delta_m^{e_1})}{2} \\ & - \sum_{m=1}^{n_{e_2}} \text{sgn}(v_m^{e_2}) \frac{1 - \text{sgn}(\delta_m^{e_2})}{2} + \sum_{m=1}^{n_{f_1}} \text{sgn}(v_m^{f_1}) \frac{1 - \text{sgn}(\delta_m^{f_1})}{2} + \sum_{m=1}^{n_{f_2}} \text{sgn}(v_m^{f_2}) \frac{1 - \text{sgn}(\delta_m^{f_2})}{2} \end{aligned} \quad (\text{S22.1})$$

$$\mathcal{W}_2^{\text{gapless}} = \sum_{m=1}^{n_{b_1}} \text{sgn}(v_m^{b_1}) \frac{1 - \text{sgn}(\delta_m^{b_1})}{2} + \sum_{m=1}^{n_{b_2}} \text{sgn}(v_m^{b_2}) \frac{1 - \text{sgn}(\delta_m^{b_2})}{2} - \sum_{m=1}^{n_{g_1}} \text{sgn}(v_m^{g_1}) \frac{1 - \text{sgn}(\delta_m^{g_1})}{2} \quad (\text{S22.2})$$

$$\begin{aligned} \mathcal{W}_3^{\text{gapless}} = & \sum_{m=1}^{n_{c_1}} \text{sgn}(v_m^{c_1}) \frac{1 - \text{sgn}(\delta_m^{c_1})}{2} + \sum_{m=1}^{n_{c_2}} \text{sgn}(v_m^{c_2}) \frac{1 - \text{sgn}(\delta_m^{c_2})}{2} + \sum_{m=1}^{n_{e_1}} \text{sgn}(v_m^{e_1}) \frac{1 - \text{sgn}(\delta_m^{e_1})}{2} + \sum_{m=1}^{n_{e_2}} \text{sgn}(v_m^{e_2}) \frac{1 - \text{sgn}(\delta_m^{e_2})}{2} \\ & - \sum_{m=1}^{n_{f_1}} \text{sgn}(v_m^{f_1}) \frac{1 - \text{sgn}(\delta_m^{f_1})}{2} - \sum_{m=1}^{n_{f_2}} \text{sgn}(v_m^{f_2}) \frac{1 - \text{sgn}(\delta_m^{f_2})}{2} + \sum_{m=1}^{n_{g_1}} \text{sgn}(v_m^{g_1}) \frac{1 - \text{sgn}(\delta_m^{g_1})}{2} \end{aligned} \quad (\text{S22.3})$$

$$\begin{aligned} \mathcal{W}_4^{\text{gapless}} = & \sum_{m=1}^{n_{d_1}} \text{sgn}(v_m^{d_1}) \frac{1 - \text{sgn}(\delta_m^{d_1})}{2} + \sum_{m=1}^{n_{d_2}} \text{sgn}(v_m^{d_2}) \frac{1 - \text{sgn}(\delta_m^{d_2})}{2} - \sum_{m=1}^{n_{f_1}} \text{sgn}(v_m^{f_1}) \frac{1 - \text{sgn}(\delta_m^{f_1})}{2} \\ & - \sum_{m=1}^{n_{f_2}} \text{sgn}(v_m^{f_2}) \frac{1 - \text{sgn}(\delta_m^{f_2})}{2} + \sum_{m=1}^{n_{g_1}} \text{sgn}(v_m^{g_1}) \frac{1 - \text{sgn}(\delta_m^{g_1})}{2} \end{aligned} \quad (\text{S22.4})$$

$$\mathcal{W}_1^{\text{gapped}} = \sum_{m=1}^{n_{c_2}} \text{sgn}(v_m^{c_2}) \frac{1 - \text{sgn}(\delta_m^{c_2})}{2} - \sum_{m=1}^{n_{d_2}} \text{sgn}(v_m^{d_2}) \frac{1 - \text{sgn}(\delta_m^{d_2})}{2} + \sum_{m=1}^{n_{e_1}} \text{sgn}(v_m^{e_1}) \frac{1 - \text{sgn}(\delta_m^{e_1})}{2} \quad (\text{S22.5})$$

$$\mathcal{W}_2^{\text{gapped}} = \sum_{m=1}^{n_{c_2}} \text{sgn}(v_m^{c_2}) \frac{1 - \text{sgn}(\delta_m^{c_2})}{2} - \sum_{m=1}^{n_{d_2}} \text{sgn}(v_m^{d_2}) \frac{1 - \text{sgn}(\delta_m^{d_2})}{2} + \sum_{m=1}^{n_{e_2}} \text{sgn}(v_m^{e_2}) \frac{1 - \text{sgn}(\delta_m^{e_2})}{2} \quad (\text{S22.6})$$

$$\mathcal{W}_3^{\text{gapped}} = \sum_{m=1}^{n_{a_2}} \text{sgn}(v_m^{a_2}) \frac{1 - \text{sgn}(\delta_m^{a_2})}{2} + \sum_{m=1}^{n_{c_2}} \text{sgn}(v_m^{c_2}) \frac{1 - \text{sgn}(\delta_m^{c_2})}{2} - \sum_{m=1}^{n_{d_2}} \text{sgn}(v_m^{d_2}) \frac{1 - \text{sgn}(\delta_m^{d_2})}{2} + \sum_{m=1}^{n_{f_1}} \text{sgn}(v_m^{f_1}) \frac{1 - \text{sgn}(\delta_m^{f_1})}{2} \quad (\text{S22.7})$$

$$\mathcal{W}_4^{\text{gapped}} = \sum_{m=1}^{n_{a_2}} \text{sgn}(v_m^{a_2}) \frac{1 - \text{sgn}(\delta_m^{a_2})}{2} + \sum_{m=1}^{n_{c_2}} \text{sgn}(v_m^{c_2}) \frac{1 - \text{sgn}(\delta_m^{c_2})}{2} - \sum_{m=1}^{n_{d_2}} \text{sgn}(v_m^{d_2}) \frac{1 - \text{sgn}(\delta_m^{d_2})}{2} + \sum_{m=1}^{n_{f_2}} \text{sgn}(v_m^{f_2}) \frac{1 - \text{sgn}(\delta_m^{f_2})}{2} \quad (\text{S22.8})$$

$$\mathcal{W}_5^{\text{gapped}} = 2 \sum_{m=1}^{n_{a_2}} \text{sgn}(v_m^{a_2}) \frac{1 - \text{sgn}(\delta_m^{a_2})}{2} + 2 \sum_{m=1}^{n_{c_2}} \text{sgn}(v_m^{c_2}) \frac{1 - \text{sgn}(\delta_m^{c_2})}{2} + \sum_{m=1}^{n_{g_1}} \text{sgn}(v_m^{g_1}) \frac{1 - \text{sgn}(\delta_m^{g_1})}{2} \quad (\text{S22.9})$$

$$\mathcal{W}_6^{\text{gapped}} = \sum_{m=1}^{n_{a_2}} \text{sgn}(v_m^{a_2}) \frac{1 - \text{sgn}(\delta_m^{a_2})}{2} + \sum_{m=1}^{n_{b_2}} \text{sgn}(v_m^{b_2}) \frac{1 - \text{sgn}(\delta_m^{b_2})}{2} + \sum_{m=1}^{n_{c_2}} \text{sgn}(v_m^{c_2}) \frac{1 - \text{sgn}(\delta_m^{c_2})}{2} \quad (\text{S22.10})$$

$$\mathcal{X}_1 = \sum_{m=1}^{n_{h_1}} \frac{1 - \text{sgn}(\delta_m^{h_1})}{2} \mod 2 \quad (\text{S22.11})$$

### S23. SPACE GROUP NO. 23

| line segment                                        | character of irrep (generators only)                                         |
|-----------------------------------------------------|------------------------------------------------------------------------------|
| $a \ (0, 0, t)$                                     | $\begin{matrix} \{2_{001}   0 & 0 & 0\} \\ a_1 & -i \\ a_2 & i \end{matrix}$ |
| $b \ (0, t, 0)$                                     | $\begin{matrix} \{2_{010}   0 & 0 & 0\} \\ b_1 & -i \\ b_2 & i \end{matrix}$ |
| $c \ (t, 0, 0)$                                     | $\begin{matrix} \{2_{100}   0 & 0 & 0\} \\ c_1 & -i \\ c_2 & i \end{matrix}$ |
| $d \ (\frac{1}{2}, \frac{1}{2}, \frac{t}{2})$       | $\begin{matrix} \{2_{001}   0 & 0 & 0\} \\ d_1 & -i \\ d_2 & i \end{matrix}$ |
| $e \ (\frac{1-t}{2}, \frac{1}{2}, \frac{1}{2})$     | $\begin{matrix} \{2_{100}   0 & 0 & 0\} \\ e_1 & -i \\ e_2 & i \end{matrix}$ |
| $f \ (\frac{1}{2}, \frac{1-t}{2}, \frac{1}{2})$     | $\begin{matrix} \{2_{010}   0 & 0 & 0\} \\ f_1 & -i \\ f_2 & i \end{matrix}$ |
| $g \ (0, \frac{t}{2}, 1 - \frac{t}{2})$             | $\begin{matrix} \{1   0 & 0 & 0\} \\ g_1 & 1 \end{matrix}$                   |
| $h \ (\frac{t}{2}, 0, 1 - \frac{t}{2})$             | $\begin{matrix} \{1   0 & 0 & 0\} \\ h_1 & 1 \end{matrix}$                   |
| $i \ (\frac{1-t}{2}, \frac{t+1}{2}, 0)$             | $\begin{matrix} \{1   0 & 0 & 0\} \\ i_1 & 1 \end{matrix}$                   |
| $j \ (\frac{1-t}{2}, \frac{1-t}{2}, \frac{t+1}{2})$ | $\begin{matrix} \{1   0 & 0 & 0\} \\ j_1 & 1 \end{matrix}$                   |

$$\mathcal{W}_1^{\text{gapless}} = \sum_{m=1}^{n_{a_1}} \text{sgn}(v_m^{a_1}) \frac{1 - \text{sgn}(\delta_m^{a_1})}{2} + \sum_{m=1}^{n_{a_2}} \text{sgn}(v_m^{a_2}) \frac{1 - \text{sgn}(\delta_m^{a_2})}{2} - \sum_{m=1}^{n_{c_1}} \text{sgn}(v_m^{c_1}) \frac{1 - \text{sgn}(\delta_m^{c_1})}{2} - \sum_{m=1}^{n_{c_2}} \text{sgn}(v_m^{c_2}) \frac{1 - \text{sgn}(\delta_m^{c_2})}{2} \quad (\text{S23.1})$$

$$\mathcal{W}_2^{\text{gapless}} = \sum_{m=1}^{n_{b_1}} \text{sgn}(v_m^{b_1}) \frac{1 - \text{sgn}(\delta_m^{b_1})}{2} + \sum_{m=1}^{n_{b_2}} \text{sgn}(v_m^{b_2}) \frac{1 - \text{sgn}(\delta_m^{b_2})}{2} - \sum_{m=1}^{n_{c_1}} \text{sgn}(v_m^{c_1}) \frac{1 - \text{sgn}(\delta_m^{c_1})}{2} - \sum_{m=1}^{n_{c_2}} \text{sgn}(v_m^{c_2}) \frac{1 - \text{sgn}(\delta_m^{c_2})}{2} \quad (\text{S23.2})$$

$$\mathcal{W}_3^{\text{gapless}} = \sum_{m=1}^{n_{d_1}} \text{sgn}(v_m^{d_1}) \frac{1 - \text{sgn}(\delta_m^{d_1})}{2} + \sum_{m=1}^{n_{d_2}} \text{sgn}(v_m^{d_2}) \frac{1 - \text{sgn}(\delta_m^{d_2})}{2} - \sum_{m=1}^{n_{i_1}} \text{sgn}(v_m^{i_1}) \frac{1 - \text{sgn}(\delta_m^{i_1})}{2} + \sum_{m=1}^{n_{j_1}} \text{sgn}(v_m^{j_1}) \frac{1 - \text{sgn}(\delta_m^{j_1})}{2} \quad (\text{S23.3})$$



$$\mathcal{W}_4^{\text{gapless}} = \sum_{m=1}^{n_{e_1}} \text{sgn}(v_m^{e_1}) \frac{1 - \text{sgn}(\delta_m^{e_1})}{2} + \sum_{m=1}^{n_{e_2}} \text{sgn}(v_m^{e_2}) \frac{1 - \text{sgn}(\delta_m^{e_2})}{2} - \sum_{m=1}^{n_{g_1}} \text{sgn}(v_m^{g_1}) \frac{1 - \text{sgn}(\delta_m^{g_1})}{2} - \sum_{m=1}^{n_{j_1}} \text{sgn}(v_m^{j_1}) \frac{1 - \text{sgn}(\delta_m^{j_1})}{2} \quad (\text{S23.4})$$

$$\mathcal{W}_5^{\text{gapless}} = \sum_{m=1}^{n_{f_1}} \text{sgn}(v_m^{f_1}) \frac{1 - \text{sgn}(\delta_m^{f_1})}{2} + \sum_{m=1}^{n_{f_2}} \text{sgn}(v_m^{f_2}) \frac{1 - \text{sgn}(\delta_m^{f_2})}{2} - \sum_{m=1}^{n_{h_1}} \text{sgn}(v_m^{h_1}) \frac{1 - \text{sgn}(\delta_m^{h_1})}{2} - \sum_{m=1}^{n_{j_1}} \text{sgn}(v_m^{j_1}) \frac{1 - \text{sgn}(\delta_m^{j_1})}{2} \quad (\text{S23.5})$$

$$\mathcal{W}_1^{\text{gapped}} = \sum_{m=1}^{n_{c_1}} \text{sgn}(v_m^{c_1}) \frac{1 - \text{sgn}(\delta_m^{c_1})}{2} - \sum_{m=1}^{n_{c_2}} \text{sgn}(v_m^{c_2}) \frac{1 - \text{sgn}(\delta_m^{c_2})}{2} \quad (\text{S23.6})$$

$$\mathcal{W}_2^{\text{gapped}} = \sum_{m=1}^{n_{b_2}} \text{sgn}(v_m^{b_2}) \frac{1 - \text{sgn}(\delta_m^{b_2})}{2} - \sum_{m=1}^{n_{c_2}} \text{sgn}(v_m^{c_2}) \frac{1 - \text{sgn}(\delta_m^{c_2})}{2} \quad (\text{S23.7})$$

$$\mathcal{W}_3^{\text{gapped}} = \sum_{m=1}^{n_{a_2}} \text{sgn}(v_m^{a_2}) \frac{1 - \text{sgn}(\delta_m^{a_2})}{2} - \sum_{m=1}^{n_{c_2}} \text{sgn}(v_m^{c_2}) \frac{1 - \text{sgn}(\delta_m^{c_2})}{2} \quad (\text{S23.8})$$

$$\begin{aligned} \mathcal{W}_4^{\text{gapped}} &= 2 \sum_{m=1}^{n_{e_2}} \text{sgn}(v_m^{e_2}) \frac{1 - \text{sgn}(\delta_m^{e_2})}{2} - 2 \sum_{m=1}^{n_{f_2}} \text{sgn}(v_m^{f_2}) \frac{1 - \text{sgn}(\delta_m^{f_2})}{2} - \sum_{m=1}^{n_{g_1}} \text{sgn}(v_m^{g_1}) \frac{1 - \text{sgn}(\delta_m^{g_1})}{2} \\ &\quad + \sum_{m=1}^{n_{h_1}} \text{sgn}(v_m^{h_1}) \frac{1 - \text{sgn}(\delta_m^{h_1})}{2} \end{aligned} \quad (\text{S23.9})$$

$$\begin{aligned} \mathcal{W}_5^{\text{gapped}} &= -2 \sum_{m=1}^{n_{d_2}} \text{sgn}(v_m^{d_2}) \frac{1 - \text{sgn}(\delta_m^{d_2})}{2} - 2 \sum_{m=1}^{n_{e_2}} \text{sgn}(v_m^{e_2}) \frac{1 - \text{sgn}(\delta_m^{e_2})}{2} + \sum_{m=1}^{n_{g_1}} \text{sgn}(v_m^{g_1}) \frac{1 - \text{sgn}(\delta_m^{g_1})}{2} \\ &\quad + \sum_{m=1}^{n_{i_1}} \text{sgn}(v_m^{i_1}) \frac{1 - \text{sgn}(\delta_m^{i_1})}{2} \end{aligned} \quad (\text{S23.10})$$

$$\mathcal{W}_6^{\text{gapped}} = -2 \sum_{m=1}^{n_{e_2}} \text{sgn}(v_m^{e_2}) \frac{1 - \text{sgn}(\delta_m^{e_2})}{2} + \sum_{m=1}^{n_{g_1}} \text{sgn}(v_m^{g_1}) \frac{1 - \text{sgn}(\delta_m^{g_1})}{2} + \sum_{m=1}^{n_{j_1}} \text{sgn}(v_m^{j_1}) \frac{1 - \text{sgn}(\delta_m^{j_1})}{2} \quad (\text{S23.11})$$

$$\mathcal{X}_1 = \sum_{m=1}^{n_{g_1}} \frac{1 - \text{sgn}(\delta_m^{g_1})}{2} \mod 2 \quad (\text{S23.12})$$

## S24. SPACE GROUP NO. 24

| line segment                                        | character of irrep (generators only)                                                           |
|-----------------------------------------------------|------------------------------------------------------------------------------------------------|
| $a \ (0, 0, t)$                                     | $\begin{matrix} \{2_{001}   0 \ \frac{1}{2} \ 0\} \\ a_1 \quad -i \\ a_2 \quad i \end{matrix}$ |
| $b \ (0, t, 0)$                                     | $\begin{matrix} \{2_{010}   \frac{1}{2} \ 0 \ 0\} \\ b_1 \quad -i \\ b_2 \quad i \end{matrix}$ |
| $c \ (t, 0, 0)$                                     | $\begin{matrix} \{2_{100}   0 \ 0 \ \frac{1}{2}\} \\ c_1 \quad -i \\ c_2 \quad i \end{matrix}$ |
| $d \ (\frac{1}{2}, \frac{1}{2}, \frac{t}{2})$       | $\begin{matrix} \{2_{001}   0 \ \frac{1}{2} \ 0\} \\ d_1 \quad i \\ d_2 \quad -i \end{matrix}$ |
| $e \ (\frac{1-t}{2}, \frac{1}{2}, \frac{1}{2})$     | $\begin{matrix} \{2_{100}   0 \ 0 \ \frac{1}{2}\} \\ e_1 \quad i \\ e_2 \quad -i \end{matrix}$ |
| $f \ (\frac{1}{2}, \frac{1-t}{2}, \frac{1}{2})$     | $\begin{matrix} \{2_{010}   \frac{1}{2} \ 0 \ 0\} \\ f_1 \quad i \\ f_2 \quad -i \end{matrix}$ |
| $g \ (0, \frac{t}{2}, 1 - \frac{t}{2})$             | $\begin{matrix} \{1   0 \ 0 \ 0\} \\ g_1 \quad 1 \end{matrix}$                                 |
| $h \ (\frac{t}{2}, 0, 1 - \frac{t}{2})$             | $\begin{matrix} \{1   0 \ 0 \ 0\} \\ h_1 \quad 1 \end{matrix}$                                 |
| $i \ (\frac{1-t}{2}, \frac{t+1}{2}, 0)$             | $\begin{matrix} \{1   0 \ 0 \ 0\} \\ i_1 \quad 1 \end{matrix}$                                 |
| $j \ (\frac{1-t}{2}, \frac{1-t}{2}, \frac{t+1}{2})$ | $\begin{matrix} \{1   0 \ 0 \ 0\} \\ j_1 \quad 1 \end{matrix}$                                 |

$$\mathcal{W}_1^{\text{gapless}} = \sum_{m=1}^{n_{a_1}} \text{sgn}(v_m^{a_1}) \frac{1 - \text{sgn}(\delta_m^{a_1})}{2} + \sum_{m=1}^{n_{a_2}} \text{sgn}(v_m^{a_2}) \frac{1 - \text{sgn}(\delta_m^{a_2})}{2} - \sum_{m=1}^{n_{c_1}} \text{sgn}(v_m^{c_1}) \frac{1 - \text{sgn}(\delta_m^{c_1})}{2} - \sum_{m=1}^{n_{c_2}} \text{sgn}(v_m^{c_2}) \frac{1 - \text{sgn}(\delta_m^{c_2})}{2} \quad (\text{S24.1})$$

$$\mathcal{W}_2^{\text{gapless}} = \sum_{m=1}^{n_{b_1}} \text{sgn}(v_m^{b_1}) \frac{1 - \text{sgn}(\delta_m^{b_1})}{2} + \sum_{m=1}^{n_{b_2}} \text{sgn}(v_m^{b_2}) \frac{1 - \text{sgn}(\delta_m^{b_2})}{2} - \sum_{m=1}^{n_{c_1}} \text{sgn}(v_m^{c_1}) \frac{1 - \text{sgn}(\delta_m^{c_1})}{2} - \sum_{m=1}^{n_{c_2}} \text{sgn}(v_m^{c_2}) \frac{1 - \text{sgn}(\delta_m^{c_2})}{2} \quad (\text{S24.2})$$

$$\mathcal{W}_3^{\text{gapless}} = \sum_{m=1}^{n_{d_1}} \text{sgn}(v_m^{d_1}) \frac{1 - \text{sgn}(\delta_m^{d_1})}{2} + \sum_{m=1}^{n_{d_2}} \text{sgn}(v_m^{d_2}) \frac{1 - \text{sgn}(\delta_m^{d_2})}{2} - \sum_{m=1}^{n_{i_1}} \text{sgn}(v_m^{i_1}) \frac{1 - \text{sgn}(\delta_m^{i_1})}{2} + \sum_{m=1}^{n_{j_1}} \text{sgn}(v_m^{j_1}) \frac{1 - \text{sgn}(\delta_m^{j_1})}{2} \quad (\text{S24.3})$$

$$\mathcal{W}_4^{\text{gapless}} = \sum_{m=1}^{n_{e_1}} \text{sgn}(v_m^{e_1}) \frac{1 - \text{sgn}(\delta_m^{e_1})}{2} + \sum_{m=1}^{n_{e_2}} \text{sgn}(v_m^{e_2}) \frac{1 - \text{sgn}(\delta_m^{e_2})}{2} - \sum_{m=1}^{n_{g_1}} \text{sgn}(v_m^{g_1}) \frac{1 - \text{sgn}(\delta_m^{g_1})}{2} - \sum_{m=1}^{n_{j_1}} \text{sgn}(v_m^{j_1}) \frac{1 - \text{sgn}(\delta_m^{j_1})}{2} \quad (\text{S24.4})$$

$$\mathcal{W}_5^{\text{gapless}} = \sum_{m=1}^{n_{f_1}} \text{sgn}(v_m^{f_1}) \frac{1 - \text{sgn}(\delta_m^{f_1})}{2} + \sum_{m=1}^{n_{f_2}} \text{sgn}(v_m^{f_2}) \frac{1 - \text{sgn}(\delta_m^{f_2})}{2} - \sum_{m=1}^{n_{h_1}} \text{sgn}(v_m^{h_1}) \frac{1 - \text{sgn}(\delta_m^{h_1})}{2} - \sum_{m=1}^{n_{j_1}} \text{sgn}(v_m^{j_1}) \frac{1 - \text{sgn}(\delta_m^{j_1})}{2} \quad (\text{S24.5})$$

$$\mathcal{W}_1^{\text{gapped}} = \sum_{m=1}^{n_{b_2}} \text{sgn}(v_m^{b_2}) \frac{1 - \text{sgn}(\delta_m^{b_2})}{2} - \sum_{m=1}^{n_{c_2}} \text{sgn}(v_m^{c_2}) \frac{1 - \text{sgn}(\delta_m^{c_2})}{2} \quad (\text{S24.6})$$

$$\mathcal{W}_2^{\text{gapped}} = \sum_{m=1}^{n_{c_1}} \text{sgn}(v_m^{c_1}) \frac{1 - \text{sgn}(\delta_m^{c_1})}{2} - \sum_{m=1}^{n_{c_2}} \text{sgn}(v_m^{c_2}) \frac{1 - \text{sgn}(\delta_m^{c_2})}{2} \quad (\text{S24.7})$$

$$\mathcal{W}_3^{\text{gapped}} = \sum_{m=1}^{n_{a_2}} \text{sgn}(v_m^{a_2}) \frac{1 - \text{sgn}(\delta_m^{a_2})}{2} - \sum_{m=1}^{n_{c_2}} \text{sgn}(v_m^{c_2}) \frac{1 - \text{sgn}(\delta_m^{c_2})}{2} \quad (\text{S24.8})$$

$$\mathcal{X}_1 = \sum_{m=1}^{n_{g_1}} \frac{1 - \text{sgn}(\delta_m^{g_1})}{2} + \sum_{m=1}^{n_{h_1}} \frac{1 - \text{sgn}(\delta_m^{h_1})}{2} + \sum_{m=1}^{n_{i_1}} \frac{1 - \text{sgn}(\delta_m^{i_1})}{2} \quad \text{mod } 2 \quad (\text{S24.9})$$

$$\mathcal{X}_2 = \sum_{m=1}^{n_{h_1}} \frac{1 - \text{sgn}(\delta_m^{h_1})}{2} \quad \text{mod } 2 \quad (\text{S24.10})$$

$$\mathcal{X}_3 = \sum_{m=1}^{n_{g_1}} \frac{1 - \text{sgn}(\delta_m^{g_1})}{2} \quad \text{mod } 2 \quad (\text{S24.11})$$

## S25. SPACE GROUP NO. 25

| line segment                                        | character of irrep (generators only)                         |
|-----------------------------------------------------|--------------------------------------------------------------|
| $a \quad (\frac{t}{2}, 0, 0)$                       | $\{m_{010}   0 \ 0 \ 0\}$<br>$a_1 \quad -i$<br>$a_2 \quad i$ |
| $b \quad (0, \frac{t}{2}, 0)$                       | $\{m_{100}   0 \ 0 \ 0\}$<br>$b_1 \quad -i$<br>$b_2 \quad i$ |
| $c \quad (\frac{1}{2}, \frac{t}{2}, 0)$             | $\{m_{100}   0 \ 0 \ 0\}$<br>$c_1 \quad -i$<br>$c_2 \quad i$ |
| $d \quad (\frac{1-t}{2}, \frac{1}{2}, 0)$           | $\{m_{010}   0 \ 0 \ 0\}$<br>$d_1 \quad -i$<br>$d_2 \quad i$ |
| $e \quad (\frac{t}{2}, 0, \frac{1}{2})$             | $\{m_{010}   0 \ 0 \ 0\}$<br>$e_1 \quad -i$<br>$e_2 \quad i$ |
| $f \quad (0, \frac{t}{2}, \frac{1}{2})$             | $\{m_{100}   0 \ 0 \ 0\}$<br>$f_1 \quad -i$<br>$f_2 \quad i$ |
| $g \quad (\frac{1}{2}, \frac{t}{2}, \frac{1}{2})$   | $\{m_{100}   0 \ 0 \ 0\}$<br>$g_1 \quad -i$<br>$g_2 \quad i$ |
| $h \quad (\frac{1-t}{2}, \frac{1}{2}, \frac{1}{2})$ | $\{m_{010}   0 \ 0 \ 0\}$<br>$h_1 \quad -i$<br>$h_2 \quad i$ |

|                                                   |       |                            |                            |
|---------------------------------------------------|-------|----------------------------|----------------------------|
| $i \quad (0, 0, \frac{t}{2})$                     | $i_1$ | $\{2_{001}   0 \ 0 \ 0 \}$ | $\{m_{100}   0 \ 0 \ 0 \}$ |
| $j \quad (\frac{1}{2}, 0, \frac{t}{2})$           | $j_1$ | $\{2_{001}   0 \ 0 \ 0 \}$ | $\{m_{100}   0 \ 0 \ 0 \}$ |
| $k \quad (\frac{1}{2}, \frac{1}{2}, \frac{t}{2})$ | $k_1$ | $\{2_{001}   0 \ 0 \ 0 \}$ | $\{m_{100}   0 \ 0 \ 0 \}$ |
| $l \quad (0, \frac{1}{2}, \frac{t}{2})$           | $l_1$ | $\{2_{001}   0 \ 0 \ 0 \}$ | $\{m_{100}   0 \ 0 \ 0 \}$ |

$$\begin{aligned}
\mathcal{W}_1^{\text{gapless}} = & \sum_{m=1}^{n_{a_1}} \text{sgn}(v_m^{a_1}) \frac{1 - \text{sgn}(\delta_m^{a_1})}{2} + \sum_{m=1}^{n_{e_2}} \text{sgn}(v_m^{e_2}) \frac{1 - \text{sgn}(\delta_m^{e_2})}{2} - \sum_{m=1}^{n_{f_1}} \text{sgn}(v_m^{f_1}) \frac{1 - \text{sgn}(\delta_m^{f_1})}{2} - \sum_{m=1}^{n_{f_2}} \text{sgn}(v_m^{f_2}) \frac{1 - \text{sgn}(\delta_m^{f_2})}{2} \\
& + \sum_{m=1}^{n_{g_1}} \text{sgn}(v_m^{g_1}) \frac{1 - \text{sgn}(\delta_m^{g_1})}{2} + \sum_{m=1}^{n_{g_2}} \text{sgn}(v_m^{g_2}) \frac{1 - \text{sgn}(\delta_m^{g_2})}{2} + \sum_{m=1}^{n_{h_1}} \text{sgn}(v_m^{h_1}) \frac{1 - \text{sgn}(\delta_m^{h_1})}{2} \\
& + \sum_{m=1}^{n_{h_2}} \text{sgn}(v_m^{h_2}) \frac{1 - \text{sgn}(\delta_m^{h_2})}{2} - \sum_{m=1}^{n_{i_1}} \text{sgn}(v_m^{i_1}) \frac{1 - \text{sgn}(\delta_m^{i_1})}{2} + \sum_{m=1}^{n_{j_1}} \text{sgn}(v_m^{j_1}) \frac{1 - \text{sgn}(\delta_m^{j_1})}{2}
\end{aligned} \tag{S25.1}$$

$$\mathcal{W}_2^{\text{gapless}} = \sum_{m=1}^{n_{a_2}} \text{sgn}(v_m^{a_2}) \frac{1 - \text{sgn}(\delta_m^{a_2})}{2} - \sum_{m=1}^{n_{e_2}} \text{sgn}(v_m^{e_2}) \frac{1 - \text{sgn}(\delta_m^{e_2})}{2} - \sum_{m=1}^{n_{i_1}} \text{sgn}(v_m^{i_1}) \frac{1 - \text{sgn}(\delta_m^{i_1})}{2} + \sum_{m=1}^{n_{j_1}} \text{sgn}(v_m^{j_1}) \frac{1 - \text{sgn}(\delta_m^{j_1})}{2} \tag{S25.2}$$

$$\mathcal{W}_3^{\text{gapless}} = \sum_{m=1}^{n_{b_1}} \text{sgn}(v_m^{b_1}) \frac{1 - \text{sgn}(\delta_m^{b_1})}{2} - \sum_{m=1}^{n_{f_1}} \text{sgn}(v_m^{f_1}) \frac{1 - \text{sgn}(\delta_m^{f_1})}{2} - \sum_{m=1}^{n_{i_1}} \text{sgn}(v_m^{i_1}) \frac{1 - \text{sgn}(\delta_m^{i_1})}{2} + \sum_{m=1}^{n_{l_1}} \text{sgn}(v_m^{l_1}) \frac{1 - \text{sgn}(\delta_m^{l_1})}{2} \tag{S25.3}$$

$$\mathcal{W}_4^{\text{gapless}} = \sum_{m=1}^{n_{b_2}} \text{sgn}(v_m^{b_2}) \frac{1 - \text{sgn}(\delta_m^{b_2})}{2} - \sum_{m=1}^{n_{f_2}} \text{sgn}(v_m^{f_2}) \frac{1 - \text{sgn}(\delta_m^{f_2})}{2} - \sum_{m=1}^{n_{i_1}} \text{sgn}(v_m^{i_1}) \frac{1 - \text{sgn}(\delta_m^{i_1})}{2} + \sum_{m=1}^{n_{l_1}} \text{sgn}(v_m^{l_1}) \frac{1 - \text{sgn}(\delta_m^{l_1})}{2} \tag{S25.4}$$

$$\mathcal{W}_5^{\text{gapless}} = \sum_{m=1}^{n_{c_1}} \text{sgn}(v_m^{c_1}) \frac{1 - \text{sgn}(\delta_m^{c_1})}{2} - \sum_{m=1}^{n_{g_1}} \text{sgn}(v_m^{g_1}) \frac{1 - \text{sgn}(\delta_m^{g_1})}{2} - \sum_{m=1}^{n_{j_1}} \text{sgn}(v_m^{j_1}) \frac{1 - \text{sgn}(\delta_m^{j_1})}{2} + \sum_{m=1}^{n_{k_1}} \text{sgn}(v_m^{k_1}) \frac{1 - \text{sgn}(\delta_m^{k_1})}{2} \tag{S25.5}$$

$$\mathcal{W}_6^{\text{gapless}} = \sum_{m=1}^{n_{c_2}} \text{sgn}(v_m^{c_2}) \frac{1 - \text{sgn}(\delta_m^{c_2})}{2} - \sum_{m=1}^{n_{g_2}} \text{sgn}(v_m^{g_2}) \frac{1 - \text{sgn}(\delta_m^{g_2})}{2} - \sum_{m=1}^{n_{j_1}} \text{sgn}(v_m^{j_1}) \frac{1 - \text{sgn}(\delta_m^{j_1})}{2} + \sum_{m=1}^{n_{k_1}} \text{sgn}(v_m^{k_1}) \frac{1 - \text{sgn}(\delta_m^{k_1})}{2} \tag{S25.6}$$

$$\mathcal{W}_7^{\text{gapless}} = \sum_{m=1}^{n_{d_1}} \text{sgn}(v_m^{d_1}) \frac{1 - \text{sgn}(\delta_m^{d_1})}{2} - \sum_{m=1}^{n_{h_1}} \text{sgn}(v_m^{h_1}) \frac{1 - \text{sgn}(\delta_m^{h_1})}{2} - \sum_{m=1}^{n_{k_1}} \text{sgn}(v_m^{k_1}) \frac{1 - \text{sgn}(\delta_m^{k_1})}{2} + \sum_{m=1}^{n_{l_1}} \text{sgn}(v_m^{l_1}) \frac{1 - \text{sgn}(\delta_m^{l_1})}{2} \tag{S25.7}$$

$$\mathcal{W}_8^{\text{gapless}} = \sum_{m=1}^{n_{d_2}} \text{sgn}(v_m^{d_2}) \frac{1 - \text{sgn}(\delta_m^{d_2})}{2} - \sum_{m=1}^{n_{h_2}} \text{sgn}(v_m^{h_2}) \frac{1 - \text{sgn}(\delta_m^{h_2})}{2} - \sum_{m=1}^{n_{k_1}} \text{sgn}(v_m^{k_1}) \frac{1 - \text{sgn}(\delta_m^{k_1})}{2} + \sum_{m=1}^{n_{l_1}} \text{sgn}(v_m^{l_1}) \frac{1 - \text{sgn}(\delta_m^{l_1})}{2} \quad (\text{S25.8})$$

$$\begin{aligned} \mathcal{W}_9^{\text{gapless}} = & \sum_{m=1}^{n_{e_1}} \text{sgn}(v_m^{e_1}) \frac{1 - \text{sgn}(\delta_m^{e_1})}{2} + \sum_{m=1}^{n_{e_2}} \text{sgn}(v_m^{e_2}) \frac{1 - \text{sgn}(\delta_m^{e_2})}{2} - \sum_{m=1}^{n_{f_1}} \text{sgn}(v_m^{f_1}) \frac{1 - \text{sgn}(\delta_m^{f_1})}{2} \\ & - \sum_{m=1}^{n_{f_2}} \text{sgn}(v_m^{f_2}) \frac{1 - \text{sgn}(\delta_m^{f_2})}{2} + \sum_{m=1}^{n_{g_1}} \text{sgn}(v_m^{g_1}) \frac{1 - \text{sgn}(\delta_m^{g_1})}{2} + \sum_{m=1}^{n_{g_2}} \text{sgn}(v_m^{g_2}) \frac{1 - \text{sgn}(\delta_m^{g_2})}{2} \\ & + \sum_{m=1}^{n_{h_1}} \text{sgn}(v_m^{h_1}) \frac{1 - \text{sgn}(\delta_m^{h_1})}{2} + \sum_{m=1}^{n_{h_2}} \text{sgn}(v_m^{h_2}) \frac{1 - \text{sgn}(\delta_m^{h_2})}{2} \end{aligned} \quad (\text{S25.9})$$

$$\mathcal{W}_1^{\text{gapped}} = \sum_{m=1}^{n_{h_1}} \text{sgn}(v_m^{h_1}) \frac{1 - \text{sgn}(\delta_m^{h_1})}{2} - \sum_{m=1}^{n_{h_2}} \text{sgn}(v_m^{h_2}) \frac{1 - \text{sgn}(\delta_m^{h_2})}{2} \quad (\text{S25.10})$$

$$\begin{aligned} \mathcal{W}_2^{\text{gapped}} = & - \sum_{m=1}^{n_{e_2}} \text{sgn}(v_m^{e_2}) \frac{1 - \text{sgn}(\delta_m^{e_2})}{2} + \sum_{m=1}^{n_{f_1}} \text{sgn}(v_m^{f_1}) \frac{1 - \text{sgn}(\delta_m^{f_1})}{2} - \sum_{m=1}^{n_{g_2}} \text{sgn}(v_m^{g_2}) \frac{1 - \text{sgn}(\delta_m^{g_2})}{2} \\ & - \sum_{m=1}^{n_{h_2}} \text{sgn}(v_m^{h_2}) \frac{1 - \text{sgn}(\delta_m^{h_2})}{2} \end{aligned} \quad (\text{S25.11})$$

$$\begin{aligned} \mathcal{W}_3^{\text{gapped}} = & - \sum_{m=1}^{n_{e_2}} \text{sgn}(v_m^{e_2}) \frac{1 - \text{sgn}(\delta_m^{e_2})}{2} + \sum_{m=1}^{n_{f_2}} \text{sgn}(v_m^{f_2}) \frac{1 - \text{sgn}(\delta_m^{f_2})}{2} - \sum_{m=1}^{n_{g_2}} \text{sgn}(v_m^{g_2}) \frac{1 - \text{sgn}(\delta_m^{g_2})}{2} \\ & - \sum_{m=1}^{n_{h_2}} \text{sgn}(v_m^{h_2}) \frac{1 - \text{sgn}(\delta_m^{h_2})}{2} \end{aligned} \quad (\text{S25.12})$$

$$\mathcal{W}_4^{\text{gapped}} = \sum_{m=1}^{n_{g_1}} \text{sgn}(v_m^{g_1}) \frac{1 - \text{sgn}(\delta_m^{g_1})}{2} - \sum_{m=1}^{n_{g_2}} \text{sgn}(v_m^{g_2}) \frac{1 - \text{sgn}(\delta_m^{g_2})}{2} \quad (\text{S25.13})$$

## S26. SPACE GROUP NO. 26

| line segment                              | character of irrep (generators only)                                   |
|-------------------------------------------|------------------------------------------------------------------------|
| $a \quad (\frac{t}{2}, 0, 0)$             | $\{m_{010}   0 \ 0 \ \frac{1}{2}\}$<br>$a_1 \quad -i$<br>$a_2 \quad i$ |
| $b \quad (0, \frac{t}{2}, 0)$             | $\{m_{100}   0 \ 0 \ 0\}$<br>$b_1 \quad -i$<br>$b_2 \quad i$           |
| $c \quad (\frac{1}{2}, \frac{t}{2}, 0)$   | $\{m_{100}   0 \ 0 \ 0\}$<br>$c_1 \quad -i$<br>$c_2 \quad i$           |
| $d \quad (\frac{1-t}{2}, \frac{1}{2}, 0)$ | $\{m_{010}   0 \ 0 \ \frac{1}{2}\}$<br>$d_1 \quad -i$<br>$d_2 \quad i$ |

|                                                     |                                                                                            |
|-----------------------------------------------------|--------------------------------------------------------------------------------------------|
| $e \quad (\frac{t}{2}, 0, \frac{1}{2})$             | $\{m_{010}   0 \ 0 \ \frac{1}{2}\}$<br>$e_1 \quad -1$<br>$e_2 \quad 1$                     |
| $f \quad (0, \frac{t}{2}, \frac{1}{2})$             | $\{m_{100}   0 \ 0 \ 0\}$<br>$f_1 \quad -i$<br>$f_2 \quad i$                               |
| $g \quad (\frac{1}{2}, \frac{t}{2}, \frac{1}{2})$   | $\{m_{100}   0 \ 0 \ 0\}$<br>$g_1 \quad -i$<br>$g_2 \quad i$                               |
| $h \quad (\frac{1-t}{2}, \frac{1}{2}, \frac{1}{2})$ | $\{m_{010}   0 \ 0 \ \frac{1}{2}\}$<br>$h_1 \quad -1$<br>$h_2 \quad 1$                     |
| $i \quad (0, 0, \frac{t}{2})$                       | $\{2_{001}   0 \ 0 \ \frac{1}{2}\} \quad \{m_{100}   0 \ 0 \ 0\}$<br>$i_1 \quad 0 \quad 0$ |
| $j \quad (\frac{1}{2}, 0, \frac{t}{2})$             | $\{2_{001}   0 \ 0 \ \frac{1}{2}\} \quad \{m_{100}   0 \ 0 \ 0\}$<br>$j_1 \quad 0 \quad 0$ |
| $k \quad (\frac{1}{2}, \frac{1}{2}, \frac{t}{2})$   | $\{2_{001}   0 \ 0 \ \frac{1}{2}\} \quad \{m_{100}   0 \ 0 \ 0\}$<br>$k_1 \quad 0 \quad 0$ |
| $l \quad (0, \frac{1}{2}, \frac{t}{2})$             | $\{2_{001}   0 \ 0 \ \frac{1}{2}\} \quad \{m_{100}   0 \ 0 \ 0\}$<br>$l_1 \quad 0 \quad 0$ |

$$\begin{aligned}
\mathcal{W}_1^{\text{gapless}} = & \sum_{m=1}^{n_{a_1}} \text{sgn}(v_m^{a_1}) \frac{1 - \text{sgn}(\delta_m^{a_1})}{2} - \sum_{m=1}^{n_{f_1}} \text{sgn}(v_m^{f_1}) \frac{1 - \text{sgn}(\delta_m^{f_1})}{2} - \sum_{m=1}^{n_{f_2}} \text{sgn}(v_m^{f_2}) \frac{1 - \text{sgn}(\delta_m^{f_2})}{2} \\
& + \sum_{m=1}^{n_{g_1}} \text{sgn}(v_m^{g_1}) \frac{1 - \text{sgn}(\delta_m^{g_1})}{2} + \sum_{m=1}^{n_{g_2}} \text{sgn}(v_m^{g_2}) \frac{1 - \text{sgn}(\delta_m^{g_2})}{2} \\
& + \sum_{m=1}^{n_{h_1}} \text{sgn}(v_m^{h_1}) \frac{1 - \text{sgn}(\delta_m^{h_1})}{2} - \sum_{m=1}^{n_{i_1}} \text{sgn}(v_m^{i_1}) \frac{1 - \text{sgn}(\delta_m^{i_1})}{2} + \sum_{m=1}^{n_{j_1}} \text{sgn}(v_m^{j_1}) \frac{1 - \text{sgn}(\delta_m^{j_1})}{2}
\end{aligned} \tag{S26.1}$$

$$\begin{aligned}
\mathcal{W}_2^{\text{gapless}} = & \sum_{m=1}^{n_{a_2}} \text{sgn}(v_m^{a_2}) \frac{1 - \text{sgn}(\delta_m^{a_2})}{2} - \sum_{m=1}^{n_{f_1}} \text{sgn}(v_m^{f_1}) \frac{1 - \text{sgn}(\delta_m^{f_1})}{2} - \sum_{m=1}^{n_{f_2}} \text{sgn}(v_m^{f_2}) \frac{1 - \text{sgn}(\delta_m^{f_2})}{2} \\
& + \sum_{m=1}^{n_{g_1}} \text{sgn}(v_m^{g_1}) \frac{1 - \text{sgn}(\delta_m^{g_1})}{2} + \sum_{m=1}^{n_{g_2}} \text{sgn}(v_m^{g_2}) \frac{1 - \text{sgn}(\delta_m^{g_2})}{2} \\
& + \sum_{m=1}^{n_{h_1}} \text{sgn}(v_m^{h_1}) \frac{1 - \text{sgn}(\delta_m^{h_1})}{2} - \sum_{m=1}^{n_{i_1}} \text{sgn}(v_m^{i_1}) \frac{1 - \text{sgn}(\delta_m^{i_1})}{2} + \sum_{m=1}^{n_{j_1}} \text{sgn}(v_m^{j_1}) \frac{1 - \text{sgn}(\delta_m^{j_1})}{2}
\end{aligned} \tag{S26.2}$$

$$\mathcal{W}_3^{\text{gapless}} = \sum_{m=1}^{n_{b_1}} \text{sgn}(v_m^{b_1}) \frac{1 - \text{sgn}(\delta_m^{b_1})}{2} - 2 \sum_{m=1}^{n_{f_1}} \text{sgn}(v_m^{f_1}) \frac{1 - \text{sgn}(\delta_m^{f_1})}{2} - \sum_{m=1}^{n_{i_1}} \text{sgn}(v_m^{i_1}) \frac{1 - \text{sgn}(\delta_m^{i_1})}{2} + \sum_{m=1}^{n_{l_1}} \text{sgn}(v_m^{l_1}) \frac{1 - \text{sgn}(\delta_m^{l_1})}{2} \tag{S26.3}$$

$$\mathcal{W}_4^{\text{gapless}} = \sum_{m=1}^{n_{b_2}} \text{sgn}(v_m^{b_2}) \frac{1 - \text{sgn}(\delta_m^{b_2})}{2} - 2 \sum_{m=1}^{n_{f_2}} \text{sgn}(v_m^{f_2}) \frac{1 - \text{sgn}(\delta_m^{f_2})}{2} - \sum_{m=1}^{n_{i_1}} \text{sgn}(v_m^{i_1}) \frac{1 - \text{sgn}(\delta_m^{i_1})}{2} + \sum_{m=1}^{n_{l_1}} \text{sgn}(v_m^{l_1}) \frac{1 - \text{sgn}(\delta_m^{l_1})}{2} \tag{S26.4}$$

$$\mathcal{W}_5^{\text{gapless}} = \sum_{m=1}^{n_{c_1}} \text{sgn}(v_m^{c_1}) \frac{1 - \text{sgn}(\delta_m^{c_1})}{2} - 2 \sum_{m=1}^{n_{g_1}} \text{sgn}(v_m^{g_1}) \frac{1 - \text{sgn}(\delta_m^{g_1})}{2} - \sum_{m=1}^{n_{j_1}} \text{sgn}(v_m^{j_1}) \frac{1 - \text{sgn}(\delta_m^{j_1})}{2} + \sum_{m=1}^{n_{k_1}} \text{sgn}(v_m^{k_1}) \frac{1 - \text{sgn}(\delta_m^{k_1})}{2} \tag{S26.5}$$

$$\mathcal{W}_6^{\text{gapless}} = \sum_{m=1}^{n_{c_2}} \text{sgn}(v_m^{c_2}) \frac{1 - \text{sgn}(\delta_m^{c_2})}{2} - 2 \sum_{m=1}^{n_{g_2}} \text{sgn}(v_m^{g_2}) \frac{1 - \text{sgn}(\delta_m^{g_2})}{2} - \sum_{m=1}^{n_{j_1}} \text{sgn}(v_m^{j_1}) \frac{1 - \text{sgn}(\delta_m^{j_1})}{2} + \sum_{m=1}^{n_{k_1}} \text{sgn}(v_m^{k_1}) \frac{1 - \text{sgn}(\delta_m^{k_1})}{2} \quad (\text{S26.6})$$

$$\mathcal{W}_7^{\text{gapless}} = \sum_{m=1}^{n_{d_1}} \text{sgn}(v_m^{d_1}) \frac{1 - \text{sgn}(\delta_m^{d_1})}{2} - \sum_{m=1}^{n_{h_1}} \text{sgn}(v_m^{h_1}) \frac{1 - \text{sgn}(\delta_m^{h_1})}{2} - \sum_{m=1}^{n_{k_1}} \text{sgn}(v_m^{k_1}) \frac{1 - \text{sgn}(\delta_m^{k_1})}{2} + \sum_{m=1}^{n_{l_1}} \text{sgn}(v_m^{l_1}) \frac{1 - \text{sgn}(\delta_m^{l_1})}{2} \quad (\text{S26.7})$$

$$\mathcal{W}_8^{\text{gapless}} = \sum_{m=1}^{n_{d_2}} \text{sgn}(v_m^{d_2}) \frac{1 - \text{sgn}(\delta_m^{d_2})}{2} - \sum_{m=1}^{n_{h_1}} \text{sgn}(v_m^{h_1}) \frac{1 - \text{sgn}(\delta_m^{h_1})}{2} - \sum_{m=1}^{n_{k_1}} \text{sgn}(v_m^{k_1}) \frac{1 - \text{sgn}(\delta_m^{k_1})}{2} + \sum_{m=1}^{n_{l_1}} \text{sgn}(v_m^{l_1}) \frac{1 - \text{sgn}(\delta_m^{l_1})}{2} \quad (\text{S26.8})$$

$$\begin{aligned} \mathcal{W}_9^{\text{gapless}} = & \sum_{m=1}^{n_{e_1}} \text{sgn}(v_m^{e_1}) \frac{1 - \text{sgn}(\delta_m^{e_1})}{2} - \sum_{m=1}^{n_{f_1}} \text{sgn}(v_m^{f_1}) \frac{1 - \text{sgn}(\delta_m^{f_1})}{2} - \sum_{m=1}^{n_{f_2}} \text{sgn}(v_m^{f_2}) \frac{1 - \text{sgn}(\delta_m^{f_2})}{2} \\ & + \sum_{m=1}^{n_{g_1}} \text{sgn}(v_m^{g_1}) \frac{1 - \text{sgn}(\delta_m^{g_1})}{2} + \sum_{m=1}^{n_{g_2}} \text{sgn}(v_m^{g_2}) \frac{1 - \text{sgn}(\delta_m^{g_2})}{2} + \sum_{m=1}^{n_{h_1}} \text{sgn}(v_m^{h_1}) \frac{1 - \text{sgn}(\delta_m^{h_1})}{2} \end{aligned} \quad (\text{S26.9})$$

$$\mathcal{W}_1^{\text{gapped}} = - \sum_{m=1}^{n_{f_1}} \text{sgn}(v_m^{f_1}) \frac{1 - \text{sgn}(\delta_m^{f_1})}{2} + \sum_{m=1}^{n_{f_2}} \text{sgn}(v_m^{f_2}) \frac{1 - \text{sgn}(\delta_m^{f_2})}{2} \quad (\text{S26.10})$$

$$\mathcal{W}_2^{\text{gapped}} = - \sum_{m=1}^{n_{g_1}} \text{sgn}(v_m^{g_1}) \frac{1 - \text{sgn}(\delta_m^{g_1})}{2} + \sum_{m=1}^{n_{g_2}} \text{sgn}(v_m^{g_2}) \frac{1 - \text{sgn}(\delta_m^{g_2})}{2} \quad (\text{S26.11})$$

$$\mathcal{X}_1 = \sum_{m=1}^{n_{h_1}} \frac{1 - \text{sgn}(\delta_m^{h_1})}{2} \quad \text{mod } 2 \quad (\text{S26.12})$$

## S27. SPACE GROUP NO. 27

| line segment                              | character of irrep (generators only)                                   |
|-------------------------------------------|------------------------------------------------------------------------|
| $a \quad (\frac{t}{2}, 0, 0)$             | $\{m_{010}   0 \ 0 \ \frac{1}{2}\}$<br>$a_1 \quad -i$<br>$a_2 \quad i$ |
| $b \quad (0, \frac{t}{2}, 0)$             | $\{m_{100}   0 \ 0 \ \frac{1}{2}\}$<br>$b_1 \quad -i$<br>$b_2 \quad i$ |
| $c \quad (\frac{1}{2}, \frac{t}{2}, 0)$   | $\{m_{100}   0 \ 0 \ \frac{1}{2}\}$<br>$c_1 \quad -i$<br>$c_2 \quad i$ |
| $d \quad (\frac{1-t}{2}, \frac{1}{2}, 0)$ | $\{m_{010}   0 \ 0 \ \frac{1}{2}\}$<br>$d_1 \quad -i$<br>$d_2 \quad i$ |

|                                                     |                                                                                            |
|-----------------------------------------------------|--------------------------------------------------------------------------------------------|
| $e \quad (\frac{t}{2}, 0, \frac{1}{2})$             | $\{m_{010}   0 \ 0 \ \frac{1}{2}\}$<br>$e_1 \quad -1$<br>$e_2 \quad 1$                     |
| $f \quad (0, \frac{t}{2}, \frac{1}{2})$             | $\{m_{100}   0 \ 0 \ \frac{1}{2}\}$<br>$f_1 \quad -1$<br>$f_2 \quad 1$                     |
| $g \quad (\frac{1}{2}, \frac{t}{2}, \frac{1}{2})$   | $\{m_{100}   0 \ 0 \ \frac{1}{2}\}$<br>$g_1 \quad -1$<br>$g_2 \quad 1$                     |
| $h \quad (\frac{1-t}{2}, \frac{1}{2}, \frac{1}{2})$ | $\{m_{010}   0 \ 0 \ \frac{1}{2}\}$<br>$h_1 \quad -1$<br>$h_2 \quad 1$                     |
| $i \quad (0, 0, \frac{t}{2})$                       | $\{2_{001}   0 \ 0 \ 0\} \quad \{m_{100}   0 \ 0 \ \frac{1}{2}\}$<br>$i_1 \quad 0 \quad 0$ |
| $j \quad (\frac{1}{2}, 0, \frac{t}{2})$             | $\{2_{001}   0 \ 0 \ 0\} \quad \{m_{100}   0 \ 0 \ \frac{1}{2}\}$<br>$j_1 \quad 0 \quad 0$ |
| $k \quad (\frac{1}{2}, \frac{1}{2}, \frac{t}{2})$   | $\{2_{001}   0 \ 0 \ 0\} \quad \{m_{100}   0 \ 0 \ \frac{1}{2}\}$<br>$k_1 \quad 0 \quad 0$ |
| $l \quad (0, \frac{1}{2}, \frac{t}{2})$             | $\{2_{001}   0 \ 0 \ 0\} \quad \{m_{100}   0 \ 0 \ \frac{1}{2}\}$<br>$l_1 \quad 0 \quad 0$ |

$$\begin{aligned}
\mathcal{W}_1^{\text{gapless}} = & \sum_{m=1}^{n_{a_1}} \text{sgn}(v_m^{a_1}) \frac{1 - \text{sgn}(\delta_m^{a_1})}{2} + \sum_{m=1}^{n_{e_1}} \text{sgn}(v_m^{e_1}) \frac{1 - \text{sgn}(\delta_m^{e_1})}{2} - 2 \sum_{m=1}^{n_{f_1}} \text{sgn}(v_m^{f_1}) \frac{1 - \text{sgn}(\delta_m^{f_1})}{2} \\
& + 2 \sum_{m=1}^{n_{g_1}} \text{sgn}(v_m^{g_1}) \frac{1 - \text{sgn}(\delta_m^{g_1})}{2} + 2 \sum_{m=1}^{n_{h_1}} \text{sgn}(v_m^{h_1}) \frac{1 - \text{sgn}(\delta_m^{h_1})}{2} - \sum_{m=1}^{n_{i_1}} \text{sgn}(v_m^{i_1}) \frac{1 - \text{sgn}(\delta_m^{i_1})}{2} \\
& + \sum_{m=1}^{n_{j_1}} \text{sgn}(v_m^{j_1}) \frac{1 - \text{sgn}(\delta_m^{j_1})}{2}
\end{aligned} \tag{S27.1}$$

$$\begin{aligned}
\mathcal{W}_2^{\text{gapless}} = & \sum_{m=1}^{n_{a_2}} \text{sgn}(v_m^{a_2}) \frac{1 - \text{sgn}(\delta_m^{a_2})}{2} + \sum_{m=1}^{n_{e_1}} \text{sgn}(v_m^{e_1}) \frac{1 - \text{sgn}(\delta_m^{e_1})}{2} - 2 \sum_{m=1}^{n_{f_1}} \text{sgn}(v_m^{f_1}) \frac{1 - \text{sgn}(\delta_m^{f_1})}{2} \\
& + 2 \sum_{m=1}^{n_{g_1}} \text{sgn}(v_m^{g_1}) \frac{1 - \text{sgn}(\delta_m^{g_1})}{2} + 2 \sum_{m=1}^{n_{h_1}} \text{sgn}(v_m^{h_1}) \frac{1 - \text{sgn}(\delta_m^{h_1})}{2} - \sum_{m=1}^{n_{i_1}} \text{sgn}(v_m^{i_1}) \frac{1 - \text{sgn}(\delta_m^{i_1})}{2} \\
& + \sum_{m=1}^{n_{j_1}} \text{sgn}(v_m^{j_1}) \frac{1 - \text{sgn}(\delta_m^{j_1})}{2}
\end{aligned} \tag{S27.2}$$

$$\mathcal{W}_3^{\text{gapless}} = \sum_{m=1}^{n_{b_1}} \text{sgn}(v_m^{b_1}) \frac{1 - \text{sgn}(\delta_m^{b_1})}{2} - \sum_{m=1}^{n_{f_1}} \text{sgn}(v_m^{f_1}) \frac{1 - \text{sgn}(\delta_m^{f_1})}{2} - \sum_{m=1}^{n_{i_1}} \text{sgn}(v_m^{i_1}) \frac{1 - \text{sgn}(\delta_m^{i_1})}{2} + \sum_{m=1}^{n_{l_1}} \text{sgn}(v_m^{l_1}) \frac{1 - \text{sgn}(\delta_m^{l_1})}{2} \tag{S27.3}$$

$$\mathcal{W}_4^{\text{gapless}} = \sum_{m=1}^{n_{b_2}} \text{sgn}(v_m^{b_2}) \frac{1 - \text{sgn}(\delta_m^{b_2})}{2} - \sum_{m=1}^{n_{f_1}} \text{sgn}(v_m^{f_1}) \frac{1 - \text{sgn}(\delta_m^{f_1})}{2} - \sum_{m=1}^{n_{i_1}} \text{sgn}(v_m^{i_1}) \frac{1 - \text{sgn}(\delta_m^{i_1})}{2} + \sum_{m=1}^{n_{l_1}} \text{sgn}(v_m^{l_1}) \frac{1 - \text{sgn}(\delta_m^{l_1})}{2} \tag{S27.4}$$

$$\mathcal{W}_5^{\text{gapless}} = \sum_{m=1}^{n_{c_1}} \text{sgn}(v_m^{c_1}) \frac{1 - \text{sgn}(\delta_m^{c_1})}{2} - \sum_{m=1}^{n_{g_1}} \text{sgn}(v_m^{g_1}) \frac{1 - \text{sgn}(\delta_m^{g_1})}{2} - \sum_{m=1}^{n_{j_1}} \text{sgn}(v_m^{j_1}) \frac{1 - \text{sgn}(\delta_m^{j_1})}{2} + \sum_{m=1}^{n_{k_1}} \text{sgn}(v_m^{k_1}) \frac{1 - \text{sgn}(\delta_m^{k_1})}{2} \tag{S27.5}$$



$$\mathcal{W}_6^{\text{gapless}} = \sum_{m=1}^{n_{c_2}} \text{sgn}(v_m^{c_2}) \frac{1 - \text{sgn}(\delta_m^{c_2})}{2} - \sum_{m=1}^{n_{g_1}} \text{sgn}(v_m^{g_1}) \frac{1 - \text{sgn}(\delta_m^{g_1})}{2} - \sum_{m=1}^{n_{j_1}} \text{sgn}(v_m^{j_1}) \frac{1 - \text{sgn}(\delta_m^{j_1})}{2} + \sum_{m=1}^{n_{k_1}} \text{sgn}(v_m^{k_1}) \frac{1 - \text{sgn}(\delta_m^{k_1})}{2} \quad (\text{S27.6})$$

$$\mathcal{W}_7^{\text{gapless}} = \sum_{m=1}^{n_{d_1}} \text{sgn}(v_m^{d_1}) \frac{1 - \text{sgn}(\delta_m^{d_1})}{2} - \sum_{m=1}^{n_{h_1}} \text{sgn}(v_m^{h_1}) \frac{1 - \text{sgn}(\delta_m^{h_1})}{2} - \sum_{m=1}^{n_{k_1}} \text{sgn}(v_m^{k_1}) \frac{1 - \text{sgn}(\delta_m^{k_1})}{2} + \sum_{m=1}^{n_{l_1}} \text{sgn}(v_m^{l_1}) \frac{1 - \text{sgn}(\delta_m^{l_1})}{2} \quad (\text{S27.7})$$

$$\mathcal{W}_8^{\text{gapless}} = \sum_{m=1}^{n_{d_2}} \text{sgn}(v_m^{d_2}) \frac{1 - \text{sgn}(\delta_m^{d_2})}{2} - \sum_{m=1}^{n_{h_1}} \text{sgn}(v_m^{h_1}) \frac{1 - \text{sgn}(\delta_m^{h_1})}{2} - \sum_{m=1}^{n_{k_1}} \text{sgn}(v_m^{k_1}) \frac{1 - \text{sgn}(\delta_m^{k_1})}{2} + \sum_{m=1}^{n_{l_1}} \text{sgn}(v_m^{l_1}) \frac{1 - \text{sgn}(\delta_m^{l_1})}{2} \quad (\text{S27.8})$$

$$\mathcal{W}_9^{\text{gapless}} = \sum_{m=1}^{n_{e_1}} \text{sgn}(v_m^{e_1}) \frac{1 - \text{sgn}(\delta_m^{e_1})}{2} - \sum_{m=1}^{n_{f_1}} \text{sgn}(v_m^{f_1}) \frac{1 - \text{sgn}(\delta_m^{f_1})}{2} + \sum_{m=1}^{n_{g_1}} \text{sgn}(v_m^{g_1}) \frac{1 - \text{sgn}(\delta_m^{g_1})}{2} + \sum_{m=1}^{n_{h_1}} \text{sgn}(v_m^{h_1}) \frac{1 - \text{sgn}(\delta_m^{h_1})}{2} \quad (\text{S27.9})$$

$$\mathcal{X}_1 = \sum_{m=1}^{n_{f_1}} \frac{1 - \text{sgn}(\delta_m^{f_1})}{2} \quad \text{mod } 2 \quad (\text{S27.10})$$

$$\mathcal{X}_2 = \sum_{m=1}^{n_{g_1}} \frac{1 - \text{sgn}(\delta_m^{g_1})}{2} + \sum_{m=1}^{n_{h_1}} \frac{1 - \text{sgn}(\delta_m^{h_1})}{2} \quad \text{mod } 2 \quad (\text{S27.11})$$

$$\mathcal{X}_3 = \sum_{m=1}^{n_{h_1}} \frac{1 - \text{sgn}(\delta_m^{h_1})}{2} \quad \text{mod } 2 \quad (\text{S27.12})$$

## S28. SPACE GROUP NO. 28

| line segment                              | character of irrep (generators only)                                                                                     |
|-------------------------------------------|--------------------------------------------------------------------------------------------------------------------------|
| $a \quad (\frac{t}{2}, 0, 0)$             | $\{m_{010}   \frac{1}{2} \ 0 \ 0\}$<br>$a_1 \quad -ie^{-\frac{1}{2}i\pi t}$<br>$a_2 \quad ie^{-\frac{1}{2}i\pi t}$       |
| $b \quad (0, \frac{t}{2}, 0)$             | $\{m_{100}   \frac{1}{2} \ 0 \ 0\}$<br>$b_1 \quad -i$<br>$b_2 \quad i$                                                   |
| $c \quad (\frac{1}{2}, \frac{t}{2}, 0)$   | $\{m_{100}   \frac{1}{2} \ 0 \ 0\}$<br>$c_1 \quad i$<br>$c_2 \quad -i$                                                   |
| $d \quad (\frac{1-t}{2}, \frac{1}{2}, 0)$ | $\{m_{010}   \frac{1}{2} \ 0 \ 0\}$<br>$d_1 \quad -ie^{-\frac{1}{2}i\pi(1-t)}$<br>$d_2 \quad ie^{-\frac{1}{2}i\pi(1-t)}$ |
| $e \quad (\frac{t}{2}, 0, \frac{1}{2})$   | $\{m_{010}   \frac{1}{2} \ 0 \ 0\}$<br>$e_1 \quad -ie^{-\frac{1}{2}i\pi t}$<br>$e_2 \quad ie^{-\frac{1}{2}i\pi t}$       |

|                                                     |                                                                                                                                                                     |
|-----------------------------------------------------|---------------------------------------------------------------------------------------------------------------------------------------------------------------------|
| $f \quad (0, \frac{t}{2}, \frac{1}{2})$             | $\begin{matrix} \{m_{100}   \frac{1}{2} & 0 & 0 \} \\ f_1 & -i \\ f_2 & i \end{matrix}$                                                                             |
| $g \quad (\frac{1}{2}, \frac{t}{2}, \frac{1}{2})$   | $\begin{matrix} \{m_{100}   \frac{1}{2} & 0 & 0 \} \\ g_1 & i \\ g_2 & -i \end{matrix}$                                                                             |
| $h \quad (\frac{1-t}{2}, \frac{1}{2}, \frac{1}{2})$ | $\begin{matrix} \{m_{010}   \frac{1}{2} & 0 & 0 \} \\ h_1 & -ie^{-\frac{1}{2}i\pi(1-t)} \\ h_2 & ie^{-\frac{1}{2}i\pi(1-t)} \end{matrix}$                           |
| $i \quad (0, 0, \frac{t}{2})$                       | $\begin{matrix} \{2_{001}   0 & 0 & 0 \} & \{m_{100}   \frac{1}{2} & 0 & 0 \} \\ i_1 & 0 & & 0 \end{matrix}$                                                        |
| $j \quad (\frac{1}{2}, 0, \frac{t}{2})$             | $\begin{matrix} \{2_{001}   0 & 0 & 0 \} & \{m_{100}   \frac{1}{2} & 0 & 0 \} \\ j_1 & -i & & i \\ j_2 & -i & & -i \\ j_3 & i & & i \\ j_4 & i & & -i \end{matrix}$ |
| $k \quad (\frac{1}{2}, \frac{1}{2}, \frac{t}{2})$   | $\begin{matrix} \{2_{001}   0 & 0 & 0 \} & \{m_{100}   \frac{1}{2} & 0 & 0 \} \\ k_1 & -i & & i \\ k_2 & -i & & -i \\ k_3 & i & & i \\ k_4 & i & & -i \end{matrix}$ |
| $l \quad (0, \frac{1}{2}, \frac{t}{2})$             | $\begin{matrix} \{2_{001}   0 & 0 & 0 \} & \{m_{100}   \frac{1}{2} & 0 & 0 \} \\ l_1 & 0 & & 0 \end{matrix}$                                                        |

$$\begin{aligned}
\mathcal{W}_1^{\text{gapless}} = & \sum_{m=1}^{n_{a_1}} \text{sgn}(v_m^{a_1}) \frac{1 - \text{sgn}(\delta_m^{a_1})}{2} + \sum_{m=1}^{n_{e_2}} \text{sgn}(v_m^{e_2}) \frac{1 - \text{sgn}(\delta_m^{e_2})}{2} - \sum_{m=1}^{n_{f_1}} \text{sgn}(v_m^{f_1}) \frac{1 - \text{sgn}(\delta_m^{f_1})}{2} \\
& - \sum_{m=1}^{n_{f_2}} \text{sgn}(v_m^{f_2}) \frac{1 - \text{sgn}(\delta_m^{f_2})}{2} + 2 \sum_{m=1}^{n_{g_1}} \text{sgn}(v_m^{g_1}) \frac{1 - \text{sgn}(\delta_m^{g_1})}{2} + \sum_{m=1}^{n_{h_1}} \text{sgn}(v_m^{h_1}) \frac{1 - \text{sgn}(\delta_m^{h_1})}{2} \\
& + \sum_{m=1}^{n_{h_2}} \text{sgn}(v_m^{h_2}) \frac{1 - \text{sgn}(\delta_m^{h_2})}{2} - \sum_{m=1}^{n_{i_1}} \text{sgn}(v_m^{i_1}) \frac{1 - \text{sgn}(\delta_m^{i_1})}{2} + \sum_{m=1}^{n_{j_2}} \text{sgn}(v_m^{j_2}) \frac{1 - \text{sgn}(\delta_m^{j_2})}{2} \\
& - \sum_{m=1}^{n_{j_3}} \text{sgn}(v_m^{j_3}) \frac{1 - \text{sgn}(\delta_m^{j_3})}{2} + 2 \sum_{m=1}^{n_{j_4}} \text{sgn}(v_m^{j_4}) \frac{1 - \text{sgn}(\delta_m^{j_4})}{2} + \sum_{m=1}^{n_{k_1}} \text{sgn}(v_m^{k_1}) \frac{1 - \text{sgn}(\delta_m^{k_1})}{2} \\
& - \sum_{m=1}^{n_{k_2}} \text{sgn}(v_m^{k_2}) \frac{1 - \text{sgn}(\delta_m^{k_2})}{2} + \sum_{m=1}^{n_{k_3}} \text{sgn}(v_m^{k_3}) \frac{1 - \text{sgn}(\delta_m^{k_3})}{2} - \sum_{m=1}^{n_{k_4}} \text{sgn}(v_m^{k_4}) \frac{1 - \text{sgn}(\delta_m^{k_4})}{2}
\end{aligned} \tag{S28.1}$$

$$\begin{aligned}
\mathcal{W}_2^{\text{gapless}} = & \sum_{m=1}^{n_{a_2}} \text{sgn}(v_m^{a_2}) \frac{1 - \text{sgn}(\delta_m^{a_2})}{2} - \sum_{m=1}^{n_{e_2}} \text{sgn}(v_m^{e_2}) \frac{1 - \text{sgn}(\delta_m^{e_2})}{2} - \sum_{m=1}^{n_{i_1}} \text{sgn}(v_m^{i_1}) \frac{1 - \text{sgn}(\delta_m^{i_1})}{2} \\
& + \sum_{m=1}^{n_{j_2}} \text{sgn}(v_m^{j_2}) \frac{1 - \text{sgn}(\delta_m^{j_2})}{2} + \sum_{m=1}^{n_{j_3}} \text{sgn}(v_m^{j_3}) \frac{1 - \text{sgn}(\delta_m^{j_3})}{2}
\end{aligned} \tag{S28.2}$$

$$\begin{aligned}
\mathcal{W}_3^{\text{gapless}} = & \sum_{m=1}^{n_{b_1}} \text{sgn}(v_m^{b_1}) \frac{1 - \text{sgn}(\delta_m^{b_1})}{2} - \sum_{m=1}^{n_{f_1}} \text{sgn}(v_m^{f_1}) \frac{1 - \text{sgn}(\delta_m^{f_1})}{2} - \sum_{m=1}^{n_{i_1}} \text{sgn}(v_m^{i_1}) \frac{1 - \text{sgn}(\delta_m^{i_1})}{2} + \sum_{m=1}^{n_{l_1}} \text{sgn}(v_m^{l_1}) \frac{1 - \text{sgn}(\delta_m^{l_1})}{2}
\end{aligned} \tag{S28.3}$$

$$\begin{aligned}
\mathcal{W}_4^{\text{gapless}} = & \sum_{m=1}^{n_{b_2}} \text{sgn}(v_m^{b_2}) \frac{1 - \text{sgn}(\delta_m^{b_2})}{2} - \sum_{m=1}^{n_{f_2}} \text{sgn}(v_m^{f_2}) \frac{1 - \text{sgn}(\delta_m^{f_2})}{2} - \sum_{m=1}^{n_{i_1}} \text{sgn}(v_m^{i_1}) \frac{1 - \text{sgn}(\delta_m^{i_1})}{2} + \sum_{m=1}^{n_{l_1}} \text{sgn}(v_m^{l_1}) \frac{1 - \text{sgn}(\delta_m^{l_1})}{2}
\end{aligned} \tag{S28.4}$$

$$\begin{aligned} \mathcal{W}_5^{\text{gapless}} = & \sum_{m=1}^{n_{c_1}} \text{sgn}(v_m^{c_1}) \frac{1 - \text{sgn}(\delta_m^{c_1})}{2} - \sum_{m=1}^{n_{g_1}} \text{sgn}(v_m^{g_1}) \frac{1 - \text{sgn}(\delta_m^{g_1})}{2} - \sum_{m=1}^{n_{j_2}} \text{sgn}(v_m^{j_2}) \frac{1 - \text{sgn}(\delta_m^{j_2})}{2} \\ & - \sum_{m=1}^{n_{j_4}} \text{sgn}(v_m^{j_4}) \frac{1 - \text{sgn}(\delta_m^{j_4})}{2} + \sum_{m=1}^{n_{k_2}} \text{sgn}(v_m^{k_2}) \frac{1 - \text{sgn}(\delta_m^{k_2})}{2} + \sum_{m=1}^{n_{k_4}} \text{sgn}(v_m^{k_4}) \frac{1 - \text{sgn}(\delta_m^{k_4})}{2} \end{aligned} \quad (\text{S28.5})$$

$$\begin{aligned} \mathcal{W}_6^{\text{gapless}} = & \sum_{m=1}^{n_{d_1}} \text{sgn}(v_m^{d_1}) \frac{1 - \text{sgn}(\delta_m^{d_1})}{2} - \sum_{m=1}^{n_{h_1}} \text{sgn}(v_m^{h_1}) \frac{1 - \text{sgn}(\delta_m^{h_1})}{2} - \sum_{m=1}^{n_{k_1}} \text{sgn}(v_m^{k_1}) \frac{1 - \text{sgn}(\delta_m^{k_1})}{2} \\ & - \sum_{m=1}^{n_{k_4}} \text{sgn}(v_m^{k_4}) \frac{1 - \text{sgn}(\delta_m^{k_4})}{2} + \sum_{m=1}^{n_{l_1}} \text{sgn}(v_m^{l_1}) \frac{1 - \text{sgn}(\delta_m^{l_1})}{2} \end{aligned} \quad (\text{S28.6})$$

$$\begin{aligned} \mathcal{W}_7^{\text{gapless}} = & \sum_{m=1}^{n_{d_2}} \text{sgn}(v_m^{d_2}) \frac{1 - \text{sgn}(\delta_m^{d_2})}{2} - \sum_{m=1}^{n_{h_2}} \text{sgn}(v_m^{h_2}) \frac{1 - \text{sgn}(\delta_m^{h_2})}{2} - \sum_{m=1}^{n_{k_2}} \text{sgn}(v_m^{k_2}) \frac{1 - \text{sgn}(\delta_m^{k_2})}{2} \\ & - \sum_{m=1}^{n_{k_3}} \text{sgn}(v_m^{k_3}) \frac{1 - \text{sgn}(\delta_m^{k_3})}{2} + \sum_{m=1}^{n_{l_1}} \text{sgn}(v_m^{l_1}) \frac{1 - \text{sgn}(\delta_m^{l_1})}{2} \end{aligned} \quad (\text{S28.7})$$

$$\begin{aligned} \mathcal{W}_8^{\text{gapless}} = & \sum_{m=1}^{n_{e_1}} \text{sgn}(v_m^{e_1}) \frac{1 - \text{sgn}(\delta_m^{e_1})}{2} + \sum_{m=1}^{n_{e_2}} \text{sgn}(v_m^{e_2}) \frac{1 - \text{sgn}(\delta_m^{e_2})}{2} - \sum_{m=1}^{n_{f_1}} \text{sgn}(v_m^{f_1}) \frac{1 - \text{sgn}(\delta_m^{f_1})}{2} - \sum_{m=1}^{n_{f_2}} \text{sgn}(v_m^{f_2}) \frac{1 - \text{sgn}(\delta_m^{f_2})}{2} \\ & + 2 \sum_{m=1}^{n_{g_1}} \text{sgn}(v_m^{g_1}) \frac{1 - \text{sgn}(\delta_m^{g_1})}{2} + \sum_{m=1}^{n_{h_1}} \text{sgn}(v_m^{h_1}) \frac{1 - \text{sgn}(\delta_m^{h_1})}{2} + \sum_{m=1}^{n_{h_2}} \text{sgn}(v_m^{h_2}) \frac{1 - \text{sgn}(\delta_m^{h_2})}{2} \end{aligned} \quad (\text{S28.8})$$

$$\begin{aligned} \mathcal{W}_9^{\text{gapless}} = & \sum_{m=1}^{n_{j_1}} \text{sgn}(v_m^{j_1}) \frac{1 - \text{sgn}(\delta_m^{j_1})}{2} - \sum_{m=1}^{n_{j_2}} \text{sgn}(v_m^{j_2}) \frac{1 - \text{sgn}(\delta_m^{j_2})}{2} + \sum_{m=1}^{n_{j_3}} \text{sgn}(v_m^{j_3}) \frac{1 - \text{sgn}(\delta_m^{j_3})}{2} \\ & - \sum_{m=1}^{n_{j_4}} \text{sgn}(v_m^{j_4}) \frac{1 - \text{sgn}(\delta_m^{j_4})}{2} - \sum_{m=1}^{n_{k_1}} \text{sgn}(v_m^{k_1}) \frac{1 - \text{sgn}(\delta_m^{k_1})}{2} + \sum_{m=1}^{n_{k_2}} \text{sgn}(v_m^{k_2}) \frac{1 - \text{sgn}(\delta_m^{k_2})}{2} \\ & - \sum_{m=1}^{n_{k_3}} \text{sgn}(v_m^{k_3}) \frac{1 - \text{sgn}(\delta_m^{k_3})}{2} + \sum_{m=1}^{n_{k_4}} \text{sgn}(v_m^{k_4}) \frac{1 - \text{sgn}(\delta_m^{k_4})}{2} \end{aligned} \quad (\text{S28.9})$$

$$\mathcal{W}_1^{\text{gapped}} = - \sum_{m=1}^{n_{j_2}} \text{sgn}(v_m^{j_2}) \frac{1 - \text{sgn}(\delta_m^{j_2})}{2} + \sum_{m=1}^{n_{j_3}} \text{sgn}(v_m^{j_3}) \frac{1 - \text{sgn}(\delta_m^{j_3})}{2} \quad (\text{S28.10})$$

$$\mathcal{W}_2^{\text{gapped}} = - \sum_{m=1}^{n_{k_2}} \text{sgn}(v_m^{k_2}) \frac{1 - \text{sgn}(\delta_m^{k_2})}{2} + \sum_{m=1}^{n_{k_3}} \text{sgn}(v_m^{k_3}) \frac{1 - \text{sgn}(\delta_m^{k_3})}{2} \quad (\text{S28.11})$$

$$\mathcal{W}_3^{\text{gapped}} = - \sum_{m=1}^{n_{k_1}} \text{sgn}(v_m^{k_1}) \frac{1 - \text{sgn}(\delta_m^{k_1})}{2} + \sum_{m=1}^{n_{k_4}} \text{sgn}(v_m^{k_4}) \frac{1 - \text{sgn}(\delta_m^{k_4})}{2} \quad (\text{S28.12})$$

$$\mathcal{W}_4^{\text{gapped}} = \sum_{m=1}^{n_{f_1}} \text{sgn}(v_m^{f_1}) \frac{1 - \text{sgn}(\delta_m^{f_1})}{2} - \sum_{m=1}^{n_{f_2}} \text{sgn}(v_m^{f_2}) \frac{1 - \text{sgn}(\delta_m^{f_2})}{2} \quad (\text{S28.13})$$

$$\mathcal{X}_1 = \sum_{m=1}^{n_{e_2}} \frac{1 - \text{sgn}(\delta_m^{e_2})}{2} + \sum_{m=1}^{n_{f_2}} \frac{1 - \text{sgn}(\delta_m^{f_2})}{2} + \sum_{m=1}^{n_{h_1}} \frac{1 - \text{sgn}(\delta_m^{h_1})}{2} \mod 2 \quad (\text{S28.14})$$

$$\mathcal{X}_2 = \sum_{m=1}^{n_{e_2}} \frac{1 - \text{sgn}(\delta_m^{e_2})}{2} + \sum_{m=1}^{n_{f_2}} \frac{1 - \text{sgn}(\delta_m^{f_2})}{2} + \sum_{m=1}^{n_{h_2}} \frac{1 - \text{sgn}(\delta_m^{h_2})}{2} \mod 2 \quad (\text{S28.15})$$

### S29. SPACE GROUP NO. 29

| line segment                                               | character of irrep (generators only) |                                                                                                                                              |
|------------------------------------------------------------|--------------------------------------|----------------------------------------------------------------------------------------------------------------------------------------------|
| $a \left( \frac{t}{2}, 0, 0 \right)$                       | $a_1$                                | $\{m_{010}   \frac{1}{2} \ 0 \ 0\}$<br>$-ie^{-\frac{1}{2}i\pi t}$                                                                            |
|                                                            | $a_2$                                | $ie^{-\frac{1}{2}i\pi t}$                                                                                                                    |
| $b \left( 0, \frac{t}{2}, 0 \right)$                       | $b_1$                                | $\{m_{100}   \frac{1}{2} \ 0 \ \frac{1}{2}\}$<br>$-i$                                                                                        |
|                                                            | $b_2$                                | $i$                                                                                                                                          |
| $c \left( \frac{1}{2}, \frac{t}{2}, 0 \right)$             | $c_1$                                | $\{m_{100}   \frac{1}{2} \ 0 \ \frac{1}{2}\}$<br>$i$                                                                                         |
|                                                            | $c_2$                                | $-i$                                                                                                                                         |
| $d \left( \frac{1-t}{2}, \frac{1}{2}, 0 \right)$           | $d_1$                                | $\{m_{010}   \frac{1}{2} \ 0 \ 0\}$<br>$-ie^{-\frac{1}{2}i\pi(1-t)}$                                                                         |
|                                                            | $d_2$                                | $ie^{-\frac{1}{2}i\pi(1-t)}$                                                                                                                 |
| $e \left( \frac{t}{2}, 0, \frac{1}{2} \right)$             | $e_1$                                | $\{m_{010}   \frac{1}{2} \ 0 \ 0\}$<br>$-ie^{-\frac{1}{2}i\pi t}$                                                                            |
|                                                            | $e_2$                                | $ie^{-\frac{1}{2}i\pi t}$                                                                                                                    |
| $f \left( 0, \frac{t}{2}, \frac{1}{2} \right)$             | $f_1$                                | $\{m_{100}   \frac{1}{2} \ 0 \ \frac{1}{2}\}$<br>$-1$                                                                                        |
|                                                            | $f_2$                                | $1$                                                                                                                                          |
| $g \left( \frac{1}{2}, \frac{t}{2}, \frac{1}{2} \right)$   | $g_1$                                | $\{m_{100}   \frac{1}{2} \ 0 \ \frac{1}{2}\}$<br>$1$                                                                                         |
|                                                            | $g_2$                                | $-1$                                                                                                                                         |
| $h \left( \frac{1-t}{2}, \frac{1}{2}, \frac{1}{2} \right)$ | $h_1$                                | $\{m_{010}   \frac{1}{2} \ 0 \ 0\}$<br>$-ie^{-\frac{1}{2}i\pi(1-t)}$                                                                         |
|                                                            | $h_2$                                | $ie^{-\frac{1}{2}i\pi(1-t)}$                                                                                                                 |
| $i \left( 0, 0, \frac{t}{2} \right)$                       | $i_1$                                | $\{2_{001}   0 \ 0 \ \frac{1}{2}\} \ \{m_{100}   \frac{1}{2} \ 0 \ \frac{1}{2}\}$<br>$0 \ 0$                                                 |
| $j \left( \frac{1}{2}, 0, \frac{t}{2} \right)$             | $j_1$                                | $\{2_{001}   0 \ 0 \ \frac{1}{2}\} \ \{m_{100}   \frac{1}{2} \ 0 \ \frac{1}{2}\}$<br>$-ie^{-\frac{1}{2}i\pi t} \ -e^{-\frac{1}{2}i\pi(t+1)}$ |
|                                                            | $j_2$                                | $-ie^{-\frac{1}{2}i\pi t} \ e^{-\frac{1}{2}i\pi(t+1)}$                                                                                       |
|                                                            | $j_3$                                | $ie^{-\frac{1}{2}i\pi t} \ -e^{-\frac{1}{2}i\pi(t+1)}$                                                                                       |
|                                                            | $j_4$                                | $ie^{-\frac{1}{2}i\pi t} \ e^{-\frac{1}{2}i\pi(t+1)}$                                                                                        |
| $k \left( \frac{1}{2}, \frac{1}{2}, \frac{t}{2} \right)$   | $k_1$                                | $\{2_{001}   0 \ 0 \ \frac{1}{2}\} \ \{m_{100}   \frac{1}{2} \ 0 \ \frac{1}{2}\}$<br>$-ie^{-\frac{1}{2}i\pi t} \ -e^{-\frac{1}{2}i\pi(t+1)}$ |
|                                                            | $k_2$                                | $-ie^{-\frac{1}{2}i\pi t} \ e^{-\frac{1}{2}i\pi(t+1)}$                                                                                       |
|                                                            | $k_3$                                | $ie^{-\frac{1}{2}i\pi t} \ -e^{-\frac{1}{2}i\pi(t+1)}$                                                                                       |
|                                                            | $k_4$                                | $ie^{-\frac{1}{2}i\pi t} \ e^{-\frac{1}{2}i\pi(t+1)}$                                                                                        |

|       |                                 |                                                                                                                                                                                 |
|-------|---------------------------------|---------------------------------------------------------------------------------------------------------------------------------------------------------------------------------|
| $l$   | $(0, \frac{1}{2}, \frac{t}{2})$ | $\{2_{001}   \begin{smallmatrix} 0 & 0 & \frac{1}{2} \\ 0 & & \end{smallmatrix} \} \{m_{100}   \begin{smallmatrix} \frac{1}{2} & 0 & \frac{1}{2} \\ 0 & & \end{smallmatrix} \}$ |
| $l_1$ |                                 |                                                                                                                                                                                 |

$$\begin{aligned}
\mathcal{W}_1^{\text{gapless}} = & \sum_{m=1}^{n_{a_1}} \text{sgn}(v_m^{a_1}) \frac{1 - \text{sgn}(\delta_m^{a_1})}{2} + 2 \sum_{m=1}^{n_{e_2}} \text{sgn}(v_m^{e_2}) \frac{1 - \text{sgn}(\delta_m^{e_2})}{2} - 2 \sum_{m=1}^{n_{f_1}} \text{sgn}(v_m^{f_1}) \frac{1 - \text{sgn}(\delta_m^{f_1})}{2} \\
& + 4 \sum_{m=1}^{n_{g_2}} \text{sgn}(v_m^{g_2}) \frac{1 - \text{sgn}(\delta_m^{g_2})}{2} + 2 \sum_{m=1}^{n_{h_1}} \text{sgn}(v_m^{h_1}) \frac{1 - \text{sgn}(\delta_m^{h_1})}{2} \\
& + 2 \sum_{m=1}^{n_{h_2}} \text{sgn}(v_m^{h_2}) \frac{1 - \text{sgn}(\delta_m^{h_2})}{2} - \sum_{m=1}^{n_{i_1}} \text{sgn}(v_m^{i_1}) \frac{1 - \text{sgn}(\delta_m^{i_1})}{2} + \sum_{m=1}^{n_{j_2}} \text{sgn}(v_m^{j_2}) \frac{1 - \text{sgn}(\delta_m^{j_2})}{2} \\
& - \sum_{m=1}^{n_{j_3}} \text{sgn}(v_m^{j_3}) \frac{1 - \text{sgn}(\delta_m^{j_3})}{2} + 2 \sum_{m=1}^{n_{j_4}} \text{sgn}(v_m^{j_4}) \frac{1 - \text{sgn}(\delta_m^{j_4})}{2} + \sum_{m=1}^{n_{k_1}} \text{sgn}(v_m^{k_1}) \frac{1 - \text{sgn}(\delta_m^{k_1})}{2} \\
& - \sum_{m=1}^{n_{k_2}} \text{sgn}(v_m^{k_2}) \frac{1 - \text{sgn}(\delta_m^{k_2})}{2} + \sum_{m=1}^{n_{k_3}} \text{sgn}(v_m^{k_3}) \frac{1 - \text{sgn}(\delta_m^{k_3})}{2} - \sum_{m=1}^{n_{k_4}} \text{sgn}(v_m^{k_4}) \frac{1 - \text{sgn}(\delta_m^{k_4})}{2}
\end{aligned} \tag{S29.1}$$

$$\begin{aligned}
\mathcal{W}_2^{\text{gapless}} = & \sum_{m=1}^{n_{a_2}} \text{sgn}(v_m^{a_2}) \frac{1 - \text{sgn}(\delta_m^{a_2})}{2} - 2 \sum_{m=1}^{n_{e_2}} \text{sgn}(v_m^{e_2}) \frac{1 - \text{sgn}(\delta_m^{e_2})}{2} - \sum_{m=1}^{n_{i_1}} \text{sgn}(v_m^{i_1}) \frac{1 - \text{sgn}(\delta_m^{i_1})}{2} \\
& + \sum_{m=1}^{n_{j_2}} \text{sgn}(v_m^{j_2}) \frac{1 - \text{sgn}(\delta_m^{j_2})}{2} + \sum_{m=1}^{n_{j_3}} \text{sgn}(v_m^{j_3}) \frac{1 - \text{sgn}(\delta_m^{j_3})}{2}
\end{aligned} \tag{S29.2}$$

$$\mathcal{W}_3^{\text{gapless}} = \sum_{m=1}^{n_{b_1}} \text{sgn}(v_m^{b_1}) \frac{1 - \text{sgn}(\delta_m^{b_1})}{2} - \sum_{m=1}^{n_{f_1}} \text{sgn}(v_m^{f_1}) \frac{1 - \text{sgn}(\delta_m^{f_1})}{2} - \sum_{m=1}^{n_{i_1}} \text{sgn}(v_m^{i_1}) \frac{1 - \text{sgn}(\delta_m^{i_1})}{2} + \sum_{m=1}^{n_{l_1}} \text{sgn}(v_m^{l_1}) \frac{1 - \text{sgn}(\delta_m^{l_1})}{2} \tag{S29.3}$$

$$\mathcal{W}_4^{\text{gapless}} = \sum_{m=1}^{n_{b_2}} \text{sgn}(v_m^{b_2}) \frac{1 - \text{sgn}(\delta_m^{b_2})}{2} - \sum_{m=1}^{n_{f_1}} \text{sgn}(v_m^{f_1}) \frac{1 - \text{sgn}(\delta_m^{f_1})}{2} - \sum_{m=1}^{n_{i_1}} \text{sgn}(v_m^{i_1}) \frac{1 - \text{sgn}(\delta_m^{i_1})}{2} + \sum_{m=1}^{n_{l_1}} \text{sgn}(v_m^{l_1}) \frac{1 - \text{sgn}(\delta_m^{l_1})}{2} \tag{S29.4}$$

$$\begin{aligned}
\mathcal{W}_5^{\text{gapless}} = & \sum_{m=1}^{n_{c_1}} \text{sgn}(v_m^{c_1}) \frac{1 - \text{sgn}(\delta_m^{c_1})}{2} - 2 \sum_{m=1}^{n_{g_2}} \text{sgn}(v_m^{g_2}) \frac{1 - \text{sgn}(\delta_m^{g_2})}{2} - \sum_{m=1}^{n_{j_2}} \text{sgn}(v_m^{j_2}) \frac{1 - \text{sgn}(\delta_m^{j_2})}{2} \\
& - \sum_{m=1}^{n_{j_4}} \text{sgn}(v_m^{j_4}) \frac{1 - \text{sgn}(\delta_m^{j_4})}{2} + \sum_{m=1}^{n_{k_2}} \text{sgn}(v_m^{k_2}) \frac{1 - \text{sgn}(\delta_m^{k_2})}{2} + \sum_{m=1}^{n_{k_4}} \text{sgn}(v_m^{k_4}) \frac{1 - \text{sgn}(\delta_m^{k_4})}{2}
\end{aligned} \tag{S29.5}$$

$$\begin{aligned}
\mathcal{W}_6^{\text{gapless}} = & \sum_{m=1}^{n_{d_1}} \text{sgn}(v_m^{d_1}) \frac{1 - \text{sgn}(\delta_m^{d_1})}{2} - 2 \sum_{m=1}^{n_{h_1}} \text{sgn}(v_m^{h_1}) \frac{1 - \text{sgn}(\delta_m^{h_1})}{2} - \sum_{m=1}^{n_{k_1}} \text{sgn}(v_m^{k_1}) \frac{1 - \text{sgn}(\delta_m^{k_1})}{2} \\
& - \sum_{m=1}^{n_{k_4}} \text{sgn}(v_m^{k_4}) \frac{1 - \text{sgn}(\delta_m^{k_4})}{2} + \sum_{m=1}^{n_{l_1}} \text{sgn}(v_m^{l_1}) \frac{1 - \text{sgn}(\delta_m^{l_1})}{2}
\end{aligned} \tag{S29.6}$$

$$\begin{aligned} \mathcal{W}_7^{\text{gapless}} = & \sum_{m=1}^{n_{d_2}} \text{sgn}(v_m^{d_2}) \frac{1 - \text{sgn}(\delta_m^{d_2})}{2} - 2 \sum_{m=1}^{n_{h_2}} \text{sgn}(v_m^{h_2}) \frac{1 - \text{sgn}(\delta_m^{h_2})}{2} - \sum_{m=1}^{n_{k_2}} \text{sgn}(v_m^{k_2}) \frac{1 - \text{sgn}(\delta_m^{k_2})}{2} \\ & - \sum_{m=1}^{n_{k_3}} \text{sgn}(v_m^{k_3}) \frac{1 - \text{sgn}(\delta_m^{k_3})}{2} + \sum_{m=1}^{n_{l_1}} \text{sgn}(v_m^{l_1}) \frac{1 - \text{sgn}(\delta_m^{l_1})}{2} \end{aligned} \quad (\text{S29.7})$$

$$\begin{aligned} \mathcal{W}_8^{\text{gapless}} = & \sum_{m=1}^{n_{e_1}} \text{sgn}(v_m^{e_1}) \frac{1 - \text{sgn}(\delta_m^{e_1})}{2} + \sum_{m=1}^{n_{e_2}} \text{sgn}(v_m^{e_2}) \frac{1 - \text{sgn}(\delta_m^{e_2})}{2} - \sum_{m=1}^{n_{f_1}} \text{sgn}(v_m^{f_1}) \frac{1 - \text{sgn}(\delta_m^{f_1})}{2} + \sum_{m=1}^{n_{g_1}} \text{sgn}(v_m^{g_1}) \frac{1 - \text{sgn}(\delta_m^{g_1})}{2} \\ & + \sum_{m=1}^{n_{g_2}} \text{sgn}(v_m^{g_2}) \frac{1 - \text{sgn}(\delta_m^{g_2})}{2} + \sum_{m=1}^{n_{h_1}} \text{sgn}(v_m^{h_1}) \frac{1 - \text{sgn}(\delta_m^{h_1})}{2} + \sum_{m=1}^{n_{h_2}} \text{sgn}(v_m^{h_2}) \frac{1 - \text{sgn}(\delta_m^{h_2})}{2} \end{aligned} \quad (\text{S29.8})$$

$$\begin{aligned} \mathcal{W}_9^{\text{gapless}} = & 2 \sum_{m=1}^{n_{g_1}} \text{sgn}(v_m^{g_1}) \frac{1 - \text{sgn}(\delta_m^{g_1})}{2} - 2 \sum_{m=1}^{n_{g_2}} \text{sgn}(v_m^{g_2}) \frac{1 - \text{sgn}(\delta_m^{g_2})}{2} + \sum_{m=1}^{n_{j_1}} \text{sgn}(v_m^{j_1}) \frac{1 - \text{sgn}(\delta_m^{j_1})}{2} \\ & - \sum_{m=1}^{n_{j_2}} \text{sgn}(v_m^{j_2}) \frac{1 - \text{sgn}(\delta_m^{j_2})}{2} + \sum_{m=1}^{n_{j_3}} \text{sgn}(v_m^{j_3}) \frac{1 - \text{sgn}(\delta_m^{j_3})}{2} - \sum_{m=1}^{n_{j_4}} \text{sgn}(v_m^{j_4}) \frac{1 - \text{sgn}(\delta_m^{j_4})}{2} \\ & - \sum_{m=1}^{n_{k_1}} \text{sgn}(v_m^{k_1}) \frac{1 - \text{sgn}(\delta_m^{k_1})}{2} + \sum_{m=1}^{n_{k_2}} \text{sgn}(v_m^{k_2}) \frac{1 - \text{sgn}(\delta_m^{k_2})}{2} - \sum_{m=1}^{n_{k_3}} \text{sgn}(v_m^{k_3}) \frac{1 - \text{sgn}(\delta_m^{k_3})}{2} \\ & + \sum_{m=1}^{n_{k_4}} \text{sgn}(v_m^{k_4}) \frac{1 - \text{sgn}(\delta_m^{k_4})}{2} \end{aligned} \quad (\text{S29.9})$$

$$\mathcal{X}_1 = \sum_{m=1}^{n_{f_1}} \frac{1 - \text{sgn}(\delta_m^{f_1})}{2} + \sum_{m=1}^{n_{k_2}} \frac{1 - \text{sgn}(\delta_m^{k_2})}{2} + \sum_{m=1}^{n_{k_3}} \frac{1 - \text{sgn}(\delta_m^{k_3})}{2} \quad \text{mod } 2 \quad (\text{S29.10})$$

$$\mathcal{X}_2 = \sum_{m=1}^{n_{f_1}} \frac{1 - \text{sgn}(\delta_m^{f_1})}{2} + \sum_{m=1}^{n_{j_1}} \frac{1 - \text{sgn}(\delta_m^{j_1})}{2} + \sum_{m=1}^{n_{j_4}} \frac{1 - \text{sgn}(\delta_m^{j_4})}{2} \quad \text{mod } 2 \quad (\text{S29.11})$$

$$\begin{aligned} \mathcal{X}_3 = & -6 \sum_{m=1}^{n_{e_2}} \text{sgn}(v_m^{e_2}) \frac{1 - \text{sgn}(\delta_m^{e_2})}{2} + 3 \sum_{m=1}^{n_{f_1}} \text{sgn}(v_m^{f_1}) \frac{1 - \text{sgn}(\delta_m^{f_1})}{2} - 6 \sum_{m=1}^{n_{g_1}} \text{sgn}(v_m^{g_1}) \frac{1 - \text{sgn}(\delta_m^{g_1})}{2} \\ & - 6 \sum_{m=1}^{n_{g_2}} \text{sgn}(v_m^{g_2}) \frac{1 - \text{sgn}(\delta_m^{g_2})}{2} - 6 \sum_{m=1}^{n_{h_1}} \text{sgn}(v_m^{h_1}) \frac{1 - \text{sgn}(\delta_m^{h_1})}{2} - 3 \sum_{m=1}^{n_{j_1}} \text{sgn}(v_m^{j_1}) \frac{1 - \text{sgn}(\delta_m^{j_1})}{2} \\ & + 3 \sum_{m=1}^{n_{j_4}} \text{sgn}(v_m^{j_4}) \frac{1 - \text{sgn}(\delta_m^{j_4})}{2} + \sum_{m=1}^{n_{k_2}} \text{sgn}(v_m^{k_2}) \frac{1 - \text{sgn}(\delta_m^{k_2})}{2} - \sum_{m=1}^{n_{k_3}} \text{sgn}(v_m^{k_3}) \frac{1 - \text{sgn}(\delta_m^{k_3})}{2} \quad \text{mod } 4 \end{aligned} \quad (\text{S29.12})$$

$$\begin{aligned} \mathcal{X}_4 = & -6 \sum_{m=1}^{n_{e_2}} \text{sgn}(v_m^{e_2}) \frac{1 - \text{sgn}(\delta_m^{e_2})}{2} + 3 \sum_{m=1}^{n_{f_1}} \text{sgn}(v_m^{f_1}) \frac{1 - \text{sgn}(\delta_m^{f_1})}{2} - 6 \sum_{m=1}^{n_{h_2}} \text{sgn}(v_m^{h_2}) \frac{1 - \text{sgn}(\delta_m^{h_2})}{2} \\ & - 2 \sum_{m=1}^{n_{j_1}} \text{sgn}(v_m^{j_1}) \frac{1 - \text{sgn}(\delta_m^{j_1})}{2} - \sum_{m=1}^{n_{j_2}} \text{sgn}(v_m^{j_2}) \frac{1 - \text{sgn}(\delta_m^{j_2})}{2} + \sum_{m=1}^{n_{j_3}} \text{sgn}(v_m^{j_3}) \frac{1 - \text{sgn}(\delta_m^{j_3})}{2} \\ & + 2 \sum_{m=1}^{n_{j_4}} \text{sgn}(v_m^{j_4}) \frac{1 - \text{sgn}(\delta_m^{j_4})}{2} + \sum_{m=1}^{n_{k_2}} \text{sgn}(v_m^{k_2}) \frac{1 - \text{sgn}(\delta_m^{k_2})}{2} - \sum_{m=1}^{n_{k_3}} \text{sgn}(v_m^{k_3}) \frac{1 - \text{sgn}(\delta_m^{k_3})}{2} \quad \text{mod } 4 \end{aligned} \quad (\text{S29.13})$$

## S30. SPACE GROUP NO. 30

| line segment                                               | character of irrep (generators only) |                                                                                                         |
|------------------------------------------------------------|--------------------------------------|---------------------------------------------------------------------------------------------------------|
| $a \left( \frac{t}{2}, 0, 0 \right)$                       | $a_1$                                | $\{m_{010}   0 \frac{1}{2} \frac{1}{2}\}$<br>-i                                                         |
|                                                            | $a_2$                                | i                                                                                                       |
| $b \left( 0, \frac{t}{2}, 0 \right)$                       | $b_1$                                | $\{m_{100}   0 \frac{1}{2} \frac{1}{2}\}$<br>$-ie^{-\frac{1}{2}i\pi t}$                                 |
|                                                            | $b_2$                                | $ie^{-\frac{1}{2}i\pi t}$                                                                               |
| $c \left( \frac{1}{2}, \frac{t}{2}, 0 \right)$             | $c_1$                                | $\{m_{100}   0 \frac{1}{2} \frac{1}{2}\}$<br>$-ie^{-\frac{1}{2}i\pi t}$                                 |
|                                                            | $c_2$                                | $ie^{-\frac{1}{2}i\pi t}$                                                                               |
| $d \left( \frac{1-t}{2}, \frac{1}{2}, 0 \right)$           | $d_1$                                | $\{m_{010}   0 \frac{1}{2} \frac{1}{2}\}$<br>i                                                          |
|                                                            | $d_2$                                | -i                                                                                                      |
| $e \left( \frac{t}{2}, 0, \frac{1}{2} \right)$             | $e_1$                                | $\{m_{010}   0 \frac{1}{2} \frac{1}{2}\}$<br>-1                                                         |
|                                                            | $e_2$                                | 1                                                                                                       |
| $f \left( 0, \frac{t}{2}, \frac{1}{2} \right)$             | $f_1$                                | $\{m_{100}   0 \frac{1}{2} \frac{1}{2}\}$<br>$-ie^{-\frac{1}{2}i\pi(t+1)}$                              |
|                                                            | $f_2$                                | $ie^{-\frac{1}{2}i\pi(t+1)}$                                                                            |
| $g \left( \frac{1}{2}, \frac{t}{2}, \frac{1}{2} \right)$   | $g_1$                                | $\{m_{100}   0 \frac{1}{2} \frac{1}{2}\}$<br>$-ie^{-\frac{1}{2}i\pi(t+1)}$                              |
|                                                            | $g_2$                                | $ie^{-\frac{1}{2}i\pi(t+1)}$                                                                            |
| $h \left( \frac{1-t}{2}, \frac{1}{2}, \frac{1}{2} \right)$ | $h_1$                                | $\{m_{010}   0 \frac{1}{2} \frac{1}{2}\}$<br>1                                                          |
|                                                            | $h_2$                                | -1                                                                                                      |
| $i \left( 0, 0, \frac{t}{2} \right)$                       | $i_1$                                | $\{2_{001}   0 \ 0 \ 0\}$ $\{m_{100}   0 \frac{1}{2} \frac{1}{2}\}$<br>0 0                              |
| $j \left( \frac{1}{2}, 0, \frac{t}{2} \right)$             | $j_1$                                | $\{2_{001}   0 \ 0 \ 0\}$ $\{m_{100}   0 \frac{1}{2} \frac{1}{2}\}$<br>0 0                              |
| $k \left( \frac{1}{2}, \frac{1}{2}, \frac{t}{2} \right)$   | $k_1$                                | $\{2_{001}   0 \ 0 \ 0\}$ $\{m_{100}   0 \frac{1}{2} \frac{1}{2}\}$<br>-i $-ie^{-\frac{1}{2}i\pi(t+1)}$ |
|                                                            | $k_2$                                | -i $ie^{-\frac{1}{2}i\pi(t+1)}$                                                                         |
|                                                            | $k_3$                                | i $-ie^{-\frac{1}{2}i\pi(t+1)}$                                                                         |
|                                                            | $k_4$                                | i $ie^{-\frac{1}{2}i\pi(t+1)}$                                                                          |
| $l \left( 0, \frac{1}{2}, \frac{t}{2} \right)$             | $l_1$                                | $\{2_{001}   0 \ 0 \ 0\}$ $\{m_{100}   0 \frac{1}{2} \frac{1}{2}\}$<br>-i $-ie^{-\frac{1}{2}i\pi(t+1)}$ |
|                                                            | $l_2$                                | -i $ie^{-\frac{1}{2}i\pi(t+1)}$                                                                         |
|                                                            | $l_3$                                | i $-ie^{-\frac{1}{2}i\pi(t+1)}$                                                                         |
|                                                            | $l_4$                                | i $ie^{-\frac{1}{2}i\pi(t+1)}$                                                                          |

(S30.2)

(S30.3)

(S30.4)

(S30.5)



$$\begin{aligned}\mathcal{W}_6^{\text{gapless}} = & \sum_{m=1}^{n_{c_2}} \text{sgn}(v_m^{c_2}) \frac{1 - \text{sgn}(\delta_m^{c_2})}{2} - \sum_{m=1}^{n_{g_1}} \text{sgn}(v_m^{g_1}) \frac{1 - \text{sgn}(\delta_m^{g_1})}{2} - \sum_{m=1}^{n_{j_1}} \text{sgn}(v_m^{j_1}) \frac{1 - \text{sgn}(\delta_m^{j_1})}{2} \\ & + \sum_{m=1}^{n_{k_2}} \text{sgn}(v_m^{k_2}) \frac{1 - \text{sgn}(\delta_m^{k_2})}{2} + \sum_{m=1}^{n_{k_4}} \text{sgn}(v_m^{k_4}) \frac{1 - \text{sgn}(\delta_m^{k_4})}{2}\end{aligned}\quad (\text{S30.6})$$

$$\begin{aligned}\mathcal{W}_7^{\text{gapless}} = & \sum_{m=1}^{n_{d_1}} \text{sgn}(v_m^{d_1}) \frac{1 - \text{sgn}(\delta_m^{d_1})}{2} - \sum_{m=1}^{n_{h_2}} \text{sgn}(v_m^{h_2}) \frac{1 - \text{sgn}(\delta_m^{h_2})}{2} - \sum_{m=1}^{n_{k_1}} \text{sgn}(v_m^{k_1}) \frac{1 - \text{sgn}(\delta_m^{k_1})}{2} \\ & - \sum_{m=1}^{n_{k_4}} \text{sgn}(v_m^{k_4}) \frac{1 - \text{sgn}(\delta_m^{k_4})}{2} + \sum_{m=1}^{n_{l_1}} \text{sgn}(v_m^{l_1}) \frac{1 - \text{sgn}(\delta_m^{l_1})}{2} + \sum_{m=1}^{n_{l_4}} \text{sgn}(v_m^{l_4}) \frac{1 - \text{sgn}(\delta_m^{l_4})}{2}\end{aligned}\quad (\text{S30.7})$$

$$\begin{aligned}\mathcal{W}_8^{\text{gapless}} = & 2 \sum_{m=1}^{n_{e_1}} \text{sgn}(v_m^{e_1}) \frac{1 - \text{sgn}(\delta_m^{e_1})}{2} - 2 \sum_{m=1}^{n_{f_1}} \text{sgn}(v_m^{f_1}) \frac{1 - \text{sgn}(\delta_m^{f_1})}{2} + 2 \sum_{m=1}^{n_{g_1}} \text{sgn}(v_m^{g_1}) \frac{1 - \text{sgn}(\delta_m^{g_1})}{2} \\ & + 2 \sum_{m=1}^{n_{h_2}} \text{sgn}(v_m^{h_2}) \frac{1 - \text{sgn}(\delta_m^{h_2})}{2} + \sum_{m=1}^{n_{k_1}} \text{sgn}(v_m^{k_1}) \frac{1 - \text{sgn}(\delta_m^{k_1})}{2} - \sum_{m=1}^{n_{k_2}} \text{sgn}(v_m^{k_2}) \frac{1 - \text{sgn}(\delta_m^{k_2})}{2} \\ & - \sum_{m=1}^{n_{k_3}} \text{sgn}(v_m^{k_3}) \frac{1 - \text{sgn}(\delta_m^{k_3})}{2} + \sum_{m=1}^{n_{k_4}} \text{sgn}(v_m^{k_4}) \frac{1 - \text{sgn}(\delta_m^{k_4})}{2} - \sum_{m=1}^{n_{l_1}} \text{sgn}(v_m^{l_1}) \frac{1 - \text{sgn}(\delta_m^{l_1})}{2} \\ & + \sum_{m=1}^{n_{l_2}} \text{sgn}(v_m^{l_2}) \frac{1 - \text{sgn}(\delta_m^{l_2})}{2} + \sum_{m=1}^{n_{l_3}} \text{sgn}(v_m^{l_3}) \frac{1 - \text{sgn}(\delta_m^{l_3})}{2} - \sum_{m=1}^{n_{l_4}} \text{sgn}(v_m^{l_4}) \frac{1 - \text{sgn}(\delta_m^{l_4})}{2}\end{aligned}\quad (\text{S30.8})$$

$$\begin{aligned}\mathcal{W}_9^{\text{gapless}} = & \sum_{m=1}^{n_{h_1}} \text{sgn}(v_m^{h_1}) \frac{1 - \text{sgn}(\delta_m^{h_1})}{2} - \sum_{m=1}^{n_{h_2}} \text{sgn}(v_m^{h_2}) \frac{1 - \text{sgn}(\delta_m^{h_2})}{2} - \sum_{m=1}^{n_{k_1}} \text{sgn}(v_m^{k_1}) \frac{1 - \text{sgn}(\delta_m^{k_1})}{2} \\ & + \sum_{m=1}^{n_{k_2}} \text{sgn}(v_m^{k_2}) \frac{1 - \text{sgn}(\delta_m^{k_2})}{2} + \sum_{m=1}^{n_{k_3}} \text{sgn}(v_m^{k_3}) \frac{1 - \text{sgn}(\delta_m^{k_3})}{2} - \sum_{m=1}^{n_{k_4}} \text{sgn}(v_m^{k_4}) \frac{1 - \text{sgn}(\delta_m^{k_4})}{2} \\ & + \sum_{m=1}^{n_{l_1}} \text{sgn}(v_m^{l_1}) \frac{1 - \text{sgn}(\delta_m^{l_1})}{2} - \sum_{m=1}^{n_{l_2}} \text{sgn}(v_m^{l_2}) \frac{1 - \text{sgn}(\delta_m^{l_2})}{2} - \sum_{m=1}^{n_{l_3}} \text{sgn}(v_m^{l_3}) \frac{1 - \text{sgn}(\delta_m^{l_3})}{2} + \sum_{m=1}^{n_{l_4}} \text{sgn}(v_m^{l_4}) \frac{1 - \text{sgn}(\delta_m^{l_4})}{2}\end{aligned}\quad (\text{S30.9})$$

$$\begin{aligned}\mathcal{W}_1^{\text{gapped}} = & - \sum_{m=1}^{n_{k_1}} \text{sgn}(v_m^{k_1}) \frac{1 - \text{sgn}(\delta_m^{k_1})}{2} - \sum_{m=1}^{n_{k_2}} \text{sgn}(v_m^{k_2}) \frac{1 - \text{sgn}(\delta_m^{k_2})}{2} + \sum_{m=1}^{n_{k_3}} \text{sgn}(v_m^{k_3}) \frac{1 - \text{sgn}(\delta_m^{k_3})}{2} \\ & + \sum_{m=1}^{n_{k_4}} \text{sgn}(v_m^{k_4}) \frac{1 - \text{sgn}(\delta_m^{k_4})}{2}\end{aligned}\quad (\text{S30.10})$$

$$\begin{aligned}\mathcal{W}_2^{\text{gapped}} = & - \sum_{m=1}^{n_{e_1}} \text{sgn}(v_m^{e_1}) \frac{1 - \text{sgn}(\delta_m^{e_1})}{2} + \sum_{m=1}^{n_{f_1}} \text{sgn}(v_m^{f_1}) \frac{1 - \text{sgn}(\delta_m^{f_1})}{2} - \sum_{m=1}^{n_{g_1}} \text{sgn}(v_m^{g_1}) \frac{1 - \text{sgn}(\delta_m^{g_1})}{2} \\ & - \sum_{m=1}^{n_{h_2}} \text{sgn}(v_m^{h_2}) \frac{1 - \text{sgn}(\delta_m^{h_2})}{2} + \sum_{m=1}^{n_{k_2}} \text{sgn}(v_m^{k_2}) \frac{1 - \text{sgn}(\delta_m^{k_2})}{2} \\ & - \sum_{m=1}^{n_{k_4}} \text{sgn}(v_m^{k_4}) \frac{1 - \text{sgn}(\delta_m^{k_4})}{2} - \sum_{m=1}^{n_{l_2}} \text{sgn}(v_m^{l_2}) \frac{1 - \text{sgn}(\delta_m^{l_2})}{2} + \sum_{m=1}^{n_{l_4}} \text{sgn}(v_m^{l_4}) \frac{1 - \text{sgn}(\delta_m^{l_4})}{2}\end{aligned}\quad (\text{S30.11})$$

$$\begin{aligned} \mathcal{X}_1 = & \sum_{m=1}^{n_{f_1}} \frac{1 - \text{sgn}(\delta_m^{f_1})}{2} + \sum_{m=1}^{n_{g_1}} \frac{1 - \text{sgn}(\delta_m^{g_1})}{2} + \sum_{m=1}^{n_{h_2}} \frac{1 - \text{sgn}(\delta_m^{h_2})}{2} + \sum_{m=1}^{n_{k_2}} \frac{1 - \text{sgn}(\delta_m^{k_2})}{2} + \sum_{m=1}^{n_{k_4}} \frac{1 - \text{sgn}(\delta_m^{k_4})}{2} \\ & + \sum_{m=1}^{n_{l_1}} \frac{1 - \text{sgn}(\delta_m^{l_1})}{2} + \sum_{m=1}^{n_{l_3}} \frac{1 - \text{sgn}(\delta_m^{l_3})}{2} \quad \text{mod } 2 \end{aligned} \quad (\text{S30.12})$$

$$\mathcal{X}_2 = \sum_{m=1}^{n_{g_1}} \frac{1 - \text{sgn}(\delta_m^{g_1})}{2} + \sum_{m=1}^{n_{k_2}} \frac{1 - \text{sgn}(\delta_m^{k_2})}{2} + \sum_{m=1}^{n_{k_4}} \frac{1 - \text{sgn}(\delta_m^{k_4})}{2} \quad \text{mod } 2 \quad (\text{S30.13})$$

$$\mathcal{X}_3 = \sum_{m=1}^{n_{g_1}} \frac{1 - \text{sgn}(\delta_m^{g_1})}{2} + \sum_{m=1}^{n_{h_2}} \frac{1 - \text{sgn}(\delta_m^{h_2})}{2} + \sum_{m=1}^{n_{k_2}} \frac{1 - \text{sgn}(\delta_m^{k_2})}{2} + \sum_{m=1}^{n_{k_4}} \frac{1 - \text{sgn}(\delta_m^{k_4})}{2} \quad \text{mod } 2 \quad (\text{S30.14})$$

### S31. SPACE GROUP NO. 31

| line segment                                        | character of irrep (generators only)                                                                                                                                                                                                                                            |
|-----------------------------------------------------|---------------------------------------------------------------------------------------------------------------------------------------------------------------------------------------------------------------------------------------------------------------------------------|
| $a \quad (\frac{t}{2}, 0, 0)$                       | $\{m_{010}   \frac{1}{2} \ 0 \ \frac{1}{2}\}$<br>$a_1 \quad -ie^{-\frac{1}{2}i\pi t}$<br>$a_2 \quad ie^{-\frac{1}{2}i\pi t}$                                                                                                                                                    |
| $b \quad (0, \frac{t}{2}, 0)$                       | $\{m_{100}   0 \ 0 \ 0\}$<br>$b_1 \quad -i$<br>$b_2 \quad i$                                                                                                                                                                                                                    |
| $c \quad (\frac{1}{2}, \frac{t}{2}, 0)$             | $\{m_{100}   0 \ 0 \ 0\}$<br>$c_1 \quad -i$<br>$c_2 \quad i$                                                                                                                                                                                                                    |
| $d \quad (\frac{1-t}{2}, \frac{1}{2}, 0)$           | $\{m_{010}   \frac{1}{2} \ 0 \ \frac{1}{2}\}$<br>$d_1 \quad -ie^{-\frac{1}{2}i\pi(1-t)}$<br>$d_2 \quad ie^{-\frac{1}{2}i\pi(1-t)}$                                                                                                                                              |
| $e \quad (\frac{t}{2}, 0, \frac{1}{2})$             | $\{m_{010}   \frac{1}{2} \ 0 \ \frac{1}{2}\}$<br>$e_1 \quad -ie^{-\frac{1}{2}i\pi(t+1)}$<br>$e_2 \quad ie^{-\frac{1}{2}i\pi(t+1)}$                                                                                                                                              |
| $f \quad (0, \frac{t}{2}, \frac{1}{2})$             | $\{m_{100}   0 \ 0 \ 0\}$<br>$f_1 \quad -i$<br>$f_2 \quad i$                                                                                                                                                                                                                    |
| $g \quad (\frac{1}{2}, \frac{t}{2}, \frac{1}{2})$   | $\{m_{100}   0 \ 0 \ 0\}$<br>$g_1 \quad -i$<br>$g_2 \quad i$                                                                                                                                                                                                                    |
| $h \quad (\frac{1-t}{2}, \frac{1}{2}, \frac{1}{2})$ | $\{m_{010}   \frac{1}{2} \ 0 \ \frac{1}{2}\}$<br>$h_1 \quad -ie^{-\frac{1}{2}i\pi(2-t)}$<br>$h_2 \quad ie^{-\frac{1}{2}i\pi(2-t)}$                                                                                                                                              |
| $i \quad (0, 0, \frac{t}{2})$                       | $\{2_{001}   \frac{1}{2} \ 0 \ \frac{1}{2}\} \ \{m_{100}   0 \ 0 \ 0\}$<br>$i_1 \quad 0 \quad 0$                                                                                                                                                                                |
| $j \quad (\frac{1}{2}, 0, \frac{t}{2})$             | $\{2_{001}   \frac{1}{2} \ 0 \ \frac{1}{2}\} \ \{m_{100}   0 \ 0 \ 0\}$<br>$j_1 \quad -e^{-\frac{1}{2}i\pi(t+1)} \quad -i$<br>$j_2 \quad -e^{-\frac{1}{2}i\pi(t+1)} \quad i$<br>$j_3 \quad e^{-\frac{1}{2}i\pi(t+1)} \quad -i$<br>$j_4 \quad e^{-\frac{1}{2}i\pi(t+1)} \quad i$ |
| $k \quad (\frac{1}{2}, \frac{1}{2}, \frac{t}{2})$   | $\{2_{001}   \frac{1}{2} \ 0 \ \frac{1}{2}\} \ \{m_{100}   0 \ 0 \ 0\}$<br>$k_1 \quad -e^{-\frac{1}{2}i\pi(t+1)} \quad -i$<br>$k_2 \quad -e^{-\frac{1}{2}i\pi(t+1)} \quad i$<br>$k_3 \quad e^{-\frac{1}{2}i\pi(t+1)} \quad -i$<br>$k_4 \quad e^{-\frac{1}{2}i\pi(t+1)} \quad i$ |

|                                         |                                                                                                                                                                                                                         |
|-----------------------------------------|-------------------------------------------------------------------------------------------------------------------------------------------------------------------------------------------------------------------------|
| $l \quad (0, \frac{1}{2}, \frac{t}{2})$ | $l_1 \quad \left\{ 2_{001} \left  \begin{smallmatrix} \frac{1}{2} & 0 & \frac{1}{2} \\ 0 \end{smallmatrix} \right\} \quad \left\{ m_{100} \left  \begin{smallmatrix} 0 & 0 & 0 \\ 0 \end{smallmatrix} \right\} \right.$ |
|-----------------------------------------|-------------------------------------------------------------------------------------------------------------------------------------------------------------------------------------------------------------------------|

$$\begin{aligned}
\mathcal{W}_1^{\text{gapless}} = & \sum_{m=1}^{n_{a_1}} \text{sgn}(v_m^{a_1}) \frac{1 - \text{sgn}(\delta_m^{a_1})}{2} - \sum_{m=1}^{n_{f_1}} \text{sgn}(v_m^{f_1}) \frac{1 - \text{sgn}(\delta_m^{f_1})}{2} - \sum_{m=1}^{n_{f_2}} \text{sgn}(v_m^{f_2}) \frac{1 - \text{sgn}(\delta_m^{f_2})}{2} \\
& + \sum_{m=1}^{n_{g_1}} \text{sgn}(v_m^{g_1}) \frac{1 - \text{sgn}(\delta_m^{g_1})}{2} + \sum_{m=1}^{n_{h_1}} \text{sgn}(v_m^{h_1}) \frac{1 - \text{sgn}(\delta_m^{h_1})}{2} \\
& - \sum_{m=1}^{n_{i_1}} \text{sgn}(v_m^{i_1}) \frac{1 - \text{sgn}(\delta_m^{i_1})}{2} + \sum_{m=1}^{n_{j_2}} \text{sgn}(v_m^{j_2}) \frac{1 - \text{sgn}(\delta_m^{j_2})}{2} + \sum_{m=1}^{n_{j_3}} \text{sgn}(v_m^{j_3}) \frac{1 - \text{sgn}(\delta_m^{j_3})}{2}
\end{aligned} \tag{S31.1}$$

$$\begin{aligned}
\mathcal{W}_2^{\text{gapless}} = & \sum_{m=1}^{n_{a_2}} \text{sgn}(v_m^{a_2}) \frac{1 - \text{sgn}(\delta_m^{a_2})}{2} - \sum_{m=1}^{n_{f_1}} \text{sgn}(v_m^{f_1}) \frac{1 - \text{sgn}(\delta_m^{f_1})}{2} - \sum_{m=1}^{n_{f_2}} \text{sgn}(v_m^{f_2}) \frac{1 - \text{sgn}(\delta_m^{f_2})}{2} + \sum_{m=1}^{n_{g_1}} \text{sgn}(v_m^{g_1}) \frac{1 - \text{sgn}(\delta_m^{g_1})}{2} \\
& + \sum_{m=1}^{n_{h_1}} \text{sgn}(v_m^{h_1}) \frac{1 - \text{sgn}(\delta_m^{h_1})}{2} - \sum_{m=1}^{n_{i_1}} \text{sgn}(v_m^{i_1}) \frac{1 - \text{sgn}(\delta_m^{i_1})}{2} + \sum_{m=1}^{n_{j_2}} \text{sgn}(v_m^{j_2}) \frac{1 - \text{sgn}(\delta_m^{j_2})}{2} \\
& - \sum_{m=1}^{n_{j_3}} \text{sgn}(v_m^{j_3}) \frac{1 - \text{sgn}(\delta_m^{j_3})}{2} + 2 \sum_{m=1}^{n_{j_4}} \text{sgn}(v_m^{j_4}) \frac{1 - \text{sgn}(\delta_m^{j_4})}{2} + \sum_{m=1}^{n_{k_1}} \text{sgn}(v_m^{k_1}) \frac{1 - \text{sgn}(\delta_m^{k_1})}{2} \\
& - \sum_{m=1}^{n_{k_2}} \text{sgn}(v_m^{k_2}) \frac{1 - \text{sgn}(\delta_m^{k_2})}{2} + \sum_{m=1}^{n_{k_3}} \text{sgn}(v_m^{k_3}) \frac{1 - \text{sgn}(\delta_m^{k_3})}{2} - \sum_{m=1}^{n_{k_4}} \text{sgn}(v_m^{k_4}) \frac{1 - \text{sgn}(\delta_m^{k_4})}{2}
\end{aligned} \tag{S31.2}$$

$$\mathcal{W}_3^{\text{gapless}} = \sum_{m=1}^{n_{b_1}} \text{sgn}(v_m^{b_1}) \frac{1 - \text{sgn}(\delta_m^{b_1})}{2} - 2 \sum_{m=1}^{n_{f_1}} \text{sgn}(v_m^{f_1}) \frac{1 - \text{sgn}(\delta_m^{f_1})}{2} - \sum_{m=1}^{n_{i_1}} \text{sgn}(v_m^{i_1}) \frac{1 - \text{sgn}(\delta_m^{i_1})}{2} + \sum_{m=1}^{n_{l_1}} \text{sgn}(v_m^{l_1}) \frac{1 - \text{sgn}(\delta_m^{l_1})}{2} \tag{S31.3}$$

$$\mathcal{W}_4^{\text{gapless}} = \sum_{m=1}^{n_{b_2}} \text{sgn}(v_m^{b_2}) \frac{1 - \text{sgn}(\delta_m^{b_2})}{2} - 2 \sum_{m=1}^{n_{f_2}} \text{sgn}(v_m^{f_2}) \frac{1 - \text{sgn}(\delta_m^{f_2})}{2} - \sum_{m=1}^{n_{i_1}} \text{sgn}(v_m^{i_1}) \frac{1 - \text{sgn}(\delta_m^{i_1})}{2} + \sum_{m=1}^{n_{l_1}} \text{sgn}(v_m^{l_1}) \frac{1 - \text{sgn}(\delta_m^{l_1})}{2} \tag{S31.4}$$

$$\begin{aligned}
\mathcal{W}_5^{\text{gapless}} = & \sum_{m=1}^{n_{c_1}} \text{sgn}(v_m^{c_1}) \frac{1 - \text{sgn}(\delta_m^{c_1})}{2} - \sum_{m=1}^{n_{g_1}} \text{sgn}(v_m^{g_1}) \frac{1 - \text{sgn}(\delta_m^{g_1})}{2} - \sum_{m=1}^{n_{j_2}} \text{sgn}(v_m^{j_2}) \frac{1 - \text{sgn}(\delta_m^{j_2})}{2} \\
& - \sum_{m=1}^{n_{j_4}} \text{sgn}(v_m^{j_4}) \frac{1 - \text{sgn}(\delta_m^{j_4})}{2} + \sum_{m=1}^{n_{k_2}} \text{sgn}(v_m^{k_2}) \frac{1 - \text{sgn}(\delta_m^{k_2})}{2} + \sum_{m=1}^{n_{k_4}} \text{sgn}(v_m^{k_4}) \frac{1 - \text{sgn}(\delta_m^{k_4})}{2}
\end{aligned} \tag{S31.5}$$

$$\begin{aligned}
\mathcal{W}_6^{\text{gapless}} = & \sum_{m=1}^{n_{d_1}} \text{sgn}(v_m^{d_1}) \frac{1 - \text{sgn}(\delta_m^{d_1})}{2} - \sum_{m=1}^{n_{h_1}} \text{sgn}(v_m^{h_1}) \frac{1 - \text{sgn}(\delta_m^{h_1})}{2} - \sum_{m=1}^{n_{k_2}} \text{sgn}(v_m^{k_2}) \frac{1 - \text{sgn}(\delta_m^{k_2})}{2} \\
& - \sum_{m=1}^{n_{k_3}} \text{sgn}(v_m^{k_3}) \frac{1 - \text{sgn}(\delta_m^{k_3})}{2} + \sum_{m=1}^{n_{l_1}} \text{sgn}(v_m^{l_1}) \frac{1 - \text{sgn}(\delta_m^{l_1})}{2}
\end{aligned} \tag{S31.6}$$

$$\begin{aligned} \mathcal{W}_7^{\text{gapless}} = & \sum_{m=1}^{n_{d_2}} \text{sgn}(v_m^{d_2}) \frac{1 - \text{sgn}(\delta_m^{d_2})}{2} - \sum_{m=1}^{n_{h_1}} \text{sgn}(v_m^{h_1}) \frac{1 - \text{sgn}(\delta_m^{h_1})}{2} - \sum_{m=1}^{n_{k_1}} \text{sgn}(v_m^{k_1}) \frac{1 - \text{sgn}(\delta_m^{k_1})}{2} \\ & - \sum_{m=1}^{n_{k_4}} \text{sgn}(v_m^{k_4}) \frac{1 - \text{sgn}(\delta_m^{k_4})}{2} + \sum_{m=1}^{n_{l_1}} \text{sgn}(v_m^{l_1}) \frac{1 - \text{sgn}(\delta_m^{l_1})}{2} \end{aligned} \quad (\text{S31.7})$$

$$\begin{aligned} \mathcal{W}_8^{\text{gapless}} = & \sum_{m=1}^{n_{e_1}} \text{sgn}(v_m^{e_1}) \frac{1 - \text{sgn}(\delta_m^{e_1})}{2} - \sum_{m=1}^{n_{f_1}} \text{sgn}(v_m^{f_1}) \frac{1 - \text{sgn}(\delta_m^{f_1})}{2} - \sum_{m=1}^{n_{f_2}} \text{sgn}(v_m^{f_2}) \frac{1 - \text{sgn}(\delta_m^{f_2})}{2} \\ & + \sum_{m=1}^{n_{g_1}} \text{sgn}(v_m^{g_1}) \frac{1 - \text{sgn}(\delta_m^{g_1})}{2} + \sum_{m=1}^{n_{h_1}} \text{sgn}(v_m^{h_1}) \frac{1 - \text{sgn}(\delta_m^{h_1})}{2} \end{aligned} \quad (\text{S31.8})$$

$$\begin{aligned} \mathcal{W}_9^{\text{gapless}} = & \sum_{m=1}^{n_{j_1}} \text{sgn}(v_m^{j_1}) \frac{1 - \text{sgn}(\delta_m^{j_1})}{2} - \sum_{m=1}^{n_{j_2}} \text{sgn}(v_m^{j_2}) \frac{1 - \text{sgn}(\delta_m^{j_2})}{2} + \sum_{m=1}^{n_{j_3}} \text{sgn}(v_m^{j_3}) \frac{1 - \text{sgn}(\delta_m^{j_3})}{2} \\ & - \sum_{m=1}^{n_{j_4}} \text{sgn}(v_m^{j_4}) \frac{1 - \text{sgn}(\delta_m^{j_4})}{2} - \sum_{m=1}^{n_{k_1}} \text{sgn}(v_m^{k_1}) \frac{1 - \text{sgn}(\delta_m^{k_1})}{2} + \sum_{m=1}^{n_{k_2}} \text{sgn}(v_m^{k_2}) \frac{1 - \text{sgn}(\delta_m^{k_2})}{2} \\ & - \sum_{m=1}^{n_{k_3}} \text{sgn}(v_m^{k_3}) \frac{1 - \text{sgn}(\delta_m^{k_3})}{2} + \sum_{m=1}^{n_{k_4}} \text{sgn}(v_m^{k_4}) \frac{1 - \text{sgn}(\delta_m^{k_4})}{2} \end{aligned} \quad (\text{S31.9})$$

$$\begin{aligned} \mathcal{W}_1^{\text{gapped}} = & - \sum_{m=1}^{n_{k_1}} \text{sgn}(v_m^{k_1}) \frac{1 - \text{sgn}(\delta_m^{k_1})}{2} + \sum_{m=1}^{n_{k_2}} \text{sgn}(v_m^{k_2}) \frac{1 - \text{sgn}(\delta_m^{k_2})}{2} - \sum_{m=1}^{n_{k_3}} \text{sgn}(v_m^{k_3}) \frac{1 - \text{sgn}(\delta_m^{k_3})}{2} \\ & + \sum_{m=1}^{n_{k_4}} \text{sgn}(v_m^{k_4}) \frac{1 - \text{sgn}(\delta_m^{k_4})}{2} \end{aligned} \quad (\text{S31.10})$$

$$\mathcal{W}_2^{\text{gapped}} = \sum_{m=1}^{n_{f_1}} \text{sgn}(v_m^{f_1}) \frac{1 - \text{sgn}(\delta_m^{f_1})}{2} - \sum_{m=1}^{n_{f_2}} \text{sgn}(v_m^{f_2}) \frac{1 - \text{sgn}(\delta_m^{f_2})}{2} \quad (\text{S31.11})$$

$$\mathcal{X}_1 = \sum_{m=1}^{n_{g_1}} \frac{1 - \text{sgn}(\delta_m^{g_1})}{2} + \sum_{m=1}^{n_{h_1}} \frac{1 - \text{sgn}(\delta_m^{h_1})}{2} + \sum_{m=1}^{n_{j_2}} \frac{1 - \text{sgn}(\delta_m^{j_2})}{2} + \sum_{m=1}^{n_{j_3}} \frac{1 - \text{sgn}(\delta_m^{j_3})}{2} \mod 2 \quad (\text{S31.12})$$

$$\mathcal{X}_2 = \sum_{m=1}^{n_{g_1}} \frac{1 - \text{sgn}(\delta_m^{g_1})}{2} + \sum_{m=1}^{n_{j_2}} \frac{1 - \text{sgn}(\delta_m^{j_2})}{2} + \sum_{m=1}^{n_{j_3}} \frac{1 - \text{sgn}(\delta_m^{j_3})}{2} + \sum_{m=1}^{n_{k_2}} \frac{1 - \text{sgn}(\delta_m^{k_2})}{2} + \sum_{m=1}^{n_{k_3}} \frac{1 - \text{sgn}(\delta_m^{k_3})}{2} \mod 2 \quad (\text{S31.13})$$

### S32. SPACE GROUP NO. 32

|              |                                      |
|--------------|--------------------------------------|
| line segment | character of irrep (generators only) |
|--------------|--------------------------------------|

|                                                     |                                                                                                                                                                 |
|-----------------------------------------------------|-----------------------------------------------------------------------------------------------------------------------------------------------------------------|
| $a \quad (\frac{t}{2}, 0, 0)$                       | $\begin{matrix} \{m_{010}   \frac{1}{2} \frac{1}{2} 0\} \\ a_1 \quad -ie^{-\frac{1}{2}i\pi t} \\ a_2 \quad ie^{-\frac{1}{2}i\pi t} \end{matrix}$                |
| $b \quad (0, \frac{t}{2}, 0)$                       | $\begin{matrix} \{m_{100}   \frac{1}{2} \frac{1}{2} 0\} \\ b_1 \quad -ie^{-\frac{1}{2}i\pi t} \\ b_2 \quad ie^{-\frac{1}{2}i\pi t} \end{matrix}$                |
| $c \quad (\frac{1}{2}, \frac{t}{2}, 0)$             | $\begin{matrix} \{m_{100}   \frac{1}{2} \frac{1}{2} 0\} \\ c_1 \quad -e^{-\frac{1}{2}i\pi(t+1)} \\ c_2 \quad e^{-\frac{1}{2}i\pi(t+1)} \end{matrix}$            |
| $d \quad (\frac{1-t}{2}, \frac{1}{2}, 0)$           | $\begin{matrix} \{m_{010}   \frac{1}{2} \frac{1}{2} 0\} \\ d_1 \quad -e^{-\frac{1}{2}i\pi(2-t)} \\ d_2 \quad e^{-\frac{1}{2}i\pi(2-t)} \end{matrix}$            |
| $e \quad (\frac{t}{2}, 0, \frac{1}{2})$             | $\begin{matrix} \{m_{010}   \frac{1}{2} \frac{1}{2} 0\} \\ e_1 \quad -ie^{-\frac{1}{2}i\pi t} \\ e_2 \quad ie^{-\frac{1}{2}i\pi t} \end{matrix}$                |
| $f \quad (0, \frac{t}{2}, \frac{1}{2})$             | $\begin{matrix} \{m_{100}   \frac{1}{2} \frac{1}{2} 0\} \\ f_1 \quad -ie^{-\frac{1}{2}i\pi t} \\ f_2 \quad ie^{-\frac{1}{2}i\pi t} \end{matrix}$                |
| $g \quad (\frac{1}{2}, \frac{t}{2}, \frac{1}{2})$   | $\begin{matrix} \{m_{100}   \frac{1}{2} \frac{1}{2} 0\} \\ g_1 \quad -e^{-\frac{1}{2}i\pi(t+1)} \\ g_2 \quad e^{-\frac{1}{2}i\pi(t+1)} \end{matrix}$            |
| $h \quad (\frac{1-t}{2}, \frac{1}{2}, \frac{1}{2})$ | $\begin{matrix} \{m_{010}   \frac{1}{2} \frac{1}{2} 0\} \\ h_1 \quad -e^{-\frac{1}{2}i\pi(2-t)} \\ h_2 \quad e^{-\frac{1}{2}i\pi(2-t)} \end{matrix}$            |
| $i \quad (0, 0, \frac{t}{2})$                       | $\begin{matrix} \{2_{001}   0 \ 0 \ 0\} & \{m_{100}   \frac{1}{2} \frac{1}{2} 0\} \\ i_1 & 0 \end{matrix}$                                                      |
| $j \quad (\frac{1}{2}, 0, \frac{t}{2})$             | $\begin{matrix} \{2_{001}   0 \ 0 \ 0\} & \{m_{100}   \frac{1}{2} \frac{1}{2} 0\} \\ j_1 & -i & i \\ j_2 & -i & -i \\ j_3 & i & i \\ j_4 & i & -i \end{matrix}$ |
| $k \quad (\frac{1}{2}, \frac{1}{2}, \frac{t}{2})$   | $\begin{matrix} \{2_{001}   0 \ 0 \ 0\} & \{m_{100}   \frac{1}{2} \frac{1}{2} 0\} \\ k_1 & 0 \end{matrix}$                                                      |
| $l \quad (0, \frac{1}{2}, \frac{t}{2})$             | $\begin{matrix} \{2_{001}   0 \ 0 \ 0\} & \{m_{100}   \frac{1}{2} \frac{1}{2} 0\} \\ l_1 & -i & -1 \\ l_2 & -i & 1 \\ l_3 & i & -1 \\ l_4 & i & 1 \end{matrix}$ |

$$\begin{aligned}
\mathcal{W}_1^{\text{gapless}} = & \sum_{m=1}^{n_{a_1}} \text{sgn}(v_m^{a_1}) \frac{1 - \text{sgn}(\delta_m^{a_1})}{2} + \sum_{m=1}^{n_{e_2}} \text{sgn}(v_m^{e_2}) \frac{1 - \text{sgn}(\delta_m^{e_2})}{2} - \sum_{m=1}^{n_{f_1}} \text{sgn}(v_m^{f_1}) \frac{1 - \text{sgn}(\delta_m^{f_1})}{2} - \sum_{m=1}^{n_{f_2}} \text{sgn}(v_m^{f_2}) \frac{1 - \text{sgn}(\delta_m^{f_2})}{2} \\
& + 2 \sum_{m=1}^{n_{g_1}} \text{sgn}(v_m^{g_1}) \frac{1 - \text{sgn}(\delta_m^{g_1})}{2} + 2 \sum_{m=1}^{n_{h_1}} \text{sgn}(v_m^{h_1}) \frac{1 - \text{sgn}(\delta_m^{h_1})}{2} - \sum_{m=1}^{n_{i_1}} \text{sgn}(v_m^{i_1}) \frac{1 - \text{sgn}(\delta_m^{i_1})}{2} \\
& + \sum_{m=1}^{n_{j_2}} \text{sgn}(v_m^{j_2}) \frac{1 - \text{sgn}(\delta_m^{j_2})}{2} - \sum_{m=1}^{n_{j_3}} \text{sgn}(v_m^{j_3}) \frac{1 - \text{sgn}(\delta_m^{j_3})}{2} + 2 \sum_{m=1}^{n_{j_4}} \text{sgn}(v_m^{j_4}) \frac{1 - \text{sgn}(\delta_m^{j_4})}{2}
\end{aligned}$$

(S32.1)

$$\begin{aligned}\mathcal{W}_2^{\text{gapless}} = & \sum_{m=1}^{n_{a_2}} \text{sgn}(v_m^{a_2}) \frac{1 - \text{sgn}(\delta_m^{a_2})}{2} - \sum_{m=1}^{n_{e_2}} \text{sgn}(v_m^{e_2}) \frac{1 - \text{sgn}(\delta_m^{e_2})}{2} - \sum_{m=1}^{n_{i_1}} \text{sgn}(v_m^{i_1}) \frac{1 - \text{sgn}(\delta_m^{i_1})}{2} \\ & + \sum_{m=1}^{n_{j_2}} \text{sgn}(v_m^{j_2}) \frac{1 - \text{sgn}(\delta_m^{j_2})}{2} + \sum_{m=1}^{n_{j_3}} \text{sgn}(v_m^{j_3}) \frac{1 - \text{sgn}(\delta_m^{j_3})}{2}\end{aligned}\quad (\text{S32.2})$$

$$\begin{aligned}\mathcal{W}_3^{\text{gapless}} = & \sum_{m=1}^{n_{b_1}} \text{sgn}(v_m^{b_1}) \frac{1 - \text{sgn}(\delta_m^{b_1})}{2} - \sum_{m=1}^{n_{f_1}} \text{sgn}(v_m^{f_1}) \frac{1 - \text{sgn}(\delta_m^{f_1})}{2} - \sum_{m=1}^{n_{i_1}} \text{sgn}(v_m^{i_1}) \frac{1 - \text{sgn}(\delta_m^{i_1})}{2} \\ & + \sum_{m=1}^{n_{l_2}} \text{sgn}(v_m^{l_2}) \frac{1 - \text{sgn}(\delta_m^{l_2})}{2} + 2 \sum_{m=1}^{n_{l_3}} \text{sgn}(v_m^{l_3}) \frac{1 - \text{sgn}(\delta_m^{l_3})}{2} - \sum_{m=1}^{n_{l_4}} \text{sgn}(v_m^{l_4}) \frac{1 - \text{sgn}(\delta_m^{l_4})}{2}\end{aligned}\quad (\text{S32.3})$$

$$\begin{aligned}\mathcal{W}_4^{\text{gapless}} = & \sum_{m=1}^{n_{b_2}} \text{sgn}(v_m^{b_2}) \frac{1 - \text{sgn}(\delta_m^{b_2})}{2} - \sum_{m=1}^{n_{f_2}} \text{sgn}(v_m^{f_2}) \frac{1 - \text{sgn}(\delta_m^{f_2})}{2} - \sum_{m=1}^{n_{i_1}} \text{sgn}(v_m^{i_1}) \frac{1 - \text{sgn}(\delta_m^{i_1})}{2} \\ & + \sum_{m=1}^{n_{l_2}} \text{sgn}(v_m^{l_2}) \frac{1 - \text{sgn}(\delta_m^{l_2})}{2} + \sum_{m=1}^{n_{l_4}} \text{sgn}(v_m^{l_4}) \frac{1 - \text{sgn}(\delta_m^{l_4})}{2}\end{aligned}\quad (\text{S32.4})$$

$$\begin{aligned}\mathcal{W}_5^{\text{gapless}} = & \sum_{m=1}^{n_{c_1}} \text{sgn}(v_m^{c_1}) \frac{1 - \text{sgn}(\delta_m^{c_1})}{2} - \sum_{m=1}^{n_{g_1}} \text{sgn}(v_m^{g_1}) \frac{1 - \text{sgn}(\delta_m^{g_1})}{2} - \sum_{m=1}^{n_{j_2}} \text{sgn}(v_m^{j_2}) \frac{1 - \text{sgn}(\delta_m^{j_2})}{2} \\ & - \sum_{m=1}^{n_{j_4}} \text{sgn}(v_m^{j_4}) \frac{1 - \text{sgn}(\delta_m^{j_4})}{2} + \sum_{m=1}^{n_{k_1}} \text{sgn}(v_m^{k_1}) \frac{1 - \text{sgn}(\delta_m^{k_1})}{2}\end{aligned}\quad (\text{S32.5})$$

$$\begin{aligned}\mathcal{W}_6^{\text{gapless}} = & \sum_{m=1}^{n_{d_1}} \text{sgn}(v_m^{d_1}) \frac{1 - \text{sgn}(\delta_m^{d_1})}{2} - \sum_{m=1}^{n_{h_1}} \text{sgn}(v_m^{h_1}) \frac{1 - \text{sgn}(\delta_m^{h_1})}{2} - \sum_{m=1}^{n_{k_1}} \text{sgn}(v_m^{k_1}) \frac{1 - \text{sgn}(\delta_m^{k_1})}{2} \\ & + \sum_{m=1}^{n_{l_2}} \text{sgn}(v_m^{l_2}) \frac{1 - \text{sgn}(\delta_m^{l_2})}{2} + \sum_{m=1}^{n_{l_3}} \text{sgn}(v_m^{l_3}) \frac{1 - \text{sgn}(\delta_m^{l_3})}{2}\end{aligned}\quad (\text{S32.6})$$

$$\begin{aligned}\mathcal{W}_7^{\text{gapless}} = & \sum_{m=1}^{n_{e_1}} \text{sgn}(v_m^{e_1}) \frac{1 - \text{sgn}(\delta_m^{e_1})}{2} + \sum_{m=1}^{n_{e_2}} \text{sgn}(v_m^{e_2}) \frac{1 - \text{sgn}(\delta_m^{e_2})}{2} - \sum_{m=1}^{n_{f_1}} \text{sgn}(v_m^{f_1}) \frac{1 - \text{sgn}(\delta_m^{f_1})}{2} \\ & - \sum_{m=1}^{n_{f_2}} \text{sgn}(v_m^{f_2}) \frac{1 - \text{sgn}(\delta_m^{f_2})}{2} + 2 \sum_{m=1}^{n_{g_1}} \text{sgn}(v_m^{g_1}) \frac{1 - \text{sgn}(\delta_m^{g_1})}{2} + 2 \sum_{m=1}^{n_{h_1}} \text{sgn}(v_m^{h_1}) \frac{1 - \text{sgn}(\delta_m^{h_1})}{2}\end{aligned}\quad (\text{S32.7})$$

$$\begin{aligned}\mathcal{W}_8^{\text{gapless}} = & \sum_{m=1}^{n_{j_1}} \text{sgn}(v_m^{j_1}) \frac{1 - \text{sgn}(\delta_m^{j_1})}{2} - \sum_{m=1}^{n_{j_2}} \text{sgn}(v_m^{j_2}) \frac{1 - \text{sgn}(\delta_m^{j_2})}{2} + \sum_{m=1}^{n_{j_3}} \text{sgn}(v_m^{j_3}) \frac{1 - \text{sgn}(\delta_m^{j_3})}{2} - \sum_{m=1}^{n_{j_4}} \text{sgn}(v_m^{j_4}) \frac{1 - \text{sgn}(\delta_m^{j_4})}{2}\end{aligned}\quad (\text{S32.8})$$

$$\begin{aligned}\mathcal{W}_9^{\text{gapless}} = & \sum_{m=1}^{n_{l_1}} \text{sgn}(v_m^{l_1}) \frac{1 - \text{sgn}(\delta_m^{l_1})}{2} - \sum_{m=1}^{n_{l_2}} \text{sgn}(v_m^{l_2}) \frac{1 - \text{sgn}(\delta_m^{l_2})}{2} - \sum_{m=1}^{n_{l_3}} \text{sgn}(v_m^{l_3}) \frac{1 - \text{sgn}(\delta_m^{l_3})}{2} + \sum_{m=1}^{n_{l_4}} \text{sgn}(v_m^{l_4}) \frac{1 - \text{sgn}(\delta_m^{l_4})}{2}\end{aligned}\quad (\text{S32.9})$$

$$\mathcal{W}_1^{\text{gapped}} = - \sum_{m=1}^{n_{j_2}} \text{sgn}(v_m^{j_2}) \frac{1 - \text{sgn}(\delta_m^{j_2})}{2} + \sum_{m=1}^{n_{j_3}} \text{sgn}(v_m^{j_3}) \frac{1 - \text{sgn}(\delta_m^{j_3})}{2} \quad (\text{S32.10})$$

$$\mathcal{W}_2^{\text{gapped}} = - \sum_{m=1}^{n_{l_2}} \text{sgn}(v_m^{l_2}) \frac{1 - \text{sgn}(\delta_m^{l_2})}{2} + \sum_{m=1}^{n_{l_4}} \text{sgn}(v_m^{l_4}) \frac{1 - \text{sgn}(\delta_m^{l_4})}{2} \quad (\text{S32.11})$$

$$\mathcal{X}_1 = \sum_{m=1}^{n_{e_2}} \frac{1 - \text{sgn}(\delta_m^{e_2})}{2} + \sum_{m=1}^{n_{f_2}} \frac{1 - \text{sgn}(\delta_m^{f_2})}{2} \quad \text{mod } 2 \quad (\text{S32.12})$$

$$\mathcal{X}_2 = \sum_{m=1}^{n_{k_1}} \frac{1 - \text{sgn}(\delta_m^{k_1})}{2} \quad \text{mod } 2 \quad (\text{S32.13})$$

$$\begin{aligned} \mathcal{X}_3 = & \sum_{m=1}^{n_{f_1}} \text{sgn}(v_m^{f_1}) \frac{1 - \text{sgn}(\delta_m^{f_1})}{2} - \sum_{m=1}^{n_{f_2}} \text{sgn}(v_m^{f_2}) \frac{1 - \text{sgn}(\delta_m^{f_2})}{2} - 2 \sum_{m=1}^{n_{h_1}} \text{sgn}(v_m^{h_1}) \frac{1 - \text{sgn}(\delta_m^{h_1})}{2} \\ & - 2 \sum_{m=1}^{n_{k_1}} \text{sgn}(v_m^{k_1}) \frac{1 - \text{sgn}(\delta_m^{k_1})}{2} \quad \text{mod } 4 \end{aligned} \quad (\text{S32.14})$$

### S33. SPACE GROUP NO. 33

| line segment                                        | character of irrep (generators only)                                                                                                     |
|-----------------------------------------------------|------------------------------------------------------------------------------------------------------------------------------------------|
| $a \quad (\frac{t}{2}, 0, 0)$                       | $\{m_{010}   \frac{1}{2} \frac{1}{2} 0\}$<br>$a_1 \quad -ie^{-\frac{1}{2}i\pi t}$<br>$a_2 \quad ie^{-\frac{1}{2}i\pi t}$                 |
| $b \quad (0, \frac{t}{2}, 0)$                       | $\{m_{100}   \frac{1}{2} \frac{1}{2} \frac{1}{2}\}$<br>$b_1 \quad -ie^{-\frac{1}{2}i\pi t}$<br>$b_2 \quad ie^{-\frac{1}{2}i\pi t}$       |
| $c \quad (\frac{1}{2}, \frac{t}{2}, 0)$             | $\{m_{100}   \frac{1}{2} \frac{1}{2} \frac{1}{2}\}$<br>$c_1 \quad -e^{-\frac{1}{2}i\pi(t+1)}$<br>$c_2 \quad e^{-\frac{1}{2}i\pi(t+1)}$   |
| $d \quad (\frac{1-t}{2}, \frac{1}{2}, 0)$           | $\{m_{010}   \frac{1}{2} \frac{1}{2} 0\}$<br>$d_1 \quad -e^{-\frac{1}{2}i\pi(2-t)}$<br>$d_2 \quad e^{-\frac{1}{2}i\pi(2-t)}$             |
| $e \quad (\frac{t}{2}, 0, \frac{1}{2})$             | $\{m_{010}   \frac{1}{2} \frac{1}{2} 0\}$<br>$e_1 \quad -ie^{-\frac{1}{2}i\pi t}$<br>$e_2 \quad ie^{-\frac{1}{2}i\pi t}$                 |
| $f \quad (0, \frac{t}{2}, \frac{1}{2})$             | $\{m_{100}   \frac{1}{2} \frac{1}{2} \frac{1}{2}\}$<br>$f_1 \quad -ie^{-\frac{1}{2}i\pi(t+1)}$<br>$f_2 \quad ie^{-\frac{1}{2}i\pi(t+1)}$ |
| $g \quad (\frac{1}{2}, \frac{t}{2}, \frac{1}{2})$   | $\{m_{100}   \frac{1}{2} \frac{1}{2} \frac{1}{2}\}$<br>$g_1 \quad -e^{-\frac{1}{2}i\pi(t+2)}$<br>$g_2 \quad e^{-\frac{1}{2}i\pi(t+2)}$   |
| $h \quad (\frac{1-t}{2}, \frac{1}{2}, \frac{1}{2})$ | $\{m_{010}   \frac{1}{2} \frac{1}{2} 0\}$<br>$h_1 \quad -e^{-\frac{1}{2}i\pi(2-t)}$<br>$h_2 \quad e^{-\frac{1}{2}i\pi(2-t)}$             |

|                                                   |       |                                     |                                                         |
|---------------------------------------------------|-------|-------------------------------------|---------------------------------------------------------|
| $i \quad (0, 0, \frac{t}{2})$                     | $i_1$ | $\{2_{001}   0 \ 0 \ \frac{1}{2}\}$ | $\{m_{100}   \frac{1}{2} \ \frac{1}{2} \ \frac{1}{2}\}$ |
|                                                   |       | 0                                   | 0                                                       |
| $j \quad (\frac{1}{2}, 0, \frac{t}{2})$           | $j_1$ | $\{2_{001}   0 \ 0 \ \frac{1}{2}\}$ | $\{m_{100}   \frac{1}{2} \ \frac{1}{2} \ \frac{1}{2}\}$ |
|                                                   |       | $-ie^{-\frac{1}{2}i\pi t}$          | $-e^{-\frac{1}{2}i\pi(t+1)}$                            |
|                                                   | $j_2$ | $-ie^{-\frac{1}{2}i\pi t}$          | $e^{-\frac{1}{2}i\pi(t+1)}$                             |
|                                                   | $j_3$ | $ie^{-\frac{1}{2}i\pi t}$           | $-e^{-\frac{1}{2}i\pi(t+1)}$                            |
|                                                   | $j_4$ | $ie^{-\frac{1}{2}i\pi t}$           | $e^{-\frac{1}{2}i\pi(t+1)}$                             |
| $k \quad (\frac{1}{2}, \frac{1}{2}, \frac{t}{2})$ | $k_1$ | $\{2_{001}   0 \ 0 \ \frac{1}{2}\}$ | $\{m_{100}   \frac{1}{2} \ \frac{1}{2} \ \frac{1}{2}\}$ |
|                                                   |       | 0                                   | 0                                                       |
| $l \quad (0, \frac{1}{2}, \frac{t}{2})$           | $l_1$ | $\{2_{001}   0 \ 0 \ \frac{1}{2}\}$ | $\{m_{100}   \frac{1}{2} \ \frac{1}{2} \ \frac{1}{2}\}$ |
|                                                   |       | $-ie^{-\frac{1}{2}i\pi t}$          | $-ie^{-\frac{1}{2}i\pi(t+1)}$                           |
|                                                   | $l_2$ | $-ie^{-\frac{1}{2}i\pi t}$          | $ie^{-\frac{1}{2}i\pi(t+1)}$                            |
|                                                   | $l_3$ | $ie^{-\frac{1}{2}i\pi t}$           | $-ie^{-\frac{1}{2}i\pi(t+1)}$                           |
|                                                   | $l_4$ | $ie^{-\frac{1}{2}i\pi t}$           | $ie^{-\frac{1}{2}i\pi(t+1)}$                            |

$$\begin{aligned}
\mathcal{W}_1^{\text{gapless}} = & \sum_{m=1}^{n_{a_1}} \text{sgn}(v_m^{a_1}) \frac{1 - \text{sgn}(\delta_m^{a_1})}{2} + 2 \sum_{m=1}^{n_{e_2}} \text{sgn}(v_m^{e_2}) \frac{1 - \text{sgn}(\delta_m^{e_2})}{2} - 2 \sum_{m=1}^{n_{f_1}} \text{sgn}(v_m^{f_1}) \frac{1 - \text{sgn}(\delta_m^{f_1})}{2} \\
& + 4 \sum_{m=1}^{n_{g_2}} \text{sgn}(v_m^{g_2}) \frac{1 - \text{sgn}(\delta_m^{g_2})}{2} + 2 \sum_{m=1}^{n_{h_1}} \text{sgn}(v_m^{h_1}) \frac{1 - \text{sgn}(\delta_m^{h_1})}{2} - \sum_{m=1}^{n_{i_1}} \text{sgn}(v_m^{i_1}) \frac{1 - \text{sgn}(\delta_m^{i_1})}{2} \\
& + \sum_{m=1}^{n_{j_2}} \text{sgn}(v_m^{j_2}) \frac{1 - \text{sgn}(\delta_m^{j_2})}{2} - \sum_{m=1}^{n_{j_3}} \text{sgn}(v_m^{j_3}) \frac{1 - \text{sgn}(\delta_m^{j_3})}{2} + 2 \sum_{m=1}^{n_{j_4}} \text{sgn}(v_m^{j_4}) \frac{1 - \text{sgn}(\delta_m^{j_4})}{2}
\end{aligned} \tag{S33.1}$$

$$\begin{aligned}
\mathcal{W}_2^{\text{gapless}} = & \sum_{m=1}^{n_{a_2}} \text{sgn}(v_m^{a_2}) \frac{1 - \text{sgn}(\delta_m^{a_2})}{2} - 2 \sum_{m=1}^{n_{e_2}} \text{sgn}(v_m^{e_2}) \frac{1 - \text{sgn}(\delta_m^{e_2})}{2} - \sum_{m=1}^{n_{i_1}} \text{sgn}(v_m^{i_1}) \frac{1 - \text{sgn}(\delta_m^{i_1})}{2} \\
& + \sum_{m=1}^{n_{j_2}} \text{sgn}(v_m^{j_2}) \frac{1 - \text{sgn}(\delta_m^{j_2})}{2} + \sum_{m=1}^{n_{j_3}} \text{sgn}(v_m^{j_3}) \frac{1 - \text{sgn}(\delta_m^{j_3})}{2}
\end{aligned} \tag{S33.2}$$

$$\begin{aligned}
\mathcal{W}_3^{\text{gapless}} = & \sum_{m=1}^{n_{b_1}} \text{sgn}(v_m^{b_1}) \frac{1 - \text{sgn}(\delta_m^{b_1})}{2} - \sum_{m=1}^{n_{f_1}} \text{sgn}(v_m^{f_1}) \frac{1 - \text{sgn}(\delta_m^{f_1})}{2} - \sum_{m=1}^{n_{i_1}} \text{sgn}(v_m^{i_1}) \frac{1 - \text{sgn}(\delta_m^{i_1})}{2} \\
& + \sum_{m=1}^{n_{l_2}} \text{sgn}(v_m^{l_2}) \frac{1 - \text{sgn}(\delta_m^{l_2})}{2} + 2 \sum_{m=1}^{n_{l_3}} \text{sgn}(v_m^{l_3}) \frac{1 - \text{sgn}(\delta_m^{l_3})}{2} - \sum_{m=1}^{n_{l_4}} \text{sgn}(v_m^{l_4}) \frac{1 - \text{sgn}(\delta_m^{l_4})}{2}
\end{aligned} \tag{S33.3}$$

$$\begin{aligned}
\mathcal{W}_4^{\text{gapless}} = & \sum_{m=1}^{n_{b_2}} \text{sgn}(v_m^{b_2}) \frac{1 - \text{sgn}(\delta_m^{b_2})}{2} - \sum_{m=1}^{n_{f_1}} \text{sgn}(v_m^{f_1}) \frac{1 - \text{sgn}(\delta_m^{f_1})}{2} - \sum_{m=1}^{n_{i_1}} \text{sgn}(v_m^{i_1}) \frac{1 - \text{sgn}(\delta_m^{i_1})}{2} \\
& + \sum_{m=1}^{n_{l_2}} \text{sgn}(v_m^{l_2}) \frac{1 - \text{sgn}(\delta_m^{l_2})}{2} + \sum_{m=1}^{n_{l_4}} \text{sgn}(v_m^{l_4}) \frac{1 - \text{sgn}(\delta_m^{l_4})}{2}
\end{aligned} \tag{S33.4}$$

$$\begin{aligned}
\mathcal{W}_5^{\text{gapless}} = & \sum_{m=1}^{n_{c_1}} \text{sgn}(v_m^{c_1}) \frac{1 - \text{sgn}(\delta_m^{c_1})}{2} - 2 \sum_{m=1}^{n_{g_2}} \text{sgn}(v_m^{g_2}) \frac{1 - \text{sgn}(\delta_m^{g_2})}{2} - \sum_{m=1}^{n_{j_2}} \text{sgn}(v_m^{j_2}) \frac{1 - \text{sgn}(\delta_m^{j_2})}{2} \\
& - \sum_{m=1}^{n_{j_4}} \text{sgn}(v_m^{j_4}) \frac{1 - \text{sgn}(\delta_m^{j_4})}{2} + \sum_{m=1}^{n_{k_1}} \text{sgn}(v_m^{k_1}) \frac{1 - \text{sgn}(\delta_m^{k_1})}{2}
\end{aligned} \tag{S33.5}$$



$$\begin{aligned} \mathcal{W}_6^{\text{gapless}} = & \sum_{m=1}^{n_{d_1}} \text{sgn}(v_m^{d_1}) \frac{1 - \text{sgn}(\delta_m^{d_1})}{2} - \sum_{m=1}^{n_{h_1}} \text{sgn}(v_m^{h_1}) \frac{1 - \text{sgn}(\delta_m^{h_1})}{2} - \sum_{m=1}^{n_{k_1}} \text{sgn}(v_m^{k_1}) \frac{1 - \text{sgn}(\delta_m^{k_1})}{2} \\ & + \sum_{m=1}^{n_{l_2}} \text{sgn}(v_m^{l_2}) \frac{1 - \text{sgn}(\delta_m^{l_2})}{2} + \sum_{m=1}^{n_{l_3}} \text{sgn}(v_m^{l_3}) \frac{1 - \text{sgn}(\delta_m^{l_3})}{2} \end{aligned} \quad (\text{S33.6})$$

$$\begin{aligned} \mathcal{W}_7^{\text{gapless}} = & \sum_{m=1}^{n_{e_1}} \text{sgn}(v_m^{e_1}) \frac{1 - \text{sgn}(\delta_m^{e_1})}{2} + \sum_{m=1}^{n_{e_2}} \text{sgn}(v_m^{e_2}) \frac{1 - \text{sgn}(\delta_m^{e_2})}{2} - \sum_{m=1}^{n_{f_1}} \text{sgn}(v_m^{f_1}) \frac{1 - \text{sgn}(\delta_m^{f_1})}{2} \\ & + \sum_{m=1}^{n_{g_1}} \text{sgn}(v_m^{g_1}) \frac{1 - \text{sgn}(\delta_m^{g_1})}{2} + \sum_{m=1}^{n_{g_2}} \text{sgn}(v_m^{g_2}) \frac{1 - \text{sgn}(\delta_m^{g_2})}{2} + \sum_{m=1}^{n_{h_1}} \text{sgn}(v_m^{h_1}) \frac{1 - \text{sgn}(\delta_m^{h_1})}{2} \end{aligned} \quad (\text{S33.7})$$

$$\begin{aligned} \mathcal{W}_8^{\text{gapless}} = & 2 \sum_{m=1}^{n_{g_1}} \text{sgn}(v_m^{g_1}) \frac{1 - \text{sgn}(\delta_m^{g_1})}{2} - 2 \sum_{m=1}^{n_{g_2}} \text{sgn}(v_m^{g_2}) \frac{1 - \text{sgn}(\delta_m^{g_2})}{2} + \sum_{m=1}^{n_{j_1}} \text{sgn}(v_m^{j_1}) \frac{1 - \text{sgn}(\delta_m^{j_1})}{2} \\ & - \sum_{m=1}^{n_{j_2}} \text{sgn}(v_m^{j_2}) \frac{1 - \text{sgn}(\delta_m^{j_2})}{2} + \sum_{m=1}^{n_{j_3}} \text{sgn}(v_m^{j_3}) \frac{1 - \text{sgn}(\delta_m^{j_3})}{2} - \sum_{m=1}^{n_{j_4}} \text{sgn}(v_m^{j_4}) \frac{1 - \text{sgn}(\delta_m^{j_4})}{2} \end{aligned} \quad (\text{S33.8})$$

$$\begin{aligned} \mathcal{W}_9^{\text{gapless}} = & \sum_{m=1}^{n_{l_1}} \text{sgn}(v_m^{l_1}) \frac{1 - \text{sgn}(\delta_m^{l_1})}{2} - \sum_{m=1}^{n_{l_2}} \text{sgn}(v_m^{l_2}) \frac{1 - \text{sgn}(\delta_m^{l_2})}{2} - \sum_{m=1}^{n_{l_3}} \text{sgn}(v_m^{l_3}) \frac{1 - \text{sgn}(\delta_m^{l_3})}{2} + \sum_{m=1}^{n_{l_4}} \text{sgn}(v_m^{l_4}) \frac{1 - \text{sgn}(\delta_m^{l_4})}{2} \end{aligned} \quad (\text{S33.9})$$

$$\mathcal{X}_1 = \sum_{m=1}^{n_{j_2}} \frac{1 - \text{sgn}(\delta_m^{j_2})}{2} + \sum_{m=1}^{n_{j_3}} \frac{1 - \text{sgn}(\delta_m^{j_3})}{2} + \sum_{m=1}^{n_{k_1}} \frac{1 - \text{sgn}(\delta_m^{k_1})}{2} \quad \text{mod } 2 \quad (\text{S33.10})$$

$$\mathcal{X}_2 = \sum_{m=1}^{n_{f_1}} \frac{1 - \text{sgn}(\delta_m^{f_1})}{2} + \sum_{m=1}^{n_{h_1}} \frac{1 - \text{sgn}(\delta_m^{h_1})}{2} + \sum_{m=1}^{n_{j_2}} \frac{1 - \text{sgn}(\delta_m^{j_2})}{2} + \sum_{m=1}^{n_{j_3}} \frac{1 - \text{sgn}(\delta_m^{j_3})}{2} + \sum_{m=1}^{n_{k_1}} \frac{1 - \text{sgn}(\delta_m^{k_1})}{2} \quad \text{mod } 2 \quad (\text{S33.11})$$

$$\mathcal{X}_3 = \sum_{m=1}^{n_{k_1}} \frac{1 - \text{sgn}(\delta_m^{k_1})}{2} \quad \text{mod } 2 \quad (\text{S33.12})$$

$$\mathcal{X}_4 = \sum_{m=1}^{n_{h_1}} \frac{1 - \text{sgn}(\delta_m^{h_1})}{2} + \sum_{m=1}^{n_{k_1}} \frac{1 - \text{sgn}(\delta_m^{k_1})}{2} + \sum_{m=1}^{n_{l_2}} \frac{1 - \text{sgn}(\delta_m^{l_2})}{2} + \sum_{m=1}^{n_{l_4}} \frac{1 - \text{sgn}(\delta_m^{l_4})}{2} \quad \text{mod } 2 \quad (\text{S33.13})$$

### S34. SPACE GROUP NO. 34

|              |                                      |
|--------------|--------------------------------------|
| line segment | character of irrep (generators only) |
|--------------|--------------------------------------|

|                                                     |                                                                                                                                                                                                                                                                                               |
|-----------------------------------------------------|-----------------------------------------------------------------------------------------------------------------------------------------------------------------------------------------------------------------------------------------------------------------------------------------------|
| $a \quad (\frac{t}{2}, 0, 0)$                       | $a_1 \quad \{m_{010}   \frac{1}{2} \frac{1}{2} \frac{1}{2}\}$<br>$-ie^{-\frac{1}{2}i\pi t}$<br>$a_2 \quad ie^{-\frac{1}{2}i\pi t}$                                                                                                                                                            |
| $b \quad (0, \frac{t}{2}, 0)$                       | $b_1 \quad \{m_{100}   \frac{1}{2} \frac{1}{2} \frac{1}{2}\}$<br>$-ie^{-\frac{1}{2}i\pi t}$<br>$b_2 \quad ie^{-\frac{1}{2}i\pi t}$                                                                                                                                                            |
| $c \quad (\frac{1}{2}, \frac{t}{2}, 0)$             | $c_1 \quad \{m_{100}   \frac{1}{2} \frac{1}{2} \frac{1}{2}\}$<br>$-e^{-\frac{1}{2}i\pi(t+1)}$<br>$c_2 \quad e^{-\frac{1}{2}i\pi(t+1)}$                                                                                                                                                        |
| $d \quad (\frac{1-t}{2}, \frac{1}{2}, 0)$           | $d_1 \quad \{m_{010}   \frac{1}{2} \frac{1}{2} \frac{1}{2}\}$<br>$-e^{-\frac{1}{2}i\pi(2-t)}$<br>$d_2 \quad e^{-\frac{1}{2}i\pi(2-t)}$                                                                                                                                                        |
| $e \quad (\frac{t}{2}, 0, \frac{1}{2})$             | $e_1 \quad \{m_{010}   \frac{1}{2} \frac{1}{2} \frac{1}{2}\}$<br>$-ie^{-\frac{1}{2}i\pi(t+1)}$<br>$e_2 \quad ie^{-\frac{1}{2}i\pi(t+1)}$                                                                                                                                                      |
| $f \quad (0, \frac{t}{2}, \frac{1}{2})$             | $f_1 \quad \{m_{100}   \frac{1}{2} \frac{1}{2} \frac{1}{2}\}$<br>$-ie^{-\frac{1}{2}i\pi(t+1)}$<br>$f_2 \quad ie^{-\frac{1}{2}i\pi(t+1)}$                                                                                                                                                      |
| $g \quad (\frac{1}{2}, \frac{t}{2}, \frac{1}{2})$   | $g_1 \quad \{m_{100}   \frac{1}{2} \frac{1}{2} \frac{1}{2}\}$<br>$-e^{-\frac{1}{2}i\pi(t+2)}$<br>$g_2 \quad e^{-\frac{1}{2}i\pi(t+2)}$                                                                                                                                                        |
| $h \quad (\frac{1-t}{2}, \frac{1}{2}, \frac{1}{2})$ | $h_1 \quad \{m_{010}   \frac{1}{2} \frac{1}{2} \frac{1}{2}\}$<br>$-e^{-\frac{1}{2}i\pi(3-t)}$<br>$h_2 \quad e^{-\frac{1}{2}i\pi(3-t)}$                                                                                                                                                        |
| $i \quad (0, 0, \frac{t}{2})$                       | $i_1 \quad \{2_{001}   0 \ 0 \ 0\} \quad \{m_{100}   \frac{1}{2} \frac{1}{2} \frac{1}{2}\}$<br>$0 \quad 0$                                                                                                                                                                                    |
| $j \quad (\frac{1}{2}, 0, \frac{t}{2})$             | $j_1 \quad \{2_{001}   0 \ 0 \ 0\} \quad \{m_{100}   \frac{1}{2} \frac{1}{2} \frac{1}{2}\}$<br>$-i \quad -e^{-\frac{1}{2}i\pi(t+1)}$<br>$j_2 \quad -i \quad e^{-\frac{1}{2}i\pi(t+1)}$<br>$j_3 \quad i \quad -e^{-\frac{1}{2}i\pi(t+1)}$<br>$j_4 \quad i \quad e^{-\frac{1}{2}i\pi(t+1)}$     |
| $k \quad (\frac{1}{2}, \frac{1}{2}, \frac{t}{2})$   | $k_1 \quad \{2_{001}   0 \ 0 \ 0\} \quad \{m_{100}   \frac{1}{2} \frac{1}{2} \frac{1}{2}\}$<br>$0 \quad 0$                                                                                                                                                                                    |
| $l \quad (0, \frac{1}{2}, \frac{t}{2})$             | $l_1 \quad \{2_{001}   0 \ 0 \ 0\} \quad \{m_{100}   \frac{1}{2} \frac{1}{2} \frac{1}{2}\}$<br>$-i \quad -ie^{-\frac{1}{2}i\pi(t+1)}$<br>$l_2 \quad -i \quad ie^{-\frac{1}{2}i\pi(t+1)}$<br>$l_3 \quad i \quad -ie^{-\frac{1}{2}i\pi(t+1)}$<br>$l_4 \quad i \quad ie^{-\frac{1}{2}i\pi(t+1)}$ |

$$\begin{aligned}
\mathcal{W}_1^{\text{gapless}} = & \sum_{m=1}^{n_{a_1}} \text{sgn}(v_m^{a_1}) \frac{1 - \text{sgn}(\delta_m^{a_1})}{2} + \sum_{m=1}^{n_{e_1}} \text{sgn}(v_m^{e_1}) \frac{1 - \text{sgn}(\delta_m^{e_1})}{2} - 2 \sum_{m=1}^{n_{f_1}} \text{sgn}(v_m^{f_1}) \frac{1 - \text{sgn}(\delta_m^{f_1})}{2} \\
& + 2 \sum_{m=1}^{n_{g_2}} \text{sgn}(v_m^{g_2}) \frac{1 - \text{sgn}(\delta_m^{g_2})}{2} + 2 \sum_{m=1}^{n_{h_2}} \text{sgn}(v_m^{h_2}) \frac{1 - \text{sgn}(\delta_m^{h_2})}{2} - \sum_{m=1}^{n_{i_1}} \text{sgn}(v_m^{i_1}) \frac{1 - \text{sgn}(\delta_m^{i_1})}{2} \\
& + \sum_{m=1}^{n_{j_2}} \text{sgn}(v_m^{j_2}) \frac{1 - \text{sgn}(\delta_m^{j_2})}{2} - \sum_{m=1}^{n_{j_3}} \text{sgn}(v_m^{j_3}) \frac{1 - \text{sgn}(\delta_m^{j_3})}{2} + 2 \sum_{m=1}^{n_{j_4}} \text{sgn}(v_m^{j_4}) \frac{1 - \text{sgn}(\delta_m^{j_4})}{2} \\
& - \sum_{m=1}^{n_{l_1}} \text{sgn}(v_m^{l_1}) \frac{1 - \text{sgn}(\delta_m^{l_1})}{2} + \sum_{m=1}^{n_{l_2}} \text{sgn}(v_m^{l_2}) \frac{1 - \text{sgn}(\delta_m^{l_2})}{2} + \sum_{m=1}^{n_{l_3}} \text{sgn}(v_m^{l_3}) \frac{1 - \text{sgn}(\delta_m^{l_3})}{2} - \sum_{m=1}^{n_{l_4}} \text{sgn}(v_m^{l_4}) \frac{1 - \text{sgn}(\delta_m^{l_4})}{2}
\end{aligned} \tag{S34.1}$$

$$\begin{aligned}
\mathcal{W}_2^{\text{gapless}} = & \sum_{m=1}^{n_{a_2}} \text{sgn}(v_m^{a_2}) \frac{1 - \text{sgn}(\delta_m^{a_2})}{2} + \sum_{m=1}^{n_{e_1}} \text{sgn}(v_m^{e_1}) \frac{1 - \text{sgn}(\delta_m^{e_1})}{2} - 2 \sum_{m=1}^{n_{f_1}} \text{sgn}(v_m^{f_1}) \frac{1 - \text{sgn}(\delta_m^{f_1})}{2} \\
& + 2 \sum_{m=1}^{n_{g_2}} \text{sgn}(v_m^{g_2}) \frac{1 - \text{sgn}(\delta_m^{g_2})}{2} + 2 \sum_{m=1}^{n_{h_2}} \text{sgn}(v_m^{h_2}) \frac{1 - \text{sgn}(\delta_m^{h_2})}{2} - \sum_{m=1}^{n_{i_1}} \text{sgn}(v_m^{i_1}) \frac{1 - \text{sgn}(\delta_m^{i_1})}{2} \\
& - \sum_{m=1}^{n_{j_1}} \text{sgn}(v_m^{j_1}) \frac{1 - \text{sgn}(\delta_m^{j_1})}{2} + 2 \sum_{m=1}^{n_{j_2}} \text{sgn}(v_m^{j_2}) \frac{1 - \text{sgn}(\delta_m^{j_2})}{2} + \sum_{m=1}^{n_{j_4}} \text{sgn}(v_m^{j_4}) \frac{1 - \text{sgn}(\delta_m^{j_4})}{2} \\
& - \sum_{m=1}^{n_{l_1}} \text{sgn}(v_m^{l_1}) \frac{1 - \text{sgn}(\delta_m^{l_1})}{2} + \sum_{m=1}^{n_{l_2}} \text{sgn}(v_m^{l_2}) \frac{1 - \text{sgn}(\delta_m^{l_2})}{2} + \sum_{m=1}^{n_{l_3}} \text{sgn}(v_m^{l_3}) \frac{1 - \text{sgn}(\delta_m^{l_3})}{2} - \sum_{m=1}^{n_{l_4}} \text{sgn}(v_m^{l_4}) \frac{1 - \text{sgn}(\delta_m^{l_4})}{2}
\end{aligned} \tag{S34.2}$$

$$\begin{aligned}
\mathcal{W}_3^{\text{gapless}} = & \sum_{m=1}^{n_{b_1}} \text{sgn}(v_m^{b_1}) \frac{1 - \text{sgn}(\delta_m^{b_1})}{2} - \sum_{m=1}^{n_{f_1}} \text{sgn}(v_m^{f_1}) \frac{1 - \text{sgn}(\delta_m^{f_1})}{2} - \sum_{m=1}^{n_{i_1}} \text{sgn}(v_m^{i_1}) \frac{1 - \text{sgn}(\delta_m^{i_1})}{2} \\
& + \sum_{m=1}^{n_{l_1}} \text{sgn}(v_m^{l_1}) \frac{1 - \text{sgn}(\delta_m^{l_1})}{2} + \sum_{m=1}^{n_{l_3}} \text{sgn}(v_m^{l_3}) \frac{1 - \text{sgn}(\delta_m^{l_3})}{2}
\end{aligned} \tag{S34.3}$$

$$\begin{aligned}
\mathcal{W}_4^{\text{gapless}} = & \sum_{m=1}^{n_{b_2}} \text{sgn}(v_m^{b_2}) \frac{1 - \text{sgn}(\delta_m^{b_2})}{2} - \sum_{m=1}^{n_{f_1}} \text{sgn}(v_m^{f_1}) \frac{1 - \text{sgn}(\delta_m^{f_1})}{2} - \sum_{m=1}^{n_{i_1}} \text{sgn}(v_m^{i_1}) \frac{1 - \text{sgn}(\delta_m^{i_1})}{2} \\
& + \sum_{m=1}^{n_{l_2}} \text{sgn}(v_m^{l_2}) \frac{1 - \text{sgn}(\delta_m^{l_2})}{2} + \sum_{m=1}^{n_{l_4}} \text{sgn}(v_m^{l_4}) \frac{1 - \text{sgn}(\delta_m^{l_4})}{2}
\end{aligned} \tag{S34.4}$$

$$\begin{aligned}
\mathcal{W}_5^{\text{gapless}} = & \sum_{m=1}^{n_{c_1}} \text{sgn}(v_m^{c_1}) \frac{1 - \text{sgn}(\delta_m^{c_1})}{2} - \sum_{m=1}^{n_{g_2}} \text{sgn}(v_m^{g_2}) \frac{1 - \text{sgn}(\delta_m^{g_2})}{2} - \sum_{m=1}^{n_{j_2}} \text{sgn}(v_m^{j_2}) \frac{1 - \text{sgn}(\delta_m^{j_2})}{2} \\
& - \sum_{m=1}^{n_{j_4}} \text{sgn}(v_m^{j_4}) \frac{1 - \text{sgn}(\delta_m^{j_4})}{2} + \sum_{m=1}^{n_{k_1}} \text{sgn}(v_m^{k_1}) \frac{1 - \text{sgn}(\delta_m^{k_1})}{2}
\end{aligned} \tag{S34.5}$$

$$\begin{aligned}
\mathcal{W}_6^{\text{gapless}} = & \sum_{m=1}^{n_{d_1}} \text{sgn}(v_m^{d_1}) \frac{1 - \text{sgn}(\delta_m^{d_1})}{2} - \sum_{m=1}^{n_{h_2}} \text{sgn}(v_m^{h_2}) \frac{1 - \text{sgn}(\delta_m^{h_2})}{2} - \sum_{m=1}^{n_{k_1}} \text{sgn}(v_m^{k_1}) \frac{1 - \text{sgn}(\delta_m^{k_1})}{2} \\
& + \sum_{m=1}^{n_{l_1}} \text{sgn}(v_m^{l_1}) \frac{1 - \text{sgn}(\delta_m^{l_1})}{2} + \sum_{m=1}^{n_{l_4}} \text{sgn}(v_m^{l_4}) \frac{1 - \text{sgn}(\delta_m^{l_4})}{2}
\end{aligned} \tag{S34.6}$$

$$\begin{aligned}
\mathcal{W}_7^{\text{gapless}} = & 2 \sum_{m=1}^{n_{e_1}} \text{sgn}(v_m^{e_1}) \frac{1 - \text{sgn}(\delta_m^{e_1})}{2} - 2 \sum_{m=1}^{n_{f_1}} \text{sgn}(v_m^{f_1}) \frac{1 - \text{sgn}(\delta_m^{f_1})}{2} + 2 \sum_{m=1}^{n_{g_2}} \text{sgn}(v_m^{g_2}) \frac{1 - \text{sgn}(\delta_m^{g_2})}{2} \\
& + 2 \sum_{m=1}^{n_{h_2}} \text{sgn}(v_m^{h_2}) \frac{1 - \text{sgn}(\delta_m^{h_2})}{2} - \sum_{m=1}^{n_{j_1}} \text{sgn}(v_m^{j_1}) \frac{1 - \text{sgn}(\delta_m^{j_1})}{2} + \sum_{m=1}^{n_{j_2}} \text{sgn}(v_m^{j_2}) \frac{1 - \text{sgn}(\delta_m^{j_2})}{2} \\
& - \sum_{m=1}^{n_{j_3}} \text{sgn}(v_m^{j_3}) \frac{1 - \text{sgn}(\delta_m^{j_3})}{2} + \sum_{m=1}^{n_{j_4}} \text{sgn}(v_m^{j_4}) \frac{1 - \text{sgn}(\delta_m^{j_4})}{2} - \sum_{m=1}^{n_{l_1}} \text{sgn}(v_m^{l_1}) \frac{1 - \text{sgn}(\delta_m^{l_1})}{2} \\
& + \sum_{m=1}^{n_{l_2}} \text{sgn}(v_m^{l_2}) \frac{1 - \text{sgn}(\delta_m^{l_2})}{2} + \sum_{m=1}^{n_{l_3}} \text{sgn}(v_m^{l_3}) \frac{1 - \text{sgn}(\delta_m^{l_3})}{2} - \sum_{m=1}^{n_{l_4}} \text{sgn}(v_m^{l_4}) \frac{1 - \text{sgn}(\delta_m^{l_4})}{2}
\end{aligned} \tag{S34.7}$$

$$\begin{aligned} \mathcal{W}_8^{\text{gapless}} = & \sum_{m=1}^{n_{g1}} \text{sgn}(v_m^{g1}) \frac{1 - \text{sgn}(\delta_m^{g1})}{2} - \sum_{m=1}^{n_{g2}} \text{sgn}(v_m^{g2}) \frac{1 - \text{sgn}(\delta_m^{g2})}{2} + \sum_{m=1}^{n_{j1}} \text{sgn}(v_m^{j1}) \frac{1 - \text{sgn}(\delta_m^{j1})}{2} \\ & - \sum_{m=1}^{n_{j2}} \text{sgn}(v_m^{j2}) \frac{1 - \text{sgn}(\delta_m^{j2})}{2} + \sum_{m=1}^{n_{j3}} \text{sgn}(v_m^{j3}) \frac{1 - \text{sgn}(\delta_m^{j3})}{2} - \sum_{m=1}^{n_{j4}} \text{sgn}(v_m^{j4}) \frac{1 - \text{sgn}(\delta_m^{j4})}{2} \end{aligned} \quad (\text{S34.8})$$

$$\begin{aligned} \mathcal{W}_9^{\text{gapless}} = & \sum_{m=1}^{n_{h1}} \text{sgn}(v_m^{h1}) \frac{1 - \text{sgn}(\delta_m^{h1})}{2} - \sum_{m=1}^{n_{h2}} \text{sgn}(v_m^{h2}) \frac{1 - \text{sgn}(\delta_m^{h2})}{2} + \sum_{m=1}^{n_{l1}} \text{sgn}(v_m^{l1}) \frac{1 - \text{sgn}(\delta_m^{l1})}{2} \\ & - \sum_{m=1}^{n_{l2}} \text{sgn}(v_m^{l2}) \frac{1 - \text{sgn}(\delta_m^{l2})}{2} - \sum_{m=1}^{n_{l3}} \text{sgn}(v_m^{l3}) \frac{1 - \text{sgn}(\delta_m^{l3})}{2} + \sum_{m=1}^{n_{l4}} \text{sgn}(v_m^{l4}) \frac{1 - \text{sgn}(\delta_m^{l4})}{2} \end{aligned} \quad (\text{S34.9})$$

$$\mathcal{W}_1^{\text{gapped}} = - \sum_{m=1}^{n_{j1}} \text{sgn}(v_m^{j1}) \frac{1 - \text{sgn}(\delta_m^{j1})}{2} - \sum_{m=1}^{n_{j2}} \text{sgn}(v_m^{j2}) \frac{1 - \text{sgn}(\delta_m^{j2})}{2} + \sum_{m=1}^{n_{j3}} \text{sgn}(v_m^{j3}) \frac{1 - \text{sgn}(\delta_m^{j3})}{2} + \sum_{m=1}^{n_{j4}} \text{sgn}(v_m^{j4}) \frac{1 - \text{sgn}(\delta_m^{j4})}{2} \quad (\text{S34.10})$$

$$\begin{aligned} \mathcal{W}_2^{\text{gapped}} = & - \sum_{m=1}^{n_{e1}} \text{sgn}(v_m^{e1}) \frac{1 - \text{sgn}(\delta_m^{e1})}{2} + \sum_{m=1}^{n_{f1}} \text{sgn}(v_m^{f1}) \frac{1 - \text{sgn}(\delta_m^{f1})}{2} - \sum_{m=1}^{n_{g2}} \text{sgn}(v_m^{g2}) \frac{1 - \text{sgn}(\delta_m^{g2})}{2} \\ & - \sum_{m=1}^{n_{h2}} \text{sgn}(v_m^{h2}) \frac{1 - \text{sgn}(\delta_m^{h2})}{2} + \sum_{m=1}^{n_{j1}} \text{sgn}(v_m^{j1}) \frac{1 - \text{sgn}(\delta_m^{j1})}{2} \\ & - \sum_{m=1}^{n_{j4}} \text{sgn}(v_m^{j4}) \frac{1 - \text{sgn}(\delta_m^{j4})}{2} - \sum_{m=1}^{n_{l2}} \text{sgn}(v_m^{l2}) \frac{1 - \text{sgn}(\delta_m^{l2})}{2} + \sum_{m=1}^{n_{l4}} \text{sgn}(v_m^{l4}) \frac{1 - \text{sgn}(\delta_m^{l4})}{2} \end{aligned} \quad (\text{S34.11})$$

$$\mathcal{X}_1 = \sum_{m=1}^{n_{f1}} \frac{1 - \text{sgn}(\delta_m^{f1})}{2} + \sum_{m=1}^{n_{g2}} \frac{1 - \text{sgn}(\delta_m^{g2})}{2} + \sum_{m=1}^{n_{h2}} \frac{1 - \text{sgn}(\delta_m^{h2})}{2} + \sum_{m=1}^{n_{l1}} \frac{1 - \text{sgn}(\delta_m^{l1})}{2} + \sum_{m=1}^{n_{l3}} \frac{1 - \text{sgn}(\delta_m^{l3})}{2} \quad \text{mod } 2 \quad (\text{S34.12})$$

$$\mathcal{X}_2 = \sum_{m=1}^{n_{f1}} \frac{1 - \text{sgn}(\delta_m^{f1})}{2} + \sum_{m=1}^{n_{h2}} \frac{1 - \text{sgn}(\delta_m^{h2})}{2} + \sum_{m=1}^{n_{k1}} \frac{1 - \text{sgn}(\delta_m^{k1})}{2} + \sum_{m=1}^{n_{l1}} \frac{1 - \text{sgn}(\delta_m^{l1})}{2} + \sum_{m=1}^{n_{l3}} \frac{1 - \text{sgn}(\delta_m^{l3})}{2} \quad \text{mod } 2 \quad (\text{S34.13})$$

$$\mathcal{X}_3 = \sum_{m=1}^{n_{f1}} \frac{1 - \text{sgn}(\delta_m^{f1})}{2} + \sum_{m=1}^{n_{l1}} \frac{1 - \text{sgn}(\delta_m^{l1})}{2} + \sum_{m=1}^{n_{l3}} \frac{1 - \text{sgn}(\delta_m^{l3})}{2} \quad \text{mod } 2 \quad (\text{S34.14})$$

### S35. SPACE GROUP NO. 35

|              |                                      |
|--------------|--------------------------------------|
| line segment | character of irrep (generators only) |
|--------------|--------------------------------------|

|                                                       |                                                                                                                                                                |
|-------------------------------------------------------|----------------------------------------------------------------------------------------------------------------------------------------------------------------|
| $a \quad (t, 0, 0)$                                   | $\{m_{010}   \begin{smallmatrix} 0 & 0 & 0 \end{smallmatrix} \}$<br>$a_1 \quad -i$<br>$a_2 \quad i$                                                            |
| $b \quad (0, t, 0)$                                   | $\{m_{100}   \begin{smallmatrix} 0 & 0 & 0 \end{smallmatrix} \}$<br>$b_1 \quad -i$<br>$b_2 \quad i$                                                            |
| $c \quad (\frac{t}{2}, 1 - \frac{t}{2}, 0)$           | $\{1   \begin{smallmatrix} 0 & 0 & 0 \end{smallmatrix} \}$<br>$c_1 \quad 1$                                                                                    |
| $d \quad (t, 0, \frac{1}{2})$                         | $\{m_{010}   \begin{smallmatrix} 0 & 0 & 0 \end{smallmatrix} \}$<br>$d_1 \quad -i$<br>$d_2 \quad i$                                                            |
| $e \quad (0, t, \frac{1}{2})$                         | $\{m_{100}   \begin{smallmatrix} 0 & 0 & 0 \end{smallmatrix} \}$<br>$e_1 \quad -i$<br>$e_2 \quad i$                                                            |
| $f \quad (\frac{t}{2}, 1 - \frac{t}{2}, \frac{1}{2})$ | $\{1   \begin{smallmatrix} 0 & 0 & 0 \end{smallmatrix} \}$<br>$f_1 \quad 1$                                                                                    |
| $g \quad (0, 0, \frac{t}{2})$                         | $\{2_{001}   \begin{smallmatrix} 0 & 0 & 0 \end{smallmatrix} \} \quad \{m_{100}   \begin{smallmatrix} 0 & 0 & 0 \end{smallmatrix} \}$<br>$g_1 \quad 0 \quad 0$ |
| $h \quad (1, 0, \frac{t}{2})$                         | $\{2_{001}   \begin{smallmatrix} 0 & 0 & 0 \end{smallmatrix} \} \quad \{m_{100}   \begin{smallmatrix} 0 & 0 & 0 \end{smallmatrix} \}$<br>$h_1 \quad 0 \quad 0$ |
| $i \quad (\frac{1}{2}, \frac{1}{2}, \frac{t}{2})$     | $\{2_{001}   \begin{smallmatrix} 0 & 0 & 0 \end{smallmatrix} \}$<br>$i_1 \quad -i$<br>$i_2 \quad i$                                                            |

$$\begin{aligned} \mathcal{W}_1^{\text{gapless}} = & \sum_{m=1}^{n_{a_1}} \text{sgn}(v_m^{a_1}) \frac{1 - \text{sgn}(\delta_m^{a_1})}{2} + \sum_{m=1}^{n_{d_2}} \text{sgn}(v_m^{d_2}) \frac{1 - \text{sgn}(\delta_m^{d_2})}{2} - \sum_{m=1}^{n_{e_1}} \text{sgn}(v_m^{e_1}) \frac{1 - \text{sgn}(\delta_m^{e_1})}{2} \\ & - \sum_{m=1}^{n_{e_2}} \text{sgn}(v_m^{e_2}) \frac{1 - \text{sgn}(\delta_m^{e_2})}{2} - \sum_{m=1}^{n_{g_1}} \text{sgn}(v_m^{g_1}) \frac{1 - \text{sgn}(\delta_m^{g_1})}{2} + \sum_{m=1}^{n_{h_1}} \text{sgn}(v_m^{h_1}) \frac{1 - \text{sgn}(\delta_m^{h_1})}{2} \end{aligned} \quad (\text{S35.1})$$

$$\mathcal{W}_2^{\text{gapless}} = \sum_{m=1}^{n_{a_2}} \text{sgn}(v_m^{a_2}) \frac{1 - \text{sgn}(\delta_m^{a_2})}{2} - \sum_{m=1}^{n_{d_2}} \text{sgn}(v_m^{d_2}) \frac{1 - \text{sgn}(\delta_m^{d_2})}{2} - \sum_{m=1}^{n_{g_1}} \text{sgn}(v_m^{g_1}) \frac{1 - \text{sgn}(\delta_m^{g_1})}{2} + \sum_{m=1}^{n_{h_1}} \text{sgn}(v_m^{h_1}) \frac{1 - \text{sgn}(\delta_m^{h_1})}{2} \quad (\text{S35.2})$$

$$\mathcal{W}_3^{\text{gapless}} = \sum_{m=1}^{n_{b_1}} \text{sgn}(v_m^{b_1}) \frac{1 - \text{sgn}(\delta_m^{b_1})}{2} - \sum_{m=1}^{n_{e_1}} \text{sgn}(v_m^{e_1}) \frac{1 - \text{sgn}(\delta_m^{e_1})}{2} - \sum_{m=1}^{n_{g_1}} \text{sgn}(v_m^{g_1}) \frac{1 - \text{sgn}(\delta_m^{g_1})}{2} + \sum_{m=1}^{n_{h_1}} \text{sgn}(v_m^{h_1}) \frac{1 - \text{sgn}(\delta_m^{h_1})}{2} \quad (\text{S35.3})$$

$$\mathcal{W}_4^{\text{gapless}} = \sum_{m=1}^{n_{b_2}} \text{sgn}(v_m^{b_2}) \frac{1 - \text{sgn}(\delta_m^{b_2})}{2} - \sum_{m=1}^{n_{e_2}} \text{sgn}(v_m^{e_2}) \frac{1 - \text{sgn}(\delta_m^{e_2})}{2} - \sum_{m=1}^{n_{g_1}} \text{sgn}(v_m^{g_1}) \frac{1 - \text{sgn}(\delta_m^{g_1})}{2} + \sum_{m=1}^{n_{h_1}} \text{sgn}(v_m^{h_1}) \frac{1 - \text{sgn}(\delta_m^{h_1})}{2} \quad (\text{S35.4})$$

$$\begin{aligned} \mathcal{W}_5^{\text{gapless}} = & \sum_{m=1}^{n_{c_1}} \text{sgn}(v_m^{c_1}) \frac{1 - \text{sgn}(\delta_m^{c_1})}{2} - \sum_{m=1}^{n_{f_1}} \text{sgn}(v_m^{f_1}) \frac{1 - \text{sgn}(\delta_m^{f_1})}{2} - 2 \sum_{m=1}^{n_{h_1}} \text{sgn}(v_m^{h_1}) \frac{1 - \text{sgn}(\delta_m^{h_1})}{2} \\ & + \sum_{m=1}^{n_{i_1}} \text{sgn}(v_m^{i_1}) \frac{1 - \text{sgn}(\delta_m^{i_1})}{2} + \sum_{m=1}^{n_{i_2}} \text{sgn}(v_m^{i_2}) \frac{1 - \text{sgn}(\delta_m^{i_2})}{2} \end{aligned} \quad (\text{S35.5})$$

$$\mathcal{W}_6^{\text{gapless}} = \sum_{m=1}^{n_{d_1}} \text{sgn}(v_m^{d_1}) \frac{1 - \text{sgn}(\delta_m^{d_1})}{2} + \sum_{m=1}^{n_{d_2}} \text{sgn}(v_m^{d_2}) \frac{1 - \text{sgn}(\delta_m^{d_2})}{2} - \sum_{m=1}^{n_{e_1}} \text{sgn}(v_m^{e_1}) \frac{1 - \text{sgn}(\delta_m^{e_1})}{2} - \sum_{m=1}^{n_{e_2}} \text{sgn}(v_m^{e_2}) \frac{1 - \text{sgn}(\delta_m^{e_2})}{2} \quad (\text{S35.6})$$

$$\mathcal{W}_1^{\text{gapped}} = - \sum_{m=1}^{n_{d_2}} \text{sgn}(v_m^{d_2}) \frac{1 - \text{sgn}(\delta_m^{d_2})}{2} + \sum_{m=1}^{n_{e_1}} \text{sgn}(v_m^{e_1}) \frac{1 - \text{sgn}(\delta_m^{e_1})}{2} \quad (\text{S35.7})$$

$$\mathcal{W}_2^{\text{gapped}} = - \sum_{m=1}^{n_{d_2}} \text{sgn}(v_m^{d_2}) \frac{1 - \text{sgn}(\delta_m^{d_2})}{2} + \sum_{m=1}^{n_{e_2}} \text{sgn}(v_m^{e_2}) \frac{1 - \text{sgn}(\delta_m^{e_2})}{2} \quad (\text{S35.8})$$

$$\mathcal{W}_3^{\text{gapped}} = - \sum_{m=1}^{n_{i_1}} \text{sgn}(v_m^{i_1}) \frac{1 - \text{sgn}(\delta_m^{i_1})}{2} + \sum_{m=1}^{n_{i_2}} \text{sgn}(v_m^{i_2}) \frac{1 - \text{sgn}(\delta_m^{i_2})}{2} \quad (\text{S35.9})$$

$$\mathcal{X}_1 = \sum_{m=1}^{n_{f_1}} \frac{1 - \text{sgn}(\delta_m^{f_1})}{2} \mod 2 \quad (\text{S35.10})$$

### S36. SPACE GROUP NO. 36

| line segment                                      | character of irrep (generators only)                                                                               |
|---------------------------------------------------|--------------------------------------------------------------------------------------------------------------------|
| $a \ (t, 0, 0)$                                   | $\{m_{010}   0 \ 0 \ \frac{1}{2}\}$<br>$a_1 \quad -i$<br>$a_2 \quad i$                                             |
| $b \ (0, t, 0)$                                   | $\{m_{100}   0 \ 0 \ 0\}$<br>$b_1 \quad -i$<br>$b_2 \quad i$                                                       |
| $c \ (\frac{t}{2}, 1 - \frac{t}{2}, 0)$           | $\{1   0 \ 0 \ 0\}$<br>$c_1 \quad 1$                                                                               |
| $d \ (t, 0, \frac{1}{2})$                         | $\{m_{010}   0 \ 0 \ \frac{1}{2}\}$<br>$d_1 \quad -1$<br>$d_2 \quad 1$                                             |
| $e \ (0, t, \frac{1}{2})$                         | $\{m_{100}   0 \ 0 \ 0\}$<br>$e_1 \quad -i$<br>$e_2 \quad i$                                                       |
| $f \ (\frac{t}{2}, 1 - \frac{t}{2}, \frac{1}{2})$ | $\{1   0 \ 0 \ 0\}$<br>$f_1 \quad 1$                                                                               |
| $g \ (0, 0, \frac{t}{2})$                         | $\{2_{001}   0 \ 0 \ \frac{1}{2}\} \ \{m_{100}   0 \ 0 \ 0\}$<br>$g_1 \quad 0 \quad 0$                             |
| $h \ (1, 0, \frac{t}{2})$                         | $\{2_{001}   0 \ 0 \ \frac{1}{2}\} \ \{m_{100}   0 \ 0 \ 0\}$<br>$h_1 \quad 0 \quad 0$                             |
| $i \ (\frac{1}{2}, \frac{1}{2}, \frac{t}{2})$     | $\{2_{001}   0 \ 0 \ \frac{1}{2}\}$<br>$i_1 \quad -ie^{-\frac{1}{2}i\pi t}$<br>$i_2 \quad ie^{-\frac{1}{2}i\pi t}$ |

$$\begin{aligned} \mathcal{W}_1^{\text{gapless}} = & \sum_{m=1}^{n_{a_1}} \text{sgn}(v_m^{a_1}) \frac{1 - \text{sgn}(\delta_m^{a_1})}{2} - \sum_{m=1}^{n_{e_1}} \text{sgn}(v_m^{e_1}) \frac{1 - \text{sgn}(\delta_m^{e_1})}{2} - \sum_{m=1}^{n_{e_2}} \text{sgn}(v_m^{e_2}) \frac{1 - \text{sgn}(\delta_m^{e_2})}{2} \\ & - \sum_{m=1}^{n_{g_1}} \text{sgn}(v_m^{g_1}) \frac{1 - \text{sgn}(\delta_m^{g_1})}{2} + \sum_{m=1}^{n_{h_1}} \text{sgn}(v_m^{h_1}) \frac{1 - \text{sgn}(\delta_m^{h_1})}{2} \end{aligned} \quad (\text{S36.1})$$

$$\begin{aligned} \mathcal{W}_2^{\text{gapless}} = & \sum_{m=1}^{n_{a_2}} \text{sgn}(v_m^{a_2}) \frac{1 - \text{sgn}(\delta_m^{a_2})}{2} - \sum_{m=1}^{n_{e_1}} \text{sgn}(v_m^{e_1}) \frac{1 - \text{sgn}(\delta_m^{e_1})}{2} - \sum_{m=1}^{n_{e_2}} \text{sgn}(v_m^{e_2}) \frac{1 - \text{sgn}(\delta_m^{e_2})}{2} \\ & - \sum_{m=1}^{n_{g_1}} \text{sgn}(v_m^{g_1}) \frac{1 - \text{sgn}(\delta_m^{g_1})}{2} + \sum_{m=1}^{n_{h_1}} \text{sgn}(v_m^{h_1}) \frac{1 - \text{sgn}(\delta_m^{h_1})}{2} \end{aligned} \quad (\text{S36.2})$$

$$\begin{aligned} \mathcal{W}_3^{\text{gapless}} = & \sum_{m=1}^{n_{b_1}} \text{sgn}(v_m^{b_1}) \frac{1 - \text{sgn}(\delta_m^{b_1})}{2} - 2 \sum_{m=1}^{n_{e_1}} \text{sgn}(v_m^{e_1}) \frac{1 - \text{sgn}(\delta_m^{e_1})}{2} - \sum_{m=1}^{n_{g_1}} \text{sgn}(v_m^{g_1}) \frac{1 - \text{sgn}(\delta_m^{g_1})}{2} \\ & + \sum_{m=1}^{n_{h_1}} \text{sgn}(v_m^{h_1}) \frac{1 - \text{sgn}(\delta_m^{h_1})}{2} \end{aligned} \quad (\text{S36.3})$$

$$\begin{aligned} \mathcal{W}_4^{\text{gapless}} = & \sum_{m=1}^{n_{b_2}} \text{sgn}(v_m^{b_2}) \frac{1 - \text{sgn}(\delta_m^{b_2})}{2} - 2 \sum_{m=1}^{n_{e_2}} \text{sgn}(v_m^{e_2}) \frac{1 - \text{sgn}(\delta_m^{e_2})}{2} - \sum_{m=1}^{n_{g_1}} \text{sgn}(v_m^{g_1}) \frac{1 - \text{sgn}(\delta_m^{g_1})}{2} \\ & + \sum_{m=1}^{n_{h_1}} \text{sgn}(v_m^{h_1}) \frac{1 - \text{sgn}(\delta_m^{h_1})}{2} \end{aligned} \quad (\text{S36.4})$$

$$\begin{aligned} \mathcal{W}_5^{\text{gapless}} = & \sum_{m=1}^{n_{c_1}} \text{sgn}(v_m^{c_1}) \frac{1 - \text{sgn}(\delta_m^{c_1})}{2} - 2 \sum_{m=1}^{n_{f_1}} \text{sgn}(v_m^{f_1}) \frac{1 - \text{sgn}(\delta_m^{f_1})}{2} - 2 \sum_{m=1}^{n_{h_1}} \text{sgn}(v_m^{h_1}) \frac{1 - \text{sgn}(\delta_m^{h_1})}{2} \\ & + \sum_{m=1}^{n_{i_1}} \text{sgn}(v_m^{i_1}) \frac{1 - \text{sgn}(\delta_m^{i_1})}{2} + \sum_{m=1}^{n_{i_2}} \text{sgn}(v_m^{i_2}) \frac{1 - \text{sgn}(\delta_m^{i_2})}{2} \end{aligned} \quad (\text{S36.5})$$

$$\mathcal{W}_6^{\text{gapless}} = \sum_{m=1}^{n_{d_1}} \text{sgn}(v_m^{d_1}) \frac{1 - \text{sgn}(\delta_m^{d_1})}{2} - \sum_{m=1}^{n_{e_1}} \text{sgn}(v_m^{e_1}) \frac{1 - \text{sgn}(\delta_m^{e_1})}{2} - \sum_{m=1}^{n_{e_2}} \text{sgn}(v_m^{e_2}) \frac{1 - \text{sgn}(\delta_m^{e_2})}{2} \quad (\text{S36.6})$$

$$\mathcal{W}_1^{\text{gapped}} = - \sum_{m=1}^{n_{e_1}} \text{sgn}(v_m^{e_1}) \frac{1 - \text{sgn}(\delta_m^{e_1})}{2} + \sum_{m=1}^{n_{e_2}} \text{sgn}(v_m^{e_2}) \frac{1 - \text{sgn}(\delta_m^{e_2})}{2} \quad (\text{S36.7})$$

$$\mathcal{X}_1 = -2 \sum_{m=1}^{n_{f_1}} \text{sgn}(v_m^{f_1}) \frac{1 - \text{sgn}(\delta_m^{f_1})}{2} + \sum_{m=1}^{n_{i_1}} \text{sgn}(v_m^{i_1}) \frac{1 - \text{sgn}(\delta_m^{i_1})}{2} - \sum_{m=1}^{n_{i_2}} \text{sgn}(v_m^{i_2}) \frac{1 - \text{sgn}(\delta_m^{i_2})}{2} \pmod{4} \quad (\text{S36.8})$$

### S37. SPACE GROUP NO. 37

|              |                                      |
|--------------|--------------------------------------|
| line segment | character of irrep (generators only) |
|--------------|--------------------------------------|

|                                                       |                                                                                                        |
|-------------------------------------------------------|--------------------------------------------------------------------------------------------------------|
| $a \quad (t, 0, 0)$                                   | $\begin{matrix} \{m_{010}  0 & 0 & \frac{1}{2}\} \\ a_1 & -i \\ a_2 & i \end{matrix}$                  |
| $b \quad (0, t, 0)$                                   | $\begin{matrix} \{m_{100}  0 & 0 & \frac{1}{2}\} \\ b_1 & -i \\ b_2 & i \end{matrix}$                  |
| $c \quad (\frac{t}{2}, 1 - \frac{t}{2}, 0)$           | $\begin{matrix} \{1  0 & 0 & 0\} \\ c_1 & 1 \end{matrix}$                                              |
| $d \quad (t, 0, \frac{1}{2})$                         | $\begin{matrix} \{m_{010}  0 & 0 & \frac{1}{2}\} \\ d_1 & -1 \\ d_2 & 1 \end{matrix}$                  |
| $e \quad (0, t, \frac{1}{2})$                         | $\begin{matrix} \{m_{100}  0 & 0 & \frac{1}{2}\} \\ e_1 & -1 \\ e_2 & 1 \end{matrix}$                  |
| $f \quad (\frac{t}{2}, 1 - \frac{t}{2}, \frac{1}{2})$ | $\begin{matrix} \{1  0 & 0 & 0\} \\ f_1 & 1 \end{matrix}$                                              |
| $g \quad (0, 0, \frac{t}{2})$                         | $\begin{matrix} \{2_{001}  0 & 0 & 0\} & \{m_{100}  0 & 0 & \frac{1}{2}\} \\ g_1 & 0 & 0 \end{matrix}$ |
| $h \quad (1, 0, \frac{t}{2})$                         | $\begin{matrix} \{2_{001}  0 & 0 & 0\} & \{m_{100}  0 & 0 & \frac{1}{2}\} \\ h_1 & 0 & 0 \end{matrix}$ |
| $i \quad (\frac{1}{2}, \frac{1}{2}, \frac{t}{2})$     | $\begin{matrix} \{2_{001}  0 & 0 & 0\} \\ i_1 & -i \\ i_2 & i \end{matrix}$                            |

$$\begin{aligned} \mathcal{W}_1^{\text{gapless}} = & \sum_{m=1}^{n_{a_1}} \text{sgn}(v_m^{a_1}) \frac{1 - \text{sgn}(\delta_m^{a_1})}{2} + \sum_{m=1}^{n_{d_1}} \text{sgn}(v_m^{d_1}) \frac{1 - \text{sgn}(\delta_m^{d_1})}{2} - 2 \sum_{m=1}^{n_{e_1}} \text{sgn}(v_m^{e_1}) \frac{1 - \text{sgn}(\delta_m^{e_1})}{2} \\ & - \sum_{m=1}^{n_{g_1}} \text{sgn}(v_m^{g_1}) \frac{1 - \text{sgn}(\delta_m^{g_1})}{2} + \sum_{m=1}^{n_{h_1}} \text{sgn}(v_m^{h_1}) \frac{1 - \text{sgn}(\delta_m^{h_1})}{2} \end{aligned} \quad (\text{S37.1})$$

$$\begin{aligned} \mathcal{W}_2^{\text{gapless}} = & \sum_{m=1}^{n_{a_2}} \text{sgn}(v_m^{a_2}) \frac{1 - \text{sgn}(\delta_m^{a_2})}{2} + \sum_{m=1}^{n_{d_1}} \text{sgn}(v_m^{d_1}) \frac{1 - \text{sgn}(\delta_m^{d_1})}{2} - 2 \sum_{m=1}^{n_{e_1}} \text{sgn}(v_m^{e_1}) \frac{1 - \text{sgn}(\delta_m^{e_1})}{2} \\ & - \sum_{m=1}^{n_{g_1}} \text{sgn}(v_m^{g_1}) \frac{1 - \text{sgn}(\delta_m^{g_1})}{2} + \sum_{m=1}^{n_{h_1}} \text{sgn}(v_m^{h_1}) \frac{1 - \text{sgn}(\delta_m^{h_1})}{2} \end{aligned} \quad (\text{S37.2})$$

$$\mathcal{W}_3^{\text{gapless}} = \sum_{m=1}^{n_{b_1}} \text{sgn}(v_m^{b_1}) \frac{1 - \text{sgn}(\delta_m^{b_1})}{2} - \sum_{m=1}^{n_{e_1}} \text{sgn}(v_m^{e_1}) \frac{1 - \text{sgn}(\delta_m^{e_1})}{2} - \sum_{m=1}^{n_{g_1}} \text{sgn}(v_m^{g_1}) \frac{1 - \text{sgn}(\delta_m^{g_1})}{2} + \sum_{m=1}^{n_{h_1}} \text{sgn}(v_m^{h_1}) \frac{1 - \text{sgn}(\delta_m^{h_1})}{2} \quad (\text{S37.3})$$

$$\mathcal{W}_4^{\text{gapless}} = \sum_{m=1}^{n_{b_2}} \text{sgn}(v_m^{b_2}) \frac{1 - \text{sgn}(\delta_m^{b_2})}{2} - \sum_{m=1}^{n_{e_1}} \text{sgn}(v_m^{e_1}) \frac{1 - \text{sgn}(\delta_m^{e_1})}{2} - \sum_{m=1}^{n_{g_1}} \text{sgn}(v_m^{g_1}) \frac{1 - \text{sgn}(\delta_m^{g_1})}{2} + \sum_{m=1}^{n_{h_1}} \text{sgn}(v_m^{h_1}) \frac{1 - \text{sgn}(\delta_m^{h_1})}{2} \quad (\text{S37.4})$$

$$\begin{aligned} \mathcal{W}_5^{\text{gapless}} = & \sum_{m=1}^{n_{c_1}} \text{sgn}(v_m^{c_1}) \frac{1 - \text{sgn}(\delta_m^{c_1})}{2} - \sum_{m=1}^{n_{f_1}} \text{sgn}(v_m^{f_1}) \frac{1 - \text{sgn}(\delta_m^{f_1})}{2} - 2 \sum_{m=1}^{n_{h_1}} \text{sgn}(v_m^{h_1}) \frac{1 - \text{sgn}(\delta_m^{h_1})}{2} \\ & + \sum_{m=1}^{n_{i_1}} \text{sgn}(v_m^{i_1}) \frac{1 - \text{sgn}(\delta_m^{i_1})}{2} + \sum_{m=1}^{n_{i_2}} \text{sgn}(v_m^{i_2}) \frac{1 - \text{sgn}(\delta_m^{i_2})}{2} \end{aligned} \quad (\text{S37.5})$$



$$\mathcal{W}_6^{\text{gapless}} = \sum_{m=1}^{n_{d_1}} \text{sgn}(v_m^{d_1}) \frac{1 - \text{sgn}(\delta_m^{d_1})}{2} - \sum_{m=1}^{n_{e_1}} \text{sgn}(v_m^{e_1}) \frac{1 - \text{sgn}(\delta_m^{e_1})}{2} \quad (\text{S37.6})$$

$$\mathcal{W}_1^{\text{gapped}} = - \sum_{m=1}^{n_{i_1}} \text{sgn}(v_m^{i_1}) \frac{1 - \text{sgn}(\delta_m^{i_1})}{2} + \sum_{m=1}^{n_{i_2}} \text{sgn}(v_m^{i_2}) \frac{1 - \text{sgn}(\delta_m^{i_2})}{2} \quad (\text{S37.7})$$

$$\mathcal{X}_1 = \sum_{m=1}^{n_{e_1}} \frac{1 - \text{sgn}(\delta_m^{e_1})}{2} + \sum_{m=1}^{n_{f_1}} \frac{1 - \text{sgn}(\delta_m^{f_1})}{2} \mod 2 \quad (\text{S37.8})$$

$$\mathcal{X}_2 = \sum_{m=1}^{n_{f_1}} \frac{1 - \text{sgn}(\delta_m^{f_1})}{2} \mod 2 \quad (\text{S37.9})$$

### S38. SPACE GROUP NO. 38

| line segment                                      | character of irrep (generators only)                                                                   |
|---------------------------------------------------|--------------------------------------------------------------------------------------------------------|
| $a \ (0, t, 0)$                                   | $\begin{matrix} \{m_{100}   0 \ 0 \ 0\} \\ a_1 \quad -i \\ a_2 \quad i \end{matrix}$                   |
| $b \ (0, 0, t)$                                   | $\begin{matrix} \{2_{001}   0 \ 0 \ 0\} \ \{m_{100}   0 \ 0 \ 0\} \\ b_1 \quad 0 \quad 0 \end{matrix}$ |
| $c \ (0, \frac{t}{2}, 1 - \frac{t}{2})$           | $\begin{matrix} \{m_{100}   0 \ 0 \ 0\} \\ c_1 \quad -i \\ c_2 \quad i \end{matrix}$                   |
| $d \ (\frac{1}{2}, t, 0)$                         | $\begin{matrix} \{m_{100}   0 \ 0 \ 0\} \\ d_1 \quad -i \\ d_2 \quad i \end{matrix}$                   |
| $e \ (\frac{1}{2}, 0, t)$                         | $\begin{matrix} \{2_{001}   0 \ 0 \ 0\} \ \{m_{100}   0 \ 0 \ 0\} \\ e_1 \quad 0 \quad 0 \end{matrix}$ |
| $f \ (\frac{1}{2}, \frac{t}{2}, 1 - \frac{t}{2})$ | $\begin{matrix} \{m_{100}   0 \ 0 \ 0\} \\ f_1 \quad -i \\ f_2 \quad i \end{matrix}$                   |
| $g \ (\frac{t}{2}, 0, 0)$                         | $\begin{matrix} \{m_{010}   0 \ 0 \ 0\} \\ g_1 \quad -i \\ g_2 \quad i \end{matrix}$                   |
| $h \ (\frac{t}{2}, 1, 0)$                         | $\begin{matrix} \{m_{010}   0 \ 0 \ 0\} \\ h_1 \quad -i \\ h_2 \quad i \end{matrix}$                   |
| $i \ (\frac{t}{2}, \frac{1}{2}, \frac{1}{2})$     | $\begin{matrix} \{1   0 \ 0 \ 0\} \\ i_1 \quad 1 \end{matrix}$                                         |

$$\begin{aligned} \mathcal{W}_1^{\text{gapless}} = & \sum_{m=1}^{n_{a_1}} \text{sgn}(v_m^{a_1}) \frac{1 - \text{sgn}(\delta_m^{a_1})}{2} + 2 \sum_{m=1}^{n_{c_2}} \text{sgn}(v_m^{c_2}) \frac{1 - \text{sgn}(\delta_m^{c_2})}{2} - \sum_{m=1}^{n_{e_1}} \text{sgn}(v_m^{e_1}) \frac{1 - \text{sgn}(\delta_m^{e_1})}{2} \\ & - \sum_{m=1}^{n_{f_1}} \text{sgn}(v_m^{f_1}) \frac{1 - \text{sgn}(\delta_m^{f_1})}{2} - \sum_{m=1}^{n_{f_2}} \text{sgn}(v_m^{f_2}) \frac{1 - \text{sgn}(\delta_m^{f_2})}{2} \\ & - \sum_{m=1}^{n_{g_2}} \text{sgn}(v_m^{g_2}) \frac{1 - \text{sgn}(\delta_m^{g_2})}{2} - \sum_{m=1}^{n_{h_1}} \text{sgn}(v_m^{h_1}) \frac{1 - \text{sgn}(\delta_m^{h_1})}{2} + \sum_{m=1}^{n_{i_1}} \text{sgn}(v_m^{i_1}) \frac{1 - \text{sgn}(\delta_m^{i_1})}{2} \end{aligned} \quad (\text{S38.1})$$

$$\begin{aligned}
\mathcal{W}_2^{\text{gapless}} = & \sum_{m=1}^{n_{a_2}} \text{sgn}(v_m^{a_2}) \frac{1 - \text{sgn}(\delta_m^{a_2})}{2} - 2 \sum_{m=1}^{n_{c_2}} \text{sgn}(v_m^{c_2}) \frac{1 - \text{sgn}(\delta_m^{c_2})}{2} - \sum_{m=1}^{n_{e_1}} \text{sgn}(v_m^{e_1}) \frac{1 - \text{sgn}(\delta_m^{e_1})}{2} \\
& + \sum_{m=1}^{n_{f_1}} \text{sgn}(v_m^{f_1}) \frac{1 - \text{sgn}(\delta_m^{f_1})}{2} + \sum_{m=1}^{n_{f_2}} \text{sgn}(v_m^{f_2}) \frac{1 - \text{sgn}(\delta_m^{f_2})}{2} - \sum_{m=1}^{n_{g_2}} \text{sgn}(v_m^{g_2}) \frac{1 - \text{sgn}(\delta_m^{g_2})}{2} \\
& + \sum_{m=1}^{n_{h_1}} \text{sgn}(v_m^{h_1}) \frac{1 - \text{sgn}(\delta_m^{h_1})}{2} + 2 \sum_{m=1}^{n_{h_2}} \text{sgn}(v_m^{h_2}) \frac{1 - \text{sgn}(\delta_m^{h_2})}{2} - \sum_{m=1}^{n_{i_1}} \text{sgn}(v_m^{i_1}) \frac{1 - \text{sgn}(\delta_m^{i_1})}{2}
\end{aligned} \tag{S38.2}$$

$$\mathcal{W}_3^{\text{gapless}} = \sum_{m=1}^{n_{b_1}} \text{sgn}(v_m^{b_1}) \frac{1 - \text{sgn}(\delta_m^{b_1})}{2} - \sum_{m=1}^{n_{e_1}} \text{sgn}(v_m^{e_1}) \frac{1 - \text{sgn}(\delta_m^{e_1})}{2} - \sum_{m=1}^{n_{g_2}} \text{sgn}(v_m^{g_2}) \frac{1 - \text{sgn}(\delta_m^{g_2})}{2} + \sum_{m=1}^{n_{h_2}} \text{sgn}(v_m^{h_2}) \frac{1 - \text{sgn}(\delta_m^{h_2})}{2} \tag{S38.3}$$

$$\begin{aligned}
\mathcal{W}_4^{\text{gapless}} = & \sum_{m=1}^{n_{c_1}} \text{sgn}(v_m^{c_1}) \frac{1 - \text{sgn}(\delta_m^{c_1})}{2} + \sum_{m=1}^{n_{c_2}} \text{sgn}(v_m^{c_2}) \frac{1 - \text{sgn}(\delta_m^{c_2})}{2} - \sum_{m=1}^{n_{f_1}} \text{sgn}(v_m^{f_1}) \frac{1 - \text{sgn}(\delta_m^{f_1})}{2} - \sum_{m=1}^{n_{f_2}} \text{sgn}(v_m^{f_2}) \frac{1 - \text{sgn}(\delta_m^{f_2})}{2} \\
& - \sum_{m=1}^{n_{h_1}} \text{sgn}(v_m^{h_1}) \frac{1 - \text{sgn}(\delta_m^{h_1})}{2} - \sum_{m=1}^{n_{h_2}} \text{sgn}(v_m^{h_2}) \frac{1 - \text{sgn}(\delta_m^{h_2})}{2} + \sum_{m=1}^{n_{i_1}} \text{sgn}(v_m^{i_1}) \frac{1 - \text{sgn}(\delta_m^{i_1})}{2}
\end{aligned} \tag{S38.4}$$

$$\mathcal{W}_5^{\text{gapless}} = \sum_{m=1}^{n_{d_1}} \text{sgn}(v_m^{d_1}) \frac{1 - \text{sgn}(\delta_m^{d_1})}{2} - \sum_{m=1}^{n_{e_1}} \text{sgn}(v_m^{e_1}) \frac{1 - \text{sgn}(\delta_m^{e_1})}{2} - \sum_{m=1}^{n_{f_1}} \text{sgn}(v_m^{f_1}) \frac{1 - \text{sgn}(\delta_m^{f_1})}{2} + \sum_{m=1}^{n_{f_2}} \text{sgn}(v_m^{f_2}) \frac{1 - \text{sgn}(\delta_m^{f_2})}{2} \tag{S38.5}$$

$$\mathcal{W}_6^{\text{gapless}} = \sum_{m=1}^{n_{d_2}} \text{sgn}(v_m^{d_2}) \frac{1 - \text{sgn}(\delta_m^{d_2})}{2} - \sum_{m=1}^{n_{e_1}} \text{sgn}(v_m^{e_1}) \frac{1 - \text{sgn}(\delta_m^{e_1})}{2} + \sum_{m=1}^{n_{f_1}} \text{sgn}(v_m^{f_1}) \frac{1 - \text{sgn}(\delta_m^{f_1})}{2} - \sum_{m=1}^{n_{f_2}} \text{sgn}(v_m^{f_2}) \frac{1 - \text{sgn}(\delta_m^{f_2})}{2} \tag{S38.6}$$

$$\mathcal{W}_7^{\text{gapless}} = \sum_{m=1}^{n_{g_1}} \text{sgn}(v_m^{g_1}) \frac{1 - \text{sgn}(\delta_m^{g_1})}{2} - \sum_{m=1}^{n_{g_2}} \text{sgn}(v_m^{g_2}) \frac{1 - \text{sgn}(\delta_m^{g_2})}{2} - \sum_{m=1}^{n_{h_1}} \text{sgn}(v_m^{h_1}) \frac{1 - \text{sgn}(\delta_m^{h_1})}{2} + \sum_{m=1}^{n_{h_2}} \text{sgn}(v_m^{h_2}) \frac{1 - \text{sgn}(\delta_m^{h_2})}{2} \tag{S38.7}$$

$$\mathcal{W}_1^{\text{gapped}} = - \sum_{m=1}^{n_{f_1}} \text{sgn}(v_m^{f_1}) \frac{1 - \text{sgn}(\delta_m^{f_1})}{2} + \sum_{m=1}^{n_{f_2}} \text{sgn}(v_m^{f_2}) \frac{1 - \text{sgn}(\delta_m^{f_2})}{2} \tag{S38.8}$$

$$\mathcal{W}_2^{\text{gapped}} = - \sum_{m=1}^{n_{h_1}} \text{sgn}(v_m^{h_1}) \frac{1 - \text{sgn}(\delta_m^{h_1})}{2} + \sum_{m=1}^{n_{h_2}} \text{sgn}(v_m^{h_2}) \frac{1 - \text{sgn}(\delta_m^{h_2})}{2} \tag{S38.9}$$

$$\begin{aligned}
\mathcal{W}_3^{\text{gapped}} = & 2 \sum_{m=1}^{n_{c_2}} \text{sgn}(v_m^{c_2}) \frac{1 - \text{sgn}(\delta_m^{c_2})}{2} - 2 \sum_{m=1}^{n_{f_1}} \text{sgn}(v_m^{f_1}) \frac{1 - \text{sgn}(\delta_m^{f_1})}{2} - 2 \sum_{m=1}^{n_{h_1}} \text{sgn}(v_m^{h_1}) \frac{1 - \text{sgn}(\delta_m^{h_1})}{2} \\
& + \sum_{m=1}^{n_{i_1}} \text{sgn}(v_m^{i_1}) \frac{1 - \text{sgn}(\delta_m^{i_1})}{2}
\end{aligned} \tag{S38.10}$$

## S39. SPACE GROUP NO. 39

| line segment                                      | character of irrep (generators only)                                                                                                    |
|---------------------------------------------------|-----------------------------------------------------------------------------------------------------------------------------------------|
| $a \ (0, t, 0)$                                   | $\begin{matrix} \{m_{100}  0 & 0 & \frac{1}{2}\} \\ a_1 & -i \\ a_2 & i \end{matrix}$                                                   |
| $b \ (0, 0, t)$                                   | $\begin{matrix} \{2_{001}  0 & 0 & 0\} & \{m_{100}  0 & 0 & \frac{1}{2}\} \\ b_1 & 0 & 0 \end{matrix}$                                  |
| $c \ (0, \frac{t}{2}, 1 - \frac{t}{2})$           | $\begin{matrix} \{m_{100}  0 & 0 & \frac{1}{2}\} \\ c_1 & -ie^{-\frac{1}{2}i\pi(2-t)} \\ c_2 & ie^{-\frac{1}{2}i\pi(2-t)} \end{matrix}$ |
| $d \ (\frac{1}{2}, t, 0)$                         | $\begin{matrix} \{m_{100}  0 & 0 & \frac{1}{2}\} \\ d_1 & -i \\ d_2 & i \end{matrix}$                                                   |
| $e \ (\frac{1}{2}, 0, t)$                         | $\begin{matrix} \{2_{001}  0 & 0 & 0\} & \{m_{100}  0 & 0 & \frac{1}{2}\} \\ e_1 & 0 & 0 \end{matrix}$                                  |
| $f \ (\frac{1}{2}, \frac{t}{2}, 1 - \frac{t}{2})$ | $\begin{matrix} \{m_{100}  0 & 0 & \frac{1}{2}\} \\ f_1 & -ie^{-\frac{1}{2}i\pi(2-t)} \\ f_2 & ie^{-\frac{1}{2}i\pi(2-t)} \end{matrix}$ |
| $g \ (\frac{t}{2}, 0, 0)$                         | $\begin{matrix} \{m_{010}  0 & 0 & \frac{1}{2}\} \\ g_1 & -i \\ g_2 & i \end{matrix}$                                                   |
| $h \ (\frac{t}{2}, 1, 0)$                         | $\begin{matrix} \{m_{010}  0 & 0 & \frac{1}{2}\} \\ h_1 & -i \\ h_2 & i \end{matrix}$                                                   |
| $i \ (\frac{t}{2}, \frac{1}{2}, \frac{1}{2})$     | $\begin{matrix} \{1  0 & 0 & 0\} \\ i_1 & 1 \end{matrix}$                                                                               |

$$\mathcal{W}_1^{\text{gapless}} = \sum_{m=1}^{n_{a_1}} \text{sgn}(v_m^{a_1}) \frac{1 - \text{sgn}(\delta_m^{a_1})}{2} - \sum_{m=1}^{n_{e_1}} \text{sgn}(v_m^{e_1}) \frac{1 - \text{sgn}(\delta_m^{e_1})}{2} - \sum_{m=1}^{n_{g_2}} \text{sgn}(v_m^{g_2}) \frac{1 - \text{sgn}(\delta_m^{g_2})}{2} + \sum_{m=1}^{n_{h_1}} \text{sgn}(v_m^{h_1}) \frac{1 - \text{sgn}(\delta_m^{h_1})}{2} \quad (\text{S39.1})$$

$$\mathcal{W}_2^{\text{gapless}} = \sum_{m=1}^{n_{a_2}} \text{sgn}(v_m^{a_2}) \frac{1 - \text{sgn}(\delta_m^{a_2})}{2} - \sum_{m=1}^{n_{e_1}} \text{sgn}(v_m^{e_1}) \frac{1 - \text{sgn}(\delta_m^{e_1})}{2} - \sum_{m=1}^{n_{g_2}} \text{sgn}(v_m^{g_2}) \frac{1 - \text{sgn}(\delta_m^{g_2})}{2} + \sum_{m=1}^{n_{h_1}} \text{sgn}(v_m^{h_1}) \frac{1 - \text{sgn}(\delta_m^{h_1})}{2} \quad (\text{S39.2})$$

$$\mathcal{W}_3^{\text{gapless}} = \sum_{m=1}^{n_{b_1}} \text{sgn}(v_m^{b_1}) \frac{1 - \text{sgn}(\delta_m^{b_1})}{2} - \sum_{m=1}^{n_{e_1}} \text{sgn}(v_m^{e_1}) \frac{1 - \text{sgn}(\delta_m^{e_1})}{2} - \sum_{m=1}^{n_{g_2}} \text{sgn}(v_m^{g_2}) \frac{1 - \text{sgn}(\delta_m^{g_2})}{2} + \sum_{m=1}^{n_{h_1}} \text{sgn}(v_m^{h_1}) \frac{1 - \text{sgn}(\delta_m^{h_1})}{2} \quad (\text{S39.3})$$

$$\begin{aligned} \mathcal{W}_4^{\text{gapless}} = & \sum_{m=1}^{n_{c_1}} \text{sgn}(v_m^{c_1}) \frac{1 - \text{sgn}(\delta_m^{c_1})}{2} + \sum_{m=1}^{n_{c_2}} \text{sgn}(v_m^{c_2}) \frac{1 - \text{sgn}(\delta_m^{c_2})}{2} - \sum_{m=1}^{n_{f_1}} \text{sgn}(v_m^{f_1}) \frac{1 - \text{sgn}(\delta_m^{f_1})}{2} - \sum_{m=1}^{n_{f_2}} \text{sgn}(v_m^{f_2}) \frac{1 - \text{sgn}(\delta_m^{f_2})}{2} \\ & - \sum_{m=1}^{n_{h_1}} \text{sgn}(v_m^{h_1}) \frac{1 - \text{sgn}(\delta_m^{h_1})}{2} - \sum_{m=1}^{n_{h_2}} \text{sgn}(v_m^{h_2}) \frac{1 - \text{sgn}(\delta_m^{h_2})}{2} + 2 \sum_{m=1}^{n_{i_1}} \text{sgn}(v_m^{i_1}) \frac{1 - \text{sgn}(\delta_m^{i_1})}{2} \end{aligned} \quad (\text{S39.4})$$

$$\mathcal{W}_5^{\text{gapless}} = \sum_{m=1}^{n_{d_1}} \text{sgn}(v_m^{d_1}) \frac{1 - \text{sgn}(\delta_m^{d_1})}{2} - \sum_{m=1}^{n_{e_1}} \text{sgn}(v_m^{e_1}) \frac{1 - \text{sgn}(\delta_m^{e_1})}{2} \quad (\text{S39.5})$$

$$\mathcal{W}_6^{\text{gapless}} = \sum_{m=1}^{n_{d_2}} \text{sgn}(v_m^{d_2}) \frac{1 - \text{sgn}(\delta_m^{d_2})}{2} - \sum_{m=1}^{n_{e_1}} \text{sgn}(v_m^{e_1}) \frac{1 - \text{sgn}(\delta_m^{e_1})}{2} \quad (\text{S39.6})$$

$$\mathcal{W}_7^{\text{gapless}} = \sum_{m=1}^{n_{g_1}} \text{sgn}(v_m^{g_1}) \frac{1 - \text{sgn}(\delta_m^{g_1})}{2} - \sum_{m=1}^{n_{g_2}} \text{sgn}(v_m^{g_2}) \frac{1 - \text{sgn}(\delta_m^{g_2})}{2} + \sum_{m=1}^{n_{h_1}} \text{sgn}(v_m^{h_1}) \frac{1 - \text{sgn}(\delta_m^{h_1})}{2} - \sum_{m=1}^{n_{h_2}} \text{sgn}(v_m^{h_2}) \frac{1 - \text{sgn}(\delta_m^{h_2})}{2} \quad (\text{S39.7})$$

$$\mathcal{W}_1^{\text{gapped}} = - \sum_{m=1}^{n_{h_1}} \text{sgn}(v_m^{h_1}) \frac{1 - \text{sgn}(\delta_m^{h_1})}{2} + \sum_{m=1}^{n_{h_2}} \text{sgn}(v_m^{h_2}) \frac{1 - \text{sgn}(\delta_m^{h_2})}{2} \quad (\text{S39.8})$$

$$\mathcal{X}_1 = \sum_{m=1}^{n_{c_2}} \frac{1 - \text{sgn}(\delta_m^{c_2})}{2} + \sum_{m=1}^{n_{f_2}} \frac{1 - \text{sgn}(\delta_m^{f_2})}{2} + \sum_{m=1}^{n_{h_1}} \frac{1 - \text{sgn}(\delta_m^{h_1})}{2} \quad \text{mod } 2 \quad (\text{S39.9})$$

$$\mathcal{X}_2 = \sum_{m=1}^{n_{c_2}} \frac{1 - \text{sgn}(\delta_m^{c_2})}{2} + \sum_{m=1}^{n_{f_1}} \frac{1 - \text{sgn}(\delta_m^{f_1})}{2} + \sum_{m=1}^{n_{h_1}} \frac{1 - \text{sgn}(\delta_m^{h_1})}{2} \quad \text{mod } 2 \quad (\text{S39.10})$$

#### S40. SPACE GROUP NO. 40

| line segment                                          | character of irrep (generators only)                                                                                                |
|-------------------------------------------------------|-------------------------------------------------------------------------------------------------------------------------------------|
| $a \quad (0, t, 0)$                                   | $\{m_{100}   \frac{1}{2} \ 0 \ 0\}$<br>$a_1 \quad -i$<br>$a_2 \quad i$                                                              |
| $b \quad (0, 0, t)$                                   | $\{2_{001}   0 \ 0 \ 0\} \ \{m_{100}   \frac{1}{2} \ 0 \ 0\}$<br>$b_1 \quad 0$                                                      |
| $c \quad (0, \frac{t}{2}, 1 - \frac{t}{2})$           | $\{m_{100}   \frac{1}{2} \ 0 \ 0\}$<br>$c_1 \quad -i$<br>$c_2 \quad i$                                                              |
| $d \quad (\frac{1}{2}, t, 0)$                         | $\{m_{100}   \frac{1}{2} \ 0 \ 0\}$<br>$d_1 \quad i$<br>$d_2 \quad -i$                                                              |
| $e \quad (\frac{1}{2}, 0, t)$                         | $\{2_{001}   0 \ 0 \ 0\} \ \{m_{100}   \frac{1}{2} \ 0 \ 0\}$<br>$e_1 \quad -i$<br>$e_2 \quad -i$<br>$e_3 \quad i$<br>$e_4 \quad i$ |
| $f \quad (\frac{1}{2}, \frac{t}{2}, 1 - \frac{t}{2})$ | $\{m_{100}   \frac{1}{2} \ 0 \ 0\}$<br>$f_1 \quad i$<br>$f_2 \quad -i$                                                              |
| $g \quad (\frac{t}{2}, 0, 0)$                         | $\{m_{010}   \frac{1}{2} \ 0 \ 0\}$<br>$g_1 \quad -ie^{-\frac{1}{2}i\pi t}$<br>$g_2 \quad ie^{-\frac{1}{2}i\pi t}$                  |
| $h \quad (\frac{t}{2}, 1, 0)$                         | $\{m_{010}   \frac{1}{2} \ 0 \ 0\}$<br>$h_1 \quad -ie^{-\frac{1}{2}i\pi t}$<br>$h_2 \quad ie^{-\frac{1}{2}i\pi t}$                  |
| $i \quad (\frac{t}{2}, \frac{1}{2}, \frac{1}{2})$     | $\{1   0 \ 0 \ 0\}$<br>$i_1 \quad 1$                                                                                                |

---


$$\begin{aligned}
\mathcal{W}_1^{\text{gapless}} = & \sum_{m=1}^{n_{a_1}} \text{sgn}(v_m^{a_1}) \frac{1 - \text{sgn}(\delta_m^{a_1})}{2} + 2 \sum_{m=1}^{n_{c_2}} \text{sgn}(v_m^{c_2}) \frac{1 - \text{sgn}(\delta_m^{c_2})}{2} - \sum_{m=1}^{n_{e_2}} \text{sgn}(v_m^{e_2}) \frac{1 - \text{sgn}(\delta_m^{e_2})}{2} + \sum_{m=1}^{n_{e_3}} \text{sgn}(v_m^{e_3}) \frac{1 - \text{sgn}(\delta_m^{e_3})}{2} \\
& - 2 \sum_{m=1}^{n_{e_4}} \text{sgn}(v_m^{e_4}) \frac{1 - \text{sgn}(\delta_m^{e_4})}{2} + \sum_{m=1}^{n_{f_1}} \text{sgn}(v_m^{f_1}) \frac{1 - \text{sgn}(\delta_m^{f_1})}{2} - 3 \sum_{m=1}^{n_{f_2}} \text{sgn}(v_m^{f_2}) \frac{1 - \text{sgn}(\delta_m^{f_2})}{2} \\
& - \sum_{m=1}^{n_{g_1}} \text{sgn}(v_m^{g_1}) \frac{1 - \text{sgn}(\delta_m^{g_1})}{2} - \sum_{m=1}^{n_{h_2}} \text{sgn}(v_m^{h_2}) \frac{1 - \text{sgn}(\delta_m^{h_2})}{2} + \sum_{m=1}^{n_{i_1}} \text{sgn}(v_m^{i_1}) \frac{1 - \text{sgn}(\delta_m^{i_1})}{2}
\end{aligned} \tag{S40.1}$$

$$\begin{aligned}
\mathcal{W}_2^{\text{gapless}} = & \sum_{m=1}^{n_{a_2}} \text{sgn}(v_m^{a_2}) \frac{1 - \text{sgn}(\delta_m^{a_2})}{2} - 2 \sum_{m=1}^{n_{c_2}} \text{sgn}(v_m^{c_2}) \frac{1 - \text{sgn}(\delta_m^{c_2})}{2} - \sum_{m=1}^{n_{e_2}} \text{sgn}(v_m^{e_2}) \frac{1 - \text{sgn}(\delta_m^{e_2})}{2} \\
& + \sum_{m=1}^{n_{e_3}} \text{sgn}(v_m^{e_3}) \frac{1 - \text{sgn}(\delta_m^{e_3})}{2} - 2 \sum_{m=1}^{n_{e_4}} \text{sgn}(v_m^{e_4}) \frac{1 - \text{sgn}(\delta_m^{e_4})}{2} + 3 \sum_{m=1}^{n_{f_1}} \text{sgn}(v_m^{f_1}) \frac{1 - \text{sgn}(\delta_m^{f_1})}{2} \\
& - \sum_{m=1}^{n_{f_2}} \text{sgn}(v_m^{f_2}) \frac{1 - \text{sgn}(\delta_m^{f_2})}{2} - \sum_{m=1}^{n_{g_1}} \text{sgn}(v_m^{g_1}) \frac{1 - \text{sgn}(\delta_m^{g_1})}{2} \\
& + 2 \sum_{m=1}^{n_{h_1}} \text{sgn}(v_m^{h_1}) \frac{1 - \text{sgn}(\delta_m^{h_1})}{2} + \sum_{m=1}^{n_{h_2}} \text{sgn}(v_m^{h_2}) \frac{1 - \text{sgn}(\delta_m^{h_2})}{2} - \sum_{m=1}^{n_{i_1}} \text{sgn}(v_m^{i_1}) \frac{1 - \text{sgn}(\delta_m^{i_1})}{2}
\end{aligned} \tag{S40.2}$$

$$\begin{aligned}
\mathcal{W}_3^{\text{gapless}} = & \sum_{m=1}^{n_{b_1}} \text{sgn}(v_m^{b_1}) \frac{1 - \text{sgn}(\delta_m^{b_1})}{2} - \sum_{m=1}^{n_{e_2}} \text{sgn}(v_m^{e_2}) \frac{1 - \text{sgn}(\delta_m^{e_2})}{2} + \sum_{m=1}^{n_{e_3}} \text{sgn}(v_m^{e_3}) \frac{1 - \text{sgn}(\delta_m^{e_3})}{2} \\
& - 2 \sum_{m=1}^{n_{e_4}} \text{sgn}(v_m^{e_4}) \frac{1 - \text{sgn}(\delta_m^{e_4})}{2} + 2 \sum_{m=1}^{n_{f_1}} \text{sgn}(v_m^{f_1}) \frac{1 - \text{sgn}(\delta_m^{f_1})}{2} \\
& - 2 \sum_{m=1}^{n_{f_2}} \text{sgn}(v_m^{f_2}) \frac{1 - \text{sgn}(\delta_m^{f_2})}{2} - \sum_{m=1}^{n_{g_1}} \text{sgn}(v_m^{g_1}) \frac{1 - \text{sgn}(\delta_m^{g_1})}{2} + \sum_{m=1}^{n_{h_1}} \text{sgn}(v_m^{h_1}) \frac{1 - \text{sgn}(\delta_m^{h_1})}{2}
\end{aligned} \tag{S40.3}$$

$$\begin{aligned}
\mathcal{W}_4^{\text{gapless}} = & \sum_{m=1}^{n_{c_1}} \text{sgn}(v_m^{c_1}) \frac{1 - \text{sgn}(\delta_m^{c_1})}{2} + \sum_{m=1}^{n_{c_2}} \text{sgn}(v_m^{c_2}) \frac{1 - \text{sgn}(\delta_m^{c_2})}{2} - \sum_{m=1}^{n_{f_1}} \text{sgn}(v_m^{f_1}) \frac{1 - \text{sgn}(\delta_m^{f_1})}{2} - \sum_{m=1}^{n_{f_2}} \text{sgn}(v_m^{f_2}) \frac{1 - \text{sgn}(\delta_m^{f_2})}{2} \\
& - \sum_{m=1}^{n_{h_1}} \text{sgn}(v_m^{h_1}) \frac{1 - \text{sgn}(\delta_m^{h_1})}{2} - \sum_{m=1}^{n_{h_2}} \text{sgn}(v_m^{h_2}) \frac{1 - \text{sgn}(\delta_m^{h_2})}{2} + \sum_{m=1}^{n_{i_1}} \text{sgn}(v_m^{i_1}) \frac{1 - \text{sgn}(\delta_m^{i_1})}{2}
\end{aligned} \tag{S40.4}$$

$$\begin{aligned}
\mathcal{W}_5^{\text{gapless}} = & \sum_{m=1}^{n_{d_1}} \text{sgn}(v_m^{d_1}) \frac{1 - \text{sgn}(\delta_m^{d_1})}{2} - \sum_{m=1}^{n_{e_2}} \text{sgn}(v_m^{e_2}) \frac{1 - \text{sgn}(\delta_m^{e_2})}{2} - \sum_{m=1}^{n_{e_4}} \text{sgn}(v_m^{e_4}) \frac{1 - \text{sgn}(\delta_m^{e_4})}{2} \\
& + \sum_{m=1}^{n_{f_1}} \text{sgn}(v_m^{f_1}) \frac{1 - \text{sgn}(\delta_m^{f_1})}{2} - \sum_{m=1}^{n_{f_2}} \text{sgn}(v_m^{f_2}) \frac{1 - \text{sgn}(\delta_m^{f_2})}{2}
\end{aligned} \tag{S40.5}$$

$$\begin{aligned} \mathcal{W}_6^{\text{gapless}} = & \sum_{m=1}^{n_{e_1}} \text{sgn}(v_m^{e_1}) \frac{1 - \text{sgn}(\delta_m^{e_1})}{2} - \sum_{m=1}^{n_{e_2}} \text{sgn}(v_m^{e_2}) \frac{1 - \text{sgn}(\delta_m^{e_2})}{2} + \sum_{m=1}^{n_{e_3}} \text{sgn}(v_m^{e_3}) \frac{1 - \text{sgn}(\delta_m^{e_3})}{2} \\ & - \sum_{m=1}^{n_{e_4}} \text{sgn}(v_m^{e_4}) \frac{1 - \text{sgn}(\delta_m^{e_4})}{2} + 2 \sum_{m=1}^{n_{f_1}} \text{sgn}(v_m^{f_1}) \frac{1 - \text{sgn}(\delta_m^{f_1})}{2} - 2 \sum_{m=1}^{n_{f_2}} \text{sgn}(v_m^{f_2}) \frac{1 - \text{sgn}(\delta_m^{f_2})}{2} \end{aligned} \quad (\text{S40.6})$$

$$\begin{aligned} \mathcal{W}_7^{\text{gapless}} = & 2 \sum_{m=1}^{n_{e_3}} \text{sgn}(v_m^{e_3}) \frac{1 - \text{sgn}(\delta_m^{e_3})}{2} - 2 \sum_{m=1}^{n_{e_4}} \text{sgn}(v_m^{e_4}) \frac{1 - \text{sgn}(\delta_m^{e_4})}{2} + 2 \sum_{m=1}^{n_{f_1}} \text{sgn}(v_m^{f_1}) \frac{1 - \text{sgn}(\delta_m^{f_1})}{2} \\ & - 2 \sum_{m=1}^{n_{f_2}} \text{sgn}(v_m^{f_2}) \frac{1 - \text{sgn}(\delta_m^{f_2})}{2} - \sum_{m=1}^{n_{g_1}} \text{sgn}(v_m^{g_1}) \frac{1 - \text{sgn}(\delta_m^{g_1})}{2} + \sum_{m=1}^{n_{g_2}} \text{sgn}(v_m^{g_2}) \frac{1 - \text{sgn}(\delta_m^{g_2})}{2} \\ & + \sum_{m=1}^{n_{h_1}} \text{sgn}(v_m^{h_1}) \frac{1 - \text{sgn}(\delta_m^{h_1})}{2} - \sum_{m=1}^{n_{h_2}} \text{sgn}(v_m^{h_2}) \frac{1 - \text{sgn}(\delta_m^{h_2})}{2} \end{aligned} \quad (\text{S40.7})$$

$$\mathcal{W}_1^{\text{gapped}} = - \sum_{m=1}^{n_{f_1}} \text{sgn}(v_m^{f_1}) \frac{1 - \text{sgn}(\delta_m^{f_1})}{2} + \sum_{m=1}^{n_{f_2}} \text{sgn}(v_m^{f_2}) \frac{1 - \text{sgn}(\delta_m^{f_2})}{2} \quad (\text{S40.8})$$

$$\begin{aligned} \mathcal{W}_2^{\text{gapped}} = & - \sum_{m=1}^{n_{e_2}} \text{sgn}(v_m^{e_2}) \frac{1 - \text{sgn}(\delta_m^{e_2})}{2} - \sum_{m=1}^{n_{e_3}} \text{sgn}(v_m^{e_3}) \frac{1 - \text{sgn}(\delta_m^{e_3})}{2} + 2 \sum_{m=1}^{n_{e_4}} \text{sgn}(v_m^{e_4}) \frac{1 - \text{sgn}(\delta_m^{e_4})}{2} \\ & - \sum_{m=1}^{n_{f_1}} \text{sgn}(v_m^{f_1}) \frac{1 - \text{sgn}(\delta_m^{f_1})}{2} + \sum_{m=1}^{n_{f_2}} \text{sgn}(v_m^{f_2}) \frac{1 - \text{sgn}(\delta_m^{f_2})}{2} + \sum_{m=1}^{n_{g_1}} \text{sgn}(v_m^{g_1}) \frac{1 - \text{sgn}(\delta_m^{g_1})}{2} \\ & - \sum_{m=1}^{n_{g_2}} \text{sgn}(v_m^{g_2}) \frac{1 - \text{sgn}(\delta_m^{g_2})}{2} - \sum_{m=1}^{n_{h_1}} \text{sgn}(v_m^{h_1}) \frac{1 - \text{sgn}(\delta_m^{h_1})}{2} + \sum_{m=1}^{n_{h_2}} \text{sgn}(v_m^{h_2}) \frac{1 - \text{sgn}(\delta_m^{h_2})}{2} \end{aligned} \quad (\text{S40.9})$$

$$\begin{aligned} \mathcal{W}_3^{\text{gapped}} = & 2 \sum_{m=1}^{n_{c_2}} \text{sgn}(v_m^{c_2}) \frac{1 - \text{sgn}(\delta_m^{c_2})}{2} - 2 \sum_{m=1}^{n_{e_2}} \text{sgn}(v_m^{e_2}) \frac{1 - \text{sgn}(\delta_m^{e_2})}{2} + 2 \sum_{m=1}^{n_{e_4}} \text{sgn}(v_m^{e_4}) \frac{1 - \text{sgn}(\delta_m^{e_4})}{2} \\ & - 2 \sum_{m=1}^{n_{f_1}} \text{sgn}(v_m^{f_1}) \frac{1 - \text{sgn}(\delta_m^{f_1})}{2} + \sum_{m=1}^{n_{g_1}} \text{sgn}(v_m^{g_1}) \frac{1 - \text{sgn}(\delta_m^{g_1})}{2} - \sum_{m=1}^{n_{g_2}} \text{sgn}(v_m^{g_2}) \frac{1 - \text{sgn}(\delta_m^{g_2})}{2} \\ & - 2 \sum_{m=1}^{n_{h_1}} \text{sgn}(v_m^{h_1}) \frac{1 - \text{sgn}(\delta_m^{h_1})}{2} + \sum_{m=1}^{n_{i_1}} \text{sgn}(v_m^{i_1}) \frac{1 - \text{sgn}(\delta_m^{i_1})}{2} \end{aligned} \quad (\text{S40.10})$$

$$\mathcal{X}_1 = \sum_{m=1}^{n_{g_1}} \frac{1 - \text{sgn}(\delta_m^{g_1})}{2} + \sum_{m=1}^{n_{g_2}} \frac{1 - \text{sgn}(\delta_m^{g_2})}{2} \quad \text{mod } 2 \quad (\text{S40.11})$$

#### S41. SPACE GROUP NO. 41

|              |                                      |
|--------------|--------------------------------------|
| line segment | character of irrep (generators only) |
|--------------|--------------------------------------|

|                                                       |                                                                                                                                                                                                                                                                           |
|-------------------------------------------------------|---------------------------------------------------------------------------------------------------------------------------------------------------------------------------------------------------------------------------------------------------------------------------|
| $a \quad (0, t, 0)$                                   | $\begin{matrix} \{m_{100}   \frac{1}{2} & 0 & \frac{1}{2} \} \\ a_1 & -i \\ a_2 & i \end{matrix}$                                                                                                                                                                         |
| $b \quad (0, 0, t)$                                   | $\begin{matrix} \{2_{001}   0 & 0 & 0 \} & \{m_{100}   \frac{1}{2} & 0 & \frac{1}{2} \} \\ b_1 & 0 & 0 \end{matrix}$                                                                                                                                                      |
| $c \quad (0, \frac{t}{2}, 1 - \frac{t}{2})$           | $\begin{matrix} \{m_{100}   \frac{1}{2} & 0 & \frac{1}{2} \} \\ c_1 & -ie^{-\frac{1}{2}i\pi(2-t)} \\ c_2 & ie^{-\frac{1}{2}i\pi(2-t)} \end{matrix}$                                                                                                                       |
| $d \quad (\frac{1}{2}, t, 0)$                         | $\begin{matrix} \{m_{100}   \frac{1}{2} & 0 & \frac{1}{2} \} \\ d_1 & i \\ d_2 & -i \end{matrix}$                                                                                                                                                                         |
| $e \quad (\frac{1}{2}, 0, t)$                         | $\begin{matrix} \{2_{001}   0 & 0 & 0 \} & \{m_{100}   \frac{1}{2} & 0 & \frac{1}{2} \} \\ e_1 & -i & -e^{-\frac{1}{2}i\pi(2t+1)} \\ e_2 & -i & e^{-\frac{1}{2}i\pi(2t+1)} \\ e_3 & i & -e^{-\frac{1}{2}i\pi(2t+1)} \\ e_4 & i & e^{-\frac{1}{2}i\pi(2t+1)} \end{matrix}$ |
| $f \quad (\frac{1}{2}, \frac{t}{2}, 1 - \frac{t}{2})$ | $\begin{matrix} \{m_{100}   \frac{1}{2} & 0 & \frac{1}{2} \} \\ f_1 & -e^{-\frac{1}{2}i\pi(3-t)} \\ f_2 & e^{-\frac{1}{2}i\pi(3-t)} \end{matrix}$                                                                                                                         |
| $g \quad (\frac{t}{2}, 0, 0)$                         | $\begin{matrix} \{m_{010}   \frac{1}{2} & 0 & \frac{1}{2} \} \\ g_1 & -ie^{-\frac{1}{2}i\pi t} \\ g_2 & ie^{-\frac{1}{2}i\pi t} \end{matrix}$                                                                                                                             |
| $h \quad (\frac{t}{2}, 1, 0)$                         | $\begin{matrix} \{m_{010}   \frac{1}{2} & 0 & \frac{1}{2} \} \\ h_1 & -ie^{-\frac{1}{2}i\pi t} \\ h_2 & ie^{-\frac{1}{2}i\pi t} \end{matrix}$                                                                                                                             |
| $i \quad (\frac{t}{2}, \frac{1}{2}, \frac{1}{2})$     | $\begin{matrix} \{1   0 & 0 & 0 \} \\ i_1 & 1 \end{matrix}$                                                                                                                                                                                                               |

$$\begin{aligned} \mathcal{W}_1^{\text{gapless}} = & \sum_{m=1}^{n_{a_1}} \text{sgn}(v_m^{a_1}) \frac{1 - \text{sgn}(\delta_m^{a_1})}{2} - \sum_{m=1}^{n_{e_2}} \text{sgn}(v_m^{e_2}) \frac{1 - \text{sgn}(\delta_m^{e_2})}{2} + \sum_{m=1}^{n_{e_3}} \text{sgn}(v_m^{e_3}) \frac{1 - \text{sgn}(\delta_m^{e_3})}{2} \\ & - 2 \sum_{m=1}^{n_{e_4}} \text{sgn}(v_m^{e_4}) \frac{1 - \text{sgn}(\delta_m^{e_4})}{2} - \sum_{m=1}^{n_{g_1}} \text{sgn}(v_m^{g_1}) \frac{1 - \text{sgn}(\delta_m^{g_1})}{2} + \sum_{m=1}^{n_{h_2}} \text{sgn}(v_m^{h_2}) \frac{1 - \text{sgn}(\delta_m^{h_2})}{2} \end{aligned} \quad (\text{S41.1})$$

$$\begin{aligned} \mathcal{W}_2^{\text{gapless}} = & \sum_{m=1}^{n_{a_2}} \text{sgn}(v_m^{a_2}) \frac{1 - \text{sgn}(\delta_m^{a_2})}{2} - \sum_{m=1}^{n_{e_2}} \text{sgn}(v_m^{e_2}) \frac{1 - \text{sgn}(\delta_m^{e_2})}{2} + \sum_{m=1}^{n_{e_3}} \text{sgn}(v_m^{e_3}) \frac{1 - \text{sgn}(\delta_m^{e_3})}{2} \\ & - 2 \sum_{m=1}^{n_{e_4}} \text{sgn}(v_m^{e_4}) \frac{1 - \text{sgn}(\delta_m^{e_4})}{2} - \sum_{m=1}^{n_{g_1}} \text{sgn}(v_m^{g_1}) \frac{1 - \text{sgn}(\delta_m^{g_1})}{2} + \sum_{m=1}^{n_{h_2}} \text{sgn}(v_m^{h_2}) \frac{1 - \text{sgn}(\delta_m^{h_2})}{2} \end{aligned} \quad (\text{S41.2})$$

$$\begin{aligned} \mathcal{W}_3^{\text{gapless}} = & \sum_{m=1}^{n_{b_1}} \text{sgn}(v_m^{b_1}) \frac{1 - \text{sgn}(\delta_m^{b_1})}{2} - \sum_{m=1}^{n_{e_2}} \text{sgn}(v_m^{e_2}) \frac{1 - \text{sgn}(\delta_m^{e_2})}{2} + \sum_{m=1}^{n_{e_3}} \text{sgn}(v_m^{e_3}) \frac{1 - \text{sgn}(\delta_m^{e_3})}{2} \\ & - 2 \sum_{m=1}^{n_{e_4}} \text{sgn}(v_m^{e_4}) \frac{1 - \text{sgn}(\delta_m^{e_4})}{2} - \sum_{m=1}^{n_{g_1}} \text{sgn}(v_m^{g_1}) \frac{1 - \text{sgn}(\delta_m^{g_1})}{2} + \sum_{m=1}^{n_{h_2}} \text{sgn}(v_m^{h_2}) \frac{1 - \text{sgn}(\delta_m^{h_2})}{2} \end{aligned} \quad (\text{S41.3})$$

$$\begin{aligned} \mathcal{W}_4^{\text{gapless}} = & \sum_{m=1}^{n_{c_1}} \text{sgn}(v_m^{c_1}) \frac{1 - \text{sgn}(\delta_m^{c_1})}{2} + \sum_{m=1}^{n_{c_2}} \text{sgn}(v_m^{c_2}) \frac{1 - \text{sgn}(\delta_m^{c_2})}{2} - \sum_{m=1}^{n_{f_1}} \text{sgn}(v_m^{f_1}) \frac{1 - \text{sgn}(\delta_m^{f_1})}{2} - \sum_{m=1}^{n_{f_2}} \text{sgn}(v_m^{f_2}) \frac{1 - \text{sgn}(\delta_m^{f_2})}{2} \\ & - \sum_{m=1}^{n_{h_1}} \text{sgn}(v_m^{h_1}) \frac{1 - \text{sgn}(\delta_m^{h_1})}{2} - \sum_{m=1}^{n_{h_2}} \text{sgn}(v_m^{h_2}) \frac{1 - \text{sgn}(\delta_m^{h_2})}{2} + 2 \sum_{m=1}^{n_{i_1}} \text{sgn}(v_m^{i_1}) \frac{1 - \text{sgn}(\delta_m^{i_1})}{2} \end{aligned} \quad (\text{S41.4})$$

$$\mathcal{W}_5^{\text{gapless}} = \sum_{m=1}^{n_{d_1}} \text{sgn}(v_m^{d_1}) \frac{1 - \text{sgn}(\delta_m^{d_1})}{2} - \sum_{m=1}^{n_{e_2}} \text{sgn}(v_m^{e_2}) \frac{1 - \text{sgn}(\delta_m^{e_2})}{2} - \sum_{m=1}^{n_{e_4}} \text{sgn}(v_m^{e_4}) \frac{1 - \text{sgn}(\delta_m^{e_4})}{2} \quad (\text{S41.5})$$

$$\mathcal{W}_6^{\text{gapless}} = \sum_{m=1}^{n_{e_1}} \text{sgn}(v_m^{e_1}) \frac{1 - \text{sgn}(\delta_m^{e_1})}{2} - \sum_{m=1}^{n_{e_2}} \text{sgn}(v_m^{e_2}) \frac{1 - \text{sgn}(\delta_m^{e_2})}{2} + \sum_{m=1}^{n_{e_3}} \text{sgn}(v_m^{e_3}) \frac{1 - \text{sgn}(\delta_m^{e_3})}{2} - \sum_{m=1}^{n_{e_4}} \text{sgn}(v_m^{e_4}) \frac{1 - \text{sgn}(\delta_m^{e_4})}{2} \quad (\text{S41.6})$$

$$\begin{aligned} \mathcal{W}_7^{\text{gapless}} = & 2 \sum_{m=1}^{n_{e_3}} \text{sgn}(v_m^{e_3}) \frac{1 - \text{sgn}(\delta_m^{e_3})}{2} - 2 \sum_{m=1}^{n_{e_4}} \text{sgn}(v_m^{e_4}) \frac{1 - \text{sgn}(\delta_m^{e_4})}{2} - \sum_{m=1}^{n_{g_1}} \text{sgn}(v_m^{g_1}) \frac{1 - \text{sgn}(\delta_m^{g_1})}{2} \\ & + \sum_{m=1}^{n_{g_2}} \text{sgn}(v_m^{g_2}) \frac{1 - \text{sgn}(\delta_m^{g_2})}{2} - \sum_{m=1}^{n_{h_1}} \text{sgn}(v_m^{h_1}) \frac{1 - \text{sgn}(\delta_m^{h_1})}{2} + \sum_{m=1}^{n_{h_2}} \text{sgn}(v_m^{h_2}) \frac{1 - \text{sgn}(\delta_m^{h_2})}{2} \end{aligned} \quad (\text{S41.7})$$

$$\mathcal{W}_1^{\text{gapped}} = - \sum_{m=1}^{n_{e_2}} \text{sgn}(v_m^{e_2}) \frac{1 - \text{sgn}(\delta_m^{e_2})}{2} + \sum_{m=1}^{n_{e_3}} \text{sgn}(v_m^{e_3}) \frac{1 - \text{sgn}(\delta_m^{e_3})}{2} \quad (\text{S41.8})$$

$$\mathcal{X}_1 = \sum_{m=1}^{n_{c_2}} \frac{1 - \text{sgn}(\delta_m^{c_2})}{2} + \sum_{m=1}^{n_{h_1}} \frac{1 - \text{sgn}(\delta_m^{h_1})}{2} \quad \text{mod } 2 \quad (\text{S41.9})$$

$$\mathcal{X}_2 = \sum_{m=1}^{n_{c_2}} \frac{1 - \text{sgn}(\delta_m^{c_2})}{2} + \sum_{m=1}^{n_{f_1}} \frac{1 - \text{sgn}(\delta_m^{f_1})}{2} + \sum_{m=1}^{n_{f_2}} \frac{1 - \text{sgn}(\delta_m^{f_2})}{2} + \sum_{m=1}^{n_{h_1}} \frac{1 - \text{sgn}(\delta_m^{h_1})}{2} \quad \text{mod } 2 \quad (\text{S41.10})$$

$$\begin{aligned} \mathcal{X}_3 = & -2 \sum_{m=1}^{n_{e_3}} \text{sgn}(v_m^{e_3}) \frac{1 - \text{sgn}(\delta_m^{e_3})}{2} + 2 \sum_{m=1}^{n_{e_4}} \text{sgn}(v_m^{e_4}) \frac{1 - \text{sgn}(\delta_m^{e_4})}{2} - 2 \sum_{m=1}^{n_{f_1}} \text{sgn}(v_m^{f_1}) \frac{1 - \text{sgn}(\delta_m^{f_1})}{2} \\ & + \sum_{m=1}^{n_{g_1}} \text{sgn}(v_m^{g_1}) \frac{1 - \text{sgn}(\delta_m^{g_1})}{2} - \sum_{m=1}^{n_{g_2}} \text{sgn}(v_m^{g_2}) \frac{1 - \text{sgn}(\delta_m^{g_2})}{2} \quad \text{mod } 4 \end{aligned} \quad (\text{S41.11})$$

#### S42. SPACE GROUP NO. 42

|              |                                      |
|--------------|--------------------------------------|
| line segment | character of irrep (generators only) |
|--------------|--------------------------------------|



|                                                     |                                                                                       |
|-----------------------------------------------------|---------------------------------------------------------------------------------------|
| $a \ (t, 0, 0)$                                     | $\{m_{010}   0 \ 0 \ 0\}$<br>$a_1 \quad -i$<br>$a_2 \quad i$                          |
| $b \ (1, t, 0)$                                     | $\{m_{100}   0 \ 0 \ 0\}$<br>$b_1 \quad -i$<br>$b_2 \quad i$                          |
| $c \ (0, 0, 1-t)$                                   | $\{2_{001}   0 \ 0 \ 0\} \ \{m_{100}   0 \ 0 \ 0\}$<br>$c_1 \quad 0$<br>$c_2 \quad 0$ |
| $d \ (1-t, 1, 0)$                                   | $\{m_{010}   0 \ 0 \ 0\}$<br>$d_1 \quad -i$<br>$d_2 \quad i$                          |
| $e \ (0, t, 0)$                                     | $\{m_{100}   0 \ 0 \ 0\}$<br>$e_1 \quad -i$<br>$e_2 \quad i$                          |
| $f \ (0, 1, 1-t)$                                   | $\{2_{001}   0 \ 0 \ 0\} \ \{m_{100}   0 \ 0 \ 0\}$<br>$f_1 \quad 0$<br>$f_2 \quad 0$ |
| $g \ (1-t, 0, t)$                                   | $\{m_{010}   0 \ 0 \ 0\}$<br>$g_1 \quad -i$<br>$g_2 \quad i$                          |
| $h \ (\frac{t+1}{2}, \frac{1-t}{2}, \frac{1-t}{2})$ | $\{1   0 \ 0 \ 0\}$<br>$h_1 \quad 1$                                                  |

$$\mathcal{W}_1^{\text{gapless}} = \sum_{m=1}^{n_{a_1}} \text{sgn}(v_m^{a_1}) \frac{1 - \text{sgn}(\delta_m^{a_1})}{2} + \sum_{m=1}^{n_{c_1}} \text{sgn}(v_m^{c_1}) \frac{1 - \text{sgn}(\delta_m^{c_1})}{2} + \sum_{m=1}^{n_{g_1}} \text{sgn}(v_m^{g_1}) \frac{1 - \text{sgn}(\delta_m^{g_1})}{2} \quad (\text{S42.1})$$

$$\mathcal{W}_2^{\text{gapless}} = \sum_{m=1}^{n_{a_2}} \text{sgn}(v_m^{a_2}) \frac{1 - \text{sgn}(\delta_m^{a_2})}{2} + \sum_{m=1}^{n_{c_1}} \text{sgn}(v_m^{c_1}) \frac{1 - \text{sgn}(\delta_m^{c_1})}{2} + \sum_{m=1}^{n_{g_2}} \text{sgn}(v_m^{g_2}) \frac{1 - \text{sgn}(\delta_m^{g_2})}{2} \quad (\text{S42.2})$$

$$\mathcal{W}_3^{\text{gapless}} = \sum_{m=1}^{n_{b_1}} \text{sgn}(v_m^{b_1}) \frac{1 - \text{sgn}(\delta_m^{b_1})}{2} + \sum_{m=1}^{n_{c_1}} \text{sgn}(v_m^{c_1}) \frac{1 - \text{sgn}(\delta_m^{c_1})}{2} + \sum_{m=1}^{n_{e_2}} \text{sgn}(v_m^{e_2}) \frac{1 - \text{sgn}(\delta_m^{e_2})}{2} - \sum_{m=1}^{n_{f_1}} \text{sgn}(v_m^{f_1}) \frac{1 - \text{sgn}(\delta_m^{f_1})}{2} \quad (\text{S42.3})$$

$$\mathcal{W}_4^{\text{gapless}} = \sum_{m=1}^{n_{b_2}} \text{sgn}(v_m^{b_2}) \frac{1 - \text{sgn}(\delta_m^{b_2})}{2} + \sum_{m=1}^{n_{c_1}} \text{sgn}(v_m^{c_1}) \frac{1 - \text{sgn}(\delta_m^{c_1})}{2} + \sum_{m=1}^{n_{e_1}} \text{sgn}(v_m^{e_1}) \frac{1 - \text{sgn}(\delta_m^{e_1})}{2} - \sum_{m=1}^{n_{f_1}} \text{sgn}(v_m^{f_1}) \frac{1 - \text{sgn}(\delta_m^{f_1})}{2} \quad (\text{S42.4})$$

$$\begin{aligned} \mathcal{W}_5^{\text{gapless}} = & 2 \sum_{m=1}^{n_{c_1}} \text{sgn}(v_m^{c_1}) \frac{1 - \text{sgn}(\delta_m^{c_1})}{2} + \sum_{m=1}^{n_{e_1}} \text{sgn}(v_m^{e_1}) \frac{1 - \text{sgn}(\delta_m^{e_1})}{2} + \sum_{m=1}^{n_{e_2}} \text{sgn}(v_m^{e_2}) \frac{1 - \text{sgn}(\delta_m^{e_2})}{2} \\ & - 2 \sum_{m=1}^{n_{f_1}} \text{sgn}(v_m^{f_1}) \frac{1 - \text{sgn}(\delta_m^{f_1})}{2} + \sum_{m=1}^{n_{g_1}} \text{sgn}(v_m^{g_1}) \frac{1 - \text{sgn}(\delta_m^{g_1})}{2} + \sum_{m=1}^{n_{g_2}} \text{sgn}(v_m^{g_2}) \frac{1 - \text{sgn}(\delta_m^{g_2})}{2} \end{aligned} \quad (\text{S42.5})$$

$$\mathcal{W}_6^{\text{gapless}} = \sum_{m=1}^{n_{d_1}} \text{sgn}(v_m^{d_1}) \frac{1 - \text{sgn}(\delta_m^{d_1})}{2} - \sum_{m=1}^{n_{f_1}} \text{sgn}(v_m^{f_1}) \frac{1 - \text{sgn}(\delta_m^{f_1})}{2} + \sum_{m=1}^{n_{g_2}} \text{sgn}(v_m^{g_2}) \frac{1 - \text{sgn}(\delta_m^{g_2})}{2} \quad (\text{S42.6})$$

$$\mathcal{W}_7^{\text{gapless}} = \sum_{m=1}^{n_{d_2}} \text{sgn}(v_m^{d_2}) \frac{1 - \text{sgn}(\delta_m^{d_2})}{2} - \sum_{m=1}^{n_{f_1}} \text{sgn}(v_m^{f_1}) \frac{1 - \text{sgn}(\delta_m^{f_1})}{2} + \sum_{m=1}^{n_{g_1}} \text{sgn}(v_m^{g_1}) \frac{1 - \text{sgn}(\delta_m^{g_1})}{2} \quad (\text{S42.7})$$

$$\begin{aligned} \mathcal{W}_1^{\text{gapped}} = & - \sum_{m=1}^{n_{c_1}} \text{sgn}(v_m^{c_1}) \frac{1 - \text{sgn}(\delta_m^{c_1})}{2} - \sum_{m=1}^{n_{e_2}} \text{sgn}(v_m^{e_2}) \frac{1 - \text{sgn}(\delta_m^{e_2})}{2} + \sum_{m=1}^{n_{f_1}} \text{sgn}(v_m^{f_1}) \frac{1 - \text{sgn}(\delta_m^{f_1})}{2} \\ & - \sum_{m=1}^{n_{g_1}} \text{sgn}(v_m^{g_1}) \frac{1 - \text{sgn}(\delta_m^{g_1})}{2} \end{aligned} \quad (\text{S42.8})$$

$$\mathcal{W}_2^{\text{gapped}} = - \sum_{m=1}^{n_{e_1}} \text{sgn}(v_m^{e_1}) \frac{1 - \text{sgn}(\delta_m^{e_1})}{2} + \sum_{m=1}^{n_{e_2}} \text{sgn}(v_m^{e_2}) \frac{1 - \text{sgn}(\delta_m^{e_2})}{2} \quad (\text{S42.9})$$

$$\mathcal{X}_1 = \sum_{m=1}^{n_{h_1}} \frac{1 - \text{sgn}(\delta_m^{h_1})}{2} \mod 2 \quad (\text{S42.10})$$

### S43. SPACE GROUP NO. 43

| line segment                                        | character of irrep (generators only)                                                                                                                                                                                                                                                          |
|-----------------------------------------------------|-----------------------------------------------------------------------------------------------------------------------------------------------------------------------------------------------------------------------------------------------------------------------------------------------|
| $a \ (t, 0, 0)$                                     | $\{m_{010}   \frac{1}{4} \ \frac{1}{4} \ \frac{1}{4}\}$<br>$a_1 \quad -ie^{-\frac{1}{2}i\pi t}$<br>$a_2 \quad ie^{-\frac{1}{2}i\pi t}$                                                                                                                                                        |
| $b \ (1, t, 0)$                                     | $\{m_{100}   \frac{1}{4} \ \frac{1}{4} \ \frac{1}{4}\}$<br>$b_1 \quad -e^{-\frac{1}{2}i\pi(t+1)}$<br>$b_2 \quad e^{-\frac{1}{2}i\pi(t+1)}$                                                                                                                                                    |
| $c \ (0, 0, 1-t)$                                   | $\{2_{001}   0 \ 0 \ 0\} \ \{m_{100}   \frac{1}{4} \ \frac{1}{4} \ \frac{1}{4}\}$<br>$c_1 \quad 0 \quad 0$                                                                                                                                                                                    |
| $d \ (1-t, 1, 0)$                                   | $\{m_{010}   \frac{1}{4} \ \frac{1}{4} \ \frac{1}{4}\}$<br>$d_1 \quad -e^{-\frac{1}{2}i\pi(2-t)}$<br>$d_2 \quad e^{-\frac{1}{2}i\pi(2-t)}$                                                                                                                                                    |
| $e \ (0, t, 0)$                                     | $\{m_{100}   \frac{1}{4} \ \frac{1}{4} \ \frac{1}{4}\}$<br>$e_1 \quad -ie^{-\frac{1}{2}i\pi t}$<br>$e_2 \quad ie^{-\frac{1}{2}i\pi t}$                                                                                                                                                        |
| $f \ (0, 1, 1-t)$                                   | $\{2_{001}   0 \ 0 \ 0\} \ \{m_{100}   \frac{1}{4} \ \frac{1}{4} \ \frac{1}{4}\}$<br>$f_1 \quad -i \quad -ie^{-\frac{1}{2}i\pi(2-t)}$<br>$f_2 \quad -i \quad ie^{-\frac{1}{2}i\pi(2-t)}$<br>$f_3 \quad i \quad -ie^{-\frac{1}{2}i\pi(2-t)}$<br>$f_4 \quad i \quad ie^{-\frac{1}{2}i\pi(2-t)}$ |
| $g \ (1-t, 0, t)$                                   | $\{m_{010}   \frac{1}{4} \ \frac{1}{4} \ \frac{1}{4}\}$<br>$g_1 \quad -1$<br>$g_2 \quad 1$                                                                                                                                                                                                    |
| $h \ (\frac{t+1}{2}, \frac{1-t}{2}, \frac{1-t}{2})$ | $\{1   0 \ 0 \ 0\}$<br>$h_1 \quad 1$                                                                                                                                                                                                                                                          |

$$\mathcal{W}_1^{\text{gapless}} = \sum_{m=1}^{n_{a_1}} \text{sgn}(v_m^{a_1}) \frac{1 - \text{sgn}(\delta_m^{a_1})}{2} + \sum_{m=1}^{n_{c_1}} \text{sgn}(v_m^{c_1}) \frac{1 - \text{sgn}(\delta_m^{c_1})}{2} + \sum_{m=1}^{n_{g_1}} \text{sgn}(v_m^{g_1}) \frac{1 - \text{sgn}(\delta_m^{g_1})}{2} \quad (\text{S43.1})$$

$$\mathcal{W}_2^{\text{gapless}} = \sum_{m=1}^{n_{a_2}} \text{sgn}(v_m^{a_2}) \frac{1 - \text{sgn}(\delta_m^{a_2})}{2} + \sum_{m=1}^{n_{c_1}} \text{sgn}(v_m^{c_1}) \frac{1 - \text{sgn}(\delta_m^{c_1})}{2} + \sum_{m=1}^{n_{g_2}} \text{sgn}(v_m^{g_2}) \frac{1 - \text{sgn}(\delta_m^{g_2})}{2} \quad (\text{S43.2})$$

$$\begin{aligned} \mathcal{W}_3^{\text{gapless}} = & \sum_{m=1}^{n_{b_1}} \text{sgn}(v_m^{b_1}) \frac{1 - \text{sgn}(\delta_m^{b_1})}{2} + \sum_{m=1}^{n_{c_1}} \text{sgn}(v_m^{c_1}) \frac{1 - \text{sgn}(\delta_m^{c_1})}{2} + \sum_{m=1}^{n_{e_2}} \text{sgn}(v_m^{e_2}) \frac{1 - \text{sgn}(\delta_m^{e_2})}{2} \\ & - \sum_{m=1}^{n_{f_2}} \text{sgn}(v_m^{f_2}) \frac{1 - \text{sgn}(\delta_m^{f_2})}{2} - \sum_{m=1}^{n_{f_4}} \text{sgn}(v_m^{f_4}) \frac{1 - \text{sgn}(\delta_m^{f_4})}{2} \end{aligned} \quad (\text{S43.3})$$

$$\begin{aligned} \mathcal{W}_4^{\text{gapless}} = & 2 \sum_{m=1}^{n_{c_1}} \text{sgn}(v_m^{c_1}) \frac{1 - \text{sgn}(\delta_m^{c_1})}{2} + 2 \sum_{m=1}^{n_{e_2}} \text{sgn}(v_m^{e_2}) \frac{1 - \text{sgn}(\delta_m^{e_2})}{2} - 2 \sum_{m=1}^{n_{f_2}} \text{sgn}(v_m^{f_2}) \frac{1 - \text{sgn}(\delta_m^{f_2})}{2} \\ & - 2 \sum_{m=1}^{n_{f_4}} \text{sgn}(v_m^{f_4}) \frac{1 - \text{sgn}(\delta_m^{f_4})}{2} + \sum_{m=1}^{n_{g_1}} \text{sgn}(v_m^{g_1}) \frac{1 - \text{sgn}(\delta_m^{g_1})}{2} + \sum_{m=1}^{n_{g_2}} \text{sgn}(v_m^{g_2}) \frac{1 - \text{sgn}(\delta_m^{g_2})}{2} \end{aligned} \quad (\text{S43.4})$$

$$\mathcal{W}_5^{\text{gapless}} = \sum_{m=1}^{n_{d_1}} \text{sgn}(v_m^{d_1}) \frac{1 - \text{sgn}(\delta_m^{d_1})}{2} - \sum_{m=1}^{n_{f_2}} \text{sgn}(v_m^{f_2}) \frac{1 - \text{sgn}(\delta_m^{f_2})}{2} - \sum_{m=1}^{n_{f_3}} \text{sgn}(v_m^{f_3}) \frac{1 - \text{sgn}(\delta_m^{f_3})}{2} + \sum_{m=1}^{n_{g_2}} \text{sgn}(v_m^{g_2}) \frac{1 - \text{sgn}(\delta_m^{g_2})}{2} \quad (\text{S43.5})$$

$$\begin{aligned} \mathcal{W}_6^{\text{gapless}} = & \sum_{m=1}^{n_{e_1}} \text{sgn}(v_m^{e_1}) \frac{1 - \text{sgn}(\delta_m^{e_1})}{2} - \sum_{m=1}^{n_{e_2}} \text{sgn}(v_m^{e_2}) \frac{1 - \text{sgn}(\delta_m^{e_2})}{2} - 2 \sum_{m=1}^{n_{f_3}} \text{sgn}(v_m^{f_3}) \frac{1 - \text{sgn}(\delta_m^{f_3})}{2} \\ & + 2 \sum_{m=1}^{n_{f_4}} \text{sgn}(v_m^{f_4}) \frac{1 - \text{sgn}(\delta_m^{f_4})}{2} - \sum_{m=1}^{n_{g_1}} \text{sgn}(v_m^{g_1}) \frac{1 - \text{sgn}(\delta_m^{g_1})}{2} + \sum_{m=1}^{n_{g_2}} \text{sgn}(v_m^{g_2}) \frac{1 - \text{sgn}(\delta_m^{g_2})}{2} \end{aligned} \quad (\text{S43.6})$$

$$\begin{aligned} \mathcal{W}_7^{\text{gapless}} = & \sum_{m=1}^{n_{f_1}} \text{sgn}(v_m^{f_1}) \frac{1 - \text{sgn}(\delta_m^{f_1})}{2} - \sum_{m=1}^{n_{f_2}} \text{sgn}(v_m^{f_2}) \frac{1 - \text{sgn}(\delta_m^{f_2})}{2} - \sum_{m=1}^{n_{f_3}} \text{sgn}(v_m^{f_3}) \frac{1 - \text{sgn}(\delta_m^{f_3})}{2} \\ & + \sum_{m=1}^{n_{f_4}} \text{sgn}(v_m^{f_4}) \frac{1 - \text{sgn}(\delta_m^{f_4})}{2} - \sum_{m=1}^{n_{g_1}} \text{sgn}(v_m^{g_1}) \frac{1 - \text{sgn}(\delta_m^{g_1})}{2} + \sum_{m=1}^{n_{g_2}} \text{sgn}(v_m^{g_2}) \frac{1 - \text{sgn}(\delta_m^{g_2})}{2} \end{aligned} \quad (\text{S43.7})$$

$$\begin{aligned} \mathcal{W}_1^{\text{gapped}} = & - \sum_{m=1}^{n_{c_1}} \text{sgn}(v_m^{c_1}) \frac{1 - \text{sgn}(\delta_m^{c_1})}{2} - \sum_{m=1}^{n_{e_2}} \text{sgn}(v_m^{e_2}) \frac{1 - \text{sgn}(\delta_m^{e_2})}{2} + 2 \sum_{m=1}^{n_{f_4}} \text{sgn}(v_m^{f_4}) \frac{1 - \text{sgn}(\delta_m^{f_4})}{2} \\ & - \sum_{m=1}^{n_{g_1}} \text{sgn}(v_m^{g_1}) \frac{1 - \text{sgn}(\delta_m^{g_1})}{2} \end{aligned} \quad (\text{S43.8})$$

$$\mathcal{X}_1 = \sum_{m=1}^{n_{g_1}} \frac{1 - \text{sgn}(\delta_m^{g_1})}{2} + \sum_{m=1}^{n_{h_1}} \frac{1 - \text{sgn}(\delta_m^{h_1})}{2} \quad \text{mod } 2 \quad (\text{S43.9})$$

$$\mathcal{X}_2 = \sum_{m=1}^{n_{h_1}} \frac{1 - \text{sgn}(\delta_m^{h_1})}{2} \quad \text{mod } 2 \quad (\text{S43.10})$$

## S44. SPACE GROUP NO. 44

| line segment                                        | character of irrep (generators only)                                                                                      |
|-----------------------------------------------------|---------------------------------------------------------------------------------------------------------------------------|
| $a \ (0, 0, t)$                                     | $a_1 \begin{Bmatrix} \{2_{001}  0 & 0 & 0\} \\ 0 \end{Bmatrix} \begin{Bmatrix} \{m_{100}  0 & 0 & 0\} \\ 0 \end{Bmatrix}$ |
| $b \ (0, t, 0)$                                     | $b_1 \begin{Bmatrix} \{m_{100}  0 & 0 & 0\} \\ -i \end{Bmatrix}$<br>$b_2 \begin{Bmatrix} i \end{Bmatrix}$                 |
| $c \ (t, 0, 0)$                                     | $c_1 \begin{Bmatrix} \{m_{010}  0 & 0 & 0\} \\ -i \end{Bmatrix}$<br>$c_2 \begin{Bmatrix} i \end{Bmatrix}$                 |
| $d \ (\frac{1}{2}, \frac{1}{2}, \frac{t}{2})$       | $d_1 \begin{Bmatrix} \{2_{001}  0 & 0 & 0\} \\ -i \end{Bmatrix}$<br>$d_2 \begin{Bmatrix} i \end{Bmatrix}$                 |
| $e \ (\frac{1-t}{2}, \frac{1}{2}, \frac{1}{2})$     | $e_1 \begin{Bmatrix} \{1  0 & 0 & 0\} \\ 1 \end{Bmatrix}$                                                                 |
| $f \ (\frac{1}{2}, \frac{1-t}{2}, \frac{1}{2})$     | $f_1 \begin{Bmatrix} \{1  0 & 0 & 0\} \\ 1 \end{Bmatrix}$                                                                 |
| $g \ (0, \frac{t}{2}, 1 - \frac{t}{2})$             | $g_1 \begin{Bmatrix} \{m_{100}  0 & 0 & 0\} \\ -i \end{Bmatrix}$<br>$g_2 \begin{Bmatrix} i \end{Bmatrix}$                 |
| $h \ (\frac{t}{2}, 0, 1 - \frac{t}{2})$             | $h_1 \begin{Bmatrix} \{m_{010}  0 & 0 & 0\} \\ -i \end{Bmatrix}$<br>$h_2 \begin{Bmatrix} i \end{Bmatrix}$                 |
| $i \ (\frac{1-t}{2}, \frac{t+1}{2}, 0)$             | $i_1 \begin{Bmatrix} \{1  0 & 0 & 0\} \\ 1 \end{Bmatrix}$                                                                 |
| $j \ (\frac{1-t}{2}, \frac{1-t}{2}, \frac{t+1}{2})$ | $j_1 \begin{Bmatrix} \{1  0 & 0 & 0\} \\ 1 \end{Bmatrix}$                                                                 |

$$\mathcal{W}_1^{\text{gapless}} = \sum_{m=1}^{n_{a_1}} \text{sgn}(v_m^{a_1}) \frac{1 - \text{sgn}(\delta_m^{a_1})}{2} - \sum_{m=1}^{n_{c_2}} \text{sgn}(v_m^{c_2}) \frac{1 - \text{sgn}(\delta_m^{c_2})}{2} - \sum_{m=1}^{n_{h_1}} \text{sgn}(v_m^{h_1}) \frac{1 - \text{sgn}(\delta_m^{h_1})}{2} + \sum_{m=1}^{n_{h_2}} \text{sgn}(v_m^{h_2}) \frac{1 - \text{sgn}(\delta_m^{h_2})}{2} \quad (\text{S44.1})$$

$$\begin{aligned} \mathcal{W}_2^{\text{gapless}} = & \sum_{m=1}^{n_{b_1}} \text{sgn}(v_m^{b_1}) \frac{1 - \text{sgn}(\delta_m^{b_1})}{2} - \sum_{m=1}^{n_{c_2}} \text{sgn}(v_m^{c_2}) \frac{1 - \text{sgn}(\delta_m^{c_2})}{2} - \sum_{m=1}^{n_{g_1}} \text{sgn}(v_m^{g_1}) \frac{1 - \text{sgn}(\delta_m^{g_1})}{2} \\ & + \sum_{m=1}^{n_{g_2}} \text{sgn}(v_m^{g_2}) \frac{1 - \text{sgn}(\delta_m^{g_2})}{2} - \sum_{m=1}^{n_{h_1}} \text{sgn}(v_m^{h_1}) \frac{1 - \text{sgn}(\delta_m^{h_1})}{2} + \sum_{m=1}^{n_{h_2}} \text{sgn}(v_m^{h_2}) \frac{1 - \text{sgn}(\delta_m^{h_2})}{2} \end{aligned} \quad (\text{S44.2})$$

$$\begin{aligned} \mathcal{W}_3^{\text{gapless}} = & \sum_{m=1}^{n_{b_2}} \text{sgn}(v_m^{b_2}) \frac{1 - \text{sgn}(\delta_m^{b_2})}{2} - \sum_{m=1}^{n_{c_2}} \text{sgn}(v_m^{c_2}) \frac{1 - \text{sgn}(\delta_m^{c_2})}{2} + \sum_{m=1}^{n_{g_1}} \text{sgn}(v_m^{g_1}) \frac{1 - \text{sgn}(\delta_m^{g_1})}{2} \\ & - \sum_{m=1}^{n_{g_2}} \text{sgn}(v_m^{g_2}) \frac{1 - \text{sgn}(\delta_m^{g_2})}{2} - \sum_{m=1}^{n_{h_1}} \text{sgn}(v_m^{h_1}) \frac{1 - \text{sgn}(\delta_m^{h_1})}{2} + \sum_{m=1}^{n_{h_2}} \text{sgn}(v_m^{h_2}) \frac{1 - \text{sgn}(\delta_m^{h_2})}{2} \end{aligned} \quad (\text{S44.3})$$

$$\begin{aligned} \mathcal{W}_4^{\text{gapless}} = & \sum_{m=1}^{n_{c_1}} \text{sgn}(v_m^{c_1}) \frac{1 - \text{sgn}(\delta_m^{c_1})}{2} - \sum_{m=1}^{n_{c_2}} \text{sgn}(v_m^{c_2}) \frac{1 - \text{sgn}(\delta_m^{c_2})}{2} - 2 \sum_{m=1}^{n_{h_1}} \text{sgn}(v_m^{h_1}) \frac{1 - \text{sgn}(\delta_m^{h_1})}{2} \\ & + 2 \sum_{m=1}^{n_{h_2}} \text{sgn}(v_m^{h_2}) \frac{1 - \text{sgn}(\delta_m^{h_2})}{2} \end{aligned} \quad (\text{S44.4})$$

$$\mathcal{W}_5^{\text{gapless}} = \sum_{m=1}^{n_{d_1}} \text{sgn}(v_m^{d_1}) \frac{1 - \text{sgn}(\delta_m^{d_1})}{2} + \sum_{m=1}^{n_{d_2}} \text{sgn}(v_m^{d_2}) \frac{1 - \text{sgn}(\delta_m^{d_2})}{2} - \sum_{m=1}^{n_{i_1}} \text{sgn}(v_m^{i_1}) \frac{1 - \text{sgn}(\delta_m^{i_1})}{2} + \sum_{m=1}^{n_{j_1}} \text{sgn}(v_m^{j_1}) \frac{1 - \text{sgn}(\delta_m^{j_1})}{2} \quad (\text{S44.5})$$

$$\mathcal{W}_6^{\text{gapless}} = \sum_{m=1}^{n_{e_1}} \text{sgn}(v_m^{e_1}) \frac{1 - \text{sgn}(\delta_m^{e_1})}{2} - \sum_{m=1}^{n_{g_1}} \text{sgn}(v_m^{g_1}) \frac{1 - \text{sgn}(\delta_m^{g_1})}{2} - \sum_{m=1}^{n_{g_2}} \text{sgn}(v_m^{g_2}) \frac{1 - \text{sgn}(\delta_m^{g_2})}{2} - \sum_{m=1}^{n_{j_1}} \text{sgn}(v_m^{j_1}) \frac{1 - \text{sgn}(\delta_m^{j_1})}{2} \quad (\text{S44.6})$$

$$\mathcal{W}_7^{\text{gapless}} = \sum_{m=1}^{n_{f_1}} \text{sgn}(v_m^{f_1}) \frac{1 - \text{sgn}(\delta_m^{f_1})}{2} - \sum_{m=1}^{n_{h_1}} \text{sgn}(v_m^{h_1}) \frac{1 - \text{sgn}(\delta_m^{h_1})}{2} - \sum_{m=1}^{n_{h_2}} \text{sgn}(v_m^{h_2}) \frac{1 - \text{sgn}(\delta_m^{h_2})}{2} - \sum_{m=1}^{n_{j_1}} \text{sgn}(v_m^{j_1}) \frac{1 - \text{sgn}(\delta_m^{j_1})}{2} \quad (\text{S44.7})$$

$$\mathcal{W}_1^{\text{gapped}} = - \sum_{m=1}^{n_{g_1}} \text{sgn}(v_m^{g_1}) \frac{1 - \text{sgn}(\delta_m^{g_1})}{2} + \sum_{m=1}^{n_{g_2}} \text{sgn}(v_m^{g_2}) \frac{1 - \text{sgn}(\delta_m^{g_2})}{2} \quad (\text{S44.8})$$

$$\mathcal{W}_2^{\text{gapped}} = - \sum_{m=1}^{n_{h_1}} \text{sgn}(v_m^{h_1}) \frac{1 - \text{sgn}(\delta_m^{h_1})}{2} + \sum_{m=1}^{n_{h_2}} \text{sgn}(v_m^{h_2}) \frac{1 - \text{sgn}(\delta_m^{h_2})}{2} \quad (\text{S44.9})$$

$$\mathcal{X}_1 = \sum_{m=1}^{n_{i_1}} \frac{1 - \text{sgn}(\delta_m^{i_1})}{2} \mod 2 \quad (\text{S44.10})$$

#### S45. SPACE GROUP NO. 45

| line segment                                    | character of irrep (generators only)                                                                                                      |
|-------------------------------------------------|-------------------------------------------------------------------------------------------------------------------------------------------|
| $a \ (0, 0, t)$                                 | $\begin{matrix} \{2_{001}   0 & 0 & 0\} \\ a_1 & 0 \end{matrix} \quad \begin{matrix} \{m_{100}   0 & 0 & \frac{1}{2}\} \\ 0 \end{matrix}$ |
| $b \ (0, t, 0)$                                 | $\begin{matrix} \{m_{100}   0 & 0 & \frac{1}{2}\} \\ b_1 & -i \\ b_2 & i \end{matrix}$                                                    |
| $c \ (t, 0, 0)$                                 | $\begin{matrix} \{m_{010}   0 & 0 & \frac{1}{2}\} \\ c_1 & -i \\ c_2 & i \end{matrix}$                                                    |
| $d \ (\frac{1}{2}, \frac{1}{2}, \frac{t}{2})$   | $\begin{matrix} \{2_{001}   0 & 0 & 0\} \\ d_1 & -i \\ d_2 & i \end{matrix}$                                                              |
| $e \ (\frac{1-t}{2}, \frac{1}{2}, \frac{1}{2})$ | $\begin{matrix} \{1   0 & 0 & 0\} \\ e_1 & 1 \end{matrix}$                                                                                |
| $f \ (\frac{1}{2}, \frac{1-t}{2}, \frac{1}{2})$ | $\begin{matrix} \{1   0 & 0 & 0\} \\ f_1 & 1 \end{matrix}$                                                                                |
| $g \ (0, \frac{t}{2}, 1 - \frac{t}{2})$         | $\begin{matrix} \{m_{100}   0 & 0 & \frac{1}{2}\} \\ g_1 & -ie^{-\frac{1}{2}i\pi(2-t)} \\ g_2 & ie^{-\frac{1}{2}i\pi(2-t)} \end{matrix}$  |
| $h \ (\frac{t}{2}, 0, 1 - \frac{t}{2})$         | $\begin{matrix} \{m_{010}   0 & 0 & \frac{1}{2}\} \\ h_1 & -ie^{-\frac{1}{2}i\pi(2-t)} \\ h_2 & ie^{-\frac{1}{2}i\pi(2-t)} \end{matrix}$  |

|                                                         |                                                           |
|---------------------------------------------------------|-----------------------------------------------------------|
| $i \quad (\frac{1-t}{2}, \frac{t+1}{2}, 0)$             | $\begin{matrix} \{1  0 & 0 & 0\} \\ i_1 & 1 \end{matrix}$ |
| $j \quad (\frac{1-t}{2}, \frac{1-t}{2}, \frac{t+1}{2})$ | $\begin{matrix} \{1  0 & 0 & 0\} \\ j_1 & 1 \end{matrix}$ |

$$\mathcal{W}_1^{\text{gapless}} = \sum_{m=1}^{n_{a_1}} \text{sgn}(v_m^{a_1}) \frac{1 - \text{sgn}(\delta_m^{a_1})}{2} - \sum_{m=1}^{n_{c_2}} \text{sgn}(v_m^{c_2}) \frac{1 - \text{sgn}(\delta_m^{c_2})}{2} \quad (\text{S45.1})$$

$$\mathcal{W}_2^{\text{gapless}} = \sum_{m=1}^{n_{b_1}} \text{sgn}(v_m^{b_1}) \frac{1 - \text{sgn}(\delta_m^{b_1})}{2} - \sum_{m=1}^{n_{c_2}} \text{sgn}(v_m^{c_2}) \frac{1 - \text{sgn}(\delta_m^{c_2})}{2} \quad (\text{S45.2})$$

$$\mathcal{W}_3^{\text{gapless}} = \sum_{m=1}^{n_{b_2}} \text{sgn}(v_m^{b_2}) \frac{1 - \text{sgn}(\delta_m^{b_2})}{2} - \sum_{m=1}^{n_{c_2}} \text{sgn}(v_m^{c_2}) \frac{1 - \text{sgn}(\delta_m^{c_2})}{2} \quad (\text{S45.3})$$

$$\mathcal{W}_4^{\text{gapless}} = \sum_{m=1}^{n_{c_1}} \text{sgn}(v_m^{c_1}) \frac{1 - \text{sgn}(\delta_m^{c_1})}{2} - \sum_{m=1}^{n_{c_2}} \text{sgn}(v_m^{c_2}) \frac{1 - \text{sgn}(\delta_m^{c_2})}{2} \quad (\text{S45.4})$$

$$\mathcal{W}_5^{\text{gapless}} = \sum_{m=1}^{n_{d_1}} \text{sgn}(v_m^{d_1}) \frac{1 - \text{sgn}(\delta_m^{d_1})}{2} + \sum_{m=1}^{n_{d_2}} \text{sgn}(v_m^{d_2}) \frac{1 - \text{sgn}(\delta_m^{d_2})}{2} - \sum_{m=1}^{n_{i_1}} \text{sgn}(v_m^{i_1}) \frac{1 - \text{sgn}(\delta_m^{i_1})}{2} + \sum_{m=1}^{n_{j_1}} \text{sgn}(v_m^{j_1}) \frac{1 - \text{sgn}(\delta_m^{j_1})}{2} \quad (\text{S45.5})$$

$$\mathcal{W}_6^{\text{gapless}} = 2 \sum_{m=1}^{n_{e_1}} \text{sgn}(v_m^{e_1}) \frac{1 - \text{sgn}(\delta_m^{e_1})}{2} - \sum_{m=1}^{n_{g_1}} \text{sgn}(v_m^{g_1}) \frac{1 - \text{sgn}(\delta_m^{g_1})}{2} - \sum_{m=1}^{n_{g_2}} \text{sgn}(v_m^{g_2}) \frac{1 - \text{sgn}(\delta_m^{g_2})}{2} - \sum_{m=1}^{n_{j_1}} \text{sgn}(v_m^{j_1}) \frac{1 - \text{sgn}(\delta_m^{j_1})}{2} \quad (\text{S45.6})$$

$$\begin{aligned} \mathcal{W}_7^{\text{gapless}} = & 2 \sum_{m=1}^{n_{f_1}} \text{sgn}(v_m^{f_1}) \frac{1 - \text{sgn}(\delta_m^{f_1})}{2} - \sum_{m=1}^{n_{h_1}} \text{sgn}(v_m^{h_1}) \frac{1 - \text{sgn}(\delta_m^{h_1})}{2} - \sum_{m=1}^{n_{h_2}} \text{sgn}(v_m^{h_2}) \frac{1 - \text{sgn}(\delta_m^{h_2})}{2} \\ & - \sum_{m=1}^{n_{j_1}} \text{sgn}(v_m^{j_1}) \frac{1 - \text{sgn}(\delta_m^{j_1})}{2} \end{aligned} \quad (\text{S45.7})$$

$$\mathcal{X}_1 = \sum_{m=1}^{n_{g_1}} \frac{1 - \text{sgn}(\delta_m^{g_1})}{2} + \sum_{m=1}^{n_{h_1}} \frac{1 - \text{sgn}(\delta_m^{h_1})}{2} + \sum_{m=1}^{n_{i_1}} \frac{1 - \text{sgn}(\delta_m^{i_1})}{2} \quad \text{mod } 2 \quad (\text{S45.8})$$

$$\mathcal{X}_2 = \sum_{m=1}^{n_{g_2}} \frac{1 - \text{sgn}(\delta_m^{g_2})}{2} + \sum_{m=1}^{n_{h_1}} \frac{1 - \text{sgn}(\delta_m^{h_1})}{2} \quad \text{mod } 2 \quad (\text{S45.9})$$

$$\mathcal{X}_3 = 2 \sum_{m=1}^{n_{d_2}} \text{sgn}(v_m^{d_2}) \frac{1 - \text{sgn}(\delta_m^{d_2})}{2} + 2 \sum_{m=1}^{n_{g_1}} \text{sgn}(v_m^{g_1}) \frac{1 - \text{sgn}(\delta_m^{g_1})}{2} - \sum_{m=1}^{n_{i_1}} \text{sgn}(v_m^{i_1}) \frac{1 - \text{sgn}(\delta_m^{i_1})}{2} \quad \text{mod } 4 \quad (\text{S45.10})$$

## S46. SPACE GROUP NO. 46

| line segment                                        | character of irrep (generators only)                                                                                                                                |
|-----------------------------------------------------|---------------------------------------------------------------------------------------------------------------------------------------------------------------------|
| $a \ (0, 0, t)$                                     | $a_1 \ \begin{Bmatrix} \{2_{001}  0 & 0 & 0\} \\ 0 \end{Bmatrix} \ \begin{Bmatrix} \{m_{100}  \frac{1}{2} & 0 & 0\} \\ 0 \end{Bmatrix}$                             |
| $b \ (0, t, 0)$                                     | $b_1 \ \begin{Bmatrix} \{m_{100}  \frac{1}{2} & 0 & 0\} \\ -i \end{Bmatrix}$<br>$b_2 \ \begin{Bmatrix} i \end{Bmatrix}$                                             |
| $c \ (t, 0, 0)$                                     | $c_1 \ \begin{Bmatrix} \{m_{010}  \frac{1}{2} & 0 & 0\} \\ -ie^{-i\pi t} \end{Bmatrix}$<br>$c_2 \ \begin{Bmatrix} ie^{-i\pi t} \end{Bmatrix}$                       |
| $d \ (\frac{1}{2}, \frac{1}{2}, \frac{t}{2})$       | $d_1 \ \begin{Bmatrix} \{2_{001}  0 & 0 & 0\} \\ -i \end{Bmatrix}$<br>$d_2 \ \begin{Bmatrix} i \end{Bmatrix}$                                                       |
| $e \ (\frac{1-t}{2}, \frac{1}{2}, \frac{1}{2})$     | $e_1 \ \begin{Bmatrix} \{1  0 & 0 & 0\} \\ 1 \end{Bmatrix}$                                                                                                         |
| $f \ (\frac{1}{2}, \frac{1-t}{2}, \frac{1}{2})$     | $f_1 \ \begin{Bmatrix} \{1  0 & 0 & 0\} \\ 1 \end{Bmatrix}$                                                                                                         |
| $g \ (0, \frac{t}{2}, 1 - \frac{t}{2})$             | $g_1 \ \begin{Bmatrix} \{m_{100}  \frac{1}{2} & 0 & 0\} \\ -i \end{Bmatrix}$<br>$g_2 \ \begin{Bmatrix} i \end{Bmatrix}$                                             |
| $h \ (\frac{t}{2}, 0, 1 - \frac{t}{2})$             | $h_1 \ \begin{Bmatrix} \{m_{010}  \frac{1}{2} & 0 & 0\} \\ -ie^{-\frac{1}{2}i\pi t} \end{Bmatrix}$<br>$h_2 \ \begin{Bmatrix} ie^{-\frac{1}{2}i\pi t} \end{Bmatrix}$ |
| $i \ (\frac{1-t}{2}, \frac{t+1}{2}, 0)$             | $i_1 \ \begin{Bmatrix} \{1  0 & 0 & 0\} \\ 1 \end{Bmatrix}$                                                                                                         |
| $j \ (\frac{1-t}{2}, \frac{1-t}{2}, \frac{t+1}{2})$ | $j_1 \ \begin{Bmatrix} \{1  0 & 0 & 0\} \\ 1 \end{Bmatrix}$                                                                                                         |

$$\mathcal{W}_1^{\text{gapless}} = \sum_{m=1}^{n_{a_1}} \text{sgn}(v_m^{a_1}) \frac{1 - \text{sgn}(\delta_m^{a_1})}{2} - \sum_{m=1}^{n_{c_2}} \text{sgn}(v_m^{c_2}) \frac{1 - \text{sgn}(\delta_m^{c_2})}{2} \quad (\text{S46.1})$$

$$\mathcal{W}_2^{\text{gapless}} = \sum_{m=1}^{n_{b_1}} \text{sgn}(v_m^{b_1}) \frac{1 - \text{sgn}(\delta_m^{b_1})}{2} - \sum_{m=1}^{n_{c_2}} \text{sgn}(v_m^{c_2}) \frac{1 - \text{sgn}(\delta_m^{c_2})}{2} - \sum_{m=1}^{n_{g_1}} \text{sgn}(v_m^{g_1}) \frac{1 - \text{sgn}(\delta_m^{g_1})}{2} + \sum_{m=1}^{n_{g_2}} \text{sgn}(v_m^{g_2}) \frac{1 - \text{sgn}(\delta_m^{g_2})}{2} \quad (\text{S46.2})$$

$$\mathcal{W}_3^{\text{gapless}} = \sum_{m=1}^{n_{b_2}} \text{sgn}(v_m^{b_2}) \frac{1 - \text{sgn}(\delta_m^{b_2})}{2} - \sum_{m=1}^{n_{c_2}} \text{sgn}(v_m^{c_2}) \frac{1 - \text{sgn}(\delta_m^{c_2})}{2} + \sum_{m=1}^{n_{g_1}} \text{sgn}(v_m^{g_1}) \frac{1 - \text{sgn}(\delta_m^{g_1})}{2} - \sum_{m=1}^{n_{g_2}} \text{sgn}(v_m^{g_2}) \frac{1 - \text{sgn}(\delta_m^{g_2})}{2} \quad (\text{S46.3})$$

$$\mathcal{W}_4^{\text{gapless}} = \sum_{m=1}^{n_{c_1}} \text{sgn}(v_m^{c_1}) \frac{1 - \text{sgn}(\delta_m^{c_1})}{2} - \sum_{m=1}^{n_{c_2}} \text{sgn}(v_m^{c_2}) \frac{1 - \text{sgn}(\delta_m^{c_2})}{2} \quad (\text{S46.4})$$

$$\mathcal{W}_5^{\text{gapless}} = \sum_{m=1}^{n_{d_1}} \text{sgn}(v_m^{d_1}) \frac{1 - \text{sgn}(\delta_m^{d_1})}{2} + \sum_{m=1}^{n_{d_2}} \text{sgn}(v_m^{d_2}) \frac{1 - \text{sgn}(\delta_m^{d_2})}{2} - \sum_{m=1}^{n_{i_1}} \text{sgn}(v_m^{i_1}) \frac{1 - \text{sgn}(\delta_m^{i_1})}{2} + \sum_{m=1}^{n_{j_1}} \text{sgn}(v_m^{j_1}) \frac{1 - \text{sgn}(\delta_m^{j_1})}{2} \quad (\text{S46.5})$$

$$\mathcal{W}_6^{\text{gapless}} = \sum_{m=1}^{n_{e_1}} \text{sgn}(v_m^{e_1}) \frac{1 - \text{sgn}(\delta_m^{e_1})}{2} - \sum_{m=1}^{n_{g_1}} \text{sgn}(v_m^{g_1}) \frac{1 - \text{sgn}(\delta_m^{g_1})}{2} - \sum_{m=1}^{n_{g_2}} \text{sgn}(v_m^{g_2}) \frac{1 - \text{sgn}(\delta_m^{g_2})}{2} - \sum_{m=1}^{n_{j_1}} \text{sgn}(v_m^{j_1}) \frac{1 - \text{sgn}(\delta_m^{j_1})}{2} \quad (\text{S46.6})$$

$$\begin{aligned} \mathcal{W}_7^{\text{gapless}} = & 2 \sum_{m=1}^{n_{f_1}} \text{sgn}(v_m^{f_1}) \frac{1 - \text{sgn}(\delta_m^{f_1})}{2} - \sum_{m=1}^{n_{h_1}} \text{sgn}(v_m^{h_1}) \frac{1 - \text{sgn}(\delta_m^{h_1})}{2} - \sum_{m=1}^{n_{h_2}} \text{sgn}(v_m^{h_2}) \frac{1 - \text{sgn}(\delta_m^{h_2})}{2} \\ & - \sum_{m=1}^{n_{j_1}} \text{sgn}(v_m^{j_1}) \frac{1 - \text{sgn}(\delta_m^{j_1})}{2} \end{aligned} \quad (\text{S46.7})$$

$$\mathcal{W}_1^{\text{gapped}} = - \sum_{m=1}^{n_{g_1}} \text{sgn}(v_m^{g_1}) \frac{1 - \text{sgn}(\delta_m^{g_1})}{2} + \sum_{m=1}^{n_{g_2}} \text{sgn}(v_m^{g_2}) \frac{1 - \text{sgn}(\delta_m^{g_2})}{2} \quad (\text{S46.8})$$

$$\begin{aligned} \mathcal{W}_2^{\text{gapped}} = & 2 \sum_{m=1}^{n_{d_2}} \text{sgn}(v_m^{d_2}) \frac{1 - \text{sgn}(\delta_m^{d_2})}{2} - 2 \sum_{m=1}^{n_{f_1}} \text{sgn}(v_m^{f_1}) \frac{1 - \text{sgn}(\delta_m^{f_1})}{2} + \sum_{m=1}^{n_{h_1}} \text{sgn}(v_m^{h_1}) \frac{1 - \text{sgn}(\delta_m^{h_1})}{2} \\ & + \sum_{m=1}^{n_{h_2}} \text{sgn}(v_m^{h_2}) \frac{1 - \text{sgn}(\delta_m^{h_2})}{2} - \sum_{m=1}^{n_{i_1}} \text{sgn}(v_m^{i_1}) \frac{1 - \text{sgn}(\delta_m^{i_1})}{2} + 2 \sum_{m=1}^{n_{j_1}} \text{sgn}(v_m^{j_1}) \frac{1 - \text{sgn}(\delta_m^{j_1})}{2} \end{aligned} \quad (\text{S46.9})$$

$$\mathcal{X}_1 = \sum_{m=1}^{n_{i_1}} \frac{1 - \text{sgn}(\delta_m^{i_1})}{2} \quad \text{mod } 2 \quad (\text{S46.10})$$

#### S47. SPACE GROUP NO. 47

| line segment                                        | character of irrep (generators only)                                                                                   |
|-----------------------------------------------------|------------------------------------------------------------------------------------------------------------------------|
| $a \quad (\frac{t}{2}, 0, 0)$                       | $a_1 \quad \begin{array}{c} \{2_{100}   0 \ 0 \ 0\} \ \{m_{010}   0 \ 0 \ 0\} \\ 0 \qquad \qquad \qquad 0 \end{array}$ |
| $b \quad (0, \frac{t}{2}, 0)$                       | $b_1 \quad \begin{array}{c} \{2_{010}   0 \ 0 \ 0\} \ \{m_{100}   0 \ 0 \ 0\} \\ 0 \qquad \qquad \qquad 0 \end{array}$ |
| $c \quad (\frac{1}{2}, \frac{t}{2}, 0)$             | $c_1 \quad \begin{array}{c} \{2_{010}   0 \ 0 \ 0\} \ \{m_{100}   0 \ 0 \ 0\} \\ 0 \qquad \qquad \qquad 0 \end{array}$ |
| $d \quad (\frac{1-t}{2}, \frac{1}{2}, 0)$           | $d_1 \quad \begin{array}{c} \{2_{100}   0 \ 0 \ 0\} \ \{m_{010}   0 \ 0 \ 0\} \\ 0 \qquad \qquad \qquad 0 \end{array}$ |
| $e \quad (\frac{t}{2}, 0, \frac{1}{2})$             | $e_1 \quad \begin{array}{c} \{2_{100}   0 \ 0 \ 0\} \ \{m_{010}   0 \ 0 \ 0\} \\ 0 \qquad \qquad \qquad 0 \end{array}$ |
| $f \quad (0, \frac{t}{2}, \frac{1}{2})$             | $f_1 \quad \begin{array}{c} \{2_{010}   0 \ 0 \ 0\} \ \{m_{100}   0 \ 0 \ 0\} \\ 0 \qquad \qquad \qquad 0 \end{array}$ |
| $g \quad (\frac{1}{2}, \frac{t}{2}, \frac{1}{2})$   | $g_1 \quad \begin{array}{c} \{2_{010}   0 \ 0 \ 0\} \ \{m_{100}   0 \ 0 \ 0\} \\ 0 \qquad \qquad \qquad 0 \end{array}$ |
| $h \quad (\frac{1-t}{2}, \frac{1}{2}, \frac{1}{2})$ | $h_1 \quad \begin{array}{c} \{2_{100}   0 \ 0 \ 0\} \ \{m_{010}   0 \ 0 \ 0\} \\ 0 \qquad \qquad \qquad 0 \end{array}$ |
| $i \quad (0, 0, \frac{t}{2})$                       | $i_1 \quad \begin{array}{c} \{2_{001}   0 \ 0 \ 0\} \ \{m_{100}   0 \ 0 \ 0\} \\ 0 \qquad \qquad \qquad 0 \end{array}$ |
| $j \quad (\frac{1}{2}, 0, \frac{t}{2})$             | $j_1 \quad \begin{array}{c} \{2_{001}   0 \ 0 \ 0\} \ \{m_{100}   0 \ 0 \ 0\} \\ 0 \qquad \qquad \qquad 0 \end{array}$ |
| $k \quad (\frac{1}{2}, \frac{1}{2}, \frac{t}{2})$   | $k_1 \quad \begin{array}{c} \{2_{001}   0 \ 0 \ 0\} \ \{m_{100}   0 \ 0 \ 0\} \\ 0 \qquad \qquad \qquad 0 \end{array}$ |



|                                         |                                                                                                                                                                                                             |
|-----------------------------------------|-------------------------------------------------------------------------------------------------------------------------------------------------------------------------------------------------------------|
| $l \quad (0, \frac{1}{2}, \frac{t}{2})$ | $l_1 \quad \left\{ 2_{001} \left  \begin{smallmatrix} 0 & 0 & 0 \\ 0 \end{smallmatrix} \right. \right\} \quad \left\{ m_{100} \left  \begin{smallmatrix} 0 & 0 & 0 \\ 0 \end{smallmatrix} \right. \right\}$ |
|-----------------------------------------|-------------------------------------------------------------------------------------------------------------------------------------------------------------------------------------------------------------|

$$\begin{aligned} \mathcal{W}_1^{\text{gapless}} = & \sum_{m=1}^{n_{a_1}} \text{sgn}(v_m^{a_1}) \frac{1 - \text{sgn}(\delta_m^{a_1})}{2} - \sum_{m=1}^{n_{f_1}} \text{sgn}(v_m^{f_1}) \frac{1 - \text{sgn}(\delta_m^{f_1})}{2} + \sum_{m=1}^{n_{g_1}} \text{sgn}(v_m^{g_1}) \frac{1 - \text{sgn}(\delta_m^{g_1})}{2} \\ & + \sum_{m=1}^{n_{h_1}} \text{sgn}(v_m^{h_1}) \frac{1 - \text{sgn}(\delta_m^{h_1})}{2} - \sum_{m=1}^{n_{i_1}} \text{sgn}(v_m^{i_1}) \frac{1 - \text{sgn}(\delta_m^{i_1})}{2} + \sum_{m=1}^{n_{j_1}} \text{sgn}(v_m^{j_1}) \frac{1 - \text{sgn}(\delta_m^{j_1})}{2} \end{aligned} \quad (\text{S47.1})$$

$$\mathcal{W}_2^{\text{gapless}} = \sum_{m=1}^{n_{b_1}} \text{sgn}(v_m^{b_1}) \frac{1 - \text{sgn}(\delta_m^{b_1})}{2} - \sum_{m=1}^{n_{f_1}} \text{sgn}(v_m^{f_1}) \frac{1 - \text{sgn}(\delta_m^{f_1})}{2} - \sum_{m=1}^{n_{i_1}} \text{sgn}(v_m^{i_1}) \frac{1 - \text{sgn}(\delta_m^{i_1})}{2} + \sum_{m=1}^{n_{l_1}} \text{sgn}(v_m^{l_1}) \frac{1 - \text{sgn}(\delta_m^{l_1})}{2} \quad (\text{S47.2})$$

$$\mathcal{W}_3^{\text{gapless}} = \sum_{m=1}^{n_{c_1}} \text{sgn}(v_m^{c_1}) \frac{1 - \text{sgn}(\delta_m^{c_1})}{2} - \sum_{m=1}^{n_{g_1}} \text{sgn}(v_m^{g_1}) \frac{1 - \text{sgn}(\delta_m^{g_1})}{2} - \sum_{m=1}^{n_{j_1}} \text{sgn}(v_m^{j_1}) \frac{1 - \text{sgn}(\delta_m^{j_1})}{2} + \sum_{m=1}^{n_{k_1}} \text{sgn}(v_m^{k_1}) \frac{1 - \text{sgn}(\delta_m^{k_1})}{2} \quad (\text{S47.3})$$

$$\mathcal{W}_4^{\text{gapless}} = \sum_{m=1}^{n_{d_1}} \text{sgn}(v_m^{d_1}) \frac{1 - \text{sgn}(\delta_m^{d_1})}{2} - \sum_{m=1}^{n_{h_1}} \text{sgn}(v_m^{h_1}) \frac{1 - \text{sgn}(\delta_m^{h_1})}{2} - \sum_{m=1}^{n_{k_1}} \text{sgn}(v_m^{k_1}) \frac{1 - \text{sgn}(\delta_m^{k_1})}{2} + \sum_{m=1}^{n_{l_1}} \text{sgn}(v_m^{l_1}) \frac{1 - \text{sgn}(\delta_m^{l_1})}{2} \quad (\text{S47.4})$$

$$\mathcal{W}_5^{\text{gapless}} = \sum_{m=1}^{n_{e_1}} \text{sgn}(v_m^{e_1}) \frac{1 - \text{sgn}(\delta_m^{e_1})}{2} - \sum_{m=1}^{n_{f_1}} \text{sgn}(v_m^{f_1}) \frac{1 - \text{sgn}(\delta_m^{f_1})}{2} + \sum_{m=1}^{n_{g_1}} \text{sgn}(v_m^{g_1}) \frac{1 - \text{sgn}(\delta_m^{g_1})}{2} + \sum_{m=1}^{n_{h_1}} \text{sgn}(v_m^{h_1}) \frac{1 - \text{sgn}(\delta_m^{h_1})}{2} \quad (\text{S47.5})$$

#### S48. SPACE GROUP NO. 48

| line segment                              | character of irrep (generators only) |                                                                                                                                                                                                                                           |
|-------------------------------------------|--------------------------------------|-------------------------------------------------------------------------------------------------------------------------------------------------------------------------------------------------------------------------------------------|
| $a \quad (\frac{t}{2}, 0, 0)$             | $a_1$                                | $\left\{ 2_{100} \left  \begin{smallmatrix} 0 & \frac{1}{2} & \frac{1}{2} \\ 0 \end{smallmatrix} \right. \right\} \quad \left\{ m_{010} \left  \begin{smallmatrix} \frac{1}{2} & 0 & \frac{1}{2} \\ 0 \end{smallmatrix} \right. \right\}$ |
| $b \quad (0, \frac{t}{2}, 0)$             | $b_1$                                | $\left\{ 2_{010} \left  \begin{smallmatrix} \frac{1}{2} & 0 & \frac{1}{2} \\ 0 \end{smallmatrix} \right. \right\} \quad \left\{ m_{100} \left  \begin{smallmatrix} 0 & \frac{1}{2} & \frac{1}{2} \\ 0 \end{smallmatrix} \right. \right\}$ |
| $c \quad (\frac{1}{2}, \frac{t}{2}, 0)$   | $c_1$                                | $\left\{ 2_{010} \left  \begin{smallmatrix} \frac{1}{2} & 0 & \frac{1}{2} \\ 0 \end{smallmatrix} \right. \right\} \quad \left\{ m_{100} \left  \begin{smallmatrix} 0 & \frac{1}{2} & \frac{1}{2} \\ 0 \end{smallmatrix} \right. \right\}$ |
|                                           | $c_2$                                | $i \quad -ie^{-\frac{1}{2}i\pi t}$                                                                                                                                                                                                        |
|                                           | $c_3$                                | $i \quad ie^{-\frac{1}{2}i\pi t}$                                                                                                                                                                                                         |
|                                           | $c_4$                                | $-i \quad -ie^{-\frac{1}{2}i\pi t}$                                                                                                                                                                                                       |
| $d \quad (\frac{1-t}{2}, \frac{1}{2}, 0)$ | $d_1$                                | $\left\{ 2_{100} \left  \begin{smallmatrix} 0 & \frac{1}{2} & \frac{1}{2} \\ 0 \end{smallmatrix} \right. \right\} \quad \left\{ m_{010} \left  \begin{smallmatrix} \frac{1}{2} & 0 & \frac{1}{2} \\ 0 \end{smallmatrix} \right. \right\}$ |
|                                           | $d_2$                                | $i \quad -ie^{-\frac{1}{2}i\pi(1-t)}$                                                                                                                                                                                                     |
|                                           | $d_3$                                | $i \quad ie^{-\frac{1}{2}i\pi(1-t)}$                                                                                                                                                                                                      |
|                                           | $d_4$                                | $-i \quad -ie^{-\frac{1}{2}i\pi(1-t)}$                                                                                                                                                                                                    |

|                                                     |                                                      |                                                      |                               |
|-----------------------------------------------------|------------------------------------------------------|------------------------------------------------------|-------------------------------|
| $e \quad (\frac{t}{2}, 0, \frac{1}{2})$             | $\{2_{100} 0 \quad \frac{1}{2} \quad \frac{1}{2} \}$ | $\{m_{010} \frac{1}{2} \quad 0 \quad \frac{1}{2} \}$ |                               |
|                                                     | $e_1$                                                | $i$                                                  | $-ie^{-\frac{1}{2}i\pi(t+1)}$ |
|                                                     | $e_2$                                                | $i$                                                  | $ie^{-\frac{1}{2}i\pi(t+1)}$  |
|                                                     | $e_3$                                                | $-i$                                                 | $-ie^{-\frac{1}{2}i\pi(t+1)}$ |
|                                                     | $e_4$                                                | $-i$                                                 | $ie^{-\frac{1}{2}i\pi(t+1)}$  |
| $f \quad (0, \frac{t}{2}, \frac{1}{2})$             | $\{2_{010} \frac{1}{2} \quad 0 \quad \frac{1}{2} \}$ | $\{m_{100} 0 \quad \frac{1}{2} \quad \frac{1}{2} \}$ |                               |
|                                                     | $f_1$                                                | $i$                                                  | $-ie^{-\frac{1}{2}i\pi(t+1)}$ |
|                                                     | $f_2$                                                | $i$                                                  | $ie^{-\frac{1}{2}i\pi(t+1)}$  |
|                                                     | $f_3$                                                | $-i$                                                 | $-ie^{-\frac{1}{2}i\pi(t+1)}$ |
|                                                     | $f_4$                                                | $-i$                                                 | $ie^{-\frac{1}{2}i\pi(t+1)}$  |
| $g \quad (\frac{1}{2}, \frac{t}{2}, \frac{1}{2})$   | $\{2_{010} \frac{1}{2} \quad 0 \quad \frac{1}{2} \}$ | $\{m_{100} 0 \quad \frac{1}{2} \quad \frac{1}{2} \}$ |                               |
|                                                     | $g_1$                                                | $0$                                                  | $0$                           |
| $h \quad (\frac{1-t}{2}, \frac{1}{2}, \frac{1}{2})$ | $\{2_{100} 0 \quad \frac{1}{2} \quad \frac{1}{2} \}$ | $\{m_{010} \frac{1}{2} \quad 0 \quad \frac{1}{2} \}$ |                               |
|                                                     | $h_1$                                                | $0$                                                  | $0$                           |
| $i \quad (0, 0, \frac{t}{2})$                       | $\{2_{001} \frac{1}{2} \quad \frac{1}{2} \quad 0 \}$ | $\{m_{100} 0 \quad \frac{1}{2} \quad \frac{1}{2} \}$ |                               |
|                                                     | $i_1$                                                | $0$                                                  | $0$                           |
| $j \quad (\frac{1}{2}, 0, \frac{t}{2})$             | $\{2_{001} \frac{1}{2} \quad \frac{1}{2} \quad 0 \}$ | $\{m_{100} 0 \quad \frac{1}{2} \quad \frac{1}{2} \}$ |                               |
|                                                     | $j_1$                                                | $i$                                                  | $-ie^{-\frac{1}{2}i\pi t}$    |
|                                                     | $j_2$                                                | $i$                                                  | $ie^{-\frac{1}{2}i\pi t}$     |
|                                                     | $j_3$                                                | $-i$                                                 | $-ie^{-\frac{1}{2}i\pi t}$    |
|                                                     | $j_4$                                                | $-i$                                                 | $ie^{-\frac{1}{2}i\pi t}$     |
| $k \quad (\frac{1}{2}, \frac{1}{2}, \frac{t}{2})$   | $\{2_{001} \frac{1}{2} \quad \frac{1}{2} \quad 0 \}$ | $\{m_{100} 0 \quad \frac{1}{2} \quad \frac{1}{2} \}$ |                               |
|                                                     | $k_1$                                                | $0$                                                  | $0$                           |
| $l \quad (0, \frac{1}{2}, \frac{t}{2})$             | $\{2_{001} \frac{1}{2} \quad \frac{1}{2} \quad 0 \}$ | $\{m_{100} 0 \quad \frac{1}{2} \quad \frac{1}{2} \}$ |                               |
|                                                     | $l_1$                                                | $i$                                                  | $-ie^{-\frac{1}{2}i\pi(t+1)}$ |
|                                                     | $l_2$                                                | $i$                                                  | $ie^{-\frac{1}{2}i\pi(t+1)}$  |
|                                                     | $l_3$                                                | $-i$                                                 | $-ie^{-\frac{1}{2}i\pi(t+1)}$ |
|                                                     | $l_4$                                                | $-i$                                                 | $ie^{-\frac{1}{2}i\pi(t+1)}$  |

$$\begin{aligned}
\mathcal{W}_1^{\text{gapless}} = & \sum_{m=1}^{n_{a_1}} \text{sgn}(v_m^{a_1}) \frac{1 - \text{sgn}(\delta_m^{a_1})}{2} - \sum_{m=1}^{n_{f_1}} \text{sgn}(v_m^{f_1}) \frac{1 - \text{sgn}(\delta_m^{f_1})}{2} - \sum_{m=1}^{n_{f_3}} \text{sgn}(v_m^{f_3}) \frac{1 - \text{sgn}(\delta_m^{f_3})}{2} \\
& + \sum_{m=1}^{n_{g_1}} \text{sgn}(v_m^{g_1}) \frac{1 - \text{sgn}(\delta_m^{g_1})}{2} + \sum_{m=1}^{n_{h_1}} \text{sgn}(v_m^{h_1}) \frac{1 - \text{sgn}(\delta_m^{h_1})}{2} \\
& - \sum_{m=1}^{n_{i_1}} \text{sgn}(v_m^{i_1}) \frac{1 - \text{sgn}(\delta_m^{i_1})}{2} + \sum_{m=1}^{n_{j_1}} \text{sgn}(v_m^{j_1}) \frac{1 - \text{sgn}(\delta_m^{j_1})}{2} + \sum_{m=1}^{n_{j_3}} \text{sgn}(v_m^{j_3}) \frac{1 - \text{sgn}(\delta_m^{j_3})}{2}
\end{aligned} \tag{S48.1}$$

$$\begin{aligned}
\mathcal{W}_2^{\text{gapless}} = & \sum_{m=1}^{n_{b_1}} \text{sgn}(v_m^{b_1}) \frac{1 - \text{sgn}(\delta_m^{b_1})}{2} - \sum_{m=1}^{n_{f_1}} \text{sgn}(v_m^{f_1}) \frac{1 - \text{sgn}(\delta_m^{f_1})}{2} - \sum_{m=1}^{n_{f_3}} \text{sgn}(v_m^{f_3}) \frac{1 - \text{sgn}(\delta_m^{f_3})}{2} \\
& - \sum_{m=1}^{n_{i_1}} \text{sgn}(v_m^{i_1}) \frac{1 - \text{sgn}(\delta_m^{i_1})}{2} + \sum_{m=1}^{n_{l_1}} \text{sgn}(v_m^{l_1}) \frac{1 - \text{sgn}(\delta_m^{l_1})}{2} + \sum_{m=1}^{n_{l_3}} \text{sgn}(v_m^{l_3}) \frac{1 - \text{sgn}(\delta_m^{l_3})}{2}
\end{aligned} \tag{S48.2}$$

$$\begin{aligned}
\mathcal{W}_3^{\text{gapless}} = & \sum_{m=1}^{n_{c_1}} \text{sgn}(v_m^{c_1}) \frac{1 - \text{sgn}(\delta_m^{c_1})}{2} + \sum_{m=1}^{n_{c_3}} \text{sgn}(v_m^{c_3}) \frac{1 - \text{sgn}(\delta_m^{c_3})}{2} - \sum_{m=1}^{n_{g_1}} \text{sgn}(v_m^{g_1}) \frac{1 - \text{sgn}(\delta_m^{g_1})}{2} \\
& - \sum_{m=1}^{n_{j_1}} \text{sgn}(v_m^{j_1}) \frac{1 - \text{sgn}(\delta_m^{j_1})}{2} - \sum_{m=1}^{n_{j_3}} \text{sgn}(v_m^{j_3}) \frac{1 - \text{sgn}(\delta_m^{j_3})}{2} + \sum_{m=1}^{n_{k_1}} \text{sgn}(v_m^{k_1}) \frac{1 - \text{sgn}(\delta_m^{k_1})}{2}
\end{aligned} \tag{S48.3}$$

$$\begin{aligned} \mathcal{W}_4^{\text{gapless}} = & \sum_{m=1}^{n_{d_1}} \text{sgn}(v_m^{d_1}) \frac{1 - \text{sgn}(\delta_m^{d_1})}{2} + \sum_{m=1}^{n_{d_3}} \text{sgn}(v_m^{d_3}) \frac{1 - \text{sgn}(\delta_m^{d_3})}{2} - \sum_{m=1}^{n_{h_1}} \text{sgn}(v_m^{h_1}) \frac{1 - \text{sgn}(\delta_m^{h_1})}{2} \\ & - \sum_{m=1}^{n_{k_1}} \text{sgn}(v_m^{k_1}) \frac{1 - \text{sgn}(\delta_m^{k_1})}{2} + \sum_{m=1}^{n_{l_1}} \text{sgn}(v_m^{l_1}) \frac{1 - \text{sgn}(\delta_m^{l_1})}{2} + \sum_{m=1}^{n_{l_3}} \text{sgn}(v_m^{l_3}) \frac{1 - \text{sgn}(\delta_m^{l_3})}{2} \end{aligned} \quad (\text{S48.4})$$

$$\begin{aligned} \mathcal{W}_5^{\text{gapless}} = & \sum_{m=1}^{n_{e_1}} \text{sgn}(v_m^{e_1}) \frac{1 - \text{sgn}(\delta_m^{e_1})}{2} + \sum_{m=1}^{n_{e_3}} \text{sgn}(v_m^{e_3}) \frac{1 - \text{sgn}(\delta_m^{e_3})}{2} - \sum_{m=1}^{n_{f_1}} \text{sgn}(v_m^{f_1}) \frac{1 - \text{sgn}(\delta_m^{f_1})}{2} \\ & - \sum_{m=1}^{n_{f_3}} \text{sgn}(v_m^{f_3}) \frac{1 - \text{sgn}(\delta_m^{f_3})}{2} + \sum_{m=1}^{n_{g_1}} \text{sgn}(v_m^{g_1}) \frac{1 - \text{sgn}(\delta_m^{g_1})}{2} + \sum_{m=1}^{n_{h_1}} \text{sgn}(v_m^{h_1}) \frac{1 - \text{sgn}(\delta_m^{h_1})}{2} \end{aligned} \quad (\text{S48.5})$$

$$\begin{aligned} \mathcal{W}_1^{\text{gapped}} = & 2 \sum_{m=1}^{n_{e_3}} \text{sgn}(v_m^{e_3}) \frac{1 - \text{sgn}(\delta_m^{e_3})}{2} - 2 \sum_{m=1}^{n_{f_3}} \text{sgn}(v_m^{f_3}) \frac{1 - \text{sgn}(\delta_m^{f_3})}{2} + \sum_{m=1}^{n_{g_1}} \text{sgn}(v_m^{g_1}) \frac{1 - \text{sgn}(\delta_m^{g_1})}{2} \\ & + \sum_{m=1}^{n_{h_1}} \text{sgn}(v_m^{h_1}) \frac{1 - \text{sgn}(\delta_m^{h_1})}{2} \end{aligned} \quad (\text{S48.6})$$

$$\mathcal{W}_2^{\text{gapped}} = \sum_{m=1}^{n_{f_1}} \text{sgn}(v_m^{f_1}) \frac{1 - \text{sgn}(\delta_m^{f_1})}{2} - \sum_{m=1}^{n_{f_3}} \text{sgn}(v_m^{f_3}) \frac{1 - \text{sgn}(\delta_m^{f_3})}{2} \quad (\text{S48.7})$$

$$\mathcal{W}_3^{\text{gapped}} = - \sum_{m=1}^{n_{j_1}} \text{sgn}(v_m^{j_1}) \frac{1 - \text{sgn}(\delta_m^{j_1})}{2} + \sum_{m=1}^{n_{j_3}} \text{sgn}(v_m^{j_3}) \frac{1 - \text{sgn}(\delta_m^{j_3})}{2} \quad (\text{S48.8})$$

$$\begin{aligned} \mathcal{W}_4^{\text{gapped}} = & 2 \sum_{m=1}^{n_{c_3}} \text{sgn}(v_m^{c_3}) \frac{1 - \text{sgn}(\delta_m^{c_3})}{2} + 2 \sum_{m=1}^{n_{e_3}} \text{sgn}(v_m^{e_3}) \frac{1 - \text{sgn}(\delta_m^{e_3})}{2} - 2 \sum_{m=1}^{n_{f_3}} \text{sgn}(v_m^{f_3}) \frac{1 - \text{sgn}(\delta_m^{f_3})}{2} \\ & + \sum_{m=1}^{n_{h_1}} \text{sgn}(v_m^{h_1}) \frac{1 - \text{sgn}(\delta_m^{h_1})}{2} - 2 \sum_{m=1}^{n_{j_1}} \text{sgn}(v_m^{j_1}) \frac{1 - \text{sgn}(\delta_m^{j_1})}{2} + \sum_{m=1}^{n_{k_1}} \text{sgn}(v_m^{k_1}) \frac{1 - \text{sgn}(\delta_m^{k_1})}{2} \end{aligned} \quad (\text{S48.9})$$

$$\begin{aligned} \mathcal{W}_5^{\text{gapped}} = & \sum_{m=1}^{n_{c_3}} \text{sgn}(v_m^{c_3}) \frac{1 - \text{sgn}(\delta_m^{c_3})}{2} + \sum_{m=1}^{n_{d_3}} \text{sgn}(v_m^{d_3}) \frac{1 - \text{sgn}(\delta_m^{d_3})}{2} + \sum_{m=1}^{n_{e_3}} \text{sgn}(v_m^{e_3}) \frac{1 - \text{sgn}(\delta_m^{e_3})}{2} \\ & - \sum_{m=1}^{n_{f_3}} \text{sgn}(v_m^{f_3}) \frac{1 - \text{sgn}(\delta_m^{f_3})}{2} - \sum_{m=1}^{n_{j_1}} \text{sgn}(v_m^{j_1}) \frac{1 - \text{sgn}(\delta_m^{j_1})}{2} + \sum_{m=1}^{n_{l_1}} \text{sgn}(v_m^{l_1}) \frac{1 - \text{sgn}(\delta_m^{l_1})}{2} \end{aligned} \quad (\text{S48.10})$$

$$\begin{aligned} \mathcal{W}_6^{\text{gapped}} = & \sum_{m=1}^{n_{c_3}} \text{sgn}(v_m^{c_3}) \frac{1 - \text{sgn}(\delta_m^{c_3})}{2} + \sum_{m=1}^{n_{d_3}} \text{sgn}(v_m^{d_3}) \frac{1 - \text{sgn}(\delta_m^{d_3})}{2} + \sum_{m=1}^{n_{e_3}} \text{sgn}(v_m^{e_3}) \frac{1 - \text{sgn}(\delta_m^{e_3})}{2} \\ & - \sum_{m=1}^{n_{f_3}} \text{sgn}(v_m^{f_3}) \frac{1 - \text{sgn}(\delta_m^{f_3})}{2} - \sum_{m=1}^{n_{j_1}} \text{sgn}(v_m^{j_1}) \frac{1 - \text{sgn}(\delta_m^{j_1})}{2} + \sum_{m=1}^{n_{l_3}} \text{sgn}(v_m^{l_3}) \frac{1 - \text{sgn}(\delta_m^{l_3})}{2} \end{aligned} \quad (\text{S48.11})$$

## S49. SPACE GROUP NO. 49

| line segment                                               | character of irrep (generators only)                                                                                                                                                               |
|------------------------------------------------------------|----------------------------------------------------------------------------------------------------------------------------------------------------------------------------------------------------|
| $a \left( \frac{t}{2}, 0, 0 \right)$                       | $a_1 \begin{array}{c} \{2_{100}  0 \ 0 \ \frac{1}{2}\} \ \{m_{010}  0 \ 0 \ \frac{1}{2}\} \\ 0 \end{array}$                                                                                        |
| $b \left( 0, \frac{t}{2}, 0 \right)$                       | $b_1 \begin{array}{c} \{2_{010}  0 \ 0 \ \frac{1}{2}\} \ \{m_{100}  0 \ 0 \ \frac{1}{2}\} \\ 0 \end{array}$                                                                                        |
| $c \left( \frac{1}{2}, \frac{t}{2}, 0 \right)$             | $c_1 \begin{array}{c} \{2_{010}  0 \ 0 \ \frac{1}{2}\} \ \{m_{100}  0 \ 0 \ \frac{1}{2}\} \\ 0 \end{array}$                                                                                        |
| $d \left( \frac{1-t}{2}, \frac{1}{2}, 0 \right)$           | $d_1 \begin{array}{c} \{2_{100}  0 \ 0 \ \frac{1}{2}\} \ \{m_{010}  0 \ 0 \ \frac{1}{2}\} \\ 0 \end{array}$                                                                                        |
| $e \left( \frac{t}{2}, 0, \frac{1}{2} \right)$             | $\begin{array}{c} \{2_{100}  0 \ 0 \ \frac{1}{2}\} \ \{m_{010}  0 \ 0 \ \frac{1}{2}\} \\ e_1 \quad i \quad -1 \\ e_2 \quad i \quad 1 \\ e_3 \quad -i \quad -1 \\ e_4 \quad -i \quad 1 \end{array}$ |
| $f \left( 0, \frac{t}{2}, \frac{1}{2} \right)$             | $\begin{array}{c} \{2_{010}  0 \ 0 \ \frac{1}{2}\} \ \{m_{100}  0 \ 0 \ \frac{1}{2}\} \\ f_1 \quad i \quad -1 \\ f_2 \quad i \quad 1 \\ f_3 \quad -i \quad -1 \\ f_4 \quad -i \quad 1 \end{array}$ |
| $g \left( \frac{1}{2}, \frac{t}{2}, \frac{1}{2} \right)$   | $\begin{array}{c} \{2_{010}  0 \ 0 \ \frac{1}{2}\} \ \{m_{100}  0 \ 0 \ \frac{1}{2}\} \\ g_1 \quad i \quad -1 \\ g_2 \quad i \quad 1 \\ g_3 \quad -i \quad -1 \\ g_4 \quad -i \quad 1 \end{array}$ |
| $h \left( \frac{1-t}{2}, \frac{1}{2}, \frac{1}{2} \right)$ | $\begin{array}{c} \{2_{100}  0 \ 0 \ \frac{1}{2}\} \ \{m_{010}  0 \ 0 \ \frac{1}{2}\} \\ h_1 \quad i \quad -1 \\ h_2 \quad i \quad 1 \\ h_3 \quad -i \quad -1 \\ h_4 \quad -i \quad 1 \end{array}$ |
| $i \left( 0, 0, \frac{t}{2} \right)$                       | $i_1 \begin{array}{c} \{2_{001}  0 \ 0 \ 0\} \ \{m_{100}  0 \ 0 \ \frac{1}{2}\} \\ 0 \end{array}$                                                                                                  |
| $j \left( \frac{1}{2}, 0, \frac{t}{2} \right)$             | $j_1 \begin{array}{c} \{2_{001}  0 \ 0 \ 0\} \ \{m_{100}  0 \ 0 \ \frac{1}{2}\} \\ 0 \end{array}$                                                                                                  |
| $k \left( \frac{1}{2}, \frac{1}{2}, \frac{t}{2} \right)$   | $k_1 \begin{array}{c} \{2_{001}  0 \ 0 \ 0\} \ \{m_{100}  0 \ 0 \ \frac{1}{2}\} \\ 0 \end{array}$                                                                                                  |
| $l \left( 0, \frac{1}{2}, \frac{t}{2} \right)$             | $l_1 \begin{array}{c} \{2_{001}  0 \ 0 \ 0\} \ \{m_{100}  0 \ 0 \ \frac{1}{2}\} \\ 0 \end{array}$                                                                                                  |

$$\begin{aligned}
\mathcal{W}_1^{\text{gapless}} = & \sum_{m=1}^{n_{a_1}} \text{sgn}(v_m^{a_1}) \frac{1 - \text{sgn}(\delta_m^{a_1})}{2} - \sum_{m=1}^{n_{f_1}} \text{sgn}(v_m^{f_1}) \frac{1 - \text{sgn}(\delta_m^{f_1})}{2} - \sum_{m=1}^{n_{f_3}} \text{sgn}(v_m^{f_3}) \frac{1 - \text{sgn}(\delta_m^{f_3})}{2} \\
& + \sum_{m=1}^{n_{g_1}} \text{sgn}(v_m^{g_1}) \frac{1 - \text{sgn}(\delta_m^{g_1})}{2} + \sum_{m=1}^{n_{g_3}} \text{sgn}(v_m^{g_3}) \frac{1 - \text{sgn}(\delta_m^{g_3})}{2} + \sum_{m=1}^{n_{h_1}} \text{sgn}(v_m^{h_1}) \frac{1 - \text{sgn}(\delta_m^{h_1})}{2} \\
& + \sum_{m=1}^{n_{h_3}} \text{sgn}(v_m^{h_3}) \frac{1 - \text{sgn}(\delta_m^{h_3})}{2} - \sum_{m=1}^{n_{i_1}} \text{sgn}(v_m^{i_1}) \frac{1 - \text{sgn}(\delta_m^{i_1})}{2} + \sum_{m=1}^{n_{j_1}} \text{sgn}(v_m^{j_1}) \frac{1 - \text{sgn}(\delta_m^{j_1})}{2}
\end{aligned} \tag{S49.1}$$

$$\begin{aligned}
\mathcal{W}_2^{\text{gapless}} = & \sum_{m=1}^{n_{b_1}} \text{sgn}(v_m^{b_1}) \frac{1 - \text{sgn}(\delta_m^{b_1})}{2} - \sum_{m=1}^{n_{f_1}} \text{sgn}(v_m^{f_1}) \frac{1 - \text{sgn}(\delta_m^{f_1})}{2} - \sum_{m=1}^{n_{f_3}} \text{sgn}(v_m^{f_3}) \frac{1 - \text{sgn}(\delta_m^{f_3})}{2} \\
& - \sum_{m=1}^{n_{i_1}} \text{sgn}(v_m^{i_1}) \frac{1 - \text{sgn}(\delta_m^{i_1})}{2} + \sum_{m=1}^{n_{l_1}} \text{sgn}(v_m^{l_1}) \frac{1 - \text{sgn}(\delta_m^{l_1})}{2}
\end{aligned} \tag{S49.2}$$

$$\begin{aligned} \mathcal{W}_3^{\text{gapless}} = & \sum_{m=1}^{n_{c_1}} \text{sgn}(v_m^{c_1}) \frac{1 - \text{sgn}(\delta_m^{c_1})}{2} - \sum_{m=1}^{n_{g_1}} \text{sgn}(v_m^{g_1}) \frac{1 - \text{sgn}(\delta_m^{g_1})}{2} - \sum_{m=1}^{n_{g_3}} \text{sgn}(v_m^{g_3}) \frac{1 - \text{sgn}(\delta_m^{g_3})}{2} \\ & - \sum_{m=1}^{n_{j_1}} \text{sgn}(v_m^{j_1}) \frac{1 - \text{sgn}(\delta_m^{j_1})}{2} + \sum_{m=1}^{n_{k_1}} \text{sgn}(v_m^{k_1}) \frac{1 - \text{sgn}(\delta_m^{k_1})}{2} \end{aligned} \quad (\text{S49.3})$$

$$\begin{aligned} \mathcal{W}_4^{\text{gapless}} = & \sum_{m=1}^{n_{d_1}} \text{sgn}(v_m^{d_1}) \frac{1 - \text{sgn}(\delta_m^{d_1})}{2} - \sum_{m=1}^{n_{h_1}} \text{sgn}(v_m^{h_1}) \frac{1 - \text{sgn}(\delta_m^{h_1})}{2} - \sum_{m=1}^{n_{h_3}} \text{sgn}(v_m^{h_3}) \frac{1 - \text{sgn}(\delta_m^{h_3})}{2} \\ & - \sum_{m=1}^{n_{k_1}} \text{sgn}(v_m^{k_1}) \frac{1 - \text{sgn}(\delta_m^{k_1})}{2} + \sum_{m=1}^{n_{l_1}} \text{sgn}(v_m^{l_1}) \frac{1 - \text{sgn}(\delta_m^{l_1})}{2} \end{aligned} \quad (\text{S49.4})$$

$$\begin{aligned} \mathcal{W}_5^{\text{gapless}} = & \sum_{m=1}^{n_{e_1}} \text{sgn}(v_m^{e_1}) \frac{1 - \text{sgn}(\delta_m^{e_1})}{2} + \sum_{m=1}^{n_{e_3}} \text{sgn}(v_m^{e_3}) \frac{1 - \text{sgn}(\delta_m^{e_3})}{2} - \sum_{m=1}^{n_{f_1}} \text{sgn}(v_m^{f_1}) \frac{1 - \text{sgn}(\delta_m^{f_1})}{2} \\ & - \sum_{m=1}^{n_{f_3}} \text{sgn}(v_m^{f_3}) \frac{1 - \text{sgn}(\delta_m^{f_3})}{2} + \sum_{m=1}^{n_{g_1}} \text{sgn}(v_m^{g_1}) \frac{1 - \text{sgn}(\delta_m^{g_1})}{2} + \sum_{m=1}^{n_{g_3}} \text{sgn}(v_m^{g_3}) \frac{1 - \text{sgn}(\delta_m^{g_3})}{2} \\ & + \sum_{m=1}^{n_{h_1}} \text{sgn}(v_m^{h_1}) \frac{1 - \text{sgn}(\delta_m^{h_1})}{2} + \sum_{m=1}^{n_{h_3}} \text{sgn}(v_m^{h_3}) \frac{1 - \text{sgn}(\delta_m^{h_3})}{2} \end{aligned} \quad (\text{S49.5})$$

$$\mathcal{W}_1^{\text{gapped}} = \sum_{m=1}^{n_{h_1}} \text{sgn}(v_m^{h_1}) \frac{1 - \text{sgn}(\delta_m^{h_1})}{2} - \sum_{m=1}^{n_{h_3}} \text{sgn}(v_m^{h_3}) \frac{1 - \text{sgn}(\delta_m^{h_3})}{2} \quad (\text{S49.6})$$

$$\begin{aligned} \mathcal{W}_2^{\text{gapped}} = & - \sum_{m=1}^{n_{e_3}} \text{sgn}(v_m^{e_3}) \frac{1 - \text{sgn}(\delta_m^{e_3})}{2} + \sum_{m=1}^{n_{f_1}} \text{sgn}(v_m^{f_1}) \frac{1 - \text{sgn}(\delta_m^{f_1})}{2} - \sum_{m=1}^{n_{g_3}} \text{sgn}(v_m^{g_3}) \frac{1 - \text{sgn}(\delta_m^{g_3})}{2} \\ & - \sum_{m=1}^{n_{h_3}} \text{sgn}(v_m^{h_3}) \frac{1 - \text{sgn}(\delta_m^{h_3})}{2} \end{aligned} \quad (\text{S49.7})$$

$$\begin{aligned} \mathcal{W}_3^{\text{gapped}} = & - \sum_{m=1}^{n_{e_3}} \text{sgn}(v_m^{e_3}) \frac{1 - \text{sgn}(\delta_m^{e_3})}{2} + \sum_{m=1}^{n_{f_3}} \text{sgn}(v_m^{f_3}) \frac{1 - \text{sgn}(\delta_m^{f_3})}{2} - \sum_{m=1}^{n_{g_3}} \text{sgn}(v_m^{g_3}) \frac{1 - \text{sgn}(\delta_m^{g_3})}{2} \\ & - \sum_{m=1}^{n_{h_3}} \text{sgn}(v_m^{h_3}) \frac{1 - \text{sgn}(\delta_m^{h_3})}{2} \end{aligned} \quad (\text{S49.8})$$

$$\mathcal{W}_4^{\text{gapped}} = \sum_{m=1}^{n_{g_1}} \text{sgn}(v_m^{g_1}) \frac{1 - \text{sgn}(\delta_m^{g_1})}{2} - \sum_{m=1}^{n_{g_3}} \text{sgn}(v_m^{g_3}) \frac{1 - \text{sgn}(\delta_m^{g_3})}{2} \quad (\text{S49.9})$$

## S50. SPACE GROUP NO. 50

| line segment                                               | character of irrep (generators only) |                                                                         |
|------------------------------------------------------------|--------------------------------------|-------------------------------------------------------------------------|
| $a \left( \frac{t}{2}, 0, 0 \right)$                       | $a_1$                                | $\{2_{100}   0 \frac{1}{2} 0\} \{m_{010}   \frac{1}{2} 0 0\}$           |
| $b \left( 0, \frac{t}{2}, 0 \right)$                       | $b_1$                                | $\{2_{010}   \frac{1}{2} 0 0\} \{m_{100}   0 \frac{1}{2} 0\}$           |
| $c \left( \frac{1}{2}, \frac{t}{2}, 0 \right)$             | $c_1$                                | $\{2_{010}   \frac{1}{2} 0 0\} \{m_{100}   0 \frac{1}{2} 0\}$           |
|                                                            |                                      | $i \quad -ie^{-\frac{1}{2}i\pi t}$                                      |
|                                                            | $c_2$                                | $i \quad ie^{-\frac{1}{2}i\pi t}$                                       |
|                                                            | $c_3$                                | $-i \quad -ie^{-\frac{1}{2}i\pi t}$                                     |
| $d \left( \frac{1-t}{2}, \frac{1}{2}, 0 \right)$           | $d_1$                                | $\{2_{100}   0 \frac{1}{2} 0\} \{m_{010}   \frac{1}{2} 0 0\}$           |
|                                                            |                                      | $i \quad -ie^{-\frac{1}{2}i\pi(1-t)}$                                   |
|                                                            | $d_2$                                | $i \quad ie^{-\frac{1}{2}i\pi(1-t)}$                                    |
|                                                            | $d_3$                                | $-i \quad -ie^{-\frac{1}{2}i\pi(1-t)}$                                  |
| $e \left( \frac{t}{2}, 0, \frac{1}{2} \right)$             | $e_1$                                | $\{2_{100}   0 \frac{1}{2} 0\} \{m_{010}   \frac{1}{2} 0 0\}$           |
|                                                            |                                      | $0 \quad 0$                                                             |
| $f \left( 0, \frac{t}{2}, \frac{1}{2} \right)$             | $f_1$                                | $\{2_{010}   \frac{1}{2} 0 0\} \{m_{100}   0 \frac{1}{2} 0\}$           |
|                                                            |                                      | $0 \quad 0$                                                             |
| $g \left( \frac{1}{2}, \frac{t}{2}, \frac{1}{2} \right)$   | $g_1$                                | $\{2_{010}   \frac{1}{2} 0 0\} \{m_{100}   0 \frac{1}{2} 0\}$           |
|                                                            |                                      | $i \quad -ie^{-\frac{1}{2}i\pi t}$                                      |
|                                                            | $g_2$                                | $i \quad ie^{-\frac{1}{2}i\pi t}$                                       |
|                                                            | $g_3$                                | $-i \quad -ie^{-\frac{1}{2}i\pi t}$                                     |
| $h \left( \frac{1-t}{2}, \frac{1}{2}, \frac{1}{2} \right)$ | $h_1$                                | $\{2_{100}   0 \frac{1}{2} 0\} \{m_{010}   \frac{1}{2} 0 0\}$           |
|                                                            |                                      | $i \quad -ie^{-\frac{1}{2}i\pi(1-t)}$                                   |
|                                                            | $h_2$                                | $i \quad ie^{-\frac{1}{2}i\pi(1-t)}$                                    |
|                                                            | $h_3$                                | $-i \quad -ie^{-\frac{1}{2}i\pi(1-t)}$                                  |
| $i \left( 0, 0, \frac{t}{2} \right)$                       | $i_1$                                | $\{2_{001}   \frac{1}{2} \frac{1}{2} 0\} \{m_{100}   0 \frac{1}{2} 0\}$ |
|                                                            |                                      | $0 \quad 0$                                                             |
| $j \left( \frac{1}{2}, 0, \frac{t}{2} \right)$             | $j_1$                                | $\{2_{001}   \frac{1}{2} \frac{1}{2} 0\} \{m_{100}   0 \frac{1}{2} 0\}$ |
|                                                            |                                      | $i \quad -i$                                                            |
|                                                            | $j_2$                                | $i \quad i$                                                             |
|                                                            | $j_3$                                | $-i \quad -i$                                                           |
| $k \left( \frac{1}{2}, \frac{1}{2}, \frac{t}{2} \right)$   | $k_1$                                | $\{2_{001}   \frac{1}{2} \frac{1}{2} 0\} \{m_{100}   0 \frac{1}{2} 0\}$ |
|                                                            |                                      | $0 \quad 0$                                                             |
| $l \left( 0, \frac{1}{2}, \frac{t}{2} \right)$             | $l_1$                                | $\{2_{001}   \frac{1}{2} \frac{1}{2} 0\} \{m_{100}   0 \frac{1}{2} 0\}$ |
|                                                            |                                      | $i \quad -1$                                                            |
|                                                            | $l_2$                                | $i \quad 1$                                                             |
|                                                            | $l_3$                                | $-i \quad -1$                                                           |
|                                                            | $l_4$                                | $-i \quad 1$                                                            |

$$\begin{aligned}
\mathcal{W}_1^{\text{gapless}} = & \sum_{m=1}^{n_{a_1}} \text{sgn}(v_m^{a_1}) \frac{1 - \text{sgn}(\delta_m^{a_1})}{2} - \sum_{m=1}^{n_{f_1}} \text{sgn}(v_m^{f_1}) \frac{1 - \text{sgn}(\delta_m^{f_1})}{2} + \sum_{m=1}^{n_{g_1}} \text{sgn}(v_m^{g_1}) \frac{1 - \text{sgn}(\delta_m^{g_1})}{2} \\
& + \sum_{m=1}^{n_{g_3}} \text{sgn}(v_m^{g_3}) \frac{1 - \text{sgn}(\delta_m^{g_3})}{2} + \sum_{m=1}^{n_{h_1}} \text{sgn}(v_m^{h_1}) \frac{1 - \text{sgn}(\delta_m^{h_1})}{2} + \sum_{m=1}^{n_{h_3}} \text{sgn}(v_m^{h_3}) \frac{1 - \text{sgn}(\delta_m^{h_3})}{2} \\
& - \sum_{m=1}^{n_{i_1}} \text{sgn}(v_m^{i_1}) \frac{1 - \text{sgn}(\delta_m^{i_1})}{2} + \sum_{m=1}^{n_{j_1}} \text{sgn}(v_m^{j_1}) \frac{1 - \text{sgn}(\delta_m^{j_1})}{2} + \sum_{m=1}^{n_{j_3}} \text{sgn}(v_m^{j_3}) \frac{1 - \text{sgn}(\delta_m^{j_3})}{2}
\end{aligned} \tag{S50.1}$$

$$\begin{aligned}\mathcal{W}_2^{\text{gapless}} = & \sum_{m=1}^{n_{b_1}} \text{sgn}(v_m^{b_1}) \frac{1 - \text{sgn}(\delta_m^{b_1})}{2} - \sum_{m=1}^{n_{f_1}} \text{sgn}(v_m^{f_1}) \frac{1 - \text{sgn}(\delta_m^{f_1})}{2} - \sum_{m=1}^{n_{i_1}} \text{sgn}(v_m^{i_1}) \frac{1 - \text{sgn}(\delta_m^{i_1})}{2} \\ & + \sum_{m=1}^{n_{l_1}} \text{sgn}(v_m^{l_1}) \frac{1 - \text{sgn}(\delta_m^{l_1})}{2} + \sum_{m=1}^{n_{l_3}} \text{sgn}(v_m^{l_3}) \frac{1 - \text{sgn}(\delta_m^{l_3})}{2}\end{aligned}\quad (\text{S50.2})$$

$$\begin{aligned}\mathcal{W}_3^{\text{gapless}} = & \sum_{m=1}^{n_{c_1}} \text{sgn}(v_m^{c_1}) \frac{1 - \text{sgn}(\delta_m^{c_1})}{2} + \sum_{m=1}^{n_{c_3}} \text{sgn}(v_m^{c_3}) \frac{1 - \text{sgn}(\delta_m^{c_3})}{2} - \sum_{m=1}^{n_{g_1}} \text{sgn}(v_m^{g_1}) \frac{1 - \text{sgn}(\delta_m^{g_1})}{2} - \sum_{m=1}^{n_{g_3}} \text{sgn}(v_m^{g_3}) \frac{1 - \text{sgn}(\delta_m^{g_3})}{2} \\ & - \sum_{m=1}^{n_{j_1}} \text{sgn}(v_m^{j_1}) \frac{1 - \text{sgn}(\delta_m^{j_1})}{2} - \sum_{m=1}^{n_{j_3}} \text{sgn}(v_m^{j_3}) \frac{1 - \text{sgn}(\delta_m^{j_3})}{2} + \sum_{m=1}^{n_{k_1}} \text{sgn}(v_m^{k_1}) \frac{1 - \text{sgn}(\delta_m^{k_1})}{2}\end{aligned}\quad (\text{S50.3})$$

$$\begin{aligned}\mathcal{W}_4^{\text{gapless}} = & \sum_{m=1}^{n_{d_1}} \text{sgn}(v_m^{d_1}) \frac{1 - \text{sgn}(\delta_m^{d_1})}{2} + \sum_{m=1}^{n_{d_3}} \text{sgn}(v_m^{d_3}) \frac{1 - \text{sgn}(\delta_m^{d_3})}{2} - \sum_{m=1}^{n_{h_1}} \text{sgn}(v_m^{h_1}) \frac{1 - \text{sgn}(\delta_m^{h_1})}{2} - \sum_{m=1}^{n_{h_3}} \text{sgn}(v_m^{h_3}) \frac{1 - \text{sgn}(\delta_m^{h_3})}{2} \\ & - \sum_{m=1}^{n_{k_1}} \text{sgn}(v_m^{k_1}) \frac{1 - \text{sgn}(\delta_m^{k_1})}{2} + \sum_{m=1}^{n_{l_1}} \text{sgn}(v_m^{l_1}) \frac{1 - \text{sgn}(\delta_m^{l_1})}{2} + \sum_{m=1}^{n_{l_3}} \text{sgn}(v_m^{l_3}) \frac{1 - \text{sgn}(\delta_m^{l_3})}{2}\end{aligned}\quad (\text{S50.4})$$

$$\begin{aligned}\mathcal{W}_5^{\text{gapless}} = & \sum_{m=1}^{n_{e_1}} \text{sgn}(v_m^{e_1}) \frac{1 - \text{sgn}(\delta_m^{e_1})}{2} - \sum_{m=1}^{n_{f_1}} \text{sgn}(v_m^{f_1}) \frac{1 - \text{sgn}(\delta_m^{f_1})}{2} + \sum_{m=1}^{n_{g_1}} \text{sgn}(v_m^{g_1}) \frac{1 - \text{sgn}(\delta_m^{g_1})}{2} \\ & + \sum_{m=1}^{n_{g_3}} \text{sgn}(v_m^{g_3}) \frac{1 - \text{sgn}(\delta_m^{g_3})}{2} + \sum_{m=1}^{n_{h_1}} \text{sgn}(v_m^{h_1}) \frac{1 - \text{sgn}(\delta_m^{h_1})}{2} + \sum_{m=1}^{n_{h_3}} \text{sgn}(v_m^{h_3}) \frac{1 - \text{sgn}(\delta_m^{h_3})}{2}\end{aligned}\quad (\text{S50.5})$$

$$\mathcal{W}_1^{\text{gapped}} = \sum_{m=1}^{n_{h_1}} \text{sgn}(v_m^{h_1}) \frac{1 - \text{sgn}(\delta_m^{h_1})}{2} - \sum_{m=1}^{n_{h_3}} \text{sgn}(v_m^{h_3}) \frac{1 - \text{sgn}(\delta_m^{h_3})}{2} \quad (\text{S50.6})$$

$$\mathcal{W}_2^{\text{gapped}} = \sum_{m=1}^{n_{g_1}} \text{sgn}(v_m^{g_1}) \frac{1 - \text{sgn}(\delta_m^{g_1})}{2} - \sum_{m=1}^{n_{g_3}} \text{sgn}(v_m^{g_3}) \frac{1 - \text{sgn}(\delta_m^{g_3})}{2} \quad (\text{S50.7})$$

$$\mathcal{W}_3^{\text{gapped}} = - \sum_{m=1}^{n_{j_1}} \text{sgn}(v_m^{j_1}) \frac{1 - \text{sgn}(\delta_m^{j_1})}{2} + \sum_{m=1}^{n_{j_3}} \text{sgn}(v_m^{j_3}) \frac{1 - \text{sgn}(\delta_m^{j_3})}{2} \quad (\text{S50.8})$$

$$\begin{aligned}\mathcal{W}_4^{\text{gapped}} = & 2 \sum_{m=1}^{n_{c_3}} \text{sgn}(v_m^{c_3}) \frac{1 - \text{sgn}(\delta_m^{c_3})}{2} - 2 \sum_{m=1}^{n_{g_3}} \text{sgn}(v_m^{g_3}) \frac{1 - \text{sgn}(\delta_m^{g_3})}{2} - 2 \sum_{m=1}^{n_{j_1}} \text{sgn}(v_m^{j_1}) \frac{1 - \text{sgn}(\delta_m^{j_1})}{2} \\ & + \sum_{m=1}^{n_{k_1}} \text{sgn}(v_m^{k_1}) \frac{1 - \text{sgn}(\delta_m^{k_1})}{2}\end{aligned}\quad (\text{S50.9})$$

$$\begin{aligned} \mathcal{W}_5^{\text{gapped}} = & \sum_{m=1}^{n_{c_3}} \text{sgn}(v_m^{c_3}) \frac{1 - \text{sgn}(\delta_m^{c_3})}{2} + \sum_{m=1}^{n_{d_3}} \text{sgn}(v_m^{d_3}) \frac{1 - \text{sgn}(\delta_m^{d_3})}{2} - \sum_{m=1}^{n_{g_3}} \text{sgn}(v_m^{g_3}) \frac{1 - \text{sgn}(\delta_m^{g_3})}{2} \\ & - \sum_{m=1}^{n_{h_3}} \text{sgn}(v_m^{h_3}) \frac{1 - \text{sgn}(\delta_m^{h_3})}{2} - \sum_{m=1}^{n_{j_1}} \text{sgn}(v_m^{j_1}) \frac{1 - \text{sgn}(\delta_m^{j_1})}{2} + \sum_{m=1}^{n_{l_1}} \text{sgn}(v_m^{l_1}) \frac{1 - \text{sgn}(\delta_m^{l_1})}{2} \end{aligned} \quad (\text{S50.10})$$

$$\begin{aligned} \mathcal{W}_6^{\text{gapped}} = & \sum_{m=1}^{n_{c_3}} \text{sgn}(v_m^{c_3}) \frac{1 - \text{sgn}(\delta_m^{c_3})}{2} + \sum_{m=1}^{n_{d_3}} \text{sgn}(v_m^{d_3}) \frac{1 - \text{sgn}(\delta_m^{d_3})}{2} - \sum_{m=1}^{n_{g_3}} \text{sgn}(v_m^{g_3}) \frac{1 - \text{sgn}(\delta_m^{g_3})}{2} \\ & - \sum_{m=1}^{n_{h_3}} \text{sgn}(v_m^{h_3}) \frac{1 - \text{sgn}(\delta_m^{h_3})}{2} - \sum_{m=1}^{n_{j_1}} \text{sgn}(v_m^{j_1}) \frac{1 - \text{sgn}(\delta_m^{j_1})}{2} + \sum_{m=1}^{n_{l_3}} \text{sgn}(v_m^{l_3}) \frac{1 - \text{sgn}(\delta_m^{l_3})}{2} \end{aligned} \quad (\text{S50.11})$$

### S51. SPACE GROUP NO. 51

| line segment                                        | character of irrep (generators only)                                                                                                                                                     |
|-----------------------------------------------------|------------------------------------------------------------------------------------------------------------------------------------------------------------------------------------------|
| $a \quad (\frac{t}{2}, 0, 0)$                       | $a_1 \quad \left\{ \begin{matrix} 2_{100}   \frac{1}{2} & 0 & 0 \\ 0 \end{matrix} \right\} \quad \left\{ \begin{matrix} m_{010}   0 & 0 & 0 \\ 0 \end{matrix} \right\}$                  |
| $b \quad (0, \frac{t}{2}, 0)$                       | $b_1 \quad \left\{ \begin{matrix} 2_{010}   0 & 0 & 0 \\ 0 \end{matrix} \right\} \quad \left\{ \begin{matrix} m_{100}   \frac{1}{2} & 0 & 0 \\ 0 \end{matrix} \right\}$                  |
| $c \quad (\frac{1}{2}, \frac{t}{2}, 0)$             | $\begin{matrix} c_1 & -i & i \\ c_2 & -i & -i \\ c_3 & i & i \\ c_4 & i & -i \end{matrix} \quad \left\{ \begin{matrix} 2_{010}   0 & 0 & 0 \\ \frac{1}{2} & 0 & 0 \end{matrix} \right\}$ |
| $d \quad (\frac{1-t}{2}, \frac{1}{2}, 0)$           | $d_1 \quad \left\{ \begin{matrix} 2_{100}   \frac{1}{2} & 0 & 0 \\ 0 \end{matrix} \right\} \quad \left\{ \begin{matrix} m_{010}   0 & 0 & 0 \\ 0 \end{matrix} \right\}$                  |
| $e \quad (\frac{t}{2}, 0, \frac{1}{2})$             | $e_1 \quad \left\{ \begin{matrix} 2_{100}   \frac{1}{2} & 0 & 0 \\ 0 \end{matrix} \right\} \quad \left\{ \begin{matrix} m_{010}   0 & 0 & 0 \\ 0 \end{matrix} \right\}$                  |
| $f \quad (0, \frac{t}{2}, \frac{1}{2})$             | $f_1 \quad \left\{ \begin{matrix} 2_{010}   0 & 0 & 0 \\ 0 \end{matrix} \right\} \quad \left\{ \begin{matrix} m_{100}   \frac{1}{2} & 0 & 0 \\ 0 \end{matrix} \right\}$                  |
| $g \quad (\frac{1}{2}, \frac{t}{2}, \frac{1}{2})$   | $\begin{matrix} g_1 & -i & i \\ g_2 & -i & -i \\ g_3 & i & i \\ g_4 & i & -i \end{matrix} \quad \left\{ \begin{matrix} 2_{010}   0 & 0 & 0 \\ \frac{1}{2} & 0 & 0 \end{matrix} \right\}$ |
| $h \quad (\frac{1-t}{2}, \frac{1}{2}, \frac{1}{2})$ | $h_1 \quad \left\{ \begin{matrix} 2_{100}   \frac{1}{2} & 0 & 0 \\ 0 \end{matrix} \right\} \quad \left\{ \begin{matrix} m_{010}   0 & 0 & 0 \\ 0 \end{matrix} \right\}$                  |
| $i \quad (0, 0, \frac{t}{2})$                       | $i_1 \quad \left\{ \begin{matrix} 2_{001}   \frac{1}{2} & 0 & 0 \\ 0 \end{matrix} \right\} \quad \left\{ \begin{matrix} m_{100}   \frac{1}{2} & 0 & 0 \\ 0 \end{matrix} \right\}$        |
| $j \quad (\frac{1}{2}, 0, \frac{t}{2})$             | $j_1 \quad \left\{ \begin{matrix} 2_{001}   \frac{1}{2} & 0 & 0 \\ 0 \end{matrix} \right\} \quad \left\{ \begin{matrix} m_{100}   \frac{1}{2} & 0 & 0 \\ 0 \end{matrix} \right\}$        |
| $k \quad (\frac{1}{2}, \frac{1}{2}, \frac{t}{2})$   | $k_1 \quad \left\{ \begin{matrix} 2_{001}   \frac{1}{2} & 0 & 0 \\ 0 \end{matrix} \right\} \quad \left\{ \begin{matrix} m_{100}   \frac{1}{2} & 0 & 0 \\ 0 \end{matrix} \right\}$        |
| $l \quad (0, \frac{1}{2}, \frac{t}{2})$             | $l_1 \quad \left\{ \begin{matrix} 2_{001}   \frac{1}{2} & 0 & 0 \\ 0 \end{matrix} \right\} \quad \left\{ \begin{matrix} m_{100}   \frac{1}{2} & 0 & 0 \\ 0 \end{matrix} \right\}$        |

$$\begin{aligned} \mathcal{W}_1^{\text{gapless}} = & \sum_{m=1}^{n_{a_1}} \text{sgn}(v_m^{a_1}) \frac{1 - \text{sgn}(\delta_m^{a_1})}{2} - \sum_{m=1}^{n_{f_1}} \text{sgn}(v_m^{f_1}) \frac{1 - \text{sgn}(\delta_m^{f_1})}{2} + \sum_{m=1}^{n_{g_1}} \text{sgn}(v_m^{g_1}) \frac{1 - \text{sgn}(\delta_m^{g_1})}{2} + \sum_{m=1}^{n_{g_2}} \text{sgn}(v_m^{g_2}) \frac{1 - \text{sgn}(\delta_m^{g_2})}{2} \\ & + \sum_{m=1}^{n_{h_1}} \text{sgn}(v_m^{h_1}) \frac{1 - \text{sgn}(\delta_m^{h_1})}{2} - \sum_{m=1}^{n_{i_1}} \text{sgn}(v_m^{i_1}) \frac{1 - \text{sgn}(\delta_m^{i_1})}{2} + 2 \sum_{m=1}^{n_{j_1}} \text{sgn}(v_m^{j_1}) \frac{1 - \text{sgn}(\delta_m^{j_1})}{2} \end{aligned} \quad (\text{S51.1})$$



$$\mathcal{W}_2^{\text{gapless}} = \sum_{m=1}^{n_{b_1}} \text{sgn}(v_m^{b_1}) \frac{1 - \text{sgn}(\delta_m^{b_1})}{2} - \sum_{m=1}^{n_{f_1}} \text{sgn}(v_m^{f_1}) \frac{1 - \text{sgn}(\delta_m^{f_1})}{2} - \sum_{m=1}^{n_{i_1}} \text{sgn}(v_m^{i_1}) \frac{1 - \text{sgn}(\delta_m^{i_1})}{2} + \sum_{m=1}^{n_{l_1}} \text{sgn}(v_m^{l_1}) \frac{1 - \text{sgn}(\delta_m^{l_1})}{2} \quad (\text{S51.2})$$

$$\mathcal{W}_3^{\text{gapless}} = \sum_{m=1}^{n_{c_1}} \text{sgn}(v_m^{c_1}) \frac{1 - \text{sgn}(\delta_m^{c_1})}{2} - \sum_{m=1}^{n_{g_1}} \text{sgn}(v_m^{g_1}) \frac{1 - \text{sgn}(\delta_m^{g_1})}{2} - \sum_{m=1}^{n_{j_1}} \text{sgn}(v_m^{j_1}) \frac{1 - \text{sgn}(\delta_m^{j_1})}{2} + \sum_{m=1}^{n_{k_1}} \text{sgn}(v_m^{k_1}) \frac{1 - \text{sgn}(\delta_m^{k_1})}{2} \quad (\text{S51.3})$$

$$\mathcal{W}_4^{\text{gapless}} = \sum_{m=1}^{n_{c_2}} \text{sgn}(v_m^{c_2}) \frac{1 - \text{sgn}(\delta_m^{c_2})}{2} - \sum_{m=1}^{n_{g_2}} \text{sgn}(v_m^{g_2}) \frac{1 - \text{sgn}(\delta_m^{g_2})}{2} - \sum_{m=1}^{n_{j_1}} \text{sgn}(v_m^{j_1}) \frac{1 - \text{sgn}(\delta_m^{j_1})}{2} + \sum_{m=1}^{n_{k_1}} \text{sgn}(v_m^{k_1}) \frac{1 - \text{sgn}(\delta_m^{k_1})}{2} \quad (\text{S51.4})$$

$$\begin{aligned} \mathcal{W}_5^{\text{gapless}} &= \sum_{m=1}^{n_{d_1}} \text{sgn}(v_m^{d_1}) \frac{1 - \text{sgn}(\delta_m^{d_1})}{2} - \sum_{m=1}^{n_{h_1}} \text{sgn}(v_m^{h_1}) \frac{1 - \text{sgn}(\delta_m^{h_1})}{2} - 2 \sum_{m=1}^{n_{k_1}} \text{sgn}(v_m^{k_1}) \frac{1 - \text{sgn}(\delta_m^{k_1})}{2} \\ &\quad + \sum_{m=1}^{n_{l_1}} \text{sgn}(v_m^{l_1}) \frac{1 - \text{sgn}(\delta_m^{l_1})}{2} \end{aligned} \quad (\text{S51.5})$$

$$\begin{aligned} \mathcal{W}_6^{\text{gapless}} &= \sum_{m=1}^{n_{e_1}} \text{sgn}(v_m^{e_1}) \frac{1 - \text{sgn}(\delta_m^{e_1})}{2} - \sum_{m=1}^{n_{f_1}} \text{sgn}(v_m^{f_1}) \frac{1 - \text{sgn}(\delta_m^{f_1})}{2} + \sum_{m=1}^{n_{g_1}} \text{sgn}(v_m^{g_1}) \frac{1 - \text{sgn}(\delta_m^{g_1})}{2} \\ &\quad + \sum_{m=1}^{n_{g_2}} \text{sgn}(v_m^{g_2}) \frac{1 - \text{sgn}(\delta_m^{g_2})}{2} + \sum_{m=1}^{n_{h_1}} \text{sgn}(v_m^{h_1}) \frac{1 - \text{sgn}(\delta_m^{h_1})}{2} \end{aligned} \quad (\text{S51.6})$$

$$\mathcal{W}_1^{\text{gapped}} = - \sum_{m=1}^{n_{g_1}} \text{sgn}(v_m^{g_1}) \frac{1 - \text{sgn}(\delta_m^{g_1})}{2} + \sum_{m=1}^{n_{g_2}} \text{sgn}(v_m^{g_2}) \frac{1 - \text{sgn}(\delta_m^{g_2})}{2} \quad (\text{S51.7})$$

## S52. SPACE GROUP NO. 52

| line segment                              | character of irrep (generators only)                                                                                                                                                                                                                                                                                                                                                                                                                                                                                                                                                                                                                          |
|-------------------------------------------|---------------------------------------------------------------------------------------------------------------------------------------------------------------------------------------------------------------------------------------------------------------------------------------------------------------------------------------------------------------------------------------------------------------------------------------------------------------------------------------------------------------------------------------------------------------------------------------------------------------------------------------------------------------|
| $a \quad (\frac{t}{2}, 0, 0)$             | $a_1 \quad \begin{Bmatrix} \{2_{100}   0 \frac{1}{2} \frac{1}{2}\} \\ 0 \end{Bmatrix} \begin{Bmatrix} \{m_{010}   \frac{1}{2} \frac{1}{2} \frac{1}{2}\} \\ 0 \end{Bmatrix}$                                                                                                                                                                                                                                                                                                                                                                                                                                                                                   |
| $b \quad (0, \frac{t}{2}, 0)$             | $b_1 \quad \begin{Bmatrix} \{2_{010}   \frac{1}{2} \frac{1}{2} \frac{1}{2}\} \\ 0 \end{Bmatrix} \begin{Bmatrix} \{m_{100}   0 \frac{1}{2} \frac{1}{2}\} \\ 0 \end{Bmatrix}$                                                                                                                                                                                                                                                                                                                                                                                                                                                                                   |
| $c \quad (\frac{1}{2}, \frac{t}{2}, 0)$   | $\begin{array}{l} c_1 \quad \begin{Bmatrix} \{2_{010}   \frac{1}{2} \frac{1}{2} \frac{1}{2}\} \\ -e^{-\frac{1}{2}i\pi(t+1)} \end{Bmatrix} \begin{Bmatrix} \{m_{100}   0 \frac{1}{2} \frac{1}{2}\} \\ -ie^{-\frac{1}{2}i\pi t} \end{Bmatrix} \\ c_2 \quad \begin{Bmatrix} -e^{-\frac{1}{2}i\pi(t+1)} \\ \end{Bmatrix} \begin{Bmatrix} ie^{-\frac{1}{2}i\pi t} \\ \end{Bmatrix} \\ c_3 \quad \begin{Bmatrix} e^{-\frac{1}{2}i\pi(t+1)} \\ \end{Bmatrix} \begin{Bmatrix} -ie^{-\frac{1}{2}i\pi t} \\ \end{Bmatrix} \\ c_4 \quad \begin{Bmatrix} e^{-\frac{1}{2}i\pi(t+1)} \\ \end{Bmatrix} \begin{Bmatrix} ie^{-\frac{1}{2}i\pi t} \\ \end{Bmatrix} \end{array}$ |
| $d \quad (\frac{1-t}{2}, \frac{1}{2}, 0)$ | $d_1 \quad \begin{Bmatrix} \{2_{100}   0 \frac{1}{2} \frac{1}{2}\} \\ 0 \end{Bmatrix} \begin{Bmatrix} \{m_{010}   \frac{1}{2} \frac{1}{2} \frac{1}{2}\} \\ 0 \end{Bmatrix}$                                                                                                                                                                                                                                                                                                                                                                                                                                                                                   |

|                                                     |                                                                  |                                                                  |                               |
|-----------------------------------------------------|------------------------------------------------------------------|------------------------------------------------------------------|-------------------------------|
| $e \quad (\frac{t}{2}, 0, \frac{1}{2})$             | $\{2_{100}   0 \quad \frac{1}{2} \quad \frac{1}{2} \}$           | $\{m_{010}   \frac{1}{2} \quad \frac{1}{2} \quad \frac{1}{2} \}$ |                               |
|                                                     | $e_1$                                                            | $i$                                                              | $-ie^{-\frac{1}{2}i\pi(t+1)}$ |
|                                                     | $e_2$                                                            | $i$                                                              | $ie^{-\frac{1}{2}i\pi(t+1)}$  |
|                                                     | $e_3$                                                            | $-i$                                                             | $-ie^{-\frac{1}{2}i\pi(t+1)}$ |
|                                                     | $e_4$                                                            | $-i$                                                             | $ie^{-\frac{1}{2}i\pi(t+1)}$  |
| $f \quad (0, \frac{t}{2}, \frac{1}{2})$             | $\{2_{010}   \frac{1}{2} \quad \frac{1}{2} \quad \frac{1}{2} \}$ | $\{m_{100}   0 \quad \frac{1}{2} \quad \frac{1}{2} \}$           |                               |
|                                                     | $f_1$                                                            | $-e^{-\frac{1}{2}i\pi(t+1)}$                                     | $-ie^{-\frac{1}{2}i\pi(t+1)}$ |
|                                                     | $f_2$                                                            | $-e^{-\frac{1}{2}i\pi(t+1)}$                                     | $ie^{-\frac{1}{2}i\pi(t+1)}$  |
|                                                     | $f_3$                                                            | $e^{-\frac{1}{2}i\pi(t+1)}$                                      | $-ie^{-\frac{1}{2}i\pi(t+1)}$ |
|                                                     | $f_4$                                                            | $e^{-\frac{1}{2}i\pi(t+1)}$                                      | $ie^{-\frac{1}{2}i\pi(t+1)}$  |
| $g \quad (\frac{1}{2}, \frac{t}{2}, \frac{1}{2})$   | $\{2_{010}   \frac{1}{2} \quad \frac{1}{2} \quad \frac{1}{2} \}$ | $\{m_{100}   0 \quad \frac{1}{2} \quad \frac{1}{2} \}$           |                               |
|                                                     | $g_1$                                                            | $0$                                                              | $0$                           |
| $h \quad (\frac{1-t}{2}, \frac{1}{2}, \frac{1}{2})$ | $\{2_{100}   0 \quad \frac{1}{2} \quad \frac{1}{2} \}$           | $\{m_{010}   \frac{1}{2} \quad \frac{1}{2} \quad \frac{1}{2} \}$ |                               |
|                                                     | $h_1$                                                            | $i$                                                              | $-e^{-\frac{1}{2}i\pi(3-t)}$  |
|                                                     | $h_2$                                                            | $i$                                                              | $e^{-\frac{1}{2}i\pi(3-t)}$   |
|                                                     | $h_3$                                                            | $-i$                                                             | $-e^{-\frac{1}{2}i\pi(3-t)}$  |
|                                                     | $h_4$                                                            | $-i$                                                             | $e^{-\frac{1}{2}i\pi(3-t)}$   |
| $i \quad (0, 0, \frac{t}{2})$                       | $\{2_{001}   \frac{1}{2} \quad 0 \quad 0 \}$                     | $\{m_{100}   0 \quad \frac{1}{2} \quad \frac{1}{2} \}$           |                               |
|                                                     | $i_1$                                                            | $0$                                                              | $0$                           |
| $j \quad (\frac{1}{2}, 0, \frac{t}{2})$             | $\{2_{001}   \frac{1}{2} \quad 0 \quad 0 \}$                     | $\{m_{100}   0 \quad \frac{1}{2} \quad \frac{1}{2} \}$           |                               |
|                                                     | $j_1$                                                            | $i$                                                              | $-ie^{-\frac{1}{2}i\pi t}$    |
|                                                     | $j_2$                                                            | $i$                                                              | $ie^{-\frac{1}{2}i\pi t}$     |
|                                                     | $j_3$                                                            | $-i$                                                             | $-ie^{-\frac{1}{2}i\pi t}$    |
|                                                     | $j_4$                                                            | $-i$                                                             | $ie^{-\frac{1}{2}i\pi t}$     |
| $k \quad (\frac{1}{2}, \frac{1}{2}, \frac{t}{2})$   | $\{2_{001}   \frac{1}{2} \quad 0 \quad 0 \}$                     | $\{m_{100}   0 \quad \frac{1}{2} \quad \frac{1}{2} \}$           |                               |
|                                                     | $k_1$                                                            | $0$                                                              | $0$                           |
| $l \quad (0, \frac{1}{2}, \frac{t}{2})$             | $\{2_{001}   \frac{1}{2} \quad 0 \quad 0 \}$                     | $\{m_{100}   0 \quad \frac{1}{2} \quad \frac{1}{2} \}$           |                               |
|                                                     | $l_1$                                                            | $-i$                                                             | $-ie^{-\frac{1}{2}i\pi(t+1)}$ |
|                                                     | $l_2$                                                            | $-i$                                                             | $ie^{-\frac{1}{2}i\pi(t+1)}$  |
|                                                     | $l_3$                                                            | $i$                                                              | $-ie^{-\frac{1}{2}i\pi(t+1)}$ |
|                                                     | $l_4$                                                            | $i$                                                              | $ie^{-\frac{1}{2}i\pi(t+1)}$  |

$$\begin{aligned}
\mathcal{W}_1^{\text{gapless}} = & \sum_{m=1}^{n_{a_1}} \text{sgn}(v_m^{a_1}) \frac{1 - \text{sgn}(\delta_m^{a_1})}{2} - \sum_{m=1}^{n_{f_1}} \text{sgn}(v_m^{f_1}) \frac{1 - \text{sgn}(\delta_m^{f_1})}{2} - \sum_{m=1}^{n_{f_3}} \text{sgn}(v_m^{f_3}) \frac{1 - \text{sgn}(\delta_m^{f_3})}{2} + \sum_{m=1}^{n_{g_1}} \text{sgn}(v_m^{g_1}) \frac{1 - \text{sgn}(\delta_m^{g_1})}{2} \\
& + 2 \sum_{m=1}^{n_{h_2}} \text{sgn}(v_m^{h_2}) \frac{1 - \text{sgn}(\delta_m^{h_2})}{2} - \sum_{m=1}^{n_{i_1}} \text{sgn}(v_m^{i_1}) \frac{1 - \text{sgn}(\delta_m^{i_1})}{2} + \sum_{m=1}^{n_{j_1}} \text{sgn}(v_m^{j_1}) \frac{1 - \text{sgn}(\delta_m^{j_1})}{2} \\
& + \sum_{m=1}^{n_{j_3}} \text{sgn}(v_m^{j_3}) \frac{1 - \text{sgn}(\delta_m^{j_3})}{2} - \sum_{m=1}^{n_{l_1}} \text{sgn}(v_m^{l_1}) \frac{1 - \text{sgn}(\delta_m^{l_1})}{2} + \sum_{m=1}^{n_{l_2}} \text{sgn}(v_m^{l_2}) \frac{1 - \text{sgn}(\delta_m^{l_2})}{2}
\end{aligned} \tag{S52.1}$$

$$\begin{aligned}
\mathcal{W}_2^{\text{gapless}} = & \sum_{m=1}^{n_{b_1}} \text{sgn}(v_m^{b_1}) \frac{1 - \text{sgn}(\delta_m^{b_1})}{2} - \sum_{m=1}^{n_{f_1}} \text{sgn}(v_m^{f_1}) \frac{1 - \text{sgn}(\delta_m^{f_1})}{2} - \sum_{m=1}^{n_{f_3}} \text{sgn}(v_m^{f_3}) \frac{1 - \text{sgn}(\delta_m^{f_3})}{2} \\
& - \sum_{m=1}^{n_{i_1}} \text{sgn}(v_m^{i_1}) \frac{1 - \text{sgn}(\delta_m^{i_1})}{2} + \sum_{m=1}^{n_{l_1}} \text{sgn}(v_m^{l_1}) \frac{1 - \text{sgn}(\delta_m^{l_1})}{2} + \sum_{m=1}^{n_{l_2}} \text{sgn}(v_m^{l_2}) \frac{1 - \text{sgn}(\delta_m^{l_2})}{2}
\end{aligned} \tag{S52.2}$$

$$\begin{aligned} \mathcal{W}_3^{\text{gapless}} = & \sum_{m=1}^{n_{c_1}} \text{sgn}(v_m^{c_1}) \frac{1 - \text{sgn}(\delta_m^{c_1})}{2} + \sum_{m=1}^{n_{c_3}} \text{sgn}(v_m^{c_3}) \frac{1 - \text{sgn}(\delta_m^{c_3})}{2} - \sum_{m=1}^{n_{g_1}} \text{sgn}(v_m^{g_1}) \frac{1 - \text{sgn}(\delta_m^{g_1})}{2} \\ & - \sum_{m=1}^{n_{j_1}} \text{sgn}(v_m^{j_1}) \frac{1 - \text{sgn}(\delta_m^{j_1})}{2} - \sum_{m=1}^{n_{j_3}} \text{sgn}(v_m^{j_3}) \frac{1 - \text{sgn}(\delta_m^{j_3})}{2} + 2 \sum_{m=1}^{n_{k_1}} \text{sgn}(v_m^{k_1}) \frac{1 - \text{sgn}(\delta_m^{k_1})}{2} \end{aligned} \quad (\text{S52.3})$$

$$\mathcal{W}_4^{\text{gapless}} = \sum_{m=1}^{n_{d_1}} \text{sgn}(v_m^{d_1}) \frac{1 - \text{sgn}(\delta_m^{d_1})}{2} - \sum_{m=1}^{n_{h_2}} \text{sgn}(v_m^{h_2}) \frac{1 - \text{sgn}(\delta_m^{h_2})}{2} - \sum_{m=1}^{n_{k_1}} \text{sgn}(v_m^{k_1}) \frac{1 - \text{sgn}(\delta_m^{k_1})}{2} + \sum_{m=1}^{n_{l_1}} \text{sgn}(v_m^{l_1}) \frac{1 - \text{sgn}(\delta_m^{l_1})}{2} \quad (\text{S52.4})$$

$$\begin{aligned} \mathcal{W}_5^{\text{gapless}} = & \sum_{m=1}^{n_{e_1}} \text{sgn}(v_m^{e_1}) \frac{1 - \text{sgn}(\delta_m^{e_1})}{2} + \sum_{m=1}^{n_{e_3}} \text{sgn}(v_m^{e_3}) \frac{1 - \text{sgn}(\delta_m^{e_3})}{2} - \sum_{m=1}^{n_{f_1}} \text{sgn}(v_m^{f_1}) \frac{1 - \text{sgn}(\delta_m^{f_1})}{2} \\ & - \sum_{m=1}^{n_{f_3}} \text{sgn}(v_m^{f_3}) \frac{1 - \text{sgn}(\delta_m^{f_3})}{2} + \sum_{m=1}^{n_{g_1}} \text{sgn}(v_m^{g_1}) \frac{1 - \text{sgn}(\delta_m^{g_1})}{2} \\ & + 2 \sum_{m=1}^{n_{h_2}} \text{sgn}(v_m^{h_2}) \frac{1 - \text{sgn}(\delta_m^{h_2})}{2} - \sum_{m=1}^{n_{l_1}} \text{sgn}(v_m^{l_1}) \frac{1 - \text{sgn}(\delta_m^{l_1})}{2} + \sum_{m=1}^{n_{l_2}} \text{sgn}(v_m^{l_2}) \frac{1 - \text{sgn}(\delta_m^{l_2})}{2} \end{aligned} \quad (\text{S52.5})$$

$$\mathcal{W}_6^{\text{gapless}} = \sum_{m=1}^{n_{h_1}} \text{sgn}(v_m^{h_1}) \frac{1 - \text{sgn}(\delta_m^{h_1})}{2} - \sum_{m=1}^{n_{h_2}} \text{sgn}(v_m^{h_2}) \frac{1 - \text{sgn}(\delta_m^{h_2})}{2} + \sum_{m=1}^{n_{l_1}} \text{sgn}(v_m^{l_1}) \frac{1 - \text{sgn}(\delta_m^{l_1})}{2} - \sum_{m=1}^{n_{l_2}} \text{sgn}(v_m^{l_2}) \frac{1 - \text{sgn}(\delta_m^{l_2})}{2} \quad (\text{S52.6})$$

$$\mathcal{W}_1^{\text{gapped}} = - \sum_{m=1}^{n_{j_1}} \text{sgn}(v_m^{j_1}) \frac{1 - \text{sgn}(\delta_m^{j_1})}{2} + \sum_{m=1}^{n_{j_3}} \text{sgn}(v_m^{j_3}) \frac{1 - \text{sgn}(\delta_m^{j_3})}{2} \quad (\text{S52.7})$$

$$\begin{aligned} \mathcal{W}_2^{\text{gapped}} = & 2 \sum_{m=1}^{n_{e_3}} \text{sgn}(v_m^{e_3}) \frac{1 - \text{sgn}(\delta_m^{e_3})}{2} - \sum_{m=1}^{n_{f_1}} \text{sgn}(v_m^{f_1}) \frac{1 - \text{sgn}(\delta_m^{f_1})}{2} - \sum_{m=1}^{n_{f_3}} \text{sgn}(v_m^{f_3}) \frac{1 - \text{sgn}(\delta_m^{f_3})}{2} + \sum_{m=1}^{n_{g_1}} \text{sgn}(v_m^{g_1}) \frac{1 - \text{sgn}(\delta_m^{g_1})}{2} \\ & + 2 \sum_{m=1}^{n_{h_2}} \text{sgn}(v_m^{h_2}) \frac{1 - \text{sgn}(\delta_m^{h_2})}{2} - \sum_{m=1}^{n_{l_1}} \text{sgn}(v_m^{l_1}) \frac{1 - \text{sgn}(\delta_m^{l_1})}{2} + \sum_{m=1}^{n_{l_2}} \text{sgn}(v_m^{l_2}) \frac{1 - \text{sgn}(\delta_m^{l_2})}{2} \end{aligned} \quad (\text{S52.8})$$

$$\mathcal{X}_1 = \sum_{m=1}^{n_{g_1}} \frac{1 - \text{sgn}(\delta_m^{g_1})}{2} \mod 2 \quad (\text{S52.9})$$

### S53. SPACE GROUP NO. 53

|              |                                      |
|--------------|--------------------------------------|
| line segment | character of irrep (generators only) |
|--------------|--------------------------------------|

|                                                     |                                  |                                                                                                                                                                              |                                                                                                                                                                                  |
|-----------------------------------------------------|----------------------------------|------------------------------------------------------------------------------------------------------------------------------------------------------------------------------|----------------------------------------------------------------------------------------------------------------------------------------------------------------------------------|
| $a \quad (\frac{t}{2}, 0, 0)$                       | $a_1$                            | $\{2_{100}   0 \ 0 \ 0 \}$                                                                                                                                                   | $\{m_{010}   \frac{1}{2} \ 0 \ \frac{1}{2} \}$                                                                                                                                   |
| $b \quad (0, \frac{t}{2}, 0)$                       | $b_1$                            | $\{2_{010}   \frac{1}{2} \ 0 \ \frac{1}{2} \}$                                                                                                                               | $\{m_{100}   0 \ 0 \ 0 \}$                                                                                                                                                       |
| $c \quad (\frac{1}{2}, \frac{t}{2}, 0)$             | $c_1$<br>$c_2$<br>$c_3$<br>$c_4$ | $\{2_{010}   \frac{1}{2} \ 0 \ \frac{1}{2} \}$<br>$i$<br>$i$<br>$-i$<br>$-i$                                                                                                 | $\{m_{100}   0 \ 0 \ 0 \}$<br>$-i$<br>$i$<br>$-i$<br>$i$                                                                                                                         |
| $d \quad (\frac{1-t}{2}, \frac{1}{2}, 0)$           | $d_1$                            | $\{2_{100}   0 \ 0 \ 0 \}$                                                                                                                                                   | $\{m_{010}   \frac{1}{2} \ 0 \ \frac{1}{2} \}$                                                                                                                                   |
| $e \quad (\frac{t}{2}, 0, \frac{1}{2})$             | $e_1$<br>$e_2$<br>$e_3$<br>$e_4$ | $\{2_{100}   0 \ 0 \ 0 \}$<br>$-i$<br>$-i$<br>$i$<br>$i$                                                                                                                     | $\{m_{010}   \frac{1}{2} \ 0 \ \frac{1}{2} \}$<br>$-ie^{-\frac{1}{2}i\pi(t+1)}$<br>$ie^{-\frac{1}{2}i\pi(t+1)}$<br>$-ie^{-\frac{1}{2}i\pi(t+1)}$<br>$ie^{-\frac{1}{2}i\pi(t+1)}$ |
| $f \quad (0, \frac{t}{2}, \frac{1}{2})$             | $f_1$                            | $\{2_{010}   \frac{1}{2} \ 0 \ \frac{1}{2} \}$                                                                                                                               | $\{m_{100}   0 \ 0 \ 0 \}$                                                                                                                                                       |
| $g \quad (\frac{1}{2}, \frac{t}{2}, \frac{1}{2})$   | $g_1$<br>$g_2$<br>$g_3$<br>$g_4$ | $\{2_{010}   \frac{1}{2} \ 0 \ \frac{1}{2} \}$<br>$i$<br>$i$<br>$-i$<br>$-i$                                                                                                 | $\{m_{100}   0 \ 0 \ 0 \}$<br>$-i$<br>$i$<br>$-i$<br>$i$                                                                                                                         |
| $h \quad (\frac{1-t}{2}, \frac{1}{2}, \frac{1}{2})$ | $h_1$<br>$h_2$<br>$h_3$<br>$h_4$ | $\{2_{100}   0 \ 0 \ 0 \}$<br>$-i$<br>$-i$<br>$i$<br>$i$                                                                                                                     | $\{m_{010}   \frac{1}{2} \ 0 \ \frac{1}{2} \}$<br>$-ie^{-\frac{1}{2}i\pi(2-t)}$<br>$ie^{-\frac{1}{2}i\pi(2-t)}$<br>$-ie^{-\frac{1}{2}i\pi(2-t)}$<br>$ie^{-\frac{1}{2}i\pi(2-t)}$ |
| $i \quad (0, 0, \frac{t}{2})$                       | $i_1$                            | $\{2_{001}   \frac{1}{2} \ 0 \ \frac{1}{2} \}$                                                                                                                               | $\{m_{100}   0 \ 0 \ 0 \}$                                                                                                                                                       |
| $j \quad (\frac{1}{2}, 0, \frac{t}{2})$             | $j_1$<br>$j_2$<br>$j_3$<br>$j_4$ | $\{2_{001}   \frac{1}{2} \ 0 \ \frac{1}{2} \}$<br>$-e^{-\frac{1}{2}i\pi(t+1)}$<br>$-e^{-\frac{1}{2}i\pi(t+1)}$<br>$e^{-\frac{1}{2}i\pi(t+1)}$<br>$e^{-\frac{1}{2}i\pi(t+1)}$ | $\{m_{100}   0 \ 0 \ 0 \}$<br>$-i$<br>$i$<br>$-i$<br>$i$                                                                                                                         |
| $k \quad (\frac{1}{2}, \frac{1}{2}, \frac{t}{2})$   | $k_1$<br>$k_2$<br>$k_3$<br>$k_4$ | $\{2_{001}   \frac{1}{2} \ 0 \ \frac{1}{2} \}$<br>$-e^{-\frac{1}{2}i\pi(t+1)}$<br>$-e^{-\frac{1}{2}i\pi(t+1)}$<br>$e^{-\frac{1}{2}i\pi(t+1)}$<br>$e^{-\frac{1}{2}i\pi(t+1)}$ | $\{m_{100}   0 \ 0 \ 0 \}$<br>$-i$<br>$i$<br>$-i$<br>$i$                                                                                                                         |
| $l \quad (0, \frac{1}{2}, \frac{t}{2})$             | $l_1$                            | $\{2_{001}   \frac{1}{2} \ 0 \ \frac{1}{2} \}$                                                                                                                               | $\{m_{100}   0 \ 0 \ 0 \}$                                                                                                                                                       |

$$\begin{aligned}
\mathcal{W}_1^{\text{gapless}} = & \sum_{m=1}^{n_{a_1}} \text{sgn}(v_m^{a_1}) \frac{1 - \text{sgn}(\delta_m^{a_1})}{2} - 2 \sum_{m=1}^{n_{f_1}} \text{sgn}(v_m^{f_1}) \frac{1 - \text{sgn}(\delta_m^{f_1})}{2} + \sum_{m=1}^{n_{g_1}} \text{sgn}(v_m^{g_1}) \frac{1 - \text{sgn}(\delta_m^{g_1})}{2} \\
& + \sum_{m=1}^{n_{g_2}} \text{sgn}(v_m^{g_2}) \frac{1 - \text{sgn}(\delta_m^{g_2})}{2} + \sum_{m=1}^{n_{h_1}} \text{sgn}(v_m^{h_1}) \frac{1 - \text{sgn}(\delta_m^{h_1})}{2} + \sum_{m=1}^{n_{h_2}} \text{sgn}(v_m^{h_2}) \frac{1 - \text{sgn}(\delta_m^{h_2})}{2} \\
& - \sum_{m=1}^{n_{i_1}} \text{sgn}(v_m^{i_1}) \frac{1 - \text{sgn}(\delta_m^{i_1})}{2} + \sum_{m=1}^{n_{j_1}} \text{sgn}(v_m^{j_1}) \frac{1 - \text{sgn}(\delta_m^{j_1})}{2} + \sum_{m=1}^{n_{j_3}} \text{sgn}(v_m^{j_3}) \frac{1 - \text{sgn}(\delta_m^{j_3})}{2}
\end{aligned} \tag{S53.1}$$

$$\mathcal{W}_2^{\text{gapless}} = \sum_{m=1}^{n_{b_1}} \text{sgn}(v_m^{b_1}) \frac{1 - \text{sgn}(\delta_m^{b_1})}{2} - 2 \sum_{m=1}^{n_{f_1}} \text{sgn}(v_m^{f_1}) \frac{1 - \text{sgn}(\delta_m^{f_1})}{2} - \sum_{m=1}^{n_{i_1}} \text{sgn}(v_m^{i_1}) \frac{1 - \text{sgn}(\delta_m^{i_1})}{2} + \sum_{m=1}^{n_{l_1}} \text{sgn}(v_m^{l_1}) \frac{1 - \text{sgn}(\delta_m^{l_1})}{2} \quad (\text{S53.2})$$

$$\begin{aligned} \mathcal{W}_3^{\text{gapless}} = & \sum_{m=1}^{n_{c_1}} \text{sgn}(v_m^{c_1}) \frac{1 - \text{sgn}(\delta_m^{c_1})}{2} + \sum_{m=1}^{n_{c_3}} \text{sgn}(v_m^{c_3}) \frac{1 - \text{sgn}(\delta_m^{c_3})}{2} - \sum_{m=1}^{n_{g_1}} \text{sgn}(v_m^{g_1}) \frac{1 - \text{sgn}(\delta_m^{g_1})}{2} \\ & - \sum_{m=1}^{n_{g_2}} \text{sgn}(v_m^{g_2}) \frac{1 - \text{sgn}(\delta_m^{g_2})}{2} - \sum_{m=1}^{n_{j_1}} \text{sgn}(v_m^{j_1}) \frac{1 - \text{sgn}(\delta_m^{j_1})}{2} - \sum_{m=1}^{n_{j_3}} \text{sgn}(v_m^{j_3}) \frac{1 - \text{sgn}(\delta_m^{j_3})}{2} \\ & + \sum_{m=1}^{n_{k_1}} \text{sgn}(v_m^{k_1}) \frac{1 - \text{sgn}(\delta_m^{k_1})}{2} + \sum_{m=1}^{n_{k_3}} \text{sgn}(v_m^{k_3}) \frac{1 - \text{sgn}(\delta_m^{k_3})}{2} \end{aligned} \quad (\text{S53.3})$$

$$\begin{aligned} \mathcal{W}_4^{\text{gapless}} = & \sum_{m=1}^{n_{d_1}} \text{sgn}(v_m^{d_1}) \frac{1 - \text{sgn}(\delta_m^{d_1})}{2} - \sum_{m=1}^{n_{h_1}} \text{sgn}(v_m^{h_1}) \frac{1 - \text{sgn}(\delta_m^{h_1})}{2} - \sum_{m=1}^{n_{h_2}} \text{sgn}(v_m^{h_2}) \frac{1 - \text{sgn}(\delta_m^{h_2})}{2} \\ & - \sum_{m=1}^{n_{k_1}} \text{sgn}(v_m^{k_1}) \frac{1 - \text{sgn}(\delta_m^{k_1})}{2} - \sum_{m=1}^{n_{k_3}} \text{sgn}(v_m^{k_3}) \frac{1 - \text{sgn}(\delta_m^{k_3})}{2} + \sum_{m=1}^{n_{l_1}} \text{sgn}(v_m^{l_1}) \frac{1 - \text{sgn}(\delta_m^{l_1})}{2} \end{aligned} \quad (\text{S53.4})$$

$$\mathcal{W}_5^{\text{gapless}} = \sum_{m=1}^{n_{e_1}} \text{sgn}(v_m^{e_1}) \frac{1 - \text{sgn}(\delta_m^{e_1})}{2} - \sum_{m=1}^{n_{f_1}} \text{sgn}(v_m^{f_1}) \frac{1 - \text{sgn}(\delta_m^{f_1})}{2} + \sum_{m=1}^{n_{g_1}} \text{sgn}(v_m^{g_1}) \frac{1 - \text{sgn}(\delta_m^{g_1})}{2} + \sum_{m=1}^{n_{h_1}} \text{sgn}(v_m^{h_1}) \frac{1 - \text{sgn}(\delta_m^{h_1})}{2} \quad (\text{S53.5})$$

$$\mathcal{W}_6^{\text{gapless}} = \sum_{m=1}^{n_{e_2}} \text{sgn}(v_m^{e_2}) \frac{1 - \text{sgn}(\delta_m^{e_2})}{2} - \sum_{m=1}^{n_{f_1}} \text{sgn}(v_m^{f_1}) \frac{1 - \text{sgn}(\delta_m^{f_1})}{2} + \sum_{m=1}^{n_{g_2}} \text{sgn}(v_m^{g_2}) \frac{1 - \text{sgn}(\delta_m^{g_2})}{2} + \sum_{m=1}^{n_{h_2}} \text{sgn}(v_m^{h_2}) \frac{1 - \text{sgn}(\delta_m^{h_2})}{2} \quad (\text{S53.6})$$

$$\begin{aligned} \mathcal{W}_1^{\text{gapped}} = & -2 \sum_{m=1}^{n_{c_3}} \text{sgn}(v_m^{c_3}) \frac{1 - \text{sgn}(\delta_m^{c_3})}{2} + \sum_{m=1}^{n_{g_1}} \text{sgn}(v_m^{g_1}) \frac{1 - \text{sgn}(\delta_m^{g_1})}{2} + \sum_{m=1}^{n_{g_2}} \text{sgn}(v_m^{g_2}) \frac{1 - \text{sgn}(\delta_m^{g_2})}{2} \\ & + \sum_{m=1}^{n_{j_1}} \text{sgn}(v_m^{j_1}) \frac{1 - \text{sgn}(\delta_m^{j_1})}{2} + \sum_{m=1}^{n_{j_3}} \text{sgn}(v_m^{j_3}) \frac{1 - \text{sgn}(\delta_m^{j_3})}{2} - \sum_{m=1}^{n_{k_1}} \text{sgn}(v_m^{k_1}) \frac{1 - \text{sgn}(\delta_m^{k_1})}{2} \\ & - \sum_{m=1}^{n_{k_3}} \text{sgn}(v_m^{k_3}) \frac{1 - \text{sgn}(\delta_m^{k_3})}{2} \end{aligned} \quad (\text{S53.7})$$

$$\mathcal{X}_1 = \sum_{m=1}^{n_{h_1}} \frac{1 - \text{sgn}(\delta_m^{h_1})}{2} + \sum_{m=1}^{n_{h_2}} \frac{1 - \text{sgn}(\delta_m^{h_2})}{2} + \sum_{m=1}^{n_{k_1}} \frac{1 - \text{sgn}(\delta_m^{k_1})}{2} + \sum_{m=1}^{n_{k_3}} \frac{1 - \text{sgn}(\delta_m^{k_3})}{2} \pmod{2} \quad (\text{S53.8})$$

#### S54. SPACE GROUP NO. 54

|              |                                      |
|--------------|--------------------------------------|
| line segment | character of irrep (generators only) |
|--------------|--------------------------------------|

|                                                     |                                  |                                                                                                                                                                              |                                                                              |
|-----------------------------------------------------|----------------------------------|------------------------------------------------------------------------------------------------------------------------------------------------------------------------------|------------------------------------------------------------------------------|
| $a \quad (\frac{t}{2}, 0, 0)$                       | $a_1$                            | $\{2_{100}   \frac{1}{2} \ 0 \ \frac{1}{2} \}$                                                                                                                               | $\{m_{010}   0 \ 0 \ \frac{1}{2} \}$                                         |
| $b \quad (0, \frac{t}{2}, 0)$                       | $b_1$                            | $\{2_{010}   0 \ 0 \ \frac{1}{2} \}$                                                                                                                                         | $\{m_{100}   \frac{1}{2} \ 0 \ \frac{1}{2} \}$                               |
| $c \quad (\frac{1}{2}, \frac{t}{2}, 0)$             | $c_1$<br>$c_2$<br>$c_3$<br>$c_4$ | $\{2_{010}   0 \ 0 \ \frac{1}{2} \}$<br>$-i$<br>$-i$<br>$i$<br>$i$                                                                                                           | $\{m_{100}   \frac{1}{2} \ 0 \ \frac{1}{2} \}$<br>$i$<br>$-i$<br>$i$<br>$-i$ |
| $d \quad (\frac{1-t}{2}, \frac{1}{2}, 0)$           | $d_1$                            | $\{2_{100}   \frac{1}{2} \ 0 \ \frac{1}{2} \}$                                                                                                                               | $\{m_{010}   0 \ 0 \ \frac{1}{2} \}$                                         |
| $e \quad (\frac{t}{2}, 0, \frac{1}{2})$             | $e_1$<br>$e_2$<br>$e_3$<br>$e_4$ | $\{2_{100}   \frac{1}{2} \ 0 \ \frac{1}{2} \}$<br>$-e^{-\frac{1}{2}i\pi(t+1)}$<br>$-e^{-\frac{1}{2}i\pi(t+1)}$<br>$e^{-\frac{1}{2}i\pi(t+1)}$<br>$e^{-\frac{1}{2}i\pi(t+1)}$ | $\{m_{010}   0 \ 0 \ \frac{1}{2} \}$<br>$-1$<br>$1$<br>$-1$<br>$1$           |
| $f \quad (0, \frac{t}{2}, \frac{1}{2})$             | $f_1$<br>$f_2$<br>$f_3$<br>$f_4$ | $\{2_{010}   0 \ 0 \ \frac{1}{2} \}$<br>$i$<br>$i$<br>$-i$<br>$-i$                                                                                                           | $\{m_{100}   \frac{1}{2} \ 0 \ \frac{1}{2} \}$<br>$-1$<br>$1$<br>$-1$<br>$1$ |
| $g \quad (\frac{1}{2}, \frac{t}{2}, \frac{1}{2})$   | $g_1$                            | $\{2_{010}   0 \ 0 \ \frac{1}{2} \}$                                                                                                                                         | $\{m_{100}   \frac{1}{2} \ 0 \ \frac{1}{2} \}$                               |
| $h \quad (\frac{1-t}{2}, \frac{1}{2}, \frac{1}{2})$ | $h_1$<br>$h_2$<br>$h_3$<br>$h_4$ | $\{2_{100}   \frac{1}{2} \ 0 \ \frac{1}{2} \}$<br>$-e^{-\frac{1}{2}i\pi(2-t)}$<br>$-e^{-\frac{1}{2}i\pi(2-t)}$<br>$e^{-\frac{1}{2}i\pi(2-t)}$<br>$e^{-\frac{1}{2}i\pi(2-t)}$ | $\{m_{010}   0 \ 0 \ \frac{1}{2} \}$<br>$-1$<br>$1$<br>$-1$<br>$1$           |
| $i \quad (0, 0, \frac{t}{2})$                       | $i_1$                            | $\{2_{001}   \frac{1}{2} \ 0 \ 0 \}$                                                                                                                                         | $\{m_{100}   \frac{1}{2} \ 0 \ \frac{1}{2} \}$                               |
| $j \quad (\frac{1}{2}, 0, \frac{t}{2})$             | $j_1$                            | $\{2_{001}   \frac{1}{2} \ 0 \ 0 \}$                                                                                                                                         | $\{m_{100}   \frac{1}{2} \ 0 \ \frac{1}{2} \}$                               |
| $k \quad (\frac{1}{2}, \frac{1}{2}, \frac{t}{2})$   | $k_1$                            | $\{2_{001}   \frac{1}{2} \ 0 \ 0 \}$                                                                                                                                         | $\{m_{100}   \frac{1}{2} \ 0 \ \frac{1}{2} \}$                               |
| $l \quad (0, \frac{1}{2}, \frac{t}{2})$             | $l_1$                            | $\{2_{001}   \frac{1}{2} \ 0 \ 0 \}$                                                                                                                                         | $\{m_{100}   \frac{1}{2} \ 0 \ \frac{1}{2} \}$                               |

$$\begin{aligned}
\mathcal{W}_1^{\text{gapless}} = & \sum_{m=1}^{n_{a_1}} \text{sgn}(v_m^{a_1}) \frac{1 - \text{sgn}(\delta_m^{a_1})}{2} - \sum_{m=1}^{n_{f_1}} \text{sgn}(v_m^{f_1}) \frac{1 - \text{sgn}(\delta_m^{f_1})}{2} - \sum_{m=1}^{n_{f_3}} \text{sgn}(v_m^{f_3}) \frac{1 - \text{sgn}(\delta_m^{f_3})}{2} \\
& + 2 \sum_{m=1}^{n_{g_1}} \text{sgn}(v_m^{g_1}) \frac{1 - \text{sgn}(\delta_m^{g_1})}{2} + \sum_{m=1}^{n_{h_1}} \text{sgn}(v_m^{h_1}) \frac{1 - \text{sgn}(\delta_m^{h_1})}{2} \\
& + \sum_{m=1}^{n_{h_3}} \text{sgn}(v_m^{h_3}) \frac{1 - \text{sgn}(\delta_m^{h_3})}{2} - \sum_{m=1}^{n_{i_1}} \text{sgn}(v_m^{i_1}) \frac{1 - \text{sgn}(\delta_m^{i_1})}{2} + 2 \sum_{m=1}^{n_{j_1}} \text{sgn}(v_m^{j_1}) \frac{1 - \text{sgn}(\delta_m^{j_1})}{2}
\end{aligned} \tag{S54.1}$$

$$\begin{aligned}
\mathcal{W}_2^{\text{gapless}} = & \sum_{m=1}^{n_{b_1}} \text{sgn}(v_m^{b_1}) \frac{1 - \text{sgn}(\delta_m^{b_1})}{2} - \sum_{m=1}^{n_{f_1}} \text{sgn}(v_m^{f_1}) \frac{1 - \text{sgn}(\delta_m^{f_1})}{2} - \sum_{m=1}^{n_{f_3}} \text{sgn}(v_m^{f_3}) \frac{1 - \text{sgn}(\delta_m^{f_3})}{2} \\
& - \sum_{m=1}^{n_{i_1}} \text{sgn}(v_m^{i_1}) \frac{1 - \text{sgn}(\delta_m^{i_1})}{2} + \sum_{m=1}^{n_{l_1}} \text{sgn}(v_m^{l_1}) \frac{1 - \text{sgn}(\delta_m^{l_1})}{2}
\end{aligned} \tag{S54.2}$$

$$\mathcal{W}_3^{\text{gapless}} = \sum_{m=1}^{n_{c_1}} \text{sgn}(v_m^{c_1}) \frac{1 - \text{sgn}(\delta_m^{c_1})}{2} - \sum_{m=1}^{n_{g_1}} \text{sgn}(v_m^{g_1}) \frac{1 - \text{sgn}(\delta_m^{g_1})}{2} - \sum_{m=1}^{n_{j_1}} \text{sgn}(v_m^{j_1}) \frac{1 - \text{sgn}(\delta_m^{j_1})}{2} + \sum_{m=1}^{n_{k_1}} \text{sgn}(v_m^{k_1}) \frac{1 - \text{sgn}(\delta_m^{k_1})}{2} \quad (\text{S54.3})$$

$$\mathcal{W}_4^{\text{gapless}} = \sum_{m=1}^{n_{c_2}} \text{sgn}(v_m^{c_2}) \frac{1 - \text{sgn}(\delta_m^{c_2})}{2} - \sum_{m=1}^{n_{g_1}} \text{sgn}(v_m^{g_1}) \frac{1 - \text{sgn}(\delta_m^{g_1})}{2} - \sum_{m=1}^{n_{j_1}} \text{sgn}(v_m^{j_1}) \frac{1 - \text{sgn}(\delta_m^{j_1})}{2} + \sum_{m=1}^{n_{k_1}} \text{sgn}(v_m^{k_1}) \frac{1 - \text{sgn}(\delta_m^{k_1})}{2} \quad (\text{S54.4})$$

$$\begin{aligned} \mathcal{W}_5^{\text{gapless}} = & \sum_{m=1}^{n_{d_1}} \text{sgn}(v_m^{d_1}) \frac{1 - \text{sgn}(\delta_m^{d_1})}{2} - \sum_{m=1}^{n_{h_1}} \text{sgn}(v_m^{h_1}) \frac{1 - \text{sgn}(\delta_m^{h_1})}{2} - \sum_{m=1}^{n_{h_3}} \text{sgn}(v_m^{h_3}) \frac{1 - \text{sgn}(\delta_m^{h_3})}{2} \\ & - 2 \sum_{m=1}^{n_{k_1}} \text{sgn}(v_m^{k_1}) \frac{1 - \text{sgn}(\delta_m^{k_1})}{2} + \sum_{m=1}^{n_{l_1}} \text{sgn}(v_m^{l_1}) \frac{1 - \text{sgn}(\delta_m^{l_1})}{2} \end{aligned} \quad (\text{S54.5})$$

$$\begin{aligned} \mathcal{W}_6^{\text{gapless}} = & \sum_{m=1}^{n_{e_1}} \text{sgn}(v_m^{e_1}) \frac{1 - \text{sgn}(\delta_m^{e_1})}{2} + \sum_{m=1}^{n_{e_3}} \text{sgn}(v_m^{e_3}) \frac{1 - \text{sgn}(\delta_m^{e_3})}{2} - \sum_{m=1}^{n_{f_1}} \text{sgn}(v_m^{f_1}) \frac{1 - \text{sgn}(\delta_m^{f_1})}{2} - \sum_{m=1}^{n_{f_3}} \text{sgn}(v_m^{f_3}) \frac{1 - \text{sgn}(\delta_m^{f_3})}{2} \\ & + 2 \sum_{m=1}^{n_{g_1}} \text{sgn}(v_m^{g_1}) \frac{1 - \text{sgn}(\delta_m^{g_1})}{2} + \sum_{m=1}^{n_{h_1}} \text{sgn}(v_m^{h_1}) \frac{1 - \text{sgn}(\delta_m^{h_1})}{2} + \sum_{m=1}^{n_{h_3}} \text{sgn}(v_m^{h_3}) \frac{1 - \text{sgn}(\delta_m^{h_3})}{2} \end{aligned} \quad (\text{S54.6})$$

$$\mathcal{W}_1^{\text{gapped}} = - \sum_{m=1}^{n_{f_1}} \text{sgn}(v_m^{f_1}) \frac{1 - \text{sgn}(\delta_m^{f_1})}{2} + \sum_{m=1}^{n_{f_3}} \text{sgn}(v_m^{f_3}) \frac{1 - \text{sgn}(\delta_m^{f_3})}{2} \quad (\text{S54.7})$$

$$\mathcal{X}_1 = \sum_{m=1}^{n_{e_3}} \frac{1 - \text{sgn}(\delta_m^{e_3})}{2} + \sum_{m=1}^{n_{f_1}} \frac{1 - \text{sgn}(\delta_m^{f_1})}{2} + \sum_{m=1}^{n_{h_1}} \frac{1 - \text{sgn}(\delta_m^{h_1})}{2} \quad \text{mod } 2 \quad (\text{S54.8})$$

$$\mathcal{X}_2 = \sum_{m=1}^{n_{e_3}} \frac{1 - \text{sgn}(\delta_m^{e_3})}{2} + \sum_{m=1}^{n_{f_1}} \frac{1 - \text{sgn}(\delta_m^{f_1})}{2} + \sum_{m=1}^{n_{h_3}} \frac{1 - \text{sgn}(\delta_m^{h_3})}{2} \quad \text{mod } 2 \quad (\text{S54.9})$$

### S55. SPACE GROUP NO. 55

| line segment                              | character of irrep (generators only)                                                                                                                                                                                              |
|-------------------------------------------|-----------------------------------------------------------------------------------------------------------------------------------------------------------------------------------------------------------------------------------|
| $a \quad (\frac{t}{2}, 0, 0)$             | $a_1 \quad \left\{ 2_{100} \middle  \begin{smallmatrix} \frac{1}{2} & \frac{1}{2} & 0 \\ 0 \end{smallmatrix} \right\} \left\{ m_{010} \middle  \begin{smallmatrix} \frac{1}{2} & \frac{1}{2} & 0 \\ 0 \end{smallmatrix} \right\}$ |
| $b \quad (0, \frac{t}{2}, 0)$             | $b_1 \quad \left\{ 2_{010} \middle  \begin{smallmatrix} \frac{1}{2} & \frac{1}{2} & 0 \\ 0 \end{smallmatrix} \right\} \left\{ m_{100} \middle  \begin{smallmatrix} \frac{1}{2} & \frac{1}{2} & 0 \\ 0 \end{smallmatrix} \right\}$ |
| $c \quad (\frac{1}{2}, \frac{t}{2}, 0)$   | $c_1 \quad \left\{ 2_{010} \middle  \begin{smallmatrix} \frac{1}{2} & \frac{1}{2} & 0 \\ 0 \end{smallmatrix} \right\} \left\{ m_{100} \middle  \begin{smallmatrix} \frac{1}{2} & \frac{1}{2} & 0 \\ 0 \end{smallmatrix} \right\}$ |
| $d \quad (\frac{1-t}{2}, \frac{1}{2}, 0)$ | $d_1 \quad \left\{ 2_{100} \middle  \begin{smallmatrix} \frac{1}{2} & \frac{1}{2} & 0 \\ 0 \end{smallmatrix} \right\} \left\{ m_{010} \middle  \begin{smallmatrix} \frac{1}{2} & \frac{1}{2} & 0 \\ 0 \end{smallmatrix} \right\}$ |
| $e \quad (\frac{t}{2}, 0, \frac{1}{2})$   | $e_1 \quad \left\{ 2_{100} \middle  \begin{smallmatrix} \frac{1}{2} & \frac{1}{2} & 0 \\ 0 \end{smallmatrix} \right\} \left\{ m_{010} \middle  \begin{smallmatrix} \frac{1}{2} & \frac{1}{2} & 0 \\ 0 \end{smallmatrix} \right\}$ |

|                                                 |                                                                                                                                             |
|-------------------------------------------------|---------------------------------------------------------------------------------------------------------------------------------------------|
| $f$ $(0, \frac{t}{2}, \frac{1}{2})$             | $f_1$ $\{2_{010}   \frac{1}{2} \frac{1}{2} 0\} \{m_{100}   \frac{1}{2} \frac{1}{2} 0\}$                                                     |
| $g$ $(\frac{1}{2}, \frac{t}{2}, \frac{1}{2})$   | $g_1$ $\{2_{010}   \frac{1}{2} \frac{1}{2} 0\} \{m_{100}   \frac{1}{2} \frac{1}{2} 0\}$                                                     |
| $h$ $(\frac{1-t}{2}, \frac{1}{2}, \frac{1}{2})$ | $h_1$ $\{2_{100}   \frac{1}{2} \frac{1}{2} 0\} \{m_{010}   \frac{1}{2} \frac{1}{2} 0\}$                                                     |
| $i$ $(0, 0, \frac{t}{2})$                       | $i_1$ $\{2_{001}   0 0 0\} \{m_{100}   \frac{1}{2} \frac{1}{2} 0\}$                                                                         |
| $j$ $(\frac{1}{2}, 0, \frac{t}{2})$             | $j_1$ $\{2_{001}   0 0 0\} \{m_{100}   \frac{1}{2} \frac{1}{2} 0\}$<br>$j_2$ $-i$ $i$<br>$j_3$ $-i$ $-i$<br>$j_4$ $i$ $i$<br>$j_5$ $i$ $-i$ |
| $k$ $(\frac{1}{2}, \frac{1}{2}, \frac{t}{2})$   | $k_1$ $\{2_{001}   0 0 0\} \{m_{100}   \frac{1}{2} \frac{1}{2} 0\}$                                                                         |
| $l$ $(0, \frac{1}{2}, \frac{t}{2})$             | $l_1$ $\{2_{001}   0 0 0\} \{m_{100}   \frac{1}{2} \frac{1}{2} 0\}$<br>$l_2$ $-i$ $-1$<br>$l_3$ $-i$ $1$<br>$l_4$ $i$ $-1$<br>$l_5$ $i$ $1$ |

$$\begin{aligned} \mathcal{W}_1^{\text{gapless}} = & \sum_{m=1}^{n_{a_1}} \text{sgn}(v_m^{a_1}) \frac{1 - \text{sgn}(\delta_m^{a_1})}{2} - \sum_{m=1}^{n_{f_1}} \text{sgn}(v_m^{f_1}) \frac{1 - \text{sgn}(\delta_m^{f_1})}{2} + 2 \sum_{m=1}^{n_{g_1}} \text{sgn}(v_m^{g_1}) \frac{1 - \text{sgn}(\delta_m^{g_1})}{2} \\ & + 2 \sum_{m=1}^{n_{h_1}} \text{sgn}(v_m^{h_1}) \frac{1 - \text{sgn}(\delta_m^{h_1})}{2} - \sum_{m=1}^{n_{i_1}} \text{sgn}(v_m^{i_1}) \frac{1 - \text{sgn}(\delta_m^{i_1})}{2} + 2 \sum_{m=1}^{n_{j_2}} \text{sgn}(v_m^{j_2}) \frac{1 - \text{sgn}(\delta_m^{j_2})}{2} \end{aligned} \quad (\text{S55.1})$$

$$\mathcal{W}_2^{\text{gapless}} = \sum_{m=1}^{n_{b_1}} \text{sgn}(v_m^{b_1}) \frac{1 - \text{sgn}(\delta_m^{b_1})}{2} - \sum_{m=1}^{n_{f_1}} \text{sgn}(v_m^{f_1}) \frac{1 - \text{sgn}(\delta_m^{f_1})}{2} - \sum_{m=1}^{n_{i_1}} \text{sgn}(v_m^{i_1}) \frac{1 - \text{sgn}(\delta_m^{i_1})}{2} + 2 \sum_{m=1}^{n_{l_2}} \text{sgn}(v_m^{l_2}) \frac{1 - \text{sgn}(\delta_m^{l_2})}{2} \quad (\text{S55.2})$$

$$\mathcal{W}_3^{\text{gapless}} = \sum_{m=1}^{n_{c_1}} \text{sgn}(v_m^{c_1}) \frac{1 - \text{sgn}(\delta_m^{c_1})}{2} - \sum_{m=1}^{n_{g_1}} \text{sgn}(v_m^{g_1}) \frac{1 - \text{sgn}(\delta_m^{g_1})}{2} - \sum_{m=1}^{n_{j_2}} \text{sgn}(v_m^{j_2}) \frac{1 - \text{sgn}(\delta_m^{j_2})}{2} + \sum_{m=1}^{n_{k_1}} \text{sgn}(v_m^{k_1}) \frac{1 - \text{sgn}(\delta_m^{k_1})}{2} \quad (\text{S55.3})$$

$$\mathcal{W}_4^{\text{gapless}} = \sum_{m=1}^{n_{d_1}} \text{sgn}(v_m^{d_1}) \frac{1 - \text{sgn}(\delta_m^{d_1})}{2} - \sum_{m=1}^{n_{h_1}} \text{sgn}(v_m^{h_1}) \frac{1 - \text{sgn}(\delta_m^{h_1})}{2} - \sum_{m=1}^{n_{k_1}} \text{sgn}(v_m^{k_1}) \frac{1 - \text{sgn}(\delta_m^{k_1})}{2} + \sum_{m=1}^{n_{l_2}} \text{sgn}(v_m^{l_2}) \frac{1 - \text{sgn}(\delta_m^{l_2})}{2} \quad (\text{S55.4})$$

$$\begin{aligned} \mathcal{W}_5^{\text{gapless}} = & \sum_{m=1}^{n_{e_1}} \text{sgn}(v_m^{e_1}) \frac{1 - \text{sgn}(\delta_m^{e_1})}{2} - \sum_{m=1}^{n_{f_1}} \text{sgn}(v_m^{f_1}) \frac{1 - \text{sgn}(\delta_m^{f_1})}{2} + 2 \sum_{m=1}^{n_{g_1}} \text{sgn}(v_m^{g_1}) \frac{1 - \text{sgn}(\delta_m^{g_1})}{2} \\ & + 2 \sum_{m=1}^{n_{h_1}} \text{sgn}(v_m^{h_1}) \frac{1 - \text{sgn}(\delta_m^{h_1})}{2} \end{aligned} \quad (\text{S55.5})$$

$$\mathcal{W}_6^{\text{gapless}} = \sum_{m=1}^{n_{j_1}} \text{sgn}(v_m^{j_1}) \frac{1 - \text{sgn}(\delta_m^{j_1})}{2} - \sum_{m=1}^{n_{j_2}} \text{sgn}(v_m^{j_2}) \frac{1 - \text{sgn}(\delta_m^{j_2})}{2} \quad (\text{S55.6})$$



$$\mathcal{W}_7^{\text{gapless}} = \sum_{m=1}^{n_{l_1}} \text{sgn}(v_m^{l_1}) \frac{1 - \text{sgn}(\delta_m^{l_1})}{2} - \sum_{m=1}^{n_{l_2}} \text{sgn}(v_m^{l_2}) \frac{1 - \text{sgn}(\delta_m^{l_2})}{2} \quad (\text{S55.7})$$

**S56. SPACE GROUP NO. 56**

| line segment                                        | character of irrep (generators only)                                                                                                                                                                                                                                                        |
|-----------------------------------------------------|---------------------------------------------------------------------------------------------------------------------------------------------------------------------------------------------------------------------------------------------------------------------------------------------|
| $a \quad (\frac{t}{2}, 0, 0)$                       | $a_1 \quad \begin{matrix} \{2_{100}   \frac{1}{2} & 0 & \frac{1}{2}\} & \{m_{010}   0 & \frac{1}{2} & \frac{1}{2}\} \\ 0 & 0 \end{matrix}$                                                                                                                                                  |
| $b \quad (0, \frac{t}{2}, 0)$                       | $b_1 \quad \begin{matrix} \{2_{010}   0 & \frac{1}{2} & \frac{1}{2}\} & \{m_{100}   \frac{1}{2} & 0 & \frac{1}{2}\} \\ 0 & 0 \end{matrix}$                                                                                                                                                  |
| $c \quad (\frac{1}{2}, \frac{t}{2}, 0)$             | $\begin{matrix} \{2_{010}   0 & \frac{1}{2} & \frac{1}{2}\} & \{m_{100}   \frac{1}{2} & 0 & \frac{1}{2}\} \\ c_1 & -ie^{-\frac{1}{2}i\pi t} & i \\ c_2 & -ie^{-\frac{1}{2}i\pi t} & -i \\ c_3 & ie^{-\frac{1}{2}i\pi t} & i \\ c_4 & ie^{-\frac{1}{2}i\pi t} & -i \end{matrix}$             |
| $d \quad (\frac{1-t}{2}, \frac{1}{2}, 0)$           | $\begin{matrix} \{2_{100}   \frac{1}{2} & 0 & \frac{1}{2}\} & \{m_{010}   0 & \frac{1}{2} & \frac{1}{2}\} \\ d_1 & -ie^{-\frac{1}{2}i\pi(1-t)} & i \\ d_2 & -ie^{-\frac{1}{2}i\pi(1-t)} & -i \\ d_3 & ie^{-\frac{1}{2}i\pi(1-t)} & i \\ d_4 & ie^{-\frac{1}{2}i\pi(1-t)} & -i \end{matrix}$ |
| $e \quad (\frac{t}{2}, 0, \frac{1}{2})$             | $\begin{matrix} \{2_{100}   \frac{1}{2} & 0 & \frac{1}{2}\} & \{m_{010}   0 & \frac{1}{2} & \frac{1}{2}\} \\ e_1 & -e^{-\frac{1}{2}i\pi(t+1)} & -1 \\ e_2 & -e^{-\frac{1}{2}i\pi(t+1)} & 1 \\ e_3 & e^{-\frac{1}{2}i\pi(t+1)} & -1 \\ e_4 & e^{-\frac{1}{2}i\pi(t+1)} & 1 \end{matrix}$     |
| $f \quad (0, \frac{t}{2}, \frac{1}{2})$             | $\begin{matrix} \{2_{010}   0 & \frac{1}{2} & \frac{1}{2}\} & \{m_{100}   \frac{1}{2} & 0 & \frac{1}{2}\} \\ f_1 & -e^{-\frac{1}{2}i\pi(t+1)} & -1 \\ f_2 & -e^{-\frac{1}{2}i\pi(t+1)} & 1 \\ f_3 & e^{-\frac{1}{2}i\pi(t+1)} & -1 \\ f_4 & e^{-\frac{1}{2}i\pi(t+1)} & 1 \end{matrix}$     |
| $g \quad (\frac{1}{2}, \frac{t}{2}, \frac{1}{2})$   | $g_1 \quad \begin{matrix} \{2_{010}   0 & \frac{1}{2} & \frac{1}{2}\} & \{m_{100}   \frac{1}{2} & 0 & \frac{1}{2}\} \\ 0 & 0 \end{matrix}$                                                                                                                                                  |
| $h \quad (\frac{1-t}{2}, \frac{1}{2}, \frac{1}{2})$ | $h_1 \quad \begin{matrix} \{2_{100}   \frac{1}{2} & 0 & \frac{1}{2}\} & \{m_{010}   0 & \frac{1}{2} & \frac{1}{2}\} \\ 0 & 0 \end{matrix}$                                                                                                                                                  |
| $i \quad (0, 0, \frac{t}{2})$                       | $i_1 \quad \begin{matrix} \{2_{001}   \frac{1}{2} & \frac{1}{2} & 0\} & \{m_{100}   \frac{1}{2} & 0 & \frac{1}{2}\} \\ 0 & 0 \end{matrix}$                                                                                                                                                  |
| $j \quad (\frac{1}{2}, 0, \frac{t}{2})$             | $j_1 \quad \begin{matrix} \{2_{001}   \frac{1}{2} & \frac{1}{2} & 0\} & \{m_{100}   \frac{1}{2} & 0 & \frac{1}{2}\} \\ 0 & 0 \end{matrix}$                                                                                                                                                  |
| $k \quad (\frac{1}{2}, \frac{1}{2}, \frac{t}{2})$   | $k_1 \quad \begin{matrix} \{2_{001}   \frac{1}{2} & \frac{1}{2} & 0\} & \{m_{100}   \frac{1}{2} & 0 & \frac{1}{2}\} \\ 0 & 0 \end{matrix}$                                                                                                                                                  |
| $l \quad (0, \frac{1}{2}, \frac{t}{2})$             | $l_1 \quad \begin{matrix} \{2_{001}   \frac{1}{2} & \frac{1}{2} & 0\} & \{m_{100}   \frac{1}{2} & 0 & \frac{1}{2}\} \\ 0 & 0 \end{matrix}$                                                                                                                                                  |

$$\begin{aligned} \mathcal{W}_1^{\text{gapless}} = & \sum_{m=1}^{n_{a_1}} \text{sgn}(v_m^{a_1}) \frac{1 - \text{sgn}(\delta_m^{a_1})}{2} - \sum_{m=1}^{n_{f_1}} \text{sgn}(v_m^{f_1}) \frac{1 - \text{sgn}(\delta_m^{f_1})}{2} - \sum_{m=1}^{n_{f_3}} \text{sgn}(v_m^{f_3}) \frac{1 - \text{sgn}(\delta_m^{f_3})}{2} \\ & + 2 \sum_{m=1}^{n_{g_1}} \text{sgn}(v_m^{g_1}) \frac{1 - \text{sgn}(\delta_m^{g_1})}{2} + 2 \sum_{m=1}^{n_{h_1}} \text{sgn}(v_m^{h_1}) \frac{1 - \text{sgn}(\delta_m^{h_1})}{2} - \sum_{m=1}^{n_{i_1}} \text{sgn}(v_m^{i_1}) \frac{1 - \text{sgn}(\delta_m^{i_1})}{2} \\ & + 2 \sum_{m=1}^{n_{j_1}} \text{sgn}(v_m^{j_1}) \frac{1 - \text{sgn}(\delta_m^{j_1})}{2} \end{aligned} \quad (\text{S56.1})$$

$$\begin{aligned} \mathcal{W}_2^{\text{gapless}} = & \sum_{m=1}^{n_{b_1}} \text{sgn}(v_m^{b_1}) \frac{1 - \text{sgn}(\delta_m^{b_1})}{2} - \sum_{m=1}^{n_{f_1}} \text{sgn}(v_m^{f_1}) \frac{1 - \text{sgn}(\delta_m^{f_1})}{2} - \sum_{m=1}^{n_{f_3}} \text{sgn}(v_m^{f_3}) \frac{1 - \text{sgn}(\delta_m^{f_3})}{2} \\ & - \sum_{m=1}^{n_{i_1}} \text{sgn}(v_m^{i_1}) \frac{1 - \text{sgn}(\delta_m^{i_1})}{2} + 2 \sum_{m=1}^{n_{l_1}} \text{sgn}(v_m^{l_1}) \frac{1 - \text{sgn}(\delta_m^{l_1})}{2} \end{aligned} \quad (\text{S56.2})$$

$$\mathcal{W}_3^{\text{gapless}} = \sum_{m=1}^{n_{c_1}} \text{sgn}(v_m^{c_1}) \frac{1 - \text{sgn}(\delta_m^{c_1})}{2} - \sum_{m=1}^{n_{g_1}} \text{sgn}(v_m^{g_1}) \frac{1 - \text{sgn}(\delta_m^{g_1})}{2} - \sum_{m=1}^{n_{j_1}} \text{sgn}(v_m^{j_1}) \frac{1 - \text{sgn}(\delta_m^{j_1})}{2} + \sum_{m=1}^{n_{k_1}} \text{sgn}(v_m^{k_1}) \frac{1 - \text{sgn}(\delta_m^{k_1})}{2} \quad (\text{S56.3})$$

$$\mathcal{W}_4^{\text{gapless}} = \sum_{m=1}^{n_{c_2}} \text{sgn}(v_m^{c_2}) \frac{1 - \text{sgn}(\delta_m^{c_2})}{2} - \sum_{m=1}^{n_{g_1}} \text{sgn}(v_m^{g_1}) \frac{1 - \text{sgn}(\delta_m^{g_1})}{2} - \sum_{m=1}^{n_{j_1}} \text{sgn}(v_m^{j_1}) \frac{1 - \text{sgn}(\delta_m^{j_1})}{2} + \sum_{m=1}^{n_{k_1}} \text{sgn}(v_m^{k_1}) \frac{1 - \text{sgn}(\delta_m^{k_1})}{2} \quad (\text{S56.4})$$

$$\mathcal{W}_5^{\text{gapless}} = \sum_{m=1}^{n_{d_1}} \text{sgn}(v_m^{d_1}) \frac{1 - \text{sgn}(\delta_m^{d_1})}{2} - \sum_{m=1}^{n_{h_1}} \text{sgn}(v_m^{h_1}) \frac{1 - \text{sgn}(\delta_m^{h_1})}{2} - \sum_{m=1}^{n_{k_1}} \text{sgn}(v_m^{k_1}) \frac{1 - \text{sgn}(\delta_m^{k_1})}{2} + \sum_{m=1}^{n_{l_1}} \text{sgn}(v_m^{l_1}) \frac{1 - \text{sgn}(\delta_m^{l_1})}{2} \quad (\text{S56.5})$$

$$\mathcal{W}_6^{\text{gapless}} = \sum_{m=1}^{n_{d_2}} \text{sgn}(v_m^{d_2}) \frac{1 - \text{sgn}(\delta_m^{d_2})}{2} - \sum_{m=1}^{n_{h_1}} \text{sgn}(v_m^{h_1}) \frac{1 - \text{sgn}(\delta_m^{h_1})}{2} - \sum_{m=1}^{n_{k_1}} \text{sgn}(v_m^{k_1}) \frac{1 - \text{sgn}(\delta_m^{k_1})}{2} + \sum_{m=1}^{n_{l_1}} \text{sgn}(v_m^{l_1}) \frac{1 - \text{sgn}(\delta_m^{l_1})}{2} \quad (\text{S56.6})$$

$$\begin{aligned} \mathcal{W}_7^{\text{gapless}} = & \sum_{m=1}^{n_{e_1}} \text{sgn}(v_m^{e_1}) \frac{1 - \text{sgn}(\delta_m^{e_1})}{2} + \sum_{m=1}^{n_{e_3}} \text{sgn}(v_m^{e_3}) \frac{1 - \text{sgn}(\delta_m^{e_3})}{2} - \sum_{m=1}^{n_{f_1}} \text{sgn}(v_m^{f_1}) \frac{1 - \text{sgn}(\delta_m^{f_1})}{2} \\ & - \sum_{m=1}^{n_{f_3}} \text{sgn}(v_m^{f_3}) \frac{1 - \text{sgn}(\delta_m^{f_3})}{2} + 2 \sum_{m=1}^{n_{g_1}} \text{sgn}(v_m^{g_1}) \frac{1 - \text{sgn}(\delta_m^{g_1})}{2} + 2 \sum_{m=1}^{n_{h_1}} \text{sgn}(v_m^{h_1}) \frac{1 - \text{sgn}(\delta_m^{h_1})}{2} \end{aligned} \quad (\text{S56.7})$$

$$\mathcal{X}_1 = \sum_{m=1}^{n_{e_3}} \frac{1 - \text{sgn}(\delta_m^{e_3})}{2} + \sum_{m=1}^{n_{f_3}} \frac{1 - \text{sgn}(\delta_m^{f_3})}{2} \quad \text{mod } 2 \quad (\text{S56.8})$$

$$\mathcal{X}_2 = \sum_{m=1}^{n_{e_3}} \frac{1 - \text{sgn}(\delta_m^{e_3})}{2} + \sum_{m=1}^{n_{f_1}} \frac{1 - \text{sgn}(\delta_m^{f_1})}{2} \quad \text{mod } 2 \quad (\text{S56.9})$$

### S57. SPACE GROUP NO. 57

| line segment | character of irrep (generators only) |
|--------------|--------------------------------------|
|--------------|--------------------------------------|

|                                                     |                                  |                                                                                                                                                                   |                                                                                     |
|-----------------------------------------------------|----------------------------------|-------------------------------------------------------------------------------------------------------------------------------------------------------------------|-------------------------------------------------------------------------------------|
| $a \quad (\frac{t}{2}, 0, 0)$                       | $a_1$                            | $\{2_{100}  0 \quad \frac{1}{2} \quad 0 \}$                                                                                                                       | $\{m_{010}  0 \quad \frac{1}{2} \quad \frac{1}{2} \}$                               |
| $b \quad (0, \frac{t}{2}, 0)$                       | $b_1$                            | $\{2_{010}  0 \quad \frac{1}{2} \quad \frac{1}{2} \}$                                                                                                             | $\{m_{100}  0 \quad \frac{1}{2} \quad 0 \}$                                         |
| $c \quad (\frac{1}{2}, \frac{t}{2}, 0)$             | $c_1$                            | $\{2_{010}  0 \quad \frac{1}{2} \quad \frac{1}{2} \}$                                                                                                             | $\{m_{100}  0 \quad \frac{1}{2} \quad 0 \}$                                         |
| $d \quad (\frac{1-t}{2}, \frac{1}{2}, 0)$           | $d_1$                            | $\{2_{100}  0 \quad \frac{1}{2} \quad 0 \}$                                                                                                                       | $\{m_{010}  0 \quad \frac{1}{2} \quad \frac{1}{2} \}$                               |
| $e \quad (\frac{t}{2}, 0, \frac{1}{2})$             | $e_1$<br>$e_2$<br>$e_3$<br>$e_4$ | $\{2_{100}  0 \quad \frac{1}{2} \quad 0 \}$<br>$-i$<br>$-i$<br>$i$<br>$i$                                                                                         | $\{m_{010}  0 \quad \frac{1}{2} \quad \frac{1}{2} \}$<br>$-1$<br>$1$<br>$-1$<br>$1$ |
| $f \quad (0, \frac{t}{2}, \frac{1}{2})$             | $f_1$                            | $\{2_{010}  0 \quad \frac{1}{2} \quad \frac{1}{2} \}$                                                                                                             | $\{m_{100}  0 \quad \frac{1}{2} \quad 0 \}$                                         |
| $g \quad (\frac{1}{2}, \frac{t}{2}, \frac{1}{2})$   | $g_1$                            | $\{2_{010}  0 \quad \frac{1}{2} \quad \frac{1}{2} \}$                                                                                                             | $\{m_{100}  0 \quad \frac{1}{2} \quad 0 \}$                                         |
| $h \quad (\frac{1-t}{2}, \frac{1}{2}, \frac{1}{2})$ | $h_1$<br>$h_2$<br>$h_3$<br>$h_4$ | $\{2_{100}  0 \quad \frac{1}{2} \quad 0 \}$<br>$i$<br>$i$<br>$-i$<br>$-i$                                                                                         | $\{m_{010}  0 \quad \frac{1}{2} \quad \frac{1}{2} \}$<br>$1$<br>$-1$<br>$1$<br>$-1$ |
| $i \quad (0, 0, \frac{t}{2})$                       | $i_1$                            | $\{2_{001}  0 \quad 0 \quad \frac{1}{2} \}$                                                                                                                       | $\{m_{100}  0 \quad \frac{1}{2} \quad 0 \}$                                         |
| $j \quad (\frac{1}{2}, 0, \frac{t}{2})$             | $j_1$                            | $\{2_{001}  0 \quad 0 \quad \frac{1}{2} \}$                                                                                                                       | $\{m_{100}  0 \quad \frac{1}{2} \quad 0 \}$                                         |
| $k \quad (\frac{1}{2}, \frac{1}{2}, \frac{t}{2})$   | $k_1$<br>$k_2$<br>$k_3$<br>$k_4$ | $\{2_{001}  0 \quad 0 \quad \frac{1}{2} \}$<br>$-ie^{-\frac{1}{2}i\pi t}$<br>$-ie^{-\frac{1}{2}i\pi t}$<br>$ie^{-\frac{1}{2}i\pi t}$<br>$ie^{-\frac{1}{2}i\pi t}$ | $\{m_{100}  0 \quad \frac{1}{2} \quad 0 \}$<br>$-1$<br>$1$<br>$-1$<br>$1$           |
| $l \quad (0, \frac{1}{2}, \frac{t}{2})$             | $l_1$<br>$l_2$<br>$l_3$<br>$l_4$ | $\{2_{001}  0 \quad 0 \quad \frac{1}{2} \}$<br>$-ie^{-\frac{1}{2}i\pi t}$<br>$-ie^{-\frac{1}{2}i\pi t}$<br>$ie^{-\frac{1}{2}i\pi t}$<br>$ie^{-\frac{1}{2}i\pi t}$ | $\{m_{100}  0 \quad \frac{1}{2} \quad 0 \}$<br>$-1$<br>$1$<br>$-1$<br>$1$           |

$$\begin{aligned}
\mathcal{W}_1^{\text{gapless}} = & \sum_{m=1}^{n_{a_1}} \text{sgn}(v_m^{a_1}) \frac{1 - \text{sgn}(\delta_m^{a_1})}{2} - 2 \sum_{m=1}^{n_{f_1}} \text{sgn}(v_m^{f_1}) \frac{1 - \text{sgn}(\delta_m^{f_1})}{2} + 2 \sum_{m=1}^{n_{g_1}} \text{sgn}(v_m^{g_1}) \frac{1 - \text{sgn}(\delta_m^{g_1})}{2} \\
& + 2 \sum_{m=1}^{n_{h_2}} \text{sgn}(v_m^{h_2}) \frac{1 - \text{sgn}(\delta_m^{h_2})}{2} + 2 \sum_{m=1}^{n_{h_4}} \text{sgn}(v_m^{h_4}) \frac{1 - \text{sgn}(\delta_m^{h_4})}{2} \\
& - \sum_{m=1}^{n_{i_1}} \text{sgn}(v_m^{i_1}) \frac{1 - \text{sgn}(\delta_m^{i_1})}{2} + \sum_{m=1}^{n_{j_1}} \text{sgn}(v_m^{j_1}) \frac{1 - \text{sgn}(\delta_m^{j_1})}{2} + \sum_{m=1}^{n_{k_1}} \text{sgn}(v_m^{k_1}) \frac{1 - \text{sgn}(\delta_m^{k_1})}{2} \\
& - \sum_{m=1}^{n_{k_2}} \text{sgn}(v_m^{k_2}) \frac{1 - \text{sgn}(\delta_m^{k_2})}{2} - \sum_{m=1}^{n_{l_1}} \text{sgn}(v_m^{l_1}) \frac{1 - \text{sgn}(\delta_m^{l_1})}{2} + \sum_{m=1}^{n_{l_2}} \text{sgn}(v_m^{l_2}) \frac{1 - \text{sgn}(\delta_m^{l_2})}{2}
\end{aligned} \tag{S57.1}$$

$$\begin{aligned}
\mathcal{W}_2^{\text{gapless}} = & \sum_{m=1}^{n_{b_1}} \text{sgn}(v_m^{b_1}) \frac{1 - \text{sgn}(\delta_m^{b_1})}{2} - 2 \sum_{m=1}^{n_{f_1}} \text{sgn}(v_m^{f_1}) \frac{1 - \text{sgn}(\delta_m^{f_1})}{2} - \sum_{m=1}^{n_{i_1}} \text{sgn}(v_m^{i_1}) \frac{1 - \text{sgn}(\delta_m^{i_1})}{2} \\
& + \sum_{m=1}^{n_{l_1}} \text{sgn}(v_m^{l_1}) \frac{1 - \text{sgn}(\delta_m^{l_1})}{2} + \sum_{m=1}^{n_{l_2}} \text{sgn}(v_m^{l_2}) \frac{1 - \text{sgn}(\delta_m^{l_2})}{2}
\end{aligned} \tag{S57.2}$$

$$\begin{aligned}\mathcal{W}_3^{\text{gapless}} = & \sum_{m=1}^{n_{c_1}} \text{sgn}(v_m^{c_1}) \frac{1 - \text{sgn}(\delta_m^{c_1})}{2} - 2 \sum_{m=1}^{n_{g_1}} \text{sgn}(v_m^{g_1}) \frac{1 - \text{sgn}(\delta_m^{g_1})}{2} - \sum_{m=1}^{n_{j_1}} \text{sgn}(v_m^{j_1}) \frac{1 - \text{sgn}(\delta_m^{j_1})}{2} \\ & + \sum_{m=1}^{n_{k_1}} \text{sgn}(v_m^{k_1}) \frac{1 - \text{sgn}(\delta_m^{k_1})}{2} + \sum_{m=1}^{n_{k_2}} \text{sgn}(v_m^{k_2}) \frac{1 - \text{sgn}(\delta_m^{k_2})}{2}\end{aligned}\quad (\text{S57.3})$$

$$\begin{aligned}\mathcal{W}_4^{\text{gapless}} = & \sum_{m=1}^{n_{d_1}} \text{sgn}(v_m^{d_1}) \frac{1 - \text{sgn}(\delta_m^{d_1})}{2} - \sum_{m=1}^{n_{h_2}} \text{sgn}(v_m^{h_2}) \frac{1 - \text{sgn}(\delta_m^{h_2})}{2} - \sum_{m=1}^{n_{h_4}} \text{sgn}(v_m^{h_4}) \frac{1 - \text{sgn}(\delta_m^{h_4})}{2} \\ & - \sum_{m=1}^{n_{k_1}} \text{sgn}(v_m^{k_1}) \frac{1 - \text{sgn}(\delta_m^{k_1})}{2} + \sum_{m=1}^{n_{l_1}} \text{sgn}(v_m^{l_1}) \frac{1 - \text{sgn}(\delta_m^{l_1})}{2}\end{aligned}\quad (\text{S57.4})$$

$$\begin{aligned}\mathcal{W}_5^{\text{gapless}} = & \sum_{m=1}^{n_{e_1}} \text{sgn}(v_m^{e_1}) \frac{1 - \text{sgn}(\delta_m^{e_1})}{2} - \sum_{m=1}^{n_{f_1}} \text{sgn}(v_m^{f_1}) \frac{1 - \text{sgn}(\delta_m^{f_1})}{2} + \sum_{m=1}^{n_{g_1}} \text{sgn}(v_m^{g_1}) \frac{1 - \text{sgn}(\delta_m^{g_1})}{2} + \sum_{m=1}^{n_{h_2}} \text{sgn}(v_m^{h_2}) \frac{1 - \text{sgn}(\delta_m^{h_2})}{2} \\ & - \sum_{m=1}^{n_{h_3}} \text{sgn}(v_m^{h_3}) \frac{1 - \text{sgn}(\delta_m^{h_3})}{2} + 2 \sum_{m=1}^{n_{h_4}} \text{sgn}(v_m^{h_4}) \frac{1 - \text{sgn}(\delta_m^{h_4})}{2} + \sum_{m=1}^{n_{k_1}} \text{sgn}(v_m^{k_1}) \frac{1 - \text{sgn}(\delta_m^{k_1})}{2} \\ & - \sum_{m=1}^{n_{k_2}} \text{sgn}(v_m^{k_2}) \frac{1 - \text{sgn}(\delta_m^{k_2})}{2} - \sum_{m=1}^{n_{l_1}} \text{sgn}(v_m^{l_1}) \frac{1 - \text{sgn}(\delta_m^{l_1})}{2} + \sum_{m=1}^{n_{l_2}} \text{sgn}(v_m^{l_2}) \frac{1 - \text{sgn}(\delta_m^{l_2})}{2}\end{aligned}\quad (\text{S57.5})$$

$$\begin{aligned}\mathcal{W}_6^{\text{gapless}} = & \sum_{m=1}^{n_{e_2}} \text{sgn}(v_m^{e_2}) \frac{1 - \text{sgn}(\delta_m^{e_2})}{2} - \sum_{m=1}^{n_{f_1}} \text{sgn}(v_m^{f_1}) \frac{1 - \text{sgn}(\delta_m^{f_1})}{2} + \sum_{m=1}^{n_{g_1}} \text{sgn}(v_m^{g_1}) \frac{1 - \text{sgn}(\delta_m^{g_1})}{2} \\ & + \sum_{m=1}^{n_{h_2}} \text{sgn}(v_m^{h_2}) \frac{1 - \text{sgn}(\delta_m^{h_2})}{2} + \sum_{m=1}^{n_{h_3}} \text{sgn}(v_m^{h_3}) \frac{1 - \text{sgn}(\delta_m^{h_3})}{2}\end{aligned}\quad (\text{S57.6})$$

$$\begin{aligned}\mathcal{W}_7^{\text{gapless}} = & \sum_{m=1}^{n_{h_1}} \text{sgn}(v_m^{h_1}) \frac{1 - \text{sgn}(\delta_m^{h_1})}{2} - \sum_{m=1}^{n_{h_2}} \text{sgn}(v_m^{h_2}) \frac{1 - \text{sgn}(\delta_m^{h_2})}{2} + \sum_{m=1}^{n_{h_3}} \text{sgn}(v_m^{h_3}) \frac{1 - \text{sgn}(\delta_m^{h_3})}{2} \\ & - \sum_{m=1}^{n_{h_4}} \text{sgn}(v_m^{h_4}) \frac{1 - \text{sgn}(\delta_m^{h_4})}{2} - \sum_{m=1}^{n_{k_1}} \text{sgn}(v_m^{k_1}) \frac{1 - \text{sgn}(\delta_m^{k_1})}{2} \\ & + \sum_{m=1}^{n_{k_2}} \text{sgn}(v_m^{k_2}) \frac{1 - \text{sgn}(\delta_m^{k_2})}{2} + \sum_{m=1}^{n_{l_1}} \text{sgn}(v_m^{l_1}) \frac{1 - \text{sgn}(\delta_m^{l_1})}{2} - \sum_{m=1}^{n_{l_2}} \text{sgn}(v_m^{l_2}) \frac{1 - \text{sgn}(\delta_m^{l_2})}{2}\end{aligned}\quad (\text{S57.7})$$

$$\mathcal{W}_1^{\text{gapped}} = - \sum_{m=1}^{n_{h_2}} \text{sgn}(v_m^{h_2}) \frac{1 - \text{sgn}(\delta_m^{h_2})}{2} + \sum_{m=1}^{n_{h_4}} \text{sgn}(v_m^{h_4}) \frac{1 - \text{sgn}(\delta_m^{h_4})}{2}\quad (\text{S57.8})$$

$$\begin{aligned}\mathcal{W}_2^{\text{gapped}} = & 2 \sum_{m=1}^{n_{h_2}} \text{sgn}(v_m^{h_2}) \frac{1 - \text{sgn}(\delta_m^{h_2})}{2} - 2 \sum_{m=1}^{n_{h_3}} \text{sgn}(v_m^{h_3}) \frac{1 - \text{sgn}(\delta_m^{h_3})}{2} + \sum_{m=1}^{n_{k_1}} \text{sgn}(v_m^{k_1}) \frac{1 - \text{sgn}(\delta_m^{k_1})}{2} \\ & - \sum_{m=1}^{n_{k_2}} \text{sgn}(v_m^{k_2}) \frac{1 - \text{sgn}(\delta_m^{k_2})}{2} - \sum_{m=1}^{n_{l_1}} \text{sgn}(v_m^{l_1}) \frac{1 - \text{sgn}(\delta_m^{l_1})}{2} + \sum_{m=1}^{n_{l_2}} \text{sgn}(v_m^{l_2}) \frac{1 - \text{sgn}(\delta_m^{l_2})}{2}\end{aligned}\quad (\text{S57.9})$$

$$\mathcal{X}_1 = \sum_{m=1}^{n_{k_1}} \frac{1 - \text{sgn}(\delta_m^{k_1})}{2} + \sum_{m=1}^{n_{k_2}} \frac{1 - \text{sgn}(\delta_m^{k_2})}{2} \mod 2 \quad (\text{S57.10})$$

### S58. SPACE GROUP NO. 58

| line segment                                               | character of irrep (generators only) |                                                                                                                                                                                                                 |
|------------------------------------------------------------|--------------------------------------|-----------------------------------------------------------------------------------------------------------------------------------------------------------------------------------------------------------------|
| $a \left( \frac{t}{2}, 0, 0 \right)$                       | $a_1$                                | $\left\{ 2_{100} \middle  \frac{1}{2} \frac{1}{2} \frac{1}{2} \right\} \left\{ m_{010} \middle  \frac{1}{2} \frac{1}{2} \frac{1}{2} \right\}$<br>0                                                              |
| $b \left( 0, \frac{t}{2}, 0 \right)$                       | $b_1$                                | $\left\{ 2_{010} \middle  \frac{1}{2} \frac{1}{2} \frac{1}{2} \right\} \left\{ m_{100} \middle  \frac{1}{2} \frac{1}{2} \frac{1}{2} \right\}$<br>0                                                              |
| $c \left( \frac{1}{2}, \frac{t}{2}, 0 \right)$             | $c_1$                                | $\left\{ 2_{010} \middle  \frac{1}{2} \frac{1}{2} \frac{1}{2} \right\} \left\{ m_{100} \middle  \frac{1}{2} \frac{1}{2} \frac{1}{2} \right\}$<br>0                                                              |
| $d \left( \frac{1-t}{2}, \frac{1}{2}, 0 \right)$           | $d_1$                                | $\left\{ 2_{100} \middle  \frac{1}{2} \frac{1}{2} \frac{1}{2} \right\} \left\{ m_{010} \middle  \frac{1}{2} \frac{1}{2} \frac{1}{2} \right\}$<br>0                                                              |
| $e \left( \frac{t}{2}, 0, \frac{1}{2} \right)$             | $e_1$                                | $\left\{ 2_{100} \middle  \frac{1}{2} \frac{1}{2} \frac{1}{2} \right\} \left\{ m_{010} \middle  \frac{1}{2} \frac{1}{2} \frac{1}{2} \right\}$<br>$-e^{-\frac{1}{2}i\pi(t+1)} \quad -ie^{-\frac{1}{2}i\pi(t+1)}$ |
|                                                            | $e_2$                                | $-e^{-\frac{1}{2}i\pi(t+1)} \quad ie^{-\frac{1}{2}i\pi(t+1)}$                                                                                                                                                   |
|                                                            | $e_3$                                | $e^{-\frac{1}{2}i\pi(t+1)} \quad -ie^{-\frac{1}{2}i\pi(t+1)}$                                                                                                                                                   |
|                                                            | $e_4$                                | $e^{-\frac{1}{2}i\pi(t+1)} \quad ie^{-\frac{1}{2}i\pi(t+1)}$                                                                                                                                                    |
| $f \left( 0, \frac{t}{2}, \frac{1}{2} \right)$             | $f_1$                                | $\left\{ 2_{010} \middle  \frac{1}{2} \frac{1}{2} \frac{1}{2} \right\} \left\{ m_{100} \middle  \frac{1}{2} \frac{1}{2} \frac{1}{2} \right\}$<br>$-e^{-\frac{1}{2}i\pi(t+1)} \quad -ie^{-\frac{1}{2}i\pi(t+1)}$ |
|                                                            | $f_2$                                | $-e^{-\frac{1}{2}i\pi(t+1)} \quad ie^{-\frac{1}{2}i\pi(t+1)}$                                                                                                                                                   |
|                                                            | $f_3$                                | $e^{-\frac{1}{2}i\pi(t+1)} \quad -ie^{-\frac{1}{2}i\pi(t+1)}$                                                                                                                                                   |
|                                                            | $f_4$                                | $e^{-\frac{1}{2}i\pi(t+1)} \quad ie^{-\frac{1}{2}i\pi(t+1)}$                                                                                                                                                    |
| $g \left( \frac{1}{2}, \frac{t}{2}, \frac{1}{2} \right)$   | $g_1$                                | $\left\{ 2_{010} \middle  \frac{1}{2} \frac{1}{2} \frac{1}{2} \right\} \left\{ m_{100} \middle  \frac{1}{2} \frac{1}{2} \frac{1}{2} \right\}$<br>$-ie^{-\frac{1}{2}i\pi(t+2)} \quad -e^{-\frac{1}{2}i\pi(t+2)}$ |
|                                                            | $g_2$                                | $-ie^{-\frac{1}{2}i\pi(t+2)} \quad e^{-\frac{1}{2}i\pi(t+2)}$                                                                                                                                                   |
|                                                            | $g_3$                                | $ie^{-\frac{1}{2}i\pi(t+2)} \quad -e^{-\frac{1}{2}i\pi(t+2)}$                                                                                                                                                   |
|                                                            | $g_4$                                | $ie^{-\frac{1}{2}i\pi(t+2)} \quad e^{-\frac{1}{2}i\pi(t+2)}$                                                                                                                                                    |
| $h \left( \frac{1-t}{2}, \frac{1}{2}, \frac{1}{2} \right)$ | $h_1$                                | $\left\{ 2_{100} \middle  \frac{1}{2} \frac{1}{2} \frac{1}{2} \right\} \left\{ m_{010} \middle  \frac{1}{2} \frac{1}{2} \frac{1}{2} \right\}$<br>$-ie^{-\frac{1}{2}i\pi(3-t)} \quad -e^{-\frac{1}{2}i\pi(3-t)}$ |
|                                                            | $h_2$                                | $-ie^{-\frac{1}{2}i\pi(3-t)} \quad e^{-\frac{1}{2}i\pi(3-t)}$                                                                                                                                                   |
|                                                            | $h_3$                                | $ie^{-\frac{1}{2}i\pi(3-t)} \quad -e^{-\frac{1}{2}i\pi(3-t)}$                                                                                                                                                   |
|                                                            | $h_4$                                | $ie^{-\frac{1}{2}i\pi(3-t)} \quad e^{-\frac{1}{2}i\pi(3-t)}$                                                                                                                                                    |
| $i \left( 0, 0, \frac{t}{2} \right)$                       | $i_1$                                | $\left\{ 2_{001} \middle  0 \ 0 \ 0 \right\} \left\{ m_{100} \middle  \frac{1}{2} \frac{1}{2} \frac{1}{2} \right\}$<br>0                                                                                        |
| $j \left( \frac{1}{2}, 0, \frac{t}{2} \right)$             | $j_1$                                | $\left\{ 2_{001} \middle  0 \ 0 \ 0 \right\} \left\{ m_{100} \middle  \frac{1}{2} \frac{1}{2} \frac{1}{2} \right\}$<br>$-i \quad -e^{-\frac{1}{2}i\pi(t+1)}$                                                    |
|                                                            | $j_2$                                | $-i \quad e^{-\frac{1}{2}i\pi(t+1)}$                                                                                                                                                                            |
|                                                            | $j_3$                                | $i \quad -e^{-\frac{1}{2}i\pi(t+1)}$                                                                                                                                                                            |
|                                                            | $j_4$                                | $i \quad e^{-\frac{1}{2}i\pi(t+1)}$                                                                                                                                                                             |
| $k \left( \frac{1}{2}, \frac{1}{2}, \frac{t}{2} \right)$   | $k_1$                                | $\left\{ 2_{001} \middle  0 \ 0 \ 0 \right\} \left\{ m_{100} \middle  \frac{1}{2} \frac{1}{2} \frac{1}{2} \right\}$<br>0                                                                                        |
| $l \left( 0, \frac{1}{2}, \frac{t}{2} \right)$             | $l_1$                                | $\left\{ 2_{001} \middle  0 \ 0 \ 0 \right\} \left\{ m_{100} \middle  \frac{1}{2} \frac{1}{2} \frac{1}{2} \right\}$<br>$-i \quad -ie^{-\frac{1}{2}i\pi(t+1)}$                                                   |
|                                                            | $l_2$                                | $-i \quad ie^{-\frac{1}{2}i\pi(t+1)}$                                                                                                                                                                           |
|                                                            | $l_3$                                | $i \quad -ie^{-\frac{1}{2}i\pi(t+1)}$                                                                                                                                                                           |
|                                                            | $l_4$                                | $i \quad ie^{-\frac{1}{2}i\pi(t+1)}$                                                                                                                                                                            |

$$\begin{aligned}
\mathcal{W}_1^{\text{gapless}} = & \sum_{m=1}^{n_{a_1}} \text{sgn}(v_m^{a_1}) \frac{1 - \text{sgn}(\delta_m^{a_1})}{2} - \sum_{m=1}^{n_{f_1}} \text{sgn}(v_m^{f_1}) \frac{1 - \text{sgn}(\delta_m^{f_1})}{2} - \sum_{m=1}^{n_{f_3}} \text{sgn}(v_m^{f_3}) \frac{1 - \text{sgn}(\delta_m^{f_3})}{2} \\
& + 2 \sum_{m=1}^{n_{g_2}} \text{sgn}(v_m^{g_2}) \frac{1 - \text{sgn}(\delta_m^{g_2})}{2} + 2 \sum_{m=1}^{n_{h_2}} \text{sgn}(v_m^{h_2}) \frac{1 - \text{sgn}(\delta_m^{h_2})}{2} - \sum_{m=1}^{n_{i_1}} \text{sgn}(v_m^{i_1}) \frac{1 - \text{sgn}(\delta_m^{i_1})}{2} \\
& + 2 \sum_{m=1}^{n_{j_2}} \text{sgn}(v_m^{j_2}) \frac{1 - \text{sgn}(\delta_m^{j_2})}{2} - \sum_{m=1}^{n_{l_1}} \text{sgn}(v_m^{l_1}) \frac{1 - \text{sgn}(\delta_m^{l_1})}{2} + \sum_{m=1}^{n_{l_2}} \text{sgn}(v_m^{l_2}) \frac{1 - \text{sgn}(\delta_m^{l_2})}{2}
\end{aligned} \tag{S58.1}$$

$$\begin{aligned}
\mathcal{W}_2^{\text{gapless}} = & \sum_{m=1}^{n_{b_1}} \text{sgn}(v_m^{b_1}) \frac{1 - \text{sgn}(\delta_m^{b_1})}{2} - \sum_{m=1}^{n_{f_1}} \text{sgn}(v_m^{f_1}) \frac{1 - \text{sgn}(\delta_m^{f_1})}{2} - \sum_{m=1}^{n_{f_3}} \text{sgn}(v_m^{f_3}) \frac{1 - \text{sgn}(\delta_m^{f_3})}{2} \\
& - \sum_{m=1}^{n_{i_1}} \text{sgn}(v_m^{i_1}) \frac{1 - \text{sgn}(\delta_m^{i_1})}{2} + \sum_{m=1}^{n_{l_1}} \text{sgn}(v_m^{l_1}) \frac{1 - \text{sgn}(\delta_m^{l_1})}{2} + \sum_{m=1}^{n_{l_2}} \text{sgn}(v_m^{l_2}) \frac{1 - \text{sgn}(\delta_m^{l_2})}{2}
\end{aligned} \tag{S58.2}$$

$$\mathcal{W}_3^{\text{gapless}} = \sum_{m=1}^{n_{c_1}} \text{sgn}(v_m^{c_1}) \frac{1 - \text{sgn}(\delta_m^{c_1})}{2} - \sum_{m=1}^{n_{g_2}} \text{sgn}(v_m^{g_2}) \frac{1 - \text{sgn}(\delta_m^{g_2})}{2} - \sum_{m=1}^{n_{j_2}} \text{sgn}(v_m^{j_2}) \frac{1 - \text{sgn}(\delta_m^{j_2})}{2} + \sum_{m=1}^{n_{k_1}} \text{sgn}(v_m^{k_1}) \frac{1 - \text{sgn}(\delta_m^{k_1})}{2} \tag{S58.3}$$

$$\mathcal{W}_4^{\text{gapless}} = \sum_{m=1}^{n_{d_1}} \text{sgn}(v_m^{d_1}) \frac{1 - \text{sgn}(\delta_m^{d_1})}{2} - \sum_{m=1}^{n_{h_2}} \text{sgn}(v_m^{h_2}) \frac{1 - \text{sgn}(\delta_m^{h_2})}{2} - \sum_{m=1}^{n_{k_1}} \text{sgn}(v_m^{k_1}) \frac{1 - \text{sgn}(\delta_m^{k_1})}{2} + \sum_{m=1}^{n_{l_1}} \text{sgn}(v_m^{l_1}) \frac{1 - \text{sgn}(\delta_m^{l_1})}{2} \tag{S58.4}$$

$$\begin{aligned}
\mathcal{W}_5^{\text{gapless}} = & \sum_{m=1}^{n_{e_1}} \text{sgn}(v_m^{e_1}) \frac{1 - \text{sgn}(\delta_m^{e_1})}{2} + \sum_{m=1}^{n_{e_3}} \text{sgn}(v_m^{e_3}) \frac{1 - \text{sgn}(\delta_m^{e_3})}{2} - \sum_{m=1}^{n_{f_1}} \text{sgn}(v_m^{f_1}) \frac{1 - \text{sgn}(\delta_m^{f_1})}{2} - \sum_{m=1}^{n_{f_3}} \text{sgn}(v_m^{f_3}) \frac{1 - \text{sgn}(\delta_m^{f_3})}{2} \\
& + 2 \sum_{m=1}^{n_{g_2}} \text{sgn}(v_m^{g_2}) \frac{1 - \text{sgn}(\delta_m^{g_2})}{2} + 2 \sum_{m=1}^{n_{h_2}} \text{sgn}(v_m^{h_2}) \frac{1 - \text{sgn}(\delta_m^{h_2})}{2} - \sum_{m=1}^{n_{j_1}} \text{sgn}(v_m^{j_1}) \frac{1 - \text{sgn}(\delta_m^{j_1})}{2} \\
& + \sum_{m=1}^{n_{j_2}} \text{sgn}(v_m^{j_2}) \frac{1 - \text{sgn}(\delta_m^{j_2})}{2} - \sum_{m=1}^{n_{l_1}} \text{sgn}(v_m^{l_1}) \frac{1 - \text{sgn}(\delta_m^{l_1})}{2} + \sum_{m=1}^{n_{l_2}} \text{sgn}(v_m^{l_2}) \frac{1 - \text{sgn}(\delta_m^{l_2})}{2}
\end{aligned} \tag{S58.5}$$

$$\mathcal{W}_6^{\text{gapless}} = \sum_{m=1}^{n_{g_1}} \text{sgn}(v_m^{g_1}) \frac{1 - \text{sgn}(\delta_m^{g_1})}{2} - \sum_{m=1}^{n_{g_2}} \text{sgn}(v_m^{g_2}) \frac{1 - \text{sgn}(\delta_m^{g_2})}{2} + \sum_{m=1}^{n_{j_1}} \text{sgn}(v_m^{j_1}) \frac{1 - \text{sgn}(\delta_m^{j_1})}{2} - \sum_{m=1}^{n_{j_2}} \text{sgn}(v_m^{j_2}) \frac{1 - \text{sgn}(\delta_m^{j_2})}{2} \tag{S58.6}$$

$$\mathcal{W}_7^{\text{gapless}} = \sum_{m=1}^{n_{h_1}} \text{sgn}(v_m^{h_1}) \frac{1 - \text{sgn}(\delta_m^{h_1})}{2} - \sum_{m=1}^{n_{h_2}} \text{sgn}(v_m^{h_2}) \frac{1 - \text{sgn}(\delta_m^{h_2})}{2} + \sum_{m=1}^{n_{l_1}} \text{sgn}(v_m^{l_1}) \frac{1 - \text{sgn}(\delta_m^{l_1})}{2} - \sum_{m=1}^{n_{l_2}} \text{sgn}(v_m^{l_2}) \frac{1 - \text{sgn}(\delta_m^{l_2})}{2} \tag{S58.7}$$

$$\mathcal{X}_1 = \sum_{m=1}^{n_{f_1}} \frac{1 - \text{sgn}(\delta_m^{f_1})}{2} + \sum_{m=1}^{n_{f_3}} \frac{1 - \text{sgn}(\delta_m^{f_3})}{2} + \sum_{m=1}^{n_{l_1}} \frac{1 - \text{sgn}(\delta_m^{l_1})}{2} + \sum_{m=1}^{n_{l_2}} \frac{1 - \text{sgn}(\delta_m^{l_2})}{2} \mod 2 \tag{S58.8}$$

## S59. SPACE GROUP NO. 59

| line segment                                               | character of irrep (generators only)                                                                                                                                                                                                                                                                                                                                                                                                                                                                                                       |
|------------------------------------------------------------|--------------------------------------------------------------------------------------------------------------------------------------------------------------------------------------------------------------------------------------------------------------------------------------------------------------------------------------------------------------------------------------------------------------------------------------------------------------------------------------------------------------------------------------------|
| $a \left( \frac{t}{2}, 0, 0 \right)$                       | $a_1 \begin{Bmatrix} \{2_{100}   \frac{1}{2} & 0 & 0\} \\ 0 \end{Bmatrix} \begin{Bmatrix} \{m_{010}   0 & \frac{1}{2} & 0\} \\ 0 \end{Bmatrix}$                                                                                                                                                                                                                                                                                                                                                                                            |
| $b \left( 0, \frac{t}{2}, 0 \right)$                       | $b_1 \begin{Bmatrix} \{2_{010}   0 & \frac{1}{2} & 0\} \\ 0 \end{Bmatrix} \begin{Bmatrix} \{m_{100}   \frac{1}{2} & 0 & 0\} \\ 0 \end{Bmatrix}$                                                                                                                                                                                                                                                                                                                                                                                            |
| $c \left( \frac{1}{2}, \frac{t}{2}, 0 \right)$             | $\begin{matrix} c_1 & \begin{Bmatrix} \{2_{010}   0 & \frac{1}{2} & 0\} \\ -ie^{-\frac{1}{2}i\pi t} \end{Bmatrix} & \begin{Bmatrix} \{m_{100}   \frac{1}{2} & 0 & 0\} \\ i \end{Bmatrix} \\ c_2 & \begin{Bmatrix} -ie^{-\frac{1}{2}i\pi t} \\ \end{Bmatrix} & \begin{Bmatrix} -i \\ \end{Bmatrix} \\ c_3 & \begin{Bmatrix} ie^{-\frac{1}{2}i\pi t} \\ \end{Bmatrix} & \begin{Bmatrix} i \\ \end{Bmatrix} \\ c_4 & \begin{Bmatrix} ie^{-\frac{1}{2}i\pi t} \\ \end{Bmatrix} & \begin{Bmatrix} -i \\ \end{Bmatrix} \end{matrix}$             |
| $d \left( \frac{1-t}{2}, \frac{1}{2}, 0 \right)$           | $\begin{matrix} d_1 & \begin{Bmatrix} \{2_{100}   \frac{1}{2} & 0 & 0\} \\ -ie^{-\frac{1}{2}i\pi(1-t)} \end{Bmatrix} & \begin{Bmatrix} \{m_{010}   0 & \frac{1}{2} & 0\} \\ i \end{Bmatrix} \\ d_2 & \begin{Bmatrix} -ie^{-\frac{1}{2}i\pi(1-t)} \\ \end{Bmatrix} & \begin{Bmatrix} -i \\ \end{Bmatrix} \\ d_3 & \begin{Bmatrix} ie^{-\frac{1}{2}i\pi(1-t)} \\ \end{Bmatrix} & \begin{Bmatrix} i \\ \end{Bmatrix} \\ d_4 & \begin{Bmatrix} ie^{-\frac{1}{2}i\pi(1-t)} \\ \end{Bmatrix} & \begin{Bmatrix} -i \\ \end{Bmatrix} \end{matrix}$ |
| $e \left( \frac{t}{2}, 0, \frac{1}{2} \right)$             | $e_1 \begin{Bmatrix} \{2_{100}   \frac{1}{2} & 0 & 0\} \\ 0 \end{Bmatrix} \begin{Bmatrix} \{m_{010}   0 & \frac{1}{2} & 0\} \\ 0 \end{Bmatrix}$                                                                                                                                                                                                                                                                                                                                                                                            |
| $f \left( 0, \frac{t}{2}, \frac{1}{2} \right)$             | $f_1 \begin{Bmatrix} \{2_{010}   0 & \frac{1}{2} & 0\} \\ 0 \end{Bmatrix} \begin{Bmatrix} \{m_{100}   \frac{1}{2} & 0 & 0\} \\ 0 \end{Bmatrix}$                                                                                                                                                                                                                                                                                                                                                                                            |
| $g \left( \frac{1}{2}, \frac{t}{2}, \frac{1}{2} \right)$   | $\begin{matrix} g_1 & \begin{Bmatrix} \{2_{010}   0 & \frac{1}{2} & 0\} \\ -ie^{-\frac{1}{2}i\pi t} \end{Bmatrix} & \begin{Bmatrix} \{m_{100}   \frac{1}{2} & 0 & 0\} \\ i \end{Bmatrix} \\ g_2 & \begin{Bmatrix} -ie^{-\frac{1}{2}i\pi t} \\ \end{Bmatrix} & \begin{Bmatrix} -i \\ \end{Bmatrix} \\ g_3 & \begin{Bmatrix} ie^{-\frac{1}{2}i\pi t} \\ \end{Bmatrix} & \begin{Bmatrix} i \\ \end{Bmatrix} \\ g_4 & \begin{Bmatrix} ie^{-\frac{1}{2}i\pi t} \\ \end{Bmatrix} & \begin{Bmatrix} -i \\ \end{Bmatrix} \end{matrix}$             |
| $h \left( \frac{1-t}{2}, \frac{1}{2}, \frac{1}{2} \right)$ | $\begin{matrix} h_1 & \begin{Bmatrix} \{2_{100}   \frac{1}{2} & 0 & 0\} \\ -ie^{-\frac{1}{2}i\pi(1-t)} \end{Bmatrix} & \begin{Bmatrix} \{m_{010}   0 & \frac{1}{2} & 0\} \\ i \end{Bmatrix} \\ h_2 & \begin{Bmatrix} -ie^{-\frac{1}{2}i\pi(1-t)} \\ \end{Bmatrix} & \begin{Bmatrix} -i \\ \end{Bmatrix} \\ h_3 & \begin{Bmatrix} ie^{-\frac{1}{2}i\pi(1-t)} \\ \end{Bmatrix} & \begin{Bmatrix} i \\ \end{Bmatrix} \\ h_4 & \begin{Bmatrix} ie^{-\frac{1}{2}i\pi(1-t)} \\ \end{Bmatrix} & \begin{Bmatrix} -i \\ \end{Bmatrix} \end{matrix}$ |
| $i \left( 0, 0, \frac{t}{2} \right)$                       | $i_1 \begin{Bmatrix} \{2_{001}   \frac{1}{2} & \frac{1}{2} & 0\} \\ 0 \end{Bmatrix} \begin{Bmatrix} \{m_{100}   \frac{1}{2} & 0 & 0\} \\ 0 \end{Bmatrix}$                                                                                                                                                                                                                                                                                                                                                                                  |
| $j \left( \frac{1}{2}, 0, \frac{t}{2} \right)$             | $j_1 \begin{Bmatrix} \{2_{001}   \frac{1}{2} & \frac{1}{2} & 0\} \\ 0 \end{Bmatrix} \begin{Bmatrix} \{m_{100}   \frac{1}{2} & 0 & 0\} \\ 0 \end{Bmatrix}$                                                                                                                                                                                                                                                                                                                                                                                  |
| $k \left( \frac{1}{2}, \frac{1}{2}, \frac{t}{2} \right)$   | $k_1 \begin{Bmatrix} \{2_{001}   \frac{1}{2} & \frac{1}{2} & 0\} \\ 0 \end{Bmatrix} \begin{Bmatrix} \{m_{100}   \frac{1}{2} & 0 & 0\} \\ 0 \end{Bmatrix}$                                                                                                                                                                                                                                                                                                                                                                                  |
| $l \left( 0, \frac{1}{2}, \frac{t}{2} \right)$             | $l_1 \begin{Bmatrix} \{2_{001}   \frac{1}{2} & \frac{1}{2} & 0\} \\ 0 \end{Bmatrix} \begin{Bmatrix} \{m_{100}   \frac{1}{2} & 0 & 0\} \\ 0 \end{Bmatrix}$                                                                                                                                                                                                                                                                                                                                                                                  |

$$\begin{aligned}
\mathcal{W}_1^{\text{gapless}} = & \sum_{m=1}^{n_{a_1}} \text{sgn}(v_m^{a_1}) \frac{1 - \text{sgn}(\delta_m^{a_1})}{2} - \sum_{m=1}^{n_{f_1}} \text{sgn}(v_m^{f_1}) \frac{1 - \text{sgn}(\delta_m^{f_1})}{2} + \sum_{m=1}^{n_{g_1}} \text{sgn}(v_m^{g_1}) \frac{1 - \text{sgn}(\delta_m^{g_1})}{2} \\
& + \sum_{m=1}^{n_{g_2}} \text{sgn}(v_m^{g_2}) \frac{1 - \text{sgn}(\delta_m^{g_2})}{2} + \sum_{m=1}^{n_{h_1}} \text{sgn}(v_m^{h_1}) \frac{1 - \text{sgn}(\delta_m^{h_1})}{2} + \sum_{m=1}^{n_{h_2}} \text{sgn}(v_m^{h_2}) \frac{1 - \text{sgn}(\delta_m^{h_2})}{2} \\
& - \sum_{m=1}^{n_{i_1}} \text{sgn}(v_m^{i_1}) \frac{1 - \text{sgn}(\delta_m^{i_1})}{2} + 2 \sum_{m=1}^{n_{j_1}} \text{sgn}(v_m^{j_1}) \frac{1 - \text{sgn}(\delta_m^{j_1})}{2}
\end{aligned} \tag{S59.1}$$

$$\begin{aligned}
\mathcal{W}_2^{\text{gapless}} = & \sum_{m=1}^{n_{b_1}} \text{sgn}(v_m^{b_1}) \frac{1 - \text{sgn}(\delta_m^{b_1})}{2} - \sum_{m=1}^{n_{f_1}} \text{sgn}(v_m^{f_1}) \frac{1 - \text{sgn}(\delta_m^{f_1})}{2} - \sum_{m=1}^{n_{i_1}} \text{sgn}(v_m^{i_1}) \frac{1 - \text{sgn}(\delta_m^{i_1})}{2} + 2 \sum_{m=1}^{n_{l_1}} \text{sgn}(v_m^{l_1}) \frac{1 - \text{sgn}(\delta_m^{l_1})}{2}
\end{aligned} \tag{S59.2}$$

$$\mathcal{W}_3^{\text{gapless}} = \sum_{m=1}^{n_{c_1}} \text{sgn}(v_m^{c_1}) \frac{1 - \text{sgn}(\delta_m^{c_1})}{2} - \sum_{m=1}^{n_{g_1}} \text{sgn}(v_m^{g_1}) \frac{1 - \text{sgn}(\delta_m^{g_1})}{2} - \sum_{m=1}^{n_{j_1}} \text{sgn}(v_m^{j_1}) \frac{1 - \text{sgn}(\delta_m^{j_1})}{2} + \sum_{m=1}^{n_{k_1}} \text{sgn}(v_m^{k_1}) \frac{1 - \text{sgn}(\delta_m^{k_1})}{2} \quad (\text{S59.3})$$

$$\mathcal{W}_4^{\text{gapless}} = \sum_{m=1}^{n_{c_2}} \text{sgn}(v_m^{c_2}) \frac{1 - \text{sgn}(\delta_m^{c_2})}{2} - \sum_{m=1}^{n_{g_2}} \text{sgn}(v_m^{g_2}) \frac{1 - \text{sgn}(\delta_m^{g_2})}{2} - \sum_{m=1}^{n_{j_1}} \text{sgn}(v_m^{j_1}) \frac{1 - \text{sgn}(\delta_m^{j_1})}{2} + \sum_{m=1}^{n_{k_1}} \text{sgn}(v_m^{k_1}) \frac{1 - \text{sgn}(\delta_m^{k_1})}{2} \quad (\text{S59.4})$$

$$\mathcal{W}_5^{\text{gapless}} = \sum_{m=1}^{n_{d_1}} \text{sgn}(v_m^{d_1}) \frac{1 - \text{sgn}(\delta_m^{d_1})}{2} - \sum_{m=1}^{n_{h_1}} \text{sgn}(v_m^{h_1}) \frac{1 - \text{sgn}(\delta_m^{h_1})}{2} - \sum_{m=1}^{n_{k_1}} \text{sgn}(v_m^{k_1}) \frac{1 - \text{sgn}(\delta_m^{k_1})}{2} + \sum_{m=1}^{n_{l_1}} \text{sgn}(v_m^{l_1}) \frac{1 - \text{sgn}(\delta_m^{l_1})}{2} \quad (\text{S59.5})$$

$$\mathcal{W}_6^{\text{gapless}} = \sum_{m=1}^{n_{d_2}} \text{sgn}(v_m^{d_2}) \frac{1 - \text{sgn}(\delta_m^{d_2})}{2} - \sum_{m=1}^{n_{h_2}} \text{sgn}(v_m^{h_2}) \frac{1 - \text{sgn}(\delta_m^{h_2})}{2} - \sum_{m=1}^{n_{k_1}} \text{sgn}(v_m^{k_1}) \frac{1 - \text{sgn}(\delta_m^{k_1})}{2} + \sum_{m=1}^{n_{l_1}} \text{sgn}(v_m^{l_1}) \frac{1 - \text{sgn}(\delta_m^{l_1})}{2} \quad (\text{S59.6})$$

$$\begin{aligned} \mathcal{W}_7^{\text{gapless}} = & \sum_{m=1}^{n_{e_1}} \text{sgn}(v_m^{e_1}) \frac{1 - \text{sgn}(\delta_m^{e_1})}{2} - \sum_{m=1}^{n_{f_1}} \text{sgn}(v_m^{f_1}) \frac{1 - \text{sgn}(\delta_m^{f_1})}{2} + \sum_{m=1}^{n_{g_1}} \text{sgn}(v_m^{g_1}) \frac{1 - \text{sgn}(\delta_m^{g_1})}{2} \\ & + \sum_{m=1}^{n_{g_2}} \text{sgn}(v_m^{g_2}) \frac{1 - \text{sgn}(\delta_m^{g_2})}{2} + \sum_{m=1}^{n_{h_1}} \text{sgn}(v_m^{h_1}) \frac{1 - \text{sgn}(\delta_m^{h_1})}{2} + \sum_{m=1}^{n_{h_2}} \text{sgn}(v_m^{h_2}) \frac{1 - \text{sgn}(\delta_m^{h_2})}{2} \end{aligned} \quad (\text{S59.7})$$

$$\mathcal{W}_1^{\text{gapped}} = - \sum_{m=1}^{n_{g_1}} \text{sgn}(v_m^{g_1}) \frac{1 - \text{sgn}(\delta_m^{g_1})}{2} + \sum_{m=1}^{n_{g_2}} \text{sgn}(v_m^{g_2}) \frac{1 - \text{sgn}(\delta_m^{g_2})}{2} \quad (\text{S59.8})$$

$$\mathcal{W}_2^{\text{gapped}} = \sum_{m=1}^{n_{h_1}} \text{sgn}(v_m^{h_1}) \frac{1 - \text{sgn}(\delta_m^{h_1})}{2} - \sum_{m=1}^{n_{h_2}} \text{sgn}(v_m^{h_2}) \frac{1 - \text{sgn}(\delta_m^{h_2})}{2} \quad (\text{S59.9})$$

### S60. SPACE GROUP NO. 60

| line segment                            | character of irrep (generators only) |                                                                                       |
|-----------------------------------------|--------------------------------------|---------------------------------------------------------------------------------------|
| $a \quad (\frac{t}{2}, 0, 0)$           | $a_1$                                | $\{2_{100}   \frac{1}{2} \frac{1}{2} 0\} \quad \{m_{010}   0 \ 0 \ \frac{1}{2}\}$     |
| $b \quad (0, \frac{t}{2}, 0)$           | $b_1$                                | $\{2_{010}   0 \ 0 \ \frac{1}{2}\} \quad \{m_{100}   \frac{1}{2} \ \frac{1}{2} \ 0\}$ |
| $c \quad (\frac{1}{2}, \frac{t}{2}, 0)$ | $c_1$                                | $\{2_{010}   0 \ 0 \ \frac{1}{2}\} \quad \{m_{100}   \frac{1}{2} \ \frac{1}{2} \ 0\}$ |
|                                         | $c_2$                                | $-i \quad -e^{-\frac{1}{2}i\pi(t+1)}$                                                 |
|                                         | $c_3$                                | $-i \quad e^{-\frac{1}{2}i\pi(t+1)}$                                                  |
|                                         | $c_4$                                | $i \quad -e^{-\frac{1}{2}i\pi(t+1)}$                                                  |
|                                         |                                      | $i \quad e^{-\frac{1}{2}i\pi(t+1)}$                                                   |



|                                                     |                                                                                                                                                                                                                                                                                                               |
|-----------------------------------------------------|---------------------------------------------------------------------------------------------------------------------------------------------------------------------------------------------------------------------------------------------------------------------------------------------------------------|
| $d \quad (\frac{1-t}{2}, \frac{1}{2}, 0)$           | $\{2_{100}   \frac{1}{2} \frac{1}{2} 0\} \quad \{m_{010}   0 \ 0 \ \frac{1}{2}\}$<br>$d_1 \quad -e^{-\frac{1}{2}i\pi(2-t)} \quad -i$<br>$d_2 \quad -e^{-\frac{1}{2}i\pi(2-t)} \quad i$<br>$d_3 \quad e^{-\frac{1}{2}i\pi(2-t)} \quad -i$<br>$d_4 \quad e^{-\frac{1}{2}i\pi(2-t)} \quad i$                     |
| $e \quad (\frac{t}{2}, 0, \frac{1}{2})$             | $\{2_{100}   \frac{1}{2} \frac{1}{2} 0\} \quad \{m_{010}   0 \ 0 \ \frac{1}{2}\}$<br>$e_1 \quad -ie^{-\frac{1}{2}i\pi t} \quad -1$<br>$e_2 \quad -ie^{-\frac{1}{2}i\pi t} \quad 1$<br>$e_3 \quad ie^{-\frac{1}{2}i\pi t} \quad -1$<br>$e_4 \quad ie^{-\frac{1}{2}i\pi t} \quad 1$                             |
| $f \quad (0, \frac{t}{2}, \frac{1}{2})$             | $\{2_{010}   0 \ 0 \ \frac{1}{2}\} \quad \{m_{100}   \frac{1}{2} \frac{1}{2} 0\}$<br>$f_1 \quad 0 \quad 0$                                                                                                                                                                                                    |
| $g \quad (\frac{1}{2}, \frac{t}{2}, \frac{1}{2})$   | $\{2_{010}   0 \ 0 \ \frac{1}{2}\} \quad \{m_{100}   \frac{1}{2} \frac{1}{2} 0\}$<br>$g_1 \quad i \quad -e^{-\frac{1}{2}i\pi(t+1)}$<br>$g_2 \quad i \quad e^{-\frac{1}{2}i\pi(t+1)}$<br>$g_3 \quad -i \quad -e^{-\frac{1}{2}i\pi(t+1)}$<br>$g_4 \quad -i \quad e^{-\frac{1}{2}i\pi(t+1)}$                     |
| $h \quad (\frac{1-t}{2}, \frac{1}{2}, \frac{1}{2})$ | $\{2_{100}   \frac{1}{2} \frac{1}{2} 0\} \quad \{m_{010}   0 \ 0 \ \frac{1}{2}\}$<br>$h_1 \quad 0 \quad 0$                                                                                                                                                                                                    |
| $i \quad (0, 0, \frac{t}{2})$                       | $\{2_{001}   \frac{1}{2} \frac{1}{2} \frac{1}{2}\} \quad \{m_{100}   \frac{1}{2} \frac{1}{2} 0\}$<br>$i_1 \quad 0 \quad 0$                                                                                                                                                                                    |
| $j \quad (\frac{1}{2}, 0, \frac{t}{2})$             | $\{2_{001}   \frac{1}{2} \frac{1}{2} \frac{1}{2}\} \quad \{m_{100}   \frac{1}{2} \frac{1}{2} 0\}$<br>$j_1 \quad 0 \quad 0$                                                                                                                                                                                    |
| $k \quad (\frac{1}{2}, \frac{1}{2}, \frac{t}{2})$   | $\{2_{001}   \frac{1}{2} \frac{1}{2} \frac{1}{2}\} \quad \{m_{100}   \frac{1}{2} \frac{1}{2} 0\}$<br>$k_1 \quad -ie^{-\frac{1}{2}i\pi(t+2)} \quad 1$<br>$k_2 \quad -ie^{-\frac{1}{2}i\pi(t+2)} \quad -1$<br>$k_3 \quad ie^{-\frac{1}{2}i\pi(t+2)} \quad 1$<br>$k_4 \quad ie^{-\frac{1}{2}i\pi(t+2)} \quad -1$ |
| $l \quad (0, \frac{1}{2}, \frac{t}{2})$             | $\{2_{001}   \frac{1}{2} \frac{1}{2} \frac{1}{2}\} \quad \{m_{100}   \frac{1}{2} \frac{1}{2} 0\}$<br>$l_1 \quad -e^{-\frac{1}{2}i\pi(t+1)} \quad -1$<br>$l_2 \quad -e^{-\frac{1}{2}i\pi(t+1)} \quad 1$<br>$l_3 \quad e^{-\frac{1}{2}i\pi(t+1)} \quad -1$<br>$l_4 \quad e^{-\frac{1}{2}i\pi(t+1)} \quad 1$     |

$$\begin{aligned}
\mathcal{W}_1^{\text{gapless}} = & \sum_{m=1}^{n_{a_1}} \text{sgn}(v_m^{a_1}) \frac{1 - \text{sgn}(\delta_m^{a_1})}{2} - 2 \sum_{m=1}^{n_{f_1}} \text{sgn}(v_m^{f_1}) \frac{1 - \text{sgn}(\delta_m^{f_1})}{2} + \sum_{m=1}^{n_{g_1}} \text{sgn}(v_m^{g_1}) \frac{1 - \text{sgn}(\delta_m^{g_1})}{2} \\
& + \sum_{m=1}^{n_{g_2}} \text{sgn}(v_m^{g_2}) \frac{1 - \text{sgn}(\delta_m^{g_2})}{2} + \sum_{m=1}^{n_{g_3}} \text{sgn}(v_m^{g_3}) \frac{1 - \text{sgn}(\delta_m^{g_3})}{2} + \sum_{m=1}^{n_{g_4}} \text{sgn}(v_m^{g_4}) \frac{1 - \text{sgn}(\delta_m^{g_4})}{2} \\
& + 2 \sum_{m=1}^{n_{h_1}} \text{sgn}(v_m^{h_1}) \frac{1 - \text{sgn}(\delta_m^{h_1})}{2} - \sum_{m=1}^{n_{i_1}} \text{sgn}(v_m^{i_1}) \frac{1 - \text{sgn}(\delta_m^{i_1})}{2} + 2 \sum_{m=1}^{n_{j_1}} \text{sgn}(v_m^{j_1}) \frac{1 - \text{sgn}(\delta_m^{j_1})}{2}
\end{aligned} \tag{S60.1}$$

$$\begin{aligned}
\mathcal{W}_2^{\text{gapless}} = & \sum_{m=1}^{n_{b_1}} \text{sgn}(v_m^{b_1}) \frac{1 - \text{sgn}(\delta_m^{b_1})}{2} - 2 \sum_{m=1}^{n_{f_1}} \text{sgn}(v_m^{f_1}) \frac{1 - \text{sgn}(\delta_m^{f_1})}{2} - \sum_{m=1}^{n_{i_1}} \text{sgn}(v_m^{i_1}) \frac{1 - \text{sgn}(\delta_m^{i_1})}{2} \\
& + \sum_{m=1}^{n_{l_1}} \text{sgn}(v_m^{l_1}) \frac{1 - \text{sgn}(\delta_m^{l_1})}{2} + \sum_{m=1}^{n_{l_3}} \text{sgn}(v_m^{l_3}) \frac{1 - \text{sgn}(\delta_m^{l_3})}{2}
\end{aligned} \tag{S60.2}$$

$$\begin{aligned} \mathcal{W}_3^{\text{gapless}} = & \sum_{m=1}^{n_{c_1}} \text{sgn}(v_m^{c_1}) \frac{1 - \text{sgn}(\delta_m^{c_1})}{2} - \sum_{m=1}^{n_{g_1}} \text{sgn}(v_m^{g_1}) \frac{1 - \text{sgn}(\delta_m^{g_1})}{2} - \sum_{m=1}^{n_{g_3}} \text{sgn}(v_m^{g_3}) \frac{1 - \text{sgn}(\delta_m^{g_3})}{2} \\ & - \sum_{m=1}^{n_{j_1}} \text{sgn}(v_m^{j_1}) \frac{1 - \text{sgn}(\delta_m^{j_1})}{2} + \sum_{m=1}^{n_{k_1}} \text{sgn}(v_m^{k_1}) \frac{1 - \text{sgn}(\delta_m^{k_1})}{2} \end{aligned} \quad (\text{S60.3})$$

$$\begin{aligned} \mathcal{W}_4^{\text{gapless}} = & \sum_{m=1}^{n_{c_2}} \text{sgn}(v_m^{c_2}) \frac{1 - \text{sgn}(\delta_m^{c_2})}{2} - \sum_{m=1}^{n_{g_2}} \text{sgn}(v_m^{g_2}) \frac{1 - \text{sgn}(\delta_m^{g_2})}{2} - \sum_{m=1}^{n_{g_4}} \text{sgn}(v_m^{g_4}) \frac{1 - \text{sgn}(\delta_m^{g_4})}{2} \\ & - \sum_{m=1}^{n_{j_1}} \text{sgn}(v_m^{j_1}) \frac{1 - \text{sgn}(\delta_m^{j_1})}{2} + \sum_{m=1}^{n_{k_2}} \text{sgn}(v_m^{k_2}) \frac{1 - \text{sgn}(\delta_m^{k_2})}{2} \end{aligned} \quad (\text{S60.4})$$

$$\begin{aligned} \mathcal{W}_5^{\text{gapless}} = & \sum_{m=1}^{n_{d_1}} \text{sgn}(v_m^{d_1}) \frac{1 - \text{sgn}(\delta_m^{d_1})}{2} + \sum_{m=1}^{n_{d_3}} \text{sgn}(v_m^{d_3}) \frac{1 - \text{sgn}(\delta_m^{d_3})}{2} - 2 \sum_{m=1}^{n_{h_1}} \text{sgn}(v_m^{h_1}) \frac{1 - \text{sgn}(\delta_m^{h_1})}{2} \\ & - \sum_{m=1}^{n_{k_1}} \text{sgn}(v_m^{k_1}) \frac{1 - \text{sgn}(\delta_m^{k_1})}{2} - \sum_{m=1}^{n_{k_2}} \text{sgn}(v_m^{k_2}) \frac{1 - \text{sgn}(\delta_m^{k_2})}{2} + \sum_{m=1}^{n_{l_1}} \text{sgn}(v_m^{l_1}) \frac{1 - \text{sgn}(\delta_m^{l_1})}{2} \\ & + \sum_{m=1}^{n_{l_3}} \text{sgn}(v_m^{l_3}) \frac{1 - \text{sgn}(\delta_m^{l_3})}{2} \end{aligned} \quad (\text{S60.5})$$

$$\begin{aligned} \mathcal{W}_6^{\text{gapless}} = & \sum_{m=1}^{n_{e_1}} \text{sgn}(v_m^{e_1}) \frac{1 - \text{sgn}(\delta_m^{e_1})}{2} - \sum_{m=1}^{n_{f_1}} \text{sgn}(v_m^{f_1}) \frac{1 - \text{sgn}(\delta_m^{f_1})}{2} + \sum_{m=1}^{n_{g_1}} \text{sgn}(v_m^{g_1}) \frac{1 - \text{sgn}(\delta_m^{g_1})}{2} \\ & + \sum_{m=1}^{n_{g_4}} \text{sgn}(v_m^{g_4}) \frac{1 - \text{sgn}(\delta_m^{g_4})}{2} + \sum_{m=1}^{n_{h_1}} \text{sgn}(v_m^{h_1}) \frac{1 - \text{sgn}(\delta_m^{h_1})}{2} \end{aligned} \quad (\text{S60.6})$$

$$\begin{aligned} \mathcal{W}_7^{\text{gapless}} = & \sum_{m=1}^{n_{e_2}} \text{sgn}(v_m^{e_2}) \frac{1 - \text{sgn}(\delta_m^{e_2})}{2} - \sum_{m=1}^{n_{f_1}} \text{sgn}(v_m^{f_1}) \frac{1 - \text{sgn}(\delta_m^{f_1})}{2} + \sum_{m=1}^{n_{g_2}} \text{sgn}(v_m^{g_2}) \frac{1 - \text{sgn}(\delta_m^{g_2})}{2} \\ & + \sum_{m=1}^{n_{g_3}} \text{sgn}(v_m^{g_3}) \frac{1 - \text{sgn}(\delta_m^{g_3})}{2} + \sum_{m=1}^{n_{h_1}} \text{sgn}(v_m^{h_1}) \frac{1 - \text{sgn}(\delta_m^{h_1})}{2} \end{aligned} \quad (\text{S60.7})$$

$$\begin{aligned} \mathcal{W}_1^{\text{gapped}} = & - \sum_{m=1}^{n_{g_1}} \text{sgn}(v_m^{g_1}) \frac{1 - \text{sgn}(\delta_m^{g_1})}{2} - \sum_{m=1}^{n_{g_2}} \text{sgn}(v_m^{g_2}) \frac{1 - \text{sgn}(\delta_m^{g_2})}{2} + \sum_{m=1}^{n_{g_3}} \text{sgn}(v_m^{g_3}) \frac{1 - \text{sgn}(\delta_m^{g_3})}{2} \\ & + \sum_{m=1}^{n_{g_4}} \text{sgn}(v_m^{g_4}) \frac{1 - \text{sgn}(\delta_m^{g_4})}{2} \end{aligned} \quad (\text{S60.8})$$

$$\begin{aligned} \mathcal{X}_1 = & 2 \sum_{m=1}^{n_{g_2}} \text{sgn}(v_m^{g_2}) \frac{1 - \text{sgn}(\delta_m^{g_2})}{2} - 2 \sum_{m=1}^{n_{g_3}} \text{sgn}(v_m^{g_3}) \frac{1 - \text{sgn}(\delta_m^{g_3})}{2} - 2 \sum_{m=1}^{n_{h_1}} \text{sgn}(v_m^{h_1}) \frac{1 - \text{sgn}(\delta_m^{h_1})}{2} \\ & + \sum_{m=1}^{n_{l_1}} \text{sgn}(v_m^{l_1}) \frac{1 - \text{sgn}(\delta_m^{l_1})}{2} - \sum_{m=1}^{n_{l_3}} \text{sgn}(v_m^{l_3}) \frac{1 - \text{sgn}(\delta_m^{l_3})}{2} \pmod{4} \end{aligned} \quad (\text{S60.9})$$

## S61. SPACE GROUP NO. 61

| line segment                                             | character of irrep (generators only) |                                                                                                                                                                                                                                                                                          |
|----------------------------------------------------------|--------------------------------------|------------------------------------------------------------------------------------------------------------------------------------------------------------------------------------------------------------------------------------------------------------------------------------------|
| $a \left(\frac{t}{2}, 0, 0\right)$                       | $a_1$                                | $\left\{2_{100} \left  \begin{smallmatrix} \frac{1}{2} & \frac{1}{2} & 0 \end{smallmatrix} \right. \right\} \left\{m_{010} \left  \begin{smallmatrix} 0 & \frac{1}{2} & \frac{1}{2} \end{smallmatrix} \right. \right\}$<br>0                                                             |
| $b \left(0, \frac{t}{2}, 0\right)$                       | $b_1$                                | $\left\{2_{010} \left  \begin{smallmatrix} 0 & \frac{1}{2} & \frac{1}{2} \end{smallmatrix} \right. \right\} \left\{m_{100} \left  \begin{smallmatrix} \frac{1}{2} & \frac{1}{2} & 0 \end{smallmatrix} \right. \right\}$<br>0                                                             |
| $c \left(\frac{1}{2}, \frac{t}{2}, 0\right)$             | $c_1$                                | $\left\{2_{010} \left  \begin{smallmatrix} 0 & \frac{1}{2} & \frac{1}{2} \end{smallmatrix} \right. \right\} \left\{m_{100} \left  \begin{smallmatrix} \frac{1}{2} & \frac{1}{2} & 0 \end{smallmatrix} \right. \right\}$<br>$-ie^{-\frac{1}{2}i\pi t} \quad -e^{-\frac{1}{2}i\pi(t+1)}$   |
|                                                          | $c_2$                                | $-ie^{-\frac{1}{2}i\pi t} \quad e^{-\frac{1}{2}i\pi(t+1)}$                                                                                                                                                                                                                               |
|                                                          | $c_3$                                | $ie^{-\frac{1}{2}i\pi t} \quad -e^{-\frac{1}{2}i\pi(t+1)}$                                                                                                                                                                                                                               |
|                                                          | $c_4$                                | $ie^{-\frac{1}{2}i\pi t} \quad e^{-\frac{1}{2}i\pi(t+1)}$                                                                                                                                                                                                                                |
| $d \left(\frac{1-t}{2}, \frac{1}{2}, 0\right)$           | $d_1$                                | $\left\{2_{100} \left  \begin{smallmatrix} \frac{1}{2} & \frac{1}{2} & 0 \end{smallmatrix} \right. \right\} \left\{m_{010} \left  \begin{smallmatrix} 0 & \frac{1}{2} & \frac{1}{2} \end{smallmatrix} \right. \right\}$<br>0                                                             |
| $e \left(\frac{t}{2}, 0, \frac{1}{2}\right)$             | $e_1$                                | $\left\{2_{100} \left  \begin{smallmatrix} \frac{1}{2} & \frac{1}{2} & 0 \end{smallmatrix} \right. \right\} \left\{m_{010} \left  \begin{smallmatrix} 0 & \frac{1}{2} & \frac{1}{2} \end{smallmatrix} \right. \right\}$<br>$-ie^{-\frac{1}{2}i\pi t} \quad -1$                           |
|                                                          | $e_2$                                | $-ie^{-\frac{1}{2}i\pi t} \quad 1$                                                                                                                                                                                                                                                       |
|                                                          | $e_3$                                | $ie^{-\frac{1}{2}i\pi t} \quad -1$                                                                                                                                                                                                                                                       |
|                                                          | $e_4$                                | $ie^{-\frac{1}{2}i\pi t} \quad 1$                                                                                                                                                                                                                                                        |
| $f \left(0, \frac{t}{2}, \frac{1}{2}\right)$             | $f_1$                                | $\left\{2_{010} \left  \begin{smallmatrix} 0 & \frac{1}{2} & \frac{1}{2} \end{smallmatrix} \right. \right\} \left\{m_{100} \left  \begin{smallmatrix} \frac{1}{2} & \frac{1}{2} & 0 \end{smallmatrix} \right. \right\}$<br>0                                                             |
| $g \left(\frac{1}{2}, \frac{t}{2}, \frac{1}{2}\right)$   | $g_1$                                | $\left\{2_{010} \left  \begin{smallmatrix} 0 & \frac{1}{2} & \frac{1}{2} \end{smallmatrix} \right. \right\} \left\{m_{100} \left  \begin{smallmatrix} \frac{1}{2} & \frac{1}{2} & 0 \end{smallmatrix} \right. \right\}$<br>$-e^{-\frac{1}{2}i\pi(t+1)} \quad -e^{-\frac{1}{2}i\pi(t+1)}$ |
|                                                          | $g_2$                                | $-e^{-\frac{1}{2}i\pi(t+1)} \quad e^{-\frac{1}{2}i\pi(t+1)}$                                                                                                                                                                                                                             |
|                                                          | $g_3$                                | $e^{-\frac{1}{2}i\pi(t+1)} \quad -e^{-\frac{1}{2}i\pi(t+1)}$                                                                                                                                                                                                                             |
|                                                          | $g_4$                                | $e^{-\frac{1}{2}i\pi(t+1)} \quad e^{-\frac{1}{2}i\pi(t+1)}$                                                                                                                                                                                                                              |
| $h \left(\frac{1-t}{2}, \frac{1}{2}, \frac{1}{2}\right)$ | $h_1$                                | $\left\{2_{100} \left  \begin{smallmatrix} \frac{1}{2} & \frac{1}{2} & 0 \end{smallmatrix} \right. \right\} \left\{m_{010} \left  \begin{smallmatrix} 0 & \frac{1}{2} & \frac{1}{2} \end{smallmatrix} \right. \right\}$<br>$-e^{-\frac{1}{2}i\pi(2-t)} \quad 1$                          |
|                                                          | $h_2$                                | $-e^{-\frac{1}{2}i\pi(2-t)} \quad -1$                                                                                                                                                                                                                                                    |
|                                                          | $h_3$                                | $e^{-\frac{1}{2}i\pi(2-t)} \quad 1$                                                                                                                                                                                                                                                      |
|                                                          | $h_4$                                | $e^{-\frac{1}{2}i\pi(2-t)} \quad -1$                                                                                                                                                                                                                                                     |
| $i \left(0, 0, \frac{t}{2}\right)$                       | $i_1$                                | $\left\{2_{001} \left  \begin{smallmatrix} \frac{1}{2} & 0 & \frac{1}{2} \end{smallmatrix} \right. \right\} \left\{m_{100} \left  \begin{smallmatrix} \frac{1}{2} & \frac{1}{2} & 0 \end{smallmatrix} \right. \right\}$<br>0                                                             |
| $j \left(\frac{1}{2}, 0, \frac{t}{2}\right)$             | $j_1$                                | $\left\{2_{001} \left  \begin{smallmatrix} \frac{1}{2} & 0 & \frac{1}{2} \end{smallmatrix} \right. \right\} \left\{m_{100} \left  \begin{smallmatrix} \frac{1}{2} & \frac{1}{2} & 0 \end{smallmatrix} \right. \right\}$<br>0                                                             |
| $k \left(\frac{1}{2}, \frac{1}{2}, \frac{t}{2}\right)$   | $k_1$                                | $\left\{2_{001} \left  \begin{smallmatrix} \frac{1}{2} & 0 & \frac{1}{2} \end{smallmatrix} \right. \right\} \left\{m_{100} \left  \begin{smallmatrix} \frac{1}{2} & \frac{1}{2} & 0 \end{smallmatrix} \right. \right\}$<br>$-e^{-\frac{1}{2}i\pi(t+1)} \quad 1$                          |
|                                                          | $k_2$                                | $-e^{-\frac{1}{2}i\pi(t+1)} \quad -1$                                                                                                                                                                                                                                                    |
|                                                          | $k_3$                                | $e^{-\frac{1}{2}i\pi(t+1)} \quad 1$                                                                                                                                                                                                                                                      |
|                                                          | $k_4$                                | $e^{-\frac{1}{2}i\pi(t+1)} \quad -1$                                                                                                                                                                                                                                                     |
| $l \left(0, \frac{1}{2}, \frac{t}{2}\right)$             | $l_1$                                | $\left\{2_{001} \left  \begin{smallmatrix} \frac{1}{2} & 0 & \frac{1}{2} \end{smallmatrix} \right. \right\} \left\{m_{100} \left  \begin{smallmatrix} \frac{1}{2} & \frac{1}{2} & 0 \end{smallmatrix} \right. \right\}$<br>$-ie^{-\frac{1}{2}i\pi t} \quad -1$                           |
|                                                          | $l_2$                                | $-ie^{-\frac{1}{2}i\pi t} \quad 1$                                                                                                                                                                                                                                                       |
|                                                          | $l_3$                                | $ie^{-\frac{1}{2}i\pi t} \quad -1$                                                                                                                                                                                                                                                       |
|                                                          | $l_4$                                | $ie^{-\frac{1}{2}i\pi t} \quad 1$                                                                                                                                                                                                                                                        |

$$\begin{aligned}
\mathcal{W}_1^{\text{gapless}} = & \sum_{m=1}^{n_{a_1}} \text{sgn}(v_m^{a_1}) \frac{1 - \text{sgn}(\delta_m^{a_1})}{2} - 2 \sum_{m=1}^{n_{f_1}} \text{sgn}(v_m^{f_1}) \frac{1 - \text{sgn}(\delta_m^{f_1})}{2} + \sum_{m=1}^{n_{g_1}} \text{sgn}(v_m^{g_1}) \frac{1 - \text{sgn}(\delta_m^{g_1})}{2} \\
& + \sum_{m=1}^{n_{g_2}} \text{sgn}(v_m^{g_2}) \frac{1 - \text{sgn}(\delta_m^{g_2})}{2} + \sum_{m=1}^{n_{g_3}} \text{sgn}(v_m^{g_3}) \frac{1 - \text{sgn}(\delta_m^{g_3})}{2} + \sum_{m=1}^{n_{g_4}} \text{sgn}(v_m^{g_4}) \frac{1 - \text{sgn}(\delta_m^{g_4})}{2} \\
& + 2 \sum_{m=1}^{n_{h_2}} \text{sgn}(v_m^{h_2}) \frac{1 - \text{sgn}(\delta_m^{h_2})}{2} + 2 \sum_{m=1}^{n_{h_4}} \text{sgn}(v_m^{h_4}) \frac{1 - \text{sgn}(\delta_m^{h_4})}{2} \\
& - \sum_{m=1}^{n_{i_1}} \text{sgn}(v_m^{i_1}) \frac{1 - \text{sgn}(\delta_m^{i_1})}{2} + 2 \sum_{m=1}^{n_{j_1}} \text{sgn}(v_m^{j_1}) \frac{1 - \text{sgn}(\delta_m^{j_1})}{2} + \sum_{m=1}^{n_{k_1}} \text{sgn}(v_m^{k_1}) \frac{1 - \text{sgn}(\delta_m^{k_1})}{2} \\
& - \sum_{m=1}^{n_{k_2}} \text{sgn}(v_m^{k_2}) \frac{1 - \text{sgn}(\delta_m^{k_2})}{2} - \sum_{m=1}^{n_{k_3}} \text{sgn}(v_m^{k_3}) \frac{1 - \text{sgn}(\delta_m^{k_3})}{2} \\
& + \sum_{m=1}^{n_{k_4}} \text{sgn}(v_m^{k_4}) \frac{1 - \text{sgn}(\delta_m^{k_4})}{2} - \sum_{m=1}^{n_{l_1}} \text{sgn}(v_m^{l_1}) \frac{1 - \text{sgn}(\delta_m^{l_1})}{2} + \sum_{m=1}^{n_{l_2}} \text{sgn}(v_m^{l_2}) \frac{1 - \text{sgn}(\delta_m^{l_2})}{2}
\end{aligned} \tag{S61.1}$$

$$\begin{aligned}
\mathcal{W}_2^{\text{gapless}} = & \sum_{m=1}^{n_{b_1}} \text{sgn}(v_m^{b_1}) \frac{1 - \text{sgn}(\delta_m^{b_1})}{2} - 2 \sum_{m=1}^{n_{f_1}} \text{sgn}(v_m^{f_1}) \frac{1 - \text{sgn}(\delta_m^{f_1})}{2} - \sum_{m=1}^{n_{i_1}} \text{sgn}(v_m^{i_1}) \frac{1 - \text{sgn}(\delta_m^{i_1})}{2} \\
& + \sum_{m=1}^{n_{l_1}} \text{sgn}(v_m^{l_1}) \frac{1 - \text{sgn}(\delta_m^{l_1})}{2} + \sum_{m=1}^{n_{l_2}} \text{sgn}(v_m^{l_2}) \frac{1 - \text{sgn}(\delta_m^{l_2})}{2}
\end{aligned} \tag{S61.2}$$

$$\begin{aligned}
\mathcal{W}_3^{\text{gapless}} = & \sum_{m=1}^{n_{c_1}} \text{sgn}(v_m^{c_1}) \frac{1 - \text{sgn}(\delta_m^{c_1})}{2} - \sum_{m=1}^{n_{g_1}} \text{sgn}(v_m^{g_1}) \frac{1 - \text{sgn}(\delta_m^{g_1})}{2} - \sum_{m=1}^{n_{g_3}} \text{sgn}(v_m^{g_3}) \frac{1 - \text{sgn}(\delta_m^{g_3})}{2} \\
& - \sum_{m=1}^{n_{j_1}} \text{sgn}(v_m^{j_1}) \frac{1 - \text{sgn}(\delta_m^{j_1})}{2} + \sum_{m=1}^{n_{k_1}} \text{sgn}(v_m^{k_1}) \frac{1 - \text{sgn}(\delta_m^{k_1})}{2} + \sum_{m=1}^{n_{k_3}} \text{sgn}(v_m^{k_3}) \frac{1 - \text{sgn}(\delta_m^{k_3})}{2}
\end{aligned} \tag{S61.3}$$

$$\begin{aligned}
\mathcal{W}_4^{\text{gapless}} = & \sum_{m=1}^{n_{c_2}} \text{sgn}(v_m^{c_2}) \frac{1 - \text{sgn}(\delta_m^{c_2})}{2} - \sum_{m=1}^{n_{g_2}} \text{sgn}(v_m^{g_2}) \frac{1 - \text{sgn}(\delta_m^{g_2})}{2} - \sum_{m=1}^{n_{g_4}} \text{sgn}(v_m^{g_4}) \frac{1 - \text{sgn}(\delta_m^{g_4})}{2} \\
& - \sum_{m=1}^{n_{j_1}} \text{sgn}(v_m^{j_1}) \frac{1 - \text{sgn}(\delta_m^{j_1})}{2} + \sum_{m=1}^{n_{k_2}} \text{sgn}(v_m^{k_2}) \frac{1 - \text{sgn}(\delta_m^{k_2})}{2} + \sum_{m=1}^{n_{k_4}} \text{sgn}(v_m^{k_4}) \frac{1 - \text{sgn}(\delta_m^{k_4})}{2}
\end{aligned} \tag{S61.4}$$

$$\begin{aligned}
\mathcal{W}_5^{\text{gapless}} = & \sum_{m=1}^{n_{d_1}} \text{sgn}(v_m^{d_1}) \frac{1 - \text{sgn}(\delta_m^{d_1})}{2} - \sum_{m=1}^{n_{h_2}} \text{sgn}(v_m^{h_2}) \frac{1 - \text{sgn}(\delta_m^{h_2})}{2} - \sum_{m=1}^{n_{h_4}} \text{sgn}(v_m^{h_4}) \frac{1 - \text{sgn}(\delta_m^{h_4})}{2} \\
& - \sum_{m=1}^{n_{k_1}} \text{sgn}(v_m^{k_1}) \frac{1 - \text{sgn}(\delta_m^{k_1})}{2} - \sum_{m=1}^{n_{k_4}} \text{sgn}(v_m^{k_4}) \frac{1 - \text{sgn}(\delta_m^{k_4})}{2} + \sum_{m=1}^{n_{l_1}} \text{sgn}(v_m^{l_1}) \frac{1 - \text{sgn}(\delta_m^{l_1})}{2}
\end{aligned} \tag{S61.5}$$

$$\begin{aligned}
\mathcal{W}_6^{\text{gapless}} = & \sum_{m=1}^{n_{e_1}} \text{sgn}(v_m^{e_1}) \frac{1 - \text{sgn}(\delta_m^{e_1})}{2} - \sum_{m=1}^{n_{f_1}} \text{sgn}(v_m^{f_1}) \frac{1 - \text{sgn}(\delta_m^{f_1})}{2} + \sum_{m=1}^{n_{g_1}} \text{sgn}(v_m^{g_1}) \frac{1 - \text{sgn}(\delta_m^{g_1})}{2} + \sum_{m=1}^{n_{g_4}} \text{sgn}(v_m^{g_4}) \frac{1 - \text{sgn}(\delta_m^{g_4})}{2} \\
& + \sum_{m=1}^{n_{h_2}} \text{sgn}(v_m^{h_2}) \frac{1 - \text{sgn}(\delta_m^{h_2})}{2} - \sum_{m=1}^{n_{h_3}} \text{sgn}(v_m^{h_3}) \frac{1 - \text{sgn}(\delta_m^{h_3})}{2} + 2 \sum_{m=1}^{n_{h_4}} \text{sgn}(v_m^{h_4}) \frac{1 - \text{sgn}(\delta_m^{h_4})}{2} \\
& + \sum_{m=1}^{n_{k_1}} \text{sgn}(v_m^{k_1}) \frac{1 - \text{sgn}(\delta_m^{k_1})}{2} - \sum_{m=1}^{n_{k_2}} \text{sgn}(v_m^{k_2}) \frac{1 - \text{sgn}(\delta_m^{k_2})}{2} - \sum_{m=1}^{n_{k_3}} \text{sgn}(v_m^{k_3}) \frac{1 - \text{sgn}(\delta_m^{k_3})}{2} \\
& + \sum_{m=1}^{n_{k_4}} \text{sgn}(v_m^{k_4}) \frac{1 - \text{sgn}(\delta_m^{k_4})}{2} - \sum_{m=1}^{n_{l_1}} \text{sgn}(v_m^{l_1}) \frac{1 - \text{sgn}(\delta_m^{l_1})}{2} + \sum_{m=1}^{n_{l_2}} \text{sgn}(v_m^{l_2}) \frac{1 - \text{sgn}(\delta_m^{l_2})}{2}
\end{aligned} \tag{S61.6}$$

$$\begin{aligned}
\mathcal{W}_7^{\text{gapless}} = & \sum_{m=1}^{n_{e_2}} \text{sgn}(v_m^{e_2}) \frac{1 - \text{sgn}(\delta_m^{e_2})}{2} - \sum_{m=1}^{n_{f_1}} \text{sgn}(v_m^{f_1}) \frac{1 - \text{sgn}(\delta_m^{f_1})}{2} + \sum_{m=1}^{n_{g_2}} \text{sgn}(v_m^{g_2}) \frac{1 - \text{sgn}(\delta_m^{g_2})}{2} \\
& + \sum_{m=1}^{n_{g_3}} \text{sgn}(v_m^{g_3}) \frac{1 - \text{sgn}(\delta_m^{g_3})}{2} + \sum_{m=1}^{n_{h_2}} \text{sgn}(v_m^{h_2}) \frac{1 - \text{sgn}(\delta_m^{h_2})}{2} + \sum_{m=1}^{n_{h_3}} \text{sgn}(v_m^{h_3}) \frac{1 - \text{sgn}(\delta_m^{h_3})}{2}
\end{aligned} \tag{S61.7}$$

$$\begin{aligned}
\mathcal{W}_8^{\text{gapless}} = & \sum_{m=1}^{n_{h_1}} \text{sgn}(v_m^{h_1}) \frac{1 - \text{sgn}(\delta_m^{h_1})}{2} - \sum_{m=1}^{n_{h_2}} \text{sgn}(v_m^{h_2}) \frac{1 - \text{sgn}(\delta_m^{h_2})}{2} + \sum_{m=1}^{n_{h_3}} \text{sgn}(v_m^{h_3}) \frac{1 - \text{sgn}(\delta_m^{h_3})}{2} - \sum_{m=1}^{n_{h_4}} \text{sgn}(v_m^{h_4}) \frac{1 - \text{sgn}(\delta_m^{h_4})}{2} \\
& - \sum_{m=1}^{n_{k_1}} \text{sgn}(v_m^{k_1}) \frac{1 - \text{sgn}(\delta_m^{k_1})}{2} + \sum_{m=1}^{n_{k_2}} \text{sgn}(v_m^{k_2}) \frac{1 - \text{sgn}(\delta_m^{k_2})}{2} + \sum_{m=1}^{n_{k_3}} \text{sgn}(v_m^{k_3}) \frac{1 - \text{sgn}(\delta_m^{k_3})}{2} \\
& - \sum_{m=1}^{n_{k_4}} \text{sgn}(v_m^{k_4}) \frac{1 - \text{sgn}(\delta_m^{k_4})}{2} + \sum_{m=1}^{n_{l_1}} \text{sgn}(v_m^{l_1}) \frac{1 - \text{sgn}(\delta_m^{l_1})}{2} - \sum_{m=1}^{n_{l_2}} \text{sgn}(v_m^{l_2}) \frac{1 - \text{sgn}(\delta_m^{l_2})}{2}
\end{aligned} \tag{S61.8}$$

$$\begin{aligned}
\mathcal{X}_1 = & \sum_{m=1}^{n_{g_1}} \text{sgn}(v_m^{g_1}) \frac{1 - \text{sgn}(\delta_m^{g_1})}{2} + \sum_{m=1}^{n_{g_2}} \text{sgn}(v_m^{g_2}) \frac{1 - \text{sgn}(\delta_m^{g_2})}{2} - \sum_{m=1}^{n_{g_3}} \text{sgn}(v_m^{g_3}) \frac{1 - \text{sgn}(\delta_m^{g_3})}{2} \\
& - \sum_{m=1}^{n_{g_4}} \text{sgn}(v_m^{g_4}) \frac{1 - \text{sgn}(\delta_m^{g_4})}{2} + 2 \sum_{m=1}^{n_{h_3}} \text{sgn}(v_m^{h_3}) \frac{1 - \text{sgn}(\delta_m^{h_3})}{2} + 2 \sum_{m=1}^{n_{h_4}} \text{sgn}(v_m^{h_4}) \frac{1 - \text{sgn}(\delta_m^{h_4})}{2} \\
& + \sum_{m=1}^{n_{k_1}} \text{sgn}(v_m^{k_1}) \frac{1 - \text{sgn}(\delta_m^{k_1})}{2} + \sum_{m=1}^{n_{k_2}} \text{sgn}(v_m^{k_2}) \frac{1 - \text{sgn}(\delta_m^{k_2})}{2} - \sum_{m=1}^{n_{k_3}} \text{sgn}(v_m^{k_3}) \frac{1 - \text{sgn}(\delta_m^{k_3})}{2} \\
& - \sum_{m=1}^{n_{k_4}} \text{sgn}(v_m^{k_4}) \frac{1 - \text{sgn}(\delta_m^{k_4})}{2} + \sum_{m=1}^{n_{l_1}} \text{sgn}(v_m^{l_1}) \frac{1 - \text{sgn}(\delta_m^{l_1})}{2} - \sum_{m=1}^{n_{l_2}} \text{sgn}(v_m^{l_2}) \frac{1 - \text{sgn}(\delta_m^{l_2})}{2} \pmod{4}
\end{aligned} \tag{S61.9}$$

$$\begin{aligned}
\mathcal{X}_2 = & -2 \sum_{m=1}^{n_{g_2}} \text{sgn}(v_m^{g_2}) \frac{1 - \text{sgn}(\delta_m^{g_2})}{2} + 2 \sum_{m=1}^{n_{g_3}} \text{sgn}(v_m^{g_3}) \frac{1 - \text{sgn}(\delta_m^{g_3})}{2} - 2 \sum_{m=1}^{n_{h_2}} \text{sgn}(v_m^{h_2}) \frac{1 - \text{sgn}(\delta_m^{h_2})}{2} \\
& - 2 \sum_{m=1}^{n_{h_3}} \text{sgn}(v_m^{h_3}) \frac{1 - \text{sgn}(\delta_m^{h_3})}{2} - \sum_{m=1}^{n_{l_1}} \text{sgn}(v_m^{l_1}) \frac{1 - \text{sgn}(\delta_m^{l_1})}{2} + \sum_{m=1}^{n_{l_2}} \text{sgn}(v_m^{l_2}) \frac{1 - \text{sgn}(\delta_m^{l_2})}{2} \pmod{4}
\end{aligned} \tag{S61.10}$$

## S62. SPACE GROUP NO. 62

| line segment                                    | character of irrep (generators only) |                                                                                                                                                                        |
|-------------------------------------------------|--------------------------------------|------------------------------------------------------------------------------------------------------------------------------------------------------------------------|
| $a \ (\frac{t}{2}, 0, 0)$                       | $a_1$                                | $\{2_{100}   \frac{1}{2} \ \frac{1}{2} \ \frac{1}{2}\} \ \{m_{010}   0 \ \frac{1}{2} \ 0\}$<br>0                                                                       |
| $b \ (0, \frac{t}{2}, 0)$                       | $b_1$                                | $\{2_{010}   0 \ \frac{1}{2} \ 0\} \ \{m_{100}   \frac{1}{2} \ \frac{1}{2} \ \frac{1}{2}\}$<br>0                                                                       |
| $c \ (\frac{1-t}{2}, \frac{t}{2}, 0)$           | $c_1$                                | $\{2_{010}   0 \ \frac{1}{2} \ 0\} \ \{m_{100}   \frac{1}{2} \ \frac{1}{2} \ \frac{1}{2}\}$<br>$-ie^{-\frac{1}{2}i\pi t} \quad -e^{-\frac{1}{2}i\pi(t+1)}$             |
|                                                 | $c_2$                                | $-ie^{-\frac{1}{2}i\pi t} \quad e^{-\frac{1}{2}i\pi(t+1)}$                                                                                                             |
|                                                 | $c_3$                                | $ie^{-\frac{1}{2}i\pi t} \quad -e^{-\frac{1}{2}i\pi(t+1)}$                                                                                                             |
|                                                 | $c_4$                                | $ie^{-\frac{1}{2}i\pi t} \quad e^{-\frac{1}{2}i\pi(t+1)}$                                                                                                              |
| $d \ (\frac{1-t}{2}, \frac{1}{2}, 0)$           | $d_1$                                | $\{2_{100}   \frac{1}{2} \ \frac{1}{2} \ \frac{1}{2}\} \ \{m_{010}   0 \ \frac{1}{2} \ 0\}$<br>0                                                                       |
| $e \ (\frac{t}{2}, 0, \frac{1}{2})$             | $e_1$                                | $\{2_{100}   \frac{1}{2} \ \frac{1}{2} \ \frac{1}{2}\} \ \{m_{010}   0 \ \frac{1}{2} \ 0\}$<br>0                                                                       |
| $f \ (0, \frac{t}{2}, \frac{1}{2})$             | $f_1$                                | $\{2_{010}   0 \ \frac{1}{2} \ 0\} \ \{m_{100}   \frac{1}{2} \ \frac{1}{2} \ \frac{1}{2}\}$<br>$-ie^{-\frac{1}{2}i\pi t} \quad -ie^{-\frac{1}{2}i\pi(t+1)}$            |
|                                                 | $f_2$                                | $-ie^{-\frac{1}{2}i\pi t} \quad ie^{-\frac{1}{2}i\pi(t+1)}$                                                                                                            |
|                                                 | $f_3$                                | $ie^{-\frac{1}{2}i\pi t} \quad -ie^{-\frac{1}{2}i\pi(t+1)}$                                                                                                            |
|                                                 | $f_4$                                | $ie^{-\frac{1}{2}i\pi t} \quad ie^{-\frac{1}{2}i\pi(t+1)}$                                                                                                             |
| $g \ (\frac{1}{2}, \frac{t}{2}, \frac{1}{2})$   | $g_1$                                | $\{2_{010}   0 \ \frac{1}{2} \ 0\} \ \{m_{100}   \frac{1}{2} \ \frac{1}{2} \ \frac{1}{2}\}$<br>0                                                                       |
| $h \ (\frac{1-t}{2}, \frac{1}{2}, \frac{1}{2})$ | $h_1$                                | $\{2_{100}   \frac{1}{2} \ \frac{1}{2} \ \frac{1}{2}\} \ \{m_{010}   0 \ \frac{1}{2} \ 0\}$<br>0                                                                       |
| $i \ (0, 0, \frac{t}{2})$                       | $i_1$                                | $\{2_{001}   \frac{1}{2} \ 0 \ \frac{1}{2}\} \ \{m_{100}   \frac{1}{2} \ \frac{1}{2} \ \frac{1}{2}\}$<br>0                                                             |
| $j \ (\frac{1}{2}, 0, \frac{t}{2})$             | $j_1$                                | $\{2_{001}   \frac{1}{2} \ 0 \ \frac{1}{2}\} \ \{m_{100}   \frac{1}{2} \ \frac{1}{2} \ \frac{1}{2}\}$<br>0                                                             |
| $k \ (\frac{1}{2}, \frac{1}{2}, \frac{t}{2})$   | $k_1$                                | $\{2_{001}   \frac{1}{2} \ 0 \ \frac{1}{2}\} \ \{m_{100}   \frac{1}{2} \ \frac{1}{2} \ \frac{1}{2}\}$<br>$-e^{-\frac{1}{2}i\pi(t+1)} \quad -e^{-\frac{1}{2}i\pi(t+2)}$ |
|                                                 | $k_2$                                | $-e^{-\frac{1}{2}i\pi(t+1)} \quad e^{-\frac{1}{2}i\pi(t+2)}$                                                                                                           |
|                                                 | $k_3$                                | $e^{-\frac{1}{2}i\pi(t+1)} \quad -e^{-\frac{1}{2}i\pi(t+2)}$                                                                                                           |
|                                                 | $k_4$                                | $e^{-\frac{1}{2}i\pi(t+1)} \quad e^{-\frac{1}{2}i\pi(t+2)}$                                                                                                            |
| $l \ (0, \frac{1}{2}, \frac{t}{2})$             | $l_1$                                | $\{2_{001}   \frac{1}{2} \ 0 \ \frac{1}{2}\} \ \{m_{100}   \frac{1}{2} \ \frac{1}{2} \ \frac{1}{2}\}$<br>$-ie^{-\frac{1}{2}i\pi t} \quad -ie^{-\frac{1}{2}i\pi(t+1)}$  |
|                                                 | $l_2$                                | $-ie^{-\frac{1}{2}i\pi t} \quad ie^{-\frac{1}{2}i\pi(t+1)}$                                                                                                            |
|                                                 | $l_3$                                | $ie^{-\frac{1}{2}i\pi t} \quad -ie^{-\frac{1}{2}i\pi(t+1)}$                                                                                                            |
|                                                 | $l_4$                                | $ie^{-\frac{1}{2}i\pi t} \quad ie^{-\frac{1}{2}i\pi(t+1)}$                                                                                                             |

$$\begin{aligned}
\mathcal{W}_1^{\text{gapless}} = & \sum_{m=1}^{n_{a_1}} \text{sgn}(v_m^{a_1}) \frac{1 - \text{sgn}(\delta_m^{a_1})}{2} - 2 \sum_{m=1}^{n_{f_2}} \text{sgn}(v_m^{f_2}) \frac{1 - \text{sgn}(\delta_m^{f_2})}{2} + 2 \sum_{m=1}^{n_{g_1}} \text{sgn}(v_m^{g_1}) \frac{1 - \text{sgn}(\delta_m^{g_1})}{2} \\
& + 2 \sum_{m=1}^{n_{h_1}} \text{sgn}(v_m^{h_1}) \frac{1 - \text{sgn}(\delta_m^{h_1})}{2} - \sum_{m=1}^{n_{i_1}} \text{sgn}(v_m^{i_1}) \frac{1 - \text{sgn}(\delta_m^{i_1})}{2} + 2 \sum_{m=1}^{n_{j_1}} \text{sgn}(v_m^{j_1}) \frac{1 - \text{sgn}(\delta_m^{j_1})}{2}
\end{aligned} \tag{S62.1}$$

$$\begin{aligned}
\mathcal{W}_2^{\text{gapless}} = & \sum_{m=1}^{n_{b_1}} \text{sgn}(v_m^{b_1}) \frac{1 - \text{sgn}(\delta_m^{b_1})}{2} - 2 \sum_{m=1}^{n_{f_2}} \text{sgn}(v_m^{f_2}) \frac{1 - \text{sgn}(\delta_m^{f_2})}{2} - \sum_{m=1}^{n_{i_1}} \text{sgn}(v_m^{i_1}) \frac{1 - \text{sgn}(\delta_m^{i_1})}{2} \\
& + \sum_{m=1}^{n_{l_1}} \text{sgn}(v_m^{l_1}) \frac{1 - \text{sgn}(\delta_m^{l_1})}{2} + \sum_{m=1}^{n_{l_2}} \text{sgn}(v_m^{l_2}) \frac{1 - \text{sgn}(\delta_m^{l_2})}{2}
\end{aligned} \tag{S62.2}$$

$$\begin{aligned}
\mathcal{W}_3^{\text{gapless}} = & \sum_{m=1}^{n_{c_1}} \text{sgn}(v_m^{c_1}) \frac{1 - \text{sgn}(\delta_m^{c_1})}{2} - \sum_{m=1}^{n_{g_1}} \text{sgn}(v_m^{g_1}) \frac{1 - \text{sgn}(\delta_m^{g_1})}{2} - \sum_{m=1}^{n_{j_1}} \text{sgn}(v_m^{j_1}) \frac{1 - \text{sgn}(\delta_m^{j_1})}{2} \\
& + \sum_{m=1}^{n_{k_2}} \text{sgn}(v_m^{k_2}) \frac{1 - \text{sgn}(\delta_m^{k_2})}{2} + 2 \sum_{m=1}^{n_{k_3}} \text{sgn}(v_m^{k_3}) \frac{1 - \text{sgn}(\delta_m^{k_3})}{2} \\
& - \sum_{m=1}^{n_{k_4}} \text{sgn}(v_m^{k_4}) \frac{1 - \text{sgn}(\delta_m^{k_4})}{2} + \sum_{m=1}^{n_{l_1}} \text{sgn}(v_m^{l_1}) \frac{1 - \text{sgn}(\delta_m^{l_1})}{2} - \sum_{m=1}^{n_{l_2}} \text{sgn}(v_m^{l_2}) \frac{1 - \text{sgn}(\delta_m^{l_2})}{2}
\end{aligned} \tag{S62.3}$$

$$\begin{aligned}
\mathcal{W}_4^{\text{gapless}} = & \sum_{m=1}^{n_{c_2}} \text{sgn}(v_m^{c_2}) \frac{1 - \text{sgn}(\delta_m^{c_2})}{2} - \sum_{m=1}^{n_{g_1}} \text{sgn}(v_m^{g_1}) \frac{1 - \text{sgn}(\delta_m^{g_1})}{2} - \sum_{m=1}^{n_{j_1}} \text{sgn}(v_m^{j_1}) \frac{1 - \text{sgn}(\delta_m^{j_1})}{2} \\
& + \sum_{m=1}^{n_{k_2}} \text{sgn}(v_m^{k_2}) \frac{1 - \text{sgn}(\delta_m^{k_2})}{2} + \sum_{m=1}^{n_{k_4}} \text{sgn}(v_m^{k_4}) \frac{1 - \text{sgn}(\delta_m^{k_4})}{2}
\end{aligned} \tag{S62.4}$$

$$\begin{aligned}
\mathcal{W}_5^{\text{gapless}} = & \sum_{m=1}^{n_{d_1}} \text{sgn}(v_m^{d_1}) \frac{1 - \text{sgn}(\delta_m^{d_1})}{2} - \sum_{m=1}^{n_{h_1}} \text{sgn}(v_m^{h_1}) \frac{1 - \text{sgn}(\delta_m^{h_1})}{2} - \sum_{m=1}^{n_{k_2}} \text{sgn}(v_m^{k_2}) \frac{1 - \text{sgn}(\delta_m^{k_2})}{2} \\
& - \sum_{m=1}^{n_{k_3}} \text{sgn}(v_m^{k_3}) \frac{1 - \text{sgn}(\delta_m^{k_3})}{2} + \sum_{m=1}^{n_{l_2}} \text{sgn}(v_m^{l_2}) \frac{1 - \text{sgn}(\delta_m^{l_2})}{2}
\end{aligned} \tag{S62.5}$$

$$\begin{aligned}
\mathcal{W}_6^{\text{gapless}} = & \sum_{m=1}^{n_{e_1}} \text{sgn}(v_m^{e_1}) \frac{1 - \text{sgn}(\delta_m^{e_1})}{2} - \sum_{m=1}^{n_{f_2}} \text{sgn}(v_m^{f_2}) \frac{1 - \text{sgn}(\delta_m^{f_2})}{2} + \sum_{m=1}^{n_{g_1}} \text{sgn}(v_m^{g_1}) \frac{1 - \text{sgn}(\delta_m^{g_1})}{2} + \sum_{m=1}^{n_{h_1}} \text{sgn}(v_m^{h_1}) \frac{1 - \text{sgn}(\delta_m^{h_1})}{2}
\end{aligned} \tag{S62.6}$$

$$\mathcal{W}_7^{\text{gapless}} = \sum_{m=1}^{n_{f_1}} \text{sgn}(v_m^{f_1}) \frac{1 - \text{sgn}(\delta_m^{f_1})}{2} - \sum_{m=1}^{n_{f_2}} \text{sgn}(v_m^{f_2}) \frac{1 - \text{sgn}(\delta_m^{f_2})}{2} \tag{S62.7}$$

$$\begin{aligned}
\mathcal{W}_8^{\text{gapless}} = & \sum_{m=1}^{n_{k_1}} \text{sgn}(v_m^{k_1}) \frac{1 - \text{sgn}(\delta_m^{k_1})}{2} - \sum_{m=1}^{n_{k_2}} \text{sgn}(v_m^{k_2}) \frac{1 - \text{sgn}(\delta_m^{k_2})}{2} - \sum_{m=1}^{n_{k_3}} \text{sgn}(v_m^{k_3}) \frac{1 - \text{sgn}(\delta_m^{k_3})}{2} \\
& + \sum_{m=1}^{n_{k_4}} \text{sgn}(v_m^{k_4}) \frac{1 - \text{sgn}(\delta_m^{k_4})}{2} - \sum_{m=1}^{n_{l_1}} \text{sgn}(v_m^{l_1}) \frac{1 - \text{sgn}(\delta_m^{l_1})}{2} + \sum_{m=1}^{n_{l_2}} \text{sgn}(v_m^{l_2}) \frac{1 - \text{sgn}(\delta_m^{l_2})}{2}
\end{aligned} \tag{S62.8}$$

$$\mathcal{W}_1^{\text{gapped}} = - \sum_{m=1}^{n_{l_1}} \text{sgn}(v_m^{l_1}) \frac{1 - \text{sgn}(\delta_m^{l_1})}{2} + \sum_{m=1}^{n_{l_2}} \text{sgn}(v_m^{l_2}) \frac{1 - \text{sgn}(\delta_m^{l_2})}{2} \tag{S62.9}$$

### S63. SPACE GROUP NO. 63

|              |                                      |
|--------------|--------------------------------------|
| line segment | character of irrep (generators only) |
|--------------|--------------------------------------|

|                                                       |                                                                                                                                                                                                                                                                                          |
|-------------------------------------------------------|------------------------------------------------------------------------------------------------------------------------------------------------------------------------------------------------------------------------------------------------------------------------------------------|
| $a \quad (t, 0, 0)$                                   | $a_1 \quad \left\{ 2_{100} \middle  \begin{smallmatrix} 0 & 0 & 0 \\ 0 \end{smallmatrix} \right\} \quad \left\{ m_{010} \middle  \begin{smallmatrix} 0 & 0 & \frac{1}{2} \\ 0 \end{smallmatrix} \right\}$                                                                                |
| $b \quad (0, t, 0)$                                   | $b_1 \quad \left\{ 2_{010} \middle  \begin{smallmatrix} 0 & 0 & \frac{1}{2} \\ 0 \end{smallmatrix} \right\} \quad \left\{ m_{100} \middle  \begin{smallmatrix} 0 & 0 & 0 \\ 0 \end{smallmatrix} \right\}$                                                                                |
| $c \quad (\frac{t}{2}, 1 - \frac{t}{2}, 0)$           | $c_1 \quad \left\{ m_{001} \middle  \begin{smallmatrix} 0 & 0 & \frac{1}{2} \\ -i \end{smallmatrix} \right\}$<br>$c_2 \quad i$                                                                                                                                                           |
| $d \quad (t, 0, \frac{1}{2})$                         | $d_1 \quad \left\{ 2_{100} \middle  \begin{smallmatrix} 0 & 0 & 0 \\ -i \end{smallmatrix} \right\} \quad \left\{ m_{010} \middle  \begin{smallmatrix} 0 & 0 & \frac{1}{2} \\ -1 \end{smallmatrix} \right\}$<br>$d_2 \quad -i \quad 1$<br>$d_3 \quad i \quad -1$<br>$d_4 \quad i \quad 1$ |
| $e \quad (0, t, \frac{1}{2})$                         | $e_1 \quad \left\{ 2_{010} \middle  \begin{smallmatrix} 0 & 0 & \frac{1}{2} \\ 0 \end{smallmatrix} \right\} \quad \left\{ m_{100} \middle  \begin{smallmatrix} 0 & 0 & 0 \\ 0 \end{smallmatrix} \right\}$                                                                                |
| $f \quad (\frac{t}{2}, 1 - \frac{t}{2}, \frac{1}{2})$ | $f_1 \quad \left\{ m_{001} \middle  \begin{smallmatrix} 0 & 0 & \frac{1}{2} \\ i \end{smallmatrix} \right\}$<br>$f_2 \quad -i$                                                                                                                                                           |
| $g \quad (0, 0, \frac{t}{2})$                         | $g_1 \quad \left\{ 2_{001} \middle  \begin{smallmatrix} 0 & 0 & \frac{1}{2} \\ 0 \end{smallmatrix} \right\} \quad \left\{ m_{100} \middle  \begin{smallmatrix} 0 & 0 & 0 \\ 0 \end{smallmatrix} \right\}$                                                                                |
| $h \quad (1, 0, \frac{t}{2})$                         | $h_1 \quad \left\{ 2_{001} \middle  \begin{smallmatrix} 0 & 0 & \frac{1}{2} \\ 0 \end{smallmatrix} \right\} \quad \left\{ m_{100} \middle  \begin{smallmatrix} 0 & 0 & 0 \\ 0 \end{smallmatrix} \right\}$                                                                                |
| $i \quad (\frac{1}{2}, \frac{1}{2}, \frac{t}{2})$     | $i_1 \quad \left\{ 2_{001} \middle  \begin{smallmatrix} 0 & 0 & \frac{1}{2} \\ -ie^{-\frac{1}{2}i\pi t} \end{smallmatrix} \right\}$<br>$i_2 \quad ie^{-\frac{1}{2}i\pi t}$                                                                                                               |

$$\begin{aligned} \mathcal{W}_1^{\text{gapless}} = & \sum_{m=1}^{n_{a_1}} \text{sgn}(v_m^{a_1}) \frac{1 - \text{sgn}(\delta_m^{a_1})}{2} - 2 \sum_{m=1}^{n_{e_1}} \text{sgn}(v_m^{e_1}) \frac{1 - \text{sgn}(\delta_m^{e_1})}{2} - \sum_{m=1}^{n_{g_1}} \text{sgn}(v_m^{g_1}) \frac{1 - \text{sgn}(\delta_m^{g_1})}{2} \\ & + \sum_{m=1}^{n_{h_1}} \text{sgn}(v_m^{h_1}) \frac{1 - \text{sgn}(\delta_m^{h_1})}{2} \end{aligned} \quad (\text{S63.1})$$

$$\begin{aligned} \mathcal{W}_2^{\text{gapless}} = & \sum_{m=1}^{n_{b_1}} \text{sgn}(v_m^{b_1}) \frac{1 - \text{sgn}(\delta_m^{b_1})}{2} - 2 \sum_{m=1}^{n_{e_1}} \text{sgn}(v_m^{e_1}) \frac{1 - \text{sgn}(\delta_m^{e_1})}{2} - \sum_{m=1}^{n_{g_1}} \text{sgn}(v_m^{g_1}) \frac{1 - \text{sgn}(\delta_m^{g_1})}{2} \\ & + \sum_{m=1}^{n_{h_1}} \text{sgn}(v_m^{h_1}) \frac{1 - \text{sgn}(\delta_m^{h_1})}{2} \end{aligned} \quad (\text{S63.2})$$

$$\begin{aligned} \mathcal{W}_3^{\text{gapless}} = & \sum_{m=1}^{n_{c_1}} \text{sgn}(v_m^{c_1}) \frac{1 - \text{sgn}(\delta_m^{c_1})}{2} - \sum_{m=1}^{n_{f_1}} \text{sgn}(v_m^{f_1}) \frac{1 - \text{sgn}(\delta_m^{f_1})}{2} - \sum_{m=1}^{n_{f_2}} \text{sgn}(v_m^{f_2}) \frac{1 - \text{sgn}(\delta_m^{f_2})}{2} \\ & - \sum_{m=1}^{n_{h_1}} \text{sgn}(v_m^{h_1}) \frac{1 - \text{sgn}(\delta_m^{h_1})}{2} + \sum_{m=1}^{n_{i_1}} \text{sgn}(v_m^{i_1}) \frac{1 - \text{sgn}(\delta_m^{i_1})}{2} \end{aligned} \quad (\text{S63.3})$$

$$\begin{aligned} \mathcal{W}_4^{\text{gapless}} = & \sum_{m=1}^{n_{d_1}} \text{sgn}(v_m^{d_1}) \frac{1 - \text{sgn}(\delta_m^{d_1})}{2} - \sum_{m=1}^{n_{e_1}} \text{sgn}(v_m^{e_1}) \frac{1 - \text{sgn}(\delta_m^{e_1})}{2} + \sum_{m=1}^{n_{f_1}} \text{sgn}(v_m^{f_1}) \frac{1 - \text{sgn}(\delta_m^{f_1})}{2} - \sum_{m=1}^{n_{f_2}} \text{sgn}(v_m^{f_2}) \frac{1 - \text{sgn}(\delta_m^{f_2})}{2} \end{aligned} \quad (\text{S63.4})$$



$$\mathcal{W}_5^{\text{gapless}} = \sum_{m=1}^{n_{d_2}} \text{sgn}(v_m^{d_2}) \frac{1 - \text{sgn}(\delta_m^{d_2})}{2} - \sum_{m=1}^{n_{e_1}} \text{sgn}(v_m^{e_1}) \frac{1 - \text{sgn}(\delta_m^{e_1})}{2} - \sum_{m=1}^{n_{f_1}} \text{sgn}(v_m^{f_1}) \frac{1 - \text{sgn}(\delta_m^{f_1})}{2} + \sum_{m=1}^{n_{f_2}} \text{sgn}(v_m^{f_2}) \frac{1 - \text{sgn}(\delta_m^{f_2})}{2} \quad (\text{S63.5})$$

$$\mathcal{W}_1^{\text{gapped}} = - \sum_{m=1}^{n_{f_1}} \text{sgn}(v_m^{f_1}) \frac{1 - \text{sgn}(\delta_m^{f_1})}{2} + \sum_{m=1}^{n_{f_2}} \text{sgn}(v_m^{f_2}) \frac{1 - \text{sgn}(\delta_m^{f_2})}{2} \quad (\text{S63.6})$$

#### S64. SPACE GROUP NO. 64

| line segment                                      | character of irrep (generators only)                                                                                                                                                                                                                                                                                                                                                                                                                                                                                     |
|---------------------------------------------------|--------------------------------------------------------------------------------------------------------------------------------------------------------------------------------------------------------------------------------------------------------------------------------------------------------------------------------------------------------------------------------------------------------------------------------------------------------------------------------------------------------------------------|
| $a \ (t, 0, 0)$                                   | $a_1 \ \begin{Bmatrix} \{2_{100}   0 \ 0 \ 0\} \\ 0 \end{Bmatrix} \ \begin{Bmatrix} \{m_{010}   \frac{1}{2} \ 0 \ \frac{1}{2}\} \\ 0 \end{Bmatrix}$                                                                                                                                                                                                                                                                                                                                                                      |
| $b \ (0, t, 0)$                                   | $b_1 \ \begin{Bmatrix} \{2_{010}   \frac{1}{2} \ 0 \ \frac{1}{2}\} \\ 0 \end{Bmatrix} \ \begin{Bmatrix} \{m_{100}   0 \ 0 \ 0\} \\ 0 \end{Bmatrix}$                                                                                                                                                                                                                                                                                                                                                                      |
| $c \ (\frac{t}{2}, 1 - \frac{t}{2}, 0)$           | $c_1 \ \begin{Bmatrix} \{m_{001}   \frac{1}{2} \ 0 \ \frac{1}{2}\} \\ -ie^{-\frac{1}{2}i\pi t} \end{Bmatrix}$<br>$c_2 \ \begin{Bmatrix} \\ ie^{-\frac{1}{2}i\pi t} \end{Bmatrix}$                                                                                                                                                                                                                                                                                                                                        |
| $d \ (t, 0, \frac{1}{2})$                         | $d_1 \ \begin{Bmatrix} \{2_{100}   0 \ 0 \ 0\} \\ -i \end{Bmatrix} \ \begin{Bmatrix} \{m_{010}   \frac{1}{2} \ 0 \ \frac{1}{2}\} \\ -ie^{-\frac{1}{2}i\pi(2t+1)} \end{Bmatrix}$<br>$d_2 \ \begin{Bmatrix} \\ -i \end{Bmatrix} \ \begin{Bmatrix} \\ ie^{-\frac{1}{2}i\pi(2t+1)} \end{Bmatrix}$<br>$d_3 \ \begin{Bmatrix} \\ i \end{Bmatrix} \ \begin{Bmatrix} \\ -ie^{-\frac{1}{2}i\pi(2t+1)} \end{Bmatrix}$<br>$d_4 \ \begin{Bmatrix} \\ i \end{Bmatrix} \ \begin{Bmatrix} \\ ie^{-\frac{1}{2}i\pi(2t+1)} \end{Bmatrix}$ |
| $e \ (0, t, \frac{1}{2})$                         | $e_1 \ \begin{Bmatrix} \{2_{010}   \frac{1}{2} \ 0 \ \frac{1}{2}\} \\ 0 \end{Bmatrix} \ \begin{Bmatrix} \{m_{100}   0 \ 0 \ 0\} \\ 0 \end{Bmatrix}$                                                                                                                                                                                                                                                                                                                                                                      |
| $f \ (\frac{t}{2}, 1 - \frac{t}{2}, \frac{1}{2})$ | $f_1 \ \begin{Bmatrix} \{m_{001}   \frac{1}{2} \ 0 \ \frac{1}{2}\} \\ -e^{-\frac{1}{2}i\pi(t+1)} \end{Bmatrix}$<br>$f_2 \ \begin{Bmatrix} \\ e^{-\frac{1}{2}i\pi(t+1)} \end{Bmatrix}$                                                                                                                                                                                                                                                                                                                                    |
| $g \ (0, 0, \frac{t}{2})$                         | $g_1 \ \begin{Bmatrix} \{2_{001}   \frac{1}{2} \ 0 \ \frac{1}{2}\} \\ 0 \end{Bmatrix} \ \begin{Bmatrix} \{m_{100}   0 \ 0 \ 0\} \\ 0 \end{Bmatrix}$                                                                                                                                                                                                                                                                                                                                                                      |
| $h \ (1, 0, \frac{t}{2})$                         | $h_1 \ \begin{Bmatrix} \{2_{001}   \frac{1}{2} \ 0 \ \frac{1}{2}\} \\ 0 \end{Bmatrix} \ \begin{Bmatrix} \{m_{100}   0 \ 0 \ 0\} \\ 0 \end{Bmatrix}$                                                                                                                                                                                                                                                                                                                                                                      |
| $i \ (\frac{1}{2}, \frac{1}{2}, \frac{t}{2})$     | $i_1 \ \begin{Bmatrix} \{2_{001}   \frac{1}{2} \ 0 \ \frac{1}{2}\} \\ -e^{-\frac{1}{2}i\pi(t+1)} \end{Bmatrix}$<br>$i_2 \ \begin{Bmatrix} \\ e^{-\frac{1}{2}i\pi(t+1)} \end{Bmatrix}$                                                                                                                                                                                                                                                                                                                                    |

$$\mathcal{W}_1^{\text{gapless}} = \sum_{m=1}^{n_{a_1}} \text{sgn}(v_m^{a_1}) \frac{1 - \text{sgn}(\delta_m^{a_1})}{2} - 2 \sum_{m=1}^{n_{e_1}} \text{sgn}(v_m^{e_1}) \frac{1 - \text{sgn}(\delta_m^{e_1})}{2} - \sum_{m=1}^{n_{g_1}} \text{sgn}(v_m^{g_1}) \frac{1 - \text{sgn}(\delta_m^{g_1})}{2} + \sum_{m=1}^{n_{h_1}} \text{sgn}(v_m^{h_1}) \frac{1 - \text{sgn}(\delta_m^{h_1})}{2} \quad (\text{S64.1})$$

$$\mathcal{W}_2^{\text{gapless}} = \sum_{m=1}^{n_{b_1}} \text{sgn}(v_m^{b_1}) \frac{1 - \text{sgn}(\delta_m^{b_1})}{2} - 2 \sum_{m=1}^{n_{e_1}} \text{sgn}(v_m^{e_1}) \frac{1 - \text{sgn}(\delta_m^{e_1})}{2} - \sum_{m=1}^{n_{g_1}} \text{sgn}(v_m^{g_1}) \frac{1 - \text{sgn}(\delta_m^{g_1})}{2} + \sum_{m=1}^{n_{h_1}} \text{sgn}(v_m^{h_1}) \frac{1 - \text{sgn}(\delta_m^{h_1})}{2} \quad (\text{S64.2})$$

$$\begin{aligned} \mathcal{W}_3^{\text{gapless}} = & \sum_{m=1}^{n_{c_1}} \text{sgn}(v_m^{c_1}) \frac{1 - \text{sgn}(\delta_m^{c_1})}{2} - \sum_{m=1}^{n_{f_1}} \text{sgn}(v_m^{f_1}) \frac{1 - \text{sgn}(\delta_m^{f_1})}{2} - \sum_{m=1}^{n_{f_2}} \text{sgn}(v_m^{f_2}) \frac{1 - \text{sgn}(\delta_m^{f_2})}{2} \\ & - \sum_{m=1}^{n_{h_1}} \text{sgn}(v_m^{h_1}) \frac{1 - \text{sgn}(\delta_m^{h_1})}{2} + \sum_{m=1}^{n_{i_1}} \text{sgn}(v_m^{i_1}) \frac{1 - \text{sgn}(\delta_m^{i_1})}{2} + \sum_{m=1}^{n_{i_2}} \text{sgn}(v_m^{i_2}) \frac{1 - \text{sgn}(\delta_m^{i_2})}{2} \end{aligned} \quad (\text{S64.3})$$

$$\mathcal{W}_4^{\text{gapless}} = \sum_{m=1}^{n_{d_1}} \text{sgn}(v_m^{d_1}) \frac{1 - \text{sgn}(\delta_m^{d_1})}{2} - \sum_{m=1}^{n_{e_1}} \text{sgn}(v_m^{e_1}) \frac{1 - \text{sgn}(\delta_m^{e_1})}{2} \quad (\text{S64.4})$$

$$\mathcal{W}_5^{\text{gapless}} = \sum_{m=1}^{n_{d_2}} \text{sgn}(v_m^{d_2}) \frac{1 - \text{sgn}(\delta_m^{d_2})}{2} - \sum_{m=1}^{n_{e_1}} \text{sgn}(v_m^{e_1}) \frac{1 - \text{sgn}(\delta_m^{e_1})}{2} \quad (\text{S64.5})$$

$$\mathcal{X}_1 = \sum_{m=1}^{n_{f_1}} \frac{1 - \text{sgn}(\delta_m^{f_1})}{2} + \sum_{m=1}^{n_{f_2}} \frac{1 - \text{sgn}(\delta_m^{f_2})}{2} + \sum_{m=1}^{n_{i_1}} \frac{1 - \text{sgn}(\delta_m^{i_1})}{2} + \sum_{m=1}^{n_{i_2}} \frac{1 - \text{sgn}(\delta_m^{i_2})}{2} \mod 2 \quad (\text{S64.6})$$

### S65. SPACE GROUP NO. 65

| line segment                                      | character of irrep (generators only)                                                                                        |
|---------------------------------------------------|-----------------------------------------------------------------------------------------------------------------------------|
| $a \ (t, 0, 0)$                                   | $a_1 \begin{Bmatrix} \{2_{100}   0 \ 0 \ 0\} \\ 0 \end{Bmatrix} \begin{Bmatrix} \{m_{010}   0 \ 0 \ 0\} \\ 0 \end{Bmatrix}$ |
| $b \ (0, t, 0)$                                   | $b_1 \begin{Bmatrix} \{2_{010}   0 \ 0 \ 0\} \\ 0 \end{Bmatrix} \begin{Bmatrix} \{m_{100}   0 \ 0 \ 0\} \\ 0 \end{Bmatrix}$ |
| $c \ (\frac{t}{2}, 1 - \frac{t}{2}, 0)$           | $\begin{matrix} c_1 \\ c_2 \end{matrix} \begin{Bmatrix} \{m_{001}   0 \ 0 \ 0\} \\ -i \\ i \end{Bmatrix}$                   |
| $d \ (t, 0, \frac{1}{2})$                         | $d_1 \begin{Bmatrix} \{2_{100}   0 \ 0 \ 0\} \\ 0 \end{Bmatrix} \begin{Bmatrix} \{m_{010}   0 \ 0 \ 0\} \\ 0 \end{Bmatrix}$ |
| $e \ (0, t, \frac{1}{2})$                         | $e_1 \begin{Bmatrix} \{2_{010}   0 \ 0 \ 0\} \\ 0 \end{Bmatrix} \begin{Bmatrix} \{m_{100}   0 \ 0 \ 0\} \\ 0 \end{Bmatrix}$ |
| $f \ (\frac{t}{2}, 1 - \frac{t}{2}, \frac{1}{2})$ | $\begin{matrix} f_1 \\ f_2 \end{matrix} \begin{Bmatrix} \{m_{001}   0 \ 0 \ 0\} \\ -i \\ i \end{Bmatrix}$                   |
| $g \ (0, 0, \frac{t}{2})$                         | $g_1 \begin{Bmatrix} \{2_{001}   0 \ 0 \ 0\} \\ 0 \end{Bmatrix} \begin{Bmatrix} \{m_{100}   0 \ 0 \ 0\} \\ 0 \end{Bmatrix}$ |
| $h \ (1, 0, \frac{t}{2})$                         | $h_1 \begin{Bmatrix} \{2_{001}   0 \ 0 \ 0\} \\ 0 \end{Bmatrix} \begin{Bmatrix} \{m_{100}   0 \ 0 \ 0\} \\ 0 \end{Bmatrix}$ |
| $i \ (\frac{1}{2}, \frac{1}{2}, \frac{t}{2})$     | $\begin{matrix} i_1 \\ i_2 \end{matrix} \begin{Bmatrix} \{2_{001}   0 \ 0 \ 0\} \\ -i \\ i \end{Bmatrix}$                   |

$$\mathcal{W}_1^{\text{gapless}} = \sum_{m=1}^{n_{a_1}} \text{sgn}(v_m^{a_1}) \frac{1 - \text{sgn}(\delta_m^{a_1})}{2} - \sum_{m=1}^{n_{e_1}} \text{sgn}(v_m^{e_1}) \frac{1 - \text{sgn}(\delta_m^{e_1})}{2} - \sum_{m=1}^{n_{g_1}} \text{sgn}(v_m^{g_1}) \frac{1 - \text{sgn}(\delta_m^{g_1})}{2} + \sum_{m=1}^{n_{h_1}} \text{sgn}(v_m^{h_1}) \frac{1 - \text{sgn}(\delta_m^{h_1})}{2} \quad (\text{S65.1})$$

$$\mathcal{W}_2^{\text{gapless}} = \sum_{m=1}^{n_{b_1}} \text{sgn}(v_m^{b_1}) \frac{1 - \text{sgn}(\delta_m^{b_1})}{2} - \sum_{m=1}^{n_{e_1}} \text{sgn}(v_m^{e_1}) \frac{1 - \text{sgn}(\delta_m^{e_1})}{2} - \sum_{m=1}^{n_{g_1}} \text{sgn}(v_m^{g_1}) \frac{1 - \text{sgn}(\delta_m^{g_1})}{2} + \sum_{m=1}^{n_{h_1}} \text{sgn}(v_m^{h_1}) \frac{1 - \text{sgn}(\delta_m^{h_1})}{2} \quad (\text{S65.2})$$

$$\mathcal{W}_3^{\text{gapless}} = \sum_{m=1}^{n_{c_1}} \text{sgn}(v_m^{c_1}) \frac{1 - \text{sgn}(\delta_m^{c_1})}{2} - \sum_{m=1}^{n_{f_1}} \text{sgn}(v_m^{f_1}) \frac{1 - \text{sgn}(\delta_m^{f_1})}{2} - \sum_{m=1}^{n_{h_1}} \text{sgn}(v_m^{h_1}) \frac{1 - \text{sgn}(\delta_m^{h_1})}{2} + \sum_{m=1}^{n_{i_1}} \text{sgn}(v_m^{i_1}) \frac{1 - \text{sgn}(\delta_m^{i_1})}{2} \quad (\text{S65.3})$$

$$\mathcal{W}_4^{\text{gapless}} = \sum_{m=1}^{n_{d_1}} \text{sgn}(v_m^{d_1}) \frac{1 - \text{sgn}(\delta_m^{d_1})}{2} - \sum_{m=1}^{n_{e_1}} \text{sgn}(v_m^{e_1}) \frac{1 - \text{sgn}(\delta_m^{e_1})}{2} \quad (\text{S65.4})$$

### S66. SPACE GROUP NO. 66

| line segment                                          | character of irrep (generators only)                                                                                                                                                                                                              |
|-------------------------------------------------------|---------------------------------------------------------------------------------------------------------------------------------------------------------------------------------------------------------------------------------------------------|
| $a \quad (t, 0, 0)$                                   | $a_1 \quad \begin{Bmatrix} \{2_{100}   0 & 0 & \frac{1}{2}\} \\ 0 \end{Bmatrix} \quad \begin{Bmatrix} \{m_{010}   0 & 0 & \frac{1}{2}\} \\ 0 \end{Bmatrix}$                                                                                       |
| $b \quad (0, t, 0)$                                   | $b_1 \quad \begin{Bmatrix} \{2_{010}   0 & 0 & \frac{1}{2}\} \\ 0 \end{Bmatrix} \quad \begin{Bmatrix} \{m_{100}   0 & 0 & \frac{1}{2}\} \\ 0 \end{Bmatrix}$                                                                                       |
| $c \quad (\frac{t}{2}, 1 - \frac{t}{2}, 0)$           | $c_1 \quad \begin{Bmatrix} \{m_{001}   0 & 0 & 0\} \\ -i \end{Bmatrix}$<br>$c_2 \quad \begin{Bmatrix} i \end{Bmatrix}$                                                                                                                            |
| $d \quad (t, 0, \frac{1}{2})$                         | $d_1 \quad \begin{Bmatrix} \{2_{100}   0 & 0 & \frac{1}{2}\} \\ i & -1 \end{Bmatrix}$<br>$d_2 \quad \begin{Bmatrix} i & 1 \end{Bmatrix}$<br>$d_3 \quad \begin{Bmatrix} -i & -1 \end{Bmatrix}$<br>$d_4 \quad \begin{Bmatrix} -i & 1 \end{Bmatrix}$ |
| $e \quad (0, t, \frac{1}{2})$                         | $e_1 \quad \begin{Bmatrix} \{2_{010}   0 & 0 & \frac{1}{2}\} \\ i & -1 \end{Bmatrix}$<br>$e_2 \quad \begin{Bmatrix} i & 1 \end{Bmatrix}$<br>$e_3 \quad \begin{Bmatrix} -i & -1 \end{Bmatrix}$<br>$e_4 \quad \begin{Bmatrix} -i & 1 \end{Bmatrix}$ |
| $f \quad (\frac{t}{2}, 1 - \frac{t}{2}, \frac{1}{2})$ | $f_1 \quad \begin{Bmatrix} \{m_{001}   0 & 0 & 0\} \\ -i \end{Bmatrix}$<br>$f_2 \quad \begin{Bmatrix} i \end{Bmatrix}$                                                                                                                            |
| $g \quad (0, 0, \frac{t}{2})$                         | $g_1 \quad \begin{Bmatrix} \{2_{001}   0 & 0 & 0\} \\ 0 \end{Bmatrix} \quad \begin{Bmatrix} \{m_{100}   0 & 0 & \frac{1}{2}\} \\ 0 \end{Bmatrix}$                                                                                                 |
| $h \quad (1, 0, \frac{t}{2})$                         | $h_1 \quad \begin{Bmatrix} \{2_{001}   0 & 0 & 0\} \\ 0 \end{Bmatrix} \quad \begin{Bmatrix} \{m_{100}   0 & 0 & \frac{1}{2}\} \\ 0 \end{Bmatrix}$                                                                                                 |
| $i \quad (\frac{1}{2}, \frac{1}{2}, \frac{t}{2})$     | $i_1 \quad \begin{Bmatrix} \{2_{001}   0 & 0 & 0\} \\ -i \end{Bmatrix}$<br>$i_2 \quad \begin{Bmatrix} i \end{Bmatrix}$                                                                                                                            |

$$\mathcal{W}_1^{\text{gapless}} = \sum_{m=1}^{n_{a_1}} \text{sgn}(v_m^{a_1}) \frac{1 - \text{sgn}(\delta_m^{a_1})}{2} - \sum_{m=1}^{n_{e_1}} \text{sgn}(v_m^{e_1}) \frac{1 - \text{sgn}(\delta_m^{e_1})}{2} - \sum_{m=1}^{n_{e_3}} \text{sgn}(v_m^{e_3}) \frac{1 - \text{sgn}(\delta_m^{e_3})}{2} - \sum_{m=1}^{n_{g_1}} \text{sgn}(v_m^{g_1}) \frac{1 - \text{sgn}(\delta_m^{g_1})}{2} + \sum_{m=1}^{n_{h_1}} \text{sgn}(v_m^{h_1}) \frac{1 - \text{sgn}(\delta_m^{h_1})}{2} \quad (\text{S66.1})$$

$$\begin{aligned} \mathcal{W}_2^{\text{gapless}} = & \sum_{m=1}^{n_{b_1}} \text{sgn}(v_m^{b_1}) \frac{1 - \text{sgn}(\delta_m^{b_1})}{2} - \sum_{m=1}^{n_{e_1}} \text{sgn}(v_m^{e_1}) \frac{1 - \text{sgn}(\delta_m^{e_1})}{2} - \sum_{m=1}^{n_{e_3}} \text{sgn}(v_m^{e_3}) \frac{1 - \text{sgn}(\delta_m^{e_3})}{2} \\ & - \sum_{m=1}^{n_{g_1}} \text{sgn}(v_m^{g_1}) \frac{1 - \text{sgn}(\delta_m^{g_1})}{2} + \sum_{m=1}^{n_{h_1}} \text{sgn}(v_m^{h_1}) \frac{1 - \text{sgn}(\delta_m^{h_1})}{2} \end{aligned} \quad (\text{S66.2})$$

$$\mathcal{W}_3^{\text{gapless}} = \sum_{m=1}^{n_{c_1}} \text{sgn}(v_m^{c_1}) \frac{1 - \text{sgn}(\delta_m^{c_1})}{2} - \sum_{m=1}^{n_{f_1}} \text{sgn}(v_m^{f_1}) \frac{1 - \text{sgn}(\delta_m^{f_1})}{2} - \sum_{m=1}^{n_{h_1}} \text{sgn}(v_m^{h_1}) \frac{1 - \text{sgn}(\delta_m^{h_1})}{2} + \sum_{m=1}^{n_{i_1}} \text{sgn}(v_m^{i_1}) \frac{1 - \text{sgn}(\delta_m^{i_1})}{2} \quad (\text{S66.3})$$

$$\mathcal{W}_4^{\text{gapless}} = \sum_{m=1}^{n_{d_1}} \text{sgn}(v_m^{d_1}) \frac{1 - \text{sgn}(\delta_m^{d_1})}{2} + \sum_{m=1}^{n_{d_3}} \text{sgn}(v_m^{d_3}) \frac{1 - \text{sgn}(\delta_m^{d_3})}{2} - \sum_{m=1}^{n_{e_1}} \text{sgn}(v_m^{e_1}) \frac{1 - \text{sgn}(\delta_m^{e_1})}{2} - \sum_{m=1}^{n_{e_3}} \text{sgn}(v_m^{e_3}) \frac{1 - \text{sgn}(\delta_m^{e_3})}{2} \quad (\text{S66.4})$$

$$\mathcal{W}_1^{\text{gapped}} = - \sum_{m=1}^{n_{d_3}} \text{sgn}(v_m^{d_3}) \frac{1 - \text{sgn}(\delta_m^{d_3})}{2} + \sum_{m=1}^{n_{e_1}} \text{sgn}(v_m^{e_1}) \frac{1 - \text{sgn}(\delta_m^{e_1})}{2} \quad (\text{S66.5})$$

$$\mathcal{W}_2^{\text{gapped}} = - \sum_{m=1}^{n_{d_3}} \text{sgn}(v_m^{d_3}) \frac{1 - \text{sgn}(\delta_m^{d_3})}{2} + \sum_{m=1}^{n_{e_3}} \text{sgn}(v_m^{e_3}) \frac{1 - \text{sgn}(\delta_m^{e_3})}{2} \quad (\text{S66.6})$$

### S67. SPACE GROUP NO. 67

| line segment                                          | character of irrep (generators only)                                                                                                                                                                                                            |
|-------------------------------------------------------|-------------------------------------------------------------------------------------------------------------------------------------------------------------------------------------------------------------------------------------------------|
| $a \quad (t, 0, 0)$                                   | $a_1 \quad \left\{ \begin{array}{c} 2_{100}   \begin{smallmatrix} 0 & 0 & 0 \\ 0 \end{smallmatrix} \end{array} \right\} \left\{ \begin{array}{c} m_{010}   \begin{smallmatrix} \frac{1}{2} & 0 & 0 \\ 0 \end{smallmatrix} \end{array} \right\}$ |
| $b \quad (0, t, 0)$                                   | $b_1 \quad \left\{ \begin{array}{c} 2_{010}   \begin{smallmatrix} \frac{1}{2} & 0 & 0 \\ 0 \end{smallmatrix} \end{array} \right\} \left\{ \begin{array}{c} m_{100}   \begin{smallmatrix} 0 & 0 & 0 \\ 0 \end{smallmatrix} \end{array} \right\}$ |
| $c \quad (\frac{t}{2}, 1 - \frac{t}{2}, 0)$           | $c_1 \quad \left\{ \begin{array}{c} m_{001}   \begin{smallmatrix} \frac{1}{2} & 0 & 0 \\ -ie^{-\frac{1}{2}i\pi t} \end{smallmatrix} \end{array} \right\}$<br>$c_2 \quad \left\{ \begin{array}{c} ie^{-\frac{1}{2}i\pi t} \end{array} \right\}$  |
| $d \quad (t, 0, \frac{1}{2})$                         | $d_1 \quad \left\{ \begin{array}{c} 2_{100}   \begin{smallmatrix} 0 & 0 & 0 \\ 0 \end{smallmatrix} \end{array} \right\} \left\{ \begin{array}{c} m_{010}   \begin{smallmatrix} \frac{1}{2} & 0 & 0 \\ 0 \end{smallmatrix} \end{array} \right\}$ |
| $e \quad (0, t, \frac{1}{2})$                         | $e_1 \quad \left\{ \begin{array}{c} 2_{010}   \begin{smallmatrix} \frac{1}{2} & 0 & 0 \\ 0 \end{smallmatrix} \end{array} \right\} \left\{ \begin{array}{c} m_{100}   \begin{smallmatrix} 0 & 0 & 0 \\ 0 \end{smallmatrix} \end{array} \right\}$ |
| $f \quad (\frac{t}{2}, 1 - \frac{t}{2}, \frac{1}{2})$ | $f_1 \quad \left\{ \begin{array}{c} m_{001}   \begin{smallmatrix} \frac{1}{2} & 0 & 0 \\ -ie^{-\frac{1}{2}i\pi t} \end{smallmatrix} \end{array} \right\}$<br>$f_2 \quad \left\{ \begin{array}{c} ie^{-\frac{1}{2}i\pi t} \end{array} \right\}$  |
| $g \quad (0, 0, \frac{t}{2})$                         | $g_1 \quad \left\{ \begin{array}{c} 2_{001}   \begin{smallmatrix} \frac{1}{2} & 0 & 0 \\ 0 \end{smallmatrix} \end{array} \right\} \left\{ \begin{array}{c} m_{100}   \begin{smallmatrix} 0 & 0 & 0 \\ 0 \end{smallmatrix} \end{array} \right\}$ |
| $h \quad (1, 0, \frac{t}{2})$                         | $h_1 \quad \left\{ \begin{array}{c} 2_{001}   \begin{smallmatrix} \frac{1}{2} & 0 & 0 \\ 0 \end{smallmatrix} \end{array} \right\} \left\{ \begin{array}{c} m_{100}   \begin{smallmatrix} 0 & 0 & 0 \\ 0 \end{smallmatrix} \end{array} \right\}$ |
| $i \quad (\frac{1}{2}, \frac{1}{2}, \frac{t}{2})$     | $i_1 \quad \left\{ \begin{array}{c} 2_{001}   \begin{smallmatrix} \frac{1}{2} & 0 & 0 \\ 1 \end{smallmatrix} \end{array} \right\}$<br>$i_2 \quad \left\{ \begin{array}{c} -i \end{array} \right\}$                                              |

$$\mathcal{W}_1^{\text{gapless}} = \sum_{m=1}^{n_{a_1}} \text{sgn}(v_m^{a_1}) \frac{1 - \text{sgn}(\delta_m^{a_1})}{2} - \sum_{m=1}^{n_{e_1}} \text{sgn}(v_m^{e_1}) \frac{1 - \text{sgn}(\delta_m^{e_1})}{2} - \sum_{m=1}^{n_{g_1}} \text{sgn}(v_m^{g_1}) \frac{1 - \text{sgn}(\delta_m^{g_1})}{2} + \sum_{m=1}^{n_{h_1}} \text{sgn}(v_m^{h_1}) \frac{1 - \text{sgn}(\delta_m^{h_1})}{2} \quad (\text{S67.1})$$

$$\mathcal{W}_2^{\text{gapless}} = \sum_{m=1}^{n_{b_1}} \text{sgn}(v_m^{b_1}) \frac{1 - \text{sgn}(\delta_m^{b_1})}{2} - \sum_{m=1}^{n_{e_1}} \text{sgn}(v_m^{e_1}) \frac{1 - \text{sgn}(\delta_m^{e_1})}{2} - \sum_{m=1}^{n_{g_1}} \text{sgn}(v_m^{g_1}) \frac{1 - \text{sgn}(\delta_m^{g_1})}{2} + \sum_{m=1}^{n_{h_1}} \text{sgn}(v_m^{h_1}) \frac{1 - \text{sgn}(\delta_m^{h_1})}{2} \quad (\text{S67.2})$$

$$\begin{aligned} \mathcal{W}_3^{\text{gapless}} = & \sum_{m=1}^{n_{c_1}} \text{sgn}(v_m^{c_1}) \frac{1 - \text{sgn}(\delta_m^{c_1})}{2} - \sum_{m=1}^{n_{f_1}} \text{sgn}(v_m^{f_1}) \frac{1 - \text{sgn}(\delta_m^{f_1})}{2} - \sum_{m=1}^{n_{h_1}} \text{sgn}(v_m^{h_1}) \frac{1 - \text{sgn}(\delta_m^{h_1})}{2} \\ & + \sum_{m=1}^{n_{i_1}} \text{sgn}(v_m^{i_1}) \frac{1 - \text{sgn}(\delta_m^{i_1})}{2} + \sum_{m=1}^{n_{i_2}} \text{sgn}(v_m^{i_2}) \frac{1 - \text{sgn}(\delta_m^{i_2})}{2} \end{aligned} \quad (\text{S67.3})$$

$$\mathcal{W}_4^{\text{gapless}} = \sum_{m=1}^{n_{d_1}} \text{sgn}(v_m^{d_1}) \frac{1 - \text{sgn}(\delta_m^{d_1})}{2} - \sum_{m=1}^{n_{e_1}} \text{sgn}(v_m^{e_1}) \frac{1 - \text{sgn}(\delta_m^{e_1})}{2} \quad (\text{S67.4})$$

$$\mathcal{W}_1^{\text{gapped}} = - \sum_{m=1}^{n_{i_1}} \text{sgn}(v_m^{i_1}) \frac{1 - \text{sgn}(\delta_m^{i_1})}{2} + \sum_{m=1}^{n_{i_2}} \text{sgn}(v_m^{i_2}) \frac{1 - \text{sgn}(\delta_m^{i_2})}{2} \quad (\text{S67.5})$$

### S68. SPACE GROUP NO. 68

| line segment                                          | character of irrep (generators only) |                                                                                                                                                                                                                                                                                     |
|-------------------------------------------------------|--------------------------------------|-------------------------------------------------------------------------------------------------------------------------------------------------------------------------------------------------------------------------------------------------------------------------------------|
| $a \quad (t, 0, 0)$                                   | $a_1$                                | $\begin{array}{cc} \{2_{100}   0 \ \frac{1}{2} \ \frac{1}{2}\} & \{m_{010}   \frac{1}{2} \ \frac{1}{2} \ \frac{1}{2}\} \\ 0 & 0 \end{array}$                                                                                                                                        |
| $b \quad (0, t, 0)$                                   | $b_1$                                | $\begin{array}{cc} \{2_{010}   0 \ 0 \ \frac{1}{2}\} & \{m_{100}   \frac{1}{2} \ 0 \ \frac{1}{2}\} \\ 0 & 0 \end{array}$                                                                                                                                                            |
| $c \quad (\frac{t}{2}, 1 - \frac{t}{2}, 0)$           | $c_1$<br>$c_2$                       | $\begin{array}{c} \{m_{001}   \frac{1}{2} \ 0 \ 0\} \\ -ie^{-\frac{1}{2}i\pi t} \\ ie^{-\frac{1}{2}i\pi t} \end{array}$                                                                                                                                                             |
| $d \quad (t, 0, \frac{1}{2})$                         | $d_1$<br>$d_2$<br>$d_3$<br>$d_4$     | $\begin{array}{cc} \{2_{100}   0 \ \frac{1}{2} \ \frac{1}{2}\} & \{m_{010}   \frac{1}{2} \ \frac{1}{2} \ \frac{1}{2}\} \\ i & -ie^{-\frac{1}{2}i\pi(2t+1)} \\ i & ie^{-\frac{1}{2}i\pi(2t+1)} \\ -i & -ie^{-\frac{1}{2}i\pi(2t+1)} \\ -i & ie^{-\frac{1}{2}i\pi(2t+1)} \end{array}$ |
| $e \quad (0, t, \frac{1}{2})$                         | $e_1$<br>$e_2$<br>$e_3$<br>$e_4$     | $\begin{array}{cc} \{2_{010}   0 \ 0 \ \frac{1}{2}\} & \{m_{100}   \frac{1}{2} \ 0 \ \frac{1}{2}\} \\ i & -1 \\ i & 1 \\ -i & -1 \\ -i & 1 \end{array}$                                                                                                                             |
| $f \quad (\frac{t}{2}, 1 - \frac{t}{2}, \frac{1}{2})$ | $f_1$<br>$f_2$                       | $\begin{array}{c} \{m_{001}   \frac{1}{2} \ 0 \ 0\} \\ -ie^{-\frac{1}{2}i\pi t} \\ ie^{-\frac{1}{2}i\pi t} \end{array}$                                                                                                                                                             |

|                                                   |                                                                                                                                                 |
|---------------------------------------------------|-------------------------------------------------------------------------------------------------------------------------------------------------|
| $g \quad (0, 0, \frac{t}{2})$                     | $g_1 \quad \left\{ 2_{001} \mid 0 \quad \frac{1}{2} \quad 0 \right\} \quad \left\{ m_{100} \mid \frac{1}{2} \quad 0 \quad \frac{1}{2} \right\}$ |
| $h \quad (1, 0, \frac{t}{2})$                     | $h_1 \quad \left\{ 2_{001} \mid 0 \quad \frac{1}{2} \quad 0 \right\} \quad \left\{ m_{100} \mid \frac{1}{2} \quad 0 \quad \frac{1}{2} \right\}$ |
| $i \quad (\frac{1}{2}, \frac{1}{2}, \frac{t}{2})$ | $i_1 \quad i$<br>$i_2 \quad -i$                                                                                                                 |

$$\begin{aligned} \mathcal{W}_1^{\text{gapless}} = & \sum_{m=1}^{n_{a_1}} \text{sgn}(v_m^{a_1}) \frac{1 - \text{sgn}(\delta_m^{a_1})}{2} - \sum_{m=1}^{n_{e_1}} \text{sgn}(v_m^{e_1}) \frac{1 - \text{sgn}(\delta_m^{e_1})}{2} - \sum_{m=1}^{n_{e_3}} \text{sgn}(v_m^{e_3}) \frac{1 - \text{sgn}(\delta_m^{e_3})}{2} \\ & - \sum_{m=1}^{n_{g_1}} \text{sgn}(v_m^{g_1}) \frac{1 - \text{sgn}(\delta_m^{g_1})}{2} + \sum_{m=1}^{n_{h_1}} \text{sgn}(v_m^{h_1}) \frac{1 - \text{sgn}(\delta_m^{h_1})}{2} \end{aligned} \quad (\text{S68.1})$$

$$\begin{aligned} \mathcal{W}_2^{\text{gapless}} = & \sum_{m=1}^{n_{b_1}} \text{sgn}(v_m^{b_1}) \frac{1 - \text{sgn}(\delta_m^{b_1})}{2} - \sum_{m=1}^{n_{e_1}} \text{sgn}(v_m^{e_1}) \frac{1 - \text{sgn}(\delta_m^{e_1})}{2} - \sum_{m=1}^{n_{e_3}} \text{sgn}(v_m^{e_3}) \frac{1 - \text{sgn}(\delta_m^{e_3})}{2} \\ & - \sum_{m=1}^{n_{g_1}} \text{sgn}(v_m^{g_1}) \frac{1 - \text{sgn}(\delta_m^{g_1})}{2} + \sum_{m=1}^{n_{h_1}} \text{sgn}(v_m^{h_1}) \frac{1 - \text{sgn}(\delta_m^{h_1})}{2} \end{aligned} \quad (\text{S68.2})$$

$$\begin{aligned} \mathcal{W}_3^{\text{gapless}} = & \sum_{m=1}^{n_{c_1}} \text{sgn}(v_m^{c_1}) \frac{1 - \text{sgn}(\delta_m^{c_1})}{2} - \sum_{m=1}^{n_{f_1}} \text{sgn}(v_m^{f_1}) \frac{1 - \text{sgn}(\delta_m^{f_1})}{2} - \sum_{m=1}^{n_{h_1}} \text{sgn}(v_m^{h_1}) \frac{1 - \text{sgn}(\delta_m^{h_1})}{2} \\ & + \sum_{m=1}^{n_{i_1}} \text{sgn}(v_m^{i_1}) \frac{1 - \text{sgn}(\delta_m^{i_1})}{2} + \sum_{m=1}^{n_{i_2}} \text{sgn}(v_m^{i_2}) \frac{1 - \text{sgn}(\delta_m^{i_2})}{2} \end{aligned} \quad (\text{S68.3})$$

$$\begin{aligned} \mathcal{W}_4^{\text{gapless}} = & \sum_{m=1}^{n_{d_1}} \text{sgn}(v_m^{d_1}) \frac{1 - \text{sgn}(\delta_m^{d_1})}{2} + \sum_{m=1}^{n_{d_3}} \text{sgn}(v_m^{d_3}) \frac{1 - \text{sgn}(\delta_m^{d_3})}{2} - \sum_{m=1}^{n_{e_1}} \text{sgn}(v_m^{e_1}) \frac{1 - \text{sgn}(\delta_m^{e_1})}{2} - \sum_{m=1}^{n_{e_3}} \text{sgn}(v_m^{e_3}) \frac{1 - \text{sgn}(\delta_m^{e_3})}{2} \end{aligned} \quad (\text{S68.4})$$

$$\mathcal{W}_1^{\text{gapped}} = - \sum_{m=1}^{n_{d_3}} \text{sgn}(v_m^{d_3}) \frac{1 - \text{sgn}(\delta_m^{d_3})}{2} + \sum_{m=1}^{n_{e_1}} \text{sgn}(v_m^{e_1}) \frac{1 - \text{sgn}(\delta_m^{e_1})}{2} \quad (\text{S68.5})$$

$$\mathcal{W}_2^{\text{gapped}} = - \sum_{m=1}^{n_{d_3}} \text{sgn}(v_m^{d_3}) \frac{1 - \text{sgn}(\delta_m^{d_3})}{2} + \sum_{m=1}^{n_{e_3}} \text{sgn}(v_m^{e_3}) \frac{1 - \text{sgn}(\delta_m^{e_3})}{2} \quad (\text{S68.6})$$

$$\mathcal{W}_3^{\text{gapped}} = - \sum_{m=1}^{n_{i_1}} \text{sgn}(v_m^{i_1}) \frac{1 - \text{sgn}(\delta_m^{i_1})}{2} + \sum_{m=1}^{n_{i_2}} \text{sgn}(v_m^{i_2}) \frac{1 - \text{sgn}(\delta_m^{i_2})}{2} \quad (\text{S68.7})$$

$$\mathcal{X}_1 = \sum_{m=1}^{n_{f_1}} \frac{1 - \text{sgn}(\delta_m^{f_1})}{2} \quad \text{mod } 2 \quad (\text{S68.8})$$

**S69. SPACE GROUP NO. 69**

| line segment                                        | character of irrep (generators only)                                                                                      |
|-----------------------------------------------------|---------------------------------------------------------------------------------------------------------------------------|
| $a \ (t, 0, 0)$                                     | $a_1 \begin{Bmatrix} \{2_{100}  0 & 0 & 0\} \\ 0 \end{Bmatrix} \begin{Bmatrix} \{m_{010}  0 & 0 & 0\} \\ 0 \end{Bmatrix}$ |
| $b \ (1, t, 0)$                                     | $b_1 \begin{Bmatrix} \{2_{010}  0 & 0 & 0\} \\ 0 \end{Bmatrix} \begin{Bmatrix} \{m_{100}  0 & 0 & 0\} \\ 0 \end{Bmatrix}$ |
| $c \ (0, 0, 1-t)$                                   | $c_1 \begin{Bmatrix} \{2_{001}  0 & 0 & 0\} \\ 0 \end{Bmatrix} \begin{Bmatrix} \{m_{100}  0 & 0 & 0\} \\ 0 \end{Bmatrix}$ |
| $d \ (1-t, 1, 0)$                                   | $d_1 \begin{Bmatrix} \{2_{100}  0 & 0 & 0\} \\ 0 \end{Bmatrix} \begin{Bmatrix} \{m_{010}  0 & 0 & 0\} \\ 0 \end{Bmatrix}$ |
| $e \ (0, t, 0)$                                     | $e_1 \begin{Bmatrix} \{2_{010}  0 & 0 & 0\} \\ 0 \end{Bmatrix} \begin{Bmatrix} \{m_{100}  0 & 0 & 0\} \\ 0 \end{Bmatrix}$ |
| $f \ (0, 1, 1-t)$                                   | $f_1 \begin{Bmatrix} \{2_{001}  0 & 0 & 0\} \\ 0 \end{Bmatrix} \begin{Bmatrix} \{m_{100}  0 & 0 & 0\} \\ 0 \end{Bmatrix}$ |
| $g \ (1-t, 0, t)$                                   | $\begin{Bmatrix} \{m_{010}  0 & 0 & 0\} \\ -i \\ i \end{Bmatrix}$<br>$g_1$<br>$g_2$                                       |
| $h \ (\frac{t+1}{2}, \frac{1-t}{2}, \frac{1-t}{2})$ | $h_1 \begin{Bmatrix} \{1  0 & 0 & 0\} \\ 1 \end{Bmatrix}$                                                                 |

$$\mathcal{W}_1^{\text{gapless}} = \sum_{m=1}^{n_{a_1}} \text{sgn}(v_m^{a_1}) \frac{1 - \text{sgn}(\delta_m^{a_1})}{2} - \sum_{m=1}^{n_{e_1}} \text{sgn}(v_m^{e_1}) \frac{1 - \text{sgn}(\delta_m^{e_1})}{2} + \sum_{m=1}^{n_{f_1}} \text{sgn}(v_m^{f_1}) \frac{1 - \text{sgn}(\delta_m^{f_1})}{2} \quad (\text{S69.1})$$

$$\mathcal{W}_2^{\text{gapless}} = \sum_{m=1}^{n_{b_1}} \text{sgn}(v_m^{b_1}) \frac{1 - \text{sgn}(\delta_m^{b_1})}{2} - \sum_{m=1}^{n_{g_1}} \text{sgn}(v_m^{g_1}) \frac{1 - \text{sgn}(\delta_m^{g_1})}{2} \quad (\text{S69.2})$$

$$\mathcal{W}_3^{\text{gapless}} = \sum_{m=1}^{n_{c_1}} \text{sgn}(v_m^{c_1}) \frac{1 - \text{sgn}(\delta_m^{c_1})}{2} + \sum_{m=1}^{n_{e_1}} \text{sgn}(v_m^{e_1}) \frac{1 - \text{sgn}(\delta_m^{e_1})}{2} - \sum_{m=1}^{n_{f_1}} \text{sgn}(v_m^{f_1}) \frac{1 - \text{sgn}(\delta_m^{f_1})}{2} + \sum_{m=1}^{n_{g_1}} \text{sgn}(v_m^{g_1}) \frac{1 - \text{sgn}(\delta_m^{g_1})}{2} \quad (\text{S69.3})$$

$$\mathcal{W}_4^{\text{gapless}} = \sum_{m=1}^{n_{d_1}} \text{sgn}(v_m^{d_1}) \frac{1 - \text{sgn}(\delta_m^{d_1})}{2} - \sum_{m=1}^{n_{f_1}} \text{sgn}(v_m^{f_1}) \frac{1 - \text{sgn}(\delta_m^{f_1})}{2} + \sum_{m=1}^{n_{g_1}} \text{sgn}(v_m^{g_1}) \frac{1 - \text{sgn}(\delta_m^{g_1})}{2} \quad (\text{S69.4})$$

**S70. SPACE GROUP NO. 70**

| line segment      | character of irrep (generators only)                                                                                                                                                                                                                                                                                        |
|-------------------|-----------------------------------------------------------------------------------------------------------------------------------------------------------------------------------------------------------------------------------------------------------------------------------------------------------------------------|
| $a \ (t, 0, 0)$   | $a_1 \begin{Bmatrix} \{2_{100}  0 & \frac{3}{4} & \frac{3}{4}\} \\ 0 \end{Bmatrix} \begin{Bmatrix} \{m_{010}  \frac{1}{4} & 0 & \frac{1}{4}\} \\ 0 \end{Bmatrix}$                                                                                                                                                           |
| $b \ (1, t, 0)$   | $\begin{Bmatrix} \{2_{010}  \frac{3}{4} & 0 & \frac{3}{4}\} \\ -i \\ -i \\ i \\ i \end{Bmatrix} \begin{Bmatrix} \{m_{100}  0 & \frac{1}{4} & \frac{1}{4}\} \\ -ie^{-\frac{1}{2}i\pi t} \\ ie^{-\frac{1}{2}i\pi t} \\ -ie^{-\frac{1}{2}i\pi t} \\ ie^{-\frac{1}{2}i\pi t} \end{Bmatrix}$<br>$b_1$<br>$b_2$<br>$b_3$<br>$b_4$ |
| $c \ (0, 0, 1-t)$ | $c_1 \begin{Bmatrix} \{2_{001}  \frac{3}{4} & \frac{3}{4} & 0\} \\ 0 \end{Bmatrix} \begin{Bmatrix} \{m_{100}  0 & \frac{1}{4} & \frac{1}{4}\} \\ 0 \end{Bmatrix}$                                                                                                                                                           |

|                                                         |                                                         |                                                                                                           |                                                                                                                                                                                                               |
|---------------------------------------------------------|---------------------------------------------------------|-----------------------------------------------------------------------------------------------------------|---------------------------------------------------------------------------------------------------------------------------------------------------------------------------------------------------------------|
| $d \quad (1-t, 1, 0)$                                   | $\begin{array}{l} d_1 \\ d_2 \\ d_3 \\ d_4 \end{array}$ | $\begin{array}{l} \{2_{100}   0 \quad \frac{3}{4} \quad \frac{3}{4} \} \\ -i \\ -i \\ i \\ i \end{array}$ | $\begin{array}{l} \{m_{010}   \frac{1}{4} \quad 0 \quad \frac{1}{4} \} \\ -ie^{-\frac{1}{2}i\pi(1-t)} \\ ie^{-\frac{1}{2}i\pi(1-t)} \\ -ie^{-\frac{1}{2}i\pi(1-t)} \\ ie^{-\frac{1}{2}i\pi(1-t)} \end{array}$ |
| $e \quad (0, t, 0)$                                     | $e_1$                                                   | $\begin{array}{l} \{2_{010}   \frac{3}{4} \quad 0 \quad \frac{3}{4} \} \\ 0 \end{array}$                  | $\begin{array}{l} \{m_{100}   0 \quad \frac{1}{4} \quad \frac{1}{4} \} \\ 0 \end{array}$                                                                                                                      |
| $f \quad (0, 1, 1-t)$                                   | $\begin{array}{l} f_1 \\ f_2 \\ f_3 \\ f_4 \end{array}$ | $\begin{array}{l} \{2_{001}   \frac{3}{4} \quad \frac{3}{4} \quad 0 \} \\ -i \\ -i \\ i \\ i \end{array}$ | $\begin{array}{l} \{m_{100}   0 \quad \frac{1}{4} \quad \frac{1}{4} \} \\ -ie^{-\frac{1}{2}i\pi(2-t)} \\ ie^{-\frac{1}{2}i\pi(2-t)} \\ -ie^{-\frac{1}{2}i\pi(2-t)} \\ ie^{-\frac{1}{2}i\pi(2-t)} \end{array}$ |
| $g \quad (1-t, 0, t)$                                   | $\begin{array}{l} g_1 \\ g_2 \end{array}$               | $\begin{array}{l} \{m_{010}   \frac{1}{4} \quad 0 \quad \frac{1}{4} \} \\ -1 \\ 1 \end{array}$            |                                                                                                                                                                                                               |
| $h \quad (\frac{t+1}{2}, \frac{1-t}{2}, \frac{1-t}{2})$ | $h_1$                                                   | $\begin{array}{l} \{1   0 \quad 0 \quad 0 \} \\ 1 \end{array}$                                            |                                                                                                                                                                                                               |

$$\mathcal{W}_1^{\text{gapless}} = \sum_{m=1}^{n_{a_1}} \text{sgn}(v_m^{a_1}) \frac{1 - \text{sgn}(\delta_m^{a_1})}{2} - \sum_{m=1}^{n_{e_1}} \text{sgn}(v_m^{e_1}) \frac{1 - \text{sgn}(\delta_m^{e_1})}{2} + \sum_{m=1}^{n_{f_1}} \text{sgn}(v_m^{f_1}) \frac{1 - \text{sgn}(\delta_m^{f_1})}{2} + \sum_{m=1}^{n_{f_3}} \text{sgn}(v_m^{f_3}) \frac{1 - \text{sgn}(\delta_m^{f_3})}{2} \quad (\text{S70.1})$$

$$\mathcal{W}_2^{\text{gapless}} = \sum_{m=1}^{n_{b_1}} \text{sgn}(v_m^{b_1}) \frac{1 - \text{sgn}(\delta_m^{b_1})}{2} + \sum_{m=1}^{n_{b_3}} \text{sgn}(v_m^{b_3}) \frac{1 - \text{sgn}(\delta_m^{b_3})}{2} - \sum_{m=1}^{n_{g_1}} \text{sgn}(v_m^{g_1}) \frac{1 - \text{sgn}(\delta_m^{g_1})}{2} \quad (\text{S70.2})$$

$$\begin{aligned} \mathcal{W}_3^{\text{gapless}} = & \sum_{m=1}^{n_{c_1}} \text{sgn}(v_m^{c_1}) \frac{1 - \text{sgn}(\delta_m^{c_1})}{2} + \sum_{m=1}^{n_{e_1}} \text{sgn}(v_m^{e_1}) \frac{1 - \text{sgn}(\delta_m^{e_1})}{2} - \sum_{m=1}^{n_{f_1}} \text{sgn}(v_m^{f_1}) \frac{1 - \text{sgn}(\delta_m^{f_1})}{2} \\ & - \sum_{m=1}^{n_{f_3}} \text{sgn}(v_m^{f_3}) \frac{1 - \text{sgn}(\delta_m^{f_3})}{2} + \sum_{m=1}^{n_{g_1}} \text{sgn}(v_m^{g_1}) \frac{1 - \text{sgn}(\delta_m^{g_1})}{2} \end{aligned} \quad (\text{S70.3})$$

$$\begin{aligned} \mathcal{W}_4^{\text{gapless}} = & \sum_{m=1}^{n_{d_1}} \text{sgn}(v_m^{d_1}) \frac{1 - \text{sgn}(\delta_m^{d_1})}{2} + \sum_{m=1}^{n_{d_3}} \text{sgn}(v_m^{d_3}) \frac{1 - \text{sgn}(\delta_m^{d_3})}{2} - \sum_{m=1}^{n_{f_1}} \text{sgn}(v_m^{f_1}) \frac{1 - \text{sgn}(\delta_m^{f_1})}{2} \\ & - \sum_{m=1}^{n_{f_3}} \text{sgn}(v_m^{f_3}) \frac{1 - \text{sgn}(\delta_m^{f_3})}{2} + \sum_{m=1}^{n_{g_1}} \text{sgn}(v_m^{g_1}) \frac{1 - \text{sgn}(\delta_m^{g_1})}{2} \end{aligned} \quad (\text{S70.4})$$

$$\mathcal{W}_1^{\text{gapped}} = - \sum_{m=1}^{n_{b_3}} \text{sgn}(v_m^{b_3}) \frac{1 - \text{sgn}(\delta_m^{b_3})}{2} - \sum_{m=1}^{n_{d_3}} \text{sgn}(v_m^{d_3}) \frac{1 - \text{sgn}(\delta_m^{d_3})}{2} + \sum_{m=1}^{n_{f_3}} \text{sgn}(v_m^{f_3}) \frac{1 - \text{sgn}(\delta_m^{f_3})}{2} \quad (\text{S70.5})$$

$$\mathcal{W}_2^{\text{gapped}} = -2 \sum_{m=1}^{n_{b_3}} \text{sgn}(v_m^{b_3}) \frac{1 - \text{sgn}(\delta_m^{b_3})}{2} + \sum_{m=1}^{n_{g_1}} \text{sgn}(v_m^{g_1}) \frac{1 - \text{sgn}(\delta_m^{g_1})}{2} \quad (\text{S70.6})$$

$$\mathcal{W}_3^{\text{gapped}} = - \sum_{m=1}^{n_{b_3}} \text{sgn}(v_m^{b_3}) \frac{1 - \text{sgn}(\delta_m^{b_3})}{2} - \sum_{m=1}^{n_{d_3}} \text{sgn}(v_m^{d_3}) \frac{1 - \text{sgn}(\delta_m^{d_3})}{2} + \sum_{m=1}^{n_{f_1}} \text{sgn}(v_m^{f_1}) \frac{1 - \text{sgn}(\delta_m^{f_1})}{2} \quad (\text{S70.7})$$



## S71. SPACE GROUP NO. 71

| line segment                                        | character of irrep (generators only)                                                                                        |
|-----------------------------------------------------|-----------------------------------------------------------------------------------------------------------------------------|
| $a \ (0, 0, t)$                                     | $a_1 \begin{Bmatrix} \{2_{001}  0 & 0 & 0 \} \\ 0 \end{Bmatrix} \begin{Bmatrix} \{m_{100}  0 & 0 & 0 \} \\ 0 \end{Bmatrix}$ |
| $b \ (0, t, 0)$                                     | $b_1 \begin{Bmatrix} \{2_{010}  0 & 0 & 0 \} \\ 0 \end{Bmatrix} \begin{Bmatrix} \{m_{100}  0 & 0 & 0 \} \\ 0 \end{Bmatrix}$ |
| $c \ (t, 0, 0)$                                     | $c_1 \begin{Bmatrix} \{2_{100}  0 & 0 & 0 \} \\ 0 \end{Bmatrix} \begin{Bmatrix} \{m_{010}  0 & 0 & 0 \} \\ 0 \end{Bmatrix}$ |
| $d \ (\frac{1}{2}, \frac{1}{2}, \frac{t}{2})$       | $d_1 \begin{Bmatrix} \{2_{001}  0 & 0 & 0 \} \\ -i \end{Bmatrix}$<br>$d_2 \begin{Bmatrix} i \end{Bmatrix}$                  |
| $e \ (\frac{1-t}{2}, \frac{1}{2}, \frac{1}{2})$     | $e_1 \begin{Bmatrix} \{2_{100}  0 & 0 & 0 \} \\ -i \end{Bmatrix}$<br>$e_2 \begin{Bmatrix} i \end{Bmatrix}$                  |
| $f \ (\frac{1}{2}, \frac{1-t}{2}, \frac{1}{2})$     | $f_1 \begin{Bmatrix} \{2_{010}  0 & 0 & 0 \} \\ -i \end{Bmatrix}$<br>$f_2 \begin{Bmatrix} i \end{Bmatrix}$                  |
| $g \ (0, \frac{t}{2}, 1 - \frac{t}{2})$             | $g_1 \begin{Bmatrix} \{m_{100}  0 & 0 & 0 \} \\ -i \end{Bmatrix}$<br>$g_2 \begin{Bmatrix} i \end{Bmatrix}$                  |
| $h \ (\frac{t}{2}, 0, 1 - \frac{t}{2})$             | $h_1 \begin{Bmatrix} \{m_{010}  0 & 0 & 0 \} \\ -i \end{Bmatrix}$<br>$h_2 \begin{Bmatrix} i \end{Bmatrix}$                  |
| $i \ (\frac{1-t}{2}, \frac{t+1}{2}, 0)$             | $i_1 \begin{Bmatrix} \{m_{001}  0 & 0 & 0 \} \\ -i \end{Bmatrix}$<br>$i_2 \begin{Bmatrix} i \end{Bmatrix}$                  |
| $j \ (\frac{1-t}{2}, \frac{1-t}{2}, \frac{t+1}{2})$ | $j_1 \begin{Bmatrix} \{1  0 & 0 & 0 \} \\ 1 \end{Bmatrix}$                                                                  |

$$\mathcal{W}_1^{\text{gapless}} = \sum_{m=1}^{n_{a_1}} \text{sgn}(v_m^{a_1}) \frac{1 - \text{sgn}(\delta_m^{a_1})}{2} - \sum_{m=1}^{n_{c_1}} \text{sgn}(v_m^{c_1}) \frac{1 - \text{sgn}(\delta_m^{c_1})}{2} \quad (\text{S71.1})$$

$$\mathcal{W}_2^{\text{gapless}} = \sum_{m=1}^{n_{b_1}} \text{sgn}(v_m^{b_1}) \frac{1 - \text{sgn}(\delta_m^{b_1})}{2} - \sum_{m=1}^{n_{c_1}} \text{sgn}(v_m^{c_1}) \frac{1 - \text{sgn}(\delta_m^{c_1})}{2} \quad (\text{S71.2})$$

$$\mathcal{W}_3^{\text{gapless}} = \sum_{m=1}^{n_{d_1}} \text{sgn}(v_m^{d_1}) \frac{1 - \text{sgn}(\delta_m^{d_1})}{2} - \sum_{m=1}^{n_{i_1}} \text{sgn}(v_m^{i_1}) \frac{1 - \text{sgn}(\delta_m^{i_1})}{2} + \sum_{m=1}^{n_{j_1}} \text{sgn}(v_m^{j_1}) \frac{1 - \text{sgn}(\delta_m^{j_1})}{2} \quad (\text{S71.3})$$

$$\mathcal{W}_4^{\text{gapless}} = \sum_{m=1}^{n_{e_1}} \text{sgn}(v_m^{e_1}) \frac{1 - \text{sgn}(\delta_m^{e_1})}{2} - \sum_{m=1}^{n_{g_1}} \text{sgn}(v_m^{g_1}) \frac{1 - \text{sgn}(\delta_m^{g_1})}{2} - \sum_{m=1}^{n_{j_1}} \text{sgn}(v_m^{j_1}) \frac{1 - \text{sgn}(\delta_m^{j_1})}{2} \quad (\text{S71.4})$$

$$\mathcal{W}_5^{\text{gapless}} = \sum_{m=1}^{n_{f_1}} \text{sgn}(v_m^{f_1}) \frac{1 - \text{sgn}(\delta_m^{f_1})}{2} - \sum_{m=1}^{n_{h_1}} \text{sgn}(v_m^{h_1}) \frac{1 - \text{sgn}(\delta_m^{h_1})}{2} - \sum_{m=1}^{n_{j_1}} \text{sgn}(v_m^{j_1}) \frac{1 - \text{sgn}(\delta_m^{j_1})}{2} \quad (\text{S71.5})$$

## S72. SPACE GROUP NO. 72

| line segment                                        | character of irrep (generators only)                                                                                                                                          |
|-----------------------------------------------------|-------------------------------------------------------------------------------------------------------------------------------------------------------------------------------|
| $a \ (0, 0, t)$                                     | $a_1 \ \begin{Bmatrix} \{2_{001}  0 & 0 & 0 \} \\ 0 \end{Bmatrix} \ \begin{Bmatrix} \{m_{100}  0 & 0 & \frac{1}{2} \} \\ 0 \end{Bmatrix}$                                     |
| $b \ (0, t, 0)$                                     | $b_1 \ \begin{Bmatrix} \{2_{010}  0 & 0 & \frac{1}{2} \} \\ 0 \end{Bmatrix} \ \begin{Bmatrix} \{m_{100}  0 & 0 & \frac{1}{2} \} \\ 0 \end{Bmatrix}$                           |
| $c \ (t, 0, 0)$                                     | $c_1 \ \begin{Bmatrix} \{2_{100}  0 & 0 & \frac{1}{2} \} \\ 0 \end{Bmatrix} \ \begin{Bmatrix} \{m_{010}  0 & 0 & \frac{1}{2} \} \\ 0 \end{Bmatrix}$                           |
| $d \ (\frac{1}{2}, \frac{1}{2}, \frac{t}{2})$       | $d_1 \ \begin{Bmatrix} \{2_{001}  0 & 0 & 0 \} \\ -i \end{Bmatrix}$<br>$d_2 \ \begin{Bmatrix} \\ i \end{Bmatrix}$                                                             |
| $e \ (\frac{1-t}{2}, \frac{1}{2}, \frac{1}{2})$     | $e_1 \ \begin{Bmatrix} \{2_{100}  0 & 0 & \frac{1}{2} \} \\ i \end{Bmatrix}$<br>$e_2 \ \begin{Bmatrix} \\ -i \end{Bmatrix}$                                                   |
| $f \ (\frac{1}{2}, \frac{1-t}{2}, \frac{1}{2})$     | $f_1 \ \begin{Bmatrix} \{2_{010}  0 & 0 & \frac{1}{2} \} \\ i \end{Bmatrix}$<br>$f_2 \ \begin{Bmatrix} \\ -i \end{Bmatrix}$                                                   |
| $g \ (0, \frac{t}{2}, 1 - \frac{t}{2})$             | $g_1 \ \begin{Bmatrix} \{m_{100}  0 & 0 & \frac{1}{2} \} \\ -ie^{-\frac{1}{2}i\pi(2-t)} \end{Bmatrix}$<br>$g_2 \ \begin{Bmatrix} \\ ie^{-\frac{1}{2}i\pi(2-t)} \end{Bmatrix}$ |
| $h \ (\frac{t}{2}, 0, 1 - \frac{t}{2})$             | $h_1 \ \begin{Bmatrix} \{m_{010}  0 & 0 & \frac{1}{2} \} \\ -ie^{-\frac{1}{2}i\pi(2-t)} \end{Bmatrix}$<br>$h_2 \ \begin{Bmatrix} \\ ie^{-\frac{1}{2}i\pi(2-t)} \end{Bmatrix}$ |
| $i \ (\frac{1-t}{2}, \frac{t+1}{2}, 0)$             | $i_1 \ \begin{Bmatrix} \{m_{001}  0 & 0 & 0 \} \\ -i \end{Bmatrix}$<br>$i_2 \ \begin{Bmatrix} \\ i \end{Bmatrix}$                                                             |
| $j \ (\frac{1-t}{2}, \frac{1-t}{2}, \frac{t+1}{2})$ | $j_1 \ \begin{Bmatrix} \{1  0 & 0 & 0 \} \\ 1 \end{Bmatrix}$                                                                                                                  |

$$\mathcal{W}_1^{\text{gapless}} = \sum_{m=1}^{n_{a_1}} \text{sgn}(v_m^{a_1}) \frac{1 - \text{sgn}(\delta_m^{a_1})}{2} - \sum_{m=1}^{n_{c_1}} \text{sgn}(v_m^{c_1}) \frac{1 - \text{sgn}(\delta_m^{c_1})}{2} \quad (\text{S72.1})$$

$$\mathcal{W}_2^{\text{gapless}} = \sum_{m=1}^{n_{b_1}} \text{sgn}(v_m^{b_1}) \frac{1 - \text{sgn}(\delta_m^{b_1})}{2} - \sum_{m=1}^{n_{c_1}} \text{sgn}(v_m^{c_1}) \frac{1 - \text{sgn}(\delta_m^{c_1})}{2} \quad (\text{S72.2})$$

$$\mathcal{W}_3^{\text{gapless}} = \sum_{m=1}^{n_{d_1}} \text{sgn}(v_m^{d_1}) \frac{1 - \text{sgn}(\delta_m^{d_1})}{2} - \sum_{m=1}^{n_{i_1}} \text{sgn}(v_m^{i_1}) \frac{1 - \text{sgn}(\delta_m^{i_1})}{2} + \sum_{m=1}^{n_{j_1}} \text{sgn}(v_m^{j_1}) \frac{1 - \text{sgn}(\delta_m^{j_1})}{2} \quad (\text{S72.3})$$

$$\mathcal{W}_4^{\text{gapless}} = \sum_{m=1}^{n_{e_1}} \text{sgn}(v_m^{e_1}) \frac{1 - \text{sgn}(\delta_m^{e_1})}{2} + \sum_{m=1}^{n_{e_2}} \text{sgn}(v_m^{e_2}) \frac{1 - \text{sgn}(\delta_m^{e_2})}{2} - \sum_{m=1}^{n_{g_1}} \text{sgn}(v_m^{g_1}) \frac{1 - \text{sgn}(\delta_m^{g_1})}{2} - \sum_{m=1}^{n_{j_1}} \text{sgn}(v_m^{j_1}) \frac{1 - \text{sgn}(\delta_m^{j_1})}{2} \quad (\text{S72.4})$$

$$\mathcal{W}_5^{\text{gapless}} = \sum_{m=1}^{n_{f_1}} \text{sgn}(v_m^{f_1}) \frac{1 - \text{sgn}(\delta_m^{f_1})}{2} + \sum_{m=1}^{n_{f_2}} \text{sgn}(v_m^{f_2}) \frac{1 - \text{sgn}(\delta_m^{f_2})}{2} - \sum_{m=1}^{n_{h_1}} \text{sgn}(v_m^{h_1}) \frac{1 - \text{sgn}(\delta_m^{h_1})}{2} - \sum_{m=1}^{n_{j_1}} \text{sgn}(v_m^{j_1}) \frac{1 - \text{sgn}(\delta_m^{j_1})}{2} \quad (\text{S72.5})$$

$$\mathcal{W}_1^{\text{gapped}} = -2 \sum_{m=1}^{n_{e_2}} \text{sgn}(v_m^{e_2}) \frac{1 - \text{sgn}(\delta_m^{e_2})}{2} + 2 \sum_{m=1}^{n_{f_2}} \text{sgn}(v_m^{f_2}) \frac{1 - \text{sgn}(\delta_m^{f_2})}{2} + \sum_{m=1}^{n_{g_1}} \text{sgn}(v_m^{g_1}) \frac{1 - \text{sgn}(\delta_m^{g_1})}{2} - \sum_{m=1}^{n_{h_1}} \text{sgn}(v_m^{h_1}) \frac{1 - \text{sgn}(\delta_m^{h_1})}{2} \quad (\text{S72.6})$$

$$\mathcal{W}_2^{\text{gapped}} = -2 \sum_{m=1}^{n_{e_2}} \text{sgn}(v_m^{e_2}) \frac{1 - \text{sgn}(\delta_m^{e_2})}{2} + \sum_{m=1}^{n_{g_1}} \text{sgn}(v_m^{g_1}) \frac{1 - \text{sgn}(\delta_m^{g_1})}{2} + \sum_{m=1}^{n_{j_1}} \text{sgn}(v_m^{j_1}) \frac{1 - \text{sgn}(\delta_m^{j_1})}{2} \quad (\text{S72.7})$$

### S73. SPACE GROUP NO. 73

| line segment                                        | character of irrep (generators only)                                                                                                                |
|-----------------------------------------------------|-----------------------------------------------------------------------------------------------------------------------------------------------------|
| $a \ (0, 0, t)$                                     | $a_1 \ \begin{Bmatrix} \{2_{001}   0 \ \frac{1}{2} \ 0\} \\ 0 \end{Bmatrix} \ \begin{Bmatrix} \{m_{100}   0 \ 0 \ \frac{1}{2}\} \\ 0 \end{Bmatrix}$ |
| $b \ (0, t, 0)$                                     | $b_1 \ \begin{Bmatrix} \{2_{010}   \frac{1}{2} \ 0 \ 0\} \\ 0 \end{Bmatrix} \ \begin{Bmatrix} \{m_{100}   0 \ 0 \ \frac{1}{2}\} \\ 0 \end{Bmatrix}$ |
| $c \ (t, 0, 0)$                                     | $c_1 \ \begin{Bmatrix} \{2_{100}   0 \ 0 \ \frac{1}{2}\} \\ 0 \end{Bmatrix} \ \begin{Bmatrix} \{m_{010}   \frac{1}{2} \ 0 \ 0\} \\ 0 \end{Bmatrix}$ |
| $d \ (\frac{1}{2}, \frac{1}{2}, \frac{t}{2})$       | $d_1 \ \begin{Bmatrix} \{2_{001}   0 \ \frac{1}{2} \ 0\} \\ i \end{Bmatrix}$<br>$d_2 \ -i$                                                          |
| $e \ (\frac{1-t}{2}, \frac{1}{2}, \frac{1}{2})$     | $e_1 \ \begin{Bmatrix} \{2_{100}   0 \ 0 \ \frac{1}{2}\} \\ i \end{Bmatrix}$<br>$e_2 \ -i$                                                          |
| $f \ (\frac{1}{2}, \frac{1-t}{2}, \frac{1}{2})$     | $f_1 \ \begin{Bmatrix} \{2_{010}   \frac{1}{2} \ 0 \ 0\} \\ i \end{Bmatrix}$<br>$f_2 \ -i$                                                          |
| $g \ (0, \frac{t}{2}, 1 - \frac{t}{2})$             | $g_1 \ \begin{Bmatrix} \{m_{100}   0 \ 0 \ \frac{1}{2}\} \\ -ie^{-\frac{1}{2}i\pi(2-t)} \end{Bmatrix}$<br>$g_2 \ ie^{-\frac{1}{2}i\pi(2-t)}$        |
| $h \ (\frac{t}{2}, 0, 1 - \frac{t}{2})$             | $h_1 \ \begin{Bmatrix} \{m_{010}   \frac{1}{2} \ 0 \ 0\} \\ -ie^{-\frac{1}{2}i\pi t} \end{Bmatrix}$<br>$h_2 \ ie^{-\frac{1}{2}i\pi t}$              |
| $i \ (\frac{1-t}{2}, \frac{t+1}{2}, 0)$             | $i_1 \ \begin{Bmatrix} \{m_{001}   0 \ \frac{1}{2} \ 0\} \\ -ie^{-\frac{1}{2}i\pi(t+1)} \end{Bmatrix}$<br>$i_2 \ ie^{-\frac{1}{2}i\pi(t+1)}$        |
| $j \ (\frac{1-t}{2}, \frac{1-t}{2}, \frac{t+1}{2})$ | $j_1 \ \begin{Bmatrix} \{1   0 \ 0 \ 0\} \\ 1 \end{Bmatrix}$                                                                                        |

$$\mathcal{W}_1^{\text{gapless}} = \sum_{m=1}^{n_{a_1}} \text{sgn}(v_m^{a_1}) \frac{1 - \text{sgn}(\delta_m^{a_1})}{2} - \sum_{m=1}^{n_{c_1}} \text{sgn}(v_m^{c_1}) \frac{1 - \text{sgn}(\delta_m^{c_1})}{2} \quad (\text{S73.1})$$

$$\mathcal{W}_2^{\text{gapless}} = \sum_{m=1}^{n_{b_1}} \text{sgn}(v_m^{b_1}) \frac{1 - \text{sgn}(\delta_m^{b_1})}{2} - \sum_{m=1}^{n_{c_1}} \text{sgn}(v_m^{c_1}) \frac{1 - \text{sgn}(\delta_m^{c_1})}{2} \quad (\text{S73.2})$$

$$\mathcal{W}_3^{\text{gapless}} = \sum_{m=1}^{n_{d_1}} \text{sgn}(v_m^{d_1}) \frac{1 - \text{sgn}(\delta_m^{d_1})}{2} + \sum_{m=1}^{n_{d_2}} \text{sgn}(v_m^{d_2}) \frac{1 - \text{sgn}(\delta_m^{d_2})}{2} - \sum_{m=1}^{n_{i_1}} \text{sgn}(v_m^{i_1}) \frac{1 - \text{sgn}(\delta_m^{i_1})}{2} + \sum_{m=1}^{n_{j_1}} \text{sgn}(v_m^{j_1}) \frac{1 - \text{sgn}(\delta_m^{j_1})}{2} \quad (\text{S73.3})$$

$$\mathcal{W}_4^{\text{gapless}} = \sum_{m=1}^{n_{e_1}} \text{sgn}(v_m^{e_1}) \frac{1 - \text{sgn}(\delta_m^{e_1})}{2} + \sum_{m=1}^{n_{e_2}} \text{sgn}(v_m^{e_2}) \frac{1 - \text{sgn}(\delta_m^{e_2})}{2} - \sum_{m=1}^{n_{g_1}} \text{sgn}(v_m^{g_1}) \frac{1 - \text{sgn}(\delta_m^{g_1})}{2} - \sum_{m=1}^{n_{j_1}} \text{sgn}(v_m^{j_1}) \frac{1 - \text{sgn}(\delta_m^{j_1})}{2} \quad (\text{S73.4})$$

$$\mathcal{W}_5^{\text{gapless}} = \sum_{m=1}^{n_{f_1}} \text{sgn}(v_m^{f_1}) \frac{1 - \text{sgn}(\delta_m^{f_1})}{2} + \sum_{m=1}^{n_{f_2}} \text{sgn}(v_m^{f_2}) \frac{1 - \text{sgn}(\delta_m^{f_2})}{2} - \sum_{m=1}^{n_{h_1}} \text{sgn}(v_m^{h_1}) \frac{1 - \text{sgn}(\delta_m^{h_1})}{2} - \sum_{m=1}^{n_{j_1}} \text{sgn}(v_m^{j_1}) \frac{1 - \text{sgn}(\delta_m^{j_1})}{2} \quad (\text{S73.5})$$

$$\mathcal{X}_1 = \sum_{m=1}^{n_{g_1}} \frac{1 - \text{sgn}(\delta_m^{g_1})}{2} + \sum_{m=1}^{n_{i_1}} \frac{1 - \text{sgn}(\delta_m^{i_1})}{2} \quad \text{mod } 2 \quad (\text{S73.6})$$

$$\mathcal{X}_2 = \sum_{m=1}^{n_{h_1}} \frac{1 - \text{sgn}(\delta_m^{h_1})}{2} + \sum_{m=1}^{n_{i_1}} \frac{1 - \text{sgn}(\delta_m^{i_1})}{2} \quad \text{mod } 2 \quad (\text{S73.7})$$

#### S74. SPACE GROUP NO. 74

| line segment                                        | character of irrep (generators only)                                                                                                                                   |
|-----------------------------------------------------|------------------------------------------------------------------------------------------------------------------------------------------------------------------------|
| $a \ (0, 0, t)$                                     | $a_1 \begin{Bmatrix} \{2_{001}   0 \ \frac{1}{2} \ 0\} \\ 0 \end{Bmatrix} \begin{Bmatrix} \{m_{100}   0 \ 0 \ 0\} \\ 0 \end{Bmatrix}$                                  |
| $b \ (0, t, 0)$                                     | $b_1 \begin{Bmatrix} \{2_{010}   0 \ \frac{1}{2} \ 0\} \\ 0 \end{Bmatrix} \begin{Bmatrix} \{m_{100}   0 \ 0 \ 0\} \\ 0 \end{Bmatrix}$                                  |
| $c \ (t, 0, 0)$                                     | $c_1 \begin{Bmatrix} \{2_{100}   0 \ 0 \ 0\} \\ 0 \end{Bmatrix} \begin{Bmatrix} \{m_{010}   0 \ \frac{1}{2} \ 0\} \\ 0 \end{Bmatrix}$                                  |
| $d \ (\frac{1}{2}, \frac{1}{2}, \frac{t}{2})$       | $d_1 \begin{Bmatrix} \{2_{001}   0 \ \frac{1}{2} \ 0\} \\ i \end{Bmatrix}$<br>$d_2 \begin{Bmatrix} -i \end{Bmatrix}$                                                   |
| $e \ (\frac{1-t}{2}, \frac{1}{2}, \frac{1}{2})$     | $e_1 \begin{Bmatrix} \{2_{100}   0 \ 0 \ 0\} \\ -i \end{Bmatrix}$<br>$e_2 \begin{Bmatrix} i \end{Bmatrix}$                                                             |
| $f \ (\frac{1}{2}, \frac{1-t}{2}, \frac{1}{2})$     | $f_1 \begin{Bmatrix} \{2_{010}   0 \ \frac{1}{2} \ 0\} \\ -ie^{-\frac{1}{2}i\pi(1-t)} \end{Bmatrix}$<br>$f_2 \begin{Bmatrix} ie^{-\frac{1}{2}i\pi(1-t)} \end{Bmatrix}$ |
| $g \ (0, \frac{t}{2}, 1 - \frac{t}{2})$             | $g_1 \begin{Bmatrix} \{m_{100}   0 \ 0 \ 0\} \\ -i \end{Bmatrix}$<br>$g_2 \begin{Bmatrix} i \end{Bmatrix}$                                                             |
| $h \ (\frac{t}{2}, 0, 1 - \frac{t}{2})$             | $h_1 \begin{Bmatrix} \{m_{010}   0 \ \frac{1}{2} \ 0\} \\ -i \end{Bmatrix}$<br>$h_2 \begin{Bmatrix} i \end{Bmatrix}$                                                   |
| $i \ (\frac{1-t}{2}, \frac{t+1}{2}, 0)$             | $i_1 \begin{Bmatrix} \{m_{001}   0 \ \frac{1}{2} \ 0\} \\ -ie^{-\frac{1}{2}i\pi(t+1)} \end{Bmatrix}$<br>$i_2 \begin{Bmatrix} ie^{-\frac{1}{2}i\pi(t+1)} \end{Bmatrix}$ |
| $j \ (\frac{1-t}{2}, \frac{1-t}{2}, \frac{t+1}{2})$ | $j_1 \begin{Bmatrix} \{1   0 \ 0 \ 0\} \\ 1 \end{Bmatrix}$                                                                                                             |

$$\mathcal{W}_1^{\text{gapless}} = \sum_{m=1}^{n_{a_1}} \text{sgn}(v_m^{a_1}) \frac{1 - \text{sgn}(\delta_m^{a_1})}{2} - \sum_{m=1}^{n_{c_1}} \text{sgn}(v_m^{c_1}) \frac{1 - \text{sgn}(\delta_m^{c_1})}{2} \quad (\text{S74.1})$$

$$\mathcal{W}_2^{\text{gapless}} = \sum_{m=1}^{n_{b_1}} \text{sgn}(v_m^{b_1}) \frac{1 - \text{sgn}(\delta_m^{b_1})}{2} - \sum_{m=1}^{n_{c_1}} \text{sgn}(v_m^{c_1}) \frac{1 - \text{sgn}(\delta_m^{c_1})}{2} \quad (\text{S74.2})$$

$$\mathcal{W}_3^{\text{gapless}} = \sum_{m=1}^{n_{d_1}} \text{sgn}(v_m^{d_1}) \frac{1 - \text{sgn}(\delta_m^{d_1})}{2} + \sum_{m=1}^{n_{d_2}} \text{sgn}(v_m^{d_2}) \frac{1 - \text{sgn}(\delta_m^{d_2})}{2} - \sum_{m=1}^{n_{i_1}} \text{sgn}(v_m^{i_1}) \frac{1 - \text{sgn}(\delta_m^{i_1})}{2} + \sum_{m=1}^{n_{j_1}} \text{sgn}(v_m^{j_1}) \frac{1 - \text{sgn}(\delta_m^{j_1})}{2} \quad (\text{S74.3})$$

$$\mathcal{W}_4^{\text{gapless}} = \sum_{m=1}^{n_{e_1}} \text{sgn}(v_m^{e_1}) \frac{1 - \text{sgn}(\delta_m^{e_1})}{2} - \sum_{m=1}^{n_{g_1}} \text{sgn}(v_m^{g_1}) \frac{1 - \text{sgn}(\delta_m^{g_1})}{2} - \sum_{m=1}^{n_{j_1}} \text{sgn}(v_m^{j_1}) \frac{1 - \text{sgn}(\delta_m^{j_1})}{2} \quad (\text{S74.4})$$

$$\mathcal{W}_5^{\text{gapless}} = \sum_{m=1}^{n_{f_1}} \text{sgn}(v_m^{f_1}) \frac{1 - \text{sgn}(\delta_m^{f_1})}{2} - \sum_{m=1}^{n_{h_1}} \text{sgn}(v_m^{h_1}) \frac{1 - \text{sgn}(\delta_m^{h_1})}{2} - \sum_{m=1}^{n_{j_1}} \text{sgn}(v_m^{j_1}) \frac{1 - \text{sgn}(\delta_m^{j_1})}{2} \quad (\text{S74.5})$$

### S75. SPACE GROUP NO. 75

| line segment                                      | character of irrep (generators only)                                                                                                                                  |
|---------------------------------------------------|-----------------------------------------------------------------------------------------------------------------------------------------------------------------------|
| $a \quad (\frac{t}{2}, 0, 0)$                     | $\{1   0 \ 0 \ 0\}$<br>$a_1 \quad 1$                                                                                                                                  |
| $b \quad (\frac{1}{2}, \frac{t}{2}, 0)$           | $\{1   0 \ 0 \ 0\}$<br>$b_1 \quad 1$                                                                                                                                  |
| $c \quad (\frac{t}{2}, 0, \frac{1}{2})$           | $\{1   0 \ 0 \ 0\}$<br>$c_1 \quad 1$                                                                                                                                  |
| $d \quad (\frac{1}{2}, \frac{t}{2}, \frac{1}{2})$ | $\{1   0 \ 0 \ 0\}$<br>$d_1 \quad 1$                                                                                                                                  |
| $e \quad (0, 0, \frac{t}{2})$                     | $\{4_{001}   0 \ 0 \ 0\}$<br>$e_1 \quad e^{-\frac{3i\pi}{4}}$<br>$e_2 \quad e^{\frac{3i\pi}{4}}$<br>$e_3 \quad e^{-\frac{i\pi}{4}}$<br>$e_4 \quad e^{\frac{i\pi}{4}}$ |
| $f \quad (\frac{1}{2}, 0, \frac{t}{2})$           | $\{2_{001}   0 \ 0 \ 0\}$<br>$f_1 \quad -i$<br>$f_2 \quad i$                                                                                                          |
| $g \quad (\frac{1}{2}, \frac{1}{2}, \frac{t}{2})$ | $\{4_{001}   0 \ 0 \ 0\}$<br>$g_1 \quad e^{-\frac{3i\pi}{4}}$<br>$g_2 \quad e^{\frac{3i\pi}{4}}$<br>$g_3 \quad e^{-\frac{i\pi}{4}}$<br>$g_4 \quad e^{\frac{i\pi}{4}}$ |

---


$$\begin{aligned}
\mathcal{W}_1^{\text{gapless}} = & \sum_{m=1}^{n_{a_1}} \text{sgn}(v_m^{a_1}) \frac{1 - \text{sgn}(\delta_m^{a_1})}{2} - \sum_{m=1}^{n_{c_1}} \text{sgn}(v_m^{c_1}) \frac{1 - \text{sgn}(\delta_m^{c_1})}{2} - \sum_{m=1}^{n_{e_1}} \text{sgn}(v_m^{e_1}) \frac{1 - \text{sgn}(\delta_m^{e_1})}{2} \\
& - \sum_{m=1}^{n_{e_2}} \text{sgn}(v_m^{e_2}) \frac{1 - \text{sgn}(\delta_m^{e_2})}{2} - \sum_{m=1}^{n_{e_3}} \text{sgn}(v_m^{e_3}) \frac{1 - \text{sgn}(\delta_m^{e_3})}{2} - \sum_{m=1}^{n_{e_4}} \text{sgn}(v_m^{e_4}) \frac{1 - \text{sgn}(\delta_m^{e_4})}{2} \\
& + \sum_{m=1}^{n_{f_1}} \text{sgn}(v_m^{f_1}) \frac{1 - \text{sgn}(\delta_m^{f_1})}{2} + \sum_{m=1}^{n_{f_2}} \text{sgn}(v_m^{f_2}) \frac{1 - \text{sgn}(\delta_m^{f_2})}{2}
\end{aligned} \tag{S75.1}$$

$$\begin{aligned}
\mathcal{W}_2^{\text{gapless}} = & \sum_{m=1}^{n_{b_1}} \text{sgn}(v_m^{b_1}) \frac{1 - \text{sgn}(\delta_m^{b_1})}{2} - \sum_{m=1}^{n_{d_1}} \text{sgn}(v_m^{d_1}) \frac{1 - \text{sgn}(\delta_m^{d_1})}{2} - \sum_{m=1}^{n_{f_1}} \text{sgn}(v_m^{f_1}) \frac{1 - \text{sgn}(\delta_m^{f_1})}{2} \\
& - \sum_{m=1}^{n_{f_2}} \text{sgn}(v_m^{f_2}) \frac{1 - \text{sgn}(\delta_m^{f_2})}{2} + \sum_{m=1}^{n_{g_1}} \text{sgn}(v_m^{g_1}) \frac{1 - \text{sgn}(\delta_m^{g_1})}{2} + \sum_{m=1}^{n_{g_2}} \text{sgn}(v_m^{g_2}) \frac{1 - \text{sgn}(\delta_m^{g_2})}{2} \\
& + \sum_{m=1}^{n_{g_3}} \text{sgn}(v_m^{g_3}) \frac{1 - \text{sgn}(\delta_m^{g_3})}{2} + \sum_{m=1}^{n_{g_4}} \text{sgn}(v_m^{g_4}) \frac{1 - \text{sgn}(\delta_m^{g_4})}{2}
\end{aligned} \tag{S75.2}$$

$$\mathcal{W}_1^{\text{gapped}} = - \sum_{m=1}^{n_{f_1}} \text{sgn}(v_m^{f_1}) \frac{1 - \text{sgn}(\delta_m^{f_1})}{2} + \sum_{m=1}^{n_{f_2}} \text{sgn}(v_m^{f_2}) \frac{1 - \text{sgn}(\delta_m^{f_2})}{2} \tag{S75.3}$$

$$\mathcal{W}_2^{\text{gapped}} = - \sum_{m=1}^{n_{e_1}} \text{sgn}(v_m^{e_1}) \frac{1 - \text{sgn}(\delta_m^{e_1})}{2} + \sum_{m=1}^{n_{e_2}} \text{sgn}(v_m^{e_2}) \frac{1 - \text{sgn}(\delta_m^{e_2})}{2} \tag{S75.4}$$

$$\mathcal{W}_3^{\text{gapped}} = - \sum_{m=1}^{n_{g_1}} \text{sgn}(v_m^{g_1}) \frac{1 - \text{sgn}(\delta_m^{g_1})}{2} + \sum_{m=1}^{n_{g_2}} \text{sgn}(v_m^{g_2}) \frac{1 - \text{sgn}(\delta_m^{g_2})}{2} \tag{S75.5}$$

$$\mathcal{W}_4^{\text{gapped}} = - \sum_{m=1}^{n_{e_3}} \text{sgn}(v_m^{e_3}) \frac{1 - \text{sgn}(\delta_m^{e_3})}{2} + \sum_{m=1}^{n_{e_4}} \text{sgn}(v_m^{e_4}) \frac{1 - \text{sgn}(\delta_m^{e_4})}{2} \tag{S75.6}$$

$$\mathcal{W}_5^{\text{gapped}} = - \sum_{m=1}^{n_{g_3}} \text{sgn}(v_m^{g_3}) \frac{1 - \text{sgn}(\delta_m^{g_3})}{2} + \sum_{m=1}^{n_{g_4}} \text{sgn}(v_m^{g_4}) \frac{1 - \text{sgn}(\delta_m^{g_4})}{2} \tag{S75.7}$$

$$\mathcal{X}_1 = \sum_{m=1}^{n_{c_1}} \frac{1 - \text{sgn}(\delta_m^{c_1})}{2} + \sum_{m=1}^{n_{d_1}} \frac{1 - \text{sgn}(\delta_m^{d_1})}{2} \mod 2 \tag{S75.8}$$

$$\mathcal{X}_2 = \sum_{m=1}^{n_{d_1}} \frac{1 - \text{sgn}(\delta_m^{d_1})}{2} \mod 2 \tag{S75.9}$$

## S76. SPACE GROUP NO. 76

| line segment                                      | character of irrep (generators only)                                                                                                                                                                                                                             |
|---------------------------------------------------|------------------------------------------------------------------------------------------------------------------------------------------------------------------------------------------------------------------------------------------------------------------|
| $a \quad (\frac{t}{2}, 0, 0)$                     | $\begin{matrix} \{1  0 & 0 & 0\} \\ a_1 & 1 \end{matrix}$                                                                                                                                                                                                        |
| $b \quad (\frac{1}{2}, \frac{t}{2}, 0)$           | $\begin{matrix} \{1  0 & 0 & 0\} \\ b_1 & 1 \end{matrix}$                                                                                                                                                                                                        |
| $c \quad (\frac{t}{2}, 0, \frac{1}{2})$           | $\begin{matrix} \{1  0 & 0 & 0\} \\ c_1 & 1 \end{matrix}$                                                                                                                                                                                                        |
| $d \quad (\frac{1}{2}, \frac{t}{2}, \frac{1}{2})$ | $\begin{matrix} \{1  0 & 0 & 0\} \\ d_1 & 1 \end{matrix}$                                                                                                                                                                                                        |
| $e \quad (0, 0, \frac{t}{2})$                     | $\begin{matrix} \{4_{001}  0 & 0 & \frac{1}{4}\} \\ e_1 & e^{-\frac{1}{4}i\pi t - \frac{3i\pi}{4}} \\ e_2 & e^{\frac{3i\pi}{4} - \frac{i\pi t}{4}} \\ e_3 & e^{-\frac{1}{4}i\pi t - \frac{i\pi}{4}} \\ e_4 & e^{\frac{i\pi}{4} - \frac{i\pi t}{4}} \end{matrix}$ |
| $f \quad (\frac{1}{2}, 0, \frac{t}{2})$           | $\begin{matrix} \{2_{001}  0 & 0 & \frac{1}{2}\} \\ f_1 & -ie^{-\frac{1}{2}i\pi t} \\ f_2 & ie^{-\frac{1}{2}i\pi t} \end{matrix}$                                                                                                                                |
| $g \quad (\frac{1}{2}, \frac{1}{2}, \frac{t}{2})$ | $\begin{matrix} \{4_{001}  0 & 0 & \frac{1}{4}\} \\ g_1 & e^{-\frac{1}{4}i\pi t - \frac{3i\pi}{4}} \\ g_2 & e^{\frac{3i\pi}{4} - \frac{i\pi t}{4}} \\ g_3 & e^{-\frac{1}{4}i\pi t - \frac{i\pi}{4}} \\ g_4 & e^{\frac{i\pi}{4} - \frac{i\pi t}{4}} \end{matrix}$ |

$$\begin{aligned}
\mathcal{W}_1^{\text{gapless}} = & \sum_{m=1}^{n_{a_1}} \text{sgn}(v_m^{a_1}) \frac{1 - \text{sgn}(\delta_m^{a_1})}{2} - 2 \sum_{m=1}^{n_{c_1}} \text{sgn}(v_m^{c_1}) \frac{1 - \text{sgn}(\delta_m^{c_1})}{2} - \sum_{m=1}^{n_{e_1}} \text{sgn}(v_m^{e_1}) \frac{1 - \text{sgn}(\delta_m^{e_1})}{2} \\
& - \sum_{m=1}^{n_{e_2}} \text{sgn}(v_m^{e_2}) \frac{1 - \text{sgn}(\delta_m^{e_2})}{2} - \sum_{m=1}^{n_{e_3}} \text{sgn}(v_m^{e_3}) \frac{1 - \text{sgn}(\delta_m^{e_3})}{2} - \sum_{m=1}^{n_{e_4}} \text{sgn}(v_m^{e_4}) \frac{1 - \text{sgn}(\delta_m^{e_4})}{2} \\
& + \sum_{m=1}^{n_{f_1}} \text{sgn}(v_m^{f_1}) \frac{1 - \text{sgn}(\delta_m^{f_1})}{2} + \sum_{m=1}^{n_{f_2}} \text{sgn}(v_m^{f_2}) \frac{1 - \text{sgn}(\delta_m^{f_2})}{2}
\end{aligned} \tag{S76.1}$$

$$\begin{aligned}
\mathcal{W}_2^{\text{gapless}} = & \sum_{m=1}^{n_{b_1}} \text{sgn}(v_m^{b_1}) \frac{1 - \text{sgn}(\delta_m^{b_1})}{2} - 2 \sum_{m=1}^{n_{d_1}} \text{sgn}(v_m^{d_1}) \frac{1 - \text{sgn}(\delta_m^{d_1})}{2} - \sum_{m=1}^{n_{f_1}} \text{sgn}(v_m^{f_1}) \frac{1 - \text{sgn}(\delta_m^{f_1})}{2} \\
& - \sum_{m=1}^{n_{f_2}} \text{sgn}(v_m^{f_2}) \frac{1 - \text{sgn}(\delta_m^{f_2})}{2} + \sum_{m=1}^{n_{g_1}} \text{sgn}(v_m^{g_1}) \frac{1 - \text{sgn}(\delta_m^{g_1})}{2} + \sum_{m=1}^{n_{g_2}} \text{sgn}(v_m^{g_2}) \frac{1 - \text{sgn}(\delta_m^{g_2})}{2} \\
& + \sum_{m=1}^{n_{g_3}} \text{sgn}(v_m^{g_3}) \frac{1 - \text{sgn}(\delta_m^{g_3})}{2} + \sum_{m=1}^{n_{g_4}} \text{sgn}(v_m^{g_4}) \frac{1 - \text{sgn}(\delta_m^{g_4})}{2}
\end{aligned} \tag{S76.2}$$

$$\mathcal{X}_1 = \sum_{m=1}^{n_{e_1}} \frac{1 - \text{sgn}(\delta_m^{e_1})}{2} + \sum_{m=1}^{n_{e_2}} \frac{1 - \text{sgn}(\delta_m^{e_2})}{2} + \sum_{m=1}^{n_{e_3}} \frac{1 - \text{sgn}(\delta_m^{e_3})}{2} + \sum_{m=1}^{n_{e_4}} \frac{1 - \text{sgn}(\delta_m^{e_4})}{2} \pmod{2} \tag{S76.3}$$

$$\begin{aligned}
\mathcal{X}_2 = & -2 \sum_{m=1}^{n_{c_1}} \text{sgn}(v_m^{c_1}) \frac{1 - \text{sgn}(\delta_m^{c_1})}{2} - \sum_{m=1}^{n_{e_1}} \text{sgn}(v_m^{e_1}) \frac{1 - \text{sgn}(\delta_m^{e_1})}{2} + \sum_{m=1}^{n_{e_2}} \text{sgn}(v_m^{e_2}) \frac{1 - \text{sgn}(\delta_m^{e_2})}{2} - 3 \sum_{m=1}^{n_{e_3}} \text{sgn}(v_m^{e_3}) \frac{1 - \text{sgn}(\delta_m^{e_3})}{2} \\
& + 3 \sum_{m=1}^{n_{e_4}} \text{sgn}(v_m^{e_4}) \frac{1 - \text{sgn}(\delta_m^{e_4})}{2} - \sum_{m=1}^{n_{f_1}} \text{sgn}(v_m^{f_1}) \frac{1 - \text{sgn}(\delta_m^{f_1})}{2} + \sum_{m=1}^{n_{f_2}} \text{sgn}(v_m^{f_2}) \frac{1 - \text{sgn}(\delta_m^{f_2})}{2} \pmod{4}
\end{aligned} \tag{S76.4}$$

$$\begin{aligned}
\mathcal{X}_3 = & 2 \sum_{m=1}^{n_{c_1}} \text{sgn}(v_m^{c_1}) \frac{1 - \text{sgn}(\delta_m^{c_1})}{2} - 2 \sum_{m=1}^{n_{d_1}} \text{sgn}(v_m^{d_1}) \frac{1 - \text{sgn}(\delta_m^{d_1})}{2} + \sum_{m=1}^{n_{e_1}} \text{sgn}(v_m^{e_1}) \frac{1 - \text{sgn}(\delta_m^{e_1})}{2} \\
& - \sum_{m=1}^{n_{e_2}} \text{sgn}(v_m^{e_2}) \frac{1 - \text{sgn}(\delta_m^{e_2})}{2} + 3 \sum_{m=1}^{n_{e_3}} \text{sgn}(v_m^{e_3}) \frac{1 - \text{sgn}(\delta_m^{e_3})}{2} - 3 \sum_{m=1}^{n_{e_4}} \text{sgn}(v_m^{e_4}) \frac{1 - \text{sgn}(\delta_m^{e_4})}{2} \\
& - 2 \sum_{m=1}^{n_{f_1}} \text{sgn}(v_m^{f_1}) \frac{1 - \text{sgn}(\delta_m^{f_1})}{2} + 2 \sum_{m=1}^{n_{f_2}} \text{sgn}(v_m^{f_2}) \frac{1 - \text{sgn}(\delta_m^{f_2})}{2} + \sum_{m=1}^{n_{g_1}} \text{sgn}(v_m^{g_1}) \frac{1 - \text{sgn}(\delta_m^{g_1})}{2} \\
& - \sum_{m=1}^{n_{g_2}} \text{sgn}(v_m^{g_2}) \frac{1 - \text{sgn}(\delta_m^{g_2})}{2} + 3 \sum_{m=1}^{n_{g_3}} \text{sgn}(v_m^{g_3}) \frac{1 - \text{sgn}(\delta_m^{g_3})}{2} - 3 \sum_{m=1}^{n_{g_4}} \text{sgn}(v_m^{g_4}) \frac{1 - \text{sgn}(\delta_m^{g_4})}{2} \pmod{8}
\end{aligned} \tag{S76.5}$$

### S77. SPACE GROUP NO. 77

| line segment                                      | character of irrep (generators only)                                                                                                                                                                                                                            |
|---------------------------------------------------|-----------------------------------------------------------------------------------------------------------------------------------------------------------------------------------------------------------------------------------------------------------------|
| $a \quad (\frac{t}{2}, 0, 0)$                     | $\begin{matrix} \{1 0 & 0 & 0\} \\ a_1 & 1 \end{matrix}$                                                                                                                                                                                                        |
| $b \quad (\frac{1}{2}, \frac{t}{2}, 0)$           | $\begin{matrix} \{1 0 & 0 & 0\} \\ b_1 & 1 \end{matrix}$                                                                                                                                                                                                        |
| $c \quad (\frac{t}{2}, 0, \frac{1}{2})$           | $\begin{matrix} \{1 0 & 0 & 0\} \\ c_1 & 1 \end{matrix}$                                                                                                                                                                                                        |
| $d \quad (\frac{1}{2}, \frac{t}{2}, \frac{1}{2})$ | $\begin{matrix} \{1 0 & 0 & 0\} \\ d_1 & 1 \end{matrix}$                                                                                                                                                                                                        |
| $e \quad (0, 0, \frac{t}{2})$                     | $\begin{matrix} \{4_{001} 0 & 0 & \frac{1}{2}\} \\ e_1 & e^{-\frac{1}{2}i\pi t - \frac{3i\pi}{4}} \\ e_2 & e^{\frac{3i\pi}{4} - \frac{i\pi t}{2}} \\ e_3 & e^{-\frac{1}{2}i\pi t - \frac{i\pi}{4}} \\ e_4 & e^{\frac{i\pi}{4} - \frac{i\pi t}{2}} \end{matrix}$ |
| $f \quad (\frac{1}{2}, 0, \frac{t}{2})$           | $\begin{matrix} \{2_{001} 0 & 0 & 0\} \\ f_1 & -i \\ f_2 & i \end{matrix}$                                                                                                                                                                                      |
| $g \quad (\frac{1}{2}, \frac{1}{2}, \frac{t}{2})$ | $\begin{matrix} \{4_{001} 0 & 0 & \frac{1}{2}\} \\ g_1 & e^{-\frac{1}{2}i\pi t - \frac{3i\pi}{4}} \\ g_2 & e^{\frac{3i\pi}{4} - \frac{i\pi t}{2}} \\ g_3 & e^{-\frac{1}{2}i\pi t - \frac{i\pi}{4}} \\ g_4 & e^{\frac{i\pi}{4} - \frac{i\pi t}{2}} \end{matrix}$ |



---


$$\begin{aligned}
\mathcal{W}_1^{\text{gapless}} = & \sum_{m=1}^{n_{a_1}} \text{sgn}(v_m^{a_1}) \frac{1 - \text{sgn}(\delta_m^{a_1})}{2} - \sum_{m=1}^{n_{c_1}} \text{sgn}(v_m^{c_1}) \frac{1 - \text{sgn}(\delta_m^{c_1})}{2} - \sum_{m=1}^{n_{e_1}} \text{sgn}(v_m^{e_1}) \frac{1 - \text{sgn}(\delta_m^{e_1})}{2} \\
& - \sum_{m=1}^{n_{e_2}} \text{sgn}(v_m^{e_2}) \frac{1 - \text{sgn}(\delta_m^{e_2})}{2} - \sum_{m=1}^{n_{e_3}} \text{sgn}(v_m^{e_3}) \frac{1 - \text{sgn}(\delta_m^{e_3})}{2} - \sum_{m=1}^{n_{e_4}} \text{sgn}(v_m^{e_4}) \frac{1 - \text{sgn}(\delta_m^{e_4})}{2} \\
& + \sum_{m=1}^{n_{f_1}} \text{sgn}(v_m^{f_1}) \frac{1 - \text{sgn}(\delta_m^{f_1})}{2} + \sum_{m=1}^{n_{f_2}} \text{sgn}(v_m^{f_2}) \frac{1 - \text{sgn}(\delta_m^{f_2})}{2}
\end{aligned} \tag{S77.1}$$

$$\begin{aligned}
\mathcal{W}_2^{\text{gapless}} = & \sum_{m=1}^{n_{b_1}} \text{sgn}(v_m^{b_1}) \frac{1 - \text{sgn}(\delta_m^{b_1})}{2} - \sum_{m=1}^{n_{d_1}} \text{sgn}(v_m^{d_1}) \frac{1 - \text{sgn}(\delta_m^{d_1})}{2} - \sum_{m=1}^{n_{f_1}} \text{sgn}(v_m^{f_1}) \frac{1 - \text{sgn}(\delta_m^{f_1})}{2} \\
& - \sum_{m=1}^{n_{f_2}} \text{sgn}(v_m^{f_2}) \frac{1 - \text{sgn}(\delta_m^{f_2})}{2} + \sum_{m=1}^{n_{g_1}} \text{sgn}(v_m^{g_1}) \frac{1 - \text{sgn}(\delta_m^{g_1})}{2} + \sum_{m=1}^{n_{g_2}} \text{sgn}(v_m^{g_2}) \frac{1 - \text{sgn}(\delta_m^{g_2})}{2} \\
& + \sum_{m=1}^{n_{g_3}} \text{sgn}(v_m^{g_3}) \frac{1 - \text{sgn}(\delta_m^{g_3})}{2} + \sum_{m=1}^{n_{g_4}} \text{sgn}(v_m^{g_4}) \frac{1 - \text{sgn}(\delta_m^{g_4})}{2}
\end{aligned} \tag{S77.2}$$

$$\begin{aligned}
\mathcal{W}_1^{\text{gapped}} = & - \sum_{m=1}^{n_{e_1}} \text{sgn}(v_m^{e_1}) \frac{1 - \text{sgn}(\delta_m^{e_1})}{2} + \sum_{m=1}^{n_{e_2}} \text{sgn}(v_m^{e_2}) \frac{1 - \text{sgn}(\delta_m^{e_2})}{2} + \sum_{m=1}^{n_{e_3}} \text{sgn}(v_m^{e_3}) \frac{1 - \text{sgn}(\delta_m^{e_3})}{2} \\
& - \sum_{m=1}^{n_{e_4}} \text{sgn}(v_m^{e_4}) \frac{1 - \text{sgn}(\delta_m^{e_4})}{2}
\end{aligned} \tag{S77.3}$$

$$\mathcal{W}_2^{\text{gapped}} = - \sum_{m=1}^{n_{f_1}} \text{sgn}(v_m^{f_1}) \frac{1 - \text{sgn}(\delta_m^{f_1})}{2} + \sum_{m=1}^{n_{f_2}} \text{sgn}(v_m^{f_2}) \frac{1 - \text{sgn}(\delta_m^{f_2})}{2} \tag{S77.4}$$

$$\begin{aligned}
\mathcal{W}_3^{\text{gapped}} = & \sum_{m=1}^{n_{g_1}} \text{sgn}(v_m^{g_1}) \frac{1 - \text{sgn}(\delta_m^{g_1})}{2} - \sum_{m=1}^{n_{g_2}} \text{sgn}(v_m^{g_2}) \frac{1 - \text{sgn}(\delta_m^{g_2})}{2} - \sum_{m=1}^{n_{g_3}} \text{sgn}(v_m^{g_3}) \frac{1 - \text{sgn}(\delta_m^{g_3})}{2} + \sum_{m=1}^{n_{g_4}} \text{sgn}(v_m^{g_4}) \frac{1 - \text{sgn}(\delta_m^{g_4})}{2}
\end{aligned} \tag{S77.5}$$

$$\mathcal{X}_1 = \sum_{m=1}^{n_{c_1}} \frac{1 - \text{sgn}(\delta_m^{c_1})}{2} \mod 2 \tag{S77.6}$$

$$\begin{aligned}
\mathcal{X}_2 = & - \sum_{m=1}^{n_{c_1}} \text{sgn}(v_m^{c_1}) \frac{1 - \text{sgn}(\delta_m^{c_1})}{2} - \sum_{m=1}^{n_{d_1}} \text{sgn}(v_m^{d_1}) \frac{1 - \text{sgn}(\delta_m^{d_1})}{2} - 2 \sum_{m=1}^{n_{e_3}} \text{sgn}(v_m^{e_3}) \frac{1 - \text{sgn}(\delta_m^{e_3})}{2} \\
& + 2 \sum_{m=1}^{n_{e_4}} \text{sgn}(v_m^{e_4}) \frac{1 - \text{sgn}(\delta_m^{e_4})}{2} - 2 \sum_{m=1}^{n_{g_1}} \text{sgn}(v_m^{g_1}) \frac{1 - \text{sgn}(\delta_m^{g_1})}{2} + 2 \sum_{m=1}^{n_{g_2}} \text{sgn}(v_m^{g_2}) \frac{1 - \text{sgn}(\delta_m^{g_2})}{2} \mod 4
\end{aligned} \tag{S77.7}$$

## S78. SPACE GROUP NO. 78

| line segment                                      | character of irrep (generators only)                                                                                                                                                                                                                               |
|---------------------------------------------------|--------------------------------------------------------------------------------------------------------------------------------------------------------------------------------------------------------------------------------------------------------------------|
| $a \quad (\frac{t}{2}, 0, 0)$                     | $\begin{matrix} \{1  0 & 0 & 0\} \\ a_1 & 1 \end{matrix}$                                                                                                                                                                                                          |
| $b \quad (\frac{1}{2}, \frac{t}{2}, 0)$           | $\begin{matrix} \{1  0 & 0 & 0\} \\ b_1 & 1 \end{matrix}$                                                                                                                                                                                                          |
| $c \quad (\frac{t}{2}, 0, \frac{1}{2})$           | $\begin{matrix} \{1  0 & 0 & 0\} \\ c_1 & 1 \end{matrix}$                                                                                                                                                                                                          |
| $d \quad (\frac{1}{2}, \frac{t}{2}, \frac{1}{2})$ | $\begin{matrix} \{1  0 & 0 & 0\} \\ d_1 & 1 \end{matrix}$                                                                                                                                                                                                          |
| $e \quad (0, 0, \frac{t}{2})$                     | $\begin{matrix} \{4_{001}  0 & 0 & \frac{3}{4}\} \\ e_1 & e^{-\frac{3}{4}i\pi t - \frac{3i\pi}{4}} \\ e_2 & e^{\frac{3i\pi}{4} - \frac{3i\pi t}{4}} \\ e_3 & e^{-\frac{3}{4}i\pi t - \frac{i\pi}{4}} \\ e_4 & e^{\frac{i\pi}{4} - \frac{3i\pi t}{4}} \end{matrix}$ |
| $f \quad (\frac{1}{2}, 0, \frac{t}{2})$           | $\begin{matrix} \{2_{001}  0 & 0 & \frac{1}{2}\} \\ f_1 & -ie^{-\frac{1}{2}i\pi t} \\ f_2 & ie^{-\frac{1}{2}i\pi t} \end{matrix}$                                                                                                                                  |
| $g \quad (\frac{1}{2}, \frac{1}{2}, \frac{t}{2})$ | $\begin{matrix} \{4_{001}  0 & 0 & \frac{3}{4}\} \\ g_1 & e^{-\frac{3}{4}i\pi t - \frac{3i\pi}{4}} \\ g_2 & e^{\frac{3i\pi}{4} - \frac{3i\pi t}{4}} \\ g_3 & e^{-\frac{3}{4}i\pi t - \frac{i\pi}{4}} \\ g_4 & e^{\frac{i\pi}{4} - \frac{3i\pi t}{4}} \end{matrix}$ |

$$\begin{aligned}
\mathcal{W}_1^{\text{gapless}} = & \sum_{m=1}^{n_{a_1}} \text{sgn}(v_m^{a_1}) \frac{1 - \text{sgn}(\delta_m^{a_1})}{2} - 2 \sum_{m=1}^{n_{c_1}} \text{sgn}(v_m^{c_1}) \frac{1 - \text{sgn}(\delta_m^{c_1})}{2} - \sum_{m=1}^{n_{e_1}} \text{sgn}(v_m^{e_1}) \frac{1 - \text{sgn}(\delta_m^{e_1})}{2} \\
& - \sum_{m=1}^{n_{e_2}} \text{sgn}(v_m^{e_2}) \frac{1 - \text{sgn}(\delta_m^{e_2})}{2} - \sum_{m=1}^{n_{e_3}} \text{sgn}(v_m^{e_3}) \frac{1 - \text{sgn}(\delta_m^{e_3})}{2} - \sum_{m=1}^{n_{e_4}} \text{sgn}(v_m^{e_4}) \frac{1 - \text{sgn}(\delta_m^{e_4})}{2} \\
& + \sum_{m=1}^{n_{f_1}} \text{sgn}(v_m^{f_1}) \frac{1 - \text{sgn}(\delta_m^{f_1})}{2} + \sum_{m=1}^{n_{f_2}} \text{sgn}(v_m^{f_2}) \frac{1 - \text{sgn}(\delta_m^{f_2})}{2}
\end{aligned} \tag{S78.1}$$

$$\begin{aligned}
\mathcal{W}_2^{\text{gapless}} = & \sum_{m=1}^{n_{b_1}} \text{sgn}(v_m^{b_1}) \frac{1 - \text{sgn}(\delta_m^{b_1})}{2} - 2 \sum_{m=1}^{n_{d_1}} \text{sgn}(v_m^{d_1}) \frac{1 - \text{sgn}(\delta_m^{d_1})}{2} - \sum_{m=1}^{n_{f_1}} \text{sgn}(v_m^{f_1}) \frac{1 - \text{sgn}(\delta_m^{f_1})}{2} \\
& - \sum_{m=1}^{n_{f_2}} \text{sgn}(v_m^{f_2}) \frac{1 - \text{sgn}(\delta_m^{f_2})}{2} + \sum_{m=1}^{n_{g_1}} \text{sgn}(v_m^{g_1}) \frac{1 - \text{sgn}(\delta_m^{g_1})}{2} + \sum_{m=1}^{n_{g_2}} \text{sgn}(v_m^{g_2}) \frac{1 - \text{sgn}(\delta_m^{g_2})}{2} \\
& + \sum_{m=1}^{n_{g_3}} \text{sgn}(v_m^{g_3}) \frac{1 - \text{sgn}(\delta_m^{g_3})}{2} + \sum_{m=1}^{n_{g_4}} \text{sgn}(v_m^{g_4}) \frac{1 - \text{sgn}(\delta_m^{g_4})}{2}
\end{aligned} \tag{S78.2}$$

$$\mathcal{X}_1 = \sum_{m=1}^{n_{e_1}} \frac{1 - \text{sgn}(\delta_m^{e_1})}{2} + \sum_{m=1}^{n_{e_2}} \frac{1 - \text{sgn}(\delta_m^{e_2})}{2} + \sum_{m=1}^{n_{e_3}} \frac{1 - \text{sgn}(\delta_m^{e_3})}{2} + \sum_{m=1}^{n_{e_4}} \frac{1 - \text{sgn}(\delta_m^{e_4})}{2} \pmod{2} \tag{S78.3}$$

$$\begin{aligned}
\mathcal{X}_2 = & -2 \sum_{m=1}^{n_{c_1}} \text{sgn}(v_m^{c_1}) \frac{1 - \text{sgn}(\delta_m^{c_1})}{2} + \sum_{m=1}^{n_{e_1}} \text{sgn}(v_m^{e_1}) \frac{1 - \text{sgn}(\delta_m^{e_1})}{2} - \sum_{m=1}^{n_{e_2}} \text{sgn}(v_m^{e_2}) \frac{1 - \text{sgn}(\delta_m^{e_2})}{2} + 3 \sum_{m=1}^{n_{e_3}} \text{sgn}(v_m^{e_3}) \frac{1 - \text{sgn}(\delta_m^{e_3})}{2} \\
& - 3 \sum_{m=1}^{n_{e_4}} \text{sgn}(v_m^{e_4}) \frac{1 - \text{sgn}(\delta_m^{e_4})}{2} - \sum_{m=1}^{n_{f_1}} \text{sgn}(v_m^{f_1}) \frac{1 - \text{sgn}(\delta_m^{f_1})}{2} + \sum_{m=1}^{n_{f_2}} \text{sgn}(v_m^{f_2}) \frac{1 - \text{sgn}(\delta_m^{f_2})}{2} + 2 \sum_{m=1}^{n_{g_1}} \text{sgn}(v_m^{g_1}) \frac{1 - \text{sgn}(\delta_m^{g_1})}{2} \\
& - 2 \sum_{m=1}^{n_{g_2}} \text{sgn}(v_m^{g_2}) \frac{1 - \text{sgn}(\delta_m^{g_2})}{2} + 2 \sum_{m=1}^{n_{g_3}} \text{sgn}(v_m^{g_3}) \frac{1 - \text{sgn}(\delta_m^{g_3})}{2} - 2 \sum_{m=1}^{n_{g_4}} \text{sgn}(v_m^{g_4}) \frac{1 - \text{sgn}(\delta_m^{g_4})}{2} \pmod{4}
\end{aligned} \tag{S78.4}$$

$$\begin{aligned}
\mathcal{X}_3 = & 2 \sum_{m=1}^{n_{c_1}} \text{sgn}(v_m^{c_1}) \frac{1 - \text{sgn}(\delta_m^{c_1})}{2} - 2 \sum_{m=1}^{n_{d_1}} \text{sgn}(v_m^{d_1}) \frac{1 - \text{sgn}(\delta_m^{d_1})}{2} - \sum_{m=1}^{n_{e_1}} \text{sgn}(v_m^{e_1}) \frac{1 - \text{sgn}(\delta_m^{e_1})}{2} \\
& + \sum_{m=1}^{n_{e_2}} \text{sgn}(v_m^{e_2}) \frac{1 - \text{sgn}(\delta_m^{e_2})}{2} - 3 \sum_{m=1}^{n_{e_3}} \text{sgn}(v_m^{e_3}) \frac{1 - \text{sgn}(\delta_m^{e_3})}{2} + 3 \sum_{m=1}^{n_{e_4}} \text{sgn}(v_m^{e_4}) \frac{1 - \text{sgn}(\delta_m^{e_4})}{2} \\
& - 2 \sum_{m=1}^{n_{f_1}} \text{sgn}(v_m^{f_1}) \frac{1 - \text{sgn}(\delta_m^{f_1})}{2} + 2 \sum_{m=1}^{n_{f_2}} \text{sgn}(v_m^{f_2}) \frac{1 - \text{sgn}(\delta_m^{f_2})}{2} - \sum_{m=1}^{n_{g_1}} \text{sgn}(v_m^{g_1}) \frac{1 - \text{sgn}(\delta_m^{g_1})}{2} \\
& + \sum_{m=1}^{n_{g_2}} \text{sgn}(v_m^{g_2}) \frac{1 - \text{sgn}(\delta_m^{g_2})}{2} - 3 \sum_{m=1}^{n_{g_3}} \text{sgn}(v_m^{g_3}) \frac{1 - \text{sgn}(\delta_m^{g_3})}{2} + 3 \sum_{m=1}^{n_{g_4}} \text{sgn}(v_m^{g_4}) \frac{1 - \text{sgn}(\delta_m^{g_4})}{2} \pmod{8}
\end{aligned} \tag{S78.5}$$

### S79. SPACE GROUP NO. 79

| line segment                                      | character of irrep (generators only)                                                                                                                  |
|---------------------------------------------------|-------------------------------------------------------------------------------------------------------------------------------------------------------|
| $a \ (0, 0, t)$                                   | $\{4_{001}   0 \ 0 \ 0\}$<br>$a_1 \ e^{-\frac{3i\pi}{4}}$<br>$a_2 \ e^{\frac{3i\pi}{4}}$<br>$a_3 \ e^{-\frac{i\pi}{4}}$<br>$a_4 \ e^{\frac{i\pi}{4}}$ |
| $b \ (\frac{1}{2}, \frac{1}{2}, \frac{t}{2})$     | $\{2_{001}   0 \ 0 \ 0\}$<br>$b_1 \ -i$<br>$b_2 \ i$                                                                                                  |
| $c \ (\frac{t}{2}, \frac{t}{2}, 1 - \frac{t}{2})$ | $\{1   0 \ 0 \ 0\}$<br>$c_1 \ 1$                                                                                                                      |
| $d \ (\frac{t}{2}, \frac{t}{2}, 0)$               | $\{1   0 \ 0 \ 0\}$<br>$d_1 \ 1$                                                                                                                      |
| $e \ (\frac{t}{2}, 1 - \frac{t}{2}, 0)$           | $\{1   0 \ 0 \ 0\}$<br>$e_1 \ 1$                                                                                                                      |
| $f \ (0, \frac{t}{2}, 1 - \frac{t}{2})$           | $\{1   0 \ 0 \ 0\}$<br>$f_1 \ 1$                                                                                                                      |

$$\begin{aligned}
\mathcal{W}_1^{\text{gapless}} = & \sum_{m=1}^{n_{a_1}} \text{sgn}(v_m^{a_1}) \frac{1 - \text{sgn}(\delta_m^{a_1})}{2} + \sum_{m=1}^{n_{a_2}} \text{sgn}(v_m^{a_2}) \frac{1 - \text{sgn}(\delta_m^{a_2})}{2} + \sum_{m=1}^{n_{a_3}} \text{sgn}(v_m^{a_3}) \frac{1 - \text{sgn}(\delta_m^{a_3})}{2} \\
& + \sum_{m=1}^{n_{a_4}} \text{sgn}(v_m^{a_4}) \frac{1 - \text{sgn}(\delta_m^{a_4})}{2} - \sum_{m=1}^{n_{d_1}} \text{sgn}(v_m^{d_1}) \frac{1 - \text{sgn}(\delta_m^{d_1})}{2} + \sum_{m=1}^{n_{e_1}} \text{sgn}(v_m^{e_1}) \frac{1 - \text{sgn}(\delta_m^{e_1})}{2}
\end{aligned} \tag{S79.1}$$

$$\mathcal{W}_2^{\text{gapless}} = \sum_{m=1}^{n_{b_1}} \text{sgn}(v_m^{b_1}) \frac{1 - \text{sgn}(\delta_m^{b_1})}{2} + \sum_{m=1}^{n_{b_2}} \text{sgn}(v_m^{b_2}) \frac{1 - \text{sgn}(\delta_m^{b_2})}{2} - \sum_{m=1}^{n_{c_1}} \text{sgn}(v_m^{c_1}) \frac{1 - \text{sgn}(\delta_m^{c_1})}{2} + \sum_{m=1}^{n_{e_1}} \text{sgn}(v_m^{e_1}) \frac{1 - \text{sgn}(\delta_m^{e_1})}{2} \quad (\text{S79.2})$$

$$\begin{aligned} \mathcal{W}_1^{\text{gapped}} = & -2 \sum_{m=1}^{n_{a_2}} \text{sgn}(v_m^{a_2}) \frac{1 - \text{sgn}(\delta_m^{a_2})}{2} - 2 \sum_{m=1}^{n_{a_4}} \text{sgn}(v_m^{a_4}) \frac{1 - \text{sgn}(\delta_m^{a_4})}{2} \\ & + 2 \sum_{m=1}^{n_{b_2}} \text{sgn}(v_m^{b_2}) \frac{1 - \text{sgn}(\delta_m^{b_2})}{2} - \sum_{m=1}^{n_{c_1}} \text{sgn}(v_m^{c_1}) \frac{1 - \text{sgn}(\delta_m^{c_1})}{2} + \sum_{m=1}^{n_{d_1}} \text{sgn}(v_m^{d_1}) \frac{1 - \text{sgn}(\delta_m^{d_1})}{2} \end{aligned} \quad (\text{S79.3})$$

$$\mathcal{W}_2^{\text{gapped}} = 2 \sum_{m=1}^{n_{b_2}} \text{sgn}(v_m^{b_2}) \frac{1 - \text{sgn}(\delta_m^{b_2})}{2} - \sum_{m=1}^{n_{c_1}} \text{sgn}(v_m^{c_1}) \frac{1 - \text{sgn}(\delta_m^{c_1})}{2} + \sum_{m=1}^{n_{e_1}} \text{sgn}(v_m^{e_1}) \frac{1 - \text{sgn}(\delta_m^{e_1})}{2} \quad (\text{S79.4})$$

$$\mathcal{W}_3^{\text{gapped}} = \sum_{m=1}^{n_{a_3}} \text{sgn}(v_m^{a_3}) \frac{1 - \text{sgn}(\delta_m^{a_3})}{2} - \sum_{m=1}^{n_{a_4}} \text{sgn}(v_m^{a_4}) \frac{1 - \text{sgn}(\delta_m^{a_4})}{2} \quad (\text{S79.5})$$

$$\mathcal{X}_1 = \sum_{m=1}^{n_{f_1}} \frac{1 - \text{sgn}(\delta_m^{f_1})}{2} \quad \text{mod } 2 \quad (\text{S79.6})$$

$$\mathcal{X}_2 = \sum_{m=1}^{n_{c_1}} \frac{1 - \text{sgn}(\delta_m^{c_1})}{2} + \sum_{m=1}^{n_{f_1}} \frac{1 - \text{sgn}(\delta_m^{f_1})}{2} \quad \text{mod } 2 \quad (\text{S79.7})$$

### S80. SPACE GROUP NO. 80

| line segment                                          | character of irrep (generators only)                                                                                                                                                                                                                                            |
|-------------------------------------------------------|---------------------------------------------------------------------------------------------------------------------------------------------------------------------------------------------------------------------------------------------------------------------------------|
| $a \quad (0, 0, t)$                                   | $\{4_{001}   0 \quad \frac{1}{2} \quad \frac{1}{4}\}$<br>$a_1 \quad e^{-\frac{1}{2}i\pi t - \frac{3i\pi}{4}}$<br>$a_2 \quad e^{\frac{3i\pi}{4} - \frac{i\pi t}{2}}$<br>$a_3 \quad e^{-\frac{1}{2}i\pi t - \frac{i\pi}{4}}$<br>$a_4 \quad e^{\frac{i\pi}{4} - \frac{i\pi t}{2}}$ |
| $b \quad (\frac{1}{2}, \frac{1}{2}, \frac{t}{2})$     | $\{2_{001}   0 \quad 0 \quad 0\}$<br>$b_1 \quad -i$<br>$b_2 \quad i$                                                                                                                                                                                                            |
| $c \quad (\frac{t}{2}, \frac{t}{2}, 1 - \frac{t}{2})$ | $\{1   0 \quad 0 \quad 0\}$<br>$c_1 \quad 1$                                                                                                                                                                                                                                    |
| $d \quad (\frac{t}{2}, \frac{t}{2}, 0)$               | $\{1   0 \quad 0 \quad 0\}$<br>$d_1 \quad 1$                                                                                                                                                                                                                                    |
| $e \quad (\frac{t}{2}, 1 - \frac{t}{2}, 0)$           | $\{1   0 \quad 0 \quad 0\}$<br>$e_1 \quad 1$                                                                                                                                                                                                                                    |
| $f \quad (0, \frac{t}{2}, 1 - \frac{t}{2})$           | $\{1   0 \quad 0 \quad 0\}$<br>$f_1 \quad 1$                                                                                                                                                                                                                                    |

---


$$\begin{aligned} \mathcal{W}_1^{\text{gapless}} = & \sum_{m=1}^{n_{a_1}} \text{sgn}(v_m^{a_1}) \frac{1 - \text{sgn}(\delta_m^{a_1})}{2} + \sum_{m=1}^{n_{a_2}} \text{sgn}(v_m^{a_2}) \frac{1 - \text{sgn}(\delta_m^{a_2})}{2} + \sum_{m=1}^{n_{a_3}} \text{sgn}(v_m^{a_3}) \frac{1 - \text{sgn}(\delta_m^{a_3})}{2} \\ & + \sum_{m=1}^{n_{a_4}} \text{sgn}(v_m^{a_4}) \frac{1 - \text{sgn}(\delta_m^{a_4})}{2} - \sum_{m=1}^{n_{d_1}} \text{sgn}(v_m^{d_1}) \frac{1 - \text{sgn}(\delta_m^{d_1})}{2} + \sum_{m=1}^{n_{e_1}} \text{sgn}(v_m^{e_1}) \frac{1 - \text{sgn}(\delta_m^{e_1})}{2} \end{aligned} \quad (\text{S80.1})$$

$$\mathcal{W}_2^{\text{gapless}} = \sum_{m=1}^{n_{b_1}} \text{sgn}(v_m^{b_1}) \frac{1 - \text{sgn}(\delta_m^{b_1})}{2} + \sum_{m=1}^{n_{b_2}} \text{sgn}(v_m^{b_2}) \frac{1 - \text{sgn}(\delta_m^{b_2})}{2} - \sum_{m=1}^{n_{c_1}} \text{sgn}(v_m^{c_1}) \frac{1 - \text{sgn}(\delta_m^{c_1})}{2} + \sum_{m=1}^{n_{e_1}} \text{sgn}(v_m^{e_1}) \frac{1 - \text{sgn}(\delta_m^{e_1})}{2} \quad (\text{S80.2})$$

$$\begin{aligned} \mathcal{W}_1^{\text{gapped}} = & 2 \sum_{m=1}^{n_{a_2}} \text{sgn}(v_m^{a_2}) \frac{1 - \text{sgn}(\delta_m^{a_2})}{2} + 2 \sum_{m=1}^{n_{a_3}} \text{sgn}(v_m^{a_3}) \frac{1 - \text{sgn}(\delta_m^{a_3})}{2} - \sum_{m=1}^{n_{d_1}} \text{sgn}(v_m^{d_1}) \frac{1 - \text{sgn}(\delta_m^{d_1})}{2} \\ & + \sum_{m=1}^{n_{e_1}} \text{sgn}(v_m^{e_1}) \frac{1 - \text{sgn}(\delta_m^{e_1})}{2} \end{aligned} \quad (\text{S80.3})$$

$$\mathcal{X}_1 = \sum_{m=1}^{n_{f_1}} \frac{1 - \text{sgn}(\delta_m^{f_1})}{2} \quad \text{mod } 2 \quad (\text{S80.4})$$

$$\begin{aligned} \mathcal{X}_2 = & 2 \sum_{m=1}^{n_{a_2}} \text{sgn}(v_m^{a_2}) \frac{1 - \text{sgn}(\delta_m^{a_2})}{2} + 6 \sum_{m=1}^{n_{a_4}} \text{sgn}(v_m^{a_4}) \frac{1 - \text{sgn}(\delta_m^{a_4})}{2} - 2 \sum_{m=1}^{n_{b_2}} \text{sgn}(v_m^{b_2}) \frac{1 - \text{sgn}(\delta_m^{b_2})}{2} \\ & - \sum_{m=1}^{n_{d_1}} \text{sgn}(v_m^{d_1}) \frac{1 - \text{sgn}(\delta_m^{d_1})}{2} - 2 \sum_{m=1}^{n_{f_1}} \text{sgn}(v_m^{f_1}) \frac{1 - \text{sgn}(\delta_m^{f_1})}{2} \quad \text{mod } 4 \end{aligned} \quad (\text{S80.5})$$

### S81. SPACE GROUP NO. 81

| line segment                                      | character of irrep (generators only)                                                  |
|---------------------------------------------------|---------------------------------------------------------------------------------------|
| $a \quad (\frac{t}{2}, 0, 0)$                     | $\begin{array}{c} \{1   0 \ 0 \ 0\} \\ a_1 \quad 1 \end{array}$                       |
| $b \quad (\frac{1}{2}, \frac{t}{2}, 0)$           | $\begin{array}{c} \{1   0 \ 0 \ 0\} \\ b_1 \quad 1 \end{array}$                       |
| $c \quad (\frac{t}{2}, 0, \frac{1}{2})$           | $\begin{array}{c} \{1   0 \ 0 \ 0\} \\ c_1 \quad 1 \end{array}$                       |
| $d \quad (\frac{1}{2}, \frac{t}{2}, \frac{1}{2})$ | $\begin{array}{c} \{1   0 \ 0 \ 0\} \\ d_1 \quad 1 \end{array}$                       |
| $e \quad (0, 0, \frac{t}{2})$                     | $\begin{array}{c} \{2_{001}   0 \ 0 \ 0\} \\ e_1 \quad -i \\ e_2 \quad i \end{array}$ |
| $f \quad (\frac{1}{2}, 0, \frac{t}{2})$           | $\begin{array}{c} \{2_{001}   0 \ 0 \ 0\} \\ f_1 \quad -i \\ f_2 \quad i \end{array}$ |

| $g$ $(\frac{1}{2}, \frac{1}{2}, \frac{t}{2})$ | $\{2_{001}   0 \ 0 \ 0 \}$ |
|-----------------------------------------------|----------------------------|
| $g_1$                                         | $-i$                       |
| $g_2$                                         | $i$                        |

$$\begin{aligned} \mathcal{W}_1^{\text{gapless}} = & \sum_{m=1}^{n_{a_1}} \text{sgn}(v_m^{a_1}) \frac{1 - \text{sgn}(\delta_m^{a_1})}{2} - \sum_{m=1}^{n_{c_1}} \text{sgn}(v_m^{c_1}) \frac{1 - \text{sgn}(\delta_m^{c_1})}{2} - 2 \sum_{m=1}^{n_{e_1}} \text{sgn}(v_m^{e_1}) \frac{1 - \text{sgn}(\delta_m^{e_1})}{2} \\ & + \sum_{m=1}^{n_{f_1}} \text{sgn}(v_m^{f_1}) \frac{1 - \text{sgn}(\delta_m^{f_1})}{2} + \sum_{m=1}^{n_{f_2}} \text{sgn}(v_m^{f_2}) \frac{1 - \text{sgn}(\delta_m^{f_2})}{2} \end{aligned} \quad (\text{S81.1})$$

$$\begin{aligned} \mathcal{W}_2^{\text{gapless}} = & \sum_{m=1}^{n_{b_1}} \text{sgn}(v_m^{b_1}) \frac{1 - \text{sgn}(\delta_m^{b_1})}{2} - \sum_{m=1}^{n_{d_1}} \text{sgn}(v_m^{d_1}) \frac{1 - \text{sgn}(\delta_m^{d_1})}{2} - \sum_{m=1}^{n_{f_1}} \text{sgn}(v_m^{f_1}) \frac{1 - \text{sgn}(\delta_m^{f_1})}{2} \\ & - \sum_{m=1}^{n_{f_2}} \text{sgn}(v_m^{f_2}) \frac{1 - \text{sgn}(\delta_m^{f_2})}{2} + 2 \sum_{m=1}^{n_{g_1}} \text{sgn}(v_m^{g_1}) \frac{1 - \text{sgn}(\delta_m^{g_1})}{2} \end{aligned} \quad (\text{S81.2})$$

$$\mathcal{W}_1^{\text{gapped}} = - \sum_{m=1}^{n_{f_1}} \text{sgn}(v_m^{f_1}) \frac{1 - \text{sgn}(\delta_m^{f_1})}{2} + \sum_{m=1}^{n_{f_2}} \text{sgn}(v_m^{f_2}) \frac{1 - \text{sgn}(\delta_m^{f_2})}{2} \quad (\text{S81.3})$$

$$\mathcal{X}_1 = \sum_{m=1}^{n_{c_1}} \frac{1 - \text{sgn}(\delta_m^{c_1})}{2} + \sum_{m=1}^{n_{d_1}} \frac{1 - \text{sgn}(\delta_m^{d_1})}{2} \quad \text{mod } 2 \quad (\text{S81.4})$$

$$\mathcal{X}_2 = \sum_{m=1}^{n_{d_1}} \frac{1 - \text{sgn}(\delta_m^{d_1})}{2} \quad \text{mod } 2 \quad (\text{S81.5})$$

## S82. SPACE GROUP NO. 82

| line segment                                      | character of irrep (generators only)                          |
|---------------------------------------------------|---------------------------------------------------------------|
| $a \ (0, 0, t)$                                   | $\{2_{001}   0 \ 0 \ 0 \}$<br>$a_1 \quad -i$<br>$a_2 \quad i$ |
| $b \ (\frac{1}{2}, \frac{1}{2}, \frac{t}{2})$     | $\{2_{001}   0 \ 0 \ 0 \}$<br>$b_1 \quad -i$<br>$b_2 \quad i$ |
| $c \ (\frac{t}{2}, \frac{t}{2}, 1 - \frac{t}{2})$ | $\{1   0 \ 0 \ 0 \}$<br>$c_1 \quad 1$                         |
| $d \ (\frac{t}{2}, \frac{t}{2}, 0)$               | $\{1   0 \ 0 \ 0 \}$<br>$d_1 \quad 1$                         |
| $e \ (\frac{t}{2}, 1 - \frac{t}{2}, 0)$           | $\{1   0 \ 0 \ 0 \}$<br>$e_1 \quad 1$                         |
| $f \ (0, \frac{t}{2}, 1 - \frac{t}{2})$           | $\{1   0 \ 0 \ 0 \}$<br>$f_1 \quad 1$                         |

$$\mathcal{W}_1^{\text{gapless}} = 2 \sum_{m=1}^{n_{a_1}} \text{sgn}(v_m^{a_1}) \frac{1 - \text{sgn}(\delta_m^{a_1})}{2} - \sum_{m=1}^{n_{d_1}} \text{sgn}(v_m^{d_1}) \frac{1 - \text{sgn}(\delta_m^{d_1})}{2} + \sum_{m=1}^{n_{e_1}} \text{sgn}(v_m^{e_1}) \frac{1 - \text{sgn}(\delta_m^{e_1})}{2} \quad (\text{S82.1})$$

$$\mathcal{W}_2^{\text{gapless}} = \sum_{m=1}^{n_{b_1}} \text{sgn}(v_m^{b_1}) \frac{1 - \text{sgn}(\delta_m^{b_1})}{2} + \sum_{m=1}^{n_{b_2}} \text{sgn}(v_m^{b_2}) \frac{1 - \text{sgn}(\delta_m^{b_2})}{2} - \sum_{m=1}^{n_{c_1}} \text{sgn}(v_m^{c_1}) \frac{1 - \text{sgn}(\delta_m^{c_1})}{2} + \sum_{m=1}^{n_{e_1}} \text{sgn}(v_m^{e_1}) \frac{1 - \text{sgn}(\delta_m^{e_1})}{2} \quad (\text{S82.2})$$

$$\mathcal{X}_1 = \sum_{m=1}^{n_{f_1}} \frac{1 - \text{sgn}(\delta_m^{f_1})}{2} \mod 2 \quad (\text{S82.3})$$

$$\mathcal{X}_2 = \sum_{m=1}^{n_{d_1}} \frac{1 - \text{sgn}(\delta_m^{d_1})}{2} \mod 2 \quad (\text{S82.4})$$

### S83. SPACE GROUP NO. 83

| line segment                                      | character of irrep (generators only)                                                                                                                                  |
|---------------------------------------------------|-----------------------------------------------------------------------------------------------------------------------------------------------------------------------|
| $a \quad (\frac{t}{2}, 0, 0)$                     | $\{m_{001}   0 \ 0 \ 0\}$<br>$a_1 \quad -i$<br>$a_2 \quad i$                                                                                                          |
| $b \quad (\frac{1}{2}, \frac{t}{2}, 0)$           | $\{m_{001}   0 \ 0 \ 0\}$<br>$b_1 \quad -i$<br>$b_2 \quad i$                                                                                                          |
| $c \quad (\frac{t}{2}, 0, \frac{1}{2})$           | $\{m_{001}   0 \ 0 \ 0\}$<br>$c_1 \quad -i$<br>$c_2 \quad i$                                                                                                          |
| $d \quad (\frac{1}{2}, \frac{t}{2}, \frac{1}{2})$ | $\{m_{001}   0 \ 0 \ 0\}$<br>$d_1 \quad -i$<br>$d_2 \quad i$                                                                                                          |
| $e \quad (0, 0, \frac{t}{2})$                     | $\{4_{001}   0 \ 0 \ 0\}$<br>$e_1 \quad e^{-\frac{3i\pi}{4}}$<br>$e_2 \quad e^{\frac{3i\pi}{4}}$<br>$e_3 \quad e^{-\frac{i\pi}{4}}$<br>$e_4 \quad e^{\frac{i\pi}{4}}$ |
| $f \quad (\frac{1}{2}, 0, \frac{t}{2})$           | $\{2_{001}   0 \ 0 \ 0\}$<br>$f_1 \quad -i$<br>$f_2 \quad i$                                                                                                          |
| $g \quad (\frac{1}{2}, \frac{1}{2}, \frac{t}{2})$ | $\{4_{001}   0 \ 0 \ 0\}$<br>$g_1 \quad e^{-\frac{3i\pi}{4}}$<br>$g_2 \quad e^{\frac{3i\pi}{4}}$<br>$g_3 \quad e^{-\frac{i\pi}{4}}$<br>$g_4 \quad e^{\frac{i\pi}{4}}$ |

---


$$\mathcal{W}_1^{\text{gapless}} = \sum_{m=1}^{n_{a_1}} \text{sgn}(v_m^{a_1}) \frac{1 - \text{sgn}(\delta_m^{a_1})}{2} - \sum_{m=1}^{n_{c_1}} \text{sgn}(v_m^{c_1}) \frac{1 - \text{sgn}(\delta_m^{c_1})}{2} - \sum_{m=1}^{n_{e_1}} \text{sgn}(v_m^{e_1}) \frac{1 - \text{sgn}(\delta_m^{e_1})}{2} \\ - \sum_{m=1}^{n_{e_3}} \text{sgn}(v_m^{e_3}) \frac{1 - \text{sgn}(\delta_m^{e_3})}{2} + \sum_{m=1}^{n_{f_1}} \text{sgn}(v_m^{f_1}) \frac{1 - \text{sgn}(\delta_m^{f_1})}{2} \quad (\text{S83.1})$$

$$\mathcal{W}_2^{\text{gapless}} = \sum_{m=1}^{n_{b_1}} \text{sgn}(v_m^{b_1}) \frac{1 - \text{sgn}(\delta_m^{b_1})}{2} - \sum_{m=1}^{n_{d_1}} \text{sgn}(v_m^{d_1}) \frac{1 - \text{sgn}(\delta_m^{d_1})}{2} - \sum_{m=1}^{n_{f_1}} \text{sgn}(v_m^{f_1}) \frac{1 - \text{sgn}(\delta_m^{f_1})}{2} \\ + \sum_{m=1}^{n_{g_1}} \text{sgn}(v_m^{g_1}) \frac{1 - \text{sgn}(\delta_m^{g_1})}{2} + \sum_{m=1}^{n_{g_3}} \text{sgn}(v_m^{g_3}) \frac{1 - \text{sgn}(\delta_m^{g_3})}{2} \quad (\text{S83.2})$$

#### S84. SPACE GROUP NO. 84

| line segment                                      | character of irrep (generators only)                                                                                                                                                                                                                          |
|---------------------------------------------------|---------------------------------------------------------------------------------------------------------------------------------------------------------------------------------------------------------------------------------------------------------------|
| $a \quad (\frac{t}{2}, 0, 0)$                     | $\{m_{001}   0 \ 0 \ 0\}$<br>$a_1 \quad -i$<br>$a_2 \quad i$                                                                                                                                                                                                  |
| $b \quad (\frac{1}{2}, \frac{t}{2}, 0)$           | $\{m_{001}   0 \ 0 \ 0\}$<br>$b_1 \quad -i$<br>$b_2 \quad i$                                                                                                                                                                                                  |
| $c \quad (\frac{t}{2}, 0, \frac{1}{2})$           | $\{m_{001}   0 \ 0 \ 0\}$<br>$c_1 \quad -i$<br>$c_2 \quad i$                                                                                                                                                                                                  |
| $d \quad (\frac{1}{2}, \frac{t}{2}, \frac{1}{2})$ | $\{m_{001}   0 \ 0 \ 0\}$<br>$d_1 \quad -i$<br>$d_2 \quad i$                                                                                                                                                                                                  |
| $e \quad (0, 0, \frac{t}{2})$                     | $\{4_{001}   0 \ 0 \ \frac{1}{2}\}$<br>$e_1 \quad e^{-\frac{1}{2}i\pi t - \frac{3i\pi}{4}}$<br>$e_2 \quad e^{\frac{3i\pi}{4} - \frac{i\pi t}{2}}$<br>$e_3 \quad e^{-\frac{1}{2}i\pi t - \frac{i\pi}{4}}$<br>$e_4 \quad e^{\frac{i\pi}{4} - \frac{i\pi t}{2}}$ |
| $f \quad (\frac{1}{2}, 0, \frac{t}{2})$           | $\{2_{001}   0 \ 0 \ 0\}$<br>$f_1 \quad -i$<br>$f_2 \quad i$                                                                                                                                                                                                  |
| $g \quad (\frac{1}{2}, \frac{1}{2}, \frac{t}{2})$ | $\{4_{001}   0 \ 0 \ \frac{1}{2}\}$<br>$g_1 \quad e^{-\frac{1}{2}i\pi t - \frac{3i\pi}{4}}$<br>$g_2 \quad e^{\frac{3i\pi}{4} - \frac{i\pi t}{2}}$<br>$g_3 \quad e^{-\frac{1}{2}i\pi t - \frac{i\pi}{4}}$<br>$g_4 \quad e^{\frac{i\pi}{4} - \frac{i\pi t}{2}}$ |

$$\mathcal{W}_1^{\text{gapless}} = \sum_{m=1}^{n_{a_1}} \text{sgn}(v_m^{a_1}) \frac{1 - \text{sgn}(\delta_m^{a_1})}{2} - \sum_{m=1}^{n_{c_1}} \text{sgn}(v_m^{c_1}) \frac{1 - \text{sgn}(\delta_m^{c_1})}{2} - \sum_{m=1}^{n_{e_1}} \text{sgn}(v_m^{e_1}) \frac{1 - \text{sgn}(\delta_m^{e_1})}{2} \\ - \sum_{m=1}^{n_{e_3}} \text{sgn}(v_m^{e_3}) \frac{1 - \text{sgn}(\delta_m^{e_3})}{2} + \sum_{m=1}^{n_{f_1}} \text{sgn}(v_m^{f_1}) \frac{1 - \text{sgn}(\delta_m^{f_1})}{2} \quad (\text{S84.1})$$



$$\begin{aligned} \mathcal{W}_2^{\text{gapless}} = & \sum_{m=1}^{n_{b_1}} \text{sgn}(v_m^{b_1}) \frac{1 - \text{sgn}(\delta_m^{b_1})}{2} - \sum_{m=1}^{n_{d_1}} \text{sgn}(v_m^{d_1}) \frac{1 - \text{sgn}(\delta_m^{d_1})}{2} - \sum_{m=1}^{n_{f_1}} \text{sgn}(v_m^{f_1}) \frac{1 - \text{sgn}(\delta_m^{f_1})}{2} \\ & + \sum_{m=1}^{n_{g_1}} \text{sgn}(v_m^{g_1}) \frac{1 - \text{sgn}(\delta_m^{g_1})}{2} + \sum_{m=1}^{n_{g_3}} \text{sgn}(v_m^{g_3}) \frac{1 - \text{sgn}(\delta_m^{g_3})}{2} \end{aligned} \quad (\text{S84.2})$$

$$\mathcal{X}_1 = \sum_{m=1}^{n_{c_1}} \frac{1 - \text{sgn}(\delta_m^{c_1})}{2} + \sum_{m=1}^{n_{d_1}} \frac{1 - \text{sgn}(\delta_m^{d_1})}{2} \quad \text{mod } 2 \quad (\text{S84.3})$$

### S85. SPACE GROUP NO. 85

| line segment                                      | character of irrep (generators only)                                                                                                                                                |
|---------------------------------------------------|-------------------------------------------------------------------------------------------------------------------------------------------------------------------------------------|
| $a \quad (\frac{t}{2}, 0, 0)$                     | $\{m_{001}   \frac{1}{2} \frac{1}{2} 0\}$<br>$a_1 \quad -ie^{-\frac{1}{2}i\pi t}$<br>$a_2 \quad ie^{-\frac{1}{2}i\pi t}$                                                            |
| $b \quad (\frac{1}{2}, \frac{t}{2}, 0)$           | $\{m_{001}   \frac{1}{2} \frac{1}{2} 0\}$<br>$b_1 \quad -ie^{-\frac{1}{2}i\pi(t+1)}$<br>$b_2 \quad ie^{-\frac{1}{2}i\pi(t+1)}$                                                      |
| $c \quad (\frac{t}{2}, 0, \frac{1}{2})$           | $\{m_{001}   \frac{1}{2} \frac{1}{2} 0\}$<br>$c_1 \quad -ie^{-\frac{1}{2}i\pi t}$<br>$c_2 \quad ie^{-\frac{1}{2}i\pi t}$                                                            |
| $d \quad (\frac{1}{2}, \frac{t}{2}, \frac{1}{2})$ | $\{m_{001}   \frac{1}{2} \frac{1}{2} 0\}$<br>$d_1 \quad -ie^{-\frac{1}{2}i\pi(t+1)}$<br>$d_2 \quad ie^{-\frac{1}{2}i\pi(t+1)}$                                                      |
| $e \quad (0, 0, \frac{t}{2})$                     | $\{4_{001}   \frac{1}{2} 0 0\}$<br>$e_1 \quad e^{-\frac{3i\pi}{4}}$<br>$e_2 \quad e^{\frac{3i\pi}{4}}$<br>$e_3 \quad e^{-\frac{i\pi}{4}}$<br>$e_4 \quad e^{\frac{i\pi}{4}}$         |
| $f \quad (\frac{1}{2}, 0, \frac{t}{2})$           | $\{2_{001}   \frac{1}{2} \frac{1}{2} 0\}$<br>$f_1 \quad i$<br>$f_2 \quad -i$                                                                                                        |
| $g \quad (\frac{1}{2}, \frac{1}{2}, \frac{t}{2})$ | $\{4_{001}   \frac{1}{2} 0 0\}$<br>$g_1 \quad -ie^{-\frac{3i\pi}{4}}$<br>$g_2 \quad -ie^{\frac{3i\pi}{4}}$<br>$g_3 \quad -ie^{-\frac{i\pi}{4}}$<br>$g_4 \quad -ie^{\frac{i\pi}{4}}$ |

$$\begin{aligned} \mathcal{W}_1^{\text{gapless}} = & \sum_{m=1}^{n_{a_1}} \text{sgn}(v_m^{a_1}) \frac{1 - \text{sgn}(\delta_m^{a_1})}{2} - \sum_{m=1}^{n_{c_1}} \text{sgn}(v_m^{c_1}) \frac{1 - \text{sgn}(\delta_m^{c_1})}{2} - \sum_{m=1}^{n_{e_1}} \text{sgn}(v_m^{e_1}) \frac{1 - \text{sgn}(\delta_m^{e_1})}{2} \\ & - \sum_{m=1}^{n_{e_3}} \text{sgn}(v_m^{e_3}) \frac{1 - \text{sgn}(\delta_m^{e_3})}{2} + \sum_{m=1}^{n_{f_1}} \text{sgn}(v_m^{f_1}) \frac{1 - \text{sgn}(\delta_m^{f_1})}{2} + \sum_{m=1}^{n_{f_2}} \text{sgn}(v_m^{f_2}) \frac{1 - \text{sgn}(\delta_m^{f_2})}{2} \end{aligned} \quad (\text{S85.1})$$

$$\begin{aligned} \mathcal{W}_2^{\text{gapless}} = & \sum_{m=1}^{n_{b_1}} \text{sgn}(v_m^{b_1}) \frac{1 - \text{sgn}(\delta_m^{b_1})}{2} - \sum_{m=1}^{n_{d_1}} \text{sgn}(v_m^{d_1}) \frac{1 - \text{sgn}(\delta_m^{d_1})}{2} - \sum_{m=1}^{n_{f_1}} \text{sgn}(v_m^{f_1}) \frac{1 - \text{sgn}(\delta_m^{f_1})}{2} \\ & - \sum_{m=1}^{n_{f_2}} \text{sgn}(v_m^{f_2}) \frac{1 - \text{sgn}(\delta_m^{f_2})}{2} + \sum_{m=1}^{n_{g_1}} \text{sgn}(v_m^{g_1}) \frac{1 - \text{sgn}(\delta_m^{g_1})}{2} + \sum_{m=1}^{n_{g_3}} \text{sgn}(v_m^{g_3}) \frac{1 - \text{sgn}(\delta_m^{g_3})}{2} \end{aligned} \quad (\text{S85.2})$$

$$\mathcal{W}_1^{\text{gapped}} = - \sum_{m=1}^{n_{f_1}} \text{sgn}(v_m^{f_1}) \frac{1 - \text{sgn}(\delta_m^{f_1})}{2} + \sum_{m=1}^{n_{f_2}} \text{sgn}(v_m^{f_2}) \frac{1 - \text{sgn}(\delta_m^{f_2})}{2} \quad (\text{S85.3})$$

$$\mathcal{W}_2^{\text{gapped}} = - \sum_{m=1}^{n_{g_1}} \text{sgn}(v_m^{g_1}) \frac{1 - \text{sgn}(\delta_m^{g_1})}{2} + \sum_{m=1}^{n_{g_3}} \text{sgn}(v_m^{g_3}) \frac{1 - \text{sgn}(\delta_m^{g_3})}{2} \quad (\text{S85.4})$$

$$\mathcal{X}_1 = \sum_{m=1}^{n_{d_1}} \frac{1 - \text{sgn}(\delta_m^{d_1})}{2} \quad \text{mod } 2 \quad (\text{S85.5})$$

### S86. SPACE GROUP NO. 86

| line segment                                      | character of irrep (generators only)                                                                                                                                                                                                                                              |
|---------------------------------------------------|-----------------------------------------------------------------------------------------------------------------------------------------------------------------------------------------------------------------------------------------------------------------------------------|
| $a \quad (\frac{t}{2}, 0, 0)$                     | $\{m_{001}   \frac{1}{2} \frac{1}{2} 0\}$<br>$a_1 \quad -ie^{-\frac{1}{2}i\pi t}$<br>$a_2 \quad ie^{-\frac{1}{2}i\pi t}$                                                                                                                                                          |
| $b \quad (\frac{1}{2}, \frac{t}{2}, 0)$           | $\{m_{001}   \frac{1}{2} \frac{1}{2} 0\}$<br>$b_1 \quad -ie^{-\frac{1}{2}i\pi(t+1)}$<br>$b_2 \quad ie^{-\frac{1}{2}i\pi(t+1)}$                                                                                                                                                    |
| $c \quad (\frac{t}{2}, 0, \frac{1}{2})$           | $\{m_{001}   \frac{1}{2} \frac{1}{2} 0\}$<br>$c_1 \quad -ie^{-\frac{1}{2}i\pi t}$<br>$c_2 \quad ie^{-\frac{1}{2}i\pi t}$                                                                                                                                                          |
| $d \quad (\frac{1}{2}, \frac{t}{2}, \frac{1}{2})$ | $\{m_{001}   \frac{1}{2} \frac{1}{2} 0\}$<br>$d_1 \quad -ie^{-\frac{1}{2}i\pi(t+1)}$<br>$d_2 \quad ie^{-\frac{1}{2}i\pi(t+1)}$                                                                                                                                                    |
| $e \quad (0, 0, \frac{t}{2})$                     | $\{4_{001}   0 \frac{1}{2} \frac{1}{2}\}$<br>$e_1 \quad e^{-\frac{1}{2}i\pi t - \frac{3i\pi}{4}}$<br>$e_2 \quad e^{\frac{3i\pi}{4} - \frac{i\pi t}{2}}$<br>$e_3 \quad e^{-\frac{1}{2}i\pi t - \frac{i\pi}{4}}$<br>$e_4 \quad e^{\frac{i\pi}{4} - \frac{i\pi t}{2}}$               |
| $f \quad (\frac{1}{2}, 0, \frac{t}{2})$           | $\{2_{001}   \frac{1}{2} \frac{1}{2} 0\}$<br>$f_1 \quad i$<br>$f_2 \quad -i$                                                                                                                                                                                                      |
| $g \quad (\frac{1}{2}, \frac{1}{2}, \frac{t}{2})$ | $\{4_{001}   0 \frac{1}{2} \frac{1}{2}\}$<br>$g_1 \quad e^{-\frac{1}{2}i\pi(t+1) - \frac{3i\pi}{4}}$<br>$g_2 \quad e^{\frac{3i\pi}{4} - \frac{1}{2}i\pi(t+1)}$<br>$g_3 \quad e^{-\frac{1}{2}i\pi(t+1) - \frac{i\pi}{4}}$<br>$g_4 \quad e^{\frac{i\pi}{4} - \frac{1}{2}i\pi(t+1)}$ |

$$\begin{aligned} \mathcal{W}_1^{\text{gapless}} = & \sum_{m=1}^{n_{a_1}} \text{sgn}(v_m^{a_1}) \frac{1 - \text{sgn}(\delta_m^{a_1})}{2} - \sum_{m=1}^{n_{c_1}} \text{sgn}(v_m^{c_1}) \frac{1 - \text{sgn}(\delta_m^{c_1})}{2} - \sum_{m=1}^{n_{e_1}} \text{sgn}(v_m^{e_1}) \frac{1 - \text{sgn}(\delta_m^{e_1})}{2} \\ & - \sum_{m=1}^{n_{e_3}} \text{sgn}(v_m^{e_3}) \frac{1 - \text{sgn}(\delta_m^{e_3})}{2} + \sum_{m=1}^{n_{f_1}} \text{sgn}(v_m^{f_1}) \frac{1 - \text{sgn}(\delta_m^{f_1})}{2} + \sum_{m=1}^{n_{f_2}} \text{sgn}(v_m^{f_2}) \frac{1 - \text{sgn}(\delta_m^{f_2})}{2} \end{aligned} \quad (\text{S86.1})$$

$$\begin{aligned} \mathcal{W}_2^{\text{gapless}} = & \sum_{m=1}^{n_{b_1}} \text{sgn}(v_m^{b_1}) \frac{1 - \text{sgn}(\delta_m^{b_1})}{2} - \sum_{m=1}^{n_{d_1}} \text{sgn}(v_m^{d_1}) \frac{1 - \text{sgn}(\delta_m^{d_1})}{2} - \sum_{m=1}^{n_{f_1}} \text{sgn}(v_m^{f_1}) \frac{1 - \text{sgn}(\delta_m^{f_1})}{2} \\ & - \sum_{m=1}^{n_{f_2}} \text{sgn}(v_m^{f_2}) \frac{1 - \text{sgn}(\delta_m^{f_2})}{2} + \sum_{m=1}^{n_{g_1}} \text{sgn}(v_m^{g_1}) \frac{1 - \text{sgn}(\delta_m^{g_1})}{2} + \sum_{m=1}^{n_{g_3}} \text{sgn}(v_m^{g_3}) \frac{1 - \text{sgn}(\delta_m^{g_3})}{2} \end{aligned} \quad (\text{S86.2})$$

$$\mathcal{W}_1^{\text{gapped}} = - \sum_{m=1}^{n_{f_1}} \text{sgn}(v_m^{f_1}) \frac{1 - \text{sgn}(\delta_m^{f_1})}{2} + \sum_{m=1}^{n_{f_2}} \text{sgn}(v_m^{f_2}) \frac{1 - \text{sgn}(\delta_m^{f_2})}{2} \quad (\text{S86.3})$$

$$\mathcal{X}_1 = \sum_{m=1}^{n_{c_1}} \frac{1 - \text{sgn}(\delta_m^{c_1})}{2} \quad \text{mod } 2 \quad (\text{S86.4})$$

$$\mathcal{X}_2 = \sum_{m=1}^{n_{c_1}} \frac{1 - \text{sgn}(\delta_m^{c_1})}{2} + \sum_{m=1}^{n_{d_1}} \frac{1 - \text{sgn}(\delta_m^{d_1})}{2} + \sum_{m=1}^{n_{g_1}} \frac{1 - \text{sgn}(\delta_m^{g_1})}{2} + \sum_{m=1}^{n_{g_3}} \frac{1 - \text{sgn}(\delta_m^{g_3})}{2} \quad \text{mod } 2 \quad (\text{S86.5})$$

### S87. SPACE GROUP NO. 87

| line segment                                          | character of irrep (generators only)                                                                                                                                  |
|-------------------------------------------------------|-----------------------------------------------------------------------------------------------------------------------------------------------------------------------|
| $a \quad (0, 0, t)$                                   | $\{4_{001}   0 \ 0 \ 0\}$<br>$a_1 \quad e^{-\frac{3i\pi}{4}}$<br>$a_2 \quad e^{\frac{3i\pi}{4}}$<br>$a_3 \quad e^{-\frac{i\pi}{4}}$<br>$a_4 \quad e^{\frac{i\pi}{4}}$ |
| $b \quad (\frac{1}{2}, \frac{1}{2}, \frac{t}{2})$     | $\{2_{001}   0 \ 0 \ 0\}$<br>$b_1 \quad -i$<br>$b_2 \quad i$                                                                                                          |
| $c \quad (\frac{t}{2}, \frac{t}{2}, 1 - \frac{t}{2})$ | $\{1   0 \ 0 \ 0\}$<br>$c_1 \quad 1$                                                                                                                                  |
| $d \quad (\frac{t}{2}, \frac{t}{2}, 0)$               | $\{m_{001}   0 \ 0 \ 0\}$<br>$d_1 \quad -i$<br>$d_2 \quad i$                                                                                                          |
| $e \quad (\frac{t}{2}, 1 - \frac{t}{2}, 0)$           | $\{m_{001}   0 \ 0 \ 0\}$<br>$e_1 \quad -i$<br>$e_2 \quad i$                                                                                                          |
| $f \quad (0, \frac{t}{2}, 1 - \frac{t}{2})$           | $\{1   0 \ 0 \ 0\}$<br>$f_1 \quad 1$                                                                                                                                  |

$$\mathcal{W}_1^{\text{gapless}} = \sum_{m=1}^{n_{a_1}} \text{sgn}(v_m^{a_1}) \frac{1 - \text{sgn}(\delta_m^{a_1})}{2} + \sum_{m=1}^{n_{a_3}} \text{sgn}(v_m^{a_3}) \frac{1 - \text{sgn}(\delta_m^{a_3})}{2} - \sum_{m=1}^{n_{d_1}} \text{sgn}(v_m^{d_1}) \frac{1 - \text{sgn}(\delta_m^{d_1})}{2} + \sum_{m=1}^{n_{e_1}} \text{sgn}(v_m^{e_1}) \frac{1 - \text{sgn}(\delta_m^{e_1})}{2} \quad (\text{S87.1})$$

$$\mathcal{W}_2^{\text{gapless}} = \sum_{m=1}^{n_{b_1}} \text{sgn}(v_m^{b_1}) \frac{1 - \text{sgn}(\delta_m^{b_1})}{2} - \sum_{m=1}^{n_{c_1}} \text{sgn}(v_m^{c_1}) \frac{1 - \text{sgn}(\delta_m^{c_1})}{2} + \sum_{m=1}^{n_{e_1}} \text{sgn}(v_m^{e_1}) \frac{1 - \text{sgn}(\delta_m^{e_1})}{2} \quad (\text{S87.2})$$

### S88. SPACE GROUP NO. 88

| line segment                                          | character of irrep (generators only)                                                                                                                                                                                                                                          |
|-------------------------------------------------------|-------------------------------------------------------------------------------------------------------------------------------------------------------------------------------------------------------------------------------------------------------------------------------|
| $a \quad (0, 0, t)$                                   | $\{4_{001}   \frac{3}{4} \frac{1}{4} \frac{1}{4}\}$<br>$a_1 \quad e^{-\frac{1}{2}i\pi t - \frac{3i\pi}{4}}$<br>$a_2 \quad e^{\frac{3i\pi}{4} - \frac{i\pi t}{2}}$<br>$a_3 \quad e^{-\frac{1}{2}i\pi t - \frac{i\pi}{4}}$<br>$a_4 \quad e^{\frac{i\pi}{4} - \frac{i\pi t}{2}}$ |
| $b \quad (\frac{1}{2}, \frac{1}{2}, \frac{t}{2})$     | $\{2_{001}   0 \frac{1}{2} 0\}$<br>$b_1 \quad i$<br>$b_2 \quad -i$                                                                                                                                                                                                            |
| $c \quad (\frac{t}{2}, \frac{t}{2}, 1 - \frac{t}{2})$ | $\{1   0 \ 0 \ 0\}$<br>$c_1 \quad 1$                                                                                                                                                                                                                                          |
| $d \quad (\frac{t}{2}, \frac{t}{2}, 0)$               | $\{m_{001}   0 \ \frac{1}{2} \ 0\}$<br>$d_1 \quad -ie^{-\frac{1}{2}i\pi t}$<br>$d_2 \quad ie^{-\frac{1}{2}i\pi t}$                                                                                                                                                            |
| $e \quad (\frac{t}{2}, 1 - \frac{t}{2}, 0)$           | $\{m_{001}   0 \ \frac{1}{2} \ 0\}$<br>$e_1 \quad -ie^{-\frac{1}{2}i\pi(2-t)}$<br>$e_2 \quad ie^{-\frac{1}{2}i\pi(2-t)}$                                                                                                                                                      |
| $f \quad (0, \frac{t}{2}, 1 - \frac{t}{2})$           | $\{1   0 \ 0 \ 0\}$<br>$f_1 \quad 1$                                                                                                                                                                                                                                          |

$$\mathcal{W}_1^{\text{gapless}} = \sum_{m=1}^{n_{a_1}} \text{sgn}(v_m^{a_1}) \frac{1 - \text{sgn}(\delta_m^{a_1})}{2} + \sum_{m=1}^{n_{a_3}} \text{sgn}(v_m^{a_3}) \frac{1 - \text{sgn}(\delta_m^{a_3})}{2} - \sum_{m=1}^{n_{d_1}} \text{sgn}(v_m^{d_1}) \frac{1 - \text{sgn}(\delta_m^{d_1})}{2} + \sum_{m=1}^{n_{e_1}} \text{sgn}(v_m^{e_1}) \frac{1 - \text{sgn}(\delta_m^{e_1})}{2} \quad (\text{S88.1})$$

$$\mathcal{W}_2^{\text{gapless}} = \sum_{m=1}^{n_{b_1}} \text{sgn}(v_m^{b_1}) \frac{1 - \text{sgn}(\delta_m^{b_1})}{2} + \sum_{m=1}^{n_{b_2}} \text{sgn}(v_m^{b_2}) \frac{1 - \text{sgn}(\delta_m^{b_2})}{2} - \sum_{m=1}^{n_{c_1}} \text{sgn}(v_m^{c_1}) \frac{1 - \text{sgn}(\delta_m^{c_1})}{2} + \sum_{m=1}^{n_{e_1}} \text{sgn}(v_m^{e_1}) \frac{1 - \text{sgn}(\delta_m^{e_1})}{2} \quad (\text{S88.2})$$

$$\mathcal{X}_1 = \sum_{m=1}^{n_{e_1}} \frac{1 - \text{sgn}(\delta_m^{e_1})}{2} \quad \text{mod } 2 \quad (\text{S88.3})$$

## S89. SPACE GROUP NO. 89

| line segment                                        | character of irrep (generators only)                                                                                                                                  |
|-----------------------------------------------------|-----------------------------------------------------------------------------------------------------------------------------------------------------------------------|
| $a \quad (0, \frac{t}{2}, 0)$                       | $\{2_{010}   0 \ 0 \ 0\}$<br>$a_1 \quad -i$<br>$a_2 \quad i$                                                                                                          |
| $b \quad (\frac{1-t}{2}, \frac{1}{2}, 0)$           | $\{2_{100}   0 \ 0 \ 0\}$<br>$b_1 \quad -i$<br>$b_2 \quad i$                                                                                                          |
| $c \quad (\frac{t}{2}, \frac{t}{2}, 0)$             | $\{2_{110}   0 \ 0 \ 0\}$<br>$c_1 \quad -i$<br>$c_2 \quad i$                                                                                                          |
| $d \quad (0, \frac{t}{2}, \frac{1}{2})$             | $\{2_{010}   0 \ 0 \ 0\}$<br>$d_1 \quad -i$<br>$d_2 \quad i$                                                                                                          |
| $e \quad (\frac{1-t}{2}, \frac{1}{2}, \frac{1}{2})$ | $\{2_{100}   0 \ 0 \ 0\}$<br>$e_1 \quad -i$<br>$e_2 \quad i$                                                                                                          |
| $f \quad (\frac{t}{2}, \frac{t}{2}, \frac{1}{2})$   | $\{2_{110}   0 \ 0 \ 0\}$<br>$f_1 \quad -i$<br>$f_2 \quad i$                                                                                                          |
| $g \quad (0, 0, \frac{t}{2})$                       | $\{4_{001}   0 \ 0 \ 0\}$<br>$g_1 \quad e^{-\frac{3i\pi}{4}}$<br>$g_2 \quad e^{\frac{3i\pi}{4}}$<br>$g_3 \quad e^{-\frac{i\pi}{4}}$<br>$g_4 \quad e^{\frac{i\pi}{4}}$ |
| $h \quad (0, \frac{1}{2}, \frac{t}{2})$             | $\{2_{001}   0 \ 0 \ 0\}$<br>$h_1 \quad -i$<br>$h_2 \quad i$                                                                                                          |
| $i \quad (\frac{1}{2}, \frac{1}{2}, \frac{t}{2})$   | $\{4_{001}   0 \ 0 \ 0\}$<br>$i_1 \quad e^{-\frac{3i\pi}{4}}$<br>$i_2 \quad e^{\frac{3i\pi}{4}}$<br>$i_3 \quad e^{-\frac{i\pi}{4}}$<br>$i_4 \quad e^{\frac{i\pi}{4}}$ |

$$\begin{aligned}
\mathcal{W}_1^{\text{gapless}} = & \sum_{m=1}^{n_{a_1}} \text{sgn}(v_m^{a_1}) \frac{1 - \text{sgn}(\delta_m^{a_1})}{2} + \sum_{m=1}^{n_{a_2}} \text{sgn}(v_m^{a_2}) \frac{1 - \text{sgn}(\delta_m^{a_2})}{2} - \sum_{m=1}^{n_{e_1}} \text{sgn}(v_m^{e_1}) \frac{1 - \text{sgn}(\delta_m^{e_1})}{2} \\
& - \sum_{m=1}^{n_{e_2}} \text{sgn}(v_m^{e_2}) \frac{1 - \text{sgn}(\delta_m^{e_2})}{2} - \sum_{m=1}^{n_{f_1}} \text{sgn}(v_m^{f_1}) \frac{1 - \text{sgn}(\delta_m^{f_1})}{2} - \sum_{m=1}^{n_{f_2}} \text{sgn}(v_m^{f_2}) \frac{1 - \text{sgn}(\delta_m^{f_2})}{2} \\
& - \sum_{m=1}^{n_{g_1}} \text{sgn}(v_m^{g_1}) \frac{1 - \text{sgn}(\delta_m^{g_1})}{2} - \sum_{m=1}^{n_{g_2}} \text{sgn}(v_m^{g_2}) \frac{1 - \text{sgn}(\delta_m^{g_2})}{2} - \sum_{m=1}^{n_{g_3}} \text{sgn}(v_m^{g_3}) \frac{1 - \text{sgn}(\delta_m^{g_3})}{2} \\
& - \sum_{m=1}^{n_{g_4}} \text{sgn}(v_m^{g_4}) \frac{1 - \text{sgn}(\delta_m^{g_4})}{2} + \sum_{m=1}^{n_{h_1}} \text{sgn}(v_m^{h_1}) \frac{1 - \text{sgn}(\delta_m^{h_1})}{2} + \sum_{m=1}^{n_{h_2}} \text{sgn}(v_m^{h_2}) \frac{1 - \text{sgn}(\delta_m^{h_2})}{2}
\end{aligned} \tag{S89.1}$$

$$\begin{aligned}
\mathcal{W}_2^{\text{gapless}} = & \sum_{m=1}^{n_{b_1}} \text{sgn}(v_m^{b_1}) \frac{1 - \text{sgn}(\delta_m^{b_1})}{2} + \sum_{m=1}^{n_{b_2}} \text{sgn}(v_m^{b_2}) \frac{1 - \text{sgn}(\delta_m^{b_2})}{2} - \sum_{m=1}^{n_{e_1}} \text{sgn}(v_m^{e_1}) \frac{1 - \text{sgn}(\delta_m^{e_1})}{2} - \sum_{m=1}^{n_{e_2}} \text{sgn}(v_m^{e_2}) \frac{1 - \text{sgn}(\delta_m^{e_2})}{2} \\
& + \sum_{m=1}^{n_{h_1}} \text{sgn}(v_m^{h_1}) \frac{1 - \text{sgn}(\delta_m^{h_1})}{2} + \sum_{m=1}^{n_{h_2}} \text{sgn}(v_m^{h_2}) \frac{1 - \text{sgn}(\delta_m^{h_2})}{2} - \sum_{m=1}^{n_{i_1}} \text{sgn}(v_m^{i_1}) \frac{1 - \text{sgn}(\delta_m^{i_1})}{2} \\
& - \sum_{m=1}^{n_{i_2}} \text{sgn}(v_m^{i_2}) \frac{1 - \text{sgn}(\delta_m^{i_2})}{2} - \sum_{m=1}^{n_{i_3}} \text{sgn}(v_m^{i_3}) \frac{1 - \text{sgn}(\delta_m^{i_3})}{2} - \sum_{m=1}^{n_{i_4}} \text{sgn}(v_m^{i_4}) \frac{1 - \text{sgn}(\delta_m^{i_4})}{2}
\end{aligned} \tag{S89.2}$$

$$\begin{aligned}
\mathcal{W}_3^{\text{gapless}} = & \sum_{m=1}^{n_{c_1}} \text{sgn}(v_m^{c_1}) \frac{1 - \text{sgn}(\delta_m^{c_1})}{2} + \sum_{m=1}^{n_{c_2}} \text{sgn}(v_m^{c_2}) \frac{1 - \text{sgn}(\delta_m^{c_2})}{2} - \sum_{m=1}^{n_{f_1}} \text{sgn}(v_m^{f_1}) \frac{1 - \text{sgn}(\delta_m^{f_1})}{2} \\
& - \sum_{m=1}^{n_{f_2}} \text{sgn}(v_m^{f_2}) \frac{1 - \text{sgn}(\delta_m^{f_2})}{2} - \sum_{m=1}^{n_{g_1}} \text{sgn}(v_m^{g_1}) \frac{1 - \text{sgn}(\delta_m^{g_1})}{2} - \sum_{m=1}^{n_{g_2}} \text{sgn}(v_m^{g_2}) \frac{1 - \text{sgn}(\delta_m^{g_2})}{2} \\
& - \sum_{m=1}^{n_{g_3}} \text{sgn}(v_m^{g_3}) \frac{1 - \text{sgn}(\delta_m^{g_3})}{2} - \sum_{m=1}^{n_{g_4}} \text{sgn}(v_m^{g_4}) \frac{1 - \text{sgn}(\delta_m^{g_4})}{2} + \sum_{m=1}^{n_{i_1}} \text{sgn}(v_m^{i_1}) \frac{1 - \text{sgn}(\delta_m^{i_1})}{2} \\
& + \sum_{m=1}^{n_{i_2}} \text{sgn}(v_m^{i_2}) \frac{1 - \text{sgn}(\delta_m^{i_2})}{2} + \sum_{m=1}^{n_{i_3}} \text{sgn}(v_m^{i_3}) \frac{1 - \text{sgn}(\delta_m^{i_3})}{2} + \sum_{m=1}^{n_{i_4}} \text{sgn}(v_m^{i_4}) \frac{1 - \text{sgn}(\delta_m^{i_4})}{2}
\end{aligned} \tag{S89.3}$$

$$\begin{aligned}
\mathcal{W}_4^{\text{gapless}} = & \sum_{m=1}^{n_{d_1}} \text{sgn}(v_m^{d_1}) \frac{1 - \text{sgn}(\delta_m^{d_1})}{2} + \sum_{m=1}^{n_{d_2}} \text{sgn}(v_m^{d_2}) \frac{1 - \text{sgn}(\delta_m^{d_2})}{2} - \sum_{m=1}^{n_{e_1}} \text{sgn}(v_m^{e_1}) \frac{1 - \text{sgn}(\delta_m^{e_1})}{2} \\
& - \sum_{m=1}^{n_{e_2}} \text{sgn}(v_m^{e_2}) \frac{1 - \text{sgn}(\delta_m^{e_2})}{2} - \sum_{m=1}^{n_{f_1}} \text{sgn}(v_m^{f_1}) \frac{1 - \text{sgn}(\delta_m^{f_1})}{2} - \sum_{m=1}^{n_{f_2}} \text{sgn}(v_m^{f_2}) \frac{1 - \text{sgn}(\delta_m^{f_2})}{2}
\end{aligned} \tag{S89.4}$$

$$\mathcal{W}_1^{\text{gapped}} = - \sum_{m=1}^{n_{f_1}} \text{sgn}(v_m^{f_1}) \frac{1 - \text{sgn}(\delta_m^{f_1})}{2} + \sum_{m=1}^{n_{f_2}} \text{sgn}(v_m^{f_2}) \frac{1 - \text{sgn}(\delta_m^{f_2})}{2} \tag{S89.5}$$

$$\begin{aligned}
\mathcal{W}_2^{\text{gapped}} = & - \sum_{m=1}^{n_{a_2}} \text{sgn}(v_m^{a_2}) \frac{1 - \text{sgn}(\delta_m^{a_2})}{2} + \sum_{m=1}^{n_{e_2}} \text{sgn}(v_m^{e_2}) \frac{1 - \text{sgn}(\delta_m^{e_2})}{2} + \sum_{m=1}^{n_{f_1}} \text{sgn}(v_m^{f_1}) \frac{1 - \text{sgn}(\delta_m^{f_1})}{2} \\
& + \sum_{m=1}^{n_{g_1}} \text{sgn}(v_m^{g_1}) \frac{1 - \text{sgn}(\delta_m^{g_1})}{2} + \sum_{m=1}^{n_{g_3}} \text{sgn}(v_m^{g_3}) \frac{1 - \text{sgn}(\delta_m^{g_3})}{2} - \sum_{m=1}^{n_{h_1}} \text{sgn}(v_m^{h_1}) \frac{1 - \text{sgn}(\delta_m^{h_1})}{2}
\end{aligned} \tag{S89.6}$$

$$\mathcal{W}_3^{\text{gapped}} = - \sum_{m=1}^{n_{g_1}} \text{sgn}(v_m^{g_1}) \frac{1 - \text{sgn}(\delta_m^{g_1})}{2} + \sum_{m=1}^{n_{g_2}} \text{sgn}(v_m^{g_2}) \frac{1 - \text{sgn}(\delta_m^{g_2})}{2} \tag{S89.7}$$

$$\begin{aligned}
\mathcal{W}_4^{\text{gapped}} = & \sum_{m=1}^{n_{c_2}} \text{sgn}(v_m^{c_2}) \frac{1 - \text{sgn}(\delta_m^{c_2})}{2} - \sum_{m=1}^{n_{f_1}} \text{sgn}(v_m^{f_1}) \frac{1 - \text{sgn}(\delta_m^{f_1})}{2} - \sum_{m=1}^{n_{g_1}} \text{sgn}(v_m^{g_1}) \frac{1 - \text{sgn}(\delta_m^{g_1})}{2} \\
& - \sum_{m=1}^{n_{g_3}} \text{sgn}(v_m^{g_3}) \frac{1 - \text{sgn}(\delta_m^{g_3})}{2} + \sum_{m=1}^{n_{i_1}} \text{sgn}(v_m^{i_1}) \frac{1 - \text{sgn}(\delta_m^{i_1})}{2} + \sum_{m=1}^{n_{i_3}} \text{sgn}(v_m^{i_3}) \frac{1 - \text{sgn}(\delta_m^{i_3})}{2}
\end{aligned} \tag{S89.8}$$

$$\mathcal{W}_5^{\text{gapped}} = - \sum_{m=1}^{n_{g3}} \text{sgn}(v_m^{g3}) \frac{1 - \text{sgn}(\delta_m^{g3})}{2} + \sum_{m=1}^{n_{g4}} \text{sgn}(v_m^{g4}) \frac{1 - \text{sgn}(\delta_m^{g4})}{2} \quad (\text{S89.9})$$

$$\begin{aligned} \mathcal{W}_6^{\text{gapped}} = & - \sum_{m=1}^{n_{a2}} \text{sgn}(v_m^{a2}) \frac{1 - \text{sgn}(\delta_m^{a2})}{2} + \sum_{m=1}^{n_{b2}} \text{sgn}(v_m^{b2}) \frac{1 - \text{sgn}(\delta_m^{b2})}{2} + \sum_{m=1}^{n_{f1}} \text{sgn}(v_m^{f1}) \frac{1 - \text{sgn}(\delta_m^{f1})}{2} \\ & + \sum_{m=1}^{n_{g1}} \text{sgn}(v_m^{g1}) \frac{1 - \text{sgn}(\delta_m^{g1})}{2} + \sum_{m=1}^{n_{g3}} \text{sgn}(v_m^{g3}) \frac{1 - \text{sgn}(\delta_m^{g3})}{2} - \sum_{m=1}^{n_{i1}} \text{sgn}(v_m^{i1}) \frac{1 - \text{sgn}(\delta_m^{i1})}{2} - \sum_{m=1}^{n_{i3}} \text{sgn}(v_m^{i3}) \frac{1 - \text{sgn}(\delta_m^{i3})}{2} \end{aligned} \quad (\text{S89.10})$$

$$\mathcal{W}_7^{\text{gapped}} = - \sum_{m=1}^{n_{h1}} \text{sgn}(v_m^{h1}) \frac{1 - \text{sgn}(\delta_m^{h1})}{2} + \sum_{m=1}^{n_{h2}} \text{sgn}(v_m^{h2}) \frac{1 - \text{sgn}(\delta_m^{h2})}{2} \quad (\text{S89.11})$$

$$\begin{aligned} \mathcal{W}_8^{\text{gapped}} = & - \sum_{m=1}^{n_{a2}} \text{sgn}(v_m^{a2}) \frac{1 - \text{sgn}(\delta_m^{a2})}{2} + \sum_{m=1}^{n_{d2}} \text{sgn}(v_m^{d2}) \frac{1 - \text{sgn}(\delta_m^{d2})}{2} + \sum_{m=1}^{n_{g1}} \text{sgn}(v_m^{g1}) \frac{1 - \text{sgn}(\delta_m^{g1})}{2} \\ & + \sum_{m=1}^{n_{g3}} \text{sgn}(v_m^{g3}) \frac{1 - \text{sgn}(\delta_m^{g3})}{2} - \sum_{m=1}^{n_{h1}} \text{sgn}(v_m^{h1}) \frac{1 - \text{sgn}(\delta_m^{h1})}{2} \end{aligned} \quad (\text{S89.12})$$

$$\mathcal{W}_9^{\text{gapped}} = - \sum_{m=1}^{n_{i1}} \text{sgn}(v_m^{i1}) \frac{1 - \text{sgn}(\delta_m^{i1})}{2} + \sum_{m=1}^{n_{i2}} \text{sgn}(v_m^{i2}) \frac{1 - \text{sgn}(\delta_m^{i2})}{2} \quad (\text{S89.13})$$

$$\begin{aligned} \mathcal{W}_{10}^{\text{gapped}} = & - \sum_{m=1}^{n_{a2}} \text{sgn}(v_m^{a2}) \frac{1 - \text{sgn}(\delta_m^{a2})}{2} + \sum_{m=1}^{n_{e1}} \text{sgn}(v_m^{e1}) \frac{1 - \text{sgn}(\delta_m^{e1})}{2} + \sum_{m=1}^{n_{f1}} \text{sgn}(v_m^{f1}) \frac{1 - \text{sgn}(\delta_m^{f1})}{2} \\ & + \sum_{m=1}^{n_{g1}} \text{sgn}(v_m^{g1}) \frac{1 - \text{sgn}(\delta_m^{g1})}{2} + \sum_{m=1}^{n_{g3}} \text{sgn}(v_m^{g3}) \frac{1 - \text{sgn}(\delta_m^{g3})}{2} - \sum_{m=1}^{n_{h1}} \text{sgn}(v_m^{h1}) \frac{1 - \text{sgn}(\delta_m^{h1})}{2} \end{aligned} \quad (\text{S89.14})$$

$$\mathcal{W}_{11}^{\text{gapped}} = - \sum_{m=1}^{n_{i3}} \text{sgn}(v_m^{i3}) \frac{1 - \text{sgn}(\delta_m^{i3})}{2} + \sum_{m=1}^{n_{i4}} \text{sgn}(v_m^{i4}) \frac{1 - \text{sgn}(\delta_m^{i4})}{2} \quad (\text{S89.15})$$

### S90. SPACE GROUP NO. 90

| line segment                              | character of irrep (generators only)      |
|-------------------------------------------|-------------------------------------------|
| $a \quad (0, \frac{t}{2}, 0)$             | $\{2_{010}   \frac{1}{2} \frac{1}{2} 0\}$ |
|                                           | $a_1 \quad -ie^{-\frac{1}{2}i\pi t}$      |
|                                           | $a_2 \quad ie^{-\frac{1}{2}i\pi t}$       |
| $b \quad (\frac{1-t}{2}, \frac{1}{2}, 0)$ | $\{2_{100}   \frac{1}{2} \frac{1}{2} 0\}$ |
|                                           | $b_1 \quad -e^{-\frac{1}{2}i\pi(2-t)}$    |
|                                           | $b_2 \quad e^{-\frac{1}{2}i\pi(2-t)}$     |

|                                                     |                                                                                                                                                                                                |
|-----------------------------------------------------|------------------------------------------------------------------------------------------------------------------------------------------------------------------------------------------------|
| $c \quad (\frac{t}{2}, \frac{t}{2}, 0)$             | $\{2_{110}   0 \ 0 \ 0 \}$<br>$c_1 \quad -i$<br>$c_2 \quad i$                                                                                                                                  |
| $d \quad (0, \frac{t}{2}, \frac{1}{2})$             | $\{2_{010}   \frac{1}{2} \ \frac{1}{2} \ 0 \}$<br>$d_1 \quad -ie^{-\frac{1}{2}i\pi t}$<br>$d_2 \quad ie^{-\frac{1}{2}i\pi t}$                                                                  |
| $e \quad (\frac{1-t}{2}, \frac{1}{2}, \frac{1}{2})$ | $\{2_{100}   \frac{1}{2} \ \frac{1}{2} \ 0 \}$<br>$e_1 \quad -e^{-\frac{1}{2}i\pi(2-t)}$<br>$e_2 \quad e^{-\frac{1}{2}i\pi(2-t)}$                                                              |
| $f \quad (\frac{t}{2}, \frac{t}{2}, \frac{1}{2})$   | $\{2_{110}   0 \ 0 \ 0 \}$<br>$f_1 \quad -i$<br>$f_2 \quad i$                                                                                                                                  |
| $g \quad (0, 0, \frac{t}{2})$                       | $\{4_{001}   \frac{1}{2} \ \frac{1}{2} \ 0 \}$<br>$g_1 \quad e^{-\frac{3i\pi}{4}}$<br>$g_2 \quad e^{\frac{3i\pi}{4}}$<br>$g_3 \quad e^{-\frac{i\pi}{4}}$<br>$g_4 \quad e^{\frac{i\pi}{4}}$     |
| $h \quad (0, \frac{1}{2}, \frac{t}{2})$             | $\{2_{001}   0 \ 0 \ 0 \}$<br>$h_1 \quad -i$<br>$h_2 \quad i$                                                                                                                                  |
| $i \quad (\frac{1}{2}, \frac{1}{2}, \frac{t}{2})$   | $\{4_{001}   \frac{1}{2} \ \frac{1}{2} \ 0 \}$<br>$i_1 \quad -e^{-\frac{3i\pi}{4}}$<br>$i_2 \quad -e^{\frac{3i\pi}{4}}$<br>$i_3 \quad -e^{-\frac{i\pi}{4}}$<br>$i_4 \quad -e^{\frac{i\pi}{4}}$ |

$$\begin{aligned}
\mathcal{W}_1^{\text{gapless}} = & \sum_{m=1}^{n_{a_1}} \text{sgn}(v_m^{a_1}) \frac{1 - \text{sgn}(\delta_m^{a_1})}{2} + \sum_{m=1}^{n_{a_2}} \text{sgn}(v_m^{a_2}) \frac{1 - \text{sgn}(\delta_m^{a_2})}{2} - 2 \sum_{m=1}^{n_{e_1}} \text{sgn}(v_m^{e_1}) \frac{1 - \text{sgn}(\delta_m^{e_1})}{2} \\
& - \sum_{m=1}^{n_{f_1}} \text{sgn}(v_m^{f_1}) \frac{1 - \text{sgn}(\delta_m^{f_1})}{2} - \sum_{m=1}^{n_{f_2}} \text{sgn}(v_m^{f_2}) \frac{1 - \text{sgn}(\delta_m^{f_2})}{2} - \sum_{m=1}^{n_{g_1}} \text{sgn}(v_m^{g_1}) \frac{1 - \text{sgn}(\delta_m^{g_1})}{2} \\
& - \sum_{m=1}^{n_{g_2}} \text{sgn}(v_m^{g_2}) \frac{1 - \text{sgn}(\delta_m^{g_2})}{2} - \sum_{m=1}^{n_{g_3}} \text{sgn}(v_m^{g_3}) \frac{1 - \text{sgn}(\delta_m^{g_3})}{2} - \sum_{m=1}^{n_{g_4}} \text{sgn}(v_m^{g_4}) \frac{1 - \text{sgn}(\delta_m^{g_4})}{2} \\
& + 2 \sum_{m=1}^{n_{h_1}} \text{sgn}(v_m^{h_1}) \frac{1 - \text{sgn}(\delta_m^{h_1})}{2}
\end{aligned} \tag{S90.1}$$

$$\begin{aligned}
\mathcal{W}_2^{\text{gapless}} = & \sum_{m=1}^{n_{b_1}} \text{sgn}(v_m^{b_1}) \frac{1 - \text{sgn}(\delta_m^{b_1})}{2} - \sum_{m=1}^{n_{e_1}} \text{sgn}(v_m^{e_1}) \frac{1 - \text{sgn}(\delta_m^{e_1})}{2} + \sum_{m=1}^{n_{h_1}} \text{sgn}(v_m^{h_1}) \frac{1 - \text{sgn}(\delta_m^{h_1})}{2} \\
& - \sum_{m=1}^{n_{i_1}} \text{sgn}(v_m^{i_1}) \frac{1 - \text{sgn}(\delta_m^{i_1})}{2} - \sum_{m=1}^{n_{i_2}} \text{sgn}(v_m^{i_2}) \frac{1 - \text{sgn}(\delta_m^{i_2})}{2}
\end{aligned} \tag{S90.2}$$



$$\begin{aligned}
\mathcal{W}_3^{\text{gapless}} = & \sum_{m=1}^{n_{c_1}} \text{sgn}(v_m^{c_1}) \frac{1 - \text{sgn}(\delta_m^{c_1})}{2} + \sum_{m=1}^{n_{c_2}} \text{sgn}(v_m^{c_2}) \frac{1 - \text{sgn}(\delta_m^{c_2})}{2} - \sum_{m=1}^{n_{f_1}} \text{sgn}(v_m^{f_1}) \frac{1 - \text{sgn}(\delta_m^{f_1})}{2} - \sum_{m=1}^{n_{f_2}} \text{sgn}(v_m^{f_2}) \frac{1 - \text{sgn}(\delta_m^{f_2})}{2} \\
& - \sum_{m=1}^{n_{g_1}} \text{sgn}(v_m^{g_1}) \frac{1 - \text{sgn}(\delta_m^{g_1})}{2} - \sum_{m=1}^{n_{g_2}} \text{sgn}(v_m^{g_2}) \frac{1 - \text{sgn}(\delta_m^{g_2})}{2} - \sum_{m=1}^{n_{g_3}} \text{sgn}(v_m^{g_3}) \frac{1 - \text{sgn}(\delta_m^{g_3})}{2} \\
& - \sum_{m=1}^{n_{g_4}} \text{sgn}(v_m^{g_4}) \frac{1 - \text{sgn}(\delta_m^{g_4})}{2} + 2 \sum_{m=1}^{n_{i_1}} \text{sgn}(v_m^{i_1}) \frac{1 - \text{sgn}(\delta_m^{i_1})}{2} + 2 \sum_{m=1}^{n_{i_2}} \text{sgn}(v_m^{i_2}) \frac{1 - \text{sgn}(\delta_m^{i_2})}{2}
\end{aligned} \tag{S90.3}$$

$$\begin{aligned}
\mathcal{W}_4^{\text{gapless}} = & \sum_{m=1}^{n_{d_1}} \text{sgn}(v_m^{d_1}) \frac{1 - \text{sgn}(\delta_m^{d_1})}{2} + \sum_{m=1}^{n_{d_2}} \text{sgn}(v_m^{d_2}) \frac{1 - \text{sgn}(\delta_m^{d_2})}{2} - 2 \sum_{m=1}^{n_{e_1}} \text{sgn}(v_m^{e_1}) \frac{1 - \text{sgn}(\delta_m^{e_1})}{2} \\
& - \sum_{m=1}^{n_{f_1}} \text{sgn}(v_m^{f_1}) \frac{1 - \text{sgn}(\delta_m^{f_1})}{2} - \sum_{m=1}^{n_{f_2}} \text{sgn}(v_m^{f_2}) \frac{1 - \text{sgn}(\delta_m^{f_2})}{2}
\end{aligned} \tag{S90.4}$$

$$\begin{aligned}
\mathcal{W}_1^{\text{gapped}} = & \sum_{m=1}^{n_{c_2}} \text{sgn}(v_m^{c_2}) \frac{1 - \text{sgn}(\delta_m^{c_2})}{2} - \sum_{m=1}^{n_{f_2}} \text{sgn}(v_m^{f_2}) \frac{1 - \text{sgn}(\delta_m^{f_2})}{2} - \sum_{m=1}^{n_{g_1}} \text{sgn}(v_m^{g_1}) \frac{1 - \text{sgn}(\delta_m^{g_1})}{2} \\
& - \sum_{m=1}^{n_{g_3}} \text{sgn}(v_m^{g_3}) \frac{1 - \text{sgn}(\delta_m^{g_3})}{2} + 2 \sum_{m=1}^{n_{i_1}} \text{sgn}(v_m^{i_1}) \frac{1 - \text{sgn}(\delta_m^{i_1})}{2}
\end{aligned} \tag{S90.5}$$

$$\mathcal{W}_2^{\text{gapped}} = - \sum_{m=1}^{n_{g_3}} \text{sgn}(v_m^{g_3}) \frac{1 - \text{sgn}(\delta_m^{g_3})}{2} + \sum_{m=1}^{n_{g_4}} \text{sgn}(v_m^{g_4}) \frac{1 - \text{sgn}(\delta_m^{g_4})}{2} \tag{S90.6}$$

$$\mathcal{W}_3^{\text{gapped}} = - \sum_{m=1}^{n_{g_1}} \text{sgn}(v_m^{g_1}) \frac{1 - \text{sgn}(\delta_m^{g_1})}{2} + \sum_{m=1}^{n_{g_2}} \text{sgn}(v_m^{g_2}) \frac{1 - \text{sgn}(\delta_m^{g_2})}{2} \tag{S90.7}$$

$$\mathcal{W}_4^{\text{gapped}} = \sum_{m=1}^{n_{f_1}} \text{sgn}(v_m^{f_1}) \frac{1 - \text{sgn}(\delta_m^{f_1})}{2} - \sum_{m=1}^{n_{f_2}} \text{sgn}(v_m^{f_2}) \frac{1 - \text{sgn}(\delta_m^{f_2})}{2} \tag{S90.8}$$

$$\mathcal{W}_5^{\text{gapped}} = - \sum_{m=1}^{n_{i_1}} \text{sgn}(v_m^{i_1}) \frac{1 - \text{sgn}(\delta_m^{i_1})}{2} + \sum_{m=1}^{n_{i_2}} \text{sgn}(v_m^{i_2}) \frac{1 - \text{sgn}(\delta_m^{i_2})}{2} \tag{S90.9}$$

$$\mathcal{X}_1 = \sum_{m=1}^{n_{a_2}} \frac{1 - \text{sgn}(\delta_m^{a_2})}{2} + \sum_{m=1}^{n_{f_2}} \frac{1 - \text{sgn}(\delta_m^{f_2})}{2} + \sum_{m=1}^{n_{g_1}} \frac{1 - \text{sgn}(\delta_m^{g_1})}{2} + \sum_{m=1}^{n_{g_3}} \frac{1 - \text{sgn}(\delta_m^{g_3})}{2} \pmod{2} \tag{S90.10}$$

$$\mathcal{X}_2 = \sum_{m=1}^{n_{a_2}} \frac{1 - \text{sgn}(\delta_m^{a_2})}{2} + \sum_{m=1}^{n_{d_2}} \frac{1 - \text{sgn}(\delta_m^{d_2})}{2} + \sum_{m=1}^{n_{g_1}} \frac{1 - \text{sgn}(\delta_m^{g_1})}{2} + \sum_{m=1}^{n_{g_3}} \frac{1 - \text{sgn}(\delta_m^{g_3})}{2} \pmod{2} \tag{S90.11}$$

## S91. SPACE GROUP NO. 91

| line segment                                        | character of irrep (generators only)                                                                                                                                                                                                                          |
|-----------------------------------------------------|---------------------------------------------------------------------------------------------------------------------------------------------------------------------------------------------------------------------------------------------------------------|
| $a \quad (0, \frac{t}{2}, 0)$                       | $\{2_{010}   0 \ 0 \ 0\}$<br>$a_1 \quad -i$<br>$a_2 \quad i$                                                                                                                                                                                                  |
| $b \quad (\frac{1-t}{2}, \frac{1}{2}, 0)$           | $\{2_{100}   0 \ 0 \ \frac{1}{2}\}$<br>$b_1 \quad -i$<br>$b_2 \quad i$                                                                                                                                                                                        |
| $c \quad (\frac{t}{2}, \frac{t}{2}, 0)$             | $\{2_{110}   0 \ 0 \ \frac{3}{4}\}$<br>$c_1 \quad -i$<br>$c_2 \quad i$                                                                                                                                                                                        |
| $d \quad (0, \frac{t}{2}, \frac{1}{2})$             | $\{2_{010}   0 \ 0 \ 0\}$<br>$d_1 \quad -i$<br>$d_2 \quad i$                                                                                                                                                                                                  |
| $e \quad (\frac{1-t}{2}, \frac{1}{2}, \frac{1}{2})$ | $\{2_{100}   0 \ 0 \ \frac{1}{2}\}$<br>$e_1 \quad i$<br>$e_2 \quad -i$                                                                                                                                                                                        |
| $f \quad (\frac{t}{2}, \frac{t}{2}, \frac{1}{2})$   | $\{2_{110}   0 \ 0 \ \frac{3}{4}\}$<br>$f_1 \quad i$<br>$f_2 \quad -i$                                                                                                                                                                                        |
| $g \quad (0, 0, \frac{t}{2})$                       | $\{4_{001}   0 \ 0 \ \frac{1}{4}\}$<br>$g_1 \quad e^{-\frac{1}{4}i\pi t - \frac{3i\pi}{4}}$<br>$g_2 \quad e^{\frac{3i\pi}{4} - \frac{i\pi t}{4}}$<br>$g_3 \quad e^{-\frac{1}{4}i\pi t - \frac{i\pi}{4}}$<br>$g_4 \quad e^{\frac{i\pi}{4} - \frac{i\pi t}{4}}$ |
| $h \quad (0, \frac{1}{2}, \frac{t}{2})$             | $\{2_{001}   0 \ 0 \ \frac{1}{2}\}$<br>$h_1 \quad -ie^{-\frac{1}{2}i\pi t}$<br>$h_2 \quad ie^{-\frac{1}{2}i\pi t}$                                                                                                                                            |
| $i \quad (\frac{1}{2}, \frac{1}{2}, \frac{t}{2})$   | $\{4_{001}   0 \ 0 \ \frac{1}{4}\}$<br>$i_1 \quad e^{-\frac{1}{4}i\pi t - \frac{3i\pi}{4}}$<br>$i_2 \quad e^{\frac{3i\pi}{4} - \frac{i\pi t}{4}}$<br>$i_3 \quad e^{-\frac{1}{4}i\pi t - \frac{i\pi}{4}}$<br>$i_4 \quad e^{\frac{i\pi}{4} - \frac{i\pi t}{4}}$ |

$$\begin{aligned}
\mathcal{W}_1^{\text{gapless}} = & \sum_{m=1}^{n_{a_1}} \text{sgn}(v_m^{a_1}) \frac{1 - \text{sgn}(\delta_m^{a_1})}{2} + \sum_{m=1}^{n_{a_2}} \text{sgn}(v_m^{a_2}) \frac{1 - \text{sgn}(\delta_m^{a_2})}{2} - 2 \sum_{m=1}^{n_{e_1}} \text{sgn}(v_m^{e_1}) \frac{1 - \text{sgn}(\delta_m^{e_1})}{2} \\
& - 2 \sum_{m=1}^{n_{f_1}} \text{sgn}(v_m^{f_1}) \frac{1 - \text{sgn}(\delta_m^{f_1})}{2} - \sum_{m=1}^{n_{g_1}} \text{sgn}(v_m^{g_1}) \frac{1 - \text{sgn}(\delta_m^{g_1})}{2} - \sum_{m=1}^{n_{g_2}} \text{sgn}(v_m^{g_2}) \frac{1 - \text{sgn}(\delta_m^{g_2})}{2} \\
& - \sum_{m=1}^{n_{g_3}} \text{sgn}(v_m^{g_3}) \frac{1 - \text{sgn}(\delta_m^{g_3})}{2} - \sum_{m=1}^{n_{g_4}} \text{sgn}(v_m^{g_4}) \frac{1 - \text{sgn}(\delta_m^{g_4})}{2} + \sum_{m=1}^{n_{h_1}} \text{sgn}(v_m^{h_1}) \frac{1 - \text{sgn}(\delta_m^{h_1})}{2} \\
& + \sum_{m=1}^{n_{h_2}} \text{sgn}(v_m^{h_2}) \frac{1 - \text{sgn}(\delta_m^{h_2})}{2}
\end{aligned} \tag{S91.1}$$

$$\begin{aligned}
\mathcal{W}_2^{\text{gapless}} = & \sum_{m=1}^{n_{b_1}} \text{sgn}(v_m^{b_1}) \frac{1 - \text{sgn}(\delta_m^{b_1})}{2} + \sum_{m=1}^{n_{b_2}} \text{sgn}(v_m^{b_2}) \frac{1 - \text{sgn}(\delta_m^{b_2})}{2} - 2 \sum_{m=1}^{n_{e_1}} \text{sgn}(v_m^{e_1}) \frac{1 - \text{sgn}(\delta_m^{e_1})}{2} \\
& + \sum_{m=1}^{n_{h_1}} \text{sgn}(v_m^{h_1}) \frac{1 - \text{sgn}(\delta_m^{h_1})}{2} + \sum_{m=1}^{n_{h_2}} \text{sgn}(v_m^{h_2}) \frac{1 - \text{sgn}(\delta_m^{h_2})}{2} - \sum_{m=1}^{n_{i_1}} \text{sgn}(v_m^{i_1}) \frac{1 - \text{sgn}(\delta_m^{i_1})}{2} \\
& - \sum_{m=1}^{n_{i_2}} \text{sgn}(v_m^{i_2}) \frac{1 - \text{sgn}(\delta_m^{i_2})}{2} - \sum_{m=1}^{n_{i_3}} \text{sgn}(v_m^{i_3}) \frac{1 - \text{sgn}(\delta_m^{i_3})}{2} - \sum_{m=1}^{n_{i_4}} \text{sgn}(v_m^{i_4}) \frac{1 - \text{sgn}(\delta_m^{i_4})}{2}
\end{aligned} \tag{S91.2}$$

$$\begin{aligned}
\mathcal{W}_3^{\text{gapless}} = & \sum_{m=1}^{n_{c_1}} \text{sgn}(v_m^{c_1}) \frac{1 - \text{sgn}(\delta_m^{c_1})}{2} + \sum_{m=1}^{n_{c_2}} \text{sgn}(v_m^{c_2}) \frac{1 - \text{sgn}(\delta_m^{c_2})}{2} - 2 \sum_{m=1}^{n_{f_1}} \text{sgn}(v_m^{f_1}) \frac{1 - \text{sgn}(\delta_m^{f_1})}{2} - \sum_{m=1}^{n_{g_1}} \text{sgn}(v_m^{g_1}) \frac{1 - \text{sgn}(\delta_m^{g_1})}{2} \\
& - \sum_{m=1}^{n_{g_2}} \text{sgn}(v_m^{g_2}) \frac{1 - \text{sgn}(\delta_m^{g_2})}{2} - \sum_{m=1}^{n_{g_3}} \text{sgn}(v_m^{g_3}) \frac{1 - \text{sgn}(\delta_m^{g_3})}{2} - \sum_{m=1}^{n_{g_4}} \text{sgn}(v_m^{g_4}) \frac{1 - \text{sgn}(\delta_m^{g_4})}{2} \\
& + \sum_{m=1}^{n_{i_1}} \text{sgn}(v_m^{i_1}) \frac{1 - \text{sgn}(\delta_m^{i_1})}{2} + \sum_{m=1}^{n_{i_2}} \text{sgn}(v_m^{i_2}) \frac{1 - \text{sgn}(\delta_m^{i_2})}{2} + \sum_{m=1}^{n_{i_3}} \text{sgn}(v_m^{i_3}) \frac{1 - \text{sgn}(\delta_m^{i_3})}{2} + \sum_{m=1}^{n_{i_4}} \text{sgn}(v_m^{i_4}) \frac{1 - \text{sgn}(\delta_m^{i_4})}{2}
\end{aligned} \tag{S91.3}$$

$$\mathcal{W}_4^{\text{gapless}} = \sum_{m=1}^{n_{d_1}} \text{sgn}(v_m^{d_1}) \frac{1 - \text{sgn}(\delta_m^{d_1})}{2} - \sum_{m=1}^{n_{e_1}} \text{sgn}(v_m^{e_1}) \frac{1 - \text{sgn}(\delta_m^{e_1})}{2} - \sum_{m=1}^{n_{f_1}} \text{sgn}(v_m^{f_1}) \frac{1 - \text{sgn}(\delta_m^{f_1})}{2} \tag{S91.4}$$

$$\mathcal{W}_1^{\text{gapped}} = - \sum_{m=1}^{n_{a_2}} \text{sgn}(v_m^{a_2}) \frac{1 - \text{sgn}(\delta_m^{a_2})}{2} + \sum_{m=1}^{n_{b_2}} \text{sgn}(v_m^{b_2}) \frac{1 - \text{sgn}(\delta_m^{b_2})}{2} + \sum_{m=1}^{n_{c_2}} \text{sgn}(v_m^{c_2}) \frac{1 - \text{sgn}(\delta_m^{c_2})}{2} \tag{S91.5}$$

$$\begin{aligned}
\mathcal{W}_2^{\text{gapped}} = & -2 \sum_{m=1}^{n_{a_2}} \text{sgn}(v_m^{a_2}) \frac{1 - \text{sgn}(\delta_m^{a_2})}{2} + 2 \sum_{m=1}^{n_{e_1}} \text{sgn}(v_m^{e_1}) \frac{1 - \text{sgn}(\delta_m^{e_1})}{2} + 2 \sum_{m=1}^{n_{f_1}} \text{sgn}(v_m^{f_1}) \frac{1 - \text{sgn}(\delta_m^{f_1})}{2} \\
& + \sum_{m=1}^{n_{g_1}} \text{sgn}(v_m^{g_1}) \frac{1 - \text{sgn}(\delta_m^{g_1})}{2} + \sum_{m=1}^{n_{g_2}} \text{sgn}(v_m^{g_2}) \frac{1 - \text{sgn}(\delta_m^{g_2})}{2} + \sum_{m=1}^{n_{g_3}} \text{sgn}(v_m^{g_3}) \frac{1 - \text{sgn}(\delta_m^{g_3})}{2} \\
& + \sum_{m=1}^{n_{g_4}} \text{sgn}(v_m^{g_4}) \frac{1 - \text{sgn}(\delta_m^{g_4})}{2} - \sum_{m=1}^{n_{h_1}} \text{sgn}(v_m^{h_1}) \frac{1 - \text{sgn}(\delta_m^{h_1})}{2} - \sum_{m=1}^{n_{h_2}} \text{sgn}(v_m^{h_2}) \frac{1 - \text{sgn}(\delta_m^{h_2})}{2}
\end{aligned} \tag{S91.6}$$

$$\begin{aligned}
\mathcal{W}_3^{\text{gapped}} = & -2 \sum_{m=1}^{n_{b_2}} \text{sgn}(v_m^{b_2}) \frac{1 - \text{sgn}(\delta_m^{b_2})}{2} + 2 \sum_{m=1}^{n_{e_1}} \text{sgn}(v_m^{e_1}) \frac{1 - \text{sgn}(\delta_m^{e_1})}{2} \\
& - \sum_{m=1}^{n_{h_1}} \text{sgn}(v_m^{h_1}) \frac{1 - \text{sgn}(\delta_m^{h_1})}{2} - \sum_{m=1}^{n_{h_2}} \text{sgn}(v_m^{h_2}) \frac{1 - \text{sgn}(\delta_m^{h_2})}{2} + \sum_{m=1}^{n_{i_1}} \text{sgn}(v_m^{i_1}) \frac{1 - \text{sgn}(\delta_m^{i_1})}{2} \\
& + \sum_{m=1}^{n_{i_2}} \text{sgn}(v_m^{i_2}) \frac{1 - \text{sgn}(\delta_m^{i_2})}{2} + \sum_{m=1}^{n_{i_3}} \text{sgn}(v_m^{i_3}) \frac{1 - \text{sgn}(\delta_m^{i_3})}{2} + \sum_{m=1}^{n_{i_4}} \text{sgn}(v_m^{i_4}) \frac{1 - \text{sgn}(\delta_m^{i_4})}{2}
\end{aligned} \tag{S91.7}$$

$$\mathcal{X}_1 = \sum_{m=1}^{n_{b_2}} \frac{1 - \text{sgn}(\delta_m^{b_2})}{2} + \sum_{m=1}^{n_{h_1}} \frac{1 - \text{sgn}(\delta_m^{h_1})}{2} + \sum_{m=1}^{n_{i_2}} \frac{1 - \text{sgn}(\delta_m^{i_2})}{2} + \sum_{m=1}^{n_{i_3}} \frac{1 - \text{sgn}(\delta_m^{i_3})}{2} \pmod{2} \tag{S91.8}$$

$$\begin{aligned} \mathcal{X}_2 = & \sum_{m=1}^{n_{a_2}} \frac{1 - \text{sgn}(\delta_m^{a_2})}{2} + \sum_{m=1}^{n_{b_2}} \frac{1 - \text{sgn}(\delta_m^{b_2})}{2} + \sum_{m=1}^{n_{g_2}} \frac{1 - \text{sgn}(\delta_m^{g_2})}{2} + \sum_{m=1}^{n_{g_3}} \frac{1 - \text{sgn}(\delta_m^{g_3})}{2} \\ & + \sum_{m=1}^{n_{h_1}} \frac{1 - \text{sgn}(\delta_m^{h_1})}{2} + \sum_{m=1}^{n_{h_2}} \frac{1 - \text{sgn}(\delta_m^{h_2})}{2} + \sum_{m=1}^{n_{i_2}} \frac{1 - \text{sgn}(\delta_m^{i_2})}{2} + \sum_{m=1}^{n_{i_3}} \frac{1 - \text{sgn}(\delta_m^{i_3})}{2} \pmod{2} \end{aligned} \quad (\text{S91.9})$$

$$\begin{aligned} \mathcal{X}_3 = & -3 \sum_{m=1}^{n_{a_2}} \text{sgn}(v_m^{a_2}) \frac{1 - \text{sgn}(\delta_m^{a_2})}{2} - \sum_{m=1}^{n_{b_2}} \text{sgn}(v_m^{b_2}) \frac{1 - \text{sgn}(\delta_m^{b_2})}{2} + 3 \sum_{m=1}^{n_{g_2}} \text{sgn}(v_m^{g_2}) \frac{1 - \text{sgn}(\delta_m^{g_2})}{2} + \sum_{m=1}^{n_{g_3}} \text{sgn}(v_m^{g_3}) \frac{1 - \text{sgn}(\delta_m^{g_3})}{2} \\ & + 2 \sum_{m=1}^{n_{g_4}} \text{sgn}(v_m^{g_4}) \frac{1 - \text{sgn}(\delta_m^{g_4})}{2} - 2 \sum_{m=1}^{n_{h_1}} \text{sgn}(v_m^{h_1}) \frac{1 - \text{sgn}(\delta_m^{h_1})}{2} - 2 \sum_{m=1}^{n_{h_2}} \text{sgn}(v_m^{h_2}) \frac{1 - \text{sgn}(\delta_m^{h_2})}{2} \\ & + 2 \sum_{m=1}^{n_{i_1}} \text{sgn}(v_m^{i_1}) \frac{1 - \text{sgn}(\delta_m^{i_1})}{2} - \sum_{m=1}^{n_{i_2}} \text{sgn}(v_m^{i_2}) \frac{1 - \text{sgn}(\delta_m^{i_2})}{2} + \sum_{m=1}^{n_{i_3}} \text{sgn}(v_m^{i_3}) \frac{1 - \text{sgn}(\delta_m^{i_3})}{2} \pmod{4} \end{aligned} \quad (\text{S91.10})$$

## S92. SPACE GROUP NO. 92

| line segment                                        | character of irrep (generators only)                                                                                                                                                                                                                                                        |
|-----------------------------------------------------|---------------------------------------------------------------------------------------------------------------------------------------------------------------------------------------------------------------------------------------------------------------------------------------------|
| $a \quad (0, \frac{t}{2}, 0)$                       | $\{2_{010}   \frac{1}{2} \frac{1}{2} \frac{1}{4}\}$<br>$a_1 \quad -ie^{-\frac{1}{2}i\pi t}$<br>$a_2 \quad ie^{-\frac{1}{2}i\pi t}$                                                                                                                                                          |
| $b \quad (\frac{1-t}{2}, \frac{1}{2}, 0)$           | $\{2_{100}   \frac{1}{2} \frac{1}{2} \frac{3}{4}\}$<br>$b_1 \quad -e^{-\frac{1}{2}i\pi(2-t)}$<br>$b_2 \quad e^{-\frac{1}{2}i\pi(2-t)}$                                                                                                                                                      |
| $c \quad (\frac{t}{2}, \frac{t}{2}, 0)$             | $\{2_{110}   0 \ 0 \ 0\}$<br>$c_1 \quad -i$<br>$c_2 \quad i$                                                                                                                                                                                                                                |
| $d \quad (0, \frac{t}{2}, \frac{1}{2})$             | $\{2_{010}   \frac{1}{2} \frac{1}{2} \frac{1}{4}\}$<br>$d_1 \quad e^{\frac{3i\pi}{4} - \frac{1}{4}i\pi(2t+1)}$<br>$d_2 \quad e^{-\frac{1}{4}i\pi(2t+1) - \frac{i\pi}{4}}$                                                                                                                   |
| $e \quad (\frac{1-t}{2}, \frac{1}{2}, \frac{1}{2})$ | $\{2_{100}   \frac{1}{2} \frac{1}{2} \frac{3}{4}\}$<br>$e_1 \quad e^{\frac{3i\pi}{4} - \frac{1}{4}i\pi(7-2t)}$<br>$e_2 \quad e^{-\frac{1}{4}i\pi(7-2t) - \frac{i\pi}{4}}$                                                                                                                   |
| $f \quad (\frac{t}{2}, \frac{t}{2}, \frac{1}{2})$   | $\{2_{110}   0 \ 0 \ 0\}$<br>$f_1 \quad -i$<br>$f_2 \quad i$                                                                                                                                                                                                                                |
| $g \quad (0, 0, \frac{t}{2})$                       | $\{4_{001}   \frac{1}{2} \frac{1}{2} \frac{1}{4}\}$<br>$g_1 \quad e^{-\frac{1}{4}i\pi t - \frac{3i\pi}{4}}$<br>$g_2 \quad e^{\frac{3i\pi}{4} - \frac{i\pi t}{4}}$<br>$g_3 \quad e^{-\frac{1}{4}i\pi t - \frac{i\pi}{4}}$<br>$g_4 \quad e^{\frac{i\pi}{4} - \frac{i\pi t}{4}}$               |
| $h \quad (0, \frac{1}{2}, \frac{t}{2})$             | $\{2_{001}   0 \ 0 \ \frac{1}{2}\}$<br>$h_1 \quad -ie^{-\frac{1}{2}i\pi t}$<br>$h_2 \quad ie^{-\frac{1}{2}i\pi t}$                                                                                                                                                                          |
| $i \quad (\frac{1}{2}, \frac{1}{2}, \frac{t}{2})$   | $\{4_{001}   \frac{1}{2} \frac{1}{2} \frac{1}{4}\}$<br>$i_1 \quad e^{-\frac{1}{4}i\pi(t+4) - \frac{3i\pi}{4}}$<br>$i_2 \quad e^{\frac{3i\pi}{4} - \frac{1}{4}i\pi(t+4)}$<br>$i_3 \quad e^{-\frac{1}{4}i\pi(t+4) - \frac{i\pi}{4}}$<br>$i_4 \quad e^{\frac{i\pi}{4} - \frac{1}{4}i\pi(t+4)}$ |

$$\begin{aligned}
\mathcal{W}_1^{\text{gapless}} = & \sum_{m=1}^{n_{a_1}} \text{sgn}(v_m^{a_1}) \frac{1 - \text{sgn}(\delta_m^{a_1})}{2} + \sum_{m=1}^{n_{a_2}} \text{sgn}(v_m^{a_2}) \frac{1 - \text{sgn}(\delta_m^{a_2})}{2} - 2 \sum_{m=1}^{n_{e_1}} \text{sgn}(v_m^{e_1}) \frac{1 - \text{sgn}(\delta_m^{e_1})}{2} \\
& - 2 \sum_{m=1}^{n_{e_2}} \text{sgn}(v_m^{e_2}) \frac{1 - \text{sgn}(\delta_m^{e_2})}{2} - 2 \sum_{m=1}^{n_{f_1}} \text{sgn}(v_m^{f_1}) \frac{1 - \text{sgn}(\delta_m^{f_1})}{2} - \sum_{m=1}^{n_{g_1}} \text{sgn}(v_m^{g_1}) \frac{1 - \text{sgn}(\delta_m^{g_1})}{2} \\
& - \sum_{m=1}^{n_{g_2}} \text{sgn}(v_m^{g_2}) \frac{1 - \text{sgn}(\delta_m^{g_2})}{2} - \sum_{m=1}^{n_{g_3}} \text{sgn}(v_m^{g_3}) \frac{1 - \text{sgn}(\delta_m^{g_3})}{2} - \sum_{m=1}^{n_{g_4}} \text{sgn}(v_m^{g_4}) \frac{1 - \text{sgn}(\delta_m^{g_4})}{2} \\
& + 2 \sum_{m=1}^{n_{h_1}} \text{sgn}(v_m^{h_1}) \frac{1 - \text{sgn}(\delta_m^{h_1})}{2}
\end{aligned} \tag{S92.1}$$

$$\begin{aligned}
\mathcal{W}_2^{\text{gapless}} = & \sum_{m=1}^{n_{b_1}} \text{sgn}(v_m^{b_1}) \frac{1 - \text{sgn}(\delta_m^{b_1})}{2} - \sum_{m=1}^{n_{e_1}} \text{sgn}(v_m^{e_1}) \frac{1 - \text{sgn}(\delta_m^{e_1})}{2} - \sum_{m=1}^{n_{e_2}} \text{sgn}(v_m^{e_2}) \frac{1 - \text{sgn}(\delta_m^{e_2})}{2} \\
& + \sum_{m=1}^{n_{h_1}} \text{sgn}(v_m^{h_1}) \frac{1 - \text{sgn}(\delta_m^{h_1})}{2} - \sum_{m=1}^{n_{i_1}} \text{sgn}(v_m^{i_1}) \frac{1 - \text{sgn}(\delta_m^{i_1})}{2} - \sum_{m=1}^{n_{i_2}} \text{sgn}(v_m^{i_2}) \frac{1 - \text{sgn}(\delta_m^{i_2})}{2}
\end{aligned} \tag{S92.2}$$

$$\begin{aligned}
\mathcal{W}_3^{\text{gapless}} = & \sum_{m=1}^{n_{c_1}} \text{sgn}(v_m^{c_1}) \frac{1 - \text{sgn}(\delta_m^{c_1})}{2} + \sum_{m=1}^{n_{c_2}} \text{sgn}(v_m^{c_2}) \frac{1 - \text{sgn}(\delta_m^{c_2})}{2} - 2 \sum_{m=1}^{n_{f_1}} \text{sgn}(v_m^{f_1}) \frac{1 - \text{sgn}(\delta_m^{f_1})}{2} \\
& - \sum_{m=1}^{n_{g_1}} \text{sgn}(v_m^{g_1}) \frac{1 - \text{sgn}(\delta_m^{g_1})}{2} - \sum_{m=1}^{n_{g_2}} \text{sgn}(v_m^{g_2}) \frac{1 - \text{sgn}(\delta_m^{g_2})}{2} - \sum_{m=1}^{n_{g_3}} \text{sgn}(v_m^{g_3}) \frac{1 - \text{sgn}(\delta_m^{g_3})}{2} \\
& - \sum_{m=1}^{n_{g_4}} \text{sgn}(v_m^{g_4}) \frac{1 - \text{sgn}(\delta_m^{g_4})}{2} + 2 \sum_{m=1}^{n_{i_1}} \text{sgn}(v_m^{i_1}) \frac{1 - \text{sgn}(\delta_m^{i_1})}{2} + 2 \sum_{m=1}^{n_{i_2}} \text{sgn}(v_m^{i_2}) \frac{1 - \text{sgn}(\delta_m^{i_2})}{2}
\end{aligned} \tag{S92.3}$$

$$\begin{aligned}
\mathcal{W}_4^{\text{gapless}} = & \sum_{m=1}^{n_{d_1}} \text{sgn}(v_m^{d_1}) \frac{1 - \text{sgn}(\delta_m^{d_1})}{2} - \sum_{m=1}^{n_{e_1}} \text{sgn}(v_m^{e_1}) \frac{1 - \text{sgn}(\delta_m^{e_1})}{2} - \sum_{m=1}^{n_{e_2}} \text{sgn}(v_m^{e_2}) \frac{1 - \text{sgn}(\delta_m^{e_2})}{2} - \sum_{m=1}^{n_{f_1}} \text{sgn}(v_m^{f_1}) \frac{1 - \text{sgn}(\delta_m^{f_1})}{2}
\end{aligned} \tag{S92.4}$$

$$\begin{aligned}
\mathcal{W}_1^{\text{gapped}} = & 2 \sum_{m=1}^{n_{c_2}} \text{sgn}(v_m^{c_2}) \frac{1 - \text{sgn}(\delta_m^{c_2})}{2} - 2 \sum_{m=1}^{n_{f_1}} \text{sgn}(v_m^{f_1}) \frac{1 - \text{sgn}(\delta_m^{f_1})}{2} - \sum_{m=1}^{n_{g_1}} \text{sgn}(v_m^{g_1}) \frac{1 - \text{sgn}(\delta_m^{g_1})}{2} \\
& - \sum_{m=1}^{n_{g_2}} \text{sgn}(v_m^{g_2}) \frac{1 - \text{sgn}(\delta_m^{g_2})}{2} - \sum_{m=1}^{n_{g_3}} \text{sgn}(v_m^{g_3}) \frac{1 - \text{sgn}(\delta_m^{g_3})}{2} - \sum_{m=1}^{n_{g_4}} \text{sgn}(v_m^{g_4}) \frac{1 - \text{sgn}(\delta_m^{g_4})}{2} \\
& + 2 \sum_{m=1}^{n_{i_1}} \text{sgn}(v_m^{i_1}) \frac{1 - \text{sgn}(\delta_m^{i_1})}{2} + 2 \sum_{m=1}^{n_{i_2}} \text{sgn}(v_m^{i_2}) \frac{1 - \text{sgn}(\delta_m^{i_2})}{2}
\end{aligned} \tag{S92.5}$$

$$\begin{aligned}
\mathcal{X}_1 = & \sum_{m=1}^{n_{a_2}} \frac{1 - \text{sgn}(\delta_m^{a_2})}{2} + \sum_{m=1}^{n_{e_1}} \frac{1 - \text{sgn}(\delta_m^{e_1})}{2} + \sum_{m=1}^{n_{e_2}} \frac{1 - \text{sgn}(\delta_m^{e_2})}{2} + \sum_{m=1}^{n_{g_1}} \frac{1 - \text{sgn}(\delta_m^{g_1})}{2} + \sum_{m=1}^{n_{g_4}} \frac{1 - \text{sgn}(\delta_m^{g_4})}{2} \\
& + \sum_{m=1}^{n_{i_1}} \frac{1 - \text{sgn}(\delta_m^{i_1})}{2} + \sum_{m=1}^{n_{i_2}} \frac{1 - \text{sgn}(\delta_m^{i_2})}{2} \quad \text{mod } 2
\end{aligned} \tag{S92.6}$$

$$\begin{aligned}
\mathcal{X}_2 = & \sum_{m=1}^{n_{c_2}} \frac{1 - \text{sgn}(\delta_m^{c_2})}{2} + \sum_{m=1}^{n_{e_1}} \frac{1 - \text{sgn}(\delta_m^{e_1})}{2} + \sum_{m=1}^{n_{e_2}} \frac{1 - \text{sgn}(\delta_m^{e_2})}{2} + \sum_{m=1}^{n_{g_1}} \frac{1 - \text{sgn}(\delta_m^{g_1})}{2} + \sum_{m=1}^{n_{g_4}} \frac{1 - \text{sgn}(\delta_m^{g_4})}{2} \\
& + \sum_{m=1}^{n_{i_1}} \frac{1 - \text{sgn}(\delta_m^{i_1})}{2} + \sum_{m=1}^{n_{i_2}} \frac{1 - \text{sgn}(\delta_m^{i_2})}{2} \pmod{2}
\end{aligned} \tag{S92.7}$$

$$\begin{aligned}
\mathcal{X}_3 = & 5 \sum_{m=1}^{n_{c_2}} \text{sgn}(v_m^{c_2}) \frac{1 - \text{sgn}(\delta_m^{c_2})}{2} - 2 \sum_{m=1}^{n_{e_1}} \text{sgn}(v_m^{e_1}) \frac{1 - \text{sgn}(\delta_m^{e_1})}{2} + 2 \sum_{m=1}^{n_{e_2}} \text{sgn}(v_m^{e_2}) \frac{1 - \text{sgn}(\delta_m^{e_2})}{2} - 2 \sum_{m=1}^{n_{g_1}} \text{sgn}(v_m^{g_1}) \frac{1 - \text{sgn}(\delta_m^{g_1})}{2} \\
& - 3 \sum_{m=1}^{n_{g_2}} \text{sgn}(v_m^{g_2}) \frac{1 - \text{sgn}(\delta_m^{g_2})}{2} - \sum_{m=1}^{n_{g_3}} \text{sgn}(v_m^{g_3}) \frac{1 - \text{sgn}(\delta_m^{g_3})}{2} + 2 \sum_{m=1}^{n_{i_2}} \text{sgn}(v_m^{i_2}) \frac{1 - \text{sgn}(\delta_m^{i_2})}{2} \pmod{4}
\end{aligned} \tag{S92.8}$$

### S93. SPACE GROUP NO. 93

| line segment                                        | character of irrep (generators only)                                                                                                                                                                                                                          |
|-----------------------------------------------------|---------------------------------------------------------------------------------------------------------------------------------------------------------------------------------------------------------------------------------------------------------------|
| $a \quad (0, \frac{t}{2}, 0)$                       | $\{2_{010}   0 \ 0 \ 0\}$<br>$a_1 \quad -i$<br>$a_2 \quad i$                                                                                                                                                                                                  |
| $b \quad (\frac{1-t}{2}, \frac{1}{2}, 0)$           | $\{2_{100}   0 \ 0 \ 0\}$<br>$b_1 \quad -i$<br>$b_2 \quad i$                                                                                                                                                                                                  |
| $c \quad (\frac{t}{2}, \frac{t}{2}, 0)$             | $\{2_{110}   0 \ 0 \ \frac{1}{2}\}$<br>$c_1 \quad -i$<br>$c_2 \quad i$                                                                                                                                                                                        |
| $d \quad (0, \frac{t}{2}, \frac{1}{2})$             | $\{2_{010}   0 \ 0 \ 0\}$<br>$d_1 \quad -i$<br>$d_2 \quad i$                                                                                                                                                                                                  |
| $e \quad (\frac{1-t}{2}, \frac{1}{2}, \frac{1}{2})$ | $\{2_{100}   0 \ 0 \ 0\}$<br>$e_1 \quad -i$<br>$e_2 \quad i$                                                                                                                                                                                                  |
| $f \quad (\frac{t}{2}, \frac{t}{2}, \frac{1}{2})$   | $\{2_{110}   0 \ 0 \ \frac{1}{2}\}$<br>$f_1 \quad i$<br>$f_2 \quad -i$                                                                                                                                                                                        |
| $g \quad (0, 0, \frac{t}{2})$                       | $\{4_{001}   0 \ 0 \ \frac{1}{2}\}$<br>$g_1 \quad e^{-\frac{1}{2}i\pi t - \frac{3i\pi}{4}}$<br>$g_2 \quad e^{\frac{3i\pi}{4} - \frac{i\pi t}{2}}$<br>$g_3 \quad e^{-\frac{1}{2}i\pi t - \frac{i\pi}{4}}$<br>$g_4 \quad e^{\frac{i\pi}{4} - \frac{i\pi t}{2}}$ |
| $h \quad (0, \frac{1}{2}, \frac{t}{2})$             | $\{2_{001}   0 \ 0 \ 0\}$<br>$h_1 \quad -i$<br>$h_2 \quad i$                                                                                                                                                                                                  |
| $i \quad (\frac{1}{2}, \frac{1}{2}, \frac{t}{2})$   | $\{4_{001}   0 \ 0 \ \frac{1}{2}\}$<br>$i_1 \quad e^{-\frac{1}{2}i\pi t - \frac{3i\pi}{4}}$<br>$i_2 \quad e^{\frac{3i\pi}{4} - \frac{i\pi t}{2}}$<br>$i_3 \quad e^{-\frac{1}{2}i\pi t - \frac{i\pi}{4}}$<br>$i_4 \quad e^{\frac{i\pi}{4} - \frac{i\pi t}{2}}$ |

---


$$\begin{aligned}
\mathcal{W}_1^{\text{gapless}} = & \sum_{m=1}^{n_{a1}} \text{sgn}(v_m^{a1}) \frac{1 - \text{sgn}(\delta_m^{a1})}{2} + \sum_{m=1}^{n_{a2}} \text{sgn}(v_m^{a2}) \frac{1 - \text{sgn}(\delta_m^{a2})}{2} - \sum_{m=1}^{n_{e1}} \text{sgn}(v_m^{e1}) \frac{1 - \text{sgn}(\delta_m^{e1})}{2} \\
& - \sum_{m=1}^{n_{e2}} \text{sgn}(v_m^{e2}) \frac{1 - \text{sgn}(\delta_m^{e2})}{2} - \sum_{m=1}^{n_{f1}} \text{sgn}(v_m^{f1}) \frac{1 - \text{sgn}(\delta_m^{f1})}{2} - \sum_{m=1}^{n_{f2}} \text{sgn}(v_m^{f2}) \frac{1 - \text{sgn}(\delta_m^{f2})}{2} \\
& - \sum_{m=1}^{n_{g1}} \text{sgn}(v_m^{g1}) \frac{1 - \text{sgn}(\delta_m^{g1})}{2} - \sum_{m=1}^{n_{g2}} \text{sgn}(v_m^{g2}) \frac{1 - \text{sgn}(\delta_m^{g2})}{2} - \sum_{m=1}^{n_{g3}} \text{sgn}(v_m^{g3}) \frac{1 - \text{sgn}(\delta_m^{g3})}{2} \\
& - \sum_{m=1}^{n_{g4}} \text{sgn}(v_m^{g4}) \frac{1 - \text{sgn}(\delta_m^{g4})}{2} + \sum_{m=1}^{n_{h1}} \text{sgn}(v_m^{h1}) \frac{1 - \text{sgn}(\delta_m^{h1})}{2} + \sum_{m=1}^{n_{h2}} \text{sgn}(v_m^{h2}) \frac{1 - \text{sgn}(\delta_m^{h2})}{2}
\end{aligned} \tag{S93.1}$$

$$\begin{aligned}
\mathcal{W}_2^{\text{gapless}} = & \sum_{m=1}^{n_{b1}} \text{sgn}(v_m^{b1}) \frac{1 - \text{sgn}(\delta_m^{b1})}{2} + \sum_{m=1}^{n_{b2}} \text{sgn}(v_m^{b2}) \frac{1 - \text{sgn}(\delta_m^{b2})}{2} - \sum_{m=1}^{n_{e1}} \text{sgn}(v_m^{e1}) \frac{1 - \text{sgn}(\delta_m^{e1})}{2} - \sum_{m=1}^{n_{e2}} \text{sgn}(v_m^{e2}) \frac{1 - \text{sgn}(\delta_m^{e2})}{2} \\
& + \sum_{m=1}^{n_{h1}} \text{sgn}(v_m^{h1}) \frac{1 - \text{sgn}(\delta_m^{h1})}{2} + \sum_{m=1}^{n_{h2}} \text{sgn}(v_m^{h2}) \frac{1 - \text{sgn}(\delta_m^{h2})}{2} - \sum_{m=1}^{n_{i1}} \text{sgn}(v_m^{i1}) \frac{1 - \text{sgn}(\delta_m^{i1})}{2} \\
& - \sum_{m=1}^{n_{i2}} \text{sgn}(v_m^{i2}) \frac{1 - \text{sgn}(\delta_m^{i2})}{2} - \sum_{m=1}^{n_{i3}} \text{sgn}(v_m^{i3}) \frac{1 - \text{sgn}(\delta_m^{i3})}{2} - \sum_{m=1}^{n_{i4}} \text{sgn}(v_m^{i4}) \frac{1 - \text{sgn}(\delta_m^{i4})}{2}
\end{aligned} \tag{S93.2}$$

$$\begin{aligned}
\mathcal{W}_3^{\text{gapless}} = & \sum_{m=1}^{n_{c1}} \text{sgn}(v_m^{c1}) \frac{1 - \text{sgn}(\delta_m^{c1})}{2} + \sum_{m=1}^{n_{c2}} \text{sgn}(v_m^{c2}) \frac{1 - \text{sgn}(\delta_m^{c2})}{2} - \sum_{m=1}^{n_{f1}} \text{sgn}(v_m^{f1}) \frac{1 - \text{sgn}(\delta_m^{f1})}{2} \\
& - \sum_{m=1}^{n_{f2}} \text{sgn}(v_m^{f2}) \frac{1 - \text{sgn}(\delta_m^{f2})}{2} - \sum_{m=1}^{n_{g1}} \text{sgn}(v_m^{g1}) \frac{1 - \text{sgn}(\delta_m^{g1})}{2} - \sum_{m=1}^{n_{g2}} \text{sgn}(v_m^{g2}) \frac{1 - \text{sgn}(\delta_m^{g2})}{2} \\
& - \sum_{m=1}^{n_{g3}} \text{sgn}(v_m^{g3}) \frac{1 - \text{sgn}(\delta_m^{g3})}{2} - \sum_{m=1}^{n_{g4}} \text{sgn}(v_m^{g4}) \frac{1 - \text{sgn}(\delta_m^{g4})}{2} + \sum_{m=1}^{n_{i1}} \text{sgn}(v_m^{i1}) \frac{1 - \text{sgn}(\delta_m^{i1})}{2} \\
& + \sum_{m=1}^{n_{i2}} \text{sgn}(v_m^{i2}) \frac{1 - \text{sgn}(\delta_m^{i2})}{2} + \sum_{m=1}^{n_{i3}} \text{sgn}(v_m^{i3}) \frac{1 - \text{sgn}(\delta_m^{i3})}{2} + \sum_{m=1}^{n_{i4}} \text{sgn}(v_m^{i4}) \frac{1 - \text{sgn}(\delta_m^{i4})}{2}
\end{aligned} \tag{S93.3}$$

$$\begin{aligned}
\mathcal{W}_4^{\text{gapless}} = & \sum_{m=1}^{n_{d1}} \text{sgn}(v_m^{d1}) \frac{1 - \text{sgn}(\delta_m^{d1})}{2} + \sum_{m=1}^{n_{d2}} \text{sgn}(v_m^{d2}) \frac{1 - \text{sgn}(\delta_m^{d2})}{2} - \sum_{m=1}^{n_{e1}} \text{sgn}(v_m^{e1}) \frac{1 - \text{sgn}(\delta_m^{e1})}{2} \\
& - \sum_{m=1}^{n_{e2}} \text{sgn}(v_m^{e2}) \frac{1 - \text{sgn}(\delta_m^{e2})}{2} - \sum_{m=1}^{n_{f1}} \text{sgn}(v_m^{f1}) \frac{1 - \text{sgn}(\delta_m^{f1})}{2} - \sum_{m=1}^{n_{f2}} \text{sgn}(v_m^{f2}) \frac{1 - \text{sgn}(\delta_m^{f2})}{2}
\end{aligned} \tag{S93.4}$$

$$\begin{aligned}
\mathcal{W}_1^{\text{gapped}} = & - \sum_{m=1}^{n_{a2}} \text{sgn}(v_m^{a2}) \frac{1 - \text{sgn}(\delta_m^{a2})}{2} + \sum_{m=1}^{n_{e2}} \text{sgn}(v_m^{e2}) \frac{1 - \text{sgn}(\delta_m^{e2})}{2} + \sum_{m=1}^{n_{f1}} \text{sgn}(v_m^{f1}) \frac{1 - \text{sgn}(\delta_m^{f1})}{2} \\
& + \sum_{m=1}^{n_{g2}} \text{sgn}(v_m^{g2}) \frac{1 - \text{sgn}(\delta_m^{g2})}{2} + \sum_{m=1}^{n_{g3}} \text{sgn}(v_m^{g3}) \frac{1 - \text{sgn}(\delta_m^{g3})}{2} - \sum_{m=1}^{n_{h1}} \text{sgn}(v_m^{h1}) \frac{1 - \text{sgn}(\delta_m^{h1})}{2}
\end{aligned} \tag{S93.5}$$

$$\mathcal{W}_2^{\text{gapped}} = - \sum_{m=1}^{n_{a_2}} \text{sgn}(v_m^{a_2}) \frac{1 - \text{sgn}(\delta_m^{a_2})}{2} + \sum_{m=1}^{n_{b_2}} \text{sgn}(v_m^{b_2}) \frac{1 - \text{sgn}(\delta_m^{b_2})}{2} + \sum_{m=1}^{n_{c_2}} \text{sgn}(v_m^{c_2}) \frac{1 - \text{sgn}(\delta_m^{c_2})}{2} \quad (\text{S93.6})$$

$$\begin{aligned} \mathcal{W}_3^{\text{gapped}} = & - \sum_{m=1}^{n_{a_2}} \text{sgn}(v_m^{a_2}) \frac{1 - \text{sgn}(\delta_m^{a_2})}{2} + \sum_{m=1}^{n_{e_2}} \text{sgn}(v_m^{e_2}) \frac{1 - \text{sgn}(\delta_m^{e_2})}{2} + \sum_{m=1}^{n_{f_1}} \text{sgn}(v_m^{f_1}) \frac{1 - \text{sgn}(\delta_m^{f_1})}{2} \\ & + \sum_{m=1}^{n_{g_1}} \text{sgn}(v_m^{g_1}) \frac{1 - \text{sgn}(\delta_m^{g_1})}{2} + \sum_{m=1}^{n_{g_4}} \text{sgn}(v_m^{g_4}) \frac{1 - \text{sgn}(\delta_m^{g_4})}{2} - \sum_{m=1}^{n_{h_1}} \text{sgn}(v_m^{h_1}) \frac{1 - \text{sgn}(\delta_m^{h_1})}{2} \end{aligned} \quad (\text{S93.7})$$

$$\mathcal{W}_4^{\text{gapped}} = - \sum_{m=1}^{n_{f_1}} \text{sgn}(v_m^{f_1}) \frac{1 - \text{sgn}(\delta_m^{f_1})}{2} + \sum_{m=1}^{n_{f_2}} \text{sgn}(v_m^{f_2}) \frac{1 - \text{sgn}(\delta_m^{f_2})}{2} \quad (\text{S93.8})$$

$$\mathcal{W}_5^{\text{gapped}} = - \sum_{m=1}^{n_{h_1}} \text{sgn}(v_m^{h_1}) \frac{1 - \text{sgn}(\delta_m^{h_1})}{2} + \sum_{m=1}^{n_{h_2}} \text{sgn}(v_m^{h_2}) \frac{1 - \text{sgn}(\delta_m^{h_2})}{2} \quad (\text{S93.9})$$

$$\mathcal{W}_6^{\text{gapped}} = \sum_{m=1}^{n_{d_2}} \text{sgn}(v_m^{d_2}) \frac{1 - \text{sgn}(\delta_m^{d_2})}{2} - \sum_{m=1}^{n_{e_2}} \text{sgn}(v_m^{e_2}) \frac{1 - \text{sgn}(\delta_m^{e_2})}{2} - \sum_{m=1}^{n_{f_1}} \text{sgn}(v_m^{f_1}) \frac{1 - \text{sgn}(\delta_m^{f_1})}{2} \quad (\text{S93.10})$$

$$\begin{aligned} \mathcal{W}_7^{\text{gapped}} = & - \sum_{m=1}^{n_{b_2}} \text{sgn}(v_m^{b_2}) \frac{1 - \text{sgn}(\delta_m^{b_2})}{2} + \sum_{m=1}^{n_{e_2}} \text{sgn}(v_m^{e_2}) \frac{1 - \text{sgn}(\delta_m^{e_2})}{2} - \sum_{m=1}^{n_{h_1}} \text{sgn}(v_m^{h_1}) \frac{1 - \text{sgn}(\delta_m^{h_1})}{2} \\ & + \sum_{m=1}^{n_{i_2}} \text{sgn}(v_m^{i_2}) \frac{1 - \text{sgn}(\delta_m^{i_2})}{2} + \sum_{m=1}^{n_{i_3}} \text{sgn}(v_m^{i_3}) \frac{1 - \text{sgn}(\delta_m^{i_3})}{2} \end{aligned} \quad (\text{S93.11})$$

$$\mathcal{W}_8^{\text{gapped}} = \sum_{m=1}^{n_{e_1}} \text{sgn}(v_m^{e_1}) \frac{1 - \text{sgn}(\delta_m^{e_1})}{2} - \sum_{m=1}^{n_{e_2}} \text{sgn}(v_m^{e_2}) \frac{1 - \text{sgn}(\delta_m^{e_2})}{2} \quad (\text{S93.12})$$

$$\begin{aligned} \mathcal{W}_9^{\text{gapped}} = & - \sum_{m=1}^{n_{b_2}} \text{sgn}(v_m^{b_2}) \frac{1 - \text{sgn}(\delta_m^{b_2})}{2} + \sum_{m=1}^{n_{e_2}} \text{sgn}(v_m^{e_2}) \frac{1 - \text{sgn}(\delta_m^{e_2})}{2} - \sum_{m=1}^{n_{h_1}} \text{sgn}(v_m^{h_1}) \frac{1 - \text{sgn}(\delta_m^{h_1})}{2} \\ & + \sum_{m=1}^{n_{i_1}} \text{sgn}(v_m^{i_1}) \frac{1 - \text{sgn}(\delta_m^{i_1})}{2} + \sum_{m=1}^{n_{i_4}} \text{sgn}(v_m^{i_4}) \frac{1 - \text{sgn}(\delta_m^{i_4})}{2} \end{aligned} \quad (\text{S93.13})$$

$$\begin{aligned} \mathcal{X}_1 = & \sum_{m=1}^{n_{a_2}} \frac{1 - \text{sgn}(\delta_m^{a_2})}{2} + \sum_{m=1}^{n_{b_2}} \frac{1 - \text{sgn}(\delta_m^{b_2})}{2} + \sum_{m=1}^{n_{g_1}} \frac{1 - \text{sgn}(\delta_m^{g_1})}{2} + \sum_{m=1}^{n_{g_3}} \frac{1 - \text{sgn}(\delta_m^{g_3})}{2} \\ & + \sum_{m=1}^{n_{i_1}} \frac{1 - \text{sgn}(\delta_m^{i_1})}{2} + \sum_{m=1}^{n_{i_3}} \frac{1 - \text{sgn}(\delta_m^{i_3})}{2} \quad \text{mod } 2 \end{aligned} \quad (\text{S93.14})$$



## S94. SPACE GROUP NO. 94

| line segment                                        | character of irrep (generators only)                                                                                                                                                                                                                                                         |
|-----------------------------------------------------|----------------------------------------------------------------------------------------------------------------------------------------------------------------------------------------------------------------------------------------------------------------------------------------------|
| $a \quad (0, \frac{t}{2}, 0)$                       | $\{2_{010}   \frac{1}{2} \frac{1}{2} \frac{1}{2} \}$<br>$a_1 \quad -ie^{-\frac{1}{2}i\pi t}$<br>$a_2 \quad ie^{-\frac{1}{2}i\pi t}$                                                                                                                                                          |
| $b \quad (\frac{1-t}{2}, \frac{1}{2}, 0)$           | $\{2_{100}   \frac{1}{2} \frac{1}{2} \frac{1}{2} \}$<br>$b_1 \quad -e^{-\frac{1}{2}i\pi(2-t)}$<br>$b_2 \quad e^{-\frac{1}{2}i\pi(2-t)}$                                                                                                                                                      |
| $c \quad (\frac{t}{2}, \frac{t}{2}, 0)$             | $\{2_{110}   0 \ 0 \ 0 \}$<br>$c_1 \quad -i$<br>$c_2 \quad i$                                                                                                                                                                                                                                |
| $d \quad (0, \frac{t}{2}, \frac{1}{2})$             | $\{2_{010}   \frac{1}{2} \frac{1}{2} \frac{1}{2} \}$<br>$d_1 \quad -e^{-\frac{1}{2}i\pi(t+1)}$<br>$d_2 \quad e^{-\frac{1}{2}i\pi(t+1)}$                                                                                                                                                      |
| $e \quad (\frac{1-t}{2}, \frac{1}{2}, \frac{1}{2})$ | $\{2_{100}   \frac{1}{2} \frac{1}{2} \frac{1}{2} \}$<br>$e_1 \quad -ie^{-\frac{1}{2}i\pi(3-t)}$<br>$e_2 \quad ie^{-\frac{1}{2}i\pi(3-t)}$                                                                                                                                                    |
| $f \quad (\frac{t}{2}, \frac{t}{2}, \frac{1}{2})$   | $\{2_{110}   0 \ 0 \ 0 \}$<br>$f_1 \quad -i$<br>$f_2 \quad i$                                                                                                                                                                                                                                |
| $g \quad (0, 0, \frac{t}{2})$                       | $\{4_{001}   \frac{1}{2} \frac{1}{2} \frac{1}{2} \}$<br>$g_1 \quad e^{-\frac{1}{2}i\pi t - \frac{3i\pi}{4}}$<br>$g_2 \quad e^{\frac{3i\pi}{4} - \frac{i\pi t}{2}}$<br>$g_3 \quad e^{-\frac{1}{2}i\pi t - \frac{i\pi}{4}}$<br>$g_4 \quad e^{\frac{i\pi}{4} - \frac{i\pi t}{2}}$               |
| $h \quad (0, \frac{1}{2}, \frac{t}{2})$             | $\{2_{001}   0 \ 0 \ 0 \}$<br>$h_1 \quad -i$<br>$h_2 \quad i$                                                                                                                                                                                                                                |
| $i \quad (\frac{1}{2}, \frac{1}{2}, \frac{t}{2})$   | $\{4_{001}   \frac{1}{2} \frac{1}{2} \frac{1}{2} \}$<br>$i_1 \quad e^{-\frac{1}{2}i\pi(t+2) - \frac{3i\pi}{4}}$<br>$i_2 \quad e^{\frac{3i\pi}{4} - \frac{1}{2}i\pi(t+2)}$<br>$i_3 \quad e^{-\frac{1}{2}i\pi(t+2) - \frac{i\pi}{4}}$<br>$i_4 \quad e^{\frac{i\pi}{4} - \frac{1}{2}i\pi(t+2)}$ |

$$\begin{aligned}
\mathcal{W}_1^{\text{gapless}} = & \sum_{m=1}^{n_{a_1}} \text{sgn}(v_m^{a_1}) \frac{1 - \text{sgn}(\delta_m^{a_1})}{2} + \sum_{m=1}^{n_{a_2}} \text{sgn}(v_m^{a_2}) \frac{1 - \text{sgn}(\delta_m^{a_2})}{2} - 2 \sum_{m=1}^{n_{e_1}} \text{sgn}(v_m^{e_1}) \frac{1 - \text{sgn}(\delta_m^{e_1})}{2} \\
& - \sum_{m=1}^{n_{f_1}} \text{sgn}(v_m^{f_1}) \frac{1 - \text{sgn}(\delta_m^{f_1})}{2} - \sum_{m=1}^{n_{f_2}} \text{sgn}(v_m^{f_2}) \frac{1 - \text{sgn}(\delta_m^{f_2})}{2} - \sum_{m=1}^{n_{g_1}} \text{sgn}(v_m^{g_1}) \frac{1 - \text{sgn}(\delta_m^{g_1})}{2} \\
& - \sum_{m=1}^{n_{g_2}} \text{sgn}(v_m^{g_2}) \frac{1 - \text{sgn}(\delta_m^{g_2})}{2} - \sum_{m=1}^{n_{g_3}} \text{sgn}(v_m^{g_3}) \frac{1 - \text{sgn}(\delta_m^{g_3})}{2} - \sum_{m=1}^{n_{g_4}} \text{sgn}(v_m^{g_4}) \frac{1 - \text{sgn}(\delta_m^{g_4})}{2} \\
& + 2 \sum_{m=1}^{n_{h_1}} \text{sgn}(v_m^{h_1}) \frac{1 - \text{sgn}(\delta_m^{h_1})}{2}
\end{aligned} \tag{S94.1}$$

$$\begin{aligned}
\mathcal{W}_2^{\text{gapless}} = & \sum_{m=1}^{n_{b_1}} \text{sgn}(v_m^{b_1}) \frac{1 - \text{sgn}(\delta_m^{b_1})}{2} - \sum_{m=1}^{n_{e_1}} \text{sgn}(v_m^{e_1}) \frac{1 - \text{sgn}(\delta_m^{e_1})}{2} + \sum_{m=1}^{n_{h_1}} \text{sgn}(v_m^{h_1}) \frac{1 - \text{sgn}(\delta_m^{h_1})}{2} \\
& - \sum_{m=1}^{n_{i_1}} \text{sgn}(v_m^{i_1}) \frac{1 - \text{sgn}(\delta_m^{i_1})}{2} - \sum_{m=1}^{n_{i_2}} \text{sgn}(v_m^{i_2}) \frac{1 - \text{sgn}(\delta_m^{i_2})}{2}
\end{aligned} \tag{S94.2}$$

$$\begin{aligned}
\mathcal{W}_3^{\text{gapless}} = & \sum_{m=1}^{n_{c_1}} \text{sgn}(v_m^{c_1}) \frac{1 - \text{sgn}(\delta_m^{c_1})}{2} + \sum_{m=1}^{n_{c_2}} \text{sgn}(v_m^{c_2}) \frac{1 - \text{sgn}(\delta_m^{c_2})}{2} - \sum_{m=1}^{n_{f_1}} \text{sgn}(v_m^{f_1}) \frac{1 - \text{sgn}(\delta_m^{f_1})}{2} - \sum_{m=1}^{n_{f_2}} \text{sgn}(v_m^{f_2}) \frac{1 - \text{sgn}(\delta_m^{f_2})}{2} \\
& - \sum_{m=1}^{n_{g_1}} \text{sgn}(v_m^{g_1}) \frac{1 - \text{sgn}(\delta_m^{g_1})}{2} - \sum_{m=1}^{n_{g_2}} \text{sgn}(v_m^{g_2}) \frac{1 - \text{sgn}(\delta_m^{g_2})}{2} - \sum_{m=1}^{n_{g_3}} \text{sgn}(v_m^{g_3}) \frac{1 - \text{sgn}(\delta_m^{g_3})}{2} \\
& - \sum_{m=1}^{n_{g_4}} \text{sgn}(v_m^{g_4}) \frac{1 - \text{sgn}(\delta_m^{g_4})}{2} + 2 \sum_{m=1}^{n_{i_1}} \text{sgn}(v_m^{i_1}) \frac{1 - \text{sgn}(\delta_m^{i_1})}{2} + 2 \sum_{m=1}^{n_{i_2}} \text{sgn}(v_m^{i_2}) \frac{1 - \text{sgn}(\delta_m^{i_2})}{2}
\end{aligned} \tag{S94.3}$$

$$\begin{aligned}
\mathcal{W}_4^{\text{gapless}} = & \sum_{m=1}^{n_{d_1}} \text{sgn}(v_m^{d_1}) \frac{1 - \text{sgn}(\delta_m^{d_1})}{2} + \sum_{m=1}^{n_{d_2}} \text{sgn}(v_m^{d_2}) \frac{1 - \text{sgn}(\delta_m^{d_2})}{2} - 2 \sum_{m=1}^{n_{e_1}} \text{sgn}(v_m^{e_1}) \frac{1 - \text{sgn}(\delta_m^{e_1})}{2} \\
& - \sum_{m=1}^{n_{f_1}} \text{sgn}(v_m^{f_1}) \frac{1 - \text{sgn}(\delta_m^{f_1})}{2} - \sum_{m=1}^{n_{f_2}} \text{sgn}(v_m^{f_2}) \frac{1 - \text{sgn}(\delta_m^{f_2})}{2}
\end{aligned} \tag{S94.4}$$

$$\mathcal{W}_1^{\text{gapped}} = \sum_{m=1}^{n_{g_1}} \text{sgn}(v_m^{g_1}) \frac{1 - \text{sgn}(\delta_m^{g_1})}{2} - \sum_{m=1}^{n_{g_2}} \text{sgn}(v_m^{g_2}) \frac{1 - \text{sgn}(\delta_m^{g_2})}{2} - \sum_{m=1}^{n_{g_3}} \text{sgn}(v_m^{g_3}) \frac{1 - \text{sgn}(\delta_m^{g_3})}{2} + \sum_{m=1}^{n_{g_4}} \text{sgn}(v_m^{g_4}) \frac{1 - \text{sgn}(\delta_m^{g_4})}{2} \tag{S94.5}$$

$$\mathcal{W}_2^{\text{gapped}} = - \sum_{m=1}^{n_{f_1}} \text{sgn}(v_m^{f_1}) \frac{1 - \text{sgn}(\delta_m^{f_1})}{2} + \sum_{m=1}^{n_{f_2}} \text{sgn}(v_m^{f_2}) \frac{1 - \text{sgn}(\delta_m^{f_2})}{2} \tag{S94.6}$$

$$\begin{aligned}
\mathcal{W}_3^{\text{gapped}} = & \sum_{m=1}^{n_{c_2}} \text{sgn}(v_m^{c_2}) \frac{1 - \text{sgn}(\delta_m^{c_2})}{2} - \sum_{m=1}^{n_{f_1}} \text{sgn}(v_m^{f_1}) \frac{1 - \text{sgn}(\delta_m^{f_1})}{2} - \sum_{m=1}^{n_{g_2}} \text{sgn}(v_m^{g_2}) \frac{1 - \text{sgn}(\delta_m^{g_2})}{2} \\
& - \sum_{m=1}^{n_{g_3}} \text{sgn}(v_m^{g_3}) \frac{1 - \text{sgn}(\delta_m^{g_3})}{2} + \sum_{m=1}^{n_{i_1}} \text{sgn}(v_m^{i_1}) \frac{1 - \text{sgn}(\delta_m^{i_1})}{2} + \sum_{m=1}^{n_{i_2}} \text{sgn}(v_m^{i_2}) \frac{1 - \text{sgn}(\delta_m^{i_2})}{2}
\end{aligned} \tag{S94.7}$$

$$\begin{aligned}
\mathcal{W}_4^{\text{gapped}} = & \sum_{m=1}^{n_{c_2}} \text{sgn}(v_m^{c_2}) \frac{1 - \text{sgn}(\delta_m^{c_2})}{2} - \sum_{m=1}^{n_{f_1}} \text{sgn}(v_m^{f_1}) \frac{1 - \text{sgn}(\delta_m^{f_1})}{2} - \sum_{m=1}^{n_{g_2}} \text{sgn}(v_m^{g_2}) \frac{1 - \text{sgn}(\delta_m^{g_2})}{2} \\
& - \sum_{m=1}^{n_{g_3}} \text{sgn}(v_m^{g_3}) \frac{1 - \text{sgn}(\delta_m^{g_3})}{2} + 2 \sum_{m=1}^{n_{i_2}} \text{sgn}(v_m^{i_2}) \frac{1 - \text{sgn}(\delta_m^{i_2})}{2}
\end{aligned} \tag{S94.8}$$

$$\mathcal{X}_1 = \sum_{m=1}^{n_{a_2}} \frac{1 - \text{sgn}(\delta_m^{a_2})}{2} + \sum_{m=1}^{n_{g_1}} \frac{1 - \text{sgn}(\delta_m^{g_1})}{2} + \sum_{m=1}^{n_{g_3}} \frac{1 - \text{sgn}(\delta_m^{g_3})}{2} \mod 2 \tag{S94.9}$$

$$\mathcal{X}_2 = \sum_{m=1}^{n_{a_2}} \frac{1 - \text{sgn}(\delta_m^{a_2})}{2} + \sum_{m=1}^{n_{f_1}} \frac{1 - \text{sgn}(\delta_m^{f_1})}{2} + \sum_{m=1}^{n_{g_2}} \frac{1 - \text{sgn}(\delta_m^{g_2})}{2} + \sum_{m=1}^{n_{g_3}} \frac{1 - \text{sgn}(\delta_m^{g_3})}{2} \mod 2 \tag{S94.10}$$

$$\mathcal{X}_3 = \sum_{m=1}^{n_{a_2}} \frac{1 - \text{sgn}(\delta_m^{a_2})}{2} + \sum_{m=1}^{n_{d_2}} \frac{1 - \text{sgn}(\delta_m^{d_2})}{2} + \sum_{m=1}^{n_{g_2}} \frac{1 - \text{sgn}(\delta_m^{g_2})}{2} + \sum_{m=1}^{n_{g_3}} \frac{1 - \text{sgn}(\delta_m^{g_3})}{2} \mod 2 \tag{S94.11}$$

## S95. SPACE GROUP NO. 95

| line segment                                        | character of irrep (generators only)                                                                                                                                                                                                                            |
|-----------------------------------------------------|-----------------------------------------------------------------------------------------------------------------------------------------------------------------------------------------------------------------------------------------------------------------|
| $a \quad (0, \frac{t}{2}, 0)$                       | $\{2_{010}   0 \ 0 \ 0\}$<br>$a_1 \quad -i$<br>$a_2 \quad i$                                                                                                                                                                                                    |
| $b \quad (\frac{1-t}{2}, \frac{1}{2}, 0)$           | $\{2_{100}   0 \ 0 \ \frac{1}{2}\}$<br>$b_1 \quad -i$<br>$b_2 \quad i$                                                                                                                                                                                          |
| $c \quad (\frac{t}{2}, \frac{t}{2}, 0)$             | $\{2_{110}   0 \ 0 \ \frac{1}{4}\}$<br>$c_1 \quad -i$<br>$c_2 \quad i$                                                                                                                                                                                          |
| $d \quad (0, \frac{t}{2}, \frac{1}{2})$             | $\{2_{010}   0 \ 0 \ 0\}$<br>$d_1 \quad -i$<br>$d_2 \quad i$                                                                                                                                                                                                    |
| $e \quad (\frac{1-t}{2}, \frac{1}{2}, \frac{1}{2})$ | $\{2_{100}   0 \ 0 \ \frac{1}{2}\}$<br>$e_1 \quad i$<br>$e_2 \quad -i$                                                                                                                                                                                          |
| $f \quad (\frac{t}{2}, \frac{t}{2}, \frac{1}{2})$   | $\{2_{110}   0 \ 0 \ \frac{1}{4}\}$<br>$f_1 \quad i$<br>$f_2 \quad -i$                                                                                                                                                                                          |
| $g \quad (0, 0, \frac{t}{2})$                       | $\{4_{001}   0 \ 0 \ \frac{3}{4}\}$<br>$g_1 \quad e^{-\frac{3}{4}i\pi t - \frac{3i\pi}{4}}$<br>$g_2 \quad e^{\frac{3i\pi}{4} - \frac{3i\pi t}{4}}$<br>$g_3 \quad e^{-\frac{3}{4}i\pi t - \frac{i\pi}{4}}$<br>$g_4 \quad e^{\frac{i\pi}{4} - \frac{3i\pi t}{4}}$ |
| $h \quad (0, \frac{1}{2}, \frac{t}{2})$             | $\{2_{001}   0 \ 0 \ \frac{1}{2}\}$<br>$h_1 \quad -ie^{-\frac{1}{2}i\pi t}$<br>$h_2 \quad ie^{-\frac{1}{2}i\pi t}$                                                                                                                                              |
| $i \quad (\frac{1}{2}, \frac{1}{2}, \frac{t}{2})$   | $\{4_{001}   0 \ 0 \ \frac{3}{4}\}$<br>$i_1 \quad e^{-\frac{3}{4}i\pi t - \frac{3i\pi}{4}}$<br>$i_2 \quad e^{\frac{3i\pi}{4} - \frac{3i\pi t}{4}}$<br>$i_3 \quad e^{-\frac{3}{4}i\pi t - \frac{i\pi}{4}}$<br>$i_4 \quad e^{\frac{i\pi}{4} - \frac{3i\pi t}{4}}$ |

$$\begin{aligned}
\mathcal{W}_1^{\text{gapless}} = & \sum_{m=1}^{n_{a_1}} \text{sgn}(v_m^{a_1}) \frac{1 - \text{sgn}(\delta_m^{a_1})}{2} + \sum_{m=1}^{n_{a_2}} \text{sgn}(v_m^{a_2}) \frac{1 - \text{sgn}(\delta_m^{a_2})}{2} - 2 \sum_{m=1}^{n_{e_1}} \text{sgn}(v_m^{e_1}) \frac{1 - \text{sgn}(\delta_m^{e_1})}{2} \\
& - 2 \sum_{m=1}^{n_{f_1}} \text{sgn}(v_m^{f_1}) \frac{1 - \text{sgn}(\delta_m^{f_1})}{2} - \sum_{m=1}^{n_{g_1}} \text{sgn}(v_m^{g_1}) \frac{1 - \text{sgn}(\delta_m^{g_1})}{2} - \sum_{m=1}^{n_{g_2}} \text{sgn}(v_m^{g_2}) \frac{1 - \text{sgn}(\delta_m^{g_2})}{2} \\
& - \sum_{m=1}^{n_{g_3}} \text{sgn}(v_m^{g_3}) \frac{1 - \text{sgn}(\delta_m^{g_3})}{2} - \sum_{m=1}^{n_{g_4}} \text{sgn}(v_m^{g_4}) \frac{1 - \text{sgn}(\delta_m^{g_4})}{2} + \sum_{m=1}^{n_{h_1}} \text{sgn}(v_m^{h_1}) \frac{1 - \text{sgn}(\delta_m^{h_1})}{2} \\
& + \sum_{m=1}^{n_{h_2}} \text{sgn}(v_m^{h_2}) \frac{1 - \text{sgn}(\delta_m^{h_2})}{2}
\end{aligned} \tag{S95.1}$$

$$\begin{aligned}
\mathcal{W}_2^{\text{gapless}} = & \sum_{m=1}^{n_{b_1}} \text{sgn}(v_m^{b_1}) \frac{1 - \text{sgn}(\delta_m^{b_1})}{2} + \sum_{m=1}^{n_{b_2}} \text{sgn}(v_m^{b_2}) \frac{1 - \text{sgn}(\delta_m^{b_2})}{2} - 2 \sum_{m=1}^{n_{e_1}} \text{sgn}(v_m^{e_1}) \frac{1 - \text{sgn}(\delta_m^{e_1})}{2} \\
& + \sum_{m=1}^{n_{h_1}} \text{sgn}(v_m^{h_1}) \frac{1 - \text{sgn}(\delta_m^{h_1})}{2} + \sum_{m=1}^{n_{h_2}} \text{sgn}(v_m^{h_2}) \frac{1 - \text{sgn}(\delta_m^{h_2})}{2} - \sum_{m=1}^{n_{i_1}} \text{sgn}(v_m^{i_1}) \frac{1 - \text{sgn}(\delta_m^{i_1})}{2} \\
& - \sum_{m=1}^{n_{i_2}} \text{sgn}(v_m^{i_2}) \frac{1 - \text{sgn}(\delta_m^{i_2})}{2} - \sum_{m=1}^{n_{i_3}} \text{sgn}(v_m^{i_3}) \frac{1 - \text{sgn}(\delta_m^{i_3})}{2} - \sum_{m=1}^{n_{i_4}} \text{sgn}(v_m^{i_4}) \frac{1 - \text{sgn}(\delta_m^{i_4})}{2}
\end{aligned} \tag{S95.2}$$

$$\begin{aligned}
\mathcal{W}_3^{\text{gapless}} = & \sum_{m=1}^{n_{c_1}} \text{sgn}(v_m^{c_1}) \frac{1 - \text{sgn}(\delta_m^{c_1})}{2} + \sum_{m=1}^{n_{c_2}} \text{sgn}(v_m^{c_2}) \frac{1 - \text{sgn}(\delta_m^{c_2})}{2} - 2 \sum_{m=1}^{n_{f_1}} \text{sgn}(v_m^{f_1}) \frac{1 - \text{sgn}(\delta_m^{f_1})}{2} - \sum_{m=1}^{n_{g_1}} \text{sgn}(v_m^{g_1}) \frac{1 - \text{sgn}(\delta_m^{g_1})}{2} \\
& - \sum_{m=1}^{n_{g_2}} \text{sgn}(v_m^{g_2}) \frac{1 - \text{sgn}(\delta_m^{g_2})}{2} - \sum_{m=1}^{n_{g_3}} \text{sgn}(v_m^{g_3}) \frac{1 - \text{sgn}(\delta_m^{g_3})}{2} - \sum_{m=1}^{n_{g_4}} \text{sgn}(v_m^{g_4}) \frac{1 - \text{sgn}(\delta_m^{g_4})}{2} \\
& + \sum_{m=1}^{n_{i_1}} \text{sgn}(v_m^{i_1}) \frac{1 - \text{sgn}(\delta_m^{i_1})}{2} + \sum_{m=1}^{n_{i_2}} \text{sgn}(v_m^{i_2}) \frac{1 - \text{sgn}(\delta_m^{i_2})}{2} + \sum_{m=1}^{n_{i_3}} \text{sgn}(v_m^{i_3}) \frac{1 - \text{sgn}(\delta_m^{i_3})}{2} + \sum_{m=1}^{n_{i_4}} \text{sgn}(v_m^{i_4}) \frac{1 - \text{sgn}(\delta_m^{i_4})}{2}
\end{aligned} \tag{S95.3}$$

$$\mathcal{W}_4^{\text{gapless}} = \sum_{m=1}^{n_{d_1}} \text{sgn}(v_m^{d_1}) \frac{1 - \text{sgn}(\delta_m^{d_1})}{2} - \sum_{m=1}^{n_{e_1}} \text{sgn}(v_m^{e_1}) \frac{1 - \text{sgn}(\delta_m^{e_1})}{2} - \sum_{m=1}^{n_{f_1}} \text{sgn}(v_m^{f_1}) \frac{1 - \text{sgn}(\delta_m^{f_1})}{2} \tag{S95.4}$$

$$\mathcal{W}_1^{\text{gapped}} = - \sum_{m=1}^{n_{a_2}} \text{sgn}(v_m^{a_2}) \frac{1 - \text{sgn}(\delta_m^{a_2})}{2} + \sum_{m=1}^{n_{b_2}} \text{sgn}(v_m^{b_2}) \frac{1 - \text{sgn}(\delta_m^{b_2})}{2} + \sum_{m=1}^{n_{c_2}} \text{sgn}(v_m^{c_2}) \frac{1 - \text{sgn}(\delta_m^{c_2})}{2} \tag{S95.5}$$

$$\begin{aligned}
\mathcal{W}_2^{\text{gapped}} = & -2 \sum_{m=1}^{n_{a_2}} \text{sgn}(v_m^{a_2}) \frac{1 - \text{sgn}(\delta_m^{a_2})}{2} + 2 \sum_{m=1}^{n_{e_1}} \text{sgn}(v_m^{e_1}) \frac{1 - \text{sgn}(\delta_m^{e_1})}{2} + 2 \sum_{m=1}^{n_{f_1}} \text{sgn}(v_m^{f_1}) \frac{1 - \text{sgn}(\delta_m^{f_1})}{2} \\
& + \sum_{m=1}^{n_{g_1}} \text{sgn}(v_m^{g_1}) \frac{1 - \text{sgn}(\delta_m^{g_1})}{2} + \sum_{m=1}^{n_{g_2}} \text{sgn}(v_m^{g_2}) \frac{1 - \text{sgn}(\delta_m^{g_2})}{2} + \sum_{m=1}^{n_{g_3}} \text{sgn}(v_m^{g_3}) \frac{1 - \text{sgn}(\delta_m^{g_3})}{2} \\
& + \sum_{m=1}^{n_{g_4}} \text{sgn}(v_m^{g_4}) \frac{1 - \text{sgn}(\delta_m^{g_4})}{2} - \sum_{m=1}^{n_{h_1}} \text{sgn}(v_m^{h_1}) \frac{1 - \text{sgn}(\delta_m^{h_1})}{2} - \sum_{m=1}^{n_{h_2}} \text{sgn}(v_m^{h_2}) \frac{1 - \text{sgn}(\delta_m^{h_2})}{2}
\end{aligned} \tag{S95.6}$$

$$\begin{aligned}
\mathcal{W}_3^{\text{gapped}} = & -2 \sum_{m=1}^{n_{b_2}} \text{sgn}(v_m^{b_2}) \frac{1 - \text{sgn}(\delta_m^{b_2})}{2} + 2 \sum_{m=1}^{n_{e_1}} \text{sgn}(v_m^{e_1}) \frac{1 - \text{sgn}(\delta_m^{e_1})}{2} \\
& - \sum_{m=1}^{n_{h_1}} \text{sgn}(v_m^{h_1}) \frac{1 - \text{sgn}(\delta_m^{h_1})}{2} - \sum_{m=1}^{n_{h_2}} \text{sgn}(v_m^{h_2}) \frac{1 - \text{sgn}(\delta_m^{h_2})}{2} + \sum_{m=1}^{n_{i_1}} \text{sgn}(v_m^{i_1}) \frac{1 - \text{sgn}(\delta_m^{i_1})}{2} \\
& + \sum_{m=1}^{n_{i_2}} \text{sgn}(v_m^{i_2}) \frac{1 - \text{sgn}(\delta_m^{i_2})}{2} + \sum_{m=1}^{n_{i_3}} \text{sgn}(v_m^{i_3}) \frac{1 - \text{sgn}(\delta_m^{i_3})}{2} + \sum_{m=1}^{n_{i_4}} \text{sgn}(v_m^{i_4}) \frac{1 - \text{sgn}(\delta_m^{i_4})}{2}
\end{aligned} \tag{S95.7}$$

$$\mathcal{X}_1 = \sum_{m=1}^{n_{b_2}} \frac{1 - \text{sgn}(\delta_m^{b_2})}{2} + \sum_{m=1}^{n_{h_2}} \frac{1 - \text{sgn}(\delta_m^{h_2})}{2} + \sum_{m=1}^{n_{i_2}} \frac{1 - \text{sgn}(\delta_m^{i_2})}{2} + \sum_{m=1}^{n_{i_3}} \frac{1 - \text{sgn}(\delta_m^{i_3})}{2} \pmod{2} \tag{S95.8}$$

$$\begin{aligned} \mathcal{X}_2 = & \sum_{m=1}^{n_{a_2}} \frac{1 - \text{sgn}(\delta_m^{a_2})}{2} + \sum_{m=1}^{n_{b_2}} \frac{1 - \text{sgn}(\delta_m^{b_2})}{2} + \sum_{m=1}^{n_{g_1}} \frac{1 - \text{sgn}(\delta_m^{g_1})}{2} + \sum_{m=1}^{n_{g_4}} \frac{1 - \text{sgn}(\delta_m^{g_4})}{2} \\ & + \sum_{m=1}^{n_{i_2}} \frac{1 - \text{sgn}(\delta_m^{i_2})}{2} + \sum_{m=1}^{n_{i_3}} \frac{1 - \text{sgn}(\delta_m^{i_3})}{2} \pmod{2} \end{aligned} \quad (\text{S95.9})$$

$$\begin{aligned} \mathcal{X}_3 = & -3 \sum_{m=1}^{n_{a_2}} \text{sgn}(v_m^{a_2}) \frac{1 - \text{sgn}(\delta_m^{a_2})}{2} + \sum_{m=1}^{n_{b_2}} \text{sgn}(v_m^{b_2}) \frac{1 - \text{sgn}(\delta_m^{b_2})}{2} + 2 \sum_{m=1}^{n_{e_1}} \text{sgn}(v_m^{e_1}) \frac{1 - \text{sgn}(\delta_m^{e_1})}{2} \\ & + 3 \sum_{m=1}^{n_{g_1}} \text{sgn}(v_m^{g_1}) \frac{1 - \text{sgn}(\delta_m^{g_1})}{2} + 2 \sum_{m=1}^{n_{g_3}} \text{sgn}(v_m^{g_3}) \frac{1 - \text{sgn}(\delta_m^{g_3})}{2} + \sum_{m=1}^{n_{g_4}} \text{sgn}(v_m^{g_4}) \frac{1 - \text{sgn}(\delta_m^{g_4})}{2} \\ & - \sum_{m=1}^{n_{h_1}} \text{sgn}(v_m^{h_1}) \frac{1 - \text{sgn}(\delta_m^{h_1})}{2} - \sum_{m=1}^{n_{h_2}} \text{sgn}(v_m^{h_2}) \frac{1 - \text{sgn}(\delta_m^{h_2})}{2} - 2 \sum_{m=1}^{n_{i_1}} \text{sgn}(v_m^{i_1}) \frac{1 - \text{sgn}(\delta_m^{i_1})}{2} + \sum_{m=1}^{n_{i_2}} \text{sgn}(v_m^{i_2}) \frac{1 - \text{sgn}(\delta_m^{i_2})}{2} \\ & - \sum_{m=1}^{n_{i_3}} \text{sgn}(v_m^{i_3}) \frac{1 - \text{sgn}(\delta_m^{i_3})}{2} \pmod{4} \end{aligned} \quad (\text{S95.10})$$

### S96. SPACE GROUP NO. 96

| line segment                                        | character of irrep (generators only)                                                                                                                                                                                                                                            |
|-----------------------------------------------------|---------------------------------------------------------------------------------------------------------------------------------------------------------------------------------------------------------------------------------------------------------------------------------|
| $a \quad (0, \frac{t}{2}, 0)$                       | $\{2_{010}   \frac{1}{2} \frac{1}{2} \frac{3}{4}\}$<br>$a_1 \quad -ie^{-\frac{1}{2}i\pi t}$<br>$a_2 \quad ie^{-\frac{1}{2}i\pi t}$                                                                                                                                              |
| $b \quad (\frac{1-t}{2}, \frac{1}{2}, 0)$           | $\{2_{100}   \frac{1}{2} \frac{1}{2} \frac{1}{4}\}$<br>$b_1 \quad -e^{-\frac{1}{2}i\pi(2-t)}$<br>$b_2 \quad e^{-\frac{1}{2}i\pi(2-t)}$                                                                                                                                          |
| $c \quad (\frac{t}{2}, \frac{t}{2}, 0)$             | $\{2_{110}   0 \ 0 \ 0\}$<br>$c_1 \quad -i$<br>$c_2 \quad i$                                                                                                                                                                                                                    |
| $d \quad (0, \frac{t}{2}, \frac{1}{2})$             | $\{2_{010}   \frac{1}{2} \frac{1}{2} \frac{3}{4}\}$<br>$d_1 \quad e^{-\frac{1}{4}i\pi(2t+3) - \frac{3i\pi}{4}}$<br>$d_2 \quad e^{\frac{i\pi}{4} - \frac{1}{4}i\pi(2t+3)}$                                                                                                       |
| $e \quad (\frac{1-t}{2}, \frac{1}{2}, \frac{1}{2})$ | $\{2_{100}   \frac{1}{2} \frac{1}{2} \frac{1}{4}\}$<br>$e_1 \quad e^{-\frac{1}{4}i\pi(5-2t) - \frac{3i\pi}{4}}$<br>$e_2 \quad e^{\frac{i\pi}{4} - \frac{1}{4}i\pi(5-2t)}$                                                                                                       |
| $f \quad (\frac{t}{2}, \frac{t}{2}, \frac{1}{2})$   | $\{2_{110}   0 \ 0 \ 0\}$<br>$f_1 \quad -i$<br>$f_2 \quad i$                                                                                                                                                                                                                    |
| $g \quad (0, 0, \frac{t}{2})$                       | $\{4_{001}   \frac{1}{2} \frac{1}{2} \frac{3}{4}\}$<br>$g_1 \quad e^{-\frac{3}{4}i\pi t - \frac{3i\pi}{4}}$<br>$g_2 \quad e^{\frac{3i\pi}{4} - \frac{3i\pi t}{4}}$<br>$g_3 \quad e^{-\frac{3}{4}i\pi t - \frac{i\pi}{4}}$<br>$g_4 \quad e^{\frac{i\pi}{4} - \frac{3i\pi t}{4}}$ |
| $h \quad (0, \frac{1}{2}, \frac{t}{2})$             | $\{2_{001}   0 \ 0 \ \frac{1}{2}\}$<br>$h_1 \quad -ie^{-\frac{1}{2}i\pi t}$<br>$h_2 \quad ie^{-\frac{1}{2}i\pi t}$                                                                                                                                                              |

|       |                                                    |
|-------|----------------------------------------------------|
|       | $\{4001   \frac{1}{2}, \frac{1}{2}, \frac{3}{4}\}$ |
| $i_1$ | $e^{-\frac{1}{4}i\pi(3t+4) - \frac{3i\pi}{4}}$     |
| $i_2$ | $e^{\frac{3i\pi}{4} - \frac{1}{4}i\pi(3t+4)}$      |
| $i_3$ | $e^{-\frac{1}{4}i\pi(3t+4) - \frac{i\pi}{4}}$      |
| $i_4$ | $e^{\frac{i\pi}{4} - \frac{1}{4}i\pi(3t+4)}$       |

$$\begin{aligned}
\mathcal{W}_1^{\text{gapless}} = & \sum_{m=1}^{n_{a_1}} \text{sgn}(v_m^{a_1}) \frac{1 - \text{sgn}(\delta_m^{a_1})}{2} + \sum_{m=1}^{n_{a_2}} \text{sgn}(v_m^{a_2}) \frac{1 - \text{sgn}(\delta_m^{a_2})}{2} - 2 \sum_{m=1}^{n_{e_1}} \text{sgn}(v_m^{e_1}) \frac{1 - \text{sgn}(\delta_m^{e_1})}{2} \\
& - 2 \sum_{m=1}^{n_{e_2}} \text{sgn}(v_m^{e_2}) \frac{1 - \text{sgn}(\delta_m^{e_2})}{2} - 2 \sum_{m=1}^{n_{f_1}} \text{sgn}(v_m^{f_1}) \frac{1 - \text{sgn}(\delta_m^{f_1})}{2} - \sum_{m=1}^{n_{g_1}} \text{sgn}(v_m^{g_1}) \frac{1 - \text{sgn}(\delta_m^{g_1})}{2} \\
& - \sum_{m=1}^{n_{g_2}} \text{sgn}(v_m^{g_2}) \frac{1 - \text{sgn}(\delta_m^{g_2})}{2} - \sum_{m=1}^{n_{g_3}} \text{sgn}(v_m^{g_3}) \frac{1 - \text{sgn}(\delta_m^{g_3})}{2} - \sum_{m=1}^{n_{g_4}} \text{sgn}(v_m^{g_4}) \frac{1 - \text{sgn}(\delta_m^{g_4})}{2} \\
& + 2 \sum_{m=1}^{n_{h_1}} \text{sgn}(v_m^{h_1}) \frac{1 - \text{sgn}(\delta_m^{h_1})}{2}
\end{aligned} \tag{S96.1}$$

$$\begin{aligned}
\mathcal{W}_2^{\text{gapless}} = & \sum_{m=1}^{n_{b_1}} \text{sgn}(v_m^{b_1}) \frac{1 - \text{sgn}(\delta_m^{b_1})}{2} - \sum_{m=1}^{n_{e_1}} \text{sgn}(v_m^{e_1}) \frac{1 - \text{sgn}(\delta_m^{e_1})}{2} - \sum_{m=1}^{n_{e_2}} \text{sgn}(v_m^{e_2}) \frac{1 - \text{sgn}(\delta_m^{e_2})}{2} \\
& + \sum_{m=1}^{n_{h_1}} \text{sgn}(v_m^{h_1}) \frac{1 - \text{sgn}(\delta_m^{h_1})}{2} - \sum_{m=1}^{n_{i_1}} \text{sgn}(v_m^{i_1}) \frac{1 - \text{sgn}(\delta_m^{i_1})}{2} - \sum_{m=1}^{n_{i_2}} \text{sgn}(v_m^{i_2}) \frac{1 - \text{sgn}(\delta_m^{i_2})}{2}
\end{aligned} \tag{S96.2}$$

$$\begin{aligned}
\mathcal{W}_3^{\text{gapless}} = & \sum_{m=1}^{n_{c_1}} \text{sgn}(v_m^{c_1}) \frac{1 - \text{sgn}(\delta_m^{c_1})}{2} + \sum_{m=1}^{n_{c_2}} \text{sgn}(v_m^{c_2}) \frac{1 - \text{sgn}(\delta_m^{c_2})}{2} - 2 \sum_{m=1}^{n_{f_1}} \text{sgn}(v_m^{f_1}) \frac{1 - \text{sgn}(\delta_m^{f_1})}{2} \\
& - \sum_{m=1}^{n_{g_1}} \text{sgn}(v_m^{g_1}) \frac{1 - \text{sgn}(\delta_m^{g_1})}{2} - \sum_{m=1}^{n_{g_2}} \text{sgn}(v_m^{g_2}) \frac{1 - \text{sgn}(\delta_m^{g_2})}{2} - \sum_{m=1}^{n_{g_3}} \text{sgn}(v_m^{g_3}) \frac{1 - \text{sgn}(\delta_m^{g_3})}{2} \\
& - \sum_{m=1}^{n_{g_4}} \text{sgn}(v_m^{g_4}) \frac{1 - \text{sgn}(\delta_m^{g_4})}{2} + 2 \sum_{m=1}^{n_{i_1}} \text{sgn}(v_m^{i_1}) \frac{1 - \text{sgn}(\delta_m^{i_1})}{2} + 2 \sum_{m=1}^{n_{i_2}} \text{sgn}(v_m^{i_2}) \frac{1 - \text{sgn}(\delta_m^{i_2})}{2}
\end{aligned} \tag{S96.3}$$

$$\begin{aligned}
\mathcal{W}_4^{\text{gapless}} = & \sum_{m=1}^{n_{d_1}} \text{sgn}(v_m^{d_1}) \frac{1 - \text{sgn}(\delta_m^{d_1})}{2} - \sum_{m=1}^{n_{e_1}} \text{sgn}(v_m^{e_1}) \frac{1 - \text{sgn}(\delta_m^{e_1})}{2} - \sum_{m=1}^{n_{e_2}} \text{sgn}(v_m^{e_2}) \frac{1 - \text{sgn}(\delta_m^{e_2})}{2} - \sum_{m=1}^{n_{f_1}} \text{sgn}(v_m^{f_1}) \frac{1 - \text{sgn}(\delta_m^{f_1})}{2}
\end{aligned} \tag{S96.4}$$

$$\begin{aligned}
\mathcal{W}_1^{\text{gapped}} = & -2 \sum_{m=1}^{n_{c_2}} \text{sgn}(v_m^{c_2}) \frac{1 - \text{sgn}(\delta_m^{c_2})}{2} + 2 \sum_{m=1}^{n_{f_1}} \text{sgn}(v_m^{f_1}) \frac{1 - \text{sgn}(\delta_m^{f_1})}{2} + \sum_{m=1}^{n_{g_1}} \text{sgn}(v_m^{g_1}) \frac{1 - \text{sgn}(\delta_m^{g_1})}{2} \\
& + \sum_{m=1}^{n_{g_2}} \text{sgn}(v_m^{g_2}) \frac{1 - \text{sgn}(\delta_m^{g_2})}{2} + \sum_{m=1}^{n_{g_3}} \text{sgn}(v_m^{g_3}) \frac{1 - \text{sgn}(\delta_m^{g_3})}{2} + \sum_{m=1}^{n_{g_4}} \text{sgn}(v_m^{g_4}) \frac{1 - \text{sgn}(\delta_m^{g_4})}{2} \\
& - 2 \sum_{m=1}^{n_{i_1}} \text{sgn}(v_m^{i_1}) \frac{1 - \text{sgn}(\delta_m^{i_1})}{2} - 2 \sum_{m=1}^{n_{i_2}} \text{sgn}(v_m^{i_2}) \frac{1 - \text{sgn}(\delta_m^{i_2})}{2}
\end{aligned} \tag{S96.5}$$

$$\begin{aligned} \mathcal{X}_1 = & \sum_{m=1}^{n_{a_2}} \frac{1 - \text{sgn}(\delta_m^{a_2})}{2} + \sum_{m=1}^{n_{e_1}} \frac{1 - \text{sgn}(\delta_m^{e_1})}{2} + \sum_{m=1}^{n_{e_2}} \frac{1 - \text{sgn}(\delta_m^{e_2})}{2} + \sum_{m=1}^{n_{g_1}} \frac{1 - \text{sgn}(\delta_m^{g_1})}{2} + \sum_{m=1}^{n_{g_4}} \frac{1 - \text{sgn}(\delta_m^{g_4})}{2} \\ & + \sum_{m=1}^{n_{i_1}} \frac{1 - \text{sgn}(\delta_m^{i_1})}{2} + \sum_{m=1}^{n_{i_2}} \frac{1 - \text{sgn}(\delta_m^{i_2})}{2} \pmod{2} \end{aligned} \quad (\text{S96.6})$$

$$\begin{aligned} \mathcal{X}_2 = & \sum_{m=1}^{n_{c_2}} \frac{1 - \text{sgn}(\delta_m^{c_2})}{2} + \sum_{m=1}^{n_{e_1}} \frac{1 - \text{sgn}(\delta_m^{e_1})}{2} + \sum_{m=1}^{n_{e_2}} \frac{1 - \text{sgn}(\delta_m^{e_2})}{2} + \sum_{m=1}^{n_{g_1}} \frac{1 - \text{sgn}(\delta_m^{g_1})}{2} + \sum_{m=1}^{n_{g_4}} \frac{1 - \text{sgn}(\delta_m^{g_4})}{2} \\ & + \sum_{m=1}^{n_{i_1}} \frac{1 - \text{sgn}(\delta_m^{i_1})}{2} + \sum_{m=1}^{n_{i_2}} \frac{1 - \text{sgn}(\delta_m^{i_2})}{2} \pmod{2} \end{aligned} \quad (\text{S96.7})$$

$$\begin{aligned} \mathcal{X}_3 = & \sum_{m=1}^{n_{c_2}} \text{sgn}(v_m^{c_2}) \frac{1 - \text{sgn}(\delta_m^{c_2})}{2} - 2 \sum_{m=1}^{n_{e_1}} \text{sgn}(v_m^{e_1}) \frac{1 - \text{sgn}(\delta_m^{e_1})}{2} + 2 \sum_{m=1}^{n_{e_2}} \text{sgn}(v_m^{e_2}) \frac{1 - \text{sgn}(\delta_m^{e_2})}{2} - \sum_{m=1}^{n_{g_1}} \text{sgn}(v_m^{g_1}) \frac{1 - \text{sgn}(\delta_m^{g_1})}{2} \\ & - 2 \sum_{m=1}^{n_{g_3}} \text{sgn}(v_m^{g_3}) \frac{1 - \text{sgn}(\delta_m^{g_3})}{2} + \sum_{m=1}^{n_{g_4}} \text{sgn}(v_m^{g_4}) \frac{1 - \text{sgn}(\delta_m^{g_4})}{2} - 2 \sum_{m=1}^{n_{i_1}} \text{sgn}(v_m^{i_1}) \frac{1 - \text{sgn}(\delta_m^{i_1})}{2} \pmod{4} \end{aligned} \quad (\text{S96.8})$$

### S97. SPACE GROUP NO. 97

| line segment                                          | character of irrep (generators only)                                                                                                                                  |
|-------------------------------------------------------|-----------------------------------------------------------------------------------------------------------------------------------------------------------------------|
| $a \quad (0, 0, t)$                                   | $\{4_{001}   0 \ 0 \ 0\}$<br>$a_1 \quad e^{-\frac{3i\pi}{4}}$<br>$a_2 \quad e^{\frac{3i\pi}{4}}$<br>$a_3 \quad e^{-\frac{i\pi}{4}}$<br>$a_4 \quad e^{\frac{i\pi}{4}}$ |
| $b \quad (\frac{1}{2}, \frac{1}{2}, \frac{t}{2})$     | $\{2_{001}   0 \ 0 \ 0\}$<br>$b_1 \quad -i$<br>$b_2 \quad i$                                                                                                          |
| $c \quad (\frac{t}{2}, \frac{t}{2}, 1 - \frac{t}{2})$ | $\{1   0 \ 0 \ 0\}$<br>$c_1 \quad 1$                                                                                                                                  |
| $d \quad (\frac{t}{2}, \frac{t}{2}, 0)$               | $\{2_{110}   0 \ 0 \ 0\}$<br>$d_1 \quad -i$<br>$d_2 \quad i$                                                                                                          |
| $e \quad (\frac{t}{2}, 1 - \frac{t}{2}, 0)$           | $\{2_{1-10}   0 \ 0 \ 0\}$<br>$e_1 \quad -i$<br>$e_2 \quad i$                                                                                                         |
| $f \quad (\frac{1-t}{2}, \frac{1}{2}, \frac{1}{2})$   | $\{2_{100}   0 \ 0 \ 0\}$<br>$f_1 \quad -i$<br>$f_2 \quad i$                                                                                                          |
| $g \quad (0, t, 0)$                                   | $\{2_{010}   0 \ 0 \ 0\}$<br>$g_1 \quad -i$<br>$g_2 \quad i$                                                                                                          |
| $h \quad (0, \frac{t}{2}, 1 - \frac{t}{2})$           | $\{1   0 \ 0 \ 0\}$<br>$h_1 \quad 1$                                                                                                                                  |

$$\begin{aligned} \mathcal{W}_1^{\text{gapless}} = & \sum_{m=1}^{n_{a_1}} \text{sgn}(v_m^{a_1}) \frac{1 - \text{sgn}(\delta_m^{a_1})}{2} + \sum_{m=1}^{n_{a_2}} \text{sgn}(v_m^{a_2}) \frac{1 - \text{sgn}(\delta_m^{a_2})}{2} + \sum_{m=1}^{n_{a_3}} \text{sgn}(v_m^{a_3}) \frac{1 - \text{sgn}(\delta_m^{a_3})}{2} \\ & + \sum_{m=1}^{n_{a_4}} \text{sgn}(v_m^{a_4}) \frac{1 - \text{sgn}(\delta_m^{a_4})}{2} - \sum_{m=1}^{n_{g_1}} \text{sgn}(v_m^{g_1}) \frac{1 - \text{sgn}(\delta_m^{g_1})}{2} - \sum_{m=1}^{n_{g_2}} \text{sgn}(v_m^{g_2}) \frac{1 - \text{sgn}(\delta_m^{g_2})}{2} \end{aligned} \quad (\text{S97.1})$$

$$\begin{aligned} \mathcal{W}_2^{\text{gapless}} = & \sum_{m=1}^{n_{b_1}} \text{sgn}(v_m^{b_1}) \frac{1 - \text{sgn}(\delta_m^{b_1})}{2} + \sum_{m=1}^{n_{b_2}} \text{sgn}(v_m^{b_2}) \frac{1 - \text{sgn}(\delta_m^{b_2})}{2} + \sum_{m=1}^{n_{e_1}} \text{sgn}(v_m^{e_1}) \frac{1 - \text{sgn}(\delta_m^{e_1})}{2} + \sum_{m=1}^{n_{e_2}} \text{sgn}(v_m^{e_2}) \frac{1 - \text{sgn}(\delta_m^{e_2})}{2} \\ & + \sum_{m=1}^{n_{f_1}} \text{sgn}(v_m^{f_1}) \frac{1 - \text{sgn}(\delta_m^{f_1})}{2} + \sum_{m=1}^{n_{f_2}} \text{sgn}(v_m^{f_2}) \frac{1 - \text{sgn}(\delta_m^{f_2})}{2} - \sum_{m=1}^{n_{h_1}} \text{sgn}(v_m^{h_1}) \frac{1 - \text{sgn}(\delta_m^{h_1})}{2} \end{aligned} \quad (\text{S97.2})$$

$$\mathcal{W}_3^{\text{gapless}} = \sum_{m=1}^{n_{c_1}} \text{sgn}(v_m^{c_1}) \frac{1 - \text{sgn}(\delta_m^{c_1})}{2} + \sum_{m=1}^{n_{f_1}} \text{sgn}(v_m^{f_1}) \frac{1 - \text{sgn}(\delta_m^{f_1})}{2} + \sum_{m=1}^{n_{f_2}} \text{sgn}(v_m^{f_2}) \frac{1 - \text{sgn}(\delta_m^{f_2})}{2} - \sum_{m=1}^{n_{h_1}} \text{sgn}(v_m^{h_1}) \frac{1 - \text{sgn}(\delta_m^{h_1})}{2} \quad (\text{S97.3})$$

$$\begin{aligned} \mathcal{W}_4^{\text{gapless}} = & \sum_{m=1}^{n_{d_1}} \text{sgn}(v_m^{d_1}) \frac{1 - \text{sgn}(\delta_m^{d_1})}{2} + \sum_{m=1}^{n_{d_2}} \text{sgn}(v_m^{d_2}) \frac{1 - \text{sgn}(\delta_m^{d_2})}{2} - \sum_{m=1}^{n_{e_1}} \text{sgn}(v_m^{e_1}) \frac{1 - \text{sgn}(\delta_m^{e_1})}{2} \\ & - \sum_{m=1}^{n_{e_2}} \text{sgn}(v_m^{e_2}) \frac{1 - \text{sgn}(\delta_m^{e_2})}{2} - \sum_{m=1}^{n_{g_1}} \text{sgn}(v_m^{g_1}) \frac{1 - \text{sgn}(\delta_m^{g_1})}{2} - \sum_{m=1}^{n_{g_2}} \text{sgn}(v_m^{g_2}) \frac{1 - \text{sgn}(\delta_m^{g_2})}{2} \end{aligned} \quad (\text{S97.4})$$

$$\mathcal{W}_1^{\text{gapped}} = \sum_{m=1}^{n_{a_2}} \text{sgn}(v_m^{a_2}) \frac{1 - \text{sgn}(\delta_m^{a_2})}{2} + \sum_{m=1}^{n_{a_3}} \text{sgn}(v_m^{a_3}) \frac{1 - \text{sgn}(\delta_m^{a_3})}{2} - \sum_{m=1}^{n_{d_2}} \text{sgn}(v_m^{d_2}) \frac{1 - \text{sgn}(\delta_m^{d_2})}{2} + \sum_{m=1}^{n_{e_1}} \text{sgn}(v_m^{e_1}) \frac{1 - \text{sgn}(\delta_m^{e_1})}{2} \quad (\text{S97.5})$$

$$\mathcal{W}_2^{\text{gapped}} = \sum_{m=1}^{n_{a_2}} \text{sgn}(v_m^{a_2}) \frac{1 - \text{sgn}(\delta_m^{a_2})}{2} + \sum_{m=1}^{n_{a_3}} \text{sgn}(v_m^{a_3}) \frac{1 - \text{sgn}(\delta_m^{a_3})}{2} - \sum_{m=1}^{n_{d_2}} \text{sgn}(v_m^{d_2}) \frac{1 - \text{sgn}(\delta_m^{d_2})}{2} + \sum_{m=1}^{n_{e_2}} \text{sgn}(v_m^{e_2}) \frac{1 - \text{sgn}(\delta_m^{e_2})}{2} \quad (\text{S97.6})$$

$$\mathcal{W}_3^{\text{gapped}} = - \sum_{m=1}^{n_{a_3}} \text{sgn}(v_m^{a_3}) \frac{1 - \text{sgn}(\delta_m^{a_3})}{2} + \sum_{m=1}^{n_{a_4}} \text{sgn}(v_m^{a_4}) \frac{1 - \text{sgn}(\delta_m^{a_4})}{2} \quad (\text{S97.7})$$

$$\mathcal{W}_4^{\text{gapped}} = - \sum_{m=1}^{n_{f_1}} \text{sgn}(v_m^{f_1}) \frac{1 - \text{sgn}(\delta_m^{f_1})}{2} + \sum_{m=1}^{n_{f_2}} \text{sgn}(v_m^{f_2}) \frac{1 - \text{sgn}(\delta_m^{f_2})}{2} \quad (\text{S97.8})$$

$$\mathcal{W}_5^{\text{gapped}} = - \sum_{m=1}^{n_{a_2}} \text{sgn}(v_m^{a_2}) \frac{1 - \text{sgn}(\delta_m^{a_2})}{2} - \sum_{m=1}^{n_{a_3}} \text{sgn}(v_m^{a_3}) \frac{1 - \text{sgn}(\delta_m^{a_3})}{2} + \sum_{m=1}^{n_{g_1}} \text{sgn}(v_m^{g_1}) \frac{1 - \text{sgn}(\delta_m^{g_1})}{2} \quad (\text{S97.9})$$



$$\mathcal{W}_6^{\text{gapped}} = - \sum_{m=1}^{n_{a_2}} \text{sgn}(v_m^{a_2}) \frac{1 - \text{sgn}(\delta_m^{a_2})}{2} - \sum_{m=1}^{n_{a_3}} \text{sgn}(v_m^{a_3}) \frac{1 - \text{sgn}(\delta_m^{a_3})}{2} + \sum_{m=1}^{n_{g_2}} \text{sgn}(v_m^{g_2}) \frac{1 - \text{sgn}(\delta_m^{g_2})}{2} \quad (\text{S97.10})$$

$$\begin{aligned} \mathcal{W}_7^{\text{gapped}} = & 2 \sum_{m=1}^{n_{a_2}} \text{sgn}(v_m^{a_2}) \frac{1 - \text{sgn}(\delta_m^{a_2})}{2} + 2 \sum_{m=1}^{n_{a_3}} \text{sgn}(v_m^{a_3}) \frac{1 - \text{sgn}(\delta_m^{a_3})}{2} - 2 \sum_{m=1}^{n_{b_2}} \text{sgn}(v_m^{b_2}) \frac{1 - \text{sgn}(\delta_m^{b_2})}{2} \\ & - 2 \sum_{m=1}^{n_{d_2}} \text{sgn}(v_m^{d_2}) \frac{1 - \text{sgn}(\delta_m^{d_2})}{2} - 2 \sum_{m=1}^{n_{f_1}} \text{sgn}(v_m^{f_1}) \frac{1 - \text{sgn}(\delta_m^{f_1})}{2} + \sum_{m=1}^{n_{h_1}} \text{sgn}(v_m^{h_1}) \frac{1 - \text{sgn}(\delta_m^{h_1})}{2} \end{aligned} \quad (\text{S97.11})$$

### S98. SPACE GROUP NO. 98

| line segment                                      | character of irrep (generators only)                                                                                                                                                                                                                    |
|---------------------------------------------------|---------------------------------------------------------------------------------------------------------------------------------------------------------------------------------------------------------------------------------------------------------|
| $a \ (0, 0, t)$                                   | $\{4_{001}   0 \ \frac{1}{2} \ \frac{1}{4}\}$<br>$a_1 \ e^{-\frac{1}{2}i\pi t - \frac{3i\pi}{4}}$<br>$a_2 \ e^{\frac{3i\pi}{4} - \frac{i\pi t}{2}}$<br>$a_3 \ e^{-\frac{1}{2}i\pi t - \frac{i\pi}{4}}$<br>$a_4 \ e^{\frac{i\pi}{4} - \frac{i\pi t}{2}}$ |
| $b \ (\frac{1}{2}, \frac{1}{2}, \frac{t}{2})$     | $\{2_{001}   0 \ 0 \ 0\}$<br>$b_1 \ -i$<br>$b_2 \ i$                                                                                                                                                                                                    |
| $c \ (\frac{t}{2}, \frac{t}{2}, 1 - \frac{t}{2})$ | $\{1   0 \ 0 \ 0\}$<br>$c_1 \ 1$                                                                                                                                                                                                                        |
| $d \ (\frac{t}{2}, \frac{t}{2}, 0)$               | $\{2_{110}   0 \ 0 \ 0\}$<br>$d_1 \ -i$<br>$d_2 \ i$                                                                                                                                                                                                    |
| $e \ (\frac{t}{2}, 1 - \frac{t}{2}, 0)$           | $\{2_{1-10}   0 \ 0 \ 0\}$<br>$e_1 \ -i$<br>$e_2 \ i$                                                                                                                                                                                                   |
| $f \ (\frac{1-t}{2}, \frac{1}{2}, \frac{1}{2})$   | $\{2_{100}   0 \ \frac{1}{2} \ \frac{1}{4}\}$<br>$f_1 \ i$<br>$f_2 \ -i$                                                                                                                                                                                |
| $g \ (0, t, 0)$                                   | $\{2_{010}   0 \ \frac{1}{2} \ \frac{1}{4}\}$<br>$g_1 \ -ie^{-i\pi t}$<br>$g_2 \ ie^{-i\pi t}$                                                                                                                                                          |
| $h \ (0, \frac{t}{2}, 1 - \frac{t}{2})$           | $\{1   0 \ 0 \ 0\}$<br>$h_1 \ 1$                                                                                                                                                                                                                        |

$$\begin{aligned} \mathcal{W}_1^{\text{gapless}} = & \sum_{m=1}^{n_{a_1}} \text{sgn}(v_m^{a_1}) \frac{1 - \text{sgn}(\delta_m^{a_1})}{2} + \sum_{m=1}^{n_{a_2}} \text{sgn}(v_m^{a_2}) \frac{1 - \text{sgn}(\delta_m^{a_2})}{2} + \sum_{m=1}^{n_{a_3}} \text{sgn}(v_m^{a_3}) \frac{1 - \text{sgn}(\delta_m^{a_3})}{2} \\ & + \sum_{m=1}^{n_{a_4}} \text{sgn}(v_m^{a_4}) \frac{1 - \text{sgn}(\delta_m^{a_4})}{2} - \sum_{m=1}^{n_{g_1}} \text{sgn}(v_m^{g_1}) \frac{1 - \text{sgn}(\delta_m^{g_1})}{2} - \sum_{m=1}^{n_{g_2}} \text{sgn}(v_m^{g_2}) \frac{1 - \text{sgn}(\delta_m^{g_2})}{2} \end{aligned} \quad (\text{S98.1})$$

$$\begin{aligned} \mathcal{W}_2^{\text{gapless}} = & \sum_{m=1}^{n_{b_1}} \text{sgn}(v_m^{b_1}) \frac{1 - \text{sgn}(\delta_m^{b_1})}{2} + \sum_{m=1}^{n_{b_2}} \text{sgn}(v_m^{b_2}) \frac{1 - \text{sgn}(\delta_m^{b_2})}{2} + \sum_{m=1}^{n_{e_1}} \text{sgn}(v_m^{e_1}) \frac{1 - \text{sgn}(\delta_m^{e_1})}{2} + \sum_{m=1}^{n_{e_2}} \text{sgn}(v_m^{e_2}) \frac{1 - \text{sgn}(\delta_m^{e_2})}{2} \\ & + \sum_{m=1}^{n_{f_1}} \text{sgn}(v_m^{f_1}) \frac{1 - \text{sgn}(\delta_m^{f_1})}{2} + \sum_{m=1}^{n_{f_2}} \text{sgn}(v_m^{f_2}) \frac{1 - \text{sgn}(\delta_m^{f_2})}{2} - \sum_{m=1}^{n_{h_1}} \text{sgn}(v_m^{h_1}) \frac{1 - \text{sgn}(\delta_m^{h_1})}{2} \end{aligned} \quad (\text{S98.2})$$

$$\mathcal{W}_3^{\text{gapless}} = \sum_{m=1}^{n_{c_1}} \text{sgn}(v_m^{c_1}) \frac{1 - \text{sgn}(\delta_m^{c_1})}{2} + \sum_{m=1}^{n_{f_1}} \text{sgn}(v_m^{f_1}) \frac{1 - \text{sgn}(\delta_m^{f_1})}{2} + \sum_{m=1}^{n_{f_2}} \text{sgn}(v_m^{f_2}) \frac{1 - \text{sgn}(\delta_m^{f_2})}{2} - \sum_{m=1}^{n_{h_1}} \text{sgn}(v_m^{h_1}) \frac{1 - \text{sgn}(\delta_m^{h_1})}{2} \quad (\text{S98.3})$$

$$\begin{aligned} \mathcal{W}_4^{\text{gapless}} = & \sum_{m=1}^{n_{d_1}} \text{sgn}(v_m^{d_1}) \frac{1 - \text{sgn}(\delta_m^{d_1})}{2} + \sum_{m=1}^{n_{d_2}} \text{sgn}(v_m^{d_2}) \frac{1 - \text{sgn}(\delta_m^{d_2})}{2} - \sum_{m=1}^{n_{e_1}} \text{sgn}(v_m^{e_1}) \frac{1 - \text{sgn}(\delta_m^{e_1})}{2} \\ & - \sum_{m=1}^{n_{e_2}} \text{sgn}(v_m^{e_2}) \frac{1 - \text{sgn}(\delta_m^{e_2})}{2} - \sum_{m=1}^{n_{g_1}} \text{sgn}(v_m^{g_1}) \frac{1 - \text{sgn}(\delta_m^{g_1})}{2} - \sum_{m=1}^{n_{g_2}} \text{sgn}(v_m^{g_2}) \frac{1 - \text{sgn}(\delta_m^{g_2})}{2} \end{aligned} \quad (\text{S98.4})$$

$$\mathcal{W}_1^{\text{gapped}} = \sum_{m=1}^{n_{a_2}} \text{sgn}(v_m^{a_2}) \frac{1 - \text{sgn}(\delta_m^{a_2})}{2} + \sum_{m=1}^{n_{a_3}} \text{sgn}(v_m^{a_3}) \frac{1 - \text{sgn}(\delta_m^{a_3})}{2} - \sum_{m=1}^{n_{d_2}} \text{sgn}(v_m^{d_2}) \frac{1 - \text{sgn}(\delta_m^{d_2})}{2} + \sum_{m=1}^{n_{e_2}} \text{sgn}(v_m^{e_2}) \frac{1 - \text{sgn}(\delta_m^{e_2})}{2} \quad (\text{S98.5})$$

$$\mathcal{W}_2^{\text{gapped}} = - \sum_{m=1}^{n_{a_2}} \text{sgn}(v_m^{a_2}) \frac{1 - \text{sgn}(\delta_m^{a_2})}{2} - \sum_{m=1}^{n_{a_3}} \text{sgn}(v_m^{a_3}) \frac{1 - \text{sgn}(\delta_m^{a_3})}{2} + \sum_{m=1}^{n_{g_1}} \text{sgn}(v_m^{g_1}) \frac{1 - \text{sgn}(\delta_m^{g_1})}{2} \quad (\text{S98.6})$$

$$\mathcal{W}_3^{\text{gapped}} = - \sum_{m=1}^{n_{a_2}} \text{sgn}(v_m^{a_2}) \frac{1 - \text{sgn}(\delta_m^{a_2})}{2} - \sum_{m=1}^{n_{a_3}} \text{sgn}(v_m^{a_3}) \frac{1 - \text{sgn}(\delta_m^{a_3})}{2} + \sum_{m=1}^{n_{g_2}} \text{sgn}(v_m^{g_2}) \frac{1 - \text{sgn}(\delta_m^{g_2})}{2} \quad (\text{S98.7})$$

$$\mathcal{W}_4^{\text{gapped}} = \sum_{m=1}^{n_{a_2}} \text{sgn}(v_m^{a_2}) \frac{1 - \text{sgn}(\delta_m^{a_2})}{2} + \sum_{m=1}^{n_{a_3}} \text{sgn}(v_m^{a_3}) \frac{1 - \text{sgn}(\delta_m^{a_3})}{2} - \sum_{m=1}^{n_{d_2}} \text{sgn}(v_m^{d_2}) \frac{1 - \text{sgn}(\delta_m^{d_2})}{2} + \sum_{m=1}^{n_{e_1}} \text{sgn}(v_m^{e_1}) \frac{1 - \text{sgn}(\delta_m^{e_1})}{2} \quad (\text{S98.8})$$

$$\mathcal{X}_1 = \sum_{m=1}^{n_{a_2}} \frac{1 - \text{sgn}(\delta_m^{a_2})}{2} + \sum_{m=1}^{n_{a_4}} \frac{1 - \text{sgn}(\delta_m^{a_4})}{2} + \sum_{m=1}^{n_{b_2}} \frac{1 - \text{sgn}(\delta_m^{b_2})}{2} + \sum_{m=1}^{n_{d_2}} \frac{1 - \text{sgn}(\delta_m^{d_2})}{2} \mod 2 \quad (\text{S98.9})$$

$$\mathcal{X}_2 = \sum_{m=1}^{n_{a_2}} \frac{1 - \text{sgn}(\delta_m^{a_2})}{2} + \sum_{m=1}^{n_{a_4}} \frac{1 - \text{sgn}(\delta_m^{a_4})}{2} + \sum_{m=1}^{n_{b_2}} \frac{1 - \text{sgn}(\delta_m^{b_2})}{2} + \sum_{m=1}^{n_{d_2}} \frac{1 - \text{sgn}(\delta_m^{d_2})}{2} + \sum_{m=1}^{n_{h_1}} \frac{1 - \text{sgn}(\delta_m^{h_1})}{2} \mod 2 \quad (\text{S98.10})$$

### S99. SPACE GROUP NO. 99

|              |                                      |
|--------------|--------------------------------------|
| line segment | character of irrep (generators only) |
|--------------|--------------------------------------|

|                                                     |                                                                                                                                        |
|-----------------------------------------------------|----------------------------------------------------------------------------------------------------------------------------------------|
| $a \quad (0, \frac{t}{2}, 0)$                       | $\begin{array}{c} \{m_{100}  0 \ 0 \ 0 \} \\ a_1 \quad -i \\ a_2 \quad i \end{array}$                                                  |
| $b \quad (\frac{1-t}{2}, \frac{1}{2}, 0)$           | $\begin{array}{c} \{m_{010}  0 \ 0 \ 0 \} \\ b_1 \quad -i \\ b_2 \quad i \end{array}$                                                  |
| $c \quad (\frac{t}{2}, \frac{t}{2}, 0)$             | $\begin{array}{c} \{m_{1-10}  0 \ 0 \ 0 \} \\ c_1 \quad -i \\ c_2 \quad i \end{array}$                                                 |
| $d \quad (0, \frac{t}{2}, \frac{1}{2})$             | $\begin{array}{c} \{m_{100}  0 \ 0 \ 0 \} \\ d_1 \quad -i \\ d_2 \quad i \end{array}$                                                  |
| $e \quad (\frac{1-t}{2}, \frac{1}{2}, \frac{1}{2})$ | $\begin{array}{c} \{m_{010}  0 \ 0 \ 0 \} \\ e_1 \quad -i \\ e_2 \quad i \end{array}$                                                  |
| $f \quad (\frac{t}{2}, \frac{t}{2}, \frac{1}{2})$   | $\begin{array}{c} \{m_{1-10}  0 \ 0 \ 0 \} \\ f_1 \quad -i \\ f_2 \quad i \end{array}$                                                 |
| $g \quad (0, 0, \frac{t}{2})$                       | $\begin{array}{cc} \{4_{001}  0 \ 0 \ 0 \} & \{m_{100}  0 \ 0 \ 0 \} \\ g_1 & -\sqrt{2} \quad 0 \\ g_2 & \sqrt{2} \quad 0 \end{array}$ |
| $h \quad (0, \frac{1}{2}, \frac{t}{2})$             | $\begin{array}{cc} \{2_{001}  0 \ 0 \ 0 \} & \{m_{100}  0 \ 0 \ 0 \} \\ h_1 & 0 \quad 0 \end{array}$                                   |
| $i \quad (\frac{1}{2}, \frac{1}{2}, \frac{t}{2})$   | $\begin{array}{cc} \{4_{001}  0 \ 0 \ 0 \} & \{m_{100}  0 \ 0 \ 0 \} \\ i_1 & -\sqrt{2} \quad 0 \\ i_2 & \sqrt{2} \quad 0 \end{array}$ |

$$\begin{aligned}
\mathcal{W}_1^{\text{gapless}} = & \sum_{m=1}^{n_{a_1}} \text{sgn}(v_m^{a_1}) \frac{1 - \text{sgn}(\delta_m^{a_1})}{2} + \sum_{m=1}^{n_{d_2}} \text{sgn}(v_m^{d_2}) \frac{1 - \text{sgn}(\delta_m^{d_2})}{2} - \sum_{m=1}^{n_{e_1}} \text{sgn}(v_m^{e_1}) \frac{1 - \text{sgn}(\delta_m^{e_1})}{2} \\
& - \sum_{m=1}^{n_{e_2}} \text{sgn}(v_m^{e_2}) \frac{1 - \text{sgn}(\delta_m^{e_2})}{2} - \sum_{m=1}^{n_{f_1}} \text{sgn}(v_m^{f_1}) \frac{1 - \text{sgn}(\delta_m^{f_1})}{2} - \sum_{m=1}^{n_{f_2}} \text{sgn}(v_m^{f_2}) \frac{1 - \text{sgn}(\delta_m^{f_2})}{2} \\
& - \sum_{m=1}^{n_{g_1}} \text{sgn}(v_m^{g_1}) \frac{1 - \text{sgn}(\delta_m^{g_1})}{2} - \sum_{m=1}^{n_{g_2}} \text{sgn}(v_m^{g_2}) \frac{1 - \text{sgn}(\delta_m^{g_2})}{2} + \sum_{m=1}^{n_{h_1}} \text{sgn}(v_m^{h_1}) \frac{1 - \text{sgn}(\delta_m^{h_1})}{2}
\end{aligned} \tag{S99.1}$$

$$\begin{aligned}
\mathcal{W}_2^{\text{gapless}} = & \sum_{m=1}^{n_{a_2}} \text{sgn}(v_m^{a_2}) \frac{1 - \text{sgn}(\delta_m^{a_2})}{2} - \sum_{m=1}^{n_{d_2}} \text{sgn}(v_m^{d_2}) \frac{1 - \text{sgn}(\delta_m^{d_2})}{2} - \sum_{m=1}^{n_{g_1}} \text{sgn}(v_m^{g_1}) \frac{1 - \text{sgn}(\delta_m^{g_1})}{2} \\
& - \sum_{m=1}^{n_{g_2}} \text{sgn}(v_m^{g_2}) \frac{1 - \text{sgn}(\delta_m^{g_2})}{2} + \sum_{m=1}^{n_{h_1}} \text{sgn}(v_m^{h_1}) \frac{1 - \text{sgn}(\delta_m^{h_1})}{2}
\end{aligned} \tag{S99.2}$$

$$\begin{aligned}
\mathcal{W}_3^{\text{gapless}} = & \sum_{m=1}^{n_{b_1}} \text{sgn}(v_m^{b_1}) \frac{1 - \text{sgn}(\delta_m^{b_1})}{2} - \sum_{m=1}^{n_{e_1}} \text{sgn}(v_m^{e_1}) \frac{1 - \text{sgn}(\delta_m^{e_1})}{2} + \sum_{m=1}^{n_{h_1}} \text{sgn}(v_m^{h_1}) \frac{1 - \text{sgn}(\delta_m^{h_1})}{2} \\
& - \sum_{m=1}^{n_{i_1}} \text{sgn}(v_m^{i_1}) \frac{1 - \text{sgn}(\delta_m^{i_1})}{2} - \sum_{m=1}^{n_{i_2}} \text{sgn}(v_m^{i_2}) \frac{1 - \text{sgn}(\delta_m^{i_2})}{2}
\end{aligned} \tag{S99.3}$$

$$\begin{aligned} \mathcal{W}_4^{\text{gapless}} = & \sum_{m=1}^{n_{b_2}} \text{sgn}(v_m^{b_2}) \frac{1 - \text{sgn}(\delta_m^{b_2})}{2} - \sum_{m=1}^{n_{e_2}} \text{sgn}(v_m^{e_2}) \frac{1 - \text{sgn}(\delta_m^{e_2})}{2} + \sum_{m=1}^{n_{h_1}} \text{sgn}(v_m^{h_1}) \frac{1 - \text{sgn}(\delta_m^{h_1})}{2} \\ & - \sum_{m=1}^{n_{i_1}} \text{sgn}(v_m^{i_1}) \frac{1 - \text{sgn}(\delta_m^{i_1})}{2} - \sum_{m=1}^{n_{i_2}} \text{sgn}(v_m^{i_2}) \frac{1 - \text{sgn}(\delta_m^{i_2})}{2} \end{aligned} \quad (\text{S99.4})$$

$$\begin{aligned} \mathcal{W}_5^{\text{gapless}} = & \sum_{m=1}^{n_{c_1}} \text{sgn}(v_m^{c_1}) \frac{1 - \text{sgn}(\delta_m^{c_1})}{2} - \sum_{m=1}^{n_{f_1}} \text{sgn}(v_m^{f_1}) \frac{1 - \text{sgn}(\delta_m^{f_1})}{2} - \sum_{m=1}^{n_{g_1}} \text{sgn}(v_m^{g_1}) \frac{1 - \text{sgn}(\delta_m^{g_1})}{2} \\ & - \sum_{m=1}^{n_{g_2}} \text{sgn}(v_m^{g_2}) \frac{1 - \text{sgn}(\delta_m^{g_2})}{2} + \sum_{m=1}^{n_{i_1}} \text{sgn}(v_m^{i_1}) \frac{1 - \text{sgn}(\delta_m^{i_1})}{2} + \sum_{m=1}^{n_{i_2}} \text{sgn}(v_m^{i_2}) \frac{1 - \text{sgn}(\delta_m^{i_2})}{2} \end{aligned} \quad (\text{S99.5})$$

$$\begin{aligned} \mathcal{W}_6^{\text{gapless}} = & \sum_{m=1}^{n_{c_2}} \text{sgn}(v_m^{c_2}) \frac{1 - \text{sgn}(\delta_m^{c_2})}{2} - \sum_{m=1}^{n_{f_2}} \text{sgn}(v_m^{f_2}) \frac{1 - \text{sgn}(\delta_m^{f_2})}{2} - \sum_{m=1}^{n_{g_1}} \text{sgn}(v_m^{g_1}) \frac{1 - \text{sgn}(\delta_m^{g_1})}{2} \\ & - \sum_{m=1}^{n_{g_2}} \text{sgn}(v_m^{g_2}) \frac{1 - \text{sgn}(\delta_m^{g_2})}{2} + \sum_{m=1}^{n_{i_1}} \text{sgn}(v_m^{i_1}) \frac{1 - \text{sgn}(\delta_m^{i_1})}{2} + \sum_{m=1}^{n_{i_2}} \text{sgn}(v_m^{i_2}) \frac{1 - \text{sgn}(\delta_m^{i_2})}{2} \end{aligned} \quad (\text{S99.6})$$

$$\begin{aligned} \mathcal{W}_7^{\text{gapless}} = & \sum_{m=1}^{n_{d_1}} \text{sgn}(v_m^{d_1}) \frac{1 - \text{sgn}(\delta_m^{d_1})}{2} + \sum_{m=1}^{n_{d_2}} \text{sgn}(v_m^{d_2}) \frac{1 - \text{sgn}(\delta_m^{d_2})}{2} - \sum_{m=1}^{n_{e_1}} \text{sgn}(v_m^{e_1}) \frac{1 - \text{sgn}(\delta_m^{e_1})}{2} \\ & - \sum_{m=1}^{n_{e_2}} \text{sgn}(v_m^{e_2}) \frac{1 - \text{sgn}(\delta_m^{e_2})}{2} - \sum_{m=1}^{n_{f_1}} \text{sgn}(v_m^{f_1}) \frac{1 - \text{sgn}(\delta_m^{f_1})}{2} - \sum_{m=1}^{n_{f_2}} \text{sgn}(v_m^{f_2}) \frac{1 - \text{sgn}(\delta_m^{f_2})}{2} \end{aligned} \quad (\text{S99.7})$$

$$\mathcal{W}_1^{\text{gapped}} = - \sum_{m=1}^{n_{e_1}} \text{sgn}(v_m^{e_1}) \frac{1 - \text{sgn}(\delta_m^{e_1})}{2} + \sum_{m=1}^{n_{e_2}} \text{sgn}(v_m^{e_2}) \frac{1 - \text{sgn}(\delta_m^{e_2})}{2} \quad (\text{S99.8})$$

$$\mathcal{W}_2^{\text{gapped}} = - \sum_{m=1}^{n_{d_2}} \text{sgn}(v_m^{d_2}) \frac{1 - \text{sgn}(\delta_m^{d_2})}{2} + \sum_{m=1}^{n_{e_1}} \text{sgn}(v_m^{e_1}) \frac{1 - \text{sgn}(\delta_m^{e_1})}{2} + \sum_{m=1}^{n_{f_1}} \text{sgn}(v_m^{f_1}) \frac{1 - \text{sgn}(\delta_m^{f_1})}{2} \quad (\text{S99.9})$$

$$\mathcal{W}_3^{\text{gapped}} = - \sum_{m=1}^{n_{d_2}} \text{sgn}(v_m^{d_2}) \frac{1 - \text{sgn}(\delta_m^{d_2})}{2} + \sum_{m=1}^{n_{e_1}} \text{sgn}(v_m^{e_1}) \frac{1 - \text{sgn}(\delta_m^{e_1})}{2} + \sum_{m=1}^{n_{f_2}} \text{sgn}(v_m^{f_2}) \frac{1 - \text{sgn}(\delta_m^{f_2})}{2} \quad (\text{S99.10})$$

### S100. SPACE GROUP NO. 100

|              |                                      |
|--------------|--------------------------------------|
| line segment | character of irrep (generators only) |
|--------------|--------------------------------------|

|                                                     |                                                                                                                                                      |
|-----------------------------------------------------|------------------------------------------------------------------------------------------------------------------------------------------------------|
| $a \quad (0, \frac{t}{2}, 0)$                       | $\begin{matrix} \{m_{100}   \frac{1}{2} \frac{1}{2} 0\} \\ a_1 \quad -ie^{-\frac{1}{2}i\pi t} \\ a_2 \quad ie^{-\frac{1}{2}i\pi t} \end{matrix}$     |
| $b \quad (\frac{1-t}{2}, \frac{1}{2}, 0)$           | $\begin{matrix} \{m_{010}   \frac{1}{2} \frac{1}{2} 0\} \\ b_1 \quad -e^{-\frac{1}{2}i\pi(2-t)} \\ b_2 \quad e^{-\frac{1}{2}i\pi(2-t)} \end{matrix}$ |
| $c \quad (\frac{t}{2}, \frac{t}{2}, 0)$             | $\begin{matrix} \{m_{1-10}   \frac{1}{2} \frac{1}{2} 0\} \\ c_1 \quad -ie^{-i\pi t} \\ c_2 \quad ie^{-i\pi t} \end{matrix}$                          |
| $d \quad (0, \frac{t}{2}, \frac{1}{2})$             | $\begin{matrix} \{m_{100}   \frac{1}{2} \frac{1}{2} 0\} \\ d_1 \quad -ie^{-\frac{1}{2}i\pi t} \\ d_2 \quad ie^{-\frac{1}{2}i\pi t} \end{matrix}$     |
| $e \quad (\frac{1-t}{2}, \frac{1}{2}, \frac{1}{2})$ | $\begin{matrix} \{m_{010}   \frac{1}{2} \frac{1}{2} 0\} \\ e_1 \quad -e^{-\frac{1}{2}i\pi(2-t)} \\ e_2 \quad e^{-\frac{1}{2}i\pi(2-t)} \end{matrix}$ |
| $f \quad (\frac{t}{2}, \frac{t}{2}, \frac{1}{2})$   | $\begin{matrix} \{m_{1-10}   \frac{1}{2} \frac{1}{2} 0\} \\ f_1 \quad -ie^{-i\pi t} \\ f_2 \quad ie^{-i\pi t} \end{matrix}$                          |
| $g \quad (0, 0, \frac{t}{2})$                       | $\begin{matrix} \{4_{001}   0 \ 0 \ 0\} & \{m_{100}   \frac{1}{2} \frac{1}{2} 0\} \\ g_1 & 0 \\ g_2 & 0 \end{matrix}$                                |
| $h \quad (0, \frac{1}{2}, \frac{t}{2})$             | $\begin{matrix} \{2_{001}   0 \ 0 \ 0\} & \{m_{100}   \frac{1}{2} \frac{1}{2} 0\} \\ h_1 & -1 \\ h_2 & 1 \\ h_3 & -1 \\ h_4 & 1 \end{matrix}$        |
| $i \quad (\frac{1}{2}, \frac{1}{2}, \frac{t}{2})$   | $\begin{matrix} \{4_{001}   0 \ 0 \ 0\} & \{m_{100}   \frac{1}{2} \frac{1}{2} 0\} \\ i_1 & 0 \\ i_2 & 0 \end{matrix}$                                |

$$\begin{aligned}
\mathcal{W}_1^{\text{gapless}} = & \sum_{m=1}^{n_{a_1}} \text{sgn}(v_m^{a_1}) \frac{1 - \text{sgn}(\delta_m^{a_1})}{2} + \sum_{m=1}^{n_{d_2}} \text{sgn}(v_m^{d_2}) \frac{1 - \text{sgn}(\delta_m^{d_2})}{2} - 2 \sum_{m=1}^{n_{e_1}} \text{sgn}(v_m^{e_1}) \frac{1 - \text{sgn}(\delta_m^{e_1})}{2} \\
& - \sum_{m=1}^{n_{f_1}} \text{sgn}(v_m^{f_1}) \frac{1 - \text{sgn}(\delta_m^{f_1})}{2} - \sum_{m=1}^{n_{f_2}} \text{sgn}(v_m^{f_2}) \frac{1 - \text{sgn}(\delta_m^{f_2})}{2} - \sum_{m=1}^{n_{g_1}} \text{sgn}(v_m^{g_1}) \frac{1 - \text{sgn}(\delta_m^{g_1})}{2} \\
& - \sum_{m=1}^{n_{g_2}} \text{sgn}(v_m^{g_2}) \frac{1 - \text{sgn}(\delta_m^{g_2})}{2} + \sum_{m=1}^{n_{h_2}} \text{sgn}(v_m^{h_2}) \frac{1 - \text{sgn}(\delta_m^{h_2})}{2} + 2 \sum_{m=1}^{n_{h_3}} \text{sgn}(v_m^{h_3}) \frac{1 - \text{sgn}(\delta_m^{h_3})}{2} \\
& - \sum_{m=1}^{n_{h_4}} \text{sgn}(v_m^{h_4}) \frac{1 - \text{sgn}(\delta_m^{h_4})}{2}
\end{aligned} \tag{S100.1}$$

$$\begin{aligned}
\mathcal{W}_2^{\text{gapless}} = & \sum_{m=1}^{n_{a_2}} \text{sgn}(v_m^{a_2}) \frac{1 - \text{sgn}(\delta_m^{a_2})}{2} - \sum_{m=1}^{n_{d_2}} \text{sgn}(v_m^{d_2}) \frac{1 - \text{sgn}(\delta_m^{d_2})}{2} - \sum_{m=1}^{n_{g_1}} \text{sgn}(v_m^{g_1}) \frac{1 - \text{sgn}(\delta_m^{g_1})}{2} \\
& - \sum_{m=1}^{n_{g_2}} \text{sgn}(v_m^{g_2}) \frac{1 - \text{sgn}(\delta_m^{g_2})}{2} + \sum_{m=1}^{n_{h_2}} \text{sgn}(v_m^{h_2}) \frac{1 - \text{sgn}(\delta_m^{h_2})}{2} + \sum_{m=1}^{n_{h_4}} \text{sgn}(v_m^{h_4}) \frac{1 - \text{sgn}(\delta_m^{h_4})}{2}
\end{aligned} \tag{S100.2}$$

$$\begin{aligned} \mathcal{W}_3^{\text{gapless}} = & \sum_{m=1}^{n_{b_1}} \text{sgn}(v_m^{b_1}) \frac{1 - \text{sgn}(\delta_m^{b_1})}{2} - \sum_{m=1}^{n_{e_1}} \text{sgn}(v_m^{e_1}) \frac{1 - \text{sgn}(\delta_m^{e_1})}{2} + \sum_{m=1}^{n_{h_2}} \text{sgn}(v_m^{h_2}) \frac{1 - \text{sgn}(\delta_m^{h_2})}{2} \\ & + \sum_{m=1}^{n_{h_3}} \text{sgn}(v_m^{h_3}) \frac{1 - \text{sgn}(\delta_m^{h_3})}{2} - \sum_{m=1}^{n_{i_1}} \text{sgn}(v_m^{i_1}) \frac{1 - \text{sgn}(\delta_m^{i_1})}{2} - \sum_{m=1}^{n_{i_2}} \text{sgn}(v_m^{i_2}) \frac{1 - \text{sgn}(\delta_m^{i_2})}{2} \end{aligned} \quad (\text{S100.3})$$

$$\begin{aligned} \mathcal{W}_4^{\text{gapless}} = & \sum_{m=1}^{n_{c_1}} \text{sgn}(v_m^{c_1}) \frac{1 - \text{sgn}(\delta_m^{c_1})}{2} - \sum_{m=1}^{n_{f_1}} \text{sgn}(v_m^{f_1}) \frac{1 - \text{sgn}(\delta_m^{f_1})}{2} - \sum_{m=1}^{n_{g_1}} \text{sgn}(v_m^{g_1}) \frac{1 - \text{sgn}(\delta_m^{g_1})}{2} \\ & - \sum_{m=1}^{n_{g_2}} \text{sgn}(v_m^{g_2}) \frac{1 - \text{sgn}(\delta_m^{g_2})}{2} + \sum_{m=1}^{n_{i_1}} \text{sgn}(v_m^{i_1}) \frac{1 - \text{sgn}(\delta_m^{i_1})}{2} + \sum_{m=1}^{n_{i_2}} \text{sgn}(v_m^{i_2}) \frac{1 - \text{sgn}(\delta_m^{i_2})}{2} \end{aligned} \quad (\text{S100.4})$$

$$\begin{aligned} \mathcal{W}_5^{\text{gapless}} = & \sum_{m=1}^{n_{c_2}} \text{sgn}(v_m^{c_2}) \frac{1 - \text{sgn}(\delta_m^{c_2})}{2} - \sum_{m=1}^{n_{f_2}} \text{sgn}(v_m^{f_2}) \frac{1 - \text{sgn}(\delta_m^{f_2})}{2} - \sum_{m=1}^{n_{g_1}} \text{sgn}(v_m^{g_1}) \frac{1 - \text{sgn}(\delta_m^{g_1})}{2} \\ & - \sum_{m=1}^{n_{g_2}} \text{sgn}(v_m^{g_2}) \frac{1 - \text{sgn}(\delta_m^{g_2})}{2} + \sum_{m=1}^{n_{i_1}} \text{sgn}(v_m^{i_1}) \frac{1 - \text{sgn}(\delta_m^{i_1})}{2} + \sum_{m=1}^{n_{i_2}} \text{sgn}(v_m^{i_2}) \frac{1 - \text{sgn}(\delta_m^{i_2})}{2} \end{aligned} \quad (\text{S100.5})$$

$$\begin{aligned} \mathcal{W}_6^{\text{gapless}} = & \sum_{m=1}^{n_{d_1}} \text{sgn}(v_m^{d_1}) \frac{1 - \text{sgn}(\delta_m^{d_1})}{2} + \sum_{m=1}^{n_{d_2}} \text{sgn}(v_m^{d_2}) \frac{1 - \text{sgn}(\delta_m^{d_2})}{2} - 2 \sum_{m=1}^{n_{e_1}} \text{sgn}(v_m^{e_1}) \frac{1 - \text{sgn}(\delta_m^{e_1})}{2} \\ & - \sum_{m=1}^{n_{f_1}} \text{sgn}(v_m^{f_1}) \frac{1 - \text{sgn}(\delta_m^{f_1})}{2} - \sum_{m=1}^{n_{f_2}} \text{sgn}(v_m^{f_2}) \frac{1 - \text{sgn}(\delta_m^{f_2})}{2} \end{aligned} \quad (\text{S100.6})$$

$$\mathcal{W}_7^{\text{gapless}} = \sum_{m=1}^{n_{h_1}} \text{sgn}(v_m^{h_1}) \frac{1 - \text{sgn}(\delta_m^{h_1})}{2} - \sum_{m=1}^{n_{h_2}} \text{sgn}(v_m^{h_2}) \frac{1 - \text{sgn}(\delta_m^{h_2})}{2} - \sum_{m=1}^{n_{h_3}} \text{sgn}(v_m^{h_3}) \frac{1 - \text{sgn}(\delta_m^{h_3})}{2} + \sum_{m=1}^{n_{h_4}} \text{sgn}(v_m^{h_4}) \frac{1 - \text{sgn}(\delta_m^{h_4})}{2} \quad (\text{S100.7})$$

$$\mathcal{W}_1^{\text{gapped}} = - \sum_{m=1}^{n_{h_2}} \text{sgn}(v_m^{h_2}) \frac{1 - \text{sgn}(\delta_m^{h_2})}{2} + \sum_{m=1}^{n_{h_4}} \text{sgn}(v_m^{h_4}) \frac{1 - \text{sgn}(\delta_m^{h_4})}{2} \quad (\text{S100.8})$$

$$\mathcal{W}_2^{\text{gapped}} = \sum_{m=1}^{n_{f_1}} \text{sgn}(v_m^{f_1}) \frac{1 - \text{sgn}(\delta_m^{f_1})}{2} - \sum_{m=1}^{n_{f_2}} \text{sgn}(v_m^{f_2}) \frac{1 - \text{sgn}(\delta_m^{f_2})}{2} \quad (\text{S100.9})$$

$$\mathcal{W}_3^{\text{gapped}} = - \sum_{m=1}^{n_{i_1}} \text{sgn}(v_m^{i_1}) \frac{1 - \text{sgn}(\delta_m^{i_1})}{2} + \sum_{m=1}^{n_{i_2}} \text{sgn}(v_m^{i_2}) \frac{1 - \text{sgn}(\delta_m^{i_2})}{2} \quad (\text{S100.10})$$

$$\mathcal{X}_1 = \sum_{m=1}^{n_{d_2}} \frac{1 - \text{sgn}(\delta_m^{d_2})}{2} + \sum_{m=1}^{n_{f_2}} \frac{1 - \text{sgn}(\delta_m^{f_2})}{2} \quad \text{mod } 2 \quad (\text{S100.11})$$

## S101. SPACE GROUP NO. 101

| line segment                                    | character of irrep (generators only)                                                                                                                                                 |
|-------------------------------------------------|--------------------------------------------------------------------------------------------------------------------------------------------------------------------------------------|
| $a \ (0, \frac{t}{2}, 0)$                       | $\{m_{100}   0 \ 0 \ \frac{1}{2}\}$<br>$a_1 \quad -i$<br>$a_2 \quad i$                                                                                                               |
| $b \ (\frac{1-t}{2}, \frac{1}{2}, 0)$           | $\{m_{010}   0 \ 0 \ \frac{1}{2}\}$<br>$b_1 \quad -i$<br>$b_2 \quad i$                                                                                                               |
| $c \ (\frac{t}{2}, \frac{t}{2}, 0)$             | $\{m_{1-10}   0 \ 0 \ 0\}$<br>$c_1 \quad -i$<br>$c_2 \quad i$                                                                                                                        |
| $d \ (0, \frac{t}{2}, \frac{1}{2})$             | $\{m_{100}   0 \ 0 \ \frac{1}{2}\}$<br>$d_1 \quad -1$<br>$d_2 \quad 1$                                                                                                               |
| $e \ (\frac{1-t}{2}, \frac{1}{2}, \frac{1}{2})$ | $\{m_{010}   0 \ 0 \ \frac{1}{2}\}$<br>$e_1 \quad -1$<br>$e_2 \quad 1$                                                                                                               |
| $f \ (\frac{t}{2}, \frac{t}{2}, \frac{1}{2})$   | $\{m_{1-10}   0 \ 0 \ 0\}$<br>$f_1 \quad -i$<br>$f_2 \quad i$                                                                                                                        |
| $g \ (0, 0, \frac{t}{2})$                       | $\{4_{001}   0 \ 0 \ \frac{1}{2}\} \ \{m_{100}   0 \ 0 \ \frac{1}{2}\}$<br>$g_1 \quad -\sqrt{2}e^{-\frac{1}{2}i\pi t} \quad 0$<br>$g_2 \quad \sqrt{2}e^{-\frac{1}{2}i\pi t} \quad 0$ |
| $h \ (0, \frac{1}{2}, \frac{t}{2})$             | $\{2_{001}   0 \ 0 \ 0\} \ \{m_{100}   0 \ 0 \ \frac{1}{2}\}$<br>$h_1 \quad 0 \quad 0$                                                                                               |
| $i \ (\frac{1}{2}, \frac{1}{2}, \frac{t}{2})$   | $\{4_{001}   0 \ 0 \ \frac{1}{2}\} \ \{m_{100}   0 \ 0 \ \frac{1}{2}\}$<br>$i_1 \quad -\sqrt{2}e^{-\frac{1}{2}i\pi t} \quad 0$<br>$i_2 \quad \sqrt{2}e^{-\frac{1}{2}i\pi t} \quad 0$ |

$$\begin{aligned}
\mathcal{W}_1^{\text{gapless}} = & \sum_{m=1}^{n_{a_1}} \text{sgn}(v_m^{a_1}) \frac{1 - \text{sgn}(\delta_m^{a_1})}{2} + \sum_{m=1}^{n_{d_1}} \text{sgn}(v_m^{d_1}) \frac{1 - \text{sgn}(\delta_m^{d_1})}{2} - 2 \sum_{m=1}^{n_{e_1}} \text{sgn}(v_m^{e_1}) \frac{1 - \text{sgn}(\delta_m^{e_1})}{2} \\
& - \sum_{m=1}^{n_{f_1}} \text{sgn}(v_m^{f_1}) \frac{1 - \text{sgn}(\delta_m^{f_1})}{2} - \sum_{m=1}^{n_{f_2}} \text{sgn}(v_m^{f_2}) \frac{1 - \text{sgn}(\delta_m^{f_2})}{2} - \sum_{m=1}^{n_{g_1}} \text{sgn}(v_m^{g_1}) \frac{1 - \text{sgn}(\delta_m^{g_1})}{2} \\
& - \sum_{m=1}^{n_{g_2}} \text{sgn}(v_m^{g_2}) \frac{1 - \text{sgn}(\delta_m^{g_2})}{2} + \sum_{m=1}^{n_{h_1}} \text{sgn}(v_m^{h_1}) \frac{1 - \text{sgn}(\delta_m^{h_1})}{2}
\end{aligned} \tag{S101.1}$$

$$\begin{aligned}
\mathcal{W}_2^{\text{gapless}} = & \sum_{m=1}^{n_{a_2}} \text{sgn}(v_m^{a_2}) \frac{1 - \text{sgn}(\delta_m^{a_2})}{2} + \sum_{m=1}^{n_{d_1}} \text{sgn}(v_m^{d_1}) \frac{1 - \text{sgn}(\delta_m^{d_1})}{2} - 2 \sum_{m=1}^{n_{e_1}} \text{sgn}(v_m^{e_1}) \frac{1 - \text{sgn}(\delta_m^{e_1})}{2} \\
& - \sum_{m=1}^{n_{f_1}} \text{sgn}(v_m^{f_1}) \frac{1 - \text{sgn}(\delta_m^{f_1})}{2} - \sum_{m=1}^{n_{f_2}} \text{sgn}(v_m^{f_2}) \frac{1 - \text{sgn}(\delta_m^{f_2})}{2} - \sum_{m=1}^{n_{g_1}} \text{sgn}(v_m^{g_1}) \frac{1 - \text{sgn}(\delta_m^{g_1})}{2} \\
& - \sum_{m=1}^{n_{g_2}} \text{sgn}(v_m^{g_2}) \frac{1 - \text{sgn}(\delta_m^{g_2})}{2} + \sum_{m=1}^{n_{h_1}} \text{sgn}(v_m^{h_1}) \frac{1 - \text{sgn}(\delta_m^{h_1})}{2}
\end{aligned} \tag{S101.2}$$

$$\begin{aligned}
\mathcal{W}_3^{\text{gapless}} = & \sum_{m=1}^{n_{b_1}} \text{sgn}(v_m^{b_1}) \frac{1 - \text{sgn}(\delta_m^{b_1})}{2} - \sum_{m=1}^{n_{e_1}} \text{sgn}(v_m^{e_1}) \frac{1 - \text{sgn}(\delta_m^{e_1})}{2} + \sum_{m=1}^{n_{h_1}} \text{sgn}(v_m^{h_1}) \frac{1 - \text{sgn}(\delta_m^{h_1})}{2} \\
& - \sum_{m=1}^{n_{i_1}} \text{sgn}(v_m^{i_1}) \frac{1 - \text{sgn}(\delta_m^{i_1})}{2} - \sum_{m=1}^{n_{i_2}} \text{sgn}(v_m^{i_2}) \frac{1 - \text{sgn}(\delta_m^{i_2})}{2}
\end{aligned} \tag{S101.3}$$

$$\begin{aligned} \mathcal{W}_4^{\text{gapless}} = & \sum_{m=1}^{n_{b_2}} \text{sgn}(v_m^{b_2}) \frac{1 - \text{sgn}(\delta_m^{b_2})}{2} - \sum_{m=1}^{n_{e_1}} \text{sgn}(v_m^{e_1}) \frac{1 - \text{sgn}(\delta_m^{e_1})}{2} + \sum_{m=1}^{n_{h_1}} \text{sgn}(v_m^{h_1}) \frac{1 - \text{sgn}(\delta_m^{h_1})}{2} \\ & - \sum_{m=1}^{n_{i_1}} \text{sgn}(v_m^{i_1}) \frac{1 - \text{sgn}(\delta_m^{i_1})}{2} - \sum_{m=1}^{n_{i_2}} \text{sgn}(v_m^{i_2}) \frac{1 - \text{sgn}(\delta_m^{i_2})}{2} \end{aligned} \quad (\text{S101.4})$$

$$\begin{aligned} \mathcal{W}_5^{\text{gapless}} = & \sum_{m=1}^{n_{c_1}} \text{sgn}(v_m^{c_1}) \frac{1 - \text{sgn}(\delta_m^{c_1})}{2} - \sum_{m=1}^{n_{f_1}} \text{sgn}(v_m^{f_1}) \frac{1 - \text{sgn}(\delta_m^{f_1})}{2} - \sum_{m=1}^{n_{g_1}} \text{sgn}(v_m^{g_1}) \frac{1 - \text{sgn}(\delta_m^{g_1})}{2} \\ & - \sum_{m=1}^{n_{g_2}} \text{sgn}(v_m^{g_2}) \frac{1 - \text{sgn}(\delta_m^{g_2})}{2} + \sum_{m=1}^{n_{i_1}} \text{sgn}(v_m^{i_1}) \frac{1 - \text{sgn}(\delta_m^{i_1})}{2} + \sum_{m=1}^{n_{i_2}} \text{sgn}(v_m^{i_2}) \frac{1 - \text{sgn}(\delta_m^{i_2})}{2} \end{aligned} \quad (\text{S101.5})$$

$$\begin{aligned} \mathcal{W}_6^{\text{gapless}} = & \sum_{m=1}^{n_{c_2}} \text{sgn}(v_m^{c_2}) \frac{1 - \text{sgn}(\delta_m^{c_2})}{2} - \sum_{m=1}^{n_{f_2}} \text{sgn}(v_m^{f_2}) \frac{1 - \text{sgn}(\delta_m^{f_2})}{2} - \sum_{m=1}^{n_{g_1}} \text{sgn}(v_m^{g_1}) \frac{1 - \text{sgn}(\delta_m^{g_1})}{2} \\ & - \sum_{m=1}^{n_{g_2}} \text{sgn}(v_m^{g_2}) \frac{1 - \text{sgn}(\delta_m^{g_2})}{2} + \sum_{m=1}^{n_{i_1}} \text{sgn}(v_m^{i_1}) \frac{1 - \text{sgn}(\delta_m^{i_1})}{2} + \sum_{m=1}^{n_{i_2}} \text{sgn}(v_m^{i_2}) \frac{1 - \text{sgn}(\delta_m^{i_2})}{2} \end{aligned} \quad (\text{S101.6})$$

$$\begin{aligned} \mathcal{W}_7^{\text{gapless}} = & 2 \sum_{m=1}^{n_{d_1}} \text{sgn}(v_m^{d_1}) \frac{1 - \text{sgn}(\delta_m^{d_1})}{2} - 2 \sum_{m=1}^{n_{e_1}} \text{sgn}(v_m^{e_1}) \frac{1 - \text{sgn}(\delta_m^{e_1})}{2} - \sum_{m=1}^{n_{f_1}} \text{sgn}(v_m^{f_1}) \frac{1 - \text{sgn}(\delta_m^{f_1})}{2} \\ & - \sum_{m=1}^{n_{f_2}} \text{sgn}(v_m^{f_2}) \frac{1 - \text{sgn}(\delta_m^{f_2})}{2} \end{aligned} \quad (\text{S101.7})$$

$$\mathcal{W}_1^{\text{gapped}} = - \sum_{m=1}^{n_{d_1}} \text{sgn}(v_m^{d_1}) \frac{1 - \text{sgn}(\delta_m^{d_1})}{2} + \sum_{m=1}^{n_{e_1}} \text{sgn}(v_m^{e_1}) \frac{1 - \text{sgn}(\delta_m^{e_1})}{2} + \sum_{m=1}^{n_{f_2}} \text{sgn}(v_m^{f_2}) \frac{1 - \text{sgn}(\delta_m^{f_2})}{2} \quad (\text{S101.8})$$

$$\mathcal{X}_1 = \sum_{m=1}^{n_{f_1}} \frac{1 - \text{sgn}(\delta_m^{f_1})}{2} \mod 2 \quad (\text{S101.9})$$

$$\mathcal{X}_2 = \sum_{m=1}^{n_{e_1}} \frac{1 - \text{sgn}(\delta_m^{e_1})}{2} \mod 2 \quad (\text{S101.10})$$

## S102. SPACE GROUP NO. 102

|              |                                      |
|--------------|--------------------------------------|
| line segment | character of irrep (generators only) |
|--------------|--------------------------------------|



|                                                     |                                                                                                                                                                                                                                                                                               |
|-----------------------------------------------------|-----------------------------------------------------------------------------------------------------------------------------------------------------------------------------------------------------------------------------------------------------------------------------------------------|
| $a \quad (0, \frac{t}{2}, 0)$                       | $\{m_{100}   \frac{1}{2} \frac{1}{2} \frac{1}{2}\}$<br>$a_1 \quad -ie^{-\frac{1}{2}i\pi t}$<br>$a_2 \quad ie^{-\frac{1}{2}i\pi t}$                                                                                                                                                            |
| $b \quad (\frac{1-t}{2}, \frac{1}{2}, 0)$           | $\{m_{010}   \frac{1}{2} \frac{1}{2} \frac{1}{2}\}$<br>$b_1 \quad -e^{-\frac{1}{2}i\pi(2-t)}$<br>$b_2 \quad e^{-\frac{1}{2}i\pi(2-t)}$                                                                                                                                                        |
| $c \quad (\frac{t}{2}, \frac{t}{2}, 0)$             | $\{m_{1-10}   0 \ 0 \ 0\}$<br>$c_1 \quad -i$<br>$c_2 \quad i$                                                                                                                                                                                                                                 |
| $d \quad (0, \frac{t}{2}, \frac{1}{2})$             | $\{m_{100}   \frac{1}{2} \frac{1}{2} \frac{1}{2}\}$<br>$d_1 \quad -ie^{-\frac{1}{2}i\pi(t+1)}$<br>$d_2 \quad ie^{-\frac{1}{2}i\pi(t+1)}$                                                                                                                                                      |
| $e \quad (\frac{1-t}{2}, \frac{1}{2}, \frac{1}{2})$ | $\{m_{010}   \frac{1}{2} \frac{1}{2} \frac{1}{2}\}$<br>$e_1 \quad -e^{-\frac{1}{2}i\pi(3-t)}$<br>$e_2 \quad e^{-\frac{1}{2}i\pi(3-t)}$                                                                                                                                                        |
| $f \quad (\frac{t}{2}, \frac{t}{2}, \frac{1}{2})$   | $\{m_{1-10}   0 \ 0 \ 0\}$<br>$f_1 \quad -i$<br>$f_2 \quad i$                                                                                                                                                                                                                                 |
| $g \quad (0, 0, \frac{t}{2})$                       | $\{4_{001}   \frac{1}{2} \frac{1}{2} \frac{1}{2}\} \quad \{m_{100}   \frac{1}{2} \frac{1}{2} \frac{1}{2}\}$<br>$g_1 \quad -\sqrt{2}e^{-\frac{1}{2}i\pi t} \quad 0$<br>$g_2 \quad \sqrt{2}e^{-\frac{1}{2}i\pi t} \quad 0$                                                                      |
| $h \quad (0, \frac{1}{2}, \frac{t}{2})$             | $\{2_{001}   0 \ 0 \ 0\} \quad \{m_{100}   \frac{1}{2} \frac{1}{2} \frac{1}{2}\}$<br>$h_1 \quad -i \quad -ie^{-\frac{1}{2}i\pi(t+1)}$<br>$h_2 \quad -i \quad ie^{-\frac{1}{2}i\pi(t+1)}$<br>$h_3 \quad i \quad -ie^{-\frac{1}{2}i\pi(t+1)}$<br>$h_4 \quad i \quad ie^{-\frac{1}{2}i\pi(t+1)}$ |
| $i \quad (\frac{1}{2}, \frac{1}{2}, \frac{t}{2})$   | $\{4_{001}   \frac{1}{2} \frac{1}{2} \frac{1}{2}\} \quad \{m_{100}   \frac{1}{2} \frac{1}{2} \frac{1}{2}\}$<br>$i_1 \quad -i\sqrt{2}e^{-\frac{1}{2}i\pi(t+2)} \quad 0$<br>$i_2 \quad i\sqrt{2}e^{-\frac{1}{2}i\pi(t+2)} \quad 0$                                                              |

$$\begin{aligned}
\mathcal{W}_1^{\text{gapless}} = & \sum_{m=1}^{n_{a_1}} \text{sgn}(v_m^{a_1}) \frac{1 - \text{sgn}(\delta_m^{a_1})}{2} + \sum_{m=1}^{n_{d_1}} \text{sgn}(v_m^{d_1}) \frac{1 - \text{sgn}(\delta_m^{d_1})}{2} - 2 \sum_{m=1}^{n_{e_2}} \text{sgn}(v_m^{e_2}) \frac{1 - \text{sgn}(\delta_m^{e_2})}{2} \\
& - \sum_{m=1}^{n_{f_1}} \text{sgn}(v_m^{f_1}) \frac{1 - \text{sgn}(\delta_m^{f_1})}{2} - \sum_{m=1}^{n_{f_2}} \text{sgn}(v_m^{f_2}) \frac{1 - \text{sgn}(\delta_m^{f_2})}{2} - \sum_{m=1}^{n_{g_1}} \text{sgn}(v_m^{g_1}) \frac{1 - \text{sgn}(\delta_m^{g_1})}{2} \\
& - \sum_{m=1}^{n_{g_2}} \text{sgn}(v_m^{g_2}) \frac{1 - \text{sgn}(\delta_m^{g_2})}{2} + 2 \sum_{m=1}^{n_{h_1}} \text{sgn}(v_m^{h_1}) \frac{1 - \text{sgn}(\delta_m^{h_1})}{2} - \sum_{m=1}^{n_{h_2}} \text{sgn}(v_m^{h_2}) \frac{1 - \text{sgn}(\delta_m^{h_2})}{2} \\
& + \sum_{m=1}^{n_{h_4}} \text{sgn}(v_m^{h_4}) \frac{1 - \text{sgn}(\delta_m^{h_4})}{2}
\end{aligned} \tag{S102.1}$$

$$\begin{aligned}
\mathcal{W}_2^{\text{gapless}} = & \sum_{m=1}^{n_{a_2}} \text{sgn}(v_m^{a_2}) \frac{1 - \text{sgn}(\delta_m^{a_2})}{2} + \sum_{m=1}^{n_{d_1}} \text{sgn}(v_m^{d_1}) \frac{1 - \text{sgn}(\delta_m^{d_1})}{2} - 2 \sum_{m=1}^{n_{e_2}} \text{sgn}(v_m^{e_2}) \frac{1 - \text{sgn}(\delta_m^{e_2})}{2} \\
& - \sum_{m=1}^{n_{f_1}} \text{sgn}(v_m^{f_1}) \frac{1 - \text{sgn}(\delta_m^{f_1})}{2} - \sum_{m=1}^{n_{f_2}} \text{sgn}(v_m^{f_2}) \frac{1 - \text{sgn}(\delta_m^{f_2})}{2} - \sum_{m=1}^{n_{g_1}} \text{sgn}(v_m^{g_1}) \frac{1 - \text{sgn}(\delta_m^{g_1})}{2} \\
& - \sum_{m=1}^{n_{g_2}} \text{sgn}(v_m^{g_2}) \frac{1 - \text{sgn}(\delta_m^{g_2})}{2} + \sum_{m=1}^{n_{h_1}} \text{sgn}(v_m^{h_1}) \frac{1 - \text{sgn}(\delta_m^{h_1})}{2} - \sum_{m=1}^{n_{h_3}} \text{sgn}(v_m^{h_3}) \frac{1 - \text{sgn}(\delta_m^{h_3})}{2} \\
& + 2 \sum_{m=1}^{n_{h_4}} \text{sgn}(v_m^{h_4}) \frac{1 - \text{sgn}(\delta_m^{h_4})}{2}
\end{aligned} \tag{S102.2}$$

$$\begin{aligned} \mathcal{W}_3^{\text{gapless}} = & \sum_{m=1}^{n_{b_1}} \text{sgn}(v_m^{b_1}) \frac{1 - \text{sgn}(\delta_m^{b_1})}{2} - \sum_{m=1}^{n_{e_2}} \text{sgn}(v_m^{e_2}) \frac{1 - \text{sgn}(\delta_m^{e_2})}{2} + \sum_{m=1}^{n_{h_1}} \text{sgn}(v_m^{h_1}) \frac{1 - \text{sgn}(\delta_m^{h_1})}{2} \\ & + \sum_{m=1}^{n_{h_4}} \text{sgn}(v_m^{h_4}) \frac{1 - \text{sgn}(\delta_m^{h_4})}{2} - \sum_{m=1}^{n_{i_1}} \text{sgn}(v_m^{i_1}) \frac{1 - \text{sgn}(\delta_m^{i_1})}{2} - \sum_{m=1}^{n_{i_2}} \text{sgn}(v_m^{i_2}) \frac{1 - \text{sgn}(\delta_m^{i_2})}{2} \end{aligned} \quad (\text{S102.3})$$

$$\begin{aligned} \mathcal{W}_4^{\text{gapless}} = & \sum_{m=1}^{n_{c_1}} \text{sgn}(v_m^{c_1}) \frac{1 - \text{sgn}(\delta_m^{c_1})}{2} - \sum_{m=1}^{n_{f_1}} \text{sgn}(v_m^{f_1}) \frac{1 - \text{sgn}(\delta_m^{f_1})}{2} - \sum_{m=1}^{n_{g_1}} \text{sgn}(v_m^{g_1}) \frac{1 - \text{sgn}(\delta_m^{g_1})}{2} \\ & - \sum_{m=1}^{n_{g_2}} \text{sgn}(v_m^{g_2}) \frac{1 - \text{sgn}(\delta_m^{g_2})}{2} + \sum_{m=1}^{n_{i_1}} \text{sgn}(v_m^{i_1}) \frac{1 - \text{sgn}(\delta_m^{i_1})}{2} + \sum_{m=1}^{n_{i_2}} \text{sgn}(v_m^{i_2}) \frac{1 - \text{sgn}(\delta_m^{i_2})}{2} \end{aligned} \quad (\text{S102.4})$$

$$\begin{aligned} \mathcal{W}_5^{\text{gapless}} = & \sum_{m=1}^{n_{c_2}} \text{sgn}(v_m^{c_2}) \frac{1 - \text{sgn}(\delta_m^{c_2})}{2} - \sum_{m=1}^{n_{f_2}} \text{sgn}(v_m^{f_2}) \frac{1 - \text{sgn}(\delta_m^{f_2})}{2} - \sum_{m=1}^{n_{g_1}} \text{sgn}(v_m^{g_1}) \frac{1 - \text{sgn}(\delta_m^{g_1})}{2} \\ & - \sum_{m=1}^{n_{g_2}} \text{sgn}(v_m^{g_2}) \frac{1 - \text{sgn}(\delta_m^{g_2})}{2} + \sum_{m=1}^{n_{i_1}} \text{sgn}(v_m^{i_1}) \frac{1 - \text{sgn}(\delta_m^{i_1})}{2} + \sum_{m=1}^{n_{i_2}} \text{sgn}(v_m^{i_2}) \frac{1 - \text{sgn}(\delta_m^{i_2})}{2} \end{aligned} \quad (\text{S102.5})$$

$$\begin{aligned} \mathcal{W}_6^{\text{gapless}} = & 2 \sum_{m=1}^{n_{d_1}} \text{sgn}(v_m^{d_1}) \frac{1 - \text{sgn}(\delta_m^{d_1})}{2} - 2 \sum_{m=1}^{n_{e_2}} \text{sgn}(v_m^{e_2}) \frac{1 - \text{sgn}(\delta_m^{e_2})}{2} - \sum_{m=1}^{n_{f_1}} \text{sgn}(v_m^{f_1}) \frac{1 - \text{sgn}(\delta_m^{f_1})}{2} \\ & - \sum_{m=1}^{n_{f_2}} \text{sgn}(v_m^{f_2}) \frac{1 - \text{sgn}(\delta_m^{f_2})}{2} + \sum_{m=1}^{n_{h_1}} \text{sgn}(v_m^{h_1}) \frac{1 - \text{sgn}(\delta_m^{h_1})}{2} - \sum_{m=1}^{n_{h_2}} \text{sgn}(v_m^{h_2}) \frac{1 - \text{sgn}(\delta_m^{h_2})}{2} \\ & - \sum_{m=1}^{n_{h_3}} \text{sgn}(v_m^{h_3}) \frac{1 - \text{sgn}(\delta_m^{h_3})}{2} + \sum_{m=1}^{n_{h_4}} \text{sgn}(v_m^{h_4}) \frac{1 - \text{sgn}(\delta_m^{h_4})}{2} \end{aligned} \quad (\text{S102.6})$$

$$\begin{aligned} \mathcal{W}_7^{\text{gapless}} = & \sum_{m=1}^{n_{e_1}} \text{sgn}(v_m^{e_1}) \frac{1 - \text{sgn}(\delta_m^{e_1})}{2} - \sum_{m=1}^{n_{e_2}} \text{sgn}(v_m^{e_2}) \frac{1 - \text{sgn}(\delta_m^{e_2})}{2} + \sum_{m=1}^{n_{h_1}} \text{sgn}(v_m^{h_1}) \frac{1 - \text{sgn}(\delta_m^{h_1})}{2} \\ & - \sum_{m=1}^{n_{h_2}} \text{sgn}(v_m^{h_2}) \frac{1 - \text{sgn}(\delta_m^{h_2})}{2} - \sum_{m=1}^{n_{h_3}} \text{sgn}(v_m^{h_3}) \frac{1 - \text{sgn}(\delta_m^{h_3})}{2} + \sum_{m=1}^{n_{h_4}} \text{sgn}(v_m^{h_4}) \frac{1 - \text{sgn}(\delta_m^{h_4})}{2} \end{aligned} \quad (\text{S102.7})$$

$$\mathcal{W}_1^{\text{gapped}} = \sum_{m=1}^{n_{f_1}} \text{sgn}(v_m^{f_1}) \frac{1 - \text{sgn}(\delta_m^{f_1})}{2} - \sum_{m=1}^{n_{f_2}} \text{sgn}(v_m^{f_2}) \frac{1 - \text{sgn}(\delta_m^{f_2})}{2} \quad (\text{S102.8})$$

$$\begin{aligned} \mathcal{W}_2^{\text{gapped}} = & - \sum_{m=1}^{n_{d_1}} \text{sgn}(v_m^{d_1}) \frac{1 - \text{sgn}(\delta_m^{d_1})}{2} + \sum_{m=1}^{n_{e_2}} \text{sgn}(v_m^{e_2}) \frac{1 - \text{sgn}(\delta_m^{e_2})}{2} + \sum_{m=1}^{n_{f_2}} \text{sgn}(v_m^{f_2}) \frac{1 - \text{sgn}(\delta_m^{f_2})}{2} \\ & - \sum_{m=1}^{n_{h_1}} \text{sgn}(v_m^{h_1}) \frac{1 - \text{sgn}(\delta_m^{h_1})}{2} + \sum_{m=1}^{n_{h_3}} \text{sgn}(v_m^{h_3}) \frac{1 - \text{sgn}(\delta_m^{h_3})}{2} \end{aligned} \quad (\text{S102.9})$$

$$\mathcal{X}_1 = \sum_{m=1}^{n_{e_2}} \frac{1 - \text{sgn}(\delta_m^{e_2})}{2} + \sum_{m=1}^{n_{f_2}} \frac{1 - \text{sgn}(\delta_m^{f_2})}{2} \mod 2 \quad (\text{S102.10})$$

$$\mathcal{X}_2 = \sum_{m=1}^{n_{f_2}} \frac{1 - \text{sgn}(\delta_m^{f_2})}{2} + \sum_{m=1}^{n_{i_1}} \frac{1 - \text{sgn}(\delta_m^{i_1})}{2} + \sum_{m=1}^{n_{i_2}} \frac{1 - \text{sgn}(\delta_m^{i_2})}{2} \mod 2 \quad (\text{S102.11})$$

### S103. SPACE GROUP NO. 103

| line segment                                        | character of irrep (generators only) |                                     |     |
|-----------------------------------------------------|--------------------------------------|-------------------------------------|-----|
| $a \quad (0, \frac{t}{2}, 0)$                       | $\{m_{100}   0 \ 0 \ \frac{1}{2}\}$  |                                     |     |
|                                                     | $a_1$                                | $-i$                                |     |
|                                                     | $a_2$                                | $i$                                 |     |
| $b \quad (\frac{1-t}{2}, \frac{1}{2}, 0)$           | $\{m_{010}   0 \ 0 \ \frac{1}{2}\}$  |                                     |     |
|                                                     | $b_1$                                | $-i$                                |     |
|                                                     | $b_2$                                | $i$                                 |     |
| $c \quad (\frac{t}{2}, \frac{t}{2}, 0)$             | $\{m_{1-10}   0 \ 0 \ \frac{1}{2}\}$ |                                     |     |
|                                                     | $c_1$                                | $-i$                                |     |
|                                                     | $c_2$                                | $i$                                 |     |
| $d \quad (0, \frac{t}{2}, \frac{1}{2})$             | $\{m_{100}   0 \ 0 \ \frac{1}{2}\}$  |                                     |     |
|                                                     | $d_1$                                | $-1$                                |     |
|                                                     | $d_2$                                | $1$                                 |     |
| $e \quad (\frac{1-t}{2}, \frac{1}{2}, \frac{1}{2})$ | $\{m_{010}   0 \ 0 \ \frac{1}{2}\}$  |                                     |     |
|                                                     | $e_1$                                | $-1$                                |     |
|                                                     | $e_2$                                | $1$                                 |     |
| $f \quad (\frac{t}{2}, \frac{t}{2}, \frac{1}{2})$   | $\{m_{1-10}   0 \ 0 \ \frac{1}{2}\}$ |                                     |     |
|                                                     | $f_1$                                | $-1$                                |     |
|                                                     | $f_2$                                | $1$                                 |     |
| $g \quad (0, 0, \frac{t}{2})$                       | $\{4_{001}   0 \ 0 \ 0\}$            | $\{m_{100}   0 \ 0 \ \frac{1}{2}\}$ |     |
|                                                     | $g_1$                                | $-\sqrt{2}$                         | $0$ |
|                                                     | $g_2$                                | $\sqrt{2}$                          | $0$ |
| $h \quad (0, \frac{1}{2}, \frac{t}{2})$             | $\{2_{001}   0 \ 0 \ 0\}$            | $\{m_{100}   0 \ 0 \ \frac{1}{2}\}$ |     |
|                                                     | $h_1$                                | $0$                                 | $0$ |
| $i \quad (\frac{1}{2}, \frac{1}{2}, \frac{t}{2})$   | $\{4_{001}   0 \ 0 \ 0\}$            | $\{m_{100}   0 \ 0 \ \frac{1}{2}\}$ |     |
|                                                     | $i_1$                                | $-\sqrt{2}$                         | $0$ |
|                                                     | $i_2$                                | $\sqrt{2}$                          | $0$ |

$$\begin{aligned} \mathcal{W}_1^{\text{gapless}} = & \sum_{m=1}^{n_{a_1}} \text{sgn}(v_m^{a_1}) \frac{1 - \text{sgn}(\delta_m^{a_1})}{2} + \sum_{m=1}^{n_{d_1}} \text{sgn}(v_m^{d_1}) \frac{1 - \text{sgn}(\delta_m^{d_1})}{2} - 2 \sum_{m=1}^{n_{e_1}} \text{sgn}(v_m^{e_1}) \frac{1 - \text{sgn}(\delta_m^{e_1})}{2} \\ & - 2 \sum_{m=1}^{n_{f_1}} \text{sgn}(v_m^{f_1}) \frac{1 - \text{sgn}(\delta_m^{f_1})}{2} - \sum_{m=1}^{n_{g_1}} \text{sgn}(v_m^{g_1}) \frac{1 - \text{sgn}(\delta_m^{g_1})}{2} - \sum_{m=1}^{n_{g_2}} \text{sgn}(v_m^{g_2}) \frac{1 - \text{sgn}(\delta_m^{g_2})}{2} \\ & + \sum_{m=1}^{n_{h_1}} \text{sgn}(v_m^{h_1}) \frac{1 - \text{sgn}(\delta_m^{h_1})}{2} \end{aligned} \quad (\text{S103.1})$$

$$\begin{aligned}
\mathcal{W}_2^{\text{gapless}} = & \sum_{m=1}^{n_{a_2}} \text{sgn}(v_m^{a_2}) \frac{1 - \text{sgn}(\delta_m^{a_2})}{2} + \sum_{m=1}^{n_{d_1}} \text{sgn}(v_m^{d_1}) \frac{1 - \text{sgn}(\delta_m^{d_1})}{2} - 2 \sum_{m=1}^{n_{e_1}} \text{sgn}(v_m^{e_1}) \frac{1 - \text{sgn}(\delta_m^{e_1})}{2} \\
& - 2 \sum_{m=1}^{n_{f_1}} \text{sgn}(v_m^{f_1}) \frac{1 - \text{sgn}(\delta_m^{f_1})}{2} - \sum_{m=1}^{n_{g_1}} \text{sgn}(v_m^{g_1}) \frac{1 - \text{sgn}(\delta_m^{g_1})}{2} - \sum_{m=1}^{n_{g_2}} \text{sgn}(v_m^{g_2}) \frac{1 - \text{sgn}(\delta_m^{g_2})}{2} \\
& + \sum_{m=1}^{n_{h_1}} \text{sgn}(v_m^{h_1}) \frac{1 - \text{sgn}(\delta_m^{h_1})}{2}
\end{aligned} \tag{S103.2}$$

$$\begin{aligned}
\mathcal{W}_3^{\text{gapless}} = & \sum_{m=1}^{n_{b_1}} \text{sgn}(v_m^{b_1}) \frac{1 - \text{sgn}(\delta_m^{b_1})}{2} - \sum_{m=1}^{n_{e_1}} \text{sgn}(v_m^{e_1}) \frac{1 - \text{sgn}(\delta_m^{e_1})}{2} + \sum_{m=1}^{n_{h_1}} \text{sgn}(v_m^{h_1}) \frac{1 - \text{sgn}(\delta_m^{h_1})}{2} \\
& - \sum_{m=1}^{n_{i_1}} \text{sgn}(v_m^{i_1}) \frac{1 - \text{sgn}(\delta_m^{i_1})}{2} - \sum_{m=1}^{n_{i_2}} \text{sgn}(v_m^{i_2}) \frac{1 - \text{sgn}(\delta_m^{i_2})}{2}
\end{aligned} \tag{S103.3}$$

$$\begin{aligned}
\mathcal{W}_4^{\text{gapless}} = & \sum_{m=1}^{n_{b_2}} \text{sgn}(v_m^{b_2}) \frac{1 - \text{sgn}(\delta_m^{b_2})}{2} - \sum_{m=1}^{n_{e_1}} \text{sgn}(v_m^{e_1}) \frac{1 - \text{sgn}(\delta_m^{e_1})}{2} + \sum_{m=1}^{n_{h_1}} \text{sgn}(v_m^{h_1}) \frac{1 - \text{sgn}(\delta_m^{h_1})}{2} \\
& - \sum_{m=1}^{n_{i_1}} \text{sgn}(v_m^{i_1}) \frac{1 - \text{sgn}(\delta_m^{i_1})}{2} - \sum_{m=1}^{n_{i_2}} \text{sgn}(v_m^{i_2}) \frac{1 - \text{sgn}(\delta_m^{i_2})}{2}
\end{aligned} \tag{S103.4}$$

$$\begin{aligned}
\mathcal{W}_5^{\text{gapless}} = & \sum_{m=1}^{n_{c_1}} \text{sgn}(v_m^{c_1}) \frac{1 - \text{sgn}(\delta_m^{c_1})}{2} - \sum_{m=1}^{n_{f_1}} \text{sgn}(v_m^{f_1}) \frac{1 - \text{sgn}(\delta_m^{f_1})}{2} - \sum_{m=1}^{n_{g_1}} \text{sgn}(v_m^{g_1}) \frac{1 - \text{sgn}(\delta_m^{g_1})}{2} \\
& - \sum_{m=1}^{n_{g_2}} \text{sgn}(v_m^{g_2}) \frac{1 - \text{sgn}(\delta_m^{g_2})}{2} + \sum_{m=1}^{n_{i_1}} \text{sgn}(v_m^{i_1}) \frac{1 - \text{sgn}(\delta_m^{i_1})}{2} + \sum_{m=1}^{n_{i_2}} \text{sgn}(v_m^{i_2}) \frac{1 - \text{sgn}(\delta_m^{i_2})}{2}
\end{aligned} \tag{S103.5}$$

$$\begin{aligned}
\mathcal{W}_6^{\text{gapless}} = & \sum_{m=1}^{n_{c_2}} \text{sgn}(v_m^{c_2}) \frac{1 - \text{sgn}(\delta_m^{c_2})}{2} - \sum_{m=1}^{n_{f_1}} \text{sgn}(v_m^{f_1}) \frac{1 - \text{sgn}(\delta_m^{f_1})}{2} - \sum_{m=1}^{n_{g_1}} \text{sgn}(v_m^{g_1}) \frac{1 - \text{sgn}(\delta_m^{g_1})}{2} \\
& - \sum_{m=1}^{n_{g_2}} \text{sgn}(v_m^{g_2}) \frac{1 - \text{sgn}(\delta_m^{g_2})}{2} + \sum_{m=1}^{n_{i_1}} \text{sgn}(v_m^{i_1}) \frac{1 - \text{sgn}(\delta_m^{i_1})}{2} + \sum_{m=1}^{n_{i_2}} \text{sgn}(v_m^{i_2}) \frac{1 - \text{sgn}(\delta_m^{i_2})}{2}
\end{aligned} \tag{S103.6}$$

$$\mathcal{W}_7^{\text{gapless}} = \sum_{m=1}^{n_{d_1}} \text{sgn}(v_m^{d_1}) \frac{1 - \text{sgn}(\delta_m^{d_1})}{2} - \sum_{m=1}^{n_{e_1}} \text{sgn}(v_m^{e_1}) \frac{1 - \text{sgn}(\delta_m^{e_1})}{2} - \sum_{m=1}^{n_{f_1}} \text{sgn}(v_m^{f_1}) \frac{1 - \text{sgn}(\delta_m^{f_1})}{2} \tag{S103.7}$$

$$\mathcal{X}_1 = \sum_{m=1}^{n_{f_1}} \frac{1 - \text{sgn}(\delta_m^{f_1})}{2} \mod 2 \tag{S103.8}$$

$$\mathcal{X}_2 = \sum_{m=1}^{n_{e_1}} \frac{1 - \text{sgn}(\delta_m^{e_1})}{2} \mod 2 \tag{S103.9}$$

## S104. SPACE GROUP NO. 104

| line segment                                        | character of irrep (generators only)                                                                                                                                                                                                                                                          |
|-----------------------------------------------------|-----------------------------------------------------------------------------------------------------------------------------------------------------------------------------------------------------------------------------------------------------------------------------------------------|
| $a \quad (0, \frac{t}{2}, 0)$                       | $\{m_{100}   \frac{1}{2} \frac{1}{2} \frac{1}{2}\}$<br>$a_1 \quad -ie^{-\frac{1}{2}i\pi t}$<br>$a_2 \quad ie^{-\frac{1}{2}i\pi t}$                                                                                                                                                            |
| $b \quad (\frac{1-t}{2}, \frac{1}{2}, 0)$           | $\{m_{010}   \frac{1}{2} \frac{1}{2} \frac{1}{2}\}$<br>$b_1 \quad -e^{-\frac{1}{2}i\pi(2-t)}$<br>$b_2 \quad e^{-\frac{1}{2}i\pi(2-t)}$                                                                                                                                                        |
| $c \quad (\frac{t}{2}, \frac{t}{2}, 0)$             | $\{m_{1-10}   \frac{1}{2} \frac{1}{2} \frac{1}{2}\}$<br>$c_1 \quad -ie^{-i\pi t}$<br>$c_2 \quad ie^{-i\pi t}$                                                                                                                                                                                 |
| $d \quad (0, \frac{t}{2}, \frac{1}{2})$             | $\{m_{100}   \frac{1}{2} \frac{1}{2} \frac{1}{2}\}$<br>$d_1 \quad -ie^{-\frac{1}{2}i\pi(t+1)}$<br>$d_2 \quad ie^{-\frac{1}{2}i\pi(t+1)}$                                                                                                                                                      |
| $e \quad (\frac{1-t}{2}, \frac{1}{2}, \frac{1}{2})$ | $\{m_{010}   \frac{1}{2} \frac{1}{2} \frac{1}{2}\}$<br>$e_1 \quad -e^{-\frac{1}{2}i\pi(3-t)}$<br>$e_2 \quad e^{-\frac{1}{2}i\pi(3-t)}$                                                                                                                                                        |
| $f \quad (\frac{t}{2}, \frac{t}{2}, \frac{1}{2})$   | $\{m_{1-10}   \frac{1}{2} \frac{1}{2} \frac{1}{2}\}$<br>$f_1 \quad -ie^{-\frac{1}{2}i\pi(2t+1)}$<br>$f_2 \quad ie^{-\frac{1}{2}i\pi(2t+1)}$                                                                                                                                                   |
| $g \quad (0, 0, \frac{t}{2})$                       | $\{4_{001}   0 \ 0 \ 0\} \quad \{m_{100}   \frac{1}{2} \frac{1}{2} \frac{1}{2}\}$<br>$g_1 \quad -\sqrt{2} \quad 0$<br>$g_2 \quad \sqrt{2} \quad 0$                                                                                                                                            |
| $h \quad (0, \frac{1}{2}, \frac{t}{2})$             | $\{2_{001}   0 \ 0 \ 0\} \quad \{m_{100}   \frac{1}{2} \frac{1}{2} \frac{1}{2}\}$<br>$h_1 \quad -i \quad -ie^{-\frac{1}{2}i\pi(t+1)}$<br>$h_2 \quad -i \quad ie^{-\frac{1}{2}i\pi(t+1)}$<br>$h_3 \quad i \quad -ie^{-\frac{1}{2}i\pi(t+1)}$<br>$h_4 \quad i \quad ie^{-\frac{1}{2}i\pi(t+1)}$ |
| $i \quad (\frac{1}{2}, \frac{1}{2}, \frac{t}{2})$   | $\{4_{001}   0 \ 0 \ 0\} \quad \{m_{100}   \frac{1}{2} \frac{1}{2} \frac{1}{2}\}$<br>$i_1 \quad -i\sqrt{2} \quad 0$<br>$i_2 \quad i\sqrt{2} \quad 0$                                                                                                                                          |

$$\begin{aligned}
\mathcal{W}_1^{\text{gapless}} = & \sum_{m=1}^{n_{a_1}} \text{sgn}(v_m^{a_1}) \frac{1 - \text{sgn}(\delta_m^{a_1})}{2} + \sum_{m=1}^{n_{d_1}} \text{sgn}(v_m^{d_1}) \frac{1 - \text{sgn}(\delta_m^{d_1})}{2} - 2 \sum_{m=1}^{n_{e_2}} \text{sgn}(v_m^{e_2}) \frac{1 - \text{sgn}(\delta_m^{e_2})}{2} \\
& - 2 \sum_{m=1}^{n_{f_1}} \text{sgn}(v_m^{f_1}) \frac{1 - \text{sgn}(\delta_m^{f_1})}{2} - \sum_{m=1}^{n_{g_1}} \text{sgn}(v_m^{g_1}) \frac{1 - \text{sgn}(\delta_m^{g_1})}{2} - \sum_{m=1}^{n_{g_2}} \text{sgn}(v_m^{g_2}) \frac{1 - \text{sgn}(\delta_m^{g_2})}{2} \\
& + 2 \sum_{m=1}^{n_{h_1}} \text{sgn}(v_m^{h_1}) \frac{1 - \text{sgn}(\delta_m^{h_1})}{2} - \sum_{m=1}^{n_{h_2}} \text{sgn}(v_m^{h_2}) \frac{1 - \text{sgn}(\delta_m^{h_2})}{2} + \sum_{m=1}^{n_{h_4}} \text{sgn}(v_m^{h_4}) \frac{1 - \text{sgn}(\delta_m^{h_4})}{2}
\end{aligned} \tag{S104.1}$$

$$\begin{aligned}
\mathcal{W}_2^{\text{gapless}} = & \sum_{m=1}^{n_{a_2}} \text{sgn}(v_m^{a_2}) \frac{1 - \text{sgn}(\delta_m^{a_2})}{2} + \sum_{m=1}^{n_{d_1}} \text{sgn}(v_m^{d_1}) \frac{1 - \text{sgn}(\delta_m^{d_1})}{2} - 2 \sum_{m=1}^{n_{e_2}} \text{sgn}(v_m^{e_2}) \frac{1 - \text{sgn}(\delta_m^{e_2})}{2} \\
& - 2 \sum_{m=1}^{n_{f_1}} \text{sgn}(v_m^{f_1}) \frac{1 - \text{sgn}(\delta_m^{f_1})}{2} - \sum_{m=1}^{n_{g_1}} \text{sgn}(v_m^{g_1}) \frac{1 - \text{sgn}(\delta_m^{g_1})}{2} - \sum_{m=1}^{n_{g_2}} \text{sgn}(v_m^{g_2}) \frac{1 - \text{sgn}(\delta_m^{g_2})}{2} \\
& + \sum_{m=1}^{n_{h_1}} \text{sgn}(v_m^{h_1}) \frac{1 - \text{sgn}(\delta_m^{h_1})}{2} - \sum_{m=1}^{n_{h_3}} \text{sgn}(v_m^{h_3}) \frac{1 - \text{sgn}(\delta_m^{h_3})}{2} + 2 \sum_{m=1}^{n_{h_4}} \text{sgn}(v_m^{h_4}) \frac{1 - \text{sgn}(\delta_m^{h_4})}{2}
\end{aligned} \tag{S104.2}$$

$$\begin{aligned} \mathcal{W}_3^{\text{gapless}} = & \sum_{m=1}^{n_{b_1}} \text{sgn}(v_m^{b_1}) \frac{1 - \text{sgn}(\delta_m^{b_1})}{2} - \sum_{m=1}^{n_{e_2}} \text{sgn}(v_m^{e_2}) \frac{1 - \text{sgn}(\delta_m^{e_2})}{2} + \sum_{m=1}^{n_{h_1}} \text{sgn}(v_m^{h_1}) \frac{1 - \text{sgn}(\delta_m^{h_1})}{2} \\ & + \sum_{m=1}^{n_{h_4}} \text{sgn}(v_m^{h_4}) \frac{1 - \text{sgn}(\delta_m^{h_4})}{2} - \sum_{m=1}^{n_{i_1}} \text{sgn}(v_m^{i_1}) \frac{1 - \text{sgn}(\delta_m^{i_1})}{2} - \sum_{m=1}^{n_{i_2}} \text{sgn}(v_m^{i_2}) \frac{1 - \text{sgn}(\delta_m^{i_2})}{2} \end{aligned} \quad (\text{S104.3})$$

$$\begin{aligned} \mathcal{W}_4^{\text{gapless}} = & \sum_{m=1}^{n_{c_1}} \text{sgn}(v_m^{c_1}) \frac{1 - \text{sgn}(\delta_m^{c_1})}{2} - \sum_{m=1}^{n_{f_1}} \text{sgn}(v_m^{f_1}) \frac{1 - \text{sgn}(\delta_m^{f_1})}{2} - \sum_{m=1}^{n_{g_1}} \text{sgn}(v_m^{g_1}) \frac{1 - \text{sgn}(\delta_m^{g_1})}{2} \\ & - \sum_{m=1}^{n_{g_2}} \text{sgn}(v_m^{g_2}) \frac{1 - \text{sgn}(\delta_m^{g_2})}{2} + \sum_{m=1}^{n_{i_1}} \text{sgn}(v_m^{i_1}) \frac{1 - \text{sgn}(\delta_m^{i_1})}{2} + \sum_{m=1}^{n_{i_2}} \text{sgn}(v_m^{i_2}) \frac{1 - \text{sgn}(\delta_m^{i_2})}{2} \end{aligned} \quad (\text{S104.4})$$

$$\begin{aligned} \mathcal{W}_5^{\text{gapless}} = & \sum_{m=1}^{n_{c_2}} \text{sgn}(v_m^{c_2}) \frac{1 - \text{sgn}(\delta_m^{c_2})}{2} - \sum_{m=1}^{n_{f_1}} \text{sgn}(v_m^{f_1}) \frac{1 - \text{sgn}(\delta_m^{f_1})}{2} - \sum_{m=1}^{n_{g_1}} \text{sgn}(v_m^{g_1}) \frac{1 - \text{sgn}(\delta_m^{g_1})}{2} \\ & - \sum_{m=1}^{n_{g_2}} \text{sgn}(v_m^{g_2}) \frac{1 - \text{sgn}(\delta_m^{g_2})}{2} + \sum_{m=1}^{n_{i_1}} \text{sgn}(v_m^{i_1}) \frac{1 - \text{sgn}(\delta_m^{i_1})}{2} + \sum_{m=1}^{n_{i_2}} \text{sgn}(v_m^{i_2}) \frac{1 - \text{sgn}(\delta_m^{i_2})}{2} \end{aligned} \quad (\text{S104.5})$$

$$\begin{aligned} \mathcal{W}_6^{\text{gapless}} = & 2 \sum_{m=1}^{n_{d_1}} \text{sgn}(v_m^{d_1}) \frac{1 - \text{sgn}(\delta_m^{d_1})}{2} - 2 \sum_{m=1}^{n_{e_2}} \text{sgn}(v_m^{e_2}) \frac{1 - \text{sgn}(\delta_m^{e_2})}{2} - 2 \sum_{m=1}^{n_{f_1}} \text{sgn}(v_m^{f_1}) \frac{1 - \text{sgn}(\delta_m^{f_1})}{2} \\ & + \sum_{m=1}^{n_{h_1}} \text{sgn}(v_m^{h_1}) \frac{1 - \text{sgn}(\delta_m^{h_1})}{2} - \sum_{m=1}^{n_{h_2}} \text{sgn}(v_m^{h_2}) \frac{1 - \text{sgn}(\delta_m^{h_2})}{2} - \sum_{m=1}^{n_{h_3}} \text{sgn}(v_m^{h_3}) \frac{1 - \text{sgn}(\delta_m^{h_3})}{2} \\ & + \sum_{m=1}^{n_{h_4}} \text{sgn}(v_m^{h_4}) \frac{1 - \text{sgn}(\delta_m^{h_4})}{2} \end{aligned} \quad (\text{S104.6})$$

$$\begin{aligned} \mathcal{W}_7^{\text{gapless}} = & \sum_{m=1}^{n_{e_1}} \text{sgn}(v_m^{e_1}) \frac{1 - \text{sgn}(\delta_m^{e_1})}{2} - \sum_{m=1}^{n_{e_2}} \text{sgn}(v_m^{e_2}) \frac{1 - \text{sgn}(\delta_m^{e_2})}{2} + \sum_{m=1}^{n_{h_1}} \text{sgn}(v_m^{h_1}) \frac{1 - \text{sgn}(\delta_m^{h_1})}{2} \\ & - \sum_{m=1}^{n_{h_2}} \text{sgn}(v_m^{h_2}) \frac{1 - \text{sgn}(\delta_m^{h_2})}{2} - \sum_{m=1}^{n_{h_3}} \text{sgn}(v_m^{h_3}) \frac{1 - \text{sgn}(\delta_m^{h_3})}{2} + \sum_{m=1}^{n_{h_4}} \text{sgn}(v_m^{h_4}) \frac{1 - \text{sgn}(\delta_m^{h_4})}{2} \end{aligned} \quad (\text{S104.7})$$

$$\begin{aligned} \mathcal{W}_1^{\text{gapped}} = & - \sum_{m=1}^{n_{d_1}} \text{sgn}(v_m^{d_1}) \frac{1 - \text{sgn}(\delta_m^{d_1})}{2} + \sum_{m=1}^{n_{e_2}} \text{sgn}(v_m^{e_2}) \frac{1 - \text{sgn}(\delta_m^{e_2})}{2} + \sum_{m=1}^{n_{f_1}} \text{sgn}(v_m^{f_1}) \frac{1 - \text{sgn}(\delta_m^{f_1})}{2} \\ & - \sum_{m=1}^{n_{h_1}} \text{sgn}(v_m^{h_1}) \frac{1 - \text{sgn}(\delta_m^{h_1})}{2} + \sum_{m=1}^{n_{h_3}} \text{sgn}(v_m^{h_3}) \frac{1 - \text{sgn}(\delta_m^{h_3})}{2} \end{aligned} \quad (\text{S104.8})$$

$$\mathcal{W}_2^{\text{gapped}} = - \sum_{m=1}^{n_{i_1}} \text{sgn}(v_m^{i_1}) \frac{1 - \text{sgn}(\delta_m^{i_1})}{2} + \sum_{m=1}^{n_{i_2}} \text{sgn}(v_m^{i_2}) \frac{1 - \text{sgn}(\delta_m^{i_2})}{2} \quad (\text{S104.9})$$

$$\mathcal{X}_1 = \sum_{m=1}^{n_{f_1}} \frac{1 - \text{sgn}(\delta_m^{f_1})}{2} \mod 2 \quad (\text{S104.10})$$

$$\mathcal{X}_2 = \sum_{m=1}^{n_{e_2}} \frac{1 - \text{sgn}(\delta_m^{e_2})}{2} + \sum_{m=1}^{n_{f_1}} \frac{1 - \text{sgn}(\delta_m^{f_1})}{2} \mod 2 \quad (\text{S104.11})$$

### S105. SPACE GROUP NO. 105

| line segment                                        | character of irrep (generators only)                                                                                                                                           |
|-----------------------------------------------------|--------------------------------------------------------------------------------------------------------------------------------------------------------------------------------|
| $a \quad (0, \frac{t}{2}, 0)$                       | $\{m_{100}   0 \ 0 \ 0\}$<br>$a_1 \quad -i$<br>$a_2 \quad i$                                                                                                                   |
| $b \quad (\frac{1-t}{2}, \frac{1}{2}, 0)$           | $\{m_{010}   0 \ 0 \ 0\}$<br>$b_1 \quad -i$<br>$b_2 \quad i$                                                                                                                   |
| $c \quad (\frac{t}{2}, \frac{t}{2}, 0)$             | $\{m_{1-10}   0 \ 0 \ \frac{1}{2}\}$<br>$c_1 \quad -i$<br>$c_2 \quad i$                                                                                                        |
| $d \quad (0, \frac{t}{2}, \frac{1}{2})$             | $\{m_{100}   0 \ 0 \ 0\}$<br>$d_1 \quad -i$<br>$d_2 \quad i$                                                                                                                   |
| $e \quad (\frac{1-t}{2}, \frac{1}{2}, \frac{1}{2})$ | $\{m_{010}   0 \ 0 \ 0\}$<br>$e_1 \quad -i$<br>$e_2 \quad i$                                                                                                                   |
| $f \quad (\frac{t}{2}, \frac{t}{2}, \frac{1}{2})$   | $\{m_{1-10}   0 \ 0 \ \frac{1}{2}\}$<br>$f_1 \quad -1$<br>$f_2 \quad 1$                                                                                                        |
| $g \quad (0, 0, \frac{t}{2})$                       | $\{4_{001}   0 \ 0 \ \frac{1}{2}\} \quad \{m_{100}   0 \ 0 \ 0\}$<br>$g_1 \quad -\sqrt{2}e^{-\frac{1}{2}i\pi t} \quad 0$<br>$g_2 \quad \sqrt{2}e^{-\frac{1}{2}i\pi t} \quad 0$ |
| $h \quad (0, \frac{1}{2}, \frac{t}{2})$             | $\{2_{001}   0 \ 0 \ 0\} \quad \{m_{100}   0 \ 0 \ 0\}$<br>$h_1 \quad 0 \quad 0$                                                                                               |
| $i \quad (\frac{1}{2}, \frac{1}{2}, \frac{t}{2})$   | $\{4_{001}   0 \ 0 \ \frac{1}{2}\} \quad \{m_{100}   0 \ 0 \ 0\}$<br>$i_1 \quad -\sqrt{2}e^{-\frac{1}{2}i\pi t} \quad 0$<br>$i_2 \quad \sqrt{2}e^{-\frac{1}{2}i\pi t} \quad 0$ |

$$\begin{aligned} \mathcal{W}_1^{\text{gapless}} = & \sum_{m=1}^{n_{a_1}} \text{sgn}(v_m^{a_1}) \frac{1 - \text{sgn}(\delta_m^{a_1})}{2} + \sum_{m=1}^{n_{d_2}} \text{sgn}(v_m^{d_2}) \frac{1 - \text{sgn}(\delta_m^{d_2})}{2} - \sum_{m=1}^{n_{e_1}} \text{sgn}(v_m^{e_1}) \frac{1 - \text{sgn}(\delta_m^{e_1})}{2} \\ & - \sum_{m=1}^{n_{e_2}} \text{sgn}(v_m^{e_2}) \frac{1 - \text{sgn}(\delta_m^{e_2})}{2} - 2 \sum_{m=1}^{n_{f_1}} \text{sgn}(v_m^{f_1}) \frac{1 - \text{sgn}(\delta_m^{f_1})}{2} - \sum_{m=1}^{n_{g_1}} \text{sgn}(v_m^{g_1}) \frac{1 - \text{sgn}(\delta_m^{g_1})}{2} \\ & - \sum_{m=1}^{n_{g_2}} \text{sgn}(v_m^{g_2}) \frac{1 - \text{sgn}(\delta_m^{g_2})}{2} + \sum_{m=1}^{n_{h_1}} \text{sgn}(v_m^{h_1}) \frac{1 - \text{sgn}(\delta_m^{h_1})}{2} \end{aligned} \quad (\text{S105.1})$$

$$\begin{aligned} \mathcal{W}_2^{\text{gapless}} = & \sum_{m=1}^{n_{a_2}} \text{sgn}(v_m^{a_2}) \frac{1 - \text{sgn}(\delta_m^{a_2})}{2} - \sum_{m=1}^{n_{d_2}} \text{sgn}(v_m^{d_2}) \frac{1 - \text{sgn}(\delta_m^{d_2})}{2} - \sum_{m=1}^{n_{g_1}} \text{sgn}(v_m^{g_1}) \frac{1 - \text{sgn}(\delta_m^{g_1})}{2} \\ & - \sum_{m=1}^{n_{g_2}} \text{sgn}(v_m^{g_2}) \frac{1 - \text{sgn}(\delta_m^{g_2})}{2} + \sum_{m=1}^{n_{h_1}} \text{sgn}(v_m^{h_1}) \frac{1 - \text{sgn}(\delta_m^{h_1})}{2} \end{aligned} \quad (\text{S105.2})$$

$$\begin{aligned} \mathcal{W}_3^{\text{gapless}} = & \sum_{m=1}^{n_{b_1}} \text{sgn}(v_m^{b_1}) \frac{1 - \text{sgn}(\delta_m^{b_1})}{2} - \sum_{m=1}^{n_{e_1}} \text{sgn}(v_m^{e_1}) \frac{1 - \text{sgn}(\delta_m^{e_1})}{2} + \sum_{m=1}^{n_{h_1}} \text{sgn}(v_m^{h_1}) \frac{1 - \text{sgn}(\delta_m^{h_1})}{2} \\ & - \sum_{m=1}^{n_{i_1}} \text{sgn}(v_m^{i_1}) \frac{1 - \text{sgn}(\delta_m^{i_1})}{2} - \sum_{m=1}^{n_{i_2}} \text{sgn}(v_m^{i_2}) \frac{1 - \text{sgn}(\delta_m^{i_2})}{2} \end{aligned} \quad (\text{S105.3})$$

$$\begin{aligned} \mathcal{W}_4^{\text{gapless}} = & \sum_{m=1}^{n_{b_2}} \text{sgn}(v_m^{b_2}) \frac{1 - \text{sgn}(\delta_m^{b_2})}{2} - \sum_{m=1}^{n_{e_2}} \text{sgn}(v_m^{e_2}) \frac{1 - \text{sgn}(\delta_m^{e_2})}{2} + \sum_{m=1}^{n_{h_1}} \text{sgn}(v_m^{h_1}) \frac{1 - \text{sgn}(\delta_m^{h_1})}{2} \\ & - \sum_{m=1}^{n_{i_1}} \text{sgn}(v_m^{i_1}) \frac{1 - \text{sgn}(\delta_m^{i_1})}{2} - \sum_{m=1}^{n_{i_2}} \text{sgn}(v_m^{i_2}) \frac{1 - \text{sgn}(\delta_m^{i_2})}{2} \end{aligned} \quad (\text{S105.4})$$

$$\begin{aligned} \mathcal{W}_5^{\text{gapless}} = & \sum_{m=1}^{n_{c_1}} \text{sgn}(v_m^{c_1}) \frac{1 - \text{sgn}(\delta_m^{c_1})}{2} - \sum_{m=1}^{n_{f_1}} \text{sgn}(v_m^{f_1}) \frac{1 - \text{sgn}(\delta_m^{f_1})}{2} - \sum_{m=1}^{n_{g_1}} \text{sgn}(v_m^{g_1}) \frac{1 - \text{sgn}(\delta_m^{g_1})}{2} \\ & - \sum_{m=1}^{n_{g_2}} \text{sgn}(v_m^{g_2}) \frac{1 - \text{sgn}(\delta_m^{g_2})}{2} + \sum_{m=1}^{n_{i_1}} \text{sgn}(v_m^{i_1}) \frac{1 - \text{sgn}(\delta_m^{i_1})}{2} + \sum_{m=1}^{n_{i_2}} \text{sgn}(v_m^{i_2}) \frac{1 - \text{sgn}(\delta_m^{i_2})}{2} \end{aligned} \quad (\text{S105.5})$$

$$\begin{aligned} \mathcal{W}_6^{\text{gapless}} = & \sum_{m=1}^{n_{c_2}} \text{sgn}(v_m^{c_2}) \frac{1 - \text{sgn}(\delta_m^{c_2})}{2} - \sum_{m=1}^{n_{f_1}} \text{sgn}(v_m^{f_1}) \frac{1 - \text{sgn}(\delta_m^{f_1})}{2} - \sum_{m=1}^{n_{g_1}} \text{sgn}(v_m^{g_1}) \frac{1 - \text{sgn}(\delta_m^{g_1})}{2} \\ & - \sum_{m=1}^{n_{g_2}} \text{sgn}(v_m^{g_2}) \frac{1 - \text{sgn}(\delta_m^{g_2})}{2} + \sum_{m=1}^{n_{i_1}} \text{sgn}(v_m^{i_1}) \frac{1 - \text{sgn}(\delta_m^{i_1})}{2} + \sum_{m=1}^{n_{i_2}} \text{sgn}(v_m^{i_2}) \frac{1 - \text{sgn}(\delta_m^{i_2})}{2} \end{aligned} \quad (\text{S105.6})$$

$$\begin{aligned} \mathcal{W}_7^{\text{gapless}} = & \sum_{m=1}^{n_{d_1}} \text{sgn}(v_m^{d_1}) \frac{1 - \text{sgn}(\delta_m^{d_1})}{2} + \sum_{m=1}^{n_{d_2}} \text{sgn}(v_m^{d_2}) \frac{1 - \text{sgn}(\delta_m^{d_2})}{2} - \sum_{m=1}^{n_{e_1}} \text{sgn}(v_m^{e_1}) \frac{1 - \text{sgn}(\delta_m^{e_1})}{2} \\ & - \sum_{m=1}^{n_{e_2}} \text{sgn}(v_m^{e_2}) \frac{1 - \text{sgn}(\delta_m^{e_2})}{2} - 2 \sum_{m=1}^{n_{f_1}} \text{sgn}(v_m^{f_1}) \frac{1 - \text{sgn}(\delta_m^{f_1})}{2} \end{aligned} \quad (\text{S105.7})$$

$$\mathcal{W}_1^{\text{gapped}} = \sum_{m=1}^{n_{e_1}} \text{sgn}(v_m^{e_1}) \frac{1 - \text{sgn}(\delta_m^{e_1})}{2} - \sum_{m=1}^{n_{e_2}} \text{sgn}(v_m^{e_2}) \frac{1 - \text{sgn}(\delta_m^{e_2})}{2} \quad (\text{S105.8})$$

$$\mathcal{W}_2^{\text{gapped}} = \sum_{m=1}^{n_{d_2}} \text{sgn}(v_m^{d_2}) \frac{1 - \text{sgn}(\delta_m^{d_2})}{2} - \sum_{m=1}^{n_{e_2}} \text{sgn}(v_m^{e_2}) \frac{1 - \text{sgn}(\delta_m^{e_2})}{2} - \sum_{m=1}^{n_{f_1}} \text{sgn}(v_m^{f_1}) \frac{1 - \text{sgn}(\delta_m^{f_1})}{2} \quad (\text{S105.9})$$

$$\mathcal{X}_1 = \sum_{m=1}^{n_{f_1}} \frac{1 - \text{sgn}(\delta_m^{f_1})}{2} \mod 2 \quad (\text{S105.10})$$



## S106. SPACE GROUP NO. 106

| line segment                                        | character of irrep (generators only)                                                                                                                                                             |
|-----------------------------------------------------|--------------------------------------------------------------------------------------------------------------------------------------------------------------------------------------------------|
| $a \quad (0, \frac{t}{2}, 0)$                       | $\{m_{100}   \frac{1}{2} \frac{1}{2} 0\}$<br>$a_1 \quad -ie^{-\frac{1}{2}i\pi t}$<br>$a_2 \quad ie^{-\frac{1}{2}i\pi t}$                                                                         |
| $b \quad (\frac{1-t}{2}, \frac{1}{2}, 0)$           | $\{m_{010}   \frac{1}{2} \frac{1}{2} 0\}$<br>$b_1 \quad -e^{-\frac{1}{2}i\pi(2-t)}$<br>$b_2 \quad e^{-\frac{1}{2}i\pi(2-t)}$                                                                     |
| $c \quad (\frac{t}{2}, \frac{t}{2}, 0)$             | $\{m_{1-10}   \frac{1}{2} \frac{1}{2} \frac{1}{2}\}$<br>$c_1 \quad -ie^{-i\pi t}$<br>$c_2 \quad ie^{-i\pi t}$                                                                                    |
| $d \quad (0, \frac{t}{2}, \frac{1}{2})$             | $\{m_{100}   \frac{1}{2} \frac{1}{2} 0\}$<br>$d_1 \quad -ie^{-\frac{1}{2}i\pi t}$<br>$d_2 \quad ie^{-\frac{1}{2}i\pi t}$                                                                         |
| $e \quad (\frac{1-t}{2}, \frac{1}{2}, \frac{1}{2})$ | $\{m_{010}   \frac{1}{2} \frac{1}{2} 0\}$<br>$e_1 \quad -e^{-\frac{1}{2}i\pi(2-t)}$<br>$e_2 \quad e^{-\frac{1}{2}i\pi(2-t)}$                                                                     |
| $f \quad (\frac{t}{2}, \frac{t}{2}, \frac{1}{2})$   | $\{m_{1-10}   \frac{1}{2} \frac{1}{2} \frac{1}{2}\}$<br>$f_1 \quad -ie^{-\frac{1}{2}i\pi(2t+1)}$<br>$f_2 \quad ie^{-\frac{1}{2}i\pi(2t+1)}$                                                      |
| $g \quad (0, 0, \frac{t}{2})$                       | $\{4_{001}   0 \ 0 \ \frac{1}{2}\} \quad \{m_{100}   \frac{1}{2} \frac{1}{2} 0\}$<br>$g_1 \quad -\sqrt{2}e^{-\frac{1}{2}i\pi t} \quad 0$<br>$g_2 \quad \sqrt{2}e^{-\frac{1}{2}i\pi t} \quad 0$   |
| $h \quad (0, \frac{1}{2}, \frac{t}{2})$             | $\{2_{001}   0 \ 0 \ 0\} \quad \{m_{100}   \frac{1}{2} \frac{1}{2} 0\}$<br>$h_1 \quad -i \quad -1$<br>$h_2 \quad -i \quad 1$<br>$h_3 \quad i \quad -1$<br>$h_4 \quad i \quad 1$                  |
| $i \quad (\frac{1}{2}, \frac{1}{2}, \frac{t}{2})$   | $\{4_{001}   0 \ 0 \ \frac{1}{2}\} \quad \{m_{100}   \frac{1}{2} \frac{1}{2} 0\}$<br>$i_1 \quad -i\sqrt{2}e^{-\frac{1}{2}i\pi t} \quad 0$<br>$i_2 \quad i\sqrt{2}e^{-\frac{1}{2}i\pi t} \quad 0$ |

$$\begin{aligned}
\mathcal{W}_1^{\text{gapless}} = & \sum_{m=1}^{n_{a_1}} \text{sgn}(v_m^{a_1}) \frac{1 - \text{sgn}(\delta_m^{a_1})}{2} + \sum_{m=1}^{n_{d_2}} \text{sgn}(v_m^{d_2}) \frac{1 - \text{sgn}(\delta_m^{d_2})}{2} - 2 \sum_{m=1}^{n_{e_1}} \text{sgn}(v_m^{e_1}) \frac{1 - \text{sgn}(\delta_m^{e_1})}{2} \\
& - 2 \sum_{m=1}^{n_{f_1}} \text{sgn}(v_m^{f_1}) \frac{1 - \text{sgn}(\delta_m^{f_1})}{2} - \sum_{m=1}^{n_{g_1}} \text{sgn}(v_m^{g_1}) \frac{1 - \text{sgn}(\delta_m^{g_1})}{2} - \sum_{m=1}^{n_{g_2}} \text{sgn}(v_m^{g_2}) \frac{1 - \text{sgn}(\delta_m^{g_2})}{2} \\
& + \sum_{m=1}^{n_{h_2}} \text{sgn}(v_m^{h_2}) \frac{1 - \text{sgn}(\delta_m^{h_2})}{2} + 2 \sum_{m=1}^{n_{h_3}} \text{sgn}(v_m^{h_3}) \frac{1 - \text{sgn}(\delta_m^{h_3})}{2} - \sum_{m=1}^{n_{h_4}} \text{sgn}(v_m^{h_4}) \frac{1 - \text{sgn}(\delta_m^{h_4})}{2}
\end{aligned} \tag{S106.1}$$

$$\begin{aligned}
\mathcal{W}_2^{\text{gapless}} = & \sum_{m=1}^{n_{a_2}} \text{sgn}(v_m^{a_2}) \frac{1 - \text{sgn}(\delta_m^{a_2})}{2} - \sum_{m=1}^{n_{d_2}} \text{sgn}(v_m^{d_2}) \frac{1 - \text{sgn}(\delta_m^{d_2})}{2} - \sum_{m=1}^{n_{g_1}} \text{sgn}(v_m^{g_1}) \frac{1 - \text{sgn}(\delta_m^{g_1})}{2} \\
& - \sum_{m=1}^{n_{g_2}} \text{sgn}(v_m^{g_2}) \frac{1 - \text{sgn}(\delta_m^{g_2})}{2} + \sum_{m=1}^{n_{h_2}} \text{sgn}(v_m^{h_2}) \frac{1 - \text{sgn}(\delta_m^{h_2})}{2} + \sum_{m=1}^{n_{h_4}} \text{sgn}(v_m^{h_4}) \frac{1 - \text{sgn}(\delta_m^{h_4})}{2}
\end{aligned} \tag{S106.2}$$

$$\begin{aligned} \mathcal{W}_3^{\text{gapless}} = & \sum_{m=1}^{n_{b_1}} \text{sgn}(v_m^{b_1}) \frac{1 - \text{sgn}(\delta_m^{b_1})}{2} - \sum_{m=1}^{n_{e_1}} \text{sgn}(v_m^{e_1}) \frac{1 - \text{sgn}(\delta_m^{e_1})}{2} + \sum_{m=1}^{n_{h_2}} \text{sgn}(v_m^{h_2}) \frac{1 - \text{sgn}(\delta_m^{h_2})}{2} \\ & + \sum_{m=1}^{n_{h_3}} \text{sgn}(v_m^{h_3}) \frac{1 - \text{sgn}(\delta_m^{h_3})}{2} - \sum_{m=1}^{n_{i_1}} \text{sgn}(v_m^{i_1}) \frac{1 - \text{sgn}(\delta_m^{i_1})}{2} - \sum_{m=1}^{n_{i_2}} \text{sgn}(v_m^{i_2}) \frac{1 - \text{sgn}(\delta_m^{i_2})}{2} \end{aligned} \quad (\text{S106.3})$$

$$\begin{aligned} \mathcal{W}_4^{\text{gapless}} = & \sum_{m=1}^{n_{c_1}} \text{sgn}(v_m^{c_1}) \frac{1 - \text{sgn}(\delta_m^{c_1})}{2} - \sum_{m=1}^{n_{f_1}} \text{sgn}(v_m^{f_1}) \frac{1 - \text{sgn}(\delta_m^{f_1})}{2} - \sum_{m=1}^{n_{g_1}} \text{sgn}(v_m^{g_1}) \frac{1 - \text{sgn}(\delta_m^{g_1})}{2} \\ & - \sum_{m=1}^{n_{g_2}} \text{sgn}(v_m^{g_2}) \frac{1 - \text{sgn}(\delta_m^{g_2})}{2} + \sum_{m=1}^{n_{i_1}} \text{sgn}(v_m^{i_1}) \frac{1 - \text{sgn}(\delta_m^{i_1})}{2} + \sum_{m=1}^{n_{i_2}} \text{sgn}(v_m^{i_2}) \frac{1 - \text{sgn}(\delta_m^{i_2})}{2} \end{aligned} \quad (\text{S106.4})$$

$$\begin{aligned} \mathcal{W}_5^{\text{gapless}} = & \sum_{m=1}^{n_{c_2}} \text{sgn}(v_m^{c_2}) \frac{1 - \text{sgn}(\delta_m^{c_2})}{2} - \sum_{m=1}^{n_{f_1}} \text{sgn}(v_m^{f_1}) \frac{1 - \text{sgn}(\delta_m^{f_1})}{2} - \sum_{m=1}^{n_{g_1}} \text{sgn}(v_m^{g_1}) \frac{1 - \text{sgn}(\delta_m^{g_1})}{2} \\ & - \sum_{m=1}^{n_{g_2}} \text{sgn}(v_m^{g_2}) \frac{1 - \text{sgn}(\delta_m^{g_2})}{2} + \sum_{m=1}^{n_{i_1}} \text{sgn}(v_m^{i_1}) \frac{1 - \text{sgn}(\delta_m^{i_1})}{2} + \sum_{m=1}^{n_{i_2}} \text{sgn}(v_m^{i_2}) \frac{1 - \text{sgn}(\delta_m^{i_2})}{2} \end{aligned} \quad (\text{S106.5})$$

$$\begin{aligned} \mathcal{W}_6^{\text{gapless}} = & \sum_{m=1}^{n_{d_1}} \text{sgn}(v_m^{d_1}) \frac{1 - \text{sgn}(\delta_m^{d_1})}{2} + \sum_{m=1}^{n_{d_2}} \text{sgn}(v_m^{d_2}) \frac{1 - \text{sgn}(\delta_m^{d_2})}{2} - 2 \sum_{m=1}^{n_{e_1}} \text{sgn}(v_m^{e_1}) \frac{1 - \text{sgn}(\delta_m^{e_1})}{2} \\ & - 2 \sum_{m=1}^{n_{f_1}} \text{sgn}(v_m^{f_1}) \frac{1 - \text{sgn}(\delta_m^{f_1})}{2} \end{aligned} \quad (\text{S106.6})$$

$$\mathcal{W}_7^{\text{gapless}} = \sum_{m=1}^{n_{h_1}} \text{sgn}(v_m^{h_1}) \frac{1 - \text{sgn}(\delta_m^{h_1})}{2} - \sum_{m=1}^{n_{h_2}} \text{sgn}(v_m^{h_2}) \frac{1 - \text{sgn}(\delta_m^{h_2})}{2} - \sum_{m=1}^{n_{h_3}} \text{sgn}(v_m^{h_3}) \frac{1 - \text{sgn}(\delta_m^{h_3})}{2} + \sum_{m=1}^{n_{h_4}} \text{sgn}(v_m^{h_4}) \frac{1 - \text{sgn}(\delta_m^{h_4})}{2} \quad (\text{S106.7})$$

$$\mathcal{W}_1^{\text{gapped}} = - \sum_{m=1}^{n_{h_2}} \text{sgn}(v_m^{h_2}) \frac{1 - \text{sgn}(\delta_m^{h_2})}{2} + \sum_{m=1}^{n_{h_4}} \text{sgn}(v_m^{h_4}) \frac{1 - \text{sgn}(\delta_m^{h_4})}{2} \quad (\text{S106.8})$$

$$\mathcal{X}_1 = \sum_{m=1}^{n_{f_1}} \frac{1 - \text{sgn}(\delta_m^{f_1})}{2} + \sum_{m=1}^{n_{i_1}} \frac{1 - \text{sgn}(\delta_m^{i_1})}{2} + \sum_{m=1}^{n_{i_2}} \frac{1 - \text{sgn}(\delta_m^{i_2})}{2} \quad \text{mod } 2 \quad (\text{S106.9})$$

$$\mathcal{X}_2 = \sum_{m=1}^{n_{d_2}} \frac{1 - \text{sgn}(\delta_m^{d_2})}{2} \quad \text{mod } 2 \quad (\text{S106.10})$$

$$\mathcal{X}_3 = \sum_{m=1}^{n_{f_1}} \frac{1 - \text{sgn}(\delta_m^{f_1})}{2} \quad \text{mod } 2 \quad (\text{S106.11})$$

## S107. SPACE GROUP NO. 107

| line segment                                      | character of irrep (generators only)                                                                                               |
|---------------------------------------------------|------------------------------------------------------------------------------------------------------------------------------------|
| $a \ (0, 0, t)$                                   | $\begin{array}{cc} \{4_{001}  0 & 0 & 0 \} & \{m_{100}  0 & 0 & 0 \} \\ a_1 & -\sqrt{2} & & 0 \\ a_2 & \sqrt{2} & & 0 \end{array}$ |
| $b \ (\frac{1}{2}, \frac{1}{2}, \frac{t}{2})$     | $\begin{array}{cc} \{2_{001}  0 & 0 & 0 \} & \{m_{110}  0 & 0 & 0 \} \\ b_1 & 0 & & 0 \end{array}$                                 |
| $c \ (\frac{t}{2}, \frac{t}{2}, 1 - \frac{t}{2})$ | $\begin{array}{cc} \{m_{1-10}  0 & 0 & 0 \} \\ c_1 & -i \\ c_2 & i \end{array}$                                                    |
| $d \ (\frac{t}{2}, \frac{t}{2}, 0)$               | $\begin{array}{cc} \{m_{1-10}  0 & 0 & 0 \} \\ d_1 & -i \\ d_2 & i \end{array}$                                                    |
| $e \ (\frac{t}{2}, 1 - \frac{t}{2}, 0)$           | $\begin{array}{cc} \{m_{110}  0 & 0 & 0 \} \\ e_1 & -i \\ e_2 & i \end{array}$                                                     |
| $f \ (\frac{1-t}{2}, \frac{1}{2}, \frac{1}{2})$   | $\begin{array}{cc} \{1  0 & 0 & 0 \} \\ f_1 & 1 \end{array}$                                                                       |
| $g \ (0, t, 0)$                                   | $\begin{array}{cc} \{m_{100}  0 & 0 & 0 \} \\ g_1 & -i \\ g_2 & i \end{array}$                                                     |
| $h \ (0, \frac{t}{2}, 1 - \frac{t}{2})$           | $\begin{array}{cc} \{m_{100}  0 & 0 & 0 \} \\ h_1 & -i \\ h_2 & i \end{array}$                                                     |

$$\begin{aligned} \mathcal{W}_1^{\text{gapless}} = & \sum_{m=1}^{n_{a_1}} \text{sgn}(v_m^{a_1}) \frac{1 - \text{sgn}(\delta_m^{a_1})}{2} + \sum_{m=1}^{n_{a_2}} \text{sgn}(v_m^{a_2}) \frac{1 - \text{sgn}(\delta_m^{a_2})}{2} - \sum_{m=1}^{n_{g_2}} \text{sgn}(v_m^{g_2}) \frac{1 - \text{sgn}(\delta_m^{g_2})}{2} \\ & - \sum_{m=1}^{n_{h_1}} \text{sgn}(v_m^{h_1}) \frac{1 - \text{sgn}(\delta_m^{h_1})}{2} + \sum_{m=1}^{n_{h_2}} \text{sgn}(v_m^{h_2}) \frac{1 - \text{sgn}(\delta_m^{h_2})}{2} \end{aligned} \quad (\text{S107.1})$$

$$\begin{aligned} \mathcal{W}_2^{\text{gapless}} = & \sum_{m=1}^{n_{b_1}} \text{sgn}(v_m^{b_1}) \frac{1 - \text{sgn}(\delta_m^{b_1})}{2} + \sum_{m=1}^{n_{c_2}} \text{sgn}(v_m^{c_2}) \frac{1 - \text{sgn}(\delta_m^{c_2})}{2} + \sum_{m=1}^{n_{e_2}} \text{sgn}(v_m^{e_2}) \frac{1 - \text{sgn}(\delta_m^{e_2})}{2} \\ & + \sum_{m=1}^{n_{f_1}} \text{sgn}(v_m^{f_1}) \frac{1 - \text{sgn}(\delta_m^{f_1})}{2} - \sum_{m=1}^{n_{h_1}} \text{sgn}(v_m^{h_1}) \frac{1 - \text{sgn}(\delta_m^{h_1})}{2} - \sum_{m=1}^{n_{h_2}} \text{sgn}(v_m^{h_2}) \frac{1 - \text{sgn}(\delta_m^{h_2})}{2} \end{aligned} \quad (\text{S107.2})$$

$$\begin{aligned} \mathcal{W}_3^{\text{gapless}} = & \sum_{m=1}^{n_{c_1}} \text{sgn}(v_m^{c_1}) \frac{1 - \text{sgn}(\delta_m^{c_1})}{2} + \sum_{m=1}^{n_{c_2}} \text{sgn}(v_m^{c_2}) \frac{1 - \text{sgn}(\delta_m^{c_2})}{2} + \sum_{m=1}^{n_{f_1}} \text{sgn}(v_m^{f_1}) \frac{1 - \text{sgn}(\delta_m^{f_1})}{2} \\ & - \sum_{m=1}^{n_{h_1}} \text{sgn}(v_m^{h_1}) \frac{1 - \text{sgn}(\delta_m^{h_1})}{2} - \sum_{m=1}^{n_{h_2}} \text{sgn}(v_m^{h_2}) \frac{1 - \text{sgn}(\delta_m^{h_2})}{2} \end{aligned} \quad (\text{S107.3})$$

$$\begin{aligned} \mathcal{W}_4^{\text{gapless}} = & 2 \sum_{m=1}^{n_{c_2}} \text{sgn}(v_m^{c_2}) \frac{1 - \text{sgn}(\delta_m^{c_2})}{2} - \sum_{m=1}^{n_{e_1}} \text{sgn}(v_m^{e_1}) \frac{1 - \text{sgn}(\delta_m^{e_1})}{2} + \sum_{m=1}^{n_{e_2}} \text{sgn}(v_m^{e_2}) \frac{1 - \text{sgn}(\delta_m^{e_2})}{2} \\ & + \sum_{m=1}^{n_{f_1}} \text{sgn}(v_m^{f_1}) \frac{1 - \text{sgn}(\delta_m^{f_1})}{2} - \sum_{m=1}^{n_{h_1}} \text{sgn}(v_m^{h_1}) \frac{1 - \text{sgn}(\delta_m^{h_1})}{2} - \sum_{m=1}^{n_{h_2}} \text{sgn}(v_m^{h_2}) \frac{1 - \text{sgn}(\delta_m^{h_2})}{2} \end{aligned} \quad (\text{S107.4})$$

$$\begin{aligned} \mathcal{W}_5^{\text{gapless}} = & \sum_{m=1}^{n_{d_1}} \text{sgn}(v_m^{d_1}) \frac{1 - \text{sgn}(\delta_m^{d_1})}{2} - \sum_{m=1}^{n_{e_2}} \text{sgn}(v_m^{e_2}) \frac{1 - \text{sgn}(\delta_m^{e_2})}{2} - \sum_{m=1}^{n_{g_2}} \text{sgn}(v_m^{g_2}) \frac{1 - \text{sgn}(\delta_m^{g_2})}{2} \\ & - \sum_{m=1}^{n_{h_1}} \text{sgn}(v_m^{h_1}) \frac{1 - \text{sgn}(\delta_m^{h_1})}{2} + \sum_{m=1}^{n_{h_2}} \text{sgn}(v_m^{h_2}) \frac{1 - \text{sgn}(\delta_m^{h_2})}{2} \end{aligned} \quad (\text{S107.5})$$

$$\begin{aligned} \mathcal{W}_6^{\text{gapless}} = & \sum_{m=1}^{n_{d_2}} \text{sgn}(v_m^{d_2}) \frac{1 - \text{sgn}(\delta_m^{d_2})}{2} - \sum_{m=1}^{n_{e_1}} \text{sgn}(v_m^{e_1}) \frac{1 - \text{sgn}(\delta_m^{e_1})}{2} - \sum_{m=1}^{n_{g_2}} \text{sgn}(v_m^{g_2}) \frac{1 - \text{sgn}(\delta_m^{g_2})}{2} \\ & - \sum_{m=1}^{n_{h_1}} \text{sgn}(v_m^{h_1}) \frac{1 - \text{sgn}(\delta_m^{h_1})}{2} + \sum_{m=1}^{n_{h_2}} \text{sgn}(v_m^{h_2}) \frac{1 - \text{sgn}(\delta_m^{h_2})}{2} \end{aligned} \quad (\text{S107.6})$$

$$\begin{aligned} \mathcal{W}_7^{\text{gapless}} = & \sum_{m=1}^{n_{g_1}} \text{sgn}(v_m^{g_1}) \frac{1 - \text{sgn}(\delta_m^{g_1})}{2} - \sum_{m=1}^{n_{g_2}} \text{sgn}(v_m^{g_2}) \frac{1 - \text{sgn}(\delta_m^{g_2})}{2} - 2 \sum_{m=1}^{n_{h_1}} \text{sgn}(v_m^{h_1}) \frac{1 - \text{sgn}(\delta_m^{h_1})}{2} \\ & + 2 \sum_{m=1}^{n_{h_2}} \text{sgn}(v_m^{h_2}) \frac{1 - \text{sgn}(\delta_m^{h_2})}{2} \end{aligned} \quad (\text{S107.7})$$

$$\mathcal{W}_1^{\text{gapped}} = \sum_{m=1}^{n_{e_1}} \text{sgn}(v_m^{e_1}) \frac{1 - \text{sgn}(\delta_m^{e_1})}{2} - \sum_{m=1}^{n_{e_2}} \text{sgn}(v_m^{e_2}) \frac{1 - \text{sgn}(\delta_m^{e_2})}{2} \quad (\text{S107.8})$$

$$\mathcal{W}_2^{\text{gapped}} = -2 \sum_{m=1}^{n_{c_2}} \text{sgn}(v_m^{c_2}) \frac{1 - \text{sgn}(\delta_m^{c_2})}{2} - \sum_{m=1}^{n_{f_1}} \text{sgn}(v_m^{f_1}) \frac{1 - \text{sgn}(\delta_m^{f_1})}{2} + 2 \sum_{m=1}^{n_{h_2}} \text{sgn}(v_m^{h_2}) \frac{1 - \text{sgn}(\delta_m^{h_2})}{2} \quad (\text{S107.9})$$

### S108. SPACE GROUP NO. 108

| line segment                                          | character of irrep (generators only)                              |
|-------------------------------------------------------|-------------------------------------------------------------------|
| $a \quad (0, 0, t)$                                   | $\{4_{001}   0 \ 0 \ 0\} \quad \{m_{100}   0 \ 0 \ \frac{1}{2}\}$ |
|                                                       | $a_1 \quad -\sqrt{2} \quad 0$                                     |
|                                                       | $a_2 \quad \sqrt{2} \quad 0$                                      |
| $b \quad (\frac{1}{2}, \frac{1}{2}, \frac{t}{2})$     | $\{2_{001}   0 \ 0 \ 0\} \quad \{m_{110}   0 \ 0 \ \frac{1}{2}\}$ |
|                                                       | $b_1 \quad 0 \quad 0$                                             |
| $c \quad (\frac{t}{2}, \frac{t}{2}, 1 - \frac{t}{2})$ | $\{m_{1-10}   0 \ 0 \ \frac{1}{2}\}$                              |
|                                                       | $c_1 \quad -ie^{-\frac{1}{2}i\pi(2-t)}$                           |
|                                                       | $c_2 \quad ie^{-\frac{1}{2}i\pi(2-t)}$                            |
| $d \quad (\frac{t}{2}, \frac{t}{2}, 0)$               | $\{m_{1-10}   0 \ 0 \ \frac{1}{2}\}$                              |
|                                                       | $d_1 \quad -i$                                                    |
|                                                       | $d_2 \quad i$                                                     |
| $e \quad (\frac{t}{2}, 1 - \frac{t}{2}, 0)$           | $\{m_{110}   0 \ 0 \ \frac{1}{2}\}$                               |
|                                                       | $e_1 \quad -i$                                                    |
|                                                       | $e_2 \quad i$                                                     |
| $f \quad (\frac{1-t}{2}, \frac{1}{2}, \frac{1}{2})$   | $\{1   0 \ 0 \ 0\}$                                               |
|                                                       | $f_1 \quad 1$                                                     |
| $g \quad (0, t, 0)$                                   | $\{m_{100}   0 \ 0 \ \frac{1}{2}\}$                               |
|                                                       | $g_1 \quad -i$                                                    |
|                                                       | $g_2 \quad i$                                                     |

|                                             |                                                                                                                                                                      |
|---------------------------------------------|----------------------------------------------------------------------------------------------------------------------------------------------------------------------|
| $h \quad (0, \frac{t}{2}, 1 - \frac{t}{2})$ | $\begin{matrix} h_1 & \{m_{100}   0 \ 0 \ \frac{1}{2}\} \\ h_2 & \begin{matrix} -ie^{-\frac{1}{2}i\pi(2-t)} \\ ie^{-\frac{1}{2}i\pi(2-t)} \end{matrix} \end{matrix}$ |
|---------------------------------------------|----------------------------------------------------------------------------------------------------------------------------------------------------------------------|

$$\mathcal{W}_1^{\text{gapless}} = \sum_{m=1}^{n_{a_1}} \text{sgn}(v_m^{a_1}) \frac{1 - \text{sgn}(\delta_m^{a_1})}{2} + \sum_{m=1}^{n_{a_2}} \text{sgn}(v_m^{a_2}) \frac{1 - \text{sgn}(\delta_m^{a_2})}{2} - \sum_{m=1}^{n_{g_2}} \text{sgn}(v_m^{g_2}) \frac{1 - \text{sgn}(\delta_m^{g_2})}{2} \quad (\text{S108.1})$$

$$\begin{aligned} \mathcal{W}_2^{\text{gapless}} = & \sum_{m=1}^{n_{b_1}} \text{sgn}(v_m^{b_1}) \frac{1 - \text{sgn}(\delta_m^{b_1})}{2} + \sum_{m=1}^{n_{c_2}} \text{sgn}(v_m^{c_2}) \frac{1 - \text{sgn}(\delta_m^{c_2})}{2} + \sum_{m=1}^{n_{e_1}} \text{sgn}(v_m^{e_1}) \frac{1 - \text{sgn}(\delta_m^{e_1})}{2} \\ & + 2 \sum_{m=1}^{n_{f_1}} \text{sgn}(v_m^{f_1}) \frac{1 - \text{sgn}(\delta_m^{f_1})}{2} - \sum_{m=1}^{n_{h_1}} \text{sgn}(v_m^{h_1}) \frac{1 - \text{sgn}(\delta_m^{h_1})}{2} - \sum_{m=1}^{n_{h_2}} \text{sgn}(v_m^{h_2}) \frac{1 - \text{sgn}(\delta_m^{h_2})}{2} \end{aligned} \quad (\text{S108.2})$$

$$\begin{aligned} \mathcal{W}_3^{\text{gapless}} = & \sum_{m=1}^{n_{c_1}} \text{sgn}(v_m^{c_1}) \frac{1 - \text{sgn}(\delta_m^{c_1})}{2} + \sum_{m=1}^{n_{c_2}} \text{sgn}(v_m^{c_2}) \frac{1 - \text{sgn}(\delta_m^{c_2})}{2} + 2 \sum_{m=1}^{n_{f_1}} \text{sgn}(v_m^{f_1}) \frac{1 - \text{sgn}(\delta_m^{f_1})}{2} \\ & - \sum_{m=1}^{n_{h_1}} \text{sgn}(v_m^{h_1}) \frac{1 - \text{sgn}(\delta_m^{h_1})}{2} - \sum_{m=1}^{n_{h_2}} \text{sgn}(v_m^{h_2}) \frac{1 - \text{sgn}(\delta_m^{h_2})}{2} \end{aligned} \quad (\text{S108.3})$$

$$\begin{aligned} \mathcal{W}_4^{\text{gapless}} = & 2 \sum_{m=1}^{n_{c_2}} \text{sgn}(v_m^{c_2}) \frac{1 - \text{sgn}(\delta_m^{c_2})}{2} + \sum_{m=1}^{n_{e_1}} \text{sgn}(v_m^{e_1}) \frac{1 - \text{sgn}(\delta_m^{e_1})}{2} - \sum_{m=1}^{n_{e_2}} \text{sgn}(v_m^{e_2}) \frac{1 - \text{sgn}(\delta_m^{e_2})}{2} \\ & + 2 \sum_{m=1}^{n_{f_1}} \text{sgn}(v_m^{f_1}) \frac{1 - \text{sgn}(\delta_m^{f_1})}{2} - \sum_{m=1}^{n_{h_1}} \text{sgn}(v_m^{h_1}) \frac{1 - \text{sgn}(\delta_m^{h_1})}{2} - \sum_{m=1}^{n_{h_2}} \text{sgn}(v_m^{h_2}) \frac{1 - \text{sgn}(\delta_m^{h_2})}{2} \end{aligned} \quad (\text{S108.4})$$

$$\mathcal{W}_5^{\text{gapless}} = \sum_{m=1}^{n_{d_1}} \text{sgn}(v_m^{d_1}) \frac{1 - \text{sgn}(\delta_m^{d_1})}{2} - \sum_{m=1}^{n_{e_1}} \text{sgn}(v_m^{e_1}) \frac{1 - \text{sgn}(\delta_m^{e_1})}{2} - \sum_{m=1}^{n_{g_2}} \text{sgn}(v_m^{g_2}) \frac{1 - \text{sgn}(\delta_m^{g_2})}{2} \quad (\text{S108.5})$$

$$\mathcal{W}_6^{\text{gapless}} = \sum_{m=1}^{n_{d_2}} \text{sgn}(v_m^{d_2}) \frac{1 - \text{sgn}(\delta_m^{d_2})}{2} - \sum_{m=1}^{n_{e_2}} \text{sgn}(v_m^{e_2}) \frac{1 - \text{sgn}(\delta_m^{e_2})}{2} - \sum_{m=1}^{n_{g_2}} \text{sgn}(v_m^{g_2}) \frac{1 - \text{sgn}(\delta_m^{g_2})}{2} \quad (\text{S108.6})$$

$$\mathcal{W}_7^{\text{gapless}} = \sum_{m=1}^{n_{g_1}} \text{sgn}(v_m^{g_1}) \frac{1 - \text{sgn}(\delta_m^{g_1})}{2} - \sum_{m=1}^{n_{g_2}} \text{sgn}(v_m^{g_2}) \frac{1 - \text{sgn}(\delta_m^{g_2})}{2} \quad (\text{S108.7})$$

$$\mathcal{W}_1^{\text{gapped}} = \sum_{m=1}^{n_{e_1}} \text{sgn}(v_m^{e_1}) \frac{1 - \text{sgn}(\delta_m^{e_1})}{2} - \sum_{m=1}^{n_{e_2}} \text{sgn}(v_m^{e_2}) \frac{1 - \text{sgn}(\delta_m^{e_2})}{2} \quad (\text{S108.8})$$

$$\mathcal{X}_1 = \sum_{m=1}^{n_{c_2}} \frac{1 - \text{sgn}(\delta_m^{c_2})}{2} + \sum_{m=1}^{n_{e_1}} \frac{1 - \text{sgn}(\delta_m^{e_1})}{2} + \sum_{m=1}^{n_{e_2}} \frac{1 - \text{sgn}(\delta_m^{e_2})}{2} + \sum_{m=1}^{n_{h_2}} \frac{1 - \text{sgn}(\delta_m^{h_2})}{2} \pmod{2} \quad (\text{S108.9})$$

## S109. SPACE GROUP NO. 109

| line segment                                          | character of irrep (generators only)           |                                               |
|-------------------------------------------------------|------------------------------------------------|-----------------------------------------------|
| $a \quad (0, 0, t)$                                   | $\{4_{001}   0 \ \frac{1}{2} \ \frac{1}{4}\}$  | $\{m_{100}   0 \ 0 \ 0\}$                     |
|                                                       | $a_1 \quad -\sqrt{2}e^{-\frac{1}{2}i\pi t}$    | 0                                             |
|                                                       | $a_2 \quad \sqrt{2}e^{-\frac{1}{2}i\pi t}$     | 0                                             |
| $b \quad (\frac{1}{2}, \frac{1}{2}, \frac{t}{2})$     | $\{2_{001}   0 \ 0 \ 0\}$                      | $\{m_{110}   0 \ \frac{1}{2} \ \frac{1}{4}\}$ |
|                                                       | $b_1 \quad -i$                                 | $-e^{-\frac{1}{4}i\pi(t+2)}$                  |
|                                                       | $b_2 \quad -i$                                 | $e^{-\frac{1}{4}i\pi(t+2)}$                   |
|                                                       | $b_3 \quad i$                                  | $-e^{-\frac{1}{4}i\pi(t+2)}$                  |
| $c \quad (\frac{t}{2}, \frac{t}{2}, 1 - \frac{t}{2})$ | $\{m_{1-10}   0 \ \frac{1}{2} \ \frac{1}{4}\}$ |                                               |
|                                                       | $c_1 \quad -ie^{-\frac{1}{4}i\pi(t+2)}$        |                                               |
|                                                       | $c_2 \quad ie^{-\frac{1}{4}i\pi(t+2)}$         |                                               |
| $d \quad (\frac{t}{2}, \frac{t}{2}, 0)$               | $\{m_{1-10}   0 \ \frac{1}{2} \ \frac{1}{4}\}$ |                                               |
|                                                       | $d_1 \quad -ie^{-\frac{1}{2}i\pi t}$           |                                               |
| $e \quad (\frac{t}{2}, 1 - \frac{t}{2}, 0)$           | $\{m_{110}   0 \ \frac{1}{2} \ \frac{1}{4}\}$  |                                               |
|                                                       | $e_1 \quad -e^{-\frac{1}{2}i\pi(2-t)}$         |                                               |
|                                                       | $e_2 \quad e^{-\frac{1}{2}i\pi(2-t)}$          |                                               |
| $f \quad (\frac{1-t}{2}, \frac{1}{2}, \frac{1}{2})$   | $\{1   0 \ 0 \ 0\}$                            |                                               |
|                                                       | $f_1 \quad 1$                                  |                                               |
| $g \quad (0, t, 0)$                                   | $\{m_{100}   0 \ 0 \ 0\}$                      |                                               |
|                                                       | $g_1 \quad -i$                                 |                                               |
| $h \quad (0, \frac{t}{2}, 1 - \frac{t}{2})$           | $\{m_{100}   0 \ 0 \ 0\}$                      |                                               |
|                                                       | $h_1 \quad -i$                                 |                                               |
|                                                       | $h_2 \quad i$                                  |                                               |

$$\begin{aligned}
\mathcal{W}_1^{\text{gapless}} = & \sum_{m=1}^{n_{a_1}} \text{sgn}(v_m^{a_1}) \frac{1 - \text{sgn}(\delta_m^{a_1})}{2} + \sum_{m=1}^{n_{a_2}} \text{sgn}(v_m^{a_2}) \frac{1 - \text{sgn}(\delta_m^{a_2})}{2} - \sum_{m=1}^{n_{g_2}} \text{sgn}(v_m^{g_2}) \frac{1 - \text{sgn}(\delta_m^{g_2})}{2} \\
& - \sum_{m=1}^{n_{h_1}} \text{sgn}(v_m^{h_1}) \frac{1 - \text{sgn}(\delta_m^{h_1})}{2} + \sum_{m=1}^{n_{h_2}} \text{sgn}(v_m^{h_2}) \frac{1 - \text{sgn}(\delta_m^{h_2})}{2}
\end{aligned} \tag{S109.1}$$

$$\begin{aligned}
\mathcal{W}_2^{\text{gapless}} = & \sum_{m=1}^{n_{b_1}} \text{sgn}(v_m^{b_1}) \frac{1 - \text{sgn}(\delta_m^{b_1})}{2} + \sum_{m=1}^{n_{b_4}} \text{sgn}(v_m^{b_4}) \frac{1 - \text{sgn}(\delta_m^{b_4})}{2} - \sum_{m=1}^{n_{c_2}} \text{sgn}(v_m^{c_2}) \frac{1 - \text{sgn}(\delta_m^{c_2})}{2} + \sum_{m=1}^{n_{d_2}} \text{sgn}(v_m^{d_2}) \frac{1 - \text{sgn}(\delta_m^{d_2})}{2} \\
& - \sum_{m=1}^{n_{g_2}} \text{sgn}(v_m^{g_2}) \frac{1 - \text{sgn}(\delta_m^{g_2})}{2} - \sum_{m=1}^{n_{h_1}} \text{sgn}(v_m^{h_1}) \frac{1 - \text{sgn}(\delta_m^{h_1})}{2} + \sum_{m=1}^{n_{h_2}} \text{sgn}(v_m^{h_2}) \frac{1 - \text{sgn}(\delta_m^{h_2})}{2}
\end{aligned} \tag{S109.2}$$

$$\begin{aligned}
\mathcal{W}_3^{\text{gapless}} = & \sum_{m=1}^{n_{b_2}} \text{sgn}(v_m^{b_2}) \frac{1 - \text{sgn}(\delta_m^{b_2})}{2} + \sum_{m=1}^{n_{b_4}} \text{sgn}(v_m^{b_4}) \frac{1 - \text{sgn}(\delta_m^{b_4})}{2} + \sum_{m=1}^{n_{c_2}} \text{sgn}(v_m^{c_2}) \frac{1 - \text{sgn}(\delta_m^{c_2})}{2} + \sum_{m=1}^{n_{e_1}} \text{sgn}(v_m^{e_1}) \frac{1 - \text{sgn}(\delta_m^{e_1})}{2} \\
& + \sum_{m=1}^{n_{f_1}} \text{sgn}(v_m^{f_1}) \frac{1 - \text{sgn}(\delta_m^{f_1})}{2} - \sum_{m=1}^{n_{h_1}} \text{sgn}(v_m^{h_1}) \frac{1 - \text{sgn}(\delta_m^{h_1})}{2} - \sum_{m=1}^{n_{h_2}} \text{sgn}(v_m^{h_2}) \frac{1 - \text{sgn}(\delta_m^{h_2})}{2}
\end{aligned} \tag{S109.3}$$

$$\begin{aligned}
\mathcal{W}_4^{\text{gapless}} = & \sum_{m=1}^{n_{b_3}} \text{sgn}(v_m^{b_3}) \frac{1 - \text{sgn}(\delta_m^{b_3})}{2} - \sum_{m=1}^{n_{b_4}} \text{sgn}(v_m^{b_4}) \frac{1 - \text{sgn}(\delta_m^{b_4})}{2} - \sum_{m=1}^{n_{d_2}} \text{sgn}(v_m^{d_2}) \frac{1 - \text{sgn}(\delta_m^{d_2})}{2} + \sum_{m=1}^{n_{e_1}} \text{sgn}(v_m^{e_1}) \frac{1 - \text{sgn}(\delta_m^{e_1})}{2} \\
& + \sum_{m=1}^{n_{g_2}} \text{sgn}(v_m^{g_2}) \frac{1 - \text{sgn}(\delta_m^{g_2})}{2} + \sum_{m=1}^{n_{h_1}} \text{sgn}(v_m^{h_1}) \frac{1 - \text{sgn}(\delta_m^{h_1})}{2} - \sum_{m=1}^{n_{h_2}} \text{sgn}(v_m^{h_2}) \frac{1 - \text{sgn}(\delta_m^{h_2})}{2}
\end{aligned} \tag{S109.4}$$

$$\begin{aligned}
\mathcal{W}_5^{\text{gapless}} = & \sum_{m=1}^{n_{c_1}} \text{sgn}(v_m^{c_1}) \frac{1 - \text{sgn}(\delta_m^{c_1})}{2} + \sum_{m=1}^{n_{c_2}} \text{sgn}(v_m^{c_2}) \frac{1 - \text{sgn}(\delta_m^{c_2})}{2} + \sum_{m=1}^{n_{f_1}} \text{sgn}(v_m^{f_1}) \frac{1 - \text{sgn}(\delta_m^{f_1})}{2} \\
& - \sum_{m=1}^{n_{h_1}} \text{sgn}(v_m^{h_1}) \frac{1 - \text{sgn}(\delta_m^{h_1})}{2} - \sum_{m=1}^{n_{h_2}} \text{sgn}(v_m^{h_2}) \frac{1 - \text{sgn}(\delta_m^{h_2})}{2}
\end{aligned} \tag{S109.5}$$

$$\begin{aligned}
\mathcal{W}_6^{\text{gapless}} = & \sum_{m=1}^{n_{d_1}} \text{sgn}(v_m^{d_1}) \frac{1 - \text{sgn}(\delta_m^{d_1})}{2} + \sum_{m=1}^{n_{d_2}} \text{sgn}(v_m^{d_2}) \frac{1 - \text{sgn}(\delta_m^{d_2})}{2} - 2 \sum_{m=1}^{n_{e_1}} \text{sgn}(v_m^{e_1}) \frac{1 - \text{sgn}(\delta_m^{e_1})}{2} \\
& - 2 \sum_{m=1}^{n_{g_2}} \text{sgn}(v_m^{g_2}) \frac{1 - \text{sgn}(\delta_m^{g_2})}{2} - 2 \sum_{m=1}^{n_{h_1}} \text{sgn}(v_m^{h_1}) \frac{1 - \text{sgn}(\delta_m^{h_1})}{2} + 2 \sum_{m=1}^{n_{h_2}} \text{sgn}(v_m^{h_2}) \frac{1 - \text{sgn}(\delta_m^{h_2})}{2}
\end{aligned} \tag{S109.6}$$

$$\begin{aligned}
\mathcal{W}_7^{\text{gapless}} = & \sum_{m=1}^{n_{g_1}} \text{sgn}(v_m^{g_1}) \frac{1 - \text{sgn}(\delta_m^{g_1})}{2} - \sum_{m=1}^{n_{g_2}} \text{sgn}(v_m^{g_2}) \frac{1 - \text{sgn}(\delta_m^{g_2})}{2} - 2 \sum_{m=1}^{n_{h_1}} \text{sgn}(v_m^{h_1}) \frac{1 - \text{sgn}(\delta_m^{h_1})}{2} \\
& + 2 \sum_{m=1}^{n_{h_2}} \text{sgn}(v_m^{h_2}) \frac{1 - \text{sgn}(\delta_m^{h_2})}{2}
\end{aligned} \tag{S109.7}$$

$$\mathcal{W}_1^{\text{gapped}} = - \sum_{m=1}^{n_{h_1}} \text{sgn}(v_m^{h_1}) \frac{1 - \text{sgn}(\delta_m^{h_1})}{2} + \sum_{m=1}^{n_{h_2}} \text{sgn}(v_m^{h_2}) \frac{1 - \text{sgn}(\delta_m^{h_2})}{2} \tag{S109.8}$$

$$\mathcal{X}_1 = \sum_{m=1}^{n_{d_2}} \frac{1 - \text{sgn}(\delta_m^{d_2})}{2} + \sum_{m=1}^{n_{g_2}} \frac{1 - \text{sgn}(\delta_m^{g_2})}{2} \mod 2 \tag{S109.9}$$

### S110. SPACE GROUP NO. 110

| line segment                                      | character of irrep (generators only)          |                                               |
|---------------------------------------------------|-----------------------------------------------|-----------------------------------------------|
| $a \quad (0, 0, t)$                               | $\{4_{001}   0 \ \frac{1}{2} \ \frac{1}{4}\}$ | $\{m_{100}   0 \ 0 \ \frac{1}{2}\}$           |
|                                                   | $a_1 \quad -\sqrt{2}e^{-\frac{1}{2}i\pi t}$   | 0                                             |
|                                                   | $a_2 \quad \sqrt{2}e^{-\frac{1}{2}i\pi t}$    | 0                                             |
| $b \quad (\frac{1}{2}, \frac{1}{2}, \frac{t}{2})$ | $\{2_{001}   0 \ 0 \ 0\}$                     | $\{m_{110}   \frac{1}{2} \ 0 \ \frac{1}{4}\}$ |
|                                                   | $b_1 \quad -i$                                | $-e^{-\frac{1}{4}i\pi(t+2)}$                  |
|                                                   | $b_2 \quad -i$                                | $e^{-\frac{1}{4}i\pi(t+2)}$                   |
|                                                   | $b_3 \quad i$                                 | $-e^{-\frac{1}{4}i\pi(t+2)}$                  |
|                                                   | $b_4 \quad i$                                 | $e^{-\frac{1}{4}i\pi(t+2)}$                   |

|                                                       |                                                                                                                                                             |
|-------------------------------------------------------|-------------------------------------------------------------------------------------------------------------------------------------------------------------|
| $c \quad (\frac{t}{2}, \frac{t}{2}, 1 - \frac{t}{2})$ | $c_1 \quad \begin{cases} \{m_{1-10}   \frac{1}{2} & 0 & \frac{1}{4}\} \\ -ie^{-\frac{1}{4}i\pi(t+2)} \end{cases}$<br>$c_2 \quad ie^{-\frac{1}{4}i\pi(t+2)}$ |
| $d \quad (\frac{t}{2}, \frac{t}{2}, 0)$               | $d_1 \quad \begin{cases} \{m_{1-10}   \frac{1}{2} & 0 & \frac{1}{4}\} \\ -ie^{-\frac{1}{2}i\pi t} \end{cases}$<br>$d_2 \quad ie^{-\frac{1}{2}i\pi t}$       |
| $e \quad (\frac{t}{2}, 1 - \frac{t}{2}, 0)$           | $e_1 \quad \begin{cases} \{m_{110}   \frac{1}{2} & 0 & \frac{1}{4}\} \\ -e^{-\frac{1}{2}i\pi t} \end{cases}$<br>$e_2 \quad e^{-\frac{1}{2}i\pi t}$          |
| $f \quad (\frac{1-t}{2}, \frac{1}{2}, \frac{1}{2})$   | $f_1 \quad \begin{cases} \{1   0 & 0 & 0\} \\ 1 \end{cases}$                                                                                                |
| $g \quad (0, t, 0)$                                   | $g_1 \quad \begin{cases} \{m_{100}   0 & 0 & \frac{1}{2}\} \\ -i \end{cases}$<br>$g_2 \quad i$                                                              |
| $h \quad (0, \frac{t}{2}, 1 - \frac{t}{2})$           | $h_1 \quad \begin{cases} \{m_{100}   0 & 0 & \frac{1}{2}\} \\ -ie^{-\frac{1}{2}i\pi(2-t)} \end{cases}$<br>$h_2 \quad ie^{-\frac{1}{2}i\pi(2-t)}$            |

$$\mathcal{W}_1^{\text{gapless}} = \sum_{m=1}^{n_{a_1}} \text{sgn}(v_m^{a_1}) \frac{1 - \text{sgn}(\delta_m^{a_1})}{2} + \sum_{m=1}^{n_{a_2}} \text{sgn}(v_m^{a_2}) \frac{1 - \text{sgn}(\delta_m^{a_2})}{2} - \sum_{m=1}^{n_{g_2}} \text{sgn}(v_m^{g_2}) \frac{1 - \text{sgn}(\delta_m^{g_2})}{2} \quad (\text{S110.1})$$

$$\begin{aligned} \mathcal{W}_2^{\text{gapless}} = & \sum_{m=1}^{n_{b_1}} \text{sgn}(v_m^{b_1}) \frac{1 - \text{sgn}(\delta_m^{b_1})}{2} + \sum_{m=1}^{n_{b_4}} \text{sgn}(v_m^{b_4}) \frac{1 - \text{sgn}(\delta_m^{b_4})}{2} - \sum_{m=1}^{n_{c_2}} \text{sgn}(v_m^{c_2}) \frac{1 - \text{sgn}(\delta_m^{c_2})}{2} \\ & + \sum_{m=1}^{n_{d_2}} \text{sgn}(v_m^{d_2}) \frac{1 - \text{sgn}(\delta_m^{d_2})}{2} - \sum_{m=1}^{n_{g_2}} \text{sgn}(v_m^{g_2}) \frac{1 - \text{sgn}(\delta_m^{g_2})}{2} \end{aligned} \quad (\text{S110.2})$$

$$\mathcal{W}_3^{\text{gapless}} = \sum_{m=1}^{n_{b_2}} \text{sgn}(v_m^{b_2}) \frac{1 - \text{sgn}(\delta_m^{b_2})}{2} + \sum_{m=1}^{n_{b_4}} \text{sgn}(v_m^{b_4}) \frac{1 - \text{sgn}(\delta_m^{b_4})}{2} - \sum_{m=1}^{n_{c_2}} \text{sgn}(v_m^{c_2}) \frac{1 - \text{sgn}(\delta_m^{c_2})}{2} + \sum_{m=1}^{n_{e_1}} \text{sgn}(v_m^{e_1}) \frac{1 - \text{sgn}(\delta_m^{e_1})}{2} \quad (\text{S110.3})$$

$$\begin{aligned} \mathcal{W}_4^{\text{gapless}} = & \sum_{m=1}^{n_{b_3}} \text{sgn}(v_m^{b_3}) \frac{1 - \text{sgn}(\delta_m^{b_3})}{2} - \sum_{m=1}^{n_{b_4}} \text{sgn}(v_m^{b_4}) \frac{1 - \text{sgn}(\delta_m^{b_4})}{2} + 2 \sum_{m=1}^{n_{c_2}} \text{sgn}(v_m^{c_2}) \frac{1 - \text{sgn}(\delta_m^{c_2})}{2} \\ & - \sum_{m=1}^{n_{d_2}} \text{sgn}(v_m^{d_2}) \frac{1 - \text{sgn}(\delta_m^{d_2})}{2} + \sum_{m=1}^{n_{e_1}} \text{sgn}(v_m^{e_1}) \frac{1 - \text{sgn}(\delta_m^{e_1})}{2} + 2 \sum_{m=1}^{n_{f_1}} \text{sgn}(v_m^{f_1}) \frac{1 - \text{sgn}(\delta_m^{f_1})}{2} \\ & + \sum_{m=1}^{n_{g_2}} \text{sgn}(v_m^{g_2}) \frac{1 - \text{sgn}(\delta_m^{g_2})}{2} - \sum_{m=1}^{n_{h_1}} \text{sgn}(v_m^{h_1}) \frac{1 - \text{sgn}(\delta_m^{h_1})}{2} - \sum_{m=1}^{n_{h_2}} \text{sgn}(v_m^{h_2}) \frac{1 - \text{sgn}(\delta_m^{h_2})}{2} \end{aligned} \quad (\text{S110.4})$$

$$\begin{aligned} \mathcal{W}_5^{\text{gapless}} = & \sum_{m=1}^{n_{c_1}} \text{sgn}(v_m^{c_1}) \frac{1 - \text{sgn}(\delta_m^{c_1})}{2} + \sum_{m=1}^{n_{c_2}} \text{sgn}(v_m^{c_2}) \frac{1 - \text{sgn}(\delta_m^{c_2})}{2} + 2 \sum_{m=1}^{n_{f_1}} \text{sgn}(v_m^{f_1}) \frac{1 - \text{sgn}(\delta_m^{f_1})}{2} \\ & - \sum_{m=1}^{n_{h_1}} \text{sgn}(v_m^{h_1}) \frac{1 - \text{sgn}(\delta_m^{h_1})}{2} - \sum_{m=1}^{n_{h_2}} \text{sgn}(v_m^{h_2}) \frac{1 - \text{sgn}(\delta_m^{h_2})}{2} \end{aligned} \quad (\text{S110.5})$$



$$\begin{aligned} \mathcal{W}_6^{\text{gapless}} = & \sum_{m=1}^{n_{d_1}} \text{sgn}(v_m^{d_1}) \frac{1 - \text{sgn}(\delta_m^{d_1})}{2} + \sum_{m=1}^{n_{d_2}} \text{sgn}(v_m^{d_2}) \frac{1 - \text{sgn}(\delta_m^{d_2})}{2} - 2 \sum_{m=1}^{n_{e_1}} \text{sgn}(v_m^{e_1}) \frac{1 - \text{sgn}(\delta_m^{e_1})}{2} \\ & - 2 \sum_{m=1}^{n_{g_2}} \text{sgn}(v_m^{g_2}) \frac{1 - \text{sgn}(\delta_m^{g_2})}{2} \end{aligned} \quad (\text{S110.6})$$

$$\mathcal{W}_7^{\text{gapless}} = \sum_{m=1}^{n_{g_1}} \text{sgn}(v_m^{g_1}) \frac{1 - \text{sgn}(\delta_m^{g_1})}{2} - \sum_{m=1}^{n_{g_2}} \text{sgn}(v_m^{g_2}) \frac{1 - \text{sgn}(\delta_m^{g_2})}{2} \quad (\text{S110.7})$$

$$\mathcal{X}_1 = \sum_{m=1}^{n_{h_2}} \frac{1 - \text{sgn}(\delta_m^{h_2})}{2} \mod 2 \quad (\text{S110.8})$$

$$\mathcal{X}_2 = \sum_{m=1}^{n_{d_2}} \frac{1 - \text{sgn}(\delta_m^{d_2})}{2} + \sum_{m=1}^{n_{g_2}} \frac{1 - \text{sgn}(\delta_m^{g_2})}{2} \mod 2 \quad (\text{S110.9})$$

$$\mathcal{X}_3 = \sum_{m=1}^{n_{h_1}} \frac{1 - \text{sgn}(\delta_m^{h_1})}{2} \mod 2 \quad (\text{S110.10})$$

### S111. SPACE GROUP NO. 111

| line segment                                        | character of irrep (generators only)                                                           |
|-----------------------------------------------------|------------------------------------------------------------------------------------------------|
| $a \quad (0, \frac{t}{2}, 0)$                       | $\begin{matrix} \{2_{010}   0 & 0 & 0\} \\ a_1 & -i \\ a_2 & i \end{matrix}$                   |
| $b \quad (\frac{1-t}{2}, \frac{1}{2}, 0)$           | $\begin{matrix} \{2_{100}   0 & 0 & 0\} \\ b_1 & -i \\ b_2 & i \end{matrix}$                   |
| $c \quad (\frac{t}{2}, \frac{t}{2}, 0)$             | $\begin{matrix} \{m_{1-10}   0 & 0 & 0\} \\ c_1 & -i \\ c_2 & i \end{matrix}$                  |
| $d \quad (0, \frac{t}{2}, \frac{1}{2})$             | $\begin{matrix} \{2_{010}   0 & 0 & 0\} \\ d_1 & -i \\ d_2 & i \end{matrix}$                   |
| $e \quad (\frac{1-t}{2}, \frac{1}{2}, \frac{1}{2})$ | $\begin{matrix} \{2_{100}   0 & 0 & 0\} \\ e_1 & -i \\ e_2 & i \end{matrix}$                   |
| $f \quad (\frac{t}{2}, \frac{t}{2}, \frac{1}{2})$   | $\begin{matrix} \{m_{1-10}   0 & 0 & 0\} \\ f_1 & -i \\ f_2 & i \end{matrix}$                  |
| $g \quad (0, 0, \frac{t}{2})$                       | $\begin{matrix} \{2_{001}   0 & 0 & 0\} & \{m_{110}   0 & 0 & 0\} \\ g_1 & 0 & 0 \end{matrix}$ |
| $h \quad (0, \frac{1}{2}, \frac{t}{2})$             | $\begin{matrix} \{2_{001}   0 & 0 & 0\} \\ h_1 & -i \\ h_2 & i \end{matrix}$                   |
| $i \quad (\frac{1}{2}, \frac{1}{2}, \frac{t}{2})$   | $\begin{matrix} \{2_{001}   0 & 0 & 0\} & \{m_{110}   0 & 0 & 0\} \\ i_1 & 0 & 0 \end{matrix}$ |

---


$$\begin{aligned}
\mathcal{W}_1^{\text{gapless}} = & \sum_{m=1}^{n_{a_1}} \text{sgn}(v_m^{a_1}) \frac{1 - \text{sgn}(\delta_m^{a_1})}{2} + \sum_{m=1}^{n_{a_2}} \text{sgn}(v_m^{a_2}) \frac{1 - \text{sgn}(\delta_m^{a_2})}{2} - \sum_{m=1}^{n_{e_1}} \text{sgn}(v_m^{e_1}) \frac{1 - \text{sgn}(\delta_m^{e_1})}{2} \\
& - \sum_{m=1}^{n_{e_2}} \text{sgn}(v_m^{e_2}) \frac{1 - \text{sgn}(\delta_m^{e_2})}{2} - \sum_{m=1}^{n_{f_1}} \text{sgn}(v_m^{f_1}) \frac{1 - \text{sgn}(\delta_m^{f_1})}{2} - \sum_{m=1}^{n_{f_2}} \text{sgn}(v_m^{f_2}) \frac{1 - \text{sgn}(\delta_m^{f_2})}{2} \\
& - 2 \sum_{m=1}^{n_{g_1}} \text{sgn}(v_m^{g_1}) \frac{1 - \text{sgn}(\delta_m^{g_1})}{2} + \sum_{m=1}^{n_{h_1}} \text{sgn}(v_m^{h_1}) \frac{1 - \text{sgn}(\delta_m^{h_1})}{2} + \sum_{m=1}^{n_{h_2}} \text{sgn}(v_m^{h_2}) \frac{1 - \text{sgn}(\delta_m^{h_2})}{2}
\end{aligned} \tag{S111.1}$$

$$\begin{aligned}
\mathcal{W}_2^{\text{gapless}} = & \sum_{m=1}^{n_{b_1}} \text{sgn}(v_m^{b_1}) \frac{1 - \text{sgn}(\delta_m^{b_1})}{2} + \sum_{m=1}^{n_{b_2}} \text{sgn}(v_m^{b_2}) \frac{1 - \text{sgn}(\delta_m^{b_2})}{2} - \sum_{m=1}^{n_{e_1}} \text{sgn}(v_m^{e_1}) \frac{1 - \text{sgn}(\delta_m^{e_1})}{2} - \sum_{m=1}^{n_{e_2}} \text{sgn}(v_m^{e_2}) \frac{1 - \text{sgn}(\delta_m^{e_2})}{2} \\
& + \sum_{m=1}^{n_{h_1}} \text{sgn}(v_m^{h_1}) \frac{1 - \text{sgn}(\delta_m^{h_1})}{2} + \sum_{m=1}^{n_{h_2}} \text{sgn}(v_m^{h_2}) \frac{1 - \text{sgn}(\delta_m^{h_2})}{2} - 2 \sum_{m=1}^{n_{i_1}} \text{sgn}(v_m^{i_1}) \frac{1 - \text{sgn}(\delta_m^{i_1})}{2}
\end{aligned} \tag{S111.2}$$

$$\mathcal{W}_3^{\text{gapless}} = \sum_{m=1}^{n_{c_1}} \text{sgn}(v_m^{c_1}) \frac{1 - \text{sgn}(\delta_m^{c_1})}{2} - \sum_{m=1}^{n_{f_1}} \text{sgn}(v_m^{f_1}) \frac{1 - \text{sgn}(\delta_m^{f_1})}{2} - \sum_{m=1}^{n_{g_1}} \text{sgn}(v_m^{g_1}) \frac{1 - \text{sgn}(\delta_m^{g_1})}{2} + \sum_{m=1}^{n_{i_1}} \text{sgn}(v_m^{i_1}) \frac{1 - \text{sgn}(\delta_m^{i_1})}{2} \tag{S111.3}$$

$$\mathcal{W}_4^{\text{gapless}} = \sum_{m=1}^{n_{c_2}} \text{sgn}(v_m^{c_2}) \frac{1 - \text{sgn}(\delta_m^{c_2})}{2} - \sum_{m=1}^{n_{f_2}} \text{sgn}(v_m^{f_2}) \frac{1 - \text{sgn}(\delta_m^{f_2})}{2} - \sum_{m=1}^{n_{g_1}} \text{sgn}(v_m^{g_1}) \frac{1 - \text{sgn}(\delta_m^{g_1})}{2} + \sum_{m=1}^{n_{i_1}} \text{sgn}(v_m^{i_1}) \frac{1 - \text{sgn}(\delta_m^{i_1})}{2} \tag{S111.4}$$

$$\begin{aligned}
\mathcal{W}_5^{\text{gapless}} = & \sum_{m=1}^{n_{d_1}} \text{sgn}(v_m^{d_1}) \frac{1 - \text{sgn}(\delta_m^{d_1})}{2} + \sum_{m=1}^{n_{d_2}} \text{sgn}(v_m^{d_2}) \frac{1 - \text{sgn}(\delta_m^{d_2})}{2} - \sum_{m=1}^{n_{e_1}} \text{sgn}(v_m^{e_1}) \frac{1 - \text{sgn}(\delta_m^{e_1})}{2} \\
& - \sum_{m=1}^{n_{e_2}} \text{sgn}(v_m^{e_2}) \frac{1 - \text{sgn}(\delta_m^{e_2})}{2} - \sum_{m=1}^{n_{f_1}} \text{sgn}(v_m^{f_1}) \frac{1 - \text{sgn}(\delta_m^{f_1})}{2} - \sum_{m=1}^{n_{f_2}} \text{sgn}(v_m^{f_2}) \frac{1 - \text{sgn}(\delta_m^{f_2})}{2}
\end{aligned} \tag{S111.5}$$

$$\begin{aligned}
\mathcal{W}_1^{\text{gapped}} = & - \sum_{m=1}^{n_{a_2}} \text{sgn}(v_m^{a_2}) \frac{1 - \text{sgn}(\delta_m^{a_2})}{2} + \sum_{m=1}^{n_{e_2}} \text{sgn}(v_m^{e_2}) \frac{1 - \text{sgn}(\delta_m^{e_2})}{2} + \sum_{m=1}^{n_{f_1}} \text{sgn}(v_m^{f_1}) \frac{1 - \text{sgn}(\delta_m^{f_1})}{2} \\
& + \sum_{m=1}^{n_{g_1}} \text{sgn}(v_m^{g_1}) \frac{1 - \text{sgn}(\delta_m^{g_1})}{2} - \sum_{m=1}^{n_{h_1}} \text{sgn}(v_m^{h_1}) \frac{1 - \text{sgn}(\delta_m^{h_1})}{2}
\end{aligned} \tag{S111.6}$$

$$\begin{aligned}
\mathcal{W}_2^{\text{gapped}} = & - \sum_{m=1}^{n_{a_2}} \text{sgn}(v_m^{a_2}) \frac{1 - \text{sgn}(\delta_m^{a_2})}{2} + \sum_{m=1}^{n_{e_2}} \text{sgn}(v_m^{e_2}) \frac{1 - \text{sgn}(\delta_m^{e_2})}{2} + \sum_{m=1}^{n_{f_2}} \text{sgn}(v_m^{f_2}) \frac{1 - \text{sgn}(\delta_m^{f_2})}{2} \\
& + \sum_{m=1}^{n_{g_1}} \text{sgn}(v_m^{g_1}) \frac{1 - \text{sgn}(\delta_m^{g_1})}{2} - \sum_{m=1}^{n_{h_1}} \text{sgn}(v_m^{h_1}) \frac{1 - \text{sgn}(\delta_m^{h_1})}{2}
\end{aligned} \tag{S111.7}$$

$$\mathcal{W}_3^{\text{gapped}} = \sum_{m=1}^{n_{e_1}} \text{sgn}(v_m^{e_1}) \frac{1 - \text{sgn}(\delta_m^{e_1})}{2} - \sum_{m=1}^{n_{e_2}} \text{sgn}(v_m^{e_2}) \frac{1 - \text{sgn}(\delta_m^{e_2})}{2} \quad (\text{S111.8})$$

$$\begin{aligned} \mathcal{W}_4^{\text{gapped}} = & - \sum_{m=1}^{n_{a_2}} \text{sgn}(v_m^{a_2}) \frac{1 - \text{sgn}(\delta_m^{a_2})}{2} + \sum_{m=1}^{n_{d_2}} \text{sgn}(v_m^{d_2}) \frac{1 - \text{sgn}(\delta_m^{d_2})}{2} + \sum_{m=1}^{n_{g_1}} \text{sgn}(v_m^{g_1}) \frac{1 - \text{sgn}(\delta_m^{g_1})}{2} \\ & - \sum_{m=1}^{n_{h_1}} \text{sgn}(v_m^{h_1}) \frac{1 - \text{sgn}(\delta_m^{h_1})}{2} \end{aligned} \quad (\text{S111.9})$$

$$\mathcal{W}_5^{\text{gapped}} = - \sum_{m=1}^{n_{h_1}} \text{sgn}(v_m^{h_1}) \frac{1 - \text{sgn}(\delta_m^{h_1})}{2} + \sum_{m=1}^{n_{h_2}} \text{sgn}(v_m^{h_2}) \frac{1 - \text{sgn}(\delta_m^{h_2})}{2} \quad (\text{S111.10})$$

$$\begin{aligned} \mathcal{W}_6^{\text{gapped}} = & - \sum_{m=1}^{n_{b_2}} \text{sgn}(v_m^{b_2}) \frac{1 - \text{sgn}(\delta_m^{b_2})}{2} + \sum_{m=1}^{n_{e_2}} \text{sgn}(v_m^{e_2}) \frac{1 - \text{sgn}(\delta_m^{e_2})}{2} - \sum_{m=1}^{n_{h_1}} \text{sgn}(v_m^{h_1}) \frac{1 - \text{sgn}(\delta_m^{h_1})}{2} \\ & + \sum_{m=1}^{n_{i_1}} \text{sgn}(v_m^{i_1}) \frac{1 - \text{sgn}(\delta_m^{i_1})}{2} \end{aligned} \quad (\text{S111.11})$$

## S112. SPACE GROUP NO. 112

| line segment                                        | character of irrep (generators only)                                                                                  |
|-----------------------------------------------------|-----------------------------------------------------------------------------------------------------------------------|
| $a \quad (0, \frac{t}{2}, 0)$                       | $\begin{array}{c} \{2_{010}   0 \ 0 \ \frac{1}{2}\} \\ a_1 \quad -i \\ a_2 \quad i \end{array}$                       |
| $b \quad (\frac{1-t}{2}, \frac{1}{2}, 0)$           | $\begin{array}{c} \{2_{100}   0 \ 0 \ \frac{1}{2}\} \\ b_1 \quad -i \\ b_2 \quad i \end{array}$                       |
| $c \quad (\frac{t}{2}, \frac{t}{2}, 0)$             | $\begin{array}{c} \{m_{1-10}   0 \ 0 \ \frac{1}{2}\} \\ c_1 \quad -i \\ c_2 \quad i \end{array}$                      |
| $d \quad (0, \frac{t}{2}, \frac{1}{2})$             | $\begin{array}{c} \{2_{010}   0 \ 0 \ \frac{1}{2}\} \\ d_1 \quad i \\ d_2 \quad -i \end{array}$                       |
| $e \quad (\frac{1-t}{2}, \frac{1}{2}, \frac{1}{2})$ | $\begin{array}{c} \{2_{100}   0 \ 0 \ \frac{1}{2}\} \\ e_1 \quad i \\ e_2 \quad -i \end{array}$                       |
| $f \quad (\frac{t}{2}, \frac{t}{2}, \frac{1}{2})$   | $\begin{array}{c} \{m_{1-10}   0 \ 0 \ \frac{1}{2}\} \\ f_1 \quad -1 \\ f_2 \quad 1 \end{array}$                      |
| $g \quad (0, 0, \frac{t}{2})$                       | $\begin{array}{c} \{2_{001}   0 \ 0 \ 0\} \quad \{m_{110}   0 \ 0 \ \frac{1}{2}\} \\ g_1 \quad 0 \quad 0 \end{array}$ |
| $h \quad (0, \frac{1}{2}, \frac{t}{2})$             | $\begin{array}{c} \{2_{001}   0 \ 0 \ 0\} \\ h_1 \quad -i \\ h_2 \quad i \end{array}$                                 |
| $i \quad (\frac{1}{2}, \frac{1}{2}, \frac{t}{2})$   | $\begin{array}{c} \{2_{001}   0 \ 0 \ 0\} \quad \{m_{110}   0 \ 0 \ \frac{1}{2}\} \\ i_1 \quad 0 \quad 0 \end{array}$ |

$$\begin{aligned}
\mathcal{W}_1^{\text{gapless}} = & \sum_{m=1}^{n_{a_1}} \text{sgn}(v_m^{a_1}) \frac{1 - \text{sgn}(\delta_m^{a_1})}{2} + \sum_{m=1}^{n_{a_2}} \text{sgn}(v_m^{a_2}) \frac{1 - \text{sgn}(\delta_m^{a_2})}{2} - \sum_{m=1}^{n_{e_1}} \text{sgn}(v_m^{e_1}) \frac{1 - \text{sgn}(\delta_m^{e_1})}{2} \\
& - \sum_{m=1}^{n_{e_2}} \text{sgn}(v_m^{e_2}) \frac{1 - \text{sgn}(\delta_m^{e_2})}{2} - 2 \sum_{m=1}^{n_{f_1}} \text{sgn}(v_m^{f_1}) \frac{1 - \text{sgn}(\delta_m^{f_1})}{2} - 2 \sum_{m=1}^{n_{g_1}} \text{sgn}(v_m^{g_1}) \frac{1 - \text{sgn}(\delta_m^{g_1})}{2} \\
& + \sum_{m=1}^{n_{h_1}} \text{sgn}(v_m^{h_1}) \frac{1 - \text{sgn}(\delta_m^{h_1})}{2} + \sum_{m=1}^{n_{h_2}} \text{sgn}(v_m^{h_2}) \frac{1 - \text{sgn}(\delta_m^{h_2})}{2}
\end{aligned} \tag{S112.1}$$

$$\begin{aligned}
\mathcal{W}_2^{\text{gapless}} = & \sum_{m=1}^{n_{b_1}} \text{sgn}(v_m^{b_1}) \frac{1 - \text{sgn}(\delta_m^{b_1})}{2} + \sum_{m=1}^{n_{b_2}} \text{sgn}(v_m^{b_2}) \frac{1 - \text{sgn}(\delta_m^{b_2})}{2} - \sum_{m=1}^{n_{e_1}} \text{sgn}(v_m^{e_1}) \frac{1 - \text{sgn}(\delta_m^{e_1})}{2} - \sum_{m=1}^{n_{e_2}} \text{sgn}(v_m^{e_2}) \frac{1 - \text{sgn}(\delta_m^{e_2})}{2} \\
& + \sum_{m=1}^{n_{h_1}} \text{sgn}(v_m^{h_1}) \frac{1 - \text{sgn}(\delta_m^{h_1})}{2} + \sum_{m=1}^{n_{h_2}} \text{sgn}(v_m^{h_2}) \frac{1 - \text{sgn}(\delta_m^{h_2})}{2} - 2 \sum_{m=1}^{n_{i_1}} \text{sgn}(v_m^{i_1}) \frac{1 - \text{sgn}(\delta_m^{i_1})}{2}
\end{aligned} \tag{S112.2}$$

$$\mathcal{W}_3^{\text{gapless}} = \sum_{m=1}^{n_{c_1}} \text{sgn}(v_m^{c_1}) \frac{1 - \text{sgn}(\delta_m^{c_1})}{2} - \sum_{m=1}^{n_{f_1}} \text{sgn}(v_m^{f_1}) \frac{1 - \text{sgn}(\delta_m^{f_1})}{2} - \sum_{m=1}^{n_{g_1}} \text{sgn}(v_m^{g_1}) \frac{1 - \text{sgn}(\delta_m^{g_1})}{2} + \sum_{m=1}^{n_{i_1}} \text{sgn}(v_m^{i_1}) \frac{1 - \text{sgn}(\delta_m^{i_1})}{2} \tag{S112.3}$$

$$\mathcal{W}_4^{\text{gapless}} = \sum_{m=1}^{n_{c_2}} \text{sgn}(v_m^{c_2}) \frac{1 - \text{sgn}(\delta_m^{c_2})}{2} - \sum_{m=1}^{n_{f_1}} \text{sgn}(v_m^{f_1}) \frac{1 - \text{sgn}(\delta_m^{f_1})}{2} - \sum_{m=1}^{n_{g_1}} \text{sgn}(v_m^{g_1}) \frac{1 - \text{sgn}(\delta_m^{g_1})}{2} + \sum_{m=1}^{n_{i_1}} \text{sgn}(v_m^{i_1}) \frac{1 - \text{sgn}(\delta_m^{i_1})}{2} \tag{S112.4}$$

$$\begin{aligned}
\mathcal{W}_5^{\text{gapless}} = & \sum_{m=1}^{n_{d_1}} \text{sgn}(v_m^{d_1}) \frac{1 - \text{sgn}(\delta_m^{d_1})}{2} + \sum_{m=1}^{n_{d_2}} \text{sgn}(v_m^{d_2}) \frac{1 - \text{sgn}(\delta_m^{d_2})}{2} - \sum_{m=1}^{n_{e_1}} \text{sgn}(v_m^{e_1}) \frac{1 - \text{sgn}(\delta_m^{e_1})}{2} \\
& - \sum_{m=1}^{n_{e_2}} \text{sgn}(v_m^{e_2}) \frac{1 - \text{sgn}(\delta_m^{e_2})}{2} - 2 \sum_{m=1}^{n_{f_1}} \text{sgn}(v_m^{f_1}) \frac{1 - \text{sgn}(\delta_m^{f_1})}{2}
\end{aligned} \tag{S112.5}$$

$$\mathcal{W}_1^{\text{gapped}} = \sum_{m=1}^{n_{e_1}} \text{sgn}(v_m^{e_1}) \frac{1 - \text{sgn}(\delta_m^{e_1})}{2} - \sum_{m=1}^{n_{e_2}} \text{sgn}(v_m^{e_2}) \frac{1 - \text{sgn}(\delta_m^{e_2})}{2} \tag{S112.6}$$

$$\mathcal{W}_2^{\text{gapped}} = \sum_{m=1}^{n_{d_2}} \text{sgn}(v_m^{d_2}) \frac{1 - \text{sgn}(\delta_m^{d_2})}{2} - \sum_{m=1}^{n_{e_2}} \text{sgn}(v_m^{e_2}) \frac{1 - \text{sgn}(\delta_m^{e_2})}{2} - \sum_{m=1}^{n_{f_1}} \text{sgn}(v_m^{f_1}) \frac{1 - \text{sgn}(\delta_m^{f_1})}{2} \tag{S112.7}$$

$$\begin{aligned}
\mathcal{W}_3^{\text{gapped}} = & \sum_{m=1}^{n_{a_2}} \text{sgn}(v_m^{a_2}) \frac{1 - \text{sgn}(\delta_m^{a_2})}{2} - \sum_{m=1}^{n_{e_2}} \text{sgn}(v_m^{e_2}) \frac{1 - \text{sgn}(\delta_m^{e_2})}{2} - \sum_{m=1}^{n_{f_1}} \text{sgn}(v_m^{f_1}) \frac{1 - \text{sgn}(\delta_m^{f_1})}{2} \\
& - \sum_{m=1}^{n_{g_1}} \text{sgn}(v_m^{g_1}) \frac{1 - \text{sgn}(\delta_m^{g_1})}{2} + \sum_{m=1}^{n_{h_1}} \text{sgn}(v_m^{h_1}) \frac{1 - \text{sgn}(\delta_m^{h_1})}{2}
\end{aligned} \tag{S112.8}$$

$$\begin{aligned} \mathcal{W}_4^{\text{gapped}} = & \sum_{m=1}^{n_{a_2}} \text{sgn}(v_m^{a_2}) \frac{1 - \text{sgn}(\delta_m^{a_2})}{2} - \sum_{m=1}^{n_{e_2}} \text{sgn}(v_m^{e_2}) \frac{1 - \text{sgn}(\delta_m^{e_2})}{2} - \sum_{m=1}^{n_{f_1}} \text{sgn}(v_m^{f_1}) \frac{1 - \text{sgn}(\delta_m^{f_1})}{2} \\ & - \sum_{m=1}^{n_{g_1}} \text{sgn}(v_m^{g_1}) \frac{1 - \text{sgn}(\delta_m^{g_1})}{2} + \sum_{m=1}^{n_{h_2}} \text{sgn}(v_m^{h_2}) \frac{1 - \text{sgn}(\delta_m^{h_2})}{2} \end{aligned} \quad (\text{S112.9})$$

$$\begin{aligned} \mathcal{W}_5^{\text{gapped}} = & \sum_{m=1}^{n_{a_2}} \text{sgn}(v_m^{a_2}) \frac{1 - \text{sgn}(\delta_m^{a_2})}{2} - \sum_{m=1}^{n_{b_2}} \text{sgn}(v_m^{b_2}) \frac{1 - \text{sgn}(\delta_m^{b_2})}{2} - \sum_{m=1}^{n_{f_1}} \text{sgn}(v_m^{f_1}) \frac{1 - \text{sgn}(\delta_m^{f_1})}{2} \\ & - \sum_{m=1}^{n_{g_1}} \text{sgn}(v_m^{g_1}) \frac{1 - \text{sgn}(\delta_m^{g_1})}{2} + \sum_{m=1}^{n_{i_1}} \text{sgn}(v_m^{i_1}) \frac{1 - \text{sgn}(\delta_m^{i_1})}{2} \end{aligned} \quad (\text{S112.10})$$

$$\mathcal{X}_1 = \sum_{m=1}^{n_{f_1}} \frac{1 - \text{sgn}(\delta_m^{f_1})}{2} \quad \text{mod } 2 \quad (\text{S112.11})$$

### S113. SPACE GROUP NO. 113

| line segment                                        | character of irrep (generators only)                                                                                         |
|-----------------------------------------------------|------------------------------------------------------------------------------------------------------------------------------|
| $a \quad (0, \frac{t}{2}, 0)$                       | $\{2_{010}   \frac{1}{2} \frac{1}{2} 0\}$<br>$a_1 \quad -ie^{-\frac{1}{2}i\pi t}$<br>$a_2 \quad ie^{-\frac{1}{2}i\pi t}$     |
| $b \quad (\frac{1-t}{2}, \frac{1}{2}, 0)$           | $\{2_{100}   \frac{1}{2} \frac{1}{2} 0\}$<br>$b_1 \quad -e^{-\frac{1}{2}i\pi(2-t)}$<br>$b_2 \quad e^{-\frac{1}{2}i\pi(2-t)}$ |
| $c \quad (\frac{t}{2}, \frac{t}{2}, 0)$             | $\{m_{1-10}   \frac{1}{2} \frac{1}{2} 0\}$<br>$c_1 \quad -ie^{-i\pi t}$<br>$c_2 \quad ie^{-i\pi t}$                          |
| $d \quad (0, \frac{t}{2}, \frac{1}{2})$             | $\{2_{010}   \frac{1}{2} \frac{1}{2} 0\}$<br>$d_1 \quad -ie^{-\frac{1}{2}i\pi t}$<br>$d_2 \quad ie^{-\frac{1}{2}i\pi t}$     |
| $e \quad (\frac{1-t}{2}, \frac{1}{2}, \frac{1}{2})$ | $\{2_{100}   \frac{1}{2} \frac{1}{2} 0\}$<br>$e_1 \quad -e^{-\frac{1}{2}i\pi(2-t)}$<br>$e_2 \quad e^{-\frac{1}{2}i\pi(2-t)}$ |
| $f \quad (\frac{t}{2}, \frac{t}{2}, \frac{1}{2})$   | $\{m_{1-10}   \frac{1}{2} \frac{1}{2} 0\}$<br>$f_1 \quad -ie^{-i\pi t}$<br>$f_2 \quad ie^{-i\pi t}$                          |
| $g \quad (0, 0, \frac{t}{2})$                       | $\{2_{001}   0 \ 0 \ 0\} \quad \{m_{110}   \frac{1}{2} \frac{1}{2} 0\}$<br>$g_1 \quad 0 \quad 0$                             |
| $h \quad (0, \frac{1}{2}, \frac{t}{2})$             | $\{2_{001}   0 \ 0 \ 0\}$<br>$h_1 \quad -i$<br>$h_2 \quad i$                                                                 |
| $i \quad (\frac{1}{2}, \frac{1}{2}, \frac{t}{2})$   | $\{2_{001}   0 \ 0 \ 0\} \quad \{m_{110}   \frac{1}{2} \frac{1}{2} 0\}$<br>$i_1 \quad 0 \quad 0$                             |

---


$$\begin{aligned}
\mathcal{W}_1^{\text{gapless}} = & \sum_{m=1}^{n_{a_1}} \text{sgn}(v_m^{a_1}) \frac{1 - \text{sgn}(\delta_m^{a_1})}{2} + \sum_{m=1}^{n_{a_2}} \text{sgn}(v_m^{a_2}) \frac{1 - \text{sgn}(\delta_m^{a_2})}{2} - 2 \sum_{m=1}^{n_{e_1}} \text{sgn}(v_m^{e_1}) \frac{1 - \text{sgn}(\delta_m^{e_1})}{2} \\
& - \sum_{m=1}^{n_{f_1}} \text{sgn}(v_m^{f_1}) \frac{1 - \text{sgn}(\delta_m^{f_1})}{2} - \sum_{m=1}^{n_{f_2}} \text{sgn}(v_m^{f_2}) \frac{1 - \text{sgn}(\delta_m^{f_2})}{2} - 2 \sum_{m=1}^{n_{g_1}} \text{sgn}(v_m^{g_1}) \frac{1 - \text{sgn}(\delta_m^{g_1})}{2} \\
& + 2 \sum_{m=1}^{n_{h_1}} \text{sgn}(v_m^{h_1}) \frac{1 - \text{sgn}(\delta_m^{h_1})}{2}
\end{aligned} \tag{S113.1}$$

$$\mathcal{W}_2^{\text{gapless}} = \sum_{m=1}^{n_{b_1}} \text{sgn}(v_m^{b_1}) \frac{1 - \text{sgn}(\delta_m^{b_1})}{2} - \sum_{m=1}^{n_{e_1}} \text{sgn}(v_m^{e_1}) \frac{1 - \text{sgn}(\delta_m^{e_1})}{2} + \sum_{m=1}^{n_{h_1}} \text{sgn}(v_m^{h_1}) \frac{1 - \text{sgn}(\delta_m^{h_1})}{2} - 2 \sum_{m=1}^{n_{i_1}} \text{sgn}(v_m^{i_1}) \frac{1 - \text{sgn}(\delta_m^{i_1})}{2} \tag{S113.2}$$

$$\mathcal{W}_3^{\text{gapless}} = \sum_{m=1}^{n_{c_1}} \text{sgn}(v_m^{c_1}) \frac{1 - \text{sgn}(\delta_m^{c_1})}{2} - \sum_{m=1}^{n_{f_1}} \text{sgn}(v_m^{f_1}) \frac{1 - \text{sgn}(\delta_m^{f_1})}{2} - \sum_{m=1}^{n_{g_1}} \text{sgn}(v_m^{g_1}) \frac{1 - \text{sgn}(\delta_m^{g_1})}{2} + 2 \sum_{m=1}^{n_{i_1}} \text{sgn}(v_m^{i_1}) \frac{1 - \text{sgn}(\delta_m^{i_1})}{2} \tag{S113.3}$$

$$\mathcal{W}_4^{\text{gapless}} = \sum_{m=1}^{n_{c_2}} \text{sgn}(v_m^{c_2}) \frac{1 - \text{sgn}(\delta_m^{c_2})}{2} - \sum_{m=1}^{n_{f_2}} \text{sgn}(v_m^{f_2}) \frac{1 - \text{sgn}(\delta_m^{f_2})}{2} - \sum_{m=1}^{n_{g_1}} \text{sgn}(v_m^{g_1}) \frac{1 - \text{sgn}(\delta_m^{g_1})}{2} + 2 \sum_{m=1}^{n_{i_1}} \text{sgn}(v_m^{i_1}) \frac{1 - \text{sgn}(\delta_m^{i_1})}{2} \tag{S113.4}$$

$$\begin{aligned}
\mathcal{W}_5^{\text{gapless}} = & \sum_{m=1}^{n_{d_1}} \text{sgn}(v_m^{d_1}) \frac{1 - \text{sgn}(\delta_m^{d_1})}{2} + \sum_{m=1}^{n_{d_2}} \text{sgn}(v_m^{d_2}) \frac{1 - \text{sgn}(\delta_m^{d_2})}{2} - 2 \sum_{m=1}^{n_{e_1}} \text{sgn}(v_m^{e_1}) \frac{1 - \text{sgn}(\delta_m^{e_1})}{2} \\
& - \sum_{m=1}^{n_{f_1}} \text{sgn}(v_m^{f_1}) \frac{1 - \text{sgn}(\delta_m^{f_1})}{2} - \sum_{m=1}^{n_{f_2}} \text{sgn}(v_m^{f_2}) \frac{1 - \text{sgn}(\delta_m^{f_2})}{2}
\end{aligned} \tag{S113.5}$$

$$\mathcal{W}_1^{\text{gapped}} = \sum_{m=1}^{n_{f_1}} \text{sgn}(v_m^{f_1}) \frac{1 - \text{sgn}(\delta_m^{f_1})}{2} - \sum_{m=1}^{n_{f_2}} \text{sgn}(v_m^{f_2}) \frac{1 - \text{sgn}(\delta_m^{f_2})}{2} \tag{S113.6}$$

$$\mathcal{X}_1 = \sum_{m=1}^{n_{a_2}} \frac{1 - \text{sgn}(\delta_m^{a_2})}{2} + \sum_{m=1}^{n_{f_2}} \frac{1 - \text{sgn}(\delta_m^{f_2})}{2} + \sum_{m=1}^{n_{g_1}} \frac{1 - \text{sgn}(\delta_m^{g_1})}{2} \pmod{2} \tag{S113.7}$$

$$\mathcal{X}_2 = \sum_{m=1}^{n_{a_2}} \frac{1 - \text{sgn}(\delta_m^{a_2})}{2} + \sum_{m=1}^{n_{d_2}} \frac{1 - \text{sgn}(\delta_m^{d_2})}{2} + \sum_{m=1}^{n_{g_1}} \frac{1 - \text{sgn}(\delta_m^{g_1})}{2} \pmod{2} \tag{S113.8}$$

## S114. SPACE GROUP NO. 114

| line segment                                        | character of irrep (generators only)                                                                                                        |
|-----------------------------------------------------|---------------------------------------------------------------------------------------------------------------------------------------------|
| $a \quad (0, \frac{t}{2}, 0)$                       | $\{2_{010}   \frac{1}{2} \frac{1}{2} \frac{1}{2}\}$<br>$a_1 \quad -ie^{-\frac{1}{2}i\pi t}$<br>$a_2 \quad ie^{-\frac{1}{2}i\pi t}$          |
| $b \quad (\frac{1-t}{2}, \frac{1}{2}, 0)$           | $\{2_{100}   \frac{1}{2} \frac{1}{2} \frac{1}{2}\}$<br>$b_1 \quad -e^{-\frac{1}{2}i\pi(2-t)}$<br>$b_2 \quad e^{-\frac{1}{2}i\pi(2-t)}$      |
| $c \quad (\frac{t}{2}, \frac{t}{2}, 0)$             | $\{m_{1-10}   \frac{1}{2} \frac{1}{2} \frac{1}{2}\}$<br>$c_1 \quad -ie^{-i\pi t}$<br>$c_2 \quad ie^{-i\pi t}$                               |
| $d \quad (0, \frac{t}{2}, \frac{1}{2})$             | $\{2_{010}   \frac{1}{2} \frac{1}{2} \frac{1}{2}\}$<br>$d_1 \quad -e^{-\frac{1}{2}i\pi(t+1)}$<br>$d_2 \quad e^{-\frac{1}{2}i\pi(t+1)}$      |
| $e \quad (\frac{1-t}{2}, \frac{1}{2}, \frac{1}{2})$ | $\{2_{100}   \frac{1}{2} \frac{1}{2} \frac{1}{2}\}$<br>$e_1 \quad -ie^{-\frac{1}{2}i\pi(3-t)}$<br>$e_2 \quad ie^{-\frac{1}{2}i\pi(3-t)}$    |
| $f \quad (\frac{t}{2}, \frac{t}{2}, \frac{1}{2})$   | $\{m_{1-10}   \frac{1}{2} \frac{1}{2} \frac{1}{2}\}$<br>$f_1 \quad -ie^{-\frac{1}{2}i\pi(2t+1)}$<br>$f_2 \quad ie^{-\frac{1}{2}i\pi(2t+1)}$ |
| $g \quad (0, 0, \frac{t}{2})$                       | $\{2_{001}   0 \ 0 \ 0\} \quad \{m_{110}   \frac{1}{2} \frac{1}{2} \frac{1}{2}\}$<br>$g_1 \quad 0 \quad 0$                                  |
| $h \quad (0, \frac{1}{2}, \frac{t}{2})$             | $\{2_{001}   0 \ 0 \ 0\}$<br>$h_1 \quad -i$<br>$h_2 \quad i$                                                                                |
| $i \quad (\frac{1}{2}, \frac{1}{2}, \frac{t}{2})$   | $\{2_{001}   0 \ 0 \ 0\} \quad \{m_{110}   \frac{1}{2} \frac{1}{2} \frac{1}{2}\}$<br>$i_1 \quad 0 \quad 0$                                  |

$$\begin{aligned} \mathcal{W}_1^{\text{gapless}} = & \sum_{m=1}^{n_{a_1}} \text{sgn}(v_m^{a_1}) \frac{1 - \text{sgn}(\delta_m^{a_1})}{2} + \sum_{m=1}^{n_{a_2}} \text{sgn}(v_m^{a_2}) \frac{1 - \text{sgn}(\delta_m^{a_2})}{2} - 2 \sum_{m=1}^{n_{e_1}} \text{sgn}(v_m^{e_1}) \frac{1 - \text{sgn}(\delta_m^{e_1})}{2} \\ & - 2 \sum_{m=1}^{n_{f_1}} \text{sgn}(v_m^{f_1}) \frac{1 - \text{sgn}(\delta_m^{f_1})}{2} - 2 \sum_{m=1}^{n_{g_1}} \text{sgn}(v_m^{g_1}) \frac{1 - \text{sgn}(\delta_m^{g_1})}{2} + 2 \sum_{m=1}^{n_{h_1}} \text{sgn}(v_m^{h_1}) \frac{1 - \text{sgn}(\delta_m^{h_1})}{2} \end{aligned} \quad (\text{S114.1})$$

$$\mathcal{W}_2^{\text{gapless}} = \sum_{m=1}^{n_{b_1}} \text{sgn}(v_m^{b_1}) \frac{1 - \text{sgn}(\delta_m^{b_1})}{2} - \sum_{m=1}^{n_{e_1}} \text{sgn}(v_m^{e_1}) \frac{1 - \text{sgn}(\delta_m^{e_1})}{2} + \sum_{m=1}^{n_{h_1}} \text{sgn}(v_m^{h_1}) \frac{1 - \text{sgn}(\delta_m^{h_1})}{2} - 2 \sum_{m=1}^{n_{i_1}} \text{sgn}(v_m^{i_1}) \frac{1 - \text{sgn}(\delta_m^{i_1})}{2} \quad (\text{S114.2})$$

$$\mathcal{W}_3^{\text{gapless}} = \sum_{m=1}^{n_{c_1}} \text{sgn}(v_m^{c_1}) \frac{1 - \text{sgn}(\delta_m^{c_1})}{2} - \sum_{m=1}^{n_{f_1}} \text{sgn}(v_m^{f_1}) \frac{1 - \text{sgn}(\delta_m^{f_1})}{2} - \sum_{m=1}^{n_{g_1}} \text{sgn}(v_m^{g_1}) \frac{1 - \text{sgn}(\delta_m^{g_1})}{2} + 2 \sum_{m=1}^{n_{i_1}} \text{sgn}(v_m^{i_1}) \frac{1 - \text{sgn}(\delta_m^{i_1})}{2} \quad (\text{S114.3})$$

$$\mathcal{W}_4^{\text{gapless}} = \sum_{m=1}^{n_{c_2}} \text{sgn}(v_m^{c_2}) \frac{1 - \text{sgn}(\delta_m^{c_2})}{2} - \sum_{m=1}^{n_{f_1}} \text{sgn}(v_m^{f_1}) \frac{1 - \text{sgn}(\delta_m^{f_1})}{2} - \sum_{m=1}^{n_{g_1}} \text{sgn}(v_m^{g_1}) \frac{1 - \text{sgn}(\delta_m^{g_1})}{2} + 2 \sum_{m=1}^{n_{i_1}} \text{sgn}(v_m^{i_1}) \frac{1 - \text{sgn}(\delta_m^{i_1})}{2} \quad (\text{S114.4})$$

$$\mathcal{W}_5^{\text{gapless}} = \sum_{m=1}^{n_{d_1}} \text{sgn}(v_m^{d_1}) \frac{1 - \text{sgn}(\delta_m^{d_1})}{2} + \sum_{m=1}^{n_{d_2}} \text{sgn}(v_m^{d_2}) \frac{1 - \text{sgn}(\delta_m^{d_2})}{2} - 2 \sum_{m=1}^{n_{e_1}} \text{sgn}(v_m^{e_1}) \frac{1 - \text{sgn}(\delta_m^{e_1})}{2} - 2 \sum_{m=1}^{n_{f_1}} \text{sgn}(v_m^{f_1}) \frac{1 - \text{sgn}(\delta_m^{f_1})}{2} \quad (\text{S114.5})$$

$$\mathcal{X}_1 = \sum_{m=1}^{n_{a_2}} \frac{1 - \text{sgn}(\delta_m^{a_2})}{2} + \sum_{m=1}^{n_{g_1}} \frac{1 - \text{sgn}(\delta_m^{g_1})}{2} \mod 2 \quad (\text{S114.6})$$

$$\mathcal{X}_2 = \sum_{m=1}^{n_{a_2}} \frac{1 - \text{sgn}(\delta_m^{a_2})}{2} + \sum_{m=1}^{n_{f_1}} \frac{1 - \text{sgn}(\delta_m^{f_1})}{2} + \sum_{m=1}^{n_{g_1}} \frac{1 - \text{sgn}(\delta_m^{g_1})}{2} \mod 2 \quad (\text{S114.7})$$

$$\mathcal{X}_3 = \sum_{m=1}^{n_{a_2}} \frac{1 - \text{sgn}(\delta_m^{a_2})}{2} + \sum_{m=1}^{n_{d_2}} \frac{1 - \text{sgn}(\delta_m^{d_2})}{2} + \sum_{m=1}^{n_{g_1}} \frac{1 - \text{sgn}(\delta_m^{g_1})}{2} \mod 2 \quad (\text{S114.8})$$

### S115. SPACE GROUP NO. 115

| line segment                                        | character of irrep (generators only)                                             |
|-----------------------------------------------------|----------------------------------------------------------------------------------|
| $a \quad (0, \frac{t}{2}, 0)$                       | $\{m_{100}   0 \ 0 \ 0\}$<br>$a_1 \quad -i$<br>$a_2 \quad i$                     |
| $b \quad (\frac{1-t}{2}, \frac{1}{2}, 0)$           | $\{m_{010}   0 \ 0 \ 0\}$<br>$b_1 \quad -i$<br>$b_2 \quad i$                     |
| $c \quad (\frac{t}{2}, \frac{t}{2}, 0)$             | $\{2_{110}   0 \ 0 \ 0\}$<br>$c_1 \quad -i$<br>$c_2 \quad i$                     |
| $d \quad (0, \frac{t}{2}, \frac{1}{2})$             | $\{m_{100}   0 \ 0 \ 0\}$<br>$d_1 \quad -i$<br>$d_2 \quad i$                     |
| $e \quad (\frac{1-t}{2}, \frac{1}{2}, \frac{1}{2})$ | $\{m_{010}   0 \ 0 \ 0\}$<br>$e_1 \quad -i$<br>$e_2 \quad i$                     |
| $f \quad (\frac{t}{2}, \frac{t}{2}, \frac{1}{2})$   | $\{2_{110}   0 \ 0 \ 0\}$<br>$f_1 \quad -i$<br>$f_2 \quad i$                     |
| $g \quad (0, 0, \frac{t}{2})$                       | $\{2_{001}   0 \ 0 \ 0\} \quad \{m_{100}   0 \ 0 \ 0\}$<br>$g_1 \quad 0 \quad 0$ |
| $h \quad (0, \frac{1}{2}, \frac{t}{2})$             | $\{2_{001}   0 \ 0 \ 0\} \quad \{m_{100}   0 \ 0 \ 0\}$<br>$h_1 \quad 0 \quad 0$ |
| $i \quad (\frac{1}{2}, \frac{1}{2}, \frac{t}{2})$   | $\{2_{001}   0 \ 0 \ 0\} \quad \{m_{100}   0 \ 0 \ 0\}$<br>$i_1 \quad 0 \quad 0$ |



---


$$\begin{aligned}
\mathcal{W}_1^{\text{gapless}} = & \sum_{m=1}^{n_{a_1}} \text{sgn}(v_m^{a_1}) \frac{1 - \text{sgn}(\delta_m^{a_1})}{2} + \sum_{m=1}^{n_{d_2}} \text{sgn}(v_m^{d_2}) \frac{1 - \text{sgn}(\delta_m^{d_2})}{2} - \sum_{m=1}^{n_{e_1}} \text{sgn}(v_m^{e_1}) \frac{1 - \text{sgn}(\delta_m^{e_1})}{2} \\
& - \sum_{m=1}^{n_{e_2}} \text{sgn}(v_m^{e_2}) \frac{1 - \text{sgn}(\delta_m^{e_2})}{2} - \sum_{m=1}^{n_{f_1}} \text{sgn}(v_m^{f_1}) \frac{1 - \text{sgn}(\delta_m^{f_1})}{2} - \sum_{m=1}^{n_{f_2}} \text{sgn}(v_m^{f_2}) \frac{1 - \text{sgn}(\delta_m^{f_2})}{2} \\
& - \sum_{m=1}^{n_{g_1}} \text{sgn}(v_m^{g_1}) \frac{1 - \text{sgn}(\delta_m^{g_1})}{2} + \sum_{m=1}^{n_{h_1}} \text{sgn}(v_m^{h_1}) \frac{1 - \text{sgn}(\delta_m^{h_1})}{2}
\end{aligned} \tag{S115.1}$$

$$\mathcal{W}_2^{\text{gapless}} = \sum_{m=1}^{n_{a_2}} \text{sgn}(v_m^{a_2}) \frac{1 - \text{sgn}(\delta_m^{a_2})}{2} - \sum_{m=1}^{n_{d_2}} \text{sgn}(v_m^{d_2}) \frac{1 - \text{sgn}(\delta_m^{d_2})}{2} - \sum_{m=1}^{n_{g_1}} \text{sgn}(v_m^{g_1}) \frac{1 - \text{sgn}(\delta_m^{g_1})}{2} + \sum_{m=1}^{n_{h_1}} \text{sgn}(v_m^{h_1}) \frac{1 - \text{sgn}(\delta_m^{h_1})}{2} \tag{S115.2}$$

$$\mathcal{W}_3^{\text{gapless}} = \sum_{m=1}^{n_{b_1}} \text{sgn}(v_m^{b_1}) \frac{1 - \text{sgn}(\delta_m^{b_1})}{2} - \sum_{m=1}^{n_{e_1}} \text{sgn}(v_m^{e_1}) \frac{1 - \text{sgn}(\delta_m^{e_1})}{2} + \sum_{m=1}^{n_{h_1}} \text{sgn}(v_m^{h_1}) \frac{1 - \text{sgn}(\delta_m^{h_1})}{2} - \sum_{m=1}^{n_{i_1}} \text{sgn}(v_m^{i_1}) \frac{1 - \text{sgn}(\delta_m^{i_1})}{2} \tag{S115.3}$$

$$\mathcal{W}_4^{\text{gapless}} = \sum_{m=1}^{n_{b_2}} \text{sgn}(v_m^{b_2}) \frac{1 - \text{sgn}(\delta_m^{b_2})}{2} - \sum_{m=1}^{n_{e_2}} \text{sgn}(v_m^{e_2}) \frac{1 - \text{sgn}(\delta_m^{e_2})}{2} + \sum_{m=1}^{n_{h_1}} \text{sgn}(v_m^{h_1}) \frac{1 - \text{sgn}(\delta_m^{h_1})}{2} - \sum_{m=1}^{n_{i_1}} \text{sgn}(v_m^{i_1}) \frac{1 - \text{sgn}(\delta_m^{i_1})}{2} \tag{S115.4}$$

$$\begin{aligned}
\mathcal{W}_5^{\text{gapless}} = & \sum_{m=1}^{n_{c_1}} \text{sgn}(v_m^{c_1}) \frac{1 - \text{sgn}(\delta_m^{c_1})}{2} + \sum_{m=1}^{n_{c_2}} \text{sgn}(v_m^{c_2}) \frac{1 - \text{sgn}(\delta_m^{c_2})}{2} - \sum_{m=1}^{n_{f_1}} \text{sgn}(v_m^{f_1}) \frac{1 - \text{sgn}(\delta_m^{f_1})}{2} \\
& - \sum_{m=1}^{n_{f_2}} \text{sgn}(v_m^{f_2}) \frac{1 - \text{sgn}(\delta_m^{f_2})}{2} - 2 \sum_{m=1}^{n_{g_1}} \text{sgn}(v_m^{g_1}) \frac{1 - \text{sgn}(\delta_m^{g_1})}{2} + 2 \sum_{m=1}^{n_{i_1}} \text{sgn}(v_m^{i_1}) \frac{1 - \text{sgn}(\delta_m^{i_1})}{2}
\end{aligned} \tag{S115.5}$$

$$\begin{aligned}
\mathcal{W}_6^{\text{gapless}} = & \sum_{m=1}^{n_{d_1}} \text{sgn}(v_m^{d_1}) \frac{1 - \text{sgn}(\delta_m^{d_1})}{2} + \sum_{m=1}^{n_{d_2}} \text{sgn}(v_m^{d_2}) \frac{1 - \text{sgn}(\delta_m^{d_2})}{2} - \sum_{m=1}^{n_{e_1}} \text{sgn}(v_m^{e_1}) \frac{1 - \text{sgn}(\delta_m^{e_1})}{2} \\
& - \sum_{m=1}^{n_{e_2}} \text{sgn}(v_m^{e_2}) \frac{1 - \text{sgn}(\delta_m^{e_2})}{2} - \sum_{m=1}^{n_{f_1}} \text{sgn}(v_m^{f_1}) \frac{1 - \text{sgn}(\delta_m^{f_1})}{2} - \sum_{m=1}^{n_{f_2}} \text{sgn}(v_m^{f_2}) \frac{1 - \text{sgn}(\delta_m^{f_2})}{2}
\end{aligned} \tag{S115.6}$$

$$\mathcal{W}_1^{\text{gapped}} = - \sum_{m=1}^{n_{f_1}} \text{sgn}(v_m^{f_1}) \frac{1 - \text{sgn}(\delta_m^{f_1})}{2} + \sum_{m=1}^{n_{f_2}} \text{sgn}(v_m^{f_2}) \frac{1 - \text{sgn}(\delta_m^{f_2})}{2} \tag{S115.7}$$

$$\mathcal{W}_2^{\text{gapped}} = - \sum_{m=1}^{n_{d_2}} \text{sgn}(v_m^{d_2}) \frac{1 - \text{sgn}(\delta_m^{d_2})}{2} + \sum_{m=1}^{n_{e_1}} \text{sgn}(v_m^{e_1}) \frac{1 - \text{sgn}(\delta_m^{e_1})}{2} + \sum_{m=1}^{n_{f_1}} \text{sgn}(v_m^{f_1}) \frac{1 - \text{sgn}(\delta_m^{f_1})}{2} \tag{S115.8}$$

$$\mathcal{W}_3^{\text{gapped}} = - \sum_{m=1}^{n_{d_2}} \text{sgn}(v_m^{d_2}) \frac{1 - \text{sgn}(\delta_m^{d_2})}{2} + \sum_{m=1}^{n_{e_2}} \text{sgn}(v_m^{e_2}) \frac{1 - \text{sgn}(\delta_m^{e_2})}{2} + \sum_{m=1}^{n_{f_1}} \text{sgn}(v_m^{f_1}) \frac{1 - \text{sgn}(\delta_m^{f_1})}{2} \quad (\text{S115.9})$$

$$\mathcal{W}_4^{\text{gapped}} = \sum_{m=1}^{n_{c_2}} \text{sgn}(v_m^{c_2}) \frac{1 - \text{sgn}(\delta_m^{c_2})}{2} - \sum_{m=1}^{n_{f_1}} \text{sgn}(v_m^{f_1}) \frac{1 - \text{sgn}(\delta_m^{f_1})}{2} - \sum_{m=1}^{n_{g_1}} \text{sgn}(v_m^{g_1}) \frac{1 - \text{sgn}(\delta_m^{g_1})}{2} + \sum_{m=1}^{n_{i_1}} \text{sgn}(v_m^{i_1}) \frac{1 - \text{sgn}(\delta_m^{i_1})}{2} \quad (\text{S115.10})$$

### S116. SPACE GROUP NO. 116

| line segment                                        | character of irrep (generators only) |                                                                      |
|-----------------------------------------------------|--------------------------------------|----------------------------------------------------------------------|
| $a \quad (0, \frac{t}{2}, 0)$                       | $a_1$                                | $\{m_{100}   0 \ 0 \ \frac{1}{2}\}$<br>-i                            |
|                                                     | $a_2$                                | i                                                                    |
| $b \quad (\frac{1-t}{2}, \frac{1}{2}, 0)$           | $b_1$                                | $\{m_{010}   0 \ 0 \ \frac{1}{2}\}$<br>-i                            |
|                                                     | $b_2$                                | i                                                                    |
| $c \quad (\frac{t}{2}, \frac{t}{2}, 0)$             | $c_1$                                | $\{2_{110}   0 \ 0 \ \frac{1}{2}\}$<br>-i                            |
|                                                     | $c_2$                                | i                                                                    |
| $d \quad (0, \frac{t}{2}, \frac{1}{2})$             | $d_1$                                | $\{m_{100}   0 \ 0 \ \frac{1}{2}\}$<br>-1                            |
|                                                     | $d_2$                                | 1                                                                    |
| $e \quad (\frac{1-t}{2}, \frac{1}{2}, \frac{1}{2})$ | $e_1$                                | $\{m_{010}   0 \ 0 \ \frac{1}{2}\}$<br>-1                            |
|                                                     | $e_2$                                | 1                                                                    |
| $f \quad (\frac{t}{2}, \frac{t}{2}, \frac{1}{2})$   | $f_1$                                | $\{2_{110}   0 \ 0 \ \frac{1}{2}\}$<br>i                             |
|                                                     | $f_2$                                | -i                                                                   |
| $g \quad (0, 0, \frac{t}{2})$                       | $g_1$                                | $\{2_{001}   0 \ 0 \ 0\}$ $\{m_{100}   0 \ 0 \ \frac{1}{2}\}$<br>0 0 |
|                                                     | $h_1$                                | $\{2_{001}   0 \ 0 \ 0\}$ $\{m_{100}   0 \ 0 \ \frac{1}{2}\}$<br>0 0 |
| $i \quad (\frac{1}{2}, \frac{1}{2}, \frac{t}{2})$   | $i_1$                                | $\{2_{001}   0 \ 0 \ 0\}$ $\{m_{100}   0 \ 0 \ \frac{1}{2}\}$<br>0 0 |

$$\begin{aligned} \mathcal{W}_1^{\text{gapless}} = & \sum_{m=1}^{n_{a_1}} \text{sgn}(v_m^{a_1}) \frac{1 - \text{sgn}(\delta_m^{a_1})}{2} + \sum_{m=1}^{n_{d_1}} \text{sgn}(v_m^{d_1}) \frac{1 - \text{sgn}(\delta_m^{d_1})}{2} - 2 \sum_{m=1}^{n_{e_1}} \text{sgn}(v_m^{e_1}) \frac{1 - \text{sgn}(\delta_m^{e_1})}{2} \\ & - \sum_{m=1}^{n_{f_1}} \text{sgn}(v_m^{f_1}) \frac{1 - \text{sgn}(\delta_m^{f_1})}{2} - \sum_{m=1}^{n_{f_2}} \text{sgn}(v_m^{f_2}) \frac{1 - \text{sgn}(\delta_m^{f_2})}{2} - \sum_{m=1}^{n_{g_1}} \text{sgn}(v_m^{g_1}) \frac{1 - \text{sgn}(\delta_m^{g_1})}{2} \\ & + \sum_{m=1}^{n_{h_1}} \text{sgn}(v_m^{h_1}) \frac{1 - \text{sgn}(\delta_m^{h_1})}{2} \end{aligned} \quad (\text{S116.1})$$

$$\begin{aligned}
\mathcal{W}_2^{\text{gapless}} = & \sum_{m=1}^{n_{a_2}} \text{sgn}(v_m^{a_2}) \frac{1 - \text{sgn}(\delta_m^{a_2})}{2} + \sum_{m=1}^{n_{d_1}} \text{sgn}(v_m^{d_1}) \frac{1 - \text{sgn}(\delta_m^{d_1})}{2} - 2 \sum_{m=1}^{n_{e_1}} \text{sgn}(v_m^{e_1}) \frac{1 - \text{sgn}(\delta_m^{e_1})}{2} \\
& - \sum_{m=1}^{n_{f_1}} \text{sgn}(v_m^{f_1}) \frac{1 - \text{sgn}(\delta_m^{f_1})}{2} - \sum_{m=1}^{n_{f_2}} \text{sgn}(v_m^{f_2}) \frac{1 - \text{sgn}(\delta_m^{f_2})}{2} - \sum_{m=1}^{n_{g_1}} \text{sgn}(v_m^{g_1}) \frac{1 - \text{sgn}(\delta_m^{g_1})}{2} \\
& + \sum_{m=1}^{n_{h_1}} \text{sgn}(v_m^{h_1}) \frac{1 - \text{sgn}(\delta_m^{h_1})}{2}
\end{aligned} \tag{S116.2}$$

$$\mathcal{W}_3^{\text{gapless}} = \sum_{m=1}^{n_{b_1}} \text{sgn}(v_m^{b_1}) \frac{1 - \text{sgn}(\delta_m^{b_1})}{2} - \sum_{m=1}^{n_{e_1}} \text{sgn}(v_m^{e_1}) \frac{1 - \text{sgn}(\delta_m^{e_1})}{2} + \sum_{m=1}^{n_{h_1}} \text{sgn}(v_m^{h_1}) \frac{1 - \text{sgn}(\delta_m^{h_1})}{2} - \sum_{m=1}^{n_{i_1}} \text{sgn}(v_m^{i_1}) \frac{1 - \text{sgn}(\delta_m^{i_1})}{2} \tag{S116.3}$$

$$\mathcal{W}_4^{\text{gapless}} = \sum_{m=1}^{n_{b_2}} \text{sgn}(v_m^{b_2}) \frac{1 - \text{sgn}(\delta_m^{b_2})}{2} - \sum_{m=1}^{n_{e_1}} \text{sgn}(v_m^{e_1}) \frac{1 - \text{sgn}(\delta_m^{e_1})}{2} + \sum_{m=1}^{n_{h_1}} \text{sgn}(v_m^{h_1}) \frac{1 - \text{sgn}(\delta_m^{h_1})}{2} - \sum_{m=1}^{n_{i_1}} \text{sgn}(v_m^{i_1}) \frac{1 - \text{sgn}(\delta_m^{i_1})}{2} \tag{S116.4}$$

$$\begin{aligned}
\mathcal{W}_5^{\text{gapless}} = & \sum_{m=1}^{n_{c_1}} \text{sgn}(v_m^{c_1}) \frac{1 - \text{sgn}(\delta_m^{c_1})}{2} + \sum_{m=1}^{n_{c_2}} \text{sgn}(v_m^{c_2}) \frac{1 - \text{sgn}(\delta_m^{c_2})}{2} - \sum_{m=1}^{n_{f_1}} \text{sgn}(v_m^{f_1}) \frac{1 - \text{sgn}(\delta_m^{f_1})}{2} \\
& - \sum_{m=1}^{n_{f_2}} \text{sgn}(v_m^{f_2}) \frac{1 - \text{sgn}(\delta_m^{f_2})}{2} - 2 \sum_{m=1}^{n_{g_1}} \text{sgn}(v_m^{g_1}) \frac{1 - \text{sgn}(\delta_m^{g_1})}{2} + 2 \sum_{m=1}^{n_{i_1}} \text{sgn}(v_m^{i_1}) \frac{1 - \text{sgn}(\delta_m^{i_1})}{2}
\end{aligned} \tag{S116.5}$$

$$\begin{aligned}
\mathcal{W}_6^{\text{gapless}} = & 2 \sum_{m=1}^{n_{d_1}} \text{sgn}(v_m^{d_1}) \frac{1 - \text{sgn}(\delta_m^{d_1})}{2} - 2 \sum_{m=1}^{n_{e_1}} \text{sgn}(v_m^{e_1}) \frac{1 - \text{sgn}(\delta_m^{e_1})}{2} - \sum_{m=1}^{n_{f_1}} \text{sgn}(v_m^{f_1}) \frac{1 - \text{sgn}(\delta_m^{f_1})}{2} \\
& - \sum_{m=1}^{n_{f_2}} \text{sgn}(v_m^{f_2}) \frac{1 - \text{sgn}(\delta_m^{f_2})}{2}
\end{aligned} \tag{S116.6}$$

$$\mathcal{W}_1^{\text{gapped}} = - \sum_{m=1}^{n_{d_1}} \text{sgn}(v_m^{d_1}) \frac{1 - \text{sgn}(\delta_m^{d_1})}{2} + \sum_{m=1}^{n_{e_1}} \text{sgn}(v_m^{e_1}) \frac{1 - \text{sgn}(\delta_m^{e_1})}{2} + \sum_{m=1}^{n_{f_2}} \text{sgn}(v_m^{f_2}) \frac{1 - \text{sgn}(\delta_m^{f_2})}{2} \tag{S116.7}$$

$$\mathcal{W}_2^{\text{gapped}} = \sum_{m=1}^{n_{c_2}} \text{sgn}(v_m^{c_2}) \frac{1 - \text{sgn}(\delta_m^{c_2})}{2} - \sum_{m=1}^{n_{f_1}} \text{sgn}(v_m^{f_1}) \frac{1 - \text{sgn}(\delta_m^{f_1})}{2} - \sum_{m=1}^{n_{g_1}} \text{sgn}(v_m^{g_1}) \frac{1 - \text{sgn}(\delta_m^{g_1})}{2} + \sum_{m=1}^{n_{i_1}} \text{sgn}(v_m^{i_1}) \frac{1 - \text{sgn}(\delta_m^{i_1})}{2} \tag{S116.8}$$

$$\mathcal{X}_1 = \sum_{m=1}^{n_{f_1}} \frac{1 - \text{sgn}(\delta_m^{f_1})}{2} \mod 2 \tag{S116.9}$$

$$\mathcal{X}_2 = \sum_{m=1}^{n_{e_1}} \frac{1 - \text{sgn}(\delta_m^{e_1})}{2} \mod 2 \tag{S116.10}$$

## S117. SPACE GROUP NO. 117

| line segment                                        | character of irrep (generators only)                                                                                                                                            |
|-----------------------------------------------------|---------------------------------------------------------------------------------------------------------------------------------------------------------------------------------|
| $a \quad (0, \frac{t}{2}, 0)$                       | $\{m_{100}   \frac{1}{2} \frac{1}{2} 0\}$<br>$a_1 \quad -ie^{-\frac{1}{2}i\pi t}$<br>$a_2 \quad ie^{-\frac{1}{2}i\pi t}$                                                        |
| $b \quad (\frac{1-t}{2}, \frac{1}{2}, 0)$           | $\{m_{010}   \frac{1}{2} \frac{1}{2} 0\}$<br>$b_1 \quad -e^{-\frac{1}{2}i\pi(2-t)}$<br>$b_2 \quad e^{-\frac{1}{2}i\pi(2-t)}$                                                    |
| $c \quad (\frac{t}{2}, \frac{t}{2}, 0)$             | $\{2_{110}   \frac{1}{2} \frac{1}{2} 0\}$<br>$c_1 \quad -ie^{-i\pi t}$<br>$c_2 \quad ie^{-i\pi t}$                                                                              |
| $d \quad (0, \frac{t}{2}, \frac{1}{2})$             | $\{m_{100}   \frac{1}{2} \frac{1}{2} 0\}$<br>$d_1 \quad -ie^{-\frac{1}{2}i\pi t}$<br>$d_2 \quad ie^{-\frac{1}{2}i\pi t}$                                                        |
| $e \quad (\frac{1-t}{2}, \frac{1}{2}, \frac{1}{2})$ | $\{m_{010}   \frac{1}{2} \frac{1}{2} 0\}$<br>$e_1 \quad -e^{-\frac{1}{2}i\pi(2-t)}$<br>$e_2 \quad e^{-\frac{1}{2}i\pi(2-t)}$                                                    |
| $f \quad (\frac{t}{2}, \frac{t}{2}, \frac{1}{2})$   | $\{2_{110}   \frac{1}{2} \frac{1}{2} 0\}$<br>$f_1 \quad -ie^{-i\pi t}$<br>$f_2 \quad ie^{-i\pi t}$                                                                              |
| $g \quad (0, 0, \frac{t}{2})$                       | $\{2_{001}   0 \ 0 \ 0\} \quad \{m_{100}   \frac{1}{2} \frac{1}{2} 0\}$<br>$g_1 \quad 0 \quad 0$                                                                                |
| $h \quad (0, \frac{1}{2}, \frac{t}{2})$             | $\{2_{001}   0 \ 0 \ 0\} \quad \{m_{100}   \frac{1}{2} \frac{1}{2} 0\}$<br>$h_1 \quad -i \quad -1$<br>$h_2 \quad -i \quad 1$<br>$h_3 \quad i \quad -1$<br>$h_4 \quad i \quad 1$ |
| $i \quad (\frac{1}{2}, \frac{1}{2}, \frac{t}{2})$   | $\{2_{001}   0 \ 0 \ 0\} \quad \{m_{100}   \frac{1}{2} \frac{1}{2} 0\}$<br>$i_1 \quad 0 \quad 0$                                                                                |

$$\begin{aligned}
\mathcal{W}_1^{\text{gapless}} = & \sum_{m=1}^{n_{a_1}} \text{sgn}(v_m^{a_1}) \frac{1 - \text{sgn}(\delta_m^{a_1})}{2} + \sum_{m=1}^{n_{d_2}} \text{sgn}(v_m^{d_2}) \frac{1 - \text{sgn}(\delta_m^{d_2})}{2} - 2 \sum_{m=1}^{n_{e_1}} \text{sgn}(v_m^{e_1}) \frac{1 - \text{sgn}(\delta_m^{e_1})}{2} \\
& - \sum_{m=1}^{n_{f_1}} \text{sgn}(v_m^{f_1}) \frac{1 - \text{sgn}(\delta_m^{f_1})}{2} - \sum_{m=1}^{n_{f_2}} \text{sgn}(v_m^{f_2}) \frac{1 - \text{sgn}(\delta_m^{f_2})}{2} - \sum_{m=1}^{n_{g_1}} \text{sgn}(v_m^{g_1}) \frac{1 - \text{sgn}(\delta_m^{g_1})}{2} \\
& + \sum_{m=1}^{n_{h_2}} \text{sgn}(v_m^{h_2}) \frac{1 - \text{sgn}(\delta_m^{h_2})}{2} + 2 \sum_{m=1}^{n_{h_3}} \text{sgn}(v_m^{h_3}) \frac{1 - \text{sgn}(\delta_m^{h_3})}{2} - \sum_{m=1}^{n_{h_4}} \text{sgn}(v_m^{h_4}) \frac{1 - \text{sgn}(\delta_m^{h_4})}{2}
\end{aligned} \tag{S117.1}$$

$$\begin{aligned}
\mathcal{W}_2^{\text{gapless}} = & \sum_{m=1}^{n_{a_2}} \text{sgn}(v_m^{a_2}) \frac{1 - \text{sgn}(\delta_m^{a_2})}{2} - \sum_{m=1}^{n_{d_2}} \text{sgn}(v_m^{d_2}) \frac{1 - \text{sgn}(\delta_m^{d_2})}{2} - \sum_{m=1}^{n_{g_1}} \text{sgn}(v_m^{g_1}) \frac{1 - \text{sgn}(\delta_m^{g_1})}{2} \\
& + \sum_{m=1}^{n_{h_2}} \text{sgn}(v_m^{h_2}) \frac{1 - \text{sgn}(\delta_m^{h_2})}{2} + \sum_{m=1}^{n_{h_4}} \text{sgn}(v_m^{h_4}) \frac{1 - \text{sgn}(\delta_m^{h_4})}{2}
\end{aligned} \tag{S117.2}$$

$$\begin{aligned}
\mathcal{W}_3^{\text{gapless}} = & \sum_{m=1}^{n_{b_1}} \text{sgn}(v_m^{b_1}) \frac{1 - \text{sgn}(\delta_m^{b_1})}{2} - \sum_{m=1}^{n_{e_1}} \text{sgn}(v_m^{e_1}) \frac{1 - \text{sgn}(\delta_m^{e_1})}{2} + \sum_{m=1}^{n_{h_2}} \text{sgn}(v_m^{h_2}) \frac{1 - \text{sgn}(\delta_m^{h_2})}{2} \\
& + \sum_{m=1}^{n_{h_3}} \text{sgn}(v_m^{h_3}) \frac{1 - \text{sgn}(\delta_m^{h_3})}{2} - \sum_{m=1}^{n_{i_1}} \text{sgn}(v_m^{i_1}) \frac{1 - \text{sgn}(\delta_m^{i_1})}{2}
\end{aligned} \tag{S117.3}$$

$$\begin{aligned} \mathcal{W}_4^{\text{gapless}} = & \sum_{m=1}^{n_{c_1}} \text{sgn}(v_m^{c_1}) \frac{1 - \text{sgn}(\delta_m^{c_1})}{2} + \sum_{m=1}^{n_{c_2}} \text{sgn}(v_m^{c_2}) \frac{1 - \text{sgn}(\delta_m^{c_2})}{2} - \sum_{m=1}^{n_{f_1}} \text{sgn}(v_m^{f_1}) \frac{1 - \text{sgn}(\delta_m^{f_1})}{2} \\ & - \sum_{m=1}^{n_{f_2}} \text{sgn}(v_m^{f_2}) \frac{1 - \text{sgn}(\delta_m^{f_2})}{2} - 2 \sum_{m=1}^{n_{g_1}} \text{sgn}(v_m^{g_1}) \frac{1 - \text{sgn}(\delta_m^{g_1})}{2} + 2 \sum_{m=1}^{n_{i_1}} \text{sgn}(v_m^{i_1}) \frac{1 - \text{sgn}(\delta_m^{i_1})}{2} \end{aligned} \quad (\text{S117.4})$$

$$\begin{aligned} \mathcal{W}_5^{\text{gapless}} = & \sum_{m=1}^{n_{d_1}} \text{sgn}(v_m^{d_1}) \frac{1 - \text{sgn}(\delta_m^{d_1})}{2} + \sum_{m=1}^{n_{d_2}} \text{sgn}(v_m^{d_2}) \frac{1 - \text{sgn}(\delta_m^{d_2})}{2} - 2 \sum_{m=1}^{n_{e_1}} \text{sgn}(v_m^{e_1}) \frac{1 - \text{sgn}(\delta_m^{e_1})}{2} \\ & - \sum_{m=1}^{n_{f_1}} \text{sgn}(v_m^{f_1}) \frac{1 - \text{sgn}(\delta_m^{f_1})}{2} - \sum_{m=1}^{n_{f_2}} \text{sgn}(v_m^{f_2}) \frac{1 - \text{sgn}(\delta_m^{f_2})}{2} \end{aligned} \quad (\text{S117.5})$$

$$\mathcal{W}_6^{\text{gapless}} = \sum_{m=1}^{n_{h_1}} \text{sgn}(v_m^{h_1}) \frac{1 - \text{sgn}(\delta_m^{h_1})}{2} - \sum_{m=1}^{n_{h_2}} \text{sgn}(v_m^{h_2}) \frac{1 - \text{sgn}(\delta_m^{h_2})}{2} - \sum_{m=1}^{n_{h_3}} \text{sgn}(v_m^{h_3}) \frac{1 - \text{sgn}(\delta_m^{h_3})}{2} + \sum_{m=1}^{n_{h_4}} \text{sgn}(v_m^{h_4}) \frac{1 - \text{sgn}(\delta_m^{h_4})}{2} \quad (\text{S117.6})$$

$$\mathcal{W}_1^{\text{gapped}} = - \sum_{m=1}^{n_{c_2}} \text{sgn}(v_m^{c_2}) \frac{1 - \text{sgn}(\delta_m^{c_2})}{2} + \sum_{m=1}^{n_{f_1}} \text{sgn}(v_m^{f_1}) \frac{1 - \text{sgn}(\delta_m^{f_1})}{2} + \sum_{m=1}^{n_{g_1}} \text{sgn}(v_m^{g_1}) \frac{1 - \text{sgn}(\delta_m^{g_1})}{2} - \sum_{m=1}^{n_{i_1}} \text{sgn}(v_m^{i_1}) \frac{1 - \text{sgn}(\delta_m^{i_1})}{2} \quad (\text{S117.7})$$

$$\mathcal{W}_2^{\text{gapped}} = - \sum_{m=1}^{n_{h_2}} \text{sgn}(v_m^{h_2}) \frac{1 - \text{sgn}(\delta_m^{h_2})}{2} + \sum_{m=1}^{n_{h_4}} \text{sgn}(v_m^{h_4}) \frac{1 - \text{sgn}(\delta_m^{h_4})}{2} \quad (\text{S117.8})$$

$$\mathcal{W}_3^{\text{gapped}} = - \sum_{m=1}^{n_{c_2}} \text{sgn}(v_m^{c_2}) \frac{1 - \text{sgn}(\delta_m^{c_2})}{2} + \sum_{m=1}^{n_{f_2}} \text{sgn}(v_m^{f_2}) \frac{1 - \text{sgn}(\delta_m^{f_2})}{2} + \sum_{m=1}^{n_{g_1}} \text{sgn}(v_m^{g_1}) \frac{1 - \text{sgn}(\delta_m^{g_1})}{2} - \sum_{m=1}^{n_{i_1}} \text{sgn}(v_m^{i_1}) \frac{1 - \text{sgn}(\delta_m^{i_1})}{2} \quad (\text{S117.9})$$

$$\mathcal{X}_1 = \sum_{m=1}^{n_{i_1}} \frac{1 - \text{sgn}(\delta_m^{i_1})}{2} \quad \text{mod } 2 \quad (\text{S117.10})$$

$$\mathcal{X}_2 = \sum_{m=1}^{n_{c_2}} \frac{1 - \text{sgn}(\delta_m^{c_2})}{2} + \sum_{m=1}^{n_{d_2}} \frac{1 - \text{sgn}(\delta_m^{d_2})}{2} + \sum_{m=1}^{n_{g_1}} \frac{1 - \text{sgn}(\delta_m^{g_1})}{2} \quad \text{mod } 2 \quad (\text{S117.11})$$

### S118. SPACE GROUP NO. 118

|              |                                      |
|--------------|--------------------------------------|
| line segment | character of irrep (generators only) |
|--------------|--------------------------------------|

|                                                     |                                                                                                                                                                                                                                                                                 |
|-----------------------------------------------------|---------------------------------------------------------------------------------------------------------------------------------------------------------------------------------------------------------------------------------------------------------------------------------|
| $a \quad (0, \frac{t}{2}, 0)$                       | $\begin{matrix} \{m_{100}   \frac{1}{2} \frac{1}{2} \frac{1}{2} \} \\ a_1 \quad -ie^{-\frac{1}{2}i\pi t} \\ a_2 \quad ie^{-\frac{1}{2}i\pi t} \end{matrix}$                                                                                                                     |
| $b \quad (\frac{1-t}{2}, \frac{1}{2}, 0)$           | $\begin{matrix} \{m_{010}   \frac{1}{2} \frac{1}{2} \frac{1}{2} \} \\ b_1 \quad -e^{-\frac{1}{2}i\pi(2-t)} \\ b_2 \quad e^{-\frac{1}{2}i\pi(2-t)} \end{matrix}$                                                                                                                 |
| $c \quad (\frac{t}{2}, \frac{t}{2}, 0)$             | $\begin{matrix} \{2_{110}   \frac{1}{2} \frac{1}{2} \frac{1}{2} \} \\ c_1 \quad -ie^{-i\pi t} \\ c_2 \quad ie^{-i\pi t} \end{matrix}$                                                                                                                                           |
| $d \quad (0, \frac{t}{2}, \frac{1}{2})$             | $\begin{matrix} \{m_{100}   \frac{1}{2} \frac{1}{2} \frac{1}{2} \} \\ d_1 \quad -ie^{-\frac{1}{2}i\pi(t+1)} \\ d_2 \quad ie^{-\frac{1}{2}i\pi(t+1)} \end{matrix}$                                                                                                               |
| $e \quad (\frac{1-t}{2}, \frac{1}{2}, \frac{1}{2})$ | $\begin{matrix} \{m_{010}   \frac{1}{2} \frac{1}{2} \frac{1}{2} \} \\ e_1 \quad -e^{-\frac{1}{2}i\pi(3-t)} \\ e_2 \quad e^{-\frac{1}{2}i\pi(3-t)} \end{matrix}$                                                                                                                 |
| $f \quad (\frac{t}{2}, \frac{t}{2}, \frac{1}{2})$   | $\begin{matrix} \{2_{110}   \frac{1}{2} \frac{1}{2} \frac{1}{2} \} \\ f_1 \quad -e^{-\frac{1}{2}i\pi(2t+1)} \\ f_2 \quad e^{-\frac{1}{2}i\pi(2t+1)} \end{matrix}$                                                                                                               |
| $g \quad (0, 0, \frac{t}{2})$                       | $\begin{matrix} \{2_{001}   0 \ 0 \ 0 \} & \{m_{100}   \frac{1}{2} \frac{1}{2} \frac{1}{2} \} \\ g_1 & 0 \end{matrix}$                                                                                                                                                          |
| $h \quad (0, \frac{1}{2}, \frac{t}{2})$             | $\begin{matrix} \{2_{001}   0 \ 0 \ 0 \} & \{m_{100}   \frac{1}{2} \frac{1}{2} \frac{1}{2} \} \\ h_1 & -i & -ie^{-\frac{1}{2}i\pi(t+1)} \\ h_2 & -i & ie^{-\frac{1}{2}i\pi(t+1)} \\ h_3 & i & -ie^{-\frac{1}{2}i\pi(t+1)} \\ h_4 & i & ie^{-\frac{1}{2}i\pi(t+1)} \end{matrix}$ |
| $i \quad (\frac{1}{2}, \frac{1}{2}, \frac{t}{2})$   | $\begin{matrix} \{2_{001}   0 \ 0 \ 0 \} & \{m_{100}   \frac{1}{2} \frac{1}{2} \frac{1}{2} \} \\ i_1 & 0 \end{matrix}$                                                                                                                                                          |

$$\begin{aligned}
\mathcal{W}_1^{\text{gapless}} = & \sum_{m=1}^{n_{a_1}} \text{sgn}(v_m^{a_1}) \frac{1 - \text{sgn}(\delta_m^{a_1})}{2} + \sum_{m=1}^{n_{d_1}} \text{sgn}(v_m^{d_1}) \frac{1 - \text{sgn}(\delta_m^{d_1})}{2} - 2 \sum_{m=1}^{n_{e_2}} \text{sgn}(v_m^{e_2}) \frac{1 - \text{sgn}(\delta_m^{e_2})}{2} \\
& - \sum_{m=1}^{n_{f_1}} \text{sgn}(v_m^{f_1}) \frac{1 - \text{sgn}(\delta_m^{f_1})}{2} - \sum_{m=1}^{n_{f_2}} \text{sgn}(v_m^{f_2}) \frac{1 - \text{sgn}(\delta_m^{f_2})}{2} - \sum_{m=1}^{n_{g_1}} \text{sgn}(v_m^{g_1}) \frac{1 - \text{sgn}(\delta_m^{g_1})}{2} \\
& + 2 \sum_{m=1}^{n_{h_1}} \text{sgn}(v_m^{h_1}) \frac{1 - \text{sgn}(\delta_m^{h_1})}{2} - \sum_{m=1}^{n_{h_2}} \text{sgn}(v_m^{h_2}) \frac{1 - \text{sgn}(\delta_m^{h_2})}{2} + \sum_{m=1}^{n_{h_4}} \text{sgn}(v_m^{h_4}) \frac{1 - \text{sgn}(\delta_m^{h_4})}{2}
\end{aligned} \tag{S118.1}$$

$$\begin{aligned}
\mathcal{W}_2^{\text{gapless}} = & \sum_{m=1}^{n_{a_2}} \text{sgn}(v_m^{a_2}) \frac{1 - \text{sgn}(\delta_m^{a_2})}{2} + \sum_{m=1}^{n_{d_1}} \text{sgn}(v_m^{d_1}) \frac{1 - \text{sgn}(\delta_m^{d_1})}{2} - 2 \sum_{m=1}^{n_{e_2}} \text{sgn}(v_m^{e_2}) \frac{1 - \text{sgn}(\delta_m^{e_2})}{2} \\
& - \sum_{m=1}^{n_{f_1}} \text{sgn}(v_m^{f_1}) \frac{1 - \text{sgn}(\delta_m^{f_1})}{2} - \sum_{m=1}^{n_{f_2}} \text{sgn}(v_m^{f_2}) \frac{1 - \text{sgn}(\delta_m^{f_2})}{2} - \sum_{m=1}^{n_{g_1}} \text{sgn}(v_m^{g_1}) \frac{1 - \text{sgn}(\delta_m^{g_1})}{2} \\
& + \sum_{m=1}^{n_{h_1}} \text{sgn}(v_m^{h_1}) \frac{1 - \text{sgn}(\delta_m^{h_1})}{2} - \sum_{m=1}^{n_{h_3}} \text{sgn}(v_m^{h_3}) \frac{1 - \text{sgn}(\delta_m^{h_3})}{2} + 2 \sum_{m=1}^{n_{h_4}} \text{sgn}(v_m^{h_4}) \frac{1 - \text{sgn}(\delta_m^{h_4})}{2}
\end{aligned} \tag{S118.2}$$

$$\begin{aligned}
\mathcal{W}_3^{\text{gapless}} = & \sum_{m=1}^{n_{b_1}} \text{sgn}(v_m^{b_1}) \frac{1 - \text{sgn}(\delta_m^{b_1})}{2} - \sum_{m=1}^{n_{e_2}} \text{sgn}(v_m^{e_2}) \frac{1 - \text{sgn}(\delta_m^{e_2})}{2} + \sum_{m=1}^{n_{h_1}} \text{sgn}(v_m^{h_1}) \frac{1 - \text{sgn}(\delta_m^{h_1})}{2} \\
& + \sum_{m=1}^{n_{h_4}} \text{sgn}(v_m^{h_4}) \frac{1 - \text{sgn}(\delta_m^{h_4})}{2} - \sum_{m=1}^{n_{i_1}} \text{sgn}(v_m^{i_1}) \frac{1 - \text{sgn}(\delta_m^{i_1})}{2}
\end{aligned} \tag{S118.3}$$

$$\begin{aligned} \mathcal{W}_4^{\text{gapless}} = & \sum_{m=1}^{n_{c_1}} \text{sgn}(v_m^{c_1}) \frac{1 - \text{sgn}(\delta_m^{c_1})}{2} + \sum_{m=1}^{n_{c_2}} \text{sgn}(v_m^{c_2}) \frac{1 - \text{sgn}(\delta_m^{c_2})}{2} - \sum_{m=1}^{n_{f_1}} \text{sgn}(v_m^{f_1}) \frac{1 - \text{sgn}(\delta_m^{f_1})}{2} \\ & - \sum_{m=1}^{n_{f_2}} \text{sgn}(v_m^{f_2}) \frac{1 - \text{sgn}(\delta_m^{f_2})}{2} - 2 \sum_{m=1}^{n_{g_1}} \text{sgn}(v_m^{g_1}) \frac{1 - \text{sgn}(\delta_m^{g_1})}{2} + 2 \sum_{m=1}^{n_{i_1}} \text{sgn}(v_m^{i_1}) \frac{1 - \text{sgn}(\delta_m^{i_1})}{2} \end{aligned} \quad (\text{S118.4})$$

$$\begin{aligned} \mathcal{W}_5^{\text{gapless}} = & 2 \sum_{m=1}^{n_{d_1}} \text{sgn}(v_m^{d_1}) \frac{1 - \text{sgn}(\delta_m^{d_1})}{2} - 2 \sum_{m=1}^{n_{e_2}} \text{sgn}(v_m^{e_2}) \frac{1 - \text{sgn}(\delta_m^{e_2})}{2} - \sum_{m=1}^{n_{f_1}} \text{sgn}(v_m^{f_1}) \frac{1 - \text{sgn}(\delta_m^{f_1})}{2} \\ & - \sum_{m=1}^{n_{f_2}} \text{sgn}(v_m^{f_2}) \frac{1 - \text{sgn}(\delta_m^{f_2})}{2} + \sum_{m=1}^{n_{h_1}} \text{sgn}(v_m^{h_1}) \frac{1 - \text{sgn}(\delta_m^{h_1})}{2} - \sum_{m=1}^{n_{h_2}} \text{sgn}(v_m^{h_2}) \frac{1 - \text{sgn}(\delta_m^{h_2})}{2} \\ & - \sum_{m=1}^{n_{h_3}} \text{sgn}(v_m^{h_3}) \frac{1 - \text{sgn}(\delta_m^{h_3})}{2} + \sum_{m=1}^{n_{h_4}} \text{sgn}(v_m^{h_4}) \frac{1 - \text{sgn}(\delta_m^{h_4})}{2} \end{aligned} \quad (\text{S118.5})$$

$$\begin{aligned} \mathcal{W}_6^{\text{gapless}} = & \sum_{m=1}^{n_{e_1}} \text{sgn}(v_m^{e_1}) \frac{1 - \text{sgn}(\delta_m^{e_1})}{2} - \sum_{m=1}^{n_{e_2}} \text{sgn}(v_m^{e_2}) \frac{1 - \text{sgn}(\delta_m^{e_2})}{2} + \sum_{m=1}^{n_{h_1}} \text{sgn}(v_m^{h_1}) \frac{1 - \text{sgn}(\delta_m^{h_1})}{2} \\ & - \sum_{m=1}^{n_{h_2}} \text{sgn}(v_m^{h_2}) \frac{1 - \text{sgn}(\delta_m^{h_2})}{2} - \sum_{m=1}^{n_{h_3}} \text{sgn}(v_m^{h_3}) \frac{1 - \text{sgn}(\delta_m^{h_3})}{2} + \sum_{m=1}^{n_{h_4}} \text{sgn}(v_m^{h_4}) \frac{1 - \text{sgn}(\delta_m^{h_4})}{2} \end{aligned} \quad (\text{S118.6})$$

$$\mathcal{W}_1^{\text{gapped}} = \sum_{m=1}^{n_{f_1}} \text{sgn}(v_m^{f_1}) \frac{1 - \text{sgn}(\delta_m^{f_1})}{2} - \sum_{m=1}^{n_{f_2}} \text{sgn}(v_m^{f_2}) \frac{1 - \text{sgn}(\delta_m^{f_2})}{2} \quad (\text{S118.7})$$

$$\begin{aligned} \mathcal{W}_2^{\text{gapped}} = & - \sum_{m=1}^{n_{d_1}} \text{sgn}(v_m^{d_1}) \frac{1 - \text{sgn}(\delta_m^{d_1})}{2} + \sum_{m=1}^{n_{e_2}} \text{sgn}(v_m^{e_2}) \frac{1 - \text{sgn}(\delta_m^{e_2})}{2} + \sum_{m=1}^{n_{f_2}} \text{sgn}(v_m^{f_2}) \frac{1 - \text{sgn}(\delta_m^{f_2})}{2} \\ & - \sum_{m=1}^{n_{h_1}} \text{sgn}(v_m^{h_1}) \frac{1 - \text{sgn}(\delta_m^{h_1})}{2} + \sum_{m=1}^{n_{h_3}} \text{sgn}(v_m^{h_3}) \frac{1 - \text{sgn}(\delta_m^{h_3})}{2} \end{aligned} \quad (\text{S118.8})$$

$$\mathcal{W}_3^{\text{gapped}} = \sum_{m=1}^{n_{c_2}} \text{sgn}(v_m^{c_2}) \frac{1 - \text{sgn}(\delta_m^{c_2})}{2} - \sum_{m=1}^{n_{f_2}} \text{sgn}(v_m^{f_2}) \frac{1 - \text{sgn}(\delta_m^{f_2})}{2} - \sum_{m=1}^{n_{g_1}} \text{sgn}(v_m^{g_1}) \frac{1 - \text{sgn}(\delta_m^{g_1})}{2} + \sum_{m=1}^{n_{i_1}} \text{sgn}(v_m^{i_1}) \frac{1 - \text{sgn}(\delta_m^{i_1})}{2} \quad (\text{S118.9})$$

$$\mathcal{X}_1 = \sum_{m=1}^{n_{c_2}} \frac{1 - \text{sgn}(\delta_m^{c_2})}{2} + \sum_{m=1}^{n_{g_1}} \frac{1 - \text{sgn}(\delta_m^{g_1})}{2} \quad \text{mod } 2 \quad (\text{S118.10})$$

$$\mathcal{X}_2 = \sum_{m=1}^{n_{e_2}} \frac{1 - \text{sgn}(\delta_m^{e_2})}{2} + \sum_{m=1}^{n_{f_2}} \frac{1 - \text{sgn}(\delta_m^{f_2})}{2} \quad \text{mod } 2 \quad (\text{S118.11})$$

## S119. SPACE GROUP NO. 119

| line segment                                      | character of irrep (generators only)                                                                                        |
|---------------------------------------------------|-----------------------------------------------------------------------------------------------------------------------------|
| $a \ (0, 0, t)$                                   | $a_1 \begin{Bmatrix} \{2_{001}   0 & 0 & 0\} \\ 0 \end{Bmatrix} \begin{Bmatrix} \{m_{100}   0 & 0 & 0\} \\ 0 \end{Bmatrix}$ |
| $b \ (\frac{1}{2}, \frac{1}{2}, \frac{t}{2})$     | $\begin{Bmatrix} b_1 \\ b_2 \end{Bmatrix} \begin{Bmatrix} \{2_{001}   0 & 0 & 0\} \\ -i \\ i \end{Bmatrix}$                 |
| $c \ (\frac{t}{2}, \frac{t}{2}, 1 - \frac{t}{2})$ | $c_1 \begin{Bmatrix} \{1   0 & 0 & 0\} \\ 1 \end{Bmatrix}$                                                                  |
| $d \ (\frac{t}{2}, \frac{t}{2}, 0)$               | $\begin{Bmatrix} d_1 \\ d_2 \end{Bmatrix} \begin{Bmatrix} \{2_{110}   0 & 0 & 0\} \\ -i \\ i \end{Bmatrix}$                 |
| $e \ (\frac{t}{2}, 1 - \frac{t}{2}, 0)$           | $\begin{Bmatrix} e_1 \\ e_2 \end{Bmatrix} \begin{Bmatrix} \{2_{1-10}   0 & 0 & 0\} \\ -i \\ i \end{Bmatrix}$                |
| $f \ (\frac{1-t}{2}, \frac{1}{2}, \frac{1}{2})$   | $f_1 \begin{Bmatrix} \{1   0 & 0 & 0\} \\ 1 \end{Bmatrix}$                                                                  |
| $g \ (0, t, 0)$                                   | $\begin{Bmatrix} g_1 \\ g_2 \end{Bmatrix} \begin{Bmatrix} \{m_{100}   0 & 0 & 0\} \\ -i \\ i \end{Bmatrix}$                 |
| $h \ (0, \frac{t}{2}, 1 - \frac{t}{2})$           | $\begin{Bmatrix} h_1 \\ h_2 \end{Bmatrix} \begin{Bmatrix} \{m_{100}   0 & 0 & 0\} \\ -i \\ i \end{Bmatrix}$                 |

$$\mathcal{W}_1^{\text{gapless}} = \sum_{m=1}^{n_{a_1}} \text{sgn}(v_m^{a_1}) \frac{1 - \text{sgn}(\delta_m^{a_1})}{2} - \sum_{m=1}^{n_{g_2}} \text{sgn}(v_m^{g_2}) \frac{1 - \text{sgn}(\delta_m^{g_2})}{2} - \sum_{m=1}^{n_{h_1}} \text{sgn}(v_m^{h_1}) \frac{1 - \text{sgn}(\delta_m^{h_1})}{2} + \sum_{m=1}^{n_{h_2}} \text{sgn}(v_m^{h_2}) \frac{1 - \text{sgn}(\delta_m^{h_2})}{2} \quad (\text{S119.1})$$

$$\begin{aligned} \mathcal{W}_2^{\text{gapless}} = & \sum_{m=1}^{n_{b_1}} \text{sgn}(v_m^{b_1}) \frac{1 - \text{sgn}(\delta_m^{b_1})}{2} + \sum_{m=1}^{n_{b_2}} \text{sgn}(v_m^{b_2}) \frac{1 - \text{sgn}(\delta_m^{b_2})}{2} + \sum_{m=1}^{n_{e_1}} \text{sgn}(v_m^{e_1}) \frac{1 - \text{sgn}(\delta_m^{e_1})}{2} + \sum_{m=1}^{n_{e_2}} \text{sgn}(v_m^{e_2}) \frac{1 - \text{sgn}(\delta_m^{e_2})}{2} \\ & + \sum_{m=1}^{n_{f_1}} \text{sgn}(v_m^{f_1}) \frac{1 - \text{sgn}(\delta_m^{f_1})}{2} - \sum_{m=1}^{n_{h_1}} \text{sgn}(v_m^{h_1}) \frac{1 - \text{sgn}(\delta_m^{h_1})}{2} - \sum_{m=1}^{n_{h_2}} \text{sgn}(v_m^{h_2}) \frac{1 - \text{sgn}(\delta_m^{h_2})}{2} \end{aligned} \quad (\text{S119.2})$$

$$\mathcal{W}_3^{\text{gapless}} = \sum_{m=1}^{n_{c_1}} \text{sgn}(v_m^{c_1}) \frac{1 - \text{sgn}(\delta_m^{c_1})}{2} + \sum_{m=1}^{n_{f_1}} \text{sgn}(v_m^{f_1}) \frac{1 - \text{sgn}(\delta_m^{f_1})}{2} - \sum_{m=1}^{n_{h_1}} \text{sgn}(v_m^{h_1}) \frac{1 - \text{sgn}(\delta_m^{h_1})}{2} - \sum_{m=1}^{n_{h_2}} \text{sgn}(v_m^{h_2}) \frac{1 - \text{sgn}(\delta_m^{h_2})}{2} \quad (\text{S119.3})$$

$$\begin{aligned} \mathcal{W}_4^{\text{gapless}} = & \sum_{m=1}^{n_{d_1}} \text{sgn}(v_m^{d_1}) \frac{1 - \text{sgn}(\delta_m^{d_1})}{2} + \sum_{m=1}^{n_{d_2}} \text{sgn}(v_m^{d_2}) \frac{1 - \text{sgn}(\delta_m^{d_2})}{2} - \sum_{m=1}^{n_{e_1}} \text{sgn}(v_m^{e_1}) \frac{1 - \text{sgn}(\delta_m^{e_1})}{2} - \sum_{m=1}^{n_{e_2}} \text{sgn}(v_m^{e_2}) \frac{1 - \text{sgn}(\delta_m^{e_2})}{2} \\ & - 2 \sum_{m=1}^{n_{g_2}} \text{sgn}(v_m^{g_2}) \frac{1 - \text{sgn}(\delta_m^{g_2})}{2} - 2 \sum_{m=1}^{n_{h_1}} \text{sgn}(v_m^{h_1}) \frac{1 - \text{sgn}(\delta_m^{h_1})}{2} + 2 \sum_{m=1}^{n_{h_2}} \text{sgn}(v_m^{h_2}) \frac{1 - \text{sgn}(\delta_m^{h_2})}{2} \end{aligned} \quad (\text{S119.4})$$



$$\begin{aligned}\mathcal{W}_5^{\text{gapless}} = & \sum_{m=1}^{n_{g_1}} \text{sgn}(v_m^{g_1}) \frac{1 - \text{sgn}(\delta_m^{g_1})}{2} - \sum_{m=1}^{n_{g_2}} \text{sgn}(v_m^{g_2}) \frac{1 - \text{sgn}(\delta_m^{g_2})}{2} - 2 \sum_{m=1}^{n_{h_1}} \text{sgn}(v_m^{h_1}) \frac{1 - \text{sgn}(\delta_m^{h_1})}{2} \\ & + 2 \sum_{m=1}^{n_{h_2}} \text{sgn}(v_m^{h_2}) \frac{1 - \text{sgn}(\delta_m^{h_2})}{2}\end{aligned}\quad (\text{S119.5})$$

$$\mathcal{W}_1^{\text{gapped}} = - \sum_{m=1}^{n_{d_2}} \text{sgn}(v_m^{d_2}) \frac{1 - \text{sgn}(\delta_m^{d_2})}{2} + \sum_{m=1}^{n_{e_1}} \text{sgn}(v_m^{e_1}) \frac{1 - \text{sgn}(\delta_m^{e_1})}{2} + \sum_{m=1}^{n_{g_2}} \text{sgn}(v_m^{g_2}) \frac{1 - \text{sgn}(\delta_m^{g_2})}{2} \quad (\text{S119.6})$$

$$\mathcal{W}_2^{\text{gapped}} = - \sum_{m=1}^{n_{e_1}} \text{sgn}(v_m^{e_1}) \frac{1 - \text{sgn}(\delta_m^{e_1})}{2} + \sum_{m=1}^{n_{e_2}} \text{sgn}(v_m^{e_2}) \frac{1 - \text{sgn}(\delta_m^{e_2})}{2} \quad (\text{S119.7})$$

$$\mathcal{W}_3^{\text{gapped}} = - \sum_{m=1}^{n_{h_1}} \text{sgn}(v_m^{h_1}) \frac{1 - \text{sgn}(\delta_m^{h_1})}{2} + \sum_{m=1}^{n_{h_2}} \text{sgn}(v_m^{h_2}) \frac{1 - \text{sgn}(\delta_m^{h_2})}{2} \quad (\text{S119.8})$$

## S120. SPACE GROUP NO. 120

| line segment                                          | character of irrep (generators only)                                                                                                                                 |
|-------------------------------------------------------|----------------------------------------------------------------------------------------------------------------------------------------------------------------------|
| $a \quad (0, 0, t)$                                   | $a_1 \quad \begin{matrix} \{2_{001}   0 & 0 & 0\} & \{m_{100}   0 & 0 & \frac{1}{2}\} \\ 0 & 0 \end{matrix}$                                                         |
| $b \quad (\frac{1}{2}, \frac{1}{2}, \frac{t}{2})$     | $\begin{matrix} b_1 & \{2_{001}   0 & 0 & 0\} \\ b_2 & \begin{matrix} -i \\ i \end{matrix} \end{matrix}$                                                             |
| $c \quad (\frac{t}{2}, \frac{t}{2}, 1 - \frac{t}{2})$ | $c_1 \quad \begin{matrix} \{1   0 & 0 & 0\} \\ 1 \end{matrix}$                                                                                                       |
| $d \quad (\frac{t}{2}, \frac{t}{2}, 0)$               | $\begin{matrix} d_1 & \{2_{110}   0 & 0 & \frac{1}{2}\} \\ d_2 & \begin{matrix} -i \\ i \end{matrix} \end{matrix}$                                                   |
| $e \quad (\frac{t}{2}, 1 - \frac{t}{2}, 0)$           | $\begin{matrix} e_1 & \{2_{1-10}   0 & 0 & \frac{1}{2}\} \\ e_2 & \begin{matrix} -i \\ i \end{matrix} \end{matrix}$                                                  |
| $f \quad (\frac{1-t}{2}, \frac{1}{2}, \frac{1}{2})$   | $f_1 \quad \begin{matrix} \{1   0 & 0 & 0\} \\ 1 \end{matrix}$                                                                                                       |
| $g \quad (0, t, 0)$                                   | $\begin{matrix} g_1 & \{m_{100}   0 & 0 & \frac{1}{2}\} \\ g_2 & \begin{matrix} -i \\ i \end{matrix} \end{matrix}$                                                   |
| $h \quad (0, \frac{t}{2}, 1 - \frac{t}{2})$           | $\begin{matrix} h_1 & \{m_{100}   0 & 0 & \frac{1}{2}\} \\ h_2 & \begin{matrix} -ie^{-\frac{1}{2}i\pi(2-t)} \\ ie^{-\frac{1}{2}i\pi(2-t)} \end{matrix} \end{matrix}$ |

$$\mathcal{W}_1^{\text{gapless}} = \sum_{m=1}^{n_{a_1}} \text{sgn}(v_m^{a_1}) \frac{1 - \text{sgn}(\delta_m^{a_1})}{2} - \sum_{m=1}^{n_{g_2}} \text{sgn}(v_m^{g_2}) \frac{1 - \text{sgn}(\delta_m^{g_2})}{2} \quad (\text{S120.1})$$

$$\begin{aligned} \mathcal{W}_2^{\text{gapless}} = & \sum_{m=1}^{n_{b_1}} \text{sgn}(v_m^{b_1}) \frac{1 - \text{sgn}(\delta_m^{b_1})}{2} + \sum_{m=1}^{n_{b_2}} \text{sgn}(v_m^{b_2}) \frac{1 - \text{sgn}(\delta_m^{b_2})}{2} + \sum_{m=1}^{n_{e_1}} \text{sgn}(v_m^{e_1}) \frac{1 - \text{sgn}(\delta_m^{e_1})}{2} + \sum_{m=1}^{n_{e_2}} \text{sgn}(v_m^{e_2}) \frac{1 - \text{sgn}(\delta_m^{e_2})}{2} \\ & + 2 \sum_{m=1}^{n_{f_1}} \text{sgn}(v_m^{f_1}) \frac{1 - \text{sgn}(\delta_m^{f_1})}{2} - \sum_{m=1}^{n_{h_1}} \text{sgn}(v_m^{h_1}) \frac{1 - \text{sgn}(\delta_m^{h_1})}{2} - \sum_{m=1}^{n_{h_2}} \text{sgn}(v_m^{h_2}) \frac{1 - \text{sgn}(\delta_m^{h_2})}{2} \end{aligned} \quad (\text{S120.2})$$

$$\begin{aligned} \mathcal{W}_3^{\text{gapless}} = & \sum_{m=1}^{n_{c_1}} \text{sgn}(v_m^{c_1}) \frac{1 - \text{sgn}(\delta_m^{c_1})}{2} + 2 \sum_{m=1}^{n_{f_1}} \text{sgn}(v_m^{f_1}) \frac{1 - \text{sgn}(\delta_m^{f_1})}{2} - \sum_{m=1}^{n_{h_1}} \text{sgn}(v_m^{h_1}) \frac{1 - \text{sgn}(\delta_m^{h_1})}{2} \\ & - \sum_{m=1}^{n_{h_2}} \text{sgn}(v_m^{h_2}) \frac{1 - \text{sgn}(\delta_m^{h_2})}{2} \end{aligned} \quad (\text{S120.3})$$

$$\begin{aligned} \mathcal{W}_4^{\text{gapless}} = & \sum_{m=1}^{n_{d_1}} \text{sgn}(v_m^{d_1}) \frac{1 - \text{sgn}(\delta_m^{d_1})}{2} + \sum_{m=1}^{n_{d_2}} \text{sgn}(v_m^{d_2}) \frac{1 - \text{sgn}(\delta_m^{d_2})}{2} - \sum_{m=1}^{n_{e_1}} \text{sgn}(v_m^{e_1}) \frac{1 - \text{sgn}(\delta_m^{e_1})}{2} \\ & - \sum_{m=1}^{n_{e_2}} \text{sgn}(v_m^{e_2}) \frac{1 - \text{sgn}(\delta_m^{e_2})}{2} - 2 \sum_{m=1}^{n_{g_2}} \text{sgn}(v_m^{g_2}) \frac{1 - \text{sgn}(\delta_m^{g_2})}{2} \end{aligned} \quad (\text{S120.4})$$

$$\mathcal{W}_5^{\text{gapless}} = \sum_{m=1}^{n_{g_1}} \text{sgn}(v_m^{g_1}) \frac{1 - \text{sgn}(\delta_m^{g_1})}{2} - \sum_{m=1}^{n_{g_2}} \text{sgn}(v_m^{g_2}) \frac{1 - \text{sgn}(\delta_m^{g_2})}{2} \quad (\text{S120.5})$$

$$\mathcal{W}_1^{\text{gapped}} = \sum_{m=1}^{n_{e_1}} \text{sgn}(v_m^{e_1}) \frac{1 - \text{sgn}(\delta_m^{e_1})}{2} - \sum_{m=1}^{n_{e_2}} \text{sgn}(v_m^{e_2}) \frac{1 - \text{sgn}(\delta_m^{e_2})}{2} \quad (\text{S120.6})$$

$$\mathcal{W}_2^{\text{gapped}} = - \sum_{m=1}^{n_{d_2}} \text{sgn}(v_m^{d_2}) \frac{1 - \text{sgn}(\delta_m^{d_2})}{2} + \sum_{m=1}^{n_{e_2}} \text{sgn}(v_m^{e_2}) \frac{1 - \text{sgn}(\delta_m^{e_2})}{2} + \sum_{m=1}^{n_{g_2}} \text{sgn}(v_m^{g_2}) \frac{1 - \text{sgn}(\delta_m^{g_2})}{2} \quad (\text{S120.7})$$

$$\mathcal{X}_1 = \sum_{m=1}^{n_{b_2}} \frac{1 - \text{sgn}(\delta_m^{b_2})}{2} + \sum_{m=1}^{n_{e_2}} \frac{1 - \text{sgn}(\delta_m^{e_2})}{2} + \sum_{m=1}^{n_{h_2}} \frac{1 - \text{sgn}(\delta_m^{h_2})}{2} \quad \text{mod } 2 \quad (\text{S120.8})$$

$$\mathcal{X}_2 = \sum_{m=1}^{n_{h_1}} \frac{1 - \text{sgn}(\delta_m^{h_1})}{2} + \sum_{m=1}^{n_{h_2}} \frac{1 - \text{sgn}(\delta_m^{h_2})}{2} \quad \text{mod } 2 \quad (\text{S120.9})$$

## S121. SPACE GROUP NO. 121

|              |                                      |
|--------------|--------------------------------------|
| line segment | character of irrep (generators only) |
|--------------|--------------------------------------|

|                                                   |                                                                                  |
|---------------------------------------------------|----------------------------------------------------------------------------------|
| $a$ $(0, 0, t)$                                   | $a_1$ $\{2_{001}   0 \ 0 \ 0 \} \ \{m_{110}   0 \ 0 \ 0 \}$<br>0                 |
| $b$ $(\frac{1}{2}, \frac{1}{2}, \frac{t}{2})$     | $b_1$ $\{2_{001}   0 \ 0 \ 0 \} \ \{m_{110}   0 \ 0 \ 0 \}$<br>0                 |
| $c$ $(\frac{t}{2}, \frac{t}{2}, 1 - \frac{t}{2})$ | $c_1$ $\{m_{1-10}   0 \ 0 \ 0 \}$<br>$c_2$ $\begin{matrix} -i \\ i \end{matrix}$ |
| $d$ $(\frac{t}{2}, \frac{t}{2}, 0)$               | $d_1$ $\{m_{1-10}   0 \ 0 \ 0 \}$<br>$d_2$ $\begin{matrix} -i \\ i \end{matrix}$ |
| $e$ $(\frac{t}{2}, 1 - \frac{t}{2}, 0)$           | $e_1$ $\{m_{110}   0 \ 0 \ 0 \}$<br>$e_2$ $\begin{matrix} -i \\ i \end{matrix}$  |
| $f$ $(\frac{1-t}{2}, \frac{1}{2}, \frac{1}{2})$   | $f_1$ $\{2_{100}   0 \ 0 \ 0 \}$<br>$f_2$ $\begin{matrix} -i \\ i \end{matrix}$  |
| $g$ $(0, t, 0)$                                   | $g_1$ $\{2_{010}   0 \ 0 \ 0 \}$<br>$g_2$ $\begin{matrix} -i \\ i \end{matrix}$  |
| $h$ $(0, \frac{t}{2}, 1 - \frac{t}{2})$           | $h_1$ $\{1   0 \ 0 \ 0 \}$<br>1                                                  |

$$\begin{aligned} \mathcal{W}_1^{\text{gapless}} = & \sum_{m=1}^{n_{a_1}} \text{sgn}(v_m^{a_1}) \frac{1 - \text{sgn}(\delta_m^{a_1})}{2} + \sum_{m=1}^{n_{d_2}} \text{sgn}(v_m^{d_2}) \frac{1 - \text{sgn}(\delta_m^{d_2})}{2} - \sum_{m=1}^{n_{e_2}} \text{sgn}(v_m^{e_2}) \frac{1 - \text{sgn}(\delta_m^{e_2})}{2} \\ & - \sum_{m=1}^{n_{g_1}} \text{sgn}(v_m^{g_1}) \frac{1 - \text{sgn}(\delta_m^{g_1})}{2} - \sum_{m=1}^{n_{g_2}} \text{sgn}(v_m^{g_2}) \frac{1 - \text{sgn}(\delta_m^{g_2})}{2} \end{aligned} \quad (\text{S121.1})$$

$$\begin{aligned} \mathcal{W}_2^{\text{gapless}} = & \sum_{m=1}^{n_{b_1}} \text{sgn}(v_m^{b_1}) \frac{1 - \text{sgn}(\delta_m^{b_1})}{2} + \sum_{m=1}^{n_{c_2}} \text{sgn}(v_m^{c_2}) \frac{1 - \text{sgn}(\delta_m^{c_2})}{2} + \sum_{m=1}^{n_{e_1}} \text{sgn}(v_m^{e_1}) \frac{1 - \text{sgn}(\delta_m^{e_1})}{2} \\ & + \sum_{m=1}^{n_{f_1}} \text{sgn}(v_m^{f_1}) \frac{1 - \text{sgn}(\delta_m^{f_1})}{2} + \sum_{m=1}^{n_{f_2}} \text{sgn}(v_m^{f_2}) \frac{1 - \text{sgn}(\delta_m^{f_2})}{2} - \sum_{m=1}^{n_{h_1}} \text{sgn}(v_m^{h_1}) \frac{1 - \text{sgn}(\delta_m^{h_1})}{2} \end{aligned} \quad (\text{S121.2})$$

$$\begin{aligned} \mathcal{W}_3^{\text{gapless}} = & \sum_{m=1}^{n_{c_1}} \text{sgn}(v_m^{c_1}) \frac{1 - \text{sgn}(\delta_m^{c_1})}{2} + \sum_{m=1}^{n_{c_2}} \text{sgn}(v_m^{c_2}) \frac{1 - \text{sgn}(\delta_m^{c_2})}{2} + \sum_{m=1}^{n_{f_1}} \text{sgn}(v_m^{f_1}) \frac{1 - \text{sgn}(\delta_m^{f_1})}{2} \\ & + \sum_{m=1}^{n_{f_2}} \text{sgn}(v_m^{f_2}) \frac{1 - \text{sgn}(\delta_m^{f_2})}{2} - \sum_{m=1}^{n_{h_1}} \text{sgn}(v_m^{h_1}) \frac{1 - \text{sgn}(\delta_m^{h_1})}{2} \end{aligned} \quad (\text{S121.3})$$

$$\begin{aligned} \mathcal{W}_4^{\text{gapless}} = & 2 \sum_{m=1}^{n_{c_2}} \text{sgn}(v_m^{c_2}) \frac{1 - \text{sgn}(\delta_m^{c_2})}{2} + \sum_{m=1}^{n_{e_1}} \text{sgn}(v_m^{e_1}) \frac{1 - \text{sgn}(\delta_m^{e_1})}{2} - \sum_{m=1}^{n_{e_2}} \text{sgn}(v_m^{e_2}) \frac{1 - \text{sgn}(\delta_m^{e_2})}{2} \\ & + \sum_{m=1}^{n_{f_1}} \text{sgn}(v_m^{f_1}) \frac{1 - \text{sgn}(\delta_m^{f_1})}{2} + \sum_{m=1}^{n_{f_2}} \text{sgn}(v_m^{f_2}) \frac{1 - \text{sgn}(\delta_m^{f_2})}{2} - \sum_{m=1}^{n_{h_1}} \text{sgn}(v_m^{h_1}) \frac{1 - \text{sgn}(\delta_m^{h_1})}{2} \end{aligned} \quad (\text{S121.4})$$

$$\begin{aligned} \mathcal{W}_5^{\text{gapless}} = & \sum_{m=1}^{n_{d_1}} \text{sgn}(v_m^{d_1}) \frac{1 - \text{sgn}(\delta_m^{d_1})}{2} + \sum_{m=1}^{n_{d_2}} \text{sgn}(v_m^{d_2}) \frac{1 - \text{sgn}(\delta_m^{d_2})}{2} - \sum_{m=1}^{n_{e_1}} \text{sgn}(v_m^{e_1}) \frac{1 - \text{sgn}(\delta_m^{e_1})}{2} \\ & - \sum_{m=1}^{n_{e_2}} \text{sgn}(v_m^{e_2}) \frac{1 - \text{sgn}(\delta_m^{e_2})}{2} - \sum_{m=1}^{n_{g_1}} \text{sgn}(v_m^{g_1}) \frac{1 - \text{sgn}(\delta_m^{g_1})}{2} - \sum_{m=1}^{n_{g_2}} \text{sgn}(v_m^{g_2}) \frac{1 - \text{sgn}(\delta_m^{g_2})}{2} \end{aligned} \quad (\text{S121.5})$$

$$\mathcal{W}_6^{\text{gapless}} = 2 \sum_{m=1}^{n_{d_2}} \text{sgn}(v_m^{d_2}) \frac{1 - \text{sgn}(\delta_m^{d_2})}{2} - 2 \sum_{m=1}^{n_{e_2}} \text{sgn}(v_m^{e_2}) \frac{1 - \text{sgn}(\delta_m^{e_2})}{2} - \sum_{m=1}^{n_{g_1}} \text{sgn}(v_m^{g_1}) \frac{1 - \text{sgn}(\delta_m^{g_1})}{2} - \sum_{m=1}^{n_{g_2}} \text{sgn}(v_m^{g_2}) \frac{1 - \text{sgn}(\delta_m^{g_2})}{2} \quad (\text{S121.6})$$

$$\mathcal{W}_1^{\text{gapped}} = \sum_{m=1}^{n_{e_1}} \text{sgn}(v_m^{e_1}) \frac{1 - \text{sgn}(\delta_m^{e_1})}{2} - \sum_{m=1}^{n_{e_2}} \text{sgn}(v_m^{e_2}) \frac{1 - \text{sgn}(\delta_m^{e_2})}{2} \quad (\text{S121.7})$$

$$\mathcal{W}_2^{\text{gapped}} = - \sum_{m=1}^{n_{d_2}} \text{sgn}(v_m^{d_2}) \frac{1 - \text{sgn}(\delta_m^{d_2})}{2} + \sum_{m=1}^{n_{e_2}} \text{sgn}(v_m^{e_2}) \frac{1 - \text{sgn}(\delta_m^{e_2})}{2} + \sum_{m=1}^{n_{g_2}} \text{sgn}(v_m^{g_2}) \frac{1 - \text{sgn}(\delta_m^{g_2})}{2} \quad (\text{S121.8})$$

$$\mathcal{W}_3^{\text{gapped}} = \sum_{m=1}^{n_{f_1}} \text{sgn}(v_m^{f_1}) \frac{1 - \text{sgn}(\delta_m^{f_1})}{2} - \sum_{m=1}^{n_{f_2}} \text{sgn}(v_m^{f_2}) \frac{1 - \text{sgn}(\delta_m^{f_2})}{2} \quad (\text{S121.9})$$

## S122. SPACE GROUP NO. 122

| line segment                                          | character of irrep (generators only)                                                                                                                                                                                                                                                                    |
|-------------------------------------------------------|---------------------------------------------------------------------------------------------------------------------------------------------------------------------------------------------------------------------------------------------------------------------------------------------------------|
| $a \quad (0, 0, t)$                                   | $a_1 \quad \begin{Bmatrix} \{2_{001}   0 & 0 & 0\} \\ 0 \end{Bmatrix} \quad \begin{Bmatrix} \{m_{110}   0 & \frac{1}{2} & \frac{1}{4}\} \\ 0 \end{Bmatrix}$                                                                                                                                             |
| $b \quad (\frac{1}{2}, \frac{1}{2}, \frac{t}{2})$     | $\begin{Bmatrix} \{2_{001}   0 & 0 & 0\} \\ b_1 & -i & -e^{-\frac{1}{4}i\pi(t+2)} \\ b_2 & -i & e^{-\frac{1}{4}i\pi(t+2)} \\ b_3 & i & -e^{-\frac{1}{4}i\pi(t+2)} \\ b_4 & i & e^{-\frac{1}{4}i\pi(t+2)} \end{Bmatrix} \quad \begin{Bmatrix} \{m_{110}   0 & \frac{1}{2} & \frac{1}{4}\} \end{Bmatrix}$ |
| $c \quad (\frac{t}{2}, \frac{t}{2}, 1 - \frac{t}{2})$ | $\begin{Bmatrix} \{m_{1-10}   0 & \frac{1}{2} & \frac{1}{4}\} \\ c_1 & -ie^{-\frac{1}{4}i\pi(t+2)} \\ c_2 & ie^{-\frac{1}{4}i\pi(t+2)} \end{Bmatrix}$                                                                                                                                                   |
| $d \quad (\frac{t}{2}, \frac{t}{2}, 0)$               | $\begin{Bmatrix} \{m_{1-10}   0 & \frac{1}{2} & \frac{1}{4}\} \\ d_1 & -ie^{-\frac{1}{2}i\pi t} \\ d_2 & ie^{-\frac{1}{2}i\pi t} \end{Bmatrix}$                                                                                                                                                         |
| $e \quad (\frac{t}{2}, 1 - \frac{t}{2}, 0)$           | $\begin{Bmatrix} \{m_{110}   0 & \frac{1}{2} & \frac{1}{4}\} \\ e_1 & -e^{-\frac{1}{2}i\pi(2-t)} \\ e_2 & e^{-\frac{1}{2}i\pi(2-t)} \end{Bmatrix}$                                                                                                                                                      |
| $f \quad (\frac{1-t}{2}, \frac{1}{2}, \frac{1}{2})$   | $\begin{Bmatrix} \{2_{100}   0 & \frac{1}{2} & \frac{1}{4}\} \\ f_1 & i \\ f_2 & -i \end{Bmatrix}$                                                                                                                                                                                                      |
| $g \quad (0, t, 0)$                                   | $\begin{Bmatrix} \{2_{010}   0 & \frac{1}{2} & \frac{1}{4}\} \\ g_1 & -ie^{-i\pi t} \\ g_2 & ie^{-i\pi t} \end{Bmatrix}$                                                                                                                                                                                |
| $h \quad (0, \frac{t}{2}, 1 - \frac{t}{2})$           | $h_1 \quad \begin{Bmatrix} \{1   0 & 0 & 0\} \\ 1 \end{Bmatrix}$                                                                                                                                                                                                                                        |

---


$$\begin{aligned}
\mathcal{W}_1^{\text{gapless}} = & \sum_{m=1}^{n_{a_1}} \text{sgn}(v_m^{a_1}) \frac{1 - \text{sgn}(\delta_m^{a_1})}{2} + \sum_{m=1}^{n_{b_3}} \text{sgn}(v_m^{b_3}) \frac{1 - \text{sgn}(\delta_m^{b_3})}{2} - \sum_{m=1}^{n_{b_4}} \text{sgn}(v_m^{b_4}) \frac{1 - \text{sgn}(\delta_m^{b_4})}{2} \\
& + 2 \sum_{m=1}^{n_{c_2}} \text{sgn}(v_m^{c_2}) \frac{1 - \text{sgn}(\delta_m^{c_2})}{2} - \sum_{m=1}^{n_{d_2}} \text{sgn}(v_m^{d_2}) \frac{1 - \text{sgn}(\delta_m^{d_2})}{2} + \sum_{m=1}^{n_{e_1}} \text{sgn}(v_m^{e_1}) \frac{1 - \text{sgn}(\delta_m^{e_1})}{2} \\
& + \sum_{m=1}^{n_{f_1}} \text{sgn}(v_m^{f_1}) \frac{1 - \text{sgn}(\delta_m^{f_1})}{2} + \sum_{m=1}^{n_{f_2}} \text{sgn}(v_m^{f_2}) \frac{1 - \text{sgn}(\delta_m^{f_2})}{2} - \sum_{m=1}^{n_{h_1}} \text{sgn}(v_m^{h_1}) \frac{1 - \text{sgn}(\delta_m^{h_1})}{2}
\end{aligned} \tag{S122.1}$$

$$\begin{aligned}
\mathcal{W}_2^{\text{gapless}} = & \sum_{m=1}^{n_{b_1}} \text{sgn}(v_m^{b_1}) \frac{1 - \text{sgn}(\delta_m^{b_1})}{2} + \sum_{m=1}^{n_{b_3}} \text{sgn}(v_m^{b_3}) \frac{1 - \text{sgn}(\delta_m^{b_3})}{2} + \sum_{m=1}^{n_{c_2}} \text{sgn}(v_m^{c_2}) \frac{1 - \text{sgn}(\delta_m^{c_2})}{2} + \sum_{m=1}^{n_{e_1}} \text{sgn}(v_m^{e_1}) \frac{1 - \text{sgn}(\delta_m^{e_1})}{2} \\
& + \sum_{m=1}^{n_{f_1}} \text{sgn}(v_m^{f_1}) \frac{1 - \text{sgn}(\delta_m^{f_1})}{2} + \sum_{m=1}^{n_{f_2}} \text{sgn}(v_m^{f_2}) \frac{1 - \text{sgn}(\delta_m^{f_2})}{2} - \sum_{m=1}^{n_{h_1}} \text{sgn}(v_m^{h_1}) \frac{1 - \text{sgn}(\delta_m^{h_1})}{2}
\end{aligned} \tag{S122.2}$$

$$\begin{aligned}
\mathcal{W}_3^{\text{gapless}} = & \sum_{m=1}^{n_{b_2}} \text{sgn}(v_m^{b_2}) \frac{1 - \text{sgn}(\delta_m^{b_2})}{2} + \sum_{m=1}^{n_{b_4}} \text{sgn}(v_m^{b_4}) \frac{1 - \text{sgn}(\delta_m^{b_4})}{2} - \sum_{m=1}^{n_{c_2}} \text{sgn}(v_m^{c_2}) \frac{1 - \text{sgn}(\delta_m^{c_2})}{2} + \sum_{m=1}^{n_{e_1}} \text{sgn}(v_m^{e_1}) \frac{1 - \text{sgn}(\delta_m^{e_1})}{2}
\end{aligned} \tag{S122.3}$$

$$\begin{aligned}
\mathcal{W}_4^{\text{gapless}} = & 2 \sum_{m=1}^{n_{b_3}} \text{sgn}(v_m^{b_3}) \frac{1 - \text{sgn}(\delta_m^{b_3})}{2} - 2 \sum_{m=1}^{n_{b_4}} \text{sgn}(v_m^{b_4}) \frac{1 - \text{sgn}(\delta_m^{b_4})}{2} + 4 \sum_{m=1}^{n_{c_2}} \text{sgn}(v_m^{c_2}) \frac{1 - \text{sgn}(\delta_m^{c_2})}{2} \\
& - 2 \sum_{m=1}^{n_{d_2}} \text{sgn}(v_m^{d_2}) \frac{1 - \text{sgn}(\delta_m^{d_2})}{2} + 2 \sum_{m=1}^{n_{e_1}} \text{sgn}(v_m^{e_1}) \frac{1 - \text{sgn}(\delta_m^{e_1})}{2} + 2 \sum_{m=1}^{n_{f_1}} \text{sgn}(v_m^{f_1}) \frac{1 - \text{sgn}(\delta_m^{f_1})}{2} \\
& + 2 \sum_{m=1}^{n_{f_2}} \text{sgn}(v_m^{f_2}) \frac{1 - \text{sgn}(\delta_m^{f_2})}{2} + \sum_{m=1}^{n_{g_1}} \text{sgn}(v_m^{g_1}) \frac{1 - \text{sgn}(\delta_m^{g_1})}{2} + \sum_{m=1}^{n_{g_2}} \text{sgn}(v_m^{g_2}) \frac{1 - \text{sgn}(\delta_m^{g_2})}{2} \\
& - 2 \sum_{m=1}^{n_{h_1}} \text{sgn}(v_m^{h_1}) \frac{1 - \text{sgn}(\delta_m^{h_1})}{2}
\end{aligned} \tag{S122.4}$$

$$\begin{aligned}
\mathcal{W}_5^{\text{gapless}} = & \sum_{m=1}^{n_{c_1}} \text{sgn}(v_m^{c_1}) \frac{1 - \text{sgn}(\delta_m^{c_1})}{2} + \sum_{m=1}^{n_{c_2}} \text{sgn}(v_m^{c_2}) \frac{1 - \text{sgn}(\delta_m^{c_2})}{2} + \sum_{m=1}^{n_{f_1}} \text{sgn}(v_m^{f_1}) \frac{1 - \text{sgn}(\delta_m^{f_1})}{2} \\
& + \sum_{m=1}^{n_{f_2}} \text{sgn}(v_m^{f_2}) \frac{1 - \text{sgn}(\delta_m^{f_2})}{2} - \sum_{m=1}^{n_{h_1}} \text{sgn}(v_m^{h_1}) \frac{1 - \text{sgn}(\delta_m^{h_1})}{2}
\end{aligned} \tag{S122.5}$$

$$\begin{aligned}
\mathcal{W}_6^{\text{gapless}} = & \sum_{m=1}^{n_{d_1}} \text{sgn}(v_m^{d_1}) \frac{1 - \text{sgn}(\delta_m^{d_1})}{2} + \sum_{m=1}^{n_{d_2}} \text{sgn}(v_m^{d_2}) \frac{1 - \text{sgn}(\delta_m^{d_2})}{2} - 2 \sum_{m=1}^{n_{e_1}} \text{sgn}(v_m^{e_1}) \frac{1 - \text{sgn}(\delta_m^{e_1})}{2} \\
& - \sum_{m=1}^{n_{g_1}} \text{sgn}(v_m^{g_1}) \frac{1 - \text{sgn}(\delta_m^{g_1})}{2} - \sum_{m=1}^{n_{g_2}} \text{sgn}(v_m^{g_2}) \frac{1 - \text{sgn}(\delta_m^{g_2})}{2}
\end{aligned} \tag{S122.6}$$

$$\begin{aligned}
\mathcal{W}_1^{\text{gapped}} = & - \sum_{m=1}^{n_{b_3}} \text{sgn}(v_m^{b_3}) \frac{1 - \text{sgn}(\delta_m^{b_3})}{2} + \sum_{m=1}^{n_{b_4}} \text{sgn}(v_m^{b_4}) \frac{1 - \text{sgn}(\delta_m^{b_4})}{2} - 2 \sum_{m=1}^{n_{c_2}} \text{sgn}(v_m^{c_2}) \frac{1 - \text{sgn}(\delta_m^{c_2})}{2} \\
& + \sum_{m=1}^{n_{d_2}} \text{sgn}(v_m^{d_2}) \frac{1 - \text{sgn}(\delta_m^{d_2})}{2} - \sum_{m=1}^{n_{e_1}} \text{sgn}(v_m^{e_1}) \frac{1 - \text{sgn}(\delta_m^{e_1})}{2} - \sum_{m=1}^{n_{f_1}} \text{sgn}(v_m^{f_1}) \frac{1 - \text{sgn}(\delta_m^{f_1})}{2} \\
& - \sum_{m=1}^{n_{f_2}} \text{sgn}(v_m^{f_2}) \frac{1 - \text{sgn}(\delta_m^{f_2})}{2} - \sum_{m=1}^{n_{g_1}} \text{sgn}(v_m^{g_1}) \frac{1 - \text{sgn}(\delta_m^{g_1})}{2} + \sum_{m=1}^{n_{h_1}} \text{sgn}(v_m^{h_1}) \frac{1 - \text{sgn}(\delta_m^{h_1})}{2}
\end{aligned} \tag{S122.7}$$

$$\mathcal{X}_1 = \sum_{m=1}^{n_{d_2}} \frac{1 - \text{sgn}(\delta_m^{d_2})}{2} + \sum_{m=1}^{n_{g_1}} \frac{1 - \text{sgn}(\delta_m^{g_1})}{2} + \sum_{m=1}^{n_{h_1}} \frac{1 - \text{sgn}(\delta_m^{h_1})}{2} \mod 2 \tag{S122.8}$$

$$\mathcal{X}_2 = \sum_{m=1}^{n_{d_2}} \frac{1 - \text{sgn}(\delta_m^{d_2})}{2} + \sum_{m=1}^{n_{g_1}} \frac{1 - \text{sgn}(\delta_m^{g_1})}{2} \mod 2 \tag{S122.9}$$

### S123. SPACE GROUP NO. 123

| line segment                                        | character of irrep (generators only)                                                                                           |
|-----------------------------------------------------|--------------------------------------------------------------------------------------------------------------------------------|
| $a \quad (0, \frac{t}{2}, 0)$                       | $a_1 \quad \begin{array}{cc} \{2_{010}   0 & 0 & 0\} & \{m_{100}   0 & 0 & 0\} \\ 0 & 0 \end{array}$                           |
| $b \quad (\frac{1-t}{2}, \frac{1}{2}, 0)$           | $b_1 \quad \begin{array}{cc} \{2_{100}   0 & 0 & 0\} & \{m_{010}   0 & 0 & 0\} \\ 0 & 0 \end{array}$                           |
| $c \quad (\frac{t}{2}, \frac{t}{2}, 0)$             | $c_1 \quad \begin{array}{cc} \{2_{110}   0 & 0 & 0\} & \{m_{001}   0 & 0 & 0\} \\ 0 & 0 \end{array}$                           |
| $d \quad (0, \frac{t}{2}, \frac{1}{2})$             | $d_1 \quad \begin{array}{cc} \{2_{010}   0 & 0 & 0\} & \{m_{100}   0 & 0 & 0\} \\ 0 & 0 \end{array}$                           |
| $e \quad (\frac{1-t}{2}, \frac{1}{2}, \frac{1}{2})$ | $e_1 \quad \begin{array}{cc} \{2_{100}   0 & 0 & 0\} & \{m_{010}   0 & 0 & 0\} \\ 0 & 0 \end{array}$                           |
| $f \quad (\frac{t}{2}, \frac{t}{2}, \frac{1}{2})$   | $f_1 \quad \begin{array}{cc} \{2_{110}   0 & 0 & 0\} & \{m_{001}   0 & 0 & 0\} \\ 0 & 0 \end{array}$                           |
| $g \quad (0, 0, \frac{t}{2})$                       | $\begin{array}{cc} \{4_{001}   0 & 0 & 0\} & \{m_{100}   0 & 0 & 0\} \\ g_1 & -\sqrt{2} & 0 \\ g_2 & \sqrt{2} & 0 \end{array}$ |
| $h \quad (0, \frac{1}{2}, \frac{t}{2})$             | $h_1 \quad \begin{array}{cc} \{2_{001}   0 & 0 & 0\} & \{m_{100}   0 & 0 & 0\} \\ 0 & 0 \end{array}$                           |
| $i \quad (\frac{1}{2}, \frac{1}{2}, \frac{t}{2})$   | $\begin{array}{cc} \{4_{001}   0 & 0 & 0\} & \{m_{100}   0 & 0 & 0\} \\ i_1 & -\sqrt{2} & 0 \\ i_2 & \sqrt{2} & 0 \end{array}$ |

$$\begin{aligned}
\mathcal{W}_1^{\text{gapless}} = & \sum_{m=1}^{n_{a_1}} \text{sgn}(v_m^{a_1}) \frac{1 - \text{sgn}(\delta_m^{a_1})}{2} - \sum_{m=1}^{n_{e_1}} \text{sgn}(v_m^{e_1}) \frac{1 - \text{sgn}(\delta_m^{e_1})}{2} - \sum_{m=1}^{n_{f_1}} \text{sgn}(v_m^{f_1}) \frac{1 - \text{sgn}(\delta_m^{f_1})}{2} \\
& - \sum_{m=1}^{n_{g_1}} \text{sgn}(v_m^{g_1}) \frac{1 - \text{sgn}(\delta_m^{g_1})}{2} - \sum_{m=1}^{n_{g_2}} \text{sgn}(v_m^{g_2}) \frac{1 - \text{sgn}(\delta_m^{g_2})}{2} + \sum_{m=1}^{n_{h_1}} \text{sgn}(v_m^{h_1}) \frac{1 - \text{sgn}(\delta_m^{h_1})}{2}
\end{aligned} \tag{S123.1}$$

$$\begin{aligned} \mathcal{W}_2^{\text{gapless}} = & \sum_{m=1}^{n_{b_1}} \text{sgn}(v_m^{b_1}) \frac{1 - \text{sgn}(\delta_m^{b_1})}{2} - \sum_{m=1}^{n_{e_1}} \text{sgn}(v_m^{e_1}) \frac{1 - \text{sgn}(\delta_m^{e_1})}{2} + \sum_{m=1}^{n_{h_1}} \text{sgn}(v_m^{h_1}) \frac{1 - \text{sgn}(\delta_m^{h_1})}{2} \\ & - \sum_{m=1}^{n_{i_1}} \text{sgn}(v_m^{i_1}) \frac{1 - \text{sgn}(\delta_m^{i_1})}{2} - \sum_{m=1}^{n_{i_2}} \text{sgn}(v_m^{i_2}) \frac{1 - \text{sgn}(\delta_m^{i_2})}{2} \end{aligned} \quad (\text{S123.2})$$

$$\begin{aligned} \mathcal{W}_3^{\text{gapless}} = & \sum_{m=1}^{n_{c_1}} \text{sgn}(v_m^{c_1}) \frac{1 - \text{sgn}(\delta_m^{c_1})}{2} - \sum_{m=1}^{n_{f_1}} \text{sgn}(v_m^{f_1}) \frac{1 - \text{sgn}(\delta_m^{f_1})}{2} - \sum_{m=1}^{n_{g_1}} \text{sgn}(v_m^{g_1}) \frac{1 - \text{sgn}(\delta_m^{g_1})}{2} \\ & - \sum_{m=1}^{n_{g_2}} \text{sgn}(v_m^{g_2}) \frac{1 - \text{sgn}(\delta_m^{g_2})}{2} + \sum_{m=1}^{n_{i_1}} \text{sgn}(v_m^{i_1}) \frac{1 - \text{sgn}(\delta_m^{i_1})}{2} + \sum_{m=1}^{n_{i_2}} \text{sgn}(v_m^{i_2}) \frac{1 - \text{sgn}(\delta_m^{i_2})}{2} \end{aligned} \quad (\text{S123.3})$$

$$\mathcal{W}_4^{\text{gapless}} = \sum_{m=1}^{n_{d_1}} \text{sgn}(v_m^{d_1}) \frac{1 - \text{sgn}(\delta_m^{d_1})}{2} - \sum_{m=1}^{n_{e_1}} \text{sgn}(v_m^{e_1}) \frac{1 - \text{sgn}(\delta_m^{e_1})}{2} - \sum_{m=1}^{n_{f_1}} \text{sgn}(v_m^{f_1}) \frac{1 - \text{sgn}(\delta_m^{f_1})}{2} \quad (\text{S123.4})$$

#### S124. SPACE GROUP NO. 124

| line segment                                        | character of irrep (generators only) |                                     |
|-----------------------------------------------------|--------------------------------------|-------------------------------------|
| $a \quad (0, \frac{t}{2}, 0)$                       | $\{2_{010}   0 \ 0 \ \frac{1}{2}\}$  | $\{m_{100}   0 \ 0 \ \frac{1}{2}\}$ |
|                                                     | $a_1 \quad 0$                        | $0$                                 |
| $b \quad (\frac{1-t}{2}, \frac{1}{2}, 0)$           | $\{2_{100}   0 \ 0 \ \frac{1}{2}\}$  | $\{m_{010}   0 \ 0 \ \frac{1}{2}\}$ |
|                                                     | $b_1 \quad 0$                        | $0$                                 |
| $c \quad (\frac{t}{2}, \frac{t}{2}, 0)$             | $\{2_{110}   0 \ 0 \ \frac{1}{2}\}$  | $\{m_{001}   0 \ 0 \ 0\}$           |
|                                                     | $c_1 \quad 0$                        | $0$                                 |
| $d \quad (0, \frac{t}{2}, \frac{1}{2})$             | $\{2_{010}   0 \ 0 \ \frac{1}{2}\}$  | $\{m_{100}   0 \ 0 \ \frac{1}{2}\}$ |
|                                                     | $d_1 \quad i$                        | $-1$                                |
|                                                     | $d_2 \quad i$                        | $1$                                 |
|                                                     | $d_3 \quad -i$                       | $-1$                                |
|                                                     | $d_4 \quad -i$                       | $1$                                 |
| $e \quad (\frac{1-t}{2}, \frac{1}{2}, \frac{1}{2})$ | $\{2_{100}   0 \ 0 \ \frac{1}{2}\}$  | $\{m_{010}   0 \ 0 \ \frac{1}{2}\}$ |
|                                                     | $e_1 \quad i$                        | $-1$                                |
|                                                     | $e_2 \quad i$                        | $1$                                 |
|                                                     | $e_3 \quad -i$                       | $-1$                                |
|                                                     | $e_4 \quad -i$                       | $1$                                 |
| $f \quad (\frac{t}{2}, \frac{t}{2}, \frac{1}{2})$   | $\{2_{110}   0 \ 0 \ \frac{1}{2}\}$  | $\{m_{001}   0 \ 0 \ 0\}$           |
|                                                     | $f_1 \quad i$                        | $-i$                                |
|                                                     | $f_2 \quad i$                        | $i$                                 |
|                                                     | $f_3 \quad -i$                       | $-i$                                |
|                                                     | $f_4 \quad -i$                       | $i$                                 |
| $g \quad (0, 0, \frac{t}{2})$                       | $\{4_{001}   0 \ 0 \ 0\}$            | $\{m_{100}   0 \ 0 \ \frac{1}{2}\}$ |
|                                                     | $g_1 \quad -\sqrt{2}$                | $0$                                 |
|                                                     | $g_2 \quad \sqrt{2}$                 | $0$                                 |
| $h \quad (0, \frac{1}{2}, \frac{t}{2})$             | $\{2_{001}   0 \ 0 \ 0\}$            | $\{m_{100}   0 \ 0 \ \frac{1}{2}\}$ |
|                                                     | $h_1 \quad 0$                        | $0$                                 |
| $i \quad (\frac{1}{2}, \frac{1}{2}, \frac{t}{2})$   | $\{4_{001}   0 \ 0 \ 0\}$            | $\{m_{100}   0 \ 0 \ \frac{1}{2}\}$ |
|                                                     | $i_1 \quad -\sqrt{2}$                | $0$                                 |
|                                                     | $i_2 \quad \sqrt{2}$                 | $0$                                 |

---


$$\begin{aligned}
\mathcal{W}_1^{\text{gapless}} = & \sum_{m=1}^{n_{a_1}} \text{sgn}(v_m^{a_1}) \frac{1 - \text{sgn}(\delta_m^{a_1})}{2} - \sum_{m=1}^{n_{e_1}} \text{sgn}(v_m^{e_1}) \frac{1 - \text{sgn}(\delta_m^{e_1})}{2} - \sum_{m=1}^{n_{e_3}} \text{sgn}(v_m^{e_3}) \frac{1 - \text{sgn}(\delta_m^{e_3})}{2} \\
& - \sum_{m=1}^{n_{f_1}} \text{sgn}(v_m^{f_1}) \frac{1 - \text{sgn}(\delta_m^{f_1})}{2} - \sum_{m=1}^{n_{f_3}} \text{sgn}(v_m^{f_3}) \frac{1 - \text{sgn}(\delta_m^{f_3})}{2} - \sum_{m=1}^{n_{g_1}} \text{sgn}(v_m^{g_1}) \frac{1 - \text{sgn}(\delta_m^{g_1})}{2} \\
& - \sum_{m=1}^{n_{g_2}} \text{sgn}(v_m^{g_2}) \frac{1 - \text{sgn}(\delta_m^{g_2})}{2} + \sum_{m=1}^{n_{h_1}} \text{sgn}(v_m^{h_1}) \frac{1 - \text{sgn}(\delta_m^{h_1})}{2}
\end{aligned} \tag{S124.1}$$

$$\begin{aligned}
\mathcal{W}_2^{\text{gapless}} = & \sum_{m=1}^{n_{b_1}} \text{sgn}(v_m^{b_1}) \frac{1 - \text{sgn}(\delta_m^{b_1})}{2} - \sum_{m=1}^{n_{e_1}} \text{sgn}(v_m^{e_1}) \frac{1 - \text{sgn}(\delta_m^{e_1})}{2} - \sum_{m=1}^{n_{e_3}} \text{sgn}(v_m^{e_3}) \frac{1 - \text{sgn}(\delta_m^{e_3})}{2} \\
& + \sum_{m=1}^{n_{h_1}} \text{sgn}(v_m^{h_1}) \frac{1 - \text{sgn}(\delta_m^{h_1})}{2} - \sum_{m=1}^{n_{i_1}} \text{sgn}(v_m^{i_1}) \frac{1 - \text{sgn}(\delta_m^{i_1})}{2} - \sum_{m=1}^{n_{i_2}} \text{sgn}(v_m^{i_2}) \frac{1 - \text{sgn}(\delta_m^{i_2})}{2}
\end{aligned} \tag{S124.2}$$

$$\begin{aligned}
\mathcal{W}_3^{\text{gapless}} = & \sum_{m=1}^{n_{c_1}} \text{sgn}(v_m^{c_1}) \frac{1 - \text{sgn}(\delta_m^{c_1})}{2} - \sum_{m=1}^{n_{f_1}} \text{sgn}(v_m^{f_1}) \frac{1 - \text{sgn}(\delta_m^{f_1})}{2} - \sum_{m=1}^{n_{f_3}} \text{sgn}(v_m^{f_3}) \frac{1 - \text{sgn}(\delta_m^{f_3})}{2} - \sum_{m=1}^{n_{g_1}} \text{sgn}(v_m^{g_1}) \frac{1 - \text{sgn}(\delta_m^{g_1})}{2} \\
& - \sum_{m=1}^{n_{g_2}} \text{sgn}(v_m^{g_2}) \frac{1 - \text{sgn}(\delta_m^{g_2})}{2} + \sum_{m=1}^{n_{i_1}} \text{sgn}(v_m^{i_1}) \frac{1 - \text{sgn}(\delta_m^{i_1})}{2} + \sum_{m=1}^{n_{i_2}} \text{sgn}(v_m^{i_2}) \frac{1 - \text{sgn}(\delta_m^{i_2})}{2}
\end{aligned} \tag{S124.3}$$

$$\begin{aligned}
\mathcal{W}_4^{\text{gapless}} = & \sum_{m=1}^{n_{d_1}} \text{sgn}(v_m^{d_1}) \frac{1 - \text{sgn}(\delta_m^{d_1})}{2} + \sum_{m=1}^{n_{d_3}} \text{sgn}(v_m^{d_3}) \frac{1 - \text{sgn}(\delta_m^{d_3})}{2} - \sum_{m=1}^{n_{e_1}} \text{sgn}(v_m^{e_1}) \frac{1 - \text{sgn}(\delta_m^{e_1})}{2} \\
& - \sum_{m=1}^{n_{e_3}} \text{sgn}(v_m^{e_3}) \frac{1 - \text{sgn}(\delta_m^{e_3})}{2} - \sum_{m=1}^{n_{f_1}} \text{sgn}(v_m^{f_1}) \frac{1 - \text{sgn}(\delta_m^{f_1})}{2} - \sum_{m=1}^{n_{f_3}} \text{sgn}(v_m^{f_3}) \frac{1 - \text{sgn}(\delta_m^{f_3})}{2}
\end{aligned} \tag{S124.4}$$

$$\mathcal{W}_1^{\text{gapped}} = - \sum_{m=1}^{n_{e_1}} \text{sgn}(v_m^{e_1}) \frac{1 - \text{sgn}(\delta_m^{e_1})}{2} + \sum_{m=1}^{n_{e_3}} \text{sgn}(v_m^{e_3}) \frac{1 - \text{sgn}(\delta_m^{e_3})}{2} \tag{S124.5}$$

$$\mathcal{W}_2^{\text{gapped}} = - \sum_{m=1}^{n_{d_3}} \text{sgn}(v_m^{d_3}) \frac{1 - \text{sgn}(\delta_m^{d_3})}{2} + \sum_{m=1}^{n_{e_1}} \text{sgn}(v_m^{e_1}) \frac{1 - \text{sgn}(\delta_m^{e_1})}{2} + \sum_{m=1}^{n_{f_1}} \text{sgn}(v_m^{f_1}) \frac{1 - \text{sgn}(\delta_m^{f_1})}{2} \tag{S124.6}$$

$$\mathcal{W}_3^{\text{gapped}} = - \sum_{m=1}^{n_{d_3}} \text{sgn}(v_m^{d_3}) \frac{1 - \text{sgn}(\delta_m^{d_3})}{2} + \sum_{m=1}^{n_{e_1}} \text{sgn}(v_m^{e_1}) \frac{1 - \text{sgn}(\delta_m^{e_1})}{2} + \sum_{m=1}^{n_{f_3}} \text{sgn}(v_m^{f_3}) \frac{1 - \text{sgn}(\delta_m^{f_3})}{2} \tag{S124.7}$$



## S125. SPACE GROUP NO. 125

| line segment                                    | character of irrep (generators only)                                                                                                                                          |
|-------------------------------------------------|-------------------------------------------------------------------------------------------------------------------------------------------------------------------------------|
| $a \ (0, \frac{t}{2}, 0)$                       | $a_1 \ \begin{Bmatrix} \{2_{010}   \frac{1}{2} & 0 & 0\} \\ 0 \end{Bmatrix} \ \begin{Bmatrix} \{m_{100}   0 & \frac{1}{2} & 0\} \\ 0 \end{Bmatrix}$                           |
| $b \ (\frac{1-t}{2}, \frac{1}{2}, 0)$           | $b_1 \ \begin{Bmatrix} \{2_{100}   0 & \frac{1}{2} & 0\} \\ i \end{Bmatrix} \ \begin{Bmatrix} \{m_{010}   \frac{1}{2} & 0 & 0\} \\ -ie^{-\frac{1}{2}i\pi(1-t)} \end{Bmatrix}$ |
|                                                 | $b_2 \ \begin{Bmatrix} i \\ ie^{-\frac{1}{2}i\pi(1-t)} \end{Bmatrix}$                                                                                                         |
|                                                 | $b_3 \ \begin{Bmatrix} -i \\ -ie^{-\frac{1}{2}i\pi(1-t)} \end{Bmatrix}$                                                                                                       |
|                                                 | $b_4 \ \begin{Bmatrix} -i \\ ie^{-\frac{1}{2}i\pi(1-t)} \end{Bmatrix}$                                                                                                        |
| $c \ (\frac{t}{2}, \frac{t}{2}, 0)$             | $c_1 \ \begin{Bmatrix} \{2_{110}   0 & 0 & 0\} \\ 0 \end{Bmatrix} \ \begin{Bmatrix} \{m_{001}   \frac{1}{2} & \frac{1}{2} & 0\} \\ 0 \end{Bmatrix}$                           |
| $d \ (0, \frac{t}{2}, \frac{1}{2})$             | $d_1 \ \begin{Bmatrix} \{2_{010}   \frac{1}{2} & 0 & 0\} \\ 0 \end{Bmatrix} \ \begin{Bmatrix} \{m_{100}   0 & \frac{1}{2} & 0\} \\ 0 \end{Bmatrix}$                           |
| $e \ (\frac{1-t}{2}, \frac{1}{2}, \frac{1}{2})$ | $e_1 \ \begin{Bmatrix} \{2_{100}   0 & \frac{1}{2} & 0\} \\ i \end{Bmatrix} \ \begin{Bmatrix} \{m_{010}   \frac{1}{2} & 0 & 0\} \\ -ie^{-\frac{1}{2}i\pi(1-t)} \end{Bmatrix}$ |
|                                                 | $e_2 \ \begin{Bmatrix} i \\ ie^{-\frac{1}{2}i\pi(1-t)} \end{Bmatrix}$                                                                                                         |
|                                                 | $e_3 \ \begin{Bmatrix} -i \\ -ie^{-\frac{1}{2}i\pi(1-t)} \end{Bmatrix}$                                                                                                       |
|                                                 | $e_4 \ \begin{Bmatrix} -i \\ ie^{-\frac{1}{2}i\pi(1-t)} \end{Bmatrix}$                                                                                                        |
| $f \ (\frac{t}{2}, \frac{t}{2}, \frac{1}{2})$   | $f_1 \ \begin{Bmatrix} \{2_{110}   0 & 0 & 0\} \\ 0 \end{Bmatrix} \ \begin{Bmatrix} \{m_{001}   \frac{1}{2} & \frac{1}{2} & 0\} \\ 0 \end{Bmatrix}$                           |
| $g \ (0, 0, \frac{t}{2})$                       | $g_1 \ \begin{Bmatrix} \{4_{001}   \frac{1}{2} & 0 & 0\} \\ -\sqrt{2} \end{Bmatrix} \ \begin{Bmatrix} \{m_{100}   0 & \frac{1}{2} & 0\} \\ 0 \end{Bmatrix}$                   |
|                                                 | $g_2 \ \begin{Bmatrix} \sqrt{2} \\ 0 \end{Bmatrix}$                                                                                                                           |
| $h \ (0, \frac{1}{2}, \frac{t}{2})$             | $h_1 \ \begin{Bmatrix} \{2_{001}   \frac{1}{2} & \frac{1}{2} & 0\} \\ i \end{Bmatrix} \ \begin{Bmatrix} \{m_{100}   0 & \frac{1}{2} & 0\} \\ -1 \end{Bmatrix}$                |
|                                                 | $h_2 \ \begin{Bmatrix} i \\ 1 \end{Bmatrix}$                                                                                                                                  |
|                                                 | $h_3 \ \begin{Bmatrix} -i \\ -1 \end{Bmatrix}$                                                                                                                                |
|                                                 | $h_4 \ \begin{Bmatrix} -i \\ 1 \end{Bmatrix}$                                                                                                                                 |
| $i \ (\frac{1}{2}, \frac{1}{2}, \frac{t}{2})$   | $i_1 \ \begin{Bmatrix} \{4_{001}   \frac{1}{2} & 0 & 0\} \\ i\sqrt{2} \end{Bmatrix} \ \begin{Bmatrix} \{m_{100}   0 & \frac{1}{2} & 0\} \\ 0 \end{Bmatrix}$                   |
|                                                 | $i_2 \ \begin{Bmatrix} -i\sqrt{2} \\ 0 \end{Bmatrix}$                                                                                                                         |

$$\begin{aligned}
\mathcal{W}_1^{\text{gapless}} = & \sum_{m=1}^{n_{a_1}} \text{sgn}(v_m^{a_1}) \frac{1 - \text{sgn}(\delta_m^{a_1})}{2} - \sum_{m=1}^{n_{e_1}} \text{sgn}(v_m^{e_1}) \frac{1 - \text{sgn}(\delta_m^{e_1})}{2} - \sum_{m=1}^{n_{e_3}} \text{sgn}(v_m^{e_3}) \frac{1 - \text{sgn}(\delta_m^{e_3})}{2} \\
& - \sum_{m=1}^{n_{f_1}} \text{sgn}(v_m^{f_1}) \frac{1 - \text{sgn}(\delta_m^{f_1})}{2} - \sum_{m=1}^{n_{g_1}} \text{sgn}(v_m^{g_1}) \frac{1 - \text{sgn}(\delta_m^{g_1})}{2} - \sum_{m=1}^{n_{g_2}} \text{sgn}(v_m^{g_2}) \frac{1 - \text{sgn}(\delta_m^{g_2})}{2} \\
& + \sum_{m=1}^{n_{h_1}} \text{sgn}(v_m^{h_1}) \frac{1 - \text{sgn}(\delta_m^{h_1})}{2} + \sum_{m=1}^{n_{h_3}} \text{sgn}(v_m^{h_3}) \frac{1 - \text{sgn}(\delta_m^{h_3})}{2}
\end{aligned} \tag{S125.1}$$

$$\begin{aligned}
\mathcal{W}_2^{\text{gapless}} = & \sum_{m=1}^{n_{b_1}} \text{sgn}(v_m^{b_1}) \frac{1 - \text{sgn}(\delta_m^{b_1})}{2} + \sum_{m=1}^{n_{b_3}} \text{sgn}(v_m^{b_3}) \frac{1 - \text{sgn}(\delta_m^{b_3})}{2} - \sum_{m=1}^{n_{e_1}} \text{sgn}(v_m^{e_1}) \frac{1 - \text{sgn}(\delta_m^{e_1})}{2} \\
& - \sum_{m=1}^{n_{e_3}} \text{sgn}(v_m^{e_3}) \frac{1 - \text{sgn}(\delta_m^{e_3})}{2} + \sum_{m=1}^{n_{h_1}} \text{sgn}(v_m^{h_1}) \frac{1 - \text{sgn}(\delta_m^{h_1})}{2} \\
& + \sum_{m=1}^{n_{h_3}} \text{sgn}(v_m^{h_3}) \frac{1 - \text{sgn}(\delta_m^{h_3})}{2} - \sum_{m=1}^{n_{i_1}} \text{sgn}(v_m^{i_1}) \frac{1 - \text{sgn}(\delta_m^{i_1})}{2} - \sum_{m=1}^{n_{i_2}} \text{sgn}(v_m^{i_2}) \frac{1 - \text{sgn}(\delta_m^{i_2})}{2}
\end{aligned} \tag{S125.2}$$

$$\begin{aligned} \mathcal{W}_3^{\text{gapless}} = & \sum_{m=1}^{n_{c_1}} \text{sgn}(v_m^{c_1}) \frac{1 - \text{sgn}(\delta_m^{c_1})}{2} - \sum_{m=1}^{n_{f_1}} \text{sgn}(v_m^{f_1}) \frac{1 - \text{sgn}(\delta_m^{f_1})}{2} - \sum_{m=1}^{n_{g_1}} \text{sgn}(v_m^{g_1}) \frac{1 - \text{sgn}(\delta_m^{g_1})}{2} \\ & - \sum_{m=1}^{n_{g_2}} \text{sgn}(v_m^{g_2}) \frac{1 - \text{sgn}(\delta_m^{g_2})}{2} + \sum_{m=1}^{n_{i_1}} \text{sgn}(v_m^{i_1}) \frac{1 - \text{sgn}(\delta_m^{i_1})}{2} + \sum_{m=1}^{n_{i_2}} \text{sgn}(v_m^{i_2}) \frac{1 - \text{sgn}(\delta_m^{i_2})}{2} \end{aligned} \quad (\text{S125.3})$$

$$\mathcal{W}_4^{\text{gapless}} = \sum_{m=1}^{n_{d_1}} \text{sgn}(v_m^{d_1}) \frac{1 - \text{sgn}(\delta_m^{d_1})}{2} - \sum_{m=1}^{n_{e_1}} \text{sgn}(v_m^{e_1}) \frac{1 - \text{sgn}(\delta_m^{e_1})}{2} - \sum_{m=1}^{n_{e_3}} \text{sgn}(v_m^{e_3}) \frac{1 - \text{sgn}(\delta_m^{e_3})}{2} - \sum_{m=1}^{n_{f_1}} \text{sgn}(v_m^{f_1}) \frac{1 - \text{sgn}(\delta_m^{f_1})}{2} \quad (\text{S125.4})$$

$$\mathcal{W}_1^{\text{gapped}} = - \sum_{m=1}^{n_{e_1}} \text{sgn}(v_m^{e_1}) \frac{1 - \text{sgn}(\delta_m^{e_1})}{2} + \sum_{m=1}^{n_{e_3}} \text{sgn}(v_m^{e_3}) \frac{1 - \text{sgn}(\delta_m^{e_3})}{2} \quad (\text{S125.5})$$

$$\mathcal{W}_2^{\text{gapped}} = - \sum_{m=1}^{n_{h_1}} \text{sgn}(v_m^{h_1}) \frac{1 - \text{sgn}(\delta_m^{h_1})}{2} + \sum_{m=1}^{n_{h_3}} \text{sgn}(v_m^{h_3}) \frac{1 - \text{sgn}(\delta_m^{h_3})}{2} \quad (\text{S125.6})$$

$$\begin{aligned} \mathcal{W}_3^{\text{gapped}} = & - \sum_{m=1}^{n_{b_3}} \text{sgn}(v_m^{b_3}) \frac{1 - \text{sgn}(\delta_m^{b_3})}{2} + \sum_{m=1}^{n_{e_1}} \text{sgn}(v_m^{e_1}) \frac{1 - \text{sgn}(\delta_m^{e_1})}{2} - \sum_{m=1}^{n_{h_1}} \text{sgn}(v_m^{h_1}) \frac{1 - \text{sgn}(\delta_m^{h_1})}{2} \\ & + \sum_{m=1}^{n_{i_1}} \text{sgn}(v_m^{i_1}) \frac{1 - \text{sgn}(\delta_m^{i_1})}{2} \end{aligned} \quad (\text{S125.7})$$

$$\begin{aligned} \mathcal{W}_4^{\text{gapped}} = & - \sum_{m=1}^{n_{b_3}} \text{sgn}(v_m^{b_3}) \frac{1 - \text{sgn}(\delta_m^{b_3})}{2} + \sum_{m=1}^{n_{e_1}} \text{sgn}(v_m^{e_1}) \frac{1 - \text{sgn}(\delta_m^{e_1})}{2} - \sum_{m=1}^{n_{h_1}} \text{sgn}(v_m^{h_1}) \frac{1 - \text{sgn}(\delta_m^{h_1})}{2} \\ & + \sum_{m=1}^{n_{i_2}} \text{sgn}(v_m^{i_2}) \frac{1 - \text{sgn}(\delta_m^{i_2})}{2} \end{aligned} \quad (\text{S125.8})$$

### S126. SPACE GROUP NO. 126

| line segment                              | character of irrep (generators only)                                                                                                                                                                                                                                                                                                                                                                                                                                                                                                                  |
|-------------------------------------------|-------------------------------------------------------------------------------------------------------------------------------------------------------------------------------------------------------------------------------------------------------------------------------------------------------------------------------------------------------------------------------------------------------------------------------------------------------------------------------------------------------------------------------------------------------|
| $a \quad (0, \frac{t}{2}, 0)$             | $a_1 \quad \left\{ 2_{010} \middle  \begin{smallmatrix} \frac{1}{2} & 0 & \frac{1}{2} \\ 0 \end{smallmatrix} \right\} \quad \left\{ m_{100} \middle  \begin{smallmatrix} 0 & \frac{1}{2} & \frac{1}{2} \\ 0 \end{smallmatrix} \right\}$                                                                                                                                                                                                                                                                                                               |
| $b \quad (\frac{1-t}{2}, \frac{1}{2}, 0)$ | $\begin{aligned} & \left\{ 2_{100} \middle  \begin{smallmatrix} 0 & \frac{1}{2} & \frac{1}{2} \\ \frac{1}{2} & \frac{1}{2} & \frac{1}{2} \end{smallmatrix} \right\} \quad \left\{ m_{010} \middle  \begin{smallmatrix} \frac{1}{2} & 0 & \frac{1}{2} \\ \frac{1}{2} & \frac{1}{2} & \frac{1}{2} \end{smallmatrix} \right\} \\ & b_1 \quad i \quad -ie^{-\frac{1}{2}i\pi(1-t)} \\ & b_2 \quad i \quad ie^{-\frac{1}{2}i\pi(1-t)} \\ & b_3 \quad -i \quad -ie^{-\frac{1}{2}i\pi(1-t)} \\ & b_4 \quad -i \quad ie^{-\frac{1}{2}i\pi(1-t)} \end{aligned}$ |
| $c \quad (\frac{t}{2}, \frac{t}{2}, 0)$   | $c_1 \quad \left\{ 2_{110} \middle  \begin{smallmatrix} 0 & 0 & \frac{1}{2} \\ 0 & \frac{1}{2} & \frac{1}{2} \end{smallmatrix} \right\} \quad \left\{ m_{001} \middle  \begin{smallmatrix} \frac{1}{2} & \frac{1}{2} & 0 \\ 0 & 0 & 0 \end{smallmatrix} \right\}$                                                                                                                                                                                                                                                                                     |

|                                                     |                                                |                                                |                               |
|-----------------------------------------------------|------------------------------------------------|------------------------------------------------|-------------------------------|
| $d \quad (0, \frac{t}{2}, \frac{1}{2})$             | $\{2_{010}   \frac{1}{2} \ 0 \ \frac{1}{2} \}$ | $\{m_{100}   0 \ \frac{1}{2} \ \frac{1}{2} \}$ |                               |
|                                                     | $d_1$                                          | $i$                                            | $-ie^{-\frac{1}{2}i\pi(t+1)}$ |
|                                                     | $d_2$                                          | $i$                                            | $ie^{-\frac{1}{2}i\pi(t+1)}$  |
|                                                     | $d_3$                                          | $-i$                                           | $-ie^{-\frac{1}{2}i\pi(t+1)}$ |
|                                                     | $d_4$                                          | $-i$                                           | $ie^{-\frac{1}{2}i\pi(t+1)}$  |
| $e \quad (\frac{1-t}{2}, \frac{1}{2}, \frac{1}{2})$ | $\{2_{100}   0 \ \frac{1}{2} \ \frac{1}{2} \}$ | $\{m_{010}   \frac{1}{2} \ 0 \ \frac{1}{2} \}$ |                               |
|                                                     | $e_1$                                          | $0$                                            | $0$                           |
| $f \quad (\frac{t}{2}, \frac{t}{2}, \frac{1}{2})$   | $\{2_{110}   0 \ 0 \ \frac{1}{2} \}$           | $\{m_{001}   \frac{1}{2} \ \frac{1}{2} \ 0 \}$ |                               |
|                                                     | $f_1$                                          | $i$                                            | $-ie^{-i\pi t}$               |
|                                                     | $f_2$                                          | $i$                                            | $ie^{-i\pi t}$                |
|                                                     | $f_3$                                          | $-i$                                           | $-ie^{-i\pi t}$               |
|                                                     | $f_4$                                          | $-i$                                           | $ie^{-i\pi t}$                |
| $g \quad (0, 0, \frac{t}{2})$                       | $\{4_{001}   \frac{1}{2} \ 0 \ 0 \}$           | $\{m_{100}   0 \ \frac{1}{2} \ \frac{1}{2} \}$ |                               |
|                                                     | $g_1$                                          | $-\sqrt{2}$                                    | $0$                           |
|                                                     | $g_2$                                          | $\sqrt{2}$                                     | $0$                           |
| $h \quad (0, \frac{1}{2}, \frac{t}{2})$             | $\{2_{001}   \frac{1}{2} \ \frac{1}{2} \ 0 \}$ | $\{m_{100}   0 \ \frac{1}{2} \ \frac{1}{2} \}$ |                               |
|                                                     | $h_1$                                          | $i$                                            | $-ie^{-\frac{1}{2}i\pi(t+1)}$ |
|                                                     | $h_2$                                          | $i$                                            | $ie^{-\frac{1}{2}i\pi(t+1)}$  |
|                                                     | $h_3$                                          | $-i$                                           | $-ie^{-\frac{1}{2}i\pi(t+1)}$ |
|                                                     | $h_4$                                          | $-i$                                           | $ie^{-\frac{1}{2}i\pi(t+1)}$  |
| $i \quad (\frac{1}{2}, \frac{1}{2}, \frac{t}{2})$   | $\{4_{001}   \frac{1}{2} \ 0 \ 0 \}$           | $\{m_{100}   0 \ \frac{1}{2} \ \frac{1}{2} \}$ |                               |
|                                                     | $i_1$                                          | $i\sqrt{2}$                                    | $0$                           |
|                                                     | $i_2$                                          | $-i\sqrt{2}$                                   | $0$                           |

$$\begin{aligned}
\mathcal{W}_1^{\text{gapless}} = & \sum_{m=1}^{n_{a_1}} \text{sgn}(v_m^{a_1}) \frac{1 - \text{sgn}(\delta_m^{a_1})}{2} - \sum_{m=1}^{n_{e_1}} \text{sgn}(v_m^{e_1}) \frac{1 - \text{sgn}(\delta_m^{e_1})}{2} - \sum_{m=1}^{n_{f_1}} \text{sgn}(v_m^{f_1}) \frac{1 - \text{sgn}(\delta_m^{f_1})}{2} \\
& - \sum_{m=1}^{n_{f_3}} \text{sgn}(v_m^{f_3}) \frac{1 - \text{sgn}(\delta_m^{f_3})}{2} - \sum_{m=1}^{n_{g_1}} \text{sgn}(v_m^{g_1}) \frac{1 - \text{sgn}(\delta_m^{g_1})}{2} - \sum_{m=1}^{n_{g_2}} \text{sgn}(v_m^{g_2}) \frac{1 - \text{sgn}(\delta_m^{g_2})}{2} \\
& + \sum_{m=1}^{n_{h_1}} \text{sgn}(v_m^{h_1}) \frac{1 - \text{sgn}(\delta_m^{h_1})}{2} + \sum_{m=1}^{n_{h_3}} \text{sgn}(v_m^{h_3}) \frac{1 - \text{sgn}(\delta_m^{h_3})}{2}
\end{aligned} \tag{S126.1}$$

$$\begin{aligned}
\mathcal{W}_2^{\text{gapless}} = & \sum_{m=1}^{n_{b_1}} \text{sgn}(v_m^{b_1}) \frac{1 - \text{sgn}(\delta_m^{b_1})}{2} + \sum_{m=1}^{n_{b_3}} \text{sgn}(v_m^{b_3}) \frac{1 - \text{sgn}(\delta_m^{b_3})}{2} - \sum_{m=1}^{n_{e_1}} \text{sgn}(v_m^{e_1}) \frac{1 - \text{sgn}(\delta_m^{e_1})}{2} + \sum_{m=1}^{n_{h_1}} \text{sgn}(v_m^{h_1}) \frac{1 - \text{sgn}(\delta_m^{h_1})}{2} \\
& + \sum_{m=1}^{n_{h_3}} \text{sgn}(v_m^{h_3}) \frac{1 - \text{sgn}(\delta_m^{h_3})}{2} - \sum_{m=1}^{n_{i_1}} \text{sgn}(v_m^{i_1}) \frac{1 - \text{sgn}(\delta_m^{i_1})}{2} - \sum_{m=1}^{n_{i_2}} \text{sgn}(v_m^{i_2}) \frac{1 - \text{sgn}(\delta_m^{i_2})}{2}
\end{aligned} \tag{S126.2}$$

$$\begin{aligned}
\mathcal{W}_3^{\text{gapless}} = & \sum_{m=1}^{n_{c_1}} \text{sgn}(v_m^{c_1}) \frac{1 - \text{sgn}(\delta_m^{c_1})}{2} - \sum_{m=1}^{n_{f_1}} \text{sgn}(v_m^{f_1}) \frac{1 - \text{sgn}(\delta_m^{f_1})}{2} - \sum_{m=1}^{n_{f_3}} \text{sgn}(v_m^{f_3}) \frac{1 - \text{sgn}(\delta_m^{f_3})}{2} - \sum_{m=1}^{n_{g_1}} \text{sgn}(v_m^{g_1}) \frac{1 - \text{sgn}(\delta_m^{g_1})}{2} \\
& - \sum_{m=1}^{n_{g_2}} \text{sgn}(v_m^{g_2}) \frac{1 - \text{sgn}(\delta_m^{g_2})}{2} + \sum_{m=1}^{n_{i_1}} \text{sgn}(v_m^{i_1}) \frac{1 - \text{sgn}(\delta_m^{i_1})}{2} + \sum_{m=1}^{n_{i_2}} \text{sgn}(v_m^{i_2}) \frac{1 - \text{sgn}(\delta_m^{i_2})}{2}
\end{aligned} \tag{S126.3}$$

$$\begin{aligned} \mathcal{W}_4^{\text{gapless}} = & \sum_{m=1}^{n_{d_1}} \text{sgn}(v_m^{d_1}) \frac{1 - \text{sgn}(\delta_m^{d_1})}{2} + \sum_{m=1}^{n_{d_3}} \text{sgn}(v_m^{d_3}) \frac{1 - \text{sgn}(\delta_m^{d_3})}{2} - \sum_{m=1}^{n_{e_1}} \text{sgn}(v_m^{e_1}) \frac{1 - \text{sgn}(\delta_m^{e_1})}{2} \\ & - \sum_{m=1}^{n_{f_1}} \text{sgn}(v_m^{f_1}) \frac{1 - \text{sgn}(\delta_m^{f_1})}{2} - \sum_{m=1}^{n_{f_3}} \text{sgn}(v_m^{f_3}) \frac{1 - \text{sgn}(\delta_m^{f_3})}{2} \end{aligned} \quad (\text{S126.4})$$

$$\begin{aligned} \mathcal{W}_1^{\text{gapped}} = & - \sum_{m=1}^{n_{b_3}} \text{sgn}(v_m^{b_3}) \frac{1 - \text{sgn}(\delta_m^{b_3})}{2} + \sum_{m=1}^{n_{d_3}} \text{sgn}(v_m^{d_3}) \frac{1 - \text{sgn}(\delta_m^{d_3})}{2} - \sum_{m=1}^{n_{f_3}} \text{sgn}(v_m^{f_3}) \frac{1 - \text{sgn}(\delta_m^{f_3})}{2} \\ & - \sum_{m=1}^{n_{h_1}} \text{sgn}(v_m^{h_1}) \frac{1 - \text{sgn}(\delta_m^{h_1})}{2} + \sum_{m=1}^{n_{i_2}} \text{sgn}(v_m^{i_2}) \frac{1 - \text{sgn}(\delta_m^{i_2})}{2} \end{aligned} \quad (\text{S126.5})$$

$$\mathcal{W}_2^{\text{gapped}} = \sum_{m=1}^{n_{f_1}} \text{sgn}(v_m^{f_1}) \frac{1 - \text{sgn}(\delta_m^{f_1})}{2} - \sum_{m=1}^{n_{f_3}} \text{sgn}(v_m^{f_3}) \frac{1 - \text{sgn}(\delta_m^{f_3})}{2} \quad (\text{S126.6})$$

$$\mathcal{W}_3^{\text{gapped}} = - \sum_{m=1}^{n_{h_1}} \text{sgn}(v_m^{h_1}) \frac{1 - \text{sgn}(\delta_m^{h_1})}{2} + \sum_{m=1}^{n_{h_3}} \text{sgn}(v_m^{h_3}) \frac{1 - \text{sgn}(\delta_m^{h_3})}{2} \quad (\text{S126.7})$$

$$\begin{aligned} \mathcal{W}_4^{\text{gapped}} = & -2 \sum_{m=1}^{n_{b_3}} \text{sgn}(v_m^{b_3}) \frac{1 - \text{sgn}(\delta_m^{b_3})}{2} + \sum_{m=1}^{n_{e_1}} \text{sgn}(v_m^{e_1}) \frac{1 - \text{sgn}(\delta_m^{e_1})}{2} \\ & - 2 \sum_{m=1}^{n_{h_1}} \text{sgn}(v_m^{h_1}) \frac{1 - \text{sgn}(\delta_m^{h_1})}{2} + \sum_{m=1}^{n_{i_1}} \text{sgn}(v_m^{i_1}) \frac{1 - \text{sgn}(\delta_m^{i_1})}{2} + \sum_{m=1}^{n_{i_2}} \text{sgn}(v_m^{i_2}) \frac{1 - \text{sgn}(\delta_m^{i_2})}{2} \end{aligned} \quad (\text{S126.8})$$

$$\begin{aligned} \mathcal{W}_5^{\text{gapped}} = & -2 \sum_{m=1}^{n_{b_3}} \text{sgn}(v_m^{b_3}) \frac{1 - \text{sgn}(\delta_m^{b_3})}{2} + \sum_{m=1}^{n_{e_1}} \text{sgn}(v_m^{e_1}) \frac{1 - \text{sgn}(\delta_m^{e_1})}{2} - 2 \sum_{m=1}^{n_{h_1}} \text{sgn}(v_m^{h_1}) \frac{1 - \text{sgn}(\delta_m^{h_1})}{2} \\ & + 2 \sum_{m=1}^{n_{i_2}} \text{sgn}(v_m^{i_2}) \frac{1 - \text{sgn}(\delta_m^{i_2})}{2} \end{aligned} \quad (\text{S126.9})$$

### S127. SPACE GROUP NO. 127

| line segment                                        | character of irrep (generators only)                                                                                                                                                                                    |
|-----------------------------------------------------|-------------------------------------------------------------------------------------------------------------------------------------------------------------------------------------------------------------------------|
| $a \quad (0, \frac{t}{2}, 0)$                       | $a_1 \quad \left\{ 2_{010} \middle  \begin{smallmatrix} \frac{1}{2} & \frac{1}{2} & 0 \end{smallmatrix} \right\} \left\{ m_{100} \middle  \begin{smallmatrix} \frac{1}{2} & \frac{1}{2} & 0 \end{smallmatrix} \right\}$ |
| $b \quad (\frac{1-t}{2}, \frac{1}{2}, 0)$           | $b_1 \quad \left\{ 2_{100} \middle  \begin{smallmatrix} \frac{1}{2} & \frac{1}{2} & 0 \end{smallmatrix} \right\} \left\{ m_{010} \middle  \begin{smallmatrix} \frac{1}{2} & \frac{1}{2} & 0 \end{smallmatrix} \right\}$ |
| $c \quad (\frac{t}{2}, \frac{t}{2}, 0)$             | $c_1 \quad \left\{ 2_{110} \middle  \begin{smallmatrix} \frac{1}{2} & \frac{1}{2} & 0 \end{smallmatrix} \right\} \left\{ m_{001} \middle  \begin{smallmatrix} 0 & 0 & 0 \end{smallmatrix} \right\}$                     |
| $d \quad (0, \frac{t}{2}, \frac{1}{2})$             | $d_1 \quad \left\{ 2_{010} \middle  \begin{smallmatrix} \frac{1}{2} & \frac{1}{2} & 0 \end{smallmatrix} \right\} \left\{ m_{100} \middle  \begin{smallmatrix} \frac{1}{2} & \frac{1}{2} & 0 \end{smallmatrix} \right\}$ |
| $e \quad (\frac{1-t}{2}, \frac{1}{2}, \frac{1}{2})$ | $e_1 \quad \left\{ 2_{100} \middle  \begin{smallmatrix} \frac{1}{2} & \frac{1}{2} & 0 \end{smallmatrix} \right\} \left\{ m_{010} \middle  \begin{smallmatrix} \frac{1}{2} & \frac{1}{2} & 0 \end{smallmatrix} \right\}$ |

|                                                   |                                  |                                                          |                                                                         |
|---------------------------------------------------|----------------------------------|----------------------------------------------------------|-------------------------------------------------------------------------|
| $f \quad (\frac{t}{2}, \frac{t}{2}, \frac{1}{2})$ | $f_1$                            | $\{2_{110}   \frac{1}{2} \frac{1}{2} 0\}$                | $\{m_{001}   0 \ 0 \ 0\}$                                               |
| $g \quad (0, 0, \frac{t}{2})$                     | $g_1$<br>$g_2$                   | $\{4_{001}   0 \ 0 \ 0\}$<br>$-\sqrt{2}$<br>$\sqrt{2}$   | $\{m_{100}   \frac{1}{2} \frac{1}{2} 0\}$<br>$0$<br>$0$                 |
| $h \quad (0, \frac{1}{2}, \frac{t}{2})$           | $h_1$<br>$h_2$<br>$h_3$<br>$h_4$ | $\{2_{001}   0 \ 0 \ 0\}$<br>$-i$<br>$-i$<br>$i$<br>$i$  | $\{m_{100}   \frac{1}{2} \frac{1}{2} 0\}$<br>$-1$<br>$1$<br>$-1$<br>$1$ |
| $i \quad (\frac{1}{2}, \frac{1}{2}, \frac{t}{2})$ | $i_1$<br>$i_2$                   | $\{4_{001}   0 \ 0 \ 0\}$<br>$-i\sqrt{2}$<br>$i\sqrt{2}$ | $\{m_{100}   \frac{1}{2} \frac{1}{2} 0\}$<br>$0$<br>$0$                 |

$$\begin{aligned} \mathcal{W}_1^{\text{gapless}} = & \sum_{m=1}^{n_{a_1}} \text{sgn}(v_m^{a_1}) \frac{1 - \text{sgn}(\delta_m^{a_1})}{2} - 2 \sum_{m=1}^{n_{e_1}} \text{sgn}(v_m^{e_1}) \frac{1 - \text{sgn}(\delta_m^{e_1})}{2} - \sum_{m=1}^{n_{f_1}} \text{sgn}(v_m^{f_1}) \frac{1 - \text{sgn}(\delta_m^{f_1})}{2} \\ & - \sum_{m=1}^{n_{g_1}} \text{sgn}(v_m^{g_1}) \frac{1 - \text{sgn}(\delta_m^{g_1})}{2} - \sum_{m=1}^{n_{g_2}} \text{sgn}(v_m^{g_2}) \frac{1 - \text{sgn}(\delta_m^{g_2})}{2} + 2 \sum_{m=1}^{n_{h_2}} \text{sgn}(v_m^{h_2}) \frac{1 - \text{sgn}(\delta_m^{h_2})}{2} \end{aligned} \quad (\text{S127.1})$$

$$\mathcal{W}_2^{\text{gapless}} = \sum_{m=1}^{n_{b_1}} \text{sgn}(v_m^{b_1}) \frac{1 - \text{sgn}(\delta_m^{b_1})}{2} - \sum_{m=1}^{n_{e_1}} \text{sgn}(v_m^{e_1}) \frac{1 - \text{sgn}(\delta_m^{e_1})}{2} + \sum_{m=1}^{n_{h_2}} \text{sgn}(v_m^{h_2}) \frac{1 - \text{sgn}(\delta_m^{h_2})}{2} - \sum_{m=1}^{n_{i_1}} \text{sgn}(v_m^{i_1}) \frac{1 - \text{sgn}(\delta_m^{i_1})}{2} \quad (\text{S127.2})$$

$$\begin{aligned} \mathcal{W}_3^{\text{gapless}} = & \sum_{m=1}^{n_{c_1}} \text{sgn}(v_m^{c_1}) \frac{1 - \text{sgn}(\delta_m^{c_1})}{2} - \sum_{m=1}^{n_{f_1}} \text{sgn}(v_m^{f_1}) \frac{1 - \text{sgn}(\delta_m^{f_1})}{2} - \sum_{m=1}^{n_{g_1}} \text{sgn}(v_m^{g_1}) \frac{1 - \text{sgn}(\delta_m^{g_1})}{2} \\ & - \sum_{m=1}^{n_{g_2}} \text{sgn}(v_m^{g_2}) \frac{1 - \text{sgn}(\delta_m^{g_2})}{2} + 2 \sum_{m=1}^{n_{i_1}} \text{sgn}(v_m^{i_1}) \frac{1 - \text{sgn}(\delta_m^{i_1})}{2} \end{aligned} \quad (\text{S127.3})$$

$$\mathcal{W}_4^{\text{gapless}} = \sum_{m=1}^{n_{d_1}} \text{sgn}(v_m^{d_1}) \frac{1 - \text{sgn}(\delta_m^{d_1})}{2} - 2 \sum_{m=1}^{n_{e_1}} \text{sgn}(v_m^{e_1}) \frac{1 - \text{sgn}(\delta_m^{e_1})}{2} - \sum_{m=1}^{n_{f_1}} \text{sgn}(v_m^{f_1}) \frac{1 - \text{sgn}(\delta_m^{f_1})}{2} \quad (\text{S127.4})$$

$$\mathcal{W}_5^{\text{gapless}} = \sum_{m=1}^{n_{h_1}} \text{sgn}(v_m^{h_1}) \frac{1 - \text{sgn}(\delta_m^{h_1})}{2} - \sum_{m=1}^{n_{h_2}} \text{sgn}(v_m^{h_2}) \frac{1 - \text{sgn}(\delta_m^{h_2})}{2} \quad (\text{S127.5})$$

### S128. SPACE GROUP NO. 128

| line segment                              | character of irrep (generators only)                                                                                     |
|-------------------------------------------|--------------------------------------------------------------------------------------------------------------------------|
| $a \quad (0, \frac{t}{2}, 0)$             | $a_1$ $\{2_{010}   \frac{1}{2} \frac{1}{2} \frac{1}{2}\}$ $\{m_{100}   \frac{1}{2} \frac{1}{2} \frac{1}{2}\}$<br>$0$ $0$ |
| $b \quad (\frac{1-t}{2}, \frac{1}{2}, 0)$ | $b_1$ $\{2_{100}   \frac{1}{2} \frac{1}{2} \frac{1}{2}\}$ $\{m_{010}   \frac{1}{2} \frac{1}{2} \frac{1}{2}\}$<br>$0$ $0$ |
| $c \quad (\frac{t}{2}, \frac{t}{2}, 0)$   | $c_1$ $\{2_{110}   \frac{1}{2} \frac{1}{2} \frac{1}{2}\}$ $\{m_{001}   0 \ 0 \ 0\}$<br>$0$ $0$                           |

|                                                     |                                                        |                                                                                                                                                                                                           |                                                                                                                                                                                                           |
|-----------------------------------------------------|--------------------------------------------------------|-----------------------------------------------------------------------------------------------------------------------------------------------------------------------------------------------------------|-----------------------------------------------------------------------------------------------------------------------------------------------------------------------------------------------------------|
| $d \quad (0, \frac{t}{2}, \frac{1}{2})$             | $\begin{matrix} d_1 \\ d_2 \\ d_3 \\ d_4 \end{matrix}$ | $\begin{matrix} \{2_{010}   \frac{1}{2} \frac{1}{2} \frac{1}{2}\} \\ -e^{-\frac{1}{2}i\pi(t+1)} \\ -e^{-\frac{1}{2}i\pi(t+1)} \\ e^{-\frac{1}{2}i\pi(t+1)} \\ e^{-\frac{1}{2}i\pi(t+1)} \end{matrix}$     | $\begin{matrix} \{m_{100}   \frac{1}{2} \frac{1}{2} \frac{1}{2}\} \\ -ie^{-\frac{1}{2}i\pi(t+1)} \\ ie^{-\frac{1}{2}i\pi(t+1)} \\ -ie^{-\frac{1}{2}i\pi(t+1)} \\ ie^{-\frac{1}{2}i\pi(t+1)} \end{matrix}$ |
| $e \quad (\frac{1-t}{2}, \frac{1}{2}, \frac{1}{2})$ | $\begin{matrix} e_1 \\ e_2 \\ e_3 \\ e_4 \end{matrix}$ | $\begin{matrix} \{2_{100}   \frac{1}{2} \frac{1}{2} \frac{1}{2}\} \\ -ie^{-\frac{1}{2}i\pi(3-t)} \\ -ie^{-\frac{1}{2}i\pi(3-t)} \\ ie^{-\frac{1}{2}i\pi(3-t)} \\ ie^{-\frac{1}{2}i\pi(3-t)} \end{matrix}$ | $\begin{matrix} \{m_{010}   \frac{1}{2} \frac{1}{2} \frac{1}{2}\} \\ -e^{-\frac{1}{2}i\pi(3-t)} \\ e^{-\frac{1}{2}i\pi(3-t)} \\ -e^{-\frac{1}{2}i\pi(3-t)} \\ e^{-\frac{1}{2}i\pi(3-t)} \end{matrix}$     |
| $f \quad (\frac{t}{2}, \frac{t}{2}, \frac{1}{2})$   | $\begin{matrix} f_1 \\ f_2 \\ f_3 \\ f_4 \end{matrix}$ | $\begin{matrix} \{2_{110}   \frac{1}{2} \frac{1}{2} \frac{1}{2}\} \\ -e^{-\frac{1}{2}i\pi(2t+1)} \\ -e^{-\frac{1}{2}i\pi(2t+1)} \\ e^{-\frac{1}{2}i\pi(2t+1)} \\ e^{-\frac{1}{2}i\pi(2t+1)} \end{matrix}$ | $\begin{matrix} \{m_{001}   0 \ 0 \ 0\} \\ -i \\ i \\ -i \\ i \end{matrix}$                                                                                                                               |
| $g \quad (0, 0, \frac{t}{2})$                       | $\begin{matrix} g_1 \\ g_2 \end{matrix}$               | $\begin{matrix} \{4_{001}   0 \ 0 \ 0\} \\ -\sqrt{2} \\ \sqrt{2} \end{matrix}$                                                                                                                            | $\begin{matrix} \{m_{100}   \frac{1}{2} \frac{1}{2} \frac{1}{2}\} \\ 0 \\ 0 \end{matrix}$                                                                                                                 |
| $h \quad (0, \frac{1}{2}, \frac{t}{2})$             | $\begin{matrix} h_1 \\ h_2 \\ h_3 \\ h_4 \end{matrix}$ | $\begin{matrix} \{2_{001}   0 \ 0 \ 0\} \\ -i \\ -i \\ i \\ i \end{matrix}$                                                                                                                               | $\begin{matrix} \{m_{100}   \frac{1}{2} \frac{1}{2} \frac{1}{2}\} \\ -ie^{-\frac{1}{2}i\pi(t+1)} \\ ie^{-\frac{1}{2}i\pi(t+1)} \\ -ie^{-\frac{1}{2}i\pi(t+1)} \\ ie^{-\frac{1}{2}i\pi(t+1)} \end{matrix}$ |
| $i \quad (\frac{1}{2}, \frac{1}{2}, \frac{t}{2})$   | $\begin{matrix} i_1 \\ i_2 \end{matrix}$               | $\begin{matrix} \{4_{001}   0 \ 0 \ 0\} \\ -i\sqrt{2} \\ i\sqrt{2} \end{matrix}$                                                                                                                          | $\begin{matrix} \{m_{100}   \frac{1}{2} \frac{1}{2} \frac{1}{2}\} \\ 0 \\ 0 \end{matrix}$                                                                                                                 |

$$\begin{aligned}
\mathcal{W}_1^{\text{gapless}} = & \sum_{m=1}^{n_{a_1}} \text{sgn}(v_m^{a_1}) \frac{1 - \text{sgn}(\delta_m^{a_1})}{2} - 2 \sum_{m=1}^{n_{e_2}} \text{sgn}(v_m^{e_2}) \frac{1 - \text{sgn}(\delta_m^{e_2})}{2} - \sum_{m=1}^{n_{f_1}} \text{sgn}(v_m^{f_1}) \frac{1 - \text{sgn}(\delta_m^{f_1})}{2} \\
& - \sum_{m=1}^{n_{f_3}} \text{sgn}(v_m^{f_3}) \frac{1 - \text{sgn}(\delta_m^{f_3})}{2} - \sum_{m=1}^{n_{g_1}} \text{sgn}(v_m^{g_1}) \frac{1 - \text{sgn}(\delta_m^{g_1})}{2} - \sum_{m=1}^{n_{g_2}} \text{sgn}(v_m^{g_2}) \frac{1 - \text{sgn}(\delta_m^{g_2})}{2} \\
& + 2 \sum_{m=1}^{n_{h_1}} \text{sgn}(v_m^{h_1}) \frac{1 - \text{sgn}(\delta_m^{h_1})}{2}
\end{aligned} \tag{S128.1}$$

$$\mathcal{W}_2^{\text{gapless}} = \sum_{m=1}^{n_{b_1}} \text{sgn}(v_m^{b_1}) \frac{1 - \text{sgn}(\delta_m^{b_1})}{2} - \sum_{m=1}^{n_{e_2}} \text{sgn}(v_m^{e_2}) \frac{1 - \text{sgn}(\delta_m^{e_2})}{2} + \sum_{m=1}^{n_{h_1}} \text{sgn}(v_m^{h_1}) \frac{1 - \text{sgn}(\delta_m^{h_1})}{2} - \sum_{m=1}^{n_{i_1}} \text{sgn}(v_m^{i_1}) \frac{1 - \text{sgn}(\delta_m^{i_1})}{2} \tag{S128.2}$$

$$\begin{aligned}
\mathcal{W}_3^{\text{gapless}} = & \sum_{m=1}^{n_{c_1}} \text{sgn}(v_m^{c_1}) \frac{1 - \text{sgn}(\delta_m^{c_1})}{2} - \sum_{m=1}^{n_{f_1}} \text{sgn}(v_m^{f_1}) \frac{1 - \text{sgn}(\delta_m^{f_1})}{2} - \sum_{m=1}^{n_{f_3}} \text{sgn}(v_m^{f_3}) \frac{1 - \text{sgn}(\delta_m^{f_3})}{2} \\
& - \sum_{m=1}^{n_{g_1}} \text{sgn}(v_m^{g_1}) \frac{1 - \text{sgn}(\delta_m^{g_1})}{2} - \sum_{m=1}^{n_{g_2}} \text{sgn}(v_m^{g_2}) \frac{1 - \text{sgn}(\delta_m^{g_2})}{2} + 2 \sum_{m=1}^{n_{i_1}} \text{sgn}(v_m^{i_1}) \frac{1 - \text{sgn}(\delta_m^{i_1})}{2}
\end{aligned} \tag{S128.3}$$

$$\begin{aligned}
\mathcal{W}_4^{\text{gapless}} = & \sum_{m=1}^{n_{d_1}} \text{sgn}(v_m^{d_1}) \frac{1 - \text{sgn}(\delta_m^{d_1})}{2} + \sum_{m=1}^{n_{d_3}} \text{sgn}(v_m^{d_3}) \frac{1 - \text{sgn}(\delta_m^{d_3})}{2} - 2 \sum_{m=1}^{n_{e_2}} \text{sgn}(v_m^{e_2}) \frac{1 - \text{sgn}(\delta_m^{e_2})}{2} \\
& - \sum_{m=1}^{n_{f_1}} \text{sgn}(v_m^{f_1}) \frac{1 - \text{sgn}(\delta_m^{f_1})}{2} - \sum_{m=1}^{n_{f_3}} \text{sgn}(v_m^{f_3}) \frac{1 - \text{sgn}(\delta_m^{f_3})}{2} + \sum_{m=1}^{n_{h_1}} \text{sgn}(v_m^{h_1}) \frac{1 - \text{sgn}(\delta_m^{h_1})}{2} \\
& - \sum_{m=1}^{n_{h_2}} \text{sgn}(v_m^{h_2}) \frac{1 - \text{sgn}(\delta_m^{h_2})}{2}
\end{aligned} \tag{S128.4}$$

$$\mathcal{W}_5^{\text{gapless}} = \sum_{m=1}^{n_{e_1}} \text{sgn}(v_m^{e_1}) \frac{1 - \text{sgn}(\delta_m^{e_1})}{2} - \sum_{m=1}^{n_{e_2}} \text{sgn}(v_m^{e_2}) \frac{1 - \text{sgn}(\delta_m^{e_2})}{2} + \sum_{m=1}^{n_{h_1}} \text{sgn}(v_m^{h_1}) \frac{1 - \text{sgn}(\delta_m^{h_1})}{2} - \sum_{m=1}^{n_{h_2}} \text{sgn}(v_m^{h_2}) \frac{1 - \text{sgn}(\delta_m^{h_2})}{2} \tag{S128.5}$$

$$\mathcal{W}_1^{\text{gapped}} = - \sum_{m=1}^{n_{f_1}} \text{sgn}(v_m^{f_1}) \frac{1 - \text{sgn}(\delta_m^{f_1})}{2} + \sum_{m=1}^{n_{f_3}} \text{sgn}(v_m^{f_3}) \frac{1 - \text{sgn}(\delta_m^{f_3})}{2} \tag{S128.6}$$

### S129. SPACE GROUP NO. 129

| line segment                                        | character of irrep (generators only)                                                                                                                                                                                                                                                                         |
|-----------------------------------------------------|--------------------------------------------------------------------------------------------------------------------------------------------------------------------------------------------------------------------------------------------------------------------------------------------------------------|
| $a \quad (0, \frac{t}{2}, 0)$                       | $a_1 \quad \begin{array}{c} \{2_{010}   0 \ \frac{1}{2} \ 0\} \quad \{m_{100}   \frac{1}{2} \ 0 \ 0\} \\ 0 \end{array}$                                                                                                                                                                                      |
| $b \quad (\frac{1-t}{2}, \frac{1}{2}, 0)$           | $\begin{array}{c} \{2_{100}   \frac{1}{2} \ 0 \ 0\} \quad \{m_{010}   0 \ \frac{1}{2} \ 0\} \\ b_1 \quad -ie^{-\frac{1}{2}i\pi(1-t)} \quad i \\ b_2 \quad -ie^{-\frac{1}{2}i\pi(1-t)} \quad -i \\ b_3 \quad ie^{-\frac{1}{2}i\pi(1-t)} \quad i \\ b_4 \quad ie^{-\frac{1}{2}i\pi(1-t)} \quad -i \end{array}$ |
| $c \quad (\frac{t}{2}, \frac{t}{2}, 0)$             | $c_1 \quad \begin{array}{c} \{2_{110}   \frac{1}{2} \ \frac{1}{2} \ 0\} \quad \{m_{001}   \frac{1}{2} \ \frac{1}{2} \ 0\} \\ 0 \end{array}$                                                                                                                                                                  |
| $d \quad (0, \frac{t}{2}, \frac{1}{2})$             | $d_1 \quad \begin{array}{c} \{2_{010}   0 \ \frac{1}{2} \ 0\} \quad \{m_{100}   \frac{1}{2} \ 0 \ 0\} \\ 0 \end{array}$                                                                                                                                                                                      |
| $e \quad (\frac{1-t}{2}, \frac{1}{2}, \frac{1}{2})$ | $\begin{array}{c} \{2_{100}   \frac{1}{2} \ 0 \ 0\} \quad \{m_{010}   0 \ \frac{1}{2} \ 0\} \\ e_1 \quad -ie^{-\frac{1}{2}i\pi(1-t)} \quad i \\ e_2 \quad -ie^{-\frac{1}{2}i\pi(1-t)} \quad -i \\ e_3 \quad ie^{-\frac{1}{2}i\pi(1-t)} \quad i \\ e_4 \quad ie^{-\frac{1}{2}i\pi(1-t)} \quad -i \end{array}$ |
| $f \quad (\frac{t}{2}, \frac{t}{2}, \frac{1}{2})$   | $f_1 \quad \begin{array}{c} \{2_{110}   \frac{1}{2} \ \frac{1}{2} \ 0\} \quad \{m_{001}   \frac{1}{2} \ \frac{1}{2} \ 0\} \\ 0 \end{array}$                                                                                                                                                                  |
| $g \quad (0, 0, \frac{t}{2})$                       | $\begin{array}{c} \{4_{001}   \frac{1}{2} \ 0 \ 0\} \quad \{m_{100}   \frac{1}{2} \ 0 \ 0\} \\ g_1 \quad -\sqrt{2} \quad 0 \\ g_2 \quad \sqrt{2} \quad 0 \end{array}$                                                                                                                                        |
| $h \quad (0, \frac{1}{2}, \frac{t}{2})$             | $h_1 \quad \begin{array}{c} \{2_{001}   \frac{1}{2} \ \frac{1}{2} \ 0\} \quad \{m_{100}   \frac{1}{2} \ 0 \ 0\} \\ 0 \end{array}$                                                                                                                                                                            |
| $i \quad (\frac{1}{2}, \frac{1}{2}, \frac{t}{2})$   | $\begin{array}{c} \{4_{001}   \frac{1}{2} \ 0 \ 0\} \quad \{m_{100}   \frac{1}{2} \ 0 \ 0\} \\ i_1 \quad -\sqrt{2} \quad 0 \\ i_2 \quad \sqrt{2} \quad 0 \end{array}$                                                                                                                                        |

$$\begin{aligned} \mathcal{W}_1^{\text{gapless}} = & \sum_{m=1}^{n_{a_1}} \text{sgn}(v_m^{a_1}) \frac{1 - \text{sgn}(\delta_m^{a_1})}{2} - \sum_{m=1}^{n_{e_1}} \text{sgn}(v_m^{e_1}) \frac{1 - \text{sgn}(\delta_m^{e_1})}{2} - \sum_{m=1}^{n_{e_2}} \text{sgn}(v_m^{e_2}) \frac{1 - \text{sgn}(\delta_m^{e_2})}{2} - \sum_{m=1}^{n_{f_1}} \text{sgn}(v_m^{f_1}) \frac{1 - \text{sgn}(\delta_m^{f_1})}{2} \\ & - \sum_{m=1}^{n_{g_1}} \text{sgn}(v_m^{g_1}) \frac{1 - \text{sgn}(\delta_m^{g_1})}{2} - \sum_{m=1}^{n_{g_2}} \text{sgn}(v_m^{g_2}) \frac{1 - \text{sgn}(\delta_m^{g_2})}{2} + 2 \sum_{m=1}^{n_{h_1}} \text{sgn}(v_m^{h_1}) \frac{1 - \text{sgn}(\delta_m^{h_1})}{2} \end{aligned} \quad (\text{S129.1})$$

$$\mathcal{W}_2^{\text{gapless}} = \sum_{m=1}^{n_{b_1}} \text{sgn}(v_m^{b_1}) \frac{1 - \text{sgn}(\delta_m^{b_1})}{2} - \sum_{m=1}^{n_{e_1}} \text{sgn}(v_m^{e_1}) \frac{1 - \text{sgn}(\delta_m^{e_1})}{2} + \sum_{m=1}^{n_{h_1}} \text{sgn}(v_m^{h_1}) \frac{1 - \text{sgn}(\delta_m^{h_1})}{2} - \sum_{m=1}^{n_{i_1}} \text{sgn}(v_m^{i_1}) \frac{1 - \text{sgn}(\delta_m^{i_1})}{2} \quad (\text{S129.2})$$

$$\mathcal{W}_3^{\text{gapless}} = \sum_{m=1}^{n_{b_2}} \text{sgn}(v_m^{b_2}) \frac{1 - \text{sgn}(\delta_m^{b_2})}{2} - \sum_{m=1}^{n_{e_2}} \text{sgn}(v_m^{e_2}) \frac{1 - \text{sgn}(\delta_m^{e_2})}{2} + \sum_{m=1}^{n_{h_1}} \text{sgn}(v_m^{h_1}) \frac{1 - \text{sgn}(\delta_m^{h_1})}{2} - \sum_{m=1}^{n_{i_1}} \text{sgn}(v_m^{i_1}) \frac{1 - \text{sgn}(\delta_m^{i_1})}{2} \quad (\text{S129.3})$$

$$\begin{aligned} \mathcal{W}_4^{\text{gapless}} = & \sum_{m=1}^{n_{c_1}} \text{sgn}(v_m^{c_1}) \frac{1 - \text{sgn}(\delta_m^{c_1})}{2} - \sum_{m=1}^{n_{f_1}} \text{sgn}(v_m^{f_1}) \frac{1 - \text{sgn}(\delta_m^{f_1})}{2} - \sum_{m=1}^{n_{g_1}} \text{sgn}(v_m^{g_1}) \frac{1 - \text{sgn}(\delta_m^{g_1})}{2} \\ & - \sum_{m=1}^{n_{g_2}} \text{sgn}(v_m^{g_2}) \frac{1 - \text{sgn}(\delta_m^{g_2})}{2} + 2 \sum_{m=1}^{n_{i_1}} \text{sgn}(v_m^{i_1}) \frac{1 - \text{sgn}(\delta_m^{i_1})}{2} \end{aligned} \quad (\text{S129.4})$$

$$\mathcal{W}_5^{\text{gapless}} = \sum_{m=1}^{n_{d_1}} \text{sgn}(v_m^{d_1}) \frac{1 - \text{sgn}(\delta_m^{d_1})}{2} - \sum_{m=1}^{n_{e_1}} \text{sgn}(v_m^{e_1}) \frac{1 - \text{sgn}(\delta_m^{e_1})}{2} - \sum_{m=1}^{n_{e_2}} \text{sgn}(v_m^{e_2}) \frac{1 - \text{sgn}(\delta_m^{e_2})}{2} - \sum_{m=1}^{n_{f_1}} \text{sgn}(v_m^{f_1}) \frac{1 - \text{sgn}(\delta_m^{f_1})}{2} \quad (\text{S129.5})$$

$$\mathcal{W}_1^{\text{gapped}} = \sum_{m=1}^{n_{e_1}} \text{sgn}(v_m^{e_1}) \frac{1 - \text{sgn}(\delta_m^{e_1})}{2} - \sum_{m=1}^{n_{e_2}} \text{sgn}(v_m^{e_2}) \frac{1 - \text{sgn}(\delta_m^{e_2})}{2} \quad (\text{S129.6})$$

### S130. SPACE GROUP NO. 130

| line segment                              | character of irrep (generators only)                                                                                                                                                                                                                                                                                     |
|-------------------------------------------|--------------------------------------------------------------------------------------------------------------------------------------------------------------------------------------------------------------------------------------------------------------------------------------------------------------------------|
| $a \quad (0, \frac{t}{2}, 0)$             | $\begin{array}{c} \{2_{010}   0 \frac{1}{2} \frac{1}{2}\} \quad \{m_{100}   \frac{1}{2} 0 \frac{1}{2}\} \\ a_1 \quad 0 \end{array}$                                                                                                                                                                                      |
| $b \quad (\frac{1-t}{2}, \frac{1}{2}, 0)$ | $\begin{array}{c} \{2_{100}   \frac{1}{2} 0 \frac{1}{2}\} \quad \{m_{010}   0 \frac{1}{2} \frac{1}{2}\} \\ b_1 \quad -ie^{-\frac{1}{2}i\pi(1-t)} \quad i \\ b_2 \quad -ie^{-\frac{1}{2}i\pi(1-t)} \quad -i \\ b_3 \quad ie^{-\frac{1}{2}i\pi(1-t)} \quad i \\ b_4 \quad ie^{-\frac{1}{2}i\pi(1-t)} \quad -i \end{array}$ |
| $c \quad (\frac{t}{2}, \frac{t}{2}, 0)$   | $\begin{array}{c} \{2_{110}   \frac{1}{2} \frac{1}{2} \frac{1}{2}\} \quad \{m_{001}   \frac{1}{2} \frac{1}{2} 0\} \\ c_1 \quad 0 \end{array}$                                                                                                                                                                            |



|                                                     |                                                                                                                                                                                                                                                                                                                                           |
|-----------------------------------------------------|-------------------------------------------------------------------------------------------------------------------------------------------------------------------------------------------------------------------------------------------------------------------------------------------------------------------------------------------|
| $d \quad (0, \frac{t}{2}, \frac{1}{2})$             | $\begin{matrix} \{2_{010}   \frac{1}{2} \frac{1}{2} \frac{1}{2}\} & \{m_{100}   \frac{1}{2} 0 \frac{1}{2}\} \\ d_1 & -e^{-\frac{1}{2}i\pi(t+1)} & -1 \\ d_2 & -e^{-\frac{1}{2}i\pi(t+1)} & 1 \\ d_3 & e^{-\frac{1}{2}i\pi(t+1)} & -1 \\ d_4 & e^{-\frac{1}{2}i\pi(t+1)} & 1 \end{matrix}$                                                 |
| $e \quad (\frac{1-t}{2}, \frac{1}{2}, \frac{1}{2})$ | $\begin{matrix} \{2_{100}   \frac{1}{2} 0 \frac{1}{2}\} & \{m_{010}   0 \frac{1}{2} \frac{1}{2}\} \\ e_1 & 0 & 0 \end{matrix}$                                                                                                                                                                                                            |
| $f \quad (\frac{t}{2}, \frac{t}{2}, \frac{1}{2})$   | $\begin{matrix} \{2_{110}   \frac{1}{2} \frac{1}{2} \frac{1}{2}\} & \{m_{001}   \frac{1}{2} \frac{1}{2} 0\} \\ f_1 & -e^{-\frac{1}{2}i\pi(2t+1)} & -ie^{-i\pi t} \\ f_2 & -e^{-\frac{1}{2}i\pi(2t+1)} & ie^{-i\pi t} \\ f_3 & e^{-\frac{1}{2}i\pi(2t+1)} & -ie^{-i\pi t} \\ f_4 & e^{-\frac{1}{2}i\pi(2t+1)} & ie^{-i\pi t} \end{matrix}$ |
| $g \quad (0, 0, \frac{t}{2})$                       | $\begin{matrix} \{4_{001}   \frac{1}{2} 0 0\} & \{m_{100}   \frac{1}{2} 0 \frac{1}{2}\} \\ g_1 & -\sqrt{2} & 0 \\ g_2 & \sqrt{2} & 0 \end{matrix}$                                                                                                                                                                                        |
| $h \quad (0, \frac{1}{2}, \frac{t}{2})$             | $\begin{matrix} \{2_{001}   \frac{1}{2} \frac{1}{2} 0\} & \{m_{100}   \frac{1}{2} 0 \frac{1}{2}\} \\ h_1 & 0 & 0 \end{matrix}$                                                                                                                                                                                                            |
| $i \quad (\frac{1}{2}, \frac{1}{2}, \frac{t}{2})$   | $\begin{matrix} \{4_{001}   \frac{1}{2} 0 0\} & \{m_{100}   \frac{1}{2} 0 \frac{1}{2}\} \\ i_1 & -\sqrt{2} & 0 \\ i_2 & \sqrt{2} & 0 \end{matrix}$                                                                                                                                                                                        |

$$\begin{aligned} \mathcal{W}_1^{\text{gapless}} = & \sum_{m=1}^{n_{a_1}} \text{sgn}(v_m^{a_1}) \frac{1 - \text{sgn}(\delta_m^{a_1})}{2} - 2 \sum_{m=1}^{n_{e_1}} \text{sgn}(v_m^{e_1}) \frac{1 - \text{sgn}(\delta_m^{e_1})}{2} - \sum_{m=1}^{n_{f_1}} \text{sgn}(v_m^{f_1}) \frac{1 - \text{sgn}(\delta_m^{f_1})}{2} \\ & - \sum_{m=1}^{n_{f_3}} \text{sgn}(v_m^{f_3}) \frac{1 - \text{sgn}(\delta_m^{f_3})}{2} - \sum_{m=1}^{n_{g_1}} \text{sgn}(v_m^{g_1}) \frac{1 - \text{sgn}(\delta_m^{g_1})}{2} - \sum_{m=1}^{n_{g_2}} \text{sgn}(v_m^{g_2}) \frac{1 - \text{sgn}(\delta_m^{g_2})}{2} \\ & + 2 \sum_{m=1}^{n_{h_1}} \text{sgn}(v_m^{h_1}) \frac{1 - \text{sgn}(\delta_m^{h_1})}{2} \end{aligned} \quad (\text{S130.1})$$

$$\mathcal{W}_2^{\text{gapless}} = \sum_{m=1}^{n_{b_1}} \text{sgn}(v_m^{b_1}) \frac{1 - \text{sgn}(\delta_m^{b_1})}{2} - \sum_{m=1}^{n_{e_1}} \text{sgn}(v_m^{e_1}) \frac{1 - \text{sgn}(\delta_m^{e_1})}{2} + \sum_{m=1}^{n_{h_1}} \text{sgn}(v_m^{h_1}) \frac{1 - \text{sgn}(\delta_m^{h_1})}{2} - \sum_{m=1}^{n_{i_1}} \text{sgn}(v_m^{i_1}) \frac{1 - \text{sgn}(\delta_m^{i_1})}{2} \quad (\text{S130.2})$$

$$\mathcal{W}_3^{\text{gapless}} = \sum_{m=1}^{n_{b_2}} \text{sgn}(v_m^{b_2}) \frac{1 - \text{sgn}(\delta_m^{b_2})}{2} - \sum_{m=1}^{n_{e_1}} \text{sgn}(v_m^{e_1}) \frac{1 - \text{sgn}(\delta_m^{e_1})}{2} + \sum_{m=1}^{n_{h_1}} \text{sgn}(v_m^{h_1}) \frac{1 - \text{sgn}(\delta_m^{h_1})}{2} - \sum_{m=1}^{n_{i_1}} \text{sgn}(v_m^{i_1}) \frac{1 - \text{sgn}(\delta_m^{i_1})}{2} \quad (\text{S130.3})$$

$$\begin{aligned} \mathcal{W}_4^{\text{gapless}} = & \sum_{m=1}^{n_{c_1}} \text{sgn}(v_m^{c_1}) \frac{1 - \text{sgn}(\delta_m^{c_1})}{2} - \sum_{m=1}^{n_{f_1}} \text{sgn}(v_m^{f_1}) \frac{1 - \text{sgn}(\delta_m^{f_1})}{2} - \sum_{m=1}^{n_{f_3}} \text{sgn}(v_m^{f_3}) \frac{1 - \text{sgn}(\delta_m^{f_3})}{2} \\ & - \sum_{m=1}^{n_{g_1}} \text{sgn}(v_m^{g_1}) \frac{1 - \text{sgn}(\delta_m^{g_1})}{2} - \sum_{m=1}^{n_{g_2}} \text{sgn}(v_m^{g_2}) \frac{1 - \text{sgn}(\delta_m^{g_2})}{2} + 2 \sum_{m=1}^{n_{i_1}} \text{sgn}(v_m^{i_1}) \frac{1 - \text{sgn}(\delta_m^{i_1})}{2} \end{aligned} \quad (\text{S130.4})$$

$$\begin{aligned} \mathcal{W}_5^{\text{gapless}} = & \sum_{m=1}^{n_{d_1}} \text{sgn}(v_m^{d_1}) \frac{1 - \text{sgn}(\delta_m^{d_1})}{2} + \sum_{m=1}^{n_{d_3}} \text{sgn}(v_m^{d_3}) \frac{1 - \text{sgn}(\delta_m^{d_3})}{2} - 2 \sum_{m=1}^{n_{e_1}} \text{sgn}(v_m^{e_1}) \frac{1 - \text{sgn}(\delta_m^{e_1})}{2} \\ & - \sum_{m=1}^{n_{f_1}} \text{sgn}(v_m^{f_1}) \frac{1 - \text{sgn}(\delta_m^{f_1})}{2} - \sum_{m=1}^{n_{f_3}} \text{sgn}(v_m^{f_3}) \frac{1 - \text{sgn}(\delta_m^{f_3})}{2} \end{aligned} \quad (\text{S130.5})$$

$$\mathcal{W}_1^{\text{gapped}} = - \sum_{m=1}^{n_{f_1}} \text{sgn}(v_m^{f_1}) \frac{1 - \text{sgn}(\delta_m^{f_1})}{2} + \sum_{m=1}^{n_{f_3}} \text{sgn}(v_m^{f_3}) \frac{1 - \text{sgn}(\delta_m^{f_3})}{2} \quad (\text{S130.6})$$

$$\mathcal{X}_1 = \sum_{m=1}^{n_{d_3}} \frac{1 - \text{sgn}(\delta_m^{d_3})}{2} + \sum_{m=1}^{n_{f_1}} \frac{1 - \text{sgn}(\delta_m^{f_1})}{2} \mod 2 \quad (\text{S130.7})$$

### S131. SPACE GROUP NO. 131

| line segment                                        | character of irrep (generators only)                                                                                                                                                                         |
|-----------------------------------------------------|--------------------------------------------------------------------------------------------------------------------------------------------------------------------------------------------------------------|
| $a \quad (0, \frac{t}{2}, 0)$                       | $a_1 \quad \begin{Bmatrix} \{2_{010}  0 & 0 & 0 \} \\ 0 \end{Bmatrix} \quad \begin{Bmatrix} \{m_{100}  0 & 0 & 0 \} \\ 0 \end{Bmatrix}$                                                                      |
| $b \quad (\frac{1-t}{2}, \frac{1}{2}, 0)$           | $b_1 \quad \begin{Bmatrix} \{2_{100}  0 & 0 & 0 \} \\ 0 \end{Bmatrix} \quad \begin{Bmatrix} \{m_{010}  0 & 0 & 0 \} \\ 0 \end{Bmatrix}$                                                                      |
| $c \quad (\frac{t}{2}, \frac{t}{2}, 0)$             | $c_1 \quad \begin{Bmatrix} \{2_{110}  0 & 0 & \frac{1}{2} \} \\ 0 \end{Bmatrix} \quad \begin{Bmatrix} \{m_{001}  0 & 0 & 0 \} \\ 0 \end{Bmatrix}$                                                            |
| $d \quad (0, \frac{t}{2}, \frac{1}{2})$             | $d_1 \quad \begin{Bmatrix} \{2_{010}  0 & 0 & 0 \} \\ 0 \end{Bmatrix} \quad \begin{Bmatrix} \{m_{100}  0 & 0 & 0 \} \\ 0 \end{Bmatrix}$                                                                      |
| $e \quad (\frac{1-t}{2}, \frac{1}{2}, \frac{1}{2})$ | $e_1 \quad \begin{Bmatrix} \{2_{100}  0 & 0 & 0 \} \\ 0 \end{Bmatrix} \quad \begin{Bmatrix} \{m_{010}  0 & 0 & 0 \} \\ 0 \end{Bmatrix}$                                                                      |
| $f \quad (\frac{t}{2}, \frac{t}{2}, \frac{1}{2})$   | $\begin{matrix} f_1 & i & -i \\ f_2 & i & i \\ f_3 & -i & -i \\ f_4 & -i & i \end{matrix} \quad \begin{Bmatrix} \{2_{110}  0 & 0 & \frac{1}{2} \} \\ \{m_{001}  0 & 0 & 0 \} \end{Bmatrix}$                  |
| $g \quad (0, 0, \frac{t}{2})$                       | $\begin{matrix} g_1 & -\sqrt{2}e^{-\frac{1}{2}i\pi t} \\ g_2 & \sqrt{2}e^{-\frac{1}{2}i\pi t} \end{matrix} \quad \begin{Bmatrix} \{4_{001}  0 & 0 & \frac{1}{2} \} \\ \{m_{100}  0 & 0 & 0 \} \end{Bmatrix}$ |
| $h \quad (0, \frac{1}{2}, \frac{t}{2})$             | $h_1 \quad \begin{Bmatrix} \{2_{001}  0 & 0 & 0 \} \\ 0 \end{Bmatrix} \quad \begin{Bmatrix} \{m_{100}  0 & 0 & 0 \} \\ 0 \end{Bmatrix}$                                                                      |
| $i \quad (\frac{1}{2}, \frac{1}{2}, \frac{t}{2})$   | $\begin{matrix} i_1 & -\sqrt{2}e^{-\frac{1}{2}i\pi t} \\ i_2 & \sqrt{2}e^{-\frac{1}{2}i\pi t} \end{matrix} \quad \begin{Bmatrix} \{4_{001}  0 & 0 & \frac{1}{2} \} \\ \{m_{100}  0 & 0 & 0 \} \end{Bmatrix}$ |

$$\begin{aligned} \mathcal{W}_1^{\text{gapless}} = & \sum_{m=1}^{n_{a_1}} \text{sgn}(v_m^{a_1}) \frac{1 - \text{sgn}(\delta_m^{a_1})}{2} - \sum_{m=1}^{n_{e_1}} \text{sgn}(v_m^{e_1}) \frac{1 - \text{sgn}(\delta_m^{e_1})}{2} - \sum_{m=1}^{n_{f_1}} \text{sgn}(v_m^{f_1}) \frac{1 - \text{sgn}(\delta_m^{f_1})}{2} - \sum_{m=1}^{n_{f_3}} \text{sgn}(v_m^{f_3}) \frac{1 - \text{sgn}(\delta_m^{f_3})}{2} \\ & - \sum_{m=1}^{n_{g_1}} \text{sgn}(v_m^{g_1}) \frac{1 - \text{sgn}(\delta_m^{g_1})}{2} - \sum_{m=1}^{n_{g_2}} \text{sgn}(v_m^{g_2}) \frac{1 - \text{sgn}(\delta_m^{g_2})}{2} + \sum_{m=1}^{n_{h_1}} \text{sgn}(v_m^{h_1}) \frac{1 - \text{sgn}(\delta_m^{h_1})}{2} \end{aligned} \quad (\text{S131.1})$$

$$\begin{aligned} \mathcal{W}_2^{\text{gapless}} = & \sum_{m=1}^{n_{b_1}} \text{sgn}(v_m^{b_1}) \frac{1 - \text{sgn}(\delta_m^{b_1})}{2} - \sum_{m=1}^{n_{e_1}} \text{sgn}(v_m^{e_1}) \frac{1 - \text{sgn}(\delta_m^{e_1})}{2} + \sum_{m=1}^{n_{h_1}} \text{sgn}(v_m^{h_1}) \frac{1 - \text{sgn}(\delta_m^{h_1})}{2} \\ & - \sum_{m=1}^{n_{i_1}} \text{sgn}(v_m^{i_1}) \frac{1 - \text{sgn}(\delta_m^{i_1})}{2} - \sum_{m=1}^{n_{i_2}} \text{sgn}(v_m^{i_2}) \frac{1 - \text{sgn}(\delta_m^{i_2})}{2} \end{aligned} \quad (\text{S131.2})$$

$$\begin{aligned} \mathcal{W}_3^{\text{gapless}} = & \sum_{m=1}^{n_{c_1}} \text{sgn}(v_m^{c_1}) \frac{1 - \text{sgn}(\delta_m^{c_1})}{2} - \sum_{m=1}^{n_{f_1}} \text{sgn}(v_m^{f_1}) \frac{1 - \text{sgn}(\delta_m^{f_1})}{2} - \sum_{m=1}^{n_{f_3}} \text{sgn}(v_m^{f_3}) \frac{1 - \text{sgn}(\delta_m^{f_3})}{2} - \sum_{m=1}^{n_{g_1}} \text{sgn}(v_m^{g_1}) \frac{1 - \text{sgn}(\delta_m^{g_1})}{2} \\ & - \sum_{m=1}^{n_{g_2}} \text{sgn}(v_m^{g_2}) \frac{1 - \text{sgn}(\delta_m^{g_2})}{2} + \sum_{m=1}^{n_{i_1}} \text{sgn}(v_m^{i_1}) \frac{1 - \text{sgn}(\delta_m^{i_1})}{2} + \sum_{m=1}^{n_{i_2}} \text{sgn}(v_m^{i_2}) \frac{1 - \text{sgn}(\delta_m^{i_2})}{2} \end{aligned} \quad (\text{S131.3})$$

$$\mathcal{W}_4^{\text{gapless}} = \sum_{m=1}^{n_{d_1}} \text{sgn}(v_m^{d_1}) \frac{1 - \text{sgn}(\delta_m^{d_1})}{2} - \sum_{m=1}^{n_{e_1}} \text{sgn}(v_m^{e_1}) \frac{1 - \text{sgn}(\delta_m^{e_1})}{2} - \sum_{m=1}^{n_{f_1}} \text{sgn}(v_m^{f_1}) \frac{1 - \text{sgn}(\delta_m^{f_1})}{2} - \sum_{m=1}^{n_{f_3}} \text{sgn}(v_m^{f_3}) \frac{1 - \text{sgn}(\delta_m^{f_3})}{2} \quad (\text{S131.4})$$

$$\mathcal{W}_1^{\text{gapped}} = \sum_{m=1}^{n_{f_1}} \text{sgn}(v_m^{f_1}) \frac{1 - \text{sgn}(\delta_m^{f_1})}{2} - \sum_{m=1}^{n_{f_3}} \text{sgn}(v_m^{f_3}) \frac{1 - \text{sgn}(\delta_m^{f_3})}{2} \quad (\text{S131.5})$$

### S132. SPACE GROUP NO. 132

| line segment                                        | character of irrep (generators only)                                                                                                                                                           |
|-----------------------------------------------------|------------------------------------------------------------------------------------------------------------------------------------------------------------------------------------------------|
| $a \quad (0, \frac{t}{2}, 0)$                       | $a_1 \quad \begin{array}{cc} \{2_{010}   0 & 0 & \frac{1}{2}\} & \{m_{100}   0 & 0 & \frac{1}{2}\} \\ 0 & 0 \end{array}$                                                                       |
| $b \quad (\frac{1-t}{2}, \frac{1}{2}, 0)$           | $b_1 \quad \begin{array}{cc} \{2_{100}   0 & 0 & \frac{1}{2}\} & \{m_{010}   0 & 0 & \frac{1}{2}\} \\ 0 & 0 \end{array}$                                                                       |
| $c \quad (\frac{t}{2}, \frac{t}{2}, 0)$             | $c_1 \quad \begin{array}{cc} \{2_{110}   0 & 0 & 0\} & \{m_{001}   0 & 0 & 0\} \\ 0 & 0 \end{array}$                                                                                           |
| $d \quad (0, \frac{t}{2}, \frac{1}{2})$             | $\begin{array}{cc} \{2_{010}   0 & 0 & \frac{1}{2}\} & \{m_{100}   0 & 0 & \frac{1}{2}\} \\ d_1 & i & -1 \\ d_2 & i & 1 \\ d_3 & -i & -1 \\ d_4 & -i & 1 \end{array}$                          |
| $e \quad (\frac{1-t}{2}, \frac{1}{2}, \frac{1}{2})$ | $\begin{array}{cc} \{2_{100}   0 & 0 & \frac{1}{2}\} & \{m_{010}   0 & 0 & \frac{1}{2}\} \\ e_1 & i & -1 \\ e_2 & i & 1 \\ e_3 & -i & -1 \\ e_4 & -i & 1 \end{array}$                          |
| $f \quad (\frac{t}{2}, \frac{t}{2}, \frac{1}{2})$   | $f_1 \quad \begin{array}{cc} \{2_{110}   0 & 0 & 0\} & \{m_{001}   0 & 0 & 0\} \\ 0 & 0 \end{array}$                                                                                           |
| $g \quad (0, 0, \frac{t}{2})$                       | $\begin{array}{cc} \{4_{001}   0 & 0 & \frac{1}{2}\} & \{m_{100}   0 & 0 & \frac{1}{2}\} \\ g_1 & -\sqrt{2}e^{-\frac{1}{2}i\pi t} & 0 \\ g_2 & \sqrt{2}e^{-\frac{1}{2}i\pi t} & 0 \end{array}$ |
| $h \quad (0, \frac{1}{2}, \frac{t}{2})$             | $h_1 \quad \begin{array}{cc} \{2_{001}   0 & 0 & 0\} & \{m_{100}   0 & 0 & \frac{1}{2}\} \\ 0 & 0 \end{array}$                                                                                 |
| $i \quad (\frac{1}{2}, \frac{1}{2}, \frac{t}{2})$   | $\begin{array}{cc} \{4_{001}   0 & 0 & \frac{1}{2}\} & \{m_{100}   0 & 0 & \frac{1}{2}\} \\ i_1 & -\sqrt{2}e^{-\frac{1}{2}i\pi t} & 0 \\ i_2 & \sqrt{2}e^{-\frac{1}{2}i\pi t} & 0 \end{array}$ |

$$\begin{aligned} \mathcal{W}_1^{\text{gapless}} = & \sum_{m=1}^{n_{a_1}} \text{sgn}(v_m^{a_1}) \frac{1 - \text{sgn}(\delta_m^{a_1})}{2} - \sum_{m=1}^{n_{e_1}} \text{sgn}(v_m^{e_1}) \frac{1 - \text{sgn}(\delta_m^{e_1})}{2} - \sum_{m=1}^{n_{e_3}} \text{sgn}(v_m^{e_3}) \frac{1 - \text{sgn}(\delta_m^{e_3})}{2} - \sum_{m=1}^{n_{f_1}} \text{sgn}(v_m^{f_1}) \frac{1 - \text{sgn}(\delta_m^{f_1})}{2} \\ & - \sum_{m=1}^{n_{g_1}} \text{sgn}(v_m^{g_1}) \frac{1 - \text{sgn}(\delta_m^{g_1})}{2} - \sum_{m=1}^{n_{g_2}} \text{sgn}(v_m^{g_2}) \frac{1 - \text{sgn}(\delta_m^{g_2})}{2} + \sum_{m=1}^{n_{h_1}} \text{sgn}(v_m^{h_1}) \frac{1 - \text{sgn}(\delta_m^{h_1})}{2} \end{aligned} \quad (\text{S132.1})$$

$$\begin{aligned}\mathcal{W}_2^{\text{gapless}} = & \sum_{m=1}^{n_{b_1}} \text{sgn}(v_m^{b_1}) \frac{1 - \text{sgn}(\delta_m^{b_1})}{2} - \sum_{m=1}^{n_{e_1}} \text{sgn}(v_m^{e_1}) \frac{1 - \text{sgn}(\delta_m^{e_1})}{2} - \sum_{m=1}^{n_{e_3}} \text{sgn}(v_m^{e_3}) \frac{1 - \text{sgn}(\delta_m^{e_3})}{2} \\ & + \sum_{m=1}^{n_{h_1}} \text{sgn}(v_m^{h_1}) \frac{1 - \text{sgn}(\delta_m^{h_1})}{2} - \sum_{m=1}^{n_{i_1}} \text{sgn}(v_m^{i_1}) \frac{1 - \text{sgn}(\delta_m^{i_1})}{2} - \sum_{m=1}^{n_{i_2}} \text{sgn}(v_m^{i_2}) \frac{1 - \text{sgn}(\delta_m^{i_2})}{2}\end{aligned}\quad (\text{S132.2})$$

$$\begin{aligned}\mathcal{W}_3^{\text{gapless}} = & \sum_{m=1}^{n_{c_1}} \text{sgn}(v_m^{c_1}) \frac{1 - \text{sgn}(\delta_m^{c_1})}{2} - \sum_{m=1}^{n_{f_1}} \text{sgn}(v_m^{f_1}) \frac{1 - \text{sgn}(\delta_m^{f_1})}{2} - \sum_{m=1}^{n_{g_1}} \text{sgn}(v_m^{g_1}) \frac{1 - \text{sgn}(\delta_m^{g_1})}{2} \\ & - \sum_{m=1}^{n_{g_2}} \text{sgn}(v_m^{g_2}) \frac{1 - \text{sgn}(\delta_m^{g_2})}{2} + \sum_{m=1}^{n_{i_1}} \text{sgn}(v_m^{i_1}) \frac{1 - \text{sgn}(\delta_m^{i_1})}{2} + \sum_{m=1}^{n_{i_2}} \text{sgn}(v_m^{i_2}) \frac{1 - \text{sgn}(\delta_m^{i_2})}{2}\end{aligned}\quad (\text{S132.3})$$

$$\begin{aligned}\mathcal{W}_4^{\text{gapless}} = & \sum_{m=1}^{n_{d_1}} \text{sgn}(v_m^{d_1}) \frac{1 - \text{sgn}(\delta_m^{d_1})}{2} + \sum_{m=1}^{n_{d_3}} \text{sgn}(v_m^{d_3}) \frac{1 - \text{sgn}(\delta_m^{d_3})}{2} - \sum_{m=1}^{n_{e_1}} \text{sgn}(v_m^{e_1}) \frac{1 - \text{sgn}(\delta_m^{e_1})}{2} \\ & - \sum_{m=1}^{n_{e_3}} \text{sgn}(v_m^{e_3}) \frac{1 - \text{sgn}(\delta_m^{e_3})}{2} - \sum_{m=1}^{n_{f_1}} \text{sgn}(v_m^{f_1}) \frac{1 - \text{sgn}(\delta_m^{f_1})}{2}\end{aligned}\quad (\text{S132.4})$$

$$\mathcal{W}_1^{\text{gapped}} = \sum_{m=1}^{n_{e_1}} \text{sgn}(v_m^{e_1}) \frac{1 - \text{sgn}(\delta_m^{e_1})}{2} - \sum_{m=1}^{n_{e_3}} \text{sgn}(v_m^{e_3}) \frac{1 - \text{sgn}(\delta_m^{e_3})}{2} \quad (\text{S132.5})$$

$$\mathcal{W}_2^{\text{gapped}} = 2 \sum_{m=1}^{n_{d_3}} \text{sgn}(v_m^{d_3}) \frac{1 - \text{sgn}(\delta_m^{d_3})}{2} - 2 \sum_{m=1}^{n_{e_3}} \text{sgn}(v_m^{e_3}) \frac{1 - \text{sgn}(\delta_m^{e_3})}{2} - \sum_{m=1}^{n_{f_1}} \text{sgn}(v_m^{f_1}) \frac{1 - \text{sgn}(\delta_m^{f_1})}{2} \quad (\text{S132.6})$$

### S133. SPACE GROUP NO. 133

| line segment                                        | character of irrep (generators only) |                                                                                                                                                                                                                               |
|-----------------------------------------------------|--------------------------------------|-------------------------------------------------------------------------------------------------------------------------------------------------------------------------------------------------------------------------------|
| $a \quad (0, \frac{t}{2}, 0)$                       | $a_1$                                | $\left\{ 2_{010} \middle  \begin{smallmatrix} \frac{1}{2} & 0 & 0 \\ 0 \end{smallmatrix} \right\} \left\{ m_{100} \middle  \begin{smallmatrix} 0 & \frac{1}{2} & 0 \\ 0 \end{smallmatrix} \right\}$                           |
| $b \quad (\frac{1-t}{2}, \frac{1}{2}, 0)$           | $b_1$                                | $\left\{ 2_{100} \middle  \begin{smallmatrix} 0 & \frac{1}{2} & 0 \\ 0 \end{smallmatrix} \right\} \left\{ m_{010} \middle  \begin{smallmatrix} \frac{1}{2} & 0 & 0 \\ -ie^{-\frac{1}{2}i\pi(1-t)} \end{smallmatrix} \right\}$ |
|                                                     | $b_2$                                | $\left\{ m_{010} \middle  \begin{smallmatrix} \frac{1}{2} & 0 & 0 \\ ie^{-\frac{1}{2}i\pi(1-t)} \end{smallmatrix} \right\}$                                                                                                   |
|                                                     | $b_3$                                | $\left\{ m_{010} \middle  \begin{smallmatrix} \frac{1}{2} & 0 & 0 \\ -ie^{-\frac{1}{2}i\pi(1-t)} \end{smallmatrix} \right\}$                                                                                                  |
|                                                     | $b_4$                                | $\left\{ m_{010} \middle  \begin{smallmatrix} \frac{1}{2} & 0 & 0 \\ ie^{-\frac{1}{2}i\pi(1-t)} \end{smallmatrix} \right\}$                                                                                                   |
| $c \quad (\frac{t}{2}, \frac{t}{2}, 0)$             | $c_1$                                | $\left\{ 2_{110} \middle  \begin{smallmatrix} 0 & 0 & \frac{1}{2} \\ 0 \end{smallmatrix} \right\} \left\{ m_{001} \middle  \begin{smallmatrix} \frac{1}{2} & \frac{1}{2} & 0 \\ 0 \end{smallmatrix} \right\}$                 |
| $d \quad (0, \frac{t}{2}, \frac{1}{2})$             | $d_1$                                | $\left\{ 2_{010} \middle  \begin{smallmatrix} \frac{1}{2} & 0 & 0 \\ 0 \end{smallmatrix} \right\} \left\{ m_{100} \middle  \begin{smallmatrix} 0 & \frac{1}{2} & 0 \\ 0 \end{smallmatrix} \right\}$                           |
| $e \quad (\frac{1-t}{2}, \frac{1}{2}, \frac{1}{2})$ | $e_1$                                | $\left\{ 2_{100} \middle  \begin{smallmatrix} 0 & \frac{1}{2} & 0 \\ 0 \end{smallmatrix} \right\} \left\{ m_{010} \middle  \begin{smallmatrix} \frac{1}{2} & 0 & 0 \\ -ie^{-\frac{1}{2}i\pi(1-t)} \end{smallmatrix} \right\}$ |
|                                                     | $e_2$                                | $\left\{ m_{010} \middle  \begin{smallmatrix} \frac{1}{2} & 0 & 0 \\ ie^{-\frac{1}{2}i\pi(1-t)} \end{smallmatrix} \right\}$                                                                                                   |
|                                                     | $e_3$                                | $\left\{ m_{010} \middle  \begin{smallmatrix} \frac{1}{2} & 0 & 0 \\ -ie^{-\frac{1}{2}i\pi(1-t)} \end{smallmatrix} \right\}$                                                                                                  |
|                                                     | $e_4$                                | $\left\{ m_{010} \middle  \begin{smallmatrix} \frac{1}{2} & 0 & 0 \\ ie^{-\frac{1}{2}i\pi(1-t)} \end{smallmatrix} \right\}$                                                                                                   |

|                                                   |                                                                                         |
|---------------------------------------------------|-----------------------------------------------------------------------------------------|
| $f \quad (\frac{t}{2}, \frac{t}{2}, \frac{1}{2})$ | $\{2_{110}   0 \ 0 \ \frac{1}{2} \} \quad \{m_{001}   \frac{1}{2} \ \frac{1}{2} \ 0 \}$ |
| $f_1$                                             | $i \quad -ie^{-i\pi t}$                                                                 |
| $f_2$                                             | $i \quad ie^{-i\pi t}$                                                                  |
| $f_3$                                             | $-i \quad -ie^{-i\pi t}$                                                                |
| $f_4$                                             | $-i \quad ie^{-i\pi t}$                                                                 |
| $g \quad (0, 0, \frac{t}{2})$                     | $\{4_{001}   \frac{1}{2} \ 0 \ \frac{1}{2} \} \quad \{m_{100}   0 \ \frac{1}{2} \ 0 \}$ |
| $g_1$                                             | $-\sqrt{2}e^{-\frac{1}{2}i\pi t} \quad 0$                                               |
| $g_2$                                             | $\sqrt{2}e^{-\frac{1}{2}i\pi t} \quad 0$                                                |
| $h \quad (0, \frac{1}{2}, \frac{t}{2})$           | $\{2_{001}   \frac{1}{2} \ \frac{1}{2} \ 0 \} \quad \{m_{100}   0 \ \frac{1}{2} \ 0 \}$ |
| $h_1$                                             | $i \quad -1$                                                                            |
| $h_2$                                             | $i \quad 1$                                                                             |
| $h_3$                                             | $-i \quad -1$                                                                           |
| $h_4$                                             | $-i \quad 1$                                                                            |
| $i \quad (\frac{1}{2}, \frac{1}{2}, \frac{t}{2})$ | $\{4_{001}   \frac{1}{2} \ 0 \ \frac{1}{2} \} \quad \{m_{100}   0 \ \frac{1}{2} \ 0 \}$ |
| $i_1$                                             | $-\sqrt{2}e^{-\frac{1}{2}i\pi(t+1)} \quad 0$                                            |
| $i_2$                                             | $\sqrt{2}e^{-\frac{1}{2}i\pi(t+1)} \quad 0$                                             |

$$\begin{aligned}
\mathcal{W}_1^{\text{gapless}} = & \sum_{m=1}^{n_{a_1}} \text{sgn}(v_m^{a_1}) \frac{1 - \text{sgn}(\delta_m^{a_1})}{2} - \sum_{m=1}^{n_{e_1}} \text{sgn}(v_m^{e_1}) \frac{1 - \text{sgn}(\delta_m^{e_1})}{2} - \sum_{m=1}^{n_{e_3}} \text{sgn}(v_m^{e_3}) \frac{1 - \text{sgn}(\delta_m^{e_3})}{2} \\
& - \sum_{m=1}^{n_{f_1}} \text{sgn}(v_m^{f_1}) \frac{1 - \text{sgn}(\delta_m^{f_1})}{2} - \sum_{m=1}^{n_{f_3}} \text{sgn}(v_m^{f_3}) \frac{1 - \text{sgn}(\delta_m^{f_3})}{2} - \sum_{m=1}^{n_{g_1}} \text{sgn}(v_m^{g_1}) \frac{1 - \text{sgn}(\delta_m^{g_1})}{2} \\
& - \sum_{m=1}^{n_{g_2}} \text{sgn}(v_m^{g_2}) \frac{1 - \text{sgn}(\delta_m^{g_2})}{2} + \sum_{m=1}^{n_{h_1}} \text{sgn}(v_m^{h_1}) \frac{1 - \text{sgn}(\delta_m^{h_1})}{2} + \sum_{m=1}^{n_{h_3}} \text{sgn}(v_m^{h_3}) \frac{1 - \text{sgn}(\delta_m^{h_3})}{2}
\end{aligned} \tag{S133.1}$$

$$\begin{aligned}
\mathcal{W}_2^{\text{gapless}} = & \sum_{m=1}^{n_{b_1}} \text{sgn}(v_m^{b_1}) \frac{1 - \text{sgn}(\delta_m^{b_1})}{2} + \sum_{m=1}^{n_{b_3}} \text{sgn}(v_m^{b_3}) \frac{1 - \text{sgn}(\delta_m^{b_3})}{2} - \sum_{m=1}^{n_{e_1}} \text{sgn}(v_m^{e_1}) \frac{1 - \text{sgn}(\delta_m^{e_1})}{2} \\
& - \sum_{m=1}^{n_{e_3}} \text{sgn}(v_m^{e_3}) \frac{1 - \text{sgn}(\delta_m^{e_3})}{2} + \sum_{m=1}^{n_{h_1}} \text{sgn}(v_m^{h_1}) \frac{1 - \text{sgn}(\delta_m^{h_1})}{2} \\
& + \sum_{m=1}^{n_{h_3}} \text{sgn}(v_m^{h_3}) \frac{1 - \text{sgn}(\delta_m^{h_3})}{2} - \sum_{m=1}^{n_{i_1}} \text{sgn}(v_m^{i_1}) \frac{1 - \text{sgn}(\delta_m^{i_1})}{2} - \sum_{m=1}^{n_{i_2}} \text{sgn}(v_m^{i_2}) \frac{1 - \text{sgn}(\delta_m^{i_2})}{2}
\end{aligned} \tag{S133.2}$$

$$\begin{aligned}
\mathcal{W}_3^{\text{gapless}} = & \sum_{m=1}^{n_{c_1}} \text{sgn}(v_m^{c_1}) \frac{1 - \text{sgn}(\delta_m^{c_1})}{2} - \sum_{m=1}^{n_{f_1}} \text{sgn}(v_m^{f_1}) \frac{1 - \text{sgn}(\delta_m^{f_1})}{2} - \sum_{m=1}^{n_{f_3}} \text{sgn}(v_m^{f_3}) \frac{1 - \text{sgn}(\delta_m^{f_3})}{2} - \sum_{m=1}^{n_{g_1}} \text{sgn}(v_m^{g_1}) \frac{1 - \text{sgn}(\delta_m^{g_1})}{2} \\
& - \sum_{m=1}^{n_{g_2}} \text{sgn}(v_m^{g_2}) \frac{1 - \text{sgn}(\delta_m^{g_2})}{2} + \sum_{m=1}^{n_{i_1}} \text{sgn}(v_m^{i_1}) \frac{1 - \text{sgn}(\delta_m^{i_1})}{2} + \sum_{m=1}^{n_{i_2}} \text{sgn}(v_m^{i_2}) \frac{1 - \text{sgn}(\delta_m^{i_2})}{2}
\end{aligned} \tag{S133.3}$$

$$\begin{aligned}
\mathcal{W}_4^{\text{gapless}} = & \sum_{m=1}^{n_{d_1}} \text{sgn}(v_m^{d_1}) \frac{1 - \text{sgn}(\delta_m^{d_1})}{2} - \sum_{m=1}^{n_{e_1}} \text{sgn}(v_m^{e_1}) \frac{1 - \text{sgn}(\delta_m^{e_1})}{2} - \sum_{m=1}^{n_{e_3}} \text{sgn}(v_m^{e_3}) \frac{1 - \text{sgn}(\delta_m^{e_3})}{2} \\
& - \sum_{m=1}^{n_{f_1}} \text{sgn}(v_m^{f_1}) \frac{1 - \text{sgn}(\delta_m^{f_1})}{2} - \sum_{m=1}^{n_{f_3}} \text{sgn}(v_m^{f_3}) \frac{1 - \text{sgn}(\delta_m^{f_3})}{2}
\end{aligned} \tag{S133.4}$$

$$\mathcal{W}_1^{\text{gapped}} = \sum_{m=1}^{n_{f_1}} \text{sgn}(v_m^{f_1}) \frac{1 - \text{sgn}(\delta_m^{f_1})}{2} - \sum_{m=1}^{n_{f_3}} \text{sgn}(v_m^{f_3}) \frac{1 - \text{sgn}(\delta_m^{f_3})}{2} \quad (\text{S133.5})$$

$$\mathcal{W}_2^{\text{gapped}} = - \sum_{m=1}^{n_{h_1}} \text{sgn}(v_m^{h_1}) \frac{1 - \text{sgn}(\delta_m^{h_1})}{2} + \sum_{m=1}^{n_{h_3}} \text{sgn}(v_m^{h_3}) \frac{1 - \text{sgn}(\delta_m^{h_3})}{2} \quad (\text{S133.6})$$

$$\mathcal{W}_3^{\text{gapped}} = - \sum_{m=1}^{n_{e_1}} \text{sgn}(v_m^{e_1}) \frac{1 - \text{sgn}(\delta_m^{e_1})}{2} + \sum_{m=1}^{n_{e_3}} \text{sgn}(v_m^{e_3}) \frac{1 - \text{sgn}(\delta_m^{e_3})}{2} \quad (\text{S133.7})$$

$$\begin{aligned} \mathcal{W}_4^{\text{gapped}} = & -2 \sum_{m=1}^{n_{b_3}} \text{sgn}(v_m^{b_3}) \frac{1 - \text{sgn}(\delta_m^{b_3})}{2} + 2 \sum_{m=1}^{n_{e_1}} \text{sgn}(v_m^{e_1}) \frac{1 - \text{sgn}(\delta_m^{e_1})}{2} \\ & - 2 \sum_{m=1}^{n_{h_1}} \text{sgn}(v_m^{h_1}) \frac{1 - \text{sgn}(\delta_m^{h_1})}{2} + \sum_{m=1}^{n_{i_1}} \text{sgn}(v_m^{i_1}) \frac{1 - \text{sgn}(\delta_m^{i_1})}{2} + \sum_{m=1}^{n_{i_2}} \text{sgn}(v_m^{i_2}) \frac{1 - \text{sgn}(\delta_m^{i_2})}{2} \end{aligned} \quad (\text{S133.8})$$

### S134. SPACE GROUP NO. 134

| line segment                                        | character of irrep (generators only)                                                                                                                                                                                                                                                                                                                                                                                      |
|-----------------------------------------------------|---------------------------------------------------------------------------------------------------------------------------------------------------------------------------------------------------------------------------------------------------------------------------------------------------------------------------------------------------------------------------------------------------------------------------|
| $a \quad (0, \frac{t}{2}, 0)$                       | $a_1 \quad \left\{ 2_{010} \middle  \begin{smallmatrix} \frac{1}{2} & 0 & \frac{1}{2} \end{smallmatrix} \right\} \quad \left\{ m_{100} \middle  \begin{smallmatrix} 0 & \frac{1}{2} & \frac{1}{2} \end{smallmatrix} \right\}$<br>0                                                                                                                                                                                        |
| $b \quad (\frac{1-t}{2}, \frac{1}{2}, 0)$           | $b_1 \quad \left\{ 2_{100} \middle  \begin{smallmatrix} 0 & \frac{1}{2} & \frac{1}{2} \end{smallmatrix} \right\} \quad \left\{ m_{010} \middle  \begin{smallmatrix} \frac{1}{2} & 0 & \frac{1}{2} \end{smallmatrix} \right\}$<br>i $-ie^{-\frac{1}{2}i\pi(1-t)}$<br>$b_2 \quad i \quad ie^{-\frac{1}{2}i\pi(1-t)}$<br>$b_3 \quad -i \quad -ie^{-\frac{1}{2}i\pi(1-t)}$<br>$b_4 \quad -i \quad ie^{-\frac{1}{2}i\pi(1-t)}$ |
| $c \quad (\frac{t}{2}, \frac{t}{2}, 0)$             | $c_1 \quad \left\{ 2_{110} \middle  \begin{smallmatrix} 0 & 0 & 0 \end{smallmatrix} \right\} \quad \left\{ m_{001} \middle  \begin{smallmatrix} \frac{1}{2} & \frac{1}{2} & 0 \end{smallmatrix} \right\}$<br>0                                                                                                                                                                                                            |
| $d \quad (0, \frac{t}{2}, \frac{1}{2})$             | $d_1 \quad \left\{ 2_{010} \middle  \begin{smallmatrix} \frac{1}{2} & 0 & \frac{1}{2} \end{smallmatrix} \right\} \quad \left\{ m_{100} \middle  \begin{smallmatrix} 0 & \frac{1}{2} & \frac{1}{2} \end{smallmatrix} \right\}$<br>i $-ie^{-\frac{1}{2}i\pi(t+1)}$<br>$d_2 \quad i \quad ie^{-\frac{1}{2}i\pi(t+1)}$<br>$d_3 \quad -i \quad -ie^{-\frac{1}{2}i\pi(t+1)}$<br>$d_4 \quad -i \quad ie^{-\frac{1}{2}i\pi(t+1)}$ |
| $e \quad (\frac{1-t}{2}, \frac{1}{2}, \frac{1}{2})$ | $e_1 \quad \left\{ 2_{100} \middle  \begin{smallmatrix} 0 & \frac{1}{2} & \frac{1}{2} \end{smallmatrix} \right\} \quad \left\{ m_{010} \middle  \begin{smallmatrix} \frac{1}{2} & 0 & \frac{1}{2} \end{smallmatrix} \right\}$<br>0                                                                                                                                                                                        |
| $f \quad (\frac{t}{2}, \frac{t}{2}, \frac{1}{2})$   | $f_1 \quad \left\{ 2_{110} \middle  \begin{smallmatrix} 0 & 0 & 0 \end{smallmatrix} \right\} \quad \left\{ m_{001} \middle  \begin{smallmatrix} \frac{1}{2} & \frac{1}{2} & 0 \end{smallmatrix} \right\}$<br>0                                                                                                                                                                                                            |
| $g \quad (0, 0, \frac{t}{2})$                       | $g_1 \quad \left\{ 4_{001} \middle  \begin{smallmatrix} \frac{1}{2} & 0 & \frac{1}{2} \end{smallmatrix} \right\} \quad \left\{ m_{100} \middle  \begin{smallmatrix} 0 & \frac{1}{2} & \frac{1}{2} \end{smallmatrix} \right\}$<br>$-\sqrt{2}e^{-\frac{1}{2}i\pi t}$ 0<br>$g_2 \quad \sqrt{2}e^{-\frac{1}{2}i\pi t}$ 0                                                                                                      |
| $h \quad (0, \frac{1}{2}, \frac{t}{2})$             | $h_1 \quad \left\{ 2_{001} \middle  \begin{smallmatrix} \frac{1}{2} & \frac{1}{2} & 0 \end{smallmatrix} \right\} \quad \left\{ m_{100} \middle  \begin{smallmatrix} 0 & \frac{1}{2} & \frac{1}{2} \end{smallmatrix} \right\}$<br>i $-ie^{-\frac{1}{2}i\pi(t+1)}$<br>$h_2 \quad i \quad ie^{-\frac{1}{2}i\pi(t+1)}$<br>$h_3 \quad -i \quad -ie^{-\frac{1}{2}i\pi(t+1)}$<br>$h_4 \quad -i \quad ie^{-\frac{1}{2}i\pi(t+1)}$ |
| $i \quad (\frac{1}{2}, \frac{1}{2}, \frac{t}{2})$   | $i_1 \quad \left\{ 4_{001} \middle  \begin{smallmatrix} \frac{1}{2} & 0 & \frac{1}{2} \end{smallmatrix} \right\} \quad \left\{ m_{100} \middle  \begin{smallmatrix} 0 & \frac{1}{2} & \frac{1}{2} \end{smallmatrix} \right\}$<br>$-\sqrt{2}e^{-\frac{1}{2}i\pi(t+1)}$ 0<br>$i_2 \quad \sqrt{2}e^{-\frac{1}{2}i\pi(t+1)}$ 0                                                                                                |

---


$$\begin{aligned} \mathcal{W}_1^{\text{gapless}} = & \sum_{m=1}^{n_{a_1}} \text{sgn}(v_m^{a_1}) \frac{1 - \text{sgn}(\delta_m^{a_1})}{2} - \sum_{m=1}^{n_{e_1}} \text{sgn}(v_m^{e_1}) \frac{1 - \text{sgn}(\delta_m^{e_1})}{2} - \sum_{m=1}^{n_{f_1}} \text{sgn}(v_m^{f_1}) \frac{1 - \text{sgn}(\delta_m^{f_1})}{2} - \sum_{m=1}^{n_{g_1}} \text{sgn}(v_m^{g_1}) \frac{1 - \text{sgn}(\delta_m^{g_1})}{2} \\ & - \sum_{m=1}^{n_{g_2}} \text{sgn}(v_m^{g_2}) \frac{1 - \text{sgn}(\delta_m^{g_2})}{2} + \sum_{m=1}^{n_{h_1}} \text{sgn}(v_m^{h_1}) \frac{1 - \text{sgn}(\delta_m^{h_1})}{2} + \sum_{m=1}^{n_{h_3}} \text{sgn}(v_m^{h_3}) \frac{1 - \text{sgn}(\delta_m^{h_3})}{2} \end{aligned} \quad (\text{S134.1})$$

$$\begin{aligned} \mathcal{W}_2^{\text{gapless}} = & \sum_{m=1}^{n_{b_1}} \text{sgn}(v_m^{b_1}) \frac{1 - \text{sgn}(\delta_m^{b_1})}{2} + \sum_{m=1}^{n_{b_3}} \text{sgn}(v_m^{b_3}) \frac{1 - \text{sgn}(\delta_m^{b_3})}{2} - \sum_{m=1}^{n_{e_1}} \text{sgn}(v_m^{e_1}) \frac{1 - \text{sgn}(\delta_m^{e_1})}{2} + \sum_{m=1}^{n_{h_1}} \text{sgn}(v_m^{h_1}) \frac{1 - \text{sgn}(\delta_m^{h_1})}{2} \\ & + \sum_{m=1}^{n_{h_3}} \text{sgn}(v_m^{h_3}) \frac{1 - \text{sgn}(\delta_m^{h_3})}{2} - \sum_{m=1}^{n_{i_1}} \text{sgn}(v_m^{i_1}) \frac{1 - \text{sgn}(\delta_m^{i_1})}{2} - \sum_{m=1}^{n_{i_2}} \text{sgn}(v_m^{i_2}) \frac{1 - \text{sgn}(\delta_m^{i_2})}{2} \end{aligned} \quad (\text{S134.2})$$

$$\begin{aligned} \mathcal{W}_3^{\text{gapless}} = & \sum_{m=1}^{n_{c_1}} \text{sgn}(v_m^{c_1}) \frac{1 - \text{sgn}(\delta_m^{c_1})}{2} - \sum_{m=1}^{n_{f_1}} \text{sgn}(v_m^{f_1}) \frac{1 - \text{sgn}(\delta_m^{f_1})}{2} - \sum_{m=1}^{n_{g_1}} \text{sgn}(v_m^{g_1}) \frac{1 - \text{sgn}(\delta_m^{g_1})}{2} \\ & - \sum_{m=1}^{n_{g_2}} \text{sgn}(v_m^{g_2}) \frac{1 - \text{sgn}(\delta_m^{g_2})}{2} + \sum_{m=1}^{n_{i_1}} \text{sgn}(v_m^{i_1}) \frac{1 - \text{sgn}(\delta_m^{i_1})}{2} + \sum_{m=1}^{n_{i_2}} \text{sgn}(v_m^{i_2}) \frac{1 - \text{sgn}(\delta_m^{i_2})}{2} \end{aligned} \quad (\text{S134.3})$$

$$\begin{aligned} \mathcal{W}_4^{\text{gapless}} = & \sum_{m=1}^{n_{d_1}} \text{sgn}(v_m^{d_1}) \frac{1 - \text{sgn}(\delta_m^{d_1})}{2} + \sum_{m=1}^{n_{d_3}} \text{sgn}(v_m^{d_3}) \frac{1 - \text{sgn}(\delta_m^{d_3})}{2} - \sum_{m=1}^{n_{e_1}} \text{sgn}(v_m^{e_1}) \frac{1 - \text{sgn}(\delta_m^{e_1})}{2} - \sum_{m=1}^{n_{f_1}} \text{sgn}(v_m^{f_1}) \frac{1 - \text{sgn}(\delta_m^{f_1})}{2} \end{aligned} \quad (\text{S134.4})$$

$$\mathcal{W}_1^{\text{gapped}} = - \sum_{m=1}^{n_{h_1}} \text{sgn}(v_m^{h_1}) \frac{1 - \text{sgn}(\delta_m^{h_1})}{2} + \sum_{m=1}^{n_{h_3}} \text{sgn}(v_m^{h_3}) \frac{1 - \text{sgn}(\delta_m^{h_3})}{2} \quad (\text{S134.5})$$

$$\mathcal{W}_2^{\text{gapped}} = -2 \sum_{m=1}^{n_{d_3}} \text{sgn}(v_m^{d_3}) \frac{1 - \text{sgn}(\delta_m^{d_3})}{2} + \sum_{m=1}^{n_{e_1}} \text{sgn}(v_m^{e_1}) \frac{1 - \text{sgn}(\delta_m^{e_1})}{2} + \sum_{m=1}^{n_{f_1}} \text{sgn}(v_m^{f_1}) \frac{1 - \text{sgn}(\delta_m^{f_1})}{2} \quad (\text{S134.6})$$

$$\begin{aligned} \mathcal{W}_3^{\text{gapped}} = & -2 \sum_{m=1}^{n_{b_3}} \text{sgn}(v_m^{b_3}) \frac{1 - \text{sgn}(\delta_m^{b_3})}{2} + 2 \sum_{m=1}^{n_{d_3}} \text{sgn}(v_m^{d_3}) \frac{1 - \text{sgn}(\delta_m^{d_3})}{2} - \sum_{m=1}^{n_{f_1}} \text{sgn}(v_m^{f_1}) \frac{1 - \text{sgn}(\delta_m^{f_1})}{2} \\ & - 2 \sum_{m=1}^{n_{h_1}} \text{sgn}(v_m^{h_1}) \frac{1 - \text{sgn}(\delta_m^{h_1})}{2} + \sum_{m=1}^{n_{i_1}} \text{sgn}(v_m^{i_1}) \frac{1 - \text{sgn}(\delta_m^{i_1})}{2} + \sum_{m=1}^{n_{i_2}} \text{sgn}(v_m^{i_2}) \frac{1 - \text{sgn}(\delta_m^{i_2})}{2} \end{aligned} \quad (\text{S134.7})$$

## S135. SPACE GROUP NO. 135

| line segment                                        | character of irrep (generators only)                                                                                                                                                                                                                                                                                                                                                                            |
|-----------------------------------------------------|-----------------------------------------------------------------------------------------------------------------------------------------------------------------------------------------------------------------------------------------------------------------------------------------------------------------------------------------------------------------------------------------------------------------|
| $a \quad (0, \frac{t}{2}, 0)$                       | $a_1 \quad \left\{ 2_{010} \middle  \begin{smallmatrix} \frac{1}{2} & \frac{1}{2} & 0 \end{smallmatrix} \right\} \left\{ m_{100} \middle  \begin{smallmatrix} \frac{1}{2} & \frac{1}{2} & 0 \end{smallmatrix} \right\}$                                                                                                                                                                                         |
| $b \quad (\frac{1-t}{2}, \frac{1}{2}, 0)$           | $b_1 \quad \left\{ 2_{100} \middle  \begin{smallmatrix} \frac{1}{2} & \frac{1}{2} & 0 \end{smallmatrix} \right\} \left\{ m_{010} \middle  \begin{smallmatrix} \frac{1}{2} & \frac{1}{2} & 0 \end{smallmatrix} \right\}$                                                                                                                                                                                         |
| $c \quad (\frac{t}{2}, \frac{t}{2}, 0)$             | $c_1 \quad \left\{ 2_{110} \middle  \begin{smallmatrix} \frac{1}{2} & \frac{1}{2} & \frac{1}{2} \end{smallmatrix} \right\} \left\{ m_{001} \middle  \begin{smallmatrix} 0 & 0 & 0 \end{smallmatrix} \right\}$                                                                                                                                                                                                   |
| $d \quad (0, \frac{t}{2}, \frac{1}{2})$             | $d_1 \quad \left\{ 2_{010} \middle  \begin{smallmatrix} \frac{1}{2} & \frac{1}{2} & 0 \end{smallmatrix} \right\} \left\{ m_{100} \middle  \begin{smallmatrix} \frac{1}{2} & \frac{1}{2} & 0 \end{smallmatrix} \right\}$                                                                                                                                                                                         |
| $e \quad (\frac{1-t}{2}, \frac{1}{2}, \frac{1}{2})$ | $e_1 \quad \left\{ 2_{100} \middle  \begin{smallmatrix} \frac{1}{2} & \frac{1}{2} & 0 \end{smallmatrix} \right\} \left\{ m_{010} \middle  \begin{smallmatrix} \frac{1}{2} & \frac{1}{2} & 0 \end{smallmatrix} \right\}$                                                                                                                                                                                         |
| $f \quad (\frac{t}{2}, \frac{t}{2}, \frac{1}{2})$   | $f_1 \quad \left\{ 2_{110} \middle  \begin{smallmatrix} \frac{1}{2} & \frac{1}{2} & \frac{1}{2} \end{smallmatrix} \right\} \left\{ m_{001} \middle  \begin{smallmatrix} 0 & 0 & 0 \end{smallmatrix} \right\}$<br>$-e^{-\frac{1}{2}i\pi(2t+1)} \quad -i$<br>$f_2 \quad -e^{-\frac{1}{2}i\pi(2t+1)} \quad i$<br>$f_3 \quad e^{-\frac{1}{2}i\pi(2t+1)} \quad -i$<br>$f_4 \quad e^{-\frac{1}{2}i\pi(2t+1)} \quad i$ |
| $g \quad (0, 0, \frac{t}{2})$                       | $g_1 \quad \left\{ 4_{001} \middle  \begin{smallmatrix} 0 & 0 & \frac{1}{2} \end{smallmatrix} \right\} \left\{ m_{100} \middle  \begin{smallmatrix} \frac{1}{2} & \frac{1}{2} & 0 \end{smallmatrix} \right\}$<br>$-\sqrt{2}e^{-\frac{1}{2}i\pi t} \quad 0$<br>$g_2 \quad \sqrt{2}e^{-\frac{1}{2}i\pi t} \quad 0$                                                                                                |
| $h \quad (0, \frac{1}{2}, \frac{t}{2})$             | $h_1 \quad \left\{ 2_{001} \middle  \begin{smallmatrix} 0 & 0 & 0 \end{smallmatrix} \right\} \left\{ m_{100} \middle  \begin{smallmatrix} \frac{1}{2} & \frac{1}{2} & 0 \end{smallmatrix} \right\}$<br>$-i \quad -1$<br>$h_2 \quad -i \quad 1$<br>$h_3 \quad i \quad -1$<br>$h_4 \quad i \quad 1$                                                                                                               |
| $i \quad (\frac{1}{2}, \frac{1}{2}, \frac{t}{2})$   | $i_1 \quad \left\{ 4_{001} \middle  \begin{smallmatrix} 0 & 0 & \frac{1}{2} \end{smallmatrix} \right\} \left\{ m_{100} \middle  \begin{smallmatrix} \frac{1}{2} & \frac{1}{2} & 0 \end{smallmatrix} \right\}$<br>$-i\sqrt{2}e^{-\frac{1}{2}i\pi t} \quad 0$<br>$i_2 \quad i\sqrt{2}e^{-\frac{1}{2}i\pi t} \quad 0$                                                                                              |

$$\begin{aligned}
\mathcal{W}_1^{\text{gapless}} = & \sum_{m=1}^{n_{a_1}} \text{sgn}(v_m^{a_1}) \frac{1 - \text{sgn}(\delta_m^{a_1})}{2} - 2 \sum_{m=1}^{n_{e_1}} \text{sgn}(v_m^{e_1}) \frac{1 - \text{sgn}(\delta_m^{e_1})}{2} - \sum_{m=1}^{n_{f_1}} \text{sgn}(v_m^{f_1}) \frac{1 - \text{sgn}(\delta_m^{f_1})}{2} \\
& - \sum_{m=1}^{n_{f_3}} \text{sgn}(v_m^{f_3}) \frac{1 - \text{sgn}(\delta_m^{f_3})}{2} - \sum_{m=1}^{n_{g_1}} \text{sgn}(v_m^{g_1}) \frac{1 - \text{sgn}(\delta_m^{g_1})}{2} - \sum_{m=1}^{n_{g_2}} \text{sgn}(v_m^{g_2}) \frac{1 - \text{sgn}(\delta_m^{g_2})}{2} \\
& + 2 \sum_{m=1}^{n_{h_2}} \text{sgn}(v_m^{h_2}) \frac{1 - \text{sgn}(\delta_m^{h_2})}{2}
\end{aligned} \tag{S135.1}$$

$$\begin{aligned}
\mathcal{W}_2^{\text{gapless}} = & \sum_{m=1}^{n_{b_1}} \text{sgn}(v_m^{b_1}) \frac{1 - \text{sgn}(\delta_m^{b_1})}{2} - \sum_{m=1}^{n_{e_1}} \text{sgn}(v_m^{e_1}) \frac{1 - \text{sgn}(\delta_m^{e_1})}{2} + \sum_{m=1}^{n_{h_2}} \text{sgn}(v_m^{h_2}) \frac{1 - \text{sgn}(\delta_m^{h_2})}{2} - \sum_{m=1}^{n_{i_1}} \text{sgn}(v_m^{i_1}) \frac{1 - \text{sgn}(\delta_m^{i_1})}{2}
\end{aligned} \tag{S135.2}$$

$$\begin{aligned}
\mathcal{W}_3^{\text{gapless}} = & \sum_{m=1}^{n_{c_1}} \text{sgn}(v_m^{c_1}) \frac{1 - \text{sgn}(\delta_m^{c_1})}{2} - \sum_{m=1}^{n_{f_1}} \text{sgn}(v_m^{f_1}) \frac{1 - \text{sgn}(\delta_m^{f_1})}{2} - \sum_{m=1}^{n_{f_3}} \text{sgn}(v_m^{f_3}) \frac{1 - \text{sgn}(\delta_m^{f_3})}{2} \\
& - \sum_{m=1}^{n_{g_1}} \text{sgn}(v_m^{g_1}) \frac{1 - \text{sgn}(\delta_m^{g_1})}{2} - \sum_{m=1}^{n_{g_2}} \text{sgn}(v_m^{g_2}) \frac{1 - \text{sgn}(\delta_m^{g_2})}{2} + 2 \sum_{m=1}^{n_{i_1}} \text{sgn}(v_m^{i_1}) \frac{1 - \text{sgn}(\delta_m^{i_1})}{2}
\end{aligned} \tag{S135.3}$$



$$\mathcal{W}_4^{\text{gapless}} = \sum_{m=1}^{n_{d_1}} \text{sgn}(v_m^{d_1}) \frac{1 - \text{sgn}(\delta_m^{d_1})}{2} - 2 \sum_{m=1}^{n_{e_1}} \text{sgn}(v_m^{e_1}) \frac{1 - \text{sgn}(\delta_m^{e_1})}{2} - \sum_{m=1}^{n_{f_1}} \text{sgn}(v_m^{f_1}) \frac{1 - \text{sgn}(\delta_m^{f_1})}{2} - \sum_{m=1}^{n_{f_3}} \text{sgn}(v_m^{f_3}) \frac{1 - \text{sgn}(\delta_m^{f_3})}{2} \quad (\text{S135.4})$$

$$\mathcal{W}_5^{\text{gapless}} = \sum_{m=1}^{n_{h_1}} \text{sgn}(v_m^{h_1}) \frac{1 - \text{sgn}(\delta_m^{h_1})}{2} - \sum_{m=1}^{n_{h_2}} \text{sgn}(v_m^{h_2}) \frac{1 - \text{sgn}(\delta_m^{h_2})}{2} \quad (\text{S135.5})$$

$$\mathcal{W}_1^{\text{gapped}} = - \sum_{m=1}^{n_{f_1}} \text{sgn}(v_m^{f_1}) \frac{1 - \text{sgn}(\delta_m^{f_1})}{2} + \sum_{m=1}^{n_{f_3}} \text{sgn}(v_m^{f_3}) \frac{1 - \text{sgn}(\delta_m^{f_3})}{2} \quad (\text{S135.6})$$

### S136. SPACE GROUP NO. 136

| line segment                                        | character of irrep (generators only)                                                                                                                                                                                                                                                                                                                                                                                                                                                                                                                      |
|-----------------------------------------------------|-----------------------------------------------------------------------------------------------------------------------------------------------------------------------------------------------------------------------------------------------------------------------------------------------------------------------------------------------------------------------------------------------------------------------------------------------------------------------------------------------------------------------------------------------------------|
| $a \quad (0, \frac{t}{2}, 0)$                       | $a_1 \quad \left\{ 2_{010} \left  \begin{smallmatrix} \frac{1}{2} & \frac{1}{2} & \frac{1}{2} \end{smallmatrix} \right. \right\} \left\{ m_{100} \left  \begin{smallmatrix} \frac{1}{2} & \frac{1}{2} & \frac{1}{2} \end{smallmatrix} \right. \right\}$<br>0                                                                                                                                                                                                                                                                                              |
| $b \quad (\frac{1-t}{2}, \frac{1}{2}, 0)$           | $b_1 \quad \left\{ 2_{100} \left  \begin{smallmatrix} \frac{1}{2} & \frac{1}{2} & \frac{1}{2} \end{smallmatrix} \right. \right\} \left\{ m_{010} \left  \begin{smallmatrix} \frac{1}{2} & \frac{1}{2} & \frac{1}{2} \end{smallmatrix} \right. \right\}$<br>0                                                                                                                                                                                                                                                                                              |
| $c \quad (\frac{t}{2}, \frac{t}{2}, 0)$             | $c_1 \quad \left\{ 2_{110} \left  \begin{smallmatrix} 0 & 0 & 0 \end{smallmatrix} \right. \right\} \left\{ m_{001} \left  \begin{smallmatrix} 0 & 0 & 0 \end{smallmatrix} \right. \right\}$<br>0                                                                                                                                                                                                                                                                                                                                                          |
| $d \quad (0, \frac{t}{2}, \frac{1}{2})$             | $d_1 \quad \left\{ 2_{010} \left  \begin{smallmatrix} \frac{1}{2} & \frac{1}{2} & \frac{1}{2} \end{smallmatrix} \right. \right\} \left\{ m_{100} \left  \begin{smallmatrix} \frac{1}{2} & \frac{1}{2} & \frac{1}{2} \end{smallmatrix} \right. \right\}$<br>$-e^{-\frac{1}{2}i\pi(t+1)} \quad -ie^{-\frac{1}{2}i\pi(t+1)}$<br>$d_2 \quad -e^{-\frac{1}{2}i\pi(t+1)} \quad ie^{-\frac{1}{2}i\pi(t+1)}$<br>$d_3 \quad e^{-\frac{1}{2}i\pi(t+1)} \quad -ie^{-\frac{1}{2}i\pi(t+1)}$<br>$d_4 \quad e^{-\frac{1}{2}i\pi(t+1)} \quad ie^{-\frac{1}{2}i\pi(t+1)}$ |
| $e \quad (\frac{1-t}{2}, \frac{1}{2}, \frac{1}{2})$ | $e_1 \quad \left\{ 2_{100} \left  \begin{smallmatrix} \frac{1}{2} & \frac{1}{2} & \frac{1}{2} \end{smallmatrix} \right. \right\} \left\{ m_{010} \left  \begin{smallmatrix} \frac{1}{2} & \frac{1}{2} & \frac{1}{2} \end{smallmatrix} \right. \right\}$<br>$-ie^{-\frac{1}{2}i\pi(3-t)} \quad -e^{-\frac{1}{2}i\pi(3-t)}$<br>$e_2 \quad -ie^{-\frac{1}{2}i\pi(3-t)} \quad e^{-\frac{1}{2}i\pi(3-t)}$<br>$e_3 \quad ie^{-\frac{1}{2}i\pi(3-t)} \quad -e^{-\frac{1}{2}i\pi(3-t)}$<br>$e_4 \quad ie^{-\frac{1}{2}i\pi(3-t)} \quad e^{-\frac{1}{2}i\pi(3-t)}$ |
| $f \quad (\frac{t}{2}, \frac{t}{2}, \frac{1}{2})$   | $f_1 \quad \left\{ 2_{110} \left  \begin{smallmatrix} 0 & 0 & 0 \end{smallmatrix} \right. \right\} \left\{ m_{001} \left  \begin{smallmatrix} 0 & 0 & 0 \end{smallmatrix} \right. \right\}$<br>0                                                                                                                                                                                                                                                                                                                                                          |
| $g \quad (0, 0, \frac{t}{2})$                       | $g_1 \quad \left\{ 4_{001} \left  \begin{smallmatrix} \frac{1}{2} & \frac{1}{2} & \frac{1}{2} \end{smallmatrix} \right. \right\} \left\{ m_{100} \left  \begin{smallmatrix} \frac{1}{2} & \frac{1}{2} & \frac{1}{2} \end{smallmatrix} \right. \right\}$<br>$-\sqrt{2}e^{-\frac{1}{2}i\pi t} \quad 0$<br>$g_2 \quad \sqrt{2}e^{-\frac{1}{2}i\pi t} \quad 0$                                                                                                                                                                                                |
| $h \quad (0, \frac{1}{2}, \frac{t}{2})$             | $h_1 \quad \left\{ 2_{001} \left  \begin{smallmatrix} 0 & 0 & 0 \end{smallmatrix} \right. \right\} \left\{ m_{100} \left  \begin{smallmatrix} \frac{1}{2} & \frac{1}{2} & \frac{1}{2} \end{smallmatrix} \right. \right\}$<br>$-i \quad -ie^{-\frac{1}{2}i\pi(t+1)}$<br>$h_2 \quad -i \quad ie^{-\frac{1}{2}i\pi(t+1)}$<br>$h_3 \quad i \quad -ie^{-\frac{1}{2}i\pi(t+1)}$<br>$h_4 \quad i \quad ie^{-\frac{1}{2}i\pi(t+1)}$                                                                                                                               |
| $i \quad (\frac{1}{2}, \frac{1}{2}, \frac{t}{2})$   | $i_1 \quad \left\{ 4_{001} \left  \begin{smallmatrix} \frac{1}{2} & \frac{1}{2} & \frac{1}{2} \end{smallmatrix} \right. \right\} \left\{ m_{100} \left  \begin{smallmatrix} \frac{1}{2} & \frac{1}{2} & \frac{1}{2} \end{smallmatrix} \right. \right\}$<br>$-i\sqrt{2}e^{-\frac{1}{2}i\pi(t+2)} \quad 0$<br>$i_2 \quad i\sqrt{2}e^{-\frac{1}{2}i\pi(t+2)} \quad 0$                                                                                                                                                                                        |

$$\begin{aligned} \mathcal{W}_1^{\text{gapless}} = & \sum_{m=1}^{n_{a_1}} \text{sgn}(v_m^{a_1}) \frac{1 - \text{sgn}(\delta_m^{a_1})}{2} - 2 \sum_{m=1}^{n_{e_2}} \text{sgn}(v_m^{e_2}) \frac{1 - \text{sgn}(\delta_m^{e_2})}{2} - \sum_{m=1}^{n_{f_1}} \text{sgn}(v_m^{f_1}) \frac{1 - \text{sgn}(\delta_m^{f_1})}{2} \\ & - \sum_{m=1}^{n_{g_1}} \text{sgn}(v_m^{g_1}) \frac{1 - \text{sgn}(\delta_m^{g_1})}{2} - \sum_{m=1}^{n_{g_2}} \text{sgn}(v_m^{g_2}) \frac{1 - \text{sgn}(\delta_m^{g_2})}{2} + 2 \sum_{m=1}^{n_{h_1}} \text{sgn}(v_m^{h_1}) \frac{1 - \text{sgn}(\delta_m^{h_1})}{2} \end{aligned} \quad (\text{S136.1})$$

$$\mathcal{W}_2^{\text{gapless}} = \sum_{m=1}^{n_{b_1}} \text{sgn}(v_m^{b_1}) \frac{1 - \text{sgn}(\delta_m^{b_1})}{2} - \sum_{m=1}^{n_{e_2}} \text{sgn}(v_m^{e_2}) \frac{1 - \text{sgn}(\delta_m^{e_2})}{2} + \sum_{m=1}^{n_{h_1}} \text{sgn}(v_m^{h_1}) \frac{1 - \text{sgn}(\delta_m^{h_1})}{2} - \sum_{m=1}^{n_{i_1}} \text{sgn}(v_m^{i_1}) \frac{1 - \text{sgn}(\delta_m^{i_1})}{2} \quad (\text{S136.2})$$

$$\begin{aligned} \mathcal{W}_3^{\text{gapless}} = & \sum_{m=1}^{n_{c_1}} \text{sgn}(v_m^{c_1}) \frac{1 - \text{sgn}(\delta_m^{c_1})}{2} - \sum_{m=1}^{n_{f_1}} \text{sgn}(v_m^{f_1}) \frac{1 - \text{sgn}(\delta_m^{f_1})}{2} - \sum_{m=1}^{n_{g_1}} \text{sgn}(v_m^{g_1}) \frac{1 - \text{sgn}(\delta_m^{g_1})}{2} \\ & - \sum_{m=1}^{n_{g_2}} \text{sgn}(v_m^{g_2}) \frac{1 - \text{sgn}(\delta_m^{g_2})}{2} + 2 \sum_{m=1}^{n_{i_1}} \text{sgn}(v_m^{i_1}) \frac{1 - \text{sgn}(\delta_m^{i_1})}{2} \end{aligned} \quad (\text{S136.3})$$

$$\begin{aligned} \mathcal{W}_4^{\text{gapless}} = & \sum_{m=1}^{n_{d_1}} \text{sgn}(v_m^{d_1}) \frac{1 - \text{sgn}(\delta_m^{d_1})}{2} + \sum_{m=1}^{n_{d_3}} \text{sgn}(v_m^{d_3}) \frac{1 - \text{sgn}(\delta_m^{d_3})}{2} - 2 \sum_{m=1}^{n_{e_2}} \text{sgn}(v_m^{e_2}) \frac{1 - \text{sgn}(\delta_m^{e_2})}{2} \\ & - \sum_{m=1}^{n_{f_1}} \text{sgn}(v_m^{f_1}) \frac{1 - \text{sgn}(\delta_m^{f_1})}{2} + \sum_{m=1}^{n_{h_1}} \text{sgn}(v_m^{h_1}) \frac{1 - \text{sgn}(\delta_m^{h_1})}{2} - \sum_{m=1}^{n_{h_2}} \text{sgn}(v_m^{h_2}) \frac{1 - \text{sgn}(\delta_m^{h_2})}{2} \end{aligned} \quad (\text{S136.4})$$

$$\mathcal{W}_5^{\text{gapless}} = \sum_{m=1}^{n_{e_1}} \text{sgn}(v_m^{e_1}) \frac{1 - \text{sgn}(\delta_m^{e_1})}{2} - \sum_{m=1}^{n_{e_2}} \text{sgn}(v_m^{e_2}) \frac{1 - \text{sgn}(\delta_m^{e_2})}{2} + \sum_{m=1}^{n_{h_1}} \text{sgn}(v_m^{h_1}) \frac{1 - \text{sgn}(\delta_m^{h_1})}{2} - \sum_{m=1}^{n_{h_2}} \text{sgn}(v_m^{h_2}) \frac{1 - \text{sgn}(\delta_m^{h_2})}{2} \quad (\text{S136.5})$$

$$\mathcal{X}_1 = \sum_{m=1}^{n_{f_1}} \frac{1 - \text{sgn}(\delta_m^{f_1})}{2} \quad \text{mod } 2 \quad (\text{S136.6})$$

### S137. SPACE GROUP NO. 137

| line segment                                        | character of irrep (generators only)                                                                                                                                                                                                                                                                                                                                                                                                                                                  |
|-----------------------------------------------------|---------------------------------------------------------------------------------------------------------------------------------------------------------------------------------------------------------------------------------------------------------------------------------------------------------------------------------------------------------------------------------------------------------------------------------------------------------------------------------------|
| $a \quad (0, \frac{t}{2}, 0)$                       | $a_1 \quad \left\{ 2_{010} \middle  \begin{smallmatrix} 0 & \frac{1}{2} & 0 \end{smallmatrix} \right\} \quad \left\{ m_{100} \middle  \begin{smallmatrix} \frac{1}{2} & 0 & 0 \end{smallmatrix} \right\}$<br>0                                                                                                                                                                                                                                                                        |
| $b \quad (\frac{1-t}{2}, \frac{1}{2}, 0)$           | $b_1 \quad \left\{ 2_{100} \middle  \begin{smallmatrix} \frac{1}{2} & 0 & 0 \end{smallmatrix} \right\} \quad \left\{ m_{010} \middle  \begin{smallmatrix} 0 & \frac{1}{2} & 0 \end{smallmatrix} \right\}$<br>$-ie^{-\frac{1}{2}i\pi(1-t)} \quad i$<br>$b_2 \quad -ie^{-\frac{1}{2}i\pi(1-t)} \quad -i$<br>$b_3 \quad ie^{-\frac{1}{2}i\pi(1-t)} \quad i$<br>$b_4 \quad ie^{-\frac{1}{2}i\pi(1-t)} \quad -i$                                                                           |
| $c \quad (\frac{t}{2}, \frac{t}{2}, 0)$             | $c_1 \quad \left\{ 2_{110} \middle  \begin{smallmatrix} \frac{1}{2} & \frac{1}{2} & \frac{1}{2} \end{smallmatrix} \right\} \quad \left\{ m_{001} \middle  \begin{smallmatrix} \frac{1}{2} & \frac{1}{2} & 0 \end{smallmatrix} \right\}$<br>0                                                                                                                                                                                                                                          |
| $d \quad (0, \frac{t}{2}, \frac{1}{2})$             | $d_1 \quad \left\{ 2_{010} \middle  \begin{smallmatrix} 0 & \frac{1}{2} & 0 \end{smallmatrix} \right\} \quad \left\{ m_{100} \middle  \begin{smallmatrix} \frac{1}{2} & 0 & 0 \end{smallmatrix} \right\}$<br>0                                                                                                                                                                                                                                                                        |
| $e \quad (\frac{1-t}{2}, \frac{1}{2}, \frac{1}{2})$ | $e_1 \quad \left\{ 2_{100} \middle  \begin{smallmatrix} \frac{1}{2} & 0 & 0 \end{smallmatrix} \right\} \quad \left\{ m_{010} \middle  \begin{smallmatrix} 0 & \frac{1}{2} & 0 \end{smallmatrix} \right\}$<br>$-ie^{-\frac{1}{2}i\pi(1-t)} \quad i$<br>$e_2 \quad -ie^{-\frac{1}{2}i\pi(1-t)} \quad -i$<br>$e_3 \quad ie^{-\frac{1}{2}i\pi(1-t)} \quad i$<br>$e_4 \quad ie^{-\frac{1}{2}i\pi(1-t)} \quad -i$                                                                           |
| $f \quad (\frac{t}{2}, \frac{t}{2}, \frac{1}{2})$   | $f_1 \quad \left\{ 2_{110} \middle  \begin{smallmatrix} \frac{1}{2} & \frac{1}{2} & \frac{1}{2} \end{smallmatrix} \right\} \quad \left\{ m_{001} \middle  \begin{smallmatrix} \frac{1}{2} & \frac{1}{2} & 0 \end{smallmatrix} \right\}$<br>$-e^{-\frac{1}{2}i\pi(2t+1)} \quad -ie^{-i\pi t}$<br>$f_2 \quad -e^{-\frac{1}{2}i\pi(2t+1)} \quad ie^{-i\pi t}$<br>$f_3 \quad e^{-\frac{1}{2}i\pi(2t+1)} \quad -ie^{-i\pi t}$<br>$f_4 \quad e^{-\frac{1}{2}i\pi(2t+1)} \quad ie^{-i\pi t}$ |

|                                                   |                                                                                                                                                                                                                  |
|---------------------------------------------------|------------------------------------------------------------------------------------------------------------------------------------------------------------------------------------------------------------------|
| $g \quad (0, 0, \frac{t}{2})$                     | $\begin{matrix} \{4_{001}   \frac{1}{2} \ 0 \ \frac{1}{2} \} & \{m_{100}   \frac{1}{2} \ 0 \ 0 \} \\ g_1 & -\sqrt{2}e^{-\frac{1}{2}i\pi t} & 0 \\ g_2 & \sqrt{2}e^{-\frac{1}{2}i\pi t} & 0 \end{matrix}$         |
| $h \quad (0, \frac{1}{2}, \frac{t}{2})$           | $\begin{matrix} \{2_{001}   \frac{1}{2} \ \frac{1}{2} \ 0 \} & \{m_{100}   \frac{1}{2} \ 0 \ 0 \} \\ h_1 & 0 & 0 \end{matrix}$                                                                                   |
| $i \quad (\frac{1}{2}, \frac{1}{2}, \frac{t}{2})$ | $\begin{matrix} \{4_{001}   \frac{1}{2} \ 0 \ \frac{1}{2} \} & \{m_{100}   \frac{1}{2} \ 0 \ 0 \} \\ i_1 & -i\sqrt{2}e^{-\frac{1}{2}i\pi(t+1)} & 0 \\ i_2 & i\sqrt{2}e^{-\frac{1}{2}i\pi(t+1)} & 0 \end{matrix}$ |

$$\begin{aligned} \mathcal{W}_1^{\text{gapless}} = & \sum_{m=1}^{n_{a_1}} \text{sgn}(v_m^{a_1}) \frac{1 - \text{sgn}(\delta_m^{a_1})}{2} - \sum_{m=1}^{n_{e_1}} \text{sgn}(v_m^{e_1}) \frac{1 - \text{sgn}(\delta_m^{e_1})}{2} - \sum_{m=1}^{n_{e_2}} \text{sgn}(v_m^{e_2}) \frac{1 - \text{sgn}(\delta_m^{e_2})}{2} \\ & - \sum_{m=1}^{n_{f_1}} \text{sgn}(v_m^{f_1}) \frac{1 - \text{sgn}(\delta_m^{f_1})}{2} - \sum_{m=1}^{n_{f_3}} \text{sgn}(v_m^{f_3}) \frac{1 - \text{sgn}(\delta_m^{f_3})}{2} - \sum_{m=1}^{n_{g_1}} \text{sgn}(v_m^{g_1}) \frac{1 - \text{sgn}(\delta_m^{g_1})}{2} \\ & - \sum_{m=1}^{n_{g_2}} \text{sgn}(v_m^{g_2}) \frac{1 - \text{sgn}(\delta_m^{g_2})}{2} + 2 \sum_{m=1}^{n_{h_1}} \text{sgn}(v_m^{h_1}) \frac{1 - \text{sgn}(\delta_m^{h_1})}{2} \end{aligned} \quad (\text{S137.1})$$

$$\mathcal{W}_2^{\text{gapless}} = \sum_{m=1}^{n_{b_1}} \text{sgn}(v_m^{b_1}) \frac{1 - \text{sgn}(\delta_m^{b_1})}{2} - \sum_{m=1}^{n_{e_1}} \text{sgn}(v_m^{e_1}) \frac{1 - \text{sgn}(\delta_m^{e_1})}{2} + \sum_{m=1}^{n_{h_1}} \text{sgn}(v_m^{h_1}) \frac{1 - \text{sgn}(\delta_m^{h_1})}{2} - \sum_{m=1}^{n_{i_1}} \text{sgn}(v_m^{i_1}) \frac{1 - \text{sgn}(\delta_m^{i_1})}{2} \quad (\text{S137.2})$$

$$\mathcal{W}_3^{\text{gapless}} = \sum_{m=1}^{n_{b_2}} \text{sgn}(v_m^{b_2}) \frac{1 - \text{sgn}(\delta_m^{b_2})}{2} - \sum_{m=1}^{n_{e_2}} \text{sgn}(v_m^{e_2}) \frac{1 - \text{sgn}(\delta_m^{e_2})}{2} + \sum_{m=1}^{n_{h_1}} \text{sgn}(v_m^{h_1}) \frac{1 - \text{sgn}(\delta_m^{h_1})}{2} - \sum_{m=1}^{n_{i_1}} \text{sgn}(v_m^{i_1}) \frac{1 - \text{sgn}(\delta_m^{i_1})}{2} \quad (\text{S137.3})$$

$$\begin{aligned} \mathcal{W}_4^{\text{gapless}} = & \sum_{m=1}^{n_{c_1}} \text{sgn}(v_m^{c_1}) \frac{1 - \text{sgn}(\delta_m^{c_1})}{2} - \sum_{m=1}^{n_{f_1}} \text{sgn}(v_m^{f_1}) \frac{1 - \text{sgn}(\delta_m^{f_1})}{2} - \sum_{m=1}^{n_{f_3}} \text{sgn}(v_m^{f_3}) \frac{1 - \text{sgn}(\delta_m^{f_3})}{2} \\ & - \sum_{m=1}^{n_{g_1}} \text{sgn}(v_m^{g_1}) \frac{1 - \text{sgn}(\delta_m^{g_1})}{2} - \sum_{m=1}^{n_{g_2}} \text{sgn}(v_m^{g_2}) \frac{1 - \text{sgn}(\delta_m^{g_2})}{2} + 2 \sum_{m=1}^{n_{i_1}} \text{sgn}(v_m^{i_1}) \frac{1 - \text{sgn}(\delta_m^{i_1})}{2} \end{aligned} \quad (\text{S137.4})$$

$$\begin{aligned} \mathcal{W}_5^{\text{gapless}} = & \sum_{m=1}^{n_{d_1}} \text{sgn}(v_m^{d_1}) \frac{1 - \text{sgn}(\delta_m^{d_1})}{2} - \sum_{m=1}^{n_{e_1}} \text{sgn}(v_m^{e_1}) \frac{1 - \text{sgn}(\delta_m^{e_1})}{2} - \sum_{m=1}^{n_{e_2}} \text{sgn}(v_m^{e_2}) \frac{1 - \text{sgn}(\delta_m^{e_2})}{2} \\ & - \sum_{m=1}^{n_{f_1}} \text{sgn}(v_m^{f_1}) \frac{1 - \text{sgn}(\delta_m^{f_1})}{2} - \sum_{m=1}^{n_{f_3}} \text{sgn}(v_m^{f_3}) \frac{1 - \text{sgn}(\delta_m^{f_3})}{2} \end{aligned} \quad (\text{S137.5})$$

$$\mathcal{W}_1^{\text{gapped}} = \sum_{m=1}^{n_{e_1}} \text{sgn}(v_m^{e_1}) \frac{1 - \text{sgn}(\delta_m^{e_1})}{2} - \sum_{m=1}^{n_{e_2}} \text{sgn}(v_m^{e_2}) \frac{1 - \text{sgn}(\delta_m^{e_2})}{2} \quad (\text{S137.6})$$

$$\mathcal{W}_2^{\text{gapped}} = - \sum_{m=1}^{n_{f_1}} \text{sgn}(v_m^{f_1}) \frac{1 - \text{sgn}(\delta_m^{f_1})}{2} + \sum_{m=1}^{n_{f_3}} \text{sgn}(v_m^{f_3}) \frac{1 - \text{sgn}(\delta_m^{f_3})}{2} \quad (\text{S137.7})$$

## S138. SPACE GROUP NO. 138

| line segment                                        | character of irrep (generators only)                                                                                                                                                                                                                                                                               |
|-----------------------------------------------------|--------------------------------------------------------------------------------------------------------------------------------------------------------------------------------------------------------------------------------------------------------------------------------------------------------------------|
| $a \quad (0, \frac{t}{2}, 0)$                       | $a_1 \quad \begin{array}{c} \{2_{010}   0 \frac{1}{2} \frac{1}{2}\} \{m_{100}   \frac{1}{2} 0 \frac{1}{2}\} \\ 0 \end{array}$                                                                                                                                                                                      |
| $b \quad (\frac{1-t}{2}, \frac{1}{2}, 0)$           | $\begin{array}{c} \{2_{100}   \frac{1}{2} 0 \frac{1}{2}\} \{m_{010}   0 \frac{1}{2} \frac{1}{2}\} \\ b_1 \quad -ie^{-\frac{1}{2}i\pi(1-t)} \quad i \\ b_2 \quad -ie^{-\frac{1}{2}i\pi(1-t)} \quad -i \\ b_3 \quad ie^{-\frac{1}{2}i\pi(1-t)} \quad i \\ b_4 \quad ie^{-\frac{1}{2}i\pi(1-t)} \quad -i \end{array}$ |
| $c \quad (\frac{t}{2}, \frac{t}{2}, 0)$             | $c_1 \quad \begin{array}{c} \{2_{110}   \frac{1}{2} \frac{1}{2} 0\} \{m_{001}   \frac{1}{2} \frac{1}{2} 0\} \\ 0 \end{array}$                                                                                                                                                                                      |
| $d \quad (0, \frac{t}{2}, \frac{1}{2})$             | $\begin{array}{c} \{2_{010}   0 \frac{1}{2} \frac{1}{2}\} \{m_{100}   \frac{1}{2} 0 \frac{1}{2}\} \\ d_1 \quad -e^{-\frac{1}{2}i\pi(t+1)} \quad -1 \\ d_2 \quad -e^{-\frac{1}{2}i\pi(t+1)} \quad 1 \\ d_3 \quad e^{-\frac{1}{2}i\pi(t+1)} \quad -1 \\ d_4 \quad e^{-\frac{1}{2}i\pi(t+1)} \quad 1 \end{array}$     |
| $e \quad (\frac{1-t}{2}, \frac{1}{2}, \frac{1}{2})$ | $e_1 \quad \begin{array}{c} \{2_{100}   \frac{1}{2} 0 \frac{1}{2}\} \{m_{010}   0 \frac{1}{2} \frac{1}{2}\} \\ 0 \end{array}$                                                                                                                                                                                      |
| $f \quad (\frac{t}{2}, \frac{t}{2}, \frac{1}{2})$   | $f_1 \quad \begin{array}{c} \{2_{110}   \frac{1}{2} \frac{1}{2} 0\} \{m_{001}   \frac{1}{2} \frac{1}{2} 0\} \\ 0 \end{array}$                                                                                                                                                                                      |
| $g \quad (0, 0, \frac{t}{2})$                       | $\begin{array}{c} \{4_{001}   \frac{1}{2} 0 \frac{1}{2}\} \{m_{100}   \frac{1}{2} 0 \frac{1}{2}\} \\ g_1 \quad -\sqrt{2}e^{-\frac{1}{2}i\pi t} \quad 0 \\ g_2 \quad \sqrt{2}e^{-\frac{1}{2}i\pi t} \quad 0 \end{array}$                                                                                            |
| $h \quad (0, \frac{1}{2}, \frac{t}{2})$             | $h_1 \quad \begin{array}{c} \{2_{001}   \frac{1}{2} \frac{1}{2} 0\} \{m_{100}   \frac{1}{2} 0 \frac{1}{2}\} \\ 0 \end{array}$                                                                                                                                                                                      |
| $i \quad (\frac{1}{2}, \frac{1}{2}, \frac{t}{2})$   | $\begin{array}{c} \{4_{001}   \frac{1}{2} 0 \frac{1}{2}\} \{m_{100}   \frac{1}{2} 0 \frac{1}{2}\} \\ i_1 \quad -i\sqrt{2}e^{-\frac{1}{2}i\pi(t+1)} \quad 0 \\ i_2 \quad i\sqrt{2}e^{-\frac{1}{2}i\pi(t+1)} \quad 0 \end{array}$                                                                                    |

$$\begin{aligned} \mathcal{W}_1^{\text{gapless}} = & \sum_{m=1}^{n_{a_1}} \text{sgn}(v_m^{a_1}) \frac{1 - \text{sgn}(\delta_m^{a_1})}{2} - 2 \sum_{m=1}^{n_{e_1}} \text{sgn}(v_m^{e_1}) \frac{1 - \text{sgn}(\delta_m^{e_1})}{2} - \sum_{m=1}^{n_{f_1}} \text{sgn}(v_m^{f_1}) \frac{1 - \text{sgn}(\delta_m^{f_1})}{2} \\ & - \sum_{m=1}^{n_{g_1}} \text{sgn}(v_m^{g_1}) \frac{1 - \text{sgn}(\delta_m^{g_1})}{2} - \sum_{m=1}^{n_{g_2}} \text{sgn}(v_m^{g_2}) \frac{1 - \text{sgn}(\delta_m^{g_2})}{2} + 2 \sum_{m=1}^{n_{h_1}} \text{sgn}(v_m^{h_1}) \frac{1 - \text{sgn}(\delta_m^{h_1})}{2} \end{aligned} \quad (\text{S138.1})$$

$$\mathcal{W}_2^{\text{gapless}} = \sum_{m=1}^{n_{b_1}} \text{sgn}(v_m^{b_1}) \frac{1 - \text{sgn}(\delta_m^{b_1})}{2} - \sum_{m=1}^{n_{e_1}} \text{sgn}(v_m^{e_1}) \frac{1 - \text{sgn}(\delta_m^{e_1})}{2} + \sum_{m=1}^{n_{h_1}} \text{sgn}(v_m^{h_1}) \frac{1 - \text{sgn}(\delta_m^{h_1})}{2} - \sum_{m=1}^{n_{i_1}} \text{sgn}(v_m^{i_1}) \frac{1 - \text{sgn}(\delta_m^{i_1})}{2} \quad (\text{S138.2})$$

$$\mathcal{W}_3^{\text{gapless}} = \sum_{m=1}^{n_{b_2}} \text{sgn}(v_m^{b_2}) \frac{1 - \text{sgn}(\delta_m^{b_2})}{2} - \sum_{m=1}^{n_{e_1}} \text{sgn}(v_m^{e_1}) \frac{1 - \text{sgn}(\delta_m^{e_1})}{2} + \sum_{m=1}^{n_{h_1}} \text{sgn}(v_m^{h_1}) \frac{1 - \text{sgn}(\delta_m^{h_1})}{2} - \sum_{m=1}^{n_{i_1}} \text{sgn}(v_m^{i_1}) \frac{1 - \text{sgn}(\delta_m^{i_1})}{2} \quad (\text{S138.3})$$

$$\begin{aligned} \mathcal{W}_4^{\text{gapless}} = & \sum_{m=1}^{n_{c_1}} \text{sgn}(v_m^{c_1}) \frac{1 - \text{sgn}(\delta_m^{c_1})}{2} - \sum_{m=1}^{n_{f_1}} \text{sgn}(v_m^{f_1}) \frac{1 - \text{sgn}(\delta_m^{f_1})}{2} - \sum_{m=1}^{n_{g_1}} \text{sgn}(v_m^{g_1}) \frac{1 - \text{sgn}(\delta_m^{g_1})}{2} \\ & - \sum_{m=1}^{n_{g_2}} \text{sgn}(v_m^{g_2}) \frac{1 - \text{sgn}(\delta_m^{g_2})}{2} + 2 \sum_{m=1}^{n_{i_1}} \text{sgn}(v_m^{i_1}) \frac{1 - \text{sgn}(\delta_m^{i_1})}{2} \end{aligned} \quad (\text{S138.4})$$

$$\mathcal{W}_5^{\text{gapless}} = \sum_{m=1}^{n_{d_1}} \text{sgn}(v_m^{d_1}) \frac{1 - \text{sgn}(\delta_m^{d_1})}{2} + \sum_{m=1}^{n_{d_3}} \text{sgn}(v_m^{d_3}) \frac{1 - \text{sgn}(\delta_m^{d_3})}{2} - 2 \sum_{m=1}^{n_{e_1}} \text{sgn}(v_m^{e_1}) \frac{1 - \text{sgn}(\delta_m^{e_1})}{2} - \sum_{m=1}^{n_{f_1}} \text{sgn}(v_m^{f_1}) \frac{1 - \text{sgn}(\delta_m^{f_1})}{2} \quad (\text{S138.5})$$

$$\mathcal{X}_1 = \sum_{m=1}^{n_{f_1}} \frac{1 - \text{sgn}(\delta_m^{f_1})}{2} \mod 2 \quad (\text{S138.6})$$

### S139. SPACE GROUP NO. 139

| line segment                                      | character of irrep (generators only)                                                                                                   |
|---------------------------------------------------|----------------------------------------------------------------------------------------------------------------------------------------|
| $a \ (0, 0, t)$                                   | $\begin{array}{cc} \{4_{001}   0 \ 0 \ 0\} & \{m_{100}   0 \ 0 \ 0\} \\ a_1 & -\sqrt{2} \quad 0 \\ a_2 & \sqrt{2} \quad 0 \end{array}$ |
| $b \ (\frac{1}{2}, \frac{1}{2}, \frac{t}{2})$     | $\begin{array}{cc} \{2_{001}   0 \ 0 \ 0\} & \{m_{110}   0 \ 0 \ 0\} \\ b_1 & 0 \quad 0 \end{array}$                                   |
| $c \ (\frac{t}{2}, \frac{t}{2}, 1 - \frac{t}{2})$ | $\begin{array}{cc} \{m_{1-10}   0 \ 0 \ 0\} \\ c_1 & -i \\ c_2 & i \end{array}$                                                        |
| $d \ (\frac{t}{2}, \frac{t}{2}, 0)$               | $\begin{array}{cc} \{2_{110}   0 \ 0 \ 0\} & \{m_{001}   0 \ 0 \ 0\} \\ d_1 & 0 \quad 0 \end{array}$                                   |
| $e \ (\frac{t}{2}, 1 - \frac{t}{2}, 0)$           | $\begin{array}{cc} \{2_{1-10}   0 \ 0 \ 0\} & \{m_{001}   0 \ 0 \ 0\} \\ e_1 & 0 \quad 0 \end{array}$                                  |
| $f \ (\frac{1-t}{2}, \frac{1}{2}, \frac{1}{2})$   | $\begin{array}{cc} \{2_{100}   0 \ 0 \ 0\} \\ f_1 & -i \\ f_2 & i \end{array}$                                                         |
| $g \ (0, t, 0)$                                   | $\begin{array}{cc} \{2_{010}   0 \ 0 \ 0\} & \{m_{100}   0 \ 0 \ 0\} \\ g_1 & 0 \quad 0 \end{array}$                                   |
| $h \ (0, \frac{t}{2}, 1 - \frac{t}{2})$           | $\begin{array}{cc} \{m_{100}   0 \ 0 \ 0\} \\ h_1 & -i \\ h_2 & i \end{array}$                                                         |

$$\mathcal{W}_1^{\text{gapless}} = \sum_{m=1}^{n_{a_1}} \text{sgn}(v_m^{a_1}) \frac{1 - \text{sgn}(\delta_m^{a_1})}{2} + \sum_{m=1}^{n_{a_2}} \text{sgn}(v_m^{a_2}) \frac{1 - \text{sgn}(\delta_m^{a_2})}{2} - \sum_{m=1}^{n_{g_1}} \text{sgn}(v_m^{g_1}) \frac{1 - \text{sgn}(\delta_m^{g_1})}{2} \quad (\text{S139.1})$$

$$\mathcal{W}_2^{\text{gapless}} = \sum_{m=1}^{n_{b_1}} \text{sgn}(v_m^{b_1}) \frac{1 - \text{sgn}(\delta_m^{b_1})}{2} + \sum_{m=1}^{n_{e_1}} \text{sgn}(v_m^{e_1}) \frac{1 - \text{sgn}(\delta_m^{e_1})}{2} + \sum_{m=1}^{n_{f_1}} \text{sgn}(v_m^{f_1}) \frac{1 - \text{sgn}(\delta_m^{f_1})}{2} - \sum_{m=1}^{n_{h_1}} \text{sgn}(v_m^{h_1}) \frac{1 - \text{sgn}(\delta_m^{h_1})}{2} \quad (\text{S139.2})$$

$$\mathcal{W}_3^{\text{gapless}} = \sum_{m=1}^{n_{c_1}} \text{sgn}(v_m^{c_1}) \frac{1 - \text{sgn}(\delta_m^{c_1})}{2} + \sum_{m=1}^{n_{f_1}} \text{sgn}(v_m^{f_1}) \frac{1 - \text{sgn}(\delta_m^{f_1})}{2} - \sum_{m=1}^{n_{h_1}} \text{sgn}(v_m^{h_1}) \frac{1 - \text{sgn}(\delta_m^{h_1})}{2} \quad (\text{S139.3})$$

$$\mathcal{W}_4^{\text{gapless}} = \sum_{m=1}^{n_{d_1}} \text{sgn}(v_m^{d_1}) \frac{1 - \text{sgn}(\delta_m^{d_1})}{2} - \sum_{m=1}^{n_{e_1}} \text{sgn}(v_m^{e_1}) \frac{1 - \text{sgn}(\delta_m^{e_1})}{2} - \sum_{m=1}^{n_{g_1}} \text{sgn}(v_m^{g_1}) \frac{1 - \text{sgn}(\delta_m^{g_1})}{2} \quad (\text{S139.4})$$

**S140. SPACE GROUP NO. 140**

| line segment                                      | character of irrep (generators only)                                  |
|---------------------------------------------------|-----------------------------------------------------------------------|
| $a$ $(0, 0, t)$                                   | $\{4_{001}  0 \ 0 \ 0\} \ \{m_{100}  0 \ 0 \ \frac{1}{2}\}$           |
|                                                   | $a_1 \quad -\sqrt{2} \quad 0$                                         |
|                                                   | $a_2 \quad \sqrt{2} \quad 0$                                          |
| $b$ $(\frac{1}{2}, \frac{1}{2}, \frac{t}{2})$     | $\{2_{001}  0 \ 0 \ 0\} \ \{m_{110}  0 \ 0 \ \frac{1}{2}\}$           |
|                                                   | $b_1 \quad 0 \quad 0$                                                 |
| $c$ $(\frac{t}{2}, \frac{t}{2}, 1 - \frac{t}{2})$ | $\{m_{1-10}  0 \ 0 \ \frac{1}{2}\}$                                   |
|                                                   | $c_1 \quad -ie^{-\frac{1}{2}i\pi(2-t)}$                               |
|                                                   | $c_2 \quad ie^{-\frac{1}{2}i\pi(2-t)}$                                |
| $d$ $(\frac{t}{2}, \frac{t}{2}, 0)$               | $\{2_{110}  0 \ 0 \ \frac{1}{2}\} \ \{m_{001}  0 \ 0 \ 0\}$           |
|                                                   | $d_1 \quad 0 \quad 0$                                                 |
| $e$ $(\frac{t}{2}, 1 - \frac{t}{2}, 0)$           | $\{2_{1-10}  0 \ 0 \ \frac{1}{2}\} \ \{m_{001}  0 \ 0 \ 0\}$          |
|                                                   | $e_1 \quad 0 \quad 0$                                                 |
| $f$ $(\frac{1-t}{2}, \frac{1}{2}, \frac{1}{2})$   | $\{2_{100}  0 \ 0 \ \frac{1}{2}\}$                                    |
|                                                   | $f_1 \quad i$                                                         |
|                                                   | $f_2 \quad -i$                                                        |
| $g$ $(0, t, 0)$                                   | $\{2_{010}  0 \ 0 \ \frac{1}{2}\} \ \{m_{100}  0 \ 0 \ \frac{1}{2}\}$ |
|                                                   | $g_1 \quad 0 \quad 0$                                                 |
| $h$ $(0, \frac{t}{2}, 1 - \frac{t}{2})$           | $\{m_{100}  0 \ 0 \ \frac{1}{2}\}$                                    |
|                                                   | $h_1 \quad -ie^{-\frac{1}{2}i\pi(2-t)}$                               |
|                                                   | $h_2 \quad ie^{-\frac{1}{2}i\pi(2-t)}$                                |

$$\mathcal{W}_1^{\text{gapless}} = \sum_{m=1}^{n_{a_1}} \text{sgn}(v_m^{a_1}) \frac{1 - \text{sgn}(\delta_m^{a_1})}{2} + \sum_{m=1}^{n_{a_2}} \text{sgn}(v_m^{a_2}) \frac{1 - \text{sgn}(\delta_m^{a_2})}{2} - \sum_{m=1}^{n_{g_1}} \text{sgn}(v_m^{g_1}) \frac{1 - \text{sgn}(\delta_m^{g_1})}{2} \quad (\text{S140.1})$$

$$\begin{aligned} \mathcal{W}_2^{\text{gapless}} = & \sum_{m=1}^{n_{b_1}} \text{sgn}(v_m^{b_1}) \frac{1 - \text{sgn}(\delta_m^{b_1})}{2} + \sum_{m=1}^{n_{e_1}} \text{sgn}(v_m^{e_1}) \frac{1 - \text{sgn}(\delta_m^{e_1})}{2} + \sum_{m=1}^{n_{f_1}} \text{sgn}(v_m^{f_1}) \frac{1 - \text{sgn}(\delta_m^{f_1})}{2} \\ & + \sum_{m=1}^{n_{f_2}} \text{sgn}(v_m^{f_2}) \frac{1 - \text{sgn}(\delta_m^{f_2})}{2} - \sum_{m=1}^{n_{h_1}} \text{sgn}(v_m^{h_1}) \frac{1 - \text{sgn}(\delta_m^{h_1})}{2} \end{aligned} \quad (\text{S140.2})$$

$$\mathcal{W}_3^{\text{gapless}} = \sum_{m=1}^{n_{c_1}} \text{sgn}(v_m^{c_1}) \frac{1 - \text{sgn}(\delta_m^{c_1})}{2} + \sum_{m=1}^{n_{f_1}} \text{sgn}(v_m^{f_1}) \frac{1 - \text{sgn}(\delta_m^{f_1})}{2} + \sum_{m=1}^{n_{f_2}} \text{sgn}(v_m^{f_2}) \frac{1 - \text{sgn}(\delta_m^{f_2})}{2} - \sum_{m=1}^{n_{h_1}} \text{sgn}(v_m^{h_1}) \frac{1 - \text{sgn}(\delta_m^{h_1})}{2} \quad (\text{S140.3})$$

$$\mathcal{W}_4^{\text{gapless}} = \sum_{m=1}^{n_{d_1}} \text{sgn}(v_m^{d_1}) \frac{1 - \text{sgn}(\delta_m^{d_1})}{2} - \sum_{m=1}^{n_{e_1}} \text{sgn}(v_m^{e_1}) \frac{1 - \text{sgn}(\delta_m^{e_1})}{2} - \sum_{m=1}^{n_{g_1}} \text{sgn}(v_m^{g_1}) \frac{1 - \text{sgn}(\delta_m^{g_1})}{2} \quad (\text{S140.4})$$

$$\mathcal{W}_1^{\text{gapped}} = - \sum_{m=1}^{n_{f_1}} \text{sgn}(v_m^{f_1}) \frac{1 - \text{sgn}(\delta_m^{f_1})}{2} + \sum_{m=1}^{n_{f_2}} \text{sgn}(v_m^{f_2}) \frac{1 - \text{sgn}(\delta_m^{f_2})}{2} \quad (\text{S140.5})$$

## S141. SPACE GROUP NO. 141

| line segment                                          | character of irrep (generators only)                                                       |                               |
|-------------------------------------------------------|--------------------------------------------------------------------------------------------|-------------------------------|
| $a \quad (0, 0, t)$                                   | $\{4_{001}   \frac{1}{4} \frac{3}{4} \frac{1}{4}\} \{m_{100}   0 \ 0 \ 0\}$                |                               |
|                                                       | $a_1 \quad -\sqrt{2}e^{-\frac{1}{2}i\pi t}$                                                | 0                             |
|                                                       | $a_2 \quad \sqrt{2}e^{-\frac{1}{2}i\pi t}$                                                 | 0                             |
| $b \quad (\frac{1}{2}, \frac{1}{2}, \frac{t}{2})$     | $\{2_{001}   0 \ \frac{1}{2} \ 0\} \{m_{110}   \frac{1}{4} \ \frac{3}{4} \ \frac{1}{4}\}$  |                               |
|                                                       | $b_1 \quad i$                                                                              | $-ie^{-\frac{1}{4}i\pi(t+4)}$ |
|                                                       | $b_2 \quad i$                                                                              | $ie^{-\frac{1}{4}i\pi(t+4)}$  |
|                                                       | $b_3 \quad -i$                                                                             | $-ie^{-\frac{1}{4}i\pi(t+4)}$ |
| $c \quad (\frac{t}{2}, \frac{t}{2}, 1 - \frac{t}{2})$ | $\{m_{1-10}   \frac{3}{4} \ \frac{3}{4} \ \frac{1}{4}\}$                                   |                               |
|                                                       | $c_1 \quad -ie^{-\frac{1}{4}i\pi(5t+2)}$                                                   |                               |
|                                                       | $c_2 \quad ie^{-\frac{1}{4}i\pi(5t+2)}$                                                    |                               |
| $d \quad (\frac{t}{2}, \frac{t}{2}, 0)$               | $\{2_{110}   \frac{3}{4} \ \frac{1}{4} \ \frac{3}{4}\} \{m_{001}   0 \ \frac{1}{2} \ 0\}$  |                               |
|                                                       | $d_1 \quad 0$                                                                              | 0                             |
| $e \quad (\frac{t}{2}, 1 - \frac{t}{2}, 0)$           | $\{2_{1-10}   \frac{1}{4} \ \frac{1}{4} \ \frac{3}{4}\} \{m_{001}   0 \ \frac{1}{2} \ 0\}$ |                               |
|                                                       | $e_1 \quad i$                                                                              | $-ie^{-\frac{1}{2}i\pi(2-t)}$ |
|                                                       | $e_2 \quad i$                                                                              | $ie^{-\frac{1}{2}i\pi(2-t)}$  |
|                                                       | $e_3 \quad -i$                                                                             | $-ie^{-\frac{1}{2}i\pi(2-t)}$ |
| $f \quad (\frac{1-t}{2}, \frac{1}{2}, \frac{1}{2})$   | $\{2_{100}   0 \ 0 \ 0\}$                                                                  |                               |
|                                                       | $f_1 \quad -i$                                                                             |                               |
|                                                       | $f_2 \quad i$                                                                              |                               |
| $g \quad (0, t, 0)$                                   | $\{2_{010}   0 \ \frac{1}{2} \ 0\} \{m_{100}   0 \ 0 \ 0\}$                                |                               |
|                                                       | $g_1 \quad 0$                                                                              | 0                             |
| $h \quad (0, \frac{t}{2}, 1 - \frac{t}{2})$           | $\{m_{100}   0 \ 0 \ 0\}$                                                                  |                               |
|                                                       | $h_1 \quad -i$                                                                             |                               |
|                                                       | $h_2 \quad i$                                                                              |                               |

$$\mathcal{W}_1^{\text{gapless}} = \sum_{m=1}^{n_{a_1}} \text{sgn}(v_m^{a_1}) \frac{1 - \text{sgn}(\delta_m^{a_1})}{2} + \sum_{m=1}^{n_{a_2}} \text{sgn}(v_m^{a_2}) \frac{1 - \text{sgn}(\delta_m^{a_2})}{2} - \sum_{m=1}^{n_{g_1}} \text{sgn}(v_m^{g_1}) \frac{1 - \text{sgn}(\delta_m^{g_1})}{2} \quad (\text{S141.1})$$

$$\begin{aligned} \mathcal{W}_2^{\text{gapless}} = & \sum_{m=1}^{n_{b_1}} \text{sgn}(v_m^{b_1}) \frac{1 - \text{sgn}(\delta_m^{b_1})}{2} + \sum_{m=1}^{n_{b_3}} \text{sgn}(v_m^{b_3}) \frac{1 - \text{sgn}(\delta_m^{b_3})}{2} + \sum_{m=1}^{n_{e_1}} \text{sgn}(v_m^{e_1}) \frac{1 - \text{sgn}(\delta_m^{e_1})}{2} \\ & + \sum_{m=1}^{n_{e_3}} \text{sgn}(v_m^{e_3}) \frac{1 - \text{sgn}(\delta_m^{e_3})}{2} + \sum_{m=1}^{n_{f_1}} \text{sgn}(v_m^{f_1}) \frac{1 - \text{sgn}(\delta_m^{f_1})}{2} - \sum_{m=1}^{n_{h_1}} \text{sgn}(v_m^{h_1}) \frac{1 - \text{sgn}(\delta_m^{h_1})}{2} \end{aligned} \quad (\text{S141.2})$$

$$\mathcal{W}_3^{\text{gapless}} = \sum_{m=1}^{n_{c_1}} \text{sgn}(v_m^{c_1}) \frac{1 - \text{sgn}(\delta_m^{c_1})}{2} + \sum_{m=1}^{n_{f_1}} \text{sgn}(v_m^{f_1}) \frac{1 - \text{sgn}(\delta_m^{f_1})}{2} - \sum_{m=1}^{n_{h_1}} \text{sgn}(v_m^{h_1}) \frac{1 - \text{sgn}(\delta_m^{h_1})}{2} \quad (\text{S141.3})$$

$$\mathcal{W}_4^{\text{gapless}} = \sum_{m=1}^{n_{d_1}} \text{sgn}(v_m^{d_1}) \frac{1 - \text{sgn}(\delta_m^{d_1})}{2} - \sum_{m=1}^{n_{e_1}} \text{sgn}(v_m^{e_1}) \frac{1 - \text{sgn}(\delta_m^{e_1})}{2} - \sum_{m=1}^{n_{e_3}} \text{sgn}(v_m^{e_3}) \frac{1 - \text{sgn}(\delta_m^{e_3})}{2} - \sum_{m=1}^{n_{g_1}} \text{sgn}(v_m^{g_1}) \frac{1 - \text{sgn}(\delta_m^{g_1})}{2} \quad (\text{S141.4})$$

$$\mathcal{W}_1^{\text{gapped}} = - \sum_{m=1}^{n_{e_1}} \text{sgn}(v_m^{e_1}) \frac{1 - \text{sgn}(\delta_m^{e_1})}{2} + \sum_{m=1}^{n_{e_3}} \text{sgn}(v_m^{e_3}) \frac{1 - \text{sgn}(\delta_m^{e_3})}{2} \quad (\text{S141.5})$$

## S142. SPACE GROUP NO. 142

| line segment                                          | character of irrep (generators only) |                                                                                                                                    |
|-------------------------------------------------------|--------------------------------------|------------------------------------------------------------------------------------------------------------------------------------|
| $a \quad (0, 0, t)$                                   | $a_1$                                | $\{4_{001}   \frac{1}{4} \frac{3}{4} \frac{1}{4}\} \{m_{100}   0 \ 0 \ \frac{1}{2}\}$<br>$-\sqrt{2}e^{-\frac{1}{2}i\pi t}$<br>$0$  |
|                                                       | $a_2$                                | $\sqrt{2}e^{-\frac{1}{2}i\pi t}$<br>$0$                                                                                            |
| $b \quad (\frac{1}{2}, \frac{1}{2}, \frac{t}{2})$     | $b_1$                                | $\{2_{001}   0 \ \frac{1}{2} \ 0\} \{m_{110}   \frac{3}{4} \ \frac{1}{4} \ \frac{1}{4}\}$<br>$i$<br>$-ie^{-\frac{1}{4}i\pi(t+4)}$  |
|                                                       | $b_2$                                | $i$<br>$ie^{-\frac{1}{4}i\pi(t+4)}$                                                                                                |
|                                                       | $b_3$                                | $-i$<br>$-ie^{-\frac{1}{4}i\pi(t+4)}$                                                                                              |
|                                                       | $b_4$                                | $-i$<br>$ie^{-\frac{1}{4}i\pi(t+4)}$                                                                                               |
| $c \quad (\frac{t}{2}, \frac{t}{2}, 1 - \frac{t}{2})$ | $c_1$                                | $\{m_{1-10}   \frac{1}{4} \ \frac{1}{4} \ \frac{1}{4}\}$<br>$-ie^{-\frac{1}{4}i\pi(t+2)}$                                          |
|                                                       | $c_2$                                | $ie^{-\frac{1}{4}i\pi(t+2)}$                                                                                                       |
| $d \quad (\frac{t}{2}, \frac{t}{2}, 0)$               | $d_1$                                | $\{2_{110}   \frac{3}{4} \ \frac{1}{4} \ \frac{1}{4}\} \{m_{001}   0 \ \frac{1}{2} \ 0\}$<br>$0$<br>$0$                            |
|                                                       | $e_1$                                | $\{2_{1-10}   \frac{1}{4} \ \frac{1}{4} \ \frac{1}{4}\} \{m_{001}   0 \ \frac{1}{2} \ 0\}$<br>$i$<br>$-ie^{-\frac{1}{2}i\pi(2-t)}$ |
| $e \quad (\frac{t}{2}, 1 - \frac{t}{2}, 0)$           | $e_2$                                | $i$<br>$ie^{-\frac{1}{2}i\pi(2-t)}$                                                                                                |
|                                                       | $e_3$                                | $-i$<br>$-ie^{-\frac{1}{2}i\pi(2-t)}$                                                                                              |
|                                                       | $e_4$                                | $-i$<br>$ie^{-\frac{1}{2}i\pi(2-t)}$                                                                                               |
| $f \quad (\frac{1-t}{2}, \frac{1}{2}, \frac{1}{2})$   | $f_1$                                | $\{2_{100}   \frac{1}{2} \ \frac{1}{2} \ 0\}$<br>$-e^{-\frac{1}{2}i\pi(2-t)}$                                                      |
|                                                       | $f_2$                                | $e^{-\frac{1}{2}i\pi(2-t)}$                                                                                                        |
| $g \quad (0, t, 0)$                                   | $g_1$                                | $\{2_{010}   \frac{1}{2} \ 0 \ 0\} \{m_{100}   0 \ 0 \ \frac{1}{2}\}$<br>$0$<br>$0$                                                |
|                                                       | $h_1$                                | $\{m_{100}   0 \ 0 \ \frac{1}{2}\}$<br>$-ie^{-\frac{1}{2}i\pi(2-t)}$                                                               |
| $h \quad (0, \frac{t}{2}, 1 - \frac{t}{2})$           | $h_2$                                | $ie^{-\frac{1}{2}i\pi(2-t)}$                                                                                                       |

$$\mathcal{W}_1^{\text{gapless}} = \sum_{m=1}^{n_{a_1}} \text{sgn}(v_m^{a_1}) \frac{1 - \text{sgn}(\delta_m^{a_1})}{2} + \sum_{m=1}^{n_{a_2}} \text{sgn}(v_m^{a_2}) \frac{1 - \text{sgn}(\delta_m^{a_2})}{2} - \sum_{m=1}^{n_{g_1}} \text{sgn}(v_m^{g_1}) \frac{1 - \text{sgn}(\delta_m^{g_1})}{2} \quad (\text{S142.1})$$

$$\begin{aligned} \mathcal{W}_2^{\text{gapless}} = & \sum_{m=1}^{n_{b_1}} \text{sgn}(v_m^{b_1}) \frac{1 - \text{sgn}(\delta_m^{b_1})}{2} + \sum_{m=1}^{n_{b_3}} \text{sgn}(v_m^{b_3}) \frac{1 - \text{sgn}(\delta_m^{b_3})}{2} + \sum_{m=1}^{n_{e_1}} \text{sgn}(v_m^{e_1}) \frac{1 - \text{sgn}(\delta_m^{e_1})}{2} + \sum_{m=1}^{n_{e_3}} \text{sgn}(v_m^{e_3}) \frac{1 - \text{sgn}(\delta_m^{e_3})}{2} \\ & + \sum_{m=1}^{n_{f_1}} \text{sgn}(v_m^{f_1}) \frac{1 - \text{sgn}(\delta_m^{f_1})}{2} + \sum_{m=1}^{n_{f_2}} \text{sgn}(v_m^{f_2}) \frac{1 - \text{sgn}(\delta_m^{f_2})}{2} - \sum_{m=1}^{n_{h_1}} \text{sgn}(v_m^{h_1}) \frac{1 - \text{sgn}(\delta_m^{h_1})}{2} \end{aligned} \quad (\text{S142.2})$$

$$\mathcal{W}_3^{\text{gapless}} = \sum_{m=1}^{n_{c_1}} \text{sgn}(v_m^{c_1}) \frac{1 - \text{sgn}(\delta_m^{c_1})}{2} + \sum_{m=1}^{n_{f_1}} \text{sgn}(v_m^{f_1}) \frac{1 - \text{sgn}(\delta_m^{f_1})}{2} + \sum_{m=1}^{n_{f_2}} \text{sgn}(v_m^{f_2}) \frac{1 - \text{sgn}(\delta_m^{f_2})}{2} - \sum_{m=1}^{n_{h_1}} \text{sgn}(v_m^{h_1}) \frac{1 - \text{sgn}(\delta_m^{h_1})}{2} \quad (\text{S142.3})$$

$$\mathcal{W}_4^{\text{gapless}} = \sum_{m=1}^{n_{d_1}} \text{sgn}(v_m^{d_1}) \frac{1 - \text{sgn}(\delta_m^{d_1})}{2} - \sum_{m=1}^{n_{e_1}} \text{sgn}(v_m^{e_1}) \frac{1 - \text{sgn}(\delta_m^{e_1})}{2} - \sum_{m=1}^{n_{e_3}} \text{sgn}(v_m^{e_3}) \frac{1 - \text{sgn}(\delta_m^{e_3})}{2} - \sum_{m=1}^{n_{g_1}} \text{sgn}(v_m^{g_1}) \frac{1 - \text{sgn}(\delta_m^{g_1})}{2} \quad (\text{S142.4})$$



$$\mathcal{W}_1^{\text{gapped}} = - \sum_{m=1}^{n_{e_1}} \text{sgn}(v_m^{e_1}) \frac{1 - \text{sgn}(\delta_m^{e_1})}{2} + \sum_{m=1}^{n_{e_3}} \text{sgn}(v_m^{e_3}) \frac{1 - \text{sgn}(\delta_m^{e_3})}{2} \quad (\text{S142.5})$$

$$\mathcal{X}_1 = \sum_{m=1}^{n_{h_1}} \frac{1 - \text{sgn}(\delta_m^{h_1})}{2} \mod 2 \quad (\text{S142.6})$$

### S143. SPACE GROUP NO. 143

| line segment                                          | character of irrep (generators only)                                                                             |
|-------------------------------------------------------|------------------------------------------------------------------------------------------------------------------|
| $a \quad (0, 0, \frac{t}{2})$                         | $\{3_{001}   0 \ 0 \ 0\}$<br>$a_1 \quad -1$<br>$a_2 \quad e^{-\frac{i\pi}{3}}$<br>$a_3 \quad e^{\frac{i\pi}{3}}$ |
| $b \quad (\frac{1}{3}, \frac{1}{3}, \frac{1}{2} - t)$ | $\{3_{001}   0 \ 0 \ 0\}$<br>$b_1 \quad -1$<br>$b_2 \quad e^{-\frac{i\pi}{3}}$<br>$b_3 \quad e^{\frac{i\pi}{3}}$ |
| $c \quad (\frac{1}{2}, 0, \frac{t}{2})$               | $\{1   0 \ 0 \ 0\}$<br>$c_1 \quad 1$                                                                             |
| $d \quad (\frac{2t}{3}, -\frac{t}{3}, \frac{1}{2})$   | $\{1   0 \ 0 \ 0\}$<br>$d_1 \quad 1$                                                                             |
| $e \quad (\frac{t+2}{6}, \frac{1-t}{3}, \frac{1}{2})$ | $\{1   0 \ 0 \ 0\}$<br>$e_1 \quad 1$                                                                             |

$$\mathcal{W}_1^{\text{gapless}} = \sum_{m=1}^{n_{b_1}} \text{sgn}(v_m^{b_1}) \frac{1 - \text{sgn}(\delta_m^{b_1})}{2} + \sum_{m=1}^{n_{b_2}} \text{sgn}(v_m^{b_2}) \frac{1 - \text{sgn}(\delta_m^{b_2})}{2} + \sum_{m=1}^{n_{b_3}} \text{sgn}(v_m^{b_3}) \frac{1 - \text{sgn}(\delta_m^{b_3})}{2} \quad (\text{S143.1})$$

$$\mathcal{W}_1^{\text{gapped}} = \sum_{m=1}^{n_{a_2}} \text{sgn}(v_m^{a_2}) \frac{1 - \text{sgn}(\delta_m^{a_2})}{2} - \sum_{m=1}^{n_{a_3}} \text{sgn}(v_m^{a_3}) \frac{1 - \text{sgn}(\delta_m^{a_3})}{2} \quad (\text{S143.2})$$

$$\mathcal{W}_2^{\text{gapped}} = \sum_{m=1}^{n_{b_2}} \text{sgn}(v_m^{b_2}) \frac{1 - \text{sgn}(\delta_m^{b_2})}{2} \quad (\text{S143.3})$$

$$\mathcal{W}_3^{\text{gapped}} = \sum_{m=1}^{n_{b_3}} \text{sgn}(v_m^{b_3}) \frac{1 - \text{sgn}(\delta_m^{b_3})}{2} \quad (\text{S143.4})$$

$$\mathcal{X}_1 = \sum_{m=1}^{n_{a_1}} \frac{1 - \text{sgn}(\delta_m^{a_1})}{2} + \sum_{m=1}^{n_{c_1}} \frac{1 - \text{sgn}(\delta_m^{c_1})}{2} + \sum_{m=1}^{n_{d_1}} \frac{1 - \text{sgn}(\delta_m^{d_1})}{2} + \sum_{m=1}^{n_{e_1}} \frac{1 - \text{sgn}(\delta_m^{e_1})}{2} \mod 2 \quad (\text{S143.5})$$

$$\mathcal{X}_2 = \sum_{m=1}^{n_{a_1}} \frac{1 - \text{sgn}(\delta_m^{a_1})}{2} \mod 2 \quad (\text{S143.6})$$

$$\mathcal{X}_3 = \sum_{m=1}^{n_{a_1}} \frac{1 - \text{sgn}(\delta_m^{a_1})}{2} + \sum_{m=1}^{n_{d_1}} \frac{1 - \text{sgn}(\delta_m^{d_1})}{2} + \sum_{m=1}^{n_{e_1}} \frac{1 - \text{sgn}(\delta_m^{e_1})}{2} \mod 2 \quad (\text{S143.7})$$

#### S144. SPACE GROUP NO. 144

| line segment                                          | character of irrep (generators only)                                                                                                                                                                |
|-------------------------------------------------------|-----------------------------------------------------------------------------------------------------------------------------------------------------------------------------------------------------|
| $a \quad (0, 0, \frac{t}{2})$                         | $\{3_{001}   0 \ 0 \ \frac{1}{3}\}$<br>$a_1 \quad -e^{-\frac{1}{3}i\pi t}$<br>$a_2 \quad e^{-\frac{1}{3}i\pi t - \frac{i\pi}{3}}$<br>$a_3 \quad e^{\frac{i\pi}{3} - \frac{i\pi t}{3}}$              |
| $b \quad (\frac{1}{3}, \frac{1}{3}, \frac{1}{2} - t)$ | $\{3_{001}   0 \ 0 \ \frac{1}{3}\}$<br>$b_1 \quad -e^{-\frac{1}{3}i\pi(1-2t)}$<br>$b_2 \quad e^{-\frac{1}{3}i\pi(1-2t) - \frac{i\pi}{3}}$<br>$b_3 \quad e^{\frac{i\pi}{3} - \frac{1}{3}i\pi(1-2t)}$ |
| $c \quad (\frac{1}{2}, 0, \frac{t}{2})$               | $\{1   0 \ 0 \ 0\}$<br>$c_1 \quad 1$                                                                                                                                                                |
| $d \quad (\frac{2t}{3}, -\frac{t}{3}, \frac{1}{2})$   | $\{1   0 \ 0 \ 0\}$<br>$d_1 \quad 1$                                                                                                                                                                |
| $e \quad (\frac{t+2}{6}, \frac{1-t}{3}, \frac{1}{2})$ | $\{1   0 \ 0 \ 0\}$<br>$e_1 \quad 1$                                                                                                                                                                |

$$\mathcal{W}_1^{\text{gapless}} = \sum_{m=1}^{n_{b_1}} \text{sgn}(v_m^{b_1}) \frac{1 - \text{sgn}(\delta_m^{b_1})}{2} + \sum_{m=1}^{n_{b_2}} \text{sgn}(v_m^{b_2}) \frac{1 - \text{sgn}(\delta_m^{b_2})}{2} + \sum_{m=1}^{n_{b_3}} \text{sgn}(v_m^{b_3}) \frac{1 - \text{sgn}(\delta_m^{b_3})}{2} \quad (\text{S144.1})$$

$$\mathcal{X}_1 = \sum_{m=1}^{n_{d_1}} \frac{1 - \text{sgn}(\delta_m^{d_1})}{2} + \sum_{m=1}^{n_{e_1}} \frac{1 - \text{sgn}(\delta_m^{e_1})}{2} \mod 2 \quad (\text{S144.2})$$

$$\mathcal{X}_2 = \sum_{m=1}^{n_{c_1}} \frac{1 - \text{sgn}(\delta_m^{c_1})}{2} + \sum_{m=1}^{n_{d_1}} \frac{1 - \text{sgn}(\delta_m^{d_1})}{2} + \sum_{m=1}^{n_{e_1}} \frac{1 - \text{sgn}(\delta_m^{e_1})}{2} \mod 2 \quad (\text{S144.3})$$

$$\begin{aligned} \mathcal{X}_3 = & 3 \sum_{m=1}^{n_{a_1}} \text{sgn}(v_m^{a_1}) \frac{1 - \text{sgn}(\delta_m^{a_1})}{2} + \sum_{m=1}^{n_{a_2}} \text{sgn}(v_m^{a_2}) \frac{1 - \text{sgn}(\delta_m^{a_2})}{2} - \sum_{m=1}^{n_{a_3}} \text{sgn}(v_m^{a_3}) \frac{1 - \text{sgn}(\delta_m^{a_3})}{2} \\ & + 8 \sum_{m=1}^{n_{b_2}} \text{sgn}(v_m^{b_2}) \frac{1 - \text{sgn}(\delta_m^{b_2})}{2} - 2 \sum_{m=1}^{n_{b_3}} \text{sgn}(v_m^{b_3}) \frac{1 - \text{sgn}(\delta_m^{b_3})}{2} + 2 \sum_{m=1}^{n_{d_1}} \text{sgn}(v_m^{d_1}) \frac{1 - \text{sgn}(\delta_m^{d_1})}{2} \mod 6 \end{aligned} \quad (\text{S144.4})$$

**S145. SPACE GROUP NO. 145**

| line segment                                          | character of irrep (generators only)                                                                                                                                                                |
|-------------------------------------------------------|-----------------------------------------------------------------------------------------------------------------------------------------------------------------------------------------------------|
| $a \quad (0, 0, \frac{t}{2})$                         | $\{3_{001}   0 \ 0 \ \frac{2}{3}\}$<br>$a_1 \quad -e^{-\frac{2}{3}i\pi t}$<br>$a_2 \quad e^{-\frac{2}{3}i\pi t - \frac{i\pi}{3}}$<br>$a_3 \quad e^{\frac{i\pi}{3} - \frac{2i\pi t}{3}}$             |
| $b \quad (\frac{1}{3}, \frac{1}{3}, \frac{1}{2} - t)$ | $\{3_{001}   0 \ 0 \ \frac{2}{3}\}$<br>$b_1 \quad -e^{-\frac{2}{3}i\pi(1-2t)}$<br>$b_2 \quad e^{-\frac{2}{3}i\pi(1-2t) - \frac{i\pi}{3}}$<br>$b_3 \quad e^{\frac{i\pi}{3} - \frac{2}{3}i\pi(1-2t)}$ |
| $c \quad (\frac{1}{2}, 0, \frac{t}{2})$               | $\{1   0 \ 0 \ 0\}$<br>$c_1 \quad 1$                                                                                                                                                                |
| $d \quad (\frac{2t}{3}, -\frac{t}{3}, \frac{1}{2})$   | $\{1   0 \ 0 \ 0\}$<br>$d_1 \quad 1$                                                                                                                                                                |
| $e \quad (\frac{t+2}{6}, \frac{1-t}{3}, \frac{1}{2})$ | $\{1   0 \ 0 \ 0\}$<br>$e_1 \quad 1$                                                                                                                                                                |

$$\mathcal{W}_1^{\text{gapless}} = \sum_{m=1}^{n_{b_1}} \text{sgn}(v_m^{b_1}) \frac{1 - \text{sgn}(\delta_m^{b_1})}{2} + \sum_{m=1}^{n_{b_2}} \text{sgn}(v_m^{b_2}) \frac{1 - \text{sgn}(\delta_m^{b_2})}{2} + \sum_{m=1}^{n_{b_3}} \text{sgn}(v_m^{b_3}) \frac{1 - \text{sgn}(\delta_m^{b_3})}{2} \quad (\text{S145.1})$$

$$\mathcal{X}_1 = \sum_{m=1}^{n_{d_1}} \frac{1 - \text{sgn}(\delta_m^{d_1})}{2} + \sum_{m=1}^{n_{e_1}} \frac{1 - \text{sgn}(\delta_m^{e_1})}{2} \quad \text{mod } 2 \quad (\text{S145.2})$$

$$\mathcal{X}_2 = \sum_{m=1}^{n_{c_1}} \frac{1 - \text{sgn}(\delta_m^{c_1})}{2} + \sum_{m=1}^{n_{d_1}} \frac{1 - \text{sgn}(\delta_m^{d_1})}{2} + \sum_{m=1}^{n_{e_1}} \frac{1 - \text{sgn}(\delta_m^{e_1})}{2} \quad \text{mod } 2 \quad (\text{S145.3})$$

$$\begin{aligned} \mathcal{X}_3 = & 3 \sum_{m=1}^{n_{a_1}} \text{sgn}(v_m^{a_1}) \frac{1 - \text{sgn}(\delta_m^{a_1})}{2} - \sum_{m=1}^{n_{a_2}} \text{sgn}(v_m^{a_2}) \frac{1 - \text{sgn}(\delta_m^{a_2})}{2} + \sum_{m=1}^{n_{a_3}} \text{sgn}(v_m^{a_3}) \frac{1 - \text{sgn}(\delta_m^{a_3})}{2} \\ & - 2 \sum_{m=1}^{n_{b_2}} \text{sgn}(v_m^{b_2}) \frac{1 - \text{sgn}(\delta_m^{b_2})}{2} - 10 \sum_{m=1}^{n_{b_3}} \text{sgn}(v_m^{b_3}) \frac{1 - \text{sgn}(\delta_m^{b_3})}{2} + 2 \sum_{m=1}^{n_{d_1}} \text{sgn}(v_m^{d_1}) \frac{1 - \text{sgn}(\delta_m^{d_1})}{2} \quad \text{mod } 6 \end{aligned} \quad (\text{S145.4})$$

**S146. SPACE GROUP NO. 146**

| line segment                                         | character of irrep (generators only)                                                                             |
|------------------------------------------------------|------------------------------------------------------------------------------------------------------------------|
| $a \quad (0, 0, \frac{3t}{2})$                       | $\{3_{001}   0 \ 0 \ 0\}$<br>$a_1 \quad -1$<br>$a_2 \quad e^{-\frac{i\pi}{3}}$<br>$a_3 \quad e^{\frac{i\pi}{3}}$ |
| $b \quad (\frac{t}{2}, -\frac{t}{2}, \frac{3-t}{2})$ | $\{1   0 \ 0 \ 0\}$<br>$b_1 \quad 1$                                                                             |
| $c \quad (\frac{t}{2}, 0, \frac{3}{2} - t)$          | $\{1   0 \ 0 \ 0\}$<br>$c_1 \quad 1$                                                                             |

|                                |                                                                |
|--------------------------------|----------------------------------------------------------------|
| $d \quad (t, -t, \frac{t}{2})$ | $\begin{array}{c} \{1  0 \ 0 \ 0\} \\ d_1 \quad 1 \end{array}$ |
|--------------------------------|----------------------------------------------------------------|

$$\mathcal{W}_1^{\text{gapless}} = \sum_{m=1}^{n_{a_1}} \text{sgn}(v_m^{a_1}) \frac{1 - \text{sgn}(\delta_m^{a_1})}{2} + \sum_{m=1}^{n_{a_2}} \text{sgn}(v_m^{a_2}) \frac{1 - \text{sgn}(\delta_m^{a_2})}{2} + \sum_{m=1}^{n_{a_3}} \text{sgn}(v_m^{a_3}) \frac{1 - \text{sgn}(\delta_m^{a_3})}{2} - \sum_{m=1}^{n_{d_1}} \text{sgn}(v_m^{d_1}) \frac{1 - \text{sgn}(\delta_m^{d_1})}{2} \quad (\text{S146.1})$$

$$\mathcal{W}_1^{\text{gapped}} = \sum_{m=1}^{n_{a_2}} \text{sgn}(v_m^{a_2}) \frac{1 - \text{sgn}(\delta_m^{a_2})}{2} - \sum_{m=1}^{n_{a_3}} \text{sgn}(v_m^{a_3}) \frac{1 - \text{sgn}(\delta_m^{a_3})}{2} \quad (\text{S146.2})$$

$$\mathcal{X}_1 = \sum_{m=1}^{n_{b_1}} \frac{1 - \text{sgn}(\delta_m^{b_1})}{2} + \sum_{m=1}^{n_{d_1}} \frac{1 - \text{sgn}(\delta_m^{d_1})}{2} \quad \text{mod } 2 \quad (\text{S146.3})$$

$$\mathcal{X}_2 = \sum_{m=1}^{n_{d_1}} \frac{1 - \text{sgn}(\delta_m^{d_1})}{2} \quad \text{mod } 2 \quad (\text{S146.4})$$

$$\mathcal{X}_3 = \sum_{m=1}^{n_{c_1}} \frac{1 - \text{sgn}(\delta_m^{c_1})}{2} + \sum_{m=1}^{n_{d_1}} \frac{1 - \text{sgn}(\delta_m^{d_1})}{2} \quad \text{mod } 2 \quad (\text{S146.5})$$

#### S147. SPACE GROUP NO. 147

| line segment                                          | character of irrep (generators only)                                                                                                   |
|-------------------------------------------------------|----------------------------------------------------------------------------------------------------------------------------------------|
| $a \quad (0, 0, \frac{t}{2})$                         | $\begin{array}{c} \{3_{001}  0 \ 0 \ 0\} \\ a_1 \quad -1 \\ a_2 \quad e^{-\frac{i\pi}{3}} \\ a_3 \quad e^{\frac{i\pi}{3}} \end{array}$ |
| $b \quad (\frac{1}{3}, \frac{1}{3}, \frac{1}{2} - t)$ | $\begin{array}{c} \{3_{001}  0 \ 0 \ 0\} \\ b_1 \quad -1 \\ b_2 \quad e^{-\frac{i\pi}{3}} \\ b_3 \quad e^{\frac{i\pi}{3}} \end{array}$ |
| $c \quad (\frac{1}{2}, 0, \frac{t}{2})$               | $\begin{array}{c} \{1  0 \ 0 \ 0\} \\ c_1 \quad 1 \end{array}$                                                                         |
| $d \quad (\frac{2t}{3}, -\frac{t}{3}, \frac{1}{2})$   | $\begin{array}{c} \{1  0 \ 0 \ 0\} \\ d_1 \quad 1 \end{array}$                                                                         |
| $e \quad (\frac{t+2}{6}, \frac{1-t}{3}, \frac{1}{2})$ | $\begin{array}{c} \{1  0 \ 0 \ 0\} \\ e_1 \quad 1 \end{array}$                                                                         |

$$\mathcal{W}_1^{\text{gapless}} = \sum_{m=1}^{n_{b_1}} \text{sgn}(v_m^{b_1}) \frac{1 - \text{sgn}(\delta_m^{b_1})}{2} + \sum_{m=1}^{n_{b_2}} \text{sgn}(v_m^{b_2}) \frac{1 - \text{sgn}(\delta_m^{b_2})}{2} \quad (\text{S147.1})$$

$$\mathcal{W}_1^{\text{gapped}} = \sum_{m=1}^{n_{b_2}} \text{sgn}(v_m^{b_2}) \frac{1 - \text{sgn}(\delta_m^{b_2})}{2} \quad (\text{S147.2})$$

**S148. SPACE GROUP NO. 148**

| line segment                                     | character of irrep (generators only)                                                                              |
|--------------------------------------------------|-------------------------------------------------------------------------------------------------------------------|
| $a \ (0, 0, \frac{3t}{2})$                       | $\{3_{001}   0 \ 0 \ 0 \}$<br>$a_1 \quad -1$<br>$a_2 \quad e^{-\frac{i\pi}{3}}$<br>$a_3 \quad e^{\frac{i\pi}{3}}$ |
| $b \ (\frac{t}{2}, -\frac{t}{2}, \frac{3-t}{2})$ | $\{1   0 \ 0 \ 0 \}$<br>$b_1 \quad 1$                                                                             |
| $c \ (\frac{t}{2}, 0, \frac{3}{2} - t)$          | $\{1   0 \ 0 \ 0 \}$<br>$c_1 \quad 1$                                                                             |
| $d \ (t, -t, \frac{t}{2})$                       | $\{1   0 \ 0 \ 0 \}$<br>$d_1 \quad 1$                                                                             |

$$\mathcal{W}_1^{\text{gapless}} = \sum_{m=1}^{n_{a_1}} \text{sgn}(v_m^{a_1}) \frac{1 - \text{sgn}(\delta_m^{a_1})}{2} + \sum_{m=1}^{n_{a_2}} \text{sgn}(v_m^{a_2}) \frac{1 - \text{sgn}(\delta_m^{a_2})}{2} - \sum_{m=1}^{n_{d_1}} \text{sgn}(v_m^{d_1}) \frac{1 - \text{sgn}(\delta_m^{d_1})}{2} \quad (\text{S148.1})$$

**S149. SPACE GROUP NO. 149**

| line segment                                      | character of irrep (generators only)                                                                              |
|---------------------------------------------------|-------------------------------------------------------------------------------------------------------------------|
| $a \ (0, 0, \frac{t}{2})$                         | $\{3_{001}   0 \ 0 \ 0 \}$<br>$a_1 \quad -1$<br>$a_2 \quad e^{-\frac{i\pi}{3}}$<br>$a_3 \quad e^{\frac{i\pi}{3}}$ |
| $b \ (\frac{1}{3}, \frac{1}{3}, \frac{1-t}{2})$   | $\{3_{001}   0 \ 0 \ 0 \}$<br>$b_1 \quad -1$<br>$b_2 \quad e^{-\frac{i\pi}{3}}$<br>$b_3 \quad e^{\frac{i\pi}{3}}$ |
| $c \ (\frac{1}{3}, \frac{1}{3}, \frac{t-1}{2})$   | $\{3_{001}   0 \ 0 \ 0 \}$<br>$c_1 \quad -1$<br>$c_2 \quad e^{-\frac{i\pi}{3}}$<br>$c_3 \quad e^{\frac{i\pi}{3}}$ |
| $d \ (\frac{1}{2}, 0, \frac{t}{2})$               | $\{1   0 \ 0 \ 0 \}$<br>$d_1 \quad 1$                                                                             |
| $e \ (\frac{t}{2}, 0, 0)$                         | $\{2_{210}   0 \ 0 \ 0 \}$<br>$e_1 \quad -i$<br>$e_2 \quad i$                                                     |
| $f \ (\frac{t}{2}, 0, \frac{1}{2})$               | $\{2_{210}   0 \ 0 \ 0 \}$<br>$f_1 \quad -i$<br>$f_2 \quad i$                                                     |
| $g \ (\frac{t}{3}, \frac{t}{3}, \frac{1}{2})$     | $\{1   0 \ 0 \ 0 \}$<br>$g_1 \quad 1$                                                                             |
| $h \ (\frac{t+2}{6}, \frac{1-t}{3}, \frac{1}{2})$ | $\{1   0 \ 0 \ 0 \}$<br>$h_1 \quad 1$                                                                             |

$$\begin{aligned}
\mathcal{W}_1^{\text{gapless}} = & \sum_{m=1}^{n_{a_1}} \text{sgn}(v_m^{a_1}) \frac{1 - \text{sgn}(\delta_m^{a_1})}{2} + \sum_{m=1}^{n_{a_2}} \text{sgn}(v_m^{a_2}) \frac{1 - \text{sgn}(\delta_m^{a_2})}{2} + \sum_{m=1}^{n_{a_3}} \text{sgn}(v_m^{a_3}) \frac{1 - \text{sgn}(\delta_m^{a_3})}{2} \\
& - \sum_{m=1}^{n_{d_1}} \text{sgn}(v_m^{d_1}) \frac{1 - \text{sgn}(\delta_m^{d_1})}{2} - \sum_{m=1}^{n_{e_1}} \text{sgn}(v_m^{e_1}) \frac{1 - \text{sgn}(\delta_m^{e_1})}{2} - \sum_{m=1}^{n_{e_2}} \text{sgn}(v_m^{e_2}) \frac{1 - \text{sgn}(\delta_m^{e_2})}{2} \\
& + \sum_{m=1}^{n_{g_1}} \text{sgn}(v_m^{g_1}) \frac{1 - \text{sgn}(\delta_m^{g_1})}{2} + \sum_{m=1}^{n_{h_1}} \text{sgn}(v_m^{h_1}) \frac{1 - \text{sgn}(\delta_m^{h_1})}{2}
\end{aligned} \tag{S149.1}$$

$$\begin{aligned}
\mathcal{W}_2^{\text{gapless}} = & \sum_{m=1}^{n_{b_1}} \text{sgn}(v_m^{b_1}) \frac{1 - \text{sgn}(\delta_m^{b_1})}{2} + \sum_{m=1}^{n_{b_2}} \text{sgn}(v_m^{b_2}) \frac{1 - \text{sgn}(\delta_m^{b_2})}{2} + \sum_{m=1}^{n_{b_3}} \text{sgn}(v_m^{b_3}) \frac{1 - \text{sgn}(\delta_m^{b_3})}{2} \\
& - \sum_{m=1}^{n_{c_1}} \text{sgn}(v_m^{c_1}) \frac{1 - \text{sgn}(\delta_m^{c_1})}{2} - \sum_{m=1}^{n_{c_2}} \text{sgn}(v_m^{c_2}) \frac{1 - \text{sgn}(\delta_m^{c_2})}{2} - \sum_{m=1}^{n_{c_3}} \text{sgn}(v_m^{c_3}) \frac{1 - \text{sgn}(\delta_m^{c_3})}{2}
\end{aligned} \tag{S149.2}$$

$$\begin{aligned}
\mathcal{W}_3^{\text{gapless}} = & \sum_{m=1}^{n_{f_1}} \text{sgn}(v_m^{f_1}) \frac{1 - \text{sgn}(\delta_m^{f_1})}{2} + \sum_{m=1}^{n_{f_2}} \text{sgn}(v_m^{f_2}) \frac{1 - \text{sgn}(\delta_m^{f_2})}{2} - \sum_{m=1}^{n_{g_1}} \text{sgn}(v_m^{g_1}) \frac{1 - \text{sgn}(\delta_m^{g_1})}{2} - \sum_{m=1}^{n_{h_1}} \text{sgn}(v_m^{h_1}) \frac{1 - \text{sgn}(\delta_m^{h_1})}{2}
\end{aligned} \tag{S149.3}$$

$$\mathcal{W}_1^{\text{gapped}} = - \sum_{m=1}^{n_{e_1}} \text{sgn}(v_m^{e_1}) \frac{1 - \text{sgn}(\delta_m^{e_1})}{2} + \sum_{m=1}^{n_{e_2}} \text{sgn}(v_m^{e_2}) \frac{1 - \text{sgn}(\delta_m^{e_2})}{2} \tag{S149.4}$$

$$\mathcal{W}_2^{\text{gapped}} = - \sum_{m=1}^{n_{a_2}} \text{sgn}(v_m^{a_2}) \frac{1 - \text{sgn}(\delta_m^{a_2})}{2} + \sum_{m=1}^{n_{a_3}} \text{sgn}(v_m^{a_3}) \frac{1 - \text{sgn}(\delta_m^{a_3})}{2} \tag{S149.5}$$

$$\mathcal{W}_3^{\text{gapped}} = \sum_{m=1}^{n_{b_3}} \text{sgn}(v_m^{b_3}) \frac{1 - \text{sgn}(\delta_m^{b_3})}{2} - \sum_{m=1}^{n_{c_3}} \text{sgn}(v_m^{c_3}) \frac{1 - \text{sgn}(\delta_m^{c_3})}{2} \tag{S149.6}$$

$$\mathcal{W}_4^{\text{gapped}} = \sum_{m=1}^{n_{b_2}} \text{sgn}(v_m^{b_2}) \frac{1 - \text{sgn}(\delta_m^{b_2})}{2} - \sum_{m=1}^{n_{c_2}} \text{sgn}(v_m^{c_2}) \frac{1 - \text{sgn}(\delta_m^{c_2})}{2} \tag{S149.7}$$

$$\mathcal{W}_5^{\text{gapped}} = -2 \sum_{m=1}^{n_{f_2}} \text{sgn}(v_m^{f_2}) \frac{1 - \text{sgn}(\delta_m^{f_2})}{2} + \sum_{m=1}^{n_{g_1}} \text{sgn}(v_m^{g_1}) \frac{1 - \text{sgn}(\delta_m^{g_1})}{2} + \sum_{m=1}^{n_{h_1}} \text{sgn}(v_m^{h_1}) \frac{1 - \text{sgn}(\delta_m^{h_1})}{2} \tag{S149.8}$$

$$\mathcal{X}_1 = \sum_{m=1}^{n_{d_1}} \frac{1 - \text{sgn}(\delta_m^{d_1})}{2} \mod 2 \tag{S149.9}$$

## S150. SPACE GROUP NO. 150

| line segment                                          | character of irrep (generators only)                                                                             |
|-------------------------------------------------------|------------------------------------------------------------------------------------------------------------------|
| $a \quad (0, 0, \frac{t}{2})$                         | $\{3_{001}   0 \ 0 \ 0\}$<br>$a_1 \quad -1$<br>$a_2 \quad e^{-\frac{i\pi}{3}}$<br>$a_3 \quad e^{\frac{i\pi}{3}}$ |
| $b \quad (\frac{1}{3}, \frac{1}{3}, \frac{1-t}{2})$   | $\{3_{001}   0 \ 0 \ 0\}$<br>$b_1 \quad -1$<br>$b_2 \quad e^{-\frac{i\pi}{3}}$<br>$b_3 \quad e^{\frac{i\pi}{3}}$ |
| $c \quad (\frac{1}{2}, 0, \frac{t}{2})$               | $\{1   0 \ 0 \ 0\}$<br>$c_1 \quad 1$                                                                             |
| $d \quad (\frac{t}{3}, \frac{t}{3}, 0)$               | $\{2_{110}   0 \ 0 \ 0\}$<br>$d_1 \quad -i$<br>$d_2 \quad i$                                                     |
| $e \quad (\frac{t}{3}, \frac{t}{3}, \frac{1}{2})$     | $\{2_{110}   0 \ 0 \ 0\}$<br>$e_1 \quad -i$<br>$e_2 \quad i$                                                     |
| $f \quad (\frac{t}{2}, 0, \frac{1}{2})$               | $\{1   0 \ 0 \ 0\}$<br>$f_1 \quad 1$                                                                             |
| $g \quad (\frac{t+2}{6}, \frac{1-t}{3}, 0)$           | $\{2_{010}   0 \ 0 \ 0\}$<br>$g_1 \quad -i$<br>$g_2 \quad i$                                                     |
| $h \quad (\frac{t+2}{6}, \frac{1-t}{3}, \frac{1}{2})$ | $\{2_{010}   0 \ 0 \ 0\}$<br>$h_1 \quad -i$<br>$h_2 \quad i$                                                     |

$$\begin{aligned}
\mathcal{W}_1^{\text{gapless}} = & \sum_{m=1}^{n_{a_1}} \text{sgn}(v_m^{a_1}) \frac{1 - \text{sgn}(\delta_m^{a_1})}{2} + \sum_{m=1}^{n_{a_2}} \text{sgn}(v_m^{a_2}) \frac{1 - \text{sgn}(\delta_m^{a_2})}{2} + \sum_{m=1}^{n_{a_3}} \text{sgn}(v_m^{a_3}) \frac{1 - \text{sgn}(\delta_m^{a_3})}{2} \\
& - \sum_{m=1}^{n_{c_1}} \text{sgn}(v_m^{c_1}) \frac{1 - \text{sgn}(\delta_m^{c_1})}{2} - \sum_{m=1}^{n_{d_1}} \text{sgn}(v_m^{d_1}) \frac{1 - \text{sgn}(\delta_m^{d_1})}{2} - \sum_{m=1}^{n_{d_2}} \text{sgn}(v_m^{d_2}) \frac{1 - \text{sgn}(\delta_m^{d_2})}{2} \\
& + \sum_{m=1}^{n_{f_1}} \text{sgn}(v_m^{f_1}) \frac{1 - \text{sgn}(\delta_m^{f_1})}{2} - \sum_{m=1}^{n_{g_1}} \text{sgn}(v_m^{g_1}) \frac{1 - \text{sgn}(\delta_m^{g_1})}{2} - \sum_{m=1}^{n_{g_2}} \text{sgn}(v_m^{g_2}) \frac{1 - \text{sgn}(\delta_m^{g_2})}{2}
\end{aligned} \tag{S150.1}$$

$$\begin{aligned}
\mathcal{W}_2^{\text{gapless}} = & \sum_{m=1}^{n_{b_1}} \text{sgn}(v_m^{b_1}) \frac{1 - \text{sgn}(\delta_m^{b_1})}{2} + \sum_{m=1}^{n_{b_2}} \text{sgn}(v_m^{b_2}) \frac{1 - \text{sgn}(\delta_m^{b_2})}{2} + \sum_{m=1}^{n_{b_3}} \text{sgn}(v_m^{b_3}) \frac{1 - \text{sgn}(\delta_m^{b_3})}{2} \\
& + \sum_{m=1}^{n_{c_1}} \text{sgn}(v_m^{c_1}) \frac{1 - \text{sgn}(\delta_m^{c_1})}{2} + \sum_{m=1}^{n_{g_1}} \text{sgn}(v_m^{g_1}) \frac{1 - \text{sgn}(\delta_m^{g_1})}{2} + \sum_{m=1}^{n_{g_2}} \text{sgn}(v_m^{g_2}) \frac{1 - \text{sgn}(\delta_m^{g_2})}{2} \\
& - \sum_{m=1}^{n_{h_1}} \text{sgn}(v_m^{h_1}) \frac{1 - \text{sgn}(\delta_m^{h_1})}{2} - \sum_{m=1}^{n_{h_2}} \text{sgn}(v_m^{h_2}) \frac{1 - \text{sgn}(\delta_m^{h_2})}{2}
\end{aligned} \tag{S150.2}$$

$$\begin{aligned}
\mathcal{W}_3^{\text{gapless}} = & \sum_{m=1}^{n_{e_1}} \text{sgn}(v_m^{e_1}) \frac{1 - \text{sgn}(\delta_m^{e_1})}{2} + \sum_{m=1}^{n_{e_2}} \text{sgn}(v_m^{e_2}) \frac{1 - \text{sgn}(\delta_m^{e_2})}{2} - \sum_{m=1}^{n_{f_1}} \text{sgn}(v_m^{f_1}) \frac{1 - \text{sgn}(\delta_m^{f_1})}{2} \\
& + \sum_{m=1}^{n_{h_1}} \text{sgn}(v_m^{h_1}) \frac{1 - \text{sgn}(\delta_m^{h_1})}{2} + \sum_{m=1}^{n_{h_2}} \text{sgn}(v_m^{h_2}) \frac{1 - \text{sgn}(\delta_m^{h_2})}{2}
\end{aligned} \tag{S150.3}$$

$$\mathcal{W}_1^{\text{gapped}} = \sum_{m=1}^{n_{b_2}} \text{sgn}(v_m^{b_2}) \frac{1 - \text{sgn}(\delta_m^{b_2})}{2} - \sum_{m=1}^{n_{b_3}} \text{sgn}(v_m^{b_3}) \frac{1 - \text{sgn}(\delta_m^{b_3})}{2} \quad (\text{S150.4})$$

$$\begin{aligned} \mathcal{W}_2^{\text{gapped}} = & - \sum_{m=1}^{n_{d_1}} \text{sgn}(v_m^{d_1}) \frac{1 - \text{sgn}(\delta_m^{d_1})}{2} + \sum_{m=1}^{n_{d_2}} \text{sgn}(v_m^{d_2}) \frac{1 - \text{sgn}(\delta_m^{d_2})}{2} - \sum_{m=1}^{n_{g_1}} \text{sgn}(v_m^{g_1}) \frac{1 - \text{sgn}(\delta_m^{g_1})}{2} \\ & + \sum_{m=1}^{n_{g_2}} \text{sgn}(v_m^{g_2}) \frac{1 - \text{sgn}(\delta_m^{g_2})}{2} \end{aligned} \quad (\text{S150.5})$$

$$\mathcal{W}_3^{\text{gapped}} = - \sum_{m=1}^{n_{a_2}} \text{sgn}(v_m^{a_2}) \frac{1 - \text{sgn}(\delta_m^{a_2})}{2} + \sum_{m=1}^{n_{a_3}} \text{sgn}(v_m^{a_3}) \frac{1 - \text{sgn}(\delta_m^{a_3})}{2} \quad (\text{S150.6})$$

$$\mathcal{W}_4^{\text{gapped}} = 2 \sum_{m=1}^{n_{e_2}} \text{sgn}(v_m^{e_2}) \frac{1 - \text{sgn}(\delta_m^{e_2})}{2} - \sum_{m=1}^{n_{f_1}} \text{sgn}(v_m^{f_1}) \frac{1 - \text{sgn}(\delta_m^{f_1})}{2} + 2 \sum_{m=1}^{n_{h_2}} \text{sgn}(v_m^{h_2}) \frac{1 - \text{sgn}(\delta_m^{h_2})}{2} \quad (\text{S150.7})$$

$$\mathcal{X}_1 = \sum_{m=1}^{n_{c_1}} \frac{1 - \text{sgn}(\delta_m^{c_1})}{2} \quad \text{mod } 2 \quad (\text{S150.8})$$

### S151. SPACE GROUP NO. 151

| line segment                                          | character of irrep (generators only)                                                                                                                                                             |
|-------------------------------------------------------|--------------------------------------------------------------------------------------------------------------------------------------------------------------------------------------------------|
| $a \quad (0, 0, \frac{t}{2})$                         | $\{3_{001}   0 \ 0 \ \frac{1}{3}\}$<br>$a_1 \quad -e^{-\frac{1}{3}i\pi t}$<br>$a_2 \quad e^{-\frac{1}{3}i\pi t - \frac{i\pi}{3}}$<br>$a_3 \quad e^{\frac{i\pi}{3} - \frac{i\pi t}{3}}$           |
| $b \quad (\frac{1}{3}, \frac{1}{3}, \frac{1-t}{2})$   | $\{3_{001}   0 \ 0 \ \frac{1}{3}\}$<br>$b_1 \quad -e^{-\frac{1}{3}i\pi(1-t)}$<br>$b_2 \quad e^{-\frac{1}{3}i\pi(1-t) - \frac{i\pi}{3}}$<br>$b_3 \quad e^{\frac{i\pi}{3} - \frac{1}{3}i\pi(1-t)}$ |
| $c \quad (\frac{1}{3}, \frac{1}{3}, \frac{t-1}{2})$   | $\{3_{001}   0 \ 0 \ \frac{1}{3}\}$<br>$c_1 \quad -e^{-\frac{1}{3}i\pi(t-1)}$<br>$c_2 \quad e^{-\frac{1}{3}i\pi(t-1) - \frac{i\pi}{3}}$<br>$c_3 \quad e^{\frac{i\pi}{3} - \frac{1}{3}i\pi(t-1)}$ |
| $d \quad (\frac{1}{2}, 0, \frac{t}{2})$               | $\{1   0 \ 0 \ 0\}$<br>$d_1 \quad 1$                                                                                                                                                             |
| $e \quad (\frac{t}{2}, 0, 0)$                         | $\{2_{210}   0 \ 0 \ 0\}$<br>$e_1 \quad -i$<br>$e_2 \quad i$                                                                                                                                     |
| $f \quad (\frac{t}{2}, 0, \frac{1}{2})$               | $\{2_{210}   0 \ 0 \ 0\}$<br>$f_1 \quad -i$<br>$f_2 \quad i$                                                                                                                                     |
| $g \quad (\frac{t}{3}, \frac{t}{3}, \frac{1}{2})$     | $\{1   0 \ 0 \ 0\}$<br>$g_1 \quad 1$                                                                                                                                                             |
| $h \quad (\frac{t+2}{6}, \frac{1-t}{3}, \frac{1}{2})$ | $\{1   0 \ 0 \ 0\}$<br>$h_1 \quad 1$                                                                                                                                                             |



$$\begin{aligned}
\mathcal{W}_1^{\text{gapless}} = & \sum_{m=1}^{n_{a_1}} \text{sgn}(v_m^{a_1}) \frac{1 - \text{sgn}(\delta_m^{a_1})}{2} + \sum_{m=1}^{n_{a_2}} \text{sgn}(v_m^{a_2}) \frac{1 - \text{sgn}(\delta_m^{a_2})}{2} + \sum_{m=1}^{n_{a_3}} \text{sgn}(v_m^{a_3}) \frac{1 - \text{sgn}(\delta_m^{a_3})}{2} \\
& - \sum_{m=1}^{n_{d_1}} \text{sgn}(v_m^{d_1}) \frac{1 - \text{sgn}(\delta_m^{d_1})}{2} - \sum_{m=1}^{n_{e_1}} \text{sgn}(v_m^{e_1}) \frac{1 - \text{sgn}(\delta_m^{e_1})}{2} - \sum_{m=1}^{n_{e_2}} \text{sgn}(v_m^{e_2}) \frac{1 - \text{sgn}(\delta_m^{e_2})}{2} \\
& + \sum_{m=1}^{n_{g_1}} \text{sgn}(v_m^{g_1}) \frac{1 - \text{sgn}(\delta_m^{g_1})}{2} + \sum_{m=1}^{n_{h_1}} \text{sgn}(v_m^{h_1}) \frac{1 - \text{sgn}(\delta_m^{h_1})}{2}
\end{aligned} \tag{S151.1}$$

$$\begin{aligned}
\mathcal{W}_2^{\text{gapless}} = & \sum_{m=1}^{n_{b_1}} \text{sgn}(v_m^{b_1}) \frac{1 - \text{sgn}(\delta_m^{b_1})}{2} + \sum_{m=1}^{n_{b_2}} \text{sgn}(v_m^{b_2}) \frac{1 - \text{sgn}(\delta_m^{b_2})}{2} + \sum_{m=1}^{n_{b_3}} \text{sgn}(v_m^{b_3}) \frac{1 - \text{sgn}(\delta_m^{b_3})}{2} \\
& - \sum_{m=1}^{n_{c_1}} \text{sgn}(v_m^{c_1}) \frac{1 - \text{sgn}(\delta_m^{c_1})}{2} - \sum_{m=1}^{n_{c_2}} \text{sgn}(v_m^{c_2}) \frac{1 - \text{sgn}(\delta_m^{c_2})}{2} - \sum_{m=1}^{n_{c_3}} \text{sgn}(v_m^{c_3}) \frac{1 - \text{sgn}(\delta_m^{c_3})}{2}
\end{aligned} \tag{S151.2}$$

$$\begin{aligned}
\mathcal{W}_3^{\text{gapless}} = & \sum_{m=1}^{n_{f_1}} \text{sgn}(v_m^{f_1}) \frac{1 - \text{sgn}(\delta_m^{f_1})}{2} + \sum_{m=1}^{n_{f_2}} \text{sgn}(v_m^{f_2}) \frac{1 - \text{sgn}(\delta_m^{f_2})}{2} - \sum_{m=1}^{n_{g_1}} \text{sgn}(v_m^{g_1}) \frac{1 - \text{sgn}(\delta_m^{g_1})}{2} - \sum_{m=1}^{n_{h_1}} \text{sgn}(v_m^{h_1}) \frac{1 - \text{sgn}(\delta_m^{h_1})}{2}
\end{aligned} \tag{S151.3}$$

$$\mathcal{W}_1^{\text{gapped}} = - \sum_{m=1}^{n_{e_1}} \text{sgn}(v_m^{e_1}) \frac{1 - \text{sgn}(\delta_m^{e_1})}{2} + \sum_{m=1}^{n_{e_2}} \text{sgn}(v_m^{e_2}) \frac{1 - \text{sgn}(\delta_m^{e_2})}{2} \tag{S151.4}$$

$$\mathcal{W}_2^{\text{gapped}} = -2 \sum_{m=1}^{n_{f_2}} \text{sgn}(v_m^{f_2}) \frac{1 - \text{sgn}(\delta_m^{f_2})}{2} + \sum_{m=1}^{n_{g_1}} \text{sgn}(v_m^{g_1}) \frac{1 - \text{sgn}(\delta_m^{g_1})}{2} + \sum_{m=1}^{n_{h_1}} \text{sgn}(v_m^{h_1}) \frac{1 - \text{sgn}(\delta_m^{h_1})}{2} \tag{S151.5}$$

$$\begin{aligned}
\mathcal{X}_1 = & -2 \sum_{m=1}^{n_{a_2}} \text{sgn}(v_m^{a_2}) \frac{1 - \text{sgn}(\delta_m^{a_2})}{2} + 2 \sum_{m=1}^{n_{a_3}} \text{sgn}(v_m^{a_3}) \frac{1 - \text{sgn}(\delta_m^{a_3})}{2} + 2 \sum_{m=1}^{n_{b_2}} \text{sgn}(v_m^{b_2}) \frac{1 - \text{sgn}(\delta_m^{b_2})}{2} \\
& - 2 \sum_{m=1}^{n_{b_3}} \text{sgn}(v_m^{b_3}) \frac{1 - \text{sgn}(\delta_m^{b_3})}{2} - 2 \sum_{m=1}^{n_{c_2}} \text{sgn}(v_m^{c_2}) \frac{1 - \text{sgn}(\delta_m^{c_2})}{2} + 2 \sum_{m=1}^{n_{c_3}} \text{sgn}(v_m^{c_3}) \frac{1 - \text{sgn}(\delta_m^{c_3})}{2} \\
& + 3 \sum_{m=1}^{n_{d_1}} \text{sgn}(v_m^{d_1}) \frac{1 - \text{sgn}(\delta_m^{d_1})}{2} + 2 \sum_{m=1}^{n_{g_1}} \text{sgn}(v_m^{g_1}) \frac{1 - \text{sgn}(\delta_m^{g_1})}{2} \pmod{6}
\end{aligned} \tag{S151.6}$$

## S152. SPACE GROUP NO. 152

|              |                                      |
|--------------|--------------------------------------|
| line segment | character of irrep (generators only) |
|--------------|--------------------------------------|

|                                                       |                                                                                                                                                                                                  |
|-------------------------------------------------------|--------------------------------------------------------------------------------------------------------------------------------------------------------------------------------------------------|
| $a \quad (0, 0, \frac{t}{2})$                         | $\{3_{001}   0 \ 0 \ \frac{1}{3}\}$<br>$a_1 \quad -e^{-\frac{1}{3}i\pi t}$<br>$a_2 \quad e^{-\frac{1}{3}i\pi t - \frac{i\pi}{3}}$<br>$a_3 \quad e^{\frac{i\pi}{3} - \frac{i\pi t}{3}}$           |
| $b \quad (\frac{1}{3}, \frac{1}{3}, \frac{1-t}{2})$   | $\{3_{001}   0 \ 0 \ \frac{1}{3}\}$<br>$b_1 \quad -e^{-\frac{1}{3}i\pi(1-t)}$<br>$b_2 \quad e^{-\frac{1}{3}i\pi(1-t) - \frac{i\pi}{3}}$<br>$b_3 \quad e^{\frac{i\pi}{3} - \frac{1}{3}i\pi(1-t)}$ |
| $c \quad (\frac{1}{2}, 0, \frac{t}{2})$               | $\{1   0 \ 0 \ 0\}$<br>$c_1 \quad 1$                                                                                                                                                             |
| $d \quad (\frac{t}{3}, \frac{t}{3}, 0)$               | $\{2_{110}   0 \ 0 \ 0\}$<br>$d_1 \quad -i$<br>$d_2 \quad i$                                                                                                                                     |
| $e \quad (\frac{t}{3}, \frac{t}{3}, \frac{1}{2})$     | $\{2_{110}   0 \ 0 \ 0\}$<br>$e_1 \quad -i$<br>$e_2 \quad i$                                                                                                                                     |
| $f \quad (\frac{t}{2}, 0, \frac{1}{2})$               | $\{1   0 \ 0 \ 0\}$<br>$f_1 \quad 1$                                                                                                                                                             |
| $g \quad (\frac{t+2}{6}, \frac{1-t}{3}, 0)$           | $\{2_{010}   0 \ 0 \ \frac{1}{3}\}$<br>$g_1 \quad -i$<br>$g_2 \quad i$                                                                                                                           |
| $h \quad (\frac{t+2}{6}, \frac{1-t}{3}, \frac{1}{2})$ | $\{2_{010}   0 \ 0 \ \frac{1}{3}\}$<br>$h_1 \quad i$<br>$h_2 \quad -i$                                                                                                                           |

$$\begin{aligned}
\mathcal{W}_1^{\text{gapless}} = & \sum_{m=1}^{n_{a_1}} \text{sgn}(v_m^{a_1}) \frac{1 - \text{sgn}(\delta_m^{a_1})}{2} + \sum_{m=1}^{n_{a_2}} \text{sgn}(v_m^{a_2}) \frac{1 - \text{sgn}(\delta_m^{a_2})}{2} + \sum_{m=1}^{n_{a_3}} \text{sgn}(v_m^{a_3}) \frac{1 - \text{sgn}(\delta_m^{a_3})}{2} \\
& - \sum_{m=1}^{n_{c_1}} \text{sgn}(v_m^{c_1}) \frac{1 - \text{sgn}(\delta_m^{c_1})}{2} - \sum_{m=1}^{n_{d_1}} \text{sgn}(v_m^{d_1}) \frac{1 - \text{sgn}(\delta_m^{d_1})}{2} - \sum_{m=1}^{n_{d_2}} \text{sgn}(v_m^{d_2}) \frac{1 - \text{sgn}(\delta_m^{d_2})}{2} \\
& + \sum_{m=1}^{n_{f_1}} \text{sgn}(v_m^{f_1}) \frac{1 - \text{sgn}(\delta_m^{f_1})}{2} - \sum_{m=1}^{n_{g_1}} \text{sgn}(v_m^{g_1}) \frac{1 - \text{sgn}(\delta_m^{g_1})}{2} - \sum_{m=1}^{n_{g_2}} \text{sgn}(v_m^{g_2}) \frac{1 - \text{sgn}(\delta_m^{g_2})}{2}
\end{aligned} \tag{S152.1}$$

$$\begin{aligned}
\mathcal{W}_2^{\text{gapless}} = & \sum_{m=1}^{n_{b_1}} \text{sgn}(v_m^{b_1}) \frac{1 - \text{sgn}(\delta_m^{b_1})}{2} + \sum_{m=1}^{n_{b_2}} \text{sgn}(v_m^{b_2}) \frac{1 - \text{sgn}(\delta_m^{b_2})}{2} + \sum_{m=1}^{n_{b_3}} \text{sgn}(v_m^{b_3}) \frac{1 - \text{sgn}(\delta_m^{b_3})}{2} \\
& + \sum_{m=1}^{n_{c_1}} \text{sgn}(v_m^{c_1}) \frac{1 - \text{sgn}(\delta_m^{c_1})}{2} + \sum_{m=1}^{n_{g_1}} \text{sgn}(v_m^{g_1}) \frac{1 - \text{sgn}(\delta_m^{g_1})}{2} + \sum_{m=1}^{n_{g_2}} \text{sgn}(v_m^{g_2}) \frac{1 - \text{sgn}(\delta_m^{g_2})}{2} \\
& - \sum_{m=1}^{n_{h_1}} \text{sgn}(v_m^{h_1}) \frac{1 - \text{sgn}(\delta_m^{h_1})}{2} - \sum_{m=1}^{n_{h_2}} \text{sgn}(v_m^{h_2}) \frac{1 - \text{sgn}(\delta_m^{h_2})}{2}
\end{aligned} \tag{S152.2}$$

$$\begin{aligned}
\mathcal{W}_3^{\text{gapless}} = & \sum_{m=1}^{n_{e_1}} \text{sgn}(v_m^{e_1}) \frac{1 - \text{sgn}(\delta_m^{e_1})}{2} + \sum_{m=1}^{n_{e_2}} \text{sgn}(v_m^{e_2}) \frac{1 - \text{sgn}(\delta_m^{e_2})}{2} - \sum_{m=1}^{n_{f_1}} \text{sgn}(v_m^{f_1}) \frac{1 - \text{sgn}(\delta_m^{f_1})}{2} \\
& + \sum_{m=1}^{n_{h_1}} \text{sgn}(v_m^{h_1}) \frac{1 - \text{sgn}(\delta_m^{h_1})}{2} + \sum_{m=1}^{n_{h_2}} \text{sgn}(v_m^{h_2}) \frac{1 - \text{sgn}(\delta_m^{h_2})}{2}
\end{aligned} \tag{S152.3}$$

$$\begin{aligned} \mathcal{W}_1^{\text{gapped}} = & - \sum_{m=1}^{n_{d_1}} \text{sgn}(v_m^{d_1}) \frac{1 - \text{sgn}(\delta_m^{d_1})}{2} + \sum_{m=1}^{n_{d_2}} \text{sgn}(v_m^{d_2}) \frac{1 - \text{sgn}(\delta_m^{d_2})}{2} - \sum_{m=1}^{n_{g_1}} \text{sgn}(v_m^{g_1}) \frac{1 - \text{sgn}(\delta_m^{g_1})}{2} \\ & + \sum_{m=1}^{n_{g_2}} \text{sgn}(v_m^{g_2}) \frac{1 - \text{sgn}(\delta_m^{g_2})}{2} \end{aligned} \quad (\text{S152.4})$$

$$\mathcal{W}_2^{\text{gapped}} = 2 \sum_{m=1}^{n_{e_2}} \text{sgn}(v_m^{e_2}) \frac{1 - \text{sgn}(\delta_m^{e_2})}{2} - \sum_{m=1}^{n_{f_1}} \text{sgn}(v_m^{f_1}) \frac{1 - \text{sgn}(\delta_m^{f_1})}{2} + 2 \sum_{m=1}^{n_{h_2}} \text{sgn}(v_m^{h_2}) \frac{1 - \text{sgn}(\delta_m^{h_2})}{2} \quad (\text{S152.5})$$

$$\begin{aligned} \mathcal{X}_1 = & 2 \sum_{m=1}^{n_{a_2}} \text{sgn}(v_m^{a_2}) \frac{1 - \text{sgn}(\delta_m^{a_2})}{2} - 2 \sum_{m=1}^{n_{a_3}} \text{sgn}(v_m^{a_3}) \frac{1 - \text{sgn}(\delta_m^{a_3})}{2} - 4 \sum_{m=1}^{n_{b_2}} \text{sgn}(v_m^{b_2}) \frac{1 - \text{sgn}(\delta_m^{b_2})}{2} \\ & - 2 \sum_{m=1}^{n_{b_3}} \text{sgn}(v_m^{b_3}) \frac{1 - \text{sgn}(\delta_m^{b_3})}{2} - 3 \sum_{m=1}^{n_{c_1}} \text{sgn}(v_m^{c_1}) \frac{1 - \text{sgn}(\delta_m^{c_1})}{2} - 10 \sum_{m=1}^{n_{e_2}} \text{sgn}(v_m^{e_2}) \frac{1 - \text{sgn}(\delta_m^{e_2})}{2} \\ & + 3 \sum_{m=1}^{n_{f_1}} \text{sgn}(v_m^{f_1}) \frac{1 - \text{sgn}(\delta_m^{f_1})}{2} + 2 \sum_{m=1}^{n_{h_1}} \text{sgn}(v_m^{h_1}) \frac{1 - \text{sgn}(\delta_m^{h_1})}{2} - 2 \sum_{m=1}^{n_{h_2}} \text{sgn}(v_m^{h_2}) \frac{1 - \text{sgn}(\delta_m^{h_2})}{2} \pmod{6} \end{aligned} \quad (\text{S152.6})$$

### S153. SPACE GROUP NO. 153

| line segment                                          | character of irrep (generators only)                                                                                                                                                             |
|-------------------------------------------------------|--------------------------------------------------------------------------------------------------------------------------------------------------------------------------------------------------|
| $a \quad (0, 0, \frac{t}{2})$                         | $\{3_{001}   0 \ 0 \ \frac{2}{3}\}$<br>$a_1 \quad -e^{-\frac{2}{3}i\pi t}$<br>$a_2 \quad e^{-\frac{2}{3}i\pi t - \frac{i\pi}{3}}$<br>$a_3 \quad e^{\frac{i\pi}{3} - \frac{2i\pi t}{3}}$          |
| $b \quad (\frac{1}{3}, \frac{1}{3}, \frac{1-t}{2})$   | $\{3_{001}   0 \ 0 \ \frac{2}{3}\}$<br>$b_1 \quad -e^{-\frac{2}{3}i\pi(1-t)}$<br>$b_2 \quad e^{-\frac{2}{3}i\pi(1-t) - \frac{i\pi}{3}}$<br>$b_3 \quad e^{\frac{i\pi}{3} - \frac{2}{3}i\pi(1-t)}$ |
| $c \quad (\frac{1}{3}, \frac{1}{3}, \frac{t-1}{2})$   | $\{3_{001}   0 \ 0 \ \frac{2}{3}\}$<br>$c_1 \quad -e^{-\frac{2}{3}i\pi(t-1)}$<br>$c_2 \quad e^{-\frac{2}{3}i\pi(t-1) - \frac{i\pi}{3}}$<br>$c_3 \quad e^{\frac{i\pi}{3} - \frac{2}{3}i\pi(t-1)}$ |
| $d \quad (\frac{1}{2}, 0, \frac{t}{2})$               | $\{1   0 \ 0 \ 0\}$<br>$d_1 \quad 1$                                                                                                                                                             |
| $e \quad (\frac{t}{2}, 0, 0)$                         | $\{2_{210}   0 \ 0 \ 0\}$<br>$e_1 \quad -i$<br>$e_2 \quad i$                                                                                                                                     |
| $f \quad (\frac{t}{2}, 0, \frac{1}{2})$               | $\{2_{210}   0 \ 0 \ 0\}$<br>$f_1 \quad -i$<br>$f_2 \quad i$                                                                                                                                     |
| $g \quad (\frac{t}{3}, \frac{t}{3}, \frac{1}{2})$     | $\{1   0 \ 0 \ 0\}$<br>$g_1 \quad 1$                                                                                                                                                             |
| $h \quad (\frac{t+2}{6}, \frac{1-t}{3}, \frac{1}{2})$ | $\{1   0 \ 0 \ 0\}$<br>$h_1 \quad 1$                                                                                                                                                             |

$$\begin{aligned}
\mathcal{W}_1^{\text{gapless}} = & \sum_{m=1}^{n_{a_1}} \text{sgn}(v_m^{a_1}) \frac{1 - \text{sgn}(\delta_m^{a_1})}{2} + \sum_{m=1}^{n_{a_2}} \text{sgn}(v_m^{a_2}) \frac{1 - \text{sgn}(\delta_m^{a_2})}{2} + \sum_{m=1}^{n_{a_3}} \text{sgn}(v_m^{a_3}) \frac{1 - \text{sgn}(\delta_m^{a_3})}{2} \\
& - \sum_{m=1}^{n_{d_1}} \text{sgn}(v_m^{d_1}) \frac{1 - \text{sgn}(\delta_m^{d_1})}{2} - \sum_{m=1}^{n_{e_1}} \text{sgn}(v_m^{e_1}) \frac{1 - \text{sgn}(\delta_m^{e_1})}{2} - \sum_{m=1}^{n_{e_2}} \text{sgn}(v_m^{e_2}) \frac{1 - \text{sgn}(\delta_m^{e_2})}{2} \\
& + \sum_{m=1}^{n_{g_1}} \text{sgn}(v_m^{g_1}) \frac{1 - \text{sgn}(\delta_m^{g_1})}{2} + \sum_{m=1}^{n_{h_1}} \text{sgn}(v_m^{h_1}) \frac{1 - \text{sgn}(\delta_m^{h_1})}{2}
\end{aligned} \tag{S153.1}$$

$$\begin{aligned}
\mathcal{W}_2^{\text{gapless}} = & \sum_{m=1}^{n_{b_1}} \text{sgn}(v_m^{b_1}) \frac{1 - \text{sgn}(\delta_m^{b_1})}{2} + \sum_{m=1}^{n_{b_2}} \text{sgn}(v_m^{b_2}) \frac{1 - \text{sgn}(\delta_m^{b_2})}{2} + \sum_{m=1}^{n_{b_3}} \text{sgn}(v_m^{b_3}) \frac{1 - \text{sgn}(\delta_m^{b_3})}{2} \\
& - \sum_{m=1}^{n_{c_1}} \text{sgn}(v_m^{c_1}) \frac{1 - \text{sgn}(\delta_m^{c_1})}{2} - \sum_{m=1}^{n_{c_2}} \text{sgn}(v_m^{c_2}) \frac{1 - \text{sgn}(\delta_m^{c_2})}{2} - \sum_{m=1}^{n_{c_3}} \text{sgn}(v_m^{c_3}) \frac{1 - \text{sgn}(\delta_m^{c_3})}{2}
\end{aligned} \tag{S153.2}$$

$$\begin{aligned}
\mathcal{W}_3^{\text{gapless}} = & \sum_{m=1}^{n_{f_1}} \text{sgn}(v_m^{f_1}) \frac{1 - \text{sgn}(\delta_m^{f_1})}{2} + \sum_{m=1}^{n_{f_2}} \text{sgn}(v_m^{f_2}) \frac{1 - \text{sgn}(\delta_m^{f_2})}{2} - \sum_{m=1}^{n_{g_1}} \text{sgn}(v_m^{g_1}) \frac{1 - \text{sgn}(\delta_m^{g_1})}{2} - \sum_{m=1}^{n_{h_1}} \text{sgn}(v_m^{h_1}) \frac{1 - \text{sgn}(\delta_m^{h_1})}{2}
\end{aligned} \tag{S153.3}$$

$$\mathcal{W}_1^{\text{gapped}} = - \sum_{m=1}^{n_{e_1}} \text{sgn}(v_m^{e_1}) \frac{1 - \text{sgn}(\delta_m^{e_1})}{2} + \sum_{m=1}^{n_{e_2}} \text{sgn}(v_m^{e_2}) \frac{1 - \text{sgn}(\delta_m^{e_2})}{2} \tag{S153.4}$$

$$\mathcal{W}_2^{\text{gapped}} = -2 \sum_{m=1}^{n_{f_2}} \text{sgn}(v_m^{f_2}) \frac{1 - \text{sgn}(\delta_m^{f_2})}{2} + \sum_{m=1}^{n_{g_1}} \text{sgn}(v_m^{g_1}) \frac{1 - \text{sgn}(\delta_m^{g_1})}{2} + \sum_{m=1}^{n_{h_1}} \text{sgn}(v_m^{h_1}) \frac{1 - \text{sgn}(\delta_m^{h_1})}{2} \tag{S153.5}$$

$$\begin{aligned}
\mathcal{X}_1 = & 2 \sum_{m=1}^{n_{a_2}} \text{sgn}(v_m^{a_2}) \frac{1 - \text{sgn}(\delta_m^{a_2})}{2} - 2 \sum_{m=1}^{n_{a_3}} \text{sgn}(v_m^{a_3}) \frac{1 - \text{sgn}(\delta_m^{a_3})}{2} - 2 \sum_{m=1}^{n_{b_2}} \text{sgn}(v_m^{b_2}) \frac{1 - \text{sgn}(\delta_m^{b_2})}{2} \\
& - 4 \sum_{m=1}^{n_{b_3}} \text{sgn}(v_m^{b_3}) \frac{1 - \text{sgn}(\delta_m^{b_3})}{2} + 2 \sum_{m=1}^{n_{c_2}} \text{sgn}(v_m^{c_2}) \frac{1 - \text{sgn}(\delta_m^{c_2})}{2} + 4 \sum_{m=1}^{n_{c_3}} \text{sgn}(v_m^{c_3}) \frac{1 - \text{sgn}(\delta_m^{c_3})}{2} \\
& + 3 \sum_{m=1}^{n_{d_1}} \text{sgn}(v_m^{d_1}) \frac{1 - \text{sgn}(\delta_m^{d_1})}{2} + 2 \sum_{m=1}^{n_{g_1}} \text{sgn}(v_m^{g_1}) \frac{1 - \text{sgn}(\delta_m^{g_1})}{2} \pmod{6}
\end{aligned} \tag{S153.6}$$

#### S154. SPACE GROUP NO. 154

|              |                                      |
|--------------|--------------------------------------|
| line segment | character of irrep (generators only) |
|--------------|--------------------------------------|

|                                                       |                                                                                                                                                                                                  |
|-------------------------------------------------------|--------------------------------------------------------------------------------------------------------------------------------------------------------------------------------------------------|
| $a \quad (0, 0, \frac{t}{2})$                         | $\{3_{001}   0 \ 0 \ \frac{2}{3}\}$<br>$a_1 \quad -e^{-\frac{2}{3}i\pi t}$<br>$a_2 \quad e^{-\frac{2}{3}i\pi t - \frac{i\pi}{3}}$<br>$a_3 \quad e^{\frac{i\pi}{3} - \frac{2i\pi t}{3}}$          |
| $b \quad (\frac{1}{3}, \frac{1}{3}, \frac{1-t}{2})$   | $\{3_{001}   0 \ 0 \ \frac{2}{3}\}$<br>$b_1 \quad -e^{-\frac{2}{3}i\pi(1-t)}$<br>$b_2 \quad e^{-\frac{2}{3}i\pi(1-t) - \frac{i\pi}{3}}$<br>$b_3 \quad e^{\frac{i\pi}{3} - \frac{2}{3}i\pi(1-t)}$ |
| $c \quad (\frac{1}{2}, 0, \frac{t}{2})$               | $\{1   0 \ 0 \ 0\}$<br>$c_1 \quad 1$                                                                                                                                                             |
| $d \quad (\frac{t}{3}, \frac{t}{3}, 0)$               | $\{2_{110}   0 \ 0 \ 0\}$<br>$d_1 \quad -i$<br>$d_2 \quad i$                                                                                                                                     |
| $e \quad (\frac{t}{3}, \frac{t}{3}, \frac{1}{2})$     | $\{2_{110}   0 \ 0 \ 0\}$<br>$e_1 \quad -i$<br>$e_2 \quad i$                                                                                                                                     |
| $f \quad (\frac{t}{2}, 0, \frac{1}{2})$               | $\{1   0 \ 0 \ 0\}$<br>$f_1 \quad 1$                                                                                                                                                             |
| $g \quad (\frac{t+2}{6}, \frac{1-t}{3}, 0)$           | $\{2_{010}   0 \ 0 \ \frac{2}{3}\}$<br>$g_1 \quad -i$<br>$g_2 \quad i$                                                                                                                           |
| $h \quad (\frac{t+2}{6}, \frac{1-t}{3}, \frac{1}{2})$ | $\{2_{010}   0 \ 0 \ \frac{2}{3}\}$<br>$h_1 \quad i$<br>$h_2 \quad -i$                                                                                                                           |

$$\begin{aligned}
\mathcal{W}_1^{\text{gapless}} = & \sum_{m=1}^{n_{a_1}} \text{sgn}(v_m^{a_1}) \frac{1 - \text{sgn}(\delta_m^{a_1})}{2} + \sum_{m=1}^{n_{a_2}} \text{sgn}(v_m^{a_2}) \frac{1 - \text{sgn}(\delta_m^{a_2})}{2} + \sum_{m=1}^{n_{a_3}} \text{sgn}(v_m^{a_3}) \frac{1 - \text{sgn}(\delta_m^{a_3})}{2} \\
& - \sum_{m=1}^{n_{c_1}} \text{sgn}(v_m^{c_1}) \frac{1 - \text{sgn}(\delta_m^{c_1})}{2} - \sum_{m=1}^{n_{d_1}} \text{sgn}(v_m^{d_1}) \frac{1 - \text{sgn}(\delta_m^{d_1})}{2} - \sum_{m=1}^{n_{d_2}} \text{sgn}(v_m^{d_2}) \frac{1 - \text{sgn}(\delta_m^{d_2})}{2} \\
& + \sum_{m=1}^{n_{f_1}} \text{sgn}(v_m^{f_1}) \frac{1 - \text{sgn}(\delta_m^{f_1})}{2} - \sum_{m=1}^{n_{g_1}} \text{sgn}(v_m^{g_1}) \frac{1 - \text{sgn}(\delta_m^{g_1})}{2} - \sum_{m=1}^{n_{g_2}} \text{sgn}(v_m^{g_2}) \frac{1 - \text{sgn}(\delta_m^{g_2})}{2}
\end{aligned} \tag{S154.1}$$

$$\begin{aligned}
\mathcal{W}_2^{\text{gapless}} = & \sum_{m=1}^{n_{b_1}} \text{sgn}(v_m^{b_1}) \frac{1 - \text{sgn}(\delta_m^{b_1})}{2} + \sum_{m=1}^{n_{b_2}} \text{sgn}(v_m^{b_2}) \frac{1 - \text{sgn}(\delta_m^{b_2})}{2} + \sum_{m=1}^{n_{b_3}} \text{sgn}(v_m^{b_3}) \frac{1 - \text{sgn}(\delta_m^{b_3})}{2} \\
& + \sum_{m=1}^{n_{c_1}} \text{sgn}(v_m^{c_1}) \frac{1 - \text{sgn}(\delta_m^{c_1})}{2} + \sum_{m=1}^{n_{g_1}} \text{sgn}(v_m^{g_1}) \frac{1 - \text{sgn}(\delta_m^{g_1})}{2} + \sum_{m=1}^{n_{g_2}} \text{sgn}(v_m^{g_2}) \frac{1 - \text{sgn}(\delta_m^{g_2})}{2} \\
& - \sum_{m=1}^{n_{h_1}} \text{sgn}(v_m^{h_1}) \frac{1 - \text{sgn}(\delta_m^{h_1})}{2} - \sum_{m=1}^{n_{h_2}} \text{sgn}(v_m^{h_2}) \frac{1 - \text{sgn}(\delta_m^{h_2})}{2}
\end{aligned} \tag{S154.2}$$

$$\begin{aligned}
\mathcal{W}_3^{\text{gapless}} = & \sum_{m=1}^{n_{e_1}} \text{sgn}(v_m^{e_1}) \frac{1 - \text{sgn}(\delta_m^{e_1})}{2} + \sum_{m=1}^{n_{e_2}} \text{sgn}(v_m^{e_2}) \frac{1 - \text{sgn}(\delta_m^{e_2})}{2} - \sum_{m=1}^{n_{f_1}} \text{sgn}(v_m^{f_1}) \frac{1 - \text{sgn}(\delta_m^{f_1})}{2} \\
& + \sum_{m=1}^{n_{h_1}} \text{sgn}(v_m^{h_1}) \frac{1 - \text{sgn}(\delta_m^{h_1})}{2} + \sum_{m=1}^{n_{h_2}} \text{sgn}(v_m^{h_2}) \frac{1 - \text{sgn}(\delta_m^{h_2})}{2}
\end{aligned} \tag{S154.3}$$

$$\mathcal{W}_1^{\text{gapped}} = 2 \sum_{m=1}^{n_{e_2}} \text{sgn}(v_m^{e_2}) \frac{1 - \text{sgn}(\delta_m^{e_2})}{2} - \sum_{m=1}^{n_{f_1}} \text{sgn}(v_m^{f_1}) \frac{1 - \text{sgn}(\delta_m^{f_1})}{2} + 2 \sum_{m=1}^{n_{h_1}} \text{sgn}(v_m^{h_1}) \frac{1 - \text{sgn}(\delta_m^{h_1})}{2} \quad (\text{S154.4})$$

$$\begin{aligned} \mathcal{W}_2^{\text{gapped}} = & - \sum_{m=1}^{n_{d_1}} \text{sgn}(v_m^{d_1}) \frac{1 - \text{sgn}(\delta_m^{d_1})}{2} + \sum_{m=1}^{n_{d_2}} \text{sgn}(v_m^{d_2}) \frac{1 - \text{sgn}(\delta_m^{d_2})}{2} - \sum_{m=1}^{n_{g_1}} \text{sgn}(v_m^{g_1}) \frac{1 - \text{sgn}(\delta_m^{g_1})}{2} \\ & + \sum_{m=1}^{n_{g_2}} \text{sgn}(v_m^{g_2}) \frac{1 - \text{sgn}(\delta_m^{g_2})}{2} \end{aligned} \quad (\text{S154.5})$$

$$\begin{aligned} \mathcal{X}_1 = & -2 \sum_{m=1}^{n_{a_2}} \text{sgn}(v_m^{a_2}) \frac{1 - \text{sgn}(\delta_m^{a_2})}{2} + 2 \sum_{m=1}^{n_{a_3}} \text{sgn}(v_m^{a_3}) \frac{1 - \text{sgn}(\delta_m^{a_3})}{2} - 2 \sum_{m=1}^{n_{b_2}} \text{sgn}(v_m^{b_2}) \frac{1 - \text{sgn}(\delta_m^{b_2})}{2} \\ & - 4 \sum_{m=1}^{n_{b_3}} \text{sgn}(v_m^{b_3}) \frac{1 - \text{sgn}(\delta_m^{b_3})}{2} - 3 \sum_{m=1}^{n_{c_1}} \text{sgn}(v_m^{c_1}) \frac{1 - \text{sgn}(\delta_m^{c_1})}{2} - 4 \sum_{m=1}^{n_{e_2}} \text{sgn}(v_m^{e_2}) \frac{1 - \text{sgn}(\delta_m^{e_2})}{2} \\ & - 2 \sum_{m=1}^{n_{h_1}} \text{sgn}(v_m^{h_1}) \frac{1 - \text{sgn}(\delta_m^{h_1})}{2} + 8 \sum_{m=1}^{n_{h_2}} \text{sgn}(v_m^{h_2}) \frac{1 - \text{sgn}(\delta_m^{h_2})}{2} \quad \text{mod } 6 \end{aligned} \quad (\text{S154.6})$$

### S155. SPACE GROUP NO. 155

| line segment                                | character of irrep (generators only)                                                                             |
|---------------------------------------------|------------------------------------------------------------------------------------------------------------------|
| $a \quad (0, 0, \frac{3t}{2})$              | $\{3_{001}   0 \ 0 \ 0\}$<br>$a_1 \quad -1$<br>$a_2 \quad e^{-\frac{i\pi}{3}}$<br>$a_3 \quad e^{\frac{i\pi}{3}}$ |
| $b \quad (0, \frac{t}{2}, \frac{3-t}{2})$   | $\{1   0 \ 0 \ 0\}$<br>$b_1 \quad 1$                                                                             |
| $c \quad (\frac{t}{2}, 0, \frac{3}{2} - t)$ | $\{1   0 \ 0 \ 0\}$<br>$c_1 \quad 1$                                                                             |
| $d \quad (0, t, \frac{t}{2})$               | $\{1   0 \ 0 \ 0\}$<br>$d_1 \quad 1$                                                                             |
| $e \quad (\frac{t}{2}, \frac{t}{2}, 0)$     | $\{2_{10-1}   0 \ 0 \ 0\}$<br>$e_1 \quad -i$<br>$e_2 \quad i$                                                    |
| $f \quad (\frac{1-t}{2}, t, \frac{1}{2})$   | $\{2_{01-1}   0 \ 0 \ 0\}$<br>$f_1 \quad -i$<br>$f_2 \quad i$                                                    |

$$\mathcal{W}_1^{\text{gapless}} = \sum_{m=1}^{n_{a_1}} \text{sgn}(v_m^{a_1}) \frac{1 - \text{sgn}(\delta_m^{a_1})}{2} + \sum_{m=1}^{n_{a_2}} \text{sgn}(v_m^{a_2}) \frac{1 - \text{sgn}(\delta_m^{a_2})}{2} + \sum_{m=1}^{n_{a_3}} \text{sgn}(v_m^{a_3}) \frac{1 - \text{sgn}(\delta_m^{a_3})}{2} - \sum_{m=1}^{n_{d_1}} \text{sgn}(v_m^{d_1}) \frac{1 - \text{sgn}(\delta_m^{d_1})}{2} \quad (\text{S155.1})$$

$$\mathcal{W}_2^{\text{gapless}} = \sum_{m=1}^{n_{b_1}} \text{sgn}(v_m^{b_1}) \frac{1 - \text{sgn}(\delta_m^{b_1})}{2} + \sum_{m=1}^{n_{d_1}} \text{sgn}(v_m^{d_1}) \frac{1 - \text{sgn}(\delta_m^{d_1})}{2} - \sum_{m=1}^{n_{e_1}} \text{sgn}(v_m^{e_1}) \frac{1 - \text{sgn}(\delta_m^{e_1})}{2} - \sum_{m=1}^{n_{e_2}} \text{sgn}(v_m^{e_2}) \frac{1 - \text{sgn}(\delta_m^{e_2})}{2} \quad (\text{S155.2})$$

$$\mathcal{W}_3^{\text{gapless}} = \sum_{m=1}^{n_{c_1}} \text{sgn}(v_m^{c_1}) \frac{1 - \text{sgn}(\delta_m^{c_1})}{2} + \sum_{m=1}^{n_{f_1}} \text{sgn}(v_m^{f_1}) \frac{1 - \text{sgn}(\delta_m^{f_1})}{2} + \sum_{m=1}^{n_{f_2}} \text{sgn}(v_m^{f_2}) \frac{1 - \text{sgn}(\delta_m^{f_2})}{2} \quad (\text{S155.3})$$

$$\mathcal{W}_1^{\text{gapped}} = - \sum_{m=1}^{n_{e_1}} \text{sgn}(v_m^{e_1}) \frac{1 - \text{sgn}(\delta_m^{e_1})}{2} + \sum_{m=1}^{n_{e_2}} \text{sgn}(v_m^{e_2}) \frac{1 - \text{sgn}(\delta_m^{e_2})}{2} \quad (\text{S155.4})$$

$$\mathcal{W}_2^{\text{gapped}} = \sum_{m=1}^{n_{a_2}} \text{sgn}(v_m^{a_2}) \frac{1 - \text{sgn}(\delta_m^{a_2})}{2} - \sum_{m=1}^{n_{a_3}} \text{sgn}(v_m^{a_3}) \frac{1 - \text{sgn}(\delta_m^{a_3})}{2} \quad (\text{S155.5})$$

$$\mathcal{W}_3^{\text{gapped}} = - \sum_{m=1}^{n_{f_1}} \text{sgn}(v_m^{f_1}) \frac{1 - \text{sgn}(\delta_m^{f_1})}{2} + \sum_{m=1}^{n_{f_2}} \text{sgn}(v_m^{f_2}) \frac{1 - \text{sgn}(\delta_m^{f_2})}{2} \quad (\text{S155.6})$$

$$\mathcal{X}_1 = \sum_{m=1}^{n_{d_1}} \frac{1 - \text{sgn}(\delta_m^{d_1})}{2} \quad \text{mod } 2 \quad (\text{S155.7})$$

#### S156. SPACE GROUP NO. 156

| line segment                                          | character of irrep (generators only)                                                                                                    |
|-------------------------------------------------------|-----------------------------------------------------------------------------------------------------------------------------------------|
| $a \quad (0, 0, \frac{t}{2})$                         | $\begin{array}{cc} \{3_{001}   0 & 0 & 0\} & \{m_{100}   0 & 0 & 0\} \\ a_1 & -1 & & -i \\ a_2 & -1 & & i \\ a_3 & 1 & & 0 \end{array}$ |
| $b \quad (\frac{1}{3}, \frac{1}{3}, \frac{1-t}{2})$   | $\begin{array}{c} \{3_{001}   0 & 0 & 0\} \\ b_1 & -1 \\ b_2 & e^{-\frac{i\pi}{3}} \\ b_3 & e^{\frac{i\pi}{3}} \end{array}$             |
| $c \quad (\frac{1}{2}, 0, \frac{t}{2})$               | $\begin{array}{c} \{m_{010}   0 & 0 & 0\} \\ c_1 & -i \\ c_2 & i \end{array}$                                                           |
| $d \quad (\frac{t}{3}, \frac{t}{3}, 0)$               | $\begin{array}{c} \{1   0 & 0 & 0\} \\ d_1 & 1 \end{array}$                                                                             |
| $e \quad (\frac{t}{3}, \frac{t}{3}, \frac{1}{2})$     | $\begin{array}{c} \{1   0 & 0 & 0\} \\ e_1 & 1 \end{array}$                                                                             |
| $f \quad (\frac{t}{2}, 0, \frac{1}{2})$               | $\begin{array}{c} \{m_{010}   0 & 0 & 0\} \\ f_1 & -i \\ f_2 & i \end{array}$                                                           |
| $g \quad (\frac{t+2}{6}, \frac{1-t}{3}, 0)$           | $\begin{array}{c} \{1   0 & 0 & 0\} \\ g_1 & 1 \end{array}$                                                                             |
| $h \quad (\frac{t+2}{6}, \frac{1-t}{3}, \frac{1}{2})$ | $\begin{array}{c} \{1   0 & 0 & 0\} \\ h_1 & 1 \end{array}$                                                                             |

$$\begin{aligned}
\mathcal{W}_1^{\text{gapless}} = & \sum_{m=1}^{n_{a_1}} \text{sgn}(v_m^{a_1}) \frac{1 - \text{sgn}(\delta_m^{a_1})}{2} + \sum_{m=1}^{n_{a_2}} \text{sgn}(v_m^{a_2}) \frac{1 - \text{sgn}(\delta_m^{a_2})}{2} + 2 \sum_{m=1}^{n_{a_3}} \text{sgn}(v_m^{a_3}) \frac{1 - \text{sgn}(\delta_m^{a_3})}{2} \\
& - \sum_{m=1}^{n_{c_1}} \text{sgn}(v_m^{c_1}) \frac{1 - \text{sgn}(\delta_m^{c_1})}{2} - \sum_{m=1}^{n_{c_2}} \text{sgn}(v_m^{c_2}) \frac{1 - \text{sgn}(\delta_m^{c_2})}{2} - \sum_{m=1}^{n_{d_1}} \text{sgn}(v_m^{d_1}) \frac{1 - \text{sgn}(\delta_m^{d_1})}{2} \\
& + \sum_{m=1}^{n_{f_1}} \text{sgn}(v_m^{f_1}) \frac{1 - \text{sgn}(\delta_m^{f_1})}{2} + \sum_{m=1}^{n_{f_2}} \text{sgn}(v_m^{f_2}) \frac{1 - \text{sgn}(\delta_m^{f_2})}{2} - \sum_{m=1}^{n_{g_1}} \text{sgn}(v_m^{g_1}) \frac{1 - \text{sgn}(\delta_m^{g_1})}{2}
\end{aligned} \tag{S156.1}$$

$$\begin{aligned}
\mathcal{W}_2^{\text{gapless}} = & 2 \sum_{m=1}^{n_{a_2}} \text{sgn}(v_m^{a_2}) \frac{1 - \text{sgn}(\delta_m^{a_2})}{2} + 2 \sum_{m=1}^{n_{a_3}} \text{sgn}(v_m^{a_3}) \frac{1 - \text{sgn}(\delta_m^{a_3})}{2} - 2 \sum_{m=1}^{n_{c_1}} \text{sgn}(v_m^{c_1}) \frac{1 - \text{sgn}(\delta_m^{c_1})}{2} \\
& - \sum_{m=1}^{n_{d_1}} \text{sgn}(v_m^{d_1}) \frac{1 - \text{sgn}(\delta_m^{d_1})}{2} + \sum_{m=1}^{n_{f_1}} \text{sgn}(v_m^{f_1}) \frac{1 - \text{sgn}(\delta_m^{f_1})}{2} + \sum_{m=1}^{n_{f_2}} \text{sgn}(v_m^{f_2}) \frac{1 - \text{sgn}(\delta_m^{f_2})}{2} \\
& - \sum_{m=1}^{n_{g_1}} \text{sgn}(v_m^{g_1}) \frac{1 - \text{sgn}(\delta_m^{g_1})}{2}
\end{aligned} \tag{S156.2}$$

$$\begin{aligned}
\mathcal{W}_3^{\text{gapless}} = & \sum_{m=1}^{n_{b_1}} \text{sgn}(v_m^{b_1}) \frac{1 - \text{sgn}(\delta_m^{b_1})}{2} + \sum_{m=1}^{n_{b_2}} \text{sgn}(v_m^{b_2}) \frac{1 - \text{sgn}(\delta_m^{b_2})}{2} + \sum_{m=1}^{n_{b_3}} \text{sgn}(v_m^{b_3}) \frac{1 - \text{sgn}(\delta_m^{b_3})}{2} + \sum_{m=1}^{n_{c_1}} \text{sgn}(v_m^{c_1}) \frac{1 - \text{sgn}(\delta_m^{c_1})}{2} \\
& + \sum_{m=1}^{n_{c_2}} \text{sgn}(v_m^{c_2}) \frac{1 - \text{sgn}(\delta_m^{c_2})}{2} + \sum_{m=1}^{n_{g_1}} \text{sgn}(v_m^{g_1}) \frac{1 - \text{sgn}(\delta_m^{g_1})}{2} - \sum_{m=1}^{n_{h_1}} \text{sgn}(v_m^{h_1}) \frac{1 - \text{sgn}(\delta_m^{h_1})}{2}
\end{aligned} \tag{S156.3}$$

$$\begin{aligned}
\mathcal{W}_4^{\text{gapless}} = & \sum_{m=1}^{n_{e_1}} \text{sgn}(v_m^{e_1}) \frac{1 - \text{sgn}(\delta_m^{e_1})}{2} - \sum_{m=1}^{n_{f_1}} \text{sgn}(v_m^{f_1}) \frac{1 - \text{sgn}(\delta_m^{f_1})}{2} - \sum_{m=1}^{n_{f_2}} \text{sgn}(v_m^{f_2}) \frac{1 - \text{sgn}(\delta_m^{f_2})}{2} + \sum_{m=1}^{n_{h_1}} \text{sgn}(v_m^{h_1}) \frac{1 - \text{sgn}(\delta_m^{h_1})}{2}
\end{aligned} \tag{S156.4}$$

$$\mathcal{W}_1^{\text{gapped}} = - \sum_{m=1}^{n_{c_1}} \text{sgn}(v_m^{c_1}) \frac{1 - \text{sgn}(\delta_m^{c_1})}{2} + \sum_{m=1}^{n_{c_2}} \text{sgn}(v_m^{c_2}) \frac{1 - \text{sgn}(\delta_m^{c_2})}{2} \tag{S156.5}$$

$$\mathcal{W}_2^{\text{gapped}} = - \sum_{m=1}^{n_{f_1}} \text{sgn}(v_m^{f_1}) \frac{1 - \text{sgn}(\delta_m^{f_1})}{2} + \sum_{m=1}^{n_{f_2}} \text{sgn}(v_m^{f_2}) \frac{1 - \text{sgn}(\delta_m^{f_2})}{2} \tag{S156.6}$$

### S157. SPACE GROUP NO. 157

|              |                                      |
|--------------|--------------------------------------|
| line segment | character of irrep (generators only) |
|--------------|--------------------------------------|



|                                                       |                                                                                                                                   |
|-------------------------------------------------------|-----------------------------------------------------------------------------------------------------------------------------------|
| $a \quad (0, 0, \frac{t}{2})$                         | $\{3_{001} 0 \ 0 \ 0\} \quad \{m_{210} 0 \ 0 \ 0\}$<br>$a_1 \quad -1 \quad -i$<br>$a_2 \quad -1 \quad i$<br>$a_3 \quad 1 \quad 0$ |
| $b \quad (\frac{1}{3}, \frac{1}{3}, \frac{1-t}{2})$   | $\{3_{001} 0 \ 0 \ 0\} \quad \{m_{210} 0 \ 0 \ 0\}$<br>$b_1 \quad -1 \quad -i$<br>$b_2 \quad -1 \quad i$<br>$b_3 \quad 1 \quad 0$ |
| $c \quad (\frac{1}{3}, \frac{1}{3}, \frac{t-1}{2})$   | $\{3_{001} 0 \ 0 \ 0\} \quad \{m_{210} 0 \ 0 \ 0\}$<br>$c_1 \quad -1 \quad -i$<br>$c_2 \quad -1 \quad i$<br>$c_3 \quad 1 \quad 0$ |
| $d \quad (\frac{1}{2}, 0, \frac{t}{2})$               | $\{m_{210} 0 \ 0 \ 0\}$<br>$d_1 \quad -i$<br>$d_2 \quad i$                                                                        |
| $e \quad (\frac{t}{2}, 0, 0)$                         | $\{1 0 \ 0 \ 0\}$<br>$e_1 \quad 1$                                                                                                |
| $f \quad (\frac{t}{2}, 0, \frac{1}{2})$               | $\{1 0 \ 0 \ 0\}$<br>$f_1 \quad 1$                                                                                                |
| $g \quad (\frac{t}{3}, \frac{t}{3}, \frac{1}{2})$     | $\{m_{-110} 0 \ 0 \ 0\}$<br>$g_1 \quad -i$<br>$g_2 \quad i$                                                                       |
| $h \quad (\frac{t+2}{6}, \frac{1-t}{3}, \frac{1}{2})$ | $\{m_{210} 0 \ 0 \ 0\}$<br>$h_1 \quad -i$<br>$h_2 \quad i$                                                                        |

$$\begin{aligned}
\mathcal{W}_1^{\text{gapless}} = & \sum_{m=1}^{n_{a_1}} \text{sgn}(v_m^{a_1}) \frac{1 - \text{sgn}(\delta_m^{a_1})}{2} + \sum_{m=1}^{n_{a_2}} \text{sgn}(v_m^{a_2}) \frac{1 - \text{sgn}(\delta_m^{a_2})}{2} + 2 \sum_{m=1}^{n_{a_3}} \text{sgn}(v_m^{a_3}) \frac{1 - \text{sgn}(\delta_m^{a_3})}{2} \\
& - \sum_{m=1}^{n_{d_1}} \text{sgn}(v_m^{d_1}) \frac{1 - \text{sgn}(\delta_m^{d_1})}{2} - \sum_{m=1}^{n_{d_2}} \text{sgn}(v_m^{d_2}) \frac{1 - \text{sgn}(\delta_m^{d_2})}{2} - \sum_{m=1}^{n_{e_1}} \text{sgn}(v_m^{e_1}) \frac{1 - \text{sgn}(\delta_m^{e_1})}{2} \\
& + \sum_{m=1}^{n_{g_1}} \text{sgn}(v_m^{g_1}) \frac{1 - \text{sgn}(\delta_m^{g_1})}{2} + \sum_{m=1}^{n_{g_2}} \text{sgn}(v_m^{g_2}) \frac{1 - \text{sgn}(\delta_m^{g_2})}{2} + \sum_{m=1}^{n_{h_1}} \text{sgn}(v_m^{h_1}) \frac{1 - \text{sgn}(\delta_m^{h_1})}{2} \\
& + \sum_{m=1}^{n_{h_2}} \text{sgn}(v_m^{h_2}) \frac{1 - \text{sgn}(\delta_m^{h_2})}{2}
\end{aligned} \tag{S157.1}$$

$$\begin{aligned}
\mathcal{W}_2^{\text{gapless}} = & 2 \sum_{m=1}^{n_{a_2}} \text{sgn}(v_m^{a_2}) \frac{1 - \text{sgn}(\delta_m^{a_2})}{2} + 2 \sum_{m=1}^{n_{a_3}} \text{sgn}(v_m^{a_3}) \frac{1 - \text{sgn}(\delta_m^{a_3})}{2} - 2 \sum_{m=1}^{n_{d_2}} \text{sgn}(v_m^{d_2}) \frac{1 - \text{sgn}(\delta_m^{d_2})}{2} \\
& - \sum_{m=1}^{n_{e_1}} \text{sgn}(v_m^{e_1}) \frac{1 - \text{sgn}(\delta_m^{e_1})}{2} + \sum_{m=1}^{n_{g_1}} \text{sgn}(v_m^{g_1}) \frac{1 - \text{sgn}(\delta_m^{g_1})}{2} + \sum_{m=1}^{n_{g_2}} \text{sgn}(v_m^{g_2}) \frac{1 - \text{sgn}(\delta_m^{g_2})}{2} \\
& + \sum_{m=1}^{n_{h_1}} \text{sgn}(v_m^{h_1}) \frac{1 - \text{sgn}(\delta_m^{h_1})}{2} + \sum_{m=1}^{n_{h_2}} \text{sgn}(v_m^{h_2}) \frac{1 - \text{sgn}(\delta_m^{h_2})}{2}
\end{aligned} \tag{S157.2}$$

$$\begin{aligned}
\mathcal{W}_3^{\text{gapless}} = & \sum_{m=1}^{n_{b_1}} \text{sgn}(v_m^{b_1}) \frac{1 - \text{sgn}(\delta_m^{b_1})}{2} + \sum_{m=1}^{n_{b_3}} \text{sgn}(v_m^{b_3}) \frac{1 - \text{sgn}(\delta_m^{b_3})}{2} - \sum_{m=1}^{n_{c_1}} \text{sgn}(v_m^{c_1}) \frac{1 - \text{sgn}(\delta_m^{c_1})}{2} \\
& - \sum_{m=1}^{n_{c_3}} \text{sgn}(v_m^{c_3}) \frac{1 - \text{sgn}(\delta_m^{c_3})}{2} + \sum_{m=1}^{n_{d_1}} \text{sgn}(v_m^{d_1}) \frac{1 - \text{sgn}(\delta_m^{d_1})}{2} - \sum_{m=1}^{n_{d_2}} \text{sgn}(v_m^{d_2}) \frac{1 - \text{sgn}(\delta_m^{d_2})}{2}
\end{aligned} \tag{S157.3}$$

$$\begin{aligned} \mathcal{W}_4^{\text{gapless}} = & \sum_{m=1}^{n_{b_2}} \text{sgn}(v_m^{b_2}) \frac{1 - \text{sgn}(\delta_m^{b_2})}{2} + \sum_{m=1}^{n_{b_3}} \text{sgn}(v_m^{b_3}) \frac{1 - \text{sgn}(\delta_m^{b_3})}{2} - \sum_{m=1}^{n_{c_2}} \text{sgn}(v_m^{c_2}) \frac{1 - \text{sgn}(\delta_m^{c_2})}{2} \\ & - \sum_{m=1}^{n_{c_3}} \text{sgn}(v_m^{c_3}) \frac{1 - \text{sgn}(\delta_m^{c_3})}{2} - \sum_{m=1}^{n_{d_1}} \text{sgn}(v_m^{d_1}) \frac{1 - \text{sgn}(\delta_m^{d_1})}{2} + \sum_{m=1}^{n_{d_2}} \text{sgn}(v_m^{d_2}) \frac{1 - \text{sgn}(\delta_m^{d_2})}{2} \end{aligned} \quad (\text{S157.4})$$

$$\begin{aligned} \mathcal{W}_5^{\text{gapless}} = & \sum_{m=1}^{n_{f_1}} \text{sgn}(v_m^{f_1}) \frac{1 - \text{sgn}(\delta_m^{f_1})}{2} - \sum_{m=1}^{n_{g_1}} \text{sgn}(v_m^{g_1}) \frac{1 - \text{sgn}(\delta_m^{g_1})}{2} - \sum_{m=1}^{n_{g_2}} \text{sgn}(v_m^{g_2}) \frac{1 - \text{sgn}(\delta_m^{g_2})}{2} \\ & - \sum_{m=1}^{n_{h_1}} \text{sgn}(v_m^{h_1}) \frac{1 - \text{sgn}(\delta_m^{h_1})}{2} - \sum_{m=1}^{n_{h_2}} \text{sgn}(v_m^{h_2}) \frac{1 - \text{sgn}(\delta_m^{h_2})}{2} \end{aligned} \quad (\text{S157.5})$$

$$\mathcal{W}_1^{\text{gapped}} = - \sum_{m=1}^{n_{d_1}} \text{sgn}(v_m^{d_1}) \frac{1 - \text{sgn}(\delta_m^{d_1})}{2} + \sum_{m=1}^{n_{d_2}} \text{sgn}(v_m^{d_2}) \frac{1 - \text{sgn}(\delta_m^{d_2})}{2} \quad (\text{S157.6})$$

$$\mathcal{W}_2^{\text{gapped}} = - \sum_{m=1}^{n_{b_3}} \text{sgn}(v_m^{b_3}) \frac{1 - \text{sgn}(\delta_m^{b_3})}{2} + \sum_{m=1}^{n_{c_3}} \text{sgn}(v_m^{c_3}) \frac{1 - \text{sgn}(\delta_m^{c_3})}{2} \quad (\text{S157.7})$$

$$\begin{aligned} \mathcal{W}_3^{\text{gapped}} = & -2 \sum_{m=1}^{n_{a_2}} \text{sgn}(v_m^{a_2}) \frac{1 - \text{sgn}(\delta_m^{a_2})}{2} - 2 \sum_{m=1}^{n_{a_3}} \text{sgn}(v_m^{a_3}) \frac{1 - \text{sgn}(\delta_m^{a_3})}{2} + 2 \sum_{m=1}^{n_{d_2}} \text{sgn}(v_m^{d_2}) \frac{1 - \text{sgn}(\delta_m^{d_2})}{2} \\ & + \sum_{m=1}^{n_{e_1}} \text{sgn}(v_m^{e_1}) \frac{1 - \text{sgn}(\delta_m^{e_1})}{2} - 2 \sum_{m=1}^{n_{g_2}} \text{sgn}(v_m^{g_2}) \frac{1 - \text{sgn}(\delta_m^{g_2})}{2} - 2 \sum_{m=1}^{n_{h_1}} \text{sgn}(v_m^{h_1}) \frac{1 - \text{sgn}(\delta_m^{h_1})}{2} \end{aligned} \quad (\text{S157.8})$$

### S158. SPACE GROUP NO. 158

| line segment                                        | character of irrep (generators only)                                                                                                                                                        |
|-----------------------------------------------------|---------------------------------------------------------------------------------------------------------------------------------------------------------------------------------------------|
| $a \quad (0, 0, \frac{t}{2})$                       | $\{3_{001}   0 \ 0 \ 0\} \quad \{m_{100}   0 \ 0 \ \frac{1}{2}\}$<br>$a_1 \quad -1 \quad -ie^{-\frac{1}{2}i\pi t}$<br>$a_2 \quad -1 \quad ie^{-\frac{1}{2}i\pi t}$<br>$a_3 \quad 1 \quad 0$ |
| $b \quad (\frac{1}{3}, \frac{1}{3}, \frac{1-t}{2})$ | $\{3_{001}   0 \ 0 \ 0\}$<br>$b_1 \quad -1$<br>$b_2 \quad e^{-\frac{i\pi}{3}}$<br>$b_3 \quad e^{\frac{i\pi}{3}}$                                                                            |
| $c \quad (\frac{1}{2}, 0, \frac{t}{2})$             | $\{m_{010}   0 \ 0 \ \frac{1}{2}\}$<br>$c_1 \quad -ie^{-\frac{1}{2}i\pi t}$<br>$c_2 \quad ie^{-\frac{1}{2}i\pi t}$                                                                          |
| $d \quad (\frac{t}{3}, \frac{t}{3}, 0)$             | $\{1   0 \ 0 \ 0\}$<br>$d_1 \quad 1$                                                                                                                                                        |
| $e \quad (\frac{t}{3}, \frac{t}{3}, \frac{1}{2})$   | $\{1   0 \ 0 \ 0\}$<br>$e_1 \quad 1$                                                                                                                                                        |
| $f \quad (\frac{t}{2}, 0, \frac{1}{2})$             | $\{m_{010}   0 \ 0 \ \frac{1}{2}\}$<br>$f_1 \quad -1$<br>$f_2 \quad 1$                                                                                                                      |

|                                                       |                                                               |
|-------------------------------------------------------|---------------------------------------------------------------|
| $g \quad (\frac{t+2}{6}, \frac{1-t}{3}, 0)$           | $\begin{array}{c} \{1 0 \ 0 \ 0\} \\ g_1 \quad 1 \end{array}$ |
| $h \quad (\frac{t+2}{6}, \frac{1-t}{3}, \frac{1}{2})$ | $\begin{array}{c} \{1 0 \ 0 \ 0\} \\ h_1 \quad 1 \end{array}$ |

$$\begin{aligned} \mathcal{W}_1^{\text{gapless}} = & \sum_{m=1}^{n_{a_1}} \text{sgn}(v_m^{a_1}) \frac{1 - \text{sgn}(\delta_m^{a_1})}{2} + \sum_{m=1}^{n_{a_2}} \text{sgn}(v_m^{a_2}) \frac{1 - \text{sgn}(\delta_m^{a_2})}{2} + 2 \sum_{m=1}^{n_{a_3}} \text{sgn}(v_m^{a_3}) \frac{1 - \text{sgn}(\delta_m^{a_3})}{2} \\ & - \sum_{m=1}^{n_{c_1}} \text{sgn}(v_m^{c_1}) \frac{1 - \text{sgn}(\delta_m^{c_1})}{2} - \sum_{m=1}^{n_{c_2}} \text{sgn}(v_m^{c_2}) \frac{1 - \text{sgn}(\delta_m^{c_2})}{2} - \sum_{m=1}^{n_{d_1}} \text{sgn}(v_m^{d_1}) \frac{1 - \text{sgn}(\delta_m^{d_1})}{2} \\ & + \sum_{m=1}^{n_{f_1}} \text{sgn}(v_m^{f_1}) \frac{1 - \text{sgn}(\delta_m^{f_1})}{2} + \sum_{m=1}^{n_{f_2}} \text{sgn}(v_m^{f_2}) \frac{1 - \text{sgn}(\delta_m^{f_2})}{2} - \sum_{m=1}^{n_{g_1}} \text{sgn}(v_m^{g_1}) \frac{1 - \text{sgn}(\delta_m^{g_1})}{2} \end{aligned} \quad (\text{S158.1})$$

$$\begin{aligned} \mathcal{W}_2^{\text{gapless}} = & 2 \sum_{m=1}^{n_{a_2}} \text{sgn}(v_m^{a_2}) \frac{1 - \text{sgn}(\delta_m^{a_2})}{2} + 2 \sum_{m=1}^{n_{a_3}} \text{sgn}(v_m^{a_3}) \frac{1 - \text{sgn}(\delta_m^{a_3})}{2} - 2 \sum_{m=1}^{n_{c_1}} \text{sgn}(v_m^{c_1}) \frac{1 - \text{sgn}(\delta_m^{c_1})}{2} \\ & - \sum_{m=1}^{n_{d_1}} \text{sgn}(v_m^{d_1}) \frac{1 - \text{sgn}(\delta_m^{d_1})}{2} + 2 \sum_{m=1}^{n_{f_1}} \text{sgn}(v_m^{f_1}) \frac{1 - \text{sgn}(\delta_m^{f_1})}{2} - \sum_{m=1}^{n_{g_1}} \text{sgn}(v_m^{g_1}) \frac{1 - \text{sgn}(\delta_m^{g_1})}{2} \end{aligned} \quad (\text{S158.2})$$

$$\begin{aligned} \mathcal{W}_3^{\text{gapless}} = & \sum_{m=1}^{n_{b_1}} \text{sgn}(v_m^{b_1}) \frac{1 - \text{sgn}(\delta_m^{b_1})}{2} + \sum_{m=1}^{n_{b_2}} \text{sgn}(v_m^{b_2}) \frac{1 - \text{sgn}(\delta_m^{b_2})}{2} + \sum_{m=1}^{n_{b_3}} \text{sgn}(v_m^{b_3}) \frac{1 - \text{sgn}(\delta_m^{b_3})}{2} + \sum_{m=1}^{n_{c_1}} \text{sgn}(v_m^{c_1}) \frac{1 - \text{sgn}(\delta_m^{c_1})}{2} \\ & + \sum_{m=1}^{n_{c_2}} \text{sgn}(v_m^{c_2}) \frac{1 - \text{sgn}(\delta_m^{c_2})}{2} + \sum_{m=1}^{n_{g_1}} \text{sgn}(v_m^{g_1}) \frac{1 - \text{sgn}(\delta_m^{g_1})}{2} - 2 \sum_{m=1}^{n_{h_1}} \text{sgn}(v_m^{h_1}) \frac{1 - \text{sgn}(\delta_m^{h_1})}{2} \end{aligned} \quad (\text{S158.3})$$

$$\begin{aligned} \mathcal{W}_4^{\text{gapless}} = & 2 \sum_{m=1}^{n_{e_1}} \text{sgn}(v_m^{e_1}) \frac{1 - \text{sgn}(\delta_m^{e_1})}{2} - \sum_{m=1}^{n_{f_1}} \text{sgn}(v_m^{f_1}) \frac{1 - \text{sgn}(\delta_m^{f_1})}{2} - \sum_{m=1}^{n_{f_2}} \text{sgn}(v_m^{f_2}) \frac{1 - \text{sgn}(\delta_m^{f_2})}{2} \\ & + 2 \sum_{m=1}^{n_{h_1}} \text{sgn}(v_m^{h_1}) \frac{1 - \text{sgn}(\delta_m^{h_1})}{2} \end{aligned} \quad (\text{S158.4})$$

$$\mathcal{X}_1 = \sum_{m=1}^{n_{f_1}} \frac{1 - \text{sgn}(\delta_m^{f_1})}{2} \quad \text{mod } 2 \quad (\text{S158.5})$$

$$\mathcal{X}_2 = \sum_{m=1}^{n_{c_1}} \frac{1 - \text{sgn}(\delta_m^{c_1})}{2} + \sum_{m=1}^{n_{c_2}} \frac{1 - \text{sgn}(\delta_m^{c_2})}{2} + \sum_{m=1}^{n_{f_1}} \frac{1 - \text{sgn}(\delta_m^{f_1})}{2} \quad \text{mod } 2 \quad (\text{S158.6})$$

## S159. SPACE GROUP NO. 159

| line segment                                          | character of irrep (generators only)                              |
|-------------------------------------------------------|-------------------------------------------------------------------|
| $a \quad (0, 0, \frac{t}{2})$                         | $\{3_{001}   0 \ 0 \ 0\} \quad \{m_{210}   0 \ 0 \ \frac{1}{2}\}$ |
|                                                       | $a_1 \quad -1 \quad -ie^{-\frac{1}{2}i\pi t}$                     |
|                                                       | $a_2 \quad -1 \quad ie^{-\frac{1}{2}i\pi t}$                      |
|                                                       | $a_3 \quad 1 \quad 0$                                             |
| $b \quad (\frac{1}{3}, \frac{1}{3}, \frac{1-t}{2})$   | $\{3_{001}   0 \ 0 \ 0\} \quad \{m_{210}   0 \ 0 \ \frac{1}{2}\}$ |
|                                                       | $b_1 \quad -1 \quad -ie^{-\frac{1}{2}i\pi(1-t)}$                  |
|                                                       | $b_2 \quad -1 \quad ie^{-\frac{1}{2}i\pi(1-t)}$                   |
|                                                       | $b_3 \quad 1 \quad 0$                                             |
| $c \quad (\frac{1}{3}, \frac{1}{3}, \frac{t-1}{2})$   | $\{3_{001}   0 \ 0 \ 0\} \quad \{m_{210}   0 \ 0 \ \frac{1}{2}\}$ |
|                                                       | $c_1 \quad -1 \quad -ie^{-\frac{1}{2}i\pi(t-1)}$                  |
|                                                       | $c_2 \quad -1 \quad ie^{-\frac{1}{2}i\pi(t-1)}$                   |
|                                                       | $c_3 \quad 1 \quad 0$                                             |
| $d \quad (\frac{1}{2}, 0, \frac{t}{2})$               | $\{m_{210}   0 \ 0 \ \frac{1}{2}\}$                               |
|                                                       | $d_1 \quad -ie^{-\frac{1}{2}i\pi t}$                              |
|                                                       | $d_2 \quad ie^{-\frac{1}{2}i\pi t}$                               |
| $e \quad (\frac{t}{2}, 0, 0)$                         | $\{1   0 \ 0 \ 0\}$                                               |
|                                                       | $e_1 \quad 1$                                                     |
| $f \quad (\frac{t}{2}, 0, \frac{1}{2})$               | $\{1   0 \ 0 \ 0\}$                                               |
|                                                       | $f_1 \quad 1$                                                     |
| $g \quad (\frac{t}{3}, \frac{t}{3}, \frac{1}{2})$     | $\{m_{-110}   0 \ 0 \ \frac{1}{2}\}$                              |
|                                                       | $g_1 \quad -1$                                                    |
|                                                       | $g_2 \quad 1$                                                     |
| $h \quad (\frac{t+2}{6}, \frac{1-t}{3}, \frac{1}{2})$ | $\{m_{210}   0 \ 0 \ \frac{1}{2}\}$                               |
|                                                       | $h_1 \quad -1$                                                    |
|                                                       | $h_2 \quad 1$                                                     |

$$\begin{aligned}
\mathcal{W}_1^{\text{gapless}} = & \sum_{m=1}^{n_{a_1}} \text{sgn}(v_m^{a_1}) \frac{1 - \text{sgn}(\delta_m^{a_1})}{2} + \sum_{m=1}^{n_{a_2}} \text{sgn}(v_m^{a_2}) \frac{1 - \text{sgn}(\delta_m^{a_2})}{2} + 2 \sum_{m=1}^{n_{a_3}} \text{sgn}(v_m^{a_3}) \frac{1 - \text{sgn}(\delta_m^{a_3})}{2} \\
& - \sum_{m=1}^{n_{d_1}} \text{sgn}(v_m^{d_1}) \frac{1 - \text{sgn}(\delta_m^{d_1})}{2} - \sum_{m=1}^{n_{d_2}} \text{sgn}(v_m^{d_2}) \frac{1 - \text{sgn}(\delta_m^{d_2})}{2} - \sum_{m=1}^{n_{e_1}} \text{sgn}(v_m^{e_1}) \frac{1 - \text{sgn}(\delta_m^{e_1})}{2} \\
& + \sum_{m=1}^{n_{g_1}} \text{sgn}(v_m^{g_1}) \frac{1 - \text{sgn}(\delta_m^{g_1})}{2} + \sum_{m=1}^{n_{g_2}} \text{sgn}(v_m^{g_2}) \frac{1 - \text{sgn}(\delta_m^{g_2})}{2} + \sum_{m=1}^{n_{h_1}} \text{sgn}(v_m^{h_1}) \frac{1 - \text{sgn}(\delta_m^{h_1})}{2} \\
& + \sum_{m=1}^{n_{h_2}} \text{sgn}(v_m^{h_2}) \frac{1 - \text{sgn}(\delta_m^{h_2})}{2}
\end{aligned} \tag{S159.1}$$

$$\begin{aligned}
\mathcal{W}_2^{\text{gapless}} = & 2 \sum_{m=1}^{n_{a_2}} \text{sgn}(v_m^{a_2}) \frac{1 - \text{sgn}(\delta_m^{a_2})}{2} + 2 \sum_{m=1}^{n_{a_3}} \text{sgn}(v_m^{a_3}) \frac{1 - \text{sgn}(\delta_m^{a_3})}{2} - 2 \sum_{m=1}^{n_{d_2}} \text{sgn}(v_m^{d_2}) \frac{1 - \text{sgn}(\delta_m^{d_2})}{2} \\
& - \sum_{m=1}^{n_{e_1}} \text{sgn}(v_m^{e_1}) \frac{1 - \text{sgn}(\delta_m^{e_1})}{2} + 2 \sum_{m=1}^{n_{g_1}} \text{sgn}(v_m^{g_1}) \frac{1 - \text{sgn}(\delta_m^{g_1})}{2} + 2 \sum_{m=1}^{n_{h_2}} \text{sgn}(v_m^{h_2}) \frac{1 - \text{sgn}(\delta_m^{h_2})}{2}
\end{aligned} \tag{S159.2}$$

$$\begin{aligned}
\mathcal{W}_3^{\text{gapless}} = & \sum_{m=1}^{n_{b_1}} \text{sgn}(v_m^{b_1}) \frac{1 - \text{sgn}(\delta_m^{b_1})}{2} + \sum_{m=1}^{n_{b_3}} \text{sgn}(v_m^{b_3}) \frac{1 - \text{sgn}(\delta_m^{b_3})}{2} - \sum_{m=1}^{n_{c_1}} \text{sgn}(v_m^{c_1}) \frac{1 - \text{sgn}(\delta_m^{c_1})}{2} \\
& - \sum_{m=1}^{n_{c_3}} \text{sgn}(v_m^{c_3}) \frac{1 - \text{sgn}(\delta_m^{c_3})}{2} + \sum_{m=1}^{n_{d_1}} \text{sgn}(v_m^{d_1}) \frac{1 - \text{sgn}(\delta_m^{d_1})}{2} - \sum_{m=1}^{n_{d_2}} \text{sgn}(v_m^{d_2}) \frac{1 - \text{sgn}(\delta_m^{d_2})}{2} \\
& - \sum_{m=1}^{n_{h_1}} \text{sgn}(v_m^{h_1}) \frac{1 - \text{sgn}(\delta_m^{h_1})}{2} + \sum_{m=1}^{n_{h_2}} \text{sgn}(v_m^{h_2}) \frac{1 - \text{sgn}(\delta_m^{h_2})}{2}
\end{aligned} \tag{S159.3}$$

$$\begin{aligned}
\mathcal{W}_4^{\text{gapless}} = & \sum_{m=1}^{n_{b_2}} \text{sgn}(v_m^{b_2}) \frac{1 - \text{sgn}(\delta_m^{b_2})}{2} + \sum_{m=1}^{n_{b_3}} \text{sgn}(v_m^{b_3}) \frac{1 - \text{sgn}(\delta_m^{b_3})}{2} - \sum_{m=1}^{n_{c_2}} \text{sgn}(v_m^{c_2}) \frac{1 - \text{sgn}(\delta_m^{c_2})}{2} \\
& - \sum_{m=1}^{n_{c_3}} \text{sgn}(v_m^{c_3}) \frac{1 - \text{sgn}(\delta_m^{c_3})}{2} - \sum_{m=1}^{n_{d_1}} \text{sgn}(v_m^{d_1}) \frac{1 - \text{sgn}(\delta_m^{d_1})}{2} + \sum_{m=1}^{n_{d_2}} \text{sgn}(v_m^{d_2}) \frac{1 - \text{sgn}(\delta_m^{d_2})}{2} \\
& + \sum_{m=1}^{n_{h_1}} \text{sgn}(v_m^{h_1}) \frac{1 - \text{sgn}(\delta_m^{h_1})}{2} - \sum_{m=1}^{n_{h_2}} \text{sgn}(v_m^{h_2}) \frac{1 - \text{sgn}(\delta_m^{h_2})}{2}
\end{aligned} \tag{S159.4}$$

$$\begin{aligned}
\mathcal{W}_5^{\text{gapless}} = & 2 \sum_{m=1}^{n_{f_1}} \text{sgn}(v_m^{f_1}) \frac{1 - \text{sgn}(\delta_m^{f_1})}{2} - \sum_{m=1}^{n_{g_1}} \text{sgn}(v_m^{g_1}) \frac{1 - \text{sgn}(\delta_m^{g_1})}{2} - \sum_{m=1}^{n_{g_2}} \text{sgn}(v_m^{g_2}) \frac{1 - \text{sgn}(\delta_m^{g_2})}{2} \\
& - \sum_{m=1}^{n_{h_1}} \text{sgn}(v_m^{h_1}) \frac{1 - \text{sgn}(\delta_m^{h_1})}{2} - \sum_{m=1}^{n_{h_2}} \text{sgn}(v_m^{h_2}) \frac{1 - \text{sgn}(\delta_m^{h_2})}{2}
\end{aligned} \tag{S159.5}$$

$$\mathcal{W}_1^{\text{gapped}} = - \sum_{m=1}^{n_{b_3}} \text{sgn}(v_m^{b_3}) \frac{1 - \text{sgn}(\delta_m^{b_3})}{2} + \sum_{m=1}^{n_{c_3}} \text{sgn}(v_m^{c_3}) \frac{1 - \text{sgn}(\delta_m^{c_3})}{2} \tag{S159.6}$$

$$\mathcal{X}_1 = \sum_{m=1}^{n_{d_1}} \frac{1 - \text{sgn}(\delta_m^{d_1})}{2} + \sum_{m=1}^{n_{d_2}} \frac{1 - \text{sgn}(\delta_m^{d_2})}{2} \pmod{2} \tag{S159.7}$$

$$\mathcal{X}_2 = \sum_{m=1}^{n_{d_1}} \frac{1 - \text{sgn}(\delta_m^{d_1})}{2} + \sum_{m=1}^{n_{d_2}} \frac{1 - \text{sgn}(\delta_m^{d_2})}{2} + \sum_{m=1}^{n_{g_2}} \frac{1 - \text{sgn}(\delta_m^{g_2})}{2} + \sum_{m=1}^{n_{h_1}} \frac{1 - \text{sgn}(\delta_m^{h_1})}{2} \pmod{2} \tag{S159.8}$$

### S160. SPACE GROUP NO. 160

| line segment                              | character of irrep (generators only)                    |
|-------------------------------------------|---------------------------------------------------------|
| $a \quad (0, 0, \frac{3t}{2})$            | $\{3_{001}   0 \ 0 \ 0\} \quad \{m_{100}   0 \ 0 \ 0\}$ |
|                                           | $a_1 \quad -1 \quad -i$                                 |
|                                           | $a_2 \quad -1 \quad i$                                  |
|                                           | $a_3 \quad 1 \quad 0$                                   |
| $b \quad (0, \frac{t}{2}, \frac{3-t}{2})$ | $\{m_{100}   0 \ 0 \ 0\}$                               |
|                                           | $b_1 \quad -i$                                          |
|                                           | $b_2 \quad i$                                           |

|                                             |                                                               |
|---------------------------------------------|---------------------------------------------------------------|
| $c \quad (\frac{t}{2}, 0, \frac{3}{2} - t)$ | $\{m_{01-1}   0 \ 0 \ 0\}$<br>$c_1 \quad -i$<br>$c_2 \quad i$ |
| $d \quad (0, t, \frac{t}{2})$               | $\{m_{100}   0 \ 0 \ 0\}$<br>$d_1 \quad -i$<br>$d_2 \quad i$  |
| $e \quad (\frac{t}{2}, \frac{t}{2}, 0)$     | $\{1   0 \ 0 \ 0\}$<br>$e_1 \quad 1$                          |
| $f \quad (\frac{1-t}{2}, t, \frac{1}{2})$   | $\{1   0 \ 0 \ 0\}$<br>$f_1 \quad 1$                          |

$$\begin{aligned} \mathcal{W}_1^{\text{gapless}} = & \sum_{m=1}^{n_{a_1}} \text{sgn}(v_m^{a_1}) \frac{1 - \text{sgn}(\delta_m^{a_1})}{2} + \sum_{m=1}^{n_{a_3}} \text{sgn}(v_m^{a_3}) \frac{1 - \text{sgn}(\delta_m^{a_3})}{2} + 2 \sum_{m=1}^{n_{c_2}} \text{sgn}(v_m^{c_2}) \frac{1 - \text{sgn}(\delta_m^{c_2})}{2} \\ & - \sum_{m=1}^{n_{d_2}} \text{sgn}(v_m^{d_2}) \frac{1 - \text{sgn}(\delta_m^{d_2})}{2} + \sum_{m=1}^{n_{f_1}} \text{sgn}(v_m^{f_1}) \frac{1 - \text{sgn}(\delta_m^{f_1})}{2} \end{aligned} \quad (\text{S160.1})$$

$$\begin{aligned} \mathcal{W}_2^{\text{gapless}} = & \sum_{m=1}^{n_{a_2}} \text{sgn}(v_m^{a_2}) \frac{1 - \text{sgn}(\delta_m^{a_2})}{2} + \sum_{m=1}^{n_{a_3}} \text{sgn}(v_m^{a_3}) \frac{1 - \text{sgn}(\delta_m^{a_3})}{2} - 2 \sum_{m=1}^{n_{c_2}} \text{sgn}(v_m^{c_2}) \frac{1 - \text{sgn}(\delta_m^{c_2})}{2} \\ & - \sum_{m=1}^{n_{d_1}} \text{sgn}(v_m^{d_1}) \frac{1 - \text{sgn}(\delta_m^{d_1})}{2} - \sum_{m=1}^{n_{f_1}} \text{sgn}(v_m^{f_1}) \frac{1 - \text{sgn}(\delta_m^{f_1})}{2} \end{aligned} \quad (\text{S160.2})$$

$$\begin{aligned} \mathcal{W}_3^{\text{gapless}} = & \sum_{m=1}^{n_{b_1}} \text{sgn}(v_m^{b_1}) \frac{1 - \text{sgn}(\delta_m^{b_1})}{2} + \sum_{m=1}^{n_{b_2}} \text{sgn}(v_m^{b_2}) \frac{1 - \text{sgn}(\delta_m^{b_2})}{2} + \sum_{m=1}^{n_{d_1}} \text{sgn}(v_m^{d_1}) \frac{1 - \text{sgn}(\delta_m^{d_1})}{2} \\ & + \sum_{m=1}^{n_{d_2}} \text{sgn}(v_m^{d_2}) \frac{1 - \text{sgn}(\delta_m^{d_2})}{2} - \sum_{m=1}^{n_{e_1}} \text{sgn}(v_m^{e_1}) \frac{1 - \text{sgn}(\delta_m^{e_1})}{2} \end{aligned} \quad (\text{S160.3})$$

$$\begin{aligned} \mathcal{W}_4^{\text{gapless}} = & 2 \sum_{m=1}^{n_{b_2}} \text{sgn}(v_m^{b_2}) \frac{1 - \text{sgn}(\delta_m^{b_2})}{2} + 2 \sum_{m=1}^{n_{c_2}} \text{sgn}(v_m^{c_2}) \frac{1 - \text{sgn}(\delta_m^{c_2})}{2} \\ & + 2 \sum_{m=1}^{n_{d_1}} \text{sgn}(v_m^{d_1}) \frac{1 - \text{sgn}(\delta_m^{d_1})}{2} - \sum_{m=1}^{n_{e_1}} \text{sgn}(v_m^{e_1}) \frac{1 - \text{sgn}(\delta_m^{e_1})}{2} + \sum_{m=1}^{n_{f_1}} \text{sgn}(v_m^{f_1}) \frac{1 - \text{sgn}(\delta_m^{f_1})}{2} \end{aligned} \quad (\text{S160.4})$$

$$\mathcal{W}_5^{\text{gapless}} = \sum_{m=1}^{n_{c_1}} \text{sgn}(v_m^{c_1}) \frac{1 - \text{sgn}(\delta_m^{c_1})}{2} + \sum_{m=1}^{n_{c_2}} \text{sgn}(v_m^{c_2}) \frac{1 - \text{sgn}(\delta_m^{c_2})}{2} + \sum_{m=1}^{n_{f_1}} \text{sgn}(v_m^{f_1}) \frac{1 - \text{sgn}(\delta_m^{f_1})}{2} \quad (\text{S160.5})$$

$$\mathcal{W}_1^{\text{gapped}} = - \sum_{m=1}^{n_{d_1}} \text{sgn}(v_m^{d_1}) \frac{1 - \text{sgn}(\delta_m^{d_1})}{2} + \sum_{m=1}^{n_{d_2}} \text{sgn}(v_m^{d_2}) \frac{1 - \text{sgn}(\delta_m^{d_2})}{2} \quad (\text{S160.6})$$

$$\mathcal{W}_2^{\text{gapped}} = -2 \sum_{m=1}^{n_{b_2}} \text{sgn}(v_m^{b_2}) \frac{1 - \text{sgn}(\delta_m^{b_2})}{2} - 2 \sum_{m=1}^{n_{d_1}} \text{sgn}(v_m^{d_1}) \frac{1 - \text{sgn}(\delta_m^{d_1})}{2} + \sum_{m=1}^{n_{e_1}} \text{sgn}(v_m^{e_1}) \frac{1 - \text{sgn}(\delta_m^{e_1})}{2} \quad (\text{S160.7})$$

## S161. SPACE GROUP NO. 161

| line segment                                | character of irrep (generators only)                                                                                                                                                        |
|---------------------------------------------|---------------------------------------------------------------------------------------------------------------------------------------------------------------------------------------------|
| $a \quad (0, 0, \frac{3t}{2})$              | $\{3_{001}   0 \ 0 \ 0\} \quad \{m_{100}   0 \ 0 \ \frac{1}{2}\}$<br>$a_1 \quad -1 \quad -ie^{-\frac{3}{2}i\pi t}$<br>$a_2 \quad -1 \quad ie^{-\frac{3}{2}i\pi t}$<br>$a_3 \quad 1 \quad 0$ |
| $b \quad (0, \frac{t}{2}, \frac{3-t}{2})$   | $\{m_{100}   0 \ 0 \ \frac{1}{2}\}$<br>$b_1 \quad -ie^{-\frac{1}{2}i\pi(3-t)}$<br>$b_2 \quad ie^{-\frac{1}{2}i\pi(3-t)}$                                                                    |
| $c \quad (\frac{t}{2}, 0, \frac{3}{2} - t)$ | $\{m_{01-1}   0 \ 0 \ \frac{1}{2}\}$<br>$c_1 \quad -ie^{-\frac{1}{2}i\pi(3-2t)}$<br>$c_2 \quad ie^{-\frac{1}{2}i\pi(3-2t)}$                                                                 |
| $d \quad (0, t, \frac{t}{2})$               | $\{m_{100}   0 \ 0 \ \frac{1}{2}\}$<br>$d_1 \quad -ie^{-\frac{1}{2}i\pi t}$<br>$d_2 \quad ie^{-\frac{1}{2}i\pi t}$                                                                          |
| $e \quad (\frac{t}{2}, \frac{t}{2}, 0)$     | $\{1   0 \ 0 \ 0\}$<br>$e_1 \quad 1$                                                                                                                                                        |
| $f \quad (\frac{1-t}{2}, t, \frac{1}{2})$   | $\{1   0 \ 0 \ 0\}$<br>$f_1 \quad 1$                                                                                                                                                        |

$$\mathcal{W}_1^{\text{gapless}} = \sum_{m=1}^{n_{a_1}} \text{sgn}(v_m^{a_1}) \frac{1 - \text{sgn}(\delta_m^{a_1})}{2} + \sum_{m=1}^{n_{a_3}} \text{sgn}(v_m^{a_3}) \frac{1 - \text{sgn}(\delta_m^{a_3})}{2} - \sum_{m=1}^{n_{d_2}} \text{sgn}(v_m^{d_2}) \frac{1 - \text{sgn}(\delta_m^{d_2})}{2} \quad (\text{S161.1})$$

$$\mathcal{W}_2^{\text{gapless}} = \sum_{m=1}^{n_{a_2}} \text{sgn}(v_m^{a_2}) \frac{1 - \text{sgn}(\delta_m^{a_2})}{2} + \sum_{m=1}^{n_{a_3}} \text{sgn}(v_m^{a_3}) \frac{1 - \text{sgn}(\delta_m^{a_3})}{2} - \sum_{m=1}^{n_{d_1}} \text{sgn}(v_m^{d_1}) \frac{1 - \text{sgn}(\delta_m^{d_1})}{2} \quad (\text{S161.2})$$

$$\begin{aligned} \mathcal{W}_3^{\text{gapless}} = & \sum_{m=1}^{n_{b_1}} \text{sgn}(v_m^{b_1}) \frac{1 - \text{sgn}(\delta_m^{b_1})}{2} + \sum_{m=1}^{n_{b_2}} \text{sgn}(v_m^{b_2}) \frac{1 - \text{sgn}(\delta_m^{b_2})}{2} + \sum_{m=1}^{n_{d_1}} \text{sgn}(v_m^{d_1}) \frac{1 - \text{sgn}(\delta_m^{d_1})}{2} \\ & + \sum_{m=1}^{n_{d_2}} \text{sgn}(v_m^{d_2}) \frac{1 - \text{sgn}(\delta_m^{d_2})}{2} - \sum_{m=1}^{n_{e_1}} \text{sgn}(v_m^{e_1}) \frac{1 - \text{sgn}(\delta_m^{e_1})}{2} \end{aligned} \quad (\text{S161.3})$$

$$\mathcal{W}_4^{\text{gapless}} = 2 \sum_{m=1}^{n_{b_2}} \text{sgn}(v_m^{b_2}) \frac{1 - \text{sgn}(\delta_m^{b_2})}{2} + 2 \sum_{m=1}^{n_{d_1}} \text{sgn}(v_m^{d_1}) \frac{1 - \text{sgn}(\delta_m^{d_1})}{2} - \sum_{m=1}^{n_{e_1}} \text{sgn}(v_m^{e_1}) \frac{1 - \text{sgn}(\delta_m^{e_1})}{2} \quad (\text{S161.4})$$

$$\mathcal{W}_5^{\text{gapless}} = \sum_{m=1}^{n_{c_1}} \text{sgn}(v_m^{c_1}) \frac{1 - \text{sgn}(\delta_m^{c_1})}{2} + \sum_{m=1}^{n_{c_2}} \text{sgn}(v_m^{c_2}) \frac{1 - \text{sgn}(\delta_m^{c_2})}{2} + 2 \sum_{m=1}^{n_{f_1}} \text{sgn}(v_m^{f_1}) \frac{1 - \text{sgn}(\delta_m^{f_1})}{2} \quad (\text{S161.5})$$

$$\mathcal{X}_1 = \sum_{m=1}^{n_{c_2}} \frac{1 - \text{sgn}(\delta_m^{c_2})}{2} \quad \text{mod } 2 \quad (\text{S161.6})$$

$$\mathcal{X}_2 = \sum_{m=1}^{n_{c_2}} \frac{1 - \text{sgn}(\delta_m^{c_2})}{2} + \sum_{m=1}^{n_{d_1}} \frac{1 - \text{sgn}(\delta_m^{d_1})}{2} + \sum_{m=1}^{n_{d_2}} \frac{1 - \text{sgn}(\delta_m^{d_2})}{2} \quad \text{mod } 2 \quad (\text{S161.7})$$

## S162. SPACE GROUP NO. 162

| line segment                                          | character of irrep (generators only)                                                                                                                     |
|-------------------------------------------------------|----------------------------------------------------------------------------------------------------------------------------------------------------------|
| $a \quad (0, 0, \frac{t}{2})$                         | $\begin{array}{c} \{3_{001} 0 \ 0 \ 0\} \quad \{m_{210} 0 \ 0 \ 0\} \\ a_1 \quad -1 \quad -i \\ a_2 \quad -1 \quad i \\ a_3 \quad 1 \quad 0 \end{array}$ |
| $b \quad (\frac{1}{3}, \frac{1}{3}, \frac{1-t}{2})$   | $\begin{array}{c} \{3_{001} 0 \ 0 \ 0\} \quad \{m_{210} 0 \ 0 \ 0\} \\ b_1 \quad -1 \quad -i \\ b_2 \quad -1 \quad i \\ b_3 \quad 1 \quad 0 \end{array}$ |
| $c \quad (\frac{1}{3}, \frac{1}{3}, \frac{t-1}{2})$   | $\begin{array}{c} \{3_{001} 0 \ 0 \ 0\} \quad \{m_{210} 0 \ 0 \ 0\} \\ c_1 \quad -1 \quad -i \\ c_2 \quad -1 \quad i \\ c_3 \quad 1 \quad 0 \end{array}$ |
| $d \quad (\frac{1}{2}, 0, \frac{t}{2})$               | $\begin{array}{c} \{m_{210} 0 \ 0 \ 0\} \\ d_1 \quad -i \\ d_2 \quad i \end{array}$                                                                      |
| $e \quad (\frac{t}{2}, 0, 0)$                         | $\begin{array}{c} \{2_{210} 0 \ 0 \ 0\} \\ e_1 \quad -i \\ e_2 \quad i \end{array}$                                                                      |
| $f \quad (\frac{t}{2}, 0, \frac{1}{2})$               | $\begin{array}{c} \{2_{210} 0 \ 0 \ 0\} \\ f_1 \quad -i \\ f_2 \quad i \end{array}$                                                                      |
| $g \quad (\frac{t}{3}, \frac{t}{3}, \frac{1}{2})$     | $\begin{array}{c} \{m_{-110} 0 \ 0 \ 0\} \\ g_1 \quad -i \\ g_2 \quad i \end{array}$                                                                     |
| $h \quad (\frac{t+2}{6}, \frac{1-t}{3}, \frac{1}{2})$ | $\begin{array}{c} \{m_{210} 0 \ 0 \ 0\} \\ h_1 \quad -i \\ h_2 \quad i \end{array}$                                                                      |

$$\begin{aligned} \mathcal{W}_1^{\text{gapless}} = & \sum_{m=1}^{n_{a_1}} \text{sgn}(v_m^{a_1}) \frac{1 - \text{sgn}(\delta_m^{a_1})}{2} + \sum_{m=1}^{n_{a_3}} \text{sgn}(v_m^{a_3}) \frac{1 - \text{sgn}(\delta_m^{a_3})}{2} - \sum_{m=1}^{n_{d_1}} \text{sgn}(v_m^{d_1}) \frac{1 - \text{sgn}(\delta_m^{d_1})}{2} \\ & - \sum_{m=1}^{n_{e_1}} \text{sgn}(v_m^{e_1}) \frac{1 - \text{sgn}(\delta_m^{e_1})}{2} + \sum_{m=1}^{n_{g_1}} \text{sgn}(v_m^{g_1}) \frac{1 - \text{sgn}(\delta_m^{g_1})}{2} + \sum_{m=1}^{n_{h_1}} \text{sgn}(v_m^{h_1}) \frac{1 - \text{sgn}(\delta_m^{h_1})}{2} \end{aligned} \quad (\text{S162.1})$$

$$\mathcal{W}_2^{\text{gapless}} = \sum_{m=1}^{n_{b_1}} \text{sgn}(v_m^{b_1}) \frac{1 - \text{sgn}(\delta_m^{b_1})}{2} + \sum_{m=1}^{n_{b_3}} \text{sgn}(v_m^{b_3}) \frac{1 - \text{sgn}(\delta_m^{b_3})}{2} - \sum_{m=1}^{n_{c_1}} \text{sgn}(v_m^{c_1}) \frac{1 - \text{sgn}(\delta_m^{c_1})}{2} - \sum_{m=1}^{n_{c_3}} \text{sgn}(v_m^{c_3}) \frac{1 - \text{sgn}(\delta_m^{c_3})}{2} \quad (\text{S162.2})$$

$$\mathcal{W}_3^{\text{gapless}} = \sum_{m=1}^{n_{f_1}} \text{sgn}(v_m^{f_1}) \frac{1 - \text{sgn}(\delta_m^{f_1})}{2} - \sum_{m=1}^{n_{g_1}} \text{sgn}(v_m^{g_1}) \frac{1 - \text{sgn}(\delta_m^{g_1})}{2} - \sum_{m=1}^{n_{h_1}} \text{sgn}(v_m^{h_1}) \frac{1 - \text{sgn}(\delta_m^{h_1})}{2} \quad (\text{S162.3})$$

$$\mathcal{W}_1^{\text{gapped}} = - \sum_{m=1}^{n_{b_3}} \text{sgn}(v_m^{b_3}) \frac{1 - \text{sgn}(\delta_m^{b_3})}{2} + \sum_{m=1}^{n_{c_3}} \text{sgn}(v_m^{c_3}) \frac{1 - \text{sgn}(\delta_m^{c_3})}{2} \quad (\text{S162.4})$$



## S163. SPACE GROUP NO. 163

| line segment                                          | character of irrep (generators only)                                                                                                                                                              |
|-------------------------------------------------------|---------------------------------------------------------------------------------------------------------------------------------------------------------------------------------------------------|
| $a \quad (0, 0, \frac{t}{2})$                         | $\{3_{001}   0 \ 0 \ 0\} \quad \{m_{210}   0 \ 0 \ \frac{1}{2}\}$<br>$a_1 \quad -1 \quad -ie^{-\frac{1}{2}i\pi t}$<br>$a_2 \quad -1 \quad ie^{-\frac{1}{2}i\pi t}$<br>$a_3 \quad 1 \quad 0$       |
| $b \quad (\frac{1}{3}, \frac{1}{3}, \frac{1-t}{2})$   | $\{3_{001}   0 \ 0 \ 0\} \quad \{m_{210}   0 \ 0 \ \frac{1}{2}\}$<br>$b_1 \quad -1 \quad -ie^{-\frac{1}{2}i\pi(1-t)}$<br>$b_2 \quad -1 \quad ie^{-\frac{1}{2}i\pi(1-t)}$<br>$b_3 \quad 1 \quad 0$ |
| $c \quad (\frac{1}{3}, \frac{1}{3}, \frac{t-1}{2})$   | $\{3_{001}   0 \ 0 \ 0\} \quad \{m_{210}   0 \ 0 \ \frac{1}{2}\}$<br>$c_1 \quad -1 \quad -ie^{-\frac{1}{2}i\pi(t-1)}$<br>$c_2 \quad -1 \quad ie^{-\frac{1}{2}i\pi(t-1)}$<br>$c_3 \quad 1 \quad 0$ |
| $d \quad (\frac{1}{2}, 0, \frac{t}{2})$               | $\{m_{210}   0 \ 0 \ \frac{1}{2}\}$<br>$d_1 \quad -ie^{-\frac{1}{2}i\pi t}$<br>$d_2 \quad ie^{-\frac{1}{2}i\pi t}$                                                                                |
| $e \quad (\frac{t}{2}, 0, 0)$                         | $\{2_{210}   0 \ 0 \ \frac{1}{2}\}$<br>$e_1 \quad -i$<br>$e_2 \quad i$                                                                                                                            |
| $f \quad (\frac{t}{2}, 0, \frac{1}{2})$               | $\{2_{210}   0 \ 0 \ \frac{1}{2}\}$<br>$f_1 \quad i$<br>$f_2 \quad -i$                                                                                                                            |
| $g \quad (\frac{t}{3}, \frac{t}{3}, \frac{1}{2})$     | $\{m_{-110}   0 \ 0 \ \frac{1}{2}\}$<br>$g_1 \quad -1$<br>$g_2 \quad 1$                                                                                                                           |
| $h \quad (\frac{t+2}{6}, \frac{1-t}{3}, \frac{1}{2})$ | $\{m_{210}   0 \ 0 \ \frac{1}{2}\}$<br>$h_1 \quad -1$<br>$h_2 \quad 1$                                                                                                                            |

$$\begin{aligned} \mathcal{W}_1^{\text{gapless}} = & \sum_{m=1}^{n_{a_1}} \text{sgn}(v_m^{a_1}) \frac{1 - \text{sgn}(\delta_m^{a_1})}{2} + \sum_{m=1}^{n_{a_3}} \text{sgn}(v_m^{a_3}) \frac{1 - \text{sgn}(\delta_m^{a_3})}{2} - \sum_{m=1}^{n_{d_1}} \text{sgn}(v_m^{d_1}) \frac{1 - \text{sgn}(\delta_m^{d_1})}{2} \\ & - \sum_{m=1}^{n_{e_1}} \text{sgn}(v_m^{e_1}) \frac{1 - \text{sgn}(\delta_m^{e_1})}{2} + \sum_{m=1}^{n_{g_1}} \text{sgn}(v_m^{g_1}) \frac{1 - \text{sgn}(\delta_m^{g_1})}{2} + \sum_{m=1}^{n_{h_1}} \text{sgn}(v_m^{h_1}) \frac{1 - \text{sgn}(\delta_m^{h_1})}{2} \end{aligned} \quad (\text{S163.1})$$

$$\begin{aligned} \mathcal{W}_2^{\text{gapless}} = & \sum_{m=1}^{n_{b_1}} \text{sgn}(v_m^{b_1}) \frac{1 - \text{sgn}(\delta_m^{b_1})}{2} + \sum_{m=1}^{n_{b_3}} \text{sgn}(v_m^{b_3}) \frac{1 - \text{sgn}(\delta_m^{b_3})}{2} - \sum_{m=1}^{n_{c_1}} \text{sgn}(v_m^{c_1}) \frac{1 - \text{sgn}(\delta_m^{c_1})}{2} - \sum_{m=1}^{n_{c_3}} \text{sgn}(v_m^{c_3}) \frac{1 - \text{sgn}(\delta_m^{c_3})}{2} \end{aligned} \quad (\text{S163.2})$$

$$\begin{aligned} \mathcal{W}_3^{\text{gapless}} = & \sum_{m=1}^{n_{f_1}} \text{sgn}(v_m^{f_1}) \frac{1 - \text{sgn}(\delta_m^{f_1})}{2} + \sum_{m=1}^{n_{f_2}} \text{sgn}(v_m^{f_2}) \frac{1 - \text{sgn}(\delta_m^{f_2})}{2} - \sum_{m=1}^{n_{g_1}} \text{sgn}(v_m^{g_1}) \frac{1 - \text{sgn}(\delta_m^{g_1})}{2} - \sum_{m=1}^{n_{h_1}} \text{sgn}(v_m^{h_1}) \frac{1 - \text{sgn}(\delta_m^{h_1})}{2} \end{aligned} \quad (\text{S163.3})$$

$$\mathcal{W}_1^{\text{gapped}} = - \sum_{m=1}^{n_{b_3}} \text{sgn}(v_m^{b_3}) \frac{1 - \text{sgn}(\delta_m^{b_3})}{2} + \sum_{m=1}^{n_{c_3}} \text{sgn}(v_m^{c_3}) \frac{1 - \text{sgn}(\delta_m^{c_3})}{2} \quad (\text{S163.4})$$

$$\mathcal{W}_2^{\text{gapped}} = -2 \sum_{m=1}^{n_{f_2}} \text{sgn}(v_m^{f_2}) \frac{1 - \text{sgn}(\delta_m^{f_2})}{2} + \sum_{m=1}^{n_{g_1}} \text{sgn}(v_m^{g_1}) \frac{1 - \text{sgn}(\delta_m^{g_1})}{2} + \sum_{m=1}^{n_{h_1}} \text{sgn}(v_m^{h_1}) \frac{1 - \text{sgn}(\delta_m^{h_1})}{2} \quad (\text{S163.5})$$

**S164. SPACE GROUP NO. 164**

| line segment                                          | character of irrep (generators only)                                                                                              |
|-------------------------------------------------------|-----------------------------------------------------------------------------------------------------------------------------------|
| $a \quad (0, 0, \frac{t}{2})$                         | $\{3_{001}  0 \ 0 \ 0 \}$ $\{m_{100}  0 \ 0 \ 0 \}$<br>$a_1 \quad -1 \quad -i$<br>$a_2 \quad -1 \quad i$<br>$a_3 \quad 1 \quad 0$ |
| $b \quad (\frac{1}{3}, \frac{1}{3}, \frac{1-t}{2})$   | $\{3_{001}  0 \ 0 \ 0 \}$<br>$b_1 \quad -1$<br>$b_2 \quad e^{-\frac{i\pi}{3}}$<br>$b_3 \quad e^{\frac{i\pi}{3}}$                  |
| $c \quad (\frac{1}{2}, 0, \frac{t}{2})$               | $\{m_{010}  0 \ 0 \ 0 \}$<br>$c_1 \quad -i$<br>$c_2 \quad i$                                                                      |
| $d \quad (\frac{t}{3}, \frac{t}{3}, 0)$               | $\{2_{110}  0 \ 0 \ 0 \}$<br>$d_1 \quad -i$<br>$d_2 \quad i$                                                                      |
| $e \quad (\frac{t}{3}, \frac{t}{3}, \frac{1}{2})$     | $\{2_{110}  0 \ 0 \ 0 \}$<br>$e_1 \quad -i$<br>$e_2 \quad i$                                                                      |
| $f \quad (\frac{t}{2}, 0, \frac{1}{2})$               | $\{m_{010}  0 \ 0 \ 0 \}$<br>$f_1 \quad -i$<br>$f_2 \quad i$                                                                      |
| $g \quad (\frac{t+2}{6}, \frac{1-t}{3}, 0)$           | $\{2_{010}  0 \ 0 \ 0 \}$<br>$g_1 \quad -i$<br>$g_2 \quad i$                                                                      |
| $h \quad (\frac{t+2}{6}, \frac{1-t}{3}, \frac{1}{2})$ | $\{2_{010}  0 \ 0 \ 0 \}$<br>$h_1 \quad -i$<br>$h_2 \quad i$                                                                      |

$$\begin{aligned}
\mathcal{W}_1^{\text{gapless}} = & \sum_{m=1}^{n_{a_1}} \text{sgn}(v_m^{a_1}) \frac{1 - \text{sgn}(\delta_m^{a_1})}{2} + \sum_{m=1}^{n_{a_3}} \text{sgn}(v_m^{a_3}) \frac{1 - \text{sgn}(\delta_m^{a_3})}{2} - \sum_{m=1}^{n_{c_1}} \text{sgn}(v_m^{c_1}) \frac{1 - \text{sgn}(\delta_m^{c_1})}{2} \\
& - \sum_{m=1}^{n_{d_1}} \text{sgn}(v_m^{d_1}) \frac{1 - \text{sgn}(\delta_m^{d_1})}{2} + \sum_{m=1}^{n_{f_1}} \text{sgn}(v_m^{f_1}) \frac{1 - \text{sgn}(\delta_m^{f_1})}{2} - \sum_{m=1}^{n_{g_1}} \text{sgn}(v_m^{g_1}) \frac{1 - \text{sgn}(\delta_m^{g_1})}{2}
\end{aligned} \tag{S164.1}$$

$$\begin{aligned}
\mathcal{W}_2^{\text{gapless}} = & \sum_{m=1}^{n_{b_1}} \text{sgn}(v_m^{b_1}) \frac{1 - \text{sgn}(\delta_m^{b_1})}{2} + \sum_{m=1}^{n_{b_2}} \text{sgn}(v_m^{b_2}) \frac{1 - \text{sgn}(\delta_m^{b_2})}{2} + \sum_{m=1}^{n_{c_1}} \text{sgn}(v_m^{c_1}) \frac{1 - \text{sgn}(\delta_m^{c_1})}{2} \\
& + \sum_{m=1}^{n_{g_1}} \text{sgn}(v_m^{g_1}) \frac{1 - \text{sgn}(\delta_m^{g_1})}{2} - \sum_{m=1}^{n_{h_1}} \text{sgn}(v_m^{h_1}) \frac{1 - \text{sgn}(\delta_m^{h_1})}{2}
\end{aligned} \tag{S164.2}$$

$$\mathcal{W}_3^{\text{gapless}} = \sum_{m=1}^{n_{e_1}} \text{sgn}(v_m^{e_1}) \frac{1 - \text{sgn}(\delta_m^{e_1})}{2} - \sum_{m=1}^{n_{f_1}} \text{sgn}(v_m^{f_1}) \frac{1 - \text{sgn}(\delta_m^{f_1})}{2} + \sum_{m=1}^{n_{h_1}} \text{sgn}(v_m^{h_1}) \frac{1 - \text{sgn}(\delta_m^{h_1})}{2} \tag{S164.3}$$

**S165. SPACE GROUP NO. 165**

| line segment | character of irrep (generators only) |
|--------------|--------------------------------------|
|--------------|--------------------------------------|

|                                                       |                                                                                                                                                                                               |
|-------------------------------------------------------|-----------------------------------------------------------------------------------------------------------------------------------------------------------------------------------------------|
| $a \quad (0, 0, \frac{t}{2})$                         | $\{3_{001}   0 \ 0 \ 0 \} \quad \{m_{100}   0 \ 0 \ \frac{1}{2} \}$<br>$a_1 \quad -1 \quad -ie^{-\frac{1}{2}i\pi t}$<br>$a_2 \quad -1 \quad ie^{-\frac{1}{2}i\pi t}$<br>$a_3 \quad 1 \quad 0$ |
| $b \quad (\frac{1}{3}, \frac{1}{3}, \frac{1-t}{2})$   | $\{3_{001}   0 \ 0 \ 0 \}$<br>$b_1 \quad -1$<br>$b_2 \quad e^{-\frac{i\pi}{3}}$<br>$b_3 \quad e^{\frac{i\pi}{3}}$                                                                             |
| $c \quad (\frac{1}{2}, 0, \frac{t}{2})$               | $\{m_{010}   0 \ 0 \ \frac{1}{2} \}$<br>$c_1 \quad -ie^{-\frac{1}{2}i\pi t}$<br>$c_2 \quad ie^{-\frac{1}{2}i\pi t}$                                                                           |
| $d \quad (\frac{t}{3}, \frac{t}{3}, 0)$               | $\{2_{110}   0 \ 0 \ \frac{1}{2} \}$<br>$d_1 \quad -i$<br>$d_2 \quad i$                                                                                                                       |
| $e \quad (\frac{t}{3}, \frac{t}{3}, \frac{1}{2})$     | $\{2_{110}   0 \ 0 \ \frac{1}{2} \}$<br>$e_1 \quad i$<br>$e_2 \quad -i$                                                                                                                       |
| $f \quad (\frac{t}{2}, 0, \frac{1}{2})$               | $\{m_{010}   0 \ 0 \ \frac{1}{2} \}$<br>$f_1 \quad -1$<br>$f_2 \quad 1$                                                                                                                       |
| $g \quad (\frac{t+2}{6}, \frac{1-t}{3}, 0)$           | $\{2_{010}   0 \ 0 \ \frac{1}{2} \}$<br>$g_1 \quad -i$<br>$g_2 \quad i$                                                                                                                       |
| $h \quad (\frac{t+2}{6}, \frac{1-t}{3}, \frac{1}{2})$ | $\{2_{010}   0 \ 0 \ \frac{1}{2} \}$<br>$h_1 \quad i$<br>$h_2 \quad -i$                                                                                                                       |

$$\begin{aligned} \mathcal{W}_1^{\text{gapless}} = & \sum_{m=1}^{n_{a_1}} \text{sgn}(v_m^{a_1}) \frac{1 - \text{sgn}(\delta_m^{a_1})}{2} + \sum_{m=1}^{n_{a_3}} \text{sgn}(v_m^{a_3}) \frac{1 - \text{sgn}(\delta_m^{a_3})}{2} - \sum_{m=1}^{n_{c_1}} \text{sgn}(v_m^{c_1}) \frac{1 - \text{sgn}(\delta_m^{c_1})}{2} \\ & - \sum_{m=1}^{n_{d_1}} \text{sgn}(v_m^{d_1}) \frac{1 - \text{sgn}(\delta_m^{d_1})}{2} + \sum_{m=1}^{n_{f_1}} \text{sgn}(v_m^{f_1}) \frac{1 - \text{sgn}(\delta_m^{f_1})}{2} - \sum_{m=1}^{n_{g_1}} \text{sgn}(v_m^{g_1}) \frac{1 - \text{sgn}(\delta_m^{g_1})}{2} \end{aligned} \quad (\text{S165.1})$$

$$\begin{aligned} \mathcal{W}_2^{\text{gapless}} = & \sum_{m=1}^{n_{b_1}} \text{sgn}(v_m^{b_1}) \frac{1 - \text{sgn}(\delta_m^{b_1})}{2} + \sum_{m=1}^{n_{b_2}} \text{sgn}(v_m^{b_2}) \frac{1 - \text{sgn}(\delta_m^{b_2})}{2} + \sum_{m=1}^{n_{c_1}} \text{sgn}(v_m^{c_1}) \frac{1 - \text{sgn}(\delta_m^{c_1})}{2} \\ & + \sum_{m=1}^{n_{g_1}} \text{sgn}(v_m^{g_1}) \frac{1 - \text{sgn}(\delta_m^{g_1})}{2} - \sum_{m=1}^{n_{h_1}} \text{sgn}(v_m^{h_1}) \frac{1 - \text{sgn}(\delta_m^{h_1})}{2} - \sum_{m=1}^{n_{h_2}} \text{sgn}(v_m^{h_2}) \frac{1 - \text{sgn}(\delta_m^{h_2})}{2} \end{aligned} \quad (\text{S165.2})$$

$$\begin{aligned} \mathcal{W}_3^{\text{gapless}} = & \sum_{m=1}^{n_{e_1}} \text{sgn}(v_m^{e_1}) \frac{1 - \text{sgn}(\delta_m^{e_1})}{2} + \sum_{m=1}^{n_{e_2}} \text{sgn}(v_m^{e_2}) \frac{1 - \text{sgn}(\delta_m^{e_2})}{2} - \sum_{m=1}^{n_{f_1}} \text{sgn}(v_m^{f_1}) \frac{1 - \text{sgn}(\delta_m^{f_1})}{2} \\ & + \sum_{m=1}^{n_{h_1}} \text{sgn}(v_m^{h_1}) \frac{1 - \text{sgn}(\delta_m^{h_1})}{2} + \sum_{m=1}^{n_{h_2}} \text{sgn}(v_m^{h_2}) \frac{1 - \text{sgn}(\delta_m^{h_2})}{2} \end{aligned} \quad (\text{S165.3})$$

$$\mathcal{W}_1^{\text{gapped}} = 2 \sum_{m=1}^{n_{e_2}} \text{sgn}(v_m^{e_2}) \frac{1 - \text{sgn}(\delta_m^{e_2})}{2} - \sum_{m=1}^{n_{f_1}} \text{sgn}(v_m^{f_1}) \frac{1 - \text{sgn}(\delta_m^{f_1})}{2} + 2 \sum_{m=1}^{n_{h_2}} \text{sgn}(v_m^{h_2}) \frac{1 - \text{sgn}(\delta_m^{h_2})}{2} \quad (\text{S165.4})$$

**S166. SPACE GROUP NO. 166**

| line segment                                | character of irrep (generators only)                                                                                                  |
|---------------------------------------------|---------------------------------------------------------------------------------------------------------------------------------------|
| $a \quad (0, 0, \frac{3t}{2})$              | $\{3_{001}   0 \ 0 \ 0\} \quad \{m_{100}   0 \ 0 \ 0\}$<br>$a_1 \quad -1 \quad -i$<br>$a_2 \quad -1 \quad i$<br>$a_3 \quad 1 \quad 0$ |
| $b \quad (0, \frac{t}{2}, \frac{3-t}{2})$   | $\{m_{100}   0 \ 0 \ 0\}$<br>$b_1 \quad -i$<br>$b_2 \quad i$                                                                          |
| $c \quad (\frac{t}{2}, 0, \frac{3}{2} - t)$ | $\{m_{01-1}   0 \ 0 \ 0\}$<br>$c_1 \quad -i$<br>$c_2 \quad i$                                                                         |
| $d \quad (0, t, \frac{t}{2})$               | $\{m_{100}   0 \ 0 \ 0\}$<br>$d_1 \quad -i$<br>$d_2 \quad i$                                                                          |
| $e \quad (\frac{t}{2}, \frac{t}{2}, 0)$     | $\{2_{10-1}   0 \ 0 \ 0\}$<br>$e_1 \quad -i$<br>$e_2 \quad i$                                                                         |
| $f \quad (\frac{1-t}{2}, t, \frac{1}{2})$   | $\{2_{01-1}   0 \ 0 \ 0\}$<br>$f_1 \quad -i$<br>$f_2 \quad i$                                                                         |

$$\mathcal{W}_1^{\text{gapless}} = \sum_{m=1}^{n_{a_1}} \text{sgn}(v_m^{a_1}) \frac{1 - \text{sgn}(\delta_m^{a_1})}{2} + \sum_{m=1}^{n_{a_3}} \text{sgn}(v_m^{a_3}) \frac{1 - \text{sgn}(\delta_m^{a_3})}{2} - \sum_{m=1}^{n_{d_1}} \text{sgn}(v_m^{d_1}) \frac{1 - \text{sgn}(\delta_m^{d_1})}{2} \quad (\text{S166.1})$$

$$\mathcal{W}_2^{\text{gapless}} = \sum_{m=1}^{n_{b_1}} \text{sgn}(v_m^{b_1}) \frac{1 - \text{sgn}(\delta_m^{b_1})}{2} + \sum_{m=1}^{n_{d_1}} \text{sgn}(v_m^{d_1}) \frac{1 - \text{sgn}(\delta_m^{d_1})}{2} - \sum_{m=1}^{n_{e_1}} \text{sgn}(v_m^{e_1}) \frac{1 - \text{sgn}(\delta_m^{e_1})}{2} \quad (\text{S166.2})$$

$$\mathcal{W}_3^{\text{gapless}} = \sum_{m=1}^{n_{c_1}} \text{sgn}(v_m^{c_1}) \frac{1 - \text{sgn}(\delta_m^{c_1})}{2} + \sum_{m=1}^{n_{f_1}} \text{sgn}(v_m^{f_1}) \frac{1 - \text{sgn}(\delta_m^{f_1})}{2} \quad (\text{S166.3})$$

**S167. SPACE GROUP NO. 167**

| line segment                                | character of irrep (generators only)                                                                                                                                                        |
|---------------------------------------------|---------------------------------------------------------------------------------------------------------------------------------------------------------------------------------------------|
| $a \quad (0, 0, \frac{3t}{2})$              | $\{3_{001}   0 \ 0 \ 0\} \quad \{m_{100}   0 \ 0 \ \frac{1}{2}\}$<br>$a_1 \quad -1 \quad -ie^{-\frac{3}{2}i\pi t}$<br>$a_2 \quad -1 \quad ie^{-\frac{3}{2}i\pi t}$<br>$a_3 \quad 1 \quad 0$ |
| $b \quad (0, \frac{t}{2}, \frac{3-t}{2})$   | $\{m_{100}   0 \ 0 \ \frac{1}{2}\}$<br>$b_1 \quad -ie^{-\frac{1}{2}i\pi(3-t)}$<br>$b_2 \quad ie^{-\frac{1}{2}i\pi(3-t)}$                                                                    |
| $c \quad (\frac{t}{2}, 0, \frac{3}{2} - t)$ | $\{m_{01-1}   0 \ 0 \ \frac{1}{2}\}$<br>$c_1 \quad -ie^{-\frac{1}{2}i\pi(3-2t)}$<br>$c_2 \quad ie^{-\frac{1}{2}i\pi(3-2t)}$                                                                 |
| $d \quad (0, t, \frac{t}{2})$               | $\{m_{100}   0 \ 0 \ \frac{1}{2}\}$<br>$d_1 \quad -ie^{-\frac{1}{2}i\pi t}$<br>$d_2 \quad ie^{-\frac{1}{2}i\pi t}$                                                                          |

|                                           |                                                                         |
|-------------------------------------------|-------------------------------------------------------------------------|
| $e \quad (\frac{t}{2}, \frac{t}{2}, 0)$   | $\{2_{10-1}   0 \ 0 \ \frac{1}{2}\}$<br>$e_1 \quad -i$<br>$e_2 \quad i$ |
| $f \quad (\frac{1-t}{2}, t, \frac{1}{2})$ | $\{2_{01-1}   0 \ 0 \ \frac{1}{2}\}$<br>$f_1 \quad i$<br>$f_2 \quad -i$ |

$$\mathcal{W}_1^{\text{gapless}} = \sum_{m=1}^{n_{a_1}} \text{sgn}(v_m^{a_1}) \frac{1 - \text{sgn}(\delta_m^{a_1})}{2} + \sum_{m=1}^{n_{a_3}} \text{sgn}(v_m^{a_3}) \frac{1 - \text{sgn}(\delta_m^{a_3})}{2} - \sum_{m=1}^{n_{d_1}} \text{sgn}(v_m^{d_1}) \frac{1 - \text{sgn}(\delta_m^{d_1})}{2} \quad (\text{S167.1})$$

$$\mathcal{W}_2^{\text{gapless}} = \sum_{m=1}^{n_{b_1}} \text{sgn}(v_m^{b_1}) \frac{1 - \text{sgn}(\delta_m^{b_1})}{2} + \sum_{m=1}^{n_{d_1}} \text{sgn}(v_m^{d_1}) \frac{1 - \text{sgn}(\delta_m^{d_1})}{2} - \sum_{m=1}^{n_{e_1}} \text{sgn}(v_m^{e_1}) \frac{1 - \text{sgn}(\delta_m^{e_1})}{2} \quad (\text{S167.2})$$

$$\mathcal{W}_3^{\text{gapless}} = \sum_{m=1}^{n_{c_1}} \text{sgn}(v_m^{c_1}) \frac{1 - \text{sgn}(\delta_m^{c_1})}{2} + \sum_{m=1}^{n_{f_1}} \text{sgn}(v_m^{f_1}) \frac{1 - \text{sgn}(\delta_m^{f_1})}{2} + \sum_{m=1}^{n_{f_2}} \text{sgn}(v_m^{f_2}) \frac{1 - \text{sgn}(\delta_m^{f_2})}{2} \quad (\text{S167.3})$$

$$\mathcal{W}_1^{\text{gapped}} = - \sum_{m=1}^{n_{f_1}} \text{sgn}(v_m^{f_1}) \frac{1 - \text{sgn}(\delta_m^{f_1})}{2} + \sum_{m=1}^{n_{f_2}} \text{sgn}(v_m^{f_2}) \frac{1 - \text{sgn}(\delta_m^{f_2})}{2} \quad (\text{S167.4})$$

### S168. SPACE GROUP NO. 168

| line segment                                        | character of irrep (generators only)                                                                                                                                                                     |
|-----------------------------------------------------|----------------------------------------------------------------------------------------------------------------------------------------------------------------------------------------------------------|
| $a \quad (0, 0, \frac{t}{2})$                       | $\{6_{001}   0 \ 0 \ 0\}$<br>$a_1 \quad e^{-\frac{5i\pi}{6}}$<br>$a_2 \quad e^{\frac{5i\pi}{6}}$<br>$a_3 \quad -i$<br>$a_4 \quad i$<br>$a_5 \quad e^{-\frac{i\pi}{6}}$<br>$a_6 \quad e^{\frac{i\pi}{6}}$ |
| $b \quad (\frac{1}{3}, \frac{1}{3}, \frac{1-t}{2})$ | $\{3_{001}   0 \ 0 \ 0\}$<br>$b_1 \quad -1$<br>$b_2 \quad e^{-\frac{i\pi}{3}}$<br>$b_3 \quad e^{\frac{i\pi}{3}}$                                                                                         |
| $c \quad (\frac{1}{2}, 0, \frac{t}{2})$             | $\{2_{001}   0 \ 0 \ 0\}$<br>$c_1 \quad -i$<br>$c_2 \quad i$                                                                                                                                             |
| $d \quad (\frac{t}{3}, \frac{t}{3}, 0)$             | $\{1   0 \ 0 \ 0\}$<br>$d_1 \quad 1$                                                                                                                                                                     |
| $e \quad (\frac{t}{3}, \frac{t}{3}, \frac{1}{2})$   | $\{1   0 \ 0 \ 0\}$<br>$e_1 \quad 1$                                                                                                                                                                     |
| $f \quad (\frac{3-t}{6}, \frac{t}{3}, 0)$           | $\{1   0 \ 0 \ 0\}$<br>$f_1 \quad 1$                                                                                                                                                                     |
| $g \quad (\frac{3-t}{6}, \frac{t}{3}, \frac{1}{2})$ | $\{1   0 \ 0 \ 0\}$<br>$g_1 \quad 1$                                                                                                                                                                     |

$$\begin{aligned}
\mathcal{W}_1^{\text{gapless}} = & \sum_{m=1}^{n_{a_1}} \text{sgn}(v_m^{a_1}) \frac{1 - \text{sgn}(\delta_m^{a_1})}{2} + \sum_{m=1}^{n_{a_2}} \text{sgn}(v_m^{a_2}) \frac{1 - \text{sgn}(\delta_m^{a_2})}{2} + \sum_{m=1}^{n_{a_3}} \text{sgn}(v_m^{a_3}) \frac{1 - \text{sgn}(\delta_m^{a_3})}{2} \\
& + \sum_{m=1}^{n_{a_4}} \text{sgn}(v_m^{a_4}) \frac{1 - \text{sgn}(\delta_m^{a_4})}{2} + \sum_{m=1}^{n_{a_5}} \text{sgn}(v_m^{a_5}) \frac{1 - \text{sgn}(\delta_m^{a_5})}{2} + \sum_{m=1}^{n_{a_6}} \text{sgn}(v_m^{a_6}) \frac{1 - \text{sgn}(\delta_m^{a_6})}{2} \\
& - \sum_{m=1}^{n_{c_1}} \text{sgn}(v_m^{c_1}) \frac{1 - \text{sgn}(\delta_m^{c_1})}{2} - \sum_{m=1}^{n_{c_2}} \text{sgn}(v_m^{c_2}) \frac{1 - \text{sgn}(\delta_m^{c_2})}{2} - \sum_{m=1}^{n_{d_1}} \text{sgn}(v_m^{d_1}) \frac{1 - \text{sgn}(\delta_m^{d_1})}{2} \\
& + \sum_{m=1}^{n_{e_1}} \text{sgn}(v_m^{e_1}) \frac{1 - \text{sgn}(\delta_m^{e_1})}{2} + \sum_{m=1}^{n_{f_1}} \text{sgn}(v_m^{f_1}) \frac{1 - \text{sgn}(\delta_m^{f_1})}{2} - \sum_{m=1}^{n_{g_1}} \text{sgn}(v_m^{g_1}) \frac{1 - \text{sgn}(\delta_m^{g_1})}{2}
\end{aligned} \tag{S168.1}$$

$$\begin{aligned}
\mathcal{W}_2^{\text{gapless}} = & \sum_{m=1}^{n_{b_1}} \text{sgn}(v_m^{b_1}) \frac{1 - \text{sgn}(\delta_m^{b_1})}{2} + \sum_{m=1}^{n_{b_2}} \text{sgn}(v_m^{b_2}) \frac{1 - \text{sgn}(\delta_m^{b_2})}{2} + \sum_{m=1}^{n_{b_3}} \text{sgn}(v_m^{b_3}) \frac{1 - \text{sgn}(\delta_m^{b_3})}{2} + \sum_{m=1}^{n_{c_1}} \text{sgn}(v_m^{c_1}) \frac{1 - \text{sgn}(\delta_m^{c_1})}{2} \\
& + \sum_{m=1}^{n_{c_2}} \text{sgn}(v_m^{c_2}) \frac{1 - \text{sgn}(\delta_m^{c_2})}{2} - \sum_{m=1}^{n_{f_1}} \text{sgn}(v_m^{f_1}) \frac{1 - \text{sgn}(\delta_m^{f_1})}{2} + \sum_{m=1}^{n_{g_1}} \text{sgn}(v_m^{g_1}) \frac{1 - \text{sgn}(\delta_m^{g_1})}{2}
\end{aligned} \tag{S168.2}$$

$$\mathcal{W}_1^{\text{gapped}} = - \sum_{m=1}^{n_{c_1}} \text{sgn}(v_m^{c_1}) \frac{1 - \text{sgn}(\delta_m^{c_1})}{2} + \sum_{m=1}^{n_{c_2}} \text{sgn}(v_m^{c_2}) \frac{1 - \text{sgn}(\delta_m^{c_2})}{2} \tag{S168.3}$$

$$\mathcal{W}_2^{\text{gapped}} = - \sum_{m=1}^{n_{b_2}} \text{sgn}(v_m^{b_2}) \frac{1 - \text{sgn}(\delta_m^{b_2})}{2} + \sum_{m=1}^{n_{b_3}} \text{sgn}(v_m^{b_3}) \frac{1 - \text{sgn}(\delta_m^{b_3})}{2} \tag{S168.4}$$

$$\mathcal{W}_3^{\text{gapped}} = - \sum_{m=1}^{n_{a_5}} \text{sgn}(v_m^{a_5}) \frac{1 - \text{sgn}(\delta_m^{a_5})}{2} + \sum_{m=1}^{n_{a_6}} \text{sgn}(v_m^{a_6}) \frac{1 - \text{sgn}(\delta_m^{a_6})}{2} \tag{S168.5}$$

$$\mathcal{W}_4^{\text{gapped}} = \sum_{m=1}^{n_{a_3}} \text{sgn}(v_m^{a_3}) \frac{1 - \text{sgn}(\delta_m^{a_3})}{2} - \sum_{m=1}^{n_{a_4}} \text{sgn}(v_m^{a_4}) \frac{1 - \text{sgn}(\delta_m^{a_4})}{2} \tag{S168.6}$$

$$\begin{aligned}
\mathcal{W}_5^{\text{gapped}} = & -2 \sum_{m=1}^{n_{a_2}} \text{sgn}(v_m^{a_2}) \frac{1 - \text{sgn}(\delta_m^{a_2})}{2} - 2 \sum_{m=1}^{n_{a_4}} \text{sgn}(v_m^{a_4}) \frac{1 - \text{sgn}(\delta_m^{a_4})}{2} \\
& - 2 \sum_{m=1}^{n_{a_5}} \text{sgn}(v_m^{a_5}) \frac{1 - \text{sgn}(\delta_m^{a_5})}{2} + 2 \sum_{m=1}^{n_{c_1}} \text{sgn}(v_m^{c_1}) \frac{1 - \text{sgn}(\delta_m^{c_1})}{2} + \sum_{m=1}^{n_{d_1}} \text{sgn}(v_m^{d_1}) \frac{1 - \text{sgn}(\delta_m^{d_1})}{2} \\
& - \sum_{m=1}^{n_{e_1}} \text{sgn}(v_m^{e_1}) \frac{1 - \text{sgn}(\delta_m^{e_1})}{2} - \sum_{m=1}^{n_{f_1}} \text{sgn}(v_m^{f_1}) \frac{1 - \text{sgn}(\delta_m^{f_1})}{2} + \sum_{m=1}^{n_{g_1}} \text{sgn}(v_m^{g_1}) \frac{1 - \text{sgn}(\delta_m^{g_1})}{2}
\end{aligned} \tag{S168.7}$$

$$\mathcal{X}_1 = \sum_{m=1}^{n_{d_1}} \frac{1 - \text{sgn}(\delta_m^{d_1})}{2} + \sum_{m=1}^{n_{f_1}} \frac{1 - \text{sgn}(\delta_m^{f_1})}{2} \mod 2 \tag{S168.8}$$

## S169. SPACE GROUP NO. 169

| line segment                                        | character of irrep (generators only)                   |
|-----------------------------------------------------|--------------------------------------------------------|
| $a \quad (0, 0, \frac{t}{2})$                       | $\{6_{001}   0 \ 0 \ \frac{1}{6}\}$                    |
|                                                     | $a_1 \quad e^{-\frac{1}{6}i\pi t - \frac{5i\pi}{6}}$   |
|                                                     | $a_2 \quad e^{\frac{5i\pi}{6} - \frac{i\pi t}{6}}$     |
|                                                     | $a_3 \quad -ie^{-\frac{1}{6}i\pi t}$                   |
|                                                     | $a_4 \quad ie^{-\frac{1}{6}i\pi t}$                    |
|                                                     | $a_5 \quad e^{-\frac{1}{6}i\pi t - \frac{i\pi}{6}}$    |
|                                                     | $a_6 \quad e^{\frac{i\pi}{6} - \frac{i\pi t}{6}}$      |
| $b \quad (\frac{1}{3}, \frac{1}{3}, \frac{1-t}{2})$ | $\{3_{001}   0 \ 0 \ \frac{1}{3}\}$                    |
|                                                     | $b_1 \quad -e^{-\frac{1}{3}i\pi(1-t)}$                 |
|                                                     | $b_2 \quad e^{-\frac{1}{3}i\pi(1-t) - \frac{i\pi}{3}}$ |
| $c \quad (\frac{1}{2}, 0, \frac{t}{2})$             | $\{2_{001}   0 \ 0 \ \frac{1}{2}\}$                    |
|                                                     | $c_1 \quad -ie^{-\frac{1}{2}i\pi t}$                   |
|                                                     | $c_2 \quad ie^{-\frac{1}{2}i\pi t}$                    |
| $d \quad (\frac{t}{3}, \frac{t}{3}, 0)$             | $\{1   0 \ 0 \ 0\}$                                    |
| $e \quad (\frac{t}{3}, \frac{t}{3}, \frac{1}{2})$   | $\{1   0 \ 0 \ 0\}$                                    |
| $f \quad (\frac{3-t}{6}, \frac{t}{3}, 0)$           | $\{1   0 \ 0 \ 0\}$                                    |
| $g \quad (\frac{3-t}{6}, \frac{t}{3}, \frac{1}{2})$ | $\{1   0 \ 0 \ 0\}$                                    |

$$\begin{aligned}
\mathcal{W}_1^{\text{gapless}} = & \sum_{m=1}^{n_{a_1}} \text{sgn}(v_m^{a_1}) \frac{1 - \text{sgn}(\delta_m^{a_1})}{2} + \sum_{m=1}^{n_{a_2}} \text{sgn}(v_m^{a_2}) \frac{1 - \text{sgn}(\delta_m^{a_2})}{2} + \sum_{m=1}^{n_{a_3}} \text{sgn}(v_m^{a_3}) \frac{1 - \text{sgn}(\delta_m^{a_3})}{2} \\
& + \sum_{m=1}^{n_{a_4}} \text{sgn}(v_m^{a_4}) \frac{1 - \text{sgn}(\delta_m^{a_4})}{2} + \sum_{m=1}^{n_{a_5}} \text{sgn}(v_m^{a_5}) \frac{1 - \text{sgn}(\delta_m^{a_5})}{2} + \sum_{m=1}^{n_{a_6}} \text{sgn}(v_m^{a_6}) \frac{1 - \text{sgn}(\delta_m^{a_6})}{2} \\
& - \sum_{m=1}^{n_{c_1}} \text{sgn}(v_m^{c_1}) \frac{1 - \text{sgn}(\delta_m^{c_1})}{2} - \sum_{m=1}^{n_{c_2}} \text{sgn}(v_m^{c_2}) \frac{1 - \text{sgn}(\delta_m^{c_2})}{2} - \sum_{m=1}^{n_{d_1}} \text{sgn}(v_m^{d_1}) \frac{1 - \text{sgn}(\delta_m^{d_1})}{2} \\
& + 2 \sum_{m=1}^{n_{e_1}} \text{sgn}(v_m^{e_1}) \frac{1 - \text{sgn}(\delta_m^{e_1})}{2} + \sum_{m=1}^{n_{f_1}} \text{sgn}(v_m^{f_1}) \frac{1 - \text{sgn}(\delta_m^{f_1})}{2} - 2 \sum_{m=1}^{n_{g_1}} \text{sgn}(v_m^{g_1}) \frac{1 - \text{sgn}(\delta_m^{g_1})}{2}
\end{aligned} \tag{S169.1}$$

$$\begin{aligned}
\mathcal{W}_2^{\text{gapless}} = & \sum_{m=1}^{n_{b_1}} \text{sgn}(v_m^{b_1}) \frac{1 - \text{sgn}(\delta_m^{b_1})}{2} + \sum_{m=1}^{n_{b_2}} \text{sgn}(v_m^{b_2}) \frac{1 - \text{sgn}(\delta_m^{b_2})}{2} + \sum_{m=1}^{n_{b_3}} \text{sgn}(v_m^{b_3}) \frac{1 - \text{sgn}(\delta_m^{b_3})}{2} + \sum_{m=1}^{n_{c_1}} \text{sgn}(v_m^{c_1}) \frac{1 - \text{sgn}(\delta_m^{c_1})}{2} \\
& + \sum_{m=1}^{n_{c_2}} \text{sgn}(v_m^{c_2}) \frac{1 - \text{sgn}(\delta_m^{c_2})}{2} - \sum_{m=1}^{n_{f_1}} \text{sgn}(v_m^{f_1}) \frac{1 - \text{sgn}(\delta_m^{f_1})}{2} + 2 \sum_{m=1}^{n_{g_1}} \text{sgn}(v_m^{g_1}) \frac{1 - \text{sgn}(\delta_m^{g_1})}{2}
\end{aligned} \tag{S169.2}$$

$$\mathcal{X}_1 = \sum_{m=1}^{n_{c_1}} \frac{1 - \text{sgn}(\delta_m^{c_1})}{2} + \sum_{m=1}^{n_{c_2}} \frac{1 - \text{sgn}(\delta_m^{c_2})}{2} \mod 2 \tag{S169.3}$$

$$\begin{aligned}
\mathcal{X}_2 = & -2 \sum_{m=1}^{n_{a_2}} \text{sgn}(v_m^{a_2}) \frac{1 - \text{sgn}(\delta_m^{a_2})}{2} + 2 \sum_{m=1}^{n_{a_3}} \text{sgn}(v_m^{a_3}) \frac{1 - \text{sgn}(\delta_m^{a_3})}{2} - 4 \sum_{m=1}^{n_{a_4}} \text{sgn}(v_m^{a_4}) \frac{1 - \text{sgn}(\delta_m^{a_4})}{2} \\
& + 4 \sum_{m=1}^{n_{a_5}} \text{sgn}(v_m^{a_5}) \frac{1 - \text{sgn}(\delta_m^{a_5})}{2} - 6 \sum_{m=1}^{n_{a_6}} \text{sgn}(v_m^{a_6}) \frac{1 - \text{sgn}(\delta_m^{a_6})}{2} + 8 \sum_{m=1}^{n_{b_2}} \text{sgn}(v_m^{b_2}) \frac{1 - \text{sgn}(\delta_m^{b_2})}{2} \\
& - 8 \sum_{m=1}^{n_{b_3}} \text{sgn}(v_m^{b_3}) \frac{1 - \text{sgn}(\delta_m^{b_3})}{2} - 2 \sum_{m=1}^{n_{c_1}} \text{sgn}(v_m^{c_1}) \frac{1 - \text{sgn}(\delta_m^{c_1})}{2} + 4 \sum_{m=1}^{n_{c_2}} \text{sgn}(v_m^{c_2}) \frac{1 - \text{sgn}(\delta_m^{c_2})}{2} \\
& + \sum_{m=1}^{n_{d_1}} \text{sgn}(v_m^{d_1}) \frac{1 - \text{sgn}(\delta_m^{d_1})}{2} - \sum_{m=1}^{n_{f_1}} \text{sgn}(v_m^{f_1}) \frac{1 - \text{sgn}(\delta_m^{f_1})}{2} - 4 \sum_{m=1}^{n_{g_1}} \text{sgn}(v_m^{g_1}) \frac{1 - \text{sgn}(\delta_m^{g_1})}{2} \pmod{12}
\end{aligned} \tag{S169.4}$$

### S170. SPACE GROUP NO. 170

| line segment                                        | character of irrep (generators only)                   |
|-----------------------------------------------------|--------------------------------------------------------|
| $a \quad (0, 0, \frac{t}{2})$                       | $\{6_{001}   0 \ 0 \ \frac{5}{6}\}$                    |
|                                                     | $a_1 \quad e^{-\frac{5}{6}i\pi t - \frac{5i\pi}{6}}$   |
|                                                     | $a_2 \quad e^{\frac{5i\pi}{6} - \frac{5i\pi t}{6}}$    |
|                                                     | $a_3 \quad -ie^{-\frac{5}{6}i\pi t}$                   |
|                                                     | $a_4 \quad ie^{-\frac{5}{6}i\pi t}$                    |
|                                                     | $a_5 \quad e^{-\frac{5}{6}i\pi t - \frac{i\pi}{6}}$    |
|                                                     | $a_6 \quad e^{\frac{i\pi}{6} - \frac{5i\pi t}{6}}$     |
| $b \quad (\frac{1}{3}, \frac{1}{3}, \frac{1-t}{2})$ | $\{3_{001}   0 \ 0 \ \frac{2}{3}\}$                    |
|                                                     | $b_1 \quad -e^{-\frac{2}{3}i\pi(1-t)}$                 |
|                                                     | $b_2 \quad e^{-\frac{2}{3}i\pi(1-t) - \frac{i\pi}{3}}$ |
|                                                     | $b_3 \quad e^{\frac{i\pi}{3} - \frac{2}{3}i\pi(1-t)}$  |
| $c \quad (\frac{1}{2}, 0, \frac{t}{2})$             | $\{2_{001}   0 \ 0 \ \frac{1}{2}\}$                    |
|                                                     | $c_1 \quad -ie^{-\frac{1}{2}i\pi t}$                   |
|                                                     | $c_2 \quad ie^{-\frac{1}{2}i\pi t}$                    |
| $d \quad (\frac{t}{3}, \frac{t}{3}, 0)$             | $\{1   0 \ 0 \ 0\}$                                    |
| $d_1$                                               | 1                                                      |
| $e \quad (\frac{t}{3}, \frac{t}{3}, \frac{1}{2})$   | $\{1   0 \ 0 \ 0\}$                                    |
| $e_1$                                               | 1                                                      |
| $f \quad (\frac{3-t}{6}, \frac{t}{3}, 0)$           | $\{1   0 \ 0 \ 0\}$                                    |
| $f_1$                                               | 1                                                      |
| $g \quad (\frac{3-t}{6}, \frac{t}{3}, \frac{1}{2})$ | $\{1   0 \ 0 \ 0\}$                                    |
| $g_1$                                               | 1                                                      |

$$\begin{aligned}
\mathcal{W}_1^{\text{gapless}} = & \sum_{m=1}^{n_{a_1}} \text{sgn}(v_m^{a_1}) \frac{1 - \text{sgn}(\delta_m^{a_1})}{2} + \sum_{m=1}^{n_{a_2}} \text{sgn}(v_m^{a_2}) \frac{1 - \text{sgn}(\delta_m^{a_2})}{2} + \sum_{m=1}^{n_{a_3}} \text{sgn}(v_m^{a_3}) \frac{1 - \text{sgn}(\delta_m^{a_3})}{2} \\
& + \sum_{m=1}^{n_{a_4}} \text{sgn}(v_m^{a_4}) \frac{1 - \text{sgn}(\delta_m^{a_4})}{2} + \sum_{m=1}^{n_{a_5}} \text{sgn}(v_m^{a_5}) \frac{1 - \text{sgn}(\delta_m^{a_5})}{2} + \sum_{m=1}^{n_{a_6}} \text{sgn}(v_m^{a_6}) \frac{1 - \text{sgn}(\delta_m^{a_6})}{2} \\
& - \sum_{m=1}^{n_{c_1}} \text{sgn}(v_m^{c_1}) \frac{1 - \text{sgn}(\delta_m^{c_1})}{2} - \sum_{m=1}^{n_{c_2}} \text{sgn}(v_m^{c_2}) \frac{1 - \text{sgn}(\delta_m^{c_2})}{2} - \sum_{m=1}^{n_{d_1}} \text{sgn}(v_m^{d_1}) \frac{1 - \text{sgn}(\delta_m^{d_1})}{2} \\
& + 2 \sum_{m=1}^{n_{e_1}} \text{sgn}(v_m^{e_1}) \frac{1 - \text{sgn}(\delta_m^{e_1})}{2} + \sum_{m=1}^{n_{f_1}} \text{sgn}(v_m^{f_1}) \frac{1 - \text{sgn}(\delta_m^{f_1})}{2} - 2 \sum_{m=1}^{n_{g_1}} \text{sgn}(v_m^{g_1}) \frac{1 - \text{sgn}(\delta_m^{g_1})}{2}
\end{aligned} \tag{S170.1}$$



$$\begin{aligned} \mathcal{W}_2^{\text{gapless}} = & \sum_{m=1}^{n_{b_1}} \text{sgn}(v_m^{b_1}) \frac{1 - \text{sgn}(\delta_m^{b_1})}{2} + \sum_{m=1}^{n_{b_2}} \text{sgn}(v_m^{b_2}) \frac{1 - \text{sgn}(\delta_m^{b_2})}{2} + \sum_{m=1}^{n_{b_3}} \text{sgn}(v_m^{b_3}) \frac{1 - \text{sgn}(\delta_m^{b_3})}{2} + \sum_{m=1}^{n_{c_1}} \text{sgn}(v_m^{c_1}) \frac{1 - \text{sgn}(\delta_m^{c_1})}{2} \\ & + \sum_{m=1}^{n_{c_2}} \text{sgn}(v_m^{c_2}) \frac{1 - \text{sgn}(\delta_m^{c_2})}{2} - \sum_{m=1}^{n_{f_1}} \text{sgn}(v_m^{f_1}) \frac{1 - \text{sgn}(\delta_m^{f_1})}{2} + 2 \sum_{m=1}^{n_{g_1}} \text{sgn}(v_m^{g_1}) \frac{1 - \text{sgn}(\delta_m^{g_1})}{2} \end{aligned} \quad (\text{S170.2})$$

$$\mathcal{X}_1 = \sum_{m=1}^{n_{c_1}} \frac{1 - \text{sgn}(\delta_m^{c_1})}{2} + \sum_{m=1}^{n_{c_2}} \frac{1 - \text{sgn}(\delta_m^{c_2})}{2} \quad \text{mod } 2 \quad (\text{S170.3})$$

$$\begin{aligned} \mathcal{X}_2 = & 2 \sum_{m=1}^{n_{a_2}} \text{sgn}(v_m^{a_2}) \frac{1 - \text{sgn}(\delta_m^{a_2})}{2} - 2 \sum_{m=1}^{n_{a_3}} \text{sgn}(v_m^{a_3}) \frac{1 - \text{sgn}(\delta_m^{a_3})}{2} + 4 \sum_{m=1}^{n_{a_4}} \text{sgn}(v_m^{a_4}) \frac{1 - \text{sgn}(\delta_m^{a_4})}{2} \\ & - 4 \sum_{m=1}^{n_{a_5}} \text{sgn}(v_m^{a_5}) \frac{1 - \text{sgn}(\delta_m^{a_5})}{2} + 6 \sum_{m=1}^{n_{a_6}} \text{sgn}(v_m^{a_6}) \frac{1 - \text{sgn}(\delta_m^{a_6})}{2} - 8 \sum_{m=1}^{n_{b_2}} \text{sgn}(v_m^{b_2}) \frac{1 - \text{sgn}(\delta_m^{b_2})}{2} \\ & + 8 \sum_{m=1}^{n_{b_3}} \text{sgn}(v_m^{b_3}) \frac{1 - \text{sgn}(\delta_m^{b_3})}{2} - 4 \sum_{m=1}^{n_{c_1}} \text{sgn}(v_m^{c_1}) \frac{1 - \text{sgn}(\delta_m^{c_1})}{2} + 2 \sum_{m=1}^{n_{c_2}} \text{sgn}(v_m^{c_2}) \frac{1 - \text{sgn}(\delta_m^{c_2})}{2} \\ & - \sum_{m=1}^{n_{d_1}} \text{sgn}(v_m^{d_1}) \frac{1 - \text{sgn}(\delta_m^{d_1})}{2} + 4 \sum_{m=1}^{n_{e_1}} \text{sgn}(v_m^{e_1}) \frac{1 - \text{sgn}(\delta_m^{e_1})}{2} + \sum_{m=1}^{n_{f_1}} \text{sgn}(v_m^{f_1}) \frac{1 - \text{sgn}(\delta_m^{f_1})}{2} \\ & - 8 \sum_{m=1}^{n_{g_1}} \text{sgn}(v_m^{g_1}) \frac{1 - \text{sgn}(\delta_m^{g_1})}{2} \quad \text{mod } 12 \end{aligned} \quad (\text{S170.4})$$

### S171. SPACE GROUP NO. 171

| line segment                                        | character of irrep (generators only)                                                                                                                                                                                                                                                                                                         |
|-----------------------------------------------------|----------------------------------------------------------------------------------------------------------------------------------------------------------------------------------------------------------------------------------------------------------------------------------------------------------------------------------------------|
| $a \quad (0, 0, \frac{t}{2})$                       | $\{6_{001}   0 \ 0 \ \frac{1}{3}\}$<br>$a_1 \quad e^{-\frac{1}{3}i\pi t - \frac{5i\pi}{6}}$<br>$a_2 \quad e^{\frac{5i\pi}{6} - \frac{i\pi t}{3}}$<br>$a_3 \quad -ie^{-\frac{1}{3}i\pi t}$<br>$a_4 \quad ie^{-\frac{1}{3}i\pi t}$<br>$a_5 \quad e^{-\frac{1}{3}i\pi t - \frac{i\pi}{6}}$<br>$a_6 \quad e^{\frac{i\pi}{6} - \frac{i\pi t}{3}}$ |
| $b \quad (\frac{1}{3}, \frac{1}{3}, \frac{1-t}{2})$ | $\{3_{001}   0 \ 0 \ \frac{2}{3}\}$<br>$b_1 \quad -e^{-\frac{2}{3}i\pi(1-t)}$<br>$b_2 \quad e^{-\frac{2}{3}i\pi(1-t) - \frac{i\pi}{3}}$<br>$b_3 \quad e^{\frac{i\pi}{3} - \frac{2}{3}i\pi(1-t)}$                                                                                                                                             |
| $c \quad (\frac{1}{2}, 0, \frac{t}{2})$             | $\{2_{001}   0 \ 0 \ 0\}$<br>$c_1 \quad -i$<br>$c_2 \quad i$                                                                                                                                                                                                                                                                                 |
| $d \quad (\frac{t}{3}, \frac{t}{3}, 0)$             | $\{1   0 \ 0 \ 0\}$<br>$d_1 \quad 1$                                                                                                                                                                                                                                                                                                         |
| $e \quad (\frac{t}{3}, \frac{t}{3}, \frac{1}{2})$   | $\{1   0 \ 0 \ 0\}$<br>$e_1 \quad 1$                                                                                                                                                                                                                                                                                                         |
| $f \quad (\frac{3-t}{6}, \frac{t}{3}, 0)$           | $\{1   0 \ 0 \ 0\}$<br>$f_1 \quad 1$                                                                                                                                                                                                                                                                                                         |
| $g \quad (\frac{3-t}{6}, \frac{t}{3}, \frac{1}{2})$ | $\{1   0 \ 0 \ 0\}$<br>$g_1 \quad 1$                                                                                                                                                                                                                                                                                                         |

$$\begin{aligned}
\mathcal{W}_1^{\text{gapless}} = & \sum_{m=1}^{n_{a_1}} \text{sgn}(v_m^{a_1}) \frac{1 - \text{sgn}(\delta_m^{a_1})}{2} + \sum_{m=1}^{n_{a_2}} \text{sgn}(v_m^{a_2}) \frac{1 - \text{sgn}(\delta_m^{a_2})}{2} + \sum_{m=1}^{n_{a_3}} \text{sgn}(v_m^{a_3}) \frac{1 - \text{sgn}(\delta_m^{a_3})}{2} \\
& + \sum_{m=1}^{n_{a_4}} \text{sgn}(v_m^{a_4}) \frac{1 - \text{sgn}(\delta_m^{a_4})}{2} + \sum_{m=1}^{n_{a_5}} \text{sgn}(v_m^{a_5}) \frac{1 - \text{sgn}(\delta_m^{a_5})}{2} + \sum_{m=1}^{n_{a_6}} \text{sgn}(v_m^{a_6}) \frac{1 - \text{sgn}(\delta_m^{a_6})}{2} \\
& - \sum_{m=1}^{n_{c_1}} \text{sgn}(v_m^{c_1}) \frac{1 - \text{sgn}(\delta_m^{c_1})}{2} - \sum_{m=1}^{n_{c_2}} \text{sgn}(v_m^{c_2}) \frac{1 - \text{sgn}(\delta_m^{c_2})}{2} - \sum_{m=1}^{n_{d_1}} \text{sgn}(v_m^{d_1}) \frac{1 - \text{sgn}(\delta_m^{d_1})}{2} \\
& + \sum_{m=1}^{n_{e_1}} \text{sgn}(v_m^{e_1}) \frac{1 - \text{sgn}(\delta_m^{e_1})}{2} + \sum_{m=1}^{n_{f_1}} \text{sgn}(v_m^{f_1}) \frac{1 - \text{sgn}(\delta_m^{f_1})}{2} - \sum_{m=1}^{n_{g_1}} \text{sgn}(v_m^{g_1}) \frac{1 - \text{sgn}(\delta_m^{g_1})}{2}
\end{aligned} \tag{S171.1}$$

$$\begin{aligned}
\mathcal{W}_2^{\text{gapless}} = & \sum_{m=1}^{n_{b_1}} \text{sgn}(v_m^{b_1}) \frac{1 - \text{sgn}(\delta_m^{b_1})}{2} + \sum_{m=1}^{n_{b_2}} \text{sgn}(v_m^{b_2}) \frac{1 - \text{sgn}(\delta_m^{b_2})}{2} + \sum_{m=1}^{n_{b_3}} \text{sgn}(v_m^{b_3}) \frac{1 - \text{sgn}(\delta_m^{b_3})}{2} + \sum_{m=1}^{n_{c_1}} \text{sgn}(v_m^{c_1}) \frac{1 - \text{sgn}(\delta_m^{c_1})}{2} \\
& + \sum_{m=1}^{n_{c_2}} \text{sgn}(v_m^{c_2}) \frac{1 - \text{sgn}(\delta_m^{c_2})}{2} - \sum_{m=1}^{n_{f_1}} \text{sgn}(v_m^{f_1}) \frac{1 - \text{sgn}(\delta_m^{f_1})}{2} + \sum_{m=1}^{n_{g_1}} \text{sgn}(v_m^{g_1}) \frac{1 - \text{sgn}(\delta_m^{g_1})}{2}
\end{aligned} \tag{S171.2}$$

$$\mathcal{W}_1^{\text{gapped}} = - \sum_{m=1}^{n_{c_1}} \text{sgn}(v_m^{c_1}) \frac{1 - \text{sgn}(\delta_m^{c_1})}{2} + \sum_{m=1}^{n_{c_2}} \text{sgn}(v_m^{c_2}) \frac{1 - \text{sgn}(\delta_m^{c_2})}{2} \tag{S171.3}$$

$$\begin{aligned}
\mathcal{W}_2^{\text{gapped}} = & -2 \sum_{m=1}^{n_{a_2}} \text{sgn}(v_m^{a_2}) \frac{1 - \text{sgn}(\delta_m^{a_2})}{2} - 2 \sum_{m=1}^{n_{a_3}} \text{sgn}(v_m^{a_3}) \frac{1 - \text{sgn}(\delta_m^{a_3})}{2} \\
& - 2 \sum_{m=1}^{n_{a_6}} \text{sgn}(v_m^{a_6}) \frac{1 - \text{sgn}(\delta_m^{a_6})}{2} + 2 \sum_{m=1}^{n_{c_1}} \text{sgn}(v_m^{c_1}) \frac{1 - \text{sgn}(\delta_m^{c_1})}{2} + \sum_{m=1}^{n_{d_1}} \text{sgn}(v_m^{d_1}) \frac{1 - \text{sgn}(\delta_m^{d_1})}{2} \\
& - \sum_{m=1}^{n_{e_1}} \text{sgn}(v_m^{e_1}) \frac{1 - \text{sgn}(\delta_m^{e_1})}{2} - \sum_{m=1}^{n_{f_1}} \text{sgn}(v_m^{f_1}) \frac{1 - \text{sgn}(\delta_m^{f_1})}{2} + \sum_{m=1}^{n_{g_1}} \text{sgn}(v_m^{g_1}) \frac{1 - \text{sgn}(\delta_m^{g_1})}{2}
\end{aligned} \tag{S171.4}$$

$$\begin{aligned}
\mathcal{X}_1 = & -4 \sum_{m=1}^{n_{a_3}} \text{sgn}(v_m^{a_3}) \frac{1 - \text{sgn}(\delta_m^{a_3})}{2} - 2 \sum_{m=1}^{n_{a_4}} \text{sgn}(v_m^{a_4}) \frac{1 - \text{sgn}(\delta_m^{a_4})}{2} + 2 \sum_{m=1}^{n_{a_5}} \text{sgn}(v_m^{a_5}) \frac{1 - \text{sgn}(\delta_m^{a_5})}{2} \\
& - 8 \sum_{m=1}^{n_{a_6}} \text{sgn}(v_m^{a_6}) \frac{1 - \text{sgn}(\delta_m^{a_6})}{2} - 2 \sum_{m=1}^{n_{b_2}} \text{sgn}(v_m^{b_2}) \frac{1 - \text{sgn}(\delta_m^{b_2})}{2} + 2 \sum_{m=1}^{n_{b_3}} \text{sgn}(v_m^{b_3}) \frac{1 - \text{sgn}(\delta_m^{b_3})}{2} \\
& + 3 \sum_{m=1}^{n_{d_1}} \text{sgn}(v_m^{d_1}) \frac{1 - \text{sgn}(\delta_m^{d_1})}{2} - 2 \sum_{m=1}^{n_{e_1}} \text{sgn}(v_m^{e_1}) \frac{1 - \text{sgn}(\delta_m^{e_1})}{2} - 3 \sum_{m=1}^{n_{f_1}} \text{sgn}(v_m^{f_1}) \frac{1 - \text{sgn}(\delta_m^{f_1})}{2} \pmod{6}
\end{aligned} \tag{S171.5}$$

## S172. SPACE GROUP NO. 172

|              |                                      |
|--------------|--------------------------------------|
| line segment | character of irrep (generators only) |
|--------------|--------------------------------------|

|                                                     |                                                        |
|-----------------------------------------------------|--------------------------------------------------------|
| $a \quad (0, 0, \frac{t}{2})$                       | $\{6_{001}   0 \ 0 \ \frac{2}{3}\}$                    |
|                                                     | $a_1 \quad e^{-\frac{2}{3}i\pi t - \frac{5i\pi}{6}}$   |
|                                                     | $a_2 \quad e^{\frac{5i\pi}{6} - \frac{2i\pi t}{3}}$    |
|                                                     | $a_3 \quad -ie^{-\frac{2}{3}i\pi t}$                   |
|                                                     | $a_4 \quad ie^{-\frac{2}{3}i\pi t}$                    |
|                                                     | $a_5 \quad e^{-\frac{2}{3}i\pi t - \frac{i\pi}{6}}$    |
|                                                     | $a_6 \quad e^{\frac{i\pi}{6} - \frac{2i\pi t}{3}}$     |
| $b \quad (\frac{1}{3}, \frac{1}{3}, \frac{1-t}{2})$ | $\{3_{001}   0 \ 0 \ \frac{1}{3}\}$                    |
|                                                     | $b_1 \quad -e^{-\frac{1}{3}i\pi(1-t)}$                 |
|                                                     | $b_2 \quad e^{-\frac{1}{3}i\pi(1-t) - \frac{i\pi}{3}}$ |
|                                                     | $b_3 \quad e^{\frac{i\pi}{3} - \frac{1}{3}i\pi(1-t)}$  |
| $c \quad (\frac{1}{2}, 0, \frac{t}{2})$             | $\{2_{001}   0 \ 0 \ 0\}$                              |
|                                                     | $c_1 \quad -i$                                         |
|                                                     | $c_2 \quad i$                                          |
| $d \quad (\frac{t}{3}, \frac{t}{3}, 0)$             | $\{1   0 \ 0 \ 0\}$                                    |
|                                                     | $d_1 \quad 1$                                          |
| $e \quad (\frac{t}{3}, \frac{t}{3}, \frac{1}{2})$   | $\{1   0 \ 0 \ 0\}$                                    |
|                                                     | $e_1 \quad 1$                                          |
| $f \quad (\frac{3-t}{6}, \frac{t}{3}, 0)$           | $\{1   0 \ 0 \ 0\}$                                    |
|                                                     | $f_1 \quad 1$                                          |
| $g \quad (\frac{3-t}{6}, \frac{t}{3}, \frac{1}{2})$ | $\{1   0 \ 0 \ 0\}$                                    |
|                                                     | $g_1 \quad 1$                                          |

$$\begin{aligned}
\mathcal{W}_1^{\text{gapless}} = & \sum_{m=1}^{n_{a_1}} \text{sgn}(v_m^{a_1}) \frac{1 - \text{sgn}(\delta_m^{a_1})}{2} + \sum_{m=1}^{n_{a_2}} \text{sgn}(v_m^{a_2}) \frac{1 - \text{sgn}(\delta_m^{a_2})}{2} + \sum_{m=1}^{n_{a_3}} \text{sgn}(v_m^{a_3}) \frac{1 - \text{sgn}(\delta_m^{a_3})}{2} \\
& + \sum_{m=1}^{n_{a_4}} \text{sgn}(v_m^{a_4}) \frac{1 - \text{sgn}(\delta_m^{a_4})}{2} + \sum_{m=1}^{n_{a_5}} \text{sgn}(v_m^{a_5}) \frac{1 - \text{sgn}(\delta_m^{a_5})}{2} + \sum_{m=1}^{n_{a_6}} \text{sgn}(v_m^{a_6}) \frac{1 - \text{sgn}(\delta_m^{a_6})}{2} \\
& - \sum_{m=1}^{n_{c_1}} \text{sgn}(v_m^{c_1}) \frac{1 - \text{sgn}(\delta_m^{c_1})}{2} - \sum_{m=1}^{n_{c_2}} \text{sgn}(v_m^{c_2}) \frac{1 - \text{sgn}(\delta_m^{c_2})}{2} - \sum_{m=1}^{n_{d_1}} \text{sgn}(v_m^{d_1}) \frac{1 - \text{sgn}(\delta_m^{d_1})}{2} \\
& + \sum_{m=1}^{n_{e_1}} \text{sgn}(v_m^{e_1}) \frac{1 - \text{sgn}(\delta_m^{e_1})}{2} + \sum_{m=1}^{n_{f_1}} \text{sgn}(v_m^{f_1}) \frac{1 - \text{sgn}(\delta_m^{f_1})}{2} - \sum_{m=1}^{n_{g_1}} \text{sgn}(v_m^{g_1}) \frac{1 - \text{sgn}(\delta_m^{g_1})}{2}
\end{aligned} \tag{S172.1}$$

$$\begin{aligned}
\mathcal{W}_2^{\text{gapless}} = & \sum_{m=1}^{n_{b_1}} \text{sgn}(v_m^{b_1}) \frac{1 - \text{sgn}(\delta_m^{b_1})}{2} + \sum_{m=1}^{n_{b_2}} \text{sgn}(v_m^{b_2}) \frac{1 - \text{sgn}(\delta_m^{b_2})}{2} + \sum_{m=1}^{n_{b_3}} \text{sgn}(v_m^{b_3}) \frac{1 - \text{sgn}(\delta_m^{b_3})}{2} + \sum_{m=1}^{n_{c_1}} \text{sgn}(v_m^{c_1}) \frac{1 - \text{sgn}(\delta_m^{c_1})}{2} \\
& + \sum_{m=1}^{n_{c_2}} \text{sgn}(v_m^{c_2}) \frac{1 - \text{sgn}(\delta_m^{c_2})}{2} - \sum_{m=1}^{n_{f_1}} \text{sgn}(v_m^{f_1}) \frac{1 - \text{sgn}(\delta_m^{f_1})}{2} + \sum_{m=1}^{n_{g_1}} \text{sgn}(v_m^{g_1}) \frac{1 - \text{sgn}(\delta_m^{g_1})}{2}
\end{aligned} \tag{S172.2}$$

$$\mathcal{W}_1^{\text{gapped}} = - \sum_{m=1}^{n_{c_1}} \text{sgn}(v_m^{c_1}) \frac{1 - \text{sgn}(\delta_m^{c_1})}{2} + \sum_{m=1}^{n_{c_2}} \text{sgn}(v_m^{c_2}) \frac{1 - \text{sgn}(\delta_m^{c_2})}{2} \tag{S172.3}$$

$$\begin{aligned}
\mathcal{W}_2^{\text{gapped}} = & -2 \sum_{m=1}^{n_{a_2}} \text{sgn}(v_m^{a_2}) \frac{1 - \text{sgn}(\delta_m^{a_2})}{2} - 2 \sum_{m=1}^{n_{a_3}} \text{sgn}(v_m^{a_3}) \frac{1 - \text{sgn}(\delta_m^{a_3})}{2} \\
& - 2 \sum_{m=1}^{n_{a_6}} \text{sgn}(v_m^{a_6}) \frac{1 - \text{sgn}(\delta_m^{a_6})}{2} + 2 \sum_{m=1}^{n_{c_1}} \text{sgn}(v_m^{c_1}) \frac{1 - \text{sgn}(\delta_m^{c_1})}{2} + \sum_{m=1}^{n_{d_1}} \text{sgn}(v_m^{d_1}) \frac{1 - \text{sgn}(\delta_m^{d_1})}{2} \\
& - \sum_{m=1}^{n_{e_1}} \text{sgn}(v_m^{e_1}) \frac{1 - \text{sgn}(\delta_m^{e_1})}{2} - \sum_{m=1}^{n_{f_1}} \text{sgn}(v_m^{f_1}) \frac{1 - \text{sgn}(\delta_m^{f_1})}{2} + \sum_{m=1}^{n_{g_1}} \text{sgn}(v_m^{g_1}) \frac{1 - \text{sgn}(\delta_m^{g_1})}{2}
\end{aligned} \tag{S172.4}$$

$$\begin{aligned}
\mathcal{X}_1 = & -8 \sum_{m=1}^{n_{a_3}} \text{sgn}(v_m^{a_3}) \frac{1 - \text{sgn}(\delta_m^{a_3})}{2} + 2 \sum_{m=1}^{n_{a_4}} \text{sgn}(v_m^{a_4}) \frac{1 - \text{sgn}(\delta_m^{a_4})}{2} - 2 \sum_{m=1}^{n_{a_5}} \text{sgn}(v_m^{a_5}) \frac{1 - \text{sgn}(\delta_m^{a_5})}{2} \\
& - 4 \sum_{m=1}^{n_{a_6}} \text{sgn}(v_m^{a_6}) \frac{1 - \text{sgn}(\delta_m^{a_6})}{2} + 2 \sum_{m=1}^{n_{b_2}} \text{sgn}(v_m^{b_2}) \frac{1 - \text{sgn}(\delta_m^{b_2})}{2} - 2 \sum_{m=1}^{n_{b_3}} \text{sgn}(v_m^{b_3}) \frac{1 - \text{sgn}(\delta_m^{b_3})}{2} \\
& + 3 \sum_{m=1}^{n_{d_1}} \text{sgn}(v_m^{d_1}) \frac{1 - \text{sgn}(\delta_m^{d_1})}{2} - 2 \sum_{m=1}^{n_{e_1}} \text{sgn}(v_m^{e_1}) \frac{1 - \text{sgn}(\delta_m^{e_1})}{2} - 3 \sum_{m=1}^{n_{f_1}} \text{sgn}(v_m^{f_1}) \frac{1 - \text{sgn}(\delta_m^{f_1})}{2} \pmod{6}
\end{aligned} \tag{S172.5}$$

### S173. SPACE GROUP NO. 173

| line segment                                        | character of irrep (generators only)                                                                                                                                                                                                                                                                                                         |
|-----------------------------------------------------|----------------------------------------------------------------------------------------------------------------------------------------------------------------------------------------------------------------------------------------------------------------------------------------------------------------------------------------------|
| $a \quad (0, 0, \frac{t}{2})$                       | $\{6_{001}   0 \ 0 \ \frac{1}{2}\}$<br>$a_1 \quad e^{-\frac{1}{2}i\pi t - \frac{5i\pi}{6}}$<br>$a_2 \quad e^{\frac{5i\pi}{6} - \frac{i\pi t}{2}}$<br>$a_3 \quad -ie^{-\frac{1}{2}i\pi t}$<br>$a_4 \quad ie^{-\frac{1}{2}i\pi t}$<br>$a_5 \quad e^{-\frac{1}{2}i\pi t - \frac{i\pi}{6}}$<br>$a_6 \quad e^{\frac{i\pi}{6} - \frac{i\pi t}{2}}$ |
| $b \quad (\frac{1}{3}, \frac{1}{3}, \frac{1-t}{2})$ | $\{3_{001}   0 \ 0 \ 0\}$<br>$b_1 \quad -1$<br>$b_2 \quad e^{-\frac{i\pi}{3}}$<br>$b_3 \quad e^{\frac{i\pi}{3}}$                                                                                                                                                                                                                             |
| $c \quad (\frac{1}{2}, 0, \frac{t}{2})$             | $\{2_{001}   0 \ 0 \ \frac{1}{2}\}$<br>$c_1 \quad -ie^{-\frac{1}{2}i\pi t}$<br>$c_2 \quad ie^{-\frac{1}{2}i\pi t}$                                                                                                                                                                                                                           |
| $d \quad (\frac{t}{3}, \frac{t}{3}, 0)$             | $\{1   0 \ 0 \ 0\}$<br>$d_1 \quad 1$                                                                                                                                                                                                                                                                                                         |
| $e \quad (\frac{t}{3}, \frac{t}{3}, \frac{1}{2})$   | $\{1   0 \ 0 \ 0\}$<br>$e_1 \quad 1$                                                                                                                                                                                                                                                                                                         |
| $f \quad (\frac{3-t}{6}, \frac{t}{3}, 0)$           | $\{1   0 \ 0 \ 0\}$<br>$f_1 \quad 1$                                                                                                                                                                                                                                                                                                         |
| $g \quad (\frac{3-t}{6}, \frac{t}{3}, \frac{1}{2})$ | $\{1   0 \ 0 \ 0\}$<br>$g_1 \quad 1$                                                                                                                                                                                                                                                                                                         |

$$\begin{aligned}
\mathcal{W}_1^{\text{gapless}} = & \sum_{m=1}^{n_{a_1}} \text{sgn}(v_m^{a_1}) \frac{1 - \text{sgn}(\delta_m^{a_1})}{2} + \sum_{m=1}^{n_{a_2}} \text{sgn}(v_m^{a_2}) \frac{1 - \text{sgn}(\delta_m^{a_2})}{2} + \sum_{m=1}^{n_{a_3}} \text{sgn}(v_m^{a_3}) \frac{1 - \text{sgn}(\delta_m^{a_3})}{2} \\
& + \sum_{m=1}^{n_{a_4}} \text{sgn}(v_m^{a_4}) \frac{1 - \text{sgn}(\delta_m^{a_4})}{2} + \sum_{m=1}^{n_{a_5}} \text{sgn}(v_m^{a_5}) \frac{1 - \text{sgn}(\delta_m^{a_5})}{2} + \sum_{m=1}^{n_{a_6}} \text{sgn}(v_m^{a_6}) \frac{1 - \text{sgn}(\delta_m^{a_6})}{2} \\
& - \sum_{m=1}^{n_{c_1}} \text{sgn}(v_m^{c_1}) \frac{1 - \text{sgn}(\delta_m^{c_1})}{2} - \sum_{m=1}^{n_{c_2}} \text{sgn}(v_m^{c_2}) \frac{1 - \text{sgn}(\delta_m^{c_2})}{2} - \sum_{m=1}^{n_{d_1}} \text{sgn}(v_m^{d_1}) \frac{1 - \text{sgn}(\delta_m^{d_1})}{2} \\
& + 2 \sum_{m=1}^{n_{e_1}} \text{sgn}(v_m^{e_1}) \frac{1 - \text{sgn}(\delta_m^{e_1})}{2} + \sum_{m=1}^{n_{f_1}} \text{sgn}(v_m^{f_1}) \frac{1 - \text{sgn}(\delta_m^{f_1})}{2} - 2 \sum_{m=1}^{n_{g_1}} \text{sgn}(v_m^{g_1}) \frac{1 - \text{sgn}(\delta_m^{g_1})}{2}
\end{aligned} \tag{S173.1}$$

$$\begin{aligned}
\mathcal{W}_2^{\text{gapless}} = & \sum_{m=1}^{n_{b_1}} \text{sgn}(v_m^{b_1}) \frac{1 - \text{sgn}(\delta_m^{b_1})}{2} + \sum_{m=1}^{n_{b_2}} \text{sgn}(v_m^{b_2}) \frac{1 - \text{sgn}(\delta_m^{b_2})}{2} + \sum_{m=1}^{n_{b_3}} \text{sgn}(v_m^{b_3}) \frac{1 - \text{sgn}(\delta_m^{b_3})}{2} + \sum_{m=1}^{n_{c_1}} \text{sgn}(v_m^{c_1}) \frac{1 - \text{sgn}(\delta_m^{c_1})}{2} \\
& + \sum_{m=1}^{n_{c_2}} \text{sgn}(v_m^{c_2}) \frac{1 - \text{sgn}(\delta_m^{c_2})}{2} - \sum_{m=1}^{n_{f_1}} \text{sgn}(v_m^{f_1}) \frac{1 - \text{sgn}(\delta_m^{f_1})}{2} + 2 \sum_{m=1}^{n_{g_1}} \text{sgn}(v_m^{g_1}) \frac{1 - \text{sgn}(\delta_m^{g_1})}{2}
\end{aligned} \tag{S173.2}$$

$$\mathcal{W}_1^{\text{gapped}} = - \sum_{m=1}^{n_{b_2}} \text{sgn}(v_m^{b_2}) \frac{1 - \text{sgn}(\delta_m^{b_2})}{2} + \sum_{m=1}^{n_{b_3}} \text{sgn}(v_m^{b_3}) \frac{1 - \text{sgn}(\delta_m^{b_3})}{2} \tag{S173.3}$$

$$\begin{aligned}
\mathcal{W}_2^{\text{gapped}} = & -2 \sum_{m=1}^{n_{a_2}} \text{sgn}(v_m^{a_2}) \frac{1 - \text{sgn}(\delta_m^{a_2})}{2} - \sum_{m=1}^{n_{a_3}} \text{sgn}(v_m^{a_3}) \frac{1 - \text{sgn}(\delta_m^{a_3})}{2} - \sum_{m=1}^{n_{a_4}} \text{sgn}(v_m^{a_4}) \frac{1 - \text{sgn}(\delta_m^{a_4})}{2} \\
& - 2 \sum_{m=1}^{n_{a_5}} \text{sgn}(v_m^{a_5}) \frac{1 - \text{sgn}(\delta_m^{a_5})}{2} + \sum_{m=1}^{n_{c_1}} \text{sgn}(v_m^{c_1}) \frac{1 - \text{sgn}(\delta_m^{c_1})}{2} + \sum_{m=1}^{n_{c_2}} \text{sgn}(v_m^{c_2}) \frac{1 - \text{sgn}(\delta_m^{c_2})}{2} \\
& + \sum_{m=1}^{n_{d_1}} \text{sgn}(v_m^{d_1}) \frac{1 - \text{sgn}(\delta_m^{d_1})}{2} - 2 \sum_{m=1}^{n_{e_1}} \text{sgn}(v_m^{e_1}) \frac{1 - \text{sgn}(\delta_m^{e_1})}{2} - \sum_{m=1}^{n_{f_1}} \text{sgn}(v_m^{f_1}) \frac{1 - \text{sgn}(\delta_m^{f_1})}{2} \\
& + 2 \sum_{m=1}^{n_{g_1}} \text{sgn}(v_m^{g_1}) \frac{1 - \text{sgn}(\delta_m^{g_1})}{2}
\end{aligned} \tag{S173.4}$$

$$\mathcal{X}_1 = \sum_{m=1}^{n_{a_3}} \frac{1 - \text{sgn}(\delta_m^{a_3})}{2} + \sum_{m=1}^{n_{a_4}} \frac{1 - \text{sgn}(\delta_m^{a_4})}{2} \mod 2 \tag{S173.5}$$

$$\begin{aligned}
\mathcal{X}_2 = & 2 \sum_{m=1}^{n_{a_2}} \text{sgn}(v_m^{a_2}) \frac{1 - \text{sgn}(\delta_m^{a_2})}{2} - 2 \sum_{m=1}^{n_{a_4}} \text{sgn}(v_m^{a_4}) \frac{1 - \text{sgn}(\delta_m^{a_4})}{2} + 2 \sum_{m=1}^{n_{a_6}} \text{sgn}(v_m^{a_6}) \frac{1 - \text{sgn}(\delta_m^{a_6})}{2} \\
& - 2 \sum_{m=1}^{n_{c_2}} \text{sgn}(v_m^{c_2}) \frac{1 - \text{sgn}(\delta_m^{c_2})}{2} - \sum_{m=1}^{n_{d_1}} \text{sgn}(v_m^{d_1}) \frac{1 - \text{sgn}(\delta_m^{d_1})}{2} + \sum_{m=1}^{n_{f_1}} \text{sgn}(v_m^{f_1}) \frac{1 - \text{sgn}(\delta_m^{f_1})}{2} \mod 4
\end{aligned} \tag{S173.6}$$

## S174. SPACE GROUP NO. 174

| line segment                                        | character of irrep (generators only)                                                                             |
|-----------------------------------------------------|------------------------------------------------------------------------------------------------------------------|
| $a \quad (0, 0, \frac{t}{2})$                       | $\{3_{001}   0 \ 0 \ 0\}$<br>$a_1 \quad -1$<br>$a_2 \quad e^{-\frac{i\pi}{3}}$<br>$a_3 \quad e^{\frac{i\pi}{3}}$ |
| $b \quad (\frac{1}{3}, \frac{1}{3}, \frac{1-t}{2})$ | $\{3_{001}   0 \ 0 \ 0\}$<br>$b_1 \quad -1$<br>$b_2 \quad e^{-\frac{i\pi}{3}}$<br>$b_3 \quad e^{\frac{i\pi}{3}}$ |
| $c \quad (\frac{1}{2}, 0, \frac{t}{2})$             | $\{1   0 \ 0 \ 0\}$<br>$c_1 \quad 1$                                                                             |
| $d \quad (\frac{t}{3}, \frac{t}{3}, 0)$             | $\{m_{001}   0 \ 0 \ 0\}$<br>$d_1 \quad -i$<br>$d_2 \quad i$                                                     |
| $e \quad (\frac{t}{3}, \frac{t}{3}, \frac{1}{2})$   | $\{m_{001}   0 \ 0 \ 0\}$<br>$e_1 \quad -i$<br>$e_2 \quad i$                                                     |
| $f \quad (\frac{3-t}{6}, \frac{t}{3}, 0)$           | $\{m_{001}   0 \ 0 \ 0\}$<br>$f_1 \quad -i$<br>$f_2 \quad i$                                                     |
| $g \quad (\frac{3-t}{6}, \frac{t}{3}, \frac{1}{2})$ | $\{m_{001}   0 \ 0 \ 0\}$<br>$g_1 \quad -i$<br>$g_2 \quad i$                                                     |

$$\begin{aligned}
\mathcal{W}_1^{\text{gapless}} = & \sum_{m=1}^{n_{a_1}} \text{sgn}(v_m^{a_1}) \frac{1 - \text{sgn}(\delta_m^{a_1})}{2} + 2 \sum_{m=1}^{n_{a_2}} \text{sgn}(v_m^{a_2}) \frac{1 - \text{sgn}(\delta_m^{a_2})}{2} - \sum_{m=1}^{n_{c_1}} \text{sgn}(v_m^{c_1}) \frac{1 - \text{sgn}(\delta_m^{c_1})}{2} \\
& - 2 \sum_{m=1}^{n_{d_2}} \text{sgn}(v_m^{d_2}) \frac{1 - \text{sgn}(\delta_m^{d_2})}{2} + 2 \sum_{m=1}^{n_{e_2}} \text{sgn}(v_m^{e_2}) \frac{1 - \text{sgn}(\delta_m^{e_2})}{2} + 2 \sum_{m=1}^{n_{f_2}} \text{sgn}(v_m^{f_2}) \frac{1 - \text{sgn}(\delta_m^{f_2})}{2} \\
& - 2 \sum_{m=1}^{n_{g_2}} \text{sgn}(v_m^{g_2}) \frac{1 - \text{sgn}(\delta_m^{g_2})}{2}
\end{aligned} \tag{S174.1}$$

$$\begin{aligned}
\mathcal{W}_2^{\text{gapless}} = & \sum_{m=1}^{n_{b_1}} \text{sgn}(v_m^{b_1}) \frac{1 - \text{sgn}(\delta_m^{b_1})}{2} + \sum_{m=1}^{n_{b_2}} \text{sgn}(v_m^{b_2}) \frac{1 - \text{sgn}(\delta_m^{b_2})}{2} + \sum_{m=1}^{n_{b_3}} \text{sgn}(v_m^{b_3}) \frac{1 - \text{sgn}(\delta_m^{b_3})}{2} \\
& + \sum_{m=1}^{n_{c_1}} \text{sgn}(v_m^{c_1}) \frac{1 - \text{sgn}(\delta_m^{c_1})}{2} - \sum_{m=1}^{n_{f_1}} \text{sgn}(v_m^{f_1}) \frac{1 - \text{sgn}(\delta_m^{f_1})}{2} - \sum_{m=1}^{n_{f_2}} \text{sgn}(v_m^{f_2}) \frac{1 - \text{sgn}(\delta_m^{f_2})}{2} \\
& + \sum_{m=1}^{n_{g_1}} \text{sgn}(v_m^{g_1}) \frac{1 - \text{sgn}(\delta_m^{g_1})}{2} + \sum_{m=1}^{n_{g_2}} \text{sgn}(v_m^{g_2}) \frac{1 - \text{sgn}(\delta_m^{g_2})}{2}
\end{aligned} \tag{S174.2}$$

$$\begin{aligned}
\mathcal{W}_3^{\text{gapless}} = & \sum_{m=1}^{n_{d_1}} \text{sgn}(v_m^{d_1}) \frac{1 - \text{sgn}(\delta_m^{d_1})}{2} - \sum_{m=1}^{n_{d_2}} \text{sgn}(v_m^{d_2}) \frac{1 - \text{sgn}(\delta_m^{d_2})}{2} - \sum_{m=1}^{n_{f_1}} \text{sgn}(v_m^{f_1}) \frac{1 - \text{sgn}(\delta_m^{f_1})}{2} + \sum_{m=1}^{n_{f_2}} \text{sgn}(v_m^{f_2}) \frac{1 - \text{sgn}(\delta_m^{f_2})}{2}
\end{aligned} \tag{S174.3}$$

$$\begin{aligned}
\mathcal{W}_4^{\text{gapless}} = & \sum_{m=1}^{n_{e_1}} \text{sgn}(v_m^{e_1}) \frac{1 - \text{sgn}(\delta_m^{e_1})}{2} - \sum_{m=1}^{n_{e_2}} \text{sgn}(v_m^{e_2}) \frac{1 - \text{sgn}(\delta_m^{e_2})}{2} - \sum_{m=1}^{n_{g_1}} \text{sgn}(v_m^{g_1}) \frac{1 - \text{sgn}(\delta_m^{g_1})}{2} + \sum_{m=1}^{n_{g_2}} \text{sgn}(v_m^{g_2}) \frac{1 - \text{sgn}(\delta_m^{g_2})}{2}
\end{aligned} \tag{S174.4}$$

$$\mathcal{X}_1 = \sum_{m=1}^{n_{c_1}} \frac{1 - \text{sgn}(\delta_m^{c_1})}{2} \mod 2 \quad (\text{S174.5})$$

### S175. SPACE GROUP NO. 175

| line segment                                        | character of irrep (generators only)                                                                                                                                                                     |
|-----------------------------------------------------|----------------------------------------------------------------------------------------------------------------------------------------------------------------------------------------------------------|
| $a \quad (0, 0, \frac{t}{2})$                       | $\{6_{001}   0 \ 0 \ 0\}$<br>$a_1 \quad e^{-\frac{5i\pi}{6}}$<br>$a_2 \quad e^{\frac{5i\pi}{6}}$<br>$a_3 \quad -i$<br>$a_4 \quad i$<br>$a_5 \quad e^{-\frac{i\pi}{6}}$<br>$a_6 \quad e^{\frac{i\pi}{6}}$ |
| $b \quad (\frac{1}{3}, \frac{1}{3}, \frac{1-t}{2})$ | $\{3_{001}   0 \ 0 \ 0\}$<br>$b_1 \quad -1$<br>$b_2 \quad e^{-\frac{i\pi}{3}}$<br>$b_3 \quad e^{\frac{i\pi}{3}}$                                                                                         |
| $c \quad (\frac{1}{2}, 0, \frac{t}{2})$             | $\{2_{001}   0 \ 0 \ 0\}$<br>$c_1 \quad -i$<br>$c_2 \quad i$                                                                                                                                             |
| $d \quad (\frac{t}{3}, \frac{t}{3}, 0)$             | $\{m_{001}   0 \ 0 \ 0\}$<br>$d_1 \quad -i$<br>$d_2 \quad i$                                                                                                                                             |
| $e \quad (\frac{t}{3}, \frac{t}{3}, \frac{1}{2})$   | $\{m_{001}   0 \ 0 \ 0\}$<br>$e_1 \quad -i$<br>$e_2 \quad i$                                                                                                                                             |
| $f \quad (\frac{3-t}{6}, \frac{t}{3}, 0)$           | $\{m_{001}   0 \ 0 \ 0\}$<br>$f_1 \quad -i$<br>$f_2 \quad i$                                                                                                                                             |
| $g \quad (\frac{3-t}{6}, \frac{t}{3}, \frac{1}{2})$ | $\{m_{001}   0 \ 0 \ 0\}$<br>$g_1 \quad -i$<br>$g_2 \quad i$                                                                                                                                             |

$$\begin{aligned}
\mathcal{W}_1^{\text{gapless}} = & \sum_{m=1}^{n_{a_1}} \text{sgn}(v_m^{a_1}) \frac{1 - \text{sgn}(\delta_m^{a_1})}{2} + \sum_{m=1}^{n_{a_3}} \text{sgn}(v_m^{a_3}) \frac{1 - \text{sgn}(\delta_m^{a_3})}{2} + \sum_{m=1}^{n_{a_5}} \text{sgn}(v_m^{a_5}) \frac{1 - \text{sgn}(\delta_m^{a_5})}{2} \\
& - \sum_{m=1}^{n_{c_1}} \text{sgn}(v_m^{c_1}) \frac{1 - \text{sgn}(\delta_m^{c_1})}{2} - \sum_{m=1}^{n_{d_1}} \text{sgn}(v_m^{d_1}) \frac{1 - \text{sgn}(\delta_m^{d_1})}{2} + \sum_{m=1}^{n_{e_1}} \text{sgn}(v_m^{e_1}) \frac{1 - \text{sgn}(\delta_m^{e_1})}{2} \\
& + \sum_{m=1}^{n_{f_1}} \text{sgn}(v_m^{f_1}) \frac{1 - \text{sgn}(\delta_m^{f_1})}{2} - \sum_{m=1}^{n_{g_1}} \text{sgn}(v_m^{g_1}) \frac{1 - \text{sgn}(\delta_m^{g_1})}{2}
\end{aligned} \quad (\text{S175.1})$$

$$\begin{aligned}
\mathcal{W}_2^{\text{gapless}} = & \sum_{m=1}^{n_{b_1}} \text{sgn}(v_m^{b_1}) \frac{1 - \text{sgn}(\delta_m^{b_1})}{2} + \sum_{m=1}^{n_{b_2}} \text{sgn}(v_m^{b_2}) \frac{1 - \text{sgn}(\delta_m^{b_2})}{2} + \sum_{m=1}^{n_{c_1}} \text{sgn}(v_m^{c_1}) \frac{1 - \text{sgn}(\delta_m^{c_1})}{2} \\
& - \sum_{m=1}^{n_{f_1}} \text{sgn}(v_m^{f_1}) \frac{1 - \text{sgn}(\delta_m^{f_1})}{2} + \sum_{m=1}^{n_{g_1}} \text{sgn}(v_m^{g_1}) \frac{1 - \text{sgn}(\delta_m^{g_1})}{2}
\end{aligned} \quad (\text{S175.2})$$

## S176. SPACE GROUP NO. 176

| line segment                                        | character of irrep (generators only)                 |
|-----------------------------------------------------|------------------------------------------------------|
| $a \quad (0, 0, \frac{t}{2})$                       | $\{6_{001}   0 \ 0 \ \frac{1}{2}\}$                  |
|                                                     | $a_1 \quad e^{-\frac{1}{2}i\pi t - \frac{5i\pi}{6}}$ |
|                                                     | $a_2 \quad e^{\frac{5i\pi}{6} - \frac{i\pi t}{2}}$   |
|                                                     | $a_3 \quad -ie^{-\frac{1}{2}i\pi t}$                 |
|                                                     | $a_4 \quad ie^{-\frac{1}{2}i\pi t}$                  |
|                                                     | $a_5 \quad e^{-\frac{1}{2}i\pi t - \frac{i\pi}{6}}$  |
|                                                     | $a_6 \quad e^{\frac{i\pi}{6} - \frac{i\pi t}{2}}$    |
| $b \quad (\frac{1}{3}, \frac{1}{3}, \frac{1-t}{2})$ | $\{3_{001}   0 \ 0 \ 0\}$                            |
|                                                     | $b_1 \quad -1$                                       |
|                                                     | $b_2 \quad e^{-\frac{i\pi}{3}}$                      |
|                                                     | $b_3 \quad e^{\frac{i\pi}{3}}$                       |
| $c \quad (\frac{1}{2}, 0, \frac{t}{2})$             | $\{2_{001}   0 \ 0 \ \frac{1}{2}\}$                  |
|                                                     | $c_1 \quad -ie^{-\frac{1}{2}i\pi t}$                 |
|                                                     | $c_2 \quad ie^{-\frac{1}{2}i\pi t}$                  |
| $d \quad (\frac{t}{3}, \frac{t}{3}, 0)$             | $\{m_{001}   0 \ 0 \ \frac{1}{2}\}$                  |
|                                                     | $d_1 \quad -i$                                       |
|                                                     | $d_2 \quad i$                                        |
| $e \quad (\frac{t}{3}, \frac{t}{3}, \frac{1}{2})$   | $\{m_{001}   0 \ 0 \ \frac{1}{2}\}$                  |
|                                                     | $e_1 \quad i$                                        |
|                                                     | $e_2 \quad -i$                                       |
| $f \quad (\frac{3-t}{6}, \frac{t}{3}, 0)$           | $\{m_{001}   0 \ 0 \ \frac{1}{2}\}$                  |
|                                                     | $f_1 \quad -i$                                       |
|                                                     | $f_2 \quad i$                                        |
| $g \quad (\frac{3-t}{6}, \frac{t}{3}, \frac{1}{2})$ | $\{m_{001}   0 \ 0 \ \frac{1}{2}\}$                  |
|                                                     | $g_1 \quad i$                                        |
|                                                     | $g_2 \quad -i$                                       |

$$\begin{aligned}
\mathcal{W}_1^{\text{gapless}} = & \sum_{m=1}^{n_{a_1}} \text{sgn}(v_m^{a_1}) \frac{1 - \text{sgn}(\delta_m^{a_1})}{2} + \sum_{m=1}^{n_{a_3}} \text{sgn}(v_m^{a_3}) \frac{1 - \text{sgn}(\delta_m^{a_3})}{2} + \sum_{m=1}^{n_{a_5}} \text{sgn}(v_m^{a_5}) \frac{1 - \text{sgn}(\delta_m^{a_5})}{2} \\
& - \sum_{m=1}^{n_{c_1}} \text{sgn}(v_m^{c_1}) \frac{1 - \text{sgn}(\delta_m^{c_1})}{2} - \sum_{m=1}^{n_{d_1}} \text{sgn}(v_m^{d_1}) \frac{1 - \text{sgn}(\delta_m^{d_1})}{2} + 2 \sum_{m=1}^{n_{e_2}} \text{sgn}(v_m^{e_2}) \frac{1 - \text{sgn}(\delta_m^{e_2})}{2} \\
& + \sum_{m=1}^{n_{f_1}} \text{sgn}(v_m^{f_1}) \frac{1 - \text{sgn}(\delta_m^{f_1})}{2} - 2 \sum_{m=1}^{n_{g_2}} \text{sgn}(v_m^{g_2}) \frac{1 - \text{sgn}(\delta_m^{g_2})}{2}
\end{aligned} \tag{S176.1}$$

$$\begin{aligned}
\mathcal{W}_2^{\text{gapless}} = & \sum_{m=1}^{n_{b_1}} \text{sgn}(v_m^{b_1}) \frac{1 - \text{sgn}(\delta_m^{b_1})}{2} + \sum_{m=1}^{n_{b_2}} \text{sgn}(v_m^{b_2}) \frac{1 - \text{sgn}(\delta_m^{b_2})}{2} + \sum_{m=1}^{n_{c_1}} \text{sgn}(v_m^{c_1}) \frac{1 - \text{sgn}(\delta_m^{c_1})}{2} \\
& - \sum_{m=1}^{n_{f_1}} \text{sgn}(v_m^{f_1}) \frac{1 - \text{sgn}(\delta_m^{f_1})}{2} + \sum_{m=1}^{n_{g_1}} \text{sgn}(v_m^{g_1}) \frac{1 - \text{sgn}(\delta_m^{g_1})}{2} + \sum_{m=1}^{n_{g_2}} \text{sgn}(v_m^{g_2}) \frac{1 - \text{sgn}(\delta_m^{g_2})}{2}
\end{aligned} \tag{S176.2}$$

$$\begin{aligned}
\mathcal{W}_3^{\text{gapless}} = & \sum_{m=1}^{n_{e_1}} \text{sgn}(v_m^{e_1}) \frac{1 - \text{sgn}(\delta_m^{e_1})}{2} - \sum_{m=1}^{n_{e_2}} \text{sgn}(v_m^{e_2}) \frac{1 - \text{sgn}(\delta_m^{e_2})}{2} - \sum_{m=1}^{n_{g_1}} \text{sgn}(v_m^{g_1}) \frac{1 - \text{sgn}(\delta_m^{g_1})}{2} + \sum_{m=1}^{n_{g_2}} \text{sgn}(v_m^{g_2}) \frac{1 - \text{sgn}(\delta_m^{g_2})}{2}
\end{aligned} \tag{S176.3}$$



## S177. SPACE GROUP NO. 177

| line segment                                               | character of irrep (generators only)                                                                                                                                                                     |
|------------------------------------------------------------|----------------------------------------------------------------------------------------------------------------------------------------------------------------------------------------------------------|
| $a \left( \frac{t}{3}, \frac{t}{3}, 0 \right)$             | $\{2_{110}   0 \ 0 \ 0\}$<br>$a_1 \quad -i$<br>$a_2 \quad i$                                                                                                                                             |
| $b \left( 0, \frac{t}{2}, 0 \right)$                       | $\{2_{010}   0 \ 0 \ 0\}$<br>$b_1 \quad -i$<br>$b_2 \quad i$                                                                                                                                             |
| $c \left( \frac{t}{3}, \frac{3-t}{6}, 0 \right)$           | $\{2_{100}   0 \ 0 \ 0\}$<br>$c_1 \quad -i$<br>$c_2 \quad i$                                                                                                                                             |
| $d \left( \frac{t}{3}, \frac{t}{3}, \frac{1}{2} \right)$   | $\{2_{110}   0 \ 0 \ 0\}$<br>$d_1 \quad -i$<br>$d_2 \quad i$                                                                                                                                             |
| $e \left( 0, \frac{t}{2}, \frac{1}{2} \right)$             | $\{2_{010}   0 \ 0 \ 0\}$<br>$e_1 \quad -i$<br>$e_2 \quad i$                                                                                                                                             |
| $f \left( \frac{t}{3}, \frac{3-t}{6}, \frac{1}{2} \right)$ | $\{2_{100}   0 \ 0 \ 0\}$<br>$f_1 \quad -i$<br>$f_2 \quad i$                                                                                                                                             |
| $g \left( 0, 0, \frac{t}{2} \right)$                       | $\{6_{001}   0 \ 0 \ 0\}$<br>$g_1 \quad e^{-\frac{5i\pi}{6}}$<br>$g_2 \quad e^{\frac{5i\pi}{6}}$<br>$g_3 \quad -i$<br>$g_4 \quad i$<br>$g_5 \quad e^{-\frac{i\pi}{6}}$<br>$g_6 \quad e^{\frac{i\pi}{6}}$ |
| $h \left( 0, \frac{1}{2}, \frac{t}{2} \right)$             | $\{2_{001}   0 \ 0 \ 0\}$<br>$h_1 \quad -i$<br>$h_2 \quad i$                                                                                                                                             |
| $i \left( \frac{1}{3}, \frac{1}{3}, \frac{t}{2} \right)$   | $\{3_{001}   0 \ 0 \ 0\}$<br>$i_1 \quad -1$<br>$i_2 \quad e^{-\frac{i\pi}{3}}$<br>$i_3 \quad e^{\frac{i\pi}{3}}$                                                                                         |

$$\begin{aligned}
\mathcal{W}_1^{\text{gapless}} = & \sum_{m=1}^{n_{a_1}} \text{sgn}(v_m^{a_1}) \frac{1 - \text{sgn}(\delta_m^{a_1})}{2} + \sum_{m=1}^{n_{a_2}} \text{sgn}(v_m^{a_2}) \frac{1 - \text{sgn}(\delta_m^{a_2})}{2} - \sum_{m=1}^{n_{e_1}} \text{sgn}(v_m^{e_1}) \frac{1 - \text{sgn}(\delta_m^{e_1})}{2} \\
& - \sum_{m=1}^{n_{e_2}} \text{sgn}(v_m^{e_2}) \frac{1 - \text{sgn}(\delta_m^{e_2})}{2} - \sum_{m=1}^{n_{f_1}} \text{sgn}(v_m^{f_1}) \frac{1 - \text{sgn}(\delta_m^{f_1})}{2} - \sum_{m=1}^{n_{f_2}} \text{sgn}(v_m^{f_2}) \frac{1 - \text{sgn}(\delta_m^{f_2})}{2} \\
& - \sum_{m=1}^{n_{g_1}} \text{sgn}(v_m^{g_1}) \frac{1 - \text{sgn}(\delta_m^{g_1})}{2} - \sum_{m=1}^{n_{g_2}} \text{sgn}(v_m^{g_2}) \frac{1 - \text{sgn}(\delta_m^{g_2})}{2} - \sum_{m=1}^{n_{g_3}} \text{sgn}(v_m^{g_3}) \frac{1 - \text{sgn}(\delta_m^{g_3})}{2} \\
& - \sum_{m=1}^{n_{g_4}} \text{sgn}(v_m^{g_4}) \frac{1 - \text{sgn}(\delta_m^{g_4})}{2} - \sum_{m=1}^{n_{g_5}} \text{sgn}(v_m^{g_5}) \frac{1 - \text{sgn}(\delta_m^{g_5})}{2} - \sum_{m=1}^{n_{g_6}} \text{sgn}(v_m^{g_6}) \frac{1 - \text{sgn}(\delta_m^{g_6})}{2} \\
& + \sum_{m=1}^{n_{i_1}} \text{sgn}(v_m^{i_1}) \frac{1 - \text{sgn}(\delta_m^{i_1})}{2} + \sum_{m=1}^{n_{i_2}} \text{sgn}(v_m^{i_2}) \frac{1 - \text{sgn}(\delta_m^{i_2})}{2} + \sum_{m=1}^{n_{i_3}} \text{sgn}(v_m^{i_3}) \frac{1 - \text{sgn}(\delta_m^{i_3})}{2}
\end{aligned} \tag{S177.1}$$

$$\begin{aligned}
\mathcal{W}_2^{\text{gapless}} = & \sum_{m=1}^{n_{b_1}} \text{sgn}(v_m^{b_1}) \frac{1 - \text{sgn}(\delta_m^{b_1})}{2} + \sum_{m=1}^{n_{b_2}} \text{sgn}(v_m^{b_2}) \frac{1 - \text{sgn}(\delta_m^{b_2})}{2} - \sum_{m=1}^{n_{e_1}} \text{sgn}(v_m^{e_1}) \frac{1 - \text{sgn}(\delta_m^{e_1})}{2} \\
& - \sum_{m=1}^{n_{e_2}} \text{sgn}(v_m^{e_2}) \frac{1 - \text{sgn}(\delta_m^{e_2})}{2} - \sum_{m=1}^{n_{g_1}} \text{sgn}(v_m^{g_1}) \frac{1 - \text{sgn}(\delta_m^{g_1})}{2} - \sum_{m=1}^{n_{g_2}} \text{sgn}(v_m^{g_2}) \frac{1 - \text{sgn}(\delta_m^{g_2})}{2} \\
& - \sum_{m=1}^{n_{g_3}} \text{sgn}(v_m^{g_3}) \frac{1 - \text{sgn}(\delta_m^{g_3})}{2} - \sum_{m=1}^{n_{g_4}} \text{sgn}(v_m^{g_4}) \frac{1 - \text{sgn}(\delta_m^{g_4})}{2} - \sum_{m=1}^{n_{g_5}} \text{sgn}(v_m^{g_5}) \frac{1 - \text{sgn}(\delta_m^{g_5})}{2} \\
& - \sum_{m=1}^{n_{g_6}} \text{sgn}(v_m^{g_6}) \frac{1 - \text{sgn}(\delta_m^{g_6})}{2} + \sum_{m=1}^{n_{h_1}} \text{sgn}(v_m^{h_1}) \frac{1 - \text{sgn}(\delta_m^{h_1})}{2} + \sum_{m=1}^{n_{h_2}} \text{sgn}(v_m^{h_2}) \frac{1 - \text{sgn}(\delta_m^{h_2})}{2}
\end{aligned} \tag{S177.2}$$

$$\begin{aligned}
\mathcal{W}_3^{\text{gapless}} = & \sum_{m=1}^{n_{c_1}} \text{sgn}(v_m^{c_1}) \frac{1 - \text{sgn}(\delta_m^{c_1})}{2} + \sum_{m=1}^{n_{c_2}} \text{sgn}(v_m^{c_2}) \frac{1 - \text{sgn}(\delta_m^{c_2})}{2} - \sum_{m=1}^{n_{f_1}} \text{sgn}(v_m^{f_1}) \frac{1 - \text{sgn}(\delta_m^{f_1})}{2} \\
& - \sum_{m=1}^{n_{f_2}} \text{sgn}(v_m^{f_2}) \frac{1 - \text{sgn}(\delta_m^{f_2})}{2} - \sum_{m=1}^{n_{h_1}} \text{sgn}(v_m^{h_1}) \frac{1 - \text{sgn}(\delta_m^{h_1})}{2} - \sum_{m=1}^{n_{h_2}} \text{sgn}(v_m^{h_2}) \frac{1 - \text{sgn}(\delta_m^{h_2})}{2} \\
& + \sum_{m=1}^{n_{i_1}} \text{sgn}(v_m^{i_1}) \frac{1 - \text{sgn}(\delta_m^{i_1})}{2} + \sum_{m=1}^{n_{i_2}} \text{sgn}(v_m^{i_2}) \frac{1 - \text{sgn}(\delta_m^{i_2})}{2} + \sum_{m=1}^{n_{i_3}} \text{sgn}(v_m^{i_3}) \frac{1 - \text{sgn}(\delta_m^{i_3})}{2}
\end{aligned} \tag{S177.3}$$

$$\begin{aligned}
\mathcal{W}_4^{\text{gapless}} = & \sum_{m=1}^{n_{d_1}} \text{sgn}(v_m^{d_1}) \frac{1 - \text{sgn}(\delta_m^{d_1})}{2} + \sum_{m=1}^{n_{d_2}} \text{sgn}(v_m^{d_2}) \frac{1 - \text{sgn}(\delta_m^{d_2})}{2} - \sum_{m=1}^{n_{e_1}} \text{sgn}(v_m^{e_1}) \frac{1 - \text{sgn}(\delta_m^{e_1})}{2} \\
& - \sum_{m=1}^{n_{e_2}} \text{sgn}(v_m^{e_2}) \frac{1 - \text{sgn}(\delta_m^{e_2})}{2} - \sum_{m=1}^{n_{f_1}} \text{sgn}(v_m^{f_1}) \frac{1 - \text{sgn}(\delta_m^{f_1})}{2} - \sum_{m=1}^{n_{f_2}} \text{sgn}(v_m^{f_2}) \frac{1 - \text{sgn}(\delta_m^{f_2})}{2}
\end{aligned} \tag{S177.4}$$

$$\mathcal{W}_1^{\text{gapped}} = - \sum_{m=1}^{n_{g_1}} \text{sgn}(v_m^{g_1}) \frac{1 - \text{sgn}(\delta_m^{g_1})}{2} + \sum_{m=1}^{n_{g_2}} \text{sgn}(v_m^{g_2}) \frac{1 - \text{sgn}(\delta_m^{g_2})}{2} \tag{S177.5}$$

$$\mathcal{W}_2^{\text{gapped}} = - \sum_{m=1}^{n_{g_3}} \text{sgn}(v_m^{g_3}) \frac{1 - \text{sgn}(\delta_m^{g_3})}{2} + \sum_{m=1}^{n_{g_4}} \text{sgn}(v_m^{g_4}) \frac{1 - \text{sgn}(\delta_m^{g_4})}{2} \tag{S177.6}$$

$$\begin{aligned}
\mathcal{W}_3^{\text{gapped}} = & \sum_{m=1}^{n_{b_2}} \text{sgn}(v_m^{b_2}) \frac{1 - \text{sgn}(\delta_m^{b_2})}{2} - \sum_{m=1}^{n_{e_2}} \text{sgn}(v_m^{e_2}) \frac{1 - \text{sgn}(\delta_m^{e_2})}{2} - \sum_{m=1}^{n_{g_1}} \text{sgn}(v_m^{g_1}) \frac{1 - \text{sgn}(\delta_m^{g_1})}{2} \\
& - \sum_{m=1}^{n_{g_3}} \text{sgn}(v_m^{g_3}) \frac{1 - \text{sgn}(\delta_m^{g_3})}{2} - \sum_{m=1}^{n_{g_5}} \text{sgn}(v_m^{g_5}) \frac{1 - \text{sgn}(\delta_m^{g_5})}{2} + \sum_{m=1}^{n_{h_1}} \text{sgn}(v_m^{h_1}) \frac{1 - \text{sgn}(\delta_m^{h_1})}{2}
\end{aligned} \tag{S177.7}$$

$$\mathcal{W}_4^{\text{gapped}} = - \sum_{m=1}^{n_{g_5}} \text{sgn}(v_m^{g_5}) \frac{1 - \text{sgn}(\delta_m^{g_5})}{2} + \sum_{m=1}^{n_{g_6}} \text{sgn}(v_m^{g_6}) \frac{1 - \text{sgn}(\delta_m^{g_6})}{2} \tag{S177.8}$$

$$\begin{aligned}
\mathcal{W}_5^{\text{gapped}} = & - \sum_{m=1}^{n_{a_2}} \text{sgn}(v_m^{a_2}) \frac{1 - \text{sgn}(\delta_m^{a_2})}{2} - \sum_{m=1}^{n_{c_2}} \text{sgn}(v_m^{c_2}) \frac{1 - \text{sgn}(\delta_m^{c_2})}{2} + \sum_{m=1}^{n_{d_2}} \text{sgn}(v_m^{d_2}) \frac{1 - \text{sgn}(\delta_m^{d_2})}{2} \\
& + \sum_{m=1}^{n_{f_2}} \text{sgn}(v_m^{f_2}) \frac{1 - \text{sgn}(\delta_m^{f_2})}{2} + \sum_{m=1}^{n_{g_1}} \text{sgn}(v_m^{g_1}) \frac{1 - \text{sgn}(\delta_m^{g_1})}{2} + \sum_{m=1}^{n_{g_3}} \text{sgn}(v_m^{g_3}) \frac{1 - \text{sgn}(\delta_m^{g_3})}{2} \\
& + \sum_{m=1}^{n_{g_5}} \text{sgn}(v_m^{g_5}) \frac{1 - \text{sgn}(\delta_m^{g_5})}{2} + \sum_{m=1}^{n_{h_1}} \text{sgn}(v_m^{h_1}) \frac{1 - \text{sgn}(\delta_m^{h_1})}{2} - \sum_{m=1}^{n_{i_1}} \text{sgn}(v_m^{i_1}) \frac{1 - \text{sgn}(\delta_m^{i_1})}{2} \\
& - 2 \sum_{m=1}^{n_{i_2}} \text{sgn}(v_m^{i_2}) \frac{1 - \text{sgn}(\delta_m^{i_2})}{2}
\end{aligned} \tag{S177.9}$$

$$\mathcal{W}_6^{\text{gapped}} = - \sum_{m=1}^{n_{h_1}} \text{sgn}(v_m^{h_1}) \frac{1 - \text{sgn}(\delta_m^{h_1})}{2} + \sum_{m=1}^{n_{h_2}} \text{sgn}(v_m^{h_2}) \frac{1 - \text{sgn}(\delta_m^{h_2})}{2} \tag{S177.10}$$

$$\mathcal{W}_7^{\text{gapped}} = \sum_{m=1}^{n_{e_1}} \text{sgn}(v_m^{e_1}) \frac{1 - \text{sgn}(\delta_m^{e_1})}{2} - \sum_{m=1}^{n_{e_2}} \text{sgn}(v_m^{e_2}) \frac{1 - \text{sgn}(\delta_m^{e_2})}{2} \tag{S177.11}$$

$$\begin{aligned}
\mathcal{W}_8^{\text{gapped}} = & - \sum_{m=1}^{n_{a_2}} \text{sgn}(v_m^{a_2}) \frac{1 - \text{sgn}(\delta_m^{a_2})}{2} - \sum_{m=1}^{n_{c_2}} \text{sgn}(v_m^{c_2}) \frac{1 - \text{sgn}(\delta_m^{c_2})}{2} + \sum_{m=1}^{n_{e_2}} \text{sgn}(v_m^{e_2}) \frac{1 - \text{sgn}(\delta_m^{e_2})}{2} \\
& + \sum_{m=1}^{n_{f_1}} \text{sgn}(v_m^{f_1}) \frac{1 - \text{sgn}(\delta_m^{f_1})}{2} + \sum_{m=1}^{n_{f_2}} \text{sgn}(v_m^{f_2}) \frac{1 - \text{sgn}(\delta_m^{f_2})}{2} + \sum_{m=1}^{n_{g_1}} \text{sgn}(v_m^{g_1}) \frac{1 - \text{sgn}(\delta_m^{g_1})}{2} \\
& + \sum_{m=1}^{n_{g_3}} \text{sgn}(v_m^{g_3}) \frac{1 - \text{sgn}(\delta_m^{g_3})}{2} + \sum_{m=1}^{n_{g_5}} \text{sgn}(v_m^{g_5}) \frac{1 - \text{sgn}(\delta_m^{g_5})}{2} + \sum_{m=1}^{n_{h_1}} \text{sgn}(v_m^{h_1}) \frac{1 - \text{sgn}(\delta_m^{h_1})}{2} \\
& - \sum_{m=1}^{n_{i_1}} \text{sgn}(v_m^{i_1}) \frac{1 - \text{sgn}(\delta_m^{i_1})}{2} - 2 \sum_{m=1}^{n_{i_2}} \text{sgn}(v_m^{i_2}) \frac{1 - \text{sgn}(\delta_m^{i_2})}{2}
\end{aligned} \tag{S177.12}$$

$$\mathcal{W}_9^{\text{gapped}} = - \sum_{m=1}^{n_{i_2}} \text{sgn}(v_m^{i_2}) \frac{1 - \text{sgn}(\delta_m^{i_2})}{2} + \sum_{m=1}^{n_{i_3}} \text{sgn}(v_m^{i_3}) \frac{1 - \text{sgn}(\delta_m^{i_3})}{2} \tag{S177.13}$$

### S178. SPACE GROUP NO. 178

| line segment                              | character of irrep (generators only) |
|-------------------------------------------|--------------------------------------|
| $a \quad (\frac{t}{3}, \frac{t}{3}, 0)$   | $\{2_{110}   0 \ 0 \ \frac{1}{3}\}$  |
|                                           | $a_1 \quad -i$<br>$a_2 \quad i$      |
| $b \quad (0, \frac{t}{2}, 0)$             | $\{2_{010}   0 \ 0 \ \frac{1}{2}\}$  |
|                                           | $b_1 \quad -i$<br>$b_2 \quad i$      |
| $c \quad (\frac{t}{3}, \frac{3-t}{6}, 0)$ | $\{2_{100}   0 \ 0 \ 0\}$            |
|                                           | $c_1 \quad -i$<br>$c_2 \quad i$      |

|                                                     |                                                                                                                                                                                                                                                                                                                                              |
|-----------------------------------------------------|----------------------------------------------------------------------------------------------------------------------------------------------------------------------------------------------------------------------------------------------------------------------------------------------------------------------------------------------|
| $d \quad (\frac{t}{3}, \frac{t}{3}, \frac{1}{2})$   | $\{2_{110}   0 \ 0 \ \frac{1}{3}\}$<br>$d_1 \quad i$<br>$d_2 \quad -i$                                                                                                                                                                                                                                                                       |
| $e \quad (0, \frac{t}{2}, \frac{1}{2})$             | $\{2_{010}   0 \ 0 \ \frac{1}{2}\}$<br>$e_1 \quad i$<br>$e_2 \quad -i$                                                                                                                                                                                                                                                                       |
| $f \quad (\frac{t}{3}, \frac{3-t}{6}, \frac{1}{2})$ | $\{2_{100}   0 \ 0 \ 0\}$<br>$f_1 \quad -i$<br>$f_2 \quad i$                                                                                                                                                                                                                                                                                 |
| $g \quad (0, 0, \frac{t}{2})$                       | $\{6_{001}   0 \ 0 \ \frac{1}{6}\}$<br>$g_1 \quad e^{-\frac{1}{6}i\pi t - \frac{5i\pi}{6}}$<br>$g_2 \quad e^{\frac{5i\pi}{6} - \frac{i\pi t}{6}}$<br>$g_3 \quad -ie^{-\frac{1}{6}i\pi t}$<br>$g_4 \quad ie^{-\frac{1}{6}i\pi t}$<br>$g_5 \quad e^{-\frac{1}{6}i\pi t - \frac{i\pi}{6}}$<br>$g_6 \quad e^{\frac{i\pi}{6} - \frac{i\pi t}{6}}$ |
| $h \quad (0, \frac{1}{2}, \frac{t}{2})$             | $\{2_{001}   0 \ 0 \ \frac{1}{2}\}$<br>$h_1 \quad -ie^{-\frac{1}{2}i\pi t}$<br>$h_2 \quad ie^{-\frac{1}{2}i\pi t}$                                                                                                                                                                                                                           |
| $i \quad (\frac{1}{3}, \frac{1}{3}, \frac{t}{2})$   | $\{3_{001}   0 \ 0 \ \frac{1}{3}\}$<br>$i_1 \quad -e^{-\frac{1}{3}i\pi t}$<br>$i_2 \quad e^{-\frac{1}{3}i\pi t - \frac{i\pi}{3}}$<br>$i_3 \quad e^{\frac{i\pi}{3} - \frac{i\pi t}{3}}$                                                                                                                                                       |

$$\begin{aligned}
\mathcal{W}_1^{\text{gapless}} = & \sum_{m=1}^{n_{a_1}} \text{sgn}(v_m^{a_1}) \frac{1 - \text{sgn}(\delta_m^{a_1})}{2} + \sum_{m=1}^{n_{a_2}} \text{sgn}(v_m^{a_2}) \frac{1 - \text{sgn}(\delta_m^{a_2})}{2} - 2 \sum_{m=1}^{n_{e_1}} \text{sgn}(v_m^{e_1}) \frac{1 - \text{sgn}(\delta_m^{e_1})}{2} \\
& - 2 \sum_{m=1}^{n_{f_1}} \text{sgn}(v_m^{f_1}) \frac{1 - \text{sgn}(\delta_m^{f_1})}{2} - \sum_{m=1}^{n_{g_1}} \text{sgn}(v_m^{g_1}) \frac{1 - \text{sgn}(\delta_m^{g_1})}{2} - \sum_{m=1}^{n_{g_2}} \text{sgn}(v_m^{g_2}) \frac{1 - \text{sgn}(\delta_m^{g_2})}{2} \\
& - \sum_{m=1}^{n_{g_3}} \text{sgn}(v_m^{g_3}) \frac{1 - \text{sgn}(\delta_m^{g_3})}{2} - \sum_{m=1}^{n_{g_4}} \text{sgn}(v_m^{g_4}) \frac{1 - \text{sgn}(\delta_m^{g_4})}{2} - \sum_{m=1}^{n_{g_5}} \text{sgn}(v_m^{g_5}) \frac{1 - \text{sgn}(\delta_m^{g_5})}{2} \\
& - \sum_{m=1}^{n_{g_6}} \text{sgn}(v_m^{g_6}) \frac{1 - \text{sgn}(\delta_m^{g_6})}{2} + \sum_{m=1}^{n_{i_1}} \text{sgn}(v_m^{i_1}) \frac{1 - \text{sgn}(\delta_m^{i_1})}{2} + \sum_{m=1}^{n_{i_2}} \text{sgn}(v_m^{i_2}) \frac{1 - \text{sgn}(\delta_m^{i_2})}{2} + \sum_{m=1}^{n_{i_3}} \text{sgn}(v_m^{i_3}) \frac{1 - \text{sgn}(\delta_m^{i_3})}{2}
\end{aligned} \tag{S178.1}$$

$$\begin{aligned}
\mathcal{W}_2^{\text{gapless}} = & \sum_{m=1}^{n_{b_1}} \text{sgn}(v_m^{b_1}) \frac{1 - \text{sgn}(\delta_m^{b_1})}{2} + \sum_{m=1}^{n_{b_2}} \text{sgn}(v_m^{b_2}) \frac{1 - \text{sgn}(\delta_m^{b_2})}{2} - 2 \sum_{m=1}^{n_{e_1}} \text{sgn}(v_m^{e_1}) \frac{1 - \text{sgn}(\delta_m^{e_1})}{2} \\
& - \sum_{m=1}^{n_{g_1}} \text{sgn}(v_m^{g_1}) \frac{1 - \text{sgn}(\delta_m^{g_1})}{2} - \sum_{m=1}^{n_{g_2}} \text{sgn}(v_m^{g_2}) \frac{1 - \text{sgn}(\delta_m^{g_2})}{2} - \sum_{m=1}^{n_{g_3}} \text{sgn}(v_m^{g_3}) \frac{1 - \text{sgn}(\delta_m^{g_3})}{2} \\
& - \sum_{m=1}^{n_{g_4}} \text{sgn}(v_m^{g_4}) \frac{1 - \text{sgn}(\delta_m^{g_4})}{2} - \sum_{m=1}^{n_{g_5}} \text{sgn}(v_m^{g_5}) \frac{1 - \text{sgn}(\delta_m^{g_5})}{2} - \sum_{m=1}^{n_{g_6}} \text{sgn}(v_m^{g_6}) \frac{1 - \text{sgn}(\delta_m^{g_6})}{2} \\
& + \sum_{m=1}^{n_{h_1}} \text{sgn}(v_m^{h_1}) \frac{1 - \text{sgn}(\delta_m^{h_1})}{2} + \sum_{m=1}^{n_{h_2}} \text{sgn}(v_m^{h_2}) \frac{1 - \text{sgn}(\delta_m^{h_2})}{2}
\end{aligned} \tag{S178.2}$$

$$\begin{aligned} \mathcal{W}_3^{\text{gapless}} = & \sum_{m=1}^{n_{c_1}} \text{sgn}(v_m^{c_1}) \frac{1 - \text{sgn}(\delta_m^{c_1})}{2} + \sum_{m=1}^{n_{c_2}} \text{sgn}(v_m^{c_2}) \frac{1 - \text{sgn}(\delta_m^{c_2})}{2} - 2 \sum_{m=1}^{n_{f_1}} \text{sgn}(v_m^{f_1}) \frac{1 - \text{sgn}(\delta_m^{f_1})}{2} - \sum_{m=1}^{n_{h_1}} \text{sgn}(v_m^{h_1}) \frac{1 - \text{sgn}(\delta_m^{h_1})}{2} \\ & - \sum_{m=1}^{n_{h_2}} \text{sgn}(v_m^{h_2}) \frac{1 - \text{sgn}(\delta_m^{h_2})}{2} + \sum_{m=1}^{n_{i_1}} \text{sgn}(v_m^{i_1}) \frac{1 - \text{sgn}(\delta_m^{i_1})}{2} + \sum_{m=1}^{n_{i_2}} \text{sgn}(v_m^{i_2}) \frac{1 - \text{sgn}(\delta_m^{i_2})}{2} + \sum_{m=1}^{n_{i_3}} \text{sgn}(v_m^{i_3}) \frac{1 - \text{sgn}(\delta_m^{i_3})}{2} \end{aligned} \quad (\text{S178.3})$$

$$\mathcal{W}_4^{\text{gapless}} = \sum_{m=1}^{n_{d_1}} \text{sgn}(v_m^{d_1}) \frac{1 - \text{sgn}(\delta_m^{d_1})}{2} - \sum_{m=1}^{n_{e_1}} \text{sgn}(v_m^{e_1}) \frac{1 - \text{sgn}(\delta_m^{e_1})}{2} - \sum_{m=1}^{n_{f_1}} \text{sgn}(v_m^{f_1}) \frac{1 - \text{sgn}(\delta_m^{f_1})}{2} \quad (\text{S178.4})$$

$$\begin{aligned} \mathcal{W}_1^{\text{gapped}} = & 2 \sum_{m=1}^{n_{b_2}} \text{sgn}(v_m^{b_2}) \frac{1 - \text{sgn}(\delta_m^{b_2})}{2} - 2 \sum_{m=1}^{n_{e_1}} \text{sgn}(v_m^{e_1}) \frac{1 - \text{sgn}(\delta_m^{e_1})}{2} - \sum_{m=1}^{n_{g_1}} \text{sgn}(v_m^{g_1}) \frac{1 - \text{sgn}(\delta_m^{g_1})}{2} \\ & - \sum_{m=1}^{n_{g_2}} \text{sgn}(v_m^{g_2}) \frac{1 - \text{sgn}(\delta_m^{g_2})}{2} - \sum_{m=1}^{n_{g_3}} \text{sgn}(v_m^{g_3}) \frac{1 - \text{sgn}(\delta_m^{g_3})}{2} - \sum_{m=1}^{n_{g_4}} \text{sgn}(v_m^{g_4}) \frac{1 - \text{sgn}(\delta_m^{g_4})}{2} \\ & - \sum_{m=1}^{n_{g_5}} \text{sgn}(v_m^{g_5}) \frac{1 - \text{sgn}(\delta_m^{g_5})}{2} - \sum_{m=1}^{n_{g_6}} \text{sgn}(v_m^{g_6}) \frac{1 - \text{sgn}(\delta_m^{g_6})}{2} + \sum_{m=1}^{n_{h_1}} \text{sgn}(v_m^{h_1}) \frac{1 - \text{sgn}(\delta_m^{h_1})}{2} \\ & + \sum_{m=1}^{n_{h_2}} \text{sgn}(v_m^{h_2}) \frac{1 - \text{sgn}(\delta_m^{h_2})}{2} \end{aligned} \quad (\text{S178.5})$$

$$\begin{aligned} \mathcal{W}_2^{\text{gapped}} = & \sum_{m=1}^{n_{a_2}} \text{sgn}(v_m^{a_2}) \frac{1 - \text{sgn}(\delta_m^{a_2})}{2} + \sum_{m=1}^{n_{b_2}} \text{sgn}(v_m^{b_2}) \frac{1 - \text{sgn}(\delta_m^{b_2})}{2} + \sum_{m=1}^{n_{c_2}} \text{sgn}(v_m^{c_2}) \frac{1 - \text{sgn}(\delta_m^{c_2})}{2} - 2 \sum_{m=1}^{n_{e_1}} \text{sgn}(v_m^{e_1}) \frac{1 - \text{sgn}(\delta_m^{e_1})}{2} \\ & - 2 \sum_{m=1}^{n_{f_1}} \text{sgn}(v_m^{f_1}) \frac{1 - \text{sgn}(\delta_m^{f_1})}{2} - \sum_{m=1}^{n_{g_1}} \text{sgn}(v_m^{g_1}) \frac{1 - \text{sgn}(\delta_m^{g_1})}{2} - \sum_{m=1}^{n_{g_2}} \text{sgn}(v_m^{g_2}) \frac{1 - \text{sgn}(\delta_m^{g_2})}{2} \\ & - \sum_{m=1}^{n_{g_3}} \text{sgn}(v_m^{g_3}) \frac{1 - \text{sgn}(\delta_m^{g_3})}{2} - \sum_{m=1}^{n_{g_4}} \text{sgn}(v_m^{g_4}) \frac{1 - \text{sgn}(\delta_m^{g_4})}{2} - \sum_{m=1}^{n_{g_5}} \text{sgn}(v_m^{g_5}) \frac{1 - \text{sgn}(\delta_m^{g_5})}{2} \\ & - \sum_{m=1}^{n_{g_6}} \text{sgn}(v_m^{g_6}) \frac{1 - \text{sgn}(\delta_m^{g_6})}{2} + \sum_{m=1}^{n_{i_1}} \text{sgn}(v_m^{i_1}) \frac{1 - \text{sgn}(\delta_m^{i_1})}{2} + \sum_{m=1}^{n_{i_2}} \text{sgn}(v_m^{i_2}) \frac{1 - \text{sgn}(\delta_m^{i_2})}{2} + \sum_{m=1}^{n_{i_3}} \text{sgn}(v_m^{i_3}) \frac{1 - \text{sgn}(\delta_m^{i_3})}{2} \end{aligned} \quad (\text{S178.6})$$

$$\mathcal{X}_1 = \sum_{m=1}^{n_{b_2}} \frac{1 - \text{sgn}(\delta_m^{b_2})}{2} + \sum_{m=1}^{n_{g_2}} \frac{1 - \text{sgn}(\delta_m^{g_2})}{2} + \sum_{m=1}^{n_{g_3}} \frac{1 - \text{sgn}(\delta_m^{g_3})}{2} + \sum_{m=1}^{n_{g_6}} \frac{1 - \text{sgn}(\delta_m^{g_6})}{2} + \sum_{m=1}^{n_{h_1}} \frac{1 - \text{sgn}(\delta_m^{h_1})}{2} \quad \text{mod } 6 \quad (\text{S178.7})$$

$$\begin{aligned} \mathcal{X}_2 = & 4 \sum_{m=1}^{n_{a_2}} \text{sgn}(v_m^{a_2}) \frac{1 - \text{sgn}(\delta_m^{a_2})}{2} + 4 \sum_{m=1}^{n_{b_2}} \text{sgn}(v_m^{b_2}) \frac{1 - \text{sgn}(\delta_m^{b_2})}{2} + 4 \sum_{m=1}^{n_{c_2}} \text{sgn}(v_m^{c_2}) \frac{1 - \text{sgn}(\delta_m^{c_2})}{2} \\ & - 3 \sum_{m=1}^{n_{g_1}} \text{sgn}(v_m^{g_1}) \frac{1 - \text{sgn}(\delta_m^{g_1})}{2} - 5 \sum_{m=1}^{n_{g_2}} \text{sgn}(v_m^{g_2}) \frac{1 - \text{sgn}(\delta_m^{g_2})}{2} - \sum_{m=1}^{n_{g_3}} \text{sgn}(v_m^{g_3}) \frac{1 - \text{sgn}(\delta_m^{g_3})}{2} \\ & - 7 \sum_{m=1}^{n_{g_4}} \text{sgn}(v_m^{g_4}) \frac{1 - \text{sgn}(\delta_m^{g_4})}{2} - 5 \sum_{m=1}^{n_{g_5}} \text{sgn}(v_m^{g_5}) \frac{1 - \text{sgn}(\delta_m^{g_5})}{2} - 3 \sum_{m=1}^{n_{g_6}} \text{sgn}(v_m^{g_6}) \frac{1 - \text{sgn}(\delta_m^{g_6})}{2} \\ & + 4 \sum_{m=1}^{n_{i_1}} \text{sgn}(v_m^{i_1}) \frac{1 - \text{sgn}(\delta_m^{i_1})}{2} + 8 \sum_{m=1}^{n_{i_2}} \text{sgn}(v_m^{i_2}) \frac{1 - \text{sgn}(\delta_m^{i_2})}{2} \quad \text{mod } 6 \end{aligned} \quad (\text{S178.8})$$

## S179. SPACE GROUP NO. 179

| line segment                                        | character of irrep (generators only)                                                                                                                                                                                                                                                                                                           |
|-----------------------------------------------------|------------------------------------------------------------------------------------------------------------------------------------------------------------------------------------------------------------------------------------------------------------------------------------------------------------------------------------------------|
| $a \quad (\frac{t}{3}, \frac{t}{3}, 0)$             | $\{2_{110}   0 \ 0 \ \frac{2}{3}\}$<br>$a_1 \quad -i$<br>$a_2 \quad i$                                                                                                                                                                                                                                                                         |
| $b \quad (0, \frac{t}{2}, 0)$                       | $\{2_{010}   0 \ 0 \ \frac{1}{2}\}$<br>$b_1 \quad -i$<br>$b_2 \quad i$                                                                                                                                                                                                                                                                         |
| $c \quad (\frac{t}{3}, \frac{3-t}{6}, 0)$           | $\{2_{100}   0 \ 0 \ 0\}$<br>$c_1 \quad -i$<br>$c_2 \quad i$                                                                                                                                                                                                                                                                                   |
| $d \quad (\frac{t}{3}, \frac{t}{3}, \frac{1}{2})$   | $\{2_{110}   0 \ 0 \ \frac{2}{3}\}$<br>$d_1 \quad i$<br>$d_2 \quad -i$                                                                                                                                                                                                                                                                         |
| $e \quad (0, \frac{t}{2}, \frac{1}{2})$             | $\{2_{010}   0 \ 0 \ \frac{1}{2}\}$<br>$e_1 \quad i$<br>$e_2 \quad -i$                                                                                                                                                                                                                                                                         |
| $f \quad (\frac{t}{3}, \frac{3-t}{6}, \frac{1}{2})$ | $\{2_{100}   0 \ 0 \ 0\}$<br>$f_1 \quad -i$<br>$f_2 \quad i$                                                                                                                                                                                                                                                                                   |
| $g \quad (0, 0, \frac{t}{2})$                       | $\{6_{001}   0 \ 0 \ \frac{5}{6}\}$<br>$g_1 \quad e^{-\frac{5}{6}i\pi t - \frac{5i\pi}{6}}$<br>$g_2 \quad e^{\frac{5i\pi}{6} - \frac{5i\pi t}{6}}$<br>$g_3 \quad -ie^{-\frac{5}{6}i\pi t}$<br>$g_4 \quad ie^{-\frac{5}{6}i\pi t}$<br>$g_5 \quad e^{-\frac{5}{6}i\pi t - \frac{i\pi}{6}}$<br>$g_6 \quad e^{\frac{i\pi}{6} - \frac{5i\pi t}{6}}$ |
| $h \quad (0, \frac{1}{2}, \frac{t}{2})$             | $\{2_{001}   0 \ 0 \ \frac{1}{2}\}$<br>$h_1 \quad -ie^{-\frac{1}{2}i\pi t}$<br>$h_2 \quad ie^{-\frac{1}{2}i\pi t}$                                                                                                                                                                                                                             |
| $i \quad (\frac{1}{3}, \frac{1}{3}, \frac{t}{2})$   | $\{3_{001}   0 \ 0 \ \frac{2}{3}\}$<br>$i_1 \quad -e^{-\frac{2}{3}i\pi t}$<br>$i_2 \quad e^{-\frac{2}{3}i\pi t - \frac{i\pi}{3}}$<br>$i_3 \quad e^{\frac{i\pi}{3} - \frac{2i\pi t}{3}}$                                                                                                                                                        |

$$\begin{aligned}
\mathcal{W}_1^{\text{gapless}} = & \sum_{m=1}^{n_{a_1}} \text{sgn}(v_m^{a_1}) \frac{1 - \text{sgn}(\delta_m^{a_1})}{2} + \sum_{m=1}^{n_{a_2}} \text{sgn}(v_m^{a_2}) \frac{1 - \text{sgn}(\delta_m^{a_2})}{2} - 2 \sum_{m=1}^{n_{e_1}} \text{sgn}(v_m^{e_1}) \frac{1 - \text{sgn}(\delta_m^{e_1})}{2} \\
& - 2 \sum_{m=1}^{n_{f_1}} \text{sgn}(v_m^{f_1}) \frac{1 - \text{sgn}(\delta_m^{f_1})}{2} - \sum_{m=1}^{n_{g_1}} \text{sgn}(v_m^{g_1}) \frac{1 - \text{sgn}(\delta_m^{g_1})}{2} - \sum_{m=1}^{n_{g_2}} \text{sgn}(v_m^{g_2}) \frac{1 - \text{sgn}(\delta_m^{g_2})}{2} \\
& - \sum_{m=1}^{n_{g_3}} \text{sgn}(v_m^{g_3}) \frac{1 - \text{sgn}(\delta_m^{g_3})}{2} - \sum_{m=1}^{n_{g_4}} \text{sgn}(v_m^{g_4}) \frac{1 - \text{sgn}(\delta_m^{g_4})}{2} - \sum_{m=1}^{n_{g_5}} \text{sgn}(v_m^{g_5}) \frac{1 - \text{sgn}(\delta_m^{g_5})}{2} \\
& - \sum_{m=1}^{n_{g_6}} \text{sgn}(v_m^{g_6}) \frac{1 - \text{sgn}(\delta_m^{g_6})}{2} + \sum_{m=1}^{n_{i_1}} \text{sgn}(v_m^{i_1}) \frac{1 - \text{sgn}(\delta_m^{i_1})}{2} + \sum_{m=1}^{n_{i_2}} \text{sgn}(v_m^{i_2}) \frac{1 - \text{sgn}(\delta_m^{i_2})}{2} + \sum_{m=1}^{n_{i_3}} \text{sgn}(v_m^{i_3}) \frac{1 - \text{sgn}(\delta_m^{i_3})}{2}
\end{aligned}$$

(S179.1)

$$\begin{aligned}
\mathcal{W}_2^{\text{gapless}} = & \sum_{m=1}^{n_{b_1}} \text{sgn}(v_m^{b_1}) \frac{1 - \text{sgn}(\delta_m^{b_1})}{2} + \sum_{m=1}^{n_{b_2}} \text{sgn}(v_m^{b_2}) \frac{1 - \text{sgn}(\delta_m^{b_2})}{2} - 2 \sum_{m=1}^{n_{e_1}} \text{sgn}(v_m^{e_1}) \frac{1 - \text{sgn}(\delta_m^{e_1})}{2} \\
& - \sum_{m=1}^{n_{g_1}} \text{sgn}(v_m^{g_1}) \frac{1 - \text{sgn}(\delta_m^{g_1})}{2} - \sum_{m=1}^{n_{g_2}} \text{sgn}(v_m^{g_2}) \frac{1 - \text{sgn}(\delta_m^{g_2})}{2} - \sum_{m=1}^{n_{g_3}} \text{sgn}(v_m^{g_3}) \frac{1 - \text{sgn}(\delta_m^{g_3})}{2} \\
& - \sum_{m=1}^{n_{g_4}} \text{sgn}(v_m^{g_4}) \frac{1 - \text{sgn}(\delta_m^{g_4})}{2} - \sum_{m=1}^{n_{g_5}} \text{sgn}(v_m^{g_5}) \frac{1 - \text{sgn}(\delta_m^{g_5})}{2} - \sum_{m=1}^{n_{g_6}} \text{sgn}(v_m^{g_6}) \frac{1 - \text{sgn}(\delta_m^{g_6})}{2} \\
& + \sum_{m=1}^{n_{h_1}} \text{sgn}(v_m^{h_1}) \frac{1 - \text{sgn}(\delta_m^{h_1})}{2} + \sum_{m=1}^{n_{h_2}} \text{sgn}(v_m^{h_2}) \frac{1 - \text{sgn}(\delta_m^{h_2})}{2}
\end{aligned} \tag{S179.2}$$

$$\begin{aligned}
\mathcal{W}_3^{\text{gapless}} = & \sum_{m=1}^{n_{c_1}} \text{sgn}(v_m^{c_1}) \frac{1 - \text{sgn}(\delta_m^{c_1})}{2} + \sum_{m=1}^{n_{c_2}} \text{sgn}(v_m^{c_2}) \frac{1 - \text{sgn}(\delta_m^{c_2})}{2} - 2 \sum_{m=1}^{n_{f_1}} \text{sgn}(v_m^{f_1}) \frac{1 - \text{sgn}(\delta_m^{f_1})}{2} - \sum_{m=1}^{n_{h_1}} \text{sgn}(v_m^{h_1}) \frac{1 - \text{sgn}(\delta_m^{h_1})}{2} \\
& - \sum_{m=1}^{n_{h_2}} \text{sgn}(v_m^{h_2}) \frac{1 - \text{sgn}(\delta_m^{h_2})}{2} + \sum_{m=1}^{n_{i_1}} \text{sgn}(v_m^{i_1}) \frac{1 - \text{sgn}(\delta_m^{i_1})}{2} + \sum_{m=1}^{n_{i_2}} \text{sgn}(v_m^{i_2}) \frac{1 - \text{sgn}(\delta_m^{i_2})}{2} + \sum_{m=1}^{n_{i_3}} \text{sgn}(v_m^{i_3}) \frac{1 - \text{sgn}(\delta_m^{i_3})}{2}
\end{aligned} \tag{S179.3}$$

$$\mathcal{W}_4^{\text{gapless}} = \sum_{m=1}^{n_{d_1}} \text{sgn}(v_m^{d_1}) \frac{1 - \text{sgn}(\delta_m^{d_1})}{2} - \sum_{m=1}^{n_{e_1}} \text{sgn}(v_m^{e_1}) \frac{1 - \text{sgn}(\delta_m^{e_1})}{2} - \sum_{m=1}^{n_{f_1}} \text{sgn}(v_m^{f_1}) \frac{1 - \text{sgn}(\delta_m^{f_1})}{2} \tag{S179.4}$$

$$\begin{aligned}
\mathcal{W}_1^{\text{gapped}} = & 2 \sum_{m=1}^{n_{b_2}} \text{sgn}(v_m^{b_2}) \frac{1 - \text{sgn}(\delta_m^{b_2})}{2} - 2 \sum_{m=1}^{n_{e_1}} \text{sgn}(v_m^{e_1}) \frac{1 - \text{sgn}(\delta_m^{e_1})}{2} - \sum_{m=1}^{n_{g_1}} \text{sgn}(v_m^{g_1}) \frac{1 - \text{sgn}(\delta_m^{g_1})}{2} \\
& - \sum_{m=1}^{n_{g_2}} \text{sgn}(v_m^{g_2}) \frac{1 - \text{sgn}(\delta_m^{g_2})}{2} - \sum_{m=1}^{n_{g_3}} \text{sgn}(v_m^{g_3}) \frac{1 - \text{sgn}(\delta_m^{g_3})}{2} - \sum_{m=1}^{n_{g_4}} \text{sgn}(v_m^{g_4}) \frac{1 - \text{sgn}(\delta_m^{g_4})}{2} \\
& - \sum_{m=1}^{n_{g_5}} \text{sgn}(v_m^{g_5}) \frac{1 - \text{sgn}(\delta_m^{g_5})}{2} - \sum_{m=1}^{n_{g_6}} \text{sgn}(v_m^{g_6}) \frac{1 - \text{sgn}(\delta_m^{g_6})}{2} + \sum_{m=1}^{n_{h_1}} \text{sgn}(v_m^{h_1}) \frac{1 - \text{sgn}(\delta_m^{h_1})}{2} \\
& + \sum_{m=1}^{n_{h_2}} \text{sgn}(v_m^{h_2}) \frac{1 - \text{sgn}(\delta_m^{h_2})}{2}
\end{aligned} \tag{S179.5}$$

$$\begin{aligned}
\mathcal{W}_2^{\text{gapped}} = & \sum_{m=1}^{n_{a_2}} \text{sgn}(v_m^{a_2}) \frac{1 - \text{sgn}(\delta_m^{a_2})}{2} + \sum_{m=1}^{n_{b_2}} \text{sgn}(v_m^{b_2}) \frac{1 - \text{sgn}(\delta_m^{b_2})}{2} + \sum_{m=1}^{n_{c_2}} \text{sgn}(v_m^{c_2}) \frac{1 - \text{sgn}(\delta_m^{c_2})}{2} - 2 \sum_{m=1}^{n_{e_1}} \text{sgn}(v_m^{e_1}) \frac{1 - \text{sgn}(\delta_m^{e_1})}{2} \\
& - 2 \sum_{m=1}^{n_{f_1}} \text{sgn}(v_m^{f_1}) \frac{1 - \text{sgn}(\delta_m^{f_1})}{2} - \sum_{m=1}^{n_{g_1}} \text{sgn}(v_m^{g_1}) \frac{1 - \text{sgn}(\delta_m^{g_1})}{2} - \sum_{m=1}^{n_{g_2}} \text{sgn}(v_m^{g_2}) \frac{1 - \text{sgn}(\delta_m^{g_2})}{2} \\
& - \sum_{m=1}^{n_{g_3}} \text{sgn}(v_m^{g_3}) \frac{1 - \text{sgn}(\delta_m^{g_3})}{2} - \sum_{m=1}^{n_{g_4}} \text{sgn}(v_m^{g_4}) \frac{1 - \text{sgn}(\delta_m^{g_4})}{2} - \sum_{m=1}^{n_{g_5}} \text{sgn}(v_m^{g_5}) \frac{1 - \text{sgn}(\delta_m^{g_5})}{2} \\
& - \sum_{m=1}^{n_{g_6}} \text{sgn}(v_m^{g_6}) \frac{1 - \text{sgn}(\delta_m^{g_6})}{2} + \sum_{m=1}^{n_{i_1}} \text{sgn}(v_m^{i_1}) \frac{1 - \text{sgn}(\delta_m^{i_1})}{2} + \sum_{m=1}^{n_{i_2}} \text{sgn}(v_m^{i_2}) \frac{1 - \text{sgn}(\delta_m^{i_2})}{2} + \sum_{m=1}^{n_{i_3}} \text{sgn}(v_m^{i_3}) \frac{1 - \text{sgn}(\delta_m^{i_3})}{2}
\end{aligned} \tag{S179.6}$$

$$\mathcal{X}_1 = \sum_{m=1}^{n_{b_2}} \frac{1 - \text{sgn}(\delta_m^{b_2})}{2} + \sum_{m=1}^{n_{g_1}} \frac{1 - \text{sgn}(\delta_m^{g_1})}{2} + \sum_{m=1}^{n_{g_4}} \frac{1 - \text{sgn}(\delta_m^{g_4})}{2} + \sum_{m=1}^{n_{g_5}} \frac{1 - \text{sgn}(\delta_m^{g_5})}{2} + \sum_{m=1}^{n_{h_1}} \frac{1 - \text{sgn}(\delta_m^{h_1})}{2} \mod (\S 179.7)$$

$$\begin{aligned} \mathcal{X}_2 = & -4 \sum_{m=1}^{n_{a_2}} \text{sgn}(v_m^{a_2}) \frac{1 - \text{sgn}(\delta_m^{a_2})}{2} - 4 \sum_{m=1}^{n_{b_2}} \text{sgn}(v_m^{b_2}) \frac{1 - \text{sgn}(\delta_m^{b_2})}{2} - 4 \sum_{m=1}^{n_{c_2}} \text{sgn}(v_m^{c_2}) \frac{1 - \text{sgn}(\delta_m^{c_2})}{2} \\ & + 10 \sum_{m=1}^{n_{e_1}} \text{sgn}(v_m^{e_1}) \frac{1 - \text{sgn}(\delta_m^{e_1})}{2} + 10 \sum_{m=1}^{n_{f_1}} \text{sgn}(v_m^{f_1}) \frac{1 - \text{sgn}(\delta_m^{f_1})}{2} + 3 \sum_{m=1}^{n_{g_1}} \text{sgn}(v_m^{g_1}) \frac{1 - \text{sgn}(\delta_m^{g_1})}{2} \\ & + 5 \sum_{m=1}^{n_{g_2}} \text{sgn}(v_m^{g_2}) \frac{1 - \text{sgn}(\delta_m^{g_2})}{2} + \sum_{m=1}^{n_{g_3}} \text{sgn}(v_m^{g_3}) \frac{1 - \text{sgn}(\delta_m^{g_3})}{2} + 7 \sum_{m=1}^{n_{g_4}} \text{sgn}(v_m^{g_4}) \frac{1 - \text{sgn}(\delta_m^{g_4})}{2} \\ & + 5 \sum_{m=1}^{n_{g_5}} \text{sgn}(v_m^{g_5}) \frac{1 - \text{sgn}(\delta_m^{g_5})}{2} + 3 \sum_{m=1}^{n_{g_6}} \text{sgn}(v_m^{g_6}) \frac{1 - \text{sgn}(\delta_m^{g_6})}{2} - 4 \sum_{m=1}^{n_{i_1}} \text{sgn}(v_m^{i_1}) \frac{1 - \text{sgn}(\delta_m^{i_1})}{2} \\ & - 8 \sum_{m=1}^{n_{i_2}} \text{sgn}(v_m^{i_2}) \frac{1 - \text{sgn}(\delta_m^{i_2})}{2} \mod 6 \end{aligned} \quad (\text{S179.8})$$

### S180. SPACE GROUP NO. 180

| line segment                                               | character of irrep (generators only)                                                                                                                                                                                                                                                                                                         |
|------------------------------------------------------------|----------------------------------------------------------------------------------------------------------------------------------------------------------------------------------------------------------------------------------------------------------------------------------------------------------------------------------------------|
| $a \left( \frac{t}{3}, \frac{t}{3}, 0 \right)$             | $\{2_{110}   0 \ 0 \ \frac{2}{3}\}$<br>$a_1 \quad -i$<br>$a_2 \quad i$                                                                                                                                                                                                                                                                       |
| $b \left( 0, \frac{t}{2}, 0 \right)$                       | $\{2_{010}   0 \ 0 \ 0\}$<br>$b_1 \quad -i$<br>$b_2 \quad i$                                                                                                                                                                                                                                                                                 |
| $c \left( \frac{t}{3}, \frac{3-t}{6}, 0 \right)$           | $\{2_{100}   0 \ 0 \ 0\}$<br>$c_1 \quad -i$<br>$c_2 \quad i$                                                                                                                                                                                                                                                                                 |
| $d \left( \frac{t}{3}, \frac{t}{3}, \frac{1}{2} \right)$   | $\{2_{110}   0 \ 0 \ \frac{2}{3}\}$<br>$d_1 \quad i$<br>$d_2 \quad -i$                                                                                                                                                                                                                                                                       |
| $e \left( 0, \frac{t}{2}, \frac{1}{2} \right)$             | $\{2_{010}   0 \ 0 \ 0\}$<br>$e_1 \quad -i$<br>$e_2 \quad i$                                                                                                                                                                                                                                                                                 |
| $f \left( \frac{t}{3}, \frac{3-t}{6}, \frac{1}{2} \right)$ | $\{2_{100}   0 \ 0 \ 0\}$<br>$f_1 \quad -i$<br>$f_2 \quad i$                                                                                                                                                                                                                                                                                 |
| $g \left( 0, 0, \frac{t}{2} \right)$                       | $\{6_{001}   0 \ 0 \ \frac{1}{3}\}$<br>$g_1 \quad e^{-\frac{1}{3}i\pi t - \frac{5i\pi}{6}}$<br>$g_2 \quad e^{\frac{5i\pi}{6} - \frac{i\pi t}{3}}$<br>$g_3 \quad -ie^{-\frac{1}{3}i\pi t}$<br>$g_4 \quad ie^{-\frac{1}{3}i\pi t}$<br>$g_5 \quad e^{-\frac{1}{3}i\pi t - \frac{i\pi}{6}}$<br>$g_6 \quad e^{\frac{i\pi}{6} - \frac{i\pi t}{3}}$ |
| $h \left( 0, \frac{1}{2}, \frac{t}{2} \right)$             | $\{2_{001}   0 \ 0 \ 0\}$<br>$h_1 \quad -i$<br>$h_2 \quad i$                                                                                                                                                                                                                                                                                 |
| $i \left( \frac{1}{3}, \frac{1}{3}, \frac{t}{2} \right)$   | $\{3_{001}   0 \ 0 \ \frac{2}{3}\}$<br>$i_1 \quad -e^{-\frac{2}{3}i\pi t}$<br>$i_2 \quad e^{-\frac{2}{3}i\pi t - \frac{i\pi}{3}}$<br>$i_3 \quad e^{\frac{i\pi}{3} - \frac{2i\pi t}{3}}$                                                                                                                                                      |



$$\begin{aligned} \mathcal{W}_1^{\text{gapless}} = & \sum_{m=1}^{n_{a1}} \text{sgn}(v_m^{a1}) \frac{1 - \text{sgn}(\delta_m^{a1})}{2} + \sum_{m=1}^{n_{a2}} \text{sgn}(v_m^{a2}) \frac{1 - \text{sgn}(\delta_m^{a2})}{2} - \sum_{m=1}^{n_{e1}} \text{sgn}(v_m^{e1}) \frac{1 - \text{sgn}(\delta_m^{e1})}{2} \\ & - \sum_{m=1}^{n_{e2}} \text{sgn}(v_m^{e2}) \frac{1 - \text{sgn}(\delta_m^{e2})}{2} - \sum_{m=1}^{n_{f1}} \text{sgn}(v_m^{f1}) \frac{1 - \text{sgn}(\delta_m^{f1})}{2} - \sum_{m=1}^{n_{f2}} \text{sgn}(v_m^{f2}) \frac{1 - \text{sgn}(\delta_m^{f2})}{2} \\ & - \sum_{m=1}^{n_{g1}} \text{sgn}(v_m^{g1}) \frac{1 - \text{sgn}(\delta_m^{g1})}{2} - \sum_{m=1}^{n_{g2}} \text{sgn}(v_m^{g2}) \frac{1 - \text{sgn}(\delta_m^{g2})}{2} - \sum_{m=1}^{n_{g3}} \text{sgn}(v_m^{g3}) \frac{1 - \text{sgn}(\delta_m^{g3})}{2} \\ & - \sum_{m=1}^{n_{g4}} \text{sgn}(v_m^{g4}) \frac{1 - \text{sgn}(\delta_m^{g4})}{2} - \sum_{m=1}^{n_{g5}} \text{sgn}(v_m^{g5}) \frac{1 - \text{sgn}(\delta_m^{g5})}{2} - \sum_{m=1}^{n_{g6}} \text{sgn}(v_m^{g6}) \frac{1 - \text{sgn}(\delta_m^{g6})}{2} \\ & + \sum_{m=1}^{n_{i1}} \text{sgn}(v_m^{i1}) \frac{1 - \text{sgn}(\delta_m^{i1})}{2} + \sum_{m=1}^{n_{i2}} \text{sgn}(v_m^{i2}) \frac{1 - \text{sgn}(\delta_m^{i2})}{2} + \sum_{m=1}^{n_{i3}} \text{sgn}(v_m^{i3}) \frac{1 - \text{sgn}(\delta_m^{i3})}{2} \end{aligned} \quad (\text{S180.1})$$
$$\begin{aligned} \mathcal{W}_2^{\text{gapless}} = & \sum_{m=1}^{n_{b_1}} \text{sgn}(v_m^{b_1}) \frac{1 - \text{sgn}(\delta_m^{b_1})}{2} + \sum_{m=1}^{n_{b_2}} \text{sgn}(v_m^{b_2}) \frac{1 - \text{sgn}(\delta_m^{b_2})}{2} - \sum_{m=1}^{n_{e_1}} \text{sgn}(v_m^{e_1}) \frac{1 - \text{sgn}(\delta_m^{e_1})}{2} \\ & - \sum_{m=1}^{n_{e_2}} \text{sgn}(v_m^{e_2}) \frac{1 - \text{sgn}(\delta_m^{e_2})}{2} - \sum_{m=1}^{n_{g_1}} \text{sgn}(v_m^{g_1}) \frac{1 - \text{sgn}(\delta_m^{g_1})}{2} - \sum_{m=1}^{n_{g_2}} \text{sgn}(v_m^{g_2}) \frac{1 - \text{sgn}(\delta_m^{g_2})}{2} \\ & - \sum_{m=1}^{n_{g_3}} \text{sgn}(v_m^{g_3}) \frac{1 - \text{sgn}(\delta_m^{g_3})}{2} - \sum_{m=1}^{n_{g_4}} \text{sgn}(v_m^{g_4}) \frac{1 - \text{sgn}(\delta_m^{g_4})}{2} - \sum_{m=1}^{n_{g_5}} \text{sgn}(v_m^{g_5}) \frac{1 - \text{sgn}(\delta_m^{g_5})}{2} \\ & - \sum_{m=1}^{n_{g_6}} \text{sgn}(v_m^{g_6}) \frac{1 - \text{sgn}(\delta_m^{g_6})}{2} + \sum_{m=1}^{n_{h_1}} \text{sgn}(v_m^{h_1}) \frac{1 - \text{sgn}(\delta_m^{h_1})}{2} + \sum_{m=1}^{n_{h_2}} \text{sgn}(v_m^{h_2}) \frac{1 - \text{sgn}(\delta_m^{h_2})}{2} \end{aligned} \quad (\text{S180.2})$$
$$\begin{aligned} \mathcal{W}_3^{\text{gapless}} = & \sum_{m=1}^{n_{c_1}} \text{sgn}(v_m^{c_1}) \frac{1 - \text{sgn}(\delta_m^{c_1})}{2} + \sum_{m=1}^{n_{c_2}} \text{sgn}(v_m^{c_2}) \frac{1 - \text{sgn}(\delta_m^{c_2})}{2} - \sum_{m=1}^{n_{f_1}} \text{sgn}(v_m^{f_1}) \frac{1 - \text{sgn}(\delta_m^{f_1})}{2} \\ & - \sum_{m=1}^{n_{f_2}} \text{sgn}(v_m^{f_2}) \frac{1 - \text{sgn}(\delta_m^{f_2})}{2} - \sum_{m=1}^{n_{h_1}} \text{sgn}(v_m^{h_1}) \frac{1 - \text{sgn}(\delta_m^{h_1})}{2} - \sum_{m=1}^{n_{h_2}} \text{sgn}(v_m^{h_2}) \frac{1 - \text{sgn}(\delta_m^{h_2})}{2} \\ & + \sum_{m=1}^{n_{i_1}} \text{sgn}(v_m^{i_1}) \frac{1 - \text{sgn}(\delta_m^{i_1})}{2} + \sum_{m=1}^{n_{i_2}} \text{sgn}(v_m^{i_2}) \frac{1 - \text{sgn}(\delta_m^{i_2})}{2} + \sum_{m=1}^{n_{i_3}} \text{sgn}(v_m^{i_3}) \frac{1 - \text{sgn}(\delta_m^{i_3})}{2} \end{aligned} \quad (\text{S180.3})$$
$$\mathcal{W}_4^{\text{gapless}} = \sum_{m=1}^{n_{d_1}} \text{sgn}(v_m^{d_1}) \frac{1 - \text{sgn}(\delta_m^{d_1})}{2} + \sum_{m=1}^{n_{d_2}} \text{sgn}(v_m^{d_2}) \frac{1 - \text{sgn}(\delta_m^{d_2})}{2} - \sum_{m=1}^{n_{e_1}} \text{sgn}(v_m^{e_1}) \frac{1 - \text{sgn}(\delta_m^{e_1})}{2} - \sum_{m=1}^{n_{e_2}} \text{sgn}(v_m^{e_2}) \frac{1 - \text{sgn}(\delta_m^{e_2})}{2} - \sum_{m=1}^{n_{f_1}} \text{sgn}(v_m^{f_1}) \frac{1 - \text{sgn}(\delta_m^{f_1})}{2} - \sum_{m=1}^{n_{f_2}} \text{sgn}(v_m^{f_2}) \frac{1 - \text{sgn}(\delta_m^{f_2})}{2} \quad (\text{S180.4})$$
$$\mathcal{W}_1^{\text{gapped}} = - \sum_{m=1}^{n_{g1}} \text{sgn}(v_m^{g1}) \frac{1 - \text{sgn}(\delta_m^{g1})}{2} + \sum_{m=1}^{n_{g2}} \text{sgn}(v_m^{g2}) \frac{1 - \text{sgn}(\delta_m^{g2})}{2} + \sum_{m=1}^{n_{g3}} \text{sgn}(v_m^{g3}) \frac{1 - \text{sgn}(\delta_m^{g3})}{2} - \sum_{m=1}^{n_{g4}} \text{sgn}(v_m^{g4}) \frac{1 - \text{sgn}(\delta_m^{g4})}{2} - \sum_{m=1}^{n_{g5}} \text{sgn}(v_m^{g5}) \frac{1 - \text{sgn}(\delta_m^{g5})}{2} + \sum_{m=1}^{n_{g6}} \text{sgn}(v_m^{g6}) \frac{1 - \text{sgn}(\delta_m^{g6})}{2} \quad (\text{S180.5})$$

$$\begin{aligned} \mathcal{W}_2^{\text{gapped}} = & \sum_{m=1}^{n_{b_2}} \text{sgn}(v_m^{b_2}) \frac{1 - \text{sgn}(\delta_m^{b_2})}{2} - \sum_{m=1}^{n_{e_2}} \text{sgn}(v_m^{e_2}) \frac{1 - \text{sgn}(\delta_m^{e_2})}{2} - \sum_{m=1}^{n_{g_1}} \text{sgn}(v_m^{g_1}) \frac{1 - \text{sgn}(\delta_m^{g_1})}{2} \\ & - \sum_{m=1}^{n_{g_4}} \text{sgn}(v_m^{g_4}) \frac{1 - \text{sgn}(\delta_m^{g_4})}{2} - \sum_{m=1}^{n_{g_5}} \text{sgn}(v_m^{g_5}) \frac{1 - \text{sgn}(\delta_m^{g_5})}{2} + \sum_{m=1}^{n_{h_1}} \text{sgn}(v_m^{h_1}) \frac{1 - \text{sgn}(\delta_m^{h_1})}{2} \end{aligned} \quad (\text{S180.6})$$

$$\mathcal{W}_3^{\text{gapped}} = - \sum_{m=1}^{n_{h_1}} \text{sgn}(v_m^{h_1}) \frac{1 - \text{sgn}(\delta_m^{h_1})}{2} + \sum_{m=1}^{n_{h_2}} \text{sgn}(v_m^{h_2}) \frac{1 - \text{sgn}(\delta_m^{h_2})}{2} \quad (\text{S180.7})$$

$$\mathcal{W}_4^{\text{gapped}} = \sum_{m=1}^{n_{e_1}} \text{sgn}(v_m^{e_1}) \frac{1 - \text{sgn}(\delta_m^{e_1})}{2} - \sum_{m=1}^{n_{e_2}} \text{sgn}(v_m^{e_2}) \frac{1 - \text{sgn}(\delta_m^{e_2})}{2} \quad (\text{S180.8})$$

$$\begin{aligned} \mathcal{W}_5^{\text{gapped}} = & \sum_{m=1}^{n_{a_2}} \text{sgn}(v_m^{a_2}) \frac{1 - \text{sgn}(\delta_m^{a_2})}{2} + \sum_{m=1}^{n_{c_2}} \text{sgn}(v_m^{c_2}) \frac{1 - \text{sgn}(\delta_m^{c_2})}{2} - \sum_{m=1}^{n_{d_2}} \text{sgn}(v_m^{d_2}) \frac{1 - \text{sgn}(\delta_m^{d_2})}{2} - \sum_{m=1}^{n_{f_1}} \text{sgn}(v_m^{f_1}) \frac{1 - \text{sgn}(\delta_m^{f_1})}{2} \\ & - \sum_{m=1}^{n_{g_1}} \text{sgn}(v_m^{g_1}) \frac{1 - \text{sgn}(\delta_m^{g_1})}{2} - \sum_{m=1}^{n_{g_4}} \text{sgn}(v_m^{g_4}) \frac{1 - \text{sgn}(\delta_m^{g_4})}{2} - \sum_{m=1}^{n_{g_5}} \text{sgn}(v_m^{g_5}) \frac{1 - \text{sgn}(\delta_m^{g_5})}{2} \\ & - \sum_{m=1}^{n_{h_1}} \text{sgn}(v_m^{h_1}) \frac{1 - \text{sgn}(\delta_m^{h_1})}{2} + \sum_{m=1}^{n_{i_1}} \text{sgn}(v_m^{i_1}) \frac{1 - \text{sgn}(\delta_m^{i_1})}{2} + \sum_{m=1}^{n_{i_2}} \text{sgn}(v_m^{i_2}) \frac{1 - \text{sgn}(\delta_m^{i_2})}{2} + \sum_{m=1}^{n_{i_3}} \text{sgn}(v_m^{i_3}) \frac{1 - \text{sgn}(\delta_m^{i_3})}{2} \end{aligned} \quad (\text{S180.9})$$

$$\mathcal{W}_6^{\text{gapped}} = - \sum_{m=1}^{n_{d_2}} \text{sgn}(v_m^{d_2}) \frac{1 - \text{sgn}(\delta_m^{d_2})}{2} + \sum_{m=1}^{n_{e_2}} \text{sgn}(v_m^{e_2}) \frac{1 - \text{sgn}(\delta_m^{e_2})}{2} + \sum_{m=1}^{n_{f_2}} \text{sgn}(v_m^{f_2}) \frac{1 - \text{sgn}(\delta_m^{f_2})}{2} \quad (\text{S180.10})$$

$$\begin{aligned} \mathcal{X}_1 = & - \sum_{m=1}^{n_{a_2}} \text{sgn}(v_m^{a_2}) \frac{1 - \text{sgn}(\delta_m^{a_2})}{2} - \sum_{m=1}^{n_{c_2}} \text{sgn}(v_m^{c_2}) \frac{1 - \text{sgn}(\delta_m^{c_2})}{2} - \sum_{m=1}^{n_{e_2}} \text{sgn}(v_m^{e_2}) \frac{1 - \text{sgn}(\delta_m^{e_2})}{2} - 2 \sum_{m=1}^{n_{g_2}} \text{sgn}(v_m^{g_2}) \frac{1 - \text{sgn}(\delta_m^{g_2})}{2} \\ & - 4 \sum_{m=1}^{n_{g_3}} \text{sgn}(v_m^{g_3}) \frac{1 - \text{sgn}(\delta_m^{g_3})}{2} + 5 \sum_{m=1}^{n_{g_4}} \text{sgn}(v_m^{g_4}) \frac{1 - \text{sgn}(\delta_m^{g_4})}{2} + \sum_{m=1}^{n_{g_5}} \text{sgn}(v_m^{g_5}) \frac{1 - \text{sgn}(\delta_m^{g_5})}{2} \\ & + \sum_{m=1}^{n_{h_1}} \text{sgn}(v_m^{h_1}) \frac{1 - \text{sgn}(\delta_m^{h_1})}{2} - \sum_{m=1}^{n_{i_1}} \text{sgn}(v_m^{i_1}) \frac{1 - \text{sgn}(\delta_m^{i_1})}{2} - 2 \sum_{m=1}^{n_{i_3}} \text{sgn}(v_m^{i_3}) \frac{1 - \text{sgn}(\delta_m^{i_3})}{2} \pmod{3} \end{aligned} \quad (\text{S180.11})$$

### S181. SPACE GROUP NO. 181

|              |                                      |
|--------------|--------------------------------------|
| line segment | character of irrep (generators only) |
|--------------|--------------------------------------|

|                                                     |                                                                                                                                                                                                                                                                                                                                                |
|-----------------------------------------------------|------------------------------------------------------------------------------------------------------------------------------------------------------------------------------------------------------------------------------------------------------------------------------------------------------------------------------------------------|
| $a \quad (\frac{t}{3}, \frac{t}{3}, 0)$             | $\{2_{110}   0 \ 0 \ \frac{1}{3}\}$<br>$a_1 \quad -i$<br>$a_2 \quad i$                                                                                                                                                                                                                                                                         |
| $b \quad (0, \frac{t}{2}, 0)$                       | $\{2_{010}   0 \ 0 \ 0\}$<br>$b_1 \quad -i$<br>$b_2 \quad i$                                                                                                                                                                                                                                                                                   |
| $c \quad (\frac{t}{3}, \frac{3-t}{6}, 0)$           | $\{2_{100}   0 \ 0 \ 0\}$<br>$c_1 \quad -i$<br>$c_2 \quad i$                                                                                                                                                                                                                                                                                   |
| $d \quad (\frac{t}{3}, \frac{t}{3}, \frac{1}{2})$   | $\{2_{110}   0 \ 0 \ \frac{1}{3}\}$<br>$d_1 \quad i$<br>$d_2 \quad -i$                                                                                                                                                                                                                                                                         |
| $e \quad (0, \frac{t}{2}, \frac{1}{2})$             | $\{2_{010}   0 \ 0 \ 0\}$<br>$e_1 \quad -i$<br>$e_2 \quad i$                                                                                                                                                                                                                                                                                   |
| $f \quad (\frac{t}{3}, \frac{3-t}{6}, \frac{1}{2})$ | $\{2_{100}   0 \ 0 \ 0\}$<br>$f_1 \quad -i$<br>$f_2 \quad i$                                                                                                                                                                                                                                                                                   |
| $g \quad (0, 0, \frac{t}{2})$                       | $\{6_{001}   0 \ 0 \ \frac{2}{3}\}$<br>$g_1 \quad e^{-\frac{2}{3}i\pi t - \frac{5i\pi}{6}}$<br>$g_2 \quad e^{\frac{5i\pi}{6} - \frac{2i\pi t}{3}}$<br>$g_3 \quad -ie^{-\frac{2}{3}i\pi t}$<br>$g_4 \quad ie^{-\frac{2}{3}i\pi t}$<br>$g_5 \quad e^{-\frac{2}{3}i\pi t - \frac{i\pi}{6}}$<br>$g_6 \quad e^{\frac{i\pi}{6} - \frac{2i\pi t}{3}}$ |
| $h \quad (0, \frac{1}{2}, \frac{t}{2})$             | $\{2_{001}   0 \ 0 \ 0\}$<br>$h_1 \quad -i$<br>$h_2 \quad i$                                                                                                                                                                                                                                                                                   |
| $i \quad (\frac{1}{3}, \frac{1}{3}, \frac{t}{2})$   | $\{3_{001}   0 \ 0 \ \frac{1}{3}\}$<br>$i_1 \quad -e^{-\frac{1}{3}i\pi t}$<br>$i_2 \quad e^{-\frac{1}{3}i\pi t - \frac{i\pi}{3}}$<br>$i_3 \quad e^{\frac{i\pi}{3} - \frac{i\pi t}{3}}$                                                                                                                                                         |

$$\begin{aligned}
\mathcal{W}_1^{\text{gapless}} = & \sum_{m=1}^{n_{a_1}} \text{sgn}(v_m^{a_1}) \frac{1 - \text{sgn}(\delta_m^{a_1})}{2} + \sum_{m=1}^{n_{a_2}} \text{sgn}(v_m^{a_2}) \frac{1 - \text{sgn}(\delta_m^{a_2})}{2} - \sum_{m=1}^{n_{e_1}} \text{sgn}(v_m^{e_1}) \frac{1 - \text{sgn}(\delta_m^{e_1})}{2} \\
& - \sum_{m=1}^{n_{e_2}} \text{sgn}(v_m^{e_2}) \frac{1 - \text{sgn}(\delta_m^{e_2})}{2} - \sum_{m=1}^{n_{f_1}} \text{sgn}(v_m^{f_1}) \frac{1 - \text{sgn}(\delta_m^{f_1})}{2} - \sum_{m=1}^{n_{f_2}} \text{sgn}(v_m^{f_2}) \frac{1 - \text{sgn}(\delta_m^{f_2})}{2} \\
& - \sum_{m=1}^{n_{g_1}} \text{sgn}(v_m^{g_1}) \frac{1 - \text{sgn}(\delta_m^{g_1})}{2} - \sum_{m=1}^{n_{g_2}} \text{sgn}(v_m^{g_2}) \frac{1 - \text{sgn}(\delta_m^{g_2})}{2} - \sum_{m=1}^{n_{g_3}} \text{sgn}(v_m^{g_3}) \frac{1 - \text{sgn}(\delta_m^{g_3})}{2} \\
& - \sum_{m=1}^{n_{g_4}} \text{sgn}(v_m^{g_4}) \frac{1 - \text{sgn}(\delta_m^{g_4})}{2} - \sum_{m=1}^{n_{g_5}} \text{sgn}(v_m^{g_5}) \frac{1 - \text{sgn}(\delta_m^{g_5})}{2} - \sum_{m=1}^{n_{g_6}} \text{sgn}(v_m^{g_6}) \frac{1 - \text{sgn}(\delta_m^{g_6})}{2} \\
& + \sum_{m=1}^{n_{i_1}} \text{sgn}(v_m^{i_1}) \frac{1 - \text{sgn}(\delta_m^{i_1})}{2} + \sum_{m=1}^{n_{i_2}} \text{sgn}(v_m^{i_2}) \frac{1 - \text{sgn}(\delta_m^{i_2})}{2} + \sum_{m=1}^{n_{i_3}} \text{sgn}(v_m^{i_3}) \frac{1 - \text{sgn}(\delta_m^{i_3})}{2}
\end{aligned} \tag{S181.1}$$

$$\begin{aligned}
\mathcal{W}_2^{\text{gapless}} = & \sum_{m=1}^{n_{b_1}} \text{sgn}(v_m^{b_1}) \frac{1 - \text{sgn}(\delta_m^{b_1})}{2} + \sum_{m=1}^{n_{b_2}} \text{sgn}(v_m^{b_2}) \frac{1 - \text{sgn}(\delta_m^{b_2})}{2} - \sum_{m=1}^{n_{e_1}} \text{sgn}(v_m^{e_1}) \frac{1 - \text{sgn}(\delta_m^{e_1})}{2} \\
& - \sum_{m=1}^{n_{e_2}} \text{sgn}(v_m^{e_2}) \frac{1 - \text{sgn}(\delta_m^{e_2})}{2} - \sum_{m=1}^{n_{g_1}} \text{sgn}(v_m^{g_1}) \frac{1 - \text{sgn}(\delta_m^{g_1})}{2} - \sum_{m=1}^{n_{g_2}} \text{sgn}(v_m^{g_2}) \frac{1 - \text{sgn}(\delta_m^{g_2})}{2} \\
& - \sum_{m=1}^{n_{g_3}} \text{sgn}(v_m^{g_3}) \frac{1 - \text{sgn}(\delta_m^{g_3})}{2} - \sum_{m=1}^{n_{g_4}} \text{sgn}(v_m^{g_4}) \frac{1 - \text{sgn}(\delta_m^{g_4})}{2} - \sum_{m=1}^{n_{g_5}} \text{sgn}(v_m^{g_5}) \frac{1 - \text{sgn}(\delta_m^{g_5})}{2} \\
& - \sum_{m=1}^{n_{g_6}} \text{sgn}(v_m^{g_6}) \frac{1 - \text{sgn}(\delta_m^{g_6})}{2} + \sum_{m=1}^{n_{h_1}} \text{sgn}(v_m^{h_1}) \frac{1 - \text{sgn}(\delta_m^{h_1})}{2} + \sum_{m=1}^{n_{h_2}} \text{sgn}(v_m^{h_2}) \frac{1 - \text{sgn}(\delta_m^{h_2})}{2}
\end{aligned} \tag{S181.2}$$

$$\begin{aligned}
\mathcal{W}_3^{\text{gapless}} = & \sum_{m=1}^{n_{c_1}} \text{sgn}(v_m^{c_1}) \frac{1 - \text{sgn}(\delta_m^{c_1})}{2} + \sum_{m=1}^{n_{c_2}} \text{sgn}(v_m^{c_2}) \frac{1 - \text{sgn}(\delta_m^{c_2})}{2} - \sum_{m=1}^{n_{f_1}} \text{sgn}(v_m^{f_1}) \frac{1 - \text{sgn}(\delta_m^{f_1})}{2} \\
& - \sum_{m=1}^{n_{f_2}} \text{sgn}(v_m^{f_2}) \frac{1 - \text{sgn}(\delta_m^{f_2})}{2} - \sum_{m=1}^{n_{h_1}} \text{sgn}(v_m^{h_1}) \frac{1 - \text{sgn}(\delta_m^{h_1})}{2} - \sum_{m=1}^{n_{h_2}} \text{sgn}(v_m^{h_2}) \frac{1 - \text{sgn}(\delta_m^{h_2})}{2} \\
& + \sum_{m=1}^{n_{i_1}} \text{sgn}(v_m^{i_1}) \frac{1 - \text{sgn}(\delta_m^{i_1})}{2} + \sum_{m=1}^{n_{i_2}} \text{sgn}(v_m^{i_2}) \frac{1 - \text{sgn}(\delta_m^{i_2})}{2} + \sum_{m=1}^{n_{i_3}} \text{sgn}(v_m^{i_3}) \frac{1 - \text{sgn}(\delta_m^{i_3})}{2}
\end{aligned} \tag{S181.3}$$

$$\begin{aligned}
\mathcal{W}_4^{\text{gapless}} = & \sum_{m=1}^{n_{d_1}} \text{sgn}(v_m^{d_1}) \frac{1 - \text{sgn}(\delta_m^{d_1})}{2} + \sum_{m=1}^{n_{d_2}} \text{sgn}(v_m^{d_2}) \frac{1 - \text{sgn}(\delta_m^{d_2})}{2} - \sum_{m=1}^{n_{e_1}} \text{sgn}(v_m^{e_1}) \frac{1 - \text{sgn}(\delta_m^{e_1})}{2} \\
& - \sum_{m=1}^{n_{e_2}} \text{sgn}(v_m^{e_2}) \frac{1 - \text{sgn}(\delta_m^{e_2})}{2} - \sum_{m=1}^{n_{f_1}} \text{sgn}(v_m^{f_1}) \frac{1 - \text{sgn}(\delta_m^{f_1})}{2} - \sum_{m=1}^{n_{f_2}} \text{sgn}(v_m^{f_2}) \frac{1 - \text{sgn}(\delta_m^{f_2})}{2}
\end{aligned} \tag{S181.4}$$

$$\begin{aligned}
\mathcal{W}_1^{\text{gapped}} = & - \sum_{m=1}^{n_{g_1}} \text{sgn}(v_m^{g_1}) \frac{1 - \text{sgn}(\delta_m^{g_1})}{2} + \sum_{m=1}^{n_{g_2}} \text{sgn}(v_m^{g_2}) \frac{1 - \text{sgn}(\delta_m^{g_2})}{2} + \sum_{m=1}^{n_{g_3}} \text{sgn}(v_m^{g_3}) \frac{1 - \text{sgn}(\delta_m^{g_3})}{2} \\
& - \sum_{m=1}^{n_{g_4}} \text{sgn}(v_m^{g_4}) \frac{1 - \text{sgn}(\delta_m^{g_4})}{2} - \sum_{m=1}^{n_{g_5}} \text{sgn}(v_m^{g_5}) \frac{1 - \text{sgn}(\delta_m^{g_5})}{2} + \sum_{m=1}^{n_{g_6}} \text{sgn}(v_m^{g_6}) \frac{1 - \text{sgn}(\delta_m^{g_6})}{2}
\end{aligned} \tag{S181.5}$$

$$\begin{aligned}
\mathcal{W}_2^{\text{gapped}} = & \sum_{m=1}^{n_{b_2}} \text{sgn}(v_m^{b_2}) \frac{1 - \text{sgn}(\delta_m^{b_2})}{2} - \sum_{m=1}^{n_{e_2}} \text{sgn}(v_m^{e_2}) \frac{1 - \text{sgn}(\delta_m^{e_2})}{2} - \sum_{m=1}^{n_{g_1}} \text{sgn}(v_m^{g_1}) \frac{1 - \text{sgn}(\delta_m^{g_1})}{2} \\
& - \sum_{m=1}^{n_{g_4}} \text{sgn}(v_m^{g_4}) \frac{1 - \text{sgn}(\delta_m^{g_4})}{2} - \sum_{m=1}^{n_{g_5}} \text{sgn}(v_m^{g_5}) \frac{1 - \text{sgn}(\delta_m^{g_5})}{2} + \sum_{m=1}^{n_{h_1}} \text{sgn}(v_m^{h_1}) \frac{1 - \text{sgn}(\delta_m^{h_1})}{2}
\end{aligned} \tag{S181.6}$$

$$\mathcal{W}_3^{\text{gapped}} = - \sum_{m=1}^{n_{h_1}} \text{sgn}(v_m^{h_1}) \frac{1 - \text{sgn}(\delta_m^{h_1})}{2} + \sum_{m=1}^{n_{h_2}} \text{sgn}(v_m^{h_2}) \frac{1 - \text{sgn}(\delta_m^{h_2})}{2} \tag{S181.7}$$

$$\mathcal{W}_4^{\text{gapped}} = \sum_{m=1}^{n_{e_1}} \text{sgn}(v_m^{e_1}) \frac{1 - \text{sgn}(\delta_m^{e_1})}{2} - \sum_{m=1}^{n_{e_2}} \text{sgn}(v_m^{e_2}) \frac{1 - \text{sgn}(\delta_m^{e_2})}{2} \tag{S181.8}$$

$$\mathcal{W}_5^{\text{gapped}} = - \sum_{m=1}^{n_{d_2}} \text{sgn}(v_m^{d_2}) \frac{1 - \text{sgn}(\delta_m^{d_2})}{2} + \sum_{m=1}^{n_{e_2}} \text{sgn}(v_m^{e_2}) \frac{1 - \text{sgn}(\delta_m^{e_2})}{2} + \sum_{m=1}^{n_{f_1}} \text{sgn}(v_m^{f_1}) \frac{1 - \text{sgn}(\delta_m^{f_1})}{2} \quad (\text{S181.9})$$

$$\begin{aligned} \mathcal{W}_6^{\text{gapped}} = & \sum_{m=1}^{n_{a_2}} \text{sgn}(v_m^{a_2}) \frac{1 - \text{sgn}(\delta_m^{a_2})}{2} + \sum_{m=1}^{n_{c_2}} \text{sgn}(v_m^{c_2}) \frac{1 - \text{sgn}(\delta_m^{c_2})}{2} - \sum_{m=1}^{n_{d_2}} \text{sgn}(v_m^{d_2}) \frac{1 - \text{sgn}(\delta_m^{d_2})}{2} - \sum_{m=1}^{n_{f_2}} \text{sgn}(v_m^{f_2}) \frac{1 - \text{sgn}(\delta_m^{f_2})}{2} \\ & - \sum_{m=1}^{n_{g_1}} \text{sgn}(v_m^{g_1}) \frac{1 - \text{sgn}(\delta_m^{g_1})}{2} - \sum_{m=1}^{n_{g_4}} \text{sgn}(v_m^{g_4}) \frac{1 - \text{sgn}(\delta_m^{g_4})}{2} - \sum_{m=1}^{n_{g_5}} \text{sgn}(v_m^{g_5}) \frac{1 - \text{sgn}(\delta_m^{g_5})}{2} \\ & - \sum_{m=1}^{n_{h_1}} \text{sgn}(v_m^{h_1}) \frac{1 - \text{sgn}(\delta_m^{h_1})}{2} + \sum_{m=1}^{n_{i_1}} \text{sgn}(v_m^{i_1}) \frac{1 - \text{sgn}(\delta_m^{i_1})}{2} + \sum_{m=1}^{n_{i_2}} \text{sgn}(v_m^{i_2}) \frac{1 - \text{sgn}(\delta_m^{i_2})}{2} + \sum_{m=1}^{n_{i_3}} \text{sgn}(v_m^{i_3}) \frac{1 - \text{sgn}(\delta_m^{i_3})}{2} \end{aligned} \quad (\text{S181.10})$$

$$\begin{aligned} \mathcal{X}_1 = & - \sum_{m=1}^{n_{a_2}} \text{sgn}(v_m^{a_2}) \frac{1 - \text{sgn}(\delta_m^{a_2})}{2} - \sum_{m=1}^{n_{c_2}} \text{sgn}(v_m^{c_2}) \frac{1 - \text{sgn}(\delta_m^{c_2})}{2} - \sum_{m=1}^{n_{e_2}} \text{sgn}(v_m^{e_2}) \frac{1 - \text{sgn}(\delta_m^{e_2})}{2} - \sum_{m=1}^{n_{g_1}} \text{sgn}(v_m^{g_1}) \frac{1 - \text{sgn}(\delta_m^{g_1})}{2} \\ & + 2 \sum_{m=1}^{n_{g_2}} \text{sgn}(v_m^{g_2}) \frac{1 - \text{sgn}(\delta_m^{g_2})}{2} + 4 \sum_{m=1}^{n_{g_3}} \text{sgn}(v_m^{g_3}) \frac{1 - \text{sgn}(\delta_m^{g_3})}{2} + \sum_{m=1}^{n_{g_5}} \text{sgn}(v_m^{g_5}) \frac{1 - \text{sgn}(\delta_m^{g_5})}{2} \\ & + \sum_{m=1}^{n_{h_1}} \text{sgn}(v_m^{h_1}) \frac{1 - \text{sgn}(\delta_m^{h_1})}{2} - \sum_{m=1}^{n_{i_1}} \text{sgn}(v_m^{i_1}) \frac{1 - \text{sgn}(\delta_m^{i_1})}{2} - 2 \sum_{m=1}^{n_{i_2}} \text{sgn}(v_m^{i_2}) \frac{1 - \text{sgn}(\delta_m^{i_2})}{2} \pmod{3} \end{aligned} \quad (\text{S181.11})$$

## S182. SPACE GROUP NO. 182

| line segment                                        | character of irrep (generators only)                                                                                                                                                                                                                                                                                                         |
|-----------------------------------------------------|----------------------------------------------------------------------------------------------------------------------------------------------------------------------------------------------------------------------------------------------------------------------------------------------------------------------------------------------|
| $a \quad (\frac{t}{3}, \frac{t}{3}, 0)$             | $\{2_{110}   0 \ 0 \ 0\}$<br>$a_1 \quad -i$<br>$a_2 \quad i$                                                                                                                                                                                                                                                                                 |
| $b \quad (0, \frac{t}{2}, 0)$                       | $\{2_{010}   0 \ 0 \ \frac{1}{2}\}$<br>$b_1 \quad -i$<br>$b_2 \quad i$                                                                                                                                                                                                                                                                       |
| $c \quad (\frac{t}{3}, \frac{3-t}{6}, 0)$           | $\{2_{100}   0 \ 0 \ 0\}$<br>$c_1 \quad -i$<br>$c_2 \quad i$                                                                                                                                                                                                                                                                                 |
| $d \quad (\frac{t}{3}, \frac{t}{3}, \frac{1}{2})$   | $\{2_{110}   0 \ 0 \ 0\}$<br>$d_1 \quad -i$<br>$d_2 \quad i$                                                                                                                                                                                                                                                                                 |
| $e \quad (0, \frac{t}{2}, \frac{1}{2})$             | $\{2_{010}   0 \ 0 \ \frac{1}{2}\}$<br>$e_1 \quad i$<br>$e_2 \quad -i$                                                                                                                                                                                                                                                                       |
| $f \quad (\frac{t}{3}, \frac{3-t}{6}, \frac{1}{2})$ | $\{2_{100}   0 \ 0 \ 0\}$<br>$f_1 \quad -i$<br>$f_2 \quad i$                                                                                                                                                                                                                                                                                 |
| $g \quad (0, 0, \frac{t}{2})$                       | $\{6_{001}   0 \ 0 \ \frac{1}{2}\}$<br>$g_1 \quad e^{-\frac{1}{2}i\pi t - \frac{5i\pi}{6}}$<br>$g_2 \quad e^{\frac{5i\pi}{6} - \frac{i\pi t}{2}}$<br>$g_3 \quad -ie^{-\frac{1}{2}i\pi t}$<br>$g_4 \quad ie^{-\frac{1}{2}i\pi t}$<br>$g_5 \quad e^{-\frac{1}{2}i\pi t - \frac{i\pi}{6}}$<br>$g_6 \quad e^{\frac{i\pi}{6} - \frac{i\pi t}{2}}$ |

|                                                   |                                                                                                                    |
|---------------------------------------------------|--------------------------------------------------------------------------------------------------------------------|
| $h \quad (0, \frac{1}{2}, \frac{t}{2})$           | $\{2_{001}   0 \ 0 \ \frac{1}{2}\}$<br>$h_1 \quad -ie^{-\frac{1}{2}i\pi t}$<br>$h_2 \quad ie^{-\frac{1}{2}i\pi t}$ |
| $i \quad (\frac{1}{3}, \frac{1}{3}, \frac{t}{2})$ | $\{3_{001}   0 \ 0 \ 0\}$<br>$i_1 \quad -1$<br>$i_2 \quad e^{-\frac{i\pi}{3}}$<br>$i_3 \quad e^{\frac{i\pi}{3}}$   |

$$\begin{aligned}
\mathcal{W}_1^{\text{gapless}} = & \sum_{m=1}^{n_{a_1}} \text{sgn}(v_m^{a_1}) \frac{1 - \text{sgn}(\delta_m^{a_1})}{2} + \sum_{m=1}^{n_{a_2}} \text{sgn}(v_m^{a_2}) \frac{1 - \text{sgn}(\delta_m^{a_2})}{2} - 2 \sum_{m=1}^{n_{e_1}} \text{sgn}(v_m^{e_1}) \frac{1 - \text{sgn}(\delta_m^{e_1})}{2} \\
& - 2 \sum_{m=1}^{n_{f_1}} \text{sgn}(v_m^{f_1}) \frac{1 - \text{sgn}(\delta_m^{f_1})}{2} - \sum_{m=1}^{n_{g_1}} \text{sgn}(v_m^{g_1}) \frac{1 - \text{sgn}(\delta_m^{g_1})}{2} - \sum_{m=1}^{n_{g_2}} \text{sgn}(v_m^{g_2}) \frac{1 - \text{sgn}(\delta_m^{g_2})}{2} \\
& - \sum_{m=1}^{n_{g_3}} \text{sgn}(v_m^{g_3}) \frac{1 - \text{sgn}(\delta_m^{g_3})}{2} - \sum_{m=1}^{n_{g_4}} \text{sgn}(v_m^{g_4}) \frac{1 - \text{sgn}(\delta_m^{g_4})}{2} - \sum_{m=1}^{n_{g_5}} \text{sgn}(v_m^{g_5}) \frac{1 - \text{sgn}(\delta_m^{g_5})}{2} \\
& - \sum_{m=1}^{n_{g_6}} \text{sgn}(v_m^{g_6}) \frac{1 - \text{sgn}(\delta_m^{g_6})}{2} + \sum_{m=1}^{n_{i_1}} \text{sgn}(v_m^{i_1}) \frac{1 - \text{sgn}(\delta_m^{i_1})}{2} + \sum_{m=1}^{n_{i_2}} \text{sgn}(v_m^{i_2}) \frac{1 - \text{sgn}(\delta_m^{i_2})}{2} + \sum_{m=1}^{n_{i_3}} \text{sgn}(v_m^{i_3}) \frac{1 - \text{sgn}(\delta_m^{i_3})}{2}
\end{aligned} \tag{S182.1}$$

$$\begin{aligned}
\mathcal{W}_2^{\text{gapless}} = & \sum_{m=1}^{n_{b_1}} \text{sgn}(v_m^{b_1}) \frac{1 - \text{sgn}(\delta_m^{b_1})}{2} + \sum_{m=1}^{n_{b_2}} \text{sgn}(v_m^{b_2}) \frac{1 - \text{sgn}(\delta_m^{b_2})}{2} - 2 \sum_{m=1}^{n_{e_1}} \text{sgn}(v_m^{e_1}) \frac{1 - \text{sgn}(\delta_m^{e_1})}{2} \\
& - \sum_{m=1}^{n_{g_1}} \text{sgn}(v_m^{g_1}) \frac{1 - \text{sgn}(\delta_m^{g_1})}{2} - \sum_{m=1}^{n_{g_2}} \text{sgn}(v_m^{g_2}) \frac{1 - \text{sgn}(\delta_m^{g_2})}{2} - \sum_{m=1}^{n_{g_3}} \text{sgn}(v_m^{g_3}) \frac{1 - \text{sgn}(\delta_m^{g_3})}{2} \\
& - \sum_{m=1}^{n_{g_4}} \text{sgn}(v_m^{g_4}) \frac{1 - \text{sgn}(\delta_m^{g_4})}{2} - \sum_{m=1}^{n_{g_5}} \text{sgn}(v_m^{g_5}) \frac{1 - \text{sgn}(\delta_m^{g_5})}{2} - \sum_{m=1}^{n_{g_6}} \text{sgn}(v_m^{g_6}) \frac{1 - \text{sgn}(\delta_m^{g_6})}{2} \\
& + \sum_{m=1}^{n_{h_1}} \text{sgn}(v_m^{h_1}) \frac{1 - \text{sgn}(\delta_m^{h_1})}{2} + \sum_{m=1}^{n_{h_2}} \text{sgn}(v_m^{h_2}) \frac{1 - \text{sgn}(\delta_m^{h_2})}{2}
\end{aligned} \tag{S182.2}$$

$$\begin{aligned}
\mathcal{W}_3^{\text{gapless}} = & \sum_{m=1}^{n_{c_1}} \text{sgn}(v_m^{c_1}) \frac{1 - \text{sgn}(\delta_m^{c_1})}{2} + \sum_{m=1}^{n_{c_2}} \text{sgn}(v_m^{c_2}) \frac{1 - \text{sgn}(\delta_m^{c_2})}{2} - 2 \sum_{m=1}^{n_{f_1}} \text{sgn}(v_m^{f_1}) \frac{1 - \text{sgn}(\delta_m^{f_1})}{2} - \sum_{m=1}^{n_{h_1}} \text{sgn}(v_m^{h_1}) \frac{1 - \text{sgn}(\delta_m^{h_1})}{2} \\
& - \sum_{m=1}^{n_{h_2}} \text{sgn}(v_m^{h_2}) \frac{1 - \text{sgn}(\delta_m^{h_2})}{2} + \sum_{m=1}^{n_{i_1}} \text{sgn}(v_m^{i_1}) \frac{1 - \text{sgn}(\delta_m^{i_1})}{2} + \sum_{m=1}^{n_{i_2}} \text{sgn}(v_m^{i_2}) \frac{1 - \text{sgn}(\delta_m^{i_2})}{2} + \sum_{m=1}^{n_{i_3}} \text{sgn}(v_m^{i_3}) \frac{1 - \text{sgn}(\delta_m^{i_3})}{2}
\end{aligned} \tag{S182.3}$$

$$\mathcal{W}_4^{\text{gapless}} = \sum_{m=1}^{n_{d_1}} \text{sgn}(v_m^{d_1}) \frac{1 - \text{sgn}(\delta_m^{d_1})}{2} - \sum_{m=1}^{n_{e_1}} \text{sgn}(v_m^{e_1}) \frac{1 - \text{sgn}(\delta_m^{e_1})}{2} - \sum_{m=1}^{n_{f_1}} \text{sgn}(v_m^{f_1}) \frac{1 - \text{sgn}(\delta_m^{f_1})}{2} \tag{S182.4}$$

$$\begin{aligned}
\mathcal{W}_1^{\text{gapped}} = & 2 \sum_{m=1}^{n_{b_2}} \text{sgn}(v_m^{b_2}) \frac{1 - \text{sgn}(\delta_m^{b_2})}{2} - 2 \sum_{m=1}^{n_{e_1}} \text{sgn}(v_m^{e_1}) \frac{1 - \text{sgn}(\delta_m^{e_1})}{2} - 2 \sum_{m=1}^{n_{g_1}} \text{sgn}(v_m^{g_1}) \frac{1 - \text{sgn}(\delta_m^{g_1})}{2} \\
& - \sum_{m=1}^{n_{g_3}} \text{sgn}(v_m^{g_3}) \frac{1 - \text{sgn}(\delta_m^{g_3})}{2} - \sum_{m=1}^{n_{g_4}} \text{sgn}(v_m^{g_4}) \frac{1 - \text{sgn}(\delta_m^{g_4})}{2} - 2 \sum_{m=1}^{n_{g_6}} \text{sgn}(v_m^{g_6}) \frac{1 - \text{sgn}(\delta_m^{g_6})}{2} \\
& + \sum_{m=1}^{n_{h_1}} \text{sgn}(v_m^{h_1}) \frac{1 - \text{sgn}(\delta_m^{h_1})}{2} + \sum_{m=1}^{n_{h_2}} \text{sgn}(v_m^{h_2}) \frac{1 - \text{sgn}(\delta_m^{h_2})}{2}
\end{aligned} \tag{S182.5}$$

$$\begin{aligned}
\mathcal{W}_2^{\text{gapped}} = & - \sum_{m=1}^{n_{a_2}} \text{sgn}(v_m^{a_2}) \frac{1 - \text{sgn}(\delta_m^{a_2})}{2} - \sum_{m=1}^{n_{b_2}} \text{sgn}(v_m^{b_2}) \frac{1 - \text{sgn}(\delta_m^{b_2})}{2} - \sum_{m=1}^{n_{c_2}} \text{sgn}(v_m^{c_2}) \frac{1 - \text{sgn}(\delta_m^{c_2})}{2} \\
& + 2 \sum_{m=1}^{n_{e_1}} \text{sgn}(v_m^{e_1}) \frac{1 - \text{sgn}(\delta_m^{e_1})}{2} + 2 \sum_{m=1}^{n_{f_1}} \text{sgn}(v_m^{f_1}) \frac{1 - \text{sgn}(\delta_m^{f_1})}{2} \\
& + 2 \sum_{m=1}^{n_{g_1}} \text{sgn}(v_m^{g_1}) \frac{1 - \text{sgn}(\delta_m^{g_1})}{2} + \sum_{m=1}^{n_{g_3}} \text{sgn}(v_m^{g_3}) \frac{1 - \text{sgn}(\delta_m^{g_3})}{2} + \sum_{m=1}^{n_{g_4}} \text{sgn}(v_m^{g_4}) \frac{1 - \text{sgn}(\delta_m^{g_4})}{2} \\
& + 2 \sum_{m=1}^{n_{g_6}} \text{sgn}(v_m^{g_6}) \frac{1 - \text{sgn}(\delta_m^{g_6})}{2} - \sum_{m=1}^{n_{i_1}} \text{sgn}(v_m^{i_1}) \frac{1 - \text{sgn}(\delta_m^{i_1})}{2} - 2 \sum_{m=1}^{n_{i_2}} \text{sgn}(v_m^{i_2}) \frac{1 - \text{sgn}(\delta_m^{i_2})}{2}
\end{aligned} \tag{S182.6}$$

$$\begin{aligned}
\mathcal{W}_3^{\text{gapped}} = & - \sum_{m=1}^{n_{g_1}} \text{sgn}(v_m^{g_1}) \frac{1 - \text{sgn}(\delta_m^{g_1})}{2} + \sum_{m=1}^{n_{g_2}} \text{sgn}(v_m^{g_2}) \frac{1 - \text{sgn}(\delta_m^{g_2})}{2} + \sum_{m=1}^{n_{g_5}} \text{sgn}(v_m^{g_5}) \frac{1 - \text{sgn}(\delta_m^{g_5})}{2} \\
& - \sum_{m=1}^{n_{g_6}} \text{sgn}(v_m^{g_6}) \frac{1 - \text{sgn}(\delta_m^{g_6})}{2}
\end{aligned} \tag{S182.7}$$

$$\mathcal{W}_4^{\text{gapped}} = - \sum_{m=1}^{n_{i_2}} \text{sgn}(v_m^{i_2}) \frac{1 - \text{sgn}(\delta_m^{i_2})}{2} + \sum_{m=1}^{n_{i_3}} \text{sgn}(v_m^{i_3}) \frac{1 - \text{sgn}(\delta_m^{i_3})}{2} \tag{S182.8}$$

$$\begin{aligned}
\mathcal{X}_1 = & \sum_{m=1}^{n_{a_2}} \frac{1 - \text{sgn}(\delta_m^{a_2})}{2} + \sum_{m=1}^{n_{c_2}} \frac{1 - \text{sgn}(\delta_m^{c_2})}{2} + \sum_{m=1}^{n_{g_1}} \frac{1 - \text{sgn}(\delta_m^{g_1})}{2} + \sum_{m=1}^{n_{g_3}} \frac{1 - \text{sgn}(\delta_m^{g_3})}{2} + \sum_{m=1}^{n_{g_5}} \frac{1 - \text{sgn}(\delta_m^{g_5})}{2} \\
& + \sum_{m=1}^{n_{h_1}} \frac{1 - \text{sgn}(\delta_m^{h_1})}{2} + \sum_{m=1}^{n_{i_1}} \frac{1 - \text{sgn}(\delta_m^{i_1})}{2} \quad \text{mod } 2
\end{aligned} \tag{S182.9}$$

$$\mathcal{X}_2 = \sum_{m=1}^{n_{b_2}} \frac{1 - \text{sgn}(\delta_m^{b_2})}{2} + \sum_{m=1}^{n_{g_1}} \frac{1 - \text{sgn}(\delta_m^{g_1})}{2} + \sum_{m=1}^{n_{g_3}} \frac{1 - \text{sgn}(\delta_m^{g_3})}{2} + \sum_{m=1}^{n_{g_5}} \frac{1 - \text{sgn}(\delta_m^{g_5})}{2} + \sum_{m=1}^{n_{h_1}} \frac{1 - \text{sgn}(\delta_m^{h_1})}{2} \quad \text{mod } 2 \tag{S182.10}$$

### S183. SPACE GROUP NO. 183

|              |                                      |
|--------------|--------------------------------------|
| line segment | character of irrep (generators only) |
|--------------|--------------------------------------|

|                                                     |                                                                                                                                                   |
|-----------------------------------------------------|---------------------------------------------------------------------------------------------------------------------------------------------------|
| $a \quad (\frac{t}{3}, \frac{t}{3}, 0)$             | $\{m_{-110}  0 \ 0 \ 0 \}$<br>$a_1 \quad -i$<br>$a_2 \quad i$                                                                                     |
| $b \quad (0, \frac{t}{2}, 0)$                       | $\{m_{100}  0 \ 0 \ 0 \}$<br>$b_1 \quad -i$<br>$b_2 \quad i$                                                                                      |
| $c \quad (\frac{t}{3}, \frac{3-t}{6}, 0)$           | $\{m_{010}  0 \ 0 \ 0 \}$<br>$c_1 \quad -i$<br>$c_2 \quad i$                                                                                      |
| $d \quad (\frac{t}{3}, \frac{t}{3}, \frac{1}{2})$   | $\{m_{-110}  0 \ 0 \ 0 \}$<br>$d_1 \quad -i$<br>$d_2 \quad i$                                                                                     |
| $e \quad (0, \frac{t}{2}, \frac{1}{2})$             | $\{m_{100}  0 \ 0 \ 0 \}$<br>$e_1 \quad -i$<br>$e_2 \quad i$                                                                                      |
| $f \quad (\frac{t}{3}, \frac{3-t}{6}, \frac{1}{2})$ | $\{m_{010}  0 \ 0 \ 0 \}$<br>$f_1 \quad -i$<br>$f_2 \quad i$                                                                                      |
| $g \quad (0, 0, \frac{t}{2})$                       | $\{6_{001}  0 \ 0 \ 0 \} \quad \{m_{100}  0 \ 0 \ 0 \}$<br>$g_1 \quad -\sqrt{3} \quad 0$<br>$g_2 \quad 0 \quad 0$<br>$g_3 \quad \sqrt{3} \quad 0$ |
| $h \quad (0, \frac{1}{2}, \frac{t}{2})$             | $\{2_{001}  0 \ 0 \ 0 \} \quad \{m_{100}  0 \ 0 \ 0 \}$<br>$h_1 \quad 0 \quad 0$                                                                  |
| $i \quad (\frac{1}{3}, \frac{1}{3}, \frac{t}{2})$   | $\{3_{001}  0 \ 0 \ 0 \} \quad \{m_{210}  0 \ 0 \ 0 \}$<br>$i_1 \quad -1 \quad -i$<br>$i_2 \quad -1 \quad i$<br>$i_3 \quad 1 \quad 0$             |

$$\begin{aligned}
\mathcal{W}_1^{\text{gapless}} = & \sum_{m=1}^{n_{a_1}} \text{sgn}(v_m^{a_1}) \frac{1 - \text{sgn}(\delta_m^{a_1})}{2} + \sum_{m=1}^{n_{d_2}} \text{sgn}(v_m^{d_2}) \frac{1 - \text{sgn}(\delta_m^{d_2})}{2} - \sum_{m=1}^{n_{e_1}} \text{sgn}(v_m^{e_1}) \frac{1 - \text{sgn}(\delta_m^{e_1})}{2} - \sum_{m=1}^{n_{e_2}} \text{sgn}(v_m^{e_2}) \frac{1 - \text{sgn}(\delta_m^{e_2})}{2} \\
& - \sum_{m=1}^{n_{f_1}} \text{sgn}(v_m^{f_1}) \frac{1 - \text{sgn}(\delta_m^{f_1})}{2} - \sum_{m=1}^{n_{f_2}} \text{sgn}(v_m^{f_2}) \frac{1 - \text{sgn}(\delta_m^{f_2})}{2} - \sum_{m=1}^{n_{g_1}} \text{sgn}(v_m^{g_1}) \frac{1 - \text{sgn}(\delta_m^{g_1})}{2} \\
& - \sum_{m=1}^{n_{g_2}} \text{sgn}(v_m^{g_2}) \frac{1 - \text{sgn}(\delta_m^{g_2})}{2} - \sum_{m=1}^{n_{g_3}} \text{sgn}(v_m^{g_3}) \frac{1 - \text{sgn}(\delta_m^{g_3})}{2} + \sum_{m=1}^{n_{i_2}} \text{sgn}(v_m^{i_2}) \frac{1 - \text{sgn}(\delta_m^{i_2})}{2} + \sum_{m=1}^{n_{i_3}} \text{sgn}(v_m^{i_3}) \frac{1 - \text{sgn}(\delta_m^{i_3})}{2}
\end{aligned} \tag{S183.1}$$

$$\begin{aligned}
\mathcal{W}_2^{\text{gapless}} = & \sum_{m=1}^{n_{a_2}} \text{sgn}(v_m^{a_2}) \frac{1 - \text{sgn}(\delta_m^{a_2})}{2} - \sum_{m=1}^{n_{d_2}} \text{sgn}(v_m^{d_2}) \frac{1 - \text{sgn}(\delta_m^{d_2})}{2} - \sum_{m=1}^{n_{g_1}} \text{sgn}(v_m^{g_1}) \frac{1 - \text{sgn}(\delta_m^{g_1})}{2} - \sum_{m=1}^{n_{g_2}} \text{sgn}(v_m^{g_2}) \frac{1 - \text{sgn}(\delta_m^{g_2})}{2} \\
& - \sum_{m=1}^{n_{g_3}} \text{sgn}(v_m^{g_3}) \frac{1 - \text{sgn}(\delta_m^{g_3})}{2} + \sum_{m=1}^{n_{i_1}} \text{sgn}(v_m^{i_1}) \frac{1 - \text{sgn}(\delta_m^{i_1})}{2} + \sum_{m=1}^{n_{i_3}} \text{sgn}(v_m^{i_3}) \frac{1 - \text{sgn}(\delta_m^{i_3})}{2}
\end{aligned} \tag{S183.2}$$

$$\begin{aligned}
\mathcal{W}_3^{\text{gapless}} = & \sum_{m=1}^{n_{b_1}} \text{sgn}(v_m^{b_1}) \frac{1 - \text{sgn}(\delta_m^{b_1})}{2} - \sum_{m=1}^{n_{e_1}} \text{sgn}(v_m^{e_1}) \frac{1 - \text{sgn}(\delta_m^{e_1})}{2} - \sum_{m=1}^{n_{g_1}} \text{sgn}(v_m^{g_1}) \frac{1 - \text{sgn}(\delta_m^{g_1})}{2} \\
& - \sum_{m=1}^{n_{g_2}} \text{sgn}(v_m^{g_2}) \frac{1 - \text{sgn}(\delta_m^{g_2})}{2} - \sum_{m=1}^{n_{g_3}} \text{sgn}(v_m^{g_3}) \frac{1 - \text{sgn}(\delta_m^{g_3})}{2} + \sum_{m=1}^{n_{h_1}} \text{sgn}(v_m^{h_1}) \frac{1 - \text{sgn}(\delta_m^{h_1})}{2}
\end{aligned} \tag{S183.3}$$



$$\begin{aligned} \mathcal{W}_4^{\text{gapless}} = & \sum_{m=1}^{n_{b_2}} \text{sgn}(v_m^{b_2}) \frac{1 - \text{sgn}(\delta_m^{b_2})}{2} - \sum_{m=1}^{n_{e_2}} \text{sgn}(v_m^{e_2}) \frac{1 - \text{sgn}(\delta_m^{e_2})}{2} - \sum_{m=1}^{n_{g_1}} \text{sgn}(v_m^{g_1}) \frac{1 - \text{sgn}(\delta_m^{g_1})}{2} \\ & - \sum_{m=1}^{n_{g_2}} \text{sgn}(v_m^{g_2}) \frac{1 - \text{sgn}(\delta_m^{g_2})}{2} - \sum_{m=1}^{n_{g_3}} \text{sgn}(v_m^{g_3}) \frac{1 - \text{sgn}(\delta_m^{g_3})}{2} + \sum_{m=1}^{n_{h_1}} \text{sgn}(v_m^{h_1}) \frac{1 - \text{sgn}(\delta_m^{h_1})}{2} \end{aligned} \quad (\text{S183.4})$$

$$\begin{aligned} \mathcal{W}_5^{\text{gapless}} = & \sum_{m=1}^{n_{c_1}} \text{sgn}(v_m^{c_1}) \frac{1 - \text{sgn}(\delta_m^{c_1})}{2} - \sum_{m=1}^{n_{f_1}} \text{sgn}(v_m^{f_1}) \frac{1 - \text{sgn}(\delta_m^{f_1})}{2} - \sum_{m=1}^{n_{h_1}} \text{sgn}(v_m^{h_1}) \frac{1 - \text{sgn}(\delta_m^{h_1})}{2} \\ & + \sum_{m=1}^{n_{i_2}} \text{sgn}(v_m^{i_2}) \frac{1 - \text{sgn}(\delta_m^{i_2})}{2} + \sum_{m=1}^{n_{i_3}} \text{sgn}(v_m^{i_3}) \frac{1 - \text{sgn}(\delta_m^{i_3})}{2} \end{aligned} \quad (\text{S183.5})$$

$$\begin{aligned} \mathcal{W}_6^{\text{gapless}} = & \sum_{m=1}^{n_{c_2}} \text{sgn}(v_m^{c_2}) \frac{1 - \text{sgn}(\delta_m^{c_2})}{2} - \sum_{m=1}^{n_{f_2}} \text{sgn}(v_m^{f_2}) \frac{1 - \text{sgn}(\delta_m^{f_2})}{2} - \sum_{m=1}^{n_{h_1}} \text{sgn}(v_m^{h_1}) \frac{1 - \text{sgn}(\delta_m^{h_1})}{2} \\ & + \sum_{m=1}^{n_{i_1}} \text{sgn}(v_m^{i_1}) \frac{1 - \text{sgn}(\delta_m^{i_1})}{2} + \sum_{m=1}^{n_{i_3}} \text{sgn}(v_m^{i_3}) \frac{1 - \text{sgn}(\delta_m^{i_3})}{2} \end{aligned} \quad (\text{S183.6})$$

$$\begin{aligned} \mathcal{W}_7^{\text{gapless}} = & \sum_{m=1}^{n_{d_1}} \text{sgn}(v_m^{d_1}) \frac{1 - \text{sgn}(\delta_m^{d_1})}{2} + \sum_{m=1}^{n_{d_2}} \text{sgn}(v_m^{d_2}) \frac{1 - \text{sgn}(\delta_m^{d_2})}{2} - \sum_{m=1}^{n_{e_1}} \text{sgn}(v_m^{e_1}) \frac{1 - \text{sgn}(\delta_m^{e_1})}{2} \\ & - \sum_{m=1}^{n_{e_2}} \text{sgn}(v_m^{e_2}) \frac{1 - \text{sgn}(\delta_m^{e_2})}{2} - \sum_{m=1}^{n_{f_1}} \text{sgn}(v_m^{f_1}) \frac{1 - \text{sgn}(\delta_m^{f_1})}{2} - \sum_{m=1}^{n_{f_2}} \text{sgn}(v_m^{f_2}) \frac{1 - \text{sgn}(\delta_m^{f_2})}{2} \end{aligned} \quad (\text{S183.7})$$

$$\mathcal{W}_1^{\text{gapped}} = \sum_{m=1}^{n_{d_2}} \text{sgn}(v_m^{d_2}) \frac{1 - \text{sgn}(\delta_m^{d_2})}{2} - \sum_{m=1}^{n_{e_2}} \text{sgn}(v_m^{e_2}) \frac{1 - \text{sgn}(\delta_m^{e_2})}{2} - \sum_{m=1}^{n_{f_2}} \text{sgn}(v_m^{f_2}) \frac{1 - \text{sgn}(\delta_m^{f_2})}{2} \quad (\text{S183.8})$$

$$\mathcal{W}_2^{\text{gapped}} = \sum_{m=1}^{n_{e_1}} \text{sgn}(v_m^{e_1}) \frac{1 - \text{sgn}(\delta_m^{e_1})}{2} - \sum_{m=1}^{n_{e_2}} \text{sgn}(v_m^{e_2}) \frac{1 - \text{sgn}(\delta_m^{e_2})}{2} \quad (\text{S183.9})$$

#### S184. SPACE GROUP NO. 184

| line segment                              | character of irrep (generators only)                                    |
|-------------------------------------------|-------------------------------------------------------------------------|
| $a \quad (\frac{t}{3}, \frac{t}{3}, 0)$   | $\{m_{-110}   0 \ 0 \ \frac{1}{2}\}$<br>$a_1 \quad -i$<br>$a_2 \quad i$ |
| $b \quad (0, \frac{t}{2}, 0)$             | $\{m_{100}   0 \ 0 \ \frac{1}{2}\}$<br>$b_1 \quad -i$<br>$b_2 \quad i$  |
| $c \quad (\frac{t}{3}, \frac{3-t}{6}, 0)$ | $\{m_{010}   0 \ 0 \ \frac{1}{2}\}$<br>$c_1 \quad -i$<br>$c_2 \quad i$  |

|                                                     |                                                                                                                                                                                             |
|-----------------------------------------------------|---------------------------------------------------------------------------------------------------------------------------------------------------------------------------------------------|
| $d \quad (\frac{t}{3}, \frac{t}{3}, \frac{1}{2})$   | $\{m_{-110}   0 \ 0 \ \frac{1}{2}\}$<br>$d_1 \quad -1$<br>$d_2 \quad 1$                                                                                                                     |
| $e \quad (0, \frac{t}{2}, \frac{1}{2})$             | $\{m_{100}   0 \ 0 \ \frac{1}{2}\}$<br>$e_1 \quad -1$<br>$e_2 \quad 1$                                                                                                                      |
| $f \quad (\frac{t}{3}, \frac{3-t}{6}, \frac{1}{2})$ | $\{m_{010}   0 \ 0 \ \frac{1}{2}\}$<br>$f_1 \quad -1$<br>$f_2 \quad 1$                                                                                                                      |
| $g \quad (0, 0, \frac{t}{2})$                       | $\{6_{001}   0 \ 0 \ 0\} \quad \{m_{100}   0 \ 0 \ \frac{1}{2}\}$<br>$g_1 \quad -\sqrt{3} \quad 0$<br>$g_2 \quad 0 \quad 0$<br>$g_3 \quad \sqrt{3} \quad 0$                                 |
| $h \quad (0, \frac{1}{2}, \frac{t}{2})$             | $\{2_{001}   0 \ 0 \ 0\} \quad \{m_{100}   0 \ 0 \ \frac{1}{2}\}$<br>$h_1 \quad 0 \quad 0$                                                                                                  |
| $i \quad (\frac{1}{3}, \frac{1}{3}, \frac{t}{2})$   | $\{3_{001}   0 \ 0 \ 0\} \quad \{m_{210}   0 \ 0 \ \frac{1}{2}\}$<br>$i_1 \quad -1 \quad -ie^{-\frac{1}{2}i\pi t}$<br>$i_2 \quad -1 \quad ie^{-\frac{1}{2}i\pi t}$<br>$i_3 \quad 1 \quad 0$ |

$$\begin{aligned}
\mathcal{W}_1^{\text{gapless}} = & \sum_{m=1}^{n_{a_1}} \text{sgn}(v_m^{a_1}) \frac{1 - \text{sgn}(\delta_m^{a_1})}{2} + \sum_{m=1}^{n_{d_1}} \text{sgn}(v_m^{d_1}) \frac{1 - \text{sgn}(\delta_m^{d_1})}{2} - 2 \sum_{m=1}^{n_{e_1}} \text{sgn}(v_m^{e_1}) \frac{1 - \text{sgn}(\delta_m^{e_1})}{2} \\
& - 2 \sum_{m=1}^{n_{f_1}} \text{sgn}(v_m^{f_1}) \frac{1 - \text{sgn}(\delta_m^{f_1})}{2} - \sum_{m=1}^{n_{g_1}} \text{sgn}(v_m^{g_1}) \frac{1 - \text{sgn}(\delta_m^{g_1})}{2} - \sum_{m=1}^{n_{g_2}} \text{sgn}(v_m^{g_2}) \frac{1 - \text{sgn}(\delta_m^{g_2})}{2} \\
& - \sum_{m=1}^{n_{g_3}} \text{sgn}(v_m^{g_3}) \frac{1 - \text{sgn}(\delta_m^{g_3})}{2} + \sum_{m=1}^{n_{i_2}} \text{sgn}(v_m^{i_2}) \frac{1 - \text{sgn}(\delta_m^{i_2})}{2} + \sum_{m=1}^{n_{i_3}} \text{sgn}(v_m^{i_3}) \frac{1 - \text{sgn}(\delta_m^{i_3})}{2}
\end{aligned} \tag{S184.1}$$

$$\begin{aligned}
\mathcal{W}_2^{\text{gapless}} = & \sum_{m=1}^{n_{a_2}} \text{sgn}(v_m^{a_2}) \frac{1 - \text{sgn}(\delta_m^{a_2})}{2} + \sum_{m=1}^{n_{d_1}} \text{sgn}(v_m^{d_1}) \frac{1 - \text{sgn}(\delta_m^{d_1})}{2} - 2 \sum_{m=1}^{n_{e_1}} \text{sgn}(v_m^{e_1}) \frac{1 - \text{sgn}(\delta_m^{e_1})}{2} \\
& - 2 \sum_{m=1}^{n_{f_1}} \text{sgn}(v_m^{f_1}) \frac{1 - \text{sgn}(\delta_m^{f_1})}{2} - \sum_{m=1}^{n_{g_1}} \text{sgn}(v_m^{g_1}) \frac{1 - \text{sgn}(\delta_m^{g_1})}{2} - \sum_{m=1}^{n_{g_2}} \text{sgn}(v_m^{g_2}) \frac{1 - \text{sgn}(\delta_m^{g_2})}{2} \\
& - \sum_{m=1}^{n_{g_3}} \text{sgn}(v_m^{g_3}) \frac{1 - \text{sgn}(\delta_m^{g_3})}{2} + \sum_{m=1}^{n_{i_1}} \text{sgn}(v_m^{i_1}) \frac{1 - \text{sgn}(\delta_m^{i_1})}{2} + \sum_{m=1}^{n_{i_3}} \text{sgn}(v_m^{i_3}) \frac{1 - \text{sgn}(\delta_m^{i_3})}{2}
\end{aligned} \tag{S184.2}$$

$$\begin{aligned}
\mathcal{W}_3^{\text{gapless}} = & \sum_{m=1}^{n_{b_1}} \text{sgn}(v_m^{b_1}) \frac{1 - \text{sgn}(\delta_m^{b_1})}{2} - \sum_{m=1}^{n_{e_1}} \text{sgn}(v_m^{e_1}) \frac{1 - \text{sgn}(\delta_m^{e_1})}{2} - \sum_{m=1}^{n_{g_1}} \text{sgn}(v_m^{g_1}) \frac{1 - \text{sgn}(\delta_m^{g_1})}{2} \\
& - \sum_{m=1}^{n_{g_2}} \text{sgn}(v_m^{g_2}) \frac{1 - \text{sgn}(\delta_m^{g_2})}{2} - \sum_{m=1}^{n_{g_3}} \text{sgn}(v_m^{g_3}) \frac{1 - \text{sgn}(\delta_m^{g_3})}{2} + \sum_{m=1}^{n_{h_1}} \text{sgn}(v_m^{h_1}) \frac{1 - \text{sgn}(\delta_m^{h_1})}{2}
\end{aligned} \tag{S184.3}$$

$$\begin{aligned}
\mathcal{W}_4^{\text{gapless}} = & \sum_{m=1}^{n_{b_2}} \text{sgn}(v_m^{b_2}) \frac{1 - \text{sgn}(\delta_m^{b_2})}{2} - \sum_{m=1}^{n_{e_1}} \text{sgn}(v_m^{e_1}) \frac{1 - \text{sgn}(\delta_m^{e_1})}{2} - \sum_{m=1}^{n_{g_1}} \text{sgn}(v_m^{g_1}) \frac{1 - \text{sgn}(\delta_m^{g_1})}{2} \\
& - \sum_{m=1}^{n_{g_2}} \text{sgn}(v_m^{g_2}) \frac{1 - \text{sgn}(\delta_m^{g_2})}{2} - \sum_{m=1}^{n_{g_3}} \text{sgn}(v_m^{g_3}) \frac{1 - \text{sgn}(\delta_m^{g_3})}{2} + \sum_{m=1}^{n_{h_1}} \text{sgn}(v_m^{h_1}) \frac{1 - \text{sgn}(\delta_m^{h_1})}{2}
\end{aligned} \tag{S184.4}$$

$$\begin{aligned} \mathcal{W}_5^{\text{gapless}} = & \sum_{m=1}^{n_{c_1}} \text{sgn}(v_m^{c_1}) \frac{1 - \text{sgn}(\delta_m^{c_1})}{2} - \sum_{m=1}^{n_{f_1}} \text{sgn}(v_m^{f_1}) \frac{1 - \text{sgn}(\delta_m^{f_1})}{2} - \sum_{m=1}^{n_{h_1}} \text{sgn}(v_m^{h_1}) \frac{1 - \text{sgn}(\delta_m^{h_1})}{2} \\ & + \sum_{m=1}^{n_{i_2}} \text{sgn}(v_m^{i_2}) \frac{1 - \text{sgn}(\delta_m^{i_2})}{2} + \sum_{m=1}^{n_{i_3}} \text{sgn}(v_m^{i_3}) \frac{1 - \text{sgn}(\delta_m^{i_3})}{2} \end{aligned} \quad (\text{S184.5})$$

$$\begin{aligned} \mathcal{W}_6^{\text{gapless}} = & \sum_{m=1}^{n_{c_2}} \text{sgn}(v_m^{c_2}) \frac{1 - \text{sgn}(\delta_m^{c_2})}{2} - \sum_{m=1}^{n_{f_1}} \text{sgn}(v_m^{f_1}) \frac{1 - \text{sgn}(\delta_m^{f_1})}{2} - \sum_{m=1}^{n_{h_1}} \text{sgn}(v_m^{h_1}) \frac{1 - \text{sgn}(\delta_m^{h_1})}{2} \\ & + \sum_{m=1}^{n_{i_1}} \text{sgn}(v_m^{i_1}) \frac{1 - \text{sgn}(\delta_m^{i_1})}{2} + \sum_{m=1}^{n_{i_3}} \text{sgn}(v_m^{i_3}) \frac{1 - \text{sgn}(\delta_m^{i_3})}{2} \end{aligned} \quad (\text{S184.6})$$

$$\mathcal{W}_7^{\text{gapless}} = \sum_{m=1}^{n_{d_1}} \text{sgn}(v_m^{d_1}) \frac{1 - \text{sgn}(\delta_m^{d_1})}{2} - \sum_{m=1}^{n_{e_1}} \text{sgn}(v_m^{e_1}) \frac{1 - \text{sgn}(\delta_m^{e_1})}{2} - \sum_{m=1}^{n_{f_1}} \text{sgn}(v_m^{f_1}) \frac{1 - \text{sgn}(\delta_m^{f_1})}{2} \quad (\text{S184.7})$$

$$\mathcal{X}_1 = \sum_{m=1}^{n_{e_1}} \frac{1 - \text{sgn}(\delta_m^{e_1})}{2} \quad \text{mod } 2 \quad (\text{S184.8})$$

### S185. SPACE GROUP NO. 185

| line segment                                        | character of irrep (generators only) |                                                                                                                    |
|-----------------------------------------------------|--------------------------------------|--------------------------------------------------------------------------------------------------------------------|
| $a \quad (\frac{t}{3}, \frac{t}{3}, 0)$             | $a_1$                                | $\{m_{-110}   0 \ 0 \ 0\}$<br>-i                                                                                   |
|                                                     | $a_2$                                | i                                                                                                                  |
| $b \quad (0, \frac{t}{2}, 0)$                       | $b_1$                                | $\{m_{100}   0 \ 0 \ \frac{1}{2}\}$<br>-i                                                                          |
|                                                     | $b_2$                                | i                                                                                                                  |
| $c \quad (\frac{t}{3}, \frac{3-t}{6}, 0)$           | $c_1$                                | $\{m_{010}   0 \ 0 \ 0\}$<br>-i                                                                                    |
|                                                     | $c_2$                                | i                                                                                                                  |
| $d \quad (\frac{t}{3}, \frac{t}{3}, \frac{1}{2})$   | $d_1$                                | $\{m_{-110}   0 \ 0 \ 0\}$<br>-i                                                                                   |
|                                                     | $d_2$                                | i                                                                                                                  |
| $e \quad (0, \frac{t}{2}, \frac{1}{2})$             | $e_1$                                | $\{m_{100}   0 \ 0 \ \frac{1}{2}\}$<br>-1                                                                          |
|                                                     | $e_2$                                | 1                                                                                                                  |
| $f \quad (\frac{t}{3}, \frac{3-t}{6}, \frac{1}{2})$ | $f_1$                                | $\{m_{010}   0 \ 0 \ 0\}$<br>-i                                                                                    |
|                                                     | $f_2$                                | i                                                                                                                  |
| $g \quad (0, 0, \frac{t}{2})$                       | $g_1$                                | $\{6_{001}   0 \ 0 \ \frac{1}{2}\} \quad \{m_{100}   0 \ 0 \ \frac{1}{2}\}$<br>$-\sqrt{3}e^{-\frac{1}{2}i\pi t}$ 0 |
|                                                     | $g_2$                                | 0      0                                                                                                           |
|                                                     | $g_3$                                | $\sqrt{3}e^{-\frac{1}{2}i\pi t}$ 0                                                                                 |
| $h \quad (0, \frac{1}{2}, \frac{t}{2})$             | $h_1$                                | $\{2_{001}   0 \ 0 \ \frac{1}{2}\} \quad \{m_{100}   0 \ 0 \ \frac{1}{2}\}$<br>0      0                            |
| $i \quad (\frac{1}{3}, \frac{1}{3}, \frac{t}{2})$   | $i_1$                                | $\{3_{001}   0 \ 0 \ 0\} \quad \{m_{210}   0 \ 0 \ 0\}$<br>-1      -i                                              |
|                                                     | $i_2$                                | -1      i                                                                                                          |
|                                                     | $i_3$                                | 1      0                                                                                                           |

---


$$\begin{aligned}
\mathcal{W}_1^{\text{gapless}} = & \sum_{m=1}^{n_{a_1}} \text{sgn}(v_m^{a_1}) \frac{1 - \text{sgn}(\delta_m^{a_1})}{2} + 2 \sum_{m=1}^{n_{d_2}} \text{sgn}(v_m^{d_2}) \frac{1 - \text{sgn}(\delta_m^{d_2})}{2} - 2 \sum_{m=1}^{n_{e_1}} \text{sgn}(v_m^{e_1}) \frac{1 - \text{sgn}(\delta_m^{e_1})}{2} \\
& - 2 \sum_{m=1}^{n_{f_1}} \text{sgn}(v_m^{f_1}) \frac{1 - \text{sgn}(\delta_m^{f_1})}{2} - 2 \sum_{m=1}^{n_{f_2}} \text{sgn}(v_m^{f_2}) \frac{1 - \text{sgn}(\delta_m^{f_2})}{2} - \sum_{m=1}^{n_{g_1}} \text{sgn}(v_m^{g_1}) \frac{1 - \text{sgn}(\delta_m^{g_1})}{2} \\
& - \sum_{m=1}^{n_{g_2}} \text{sgn}(v_m^{g_2}) \frac{1 - \text{sgn}(\delta_m^{g_2})}{2} - \sum_{m=1}^{n_{g_3}} \text{sgn}(v_m^{g_3}) \frac{1 - \text{sgn}(\delta_m^{g_3})}{2} + \sum_{m=1}^{n_{i_2}} \text{sgn}(v_m^{i_2}) \frac{1 - \text{sgn}(\delta_m^{i_2})}{2} + \sum_{m=1}^{n_{i_3}} \text{sgn}(v_m^{i_3}) \frac{1 - \text{sgn}(\delta_m^{i_3})}{2}
\end{aligned} \tag{S185.1}$$

$$\begin{aligned}
\mathcal{W}_2^{\text{gapless}} = & \sum_{m=1}^{n_{a_2}} \text{sgn}(v_m^{a_2}) \frac{1 - \text{sgn}(\delta_m^{a_2})}{2} - 2 \sum_{m=1}^{n_{d_2}} \text{sgn}(v_m^{d_2}) \frac{1 - \text{sgn}(\delta_m^{d_2})}{2} - \sum_{m=1}^{n_{g_1}} \text{sgn}(v_m^{g_1}) \frac{1 - \text{sgn}(\delta_m^{g_1})}{2} \\
& - \sum_{m=1}^{n_{g_2}} \text{sgn}(v_m^{g_2}) \frac{1 - \text{sgn}(\delta_m^{g_2})}{2} - \sum_{m=1}^{n_{g_3}} \text{sgn}(v_m^{g_3}) \frac{1 - \text{sgn}(\delta_m^{g_3})}{2} + \sum_{m=1}^{n_{i_1}} \text{sgn}(v_m^{i_1}) \frac{1 - \text{sgn}(\delta_m^{i_1})}{2} + \sum_{m=1}^{n_{i_3}} \text{sgn}(v_m^{i_3}) \frac{1 - \text{sgn}(\delta_m^{i_3})}{2}
\end{aligned} \tag{S185.2}$$

$$\begin{aligned}
\mathcal{W}_3^{\text{gapless}} = & \sum_{m=1}^{n_{b_1}} \text{sgn}(v_m^{b_1}) \frac{1 - \text{sgn}(\delta_m^{b_1})}{2} - \sum_{m=1}^{n_{e_1}} \text{sgn}(v_m^{e_1}) \frac{1 - \text{sgn}(\delta_m^{e_1})}{2} - \sum_{m=1}^{n_{g_1}} \text{sgn}(v_m^{g_1}) \frac{1 - \text{sgn}(\delta_m^{g_1})}{2} \\
& - \sum_{m=1}^{n_{g_2}} \text{sgn}(v_m^{g_2}) \frac{1 - \text{sgn}(\delta_m^{g_2})}{2} - \sum_{m=1}^{n_{g_3}} \text{sgn}(v_m^{g_3}) \frac{1 - \text{sgn}(\delta_m^{g_3})}{2} + \sum_{m=1}^{n_{h_1}} \text{sgn}(v_m^{h_1}) \frac{1 - \text{sgn}(\delta_m^{h_1})}{2}
\end{aligned} \tag{S185.3}$$

$$\begin{aligned}
\mathcal{W}_4^{\text{gapless}} = & \sum_{m=1}^{n_{b_2}} \text{sgn}(v_m^{b_2}) \frac{1 - \text{sgn}(\delta_m^{b_2})}{2} - \sum_{m=1}^{n_{e_1}} \text{sgn}(v_m^{e_1}) \frac{1 - \text{sgn}(\delta_m^{e_1})}{2} - \sum_{m=1}^{n_{g_1}} \text{sgn}(v_m^{g_1}) \frac{1 - \text{sgn}(\delta_m^{g_1})}{2} \\
& - \sum_{m=1}^{n_{g_2}} \text{sgn}(v_m^{g_2}) \frac{1 - \text{sgn}(\delta_m^{g_2})}{2} - \sum_{m=1}^{n_{g_3}} \text{sgn}(v_m^{g_3}) \frac{1 - \text{sgn}(\delta_m^{g_3})}{2} + \sum_{m=1}^{n_{h_1}} \text{sgn}(v_m^{h_1}) \frac{1 - \text{sgn}(\delta_m^{h_1})}{2}
\end{aligned} \tag{S185.4}$$

$$\begin{aligned}
\mathcal{W}_5^{\text{gapless}} = & \sum_{m=1}^{n_{c_1}} \text{sgn}(v_m^{c_1}) \frac{1 - \text{sgn}(\delta_m^{c_1})}{2} - 2 \sum_{m=1}^{n_{f_1}} \text{sgn}(v_m^{f_1}) \frac{1 - \text{sgn}(\delta_m^{f_1})}{2} - \sum_{m=1}^{n_{h_1}} \text{sgn}(v_m^{h_1}) \frac{1 - \text{sgn}(\delta_m^{h_1})}{2} \\
& + \sum_{m=1}^{n_{i_2}} \text{sgn}(v_m^{i_2}) \frac{1 - \text{sgn}(\delta_m^{i_2})}{2} + \sum_{m=1}^{n_{i_3}} \text{sgn}(v_m^{i_3}) \frac{1 - \text{sgn}(\delta_m^{i_3})}{2}
\end{aligned} \tag{S185.5}$$

$$\begin{aligned}
\mathcal{W}_6^{\text{gapless}} = & \sum_{m=1}^{n_{c_2}} \text{sgn}(v_m^{c_2}) \frac{1 - \text{sgn}(\delta_m^{c_2})}{2} - 2 \sum_{m=1}^{n_{f_2}} \text{sgn}(v_m^{f_2}) \frac{1 - \text{sgn}(\delta_m^{f_2})}{2} - \sum_{m=1}^{n_{h_1}} \text{sgn}(v_m^{h_1}) \frac{1 - \text{sgn}(\delta_m^{h_1})}{2} \\
& + \sum_{m=1}^{n_{i_1}} \text{sgn}(v_m^{i_1}) \frac{1 - \text{sgn}(\delta_m^{i_1})}{2} + \sum_{m=1}^{n_{i_3}} \text{sgn}(v_m^{i_3}) \frac{1 - \text{sgn}(\delta_m^{i_3})}{2}
\end{aligned} \tag{S185.6}$$

$$\begin{aligned} \mathcal{W}_7^{\text{gapless}} = & \sum_{m=1}^{n_{d_1}} \text{sgn}(v_m^{d_1}) \frac{1 - \text{sgn}(\delta_m^{d_1})}{2} + \sum_{m=1}^{n_{d_2}} \text{sgn}(v_m^{d_2}) \frac{1 - \text{sgn}(\delta_m^{d_2})}{2} - \sum_{m=1}^{n_{e_1}} \text{sgn}(v_m^{e_1}) \frac{1 - \text{sgn}(\delta_m^{e_1})}{2} \\ & - \sum_{m=1}^{n_{f_1}} \text{sgn}(v_m^{f_1}) \frac{1 - \text{sgn}(\delta_m^{f_1})}{2} - \sum_{m=1}^{n_{f_2}} \text{sgn}(v_m^{f_2}) \frac{1 - \text{sgn}(\delta_m^{f_2})}{2} \end{aligned} \quad (\text{S185.7})$$

$$\mathcal{W}_1^{\text{gapped}} = -2 \sum_{m=1}^{n_{d_2}} \text{sgn}(v_m^{d_2}) \frac{1 - \text{sgn}(\delta_m^{d_2})}{2} + \sum_{m=1}^{n_{e_1}} \text{sgn}(v_m^{e_1}) \frac{1 - \text{sgn}(\delta_m^{e_1})}{2} + 2 \sum_{m=1}^{n_{f_2}} \text{sgn}(v_m^{f_2}) \frac{1 - \text{sgn}(\delta_m^{f_2})}{2} \quad (\text{S185.8})$$

**S186. SPACE GROUP NO. 186**

| line segment                                               | character of irrep (generators only)                                                                                                                                                                    |
|------------------------------------------------------------|---------------------------------------------------------------------------------------------------------------------------------------------------------------------------------------------------------|
| $a \left( \frac{t}{3}, \frac{t}{3}, 0 \right)$             | $\{m_{-110}   0 \ 0 \ \frac{1}{2}\}$<br>$a_1 \quad -i$<br>$a_2 \quad i$                                                                                                                                 |
| $b \left( 0, \frac{t}{2}, 0 \right)$                       | $\{m_{100}   0 \ 0 \ 0\}$<br>$b_1 \quad -i$<br>$b_2 \quad i$                                                                                                                                            |
| $c \left( \frac{t}{3}, \frac{3-t}{6}, 0 \right)$           | $\{m_{010}   0 \ 0 \ \frac{1}{2}\}$<br>$c_1 \quad -i$<br>$c_2 \quad i$                                                                                                                                  |
| $d \left( \frac{t}{3}, \frac{t}{3}, \frac{1}{2} \right)$   | $\{m_{-110}   0 \ 0 \ \frac{1}{2}\}$<br>$d_1 \quad -1$<br>$d_2 \quad 1$                                                                                                                                 |
| $e \left( 0, \frac{t}{2}, \frac{1}{2} \right)$             | $\{m_{100}   0 \ 0 \ 0\}$<br>$e_1 \quad -i$<br>$e_2 \quad i$                                                                                                                                            |
| $f \left( \frac{t}{3}, \frac{3-t}{6}, \frac{1}{2} \right)$ | $\{m_{010}   0 \ 0 \ \frac{1}{2}\}$<br>$f_1 \quad -1$<br>$f_2 \quad 1$                                                                                                                                  |
| $g \left( 0, 0, \frac{t}{2} \right)$                       | $\{6_{001}   0 \ 0 \ \frac{1}{2}\} \quad \{m_{100}   0 \ 0 \ 0\}$<br>$g_1 \quad -\sqrt{3}e^{-\frac{1}{2}i\pi t} \quad 0$<br>$g_2 \quad 0 \quad 0$<br>$g_3 \quad \sqrt{3}e^{-\frac{1}{2}i\pi t} \quad 0$ |
| $h \left( 0, \frac{1}{2}, \frac{t}{2} \right)$             | $\{2_{001}   0 \ 0 \ \frac{1}{2}\} \quad \{m_{100}   0 \ 0 \ 0\}$<br>$h_1 \quad 0 \quad 0$                                                                                                              |
| $i \left( \frac{1}{3}, \frac{1}{3}, \frac{t}{2} \right)$   | $\{3_{001}   0 \ 0 \ 0\} \quad \{m_{210}   0 \ 0 \ \frac{1}{2}\}$<br>$i_1 \quad -1 \quad -ie^{-\frac{1}{2}i\pi t}$<br>$i_2 \quad -1 \quad ie^{-\frac{1}{2}i\pi t}$<br>$i_3 \quad 1 \quad 0$             |

$$\begin{aligned} \mathcal{W}_1^{\text{gapless}} = & \sum_{m=1}^{n_{a_1}} \text{sgn}(v_m^{a_1}) \frac{1 - \text{sgn}(\delta_m^{a_1})}{2} - \sum_{m=1}^{n_{e_1}} \text{sgn}(v_m^{e_1}) \frac{1 - \text{sgn}(\delta_m^{e_1})}{2} - \sum_{m=1}^{n_{e_2}} \text{sgn}(v_m^{e_2}) \frac{1 - \text{sgn}(\delta_m^{e_2})}{2} \\ & - \sum_{m=1}^{n_{f_1}} \text{sgn}(v_m^{f_1}) \frac{1 - \text{sgn}(\delta_m^{f_1})}{2} - \sum_{m=1}^{n_{g_1}} \text{sgn}(v_m^{g_1}) \frac{1 - \text{sgn}(\delta_m^{g_1})}{2} - \sum_{m=1}^{n_{g_2}} \text{sgn}(v_m^{g_2}) \frac{1 - \text{sgn}(\delta_m^{g_2})}{2} \\ & - \sum_{m=1}^{n_{g_3}} \text{sgn}(v_m^{g_3}) \frac{1 - \text{sgn}(\delta_m^{g_3})}{2} + \sum_{m=1}^{n_{i_2}} \text{sgn}(v_m^{i_2}) \frac{1 - \text{sgn}(\delta_m^{i_2})}{2} + \sum_{m=1}^{n_{i_3}} \text{sgn}(v_m^{i_3}) \frac{1 - \text{sgn}(\delta_m^{i_3})}{2} \end{aligned} \quad (\text{S186.1})$$

$$\begin{aligned}
\mathcal{W}_2^{\text{gapless}} = & \sum_{m=1}^{n_{a_2}} \text{sgn}(v_m^{a_2}) \frac{1 - \text{sgn}(\delta_m^{a_2})}{2} - \sum_{m=1}^{n_{e_1}} \text{sgn}(v_m^{e_1}) \frac{1 - \text{sgn}(\delta_m^{e_1})}{2} - \sum_{m=1}^{n_{e_2}} \text{sgn}(v_m^{e_2}) \frac{1 - \text{sgn}(\delta_m^{e_2})}{2} \\
& - \sum_{m=1}^{n_{f_1}} \text{sgn}(v_m^{f_1}) \frac{1 - \text{sgn}(\delta_m^{f_1})}{2} - \sum_{m=1}^{n_{g_1}} \text{sgn}(v_m^{g_1}) \frac{1 - \text{sgn}(\delta_m^{g_1})}{2} - \sum_{m=1}^{n_{g_2}} \text{sgn}(v_m^{g_2}) \frac{1 - \text{sgn}(\delta_m^{g_2})}{2} \\
& - \sum_{m=1}^{n_{g_3}} \text{sgn}(v_m^{g_3}) \frac{1 - \text{sgn}(\delta_m^{g_3})}{2} + \sum_{m=1}^{n_{i_1}} \text{sgn}(v_m^{i_1}) \frac{1 - \text{sgn}(\delta_m^{i_1})}{2} + \sum_{m=1}^{n_{i_3}} \text{sgn}(v_m^{i_3}) \frac{1 - \text{sgn}(\delta_m^{i_3})}{2}
\end{aligned} \tag{S186.2}$$

$$\begin{aligned}
\mathcal{W}_3^{\text{gapless}} = & \sum_{m=1}^{n_{b_1}} \text{sgn}(v_m^{b_1}) \frac{1 - \text{sgn}(\delta_m^{b_1})}{2} - 2 \sum_{m=1}^{n_{e_1}} \text{sgn}(v_m^{e_1}) \frac{1 - \text{sgn}(\delta_m^{e_1})}{2} - \sum_{m=1}^{n_{g_1}} \text{sgn}(v_m^{g_1}) \frac{1 - \text{sgn}(\delta_m^{g_1})}{2} \\
& - \sum_{m=1}^{n_{g_2}} \text{sgn}(v_m^{g_2}) \frac{1 - \text{sgn}(\delta_m^{g_2})}{2} - \sum_{m=1}^{n_{g_3}} \text{sgn}(v_m^{g_3}) \frac{1 - \text{sgn}(\delta_m^{g_3})}{2} + \sum_{m=1}^{n_{h_1}} \text{sgn}(v_m^{h_1}) \frac{1 - \text{sgn}(\delta_m^{h_1})}{2}
\end{aligned} \tag{S186.3}$$

$$\begin{aligned}
\mathcal{W}_4^{\text{gapless}} = & \sum_{m=1}^{n_{b_2}} \text{sgn}(v_m^{b_2}) \frac{1 - \text{sgn}(\delta_m^{b_2})}{2} - 2 \sum_{m=1}^{n_{e_2}} \text{sgn}(v_m^{e_2}) \frac{1 - \text{sgn}(\delta_m^{e_2})}{2} - \sum_{m=1}^{n_{g_1}} \text{sgn}(v_m^{g_1}) \frac{1 - \text{sgn}(\delta_m^{g_1})}{2} \\
& - \sum_{m=1}^{n_{g_2}} \text{sgn}(v_m^{g_2}) \frac{1 - \text{sgn}(\delta_m^{g_2})}{2} - \sum_{m=1}^{n_{g_3}} \text{sgn}(v_m^{g_3}) \frac{1 - \text{sgn}(\delta_m^{g_3})}{2} + \sum_{m=1}^{n_{h_1}} \text{sgn}(v_m^{h_1}) \frac{1 - \text{sgn}(\delta_m^{h_1})}{2}
\end{aligned} \tag{S186.4}$$

$$\begin{aligned}
\mathcal{W}_5^{\text{gapless}} = & \sum_{m=1}^{n_{c_1}} \text{sgn}(v_m^{c_1}) \frac{1 - \text{sgn}(\delta_m^{c_1})}{2} - \sum_{m=1}^{n_{f_1}} \text{sgn}(v_m^{f_1}) \frac{1 - \text{sgn}(\delta_m^{f_1})}{2} - \sum_{m=1}^{n_{h_1}} \text{sgn}(v_m^{h_1}) \frac{1 - \text{sgn}(\delta_m^{h_1})}{2} \\
& + \sum_{m=1}^{n_{i_2}} \text{sgn}(v_m^{i_2}) \frac{1 - \text{sgn}(\delta_m^{i_2})}{2} + \sum_{m=1}^{n_{i_3}} \text{sgn}(v_m^{i_3}) \frac{1 - \text{sgn}(\delta_m^{i_3})}{2}
\end{aligned} \tag{S186.5}$$

$$\begin{aligned}
\mathcal{W}_6^{\text{gapless}} = & \sum_{m=1}^{n_{c_2}} \text{sgn}(v_m^{c_2}) \frac{1 - \text{sgn}(\delta_m^{c_2})}{2} - \sum_{m=1}^{n_{f_1}} \text{sgn}(v_m^{f_1}) \frac{1 - \text{sgn}(\delta_m^{f_1})}{2} - \sum_{m=1}^{n_{h_1}} \text{sgn}(v_m^{h_1}) \frac{1 - \text{sgn}(\delta_m^{h_1})}{2} \\
& + \sum_{m=1}^{n_{i_1}} \text{sgn}(v_m^{i_1}) \frac{1 - \text{sgn}(\delta_m^{i_1})}{2} + \sum_{m=1}^{n_{i_3}} \text{sgn}(v_m^{i_3}) \frac{1 - \text{sgn}(\delta_m^{i_3})}{2}
\end{aligned} \tag{S186.6}$$

$$\begin{aligned}
\mathcal{W}_7^{\text{gapless}} = & \sum_{m=1}^{n_{d_1}} \text{sgn}(v_m^{d_1}) \frac{1 - \text{sgn}(\delta_m^{d_1})}{2} - \sum_{m=1}^{n_{e_1}} \text{sgn}(v_m^{e_1}) \frac{1 - \text{sgn}(\delta_m^{e_1})}{2} - \sum_{m=1}^{n_{e_2}} \text{sgn}(v_m^{e_2}) \frac{1 - \text{sgn}(\delta_m^{e_2})}{2} - \sum_{m=1}^{n_{f_1}} \text{sgn}(v_m^{f_1}) \frac{1 - \text{sgn}(\delta_m^{f_1})}{2}
\end{aligned} \tag{S186.7}$$

$$\mathcal{W}_1^{\text{gapped}} = \sum_{m=1}^{n_{e_1}} \text{sgn}(v_m^{e_1}) \frac{1 - \text{sgn}(\delta_m^{e_1})}{2} - \sum_{m=1}^{n_{e_2}} \text{sgn}(v_m^{e_2}) \frac{1 - \text{sgn}(\delta_m^{e_2})}{2} \tag{S186.8}$$

## S187. SPACE GROUP NO. 187

| line segment                                               | character of irrep (generators only)                                                                                                                         |
|------------------------------------------------------------|--------------------------------------------------------------------------------------------------------------------------------------------------------------|
| $a \left( \frac{t}{3}, \frac{t}{3}, 0 \right)$             | $\begin{array}{c} \{m_{001}   0 \ 0 \ 0\} \\ a_1 \quad -i \\ a_2 \quad i \end{array}$                                                                        |
| $b \left( 0, \frac{t}{2}, 0 \right)$                       | $\begin{array}{c} \{2_{010}   0 \ 0 \ 0\} \quad \{m_{001}   0 \ 0 \ 0\} \\ b_1 \quad 0 \quad 0 \end{array}$                                                  |
| $c \left( \frac{t}{3}, \frac{3-t}{6}, 0 \right)$           | $\begin{array}{c} \{m_{001}   0 \ 0 \ 0\} \\ c_1 \quad -i \\ c_2 \quad i \end{array}$                                                                        |
| $d \left( \frac{t}{3}, \frac{t}{3}, \frac{1}{2} \right)$   | $\begin{array}{c} \{m_{001}   0 \ 0 \ 0\} \\ d_1 \quad -i \\ d_2 \quad i \end{array}$                                                                        |
| $e \left( 0, \frac{t}{2}, \frac{1}{2} \right)$             | $\begin{array}{c} \{2_{010}   0 \ 0 \ 0\} \quad \{m_{001}   0 \ 0 \ 0\} \\ e_1 \quad 0 \quad 0 \end{array}$                                                  |
| $f \left( \frac{t}{3}, \frac{3-t}{6}, \frac{1}{2} \right)$ | $\begin{array}{c} \{m_{001}   0 \ 0 \ 0\} \\ f_1 \quad -i \\ f_2 \quad i \end{array}$                                                                        |
| $g \left( 0, 0, \frac{t}{2} \right)$                       | $\begin{array}{c} \{3_{001}   0 \ 0 \ 0\} \quad \{m_{100}   0 \ 0 \ 0\} \\ g_1 \quad -1 \quad -i \\ g_2 \quad -1 \quad i \\ g_3 \quad 1 \quad 0 \end{array}$ |
| $h \left( 0, \frac{1}{2}, \frac{t}{2} \right)$             | $\begin{array}{c} \{m_{100}   0 \ 0 \ 0\} \\ h_1 \quad -i \\ h_2 \quad i \end{array}$                                                                        |
| $i \left( \frac{1}{3}, \frac{1}{3}, \frac{t}{2} \right)$   | $\begin{array}{c} \{3_{001}   0 \ 0 \ 0\} \\ i_1 \quad -1 \\ i_2 \quad e^{-\frac{i\pi}{3}} \\ i_3 \quad e^{\frac{i\pi}{3}} \end{array}$                      |

$$\begin{aligned}
\mathcal{W}_1^{\text{gapless}} = & \sum_{m=1}^{n_{a_1}} \text{sgn}(v_m^{a_1}) \frac{1 - \text{sgn}(\delta_m^{a_1})}{2} + \sum_{m=1}^{n_{c_2}} \text{sgn}(v_m^{c_2}) \frac{1 - \text{sgn}(\delta_m^{c_2})}{2} - \sum_{m=1}^{n_{e_1}} \text{sgn}(v_m^{e_1}) \frac{1 - \text{sgn}(\delta_m^{e_1})}{2} - \sum_{m=1}^{n_{f_1}} \text{sgn}(v_m^{f_1}) \frac{1 - \text{sgn}(\delta_m^{f_1})}{2} \\
& - \sum_{m=1}^{n_{f_2}} \text{sgn}(v_m^{f_2}) \frac{1 - \text{sgn}(\delta_m^{f_2})}{2} - \sum_{m=1}^{n_{g_2}} \text{sgn}(v_m^{g_2}) \frac{1 - \text{sgn}(\delta_m^{g_2})}{2} - \sum_{m=1}^{n_{g_3}} \text{sgn}(v_m^{g_3}) \frac{1 - \text{sgn}(\delta_m^{g_3})}{2} \\
& - \sum_{m=1}^{n_{h_1}} \text{sgn}(v_m^{h_1}) \frac{1 - \text{sgn}(\delta_m^{h_1})}{2} + \sum_{m=1}^{n_{i_1}} \text{sgn}(v_m^{i_1}) \frac{1 - \text{sgn}(\delta_m^{i_1})}{2} + \sum_{m=1}^{n_{i_2}} \text{sgn}(v_m^{i_2}) \frac{1 - \text{sgn}(\delta_m^{i_2})}{2} + \sum_{m=1}^{n_{i_3}} \text{sgn}(v_m^{i_3}) \frac{1 - \text{sgn}(\delta_m^{i_3})}{2}
\end{aligned} \tag{S187.1}$$

$$\begin{aligned}
\mathcal{W}_2^{\text{gapless}} = & \sum_{m=1}^{n_{a_2}} \text{sgn}(v_m^{a_2}) \frac{1 - \text{sgn}(\delta_m^{a_2})}{2} - \sum_{m=1}^{n_{c_2}} \text{sgn}(v_m^{c_2}) \frac{1 - \text{sgn}(\delta_m^{c_2})}{2} - \sum_{m=1}^{n_{e_1}} \text{sgn}(v_m^{e_1}) \frac{1 - \text{sgn}(\delta_m^{e_1})}{2} \\
& - \sum_{m=1}^{n_{g_2}} \text{sgn}(v_m^{g_2}) \frac{1 - \text{sgn}(\delta_m^{g_2})}{2} - \sum_{m=1}^{n_{g_3}} \text{sgn}(v_m^{g_3}) \frac{1 - \text{sgn}(\delta_m^{g_3})}{2} + \sum_{m=1}^{n_{h_2}} \text{sgn}(v_m^{h_2}) \frac{1 - \text{sgn}(\delta_m^{h_2})}{2}
\end{aligned} \tag{S187.2}$$

$$\begin{aligned}
\mathcal{W}_3^{\text{gapless}} = & \sum_{m=1}^{n_{b_1}} \text{sgn}(v_m^{b_1}) \frac{1 - \text{sgn}(\delta_m^{b_1})}{2} - \sum_{m=1}^{n_{e_1}} \text{sgn}(v_m^{e_1}) \frac{1 - \text{sgn}(\delta_m^{e_1})}{2} - \sum_{m=1}^{n_{g_2}} \text{sgn}(v_m^{g_2}) \frac{1 - \text{sgn}(\delta_m^{g_2})}{2} \\
& - \sum_{m=1}^{n_{g_3}} \text{sgn}(v_m^{g_3}) \frac{1 - \text{sgn}(\delta_m^{g_3})}{2} + \sum_{m=1}^{n_{h_2}} \text{sgn}(v_m^{h_2}) \frac{1 - \text{sgn}(\delta_m^{h_2})}{2}
\end{aligned} \tag{S187.3}$$

$$\begin{aligned}
\mathcal{W}_4^{\text{gapless}} = & \sum_{m=1}^{n_{c_1}} \text{sgn}(v_m^{c_1}) \frac{1 - \text{sgn}(\delta_m^{c_1})}{2} + \sum_{m=1}^{n_{c_2}} \text{sgn}(v_m^{c_2}) \frac{1 - \text{sgn}(\delta_m^{c_2})}{2} - \sum_{m=1}^{n_{f_1}} \text{sgn}(v_m^{f_1}) \frac{1 - \text{sgn}(\delta_m^{f_1})}{2} \\
& - \sum_{m=1}^{n_{f_2}} \text{sgn}(v_m^{f_2}) \frac{1 - \text{sgn}(\delta_m^{f_2})}{2} - \sum_{m=1}^{n_{h_1}} \text{sgn}(v_m^{h_1}) \frac{1 - \text{sgn}(\delta_m^{h_1})}{2} - \sum_{m=1}^{n_{h_2}} \text{sgn}(v_m^{h_2}) \frac{1 - \text{sgn}(\delta_m^{h_2})}{2} \\
& + \sum_{m=1}^{n_{i_1}} \text{sgn}(v_m^{i_1}) \frac{1 - \text{sgn}(\delta_m^{i_1})}{2} + \sum_{m=1}^{n_{i_2}} \text{sgn}(v_m^{i_2}) \frac{1 - \text{sgn}(\delta_m^{i_2})}{2} + \sum_{m=1}^{n_{i_3}} \text{sgn}(v_m^{i_3}) \frac{1 - \text{sgn}(\delta_m^{i_3})}{2}
\end{aligned} \tag{S187.4}$$

$$\mathcal{W}_5^{\text{gapless}} = \sum_{m=1}^{n_{d_1}} \text{sgn}(v_m^{d_1}) \frac{1 - \text{sgn}(\delta_m^{d_1})}{2} - \sum_{m=1}^{n_{e_1}} \text{sgn}(v_m^{e_1}) \frac{1 - \text{sgn}(\delta_m^{e_1})}{2} - \sum_{m=1}^{n_{f_1}} \text{sgn}(v_m^{f_1}) \frac{1 - \text{sgn}(\delta_m^{f_1})}{2} \tag{S187.5}$$

$$\mathcal{W}_6^{\text{gapless}} = \sum_{m=1}^{n_{d_2}} \text{sgn}(v_m^{d_2}) \frac{1 - \text{sgn}(\delta_m^{d_2})}{2} - \sum_{m=1}^{n_{e_1}} \text{sgn}(v_m^{e_1}) \frac{1 - \text{sgn}(\delta_m^{e_1})}{2} - \sum_{m=1}^{n_{f_2}} \text{sgn}(v_m^{f_2}) \frac{1 - \text{sgn}(\delta_m^{f_2})}{2} \tag{S187.6}$$

$$\mathcal{W}_7^{\text{gapless}} = \sum_{m=1}^{n_{g_1}} \text{sgn}(v_m^{g_1}) \frac{1 - \text{sgn}(\delta_m^{g_1})}{2} - \sum_{m=1}^{n_{g_2}} \text{sgn}(v_m^{g_2}) \frac{1 - \text{sgn}(\delta_m^{g_2})}{2} - \sum_{m=1}^{n_{h_1}} \text{sgn}(v_m^{h_1}) \frac{1 - \text{sgn}(\delta_m^{h_1})}{2} + \sum_{m=1}^{n_{h_2}} \text{sgn}(v_m^{h_2}) \frac{1 - \text{sgn}(\delta_m^{h_2})}{2} \tag{S187.7}$$

$$\mathcal{W}_1^{\text{gapped}} = - \sum_{m=1}^{n_{h_1}} \text{sgn}(v_m^{h_1}) \frac{1 - \text{sgn}(\delta_m^{h_1})}{2} + \sum_{m=1}^{n_{h_2}} \text{sgn}(v_m^{h_2}) \frac{1 - \text{sgn}(\delta_m^{h_2})}{2} \tag{S187.8}$$

### S188. SPACE GROUP NO. 188

| line segment                                               | character of irrep (generators only)                                                                                                                                                    |
|------------------------------------------------------------|-----------------------------------------------------------------------------------------------------------------------------------------------------------------------------------------|
| $a \left( \frac{t}{3}, \frac{t}{3}, 0 \right)$             | $\{m_{001}   0 \ 0 \ \frac{1}{2}\}$<br>$a_1 \quad -i$<br>$a_2 \quad i$                                                                                                                  |
| $b \left( 0, \frac{t}{2}, 0 \right)$                       | $\{2_{010}   0 \ 0 \ 0\} \ \{m_{001}   0 \ 0 \ \frac{1}{2}\}$<br>$b_1 \quad 0 \quad 0$                                                                                                  |
| $c \left( \frac{t}{3}, \frac{3-t}{6}, 0 \right)$           | $\{m_{001}   0 \ 0 \ \frac{1}{2}\}$<br>$c_1 \quad -i$<br>$c_2 \quad i$                                                                                                                  |
| $d \left( \frac{t}{3}, \frac{t}{3}, \frac{1}{2} \right)$   | $\{m_{001}   0 \ 0 \ \frac{1}{2}\}$<br>$d_1 \quad i$<br>$d_2 \quad -i$                                                                                                                  |
| $e \left( 0, \frac{t}{2}, \frac{1}{2} \right)$             | $\{2_{010}   0 \ 0 \ 0\} \ \{m_{001}   0 \ 0 \ \frac{1}{2}\}$<br>$e_1 \quad -i \quad i$<br>$e_2 \quad -i \quad -i$<br>$e_3 \quad i \quad i$<br>$e_4 \quad i \quad -i$                   |
| $f \left( \frac{t}{3}, \frac{3-t}{6}, \frac{1}{2} \right)$ | $\{m_{001}   0 \ 0 \ \frac{1}{2}\}$<br>$f_1 \quad i$<br>$f_2 \quad -i$                                                                                                                  |
| $g \left( 0, 0, \frac{t}{2} \right)$                       | $\{3_{001}   0 \ 0 \ 0\} \ \{m_{100}   0 \ 0 \ \frac{1}{2}\}$<br>$g_1 \quad -1 \quad -ie^{-\frac{1}{2}i\pi t}$<br>$g_2 \quad -1 \quad ie^{-\frac{1}{2}i\pi t}$<br>$g_3 \quad 1 \quad 0$ |



|                                                   |                                                                                                                    |
|---------------------------------------------------|--------------------------------------------------------------------------------------------------------------------|
| $h \quad (0, \frac{1}{2}, \frac{t}{2})$           | $\{m_{100}   0 \ 0 \ \frac{1}{2}\}$<br>$h_1 \quad -ie^{-\frac{1}{2}i\pi t}$<br>$h_2 \quad ie^{-\frac{1}{2}i\pi t}$ |
| $i \quad (\frac{1}{3}, \frac{1}{3}, \frac{t}{2})$ | $\{3_{001}   0 \ 0 \ 0\}$<br>$i_1 \quad -1$<br>$i_2 \quad e^{-\frac{i\pi}{3}}$<br>$i_3 \quad e^{\frac{i\pi}{3}}$   |

$$\begin{aligned}
\mathcal{W}_1^{\text{gapless}} = & \sum_{m=1}^{n_{a_1}} \text{sgn}(v_m^{a_1}) \frac{1 - \text{sgn}(\delta_m^{a_1})}{2} + \sum_{m=1}^{n_{c_2}} \text{sgn}(v_m^{c_2}) \frac{1 - \text{sgn}(\delta_m^{c_2})}{2} - \sum_{m=1}^{n_{e_2}} \text{sgn}(v_m^{e_2}) \frac{1 - \text{sgn}(\delta_m^{e_2})}{2} \\
& + \sum_{m=1}^{n_{e_3}} \text{sgn}(v_m^{e_3}) \frac{1 - \text{sgn}(\delta_m^{e_3})}{2} - 2 \sum_{m=1}^{n_{e_4}} \text{sgn}(v_m^{e_4}) \frac{1 - \text{sgn}(\delta_m^{e_4})}{2} - 2 \sum_{m=1}^{n_{f_1}} \text{sgn}(v_m^{f_1}) \frac{1 - \text{sgn}(\delta_m^{f_1})}{2} \\
& - \sum_{m=1}^{n_{g_1}} \text{sgn}(v_m^{g_1}) \frac{1 - \text{sgn}(\delta_m^{g_1})}{2} - \sum_{m=1}^{n_{g_3}} \text{sgn}(v_m^{g_3}) \frac{1 - \text{sgn}(\delta_m^{g_3})}{2} - \sum_{m=1}^{n_{h_2}} \text{sgn}(v_m^{h_2}) \frac{1 - \text{sgn}(\delta_m^{h_2})}{2} \\
& + \sum_{m=1}^{n_{i_1}} \text{sgn}(v_m^{i_1}) \frac{1 - \text{sgn}(\delta_m^{i_1})}{2} + \sum_{m=1}^{n_{i_2}} \text{sgn}(v_m^{i_2}) \frac{1 - \text{sgn}(\delta_m^{i_2})}{2} + \sum_{m=1}^{n_{i_3}} \text{sgn}(v_m^{i_3}) \frac{1 - \text{sgn}(\delta_m^{i_3})}{2}
\end{aligned} \tag{S188.1}$$

$$\begin{aligned}
\mathcal{W}_2^{\text{gapless}} = & \sum_{m=1}^{n_{a_2}} \text{sgn}(v_m^{a_2}) \frac{1 - \text{sgn}(\delta_m^{a_2})}{2} - \sum_{m=1}^{n_{c_2}} \text{sgn}(v_m^{c_2}) \frac{1 - \text{sgn}(\delta_m^{c_2})}{2} - \sum_{m=1}^{n_{e_2}} \text{sgn}(v_m^{e_2}) \frac{1 - \text{sgn}(\delta_m^{e_2})}{2} \\
& + \sum_{m=1}^{n_{e_3}} \text{sgn}(v_m^{e_3}) \frac{1 - \text{sgn}(\delta_m^{e_3})}{2} - 2 \sum_{m=1}^{n_{e_4}} \text{sgn}(v_m^{e_4}) \frac{1 - \text{sgn}(\delta_m^{e_4})}{2} - \sum_{m=1}^{n_{g_1}} \text{sgn}(v_m^{g_1}) \frac{1 - \text{sgn}(\delta_m^{g_1})}{2} \\
& - \sum_{m=1}^{n_{g_3}} \text{sgn}(v_m^{g_3}) \frac{1 - \text{sgn}(\delta_m^{g_3})}{2} + \sum_{m=1}^{n_{h_1}} \text{sgn}(v_m^{h_1}) \frac{1 - \text{sgn}(\delta_m^{h_1})}{2}
\end{aligned} \tag{S188.2}$$

$$\begin{aligned}
\mathcal{W}_3^{\text{gapless}} = & \sum_{m=1}^{n_{b_1}} \text{sgn}(v_m^{b_1}) \frac{1 - \text{sgn}(\delta_m^{b_1})}{2} - \sum_{m=1}^{n_{e_2}} \text{sgn}(v_m^{e_2}) \frac{1 - \text{sgn}(\delta_m^{e_2})}{2} + \sum_{m=1}^{n_{e_3}} \text{sgn}(v_m^{e_3}) \frac{1 - \text{sgn}(\delta_m^{e_3})}{2} - 2 \sum_{m=1}^{n_{e_4}} \text{sgn}(v_m^{e_4}) \frac{1 - \text{sgn}(\delta_m^{e_4})}{2} \\
& - \sum_{m=1}^{n_{g_1}} \text{sgn}(v_m^{g_1}) \frac{1 - \text{sgn}(\delta_m^{g_1})}{2} - \sum_{m=1}^{n_{g_3}} \text{sgn}(v_m^{g_3}) \frac{1 - \text{sgn}(\delta_m^{g_3})}{2} + \sum_{m=1}^{n_{h_1}} \text{sgn}(v_m^{h_1}) \frac{1 - \text{sgn}(\delta_m^{h_1})}{2}
\end{aligned} \tag{S188.3}$$

$$\begin{aligned}
\mathcal{W}_4^{\text{gapless}} = & \sum_{m=1}^{n_{c_1}} \text{sgn}(v_m^{c_1}) \frac{1 - \text{sgn}(\delta_m^{c_1})}{2} + \sum_{m=1}^{n_{c_2}} \text{sgn}(v_m^{c_2}) \frac{1 - \text{sgn}(\delta_m^{c_2})}{2} - 2 \sum_{m=1}^{n_{f_1}} \text{sgn}(v_m^{f_1}) \frac{1 - \text{sgn}(\delta_m^{f_1})}{2} - \sum_{m=1}^{n_{h_1}} \text{sgn}(v_m^{h_1}) \frac{1 - \text{sgn}(\delta_m^{h_1})}{2} \\
& - \sum_{m=1}^{n_{h_2}} \text{sgn}(v_m^{h_2}) \frac{1 - \text{sgn}(\delta_m^{h_2})}{2} + \sum_{m=1}^{n_{i_1}} \text{sgn}(v_m^{i_1}) \frac{1 - \text{sgn}(\delta_m^{i_1})}{2} + \sum_{m=1}^{n_{i_2}} \text{sgn}(v_m^{i_2}) \frac{1 - \text{sgn}(\delta_m^{i_2})}{2} + \sum_{m=1}^{n_{i_3}} \text{sgn}(v_m^{i_3}) \frac{1 - \text{sgn}(\delta_m^{i_3})}{2}
\end{aligned} \tag{S188.4}$$

$$\begin{aligned}
\mathcal{W}_5^{\text{gapless}} = & \sum_{m=1}^{n_{d_1}} \text{sgn}(v_m^{d_1}) \frac{1 - \text{sgn}(\delta_m^{d_1})}{2} - \sum_{m=1}^{n_{e_2}} \text{sgn}(v_m^{e_2}) \frac{1 - \text{sgn}(\delta_m^{e_2})}{2} - \sum_{m=1}^{n_{e_4}} \text{sgn}(v_m^{e_4}) \frac{1 - \text{sgn}(\delta_m^{e_4})}{2} - \sum_{m=1}^{n_{f_1}} \text{sgn}(v_m^{f_1}) \frac{1 - \text{sgn}(\delta_m^{f_1})}{2}
\end{aligned} \tag{S188.5}$$

$$\mathcal{W}_6^{\text{gapless}} = \sum_{m=1}^{n_{e_1}} \text{sgn}(v_m^{e_1}) \frac{1 - \text{sgn}(\delta_m^{e_1})}{2} - \sum_{m=1}^{n_{e_2}} \text{sgn}(v_m^{e_2}) \frac{1 - \text{sgn}(\delta_m^{e_2})}{2} + \sum_{m=1}^{n_{e_3}} \text{sgn}(v_m^{e_3}) \frac{1 - \text{sgn}(\delta_m^{e_3})}{2} - \sum_{m=1}^{n_{e_4}} \text{sgn}(v_m^{e_4}) \frac{1 - \text{sgn}(\delta_m^{e_4})}{2} \quad (\text{S188.6})$$

$$\begin{aligned} \mathcal{W}_7^{\text{gapless}} = & 2 \sum_{m=1}^{n_{e_3}} \text{sgn}(v_m^{e_3}) \frac{1 - \text{sgn}(\delta_m^{e_3})}{2} - 2 \sum_{m=1}^{n_{e_4}} \text{sgn}(v_m^{e_4}) \frac{1 - \text{sgn}(\delta_m^{e_4})}{2} - \sum_{m=1}^{n_{g_1}} \text{sgn}(v_m^{g_1}) \frac{1 - \text{sgn}(\delta_m^{g_1})}{2} \\ & + \sum_{m=1}^{n_{g_2}} \text{sgn}(v_m^{g_2}) \frac{1 - \text{sgn}(\delta_m^{g_2})}{2} + \sum_{m=1}^{n_{h_1}} \text{sgn}(v_m^{h_1}) \frac{1 - \text{sgn}(\delta_m^{h_1})}{2} - \sum_{m=1}^{n_{h_2}} \text{sgn}(v_m^{h_2}) \frac{1 - \text{sgn}(\delta_m^{h_2})}{2} \end{aligned} \quad (\text{S188.7})$$

$$\begin{aligned} \mathcal{W}_1^{\text{gapped}} = & \sum_{m=1}^{n_{e_2}} \text{sgn}(v_m^{e_2}) \frac{1 - \text{sgn}(\delta_m^{e_2})}{2} + \sum_{m=1}^{n_{e_3}} \text{sgn}(v_m^{e_3}) \frac{1 - \text{sgn}(\delta_m^{e_3})}{2} - 2 \sum_{m=1}^{n_{e_4}} \text{sgn}(v_m^{e_4}) \frac{1 - \text{sgn}(\delta_m^{e_4})}{2} - \sum_{m=1}^{n_{g_1}} \text{sgn}(v_m^{g_1}) \frac{1 - \text{sgn}(\delta_m^{g_1})}{2} \\ & + \sum_{m=1}^{n_{g_2}} \text{sgn}(v_m^{g_2}) \frac{1 - \text{sgn}(\delta_m^{g_2})}{2} + \sum_{m=1}^{n_{h_1}} \text{sgn}(v_m^{h_1}) \frac{1 - \text{sgn}(\delta_m^{h_1})}{2} - \sum_{m=1}^{n_{h_2}} \text{sgn}(v_m^{h_2}) \frac{1 - \text{sgn}(\delta_m^{h_2})}{2} \end{aligned} \quad (\text{S188.8})$$

$$\mathcal{X}_1 = \sum_{m=1}^{n_{g_1}} \frac{1 - \text{sgn}(\delta_m^{g_1})}{2} + \sum_{m=1}^{n_{g_2}} \frac{1 - \text{sgn}(\delta_m^{g_2})}{2} \quad \text{mod } 2 \quad (\text{S188.9})$$

### S189. SPACE GROUP NO. 189

| line segment                                        | character of irrep (generators only)                                                                                                                                                                    |
|-----------------------------------------------------|---------------------------------------------------------------------------------------------------------------------------------------------------------------------------------------------------------|
| $a \quad (\frac{t}{3}, \frac{t}{3}, 0)$             | $a_1 \quad \begin{array}{c} \{2_{110}   0 \ 0 \ 0\} \\ 0 \end{array} \quad \begin{array}{c} \{m_{001}   0 \ 0 \ 0\} \\ 0 \end{array}$                                                                   |
| $b \quad (0, \frac{t}{2}, 0)$                       | $\begin{array}{c} b_1 \\ b_2 \end{array} \quad \begin{array}{c} \{m_{001}   0 \ 0 \ 0\} \\ -i \\ i \end{array}$                                                                                         |
| $c \quad (\frac{t}{3}, \frac{3-t}{6}, 0)$           | $c_1 \quad \begin{array}{c} \{2_{100}   0 \ 0 \ 0\} \\ 0 \end{array} \quad \begin{array}{c} \{m_{001}   0 \ 0 \ 0\} \\ 0 \end{array}$                                                                   |
| $d \quad (\frac{t}{3}, \frac{t}{3}, \frac{1}{2})$   | $d_1 \quad \begin{array}{c} \{2_{110}   0 \ 0 \ 0\} \\ 0 \end{array} \quad \begin{array}{c} \{m_{001}   0 \ 0 \ 0\} \\ 0 \end{array}$                                                                   |
| $e \quad (0, \frac{t}{2}, \frac{1}{2})$             | $\begin{array}{c} e_1 \\ e_2 \end{array} \quad \begin{array}{c} \{m_{001}   0 \ 0 \ 0\} \\ -i \\ i \end{array}$                                                                                         |
| $f \quad (\frac{t}{3}, \frac{3-t}{6}, \frac{1}{2})$ | $f_1 \quad \begin{array}{c} \{2_{100}   0 \ 0 \ 0\} \\ 0 \end{array} \quad \begin{array}{c} \{m_{001}   0 \ 0 \ 0\} \\ 0 \end{array}$                                                                   |
| $g \quad (0, 0, \frac{t}{2})$                       | $\begin{array}{c} g_1 \\ g_2 \\ g_3 \end{array} \quad \begin{array}{c} \{3_{001}   0 \ 0 \ 0\} \\ -1 \\ -1 \\ 1 \end{array} \quad \begin{array}{c} \{m_{210}   0 \ 0 \ 0\} \\ -i \\ i \\ 0 \end{array}$ |
| $h \quad (0, \frac{1}{2}, \frac{t}{2})$             | $\begin{array}{c} h_1 \\ h_2 \end{array} \quad \begin{array}{c} \{m_{010}   0 \ 0 \ 0\} \\ -i \\ i \end{array}$                                                                                         |
| $i \quad (\frac{1}{3}, \frac{1}{3}, \frac{t}{2})$   | $\begin{array}{c} i_1 \\ i_2 \\ i_3 \end{array} \quad \begin{array}{c} \{3_{001}   0 \ 0 \ 0\} \\ -1 \\ -1 \\ 1 \end{array} \quad \begin{array}{c} \{m_{210}   0 \ 0 \ 0\} \\ -i \\ i \\ 0 \end{array}$ |

$$\begin{aligned} \mathcal{W}_1^{\text{gapless}} = & \sum_{m=1}^{n_{a_1}} \text{sgn}(v_m^{a_1}) \frac{1 - \text{sgn}(\delta_m^{a_1})}{2} - \sum_{m=1}^{n_{e_2}} \text{sgn}(v_m^{e_2}) \frac{1 - \text{sgn}(\delta_m^{e_2})}{2} - \sum_{m=1}^{n_{f_1}} \text{sgn}(v_m^{f_1}) \frac{1 - \text{sgn}(\delta_m^{f_1})}{2} - \sum_{m=1}^{n_{g_2}} \text{sgn}(v_m^{g_2}) \frac{1 - \text{sgn}(\delta_m^{g_2})}{2} \\ & - \sum_{m=1}^{n_{g_3}} \text{sgn}(v_m^{g_3}) \frac{1 - \text{sgn}(\delta_m^{g_3})}{2} + \sum_{m=1}^{n_{i_2}} \text{sgn}(v_m^{i_2}) \frac{1 - \text{sgn}(\delta_m^{i_2})}{2} + \sum_{m=1}^{n_{i_3}} \text{sgn}(v_m^{i_3}) \frac{1 - \text{sgn}(\delta_m^{i_3})}{2} \end{aligned} \quad (\text{S189.1})$$

$$\begin{aligned} \mathcal{W}_2^{\text{gapless}} = & \sum_{m=1}^{n_{b_1}} \text{sgn}(v_m^{b_1}) \frac{1 - \text{sgn}(\delta_m^{b_1})}{2} - \sum_{m=1}^{n_{e_2}} \text{sgn}(v_m^{e_2}) \frac{1 - \text{sgn}(\delta_m^{e_2})}{2} - \sum_{m=1}^{n_{g_2}} \text{sgn}(v_m^{g_2}) \frac{1 - \text{sgn}(\delta_m^{g_2})}{2} - \sum_{m=1}^{n_{g_3}} \text{sgn}(v_m^{g_3}) \frac{1 - \text{sgn}(\delta_m^{g_3})}{2} \\ & + \sum_{m=1}^{n_{h_2}} \text{sgn}(v_m^{h_2}) \frac{1 - \text{sgn}(\delta_m^{h_2})}{2} - \sum_{m=1}^{n_{i_1}} \text{sgn}(v_m^{i_1}) \frac{1 - \text{sgn}(\delta_m^{i_1})}{2} + \sum_{m=1}^{n_{i_2}} \text{sgn}(v_m^{i_2}) \frac{1 - \text{sgn}(\delta_m^{i_2})}{2} \end{aligned} \quad (\text{S189.2})$$

$$\begin{aligned} \mathcal{W}_3^{\text{gapless}} = & \sum_{m=1}^{n_{b_2}} \text{sgn}(v_m^{b_2}) \frac{1 - \text{sgn}(\delta_m^{b_2})}{2} - \sum_{m=1}^{n_{e_2}} \text{sgn}(v_m^{e_2}) \frac{1 - \text{sgn}(\delta_m^{e_2})}{2} - \sum_{m=1}^{n_{g_2}} \text{sgn}(v_m^{g_2}) \frac{1 - \text{sgn}(\delta_m^{g_2})}{2} - \sum_{m=1}^{n_{g_3}} \text{sgn}(v_m^{g_3}) \frac{1 - \text{sgn}(\delta_m^{g_3})}{2} \\ & + \sum_{m=1}^{n_{h_2}} \text{sgn}(v_m^{h_2}) \frac{1 - \text{sgn}(\delta_m^{h_2})}{2} - \sum_{m=1}^{n_{i_1}} \text{sgn}(v_m^{i_1}) \frac{1 - \text{sgn}(\delta_m^{i_1})}{2} + \sum_{m=1}^{n_{i_2}} \text{sgn}(v_m^{i_2}) \frac{1 - \text{sgn}(\delta_m^{i_2})}{2} \end{aligned} \quad (\text{S189.3})$$

$$\begin{aligned} \mathcal{W}_4^{\text{gapless}} = & \sum_{m=1}^{n_{c_1}} \text{sgn}(v_m^{c_1}) \frac{1 - \text{sgn}(\delta_m^{c_1})}{2} - \sum_{m=1}^{n_{f_1}} \text{sgn}(v_m^{f_1}) \frac{1 - \text{sgn}(\delta_m^{f_1})}{2} - \sum_{m=1}^{n_{h_2}} \text{sgn}(v_m^{h_2}) \frac{1 - \text{sgn}(\delta_m^{h_2})}{2} \\ & + \sum_{m=1}^{n_{i_1}} \text{sgn}(v_m^{i_1}) \frac{1 - \text{sgn}(\delta_m^{i_1})}{2} + \sum_{m=1}^{n_{i_3}} \text{sgn}(v_m^{i_3}) \frac{1 - \text{sgn}(\delta_m^{i_3})}{2} \end{aligned} \quad (\text{S189.4})$$

$$\mathcal{W}_5^{\text{gapless}} = \sum_{m=1}^{n_{d_1}} \text{sgn}(v_m^{d_1}) \frac{1 - \text{sgn}(\delta_m^{d_1})}{2} - \sum_{m=1}^{n_{e_2}} \text{sgn}(v_m^{e_2}) \frac{1 - \text{sgn}(\delta_m^{e_2})}{2} - \sum_{m=1}^{n_{f_1}} \text{sgn}(v_m^{f_1}) \frac{1 - \text{sgn}(\delta_m^{f_1})}{2} \quad (\text{S189.5})$$

$$\mathcal{W}_6^{\text{gapless}} = \sum_{m=1}^{n_{e_1}} \text{sgn}(v_m^{e_1}) \frac{1 - \text{sgn}(\delta_m^{e_1})}{2} - \sum_{m=1}^{n_{e_2}} \text{sgn}(v_m^{e_2}) \frac{1 - \text{sgn}(\delta_m^{e_2})}{2} \quad (\text{S189.6})$$

$$\mathcal{W}_7^{\text{gapless}} = \sum_{m=1}^{n_{g_1}} \text{sgn}(v_m^{g_1}) \frac{1 - \text{sgn}(\delta_m^{g_1})}{2} - \sum_{m=1}^{n_{g_2}} \text{sgn}(v_m^{g_2}) \frac{1 - \text{sgn}(\delta_m^{g_2})}{2} - \sum_{m=1}^{n_{i_1}} \text{sgn}(v_m^{i_1}) \frac{1 - \text{sgn}(\delta_m^{i_1})}{2} + \sum_{m=1}^{n_{i_2}} \text{sgn}(v_m^{i_2}) \frac{1 - \text{sgn}(\delta_m^{i_2})}{2} \quad (\text{S189.7})$$

$$\mathcal{W}_8^{\text{gapless}} = \sum_{m=1}^{n_{h_1}} \text{sgn}(v_m^{h_1}) \frac{1 - \text{sgn}(\delta_m^{h_1})}{2} - \sum_{m=1}^{n_{h_2}} \text{sgn}(v_m^{h_2}) \frac{1 - \text{sgn}(\delta_m^{h_2})}{2} + \sum_{m=1}^{n_{i_1}} \text{sgn}(v_m^{i_1}) \frac{1 - \text{sgn}(\delta_m^{i_1})}{2} - \sum_{m=1}^{n_{i_2}} \text{sgn}(v_m^{i_2}) \frac{1 - \text{sgn}(\delta_m^{i_2})}{2} \quad (\text{S189.8})$$

$$\mathcal{W}_1^{\text{gapped}} = - \sum_{m=1}^{n_{i_1}} \text{sgn}(v_m^{i_1}) \frac{1 - \text{sgn}(\delta_m^{i_1})}{2} + \sum_{m=1}^{n_{i_2}} \text{sgn}(v_m^{i_2}) \frac{1 - \text{sgn}(\delta_m^{i_2})}{2} \quad (\text{S189.9})$$

## S190. SPACE GROUP NO. 190

| line segment                                               | character of irrep (generators only)                                                                                                                                                          |
|------------------------------------------------------------|-----------------------------------------------------------------------------------------------------------------------------------------------------------------------------------------------|
| $a \left( \frac{t}{3}, \frac{t}{3}, 0 \right)$             | $a_1 \begin{array}{cc} \{2_{110}   0 & 0 & 0\} & \{m_{001}   0 & 0 & \frac{1}{2}\} \\ 0 & & & 0 \end{array}$                                                                                  |
| $b \left( 0, \frac{t}{2}, 0 \right)$                       | $b_1 \begin{array}{cc} \{m_{001}   0 & 0 & \frac{1}{2}\} \\ -i & & \\ b_2 & i & \end{array}$                                                                                                  |
| $c \left( \frac{t}{3}, \frac{3-t}{6}, 0 \right)$           | $c_1 \begin{array}{cc} \{2_{100}   0 & 0 & 0\} & \{m_{001}   0 & 0 & \frac{1}{2}\} \\ 0 & & & 0 \end{array}$                                                                                  |
| $d \left( \frac{t}{3}, \frac{t}{3}, \frac{1}{2} \right)$   | $d_1 \begin{array}{cc} \{2_{110}   0 & 0 & 0\} & \{m_{001}   0 & 0 & \frac{1}{2}\} \\ -i & & & i \\ d_2 & -i & & -i \\ d_3 & i & & i \\ d_4 & i & & -i \end{array}$                           |
| $e \left( 0, \frac{t}{2}, \frac{1}{2} \right)$             | $e_1 \begin{array}{cc} \{m_{001}   0 & 0 & \frac{1}{2}\} \\ i & & \\ e_2 & -i & \end{array}$                                                                                                  |
| $f \left( \frac{t}{3}, \frac{3-t}{6}, \frac{1}{2} \right)$ | $f_1 \begin{array}{cc} \{2_{100}   0 & 0 & 0\} & \{m_{001}   0 & 0 & \frac{1}{2}\} \\ -i & & & i \\ f_2 & -i & & -i \\ f_3 & i & & i \\ f_4 & i & & -i \end{array}$                           |
| $g \left( 0, 0, \frac{t}{2} \right)$                       | $g_1 \begin{array}{cc} \{3_{001}   0 & 0 & 0\} & \{m_{210}   0 & 0 & \frac{1}{2}\} \\ -1 & & & -ie^{-\frac{1}{2}i\pi t} \\ g_2 & -1 & & ie^{-\frac{1}{2}i\pi t} \\ g_3 & 1 & & 0 \end{array}$ |
| $h \left( 0, \frac{1}{2}, \frac{t}{2} \right)$             | $h_1 \begin{array}{cc} \{m_{010}   0 & 0 & \frac{1}{2}\} \\ -ie^{-\frac{1}{2}i\pi t} & & \\ h_2 & ie^{-\frac{1}{2}i\pi t} & \end{array}$                                                      |
| $i \left( \frac{1}{3}, \frac{1}{3}, \frac{t}{2} \right)$   | $i_1 \begin{array}{cc} \{3_{001}   0 & 0 & 0\} & \{m_{210}   0 & 0 & \frac{1}{2}\} \\ -1 & & & -ie^{-\frac{1}{2}i\pi t} \\ i_2 & -1 & & ie^{-\frac{1}{2}i\pi t} \\ i_3 & 1 & & 0 \end{array}$ |

$$\begin{aligned}
\mathcal{W}_1^{\text{gapless}} = & \sum_{m=1}^{n_{a_1}} \text{sgn}(v_m^{a_1}) \frac{1 - \text{sgn}(\delta_m^{a_1})}{2} + \sum_{m=1}^{n_{d_3}} \text{sgn}(v_m^{d_3}) \frac{1 - \text{sgn}(\delta_m^{d_3})}{2} - \sum_{m=1}^{n_{d_4}} \text{sgn}(v_m^{d_4}) \frac{1 - \text{sgn}(\delta_m^{d_4})}{2} \\
& - \sum_{m=1}^{n_{e_1}} \text{sgn}(v_m^{e_1}) \frac{1 - \text{sgn}(\delta_m^{e_1})}{2} - \sum_{m=1}^{n_{f_2}} \text{sgn}(v_m^{f_2}) \frac{1 - \text{sgn}(\delta_m^{f_2})}{2} - 2 \sum_{m=1}^{n_{f_3}} \text{sgn}(v_m^{f_3}) \frac{1 - \text{sgn}(\delta_m^{f_3})}{2} \\
& + \sum_{m=1}^{n_{f_4}} \text{sgn}(v_m^{f_4}) \frac{1 - \text{sgn}(\delta_m^{f_4})}{2} - \sum_{m=1}^{n_{g_2}} \text{sgn}(v_m^{g_2}) \frac{1 - \text{sgn}(\delta_m^{g_2})}{2} - \sum_{m=1}^{n_{g_3}} \text{sgn}(v_m^{g_3}) \frac{1 - \text{sgn}(\delta_m^{g_3})}{2} \\
& - \sum_{m=1}^{n_{h_1}} \text{sgn}(v_m^{h_1}) \frac{1 - \text{sgn}(\delta_m^{h_1})}{2} + \sum_{m=1}^{n_{h_2}} \text{sgn}(v_m^{h_2}) \frac{1 - \text{sgn}(\delta_m^{h_2})}{2} - \sum_{m=1}^{n_{i_1}} \text{sgn}(v_m^{i_1}) \frac{1 - \text{sgn}(\delta_m^{i_1})}{2} \\
& + 2 \sum_{m=1}^{n_{i_2}} \text{sgn}(v_m^{i_2}) \frac{1 - \text{sgn}(\delta_m^{i_2})}{2} + \sum_{m=1}^{n_{i_3}} \text{sgn}(v_m^{i_3}) \frac{1 - \text{sgn}(\delta_m^{i_3})}{2}
\end{aligned} \tag{S190.1}$$

$$\begin{aligned}
\mathcal{W}_2^{\text{gapless}} = & \sum_{m=1}^{n_{b_1}} \text{sgn}(v_m^{b_1}) \frac{1 - \text{sgn}(\delta_m^{b_1})}{2} + \sum_{m=1}^{n_{d_3}} \text{sgn}(v_m^{d_3}) \frac{1 - \text{sgn}(\delta_m^{d_3})}{2} - \sum_{m=1}^{n_{d_4}} \text{sgn}(v_m^{d_4}) \frac{1 - \text{sgn}(\delta_m^{d_4})}{2} \\
& - \sum_{m=1}^{n_{e_1}} \text{sgn}(v_m^{e_1}) \frac{1 - \text{sgn}(\delta_m^{e_1})}{2} - \sum_{m=1}^{n_{f_3}} \text{sgn}(v_m^{f_3}) \frac{1 - \text{sgn}(\delta_m^{f_3})}{2} + \sum_{m=1}^{n_{f_4}} \text{sgn}(v_m^{f_4}) \frac{1 - \text{sgn}(\delta_m^{f_4})}{2} \\
& - \sum_{m=1}^{n_{g_2}} \text{sgn}(v_m^{g_2}) \frac{1 - \text{sgn}(\delta_m^{g_2})}{2} - \sum_{m=1}^{n_{g_3}} \text{sgn}(v_m^{g_3}) \frac{1 - \text{sgn}(\delta_m^{g_3})}{2} \\
& + \sum_{m=1}^{n_{h_2}} \text{sgn}(v_m^{h_2}) \frac{1 - \text{sgn}(\delta_m^{h_2})}{2} - \sum_{m=1}^{n_{i_1}} \text{sgn}(v_m^{i_1}) \frac{1 - \text{sgn}(\delta_m^{i_1})}{2} + \sum_{m=1}^{n_{i_2}} \text{sgn}(v_m^{i_2}) \frac{1 - \text{sgn}(\delta_m^{i_2})}{2}
\end{aligned} \tag{S190.2}$$

$$\begin{aligned}
\mathcal{W}_3^{\text{gapless}} = & \sum_{m=1}^{n_{b_2}} \text{sgn}(v_m^{b_2}) \frac{1 - \text{sgn}(\delta_m^{b_2})}{2} + \sum_{m=1}^{n_{d_3}} \text{sgn}(v_m^{d_3}) \frac{1 - \text{sgn}(\delta_m^{d_3})}{2} - \sum_{m=1}^{n_{d_4}} \text{sgn}(v_m^{d_4}) \frac{1 - \text{sgn}(\delta_m^{d_4})}{2} \\
& - \sum_{m=1}^{n_{e_1}} \text{sgn}(v_m^{e_1}) \frac{1 - \text{sgn}(\delta_m^{e_1})}{2} - \sum_{m=1}^{n_{f_3}} \text{sgn}(v_m^{f_3}) \frac{1 - \text{sgn}(\delta_m^{f_3})}{2} + \sum_{m=1}^{n_{f_4}} \text{sgn}(v_m^{f_4}) \frac{1 - \text{sgn}(\delta_m^{f_4})}{2} \\
& - \sum_{m=1}^{n_{g_2}} \text{sgn}(v_m^{g_2}) \frac{1 - \text{sgn}(\delta_m^{g_2})}{2} - \sum_{m=1}^{n_{g_3}} \text{sgn}(v_m^{g_3}) \frac{1 - \text{sgn}(\delta_m^{g_3})}{2} \\
& + \sum_{m=1}^{n_{h_2}} \text{sgn}(v_m^{h_2}) \frac{1 - \text{sgn}(\delta_m^{h_2})}{2} - \sum_{m=1}^{n_{i_1}} \text{sgn}(v_m^{i_1}) \frac{1 - \text{sgn}(\delta_m^{i_1})}{2} + \sum_{m=1}^{n_{i_2}} \text{sgn}(v_m^{i_2}) \frac{1 - \text{sgn}(\delta_m^{i_2})}{2}
\end{aligned} \tag{S190.3}$$

$$\begin{aligned}
\mathcal{W}_4^{\text{gapless}} = & \sum_{m=1}^{n_{c_1}} \text{sgn}(v_m^{c_1}) \frac{1 - \text{sgn}(\delta_m^{c_1})}{2} - \sum_{m=1}^{n_{f_2}} \text{sgn}(v_m^{f_2}) \frac{1 - \text{sgn}(\delta_m^{f_2})}{2} - \sum_{m=1}^{n_{f_3}} \text{sgn}(v_m^{f_3}) \frac{1 - \text{sgn}(\delta_m^{f_3})}{2} \\
& - \sum_{m=1}^{n_{h_1}} \text{sgn}(v_m^{h_1}) \frac{1 - \text{sgn}(\delta_m^{h_1})}{2} + \sum_{m=1}^{n_{i_2}} \text{sgn}(v_m^{i_2}) \frac{1 - \text{sgn}(\delta_m^{i_2})}{2} + \sum_{m=1}^{n_{i_3}} \text{sgn}(v_m^{i_3}) \frac{1 - \text{sgn}(\delta_m^{i_3})}{2}
\end{aligned} \tag{S190.4}$$

$$\begin{aligned}
\mathcal{W}_5^{\text{gapless}} = & \sum_{m=1}^{n_{d_1}} \text{sgn}(v_m^{d_1}) \frac{1 - \text{sgn}(\delta_m^{d_1})}{2} + \sum_{m=1}^{n_{d_3}} \text{sgn}(v_m^{d_3}) \frac{1 - \text{sgn}(\delta_m^{d_3})}{2} - \sum_{m=1}^{n_{e_1}} \text{sgn}(v_m^{e_1}) \frac{1 - \text{sgn}(\delta_m^{e_1})}{2} - \sum_{m=1}^{n_{f_2}} \text{sgn}(v_m^{f_2}) \frac{1 - \text{sgn}(\delta_m^{f_2})}{2} \\
& - 2 \sum_{m=1}^{n_{f_3}} \text{sgn}(v_m^{f_3}) \frac{1 - \text{sgn}(\delta_m^{f_3})}{2} + \sum_{m=1}^{n_{f_4}} \text{sgn}(v_m^{f_4}) \frac{1 - \text{sgn}(\delta_m^{f_4})}{2} - \sum_{m=1}^{n_{h_1}} \text{sgn}(v_m^{h_1}) \frac{1 - \text{sgn}(\delta_m^{h_1})}{2} \\
& + \sum_{m=1}^{n_{h_2}} \text{sgn}(v_m^{h_2}) \frac{1 - \text{sgn}(\delta_m^{h_2})}{2} - \sum_{m=1}^{n_{i_1}} \text{sgn}(v_m^{i_1}) \frac{1 - \text{sgn}(\delta_m^{i_1})}{2} + \sum_{m=1}^{n_{i_2}} \text{sgn}(v_m^{i_2}) \frac{1 - \text{sgn}(\delta_m^{i_2})}{2}
\end{aligned} \tag{S190.5}$$

$$\begin{aligned}
\mathcal{W}_6^{\text{gapless}} = & \sum_{m=1}^{n_{d_2}} \text{sgn}(v_m^{d_2}) \frac{1 - \text{sgn}(\delta_m^{d_2})}{2} + \sum_{m=1}^{n_{d_4}} \text{sgn}(v_m^{d_4}) \frac{1 - \text{sgn}(\delta_m^{d_4})}{2} - \sum_{m=1}^{n_{e_1}} \text{sgn}(v_m^{e_1}) \frac{1 - \text{sgn}(\delta_m^{e_1})}{2} \\
& - \sum_{m=1}^{n_{f_2}} \text{sgn}(v_m^{f_2}) \frac{1 - \text{sgn}(\delta_m^{f_2})}{2} - \sum_{m=1}^{n_{f_4}} \text{sgn}(v_m^{f_4}) \frac{1 - \text{sgn}(\delta_m^{f_4})}{2}
\end{aligned} \tag{S190.6}$$

$$\begin{aligned}
\mathcal{W}_7^{\text{gapless}} = & 2 \sum_{m=1}^{n_{d_3}} \text{sgn}(v_m^{d_3}) \frac{1 - \text{sgn}(\delta_m^{d_3})}{2} - 2 \sum_{m=1}^{n_{d_4}} \text{sgn}(v_m^{d_4}) \frac{1 - \text{sgn}(\delta_m^{d_4})}{2} - 2 \sum_{m=1}^{n_{f_3}} \text{sgn}(v_m^{f_3}) \frac{1 - \text{sgn}(\delta_m^{f_3})}{2} \\
& + 2 \sum_{m=1}^{n_{f_4}} \text{sgn}(v_m^{f_4}) \frac{1 - \text{sgn}(\delta_m^{f_4})}{2} + \sum_{m=1}^{n_{g_1}} \text{sgn}(v_m^{g_1}) \frac{1 - \text{sgn}(\delta_m^{g_1})}{2} - \sum_{m=1}^{n_{g_2}} \text{sgn}(v_m^{g_2}) \frac{1 - \text{sgn}(\delta_m^{g_2})}{2} \\
& - \sum_{m=1}^{n_{h_1}} \text{sgn}(v_m^{h_1}) \frac{1 - \text{sgn}(\delta_m^{h_1})}{2} + \sum_{m=1}^{n_{h_2}} \text{sgn}(v_m^{h_2}) \frac{1 - \text{sgn}(\delta_m^{h_2})}{2} - 2 \sum_{m=1}^{n_{i_1}} \text{sgn}(v_m^{i_1}) \frac{1 - \text{sgn}(\delta_m^{i_1})}{2} \\
& + 2 \sum_{m=1}^{n_{i_2}} \text{sgn}(v_m^{i_2}) \frac{1 - \text{sgn}(\delta_m^{i_2})}{2}
\end{aligned} \tag{S190.7}$$

$$\begin{aligned}
\mathcal{W}_8^{\text{gapless}} = & \sum_{m=1}^{n_{f_1}} \text{sgn}(v_m^{f_1}) \frac{1 - \text{sgn}(\delta_m^{f_1})}{2} - \sum_{m=1}^{n_{f_2}} \text{sgn}(v_m^{f_2}) \frac{1 - \text{sgn}(\delta_m^{f_2})}{2} - \sum_{m=1}^{n_{f_3}} \text{sgn}(v_m^{f_3}) \frac{1 - \text{sgn}(\delta_m^{f_3})}{2} \\
& + \sum_{m=1}^{n_{f_4}} \text{sgn}(v_m^{f_4}) \frac{1 - \text{sgn}(\delta_m^{f_4})}{2} - \sum_{m=1}^{n_{h_1}} \text{sgn}(v_m^{h_1}) \frac{1 - \text{sgn}(\delta_m^{h_1})}{2} \\
& + \sum_{m=1}^{n_{h_2}} \text{sgn}(v_m^{h_2}) \frac{1 - \text{sgn}(\delta_m^{h_2})}{2} - \sum_{m=1}^{n_{i_1}} \text{sgn}(v_m^{i_1}) \frac{1 - \text{sgn}(\delta_m^{i_1})}{2} + \sum_{m=1}^{n_{i_2}} \text{sgn}(v_m^{i_2}) \frac{1 - \text{sgn}(\delta_m^{i_2})}{2}
\end{aligned} \tag{S190.8}$$

$$\begin{aligned}
\mathcal{W}_1^{\text{gapped}} = & - \sum_{m=1}^{n_{d_3}} \text{sgn}(v_m^{d_3}) \frac{1 - \text{sgn}(\delta_m^{d_3})}{2} + 3 \sum_{m=1}^{n_{d_4}} \text{sgn}(v_m^{d_4}) \frac{1 - \text{sgn}(\delta_m^{d_4})}{2} - \sum_{m=1}^{n_{e_1}} \text{sgn}(v_m^{e_1}) \frac{1 - \text{sgn}(\delta_m^{e_1})}{2} \\
& - 2 \sum_{m=1}^{n_{f_2}} \text{sgn}(v_m^{f_2}) \frac{1 - \text{sgn}(\delta_m^{f_2})}{2} + \sum_{m=1}^{n_{f_3}} \text{sgn}(v_m^{f_3}) \frac{1 - \text{sgn}(\delta_m^{f_3})}{2} - \sum_{m=1}^{n_{f_4}} \text{sgn}(v_m^{f_4}) \frac{1 - \text{sgn}(\delta_m^{f_4})}{2} \\
& - \sum_{m=1}^{n_{g_1}} \text{sgn}(v_m^{g_1}) \frac{1 - \text{sgn}(\delta_m^{g_1})}{2} + \sum_{m=1}^{n_{g_2}} \text{sgn}(v_m^{g_2}) \frac{1 - \text{sgn}(\delta_m^{g_2})}{2} + \sum_{m=1}^{n_{i_1}} \text{sgn}(v_m^{i_1}) \frac{1 - \text{sgn}(\delta_m^{i_1})}{2} - \sum_{m=1}^{n_{i_2}} \text{sgn}(v_m^{i_2}) \frac{1 - \text{sgn}(\delta_m^{i_2})}{2}
\end{aligned} \tag{S190.9}$$

$$\mathcal{X}_1 = \sum_{m=1}^{n_{g_1}} \frac{1 - \text{sgn}(\delta_m^{g_1})}{2} + \sum_{m=1}^{n_{g_2}} \frac{1 - \text{sgn}(\delta_m^{g_2})}{2} \quad \text{mod } 2 \tag{S190.10}$$

### S191. SPACE GROUP NO. 191

| line segment                                        | character of irrep (generators only)                                                                                                    |
|-----------------------------------------------------|-----------------------------------------------------------------------------------------------------------------------------------------|
| $a \quad (\frac{t}{3}, \frac{t}{3}, 0)$             | $a_1 \quad \begin{Bmatrix} \{2_{110}   0 & 0 & 0\} \\ 0 \end{Bmatrix} \quad \begin{Bmatrix} \{m_{001}   0 & 0 & 0\} \\ 0 \end{Bmatrix}$ |
| $b \quad (0, \frac{t}{2}, 0)$                       | $b_1 \quad \begin{Bmatrix} \{2_{010}   0 & 0 & 0\} \\ 0 \end{Bmatrix} \quad \begin{Bmatrix} \{m_{001}   0 & 0 & 0\} \\ 0 \end{Bmatrix}$ |
| $c \quad (\frac{t}{3}, \frac{3-t}{6}, 0)$           | $c_1 \quad \begin{Bmatrix} \{2_{100}   0 & 0 & 0\} \\ 0 \end{Bmatrix} \quad \begin{Bmatrix} \{m_{001}   0 & 0 & 0\} \\ 0 \end{Bmatrix}$ |
| $d \quad (\frac{t}{3}, \frac{t}{3}, \frac{1}{2})$   | $d_1 \quad \begin{Bmatrix} \{2_{110}   0 & 0 & 0\} \\ 0 \end{Bmatrix} \quad \begin{Bmatrix} \{m_{001}   0 & 0 & 0\} \\ 0 \end{Bmatrix}$ |
| $e \quad (0, \frac{t}{2}, \frac{1}{2})$             | $e_1 \quad \begin{Bmatrix} \{2_{010}   0 & 0 & 0\} \\ 0 \end{Bmatrix} \quad \begin{Bmatrix} \{m_{001}   0 & 0 & 0\} \\ 0 \end{Bmatrix}$ |
| $f \quad (\frac{t}{3}, \frac{3-t}{6}, \frac{1}{2})$ | $f_1 \quad \begin{Bmatrix} \{2_{100}   0 & 0 & 0\} \\ 0 \end{Bmatrix} \quad \begin{Bmatrix} \{m_{001}   0 & 0 & 0\} \\ 0 \end{Bmatrix}$ |

|                                                   |                            |                            |
|---------------------------------------------------|----------------------------|----------------------------|
| $g \quad (0, 0, \frac{t}{2})$                     | $\{6_{001}   0 \ 0 \ 0 \}$ | $\{m_{100}   0 \ 0 \ 0 \}$ |
|                                                   | $g_1$                      | $-\sqrt{3}$                |
|                                                   | $g_2$                      | $0$                        |
|                                                   | $g_3$                      | $\sqrt{3}$                 |
| $h \quad (0, \frac{1}{2}, \frac{t}{2})$           | $\{2_{001}   0 \ 0 \ 0 \}$ | $\{m_{100}   0 \ 0 \ 0 \}$ |
|                                                   | $h_1$                      | $0$                        |
| $i \quad (\frac{1}{3}, \frac{1}{3}, \frac{t}{2})$ | $\{3_{001}   0 \ 0 \ 0 \}$ | $\{m_{210}   0 \ 0 \ 0 \}$ |
|                                                   | $i_1$                      | $-1$                       |
|                                                   | $i_2$                      | $-1$                       |
|                                                   | $i_3$                      | $1$                        |

$$\begin{aligned} \mathcal{W}_1^{\text{gapless}} = & \sum_{m=1}^{n_{a_1}} \text{sgn}(v_m^{a_1}) \frac{1 - \text{sgn}(\delta_m^{a_1})}{2} - \sum_{m=1}^{n_{e_1}} \text{sgn}(v_m^{e_1}) \frac{1 - \text{sgn}(\delta_m^{e_1})}{2} - \sum_{m=1}^{n_{f_1}} \text{sgn}(v_m^{f_1}) \frac{1 - \text{sgn}(\delta_m^{f_1})}{2} - \sum_{m=1}^{n_{g_1}} \text{sgn}(v_m^{g_1}) \frac{1 - \text{sgn}(\delta_m^{g_1})}{2} \\ & - \sum_{m=1}^{n_{g_2}} \text{sgn}(v_m^{g_2}) \frac{1 - \text{sgn}(\delta_m^{g_2})}{2} - \sum_{m=1}^{n_{g_3}} \text{sgn}(v_m^{g_3}) \frac{1 - \text{sgn}(\delta_m^{g_3})}{2} + \sum_{m=1}^{n_{i_1}} \text{sgn}(v_m^{i_1}) \frac{1 - \text{sgn}(\delta_m^{i_1})}{2} + \sum_{m=1}^{n_{i_3}} \text{sgn}(v_m^{i_3}) \frac{1 - \text{sgn}(\delta_m^{i_3})}{2} \end{aligned} \quad (\text{S191.1})$$

$$\begin{aligned} \mathcal{W}_2^{\text{gapless}} = & \sum_{m=1}^{n_{b_1}} \text{sgn}(v_m^{b_1}) \frac{1 - \text{sgn}(\delta_m^{b_1})}{2} - \sum_{m=1}^{n_{e_1}} \text{sgn}(v_m^{e_1}) \frac{1 - \text{sgn}(\delta_m^{e_1})}{2} - \sum_{m=1}^{n_{g_1}} \text{sgn}(v_m^{g_1}) \frac{1 - \text{sgn}(\delta_m^{g_1})}{2} \\ & - \sum_{m=1}^{n_{g_2}} \text{sgn}(v_m^{g_2}) \frac{1 - \text{sgn}(\delta_m^{g_2})}{2} - \sum_{m=1}^{n_{g_3}} \text{sgn}(v_m^{g_3}) \frac{1 - \text{sgn}(\delta_m^{g_3})}{2} + \sum_{m=1}^{n_{h_1}} \text{sgn}(v_m^{h_1}) \frac{1 - \text{sgn}(\delta_m^{h_1})}{2} \end{aligned} \quad (\text{S191.2})$$

$$\begin{aligned} \mathcal{W}_3^{\text{gapless}} = & \sum_{m=1}^{n_{c_1}} \text{sgn}(v_m^{c_1}) \frac{1 - \text{sgn}(\delta_m^{c_1})}{2} - \sum_{m=1}^{n_{f_1}} \text{sgn}(v_m^{f_1}) \frac{1 - \text{sgn}(\delta_m^{f_1})}{2} - \sum_{m=1}^{n_{h_1}} \text{sgn}(v_m^{h_1}) \frac{1 - \text{sgn}(\delta_m^{h_1})}{2} \\ & + \sum_{m=1}^{n_{i_1}} \text{sgn}(v_m^{i_1}) \frac{1 - \text{sgn}(\delta_m^{i_1})}{2} + \sum_{m=1}^{n_{i_3}} \text{sgn}(v_m^{i_3}) \frac{1 - \text{sgn}(\delta_m^{i_3})}{2} \end{aligned} \quad (\text{S191.3})$$

$$\mathcal{W}_4^{\text{gapless}} = \sum_{m=1}^{n_{d_1}} \text{sgn}(v_m^{d_1}) \frac{1 - \text{sgn}(\delta_m^{d_1})}{2} - \sum_{m=1}^{n_{e_1}} \text{sgn}(v_m^{e_1}) \frac{1 - \text{sgn}(\delta_m^{e_1})}{2} - \sum_{m=1}^{n_{f_1}} \text{sgn}(v_m^{f_1}) \frac{1 - \text{sgn}(\delta_m^{f_1})}{2} \quad (\text{S191.4})$$

## S192. SPACE GROUP NO. 192

| line segment                                      | character of irrep (generators only) |                            |
|---------------------------------------------------|--------------------------------------|----------------------------|
| $a \quad (\frac{t}{3}, \frac{t}{3}, 0)$           | $\{2_{110}   0 \ 0 \ \frac{1}{2} \}$ | $\{m_{001}   0 \ 0 \ 0 \}$ |
|                                                   | $a_1$                                | $0$                        |
| $b \quad (0, \frac{t}{2}, 0)$                     | $\{2_{010}   0 \ 0 \ \frac{1}{2} \}$ | $\{m_{001}   0 \ 0 \ 0 \}$ |
|                                                   | $b_1$                                | $0$                        |
| $c \quad (\frac{t}{3}, \frac{3-t}{6}, 0)$         | $\{2_{100}   0 \ 0 \ \frac{1}{2} \}$ | $\{m_{001}   0 \ 0 \ 0 \}$ |
|                                                   | $c_1$                                | $0$                        |
| $d \quad (\frac{t}{3}, \frac{t}{3}, \frac{1}{2})$ | $\{2_{110}   0 \ 0 \ \frac{1}{2} \}$ | $\{m_{001}   0 \ 0 \ 0 \}$ |
|                                                   | $d_1$                                | $i$                        |
|                                                   | $d_2$                                | $i$                        |
|                                                   | $d_3$                                | $-i$                       |
|                                                   | $d_4$                                | $-i$                       |

|                                                     |                                                                 |
|-----------------------------------------------------|-----------------------------------------------------------------|
| $e \quad (0, \frac{t}{2}, \frac{1}{2})$             | $\{2_{010}  0 \ 0 \ \frac{1}{2}\} \quad \{m_{001}  0 \ 0 \ 0\}$ |
|                                                     | $e_1 \quad i \quad -i$                                          |
|                                                     | $e_2 \quad i \quad i$                                           |
|                                                     | $e_3 \quad -i \quad -i$                                         |
|                                                     | $e_4 \quad -i \quad i$                                          |
| $f \quad (\frac{t}{3}, \frac{3-t}{6}, \frac{1}{2})$ | $\{2_{100}  0 \ 0 \ \frac{1}{2}\} \quad \{m_{001}  0 \ 0 \ 0\}$ |
|                                                     | $f_1 \quad i \quad -i$                                          |
|                                                     | $f_2 \quad i \quad i$                                           |
|                                                     | $f_3 \quad -i \quad -i$                                         |
|                                                     | $f_4 \quad -i \quad i$                                          |
| $g \quad (0, 0, \frac{t}{2})$                       | $\{6_{001}  0 \ 0 \ 0\} \quad \{m_{100}  0 \ 0 \ \frac{1}{2}\}$ |
|                                                     | $g_1 \quad -\sqrt{3} \quad 0$                                   |
|                                                     | $g_2 \quad 0 \quad 0$                                           |
|                                                     | $g_3 \quad \sqrt{3} \quad 0$                                    |
| $h \quad (0, \frac{1}{2}, \frac{t}{2})$             | $\{2_{001}  0 \ 0 \ 0\} \quad \{m_{100}  0 \ 0 \ \frac{1}{2}\}$ |
|                                                     | $h_1 \quad 0 \quad 0$                                           |
| $i \quad (\frac{1}{3}, \frac{1}{3}, \frac{t}{2})$   | $\{3_{001}  0 \ 0 \ 0\} \quad \{m_{210}  0 \ 0 \ \frac{1}{2}\}$ |
|                                                     | $i_1 \quad -1 \quad -ie^{-\frac{1}{2}i\pi t}$                   |
|                                                     | $i_2 \quad -1 \quad ie^{-\frac{1}{2}i\pi t}$                    |
|                                                     | $i_3 \quad 1 \quad 0$                                           |

$$\begin{aligned}
\mathcal{W}_1^{\text{gapless}} = & \sum_{m=1}^{n_{a_1}} \text{sgn}(v_m^{a_1}) \frac{1 - \text{sgn}(\delta_m^{a_1})}{2} - \sum_{m=1}^{n_{e_1}} \text{sgn}(v_m^{e_1}) \frac{1 - \text{sgn}(\delta_m^{e_1})}{2} - \sum_{m=1}^{n_{e_3}} \text{sgn}(v_m^{e_3}) \frac{1 - \text{sgn}(\delta_m^{e_3})}{2} - \sum_{m=1}^{n_{f_1}} \text{sgn}(v_m^{f_1}) \frac{1 - \text{sgn}(\delta_m^{f_1})}{2} \\
& - \sum_{m=1}^{n_{f_3}} \text{sgn}(v_m^{f_3}) \frac{1 - \text{sgn}(\delta_m^{f_3})}{2} - \sum_{m=1}^{n_{g_1}} \text{sgn}(v_m^{g_1}) \frac{1 - \text{sgn}(\delta_m^{g_1})}{2} - \sum_{m=1}^{n_{g_2}} \text{sgn}(v_m^{g_2}) \frac{1 - \text{sgn}(\delta_m^{g_2})}{2} \\
& - \sum_{m=1}^{n_{g_3}} \text{sgn}(v_m^{g_3}) \frac{1 - \text{sgn}(\delta_m^{g_3})}{2} + \sum_{m=1}^{n_{i_1}} \text{sgn}(v_m^{i_1}) \frac{1 - \text{sgn}(\delta_m^{i_1})}{2} + \sum_{m=1}^{n_{i_3}} \text{sgn}(v_m^{i_3}) \frac{1 - \text{sgn}(\delta_m^{i_3})}{2}
\end{aligned} \tag{S192.1}$$

$$\begin{aligned}
\mathcal{W}_2^{\text{gapless}} = & \sum_{m=1}^{n_{b_1}} \text{sgn}(v_m^{b_1}) \frac{1 - \text{sgn}(\delta_m^{b_1})}{2} - \sum_{m=1}^{n_{e_1}} \text{sgn}(v_m^{e_1}) \frac{1 - \text{sgn}(\delta_m^{e_1})}{2} - \sum_{m=1}^{n_{e_3}} \text{sgn}(v_m^{e_3}) \frac{1 - \text{sgn}(\delta_m^{e_3})}{2} - \sum_{m=1}^{n_{g_1}} \text{sgn}(v_m^{g_1}) \frac{1 - \text{sgn}(\delta_m^{g_1})}{2} \\
& - \sum_{m=1}^{n_{g_2}} \text{sgn}(v_m^{g_2}) \frac{1 - \text{sgn}(\delta_m^{g_2})}{2} - \sum_{m=1}^{n_{g_3}} \text{sgn}(v_m^{g_3}) \frac{1 - \text{sgn}(\delta_m^{g_3})}{2} + \sum_{m=1}^{n_{h_1}} \text{sgn}(v_m^{h_1}) \frac{1 - \text{sgn}(\delta_m^{h_1})}{2}
\end{aligned} \tag{S192.2}$$

$$\begin{aligned}
\mathcal{W}_3^{\text{gapless}} = & \sum_{m=1}^{n_{c_1}} \text{sgn}(v_m^{c_1}) \frac{1 - \text{sgn}(\delta_m^{c_1})}{2} - \sum_{m=1}^{n_{f_1}} \text{sgn}(v_m^{f_1}) \frac{1 - \text{sgn}(\delta_m^{f_1})}{2} - \sum_{m=1}^{n_{f_3}} \text{sgn}(v_m^{f_3}) \frac{1 - \text{sgn}(\delta_m^{f_3})}{2} \\
& - \sum_{m=1}^{n_{h_1}} \text{sgn}(v_m^{h_1}) \frac{1 - \text{sgn}(\delta_m^{h_1})}{2} + \sum_{m=1}^{n_{i_1}} \text{sgn}(v_m^{i_1}) \frac{1 - \text{sgn}(\delta_m^{i_1})}{2} + \sum_{m=1}^{n_{i_3}} \text{sgn}(v_m^{i_3}) \frac{1 - \text{sgn}(\delta_m^{i_3})}{2}
\end{aligned} \tag{S192.3}$$

$$\begin{aligned}
\mathcal{W}_4^{\text{gapless}} = & \sum_{m=1}^{n_{d_1}} \text{sgn}(v_m^{d_1}) \frac{1 - \text{sgn}(\delta_m^{d_1})}{2} + \sum_{m=1}^{n_{d_3}} \text{sgn}(v_m^{d_3}) \frac{1 - \text{sgn}(\delta_m^{d_3})}{2} - \sum_{m=1}^{n_{e_1}} \text{sgn}(v_m^{e_1}) \frac{1 - \text{sgn}(\delta_m^{e_1})}{2} \\
& - \sum_{m=1}^{n_{e_3}} \text{sgn}(v_m^{e_3}) \frac{1 - \text{sgn}(\delta_m^{e_3})}{2} - \sum_{m=1}^{n_{f_1}} \text{sgn}(v_m^{f_1}) \frac{1 - \text{sgn}(\delta_m^{f_1})}{2} - \sum_{m=1}^{n_{f_3}} \text{sgn}(v_m^{f_3}) \frac{1 - \text{sgn}(\delta_m^{f_3})}{2}
\end{aligned} \tag{S192.4}$$



$$\mathcal{W}_1^{\text{gapped}} = - \sum_{m=1}^{n_{e_1}} \text{sgn}(v_m^{e_1}) \frac{1 - \text{sgn}(\delta_m^{e_1})}{2} + \sum_{m=1}^{n_{e_3}} \text{sgn}(v_m^{e_3}) \frac{1 - \text{sgn}(\delta_m^{e_3})}{2} \quad (\text{S192.5})$$

$$\mathcal{W}_2^{\text{gapped}} = \sum_{m=1}^{n_{d_3}} \text{sgn}(v_m^{d_3}) \frac{1 - \text{sgn}(\delta_m^{d_3})}{2} - \sum_{m=1}^{n_{e_1}} \text{sgn}(v_m^{e_1}) \frac{1 - \text{sgn}(\delta_m^{e_1})}{2} - \sum_{m=1}^{n_{f_1}} \text{sgn}(v_m^{f_1}) \frac{1 - \text{sgn}(\delta_m^{f_1})}{2} \quad (\text{S192.6})$$

### S193. SPACE GROUP NO. 193

| line segment                                               | character of irrep (generators only)                                                                                                                                                                          |
|------------------------------------------------------------|---------------------------------------------------------------------------------------------------------------------------------------------------------------------------------------------------------------|
| $a \left( \frac{t}{3}, \frac{t}{3}, 0 \right)$             | $a_1 \begin{array}{cc} \{2_{110}   0 & 0 & \frac{1}{2}\} & \{m_{001}   0 & 0 & \frac{1}{2}\} \\ 0 & 0 \end{array}$                                                                                            |
| $b \left( 0, \frac{t}{2}, 0 \right)$                       | $b_1 \begin{array}{cc} \{2_{010}   0 & 0 & 0\} & \{m_{001}   0 & 0 & \frac{1}{2}\} \\ 0 & 0 \end{array}$                                                                                                      |
| $c \left( \frac{t}{3}, \frac{3-t}{6}, 0 \right)$           | $c_1 \begin{array}{cc} \{2_{100}   0 & 0 & \frac{1}{2}\} & \{m_{001}   0 & 0 & \frac{1}{2}\} \\ 0 & 0 \end{array}$                                                                                            |
| $d \left( \frac{t}{3}, \frac{t}{3}, \frac{1}{2} \right)$   | $d_1 \begin{array}{cc} \{2_{110}   0 & 0 & \frac{1}{2}\} & \{m_{001}   0 & 0 & \frac{1}{2}\} \\ 0 & 0 \end{array}$                                                                                            |
| $e \left( 0, \frac{t}{2}, \frac{1}{2} \right)$             | $\begin{array}{cc} \{2_{010}   0 & 0 & 0\} & \{m_{001}   0 & 0 & \frac{1}{2}\} \\ e_1 & -i & i \\ e_2 & -i & -i \\ e_3 & i & i \\ e_4 & i & -i \end{array}$                                                   |
| $f \left( \frac{t}{3}, \frac{3-t}{6}, \frac{1}{2} \right)$ | $f_1 \begin{array}{cc} \{2_{100}   0 & 0 & \frac{1}{2}\} & \{m_{001}   0 & 0 & \frac{1}{2}\} \\ 0 & 0 \end{array}$                                                                                            |
| $g \left( 0, 0, \frac{t}{2} \right)$                       | $\begin{array}{cc} \{6_{001}   0 & 0 & \frac{1}{2}\} & \{m_{100}   0 & 0 & \frac{1}{2}\} \\ g_1 & -\sqrt{3}e^{-\frac{1}{2}i\pi t} & 0 \\ g_2 & 0 & 0 \\ g_3 & \sqrt{3}e^{-\frac{1}{2}i\pi t} & 0 \end{array}$ |
| $h \left( 0, \frac{1}{2}, \frac{t}{2} \right)$             | $h_1 \begin{array}{cc} \{2_{001}   0 & 0 & \frac{1}{2}\} & \{m_{100}   0 & 0 & \frac{1}{2}\} \\ 0 & 0 \end{array}$                                                                                            |
| $i \left( \frac{1}{3}, \frac{1}{3}, \frac{t}{2} \right)$   | $\begin{array}{cc} \{3_{001}   0 & 0 & 0\} & \{m_{210}   0 & 0 & 0\} \\ i_1 & -1 & -i \\ i_2 & -1 & i \\ i_3 & 1 & 0 \end{array}$                                                                             |

$$\begin{aligned} \mathcal{W}_1^{\text{gapless}} = & \sum_{m=1}^{n_{a_1}} \text{sgn}(v_m^{a_1}) \frac{1 - \text{sgn}(\delta_m^{a_1})}{2} - 2 \sum_{m=1}^{n_{e_2}} \text{sgn}(v_m^{e_2}) \frac{1 - \text{sgn}(\delta_m^{e_2})}{2} - 2 \sum_{m=1}^{n_{f_1}} \text{sgn}(v_m^{f_1}) \frac{1 - \text{sgn}(\delta_m^{f_1})}{2} \\ & - \sum_{m=1}^{n_{g_1}} \text{sgn}(v_m^{g_1}) \frac{1 - \text{sgn}(\delta_m^{g_1})}{2} - \sum_{m=1}^{n_{g_2}} \text{sgn}(v_m^{g_2}) \frac{1 - \text{sgn}(\delta_m^{g_2})}{2} \\ & - \sum_{m=1}^{n_{g_3}} \text{sgn}(v_m^{g_3}) \frac{1 - \text{sgn}(\delta_m^{g_3})}{2} + \sum_{m=1}^{n_{i_1}} \text{sgn}(v_m^{i_1}) \frac{1 - \text{sgn}(\delta_m^{i_1})}{2} + \sum_{m=1}^{n_{i_3}} \text{sgn}(v_m^{i_3}) \frac{1 - \text{sgn}(\delta_m^{i_3})}{2} \end{aligned} \quad (\text{S193.1})$$

$$\begin{aligned} \mathcal{W}_2^{\text{gapless}} = & \sum_{m=1}^{n_{b_1}} \text{sgn}(v_m^{b_1}) \frac{1 - \text{sgn}(\delta_m^{b_1})}{2} - 2 \sum_{m=1}^{n_{e_2}} \text{sgn}(v_m^{e_2}) \frac{1 - \text{sgn}(\delta_m^{e_2})}{2} - \sum_{m=1}^{n_{g_1}} \text{sgn}(v_m^{g_1}) \frac{1 - \text{sgn}(\delta_m^{g_1})}{2} \\ & - \sum_{m=1}^{n_{g_2}} \text{sgn}(v_m^{g_2}) \frac{1 - \text{sgn}(\delta_m^{g_2})}{2} - \sum_{m=1}^{n_{g_3}} \text{sgn}(v_m^{g_3}) \frac{1 - \text{sgn}(\delta_m^{g_3})}{2} + \sum_{m=1}^{n_{h_1}} \text{sgn}(v_m^{h_1}) \frac{1 - \text{sgn}(\delta_m^{h_1})}{2} \end{aligned} \quad (\text{S193.2})$$

$$\begin{aligned} \mathcal{W}_3^{\text{gapless}} = & \sum_{m=1}^{n_{c_1}} \text{sgn}(v_m^{c_1}) \frac{1 - \text{sgn}(\delta_m^{c_1})}{2} - 2 \sum_{m=1}^{n_{f_1}} \text{sgn}(v_m^{f_1}) \frac{1 - \text{sgn}(\delta_m^{f_1})}{2} - \sum_{m=1}^{n_{h_1}} \text{sgn}(v_m^{h_1}) \frac{1 - \text{sgn}(\delta_m^{h_1})}{2} \\ & + \sum_{m=1}^{n_{i_1}} \text{sgn}(v_m^{i_1}) \frac{1 - \text{sgn}(\delta_m^{i_1})}{2} + \sum_{m=1}^{n_{i_3}} \text{sgn}(v_m^{i_3}) \frac{1 - \text{sgn}(\delta_m^{i_3})}{2} \end{aligned} \quad (\text{S193.3})$$

$$\mathcal{W}_4^{\text{gapless}} = \sum_{m=1}^{n_{d_1}} \text{sgn}(v_m^{d_1}) \frac{1 - \text{sgn}(\delta_m^{d_1})}{2} - \sum_{m=1}^{n_{e_2}} \text{sgn}(v_m^{e_2}) \frac{1 - \text{sgn}(\delta_m^{e_2})}{2} - \sum_{m=1}^{n_{f_1}} \text{sgn}(v_m^{f_1}) \frac{1 - \text{sgn}(\delta_m^{f_1})}{2} \quad (\text{S193.4})$$

$$\mathcal{W}_5^{\text{gapless}} = \sum_{m=1}^{n_{e_1}} \text{sgn}(v_m^{e_1}) \frac{1 - \text{sgn}(\delta_m^{e_1})}{2} - \sum_{m=1}^{n_{e_2}} \text{sgn}(v_m^{e_2}) \frac{1 - \text{sgn}(\delta_m^{e_2})}{2} \quad (\text{S193.5})$$

#### S194. SPACE GROUP NO. 194

| line segment                                        | character of irrep (generators only) |                                                                                                                                                 |
|-----------------------------------------------------|--------------------------------------|-------------------------------------------------------------------------------------------------------------------------------------------------|
| $a \quad (\frac{t}{3}, \frac{t}{3}, 0)$             | $a_1$                                | $\{2_{110}   0 \ 0 \ 0\} \quad \{m_{001}   0 \ 0 \ \frac{1}{2}\}$<br>0                                                                          |
| $b \quad (0, \frac{t}{2}, 0)$                       | $b_1$                                | $\{2_{010}   0 \ 0 \ \frac{1}{2}\} \quad \{m_{001}   0 \ 0 \ \frac{1}{2}\}$<br>0                                                                |
| $c \quad (\frac{t}{3}, \frac{3-t}{6}, 0)$           | $c_1$                                | $\{2_{100}   0 \ 0 \ 0\} \quad \{m_{001}   0 \ 0 \ \frac{1}{2}\}$<br>0                                                                          |
| $d \quad (\frac{t}{3}, \frac{t}{3}, \frac{1}{2})$   | $d_1$<br>$d_2$<br>$d_3$<br>$d_4$     | $\{2_{110}   0 \ 0 \ 0\} \quad \{m_{001}   0 \ 0 \ \frac{1}{2}\}$<br>-i<br>-i<br>i<br>i                                                         |
| $e \quad (0, \frac{t}{2}, \frac{1}{2})$             | $e_1$                                | $\{2_{010}   0 \ 0 \ \frac{1}{2}\} \quad \{m_{001}   0 \ 0 \ \frac{1}{2}\}$<br>0                                                                |
| $f \quad (\frac{t}{3}, \frac{3-t}{6}, \frac{1}{2})$ | $f_1$<br>$f_2$<br>$f_3$<br>$f_4$     | $\{2_{100}   0 \ 0 \ 0\} \quad \{m_{001}   0 \ 0 \ \frac{1}{2}\}$<br>-i<br>-i<br>i<br>i                                                         |
| $g \quad (0, 0, \frac{t}{2})$                       | $g_1$<br>$g_2$<br>$g_3$              | $\{6_{001}   0 \ 0 \ \frac{1}{2}\} \quad \{m_{100}   0 \ 0 \ 0\}$<br>$-\sqrt{3}e^{-\frac{1}{2}i\pi t}$<br>0<br>$\sqrt{3}e^{-\frac{1}{2}i\pi t}$ |
| $h \quad (0, \frac{1}{2}, \frac{t}{2})$             | $h_1$                                | $\{2_{001}   0 \ 0 \ \frac{1}{2}\} \quad \{m_{100}   0 \ 0 \ 0\}$<br>0                                                                          |
| $i \quad (\frac{1}{3}, \frac{1}{3}, \frac{t}{2})$   | $i_1$<br>$i_2$<br>$i_3$              | $\{3_{001}   0 \ 0 \ 0\} \quad \{m_{210}   0 \ 0 \ \frac{1}{2}\}$<br>-1<br>-1<br>1                                                              |

$$\begin{aligned}
\mathcal{W}_1^{\text{gapless}} = & \sum_{m=1}^{n_{a_1}} \text{sgn}(v_m^{a_1}) \frac{1 - \text{sgn}(\delta_m^{a_1})}{2} - 2 \sum_{m=1}^{n_{e_1}} \text{sgn}(v_m^{e_1}) \frac{1 - \text{sgn}(\delta_m^{e_1})}{2} - \sum_{m=1}^{n_{f_1}} \text{sgn}(v_m^{f_1}) \frac{1 - \text{sgn}(\delta_m^{f_1})}{2} \\
& - \sum_{m=1}^{n_{f_2}} \text{sgn}(v_m^{f_2}) \frac{1 - \text{sgn}(\delta_m^{f_2})}{2} - \sum_{m=1}^{n_{g_1}} \text{sgn}(v_m^{g_1}) \frac{1 - \text{sgn}(\delta_m^{g_1})}{2} - \sum_{m=1}^{n_{g_2}} \text{sgn}(v_m^{g_2}) \frac{1 - \text{sgn}(\delta_m^{g_2})}{2} \\
& - \sum_{m=1}^{n_{g_3}} \text{sgn}(v_m^{g_3}) \frac{1 - \text{sgn}(\delta_m^{g_3})}{2} + \sum_{m=1}^{n_{i_1}} \text{sgn}(v_m^{i_1}) \frac{1 - \text{sgn}(\delta_m^{i_1})}{2} + \sum_{m=1}^{n_{i_3}} \text{sgn}(v_m^{i_3}) \frac{1 - \text{sgn}(\delta_m^{i_3})}{2}
\end{aligned} \tag{S194.1}$$

$$\begin{aligned}
\mathcal{W}_2^{\text{gapless}} = & \sum_{m=1}^{n_{b_1}} \text{sgn}(v_m^{b_1}) \frac{1 - \text{sgn}(\delta_m^{b_1})}{2} - 2 \sum_{m=1}^{n_{e_1}} \text{sgn}(v_m^{e_1}) \frac{1 - \text{sgn}(\delta_m^{e_1})}{2} - \sum_{m=1}^{n_{g_1}} \text{sgn}(v_m^{g_1}) \frac{1 - \text{sgn}(\delta_m^{g_1})}{2} \\
& - \sum_{m=1}^{n_{g_2}} \text{sgn}(v_m^{g_2}) \frac{1 - \text{sgn}(\delta_m^{g_2})}{2} - \sum_{m=1}^{n_{g_3}} \text{sgn}(v_m^{g_3}) \frac{1 - \text{sgn}(\delta_m^{g_3})}{2} + \sum_{m=1}^{n_{h_1}} \text{sgn}(v_m^{h_1}) \frac{1 - \text{sgn}(\delta_m^{h_1})}{2}
\end{aligned} \tag{S194.2}$$

$$\begin{aligned}
\mathcal{W}_3^{\text{gapless}} = & \sum_{m=1}^{n_{c_1}} \text{sgn}(v_m^{c_1}) \frac{1 - \text{sgn}(\delta_m^{c_1})}{2} - \sum_{m=1}^{n_{f_1}} \text{sgn}(v_m^{f_1}) \frac{1 - \text{sgn}(\delta_m^{f_1})}{2} - \sum_{m=1}^{n_{f_2}} \text{sgn}(v_m^{f_2}) \frac{1 - \text{sgn}(\delta_m^{f_2})}{2} \\
& - \sum_{m=1}^{n_{h_1}} \text{sgn}(v_m^{h_1}) \frac{1 - \text{sgn}(\delta_m^{h_1})}{2} + \sum_{m=1}^{n_{i_1}} \text{sgn}(v_m^{i_1}) \frac{1 - \text{sgn}(\delta_m^{i_1})}{2} + \sum_{m=1}^{n_{i_3}} \text{sgn}(v_m^{i_3}) \frac{1 - \text{sgn}(\delta_m^{i_3})}{2}
\end{aligned} \tag{S194.3}$$

$$\mathcal{W}_4^{\text{gapless}} = \sum_{m=1}^{n_{d_1}} \text{sgn}(v_m^{d_1}) \frac{1 - \text{sgn}(\delta_m^{d_1})}{2} - \sum_{m=1}^{n_{e_1}} \text{sgn}(v_m^{e_1}) \frac{1 - \text{sgn}(\delta_m^{e_1})}{2} - \sum_{m=1}^{n_{f_1}} \text{sgn}(v_m^{f_1}) \frac{1 - \text{sgn}(\delta_m^{f_1})}{2} \tag{S194.4}$$

$$\mathcal{W}_5^{\text{gapless}} = \sum_{m=1}^{n_{d_2}} \text{sgn}(v_m^{d_2}) \frac{1 - \text{sgn}(\delta_m^{d_2})}{2} - \sum_{m=1}^{n_{e_1}} \text{sgn}(v_m^{e_1}) \frac{1 - \text{sgn}(\delta_m^{e_1})}{2} - \sum_{m=1}^{n_{f_2}} \text{sgn}(v_m^{f_2}) \frac{1 - \text{sgn}(\delta_m^{f_2})}{2} \tag{S194.5}$$

### S195. SPACE GROUP NO. 195

| line segment                                                       | character of irrep (generators only)                                                                                                  |
|--------------------------------------------------------------------|---------------------------------------------------------------------------------------------------------------------------------------|
| $a \quad \left(\frac{1}{2}, \frac{t}{2}, \frac{t}{2}\right)$       | $\begin{array}{c} \{1 0 \ 0 \ 0\} \\ a_1 \quad 1 \end{array}$                                                                         |
| $b \quad \left(\frac{1-t}{2}, \frac{1-t}{2}, \frac{1-t}{2}\right)$ | $\begin{array}{c} \{3_{111} 0 \ 0 \ 0\} \\ b_1 \quad -1 \\ b_2 \quad e^{-\frac{i\pi}{3}} \\ b_3 \quad e^{\frac{i\pi}{3}} \end{array}$ |
| $c \quad \left(\frac{t}{2}, 0, 0\right)$                           | $\begin{array}{c} \{2_{100} 0 \ 0 \ 0\} \\ c_1 \quad -i \\ c_2 \quad i \end{array}$                                                   |
| $d \quad \left(\frac{1}{2}, \frac{1}{2}, \frac{t}{2}\right)$       | $\begin{array}{c} \{2_{001} 0 \ 0 \ 0\} \\ d_1 \quad -i \\ d_2 \quad i \end{array}$                                                   |

|                                           |                                                               |
|-------------------------------------------|---------------------------------------------------------------|
| $e \quad (\frac{1}{2}, \frac{t}{2}, 0)$   | $\{2_{010}   0 \ 0 \ 0 \}$<br>$e_1 \quad -i$<br>$e_2 \quad i$ |
| $f \quad (\frac{1-t}{2}, \frac{1}{2}, 0)$ | $\{2_{100}   0 \ 0 \ 0 \}$<br>$f_1 \quad -i$<br>$f_2 \quad i$ |

$$\begin{aligned} \mathcal{W}_1^{\text{gapless}} = & \sum_{m=1}^{n_{a_1}} \text{sgn}(v_m^{a_1}) \frac{1 - \text{sgn}(\delta_m^{a_1})}{2} - \sum_{m=1}^{n_{d_1}} \text{sgn}(v_m^{d_1}) \frac{1 - \text{sgn}(\delta_m^{d_1})}{2} - \sum_{m=1}^{n_{d_2}} \text{sgn}(v_m^{d_2}) \frac{1 - \text{sgn}(\delta_m^{d_2})}{2} \\ & + \sum_{m=1}^{n_{f_1}} \text{sgn}(v_m^{f_1}) \frac{1 - \text{sgn}(\delta_m^{f_1})}{2} + \sum_{m=1}^{n_{f_2}} \text{sgn}(v_m^{f_2}) \frac{1 - \text{sgn}(\delta_m^{f_2})}{2} \end{aligned} \quad (\text{S195.1})$$

$$\begin{aligned} \mathcal{W}_2^{\text{gapless}} = & \sum_{m=1}^{n_{b_1}} \text{sgn}(v_m^{b_1}) \frac{1 - \text{sgn}(\delta_m^{b_1})}{2} + \sum_{m=1}^{n_{b_2}} \text{sgn}(v_m^{b_2}) \frac{1 - \text{sgn}(\delta_m^{b_2})}{2} + \sum_{m=1}^{n_{b_3}} \text{sgn}(v_m^{b_3}) \frac{1 - \text{sgn}(\delta_m^{b_3})}{2} \\ & + \sum_{m=1}^{n_{c_1}} \text{sgn}(v_m^{c_1}) \frac{1 - \text{sgn}(\delta_m^{c_1})}{2} + \sum_{m=1}^{n_{c_2}} \text{sgn}(v_m^{c_2}) \frac{1 - \text{sgn}(\delta_m^{c_2})}{2} + \sum_{m=1}^{n_{d_1}} \text{sgn}(v_m^{d_1}) \frac{1 - \text{sgn}(\delta_m^{d_1})}{2} \\ & + \sum_{m=1}^{n_{d_2}} \text{sgn}(v_m^{d_2}) \frac{1 - \text{sgn}(\delta_m^{d_2})}{2} - \sum_{m=1}^{n_{f_1}} \text{sgn}(v_m^{f_1}) \frac{1 - \text{sgn}(\delta_m^{f_1})}{2} - \sum_{m=1}^{n_{f_2}} \text{sgn}(v_m^{f_2}) \frac{1 - \text{sgn}(\delta_m^{f_2})}{2} \end{aligned} \quad (\text{S195.2})$$

$$\mathcal{W}_3^{\text{gapless}} = \sum_{m=1}^{n_{e_1}} \text{sgn}(v_m^{e_1}) \frac{1 - \text{sgn}(\delta_m^{e_1})}{2} + \sum_{m=1}^{n_{e_2}} \text{sgn}(v_m^{e_2}) \frac{1 - \text{sgn}(\delta_m^{e_2})}{2} + \sum_{m=1}^{n_{f_1}} \text{sgn}(v_m^{f_1}) \frac{1 - \text{sgn}(\delta_m^{f_1})}{2} + \sum_{m=1}^{n_{f_2}} \text{sgn}(v_m^{f_2}) \frac{1 - \text{sgn}(\delta_m^{f_2})}{2} \quad (\text{S195.3})$$

$$\mathcal{W}_1^{\text{gapped}} = - \sum_{m=1}^{n_{d_1}} \text{sgn}(v_m^{d_1}) \frac{1 - \text{sgn}(\delta_m^{d_1})}{2} + \sum_{m=1}^{n_{d_2}} \text{sgn}(v_m^{d_2}) \frac{1 - \text{sgn}(\delta_m^{d_2})}{2} \quad (\text{S195.4})$$

$$\mathcal{W}_2^{\text{gapped}} = \sum_{m=1}^{n_{b_2}} \text{sgn}(v_m^{b_2}) \frac{1 - \text{sgn}(\delta_m^{b_2})}{2} - \sum_{m=1}^{n_{b_3}} \text{sgn}(v_m^{b_3}) \frac{1 - \text{sgn}(\delta_m^{b_3})}{2} \quad (\text{S195.5})$$

$$\mathcal{W}_3^{\text{gapped}} = - \sum_{m=1}^{n_{c_1}} \text{sgn}(v_m^{c_1}) \frac{1 - \text{sgn}(\delta_m^{c_1})}{2} + \sum_{m=1}^{n_{c_2}} \text{sgn}(v_m^{c_2}) \frac{1 - \text{sgn}(\delta_m^{c_2})}{2} \quad (\text{S195.6})$$

$$\mathcal{W}_4^{\text{gapped}} = \sum_{m=1}^{n_{e_2}} \text{sgn}(v_m^{e_2}) \frac{1 - \text{sgn}(\delta_m^{e_2})}{2} + \sum_{m=1}^{n_{f_1}} \text{sgn}(v_m^{f_1}) \frac{1 - \text{sgn}(\delta_m^{f_1})}{2} \quad (\text{S195.7})$$

$$\mathcal{W}_5^{\text{gapped}} = \sum_{m=1}^{n_{e_2}} \text{sgn}(v_m^{e_2}) \frac{1 - \text{sgn}(\delta_m^{e_2})}{2} + \sum_{m=1}^{n_{f_2}} \text{sgn}(v_m^{f_2}) \frac{1 - \text{sgn}(\delta_m^{f_2})}{2} \quad (\text{S195.8})$$

**S196. SPACE GROUP NO. 196**

| line segment                                      | character of irrep (generators only)                                                                             |
|---------------------------------------------------|------------------------------------------------------------------------------------------------------------------|
| $a \ (0, t, 0)$                                   | $\{2_{010}   0 \ 0 \ 0\}$<br>$a_1 \quad -i$<br>$a_2 \quad i$                                                     |
| $b \ (t, 1, 0)$                                   | $\{2_{100}   0 \ 0 \ 0\}$<br>$b_1 \quad -i$<br>$b_2 \quad i$                                                     |
| $c \ (\frac{t}{2}, \frac{t}{2}, \frac{t}{2})$     | $\{3_{111}   0 \ 0 \ 0\}$<br>$c_1 \quad -1$<br>$c_2 \quad e^{-\frac{i\pi}{3}}$<br>$c_3 \quad e^{\frac{i\pi}{3}}$ |
| $d \ (\frac{t}{2}, 1 - \frac{t}{2}, \frac{t}{2})$ | $\{1   0 \ 0 \ 0\}$<br>$d_1 \quad 1$                                                                             |

$$\begin{aligned} \mathcal{W}_1^{\text{gapless}} = & \sum_{m=1}^{n_{a_1}} \text{sgn}(v_m^{a_1}) \frac{1 - \text{sgn}(\delta_m^{a_1})}{2} + \sum_{m=1}^{n_{a_2}} \text{sgn}(v_m^{a_2}) \frac{1 - \text{sgn}(\delta_m^{a_2})}{2} - \sum_{m=1}^{n_{c_1}} \text{sgn}(v_m^{c_1}) \frac{1 - \text{sgn}(\delta_m^{c_1})}{2} \\ & - \sum_{m=1}^{n_{c_2}} \text{sgn}(v_m^{c_2}) \frac{1 - \text{sgn}(\delta_m^{c_2})}{2} - \sum_{m=1}^{n_{c_3}} \text{sgn}(v_m^{c_3}) \frac{1 - \text{sgn}(\delta_m^{c_3})}{2} + \sum_{m=1}^{n_{d_1}} \text{sgn}(v_m^{d_1}) \frac{1 - \text{sgn}(\delta_m^{d_1})}{2} \end{aligned} \quad (\text{S196.1})$$

$$\mathcal{W}_2^{\text{gapless}} = \sum_{m=1}^{n_{b_1}} \text{sgn}(v_m^{b_1}) \frac{1 - \text{sgn}(\delta_m^{b_1})}{2} + \sum_{m=1}^{n_{b_2}} \text{sgn}(v_m^{b_2}) \frac{1 - \text{sgn}(\delta_m^{b_2})}{2} \quad (\text{S196.2})$$

$$\mathcal{W}_1^{\text{gapped}} = \sum_{m=1}^{n_{b_2}} \text{sgn}(v_m^{b_2}) \frac{1 - \text{sgn}(\delta_m^{b_2})}{2} \quad (\text{S196.3})$$

$$\mathcal{W}_2^{\text{gapped}} = - \sum_{m=1}^{n_{c_2}} \text{sgn}(v_m^{c_2}) \frac{1 - \text{sgn}(\delta_m^{c_2})}{2} + \sum_{m=1}^{n_{c_3}} \text{sgn}(v_m^{c_3}) \frac{1 - \text{sgn}(\delta_m^{c_3})}{2} \quad (\text{S196.4})$$

$$\begin{aligned} \mathcal{W}_3^{\text{gapped}} = & 2 \sum_{m=1}^{n_{a_2}} \text{sgn}(v_m^{a_2}) \frac{1 - \text{sgn}(\delta_m^{a_2})}{2} - \sum_{m=1}^{n_{c_1}} \text{sgn}(v_m^{c_1}) \frac{1 - \text{sgn}(\delta_m^{c_1})}{2} - 2 \sum_{m=1}^{n_{c_2}} \text{sgn}(v_m^{c_2}) \frac{1 - \text{sgn}(\delta_m^{c_2})}{2} \\ & + \sum_{m=1}^{n_{d_1}} \text{sgn}(v_m^{d_1}) \frac{1 - \text{sgn}(\delta_m^{d_1})}{2} \end{aligned} \quad (\text{S196.5})$$

$$\mathcal{X}_1 = \sum_{m=1}^{n_{c_1}} \frac{1 - \text{sgn}(\delta_m^{c_1})}{2} \mod 2 \quad (\text{S196.6})$$

## S197. SPACE GROUP NO. 197

| line segment                                      | character of irrep (generators only)                                                                                     |
|---------------------------------------------------|--------------------------------------------------------------------------------------------------------------------------|
| $a \ (0, t, 0)$                                   | $\{2_{010}   0 \ 0 \ 0\}$<br>$a_1 \quad -i$<br>$a_2 \quad i$                                                             |
| $b \ (\frac{1}{2}, \frac{1}{2}, \frac{t}{2})$     | $\{2_{001}   0 \ 0 \ 0\}$<br>$b_1 \quad -i$<br>$b_2 \quad i$                                                             |
| $c \ (\frac{t}{2}, \frac{t}{2}, \frac{t}{2})$     | $\{3_{111}   0 \ 0 \ 0\}$<br>$c_1 \quad -1$<br>$c_2 \quad e^{-\frac{i\pi}{3}}$<br>$c_3 \quad e^{\frac{i\pi}{3}}$         |
| $d \ (\frac{t}{2}, 1 - \frac{t}{2}, \frac{t}{2})$ | $\{3^{-1}1\bar{1}1   0 \ 0 \ 0\}$<br>$d_1 \quad -1$<br>$d_2 \quad e^{-\frac{i\pi}{3}}$<br>$d_3 \quad e^{\frac{i\pi}{3}}$ |
| $e \ (\frac{t}{2}, 1 - \frac{t}{2}, 0)$           | $\{1   0 \ 0 \ 0\}$<br>$e_1 \quad 1$                                                                                     |

$$\begin{aligned}
\mathcal{W}_1^{\text{gapless}} = & \sum_{m=1}^{n_{a_1}} \text{sgn}(v_m^{a_1}) \frac{1 - \text{sgn}(\delta_m^{a_1})}{2} + \sum_{m=1}^{n_{a_2}} \text{sgn}(v_m^{a_2}) \frac{1 - \text{sgn}(\delta_m^{a_2})}{2} - \sum_{m=1}^{n_{c_1}} \text{sgn}(v_m^{c_1}) \frac{1 - \text{sgn}(\delta_m^{c_1})}{2} \\
& - \sum_{m=1}^{n_{c_2}} \text{sgn}(v_m^{c_2}) \frac{1 - \text{sgn}(\delta_m^{c_2})}{2} - \sum_{m=1}^{n_{c_3}} \text{sgn}(v_m^{c_3}) \frac{1 - \text{sgn}(\delta_m^{c_3})}{2} + \sum_{m=1}^{n_{d_1}} \text{sgn}(v_m^{d_1}) \frac{1 - \text{sgn}(\delta_m^{d_1})}{2} \\
& + \sum_{m=1}^{n_{d_2}} \text{sgn}(v_m^{d_2}) \frac{1 - \text{sgn}(\delta_m^{d_2})}{2} + \sum_{m=1}^{n_{d_3}} \text{sgn}(v_m^{d_3}) \frac{1 - \text{sgn}(\delta_m^{d_3})}{2}
\end{aligned} \tag{S197.1}$$

$$\begin{aligned}
\mathcal{W}_2^{\text{gapless}} = & \sum_{m=1}^{n_{b_1}} \text{sgn}(v_m^{b_1}) \frac{1 - \text{sgn}(\delta_m^{b_1})}{2} + \sum_{m=1}^{n_{b_2}} \text{sgn}(v_m^{b_2}) \frac{1 - \text{sgn}(\delta_m^{b_2})}{2} - \sum_{m=1}^{n_{d_1}} \text{sgn}(v_m^{d_1}) \frac{1 - \text{sgn}(\delta_m^{d_1})}{2} \\
& - \sum_{m=1}^{n_{d_2}} \text{sgn}(v_m^{d_2}) \frac{1 - \text{sgn}(\delta_m^{d_2})}{2} - \sum_{m=1}^{n_{d_3}} \text{sgn}(v_m^{d_3}) \frac{1 - \text{sgn}(\delta_m^{d_3})}{2} + \sum_{m=1}^{n_{e_1}} \text{sgn}(v_m^{e_1}) \frac{1 - \text{sgn}(\delta_m^{e_1})}{2}
\end{aligned} \tag{S197.2}$$

$$\begin{aligned}
\mathcal{W}_1^{\text{gapped}} = & 2 \sum_{m=1}^{n_{a_2}} \text{sgn}(v_m^{a_2}) \frac{1 - \text{sgn}(\delta_m^{a_2})}{2} - \sum_{m=1}^{n_{c_1}} \text{sgn}(v_m^{c_1}) \frac{1 - \text{sgn}(\delta_m^{c_1})}{2} - \sum_{m=1}^{n_{c_2}} \text{sgn}(v_m^{c_2}) \frac{1 - \text{sgn}(\delta_m^{c_2})}{2} - \sum_{m=1}^{n_{c_3}} \text{sgn}(v_m^{c_3}) \frac{1 - \text{sgn}(\delta_m^{c_3})}{2} \\
& + \sum_{m=1}^{n_{d_1}} \text{sgn}(v_m^{d_1}) \frac{1 - \text{sgn}(\delta_m^{d_1})}{2} + \sum_{m=1}^{n_{d_2}} \text{sgn}(v_m^{d_2}) \frac{1 - \text{sgn}(\delta_m^{d_2})}{2} + \sum_{m=1}^{n_{d_3}} \text{sgn}(v_m^{d_3}) \frac{1 - \text{sgn}(\delta_m^{d_3})}{2}
\end{aligned} \tag{S197.3}$$

$$\begin{aligned}
\mathcal{W}_2^{\text{gapped}} = & 2 \sum_{m=1}^{n_{a_2}} \text{sgn}(v_m^{a_2}) \frac{1 - \text{sgn}(\delta_m^{a_2})}{2} - \sum_{m=1}^{n_{c_1}} \text{sgn}(v_m^{c_1}) \frac{1 - \text{sgn}(\delta_m^{c_1})}{2} - 2 \sum_{m=1}^{n_{c_2}} \text{sgn}(v_m^{c_2}) \frac{1 - \text{sgn}(\delta_m^{c_2})}{2} \\
& + \sum_{m=1}^{n_{d_1}} \text{sgn}(v_m^{d_1}) \frac{1 - \text{sgn}(\delta_m^{d_1})}{2} + 2 \sum_{m=1}^{n_{d_3}} \text{sgn}(v_m^{d_3}) \frac{1 - \text{sgn}(\delta_m^{d_3})}{2}
\end{aligned} \tag{S197.4}$$

$$\begin{aligned} \mathcal{W}_3^{\text{gapped}} = & 2 \sum_{m=1}^{n_{a_2}} \text{sgn}(v_m^{a_2}) \frac{1 - \text{sgn}(\delta_m^{a_2})}{2} + 2 \sum_{m=1}^{n_{b_2}} \text{sgn}(v_m^{b_2}) \frac{1 - \text{sgn}(\delta_m^{b_2})}{2} - \sum_{m=1}^{n_{c_1}} \text{sgn}(v_m^{c_1}) \frac{1 - \text{sgn}(\delta_m^{c_1})}{2} \\ & - \sum_{m=1}^{n_{c_2}} \text{sgn}(v_m^{c_2}) \frac{1 - \text{sgn}(\delta_m^{c_2})}{2} - \sum_{m=1}^{n_{c_3}} \text{sgn}(v_m^{c_3}) \frac{1 - \text{sgn}(\delta_m^{c_3})}{2} + \sum_{m=1}^{n_{e_1}} \text{sgn}(v_m^{e_1}) \frac{1 - \text{sgn}(\delta_m^{e_1})}{2} \end{aligned} \quad (\text{S197.5})$$

$$\mathcal{X}_1 = \sum_{m=1}^{n_{c_1}} \frac{1 - \text{sgn}(\delta_m^{c_1})}{2} + \sum_{m=1}^{n_{c_2}} \frac{1 - \text{sgn}(\delta_m^{c_2})}{2} + \sum_{m=1}^{n_{c_3}} \frac{1 - \text{sgn}(\delta_m^{c_3})}{2} \mod 2 \quad (\text{S197.6})$$

### S198. SPACE GROUP NO. 198

| line segment                                                   | character of irrep (generators only)                                                                                                                      |
|----------------------------------------------------------------|-----------------------------------------------------------------------------------------------------------------------------------------------------------|
| $a \left( \frac{1}{2}, \frac{t}{2}, \frac{t}{2} \right)$       | $\begin{array}{c} \{1   0 \ 0 \ 0\} \\ a_1 \quad 1 \end{array}$                                                                                           |
| $b \left( \frac{1-t}{2}, \frac{1-t}{2}, \frac{1-t}{2} \right)$ | $\begin{array}{c} \{3_{111}   0 \ 0 \ 0\} \\ b_1 \quad -1 \\ b_2 \quad e^{-\frac{i\pi}{3}} \\ b_3 \quad e^{\frac{i\pi}{3}} \end{array}$                   |
| $c \left( \frac{t}{2}, 0, 0 \right)$                           | $\begin{array}{c} \{2_{100}   \frac{1}{2} \ \frac{1}{2} \ 0\} \\ c_1 \quad -ie^{-\frac{1}{2}i\pi t} \\ c_2 \quad ie^{-\frac{1}{2}i\pi t} \end{array}$     |
| $d \left( \frac{1}{2}, \frac{1}{2}, \frac{t}{2} \right)$       | $\begin{array}{c} \{2_{001}   \frac{1}{2} \ 0 \ \frac{1}{2}\} \\ d_1 \quad -e^{-\frac{1}{2}i\pi(t+1)} \\ d_2 \quad e^{-\frac{1}{2}i\pi(t+1)} \end{array}$ |
| $e \left( \frac{1}{2}, \frac{t}{2}, 0 \right)$                 | $\begin{array}{c} \{2_{010}   0 \ \frac{1}{2} \ \frac{1}{2}\} \\ e_1 \quad -ie^{-\frac{1}{2}i\pi t} \\ e_2 \quad ie^{-\frac{1}{2}i\pi t} \end{array}$     |
| $f \left( \frac{1-t}{2}, \frac{1}{2}, 0 \right)$               | $\begin{array}{c} \{2_{100}   \frac{1}{2} \ \frac{1}{2} \ 0\} \\ f_1 \quad -e^{-\frac{1}{2}i\pi(2-t)} \\ f_2 \quad e^{-\frac{1}{2}i\pi(2-t)} \end{array}$ |

$$\mathcal{W}_1^{\text{gapless}} = \sum_{m=1}^{n_{a_1}} \text{sgn}(v_m^{a_1}) \frac{1 - \text{sgn}(\delta_m^{a_1})}{2} - \sum_{m=1}^{n_{d_1}} \text{sgn}(v_m^{d_1}) \frac{1 - \text{sgn}(\delta_m^{d_1})}{2} - \sum_{m=1}^{n_{d_2}} \text{sgn}(v_m^{d_2}) \frac{1 - \text{sgn}(\delta_m^{d_2})}{2} + \sum_{m=1}^{n_{f_1}} \text{sgn}(v_m^{f_1}) \frac{1 - \text{sgn}(\delta_m^{f_1})}{2} \quad (\text{S198.1})$$

$$\begin{aligned} \mathcal{W}_2^{\text{gapless}} = & \sum_{m=1}^{n_{b_1}} \text{sgn}(v_m^{b_1}) \frac{1 - \text{sgn}(\delta_m^{b_1})}{2} + \sum_{m=1}^{n_{b_2}} \text{sgn}(v_m^{b_2}) \frac{1 - \text{sgn}(\delta_m^{b_2})}{2} + \sum_{m=1}^{n_{b_3}} \text{sgn}(v_m^{b_3}) \frac{1 - \text{sgn}(\delta_m^{b_3})}{2} \\ & + \sum_{m=1}^{n_{c_1}} \text{sgn}(v_m^{c_1}) \frac{1 - \text{sgn}(\delta_m^{c_1})}{2} + \sum_{m=1}^{n_{c_2}} \text{sgn}(v_m^{c_2}) \frac{1 - \text{sgn}(\delta_m^{c_2})}{2} + 2 \sum_{m=1}^{n_{d_1}} \text{sgn}(v_m^{d_1}) \frac{1 - \text{sgn}(\delta_m^{d_1})}{2} \\ & + 2 \sum_{m=1}^{n_{d_2}} \text{sgn}(v_m^{d_2}) \frac{1 - \text{sgn}(\delta_m^{d_2})}{2} - 2 \sum_{m=1}^{n_{f_1}} \text{sgn}(v_m^{f_1}) \frac{1 - \text{sgn}(\delta_m^{f_1})}{2} \end{aligned} \quad (\text{S198.2})$$

$$\mathcal{W}_3^{\text{gapless}} = \sum_{m=1}^{n_{e_1}} \text{sgn}(v_m^{e_1}) \frac{1 - \text{sgn}(\delta_m^{e_1})}{2} + \sum_{m=1}^{n_{f_1}} \text{sgn}(v_m^{f_1}) \frac{1 - \text{sgn}(\delta_m^{f_1})}{2} \quad (\text{S198.3})$$

$$\mathcal{W}_1^{\text{gapped}} = \sum_{m=1}^{n_{b_2}} \text{sgn}(v_m^{b_2}) \frac{1 - \text{sgn}(\delta_m^{b_2})}{2} - \sum_{m=1}^{n_{b_3}} \text{sgn}(v_m^{b_3}) \frac{1 - \text{sgn}(\delta_m^{b_3})}{2} \quad (\text{S198.4})$$

$$\mathcal{X}_1 = - \sum_{m=1}^{n_{c_1}} \text{sgn}(v_m^{c_1}) \frac{1 - \text{sgn}(\delta_m^{c_1})}{2} + \sum_{m=1}^{n_{c_2}} \text{sgn}(v_m^{c_2}) \frac{1 - \text{sgn}(\delta_m^{c_2})}{2} + 2 \sum_{m=1}^{n_{f_1}} \text{sgn}(v_m^{f_1}) \frac{1 - \text{sgn}(\delta_m^{f_1})}{2} \mod 4 \quad (\text{S198.5})$$

### S199. SPACE GROUP NO. 199

| line segment                                      | character of irrep (generators only)                                                                                                                                                              |
|---------------------------------------------------|---------------------------------------------------------------------------------------------------------------------------------------------------------------------------------------------------|
| $a \ (0, t, 0)$                                   | $\{2_{010}   \frac{1}{2} \ 0 \ 0\}$<br>$a_1 \quad -i$<br>$a_2 \quad i$                                                                                                                            |
| $b \ (\frac{1}{2}, \frac{1}{2}, \frac{t}{2})$     | $\{2_{001}   0 \ \frac{1}{2} \ 0\}$<br>$b_1 \quad i$<br>$b_2 \quad -i$                                                                                                                            |
| $c \ (\frac{t}{2}, \frac{t}{2}, \frac{t}{2})$     | $\{3_{111}   0 \ 0 \ 0\}$<br>$c_1 \quad -1$<br>$c_2 \quad e^{-\frac{i\pi}{3}}$<br>$c_3 \quad e^{\frac{i\pi}{3}}$                                                                                  |
| $d \ (\frac{t}{2}, 1 - \frac{t}{2}, \frac{t}{2})$ | $\{3^{-1}11   0 \ \frac{1}{2} \ 0\}$<br>$d_1 \quad -e^{-\frac{1}{2}i\pi(2-t)}$<br>$d_2 \quad e^{-\frac{1}{2}i\pi(2-t) - \frac{i\pi}{3}}$<br>$d_3 \quad e^{\frac{i\pi}{3} - \frac{1}{2}i\pi(2-t)}$ |
| $e \ (\frac{t}{2}, 1 - \frac{t}{2}, 0)$           | $\{1   0 \ 0 \ 0\}$<br>$e_1 \quad 1$                                                                                                                                                              |

$$\begin{aligned} \mathcal{W}_1^{\text{gapless}} = & \sum_{m=1}^{n_{a_1}} \text{sgn}(v_m^{a_1}) \frac{1 - \text{sgn}(\delta_m^{a_1})}{2} + \sum_{m=1}^{n_{a_2}} \text{sgn}(v_m^{a_2}) \frac{1 - \text{sgn}(\delta_m^{a_2})}{2} - \sum_{m=1}^{n_{c_1}} \text{sgn}(v_m^{c_1}) \frac{1 - \text{sgn}(\delta_m^{c_1})}{2} \\ & - \sum_{m=1}^{n_{c_2}} \text{sgn}(v_m^{c_2}) \frac{1 - \text{sgn}(\delta_m^{c_2})}{2} - \sum_{m=1}^{n_{c_3}} \text{sgn}(v_m^{c_3}) \frac{1 - \text{sgn}(\delta_m^{c_3})}{2} + \sum_{m=1}^{n_{d_1}} \text{sgn}(v_m^{d_1}) \frac{1 - \text{sgn}(\delta_m^{d_1})}{2} \\ & + \sum_{m=1}^{n_{d_2}} \text{sgn}(v_m^{d_2}) \frac{1 - \text{sgn}(\delta_m^{d_2})}{2} + \sum_{m=1}^{n_{d_3}} \text{sgn}(v_m^{d_3}) \frac{1 - \text{sgn}(\delta_m^{d_3})}{2} \end{aligned} \quad (\text{S199.1})$$

$$\begin{aligned} \mathcal{W}_2^{\text{gapless}} = & \sum_{m=1}^{n_{b_1}} \text{sgn}(v_m^{b_1}) \frac{1 - \text{sgn}(\delta_m^{b_1})}{2} + \sum_{m=1}^{n_{b_2}} \text{sgn}(v_m^{b_2}) \frac{1 - \text{sgn}(\delta_m^{b_2})}{2} - \sum_{m=1}^{n_{d_1}} \text{sgn}(v_m^{d_1}) \frac{1 - \text{sgn}(\delta_m^{d_1})}{2} \\ & - \sum_{m=1}^{n_{d_2}} \text{sgn}(v_m^{d_2}) \frac{1 - \text{sgn}(\delta_m^{d_2})}{2} - \sum_{m=1}^{n_{d_3}} \text{sgn}(v_m^{d_3}) \frac{1 - \text{sgn}(\delta_m^{d_3})}{2} + \sum_{m=1}^{n_{e_1}} \text{sgn}(v_m^{e_1}) \frac{1 - \text{sgn}(\delta_m^{e_1})}{2} \end{aligned} \quad (\text{S199.2})$$



$$\begin{aligned}\mathcal{W}_1^{\text{gapped}} = & - \sum_{m=1}^{n_{c_2}} \text{sgn}(v_m^{c_2}) \frac{1 - \text{sgn}(\delta_m^{c_2})}{2} + \sum_{m=1}^{n_{c_3}} \text{sgn}(v_m^{c_3}) \frac{1 - \text{sgn}(\delta_m^{c_3})}{2} - \sum_{m=1}^{n_{d_2}} \text{sgn}(v_m^{d_2}) \frac{1 - \text{sgn}(\delta_m^{d_2})}{2} \\ & + \sum_{m=1}^{n_{d_3}} \text{sgn}(v_m^{d_3}) \frac{1 - \text{sgn}(\delta_m^{d_3})}{2}\end{aligned}\quad (\text{S199.3})$$

$$\begin{aligned}\mathcal{W}_2^{\text{gapped}} = & -2 \sum_{m=1}^{n_{a_2}} \text{sgn}(v_m^{a_2}) \frac{1 - \text{sgn}(\delta_m^{a_2})}{2} + \sum_{m=1}^{n_{c_1}} \text{sgn}(v_m^{c_1}) \frac{1 - \text{sgn}(\delta_m^{c_1})}{2} + 2 \sum_{m=1}^{n_{c_3}} \text{sgn}(v_m^{c_3}) \frac{1 - \text{sgn}(\delta_m^{c_3})}{2} \\ & - \sum_{m=1}^{n_{d_1}} \text{sgn}(v_m^{d_1}) \frac{1 - \text{sgn}(\delta_m^{d_1})}{2} - 2 \sum_{m=1}^{n_{d_2}} \text{sgn}(v_m^{d_2}) \frac{1 - \text{sgn}(\delta_m^{d_2})}{2}\end{aligned}\quad (\text{S199.4})$$

$$\mathcal{X}_1 = \sum_{m=1}^{n_{c_1}} \frac{1 - \text{sgn}(\delta_m^{c_1})}{2} + \sum_{m=1}^{n_{d_1}} \frac{1 - \text{sgn}(\delta_m^{d_1})}{2} + \sum_{m=1}^{n_{e_1}} \frac{1 - \text{sgn}(\delta_m^{e_1})}{2} \quad \text{mod } 2 \quad (\text{S199.5})$$

## S200. SPACE GROUP NO. 200

| line segment                                                   | character of irrep (generators only)                                                                             |
|----------------------------------------------------------------|------------------------------------------------------------------------------------------------------------------|
| $a \left( \frac{1}{2}, \frac{t}{2}, \frac{t}{2} \right)$       | $\{m_{100}   0 \ 0 \ 0\}$<br>$a_1 \quad -i$<br>$a_2 \quad i$                                                     |
| $b \left( \frac{1-t}{2}, \frac{1-t}{2}, \frac{1-t}{2} \right)$ | $\{3_{111}   0 \ 0 \ 0\}$<br>$b_1 \quad -1$<br>$b_2 \quad e^{-\frac{i\pi}{3}}$<br>$b_3 \quad e^{\frac{i\pi}{3}}$ |
| $c \left( \frac{t}{2}, 0, 0 \right)$                           | $\{2_{100}   0 \ 0 \ 0\} \quad \{m_{010}   0 \ 0 \ 0\}$<br>$c_1 \quad 0 \quad 0$                                 |
| $d \left( \frac{1}{2}, \frac{1}{2}, \frac{t}{2} \right)$       | $\{2_{001}   0 \ 0 \ 0\} \quad \{m_{100}   0 \ 0 \ 0\}$<br>$d_1 \quad 0 \quad 0$                                 |
| $e \left( \frac{1}{2}, \frac{t}{2}, 0 \right)$                 | $\{2_{010}   0 \ 0 \ 0\} \quad \{m_{100}   0 \ 0 \ 0\}$<br>$e_1 \quad 0 \quad 0$                                 |
| $f \left( \frac{1-t}{2}, \frac{1}{2}, 0 \right)$               | $\{2_{100}   0 \ 0 \ 0\} \quad \{m_{010}   0 \ 0 \ 0\}$<br>$f_1 \quad 0 \quad 0$                                 |

$$\mathcal{W}_1^{\text{gapless}} = \sum_{m=1}^{n_{a_1}} \text{sgn}(v_m^{a_1}) \frac{1 - \text{sgn}(\delta_m^{a_1})}{2} - \sum_{m=1}^{n_{d_1}} \text{sgn}(v_m^{d_1}) \frac{1 - \text{sgn}(\delta_m^{d_1})}{2} + \sum_{m=1}^{n_{f_1}} \text{sgn}(v_m^{f_1}) \frac{1 - \text{sgn}(\delta_m^{f_1})}{2} \quad (\text{S200.1})$$

$$\begin{aligned}\mathcal{W}_2^{\text{gapless}} = & \sum_{m=1}^{n_{b_1}} \text{sgn}(v_m^{b_1}) \frac{1 - \text{sgn}(\delta_m^{b_1})}{2} + \sum_{m=1}^{n_{b_2}} \text{sgn}(v_m^{b_2}) \frac{1 - \text{sgn}(\delta_m^{b_2})}{2} + \sum_{m=1}^{n_{c_1}} \text{sgn}(v_m^{c_1}) \frac{1 - \text{sgn}(\delta_m^{c_1})}{2} \\ & + \sum_{m=1}^{n_{d_1}} \text{sgn}(v_m^{d_1}) \frac{1 - \text{sgn}(\delta_m^{d_1})}{2} - \sum_{m=1}^{n_{f_1}} \text{sgn}(v_m^{f_1}) \frac{1 - \text{sgn}(\delta_m^{f_1})}{2}\end{aligned}\quad (\text{S200.2})$$

$$\mathcal{W}_3^{\text{gapless}} = \sum_{m=1}^{n_{e_1}} \text{sgn}(v_m^{e_1}) \frac{1 - \text{sgn}(\delta_m^{e_1})}{2} + \sum_{m=1}^{n_{f_1}} \text{sgn}(v_m^{f_1}) \frac{1 - \text{sgn}(\delta_m^{f_1})}{2} \quad (\text{S200.3})$$

## S201. SPACE GROUP NO. 201

| line segment                                                   | character of irrep (generators only)                                                                                                                                                                                                                                                                        |
|----------------------------------------------------------------|-------------------------------------------------------------------------------------------------------------------------------------------------------------------------------------------------------------------------------------------------------------------------------------------------------------|
| $a \left( \frac{1}{2}, \frac{t}{2}, \frac{t}{2} \right)$       | $\{m_{100}   0 \frac{1}{2} \frac{1}{2}\}$<br>$a_1 \quad -ie^{-i\pi t}$<br>$a_2 \quad ie^{-i\pi t}$                                                                                                                                                                                                          |
| $b \left( \frac{1-t}{2}, \frac{1-t}{2}, \frac{1-t}{2} \right)$ | $\{3_{111}   0 \ 0 \ 0\}$<br>$b_1 \quad -1$<br>$b_2 \quad e^{-\frac{i\pi}{3}}$<br>$b_3 \quad e^{\frac{i\pi}{3}}$                                                                                                                                                                                            |
| $c \left( \frac{t}{2}, 0, 0 \right)$                           | $\{2_{100}   0 \ \frac{1}{2} \ \frac{1}{2}\} \quad \{m_{010}   \frac{1}{2} \ 0 \ \frac{1}{2}\}$<br>$c_1 \quad 0 \quad 0$                                                                                                                                                                                    |
| $d \left( \frac{1}{2}, \frac{1}{2}, \frac{t}{2} \right)$       | $\{2_{001}   \frac{1}{2} \ \frac{1}{2} \ 0\} \quad \{m_{100}   0 \ \frac{1}{2} \ \frac{1}{2}\}$<br>$d_1 \quad 0 \quad 0$                                                                                                                                                                                    |
| $e \left( \frac{1}{2}, \frac{t}{2}, 0 \right)$                 | $\{2_{010}   \frac{1}{2} \ 0 \ \frac{1}{2}\} \quad \{m_{100}   0 \ \frac{1}{2} \ \frac{1}{2}\}$<br>$e_1 \quad i \quad -ie^{-\frac{1}{2}i\pi t}$<br>$e_2 \quad i \quad ie^{-\frac{1}{2}i\pi t}$<br>$e_3 \quad -i \quad -ie^{-\frac{1}{2}i\pi t}$<br>$e_4 \quad -i \quad ie^{-\frac{1}{2}i\pi t}$             |
| $f \left( \frac{1-t}{2}, \frac{1}{2}, 0 \right)$               | $\{2_{100}   0 \ \frac{1}{2} \ \frac{1}{2}\} \quad \{m_{010}   \frac{1}{2} \ 0 \ \frac{1}{2}\}$<br>$f_1 \quad i \quad -ie^{-\frac{1}{2}i\pi(1-t)}$<br>$f_2 \quad i \quad ie^{-\frac{1}{2}i\pi(1-t)}$<br>$f_3 \quad -i \quad -ie^{-\frac{1}{2}i\pi(1-t)}$<br>$f_4 \quad -i \quad ie^{-\frac{1}{2}i\pi(1-t)}$ |

$$\mathcal{W}_1^{\text{gapless}} = \sum_{m=1}^{n_{a_1}} \text{sgn}(v_m^{a_1}) \frac{1 - \text{sgn}(\delta_m^{a_1})}{2} - \sum_{m=1}^{n_{d_1}} \text{sgn}(v_m^{d_1}) \frac{1 - \text{sgn}(\delta_m^{d_1})}{2} + \sum_{m=1}^{n_{f_1}} \text{sgn}(v_m^{f_1}) \frac{1 - \text{sgn}(\delta_m^{f_1})}{2} + \sum_{m=1}^{n_{f_3}} \text{sgn}(v_m^{f_3}) \frac{1 - \text{sgn}(\delta_m^{f_3})}{2} \quad (\text{S201.1})$$

$$\begin{aligned} \mathcal{W}_2^{\text{gapless}} = & \sum_{m=1}^{n_{b_1}} \text{sgn}(v_m^{b_1}) \frac{1 - \text{sgn}(\delta_m^{b_1})}{2} + \sum_{m=1}^{n_{b_2}} \text{sgn}(v_m^{b_2}) \frac{1 - \text{sgn}(\delta_m^{b_2})}{2} + \sum_{m=1}^{n_{c_1}} \text{sgn}(v_m^{c_1}) \frac{1 - \text{sgn}(\delta_m^{c_1})}{2} \\ & + \sum_{m=1}^{n_{d_1}} \text{sgn}(v_m^{d_1}) \frac{1 - \text{sgn}(\delta_m^{d_1})}{2} - \sum_{m=1}^{n_{f_1}} \text{sgn}(v_m^{f_1}) \frac{1 - \text{sgn}(\delta_m^{f_1})}{2} - \sum_{m=1}^{n_{f_3}} \text{sgn}(v_m^{f_3}) \frac{1 - \text{sgn}(\delta_m^{f_3})}{2} \end{aligned} \quad (\text{S201.2})$$

$$\mathcal{W}_3^{\text{gapless}} = \sum_{m=1}^{n_{e_1}} \text{sgn}(v_m^{e_1}) \frac{1 - \text{sgn}(\delta_m^{e_1})}{2} + \sum_{m=1}^{n_{e_3}} \text{sgn}(v_m^{e_3}) \frac{1 - \text{sgn}(\delta_m^{e_3})}{2} + \sum_{m=1}^{n_{f_1}} \text{sgn}(v_m^{f_1}) \frac{1 - \text{sgn}(\delta_m^{f_1})}{2} + \sum_{m=1}^{n_{f_3}} \text{sgn}(v_m^{f_3}) \frac{1 - \text{sgn}(\delta_m^{f_3})}{2} \quad (\text{S201.3})$$

$$\mathcal{W}_1^{\text{gapped}} = \sum_{m=1}^{n_{e_3}} \text{sgn}(v_m^{e_3}) \frac{1 - \text{sgn}(\delta_m^{e_3})}{2} + \sum_{m=1}^{n_{f_1}} \text{sgn}(v_m^{f_1}) \frac{1 - \text{sgn}(\delta_m^{f_1})}{2} \quad (\text{S201.4})$$

$$\mathcal{W}_2^{\text{gapped}} = \sum_{m=1}^{n_{e_3}} \text{sgn}(v_m^{e_3}) \frac{1 - \text{sgn}(\delta_m^{e_3})}{2} + \sum_{m=1}^{n_{f_3}} \text{sgn}(v_m^{f_3}) \frac{1 - \text{sgn}(\delta_m^{f_3})}{2} \quad (\text{S201.5})$$

**S202. SPACE GROUP NO. 202**

| line segment                                      | character of irrep (generators only)                                                                                                                    |
|---------------------------------------------------|---------------------------------------------------------------------------------------------------------------------------------------------------------|
| $a \ (0, t, 0)$                                   | $a_1 \ \begin{Bmatrix} \{2_{010}   0 & 0 & 0\} & \{m_{100}   0 & 0 & 0\} \\ 0 & 0 \end{Bmatrix}$                                                        |
| $b \ (t, 1, 0)$                                   | $b_1 \ \begin{Bmatrix} \{2_{100}   0 & 0 & 0\} & \{m_{010}   0 & 0 & 0\} \\ 0 & 0 \end{Bmatrix}$                                                        |
| $c \ (\frac{t}{2}, \frac{t}{2}, \frac{t}{2})$     | $\begin{matrix} c_1 & -1 \\ c_2 & e^{-\frac{i\pi}{3}} \\ c_3 & e^{\frac{i\pi}{3}} \end{matrix} \ \begin{Bmatrix} \{3_{111}   0 & 0 & 0\} \end{Bmatrix}$ |
| $d \ (\frac{t}{2}, 1 - \frac{t}{2}, \frac{t}{2})$ | $d_1 \ \begin{Bmatrix} \{1   0 & 0 & 0\} \\ 1 \end{Bmatrix}$                                                                                            |

$$\mathcal{W}_1^{\text{gapless}} = \sum_{m=1}^{n_{a_1}} \text{sgn}(v_m^{a_1}) \frac{1 - \text{sgn}(\delta_m^{a_1})}{2} - \sum_{m=1}^{n_{c_1}} \text{sgn}(v_m^{c_1}) \frac{1 - \text{sgn}(\delta_m^{c_1})}{2} - \sum_{m=1}^{n_{c_2}} \text{sgn}(v_m^{c_2}) \frac{1 - \text{sgn}(\delta_m^{c_2})}{2} + \sum_{m=1}^{n_{d_1}} \text{sgn}(v_m^{d_1}) \frac{1 - \text{sgn}(\delta_m^{d_1})}{2} \quad (\text{S202.1})$$

$$\mathcal{W}_2^{\text{gapless}} = \sum_{m=1}^{n_{b_1}} \text{sgn}(v_m^{b_1}) \frac{1 - \text{sgn}(\delta_m^{b_1})}{2} \quad (\text{S202.2})$$

**S203. SPACE GROUP NO. 203**

| line segment                                      | character of irrep (generators only)                                                                                                                                                                                                                                                                         |
|---------------------------------------------------|--------------------------------------------------------------------------------------------------------------------------------------------------------------------------------------------------------------------------------------------------------------------------------------------------------------|
| $a \ (0, t, 0)$                                   | $a_1 \ \begin{Bmatrix} \{2_{010}   \frac{3}{4} & 0 & \frac{3}{4}\} & \{m_{100}   0 & \frac{1}{4} & \frac{1}{4}\} \\ 0 & 0 \end{Bmatrix}$                                                                                                                                                                     |
| $b \ (t, 1, 0)$                                   | $\begin{matrix} b_1 & -i & -ie^{-\frac{1}{2}i\pi t} \\ b_2 & -i & ie^{-\frac{1}{2}i\pi t} \\ b_3 & i & -ie^{-\frac{1}{2}i\pi t} \\ b_4 & i & ie^{-\frac{1}{2}i\pi t} \end{matrix} \ \begin{Bmatrix} \{2_{100}   0 & \frac{3}{4} & \frac{3}{4}\} & \{m_{010}   \frac{1}{4} & 0 & \frac{1}{4}\} \end{Bmatrix}$ |
| $c \ (\frac{t}{2}, \frac{t}{2}, \frac{t}{2})$     | $\begin{matrix} c_1 & -1 \\ c_2 & e^{-\frac{i\pi}{3}} \\ c_3 & e^{\frac{i\pi}{3}} \end{matrix} \ \begin{Bmatrix} \{3_{111}   0 & 0 & 0\} \end{Bmatrix}$                                                                                                                                                      |
| $d \ (\frac{t}{2}, 1 - \frac{t}{2}, \frac{t}{2})$ | $d_1 \ \begin{Bmatrix} \{1   0 & 0 & 0\} \\ 1 \end{Bmatrix}$                                                                                                                                                                                                                                                 |

$$\mathcal{W}_1^{\text{gapless}} = \sum_{m=1}^{n_{a_1}} \text{sgn}(v_m^{a_1}) \frac{1 - \text{sgn}(\delta_m^{a_1})}{2} - \sum_{m=1}^{n_{c_1}} \text{sgn}(v_m^{c_1}) \frac{1 - \text{sgn}(\delta_m^{c_1})}{2} - \sum_{m=1}^{n_{c_2}} \text{sgn}(v_m^{c_2}) \frac{1 - \text{sgn}(\delta_m^{c_2})}{2} + \sum_{m=1}^{n_{d_1}} \text{sgn}(v_m^{d_1}) \frac{1 - \text{sgn}(\delta_m^{d_1})}{2} \quad (\text{S203.1})$$

$$\mathcal{W}_2^{\text{gapless}} = \sum_{m=1}^{n_{b_1}} \text{sgn}(v_m^{b_1}) \frac{1 - \text{sgn}(\delta_m^{b_1})}{2} + \sum_{m=1}^{n_{b_3}} \text{sgn}(v_m^{b_3}) \frac{1 - \text{sgn}(\delta_m^{b_3})}{2} \quad (\text{S203.2})$$

$$\mathcal{W}_1^{\text{gapped}} = \sum_{m=1}^{n_{b_3}} \text{sgn}(v_m^{b_3}) \frac{1 - \text{sgn}(\delta_m^{b_3})}{2} \quad (\text{S203.3})$$

**S204. SPACE GROUP NO. 204**

| line segment                                      | character of irrep (generators only)                                                                                        |
|---------------------------------------------------|-----------------------------------------------------------------------------------------------------------------------------|
| $a \ (0, t, 0)$                                   | $\begin{matrix} \{2_{010}  0 & 0 & 0 \} \\ a_1 & 0 \end{matrix} \quad \{m_{100}  0 & 0 & 0 \}$                              |
| $b \ (\frac{1}{2}, \frac{1}{2}, \frac{t}{2})$     | $\begin{matrix} \{2_{001}  0 & 0 & 0 \} \\ b_1 & -i \\ b_2 & i \end{matrix}$                                                |
| $c \ (\frac{t}{2}, \frac{t}{2}, \frac{t}{2})$     | $\begin{matrix} \{3_{111}  0 & 0 & 0 \} \\ c_1 & -1 \\ c_2 & e^{-\frac{i\pi}{3}} \\ c_3 & e^{\frac{i\pi}{3}} \end{matrix}$  |
| $d \ (\frac{t}{2}, 1 - \frac{t}{2}, \frac{t}{2})$ | $\begin{matrix} \{3^{-111}  0 & 0 & 0 \} \\ d_1 & -1 \\ d_2 & e^{-\frac{i\pi}{3}} \\ d_3 & e^{\frac{i\pi}{3}} \end{matrix}$ |
| $e \ (\frac{t}{2}, 1 - \frac{t}{2}, 0)$           | $\begin{matrix} \{m_{001}  0 & 0 & 0 \} \\ e_1 & -i \\ e_2 & i \end{matrix}$                                                |

$$\begin{aligned} \mathcal{W}_1^{\text{gapless}} = & \sum_{m=1}^{n_{a_1}} \text{sgn}(v_m^{a_1}) \frac{1 - \text{sgn}(\delta_m^{a_1})}{2} - \sum_{m=1}^{n_{c_1}} \text{sgn}(v_m^{c_1}) \frac{1 - \text{sgn}(\delta_m^{c_1})}{2} - \sum_{m=1}^{n_{c_2}} \text{sgn}(v_m^{c_2}) \frac{1 - \text{sgn}(\delta_m^{c_2})}{2} \\ & + \sum_{m=1}^{n_{d_1}} \text{sgn}(v_m^{d_1}) \frac{1 - \text{sgn}(\delta_m^{d_1})}{2} + \sum_{m=1}^{n_{d_2}} \text{sgn}(v_m^{d_2}) \frac{1 - \text{sgn}(\delta_m^{d_2})}{2} \end{aligned} \quad (\text{S204.1})$$

$$\mathcal{W}_2^{\text{gapless}} = \sum_{m=1}^{n_{b_1}} \text{sgn}(v_m^{b_1}) \frac{1 - \text{sgn}(\delta_m^{b_1})}{2} - \sum_{m=1}^{n_{d_1}} \text{sgn}(v_m^{d_1}) \frac{1 - \text{sgn}(\delta_m^{d_1})}{2} - \sum_{m=1}^{n_{d_2}} \text{sgn}(v_m^{d_2}) \frac{1 - \text{sgn}(\delta_m^{d_2})}{2} + \sum_{m=1}^{n_{e_1}} \text{sgn}(v_m^{e_1}) \frac{1 - \text{sgn}(\delta_m^{e_1})}{2} \quad (\text{S204.2})$$

**S205. SPACE GROUP NO. 205**

| line segment                                        | character of irrep (generators only)                                                                                                             |
|-----------------------------------------------------|--------------------------------------------------------------------------------------------------------------------------------------------------|
| $a \ (\frac{1}{2}, \frac{t}{2}, \frac{t}{2})$       | $\begin{matrix} \{m_{100}  \frac{1}{2} & \frac{1}{2} & 0 \} \\ a_1 & -e^{-\frac{1}{2}i\pi(t+1)} \\ a_2 & e^{-\frac{1}{2}i\pi(t+1)} \end{matrix}$ |
| $b \ (\frac{1-t}{2}, \frac{1-t}{2}, \frac{1-t}{2})$ | $\begin{matrix} \{3_{111}  0 & 0 & 0 \} \\ b_1 & -1 \\ b_2 & e^{-\frac{i\pi}{3}} \\ b_3 & e^{\frac{i\pi}{3}} \end{matrix}$                       |
| $c \ (\frac{t}{2}, 0, 0)$                           | $\begin{matrix} \{2_{100}  \frac{1}{2} & \frac{1}{2} & 0 \} & \{m_{010}  0 & \frac{1}{2} & \frac{1}{2} \} \\ c_1 & 0 & 0 \end{matrix}$           |

|                                                   |       |                                                                                               |
|---------------------------------------------------|-------|-----------------------------------------------------------------------------------------------|
| $d \quad (\frac{1}{2}, \frac{1}{2}, \frac{t}{2})$ | $d_1$ | $\{2_{001}   \frac{1}{2} \ 0 \ \frac{1}{2} \} \ \{m_{100}   \frac{1}{2} \ \frac{1}{2} \ 0 \}$ |
|                                                   |       | $-e^{-\frac{1}{2}i\pi(t+1)} \quad 1$                                                          |
|                                                   | $d_2$ | $-e^{-\frac{1}{2}i\pi(t+1)} \quad -1$                                                         |
|                                                   | $d_3$ | $e^{-\frac{1}{2}i\pi(t+1)} \quad 1$                                                           |
|                                                   | $d_4$ | $e^{-\frac{1}{2}i\pi(t+1)} \quad -1$                                                          |
| $e \quad (\frac{1}{2}, \frac{t}{2}, 0)$           | $e_1$ | $\{2_{010}   0 \ \frac{1}{2} \ \frac{1}{2} \} \ \{m_{100}   \frac{1}{2} \ \frac{1}{2} \ 0 \}$ |
|                                                   |       | $-ie^{-\frac{1}{2}i\pi t} \quad -e^{-\frac{1}{2}i\pi(t+1)}$                                   |
|                                                   | $e_2$ | $-ie^{-\frac{1}{2}i\pi t} \quad e^{-\frac{1}{2}i\pi(t+1)}$                                    |
|                                                   | $e_3$ | $ie^{-\frac{1}{2}i\pi t} \quad -e^{-\frac{1}{2}i\pi(t+1)}$                                    |
|                                                   | $e_4$ | $ie^{-\frac{1}{2}i\pi t} \quad e^{-\frac{1}{2}i\pi(t+1)}$                                     |
| $f \quad (\frac{1-t}{2}, \frac{1}{2}, 0)$         | $f_1$ | $\{2_{100}   \frac{1}{2} \ \frac{1}{2} \ 0 \} \ \{m_{010}   0 \ \frac{1}{2} \ \frac{1}{2} \}$ |
|                                                   |       | $0 \quad 0$                                                                                   |

$$\mathcal{W}_1^{\text{gapless}} = \sum_{m=1}^{n_{a_1}} \text{sgn}(v_m^{a_1}) \frac{1 - \text{sgn}(\delta_m^{a_1})}{2} - \sum_{m=1}^{n_{d_2}} \text{sgn}(v_m^{d_2}) \frac{1 - \text{sgn}(\delta_m^{d_2})}{2} - \sum_{m=1}^{n_{d_3}} \text{sgn}(v_m^{d_3}) \frac{1 - \text{sgn}(\delta_m^{d_3})}{2} + \sum_{m=1}^{n_{f_1}} \text{sgn}(v_m^{f_1}) \frac{1 - \text{sgn}(\delta_m^{f_1})}{2} \quad (\text{S205.1})$$

$$\mathcal{W}_2^{\text{gapless}} = \sum_{m=1}^{n_{a_2}} \text{sgn}(v_m^{a_2}) \frac{1 - \text{sgn}(\delta_m^{a_2})}{2} - \sum_{m=1}^{n_{d_2}} \text{sgn}(v_m^{d_2}) \frac{1 - \text{sgn}(\delta_m^{d_2})}{2} - \sum_{m=1}^{n_{d_4}} \text{sgn}(v_m^{d_4}) \frac{1 - \text{sgn}(\delta_m^{d_4})}{2} - \sum_{m=1}^{n_{e_2}} \text{sgn}(v_m^{e_2}) \frac{1 - \text{sgn}(\delta_m^{e_2})}{2} \quad (\text{S205.2})$$

$$\begin{aligned} \mathcal{W}_3^{\text{gapless}} = & \sum_{m=1}^{n_{b_1}} \text{sgn}(v_m^{b_1}) \frac{1 - \text{sgn}(\delta_m^{b_1})}{2} + \sum_{m=1}^{n_{b_2}} \text{sgn}(v_m^{b_2}) \frac{1 - \text{sgn}(\delta_m^{b_2})}{2} + \sum_{m=1}^{n_{c_1}} \text{sgn}(v_m^{c_1}) \frac{1 - \text{sgn}(\delta_m^{c_1})}{2} \\ & + 2 \sum_{m=1}^{n_{d_2}} \text{sgn}(v_m^{d_2}) \frac{1 - \text{sgn}(\delta_m^{d_2})}{2} + \sum_{m=1}^{n_{d_3}} \text{sgn}(v_m^{d_3}) \frac{1 - \text{sgn}(\delta_m^{d_3})}{2} \\ & + \sum_{m=1}^{n_{d_4}} \text{sgn}(v_m^{d_4}) \frac{1 - \text{sgn}(\delta_m^{d_4})}{2} + \sum_{m=1}^{n_{e_2}} \text{sgn}(v_m^{e_2}) \frac{1 - \text{sgn}(\delta_m^{e_2})}{2} - \sum_{m=1}^{n_{f_1}} \text{sgn}(v_m^{f_1}) \frac{1 - \text{sgn}(\delta_m^{f_1})}{2} \end{aligned} \quad (\text{S205.3})$$

$$\mathcal{W}_4^{\text{gapless}} = \sum_{m=1}^{n_{d_1}} \text{sgn}(v_m^{d_1}) \frac{1 - \text{sgn}(\delta_m^{d_1})}{2} - \sum_{m=1}^{n_{d_2}} \text{sgn}(v_m^{d_2}) \frac{1 - \text{sgn}(\delta_m^{d_2})}{2} - \sum_{m=1}^{n_{e_2}} \text{sgn}(v_m^{e_2}) \frac{1 - \text{sgn}(\delta_m^{e_2})}{2} - \sum_{m=1}^{n_{f_1}} \text{sgn}(v_m^{f_1}) \frac{1 - \text{sgn}(\delta_m^{f_1})}{2} \quad (\text{S205.4})$$

$$\mathcal{W}_5^{\text{gapless}} = \sum_{m=1}^{n_{e_1}} \text{sgn}(v_m^{e_1}) \frac{1 - \text{sgn}(\delta_m^{e_1})}{2} + \sum_{m=1}^{n_{e_2}} \text{sgn}(v_m^{e_2}) \frac{1 - \text{sgn}(\delta_m^{e_2})}{2} + 2 \sum_{m=1}^{n_{f_1}} \text{sgn}(v_m^{f_1}) \frac{1 - \text{sgn}(\delta_m^{f_1})}{2} \quad (\text{S205.5})$$

## S206. SPACE GROUP NO. 206

|              |                                      |
|--------------|--------------------------------------|
| line segment | character of irrep (generators only) |
|--------------|--------------------------------------|

|                                                                    |                                                                                                                                                                                                                                                                                                          |
|--------------------------------------------------------------------|----------------------------------------------------------------------------------------------------------------------------------------------------------------------------------------------------------------------------------------------------------------------------------------------------------|
| $a \quad (0, t, 0)$                                                | $a_1 \quad \left\{ 2_{010} \left  \begin{smallmatrix} \frac{1}{2} & 0 & 0 \end{smallmatrix} \right. \right\} \quad \left\{ m_{100} \left  \begin{smallmatrix} 0 & 0 & \frac{1}{2} \end{smallmatrix} \right. \right\}$<br>$0$                                                                             |
| $b \quad \left( \frac{1}{2}, \frac{1}{2}, \frac{t}{2} \right)$     | $b_1 \quad \left\{ 2_{001} \left  \begin{smallmatrix} 0 & \frac{1}{2} & 0 \end{smallmatrix} \right. \right\}$<br>$b_2 \quad \begin{smallmatrix} i \\ -i \end{smallmatrix}$                                                                                                                               |
| $c \quad \left( \frac{t}{2}, \frac{t}{2}, \frac{t}{2} \right)$     | $c_1 \quad \left\{ 3_{111} \left  \begin{smallmatrix} 0 & 0 & 0 \end{smallmatrix} \right. \right\}$<br>$c_2 \quad \begin{smallmatrix} -1 \\ e^{-\frac{i\pi}{3}} \end{smallmatrix}$<br>$c_3 \quad e^{\frac{i\pi}{3}}$                                                                                     |
| $d \quad \left( \frac{t}{2}, 1 - \frac{t}{2}, \frac{t}{2} \right)$ | $d_1 \quad \left\{ 3_{-11-1}^- \left  \begin{smallmatrix} 0 & \frac{1}{2} & 0 \end{smallmatrix} \right. \right\}$<br>$d_2 \quad \begin{smallmatrix} -e^{-\frac{1}{2}i\pi(2-t)} \\ e^{-\frac{1}{2}i\pi(2-t) - \frac{i\pi}{3}} \end{smallmatrix}$<br>$d_3 \quad e^{\frac{i\pi}{3} - \frac{1}{2}i\pi(2-t)}$ |
| $e \quad \left( \frac{t}{2}, 1 - \frac{t}{2}, 0 \right)$           | $e_1 \quad \left\{ m_{001} \left  \begin{smallmatrix} 0 & \frac{1}{2} & 0 \end{smallmatrix} \right. \right\}$<br>$e_2 \quad \begin{smallmatrix} -ie^{-\frac{1}{2}i\pi(2-t)} \\ ie^{-\frac{1}{2}i\pi(2-t)} \end{smallmatrix}$                                                                             |

$$\begin{aligned} \mathcal{W}_1^{\text{gapless}} = & \sum_{m=1}^{n_{a_1}} \text{sgn}(v_m^{a_1}) \frac{1 - \text{sgn}(\delta_m^{a_1})}{2} - \sum_{m=1}^{n_{c_1}} \text{sgn}(v_m^{c_1}) \frac{1 - \text{sgn}(\delta_m^{c_1})}{2} - \sum_{m=1}^{n_{c_2}} \text{sgn}(v_m^{c_2}) \frac{1 - \text{sgn}(\delta_m^{c_2})}{2} \\ & + \sum_{m=1}^{n_{d_1}} \text{sgn}(v_m^{d_1}) \frac{1 - \text{sgn}(\delta_m^{d_1})}{2} + \sum_{m=1}^{n_{d_2}} \text{sgn}(v_m^{d_2}) \frac{1 - \text{sgn}(\delta_m^{d_2})}{2} \end{aligned} \quad (\text{S206.1})$$

$$\begin{aligned} \mathcal{W}_2^{\text{gapless}} = & \sum_{m=1}^{n_{b_1}} \text{sgn}(v_m^{b_1}) \frac{1 - \text{sgn}(\delta_m^{b_1})}{2} + \sum_{m=1}^{n_{b_2}} \text{sgn}(v_m^{b_2}) \frac{1 - \text{sgn}(\delta_m^{b_2})}{2} - \sum_{m=1}^{n_{d_1}} \text{sgn}(v_m^{d_1}) \frac{1 - \text{sgn}(\delta_m^{d_1})}{2} \\ & - \sum_{m=1}^{n_{d_2}} \text{sgn}(v_m^{d_2}) \frac{1 - \text{sgn}(\delta_m^{d_2})}{2} + \sum_{m=1}^{n_{e_1}} \text{sgn}(v_m^{e_1}) \frac{1 - \text{sgn}(\delta_m^{e_1})}{2} \end{aligned} \quad (\text{S206.2})$$

### S207. SPACE GROUP NO. 207

| line segment                                                   | character of irrep (generators only)                                                                                                                                                                                                  |
|----------------------------------------------------------------|---------------------------------------------------------------------------------------------------------------------------------------------------------------------------------------------------------------------------------------|
| $a \quad \left( \frac{t}{2}, 0, 0 \right)$                     | $\left\{ 4_{100} \left  \begin{smallmatrix} 0 & 0 & 0 \end{smallmatrix} \right. \right\}$<br>$a_1 \quad e^{-\frac{3i\pi}{4}}$<br>$a_2 \quad e^{\frac{3i\pi}{4}}$<br>$a_3 \quad e^{-\frac{i\pi}{4}}$<br>$a_4 \quad e^{\frac{i\pi}{4}}$ |
| $b \quad \left( \frac{1}{2}, \frac{t}{2}, 0 \right)$           | $\left\{ 2_{010} \left  \begin{smallmatrix} 0 & 0 & 0 \end{smallmatrix} \right. \right\}$<br>$b_1 \quad -i$<br>$b_2 \quad i$                                                                                                          |
| $c \quad \left( \frac{t}{2}, \frac{t}{2}, 0 \right)$           | $\left\{ 2_{110} \left  \begin{smallmatrix} 0 & 0 & 0 \end{smallmatrix} \right. \right\}$<br>$c_1 \quad -i$<br>$c_2 \quad i$                                                                                                          |
| $d \quad \left( \frac{1}{2}, \frac{1}{2}, \frac{t}{2} \right)$ | $\left\{ 4_{001} \left  \begin{smallmatrix} 0 & 0 & 0 \end{smallmatrix} \right. \right\}$<br>$d_1 \quad e^{-\frac{3i\pi}{4}}$<br>$d_2 \quad e^{\frac{3i\pi}{4}}$<br>$d_3 \quad e^{-\frac{i\pi}{4}}$<br>$d_4 \quad e^{\frac{i\pi}{4}}$ |

|                                                   |                       |                       |  |
|---------------------------------------------------|-----------------------|-----------------------|--|
| $e \quad (\frac{t}{2}, \frac{t}{2}, \frac{t}{2})$ | $\{3_{111} 0\ 0\ 0\}$ |                       |  |
|                                                   | $e_1$                 | $-1$                  |  |
|                                                   | $e_2$                 | $e^{-\frac{i\pi}{3}}$ |  |
|                                                   | $e_3$                 | $e^{\frac{i\pi}{3}}$  |  |
| $f \quad (\frac{1}{2}, \frac{t}{2}, \frac{t}{2})$ | $\{2_{011} 0\ 0\ 0\}$ |                       |  |
|                                                   | $f_1$                 | $-i$                  |  |
|                                                   | $f_2$                 | $i$                   |  |

$$\begin{aligned}
\mathcal{W}_1^{\text{gapless}} = & \sum_{m=1}^{n_{a_1}} \text{sgn}(v_m^{a_1}) \frac{1 - \text{sgn}(\delta_m^{a_1})}{2} + \sum_{m=1}^{n_{a_2}} \text{sgn}(v_m^{a_2}) \frac{1 - \text{sgn}(\delta_m^{a_2})}{2} + \sum_{m=1}^{n_{a_3}} \text{sgn}(v_m^{a_3}) \frac{1 - \text{sgn}(\delta_m^{a_3})}{2} \\
& + \sum_{m=1}^{n_{a_4}} \text{sgn}(v_m^{a_4}) \frac{1 - \text{sgn}(\delta_m^{a_4})}{2} - \sum_{m=1}^{n_{e_1}} \text{sgn}(v_m^{e_1}) \frac{1 - \text{sgn}(\delta_m^{e_1})}{2} - \sum_{m=1}^{n_{e_2}} \text{sgn}(v_m^{e_2}) \frac{1 - \text{sgn}(\delta_m^{e_2})}{2} \\
& - \sum_{m=1}^{n_{e_3}} \text{sgn}(v_m^{e_3}) \frac{1 - \text{sgn}(\delta_m^{e_3})}{2} + \sum_{m=1}^{n_{f_1}} \text{sgn}(v_m^{f_1}) \frac{1 - \text{sgn}(\delta_m^{f_1})}{2} + \sum_{m=1}^{n_{f_2}} \text{sgn}(v_m^{f_2}) \frac{1 - \text{sgn}(\delta_m^{f_2})}{2}
\end{aligned} \tag{S207.1}$$

$$\begin{aligned}
\mathcal{W}_2^{\text{gapless}} = & \sum_{m=1}^{n_{b_1}} \text{sgn}(v_m^{b_1}) \frac{1 - \text{sgn}(\delta_m^{b_1})}{2} + \sum_{m=1}^{n_{b_2}} \text{sgn}(v_m^{b_2}) \frac{1 - \text{sgn}(\delta_m^{b_2})}{2} + \sum_{m=1}^{n_{d_1}} \text{sgn}(v_m^{d_1}) \frac{1 - \text{sgn}(\delta_m^{d_1})}{2} \\
& + \sum_{m=1}^{n_{d_2}} \text{sgn}(v_m^{d_2}) \frac{1 - \text{sgn}(\delta_m^{d_2})}{2} + \sum_{m=1}^{n_{d_3}} \text{sgn}(v_m^{d_3}) \frac{1 - \text{sgn}(\delta_m^{d_3})}{2} + \sum_{m=1}^{n_{d_4}} \text{sgn}(v_m^{d_4}) \frac{1 - \text{sgn}(\delta_m^{d_4})}{2} \\
& - \sum_{m=1}^{n_{f_1}} \text{sgn}(v_m^{f_1}) \frac{1 - \text{sgn}(\delta_m^{f_1})}{2} - \sum_{m=1}^{n_{f_2}} \text{sgn}(v_m^{f_2}) \frac{1 - \text{sgn}(\delta_m^{f_2})}{2}
\end{aligned} \tag{S207.2}$$

$$\begin{aligned}
\mathcal{W}_3^{\text{gapless}} = & \sum_{m=1}^{n_{c_1}} \text{sgn}(v_m^{c_1}) \frac{1 - \text{sgn}(\delta_m^{c_1})}{2} + \sum_{m=1}^{n_{c_2}} \text{sgn}(v_m^{c_2}) \frac{1 - \text{sgn}(\delta_m^{c_2})}{2} + \sum_{m=1}^{n_{d_1}} \text{sgn}(v_m^{d_1}) \frac{1 - \text{sgn}(\delta_m^{d_1})}{2} \\
& + \sum_{m=1}^{n_{d_2}} \text{sgn}(v_m^{d_2}) \frac{1 - \text{sgn}(\delta_m^{d_2})}{2} + \sum_{m=1}^{n_{d_3}} \text{sgn}(v_m^{d_3}) \frac{1 - \text{sgn}(\delta_m^{d_3})}{2} + \sum_{m=1}^{n_{d_4}} \text{sgn}(v_m^{d_4}) \frac{1 - \text{sgn}(\delta_m^{d_4})}{2} \\
& - \sum_{m=1}^{n_{e_1}} \text{sgn}(v_m^{e_1}) \frac{1 - \text{sgn}(\delta_m^{e_1})}{2} - \sum_{m=1}^{n_{e_2}} \text{sgn}(v_m^{e_2}) \frac{1 - \text{sgn}(\delta_m^{e_2})}{2} - \sum_{m=1}^{n_{e_3}} \text{sgn}(v_m^{e_3}) \frac{1 - \text{sgn}(\delta_m^{e_3})}{2}
\end{aligned} \tag{S207.3}$$

$$\mathcal{W}_1^{\text{gapped}} = - \sum_{m=1}^{n_{d_1}} \text{sgn}(v_m^{d_1}) \frac{1 - \text{sgn}(\delta_m^{d_1})}{2} + \sum_{m=1}^{n_{d_2}} \text{sgn}(v_m^{d_2}) \frac{1 - \text{sgn}(\delta_m^{d_2})}{2} \tag{S207.4}$$

$$\mathcal{W}_2^{\text{gapped}} = \sum_{m=1}^{n_{a_3}} \text{sgn}(v_m^{a_3}) \frac{1 - \text{sgn}(\delta_m^{a_3})}{2} - \sum_{m=1}^{n_{a_4}} \text{sgn}(v_m^{a_4}) \frac{1 - \text{sgn}(\delta_m^{a_4})}{2} \tag{S207.5}$$

$$\mathcal{W}_3^{\text{gapped}} = - \sum_{m=1}^{n_{d_3}} \text{sgn}(v_m^{d_3}) \frac{1 - \text{sgn}(\delta_m^{d_3})}{2} + \sum_{m=1}^{n_{d_4}} \text{sgn}(v_m^{d_4}) \frac{1 - \text{sgn}(\delta_m^{d_4})}{2} \tag{S207.6}$$

$$\mathcal{W}_4^{\text{gapped}} = \sum_{m=1}^{n_{a_2}} \text{sgn}(v_m^{a_2}) \frac{1 - \text{sgn}(\delta_m^{a_2})}{2} + \sum_{m=1}^{n_{a_4}} \text{sgn}(v_m^{a_4}) \frac{1 - \text{sgn}(\delta_m^{a_4})}{2} + \sum_{m=1}^{n_{b_2}} \text{sgn}(v_m^{b_2}) \frac{1 - \text{sgn}(\delta_m^{b_2})}{2} - \sum_{m=1}^{n_{c_2}} \text{sgn}(v_m^{c_2}) \frac{1 - \text{sgn}(\delta_m^{c_2})}{2} \quad (\text{S207.7})$$

$$\begin{aligned} \mathcal{W}_5^{\text{gapped}} = & -2 \sum_{m=1}^{n_{c_2}} \text{sgn}(v_m^{c_2}) \frac{1 - \text{sgn}(\delta_m^{c_2})}{2} - 2 \sum_{m=1}^{n_{d_1}} \text{sgn}(v_m^{d_1}) \frac{1 - \text{sgn}(\delta_m^{d_1})}{2} - 2 \sum_{m=1}^{n_{d_3}} \text{sgn}(v_m^{d_3}) \frac{1 - \text{sgn}(\delta_m^{d_3})}{2} \\ & + \sum_{m=1}^{n_{e_1}} \text{sgn}(v_m^{e_1}) \frac{1 - \text{sgn}(\delta_m^{e_1})}{2} + \sum_{m=1}^{n_{e_2}} \text{sgn}(v_m^{e_2}) \frac{1 - \text{sgn}(\delta_m^{e_2})}{2} + \sum_{m=1}^{n_{e_3}} \text{sgn}(v_m^{e_3}) \frac{1 - \text{sgn}(\delta_m^{e_3})}{2} \end{aligned} \quad (\text{S207.8})$$

$$\begin{aligned} \mathcal{W}_6^{\text{gapped}} = & -2 \sum_{m=1}^{n_{c_2}} \text{sgn}(v_m^{c_2}) \frac{1 - \text{sgn}(\delta_m^{c_2})}{2} - 2 \sum_{m=1}^{n_{d_1}} \text{sgn}(v_m^{d_1}) \frac{1 - \text{sgn}(\delta_m^{d_1})}{2} \\ & - 2 \sum_{m=1}^{n_{d_3}} \text{sgn}(v_m^{d_3}) \frac{1 - \text{sgn}(\delta_m^{d_3})}{2} + \sum_{m=1}^{n_{e_1}} \text{sgn}(v_m^{e_1}) \frac{1 - \text{sgn}(\delta_m^{e_1})}{2} + 2 \sum_{m=1}^{n_{e_3}} \text{sgn}(v_m^{e_3}) \frac{1 - \text{sgn}(\delta_m^{e_3})}{2} \end{aligned} \quad (\text{S207.9})$$

$$\begin{aligned} \mathcal{W}_7^{\text{gapped}} = & \sum_{m=1}^{n_{a_2}} \text{sgn}(v_m^{a_2}) \frac{1 - \text{sgn}(\delta_m^{a_2})}{2} + \sum_{m=1}^{n_{a_4}} \text{sgn}(v_m^{a_4}) \frac{1 - \text{sgn}(\delta_m^{a_4})}{2} - \sum_{m=1}^{n_{c_2}} \text{sgn}(v_m^{c_2}) \frac{1 - \text{sgn}(\delta_m^{c_2})}{2} \\ & - \sum_{m=1}^{n_{d_1}} \text{sgn}(v_m^{d_1}) \frac{1 - \text{sgn}(\delta_m^{d_1})}{2} - \sum_{m=1}^{n_{d_3}} \text{sgn}(v_m^{d_3}) \frac{1 - \text{sgn}(\delta_m^{d_3})}{2} + \sum_{m=1}^{n_{f_1}} \text{sgn}(v_m^{f_1}) \frac{1 - \text{sgn}(\delta_m^{f_1})}{2} \end{aligned} \quad (\text{S207.10})$$

$$\begin{aligned} \mathcal{W}_8^{\text{gapped}} = & \sum_{m=1}^{n_{a_2}} \text{sgn}(v_m^{a_2}) \frac{1 - \text{sgn}(\delta_m^{a_2})}{2} + \sum_{m=1}^{n_{a_4}} \text{sgn}(v_m^{a_4}) \frac{1 - \text{sgn}(\delta_m^{a_4})}{2} - \sum_{m=1}^{n_{c_2}} \text{sgn}(v_m^{c_2}) \frac{1 - \text{sgn}(\delta_m^{c_2})}{2} \\ & - \sum_{m=1}^{n_{d_1}} \text{sgn}(v_m^{d_1}) \frac{1 - \text{sgn}(\delta_m^{d_1})}{2} - \sum_{m=1}^{n_{d_3}} \text{sgn}(v_m^{d_3}) \frac{1 - \text{sgn}(\delta_m^{d_3})}{2} + \sum_{m=1}^{n_{f_2}} \text{sgn}(v_m^{f_2}) \frac{1 - \text{sgn}(\delta_m^{f_2})}{2} \end{aligned} \quad (\text{S207.11})$$

## S208. SPACE GROUP NO. 208

| line segment                                      | character of irrep (generators only)                                                                                                                                                                                                                                                        |
|---------------------------------------------------|---------------------------------------------------------------------------------------------------------------------------------------------------------------------------------------------------------------------------------------------------------------------------------------------|
| $a \quad (\frac{t}{2}, 0, 0)$                     | $\{4_{100}   \frac{1}{2} \frac{1}{2} \frac{1}{2}\}$<br>$a_1 \quad e^{-\frac{1}{2}i\pi t - \frac{3i\pi}{4}}$<br>$a_2 \quad e^{\frac{3i\pi}{4} - \frac{i\pi t}{2}}$<br>$a_3 \quad e^{-\frac{1}{2}i\pi t - \frac{i\pi}{4}}$<br>$a_4 \quad e^{\frac{i\pi}{4} - \frac{i\pi t}{2}}$               |
| $b \quad (\frac{1}{2}, \frac{t}{2}, 0)$           | $\{2_{010}   0 \ 0 \ 0\}$<br>$b_1 \quad -i$<br>$b_2 \quad i$                                                                                                                                                                                                                                |
| $c \quad (\frac{t}{2}, \frac{t}{2}, 0)$           | $\{2_{110}   \frac{1}{2} \frac{1}{2} \frac{1}{2}\}$<br>$c_1 \quad -ie^{-i\pi t}$<br>$c_2 \quad ie^{-i\pi t}$                                                                                                                                                                                |
| $d \quad (\frac{1}{2}, \frac{1}{2}, \frac{t}{2})$ | $\{4_{001}   \frac{1}{2} \frac{1}{2} \frac{1}{2}\}$<br>$d_1 \quad e^{-\frac{1}{2}i\pi(t+2) - \frac{3i\pi}{4}}$<br>$d_2 \quad e^{\frac{3i\pi}{4} - \frac{1}{2}i\pi(t+2)}$<br>$d_3 \quad e^{-\frac{1}{2}i\pi(t+2) - \frac{i\pi}{4}}$<br>$d_4 \quad e^{\frac{i\pi}{4} - \frac{1}{2}i\pi(t+2)}$ |



|                                                   |       |                                                         |
|---------------------------------------------------|-------|---------------------------------------------------------|
| $e \quad (\frac{t}{2}, \frac{t}{2}, \frac{t}{2})$ | $e_1$ | $\{3_{111}   0 \ 0 \ 0\}$                               |
|                                                   | $e_2$ | $-1$                                                    |
|                                                   | $e_3$ | $e^{-\frac{i\pi}{3}}$                                   |
|                                                   |       | $e^{\frac{i\pi}{3}}$                                    |
| $f \quad (\frac{1}{2}, \frac{t}{2}, \frac{t}{2})$ | $f_1$ | $\{2_{011}   \frac{1}{2} \ \frac{1}{2} \ \frac{1}{2}\}$ |
|                                                   | $f_2$ | $-e^{-\frac{1}{2}i\pi(2t+1)}$                           |
|                                                   |       | $e^{-\frac{1}{2}i\pi(2t+1)}$                            |

$$\begin{aligned}
\mathcal{W}_1^{\text{gapless}} = & \sum_{m=1}^{n_{a_1}} \text{sgn}(v_m^{a_1}) \frac{1 - \text{sgn}(\delta_m^{a_1})}{2} + \sum_{m=1}^{n_{a_2}} \text{sgn}(v_m^{a_2}) \frac{1 - \text{sgn}(\delta_m^{a_2})}{2} + \sum_{m=1}^{n_{a_3}} \text{sgn}(v_m^{a_3}) \frac{1 - \text{sgn}(\delta_m^{a_3})}{2} \\
& + \sum_{m=1}^{n_{a_4}} \text{sgn}(v_m^{a_4}) \frac{1 - \text{sgn}(\delta_m^{a_4})}{2} - \sum_{m=1}^{n_{e_1}} \text{sgn}(v_m^{e_1}) \frac{1 - \text{sgn}(\delta_m^{e_1})}{2} - \sum_{m=1}^{n_{e_2}} \text{sgn}(v_m^{e_2}) \frac{1 - \text{sgn}(\delta_m^{e_2})}{2} \\
& - \sum_{m=1}^{n_{e_3}} \text{sgn}(v_m^{e_3}) \frac{1 - \text{sgn}(\delta_m^{e_3})}{2} + \sum_{m=1}^{n_{f_1}} \text{sgn}(v_m^{f_1}) \frac{1 - \text{sgn}(\delta_m^{f_1})}{2} + \sum_{m=1}^{n_{f_2}} \text{sgn}(v_m^{f_2}) \frac{1 - \text{sgn}(\delta_m^{f_2})}{2}
\end{aligned} \tag{S208.1}$$

$$\begin{aligned}
\mathcal{W}_2^{\text{gapless}} = & \sum_{m=1}^{n_{b_1}} \text{sgn}(v_m^{b_1}) \frac{1 - \text{sgn}(\delta_m^{b_1})}{2} + \sum_{m=1}^{n_{b_2}} \text{sgn}(v_m^{b_2}) \frac{1 - \text{sgn}(\delta_m^{b_2})}{2} + \sum_{m=1}^{n_{d_1}} \text{sgn}(v_m^{d_1}) \frac{1 - \text{sgn}(\delta_m^{d_1})}{2} \\
& + \sum_{m=1}^{n_{d_2}} \text{sgn}(v_m^{d_2}) \frac{1 - \text{sgn}(\delta_m^{d_2})}{2} + \sum_{m=1}^{n_{d_3}} \text{sgn}(v_m^{d_3}) \frac{1 - \text{sgn}(\delta_m^{d_3})}{2} + \sum_{m=1}^{n_{d_4}} \text{sgn}(v_m^{d_4}) \frac{1 - \text{sgn}(\delta_m^{d_4})}{2} \\
& - \sum_{m=1}^{n_{f_1}} \text{sgn}(v_m^{f_1}) \frac{1 - \text{sgn}(\delta_m^{f_1})}{2} - \sum_{m=1}^{n_{f_2}} \text{sgn}(v_m^{f_2}) \frac{1 - \text{sgn}(\delta_m^{f_2})}{2}
\end{aligned} \tag{S208.2}$$

$$\begin{aligned}
\mathcal{W}_3^{\text{gapless}} = & \sum_{m=1}^{n_{c_1}} \text{sgn}(v_m^{c_1}) \frac{1 - \text{sgn}(\delta_m^{c_1})}{2} + \sum_{m=1}^{n_{c_2}} \text{sgn}(v_m^{c_2}) \frac{1 - \text{sgn}(\delta_m^{c_2})}{2} + \sum_{m=1}^{n_{d_1}} \text{sgn}(v_m^{d_1}) \frac{1 - \text{sgn}(\delta_m^{d_1})}{2} \\
& + \sum_{m=1}^{n_{d_2}} \text{sgn}(v_m^{d_2}) \frac{1 - \text{sgn}(\delta_m^{d_2})}{2} + \sum_{m=1}^{n_{d_3}} \text{sgn}(v_m^{d_3}) \frac{1 - \text{sgn}(\delta_m^{d_3})}{2} + \sum_{m=1}^{n_{d_4}} \text{sgn}(v_m^{d_4}) \frac{1 - \text{sgn}(\delta_m^{d_4})}{2} \\
& - \sum_{m=1}^{n_{e_1}} \text{sgn}(v_m^{e_1}) \frac{1 - \text{sgn}(\delta_m^{e_1})}{2} - \sum_{m=1}^{n_{e_2}} \text{sgn}(v_m^{e_2}) \frac{1 - \text{sgn}(\delta_m^{e_2})}{2} - \sum_{m=1}^{n_{e_3}} \text{sgn}(v_m^{e_3}) \frac{1 - \text{sgn}(\delta_m^{e_3})}{2}
\end{aligned} \tag{S208.3}$$

$$\begin{aligned}
\mathcal{W}_1^{\text{gapped}} = & \sum_{m=1}^{n_{d_1}} \text{sgn}(v_m^{d_1}) \frac{1 - \text{sgn}(\delta_m^{d_1})}{2} - \sum_{m=1}^{n_{d_2}} \text{sgn}(v_m^{d_2}) \frac{1 - \text{sgn}(\delta_m^{d_2})}{2} - \sum_{m=1}^{n_{d_3}} \text{sgn}(v_m^{d_3}) \frac{1 - \text{sgn}(\delta_m^{d_3})}{2} + \sum_{m=1}^{n_{d_4}} \text{sgn}(v_m^{d_4}) \frac{1 - \text{sgn}(\delta_m^{d_4})}{2}
\end{aligned} \tag{S208.4}$$

$$\begin{aligned}
\mathcal{W}_2^{\text{gapped}} = & \sum_{m=1}^{n_{a_2}} \text{sgn}(v_m^{a_2}) \frac{1 - \text{sgn}(\delta_m^{a_2})}{2} + \sum_{m=1}^{n_{a_3}} \text{sgn}(v_m^{a_3}) \frac{1 - \text{sgn}(\delta_m^{a_3})}{2} + \sum_{m=1}^{n_{b_2}} \text{sgn}(v_m^{b_2}) \frac{1 - \text{sgn}(\delta_m^{b_2})}{2} - \sum_{m=1}^{n_{c_2}} \text{sgn}(v_m^{c_2}) \frac{1 - \text{sgn}(\delta_m^{c_2})}{2}
\end{aligned} \tag{S208.5}$$

$$\begin{aligned}\mathcal{W}_3^{\text{gapped}} = & -2 \sum_{m=1}^{n_{c_2}} \text{sgn}(v_m^{c_2}) \frac{1 - \text{sgn}(\delta_m^{c_2})}{2} - 2 \sum_{m=1}^{n_{d_2}} \text{sgn}(v_m^{d_2}) \frac{1 - \text{sgn}(\delta_m^{d_2})}{2} - 2 \sum_{m=1}^{n_{d_3}} \text{sgn}(v_m^{d_3}) \frac{1 - \text{sgn}(\delta_m^{d_3})}{2} \\ & + \sum_{m=1}^{n_{e_1}} \text{sgn}(v_m^{e_1}) \frac{1 - \text{sgn}(\delta_m^{e_1})}{2} + \sum_{m=1}^{n_{e_2}} \text{sgn}(v_m^{e_2}) \frac{1 - \text{sgn}(\delta_m^{e_2})}{2} + \sum_{m=1}^{n_{e_3}} \text{sgn}(v_m^{e_3}) \frac{1 - \text{sgn}(\delta_m^{e_3})}{2}\end{aligned}\quad (\text{S208.6})$$

$$\begin{aligned}\mathcal{W}_4^{\text{gapped}} = & -2 \sum_{m=1}^{n_{c_2}} \text{sgn}(v_m^{c_2}) \frac{1 - \text{sgn}(\delta_m^{c_2})}{2} - 2 \sum_{m=1}^{n_{d_2}} \text{sgn}(v_m^{d_2}) \frac{1 - \text{sgn}(\delta_m^{d_2})}{2} \\ & - 2 \sum_{m=1}^{n_{d_3}} \text{sgn}(v_m^{d_3}) \frac{1 - \text{sgn}(\delta_m^{d_3})}{2} + \sum_{m=1}^{n_{e_1}} \text{sgn}(v_m^{e_1}) \frac{1 - \text{sgn}(\delta_m^{e_1})}{2} + 2 \sum_{m=1}^{n_{e_3}} \text{sgn}(v_m^{e_3}) \frac{1 - \text{sgn}(\delta_m^{e_3})}{2}\end{aligned}\quad (\text{S208.7})$$

$$\begin{aligned}\mathcal{W}_5^{\text{gapped}} = & \sum_{m=1}^{n_{a_2}} \text{sgn}(v_m^{a_2}) \frac{1 - \text{sgn}(\delta_m^{a_2})}{2} + \sum_{m=1}^{n_{a_3}} \text{sgn}(v_m^{a_3}) \frac{1 - \text{sgn}(\delta_m^{a_3})}{2} - \sum_{m=1}^{n_{c_2}} \text{sgn}(v_m^{c_2}) \frac{1 - \text{sgn}(\delta_m^{c_2})}{2} \\ & - \sum_{m=1}^{n_{d_2}} \text{sgn}(v_m^{d_2}) \frac{1 - \text{sgn}(\delta_m^{d_2})}{2} - \sum_{m=1}^{n_{d_3}} \text{sgn}(v_m^{d_3}) \frac{1 - \text{sgn}(\delta_m^{d_3})}{2} + \sum_{m=1}^{n_{f_1}} \text{sgn}(v_m^{f_1}) \frac{1 - \text{sgn}(\delta_m^{f_1})}{2}\end{aligned}\quad (\text{S208.8})$$

$$\begin{aligned}\mathcal{W}_6^{\text{gapped}} = & \sum_{m=1}^{n_{a_2}} \text{sgn}(v_m^{a_2}) \frac{1 - \text{sgn}(\delta_m^{a_2})}{2} + \sum_{m=1}^{n_{a_3}} \text{sgn}(v_m^{a_3}) \frac{1 - \text{sgn}(\delta_m^{a_3})}{2} - \sum_{m=1}^{n_{c_2}} \text{sgn}(v_m^{c_2}) \frac{1 - \text{sgn}(\delta_m^{c_2})}{2} \\ & - \sum_{m=1}^{n_{d_2}} \text{sgn}(v_m^{d_2}) \frac{1 - \text{sgn}(\delta_m^{d_2})}{2} - \sum_{m=1}^{n_{d_3}} \text{sgn}(v_m^{d_3}) \frac{1 - \text{sgn}(\delta_m^{d_3})}{2} + \sum_{m=1}^{n_{f_2}} \text{sgn}(v_m^{f_2}) \frac{1 - \text{sgn}(\delta_m^{f_2})}{2}\end{aligned}\quad (\text{S208.9})$$

$$\mathcal{X}_1 = \sum_{m=1}^{n_{a_2}} \frac{1 - \text{sgn}(\delta_m^{a_2})}{2} + \sum_{m=1}^{n_{a_4}} \frac{1 - \text{sgn}(\delta_m^{a_4})}{2} + \sum_{m=1}^{n_{c_2}} \frac{1 - \text{sgn}(\delta_m^{c_2})}{2} + \sum_{m=1}^{n_{d_1}} \frac{1 - \text{sgn}(\delta_m^{d_1})}{2} + \sum_{m=1}^{n_{d_3}} \frac{1 - \text{sgn}(\delta_m^{d_3})}{2} \pmod{2} \quad (\text{S208.10})$$

## S209. SPACE GROUP NO. 209

| line segment                                      | character of irrep (generators only) |
|---------------------------------------------------|--------------------------------------|
| $a \quad (0, t, 0)$                               | $\{4_{010}   0 \ 0 \ 0\}$            |
|                                                   | $a_1 \quad e^{-\frac{3i\pi}{4}}$     |
|                                                   | $a_2 \quad e^{\frac{3i\pi}{4}}$      |
|                                                   | $a_3 \quad e^{-\frac{i\pi}{4}}$      |
| $b \quad (t, t, 0)$                               | $e^{\frac{i\pi}{4}}$                 |
|                                                   | $a_4$                                |
| $b \quad (t, t, 0)$                               | $\{2_{110}   0 \ 0 \ 0\}$            |
|                                                   | $b_1 \quad -i$                       |
|                                                   | $b_2 \quad i$                        |
| $c \quad (\frac{t}{2}, 1, 0)$                     | $\{2_{100}   0 \ 0 \ 0\}$            |
|                                                   | $c_1 \quad -i$                       |
| $d \quad (\frac{t}{2}, \frac{t}{2}, \frac{t}{2})$ | $c_2 \quad i$                        |
|                                                   | $\{3_{111}   0 \ 0 \ 0\}$            |
|                                                   | $d_1 \quad -1$                       |
|                                                   | $d_2 \quad e^{-\frac{i\pi}{3}}$      |
|                                                   | $d_3 \quad e^{\frac{i\pi}{3}}$       |

|     |                                                   |                |                                   |
|-----|---------------------------------------------------|----------------|-----------------------------------|
| $e$ | $(1 - \frac{t}{2}, 1 - \frac{t}{2}, \frac{t}{2})$ | $e_1$          | $\{1 0\ 0\ 0\}$<br>1              |
| $f$ | $(\frac{1}{2}, 1 - \frac{t}{2}, \frac{t}{2})$     | $f_1$<br>$f_2$ | $\{2_{01-1} 0\ 0\ 0\}$<br>-i<br>i |

$$\begin{aligned} \mathcal{W}_1^{\text{gapless}} = & \sum_{m=1}^{n_{a_1}} \text{sgn}(v_m^{a_1}) \frac{1 - \text{sgn}(\delta_m^{a_1})}{2} + \sum_{m=1}^{n_{a_2}} \text{sgn}(v_m^{a_2}) \frac{1 - \text{sgn}(\delta_m^{a_2})}{2} + \sum_{m=1}^{n_{a_3}} \text{sgn}(v_m^{a_3}) \frac{1 - \text{sgn}(\delta_m^{a_3})}{2} \\ & + \sum_{m=1}^{n_{a_4}} \text{sgn}(v_m^{a_4}) \frac{1 - \text{sgn}(\delta_m^{a_4})}{2} - \sum_{m=1}^{n_{d_1}} \text{sgn}(v_m^{d_1}) \frac{1 - \text{sgn}(\delta_m^{d_1})}{2} - \sum_{m=1}^{n_{d_2}} \text{sgn}(v_m^{d_2}) \frac{1 - \text{sgn}(\delta_m^{d_2})}{2} \\ & - \sum_{m=1}^{n_{d_3}} \text{sgn}(v_m^{d_3}) \frac{1 - \text{sgn}(\delta_m^{d_3})}{2} + \sum_{m=1}^{n_{e_1}} \text{sgn}(v_m^{e_1}) \frac{1 - \text{sgn}(\delta_m^{e_1})}{2} \end{aligned} \quad (\text{S209.1})$$

$$\begin{aligned} \mathcal{W}_2^{\text{gapless}} = & \sum_{m=1}^{n_{b_1}} \text{sgn}(v_m^{b_1}) \frac{1 - \text{sgn}(\delta_m^{b_1})}{2} + \sum_{m=1}^{n_{b_2}} \text{sgn}(v_m^{b_2}) \frac{1 - \text{sgn}(\delta_m^{b_2})}{2} - \sum_{m=1}^{n_{d_1}} \text{sgn}(v_m^{d_1}) \frac{1 - \text{sgn}(\delta_m^{d_1})}{2} \\ & - \sum_{m=1}^{n_{d_2}} \text{sgn}(v_m^{d_2}) \frac{1 - \text{sgn}(\delta_m^{d_2})}{2} - \sum_{m=1}^{n_{d_3}} \text{sgn}(v_m^{d_3}) \frac{1 - \text{sgn}(\delta_m^{d_3})}{2} + \sum_{m=1}^{n_{e_1}} \text{sgn}(v_m^{e_1}) \frac{1 - \text{sgn}(\delta_m^{e_1})}{2} \end{aligned} \quad (\text{S209.2})$$

$$\begin{aligned} \mathcal{W}_3^{\text{gapless}} = & \sum_{m=1}^{n_{c_1}} \text{sgn}(v_m^{c_1}) \frac{1 - \text{sgn}(\delta_m^{c_1})}{2} + \sum_{m=1}^{n_{c_2}} \text{sgn}(v_m^{c_2}) \frac{1 - \text{sgn}(\delta_m^{c_2})}{2} - \sum_{m=1}^{n_{e_1}} \text{sgn}(v_m^{e_1}) \frac{1 - \text{sgn}(\delta_m^{e_1})}{2} \\ & + \sum_{m=1}^{n_{f_1}} \text{sgn}(v_m^{f_1}) \frac{1 - \text{sgn}(\delta_m^{f_1})}{2} + \sum_{m=1}^{n_{f_2}} \text{sgn}(v_m^{f_2}) \frac{1 - \text{sgn}(\delta_m^{f_2})}{2} \end{aligned} \quad (\text{S209.3})$$

$$\mathcal{W}_1^{\text{gapped}} = - \sum_{m=1}^{n_{a_2}} \text{sgn}(v_m^{a_2}) \frac{1 - \text{sgn}(\delta_m^{a_2})}{2} - \sum_{m=1}^{n_{a_4}} \text{sgn}(v_m^{a_4}) \frac{1 - \text{sgn}(\delta_m^{a_4})}{2} + \sum_{m=1}^{n_{b_2}} \text{sgn}(v_m^{b_2}) \frac{1 - \text{sgn}(\delta_m^{b_2})}{2} \quad (\text{S209.4})$$

$$\mathcal{W}_2^{\text{gapped}} = \sum_{m=1}^{n_{a_3}} \text{sgn}(v_m^{a_3}) \frac{1 - \text{sgn}(\delta_m^{a_3})}{2} - \sum_{m=1}^{n_{a_4}} \text{sgn}(v_m^{a_4}) \frac{1 - \text{sgn}(\delta_m^{a_4})}{2} \quad (\text{S209.5})$$

$$\mathcal{W}_3^{\text{gapped}} = - \sum_{m=1}^{n_{d_2}} \text{sgn}(v_m^{d_2}) \frac{1 - \text{sgn}(\delta_m^{d_2})}{2} + \sum_{m=1}^{n_{d_3}} \text{sgn}(v_m^{d_3}) \frac{1 - \text{sgn}(\delta_m^{d_3})}{2} \quad (\text{S209.6})$$

$$\begin{aligned} \mathcal{W}_4^{\text{gapped}} = & 2 \sum_{m=1}^{n_{a_2}} \text{sgn}(v_m^{a_2}) \frac{1 - \text{sgn}(\delta_m^{a_2})}{2} + 2 \sum_{m=1}^{n_{a_4}} \text{sgn}(v_m^{a_4}) \frac{1 - \text{sgn}(\delta_m^{a_4})}{2} - \sum_{m=1}^{n_{d_1}} \text{sgn}(v_m^{d_1}) \frac{1 - \text{sgn}(\delta_m^{d_1})}{2} \\ & - 2 \sum_{m=1}^{n_{d_2}} \text{sgn}(v_m^{d_2}) \frac{1 - \text{sgn}(\delta_m^{d_2})}{2} + \sum_{m=1}^{n_{e_1}} \text{sgn}(v_m^{e_1}) \frac{1 - \text{sgn}(\delta_m^{e_1})}{2} \end{aligned} \quad (\text{S209.7})$$

$$\begin{aligned}
\mathcal{W}_5^{\text{gapped}} = & 2 \sum_{m=1}^{n_{a_2}} \text{sgn}(v_m^{a_2}) \frac{1 - \text{sgn}(\delta_m^{a_2})}{2} + 2 \sum_{m=1}^{n_{a_4}} \text{sgn}(v_m^{a_4}) \frac{1 - \text{sgn}(\delta_m^{a_4})}{2} + 2 \sum_{m=1}^{n_{c_2}} \text{sgn}(v_m^{c_2}) \frac{1 - \text{sgn}(\delta_m^{c_2})}{2} \\
& - \sum_{m=1}^{n_{d_1}} \text{sgn}(v_m^{d_1}) \frac{1 - \text{sgn}(\delta_m^{d_1})}{2} - 2 \sum_{m=1}^{n_{d_2}} \text{sgn}(v_m^{d_2}) \frac{1 - \text{sgn}(\delta_m^{d_2})}{2} + \sum_{m=1}^{n_{f_1}} \text{sgn}(v_m^{f_1}) \frac{1 - \text{sgn}(\delta_m^{f_1})}{2} \\
& + \sum_{m=1}^{n_{f_2}} \text{sgn}(v_m^{f_2}) \frac{1 - \text{sgn}(\delta_m^{f_2})}{2}
\end{aligned} \tag{S209.8}$$

$$\begin{aligned}
\mathcal{W}_6^{\text{gapped}} = & 2 \sum_{m=1}^{n_{a_2}} \text{sgn}(v_m^{a_2}) \frac{1 - \text{sgn}(\delta_m^{a_2})}{2} + 2 \sum_{m=1}^{n_{a_4}} \text{sgn}(v_m^{a_4}) \frac{1 - \text{sgn}(\delta_m^{a_4})}{2} + 2 \sum_{m=1}^{n_{c_2}} \text{sgn}(v_m^{c_2}) \frac{1 - \text{sgn}(\delta_m^{c_2})}{2} \\
& - \sum_{m=1}^{n_{d_1}} \text{sgn}(v_m^{d_1}) \frac{1 - \text{sgn}(\delta_m^{d_1})}{2} - 2 \sum_{m=1}^{n_{d_2}} \text{sgn}(v_m^{d_2}) \frac{1 - \text{sgn}(\delta_m^{d_2})}{2} + 2 \sum_{m=1}^{n_{f_2}} \text{sgn}(v_m^{f_2}) \frac{1 - \text{sgn}(\delta_m^{f_2})}{2}
\end{aligned} \tag{S209.9}$$

### S210. SPACE GROUP NO. 210

| line segment                                          | character of irrep (generators only)                                                                                                                                                                                                                               |
|-------------------------------------------------------|--------------------------------------------------------------------------------------------------------------------------------------------------------------------------------------------------------------------------------------------------------------------|
| $a \ (0, t, 0)$                                       | $\{4_{010}   \frac{1}{4} \ \frac{1}{4} \ \frac{1}{4} \}$<br>$a_1 \ e^{-\frac{1}{2}i\pi t - \frac{3i\pi}{4}}$<br>$a_2 \ e^{\frac{3i\pi}{4} - \frac{i\pi t}{2}}$<br>$a_3 \ e^{-\frac{1}{2}i\pi t - \frac{i\pi}{4}}$<br>$a_4 \ e^{\frac{i\pi}{4} - \frac{i\pi t}{2}}$ |
| $b \ (t, t, 0)$                                       | $\{2_{110}   \frac{1}{4} \ \frac{1}{4} \ \frac{1}{4} \}$<br>$b_1 \ -ie^{-i\pi t}$<br>$b_2 \ ie^{-i\pi t}$                                                                                                                                                          |
| $c \ (\frac{t}{2}, 1, 0)$                             | $\{2_{100}   0 \ 0 \ 0 \}$<br>$c_1 \ -i$<br>$c_2 \ i$                                                                                                                                                                                                              |
| $d \ (\frac{t}{2}, \frac{t}{2}, \frac{t}{2})$         | $\{3_{111}   0 \ 0 \ 0 \}$<br>$d_1 \ -1$<br>$d_2 \ e^{-\frac{i\pi}{3}}$<br>$d_3 \ e^{\frac{i\pi}{3}}$                                                                                                                                                              |
| $e \ (1 - \frac{t}{2}, 1 - \frac{t}{2}, \frac{t}{2})$ | $\{1   0 \ 0 \ 0 \}$<br>$e_1 \ 1$                                                                                                                                                                                                                                  |
| $f \ (\frac{1}{2}, 1 - \frac{t}{2}, \frac{t}{2})$     | $\{2_{01-1}   \frac{1}{4} \ \frac{1}{4} \ \frac{1}{4} \}$<br>$f_1 \ i$<br>$f_2 \ -i$                                                                                                                                                                               |

$$\begin{aligned}
\mathcal{W}_1^{\text{gapless}} = & \sum_{m=1}^{n_{a_1}} \text{sgn}(v_m^{a_1}) \frac{1 - \text{sgn}(\delta_m^{a_1})}{2} + \sum_{m=1}^{n_{a_2}} \text{sgn}(v_m^{a_2}) \frac{1 - \text{sgn}(\delta_m^{a_2})}{2} + \sum_{m=1}^{n_{a_3}} \text{sgn}(v_m^{a_3}) \frac{1 - \text{sgn}(\delta_m^{a_3})}{2} \\
& + \sum_{m=1}^{n_{a_4}} \text{sgn}(v_m^{a_4}) \frac{1 - \text{sgn}(\delta_m^{a_4})}{2} - \sum_{m=1}^{n_{d_1}} \text{sgn}(v_m^{d_1}) \frac{1 - \text{sgn}(\delta_m^{d_1})}{2} - \sum_{m=1}^{n_{d_2}} \text{sgn}(v_m^{d_2}) \frac{1 - \text{sgn}(\delta_m^{d_2})}{2} \\
& - \sum_{m=1}^{n_{d_3}} \text{sgn}(v_m^{d_3}) \frac{1 - \text{sgn}(\delta_m^{d_3})}{2} + \sum_{m=1}^{n_{e_1}} \text{sgn}(v_m^{e_1}) \frac{1 - \text{sgn}(\delta_m^{e_1})}{2}
\end{aligned} \tag{S210.1}$$

$$\begin{aligned} \mathcal{W}_2^{\text{gapless}} = & \sum_{m=1}^{n_{b_1}} \text{sgn}(v_m^{b_1}) \frac{1 - \text{sgn}(\delta_m^{b_1})}{2} + \sum_{m=1}^{n_{b_2}} \text{sgn}(v_m^{b_2}) \frac{1 - \text{sgn}(\delta_m^{b_2})}{2} - \sum_{m=1}^{n_{d_1}} \text{sgn}(v_m^{d_1}) \frac{1 - \text{sgn}(\delta_m^{d_1})}{2} \\ & - \sum_{m=1}^{n_{d_2}} \text{sgn}(v_m^{d_2}) \frac{1 - \text{sgn}(\delta_m^{d_2})}{2} - \sum_{m=1}^{n_{d_3}} \text{sgn}(v_m^{d_3}) \frac{1 - \text{sgn}(\delta_m^{d_3})}{2} + \sum_{m=1}^{n_{e_1}} \text{sgn}(v_m^{e_1}) \frac{1 - \text{sgn}(\delta_m^{e_1})}{2} \end{aligned} \quad (\text{S210.2})$$

$$\begin{aligned} \mathcal{W}_3^{\text{gapless}} = & \sum_{m=1}^{n_{c_1}} \text{sgn}(v_m^{c_1}) \frac{1 - \text{sgn}(\delta_m^{c_1})}{2} + \sum_{m=1}^{n_{c_2}} \text{sgn}(v_m^{c_2}) \frac{1 - \text{sgn}(\delta_m^{c_2})}{2} - \sum_{m=1}^{n_{e_1}} \text{sgn}(v_m^{e_1}) \frac{1 - \text{sgn}(\delta_m^{e_1})}{2} \\ & + \sum_{m=1}^{n_{f_1}} \text{sgn}(v_m^{f_1}) \frac{1 - \text{sgn}(\delta_m^{f_1})}{2} + \sum_{m=1}^{n_{f_2}} \text{sgn}(v_m^{f_2}) \frac{1 - \text{sgn}(\delta_m^{f_2})}{2} \end{aligned} \quad (\text{S210.3})$$

$$\begin{aligned} \mathcal{W}_1^{\text{gapped}} = & 2 \sum_{m=1}^{n_{a_2}} \text{sgn}(v_m^{a_2}) \frac{1 - \text{sgn}(\delta_m^{a_2})}{2} + 2 \sum_{m=1}^{n_{a_3}} \text{sgn}(v_m^{a_3}) \frac{1 - \text{sgn}(\delta_m^{a_3})}{2} - \sum_{m=1}^{n_{d_1}} \text{sgn}(v_m^{d_1}) \frac{1 - \text{sgn}(\delta_m^{d_1})}{2} \\ & - 2 \sum_{m=1}^{n_{d_2}} \text{sgn}(v_m^{d_2}) \frac{1 - \text{sgn}(\delta_m^{d_2})}{2} + \sum_{m=1}^{n_{e_1}} \text{sgn}(v_m^{e_1}) \frac{1 - \text{sgn}(\delta_m^{e_1})}{2} \end{aligned} \quad (\text{S210.4})$$

$$\mathcal{W}_2^{\text{gapped}} = - \sum_{m=1}^{n_{d_2}} \text{sgn}(v_m^{d_2}) \frac{1 - \text{sgn}(\delta_m^{d_2})}{2} + \sum_{m=1}^{n_{d_3}} \text{sgn}(v_m^{d_3}) \frac{1 - \text{sgn}(\delta_m^{d_3})}{2} \quad (\text{S210.5})$$

$$\mathcal{W}_3^{\text{gapped}} = - \sum_{m=1}^{n_{a_2}} \text{sgn}(v_m^{a_2}) \frac{1 - \text{sgn}(\delta_m^{a_2})}{2} - \sum_{m=1}^{n_{a_3}} \text{sgn}(v_m^{a_3}) \frac{1 - \text{sgn}(\delta_m^{a_3})}{2} + \sum_{m=1}^{n_{b_2}} \text{sgn}(v_m^{b_2}) \frac{1 - \text{sgn}(\delta_m^{b_2})}{2} \quad (\text{S210.6})$$

$$\mathcal{X}_1 = \sum_{m=1}^{n_{a_3}} \frac{1 - \text{sgn}(\delta_m^{a_3})}{2} + \sum_{m=1}^{n_{a_4}} \frac{1 - \text{sgn}(\delta_m^{a_4})}{2} + \sum_{m=1}^{n_{c_2}} \frac{1 - \text{sgn}(\delta_m^{c_2})}{2} \quad \text{mod } 2 \quad (\text{S210.7})$$

$$\mathcal{X}_2 = \sum_{m=1}^{n_{a_3}} \frac{1 - \text{sgn}(\delta_m^{a_3})}{2} + \sum_{m=1}^{n_{a_4}} \frac{1 - \text{sgn}(\delta_m^{a_4})}{2} + \sum_{m=1}^{n_{c_2}} \frac{1 - \text{sgn}(\delta_m^{c_2})}{2} + \sum_{m=1}^{n_{d_1}} \frac{1 - \text{sgn}(\delta_m^{d_1})}{2} \quad \text{mod } 2 \quad (\text{S210.8})$$

## S211. SPACE GROUP NO. 211

| line segment                                | character of irrep (generators only) |
|---------------------------------------------|--------------------------------------|
| $a \quad (t, 0, 0)$                         | $\{4_{100}   0 \ 0 \ 0\}$            |
|                                             | $a_1 \quad e^{-\frac{3i\pi}{4}}$     |
|                                             | $a_2 \quad e^{\frac{3i\pi}{4}}$      |
|                                             | $a_3 \quad e^{-\frac{i\pi}{4}}$      |
|                                             | $a_4 \quad e^{\frac{i\pi}{4}}$       |
| $b \quad (\frac{t+1}{2}, \frac{1-t}{2}, 0)$ | $\{2_{1-10}   0 \ 0 \ 0\}$           |
|                                             | $b_1 \quad -i$<br>$b_2 \quad i$      |

|                                                              |                                                                                                                        |
|--------------------------------------------------------------|------------------------------------------------------------------------------------------------------------------------|
| $c \left( \frac{t}{2}, \frac{t}{2}, 0 \right)$               | $\{2_{110}   0 \ 0 \ 0 \}$<br>$c_1 \quad -i$<br>$c_2 \quad i$                                                          |
| $d \left( \frac{1}{2}, \frac{1}{2}, \frac{t}{2} \right)$     | $\{2_{001}   0 \ 0 \ 0 \}$<br>$d_1 \quad -i$<br>$d_2 \quad i$                                                          |
| $e \left( \frac{t}{2}, \frac{t}{2}, \frac{t}{2} \right)$     | $\{3_{111}   0 \ 0 \ 0 \}$<br>$e_1 \quad -1$<br>$e_2 \quad e^{-\frac{i\pi}{3}}$<br>$e_3 \quad e^{\frac{i\pi}{3}}$      |
| $f \left( 1 - \frac{t}{2}, \frac{t}{2}, \frac{t}{2} \right)$ | $\{3_{-1-1-1}^-   0 \ 0 \ 0 \}$<br>$f_1 \quad -1$<br>$f_2 \quad e^{-\frac{i\pi}{3}}$<br>$f_3 \quad e^{\frac{i\pi}{3}}$ |

$$\begin{aligned}
\mathcal{W}_1^{\text{gapless}} = & \sum_{m=1}^{n_{a_1}} \text{sgn}(v_m^{a_1}) \frac{1 - \text{sgn}(\delta_m^{a_1})}{2} + \sum_{m=1}^{n_{a_2}} \text{sgn}(v_m^{a_2}) \frac{1 - \text{sgn}(\delta_m^{a_2})}{2} + \sum_{m=1}^{n_{a_3}} \text{sgn}(v_m^{a_3}) \frac{1 - \text{sgn}(\delta_m^{a_3})}{2} + \sum_{m=1}^{n_{a_4}} \text{sgn}(v_m^{a_4}) \frac{1 - \text{sgn}(\delta_m^{a_4})}{2} \\
& - \sum_{m=1}^{n_{e_1}} \text{sgn}(v_m^{e_1}) \frac{1 - \text{sgn}(\delta_m^{e_1})}{2} - \sum_{m=1}^{n_{e_2}} \text{sgn}(v_m^{e_2}) \frac{1 - \text{sgn}(\delta_m^{e_2})}{2} - \sum_{m=1}^{n_{e_3}} \text{sgn}(v_m^{e_3}) \frac{1 - \text{sgn}(\delta_m^{e_3})}{2} \\
& + \sum_{m=1}^{n_{f_1}} \text{sgn}(v_m^{f_1}) \frac{1 - \text{sgn}(\delta_m^{f_1})}{2} + \sum_{m=1}^{n_{f_2}} \text{sgn}(v_m^{f_2}) \frac{1 - \text{sgn}(\delta_m^{f_2})}{2} + \sum_{m=1}^{n_{f_3}} \text{sgn}(v_m^{f_3}) \frac{1 - \text{sgn}(\delta_m^{f_3})}{2}
\end{aligned} \tag{S211.1}$$

$$\begin{aligned}
\mathcal{W}_2^{\text{gapless}} = & \sum_{m=1}^{n_{b_1}} \text{sgn}(v_m^{b_1}) \frac{1 - \text{sgn}(\delta_m^{b_1})}{2} + \sum_{m=1}^{n_{b_2}} \text{sgn}(v_m^{b_2}) \frac{1 - \text{sgn}(\delta_m^{b_2})}{2} - \sum_{m=1}^{n_{d_1}} \text{sgn}(v_m^{d_1}) \frac{1 - \text{sgn}(\delta_m^{d_1})}{2} - \sum_{m=1}^{n_{d_2}} \text{sgn}(v_m^{d_2}) \frac{1 - \text{sgn}(\delta_m^{d_2})}{2} \\
& + \sum_{m=1}^{n_{f_1}} \text{sgn}(v_m^{f_1}) \frac{1 - \text{sgn}(\delta_m^{f_1})}{2} + \sum_{m=1}^{n_{f_2}} \text{sgn}(v_m^{f_2}) \frac{1 - \text{sgn}(\delta_m^{f_2})}{2} + \sum_{m=1}^{n_{f_3}} \text{sgn}(v_m^{f_3}) \frac{1 - \text{sgn}(\delta_m^{f_3})}{2}
\end{aligned} \tag{S211.2}$$

$$\begin{aligned}
\mathcal{W}_3^{\text{gapless}} = & \sum_{m=1}^{n_{c_1}} \text{sgn}(v_m^{c_1}) \frac{1 - \text{sgn}(\delta_m^{c_1})}{2} + \sum_{m=1}^{n_{c_2}} \text{sgn}(v_m^{c_2}) \frac{1 - \text{sgn}(\delta_m^{c_2})}{2} + \sum_{m=1}^{n_{d_1}} \text{sgn}(v_m^{d_1}) \frac{1 - \text{sgn}(\delta_m^{d_1})}{2} + \sum_{m=1}^{n_{d_2}} \text{sgn}(v_m^{d_2}) \frac{1 - \text{sgn}(\delta_m^{d_2})}{2} \\
& - \sum_{m=1}^{n_{e_1}} \text{sgn}(v_m^{e_1}) \frac{1 - \text{sgn}(\delta_m^{e_1})}{2} - \sum_{m=1}^{n_{e_2}} \text{sgn}(v_m^{e_2}) \frac{1 - \text{sgn}(\delta_m^{e_2})}{2} - \sum_{m=1}^{n_{e_3}} \text{sgn}(v_m^{e_3}) \frac{1 - \text{sgn}(\delta_m^{e_3})}{2}
\end{aligned} \tag{S211.3}$$

$$\begin{aligned}
\mathcal{W}_1^{\text{gapped}} = & - \sum_{m=1}^{n_{a_2}} \text{sgn}(v_m^{a_2}) \frac{1 - \text{sgn}(\delta_m^{a_2})}{2} - \sum_{m=1}^{n_{a_4}} \text{sgn}(v_m^{a_4}) \frac{1 - \text{sgn}(\delta_m^{a_4})}{2} + \sum_{m=1}^{n_{b_2}} \text{sgn}(v_m^{b_2}) \frac{1 - \text{sgn}(\delta_m^{b_2})}{2} \\
& + \sum_{m=1}^{n_{c_2}} \text{sgn}(v_m^{c_2}) \frac{1 - \text{sgn}(\delta_m^{c_2})}{2}
\end{aligned} \tag{S211.4}$$

$$\mathcal{W}_2^{\text{gapped}} = - \sum_{m=1}^{n_{d_1}} \text{sgn}(v_m^{d_1}) \frac{1 - \text{sgn}(\delta_m^{d_1})}{2} + \sum_{m=1}^{n_{d_2}} \text{sgn}(v_m^{d_2}) \frac{1 - \text{sgn}(\delta_m^{d_2})}{2} \tag{S211.5}$$

$$\begin{aligned}\mathcal{W}_3^{\text{gapped}} = & -2 \sum_{m=1}^{n_{c_2}} \text{sgn}(v_m^{c_2}) \frac{1 - \text{sgn}(\delta_m^{c_2})}{2} - 2 \sum_{m=1}^{n_{d_1}} \text{sgn}(v_m^{d_1}) \frac{1 - \text{sgn}(\delta_m^{d_1})}{2} \\ & + \sum_{m=1}^{n_{e_1}} \text{sgn}(v_m^{e_1}) \frac{1 - \text{sgn}(\delta_m^{e_1})}{2} + \sum_{m=1}^{n_{e_2}} \text{sgn}(v_m^{e_2}) \frac{1 - \text{sgn}(\delta_m^{e_2})}{2} + \sum_{m=1}^{n_{e_3}} \text{sgn}(v_m^{e_3}) \frac{1 - \text{sgn}(\delta_m^{e_3})}{2}\end{aligned}\quad (\text{S211.6})$$

$$\mathcal{W}_4^{\text{gapped}} = \sum_{m=1}^{n_{a_3}} \text{sgn}(v_m^{a_3}) \frac{1 - \text{sgn}(\delta_m^{a_3})}{2} - \sum_{m=1}^{n_{a_4}} \text{sgn}(v_m^{a_4}) \frac{1 - \text{sgn}(\delta_m^{a_4})}{2} \quad (\text{S211.7})$$

$$\begin{aligned}\mathcal{W}_5^{\text{gapped}} = & 2 \sum_{m=1}^{n_{a_2}} \text{sgn}(v_m^{a_2}) \frac{1 - \text{sgn}(\delta_m^{a_2})}{2} + 2 \sum_{m=1}^{n_{a_4}} \text{sgn}(v_m^{a_4}) \frac{1 - \text{sgn}(\delta_m^{a_4})}{2} - 2 \sum_{m=1}^{n_{c_2}} \text{sgn}(v_m^{c_2}) \frac{1 - \text{sgn}(\delta_m^{c_2})}{2} \\ & - 2 \sum_{m=1}^{n_{d_1}} \text{sgn}(v_m^{d_1}) \frac{1 - \text{sgn}(\delta_m^{d_1})}{2} + \sum_{m=1}^{n_{f_1}} \text{sgn}(v_m^{f_1}) \frac{1 - \text{sgn}(\delta_m^{f_1})}{2} + \sum_{m=1}^{n_{f_2}} \text{sgn}(v_m^{f_2}) \frac{1 - \text{sgn}(\delta_m^{f_2})}{2} \\ & + \sum_{m=1}^{n_{f_3}} \text{sgn}(v_m^{f_3}) \frac{1 - \text{sgn}(\delta_m^{f_3})}{2}\end{aligned}\quad (\text{S211.8})$$

$$\begin{aligned}\mathcal{W}_6^{\text{gapped}} = & 2 \sum_{m=1}^{n_{a_2}} \text{sgn}(v_m^{a_2}) \frac{1 - \text{sgn}(\delta_m^{a_2})}{2} + 2 \sum_{m=1}^{n_{a_4}} \text{sgn}(v_m^{a_4}) \frac{1 - \text{sgn}(\delta_m^{a_4})}{2} - \sum_{m=1}^{n_{e_1}} \text{sgn}(v_m^{e_1}) \frac{1 - \text{sgn}(\delta_m^{e_1})}{2} \\ & - 2 \sum_{m=1}^{n_{e_2}} \text{sgn}(v_m^{e_2}) \frac{1 - \text{sgn}(\delta_m^{e_2})}{2} + \sum_{m=1}^{n_{f_1}} \text{sgn}(v_m^{f_1}) \frac{1 - \text{sgn}(\delta_m^{f_1})}{2} + 2 \sum_{m=1}^{n_{f_3}} \text{sgn}(v_m^{f_3}) \frac{1 - \text{sgn}(\delta_m^{f_3})}{2}\end{aligned}\quad (\text{S211.9})$$

## S212. SPACE GROUP NO. 212

| line segment                                      | character of irrep (generators only)                                                                                                                                                                                                                                                            |
|---------------------------------------------------|-------------------------------------------------------------------------------------------------------------------------------------------------------------------------------------------------------------------------------------------------------------------------------------------------|
| $a \quad (\frac{t}{2}, 0, 0)$                     | $\{4_{100}   \frac{3}{4} \frac{3}{4} \frac{1}{4}\}$<br>$a_1 \quad e^{-\frac{3}{4}i\pi t - \frac{3i\pi}{4}}$<br>$a_2 \quad e^{\frac{3i\pi}{4} - \frac{3i\pi t}{4}}$<br>$a_3 \quad e^{-\frac{3}{4}i\pi t - \frac{i\pi}{4}}$<br>$a_4 \quad e^{\frac{i\pi}{4} - \frac{3i\pi t}{4}}$                 |
| $b \quad (\frac{1}{2}, \frac{t}{2}, 0)$           | $\{2_{010}   0 \frac{1}{2} \frac{1}{2}\}$<br>$b_1 \quad -ie^{-\frac{1}{2}i\pi t}$<br>$b_2 \quad ie^{-\frac{1}{2}i\pi t}$                                                                                                                                                                        |
| $c \quad (\frac{t}{2}, \frac{t}{2}, 0)$           | $\{2_{110}   \frac{1}{4} \frac{3}{4} \frac{3}{4}\}$<br>$c_1 \quad -ie^{-i\pi t}$<br>$c_2 \quad ie^{-i\pi t}$                                                                                                                                                                                    |
| $d \quad (\frac{1}{2}, \frac{1}{2}, \frac{t}{2})$ | $\{4_{001}   \frac{3}{4} \frac{1}{4} \frac{3}{4}\}$<br>$d_1 \quad e^{-\frac{1}{4}i\pi(3t+4) - \frac{3i\pi}{4}}$<br>$d_2 \quad e^{\frac{3i\pi}{4} - \frac{1}{4}i\pi(3t+4)}$<br>$d_3 \quad e^{-\frac{1}{4}i\pi(3t+4) - \frac{i\pi}{4}}$<br>$d_4 \quad e^{\frac{i\pi}{4} - \frac{1}{4}i\pi(3t+4)}$ |
| $e \quad (\frac{t}{2}, \frac{t}{2}, \frac{t}{2})$ | $\{3_{111}   0 \ 0 \ 0\}$<br>$e_1 \quad -1$<br>$e_2 \quad e^{-\frac{i\pi}{3}}$<br>$e_3 \quad e^{\frac{i\pi}{3}}$                                                                                                                                                                                |

|     |                                                      |       |                                              |
|-----|------------------------------------------------------|-------|----------------------------------------------|
| $f$ | $\left(\frac{1}{2}, \frac{t}{2}, \frac{t}{2}\right)$ | $f_1$ | $e^{-\frac{1}{4}i\pi(4t+3)-\frac{3i\pi}{4}}$ |
|     |                                                      | $f_2$ | $e^{\frac{i\pi}{4}-\frac{1}{4}i\pi(4t+3)}$   |

$$\begin{aligned} \mathcal{W}_1^{\text{gapless}} = & \sum_{m=1}^{n_{a_1}} \text{sgn}(v_m^{a_1}) \frac{1 - \text{sgn}(\delta_m^{a_1})}{2} + \sum_{m=1}^{n_{a_2}} \text{sgn}(v_m^{a_2}) \frac{1 - \text{sgn}(\delta_m^{a_2})}{2} + \sum_{m=1}^{n_{a_3}} \text{sgn}(v_m^{a_3}) \frac{1 - \text{sgn}(\delta_m^{a_3})}{2} \\ & + \sum_{m=1}^{n_{a_4}} \text{sgn}(v_m^{a_4}) \frac{1 - \text{sgn}(\delta_m^{a_4})}{2} - \sum_{m=1}^{n_{e_1}} \text{sgn}(v_m^{e_1}) \frac{1 - \text{sgn}(\delta_m^{e_1})}{2} - \sum_{m=1}^{n_{e_2}} \text{sgn}(v_m^{e_2}) \frac{1 - \text{sgn}(\delta_m^{e_2})}{2} \\ & - \sum_{m=1}^{n_{e_3}} \text{sgn}(v_m^{e_3}) \frac{1 - \text{sgn}(\delta_m^{e_3})}{2} + 2 \sum_{m=1}^{n_{f_1}} \text{sgn}(v_m^{f_1}) \frac{1 - \text{sgn}(\delta_m^{f_1})}{2} \end{aligned} \quad (\text{S212.1})$$

$$\mathcal{W}_2^{\text{gapless}} = \sum_{m=1}^{n_{b_1}} \text{sgn}(v_m^{b_1}) \frac{1 - \text{sgn}(\delta_m^{b_1})}{2} + \sum_{m=1}^{n_{d_1}} \text{sgn}(v_m^{d_1}) \frac{1 - \text{sgn}(\delta_m^{d_1})}{2} + \sum_{m=1}^{n_{d_2}} \text{sgn}(v_m^{d_2}) \frac{1 - \text{sgn}(\delta_m^{d_2})}{2} - \sum_{m=1}^{n_{f_1}} \text{sgn}(v_m^{f_1}) \frac{1 - \text{sgn}(\delta_m^{f_1})}{2} \quad (\text{S212.2})$$

$$\begin{aligned} \mathcal{W}_3^{\text{gapless}} = & \sum_{m=1}^{n_{c_1}} \text{sgn}(v_m^{c_1}) \frac{1 - \text{sgn}(\delta_m^{c_1})}{2} + \sum_{m=1}^{n_{c_2}} \text{sgn}(v_m^{c_2}) \frac{1 - \text{sgn}(\delta_m^{c_2})}{2} + 2 \sum_{m=1}^{n_{d_1}} \text{sgn}(v_m^{d_1}) \frac{1 - \text{sgn}(\delta_m^{d_1})}{2} \\ & + 2 \sum_{m=1}^{n_{d_2}} \text{sgn}(v_m^{d_2}) \frac{1 - \text{sgn}(\delta_m^{d_2})}{2} - \sum_{m=1}^{n_{e_1}} \text{sgn}(v_m^{e_1}) \frac{1 - \text{sgn}(\delta_m^{e_1})}{2} - \sum_{m=1}^{n_{e_2}} \text{sgn}(v_m^{e_2}) \frac{1 - \text{sgn}(\delta_m^{e_2})}{2} \\ & - \sum_{m=1}^{n_{e_3}} \text{sgn}(v_m^{e_3}) \frac{1 - \text{sgn}(\delta_m^{e_3})}{2} \end{aligned} \quad (\text{S212.3})$$

$$\mathcal{W}_1^{\text{gapped}} = - \sum_{m=1}^{n_{e_2}} \text{sgn}(v_m^{e_2}) \frac{1 - \text{sgn}(\delta_m^{e_2})}{2} + \sum_{m=1}^{n_{e_3}} \text{sgn}(v_m^{e_3}) \frac{1 - \text{sgn}(\delta_m^{e_3})}{2} \quad (\text{S212.4})$$

$$\begin{aligned} \mathcal{W}_2^{\text{gapped}} = & 2 \sum_{m=1}^{n_{c_2}} \text{sgn}(v_m^{c_2}) \frac{1 - \text{sgn}(\delta_m^{c_2})}{2} + 2 \sum_{m=1}^{n_{d_1}} \text{sgn}(v_m^{d_1}) \frac{1 - \text{sgn}(\delta_m^{d_1})}{2} + 2 \sum_{m=1}^{n_{d_2}} \text{sgn}(v_m^{d_2}) \frac{1 - \text{sgn}(\delta_m^{d_2})}{2} \\ & - \sum_{m=1}^{n_{e_1}} \text{sgn}(v_m^{e_1}) \frac{1 - \text{sgn}(\delta_m^{e_1})}{2} - 2 \sum_{m=1}^{n_{e_2}} \text{sgn}(v_m^{e_2}) \frac{1 - \text{sgn}(\delta_m^{e_2})}{2} \end{aligned} \quad (\text{S212.5})$$

$$\begin{aligned} \mathcal{X}_1 = & \sum_{m=1}^{n_{a_2}} \text{sgn}(v_m^{a_2}) \frac{1 - \text{sgn}(\delta_m^{a_2})}{2} - \sum_{m=1}^{n_{a_3}} \text{sgn}(v_m^{a_3}) \frac{1 - \text{sgn}(\delta_m^{a_3})}{2} + 2 \sum_{m=1}^{n_{a_4}} \text{sgn}(v_m^{a_4}) \frac{1 - \text{sgn}(\delta_m^{a_4})}{2} + 9 \sum_{m=1}^{n_{c_2}} \text{sgn}(v_m^{c_2}) \frac{1 - \text{sgn}(\delta_m^{c_2})}{2} \\ & + 14 \sum_{m=1}^{n_{d_2}} \text{sgn}(v_m^{d_2}) \frac{1 - \text{sgn}(\delta_m^{d_2})}{2} - 5 \sum_{m=1}^{n_{e_1}} \text{sgn}(v_m^{e_1}) \frac{1 - \text{sgn}(\delta_m^{e_1})}{2} - 10 \sum_{m=1}^{n_{e_2}} \text{sgn}(v_m^{e_2}) \frac{1 - \text{sgn}(\delta_m^{e_2})}{2} \\ & + 2 \sum_{m=1}^{n_{f_1}} \text{sgn}(v_m^{f_1}) \frac{1 - \text{sgn}(\delta_m^{f_1})}{2} \quad \text{mod } 4 \end{aligned} \quad (\text{S212.6})$$



## S213. SPACE GROUP NO. 213

| line segment                                      | character of irrep (generators only)                                                                                                                                                                                                                                                        |
|---------------------------------------------------|---------------------------------------------------------------------------------------------------------------------------------------------------------------------------------------------------------------------------------------------------------------------------------------------|
| $a \quad (\frac{t}{2}, 0, 0)$                     | $\{4_{100}   \frac{1}{4} \frac{1}{4} \frac{3}{4}\}$<br>$a_1 \quad e^{-\frac{1}{4}i\pi t - \frac{3i\pi}{4}}$<br>$a_2 \quad e^{\frac{3i\pi}{4} - \frac{i\pi t}{4}}$<br>$a_3 \quad e^{-\frac{1}{4}i\pi t - \frac{i\pi}{4}}$<br>$a_4 \quad e^{\frac{i\pi}{4} - \frac{i\pi t}{4}}$               |
| $b \quad (\frac{1}{2}, \frac{t}{2}, 0)$           | $\{2_{010}   0 \frac{1}{2} \frac{1}{2}\}$<br>$b_1 \quad -ie^{-\frac{1}{2}i\pi t}$<br>$b_2 \quad ie^{-\frac{1}{2}i\pi t}$                                                                                                                                                                    |
| $c \quad (\frac{t}{2}, \frac{t}{2}, 0)$           | $\{2_{110}   \frac{3}{4} \frac{1}{4} \frac{1}{4}\}$<br>$c_1 \quad -ie^{-i\pi t}$<br>$c_2 \quad ie^{-i\pi t}$                                                                                                                                                                                |
| $d \quad (\frac{1}{2}, \frac{1}{2}, \frac{t}{2})$ | $\{4_{001}   \frac{1}{4} \frac{3}{4} \frac{1}{4}\}$<br>$d_1 \quad e^{-\frac{1}{4}i\pi(t+4) - \frac{3i\pi}{4}}$<br>$d_2 \quad e^{\frac{3i\pi}{4} - \frac{1}{4}i\pi(t+4)}$<br>$d_3 \quad e^{-\frac{1}{4}i\pi(t+4) - \frac{i\pi}{4}}$<br>$d_4 \quad e^{\frac{i\pi}{4} - \frac{1}{4}i\pi(t+4)}$ |
| $e \quad (\frac{t}{2}, \frac{t}{2}, \frac{t}{2})$ | $\{3_{111}   0 \ 0 \ 0\}$<br>$e_1 \quad -1$<br>$e_2 \quad e^{-\frac{i\pi}{3}}$<br>$e_3 \quad e^{\frac{i\pi}{3}}$                                                                                                                                                                            |
| $f \quad (\frac{1}{2}, \frac{t}{2}, \frac{t}{2})$ | $\{2_{011}   \frac{1}{4} \frac{3}{4} \frac{1}{4}\}$<br>$f_1 \quad e^{\frac{3i\pi}{4} - \frac{1}{4}i\pi(4t+1)}$<br>$f_2 \quad e^{-\frac{1}{4}i\pi(4t+1) - \frac{i\pi}{4}}$                                                                                                                   |

$$\begin{aligned}
\mathcal{W}_1^{\text{gapless}} = & \sum_{m=1}^{n_{a_1}} \text{sgn}(v_m^{a_1}) \frac{1 - \text{sgn}(\delta_m^{a_1})}{2} + \sum_{m=1}^{n_{a_2}} \text{sgn}(v_m^{a_2}) \frac{1 - \text{sgn}(\delta_m^{a_2})}{2} + \sum_{m=1}^{n_{a_3}} \text{sgn}(v_m^{a_3}) \frac{1 - \text{sgn}(\delta_m^{a_3})}{2} \\
& + \sum_{m=1}^{n_{a_4}} \text{sgn}(v_m^{a_4}) \frac{1 - \text{sgn}(\delta_m^{a_4})}{2} - \sum_{m=1}^{n_{e_1}} \text{sgn}(v_m^{e_1}) \frac{1 - \text{sgn}(\delta_m^{e_1})}{2} - \sum_{m=1}^{n_{e_2}} \text{sgn}(v_m^{e_2}) \frac{1 - \text{sgn}(\delta_m^{e_2})}{2} \\
& - \sum_{m=1}^{n_{e_3}} \text{sgn}(v_m^{e_3}) \frac{1 - \text{sgn}(\delta_m^{e_3})}{2} + 2 \sum_{m=1}^{n_{f_1}} \text{sgn}(v_m^{f_1}) \frac{1 - \text{sgn}(\delta_m^{f_1})}{2}
\end{aligned} \tag{S213.1}$$

$$\begin{aligned}
\mathcal{W}_2^{\text{gapless}} = & \sum_{m=1}^{n_{b_1}} \text{sgn}(v_m^{b_1}) \frac{1 - \text{sgn}(\delta_m^{b_1})}{2} + \sum_{m=1}^{n_{d_1}} \text{sgn}(v_m^{d_1}) \frac{1 - \text{sgn}(\delta_m^{d_1})}{2} + \sum_{m=1}^{n_{d_2}} \text{sgn}(v_m^{d_2}) \frac{1 - \text{sgn}(\delta_m^{d_2})}{2} - \sum_{m=1}^{n_{f_1}} \text{sgn}(v_m^{f_1}) \frac{1 - \text{sgn}(\delta_m^{f_1})}{2}
\end{aligned} \tag{S213.2}$$

$$\begin{aligned}
\mathcal{W}_3^{\text{gapless}} = & \sum_{m=1}^{n_{c_1}} \text{sgn}(v_m^{c_1}) \frac{1 - \text{sgn}(\delta_m^{c_1})}{2} + \sum_{m=1}^{n_{c_2}} \text{sgn}(v_m^{c_2}) \frac{1 - \text{sgn}(\delta_m^{c_2})}{2} + 2 \sum_{m=1}^{n_{d_1}} \text{sgn}(v_m^{d_1}) \frac{1 - \text{sgn}(\delta_m^{d_1})}{2} \\
& + 2 \sum_{m=1}^{n_{d_2}} \text{sgn}(v_m^{d_2}) \frac{1 - \text{sgn}(\delta_m^{d_2})}{2} - \sum_{m=1}^{n_{e_1}} \text{sgn}(v_m^{e_1}) \frac{1 - \text{sgn}(\delta_m^{e_1})}{2} - \sum_{m=1}^{n_{e_2}} \text{sgn}(v_m^{e_2}) \frac{1 - \text{sgn}(\delta_m^{e_2})}{2} \\
& - \sum_{m=1}^{n_{e_3}} \text{sgn}(v_m^{e_3}) \frac{1 - \text{sgn}(\delta_m^{e_3})}{2}
\end{aligned} \tag{S213.3}$$

$$\mathcal{W}_1^{\text{gapped}} = - \sum_{m=1}^{n_{e_2}} \text{sgn}(v_m^{e_2}) \frac{1 - \text{sgn}(\delta_m^{e_2})}{2} + \sum_{m=1}^{n_{e_3}} \text{sgn}(v_m^{e_3}) \frac{1 - \text{sgn}(\delta_m^{e_3})}{2} \quad (\text{S213.4})$$

$$\begin{aligned} \mathcal{W}_2^{\text{gapped}} = & 2 \sum_{m=1}^{n_{c_2}} \text{sgn}(v_m^{c_2}) \frac{1 - \text{sgn}(\delta_m^{c_2})}{2} + 2 \sum_{m=1}^{n_{d_1}} \text{sgn}(v_m^{d_1}) \frac{1 - \text{sgn}(\delta_m^{d_1})}{2} + 2 \sum_{m=1}^{n_{d_2}} \text{sgn}(v_m^{d_2}) \frac{1 - \text{sgn}(\delta_m^{d_2})}{2} \\ & - \sum_{m=1}^{n_{e_1}} \text{sgn}(v_m^{e_1}) \frac{1 - \text{sgn}(\delta_m^{e_1})}{2} - 2 \sum_{m=1}^{n_{e_2}} \text{sgn}(v_m^{e_2}) \frac{1 - \text{sgn}(\delta_m^{e_2})}{2} \end{aligned} \quad (\text{S213.5})$$

$$\begin{aligned} \mathcal{X}_1 = & - \sum_{m=1}^{n_{a_2}} \text{sgn}(v_m^{a_2}) \frac{1 - \text{sgn}(\delta_m^{a_2})}{2} + \sum_{m=1}^{n_{a_3}} \text{sgn}(v_m^{a_3}) \frac{1 - \text{sgn}(\delta_m^{a_3})}{2} - 2 \sum_{m=1}^{n_{a_4}} \text{sgn}(v_m^{a_4}) \frac{1 - \text{sgn}(\delta_m^{a_4})}{2} \\ & + 9 \sum_{m=1}^{n_{c_2}} \text{sgn}(v_m^{c_2}) \frac{1 - \text{sgn}(\delta_m^{c_2})}{2} + 14 \sum_{m=1}^{n_{d_1}} \text{sgn}(v_m^{d_1}) \frac{1 - \text{sgn}(\delta_m^{d_1})}{2} \pmod{4} \end{aligned} \quad (\text{S213.6})$$

#### S214. SPACE GROUP NO. 214

| line segment                                          | character of irrep (generators only)                                                                                                                                                                                                                                          |
|-------------------------------------------------------|-------------------------------------------------------------------------------------------------------------------------------------------------------------------------------------------------------------------------------------------------------------------------------|
| $a \quad (t, 0, 0)$                                   | $\{4_{100}   \frac{1}{4} \frac{1}{4} \frac{3}{4}\}$<br>$a_1 \quad e^{-\frac{1}{2}i\pi t - \frac{3i\pi}{4}}$<br>$a_2 \quad e^{\frac{3i\pi}{4} - \frac{i\pi t}{2}}$<br>$a_3 \quad e^{-\frac{1}{2}i\pi t - \frac{i\pi}{4}}$<br>$a_4 \quad e^{\frac{i\pi}{4} - \frac{i\pi t}{2}}$ |
| $b \quad (\frac{t+1}{2}, \frac{1-t}{2}, 0)$           | $\{2_{1-10}   \frac{1}{4} \frac{1}{4} \frac{1}{4}\}$<br>$b_1 \quad i$<br>$b_2 \quad -i$                                                                                                                                                                                       |
| $c \quad (\frac{t}{2}, \frac{t}{2}, 0)$               | $\{2_{110}   \frac{3}{4} \frac{1}{4} \frac{1}{4}\}$<br>$c_1 \quad -ie^{-i\pi t}$<br>$c_2 \quad ie^{-i\pi t}$                                                                                                                                                                  |
| $d \quad (\frac{1}{2}, \frac{1}{2}, \frac{t}{2})$     | $\{2_{001}   0 \frac{1}{2} 0\}$<br>$d_1 \quad i$<br>$d_2 \quad -i$                                                                                                                                                                                                            |
| $e \quad (\frac{t}{2}, \frac{t}{2}, \frac{t}{2})$     | $\{3_{111}   0 \ 0 \ 0\}$<br>$e_1 \quad -1$<br>$e_2 \quad e^{-\frac{i\pi}{3}}$<br>$e_3 \quad e^{\frac{i\pi}{3}}$                                                                                                                                                              |
| $f \quad (1 - \frac{t}{2}, \frac{t}{2}, \frac{t}{2})$ | $\{3_{-1-1-1}   \frac{1}{2} \ 0 \ 0\}$<br>$f_1 \quad -e^{-\frac{1}{2}i\pi(2-t)}$<br>$f_2 \quad e^{-\frac{1}{2}i\pi(2-t) - \frac{i\pi}{3}}$<br>$f_3 \quad e^{\frac{i\pi}{3} - \frac{1}{2}i\pi(2-t)}$                                                                           |

$$\begin{aligned} \mathcal{W}_1^{\text{gapless}} = & \sum_{m=1}^{n_{a1}} \text{sgn}(v_m^{a1}) \frac{1 - \text{sgn}(\delta_m^{a1})}{2} + \sum_{m=1}^{n_{a2}} \text{sgn}(v_m^{a2}) \frac{1 - \text{sgn}(\delta_m^{a2})}{2} + \sum_{m=1}^{n_{a3}} \text{sgn}(v_m^{a3}) \frac{1 - \text{sgn}(\delta_m^{a3})}{2} + \sum_{m=1}^{n_{a4}} \text{sgn}(v_m^{a4}) \frac{1 - \text{sgn}(\delta_m^{a4})}{2} \\ & - \sum_{m=1}^{n_{e1}} \text{sgn}(v_m^{e1}) \frac{1 - \text{sgn}(\delta_m^{e1})}{2} - \sum_{m=1}^{n_{e2}} \text{sgn}(v_m^{e2}) \frac{1 - \text{sgn}(\delta_m^{e2})}{2} - \sum_{m=1}^{n_{e3}} \text{sgn}(v_m^{e3}) \frac{1 - \text{sgn}(\delta_m^{e3})}{2} \\ & + \sum_{m=1}^{n_{f1}} \text{sgn}(v_m^{f1}) \frac{1 - \text{sgn}(\delta_m^{f1})}{2} + \sum_{m=1}^{n_{f2}} \text{sgn}(v_m^{f2}) \frac{1 - \text{sgn}(\delta_m^{f2})}{2} + \sum_{m=1}^{n_{f3}} \text{sgn}(v_m^{f3}) \frac{1 - \text{sgn}(\delta_m^{f3})}{2} \end{aligned} \quad (\text{S214.1})$$

$$\begin{aligned} \mathcal{W}_2^{\text{gapless}} = & \sum_{m=1}^{n_{b_1}} \text{sgn}(v_m^{b_1}) \frac{1 - \text{sgn}(\delta_m^{b_1})}{2} + \sum_{m=1}^{n_{b_2}} \text{sgn}(v_m^{b_2}) \frac{1 - \text{sgn}(\delta_m^{b_2})}{2} - \sum_{m=1}^{n_{d_1}} \text{sgn}(v_m^{d_1}) \frac{1 - \text{sgn}(\delta_m^{d_1})}{2} - \sum_{m=1}^{n_{d_2}} \text{sgn}(v_m^{d_2}) \frac{1 - \text{sgn}(\delta_m^{d_2})}{2} \\ & + \sum_{m=1}^{n_{f_1}} \text{sgn}(v_m^{f_1}) \frac{1 - \text{sgn}(\delta_m^{f_1})}{2} + \sum_{m=1}^{n_{f_2}} \text{sgn}(v_m^{f_2}) \frac{1 - \text{sgn}(\delta_m^{f_2})}{2} + \sum_{m=1}^{n_{f_3}} \text{sgn}(v_m^{f_3}) \frac{1 - \text{sgn}(\delta_m^{f_3})}{2} \end{aligned} \quad (\text{S214.2})$$

$$\begin{aligned} \mathcal{W}_3^{\text{gapless}} = & \sum_{m=1}^{n_{c_1}} \text{sgn}(v_m^{c_1}) \frac{1 - \text{sgn}(\delta_m^{c_1})}{2} + \sum_{m=1}^{n_{c_2}} \text{sgn}(v_m^{c_2}) \frac{1 - \text{sgn}(\delta_m^{c_2})}{2} + \sum_{m=1}^{n_{d_1}} \text{sgn}(v_m^{d_1}) \frac{1 - \text{sgn}(\delta_m^{d_1})}{2} + \sum_{m=1}^{n_{d_2}} \text{sgn}(v_m^{d_2}) \frac{1 - \text{sgn}(\delta_m^{d_2})}{2} \\ & - \sum_{m=1}^{n_{e_1}} \text{sgn}(v_m^{e_1}) \frac{1 - \text{sgn}(\delta_m^{e_1})}{2} - \sum_{m=1}^{n_{e_2}} \text{sgn}(v_m^{e_2}) \frac{1 - \text{sgn}(\delta_m^{e_2})}{2} - \sum_{m=1}^{n_{e_3}} \text{sgn}(v_m^{e_3}) \frac{1 - \text{sgn}(\delta_m^{e_3})}{2} \end{aligned} \quad (\text{S214.3})$$

$$\mathcal{W}_1^{\text{gapped}} = - \sum_{m=1}^{n_{a_2}} \text{sgn}(v_m^{a_2}) \frac{1 - \text{sgn}(\delta_m^{a_2})}{2} - \sum_{m=1}^{n_{a_3}} \text{sgn}(v_m^{a_3}) \frac{1 - \text{sgn}(\delta_m^{a_3})}{2} + \sum_{m=1}^{n_{b_2}} \text{sgn}(v_m^{b_2}) \frac{1 - \text{sgn}(\delta_m^{b_2})}{2} + \sum_{m=1}^{n_{c_2}} \text{sgn}(v_m^{c_2}) \frac{1 - \text{sgn}(\delta_m^{c_2})}{2} \quad (\text{S214.4})$$

$$\mathcal{W}_2^{\text{gapped}} = 2 \sum_{m=1}^{n_{e_2}} \text{sgn}(v_m^{e_2}) \frac{1 - \text{sgn}(\delta_m^{e_2})}{2} + \sum_{m=1}^{n_{d_1}} \text{sgn}(v_m^{d_1}) \frac{1 - \text{sgn}(\delta_m^{d_1})}{2} + \sum_{m=1}^{n_{d_2}} \text{sgn}(v_m^{d_2}) \frac{1 - \text{sgn}(\delta_m^{d_2})}{2} - \sum_{m=1}^{n_{e_1}} \text{sgn}(v_m^{e_1}) \frac{1 - \text{sgn}(\delta_m^{e_1})}{2} - \sum_{m=1}^{n_{e_2}} \text{sgn}(v_m^{e_2}) \frac{1 - \text{sgn}(\delta_m^{e_2})}{2} - \sum_{m=1}^{n_{e_3}} \text{sgn}(v_m^{e_3}) \frac{1 - \text{sgn}(\delta_m^{e_3})}{2} \quad (\text{S214.5})$$

$$\begin{aligned} \mathcal{W}_3^{\text{gapped}} = & 2 \sum_{m=1}^{n_{a2}} \text{sgn}(v_m^{a2}) \frac{1 - \text{sgn}(\delta_m^{a2})}{2} + 2 \sum_{m=1}^{n_{a3}} \text{sgn}(v_m^{a3}) \frac{1 - \text{sgn}(\delta_m^{a3})}{2} \\ & - \sum_{m=1}^{n_{e1}} \text{sgn}(v_m^{e1}) \frac{1 - \text{sgn}(\delta_m^{e1})}{2} - \sum_{m=1}^{n_{e2}} \text{sgn}(v_m^{e2}) \frac{1 - \text{sgn}(\delta_m^{e2})}{2} - \sum_{m=1}^{n_{e3}} \text{sgn}(v_m^{e3}) \frac{1 - \text{sgn}(\delta_m^{e3})}{2} \\ & + \sum_{m=1}^{n_{f1}} \text{sgn}(v_m^{f1}) \frac{1 - \text{sgn}(\delta_m^{f1})}{2} + \sum_{m=1}^{n_{f2}} \text{sgn}(v_m^{f2}) \frac{1 - \text{sgn}(\delta_m^{f2})}{2} + \sum_{m=1}^{n_{f3}} \text{sgn}(v_m^{f3}) \frac{1 - \text{sgn}(\delta_m^{f3})}{2} \end{aligned} \quad (\text{S214.6})$$

$$\begin{aligned} \mathcal{W}_4^{\text{gapped}} = & 2 \sum_{m=1}^{n_{a_2}} \text{sgn}(v_m^{a_2}) \frac{1 - \text{sgn}(\delta_m^{a_2})}{2} + 2 \sum_{m=1}^{n_{a_3}} \text{sgn}(v_m^{a_3}) \frac{1 - \text{sgn}(\delta_m^{a_3})}{2} - \sum_{m=1}^{n_{e_1}} \text{sgn}(v_m^{e_1}) \frac{1 - \text{sgn}(\delta_m^{e_1})}{2} \\ & - 2 \sum_{m=1}^{n_{e_2}} \text{sgn}(v_m^{e_2}) \frac{1 - \text{sgn}(\delta_m^{e_2})}{2} + \sum_{m=1}^{n_{f_1}} \text{sgn}(v_m^{f_1}) \frac{1 - \text{sgn}(\delta_m^{f_1})}{2} + 2 \sum_{m=1}^{n_{f_3}} \text{sgn}(v_m^{f_3}) \frac{1 - \text{sgn}(\delta_m^{f_3})}{2} \end{aligned} \quad (\text{S214.7})$$

$$\begin{aligned} \mathcal{X}_1 = & \sum_{m=1}^{n_{a_2}} \frac{1 - \text{sgn}(\delta_m^{a_2})}{2} + \sum_{m=1}^{n_{a_4}} \frac{1 - \text{sgn}(\delta_m^{a_4})}{2} + \sum_{m=1}^{n_{c_2}} \frac{1 - \text{sgn}(\delta_m^{c_2})}{2} + \sum_{m=1}^{n_{d_1}} \frac{1 - \text{sgn}(\delta_m^{d_1})}{2} \\ & + \sum_{m=1}^{n_{e_1}} \frac{1 - \text{sgn}(\delta_m^{e_1})}{2} + \sum_{m=1}^{n_{f_1}} \frac{1 - \text{sgn}(\delta_m^{f_1})}{2} \pmod{2} \end{aligned} \quad (\text{S214.8})$$

### S215. SPACE GROUP NO. 215

| line segment                                      | character of irrep (generators only)                                                                                                 |
|---------------------------------------------------|--------------------------------------------------------------------------------------------------------------------------------------|
| $a \quad (\frac{t}{2}, 0, 0)$                     | $\begin{matrix} \{2_{100}  0 & 0 & 0\} & \{m_{011}  0 & 0 & 0\} \\ a_1 & 0 & & 0 \end{matrix}$                                       |
| $b \quad (\frac{1}{2}, \frac{t}{2}, 0)$           | $\begin{matrix} \{2_{010}  0 & 0 & 0\} \\ b_1 & -i \\ b_2 & i \end{matrix}$                                                          |
| $c \quad (\frac{t}{2}, \frac{t}{2}, 0)$           | $\begin{matrix} \{m_{1-10}  0 & 0 & 0\} \\ c_1 & -i \\ c_2 & i \end{matrix}$                                                         |
| $d \quad (\frac{1}{2}, \frac{1}{2}, \frac{t}{2})$ | $\begin{matrix} \{2_{001}  0 & 0 & 0\} & \{m_{110}  0 & 0 & 0\} \\ d_1 & 0 & & 0 \end{matrix}$                                       |
| $e \quad (\frac{t}{2}, \frac{t}{2}, \frac{t}{2})$ | $\begin{matrix} \{3_{111}  0 & 0 & 0\} & \{m_{1-10}  0 & 0 & 0\} \\ e_1 & -1 & & -i \\ e_2 & -1 & & i \\ e_3 & 1 & & 0 \end{matrix}$ |
| $f \quad (\frac{1}{2}, \frac{t}{2}, \frac{t}{2})$ | $\begin{matrix} \{m_{01-1}  0 & 0 & 0\} \\ f_1 & -i \\ f_2 & i \end{matrix}$                                                         |

$$\mathcal{W}_1^{\text{gapless}} = \sum_{m=1}^{n_{a_1}} \text{sgn}(v_m^{a_1}) \frac{1 - \text{sgn}(\delta_m^{a_1})}{2} - \sum_{m=1}^{n_{e_2}} \text{sgn}(v_m^{e_2}) \frac{1 - \text{sgn}(\delta_m^{e_2})}{2} - \sum_{m=1}^{n_{e_3}} \text{sgn}(v_m^{e_3}) \frac{1 - \text{sgn}(\delta_m^{e_3})}{2} + \sum_{m=1}^{n_{f_2}} \text{sgn}(v_m^{f_2}) \frac{1 - \text{sgn}(\delta_m^{f_2})}{2} \quad (\text{S215.1})$$

$$\begin{aligned} \mathcal{W}_2^{\text{gapless}} = & \sum_{m=1}^{n_{b_1}} \text{sgn}(v_m^{b_1}) \frac{1 - \text{sgn}(\delta_m^{b_1})}{2} + \sum_{m=1}^{n_{b_2}} \text{sgn}(v_m^{b_2}) \frac{1 - \text{sgn}(\delta_m^{b_2})}{2} + 2 \sum_{m=1}^{n_{d_1}} \text{sgn}(v_m^{d_1}) \frac{1 - \text{sgn}(\delta_m^{d_1})}{2} \\ & - \sum_{m=1}^{n_{f_1}} \text{sgn}(v_m^{f_1}) \frac{1 - \text{sgn}(\delta_m^{f_1})}{2} - \sum_{m=1}^{n_{f_2}} \text{sgn}(v_m^{f_2}) \frac{1 - \text{sgn}(\delta_m^{f_2})}{2} \end{aligned} \quad (\text{S215.2})$$

$$\begin{aligned} \mathcal{W}_3^{\text{gapless}} = & \sum_{m=1}^{n_{c_1}} \text{sgn}(v_m^{c_1}) \frac{1 - \text{sgn}(\delta_m^{c_1})}{2} + \sum_{m=1}^{n_{d_1}} \text{sgn}(v_m^{d_1}) \frac{1 - \text{sgn}(\delta_m^{d_1})}{2} - \sum_{m=1}^{n_{e_2}} \text{sgn}(v_m^{e_2}) \frac{1 - \text{sgn}(\delta_m^{e_2})}{2} \\ & - \sum_{m=1}^{n_{e_3}} \text{sgn}(v_m^{e_3}) \frac{1 - \text{sgn}(\delta_m^{e_3})}{2} - \sum_{m=1}^{n_{f_1}} \text{sgn}(v_m^{f_1}) \frac{1 - \text{sgn}(\delta_m^{f_1})}{2} + \sum_{m=1}^{n_{f_2}} \text{sgn}(v_m^{f_2}) \frac{1 - \text{sgn}(\delta_m^{f_2})}{2} \end{aligned} \quad (\text{S215.3})$$

$$\mathcal{W}_4^{\text{gapless}} = \sum_{m=1}^{n_{c_2}} \text{sgn}(v_m^{c_2}) \frac{1 - \text{sgn}(\delta_m^{c_2})}{2} + \sum_{m=1}^{n_{d_1}} \text{sgn}(v_m^{d_1}) \frac{1 - \text{sgn}(\delta_m^{d_1})}{2} - \sum_{m=1}^{n_{e_2}} \text{sgn}(v_m^{e_2}) \frac{1 - \text{sgn}(\delta_m^{e_2})}{2} - \sum_{m=1}^{n_{e_3}} \text{sgn}(v_m^{e_3}) \frac{1 - \text{sgn}(\delta_m^{e_3})}{2} \quad (\text{S215.4})$$

$$\mathcal{W}_5^{\text{gapless}} = \sum_{m=1}^{n_{e_1}} \text{sgn}(v_m^{e_1}) \frac{1 - \text{sgn}(\delta_m^{e_1})}{2} - \sum_{m=1}^{n_{e_2}} \text{sgn}(v_m^{e_2}) \frac{1 - \text{sgn}(\delta_m^{e_2})}{2} - \sum_{m=1}^{n_{f_1}} \text{sgn}(v_m^{f_1}) \frac{1 - \text{sgn}(\delta_m^{f_1})}{2} + \sum_{m=1}^{n_{f_2}} \text{sgn}(v_m^{f_2}) \frac{1 - \text{sgn}(\delta_m^{f_2})}{2} \quad (\text{S215.5})$$

$$\mathcal{W}_1^{\text{gapped}} = - \sum_{m=1}^{n_{b_2}} \text{sgn}(v_m^{b_2}) \frac{1 - \text{sgn}(\delta_m^{b_2})}{2} - \sum_{m=1}^{n_{d_1}} \text{sgn}(v_m^{d_1}) \frac{1 - \text{sgn}(\delta_m^{d_1})}{2} + \sum_{m=1}^{n_{f_1}} \text{sgn}(v_m^{f_1}) \frac{1 - \text{sgn}(\delta_m^{f_1})}{2} \quad (\text{S215.6})$$

$$\mathcal{W}_2^{\text{gapped}} = - \sum_{m=1}^{n_{b_2}} \text{sgn}(v_m^{b_2}) \frac{1 - \text{sgn}(\delta_m^{b_2})}{2} - \sum_{m=1}^{n_{d_1}} \text{sgn}(v_m^{d_1}) \frac{1 - \text{sgn}(\delta_m^{d_1})}{2} + \sum_{m=1}^{n_{f_2}} \text{sgn}(v_m^{f_2}) \frac{1 - \text{sgn}(\delta_m^{f_2})}{2} \quad (\text{S215.7})$$

## S216. SPACE GROUP NO. 216

| line segment                                          | character of irrep (generators only)                                                                                                   |
|-------------------------------------------------------|----------------------------------------------------------------------------------------------------------------------------------------|
| $a \ (0, t, 0)$                                       | $\begin{matrix} \{2_{010}   0 & 0 & 0\} & \{m_{101}   0 & 0 & 0\} \\ a_1 & 0 & & 0 \end{matrix}$                                       |
| $b \ (t, t, 0)$                                       | $\begin{matrix} \{m_{1-10}   0 & 0 & 0\} \\ b_1 & -i \\ b_2 & i \end{matrix}$                                                          |
| $c \ (\frac{t}{2}, 1, 0)$                             | $\begin{matrix} \{2_{100}   0 & 0 & 0\} \\ c_1 & -i \\ c_2 & i \end{matrix}$                                                           |
| $d \ (\frac{t}{2}, \frac{t}{2}, \frac{t}{2})$         | $\begin{matrix} \{3_{111}   0 & 0 & 0\} & \{m_{1-10}   0 & 0 & 0\} \\ d_1 & -1 & & -i \\ d_2 & -1 & & i \\ d_3 & 1 & & 0 \end{matrix}$ |
| $e \ (1 - \frac{t}{2}, 1 - \frac{t}{2}, \frac{t}{2})$ | $\begin{matrix} \{m_{1-10}   0 & 0 & 0\} \\ e_1 & -i \\ e_2 & i \end{matrix}$                                                          |
| $f \ (\frac{1}{2}, 1 - \frac{t}{2}, \frac{t}{2})$     | $\begin{matrix} \{1   0 & 0 & 0\} \\ f_1 & 1 \end{matrix}$                                                                             |

$$\mathcal{W}_1^{\text{gapless}} = \sum_{m=1}^{n_{a_1}} \text{sgn}(v_m^{a_1}) \frac{1 - \text{sgn}(\delta_m^{a_1})}{2} - \sum_{m=1}^{n_{d_2}} \text{sgn}(v_m^{d_2}) \frac{1 - \text{sgn}(\delta_m^{d_2})}{2} - \sum_{m=1}^{n_{d_3}} \text{sgn}(v_m^{d_3}) \frac{1 - \text{sgn}(\delta_m^{d_3})}{2} + \sum_{m=1}^{n_{e_1}} \text{sgn}(v_m^{e_1}) \frac{1 - \text{sgn}(\delta_m^{e_1})}{2} \quad (\text{S216.1})$$

$$\begin{aligned} \mathcal{W}_2^{\text{gapless}} = & \sum_{m=1}^{n_{b_1}} \text{sgn}(v_m^{b_1}) \frac{1 - \text{sgn}(\delta_m^{b_1})}{2} - \sum_{m=1}^{n_{d_2}} \text{sgn}(v_m^{d_2}) \frac{1 - \text{sgn}(\delta_m^{d_2})}{2} - \sum_{m=1}^{n_{d_3}} \text{sgn}(v_m^{d_3}) \frac{1 - \text{sgn}(\delta_m^{d_3})}{2} \\ & + 2 \sum_{m=1}^{n_{e_1}} \text{sgn}(v_m^{e_1}) \frac{1 - \text{sgn}(\delta_m^{e_1})}{2} - \sum_{m=1}^{n_{e_2}} \text{sgn}(v_m^{e_2}) \frac{1 - \text{sgn}(\delta_m^{e_2})}{2} \end{aligned} \quad (\text{S216.2})$$

$$\mathcal{W}_3^{\text{gapless}} = \sum_{m=1}^{n_{b_2}} \text{sgn}(v_m^{b_2}) \frac{1 - \text{sgn}(\delta_m^{b_2})}{2} - \sum_{m=1}^{n_{d_2}} \text{sgn}(v_m^{d_2}) \frac{1 - \text{sgn}(\delta_m^{d_2})}{2} - \sum_{m=1}^{n_{d_3}} \text{sgn}(v_m^{d_3}) \frac{1 - \text{sgn}(\delta_m^{d_3})}{2} + \sum_{m=1}^{n_{e_2}} \text{sgn}(v_m^{e_2}) \frac{1 - \text{sgn}(\delta_m^{e_2})}{2} \quad (\text{S216.3})$$

$$\begin{aligned} \mathcal{W}_4^{\text{gapless}} = & \sum_{m=1}^{n_{c_1}} \text{sgn}(v_m^{c_1}) \frac{1 - \text{sgn}(\delta_m^{c_1})}{2} + \sum_{m=1}^{n_{c_2}} \text{sgn}(v_m^{c_2}) \frac{1 - \text{sgn}(\delta_m^{c_2})}{2} - \sum_{m=1}^{n_{e_1}} \text{sgn}(v_m^{e_1}) \frac{1 - \text{sgn}(\delta_m^{e_1})}{2} \\ & - \sum_{m=1}^{n_{e_2}} \text{sgn}(v_m^{e_2}) \frac{1 - \text{sgn}(\delta_m^{e_2})}{2} + \sum_{m=1}^{n_{f_1}} \text{sgn}(v_m^{f_1}) \frac{1 - \text{sgn}(\delta_m^{f_1})}{2} \end{aligned} \quad (\text{S216.4})$$

$$\mathcal{W}_5^{\text{gapless}} = \sum_{m=1}^{n_{d_1}} \text{sgn}(v_m^{d_1}) \frac{1 - \text{sgn}(\delta_m^{d_1})}{2} - \sum_{m=1}^{n_{d_2}} \text{sgn}(v_m^{d_2}) \frac{1 - \text{sgn}(\delta_m^{d_2})}{2} + \sum_{m=1}^{n_{e_1}} \text{sgn}(v_m^{e_1}) \frac{1 - \text{sgn}(\delta_m^{e_1})}{2} - \sum_{m=1}^{n_{e_2}} \text{sgn}(v_m^{e_2}) \frac{1 - \text{sgn}(\delta_m^{e_2})}{2} \quad (\text{S216.5})$$

$$\mathcal{W}_1^{\text{gapped}} = - \sum_{m=1}^{n_{e_1}} \text{sgn}(v_m^{e_1}) \frac{1 - \text{sgn}(\delta_m^{e_1})}{2} + \sum_{m=1}^{n_{e_2}} \text{sgn}(v_m^{e_2}) \frac{1 - \text{sgn}(\delta_m^{e_2})}{2} \quad (\text{S216.6})$$

### S217. SPACE GROUP NO. 217

| line segment                                          | character of irrep (generators only)                                                                                                         |
|-------------------------------------------------------|----------------------------------------------------------------------------------------------------------------------------------------------|
| $a \quad (t, 0, 0)$                                   | $\begin{array}{cc} \{2_{100}  0 & 0 & 0 \} & \{m_{011}  0 & 0 & 0 \} \\ a_1 & 0 & & 0 \end{array}$                                           |
| $b \quad (\frac{t+1}{2}, \frac{1-t}{2}, 0)$           | $\begin{array}{cc} \{m_{110}  0 & 0 & 0 \} \\ b_1 & -i \\ b_2 & i \end{array}$                                                               |
| $c \quad (\frac{t}{2}, \frac{t}{2}, 0)$               | $\begin{array}{cc} \{m_{1-10}  0 & 0 & 0 \} \\ c_1 & -i \\ c_2 & i \end{array}$                                                              |
| $d \quad (\frac{1}{2}, \frac{1}{2}, \frac{t}{2})$     | $\begin{array}{cc} \{2_{001}  0 & 0 & 0 \} & \{m_{110}  0 & 0 & 0 \} \\ d_1 & 0 & & 0 \end{array}$                                           |
| $e \quad (\frac{t}{2}, \frac{t}{2}, \frac{t}{2})$     | $\begin{array}{cc} \{3_{111}  0 & 0 & 0 \} & \{m_{1-10}  0 & 0 & 0 \} \\ e_1 & -1 & & -i \\ e_2 & -1 & & i \\ e_3 & 1 & & 0 \end{array}$     |
| $f \quad (1 - \frac{t}{2}, \frac{t}{2}, \frac{t}{2})$ | $\begin{array}{cc} \{3_{-1-1-1}^-  0 & 0 & 0 \} & \{m_{110}  0 & 0 & 0 \} \\ f_1 & -1 & & -i \\ f_2 & -1 & & i \\ f_3 & 1 & & 0 \end{array}$ |

$$\begin{aligned} \mathcal{W}_1^{\text{gapless}} = & \sum_{m=1}^{n_{a_1}} \text{sgn}(v_m^{a_1}) \frac{1 - \text{sgn}(\delta_m^{a_1})}{2} - \sum_{m=1}^{n_{e_2}} \text{sgn}(v_m^{e_2}) \frac{1 - \text{sgn}(\delta_m^{e_2})}{2} - \sum_{m=1}^{n_{e_3}} \text{sgn}(v_m^{e_3}) \frac{1 - \text{sgn}(\delta_m^{e_3})}{2} \\ & + \sum_{m=1}^{n_{f_1}} \text{sgn}(v_m^{f_1}) \frac{1 - \text{sgn}(\delta_m^{f_1})}{2} + \sum_{m=1}^{n_{f_3}} \text{sgn}(v_m^{f_3}) \frac{1 - \text{sgn}(\delta_m^{f_3})}{2} \end{aligned} \quad (\text{S217.1})$$

$$\mathcal{W}_2^{\text{gapless}} = \sum_{m=1}^{n_{b_1}} \text{sgn}(v_m^{b_1}) \frac{1 - \text{sgn}(\delta_m^{b_1})}{2} - \sum_{m=1}^{n_{d_1}} \text{sgn}(v_m^{d_1}) \frac{1 - \text{sgn}(\delta_m^{d_1})}{2} + \sum_{m=1}^{n_{f_1}} \text{sgn}(v_m^{f_1}) \frac{1 - \text{sgn}(\delta_m^{f_1})}{2} + \sum_{m=1}^{n_{f_3}} \text{sgn}(v_m^{f_3}) \frac{1 - \text{sgn}(\delta_m^{f_3})}{2} \quad (\text{S217.2})$$

$$\mathcal{W}_3^{\text{gapless}} = \sum_{m=1}^{n_{b_2}} \text{sgn}(v_m^{b_2}) \frac{1 - \text{sgn}(\delta_m^{b_2})}{2} - \sum_{m=1}^{n_{d_1}} \text{sgn}(v_m^{d_1}) \frac{1 - \text{sgn}(\delta_m^{d_1})}{2} + \sum_{m=1}^{n_{f_2}} \text{sgn}(v_m^{f_2}) \frac{1 - \text{sgn}(\delta_m^{f_2})}{2} + \sum_{m=1}^{n_{f_3}} \text{sgn}(v_m^{f_3}) \frac{1 - \text{sgn}(\delta_m^{f_3})}{2} \quad (\text{S217.3})$$

$$\begin{aligned} \mathcal{W}_4^{\text{gapless}} = & \sum_{m=1}^{n_{c_1}} \text{sgn}(v_m^{c_1}) \frac{1 - \text{sgn}(\delta_m^{c_1})}{2} + \sum_{m=1}^{n_{d_1}} \text{sgn}(v_m^{d_1}) \frac{1 - \text{sgn}(\delta_m^{d_1})}{2} - \sum_{m=1}^{n_{e_2}} \text{sgn}(v_m^{e_2}) \frac{1 - \text{sgn}(\delta_m^{e_2})}{2} \\ & - \sum_{m=1}^{n_{e_3}} \text{sgn}(v_m^{e_3}) \frac{1 - \text{sgn}(\delta_m^{e_3})}{2} + \sum_{m=1}^{n_{f_1}} \text{sgn}(v_m^{f_1}) \frac{1 - \text{sgn}(\delta_m^{f_1})}{2} - \sum_{m=1}^{n_{f_2}} \text{sgn}(v_m^{f_2}) \frac{1 - \text{sgn}(\delta_m^{f_2})}{2} \end{aligned} \quad (\text{S217.4})$$

$$\mathcal{W}_5^{\text{gapless}} = \sum_{m=1}^{n_{c_2}} \text{sgn}(v_m^{c_2}) \frac{1 - \text{sgn}(\delta_m^{c_2})}{2} + \sum_{m=1}^{n_{d_1}} \text{sgn}(v_m^{d_1}) \frac{1 - \text{sgn}(\delta_m^{d_1})}{2} - \sum_{m=1}^{n_{e_2}} \text{sgn}(v_m^{e_2}) \frac{1 - \text{sgn}(\delta_m^{e_2})}{2} - \sum_{m=1}^{n_{e_3}} \text{sgn}(v_m^{e_3}) \frac{1 - \text{sgn}(\delta_m^{e_3})}{2} \quad (\text{S217.5})$$

$$\mathcal{W}_6^{\text{gapless}} = \sum_{m=1}^{n_{e_1}} \text{sgn}(v_m^{e_1}) \frac{1 - \text{sgn}(\delta_m^{e_1})}{2} - \sum_{m=1}^{n_{e_2}} \text{sgn}(v_m^{e_2}) \frac{1 - \text{sgn}(\delta_m^{e_2})}{2} + \sum_{m=1}^{n_{f_1}} \text{sgn}(v_m^{f_1}) \frac{1 - \text{sgn}(\delta_m^{f_1})}{2} - \sum_{m=1}^{n_{f_2}} \text{sgn}(v_m^{f_2}) \frac{1 - \text{sgn}(\delta_m^{f_2})}{2} \quad (\text{S217.6})$$

$$\mathcal{W}_1^{\text{gapped}} = - \sum_{m=1}^{n_{f_1}} \text{sgn}(v_m^{f_1}) \frac{1 - \text{sgn}(\delta_m^{f_1})}{2} + \sum_{m=1}^{n_{f_2}} \text{sgn}(v_m^{f_2}) \frac{1 - \text{sgn}(\delta_m^{f_2})}{2} \quad (\text{S217.7})$$

## S218. SPACE GROUP NO. 218

| line segment                                      | character of irrep (generators only)                                                                                                                                                                                                                                                                                                                           |
|---------------------------------------------------|----------------------------------------------------------------------------------------------------------------------------------------------------------------------------------------------------------------------------------------------------------------------------------------------------------------------------------------------------------------|
| $a \quad (\frac{t}{2}, 0, 0)$                     | $a_1 \quad \begin{Bmatrix} \{2_{100}   0 & 0 & 0\} \\ 0 \end{Bmatrix} \quad \begin{Bmatrix} \{m_{011}   \frac{1}{2} & \frac{1}{2} & \frac{1}{2}\} \\ 0 \end{Bmatrix}$                                                                                                                                                                                          |
| $b \quad (\frac{1}{2}, \frac{t}{2}, 0)$           | $b_1 \quad \begin{Bmatrix} \{2_{010}   0 & 0 & 0\} \\ -i \end{Bmatrix}$<br>$b_2 \quad \begin{Bmatrix} i \end{Bmatrix}$                                                                                                                                                                                                                                         |
| $c \quad (\frac{t}{2}, \frac{t}{2}, 0)$           | $c_1 \quad \begin{Bmatrix} \{m_{1-10}   \frac{1}{2} & \frac{1}{2} & \frac{1}{2}\} \\ -ie^{-i\pi t} \end{Bmatrix}$<br>$c_2 \quad \begin{Bmatrix} ie^{-i\pi t} \end{Bmatrix}$                                                                                                                                                                                    |
| $d \quad (\frac{1}{2}, \frac{1}{2}, \frac{t}{2})$ | $d_1 \quad \begin{Bmatrix} \{2_{001}   0 & 0 & 0\} \\ 0 \end{Bmatrix} \quad \begin{Bmatrix} \{m_{110}   \frac{1}{2} & \frac{1}{2} & \frac{1}{2}\} \\ 0 \end{Bmatrix}$                                                                                                                                                                                          |
| $e \quad (\frac{t}{2}, \frac{t}{2}, \frac{t}{2})$ | $e_1 \quad \begin{Bmatrix} \{3_{111}   0 & 0 & 0\} \\ -1 \end{Bmatrix} \quad \begin{Bmatrix} \{m_{1-10}   \frac{1}{2} & \frac{1}{2} & \frac{1}{2}\} \\ -ie^{-\frac{3}{2}i\pi t} \end{Bmatrix}$<br>$e_2 \quad \begin{Bmatrix} -1 \end{Bmatrix} \quad \begin{Bmatrix} ie^{-\frac{3}{2}i\pi t} \end{Bmatrix}$<br>$e_3 \quad \begin{Bmatrix} 1 \\ 0 \end{Bmatrix}$ |
| $f \quad (\frac{1}{2}, \frac{t}{2}, \frac{t}{2})$ | $f_1 \quad \begin{Bmatrix} \{m_{01-1}   \frac{1}{2} & \frac{1}{2} & \frac{1}{2}\} \\ -ie^{-\frac{1}{2}i\pi(2t+1)} \end{Bmatrix}$<br>$f_2 \quad \begin{Bmatrix} ie^{-\frac{1}{2}i\pi(2t+1)} \end{Bmatrix}$                                                                                                                                                      |

$$\mathcal{W}_1^{\text{gapless}} = \sum_{m=1}^{n_{a_1}} \text{sgn}(v_m^{a_1}) \frac{1 - \text{sgn}(\delta_m^{a_1})}{2} - \sum_{m=1}^{n_{e_2}} \text{sgn}(v_m^{e_2}) \frac{1 - \text{sgn}(\delta_m^{e_2})}{2} - \sum_{m=1}^{n_{e_3}} \text{sgn}(v_m^{e_3}) \frac{1 - \text{sgn}(\delta_m^{e_3})}{2} + \sum_{m=1}^{n_{f_1}} \text{sgn}(v_m^{f_1}) \frac{1 - \text{sgn}(\delta_m^{f_1})}{2} \quad (\text{S218.1})$$

$$\begin{aligned} \mathcal{W}_2^{\text{gapless}} = & \sum_{m=1}^{n_{b_1}} \text{sgn}(v_m^{b_1}) \frac{1 - \text{sgn}(\delta_m^{b_1})}{2} + \sum_{m=1}^{n_{b_2}} \text{sgn}(v_m^{b_2}) \frac{1 - \text{sgn}(\delta_m^{b_2})}{2} + 2 \sum_{m=1}^{n_{d_1}} \text{sgn}(v_m^{d_1}) \frac{1 - \text{sgn}(\delta_m^{d_1})}{2} \\ & - 2 \sum_{m=1}^{n_{f_1}} \text{sgn}(v_m^{f_1}) \frac{1 - \text{sgn}(\delta_m^{f_1})}{2} \end{aligned} \quad (\text{S218.2})$$

$$\mathcal{W}_3^{\text{gapless}} = \sum_{m=1}^{n_{c_1}} \text{sgn}(v_m^{c_1}) \frac{1 - \text{sgn}(\delta_m^{c_1})}{2} + \sum_{m=1}^{n_{d_1}} \text{sgn}(v_m^{d_1}) \frac{1 - \text{sgn}(\delta_m^{d_1})}{2} - \sum_{m=1}^{n_{e_2}} \text{sgn}(v_m^{e_2}) \frac{1 - \text{sgn}(\delta_m^{e_2})}{2} - \sum_{m=1}^{n_{e_3}} \text{sgn}(v_m^{e_3}) \frac{1 - \text{sgn}(\delta_m^{e_3})}{2} \quad (\text{S218.3})$$

$$\mathcal{W}_4^{\text{gapless}} = \sum_{m=1}^{n_{c_2}} \text{sgn}(v_m^{c_2}) \frac{1 - \text{sgn}(\delta_m^{c_2})}{2} + \sum_{m=1}^{n_{d_1}} \text{sgn}(v_m^{d_1}) \frac{1 - \text{sgn}(\delta_m^{d_1})}{2} - \sum_{m=1}^{n_{e_2}} \text{sgn}(v_m^{e_2}) \frac{1 - \text{sgn}(\delta_m^{e_2})}{2} - \sum_{m=1}^{n_{e_3}} \text{sgn}(v_m^{e_3}) \frac{1 - \text{sgn}(\delta_m^{e_3})}{2} \quad (\text{S218.4})$$

$$\mathcal{W}_5^{\text{gapless}} = \sum_{m=1}^{n_{e_1}} \text{sgn}(v_m^{e_1}) \frac{1 - \text{sgn}(\delta_m^{e_1})}{2} - \sum_{m=1}^{n_{e_2}} \text{sgn}(v_m^{e_2}) \frac{1 - \text{sgn}(\delta_m^{e_2})}{2} \quad (\text{S218.5})$$

$$\mathcal{W}_1^{\text{gapped}} = - \sum_{m=1}^{n_{b_2}} \text{sgn}(v_m^{b_2}) \frac{1 - \text{sgn}(\delta_m^{b_2})}{2} - \sum_{m=1}^{n_{d_1}} \text{sgn}(v_m^{d_1}) \frac{1 - \text{sgn}(\delta_m^{d_1})}{2} + \sum_{m=1}^{n_{f_1}} \text{sgn}(v_m^{f_1}) \frac{1 - \text{sgn}(\delta_m^{f_1})}{2} \quad (\text{S218.6})$$

$$\mathcal{X}_1 = \sum_{m=1}^{n_{b_2}} \frac{1 - \text{sgn}(\delta_m^{b_2})}{2} + \sum_{m=1}^{n_{d_1}} \frac{1 - \text{sgn}(\delta_m^{d_1})}{2} \quad \text{mod } 2 \quad (\text{S218.7})$$

### S219. SPACE GROUP NO. 219

| line segment                  | character of irrep (generators only)                                                                                                         |
|-------------------------------|----------------------------------------------------------------------------------------------------------------------------------------------|
| $a \quad (0, t, 0)$           | $a_1 \quad \begin{array}{l} \{2_{010}   0 \ 0 \ 0\} \quad \{m_{101}   \frac{1}{2} \ \frac{1}{2} \ \frac{1}{2}\} \\ 0 \end{array}$            |
| $b \quad (t, t, 0)$           | $\begin{array}{l} \{m_{1-10}   \frac{1}{2} \ \frac{1}{2} \ \frac{1}{2}\} \\ b_1 \quad -ie^{-2i\pi t} \\ b_2 \quad ie^{-2i\pi t} \end{array}$ |
| $c \quad (\frac{t}{2}, 1, 0)$ | $\begin{array}{l} \{2_{100}   0 \ 0 \ 0\} \\ c_1 \quad -i \\ c_2 \quad i \end{array}$                                                        |



|                                                           |                                                                                                                                                                                                                    |
|-----------------------------------------------------------|--------------------------------------------------------------------------------------------------------------------------------------------------------------------------------------------------------------------|
| $d \quad (\frac{t}{2}, \frac{t}{2}, \frac{t}{2})$         | $\{3_{111}   0 \ 0 \ 0 \} \quad \{m_{1-10}   \frac{1}{2} \ \frac{1}{2} \ \frac{1}{2} \}$<br>$d_1 \quad -1 \quad -ie^{-\frac{3}{2}i\pi t}$<br>$d_2 \quad -1 \quad ie^{-\frac{3}{2}i\pi t}$<br>$d_3 \quad 1 \quad 0$ |
| $e \quad (1 - \frac{t}{2}, 1 - \frac{t}{2}, \frac{t}{2})$ | $\{m_{1-10}   \frac{1}{2} \ \frac{1}{2} \ \frac{1}{2} \}$<br>$e_1 \quad -ie^{-2i\pi(1-\frac{t}{4})}$<br>$e_2 \quad ie^{-2i\pi(1-\frac{t}{4})}$                                                                     |
| $f \quad (\frac{1}{2}, 1 - \frac{t}{2}, \frac{t}{2})$     | $\{1   0 \ 0 \ 0 \}$<br>$f_1 \quad 1$                                                                                                                                                                              |

$$\mathcal{W}_1^{\text{gapless}} = \sum_{m=1}^{n_{a_1}} \text{sgn}(v_m^{a_1}) \frac{1 - \text{sgn}(\delta_m^{a_1})}{2} - \sum_{m=1}^{n_{d_2}} \text{sgn}(v_m^{d_2}) \frac{1 - \text{sgn}(\delta_m^{d_2})}{2} - \sum_{m=1}^{n_{d_3}} \text{sgn}(v_m^{d_3}) \frac{1 - \text{sgn}(\delta_m^{d_3})}{2} + \sum_{m=1}^{n_{e_2}} \text{sgn}(v_m^{e_2}) \frac{1 - \text{sgn}(\delta_m^{e_2})}{2} \quad (\text{S219.1})$$

$$\mathcal{W}_2^{\text{gapless}} = \sum_{m=1}^{n_{b_1}} \text{sgn}(v_m^{b_1}) \frac{1 - \text{sgn}(\delta_m^{b_1})}{2} - \sum_{m=1}^{n_{d_2}} \text{sgn}(v_m^{d_2}) \frac{1 - \text{sgn}(\delta_m^{d_2})}{2} - \sum_{m=1}^{n_{d_3}} \text{sgn}(v_m^{d_3}) \frac{1 - \text{sgn}(\delta_m^{d_3})}{2} + \sum_{m=1}^{n_{e_2}} \text{sgn}(v_m^{e_2}) \frac{1 - \text{sgn}(\delta_m^{e_2})}{2} \quad (\text{S219.2})$$

$$\mathcal{W}_3^{\text{gapless}} = \sum_{m=1}^{n_{b_2}} \text{sgn}(v_m^{b_2}) \frac{1 - \text{sgn}(\delta_m^{b_2})}{2} - \sum_{m=1}^{n_{d_2}} \text{sgn}(v_m^{d_2}) \frac{1 - \text{sgn}(\delta_m^{d_2})}{2} - \sum_{m=1}^{n_{d_3}} \text{sgn}(v_m^{d_3}) \frac{1 - \text{sgn}(\delta_m^{d_3})}{2} + \sum_{m=1}^{n_{e_2}} \text{sgn}(v_m^{e_2}) \frac{1 - \text{sgn}(\delta_m^{e_2})}{2} \quad (\text{S219.3})$$

$$\begin{aligned} \mathcal{W}_4^{\text{gapless}} = & \sum_{m=1}^{n_{c_1}} \text{sgn}(v_m^{c_1}) \frac{1 - \text{sgn}(\delta_m^{c_1})}{2} + \sum_{m=1}^{n_{c_2}} \text{sgn}(v_m^{c_2}) \frac{1 - \text{sgn}(\delta_m^{c_2})}{2} - \sum_{m=1}^{n_{e_1}} \text{sgn}(v_m^{e_1}) \frac{1 - \text{sgn}(\delta_m^{e_1})}{2} \\ & - \sum_{m=1}^{n_{e_2}} \text{sgn}(v_m^{e_2}) \frac{1 - \text{sgn}(\delta_m^{e_2})}{2} + 2 \sum_{m=1}^{n_{f_1}} \text{sgn}(v_m^{f_1}) \frac{1 - \text{sgn}(\delta_m^{f_1})}{2} \end{aligned} \quad (\text{S219.4})$$

$$\mathcal{W}_5^{\text{gapless}} = \sum_{m=1}^{n_{d_1}} \text{sgn}(v_m^{d_1}) \frac{1 - \text{sgn}(\delta_m^{d_1})}{2} - \sum_{m=1}^{n_{d_2}} \text{sgn}(v_m^{d_2}) \frac{1 - \text{sgn}(\delta_m^{d_2})}{2} - \sum_{m=1}^{n_{e_1}} \text{sgn}(v_m^{e_1}) \frac{1 - \text{sgn}(\delta_m^{e_1})}{2} + \sum_{m=1}^{n_{e_2}} \text{sgn}(v_m^{e_2}) \frac{1 - \text{sgn}(\delta_m^{e_2})}{2} \quad (\text{S219.5})$$

$$\mathcal{X}_1 = \sum_{m=1}^{n_{c_2}} \frac{1 - \text{sgn}(\delta_m^{c_2})}{2} + \sum_{m=1}^{n_{e_2}} \frac{1 - \text{sgn}(\delta_m^{e_2})}{2} \quad \text{mod } 2 \quad (\text{S219.6})$$

$$\mathcal{X}_2 = \sum_{m=1}^{n_{e_1}} \frac{1 - \text{sgn}(\delta_m^{e_1})}{2} + \sum_{m=1}^{n_{e_2}} \frac{1 - \text{sgn}(\delta_m^{e_2})}{2} \quad \text{mod } 2 \quad (\text{S219.7})$$

## S220. SPACE GROUP NO. 220

| line segment                                          | character of irrep (generators only)                     |                                                                |
|-------------------------------------------------------|----------------------------------------------------------|----------------------------------------------------------------|
| $a \quad (t, 0, 0)$                                   | $\{2_{100}   0 \ 0 \ \frac{1}{2}\}$                      | $\{m_{011}   \frac{1}{4} \ \frac{3}{4} \ \frac{1}{4}\}$        |
|                                                       | $a_1$                                                    | 0                                                              |
| $b \quad (\frac{t+1}{2}, \frac{1-t}{2}, 0)$           | $\{m_{110}   \frac{3}{4} \ \frac{1}{4} \ \frac{1}{4}\}$  |                                                                |
|                                                       | $b_1$                                                    | $-ie^{-\frac{1}{2}i\pi(t+2)}$                                  |
|                                                       | $b_2$                                                    | $ie^{-\frac{1}{2}i\pi(t+2)}$                                   |
| $c \quad (\frac{t}{2}, \frac{t}{2}, 0)$               | $\{m_{1-10}   \frac{1}{4} \ \frac{1}{4} \ \frac{1}{4}\}$ |                                                                |
|                                                       | $c_1$                                                    | $-ie^{-\frac{1}{2}i\pi t}$                                     |
|                                                       | $c_2$                                                    | $ie^{-\frac{1}{2}i\pi t}$                                      |
| $d \quad (\frac{1}{2}, \frac{1}{2}, \frac{t}{2})$     | $\{2_{001}   0 \ \frac{1}{2} \ 0\}$                      | $\{m_{110}   \frac{3}{4} \ \frac{1}{4} \ \frac{1}{4}\}$        |
|                                                       | $d_1$                                                    | $i \quad -ie^{-\frac{1}{4}i\pi(t+4)}$                          |
|                                                       | $d_2$                                                    | $i \quad ie^{-\frac{1}{4}i\pi(t+4)}$                           |
|                                                       | $d_3$                                                    | $-i \quad -ie^{-\frac{1}{4}i\pi(t+4)}$                         |
|                                                       | $d_4$                                                    | $-i \quad ie^{-\frac{1}{4}i\pi(t+4)}$                          |
| $e \quad (\frac{t}{2}, \frac{t}{2}, \frac{t}{2})$     | $\{3_{111}   0 \ 0 \ 0\}$                                | $\{m_{1-10}   \frac{1}{4} \ \frac{1}{4} \ \frac{1}{4}\}$       |
|                                                       | $e_1$                                                    | $-1 \quad -ie^{-\frac{3}{4}i\pi t}$                            |
|                                                       | $e_2$                                                    | $-1 \quad ie^{-\frac{3}{4}i\pi t}$                             |
|                                                       | $e_3$                                                    | $1 \quad 0$                                                    |
| $f \quad (1 - \frac{t}{2}, \frac{t}{2}, \frac{t}{2})$ | $\{3_{-1-1-1}   \frac{1}{2} \ 0 \ 0\}$                   | $\{m_{110}   \frac{3}{4} \ \frac{1}{4} \ \frac{1}{4}\}$        |
|                                                       | $f_1$                                                    | $-e^{-\frac{1}{2}i\pi(2-t)} \quad -ie^{-\frac{1}{4}i\pi(6-t)}$ |
|                                                       | $f_2$                                                    | $-e^{-\frac{1}{2}i\pi(2-t)} \quad ie^{-\frac{1}{4}i\pi(6-t)}$  |
|                                                       | $f_3$                                                    | $e^{-\frac{1}{2}i\pi(2-t)} \quad 0$                            |

$$\begin{aligned} \mathcal{W}_1^{\text{gapless}} = & \sum_{m=1}^{n_{a_1}} \text{sgn}(v_m^{a_1}) \frac{1 - \text{sgn}(\delta_m^{a_1})}{2} - \sum_{m=1}^{n_{e_2}} \text{sgn}(v_m^{e_2}) \frac{1 - \text{sgn}(\delta_m^{e_2})}{2} - \sum_{m=1}^{n_{e_3}} \text{sgn}(v_m^{e_3}) \frac{1 - \text{sgn}(\delta_m^{e_3})}{2} \\ & + \sum_{m=1}^{n_{f_1}} \text{sgn}(v_m^{f_1}) \frac{1 - \text{sgn}(\delta_m^{f_1})}{2} + \sum_{m=1}^{n_{f_3}} \text{sgn}(v_m^{f_3}) \frac{1 - \text{sgn}(\delta_m^{f_3})}{2} \end{aligned} \quad (\text{S220.1})$$

$$\begin{aligned} \mathcal{W}_2^{\text{gapless}} = & \sum_{m=1}^{n_{b_1}} \text{sgn}(v_m^{b_1}) \frac{1 - \text{sgn}(\delta_m^{b_1})}{2} - \sum_{m=1}^{n_{d_2}} \text{sgn}(v_m^{d_2}) \frac{1 - \text{sgn}(\delta_m^{d_2})}{2} - \sum_{m=1}^{n_{d_4}} \text{sgn}(v_m^{d_4}) \frac{1 - \text{sgn}(\delta_m^{d_4})}{2} \\ & + \sum_{m=1}^{n_{f_2}} \text{sgn}(v_m^{f_2}) \frac{1 - \text{sgn}(\delta_m^{f_2})}{2} + \sum_{m=1}^{n_{f_3}} \text{sgn}(v_m^{f_3}) \frac{1 - \text{sgn}(\delta_m^{f_3})}{2} \end{aligned} \quad (\text{S220.2})$$

$$\begin{aligned} \mathcal{W}_3^{\text{gapless}} = & \sum_{m=1}^{n_{c_1}} \text{sgn}(v_m^{c_1}) \frac{1 - \text{sgn}(\delta_m^{c_1})}{2} + \sum_{m=1}^{n_{d_2}} \text{sgn}(v_m^{d_2}) \frac{1 - \text{sgn}(\delta_m^{d_2})}{2} - \sum_{m=1}^{n_{d_3}} \text{sgn}(v_m^{d_3}) \frac{1 - \text{sgn}(\delta_m^{d_3})}{2} \\ & + 2 \sum_{m=1}^{n_{d_4}} \text{sgn}(v_m^{d_4}) \frac{1 - \text{sgn}(\delta_m^{d_4})}{2} - \sum_{m=1}^{n_{e_2}} \text{sgn}(v_m^{e_2}) \frac{1 - \text{sgn}(\delta_m^{e_2})}{2} - \sum_{m=1}^{n_{e_3}} \text{sgn}(v_m^{e_3}) \frac{1 - \text{sgn}(\delta_m^{e_3})}{2} \\ & + 2 \sum_{m=1}^{n_{f_1}} \text{sgn}(v_m^{f_1}) \frac{1 - \text{sgn}(\delta_m^{f_1})}{2} - 2 \sum_{m=1}^{n_{f_2}} \text{sgn}(v_m^{f_2}) \frac{1 - \text{sgn}(\delta_m^{f_2})}{2} \end{aligned} \quad (\text{S220.3})$$

$$\begin{aligned} \mathcal{W}_4^{\text{gapless}} = & \sum_{m=1}^{n_{c_2}} \text{sgn}(v_m^{c_2}) \frac{1 - \text{sgn}(\delta_m^{c_2})}{2} + \sum_{m=1}^{n_{d_2}} \text{sgn}(v_m^{d_2}) \frac{1 - \text{sgn}(\delta_m^{d_2})}{2} + \sum_{m=1}^{n_{d_3}} \text{sgn}(v_m^{d_3}) \frac{1 - \text{sgn}(\delta_m^{d_3})}{2} \\ & - \sum_{m=1}^{n_{e_2}} \text{sgn}(v_m^{e_2}) \frac{1 - \text{sgn}(\delta_m^{e_2})}{2} - \sum_{m=1}^{n_{e_3}} \text{sgn}(v_m^{e_3}) \frac{1 - \text{sgn}(\delta_m^{e_3})}{2} \end{aligned} \quad (\text{S220.4})$$

$$\begin{aligned} \mathcal{W}_5^{\text{gapless}} = & \sum_{m=1}^{n_{d_1}} \text{sgn}(v_m^{d_1}) \frac{1 - \text{sgn}(\delta_m^{d_1})}{2} - \sum_{m=1}^{n_{d_2}} \text{sgn}(v_m^{d_2}) \frac{1 - \text{sgn}(\delta_m^{d_2})}{2} + \sum_{m=1}^{n_{d_3}} \text{sgn}(v_m^{d_3}) \frac{1 - \text{sgn}(\delta_m^{d_3})}{2} \\ & - \sum_{m=1}^{n_{d_4}} \text{sgn}(v_m^{d_4}) \frac{1 - \text{sgn}(\delta_m^{d_4})}{2} - \sum_{m=1}^{n_{f_1}} \text{sgn}(v_m^{f_1}) \frac{1 - \text{sgn}(\delta_m^{f_1})}{2} + \sum_{m=1}^{n_{f_2}} \text{sgn}(v_m^{f_2}) \frac{1 - \text{sgn}(\delta_m^{f_2})}{2} \end{aligned} \quad (\text{S220.5})$$

$$\begin{aligned} \mathcal{W}_6^{\text{gapless}} = & \sum_{m=1}^{n_{e_1}} \text{sgn}(v_m^{e_1}) \frac{1 - \text{sgn}(\delta_m^{e_1})}{2} - \sum_{m=1}^{n_{e_2}} \text{sgn}(v_m^{e_2}) \frac{1 - \text{sgn}(\delta_m^{e_2})}{2} + \sum_{m=1}^{n_{f_1}} \text{sgn}(v_m^{f_1}) \frac{1 - \text{sgn}(\delta_m^{f_1})}{2} - \sum_{m=1}^{n_{f_2}} \text{sgn}(v_m^{f_2}) \frac{1 - \text{sgn}(\delta_m^{f_2})}{2} \end{aligned} \quad (\text{S220.6})$$

$$\mathcal{X}_1 = \sum_{m=1}^{n_{d_2}} \frac{1 - \text{sgn}(\delta_m^{d_2})}{2} + \sum_{m=1}^{n_{d_3}} \frac{1 - \text{sgn}(\delta_m^{d_3})}{2} + \sum_{m=1}^{n_{f_1}} \frac{1 - \text{sgn}(\delta_m^{f_1})}{2} + \sum_{m=1}^{n_{f_3}} \frac{1 - \text{sgn}(\delta_m^{f_3})}{2} \pmod{2} \quad (\text{S220.7})$$

## S221. SPACE GROUP NO. 221

| line segment                                      | character of irrep (generators only) |                            |
|---------------------------------------------------|--------------------------------------|----------------------------|
| $a \quad (\frac{t}{2}, 0, 0)$                     | $\{4_{100}   0 \ 0 \ 0\}$            | $\{m_{010}   0 \ 0 \ 0\}$  |
|                                                   | $a_1 \quad -\sqrt{2}$                | 0                          |
|                                                   | $a_2 \quad \sqrt{2}$                 | 0                          |
| $b \quad (\frac{1}{2}, \frac{t}{2}, 0)$           | $\{2_{010}   0 \ 0 \ 0\}$            | $\{m_{100}   0 \ 0 \ 0\}$  |
|                                                   | $b_1 \quad 0$                        | 0                          |
| $c \quad (\frac{t}{2}, \frac{t}{2}, 0)$           | $\{2_{110}   0 \ 0 \ 0\}$            | $\{m_{001}   0 \ 0 \ 0\}$  |
|                                                   | $c_1 \quad 0$                        | 0                          |
| $d \quad (\frac{1}{2}, \frac{1}{2}, \frac{t}{2})$ | $\{4_{001}   0 \ 0 \ 0\}$            | $\{m_{100}   0 \ 0 \ 0\}$  |
|                                                   | $d_1 \quad -\sqrt{2}$                | 0                          |
|                                                   | $d_2 \quad \sqrt{2}$                 | 0                          |
| $e \quad (\frac{t}{2}, \frac{t}{2}, \frac{t}{2})$ | $\{3_{111}   0 \ 0 \ 0\}$            | $\{m_{1-10}   0 \ 0 \ 0\}$ |
|                                                   | $e_1 \quad -1$                       | -i                         |
|                                                   | $e_2 \quad -1$                       | i                          |
|                                                   | $e_3 \quad 1$                        | 0                          |
| $f \quad (\frac{1}{2}, \frac{t}{2}, \frac{t}{2})$ | $\{2_{011}   0 \ 0 \ 0\}$            | $\{m_{100}   0 \ 0 \ 0\}$  |
|                                                   | $f_1 \quad 0$                        | 0                          |

$$\begin{aligned} \mathcal{W}_1^{\text{gapless}} = & \sum_{m=1}^{n_{a_1}} \text{sgn}(v_m^{a_1}) \frac{1 - \text{sgn}(\delta_m^{a_1})}{2} + \sum_{m=1}^{n_{a_2}} \text{sgn}(v_m^{a_2}) \frac{1 - \text{sgn}(\delta_m^{a_2})}{2} - \sum_{m=1}^{n_{e_1}} \text{sgn}(v_m^{e_1}) \frac{1 - \text{sgn}(\delta_m^{e_1})}{2} \\ & - \sum_{m=1}^{n_{e_3}} \text{sgn}(v_m^{e_3}) \frac{1 - \text{sgn}(\delta_m^{e_3})}{2} + \sum_{m=1}^{n_{f_1}} \text{sgn}(v_m^{f_1}) \frac{1 - \text{sgn}(\delta_m^{f_1})}{2} \end{aligned} \quad (\text{S221.1})$$

$$\mathcal{W}_2^{\text{gapless}} = \sum_{m=1}^{n_{b_1}} \text{sgn}(v_m^{b_1}) \frac{1 - \text{sgn}(\delta_m^{b_1})}{2} + \sum_{m=1}^{n_{d_1}} \text{sgn}(v_m^{d_1}) \frac{1 - \text{sgn}(\delta_m^{d_1})}{2} + \sum_{m=1}^{n_{d_2}} \text{sgn}(v_m^{d_2}) \frac{1 - \text{sgn}(\delta_m^{d_2})}{2} - \sum_{m=1}^{n_{f_1}} \text{sgn}(v_m^{f_1}) \frac{1 - \text{sgn}(\delta_m^{f_1})}{2} \quad (\text{S221.2})$$

$$\begin{aligned} \mathcal{W}_3^{\text{gapless}} = & \sum_{m=1}^{n_{c_1}} \text{sgn}(v_m^{c_1}) \frac{1 - \text{sgn}(\delta_m^{c_1})}{2} + \sum_{m=1}^{n_{d_1}} \text{sgn}(v_m^{d_1}) \frac{1 - \text{sgn}(\delta_m^{d_1})}{2} + \sum_{m=1}^{n_{d_2}} \text{sgn}(v_m^{d_2}) \frac{1 - \text{sgn}(\delta_m^{d_2})}{2} \\ & - \sum_{m=1}^{n_{e_1}} \text{sgn}(v_m^{e_1}) \frac{1 - \text{sgn}(\delta_m^{e_1})}{2} - \sum_{m=1}^{n_{e_3}} \text{sgn}(v_m^{e_3}) \frac{1 - \text{sgn}(\delta_m^{e_3})}{2} \end{aligned} \quad (\text{S221.3})$$

## S222. SPACE GROUP NO. 222

| line segment                                      | character of irrep (generators only) |                                                                                                 |
|---------------------------------------------------|--------------------------------------|-------------------------------------------------------------------------------------------------|
| $a \quad (\frac{t}{2}, 0, 0)$                     | $a_1$                                | $\{4_{100}   0 \ \frac{1}{2} \ 0\} \quad \{m_{010}   \frac{1}{2} \ 0 \ \frac{1}{2}\}$           |
|                                                   |                                      | $-\sqrt{2}$                                                                                     |
|                                                   | $a_2$                                | $\sqrt{2}$                                                                                      |
| $b \quad (\frac{1}{2}, \frac{t}{2}, 0)$           | $b_1$                                | $\{2_{010}   \frac{1}{2} \ 0 \ \frac{1}{2}\} \quad \{m_{100}   0 \ \frac{1}{2} \ \frac{1}{2}\}$ |
|                                                   |                                      | $i$                                                                                             |
|                                                   | $b_2$                                | $-ie^{-\frac{1}{2}i\pi t}$                                                                      |
|                                                   | $b_3$                                | $ie^{-\frac{1}{2}i\pi t}$                                                                       |
| $c \quad (\frac{t}{2}, \frac{t}{2}, 0)$           | $c_1$                                | $\{2_{110}   0 \ 0 \ \frac{1}{2}\} \quad \{m_{001}   \frac{1}{2} \ \frac{1}{2} \ 0\}$           |
|                                                   |                                      | $0$                                                                                             |
|                                                   | $d_1$                                | $\{4_{001}   \frac{1}{2} \ 0 \ 0\} \quad \{m_{100}   0 \ \frac{1}{2} \ \frac{1}{2}\}$           |
|                                                   | $d_2$                                | $i\sqrt{2}$                                                                                     |
| $e \quad (\frac{t}{2}, \frac{t}{2}, \frac{t}{2})$ | $e_1$                                | $\{3_{111}   0 \ 0 \ 0\} \quad \{m_{1-10}   \frac{1}{2} \ \frac{1}{2} \ \frac{1}{2}\}$          |
|                                                   |                                      | $-1$                                                                                            |
|                                                   | $e_2$                                | $-ie^{-\frac{3}{2}i\pi t}$                                                                      |
|                                                   | $e_3$                                | $ie^{-\frac{3}{2}i\pi t}$                                                                       |
| $f \quad (\frac{1}{2}, \frac{t}{2}, \frac{t}{2})$ | $f_1$                                | $\{2_{011}   \frac{1}{2} \ 0 \ 0\} \quad \{m_{100}   0 \ \frac{1}{2} \ \frac{1}{2}\}$           |
|                                                   |                                      | $i$                                                                                             |
|                                                   | $f_2$                                | $-ie^{-i\pi t}$                                                                                 |
|                                                   | $f_3$                                | $ie^{-i\pi t}$                                                                                  |
| $f \quad (\frac{1}{2}, \frac{t}{2}, \frac{t}{2})$ | $f_4$                                | $-ie^{-i\pi t}$                                                                                 |
|                                                   |                                      | $ie^{-i\pi t}$                                                                                  |

$$\begin{aligned} \mathcal{W}_1^{\text{gapless}} = & \sum_{m=1}^{n_{a_1}} \text{sgn}(v_m^{a_1}) \frac{1 - \text{sgn}(\delta_m^{a_1})}{2} + \sum_{m=1}^{n_{a_2}} \text{sgn}(v_m^{a_2}) \frac{1 - \text{sgn}(\delta_m^{a_2})}{2} - \sum_{m=1}^{n_{e_1}} \text{sgn}(v_m^{e_1}) \frac{1 - \text{sgn}(\delta_m^{e_1})}{2} \\ & - \sum_{m=1}^{n_{e_3}} \text{sgn}(v_m^{e_3}) \frac{1 - \text{sgn}(\delta_m^{e_3})}{2} + \sum_{m=1}^{n_{f_1}} \text{sgn}(v_m^{f_1}) \frac{1 - \text{sgn}(\delta_m^{f_1})}{2} + \sum_{m=1}^{n_{f_3}} \text{sgn}(v_m^{f_3}) \frac{1 - \text{sgn}(\delta_m^{f_3})}{2} \end{aligned} \quad (\text{S222.1})$$

$$\begin{aligned} \mathcal{W}_2^{\text{gapless}} = & \sum_{m=1}^{n_{b_1}} \text{sgn}(v_m^{b_1}) \frac{1 - \text{sgn}(\delta_m^{b_1})}{2} + \sum_{m=1}^{n_{b_3}} \text{sgn}(v_m^{b_3}) \frac{1 - \text{sgn}(\delta_m^{b_3})}{2} + \sum_{m=1}^{n_{d_1}} \text{sgn}(v_m^{d_1}) \frac{1 - \text{sgn}(\delta_m^{d_1})}{2} \\ & + \sum_{m=1}^{n_{d_2}} \text{sgn}(v_m^{d_2}) \frac{1 - \text{sgn}(\delta_m^{d_2})}{2} - \sum_{m=1}^{n_{f_1}} \text{sgn}(v_m^{f_1}) \frac{1 - \text{sgn}(\delta_m^{f_1})}{2} - \sum_{m=1}^{n_{f_3}} \text{sgn}(v_m^{f_3}) \frac{1 - \text{sgn}(\delta_m^{f_3})}{2} \end{aligned} \quad (\text{S222.2})$$

$$\begin{aligned} \mathcal{W}_3^{\text{gapless}} = & \sum_{m=1}^{n_{c_1}} \text{sgn}(v_m^{c_1}) \frac{1 - \text{sgn}(\delta_m^{c_1})}{2} + \sum_{m=1}^{n_{d_1}} \text{sgn}(v_m^{d_1}) \frac{1 - \text{sgn}(\delta_m^{d_1})}{2} + \sum_{m=1}^{n_{d_2}} \text{sgn}(v_m^{d_2}) \frac{1 - \text{sgn}(\delta_m^{d_2})}{2} \\ & - \sum_{m=1}^{n_{e_1}} \text{sgn}(v_m^{e_1}) \frac{1 - \text{sgn}(\delta_m^{e_1})}{2} - \sum_{m=1}^{n_{e_3}} \text{sgn}(v_m^{e_3}) \frac{1 - \text{sgn}(\delta_m^{e_3})}{2} \end{aligned} \quad (\text{S222.3})$$

$$\mathcal{W}_1^{\text{gapped}} = - \sum_{m=1}^{n_{d_1}} \text{sgn}(v_m^{d_1}) \frac{1 - \text{sgn}(\delta_m^{d_1})}{2} + \sum_{m=1}^{n_{d_2}} \text{sgn}(v_m^{d_2}) \frac{1 - \text{sgn}(\delta_m^{d_2})}{2} \quad (\text{S222.4})$$

$$\mathcal{W}_2^{\text{gapped}} = - \sum_{m=1}^{n_{b_3}} \text{sgn}(v_m^{b_3}) \frac{1 - \text{sgn}(\delta_m^{b_3})}{2} - \sum_{m=1}^{n_{d_1}} \text{sgn}(v_m^{d_1}) \frac{1 - \text{sgn}(\delta_m^{d_1})}{2} + \sum_{m=1}^{n_{f_1}} \text{sgn}(v_m^{f_1}) \frac{1 - \text{sgn}(\delta_m^{f_1})}{2} \quad (\text{S222.5})$$

$$\mathcal{W}_3^{\text{gapped}} = - \sum_{m=1}^{n_{b_3}} \text{sgn}(v_m^{b_3}) \frac{1 - \text{sgn}(\delta_m^{b_3})}{2} - \sum_{m=1}^{n_{d_1}} \text{sgn}(v_m^{d_1}) \frac{1 - \text{sgn}(\delta_m^{d_1})}{2} + \sum_{m=1}^{n_{f_3}} \text{sgn}(v_m^{f_3}) \frac{1 - \text{sgn}(\delta_m^{f_3})}{2} \quad (\text{S222.6})$$

### S223. SPACE GROUP NO. 223

| line segment                                      | character of irrep (generators only) |                                                                                          |
|---------------------------------------------------|--------------------------------------|------------------------------------------------------------------------------------------|
| $a \quad (\frac{t}{2}, 0, 0)$                     | $a_1$                                | $\{4_{100}   \frac{1}{2} \quad \frac{1}{2} \quad \frac{1}{2}\} \{m_{010}   0 \ 0 \ 0\}$  |
|                                                   |                                      | $-\sqrt{2}e^{-\frac{1}{2}i\pi t}$                                                        |
|                                                   | $a_2$                                | $\sqrt{2}e^{-\frac{1}{2}i\pi t}$                                                         |
| $b \quad (\frac{1}{2}, \frac{t}{2}, 0)$           | $b_1$                                | $\{2_{010}   0 \ 0 \ 0\} \{m_{100}   0 \ 0 \ 0\}$                                        |
|                                                   |                                      | 0                                                                                        |
| $c \quad (\frac{t}{2}, \frac{t}{2}, 0)$           | $c_1$                                | $\{2_{110}   \frac{1}{2} \quad \frac{1}{2} \quad \frac{1}{2}\} \{m_{001}   0 \ 0 \ 0\}$  |
|                                                   |                                      | 0                                                                                        |
| $d \quad (\frac{1}{2}, \frac{1}{2}, \frac{t}{2})$ | $d_1$                                | $\{4_{001}   \frac{1}{2} \quad \frac{1}{2} \quad \frac{1}{2}\} \{m_{100}   0 \ 0 \ 0\}$  |
|                                                   |                                      | $-\sqrt{2}e^{-\frac{1}{2}i\pi(t+2)}$                                                     |
|                                                   | $d_2$                                | $\sqrt{2}e^{-\frac{1}{2}i\pi(t+2)}$                                                      |
| $e \quad (\frac{t}{2}, \frac{t}{2}, \frac{t}{2})$ |                                      | $\{3_{111}   0 \ 0 \ 0\} \{m_{1-10}   \frac{1}{2} \quad \frac{1}{2} \quad \frac{1}{2}\}$ |
|                                                   | $e_1$                                | -1                                                                                       |
|                                                   | $e_2$                                | -1                                                                                       |
|                                                   | $e_3$                                | 1                                                                                        |
| $f \quad (\frac{1}{2}, \frac{t}{2}, \frac{t}{2})$ |                                      | $\{2_{011}   \frac{1}{2} \quad \frac{1}{2} \quad \frac{1}{2}\} \{m_{100}   0 \ 0 \ 0\}$  |
|                                                   | $f_1$                                | $-e^{-\frac{1}{2}i\pi(2t+1)}$                                                            |
|                                                   | $f_2$                                | $-e^{-\frac{1}{2}i\pi(2t+1)}$                                                            |
|                                                   | $f_3$                                | $e^{-\frac{1}{2}i\pi(2t+1)}$                                                             |
|                                                   | $f_4$                                | $e^{-\frac{1}{2}i\pi(2t+1)}$                                                             |

$$\begin{aligned} \mathcal{W}_1^{\text{gapless}} = & \sum_{m=1}^{n_{a_1}} \text{sgn}(v_m^{a_1}) \frac{1 - \text{sgn}(\delta_m^{a_1})}{2} + \sum_{m=1}^{n_{a_2}} \text{sgn}(v_m^{a_2}) \frac{1 - \text{sgn}(\delta_m^{a_2})}{2} - \sum_{m=1}^{n_{e_1}} \text{sgn}(v_m^{e_1}) \frac{1 - \text{sgn}(\delta_m^{e_1})}{2} \\ & - \sum_{m=1}^{n_{e_3}} \text{sgn}(v_m^{e_3}) \frac{1 - \text{sgn}(\delta_m^{e_3})}{2} + \sum_{m=1}^{n_{f_1}} \text{sgn}(v_m^{f_1}) \frac{1 - \text{sgn}(\delta_m^{f_1})}{2} + \sum_{m=1}^{n_{f_3}} \text{sgn}(v_m^{f_3}) \frac{1 - \text{sgn}(\delta_m^{f_3})}{2} \end{aligned} \quad (\text{S223.1})$$

$$\begin{aligned} \mathcal{W}_2^{\text{gapless}} = & \sum_{m=1}^{n_{b_1}} \text{sgn}(v_m^{b_1}) \frac{1 - \text{sgn}(\delta_m^{b_1})}{2} + \sum_{m=1}^{n_{d_1}} \text{sgn}(v_m^{d_1}) \frac{1 - \text{sgn}(\delta_m^{d_1})}{2} + \sum_{m=1}^{n_{d_2}} \text{sgn}(v_m^{d_2}) \frac{1 - \text{sgn}(\delta_m^{d_2})}{2} \\ & - \sum_{m=1}^{n_{f_1}} \text{sgn}(v_m^{f_1}) \frac{1 - \text{sgn}(\delta_m^{f_1})}{2} - \sum_{m=1}^{n_{f_3}} \text{sgn}(v_m^{f_3}) \frac{1 - \text{sgn}(\delta_m^{f_3})}{2} \end{aligned} \quad (\text{S223.2})$$

$$\begin{aligned} \mathcal{W}_3^{\text{gapless}} = & \sum_{m=1}^{n_{c_1}} \text{sgn}(v_m^{c_1}) \frac{1 - \text{sgn}(\delta_m^{c_1})}{2} + \sum_{m=1}^{n_{d_1}} \text{sgn}(v_m^{d_1}) \frac{1 - \text{sgn}(\delta_m^{d_1})}{2} + \sum_{m=1}^{n_{d_2}} \text{sgn}(v_m^{d_2}) \frac{1 - \text{sgn}(\delta_m^{d_2})}{2} \\ & - \sum_{m=1}^{n_{e_1}} \text{sgn}(v_m^{e_1}) \frac{1 - \text{sgn}(\delta_m^{e_1})}{2} - \sum_{m=1}^{n_{e_3}} \text{sgn}(v_m^{e_3}) \frac{1 - \text{sgn}(\delta_m^{e_3})}{2} \end{aligned} \quad (\text{S223.3})$$

$$\mathcal{W}_1^{\text{gapped}} = - \sum_{m=1}^{n_{f_1}} \text{sgn}(v_m^{f_1}) \frac{1 - \text{sgn}(\delta_m^{f_1})}{2} + \sum_{m=1}^{n_{f_3}} \text{sgn}(v_m^{f_3}) \frac{1 - \text{sgn}(\delta_m^{f_3})}{2} \quad (\text{S223.4})$$

#### S224. SPACE GROUP NO. 224

| line segment                                      | character of irrep (generators only)           |                                               |
|---------------------------------------------------|------------------------------------------------|-----------------------------------------------|
| $a \quad (\frac{t}{2}, 0, 0)$                     | $\{4_{100}   \frac{1}{2} \ 0 \ \frac{1}{2}\}$  | $\{m_{010}   \frac{1}{2} \ 0 \ \frac{1}{2}\}$ |
|                                                   | $a_1 \quad -\sqrt{2}e^{-\frac{1}{2}i\pi t}$    | 0                                             |
|                                                   | $a_2 \quad \sqrt{2}e^{-\frac{1}{2}i\pi t}$     | 0                                             |
| $b \quad (\frac{1}{2}, \frac{t}{2}, 0)$           | $\{2_{010}   \frac{1}{2} \ 0 \ \frac{1}{2}\}$  | $\{m_{100}   0 \ \frac{1}{2} \ \frac{1}{2}\}$ |
|                                                   | $b_1 \quad i$                                  | $-ie^{-\frac{1}{2}i\pi t}$                    |
|                                                   | $b_2 \quad i$                                  | $ie^{-\frac{1}{2}i\pi t}$                     |
|                                                   | $b_3 \quad -i$                                 | $-ie^{-\frac{1}{2}i\pi t}$                    |
| $c \quad (\frac{t}{2}, \frac{t}{2}, 0)$           | $\{2_{110}   \frac{1}{2} \ \frac{1}{2} \ 0\}$  | $\{m_{001}   \frac{1}{2} \ \frac{1}{2} \ 0\}$ |
|                                                   | $c_1 \quad 0$                                  | 0                                             |
| $d \quad (\frac{1}{2}, \frac{1}{2}, \frac{t}{2})$ | $\{4_{001}   0 \ \frac{1}{2} \ \frac{1}{2}\}$  | $\{m_{100}   0 \ \frac{1}{2} \ \frac{1}{2}\}$ |
|                                                   | $d_1 \quad -\sqrt{2}e^{-\frac{1}{2}i\pi(t+1)}$ | 0                                             |
|                                                   | $d_2 \quad \sqrt{2}e^{-\frac{1}{2}i\pi(t+1)}$  | 0                                             |
| $e \quad (\frac{t}{2}, \frac{t}{2}, \frac{t}{2})$ | $\{3_{111}   0 \ 0 \ 0\}$                      | $\{m_{1-10}   0 \ 0 \ 0\}$                    |
|                                                   | $e_1 \quad -1$                                 | $-i$                                          |
|                                                   | $e_2 \quad -1$                                 | $i$                                           |
| $f \quad (\frac{1}{2}, \frac{t}{2}, \frac{t}{2})$ | $\{2_{011}   0 \ \frac{1}{2} \ \frac{1}{2}\}$  | $\{m_{100}   0 \ \frac{1}{2} \ \frac{1}{2}\}$ |
|                                                   | $f_1 \quad 0$                                  | 0                                             |

$$\begin{aligned} \mathcal{W}_1^{\text{gapless}} = & \sum_{m=1}^{n_{a_1}} \text{sgn}(v_m^{a_1}) \frac{1 - \text{sgn}(\delta_m^{a_1})}{2} + \sum_{m=1}^{n_{a_2}} \text{sgn}(v_m^{a_2}) \frac{1 - \text{sgn}(\delta_m^{a_2})}{2} - \sum_{m=1}^{n_{e_1}} \text{sgn}(v_m^{e_1}) \frac{1 - \text{sgn}(\delta_m^{e_1})}{2} \\ & - \sum_{m=1}^{n_{e_3}} \text{sgn}(v_m^{e_3}) \frac{1 - \text{sgn}(\delta_m^{e_3})}{2} + \sum_{m=1}^{n_{f_1}} \text{sgn}(v_m^{f_1}) \frac{1 - \text{sgn}(\delta_m^{f_1})}{2} \end{aligned} \quad (\text{S224.1})$$

$$\begin{aligned} \mathcal{W}_2^{\text{gapless}} = & \sum_{m=1}^{n_{b_1}} \text{sgn}(v_m^{b_1}) \frac{1 - \text{sgn}(\delta_m^{b_1})}{2} + \sum_{m=1}^{n_{b_3}} \text{sgn}(v_m^{b_3}) \frac{1 - \text{sgn}(\delta_m^{b_3})}{2} + \sum_{m=1}^{n_{d_1}} \text{sgn}(v_m^{d_1}) \frac{1 - \text{sgn}(\delta_m^{d_1})}{2} \\ & + \sum_{m=1}^{n_{d_2}} \text{sgn}(v_m^{d_2}) \frac{1 - \text{sgn}(\delta_m^{d_2})}{2} - \sum_{m=1}^{n_{f_1}} \text{sgn}(v_m^{f_1}) \frac{1 - \text{sgn}(\delta_m^{f_1})}{2} \end{aligned} \quad (\text{S224.2})$$

$$\begin{aligned} \mathcal{W}_3^{\text{gapless}} = & \sum_{m=1}^{n_{c_1}} \text{sgn}(v_m^{c_1}) \frac{1 - \text{sgn}(\delta_m^{c_1})}{2} + \sum_{m=1}^{n_{d_1}} \text{sgn}(v_m^{d_1}) \frac{1 - \text{sgn}(\delta_m^{d_1})}{2} + \sum_{m=1}^{n_{d_2}} \text{sgn}(v_m^{d_2}) \frac{1 - \text{sgn}(\delta_m^{d_2})}{2} \\ & - \sum_{m=1}^{n_{e_1}} \text{sgn}(v_m^{e_1}) \frac{1 - \text{sgn}(\delta_m^{e_1})}{2} - \sum_{m=1}^{n_{e_3}} \text{sgn}(v_m^{e_3}) \frac{1 - \text{sgn}(\delta_m^{e_3})}{2} \end{aligned} \quad (\text{S224.3})$$

$$\begin{aligned} \mathcal{W}_1^{\text{gapped}} = & -2 \sum_{m=1}^{n_{b_3}} \text{sgn}(v_m^{b_3}) \frac{1 - \text{sgn}(\delta_m^{b_3})}{2} - \sum_{m=1}^{n_{d_1}} \text{sgn}(v_m^{d_1}) \frac{1 - \text{sgn}(\delta_m^{d_1})}{2} - \sum_{m=1}^{n_{d_2}} \text{sgn}(v_m^{d_2}) \frac{1 - \text{sgn}(\delta_m^{d_2})}{2} \\ & + \sum_{m=1}^{n_{f_1}} \text{sgn}(v_m^{f_1}) \frac{1 - \text{sgn}(\delta_m^{f_1})}{2} \end{aligned} \quad (\text{S224.4})$$

### S225. SPACE GROUP NO. 225

| line segment                                              | character of irrep (generators only)                                                                                                                          |
|-----------------------------------------------------------|---------------------------------------------------------------------------------------------------------------------------------------------------------------|
| $a \quad (0, t, 0)$                                       | $\begin{array}{l} \{4_{010}   0 \ 0 \ 0\} \quad \{m_{100}   0 \ 0 \ 0\} \\ a_1 \quad -\sqrt{2} \quad 0 \\ a_2 \quad \sqrt{2} \quad 0 \end{array}$             |
| $b \quad (t, t, 0)$                                       | $\begin{array}{l} \{2_{110}   0 \ 0 \ 0\} \quad \{m_{001}   0 \ 0 \ 0\} \\ b_1 \quad 0 \quad 0 \end{array}$                                                   |
| $c \quad (\frac{t}{2}, 1, 0)$                             | $\begin{array}{l} \{2_{100}   0 \ 0 \ 0\} \quad \{m_{010}   0 \ 0 \ 0\} \\ c_1 \quad 0 \quad 0 \end{array}$                                                   |
| $d \quad (\frac{t}{2}, \frac{t}{2}, \frac{t}{2})$         | $\begin{array}{l} \{3_{111}   0 \ 0 \ 0\} \quad \{m_{1-10}   0 \ 0 \ 0\} \\ d_1 \quad -1 \quad -i \\ d_2 \quad -1 \quad i \\ d_3 \quad 1 \quad 0 \end{array}$ |
| $e \quad (1 - \frac{t}{2}, 1 - \frac{t}{2}, \frac{t}{2})$ | $\begin{array}{l} \{m_{1-10}   0 \ 0 \ 0\} \\ e_1 \quad -i \\ e_2 \quad i \end{array}$                                                                        |
| $f \quad (\frac{1}{2}, 1 - \frac{t}{2}, \frac{t}{2})$     | $\begin{array}{l} \{2_{01-1}   0 \ 0 \ 0\} \\ f_1 \quad -i \\ f_2 \quad i \end{array}$                                                                        |

$$\begin{aligned} \mathcal{W}_1^{\text{gapless}} = & \sum_{m=1}^{n_{a_1}} \text{sgn}(v_m^{a_1}) \frac{1 - \text{sgn}(\delta_m^{a_1})}{2} + \sum_{m=1}^{n_{a_2}} \text{sgn}(v_m^{a_2}) \frac{1 - \text{sgn}(\delta_m^{a_2})}{2} - \sum_{m=1}^{n_{d_1}} \text{sgn}(v_m^{d_1}) \frac{1 - \text{sgn}(\delta_m^{d_1})}{2} \\ & - \sum_{m=1}^{n_{d_3}} \text{sgn}(v_m^{d_3}) \frac{1 - \text{sgn}(\delta_m^{d_3})}{2} + \sum_{m=1}^{n_{e_1}} \text{sgn}(v_m^{e_1}) \frac{1 - \text{sgn}(\delta_m^{e_1})}{2} \end{aligned} \quad (\text{S225.1})$$

$$\mathcal{W}_2^{\text{gapless}} = \sum_{m=1}^{n_{b_1}} \text{sgn}(v_m^{b_1}) \frac{1 - \text{sgn}(\delta_m^{b_1})}{2} - \sum_{m=1}^{n_{d_1}} \text{sgn}(v_m^{d_1}) \frac{1 - \text{sgn}(\delta_m^{d_1})}{2} - \sum_{m=1}^{n_{d_3}} \text{sgn}(v_m^{d_3}) \frac{1 - \text{sgn}(\delta_m^{d_3})}{2} + \sum_{m=1}^{n_{e_1}} \text{sgn}(v_m^{e_1}) \frac{1 - \text{sgn}(\delta_m^{e_1})}{2} \quad (\text{S225.2})$$

$$\mathcal{W}_3^{\text{gapless}} = \sum_{m=1}^{n_{c_1}} \text{sgn}(v_m^{c_1}) \frac{1 - \text{sgn}(\delta_m^{c_1})}{2} - \sum_{m=1}^{n_{e_1}} \text{sgn}(v_m^{e_1}) \frac{1 - \text{sgn}(\delta_m^{e_1})}{2} + \sum_{m=1}^{n_{f_1}} \text{sgn}(v_m^{f_1}) \frac{1 - \text{sgn}(\delta_m^{f_1})}{2} \quad (\text{S225.3})$$

### S226. SPACE GROUP NO. 226

| line segment                                              | character of irrep (generators only)                                                                                                                                                                   |
|-----------------------------------------------------------|--------------------------------------------------------------------------------------------------------------------------------------------------------------------------------------------------------|
| $a \quad (0, t, 0)$                                       | $\begin{matrix} \{4_{010}   \frac{1}{2} \frac{1}{2} \frac{1}{2}\} & \{m_{100}   0 \ 0 \ 0\} \\ a_1 & -\sqrt{2}e^{-i\pi t} & 0 \\ a_2 & \sqrt{2}e^{-i\pi t} & 0 \end{matrix}$                           |
| $b \quad (t, t, 0)$                                       | $\begin{matrix} \{2_{110}   \frac{1}{2} \frac{1}{2} \frac{1}{2}\} & \{m_{001}   0 \ 0 \ 0\} \\ b_1 & 0 & 0 \end{matrix}$                                                                               |
| $c \quad (\frac{t}{2}, 1, 0)$                             | $\begin{matrix} \{2_{100}   0 \ 0 \ 0\} & \{m_{010}   0 \ 0 \ 0\} \\ c_1 & 0 & 0 \end{matrix}$                                                                                                         |
| $d \quad (\frac{t}{2}, \frac{t}{2}, \frac{t}{2})$         | $\begin{matrix} \{3_{111}   0 \ 0 \ 0\} & \{m_{1-10}   \frac{1}{2} \frac{1}{2} \frac{1}{2}\} \\ d_1 & -1 & -ie^{-\frac{3}{2}i\pi t} \\ d_2 & -1 & ie^{-\frac{3}{2}i\pi t} \\ d_3 & 1 & 0 \end{matrix}$ |
| $e \quad (1 - \frac{t}{2}, 1 - \frac{t}{2}, \frac{t}{2})$ | $\begin{matrix} \{m_{1-10}   \frac{1}{2} \frac{1}{2} \frac{1}{2}\} \\ e_1 & -ie^{-2i\pi(1-\frac{t}{4})} \\ e_2 & ie^{-2i\pi(1-\frac{t}{4})} \end{matrix}$                                              |
| $f \quad (\frac{1}{2}, 1 - \frac{t}{2}, \frac{t}{2})$     | $\begin{matrix} \{2_{01-1}   \frac{1}{2} \frac{1}{2} \frac{1}{2}\} \\ f_1 & -i \\ f_2 & i \end{matrix}$                                                                                                |

$$\begin{aligned} \mathcal{W}_1^{\text{gapless}} = & \sum_{m=1}^{n_{a_1}} \text{sgn}(v_m^{a_1}) \frac{1 - \text{sgn}(\delta_m^{a_1})}{2} + \sum_{m=1}^{n_{a_2}} \text{sgn}(v_m^{a_2}) \frac{1 - \text{sgn}(\delta_m^{a_2})}{2} - \sum_{m=1}^{n_{d_1}} \text{sgn}(v_m^{d_1}) \frac{1 - \text{sgn}(\delta_m^{d_1})}{2} \\ & - \sum_{m=1}^{n_{d_3}} \text{sgn}(v_m^{d_3}) \frac{1 - \text{sgn}(\delta_m^{d_3})}{2} + \sum_{m=1}^{n_{e_1}} \text{sgn}(v_m^{e_1}) \frac{1 - \text{sgn}(\delta_m^{e_1})}{2} \end{aligned} \quad (\text{S226.1})$$

$$\mathcal{W}_2^{\text{gapless}} = \sum_{m=1}^{n_{b_1}} \text{sgn}(v_m^{b_1}) \frac{1 - \text{sgn}(\delta_m^{b_1})}{2} - \sum_{m=1}^{n_{d_1}} \text{sgn}(v_m^{d_1}) \frac{1 - \text{sgn}(\delta_m^{d_1})}{2} - \sum_{m=1}^{n_{d_3}} \text{sgn}(v_m^{d_3}) \frac{1 - \text{sgn}(\delta_m^{d_3})}{2} + \sum_{m=1}^{n_{e_1}} \text{sgn}(v_m^{e_1}) \frac{1 - \text{sgn}(\delta_m^{e_1})}{2} \quad (\text{S226.2})$$

$$\mathcal{W}_3^{\text{gapless}} = \sum_{m=1}^{n_{c_1}} \text{sgn}(v_m^{c_1}) \frac{1 - \text{sgn}(\delta_m^{c_1})}{2} - \sum_{m=1}^{n_{e_1}} \text{sgn}(v_m^{e_1}) \frac{1 - \text{sgn}(\delta_m^{e_1})}{2} + \sum_{m=1}^{n_{f_1}} \text{sgn}(v_m^{f_1}) \frac{1 - \text{sgn}(\delta_m^{f_1})}{2} + \sum_{m=1}^{n_{f_2}} \text{sgn}(v_m^{f_2}) \frac{1 - \text{sgn}(\delta_m^{f_2})}{2} \quad (\text{S226.3})$$

$$\mathcal{W}_1^{\text{gapped}} = - \sum_{m=1}^{n_{f_1}} \text{sgn}(v_m^{f_1}) \frac{1 - \text{sgn}(\delta_m^{f_1})}{2} + \sum_{m=1}^{n_{f_2}} \text{sgn}(v_m^{f_2}) \frac{1 - \text{sgn}(\delta_m^{f_2})}{2} \quad (\text{S226.4})$$



**S227. SPACE GROUP NO. 227**

| line segment                                              | character of irrep (generators only)        |                                           |
|-----------------------------------------------------------|---------------------------------------------|-------------------------------------------|
| $a \quad (0, t, 0)$                                       | $\{4_{010}   \frac{1}{4} \frac{1}{4} 0\}$   | $\{m_{100}   0 \frac{1}{4} \frac{1}{4}\}$ |
|                                                           | $a_1 \quad -\sqrt{2}e^{-\frac{1}{2}i\pi t}$ | 0                                         |
|                                                           | $a_2 \quad \sqrt{2}e^{-\frac{1}{2}i\pi t}$  | 0                                         |
| $b \quad (t, t, 0)$                                       | $\{2_{110}   \frac{1}{4} \frac{1}{4} 0\}$   | $\{m_{001}   \frac{1}{4} \frac{1}{4} 0\}$ |
|                                                           | $b_1 \quad 0$                               | 0                                         |
| $c \quad (\frac{t}{2}, 1, 0)$                             | $\{2_{100}   0 \frac{1}{4} \frac{1}{4}\}$   | $\{m_{010}   \frac{1}{4} 0 \frac{1}{4}\}$ |
|                                                           | $c_1 \quad i$                               | $-ie^{-\frac{1}{4}i\pi t}$                |
|                                                           | $c_2 \quad i$                               | $ie^{-\frac{1}{4}i\pi t}$                 |
|                                                           | $c_3 \quad -i$                              | $-ie^{-\frac{1}{4}i\pi t}$                |
|                                                           | $c_4 \quad -i$                              | $ie^{-\frac{1}{4}i\pi t}$                 |
| $d \quad (\frac{t}{2}, \frac{t}{2}, \frac{t}{2})$         | $\{3_{111}   0 0 0\}$                       | $\{m_{1-10}   0 0 0\}$                    |
|                                                           | $d_1 \quad -1$                              | $-i$                                      |
|                                                           | $d_2 \quad -1$                              | $i$                                       |
|                                                           | $d_3 \quad 1$                               | 0                                         |
| $e \quad (1 - \frac{t}{2}, 1 - \frac{t}{2}, \frac{t}{2})$ | $\{m_{1-10}   0 0 0\}$                      |                                           |
|                                                           | $e_1 \quad -i$                              |                                           |
|                                                           | $e_2 \quad i$                               |                                           |
| $f \quad (\frac{1}{2}, 1 - \frac{t}{2}, \frac{t}{2})$     | $\{2_{01-1}   0 0 0\}$                      |                                           |
|                                                           | $f_1 \quad -i$                              |                                           |
|                                                           | $f_2 \quad i$                               |                                           |

$$\begin{aligned} \mathcal{W}_1^{\text{gapless}} = & \sum_{m=1}^{n_{a_1}} \text{sgn}(v_m^{a_1}) \frac{1 - \text{sgn}(\delta_m^{a_1})}{2} + \sum_{m=1}^{n_{a_2}} \text{sgn}(v_m^{a_2}) \frac{1 - \text{sgn}(\delta_m^{a_2})}{2} - \sum_{m=1}^{n_{d_1}} \text{sgn}(v_m^{d_1}) \frac{1 - \text{sgn}(\delta_m^{d_1})}{2} \\ & - \sum_{m=1}^{n_{d_3}} \text{sgn}(v_m^{d_3}) \frac{1 - \text{sgn}(\delta_m^{d_3})}{2} + \sum_{m=1}^{n_{e_1}} \text{sgn}(v_m^{e_1}) \frac{1 - \text{sgn}(\delta_m^{e_1})}{2} \end{aligned} \quad (\text{S227.1})$$

$$\mathcal{W}_2^{\text{gapless}} = \sum_{m=1}^{n_{b_1}} \text{sgn}(v_m^{b_1}) \frac{1 - \text{sgn}(\delta_m^{b_1})}{2} - \sum_{m=1}^{n_{d_1}} \text{sgn}(v_m^{d_1}) \frac{1 - \text{sgn}(\delta_m^{d_1})}{2} - \sum_{m=1}^{n_{d_3}} \text{sgn}(v_m^{d_3}) \frac{1 - \text{sgn}(\delta_m^{d_3})}{2} + \sum_{m=1}^{n_{e_1}} \text{sgn}(v_m^{e_1}) \frac{1 - \text{sgn}(\delta_m^{e_1})}{2} \quad (\text{S227.2})$$

$$\mathcal{W}_3^{\text{gapless}} = \sum_{m=1}^{n_{c_1}} \text{sgn}(v_m^{c_1}) \frac{1 - \text{sgn}(\delta_m^{c_1})}{2} + \sum_{m=1}^{n_{c_3}} \text{sgn}(v_m^{c_3}) \frac{1 - \text{sgn}(\delta_m^{c_3})}{2} - \sum_{m=1}^{n_{e_1}} \text{sgn}(v_m^{e_1}) \frac{1 - \text{sgn}(\delta_m^{e_1})}{2} + \sum_{m=1}^{n_{f_1}} \text{sgn}(v_m^{f_1}) \frac{1 - \text{sgn}(\delta_m^{f_1})}{2} \quad (\text{S227.3})$$

**S228. SPACE GROUP NO. 228**

| line segment        | character of irrep (generators only)                |                                           |
|---------------------|-----------------------------------------------------|-------------------------------------------|
| $a \quad (0, t, 0)$ | $\{4_{010}   \frac{1}{4} \frac{1}{4} \frac{1}{2}\}$ | $\{m_{100}   0 \frac{1}{4} \frac{1}{4}\}$ |
|                     | $a_1 \quad -\sqrt{2}e^{-\frac{1}{2}i\pi t}$         | 0                                         |
|                     | $a_2 \quad \sqrt{2}e^{-\frac{1}{2}i\pi t}$          | 0                                         |
| $b \quad (t, t, 0)$ | $\{2_{110}   \frac{1}{4} \frac{1}{4} \frac{1}{2}\}$ | $\{m_{001}   \frac{1}{4} \frac{1}{4} 0\}$ |
|                     | $b_1 \quad 0$                                       | 0                                         |

|                                                                  |       |                                                                                     |
|------------------------------------------------------------------|-------|-------------------------------------------------------------------------------------|
| $c \left( \frac{t}{2}, 1, 0 \right)$                             | $c_1$ | $\{2_{100}   0 \frac{1}{4} \frac{1}{4} \} \{m_{010}   \frac{1}{4} 0 \frac{1}{4} \}$ |
|                                                                  | $c_2$ | $i \quad -ie^{-\frac{1}{4}i\pi t}$                                                  |
|                                                                  | $c_3$ | $-i \quad ie^{-\frac{1}{4}i\pi t}$                                                  |
|                                                                  | $c_4$ | $-i \quad -ie^{-\frac{1}{4}i\pi t}$                                                 |
| $d \left( \frac{t}{2}, \frac{t}{2}, \frac{t}{2} \right)$         | $d_1$ | $\{3_{111}   0 0 0 \} \{m_{1-10}   \frac{1}{2} \frac{1}{2} \frac{1}{2} \}$          |
|                                                                  | $d_2$ | $-1 \quad -ie^{-\frac{3}{2}i\pi t}$                                                 |
|                                                                  | $d_3$ | $-1 \quad ie^{-\frac{3}{2}i\pi t}$                                                  |
| $e \left( 1 - \frac{t}{2}, 1 - \frac{t}{2}, \frac{t}{2} \right)$ | $e_1$ | $\{m_{1-10}   \frac{1}{2} \frac{1}{2} \frac{1}{2} \}$                               |
|                                                                  | $e_2$ | $-ie^{-2i\pi(1-\frac{t}{4})} \quad ie^{-2i\pi(1-\frac{t}{4})}$                      |
| $f \left( \frac{1}{2}, 1 - \frac{t}{2}, \frac{t}{2} \right)$     | $f_1$ | $\{2_{01-1}   \frac{1}{2} \frac{1}{2} \frac{1}{2} \}$                               |
|                                                                  | $f_2$ | $-i \quad i$                                                                        |

$$\begin{aligned} \mathcal{W}_1^{\text{gapless}} = & \sum_{m=1}^{n_{a_1}} \text{sgn}(v_m^{a_1}) \frac{1 - \text{sgn}(\delta_m^{a_1})}{2} + \sum_{m=1}^{n_{a_2}} \text{sgn}(v_m^{a_2}) \frac{1 - \text{sgn}(\delta_m^{a_2})}{2} - \sum_{m=1}^{n_{d_1}} \text{sgn}(v_m^{d_1}) \frac{1 - \text{sgn}(\delta_m^{d_1})}{2} \\ & - \sum_{m=1}^{n_{d_3}} \text{sgn}(v_m^{d_3}) \frac{1 - \text{sgn}(\delta_m^{d_3})}{2} + \sum_{m=1}^{n_{e_1}} \text{sgn}(v_m^{e_1}) \frac{1 - \text{sgn}(\delta_m^{e_1})}{2} \end{aligned} \quad (\text{S228.1})$$

$$\mathcal{W}_2^{\text{gapless}} = \sum_{m=1}^{n_{b_1}} \text{sgn}(v_m^{b_1}) \frac{1 - \text{sgn}(\delta_m^{b_1})}{2} - \sum_{m=1}^{n_{d_1}} \text{sgn}(v_m^{d_1}) \frac{1 - \text{sgn}(\delta_m^{d_1})}{2} - \sum_{m=1}^{n_{d_3}} \text{sgn}(v_m^{d_3}) \frac{1 - \text{sgn}(\delta_m^{d_3})}{2} + \sum_{m=1}^{n_{e_1}} \text{sgn}(v_m^{e_1}) \frac{1 - \text{sgn}(\delta_m^{e_1})}{2} \quad (\text{S228.2})$$

$$\begin{aligned} \mathcal{W}_3^{\text{gapless}} = & \sum_{m=1}^{n_{c_1}} \text{sgn}(v_m^{c_1}) \frac{1 - \text{sgn}(\delta_m^{c_1})}{2} + \sum_{m=1}^{n_{c_3}} \text{sgn}(v_m^{c_3}) \frac{1 - \text{sgn}(\delta_m^{c_3})}{2} - \sum_{m=1}^{n_{e_1}} \text{sgn}(v_m^{e_1}) \frac{1 - \text{sgn}(\delta_m^{e_1})}{2} \\ & + \sum_{m=1}^{n_{f_1}} \text{sgn}(v_m^{f_1}) \frac{1 - \text{sgn}(\delta_m^{f_1})}{2} + \sum_{m=1}^{n_{f_2}} \text{sgn}(v_m^{f_2}) \frac{1 - \text{sgn}(\delta_m^{f_2})}{2} \end{aligned} \quad (\text{S228.3})$$

$$\mathcal{X}_1 = \sum_{m=1}^{n_{e_1}} \frac{1 - \text{sgn}(\delta_m^{e_1})}{2} \quad \text{mod } 2 \quad (\text{S228.4})$$

## S229. SPACE GROUP NO. 229

| line segment                                       | character of irrep (generators only)         |     |
|----------------------------------------------------|----------------------------------------------|-----|
| $a \left( t, 0, 0 \right)$                         | $\{4_{100}   0 0 0 \} \{m_{010}   0 0 0 \}$  |     |
|                                                    | $a_1 \quad -\sqrt{2}$                        | $0$ |
|                                                    | $a_2 \quad \sqrt{2}$                         | $0$ |
| $b \left( \frac{t+1}{2}, \frac{1-t}{2}, 0 \right)$ | $\{2_{1-10}   0 0 0 \} \{m_{001}   0 0 0 \}$ |     |
|                                                    | $b_1 \quad 0$                                | $0$ |
| $c \left( \frac{t}{2}, \frac{t}{2}, 0 \right)$     | $\{2_{110}   0 0 0 \} \{m_{001}   0 0 0 \}$  |     |
|                                                    | $c_1 \quad 0$                                | $0$ |

|                                                              |       |                                |                            |
|--------------------------------------------------------------|-------|--------------------------------|----------------------------|
| $d \left( \frac{1}{2}, \frac{1}{2}, \frac{t}{2} \right)$     | $d_1$ | $\{2_{001}   0 \ 0 \ 0\}$      | $\{m_{110}   0 \ 0 \ 0\}$  |
|                                                              |       | 0                              | 0                          |
| $e \left( \frac{t}{2}, \frac{t}{2}, \frac{t}{2} \right)$     | $e_1$ | $\{3_{111}   0 \ 0 \ 0\}$      | $\{m_{1-10}   0 \ 0 \ 0\}$ |
|                                                              | $e_2$ | -1                             | -i                         |
|                                                              | $e_3$ | -1                             | i                          |
|                                                              | $e_3$ | 1                              | 0                          |
| $f \left( 1 - \frac{t}{2}, \frac{t}{2}, \frac{t}{2} \right)$ | $f_1$ | $\{3_{-1-1-1}^-   0 \ 0 \ 0\}$ | $\{m_{110}   0 \ 0 \ 0\}$  |
|                                                              | $f_2$ | -1                             | -i                         |
|                                                              | $f_2$ | -1                             | i                          |
|                                                              | $f_3$ | 1                              | 0                          |

$$\begin{aligned} \mathcal{W}_1^{\text{gapless}} = & \sum_{m=1}^{n_{a_1}} \text{sgn}(v_m^{a_1}) \frac{1 - \text{sgn}(\delta_m^{a_1})}{2} + \sum_{m=1}^{n_{a_2}} \text{sgn}(v_m^{a_2}) \frac{1 - \text{sgn}(\delta_m^{a_2})}{2} - \sum_{m=1}^{n_{e_1}} \text{sgn}(v_m^{e_1}) \frac{1 - \text{sgn}(\delta_m^{e_1})}{2} \\ & - \sum_{m=1}^{n_{e_3}} \text{sgn}(v_m^{e_3}) \frac{1 - \text{sgn}(\delta_m^{e_3})}{2} + \sum_{m=1}^{n_{f_1}} \text{sgn}(v_m^{f_1}) \frac{1 - \text{sgn}(\delta_m^{f_1})}{2} + \sum_{m=1}^{n_{f_3}} \text{sgn}(v_m^{f_3}) \frac{1 - \text{sgn}(\delta_m^{f_3})}{2} \end{aligned} \quad (\text{S229.1})$$

$$\mathcal{W}_2^{\text{gapless}} = \sum_{m=1}^{n_{b_1}} \text{sgn}(v_m^{b_1}) \frac{1 - \text{sgn}(\delta_m^{b_1})}{2} - \sum_{m=1}^{n_{d_1}} \text{sgn}(v_m^{d_1}) \frac{1 - \text{sgn}(\delta_m^{d_1})}{2} + \sum_{m=1}^{n_{f_1}} \text{sgn}(v_m^{f_1}) \frac{1 - \text{sgn}(\delta_m^{f_1})}{2} + \sum_{m=1}^{n_{f_3}} \text{sgn}(v_m^{f_3}) \frac{1 - \text{sgn}(\delta_m^{f_3})}{2} \quad (\text{S229.2})$$

$$\mathcal{W}_3^{\text{gapless}} = \sum_{m=1}^{n_{c_1}} \text{sgn}(v_m^{c_1}) \frac{1 - \text{sgn}(\delta_m^{c_1})}{2} + \sum_{m=1}^{n_{d_1}} \text{sgn}(v_m^{d_1}) \frac{1 - \text{sgn}(\delta_m^{d_1})}{2} - \sum_{m=1}^{n_{e_1}} \text{sgn}(v_m^{e_1}) \frac{1 - \text{sgn}(\delta_m^{e_1})}{2} - \sum_{m=1}^{n_{e_3}} \text{sgn}(v_m^{e_3}) \frac{1 - \text{sgn}(\delta_m^{e_3})}{2} \quad (\text{S229.3})$$

### S230. SPACE GROUP NO. 230

| line segment                                               | character of irrep (generators only)                     |                                                          |
|------------------------------------------------------------|----------------------------------------------------------|----------------------------------------------------------|
| $a \ (t, 0, 0)$                                            | $\{4_{100}   \frac{1}{4} \ \frac{1}{4} \ \frac{3}{4}\}$  | $\{m_{010}   \frac{1}{2} \ 0 \ 0\}$                      |
|                                                            | $a_1$                                                    | $-\sqrt{2}e^{-\frac{1}{2}i\pi t}$                        |
|                                                            | $a_2$                                                    | $\sqrt{2}e^{-\frac{1}{2}i\pi t}$                         |
| $b \ \left( \frac{t+1}{2}, \frac{1-t}{2}, 0 \right)$       | $\{2_{1-10}   \frac{1}{4} \ \frac{1}{4} \ \frac{1}{4}\}$ | $\{m_{001}   0 \ \frac{1}{2} \ 0\}$                      |
|                                                            | $b_1$                                                    | $i$                                                      |
|                                                            | $b_2$                                                    | $i$                                                      |
|                                                            | $b_3$                                                    | $-i$                                                     |
| $c \ \left( \frac{t}{2}, \frac{t}{2}, 0 \right)$           | $\{2_{110}   \frac{3}{4} \ \frac{1}{4} \ \frac{1}{4}\}$  | $\{m_{001}   0 \ \frac{1}{2} \ 0\}$                      |
|                                                            | $c_1$                                                    | 0                                                        |
| $d \ \left( \frac{1}{2}, \frac{1}{2}, \frac{t}{2} \right)$ | $\{2_{001}   0 \ \frac{1}{2} \ 0\}$                      | $\{m_{110}   \frac{3}{4} \ \frac{1}{4} \ \frac{1}{4}\}$  |
|                                                            | $d_1$                                                    | $i$                                                      |
|                                                            | $d_2$                                                    | $i$                                                      |
|                                                            | $d_3$                                                    | $-i$                                                     |
| $e \ \left( \frac{t}{2}, \frac{t}{2}, \frac{t}{2} \right)$ | $\{3_{111}   0 \ 0 \ 0\}$                                | $\{m_{1-10}   \frac{1}{4} \ \frac{1}{4} \ \frac{1}{4}\}$ |
|                                                            | $e_1$                                                    | $-1$                                                     |
|                                                            | $e_2$                                                    | $-1$                                                     |
|                                                            | $e_3$                                                    | 1                                                        |

|       |                                               |                                                         |
|-------|-----------------------------------------------|---------------------------------------------------------|
|       | $\{3^{-1-1-1}   \frac{1}{2} \ 0 \ 0\}$        | $\{m_{110}   \frac{3}{4} \ \frac{1}{4} \ \frac{1}{4}\}$ |
| $f$   | $(1 - \frac{t}{2}, \frac{t}{2}, \frac{t}{2})$ |                                                         |
| $f_1$ | $-e^{-\frac{1}{2}i\pi(2-t)}$                  | $-ie^{-\frac{1}{4}i\pi(6-t)}$                           |
| $f_2$ | $-e^{-\frac{1}{2}i\pi(2-t)}$                  | $ie^{-\frac{1}{4}i\pi(6-t)}$                            |
| $f_3$ | $e^{-\frac{1}{2}i\pi(2-t)}$                   | $0$                                                     |

$$\begin{aligned} \mathcal{W}_1^{\text{gapless}} = & \sum_{m=1}^{n_{a_1}} \text{sgn}(v_m^{a_1}) \frac{1 - \text{sgn}(\delta_m^{a_1})}{2} + \sum_{m=1}^{n_{a_2}} \text{sgn}(v_m^{a_2}) \frac{1 - \text{sgn}(\delta_m^{a_2})}{2} - \sum_{m=1}^{n_{e_1}} \text{sgn}(v_m^{e_1}) \frac{1 - \text{sgn}(\delta_m^{e_1})}{2} \\ & - \sum_{m=1}^{n_{e_3}} \text{sgn}(v_m^{e_3}) \frac{1 - \text{sgn}(\delta_m^{e_3})}{2} + \sum_{m=1}^{n_{f_1}} \text{sgn}(v_m^{f_1}) \frac{1 - \text{sgn}(\delta_m^{f_1})}{2} + \sum_{m=1}^{n_{f_3}} \text{sgn}(v_m^{f_3}) \frac{1 - \text{sgn}(\delta_m^{f_3})}{2} \end{aligned} \quad (\text{S230.1})$$

$$\begin{aligned} \mathcal{W}_2^{\text{gapless}} = & \sum_{m=1}^{n_{b_1}} \text{sgn}(v_m^{b_1}) \frac{1 - \text{sgn}(\delta_m^{b_1})}{2} + \sum_{m=1}^{n_{b_3}} \text{sgn}(v_m^{b_3}) \frac{1 - \text{sgn}(\delta_m^{b_3})}{2} - \sum_{m=1}^{n_{d_1}} \text{sgn}(v_m^{d_1}) \frac{1 - \text{sgn}(\delta_m^{d_1})}{2} \\ & - \sum_{m=1}^{n_{d_3}} \text{sgn}(v_m^{d_3}) \frac{1 - \text{sgn}(\delta_m^{d_3})}{2} + \sum_{m=1}^{n_{f_1}} \text{sgn}(v_m^{f_1}) \frac{1 - \text{sgn}(\delta_m^{f_1})}{2} + \sum_{m=1}^{n_{f_3}} \text{sgn}(v_m^{f_3}) \frac{1 - \text{sgn}(\delta_m^{f_3})}{2} \end{aligned} \quad (\text{S230.2})$$

$$\begin{aligned} \mathcal{W}_3^{\text{gapless}} = & \sum_{m=1}^{n_{c_1}} \text{sgn}(v_m^{c_1}) \frac{1 - \text{sgn}(\delta_m^{c_1})}{2} + \sum_{m=1}^{n_{d_1}} \text{sgn}(v_m^{d_1}) \frac{1 - \text{sgn}(\delta_m^{d_1})}{2} + \sum_{m=1}^{n_{d_3}} \text{sgn}(v_m^{d_3}) \frac{1 - \text{sgn}(\delta_m^{d_3})}{2} \\ & - \sum_{m=1}^{n_{e_1}} \text{sgn}(v_m^{e_1}) \frac{1 - \text{sgn}(\delta_m^{e_1})}{2} - \sum_{m=1}^{n_{e_3}} \text{sgn}(v_m^{e_3}) \frac{1 - \text{sgn}(\delta_m^{e_3})}{2} \end{aligned} \quad (\text{S230.3})$$

$$\begin{aligned} \mathcal{W}_1^{\text{gapped}} = & 2 \sum_{m=1}^{n_{b_3}} \text{sgn}(v_m^{b_3}) \frac{1 - \text{sgn}(\delta_m^{b_3})}{2} - \sum_{m=1}^{n_{d_1}} \text{sgn}(v_m^{d_1}) \frac{1 - \text{sgn}(\delta_m^{d_1})}{2} - \sum_{m=1}^{n_{d_3}} \text{sgn}(v_m^{d_3}) \frac{1 - \text{sgn}(\delta_m^{d_3})}{2} \\ & + \sum_{m=1}^{n_{f_1}} \text{sgn}(v_m^{f_1}) \frac{1 - \text{sgn}(\delta_m^{f_1})}{2} + \sum_{m=1}^{n_{f_3}} \text{sgn}(v_m^{f_3}) \frac{1 - \text{sgn}(\delta_m^{f_3})}{2} \end{aligned} \quad (\text{S230.4})$$

**L1. LAYER GROUP NO. 1**

| line segment                                   | character of irrep (generators only)                       |
|------------------------------------------------|------------------------------------------------------------|
| $a \left( \frac{t}{2}, 0, 0 \right)$           | $\begin{matrix} \{1  0 & 0 & 0 \} \\ a_1 & 1 \end{matrix}$ |
| $b \left( \frac{1}{2}, \frac{t}{2}, 0 \right)$ | $\begin{matrix} \{1  0 & 0 & 0 \} \\ b_1 & 1 \end{matrix}$ |
| $c \left( \frac{t}{2}, \frac{1}{2}, 0 \right)$ | $\begin{matrix} \{1  0 & 0 & 0 \} \\ c_1 & 1 \end{matrix}$ |

$$\mathcal{X}_1 = \sum_{m=1}^{n_{a_1}} \frac{1 - \text{sgn}(\delta_m^{a_1})}{2} + \sum_{m=1}^{n_{b_1}} \frac{1 - \text{sgn}(\delta_m^{b_1})}{2} \mod 2 \quad (\text{L1.1})$$

$$\mathcal{X}_2 = \sum_{m=1}^{n_{b_1}} \frac{1 - \text{sgn}(\delta_m^{b_1})}{2} \mod 2 \quad (\text{L1.2})$$

$$\mathcal{X}_3 = \sum_{m=1}^{n_{c_1}} \frac{1 - \text{sgn}(\delta_m^{c_1})}{2} \mod 2 \quad (\text{L1.3})$$

**L2. LAYER GROUP NO. 2**

| line segment                                   | character of irrep (generators only)                       |
|------------------------------------------------|------------------------------------------------------------|
| $a \left( \frac{t}{2}, 0, 0 \right)$           | $\begin{matrix} \{1  0 & 0 & 0 \} \\ a_1 & 1 \end{matrix}$ |
| $b \left( \frac{1}{2}, \frac{t}{2}, 0 \right)$ | $\begin{matrix} \{1  0 & 0 & 0 \} \\ b_1 & 1 \end{matrix}$ |
| $c \left( \frac{t}{2}, \frac{1}{2}, 0 \right)$ | $\begin{matrix} \{1  0 & 0 & 0 \} \\ c_1 & 1 \end{matrix}$ |

**L3. LAYER GROUP NO. 3**

| line segment                                   | character of irrep (generators only)                       |
|------------------------------------------------|------------------------------------------------------------|
| $a \left( \frac{t}{2}, 0, 0 \right)$           | $\begin{matrix} \{1  0 & 0 & 0 \} \\ a_1 & 1 \end{matrix}$ |
| $b \left( \frac{1}{2}, \frac{t}{2}, 0 \right)$ | $\begin{matrix} \{1  0 & 0 & 0 \} \\ b_1 & 1 \end{matrix}$ |
| $c \left( \frac{t}{2}, \frac{1}{2}, 0 \right)$ | $\begin{matrix} \{1  0 & 0 & 0 \} \\ c_1 & 1 \end{matrix}$ |

$$\mathcal{X}_1 = \sum_{m=1}^{n_{a_1}} \frac{1 - \text{sgn}(\delta_m^{a_1})}{2} + \sum_{m=1}^{n_{b_1}} \frac{1 - \text{sgn}(\delta_m^{b_1})}{2} \mod 2 \quad (\text{L3.1})$$

$$\mathcal{X}_2 = \sum_{m=1}^{n_{b_1}} \frac{1 - \text{sgn}(\delta_m^{b_1})}{2} \mod 2 \quad (\text{L3.2})$$

$$\mathcal{X}_3 = \sum_{m=1}^{n_{c_1}} \frac{1 - \text{sgn}(\delta_m^{c_1})}{2} \mod 2 \quad (\text{L3.3})$$

#### L4. LAYER GROUP NO. 4

| line segment                            | character of irrep (generators only)                                                                |
|-----------------------------------------|-----------------------------------------------------------------------------------------------------|
| $a \quad (\frac{t}{2}, 0, 0)$           | $\{m_{001}   \begin{smallmatrix} 0 & 0 & 0 \end{smallmatrix} \}$<br>$a_1 \quad -i$<br>$a_2 \quad i$ |
| $b \quad (\frac{1}{2}, \frac{t}{2}, 0)$ | $\{m_{001}   \begin{smallmatrix} 0 & 0 & 0 \end{smallmatrix} \}$<br>$b_1 \quad -i$<br>$b_2 \quad i$ |
| $c \quad (\frac{t}{2}, \frac{1}{2}, 0)$ | $\{m_{001}   \begin{smallmatrix} 0 & 0 & 0 \end{smallmatrix} \}$<br>$c_1 \quad -i$<br>$c_2 \quad i$ |

$$\mathcal{W}_1^{\text{gapless}} = \sum_{m=1}^{n_{a_1}} \text{sgn}(v_m^{a_1}) \frac{1 - \text{sgn}(\delta_m^{a_1})}{2} - \sum_{m=1}^{n_{a_2}} \text{sgn}(v_m^{a_2}) \frac{1 - \text{sgn}(\delta_m^{a_2})}{2} - \sum_{m=1}^{n_{c_1}} \text{sgn}(v_m^{c_1}) \frac{1 - \text{sgn}(\delta_m^{c_1})}{2} + \sum_{m=1}^{n_{c_2}} \text{sgn}(v_m^{c_2}) \frac{1 - \text{sgn}(\delta_m^{c_2})}{2} \quad (\text{L4.1})$$

$$\mathcal{W}_1^{\text{gapped}} = - \sum_{m=1}^{n_{b_1}} \text{sgn}(v_m^{b_1}) \frac{1 - \text{sgn}(\delta_m^{b_1})}{2} + \sum_{m=1}^{n_{b_2}} \text{sgn}(v_m^{b_2}) \frac{1 - \text{sgn}(\delta_m^{b_2})}{2} \quad (\text{L4.2})$$

$$\mathcal{W}_2^{\text{gapped}} = - \sum_{m=1}^{n_{c_1}} \text{sgn}(v_m^{c_1}) \frac{1 - \text{sgn}(\delta_m^{c_1})}{2} + \sum_{m=1}^{n_{c_2}} \text{sgn}(v_m^{c_2}) \frac{1 - \text{sgn}(\delta_m^{c_2})}{2} \quad (\text{L4.3})$$

#### L5. LAYER GROUP NO. 5

| line segment                            | character of irrep (generators only)                                                                                                                      |
|-----------------------------------------|-----------------------------------------------------------------------------------------------------------------------------------------------------------|
| $a \quad (\frac{t}{2}, 0, 0)$           | $\{m_{001}   \begin{smallmatrix} \frac{1}{2} & 0 & 0 \end{smallmatrix} \}$<br>$a_1 \quad -ie^{-\frac{1}{2}i\pi t}$<br>$a_2 \quad ie^{-\frac{1}{2}i\pi t}$ |
| $b \quad (\frac{1}{2}, \frac{t}{2}, 0)$ | $\{m_{001}   \begin{smallmatrix} \frac{1}{2} & 0 & 0 \end{smallmatrix} \}$<br>$b_1 \quad -1$<br>$b_2 \quad 1$                                             |
| $c \quad (\frac{t}{2}, \frac{1}{2}, 0)$ | $\{m_{001}   \begin{smallmatrix} \frac{1}{2} & 0 & 0 \end{smallmatrix} \}$<br>$c_1 \quad -ie^{-\frac{1}{2}i\pi t}$<br>$c_2 \quad ie^{-\frac{1}{2}i\pi t}$ |

$$\mathcal{W}_1^{\text{gapless}} = \sum_{m=1}^{n_{a_1}} \text{sgn}(v_m^{a_1}) \frac{1 - \text{sgn}(\delta_m^{a_1})}{2} - \sum_{m=1}^{n_{a_2}} \text{sgn}(v_m^{a_2}) \frac{1 - \text{sgn}(\delta_m^{a_2})}{2} + \sum_{m=1}^{n_{b_1}} \text{sgn}(v_m^{b_1}) \frac{1 - \text{sgn}(\delta_m^{b_1})}{2} \\ - \sum_{m=1}^{n_{b_2}} \text{sgn}(v_m^{b_2}) \frac{1 - \text{sgn}(\delta_m^{b_2})}{2} - \sum_{m=1}^{n_{c_1}} \text{sgn}(v_m^{c_1}) \frac{1 - \text{sgn}(\delta_m^{c_1})}{2} + \sum_{m=1}^{n_{c_2}} \text{sgn}(v_m^{c_2}) \frac{1 - \text{sgn}(\delta_m^{c_2})}{2} \quad (\text{L5.1})$$

$$\mathcal{X}_1 = \sum_{m=1}^{n_{b_1}} \frac{1 - \text{sgn}(\delta_m^{b_1})}{2} + \sum_{m=1}^{n_{b_2}} \frac{1 - \text{sgn}(\delta_m^{b_2})}{2} + \sum_{m=1}^{n_{c_1}} \frac{1 - \text{sgn}(\delta_m^{c_1})}{2} + \sum_{m=1}^{n_{c_2}} \frac{1 - \text{sgn}(\delta_m^{c_2})}{2} \mod 2 \quad (\text{L5.2})$$

$$\mathcal{X}_2 = \sum_{m=1}^{n_{b_1}} \frac{1 - \text{sgn}(\delta_m^{b_1})}{2} + \sum_{m=1}^{n_{c_1}} \frac{1 - \text{sgn}(\delta_m^{c_1})}{2} + \sum_{m=1}^{n_{c_2}} \frac{1 - \text{sgn}(\delta_m^{c_2})}{2} \mod 2 \quad (\text{L5.3})$$

$$\mathcal{X}_3 = \sum_{m=1}^{n_{b_1}} \frac{1 - \text{sgn}(\delta_m^{b_1})}{2} \mod 2 \quad (\text{L5.4})$$

#### L6. LAYER GROUP NO. 6

| line segment                            | character of irrep (generators only)                                        |
|-----------------------------------------|-----------------------------------------------------------------------------|
| $a \quad (\frac{t}{2}, 0, 0)$           | $\{m_{001}   \begin{smallmatrix} 0 & 0 & 0 \\ -i \\ i \end{smallmatrix} \}$ |
| $b \quad (\frac{1}{2}, \frac{t}{2}, 0)$ | $\{m_{001}   \begin{smallmatrix} 0 & 0 & 0 \\ -i \\ i \end{smallmatrix} \}$ |
| $c \quad (\frac{t}{2}, \frac{1}{2}, 0)$ | $\{m_{001}   \begin{smallmatrix} 0 & 0 & 0 \\ -i \\ i \end{smallmatrix} \}$ |

#### L7. LAYER GROUP NO. 7

| line segment                            | character of irrep (generators only)                                                                                              |
|-----------------------------------------|-----------------------------------------------------------------------------------------------------------------------------------|
| $a \quad (\frac{t}{2}, 0, 0)$           | $\{m_{001}   \begin{smallmatrix} \frac{1}{2} & 0 & 0 \\ -ie^{-\frac{1}{2}i\pi t} \\ ie^{-\frac{1}{2}i\pi t} \end{smallmatrix} \}$ |
| $b \quad (\frac{1}{2}, \frac{t}{2}, 0)$ | $\{m_{001}   \begin{smallmatrix} \frac{1}{2} & 0 & 0 \\ -1 \\ 1 \end{smallmatrix} \}$                                             |
| $c \quad (\frac{t}{2}, \frac{1}{2}, 0)$ | $\{m_{001}   \begin{smallmatrix} \frac{1}{2} & 0 & 0 \\ -ie^{-\frac{1}{2}i\pi t} \\ ie^{-\frac{1}{2}i\pi t} \end{smallmatrix} \}$ |

---


$$\mathcal{X}_1 = \sum_{m=1}^{n_{b_1}} \frac{1 - \text{sgn}(\delta_m^{b_1})}{2} \mod 2 \quad (\text{L7.1})$$

### L8. LAYER GROUP NO. 8

| line segment                            | character of irrep (generators only)                                                  |
|-----------------------------------------|---------------------------------------------------------------------------------------|
| $a \quad (\frac{t}{2}, 0, 0)$           | $\begin{array}{c} \{2_{100}   0 \ 0 \ 0\} \\ a_1 \quad -i \\ a_2 \quad i \end{array}$ |
| $b \quad (0, \frac{t}{2}, 0)$           | $\begin{array}{c} \{1   0 \ 0 \ 0\} \\ b_1 \quad 1 \end{array}$                       |
| $c \quad (\frac{1}{2}, \frac{t}{2}, 0)$ | $\begin{array}{c} \{1   0 \ 0 \ 0\} \\ c_1 \quad 1 \end{array}$                       |
| $d \quad (\frac{t}{2}, \frac{1}{2}, 0)$ | $\begin{array}{c} \{2_{100}   0 \ 0 \ 0\} \\ d_1 \quad -i \\ d_2 \quad i \end{array}$ |

$$\begin{aligned} \mathcal{W}_1^{\text{gapless}} = & \sum_{m=1}^{n_{a_1}} \text{sgn}(v_m^{a_1}) \frac{1 - \text{sgn}(\delta_m^{a_1})}{2} + \sum_{m=1}^{n_{a_2}} \text{sgn}(v_m^{a_2}) \frac{1 - \text{sgn}(\delta_m^{a_2})}{2} - \sum_{m=1}^{n_{b_1}} \text{sgn}(v_m^{b_1}) \frac{1 - \text{sgn}(\delta_m^{b_1})}{2} \\ & + \sum_{m=1}^{n_{c_1}} \text{sgn}(v_m^{c_1}) \frac{1 - \text{sgn}(\delta_m^{c_1})}{2} - \sum_{m=1}^{n_{d_1}} \text{sgn}(v_m^{d_1}) \frac{1 - \text{sgn}(\delta_m^{d_1})}{2} - \sum_{m=1}^{n_{d_2}} \text{sgn}(v_m^{d_2}) \frac{1 - \text{sgn}(\delta_m^{d_2})}{2} \end{aligned} \quad (\text{L8.1})$$

$$\begin{aligned} \mathcal{W}_1^{\text{gapped}} = & -2 \sum_{m=1}^{n_{a_2}} \text{sgn}(v_m^{a_2}) \frac{1 - \text{sgn}(\delta_m^{a_2})}{2} + \sum_{m=1}^{n_{b_1}} \text{sgn}(v_m^{b_1}) \frac{1 - \text{sgn}(\delta_m^{b_1})}{2} - \sum_{m=1}^{n_{c_1}} \text{sgn}(v_m^{c_1}) \frac{1 - \text{sgn}(\delta_m^{c_1})}{2} \\ & + \sum_{m=1}^{n_{d_1}} \text{sgn}(v_m^{d_1}) \frac{1 - \text{sgn}(\delta_m^{d_1})}{2} + \sum_{m=1}^{n_{d_2}} \text{sgn}(v_m^{d_2}) \frac{1 - \text{sgn}(\delta_m^{d_2})}{2} \end{aligned} \quad (\text{L8.2})$$

$$\begin{aligned} \mathcal{W}_2^{\text{gapped}} = & -2 \sum_{m=1}^{n_{a_2}} \text{sgn}(v_m^{a_2}) \frac{1 - \text{sgn}(\delta_m^{a_2})}{2} + \sum_{m=1}^{n_{b_1}} \text{sgn}(v_m^{b_1}) \frac{1 - \text{sgn}(\delta_m^{b_1})}{2} - \sum_{m=1}^{n_{c_1}} \text{sgn}(v_m^{c_1}) \frac{1 - \text{sgn}(\delta_m^{c_1})}{2} \\ & + 2 \sum_{m=1}^{n_{d_2}} \text{sgn}(v_m^{d_2}) \frac{1 - \text{sgn}(\delta_m^{d_2})}{2} \end{aligned} \quad (\text{L8.3})$$

$$\mathcal{X}_1 = \sum_{m=1}^{n_{c_1}} \frac{1 - \text{sgn}(\delta_m^{c_1})}{2} \mod 2 \quad (\text{L8.4})$$



**L9. LAYER GROUP NO. 9**

| line segment                            | character of irrep (generators only)                                                                                                        |
|-----------------------------------------|---------------------------------------------------------------------------------------------------------------------------------------------|
| $a \quad (\frac{t}{2}, 0, 0)$           | $\begin{matrix} \{2_{100}   \frac{1}{2} \ 0 \ 0 \} \\ a_1 \quad -ie^{-\frac{1}{2}i\pi t} \\ a_2 \quad ie^{-\frac{1}{2}i\pi t} \end{matrix}$ |
| $b \quad (0, \frac{t}{2}, 0)$           | $\begin{matrix} \{1   0 \ 0 \ 0 \} \\ b_1 \quad 1 \end{matrix}$                                                                             |
| $c \quad (\frac{1}{2}, \frac{t}{2}, 0)$ | $\begin{matrix} \{1   0 \ 0 \ 0 \} \\ c_1 \quad 1 \end{matrix}$                                                                             |
| $d \quad (\frac{t}{2}, \frac{1}{2}, 0)$ | $\begin{matrix} \{2_{100}   \frac{1}{2} \ 0 \ 0 \} \\ d_1 \quad -ie^{-\frac{1}{2}i\pi t} \\ d_2 \quad ie^{-\frac{1}{2}i\pi t} \end{matrix}$ |

$$\begin{aligned} \mathcal{W}_1^{\text{gapless}} = & \sum_{m=1}^{n_{a_1}} \text{sgn}(v_m^{a_1}) \frac{1 - \text{sgn}(\delta_m^{a_1})}{2} + \sum_{m=1}^{n_{a_2}} \text{sgn}(v_m^{a_2}) \frac{1 - \text{sgn}(\delta_m^{a_2})}{2} - \sum_{m=1}^{n_{b_1}} \text{sgn}(v_m^{b_1}) \frac{1 - \text{sgn}(\delta_m^{b_1})}{2} \\ & + 2 \sum_{m=1}^{n_{c_1}} \text{sgn}(v_m^{c_1}) \frac{1 - \text{sgn}(\delta_m^{c_1})}{2} - \sum_{m=1}^{n_{d_1}} \text{sgn}(v_m^{d_1}) \frac{1 - \text{sgn}(\delta_m^{d_1})}{2} - \sum_{m=1}^{n_{d_2}} \text{sgn}(v_m^{d_2}) \frac{1 - \text{sgn}(\delta_m^{d_2})}{2} \end{aligned} \quad (\text{L9.1})$$

$$\mathcal{X}_1 = \sum_{m=1}^{n_{b_1}} \frac{1 - \text{sgn}(\delta_m^{b_1})}{2} + \sum_{m=1}^{n_{d_1}} \frac{1 - \text{sgn}(\delta_m^{d_1})}{2} + \sum_{m=1}^{n_{d_2}} \frac{1 - \text{sgn}(\delta_m^{d_2})}{2} \quad \text{mod } 2 \quad (\text{L9.2})$$

$$\mathcal{X}_2 = 2 \sum_{m=1}^{n_{a_2}} \text{sgn}(v_m^{a_2}) \frac{1 - \text{sgn}(\delta_m^{a_2})}{2} - \sum_{m=1}^{n_{b_1}} \text{sgn}(v_m^{b_1}) \frac{1 - \text{sgn}(\delta_m^{b_1})}{2} - 2 \sum_{m=1}^{n_{d_1}} \text{sgn}(v_m^{d_1}) \frac{1 - \text{sgn}(\delta_m^{d_1})}{2} \quad \text{mod } 4 \quad (\text{L9.3})$$

**L10. LAYER GROUP NO. 10**

| line segment                                | character of irrep (generators only)                                                  |
|---------------------------------------------|---------------------------------------------------------------------------------------|
| $a \quad (t, 0, 0)$                         | $\begin{matrix} \{2_{100}   0 \ 0 \ 0 \} \\ a_1 \quad -i \\ a_2 \quad i \end{matrix}$ |
| $b \quad (0, t, 0)$                         | $\begin{matrix} \{1   0 \ 0 \ 0 \} \\ b_1 \quad 1 \end{matrix}$                       |
| $c \quad (\frac{t}{2}, 1 - \frac{t}{2}, 0)$ | $\begin{matrix} \{1   0 \ 0 \ 0 \} \\ c_1 \quad 1 \end{matrix}$                       |

$$\mathcal{W}_1^{\text{gapless}} = \sum_{m=1}^{n_{a_1}} \text{sgn}(v_m^{a_1}) \frac{1 - \text{sgn}(\delta_m^{a_1})}{2} + \sum_{m=1}^{n_{a_2}} \text{sgn}(v_m^{a_2}) \frac{1 - \text{sgn}(\delta_m^{a_2})}{2} - \sum_{m=1}^{n_{b_1}} \text{sgn}(v_m^{b_1}) \frac{1 - \text{sgn}(\delta_m^{b_1})}{2} \quad (\text{L10.1})$$

$$\mathcal{W}_1^{\text{gapped}} = -2 \sum_{m=1}^{n_{a_2}} \text{sgn}(v_m^{a_2}) \frac{1 - \text{sgn}(\delta_m^{a_2})}{2} + \sum_{m=1}^{n_{b_1}} \text{sgn}(v_m^{b_1}) \frac{1 - \text{sgn}(\delta_m^{b_1})}{2} \quad (\text{L10.2})$$

$$\mathcal{X}_1 = \sum_{m=1}^{n_{c_1}} \frac{1 - \text{sgn}(\delta_m^{c_1})}{2} \quad \text{mod } 2 \quad (\text{L10.3})$$

**L11. LAYER GROUP NO. 11**

| line segment                            | character of irrep (generators only)                                                 |
|-----------------------------------------|--------------------------------------------------------------------------------------|
| $a \quad (\frac{t}{2}, 0, 0)$           | $\begin{array}{c} \{1  0 \ 0 \ 0\} \\ a_1 \quad 1 \end{array}$                       |
| $b \quad (0, \frac{t}{2}, 0)$           | $\begin{array}{c} \{m_{100}  0 \ 0 \ 0\} \\ b_1 \quad -i \\ b_2 \quad i \end{array}$ |
| $c \quad (\frac{1}{2}, \frac{t}{2}, 0)$ | $\begin{array}{c} \{m_{100}  0 \ 0 \ 0\} \\ c_1 \quad -i \\ c_2 \quad i \end{array}$ |
| $d \quad (\frac{t}{2}, \frac{1}{2}, 0)$ | $\begin{array}{c} \{1  0 \ 0 \ 0\} \\ d_1 \quad 1 \end{array}$                       |

$$\begin{aligned} \mathcal{W}_1^{\text{gapless}} = & \sum_{m=1}^{n_{a_1}} \text{sgn}(v_m^{a_1}) \frac{1 - \text{sgn}(\delta_m^{a_1})}{2} - \sum_{m=1}^{n_{b_1}} \text{sgn}(v_m^{b_1}) \frac{1 - \text{sgn}(\delta_m^{b_1})}{2} - \sum_{m=1}^{n_{b_2}} \text{sgn}(v_m^{b_2}) \frac{1 - \text{sgn}(\delta_m^{b_2})}{2} \\ & + \sum_{m=1}^{n_{c_1}} \text{sgn}(v_m^{c_1}) \frac{1 - \text{sgn}(\delta_m^{c_1})}{2} + \sum_{m=1}^{n_{c_2}} \text{sgn}(v_m^{c_2}) \frac{1 - \text{sgn}(\delta_m^{c_2})}{2} - \sum_{m=1}^{n_{d_1}} \text{sgn}(v_m^{d_1}) \frac{1 - \text{sgn}(\delta_m^{d_1})}{2} \end{aligned} \quad (\text{L11.1})$$

$$\mathcal{W}_1^{\text{gapped}} = - \sum_{m=1}^{n_{c_1}} \text{sgn}(v_m^{c_1}) \frac{1 - \text{sgn}(\delta_m^{c_1})}{2} + \sum_{m=1}^{n_{c_2}} \text{sgn}(v_m^{c_2}) \frac{1 - \text{sgn}(\delta_m^{c_2})}{2} \quad (\text{L11.2})$$

$$\mathcal{W}_2^{\text{gapped}} = - \sum_{m=1}^{n_{b_1}} \text{sgn}(v_m^{b_1}) \frac{1 - \text{sgn}(\delta_m^{b_1})}{2} + \sum_{m=1}^{n_{b_2}} \text{sgn}(v_m^{b_2}) \frac{1 - \text{sgn}(\delta_m^{b_2})}{2} \quad (\text{L11.3})$$

$$\mathcal{X}_1 = \sum_{m=1}^{n_{d_1}} \frac{1 - \text{sgn}(\delta_m^{d_1})}{2} \quad \text{mod } 2 \quad (\text{L11.4})$$

**L12. LAYER GROUP NO. 12**

| line segment                            | character of irrep (generators only)                                                                                                       |
|-----------------------------------------|--------------------------------------------------------------------------------------------------------------------------------------------|
| $a \quad (\frac{t}{2}, 0, 0)$           | $\begin{array}{c} \{1  0 \ 0 \ 0\} \\ a_1 \quad 1 \end{array}$                                                                             |
| $b \quad (0, \frac{t}{2}, 0)$           | $\begin{array}{c} \{m_{100}  0 \ \frac{1}{2} \ 0\} \\ b_1 \quad -ie^{-\frac{1}{2}i\pi t} \\ b_2 \quad ie^{-\frac{1}{2}i\pi t} \end{array}$ |
| $c \quad (\frac{1}{2}, \frac{t}{2}, 0)$ | $\begin{array}{c} \{m_{100}  0 \ \frac{1}{2} \ 0\} \\ c_1 \quad -ie^{-\frac{1}{2}i\pi t} \\ c_2 \quad ie^{-\frac{1}{2}i\pi t} \end{array}$ |
| $d \quad (\frac{t}{2}, \frac{1}{2}, 0)$ | $\begin{array}{c} \{1  0 \ 0 \ 0\} \\ d_1 \quad 1 \end{array}$                                                                             |

---


$$\begin{aligned} \mathcal{W}_1^{\text{gapless}} = & \sum_{m=1}^{n_{a_1}} \text{sgn}(v_m^{a_1}) \frac{1 - \text{sgn}(\delta_m^{a_1})}{2} - \sum_{m=1}^{n_{b_1}} \text{sgn}(v_m^{b_1}) \frac{1 - \text{sgn}(\delta_m^{b_1})}{2} - \sum_{m=1}^{n_{b_2}} \text{sgn}(v_m^{b_2}) \frac{1 - \text{sgn}(\delta_m^{b_2})}{2} \\ & + \sum_{m=1}^{n_{c_1}} \text{sgn}(v_m^{c_1}) \frac{1 - \text{sgn}(\delta_m^{c_1})}{2} + \sum_{m=1}^{n_{c_2}} \text{sgn}(v_m^{c_2}) \frac{1 - \text{sgn}(\delta_m^{c_2})}{2} - 2 \sum_{m=1}^{n_{d_1}} \text{sgn}(v_m^{d_1}) \frac{1 - \text{sgn}(\delta_m^{d_1})}{2} \end{aligned} \quad (\text{L12.1})$$

$$\mathcal{X}_1 = \sum_{m=1}^{n_{c_1}} \frac{1 - \text{sgn}(\delta_m^{c_1})}{2} + \sum_{m=1}^{n_{c_2}} \frac{1 - \text{sgn}(\delta_m^{c_2})}{2} \mod 2 \quad (\text{L12.2})$$

$$\begin{aligned} \mathcal{X}_2 = & - \sum_{m=1}^{n_{b_1}} \text{sgn}(v_m^{b_1}) \frac{1 - \text{sgn}(\delta_m^{b_1})}{2} + \sum_{m=1}^{n_{b_2}} \text{sgn}(v_m^{b_2}) \frac{1 - \text{sgn}(\delta_m^{b_2})}{2} - \sum_{m=1}^{n_{c_1}} \text{sgn}(v_m^{c_1}) \frac{1 - \text{sgn}(\delta_m^{c_1})}{2} + \sum_{m=1}^{n_{c_2}} \text{sgn}(v_m^{c_2}) \frac{1 - \text{sgn}(\delta_m^{c_2})}{2} \\ & - 2 \sum_{m=1}^{n_{d_1}} \text{sgn}(v_m^{d_1}) \frac{1 - \text{sgn}(\delta_m^{d_1})}{2} \mod 4 \end{aligned} \quad (\text{L12.3})$$

### L13. LAYER GROUP NO. 13

| line segment                            | character of irrep (generators only)                                        |
|-----------------------------------------|-----------------------------------------------------------------------------|
| $a \ (t, 0, 0)$                         | $\begin{matrix} \{1  0 & 0 & 0\} \\ a_1 & 1 \end{matrix}$                   |
| $b \ (0, t, 0)$                         | $\begin{matrix} \{m_{100}  0 & 0 & 0\} \\ b_1 & -i \\ b_2 & i \end{matrix}$ |
| $c \ (\frac{t}{2}, 1 - \frac{t}{2}, 0)$ | $\begin{matrix} \{1  0 & 0 & 0\} \\ c_1 & 1 \end{matrix}$                   |

$$\mathcal{W}_1^{\text{gapless}} = \sum_{m=1}^{n_{a_1}} \text{sgn}(v_m^{a_1}) \frac{1 - \text{sgn}(\delta_m^{a_1})}{2} - \sum_{m=1}^{n_{b_1}} \text{sgn}(v_m^{b_1}) \frac{1 - \text{sgn}(\delta_m^{b_1})}{2} - \sum_{m=1}^{n_{b_2}} \text{sgn}(v_m^{b_2}) \frac{1 - \text{sgn}(\delta_m^{b_2})}{2} \quad (\text{L13.1})$$

$$\mathcal{W}_1^{\text{gapped}} = - \sum_{m=1}^{n_{b_1}} \text{sgn}(v_m^{b_1}) \frac{1 - \text{sgn}(\delta_m^{b_1})}{2} + \sum_{m=1}^{n_{b_2}} \text{sgn}(v_m^{b_2}) \frac{1 - \text{sgn}(\delta_m^{b_2})}{2} \quad (\text{L13.2})$$

$$\mathcal{X}_1 = \sum_{m=1}^{n_{c_1}} \frac{1 - \text{sgn}(\delta_m^{c_1})}{2} \mod 2 \quad (\text{L13.3})$$

**L14. LAYER GROUP NO. 14**

| line segment                            | character of irrep (generators only)                                                                |
|-----------------------------------------|-----------------------------------------------------------------------------------------------------|
| $a \quad (\frac{t}{2}, 0, 0)$           | $\{2_{100}   \begin{smallmatrix} 0 & 0 & 0 \end{smallmatrix} \}$<br>$a_1 \quad -i$<br>$a_2 \quad i$ |
| $b \quad (0, \frac{t}{2}, 0)$           | $\{m_{100}   \begin{smallmatrix} 0 & 0 & 0 \end{smallmatrix} \}$<br>$b_1 \quad -i$<br>$b_2 \quad i$ |
| $c \quad (\frac{1}{2}, \frac{t}{2}, 0)$ | $\{m_{100}   \begin{smallmatrix} 0 & 0 & 0 \end{smallmatrix} \}$<br>$c_1 \quad -i$<br>$c_2 \quad i$ |
| $d \quad (\frac{t}{2}, \frac{1}{2}, 0)$ | $\{2_{100}   \begin{smallmatrix} 0 & 0 & 0 \end{smallmatrix} \}$<br>$d_1 \quad -i$<br>$d_2 \quad i$ |

$$\mathcal{W}_1^{\text{gapless}} = \sum_{m=1}^{n_{a_1}} \text{sgn}(v_m^{a_1}) \frac{1 - \text{sgn}(\delta_m^{a_1})}{2} - \sum_{m=1}^{n_{b_1}} \text{sgn}(v_m^{b_1}) \frac{1 - \text{sgn}(\delta_m^{b_1})}{2} + \sum_{m=1}^{n_{c_1}} \text{sgn}(v_m^{c_1}) \frac{1 - \text{sgn}(\delta_m^{c_1})}{2} - \sum_{m=1}^{n_{d_1}} \text{sgn}(v_m^{d_1}) \frac{1 - \text{sgn}(\delta_m^{d_1})}{2} \quad (\text{L14.1})$$

**L15. LAYER GROUP NO. 15**

| line segment                            | character of irrep (generators only)                                                                                                                      |
|-----------------------------------------|-----------------------------------------------------------------------------------------------------------------------------------------------------------|
| $a \quad (\frac{t}{2}, 0, 0)$           | $\{2_{100}   \begin{smallmatrix} \frac{1}{2} & 0 & 0 \end{smallmatrix} \}$<br>$a_1 \quad -ie^{-\frac{1}{2}i\pi t}$<br>$a_2 \quad ie^{-\frac{1}{2}i\pi t}$ |
| $b \quad (0, \frac{t}{2}, 0)$           | $\{m_{100}   \begin{smallmatrix} \frac{1}{2} & 0 & 0 \end{smallmatrix} \}$<br>$b_1 \quad -i$<br>$b_2 \quad i$                                             |
| $c \quad (\frac{1}{2}, \frac{t}{2}, 0)$ | $\{m_{100}   \begin{smallmatrix} \frac{1}{2} & 0 & 0 \end{smallmatrix} \}$<br>$c_1 \quad i$<br>$c_2 \quad -i$                                             |
| $d \quad (\frac{t}{2}, \frac{1}{2}, 0)$ | $\{2_{100}   \begin{smallmatrix} \frac{1}{2} & 0 & 0 \end{smallmatrix} \}$<br>$d_1 \quad -ie^{-\frac{1}{2}i\pi t}$<br>$d_2 \quad ie^{-\frac{1}{2}i\pi t}$ |

$$\begin{aligned} \mathcal{W}_1^{\text{gapless}} = & \sum_{m=1}^{n_{a_1}} \text{sgn}(v_m^{a_1}) \frac{1 - \text{sgn}(\delta_m^{a_1})}{2} - \sum_{m=1}^{n_{b_1}} \text{sgn}(v_m^{b_1}) \frac{1 - \text{sgn}(\delta_m^{b_1})}{2} + \sum_{m=1}^{n_{c_1}} \text{sgn}(v_m^{c_1}) \frac{1 - \text{sgn}(\delta_m^{c_1})}{2} \\ & + \sum_{m=1}^{n_{c_2}} \text{sgn}(v_m^{c_2}) \frac{1 - \text{sgn}(\delta_m^{c_2})}{2} - \sum_{m=1}^{n_{d_1}} \text{sgn}(v_m^{d_1}) \frac{1 - \text{sgn}(\delta_m^{d_1})}{2} \end{aligned} \quad (\text{L15.1})$$

$$\mathcal{W}_1^{\text{gapped}} = - \sum_{m=1}^{n_{c_1}} \text{sgn}(v_m^{c_1}) \frac{1 - \text{sgn}(\delta_m^{c_1})}{2} + \sum_{m=1}^{n_{c_2}} \text{sgn}(v_m^{c_2}) \frac{1 - \text{sgn}(\delta_m^{c_2})}{2} \quad (\text{L15.2})$$

**L16. LAYER GROUP NO. 16**

| line segment                            | character of irrep (generators only)                                                                                        |
|-----------------------------------------|-----------------------------------------------------------------------------------------------------------------------------|
| $a \quad (\frac{t}{2}, 0, 0)$           | $\{2_{100}   0 \quad \frac{1}{2} \quad 0 \}$<br>$a_1 \quad -i$<br>$a_2 \quad i$                                             |
| $b \quad (0, \frac{t}{2}, 0)$           | $\{m_{100}   0 \quad \frac{1}{2} \quad 0 \}$<br>$b_1 \quad -ie^{-\frac{1}{2}i\pi t}$<br>$b_2 \quad ie^{-\frac{1}{2}i\pi t}$ |
| $c \quad (\frac{1}{2}, \frac{t}{2}, 0)$ | $\{m_{100}   0 \quad \frac{1}{2} \quad 0 \}$<br>$c_1 \quad -ie^{-\frac{1}{2}i\pi t}$<br>$c_2 \quad ie^{-\frac{1}{2}i\pi t}$ |
| $d \quad (\frac{t}{2}, \frac{1}{2}, 0)$ | $\{2_{100}   0 \quad \frac{1}{2} \quad 0 \}$<br>$d_1 \quad i$<br>$d_2 \quad -i$                                             |

$$\begin{aligned} \mathcal{W}_1^{\text{gapless}} = & \sum_{m=1}^{n_{a_1}} \text{sgn}(v_m^{a_1}) \frac{1 - \text{sgn}(\delta_m^{a_1})}{2} - \sum_{m=1}^{n_{b_1}} \text{sgn}(v_m^{b_1}) \frac{1 - \text{sgn}(\delta_m^{b_1})}{2} + \sum_{m=1}^{n_{c_1}} \text{sgn}(v_m^{c_1}) \frac{1 - \text{sgn}(\delta_m^{c_1})}{2} \\ & - \sum_{m=1}^{n_{d_1}} \text{sgn}(v_m^{d_1}) \frac{1 - \text{sgn}(\delta_m^{d_1})}{2} - \sum_{m=1}^{n_{d_2}} \text{sgn}(v_m^{d_2}) \frac{1 - \text{sgn}(\delta_m^{d_2})}{2} \end{aligned} \quad (\text{L16.1})$$

$$\mathcal{W}_1^{\text{gapped}} = - \sum_{m=1}^{n_{d_1}} \text{sgn}(v_m^{d_1}) \frac{1 - \text{sgn}(\delta_m^{d_1})}{2} + \sum_{m=1}^{n_{d_2}} \text{sgn}(v_m^{d_2}) \frac{1 - \text{sgn}(\delta_m^{d_2})}{2} \quad (\text{L16.2})$$

**L17. LAYER GROUP NO. 17**

| line segment                            | character of irrep (generators only)                                                                                                      |
|-----------------------------------------|-------------------------------------------------------------------------------------------------------------------------------------------|
| $a \quad (\frac{t}{2}, 0, 0)$           | $\{2_{100}   \frac{1}{2} \quad \frac{1}{2} \quad 0 \}$<br>$a_1 \quad -ie^{-\frac{1}{2}i\pi t}$<br>$a_2 \quad ie^{-\frac{1}{2}i\pi t}$     |
| $b \quad (0, \frac{t}{2}, 0)$           | $\{m_{100}   \frac{1}{2} \quad \frac{1}{2} \quad 0 \}$<br>$b_1 \quad -ie^{-\frac{1}{2}i\pi t}$<br>$b_2 \quad ie^{-\frac{1}{2}i\pi t}$     |
| $c \quad (\frac{1}{2}, \frac{t}{2}, 0)$ | $\{m_{100}   \frac{1}{2} \quad \frac{1}{2} \quad 0 \}$<br>$c_1 \quad -e^{-\frac{1}{2}i\pi(t+1)}$<br>$c_2 \quad e^{-\frac{1}{2}i\pi(t+1)}$ |
| $d \quad (\frac{t}{2}, \frac{1}{2}, 0)$ | $\{2_{100}   \frac{1}{2} \quad \frac{1}{2} \quad 0 \}$<br>$d_1 \quad -e^{-\frac{1}{2}i\pi(t+1)}$<br>$d_2 \quad e^{-\frac{1}{2}i\pi(t+1)}$ |

$$\begin{aligned} \mathcal{W}_1^{\text{gapless}} = & \sum_{m=1}^{n_{a_1}} \text{sgn}(v_m^{a_1}) \frac{1 - \text{sgn}(\delta_m^{a_1})}{2} - \sum_{m=1}^{n_{b_1}} \text{sgn}(v_m^{b_1}) \frac{1 - \text{sgn}(\delta_m^{b_1})}{2} + \sum_{m=1}^{n_{c_1}} \text{sgn}(v_m^{c_1}) \frac{1 - \text{sgn}(\delta_m^{c_1})}{2} \\ & + \sum_{m=1}^{n_{c_2}} \text{sgn}(v_m^{c_2}) \frac{1 - \text{sgn}(\delta_m^{c_2})}{2} - \sum_{m=1}^{n_{d_1}} \text{sgn}(v_m^{d_1}) \frac{1 - \text{sgn}(\delta_m^{d_1})}{2} - \sum_{m=1}^{n_{d_2}} \text{sgn}(v_m^{d_2}) \frac{1 - \text{sgn}(\delta_m^{d_2})}{2} \end{aligned} \quad (\text{L17.1})$$

$$\mathcal{X}_1 = \sum_{m=1}^{n_{c_1}} \frac{1 - \text{sgn}(\delta_m^{c_1})}{2} + \sum_{m=1}^{n_{c_2}} \frac{1 - \text{sgn}(\delta_m^{c_2})}{2} + \sum_{m=1}^{n_{d_1}} \frac{1 - \text{sgn}(\delta_m^{d_1})}{2} + \sum_{m=1}^{n_{d_2}} \frac{1 - \text{sgn}(\delta_m^{d_2})}{2} \pmod{2} \quad (\text{L17.2})$$

**L18. LAYER GROUP NO. 18**

| line segment                            | character of irrep (generators only)                         |
|-----------------------------------------|--------------------------------------------------------------|
| $a \ (t, 0, 0)$                         | $\{2_{100}   0 \ 0 \ 0\}$<br>$a_1 \quad -i$<br>$a_2 \quad i$ |
| $b \ (0, t, 0)$                         | $\{m_{100}   0 \ 0 \ 0\}$<br>$b_1 \quad -i$<br>$b_2 \quad i$ |
| $c \ (\frac{t}{2}, 1 - \frac{t}{2}, 0)$ | $\{1   0 \ 0 \ 0\}$<br>$c_1 \quad 1$                         |

$$\mathcal{W}_1^{\text{gapless}} = \sum_{m=1}^{n_{a_1}} \text{sgn}(v_m^{a_1}) \frac{1 - \text{sgn}(\delta_m^{a_1})}{2} - \sum_{m=1}^{n_{b_1}} \text{sgn}(v_m^{b_1}) \frac{1 - \text{sgn}(\delta_m^{b_1})}{2} \quad (\text{L18.1})$$

**L19. LAYER GROUP NO. 19**

| line segment                        | character of irrep (generators only)                         |
|-------------------------------------|--------------------------------------------------------------|
| $a \ (\frac{t}{2}, 0, 0)$           | $\{2_{100}   0 \ 0 \ 0\}$<br>$a_1 \quad -i$<br>$a_2 \quad i$ |
| $b \ (0, \frac{t}{2}, 0)$           | $\{2_{010}   0 \ 0 \ 0\}$<br>$b_1 \quad -i$<br>$b_2 \quad i$ |
| $c \ (\frac{1}{2}, \frac{t}{2}, 0)$ | $\{2_{010}   0 \ 0 \ 0\}$<br>$c_1 \quad -i$<br>$c_2 \quad i$ |
| $d \ (\frac{t}{2}, \frac{1}{2}, 0)$ | $\{2_{100}   0 \ 0 \ 0\}$<br>$d_1 \quad -i$<br>$d_2 \quad i$ |

$$\begin{aligned} \mathcal{W}_1^{\text{gapless}} = & \sum_{m=1}^{n_{a_1}} \text{sgn}(v_m^{a_1}) \frac{1 - \text{sgn}(\delta_m^{a_1})}{2} + \sum_{m=1}^{n_{a_2}} \text{sgn}(v_m^{a_2}) \frac{1 - \text{sgn}(\delta_m^{a_2})}{2} - \sum_{m=1}^{n_{b_1}} \text{sgn}(v_m^{b_1}) \frac{1 - \text{sgn}(\delta_m^{b_1})}{2} \\ & - \sum_{m=1}^{n_{b_2}} \text{sgn}(v_m^{b_2}) \frac{1 - \text{sgn}(\delta_m^{b_2})}{2} + \sum_{m=1}^{n_{c_1}} \text{sgn}(v_m^{c_1}) \frac{1 - \text{sgn}(\delta_m^{c_1})}{2} + \sum_{m=1}^{n_{c_2}} \text{sgn}(v_m^{c_2}) \frac{1 - \text{sgn}(\delta_m^{c_2})}{2} \\ & - \sum_{m=1}^{n_{d_1}} \text{sgn}(v_m^{d_1}) \frac{1 - \text{sgn}(\delta_m^{d_1})}{2} - \sum_{m=1}^{n_{d_2}} \text{sgn}(v_m^{d_2}) \frac{1 - \text{sgn}(\delta_m^{d_2})}{2} \end{aligned} \quad (\text{L19.1})$$

$$\mathcal{W}_1^{\text{gapped}} = - \sum_{m=1}^{n_{b_1}} \text{sgn}(v_m^{b_1}) \frac{1 - \text{sgn}(\delta_m^{b_1})}{2} + \sum_{m=1}^{n_{b_2}} \text{sgn}(v_m^{b_2}) \frac{1 - \text{sgn}(\delta_m^{b_2})}{2} \quad (\text{L19.2})$$

$$\mathcal{W}_2^{\text{gapped}} = - \sum_{m=1}^{n_{c_1}} \text{sgn}(v_m^{c_1}) \frac{1 - \text{sgn}(\delta_m^{c_1})}{2} + \sum_{m=1}^{n_{c_2}} \text{sgn}(v_m^{c_2}) \frac{1 - \text{sgn}(\delta_m^{c_2})}{2} \quad (\text{L19.3})$$

$$\begin{aligned} \mathcal{W}_3^{\text{gapped}} = & - \sum_{m=1}^{n_{a_2}} \text{sgn}(v_m^{a_2}) \frac{1 - \text{sgn}(\delta_m^{a_2})}{2} + \sum_{m=1}^{n_{b_1}} \text{sgn}(v_m^{b_1}) \frac{1 - \text{sgn}(\delta_m^{b_1})}{2} - \sum_{m=1}^{n_{c_1}} \text{sgn}(v_m^{c_1}) \frac{1 - \text{sgn}(\delta_m^{c_1})}{2} \\ & + \sum_{m=1}^{n_{d_1}} \text{sgn}(v_m^{d_1}) \frac{1 - \text{sgn}(\delta_m^{d_1})}{2} \end{aligned} \quad (\text{L19.4})$$

$$\begin{aligned} \mathcal{W}_4^{\text{gapped}} = & - \sum_{m=1}^{n_{a_2}} \text{sgn}(v_m^{a_2}) \frac{1 - \text{sgn}(\delta_m^{a_2})}{2} + \sum_{m=1}^{n_{b_1}} \text{sgn}(v_m^{b_1}) \frac{1 - \text{sgn}(\delta_m^{b_1})}{2} - \sum_{m=1}^{n_{c_1}} \text{sgn}(v_m^{c_1}) \frac{1 - \text{sgn}(\delta_m^{c_1})}{2} \\ & + \sum_{m=1}^{n_{d_2}} \text{sgn}(v_m^{d_2}) \frac{1 - \text{sgn}(\delta_m^{d_2})}{2} \end{aligned} \quad (\text{L19.5})$$

## L20. LAYER GROUP NO. 20

| line segment                            | character of irrep (generators only)                                                                                |
|-----------------------------------------|---------------------------------------------------------------------------------------------------------------------|
| $a \quad (\frac{t}{2}, 0, 0)$           | $\{2_{100}   \frac{1}{2} \ 0 \ 0 \}$<br>$a_1 \quad -ie^{-\frac{1}{2}i\pi t}$<br>$a_2 \quad ie^{-\frac{1}{2}i\pi t}$ |
| $b \quad (0, \frac{t}{2}, 0)$           | $\{2_{010}   \frac{1}{2} \ 0 \ 0 \}$<br>$b_1 \quad -i$<br>$b_2 \quad i$                                             |
| $c \quad (\frac{1}{2}, \frac{t}{2}, 0)$ | $\{2_{010}   \frac{1}{2} \ 0 \ 0 \}$<br>$c_1 \quad i$<br>$c_2 \quad -i$                                             |
| $d \quad (\frac{t}{2}, \frac{1}{2}, 0)$ | $\{2_{100}   \frac{1}{2} \ 0 \ 0 \}$<br>$d_1 \quad -ie^{-\frac{1}{2}i\pi t}$<br>$d_2 \quad ie^{-\frac{1}{2}i\pi t}$ |

$$\begin{aligned} \mathcal{W}_1^{\text{gapped}} = & \sum_{m=1}^{n_{a_1}} \text{sgn}(v_m^{a_1}) \frac{1 - \text{sgn}(\delta_m^{a_1})}{2} + \sum_{m=1}^{n_{a_2}} \text{sgn}(v_m^{a_2}) \frac{1 - \text{sgn}(\delta_m^{a_2})}{2} - \sum_{m=1}^{n_{b_1}} \text{sgn}(v_m^{b_1}) \frac{1 - \text{sgn}(\delta_m^{b_1})}{2} - \sum_{m=1}^{n_{b_2}} \text{sgn}(v_m^{b_2}) \frac{1 - \text{sgn}(\delta_m^{b_2})}{2} \\ & + 2 \sum_{m=1}^{n_{c_1}} \text{sgn}(v_m^{c_1}) \frac{1 - \text{sgn}(\delta_m^{c_1})}{2} - \sum_{m=1}^{n_{d_1}} \text{sgn}(v_m^{d_1}) \frac{1 - \text{sgn}(\delta_m^{d_1})}{2} - \sum_{m=1}^{n_{d_2}} \text{sgn}(v_m^{d_2}) \frac{1 - \text{sgn}(\delta_m^{d_2})}{2} \end{aligned} \quad (\text{L20.1})$$

$$\mathcal{W}_1^{\text{gapped}} = \sum_{m=1}^{n_{b_1}} \text{sgn}(v_m^{b_1}) \frac{1 - \text{sgn}(\delta_m^{b_1})}{2} - \sum_{m=1}^{n_{b_2}} \text{sgn}(v_m^{b_2}) \frac{1 - \text{sgn}(\delta_m^{b_2})}{2} \quad (\text{L20.2})$$

$$\mathcal{X}_1 = \sum_{m=1}^{n_{a_2}} \frac{1 - \text{sgn}(\delta_m^{a_2})}{2} + \sum_{m=1}^{n_{b_2}} \frac{1 - \text{sgn}(\delta_m^{b_2})}{2} + \sum_{m=1}^{n_{d_2}} \frac{1 - \text{sgn}(\delta_m^{d_2})}{2} \quad \text{mod } 2 \quad (\text{L20.3})$$

$$\mathcal{X}_2 = \sum_{m=1}^{n_{a_2}} \frac{1 - \text{sgn}(\delta_m^{a_2})}{2} + \sum_{m=1}^{n_{b_2}} \frac{1 - \text{sgn}(\delta_m^{b_2})}{2} + \sum_{m=1}^{n_{d_1}} \frac{1 - \text{sgn}(\delta_m^{d_1})}{2} \mod 2 \quad (\text{L20.4})$$

### L21. LAYER GROUP NO. 21

| line segment                            | character of irrep (generators only)                                                                                         |
|-----------------------------------------|------------------------------------------------------------------------------------------------------------------------------|
| $a \quad (\frac{t}{2}, 0, 0)$           | $\{2_{100}   \frac{1}{2} \frac{1}{2} 0\}$<br>$a_1 \quad -ie^{-\frac{1}{2}i\pi t}$<br>$a_2 \quad ie^{-\frac{1}{2}i\pi t}$     |
| $b \quad (0, \frac{t}{2}, 0)$           | $\{2_{010}   \frac{1}{2} \frac{1}{2} 0\}$<br>$b_1 \quad -ie^{-\frac{1}{2}i\pi t}$<br>$b_2 \quad ie^{-\frac{1}{2}i\pi t}$     |
| $c \quad (\frac{1}{2}, \frac{t}{2}, 0)$ | $\{2_{010}   \frac{1}{2} \frac{1}{2} 0\}$<br>$c_1 \quad -e^{-\frac{1}{2}i\pi(t+1)}$<br>$c_2 \quad e^{-\frac{1}{2}i\pi(t+1)}$ |
| $d \quad (\frac{t}{2}, \frac{1}{2}, 0)$ | $\{2_{100}   \frac{1}{2} \frac{1}{2} 0\}$<br>$d_1 \quad -e^{-\frac{1}{2}i\pi(t+1)}$<br>$d_2 \quad e^{-\frac{1}{2}i\pi(t+1)}$ |

$$\begin{aligned} \mathcal{W}_1^{\text{gapless}} = & \sum_{m=1}^{n_{a_1}} \text{sgn}(v_m^{a_1}) \frac{1 - \text{sgn}(\delta_m^{a_1})}{2} + \sum_{m=1}^{n_{a_2}} \text{sgn}(v_m^{a_2}) \frac{1 - \text{sgn}(\delta_m^{a_2})}{2} - \sum_{m=1}^{n_{b_1}} \text{sgn}(v_m^{b_1}) \frac{1 - \text{sgn}(\delta_m^{b_1})}{2} \\ & - \sum_{m=1}^{n_{b_2}} \text{sgn}(v_m^{b_2}) \frac{1 - \text{sgn}(\delta_m^{b_2})}{2} + 2 \sum_{m=1}^{n_{c_1}} \text{sgn}(v_m^{c_1}) \frac{1 - \text{sgn}(\delta_m^{c_1})}{2} - 2 \sum_{m=1}^{n_{d_1}} \text{sgn}(v_m^{d_1}) \frac{1 - \text{sgn}(\delta_m^{d_1})}{2} \end{aligned} \quad (\text{L21.1})$$

$$\mathcal{X}_1 = \sum_{m=1}^{n_{a_2}} \frac{1 - \text{sgn}(\delta_m^{a_2})}{2} + \sum_{m=1}^{n_{b_1}} \frac{1 - \text{sgn}(\delta_m^{b_1})}{2} \mod 2 \quad (\text{L21.2})$$

$$\begin{aligned} \mathcal{X}_2 = & 2 \sum_{m=1}^{n_{a_2}} \text{sgn}(v_m^{a_2}) \frac{1 - \text{sgn}(\delta_m^{a_2})}{2} - \sum_{m=1}^{n_{b_1}} \text{sgn}(v_m^{b_1}) \frac{1 - \text{sgn}(\delta_m^{b_1})}{2} - \sum_{m=1}^{n_{b_2}} \text{sgn}(v_m^{b_2}) \frac{1 - \text{sgn}(\delta_m^{b_2})}{2} \\ & - 2 \sum_{m=1}^{n_{d_1}} \text{sgn}(v_m^{d_1}) \frac{1 - \text{sgn}(\delta_m^{d_1})}{2} \mod 4 \end{aligned} \quad (\text{L21.3})$$

### L22. LAYER GROUP NO. 22

| line segment        | character of irrep (generators only)                         |
|---------------------|--------------------------------------------------------------|
| $a \quad (t, 0, 0)$ | $\{2_{100}   0 \ 0 \ 0\}$<br>$a_1 \quad -i$<br>$a_2 \quad i$ |
| $b \quad (0, t, 0)$ | $\{2_{010}   0 \ 0 \ 0\}$<br>$b_1 \quad -i$<br>$b_2 \quad i$ |



|                                             |                                                                    |
|---------------------------------------------|--------------------------------------------------------------------|
| $c \quad (\frac{t}{2}, 1 - \frac{t}{2}, 0)$ | $c_1 \quad \begin{array}{c} \{1 \mid 0 \ 0 \ 0\} \\ 1 \end{array}$ |
|---------------------------------------------|--------------------------------------------------------------------|

$$\mathcal{W}_1^{\text{gapless}} = \sum_{m=1}^{n_{a_1}} \text{sgn}(v_m^{a_1}) \frac{1 - \text{sgn}(\delta_m^{a_1})}{2} + \sum_{m=1}^{n_{a_2}} \text{sgn}(v_m^{a_2}) \frac{1 - \text{sgn}(\delta_m^{a_2})}{2} - \sum_{m=1}^{n_{b_1}} \text{sgn}(v_m^{b_1}) \frac{1 - \text{sgn}(\delta_m^{b_1})}{2} - \sum_{m=1}^{n_{b_2}} \text{sgn}(v_m^{b_2}) \frac{1 - \text{sgn}(\delta_m^{b_2})}{2} \quad (\text{L22.1})$$

$$\mathcal{W}_1^{\text{gapped}} = - \sum_{m=1}^{n_{a_2}} \text{sgn}(v_m^{a_2}) \frac{1 - \text{sgn}(\delta_m^{a_2})}{2} + \sum_{m=1}^{n_{b_2}} \text{sgn}(v_m^{b_2}) \frac{1 - \text{sgn}(\delta_m^{b_2})}{2} \quad (\text{L22.2})$$

$$\mathcal{W}_2^{\text{gapped}} = - \sum_{m=1}^{n_{a_2}} \text{sgn}(v_m^{a_2}) \frac{1 - \text{sgn}(\delta_m^{a_2})}{2} + \sum_{m=1}^{n_{b_1}} \text{sgn}(v_m^{b_1}) \frac{1 - \text{sgn}(\delta_m^{b_1})}{2} \quad (\text{L22.3})$$

$$\mathcal{X}_1 = \sum_{m=1}^{n_{c_1}} \frac{1 - \text{sgn}(\delta_m^{c_1})}{2} \quad \text{mod } 2 \quad (\text{L22.4})$$

### L23. LAYER GROUP NO. 23

| line segment                            | character of irrep (generators only)                                                     |
|-----------------------------------------|------------------------------------------------------------------------------------------|
| $a \quad (\frac{t}{2}, 0, 0)$           | $\begin{array}{c} \{m_{010} \mid 0 \ 0 \ 0\} \\ a_1 \quad -i \\ a_2 \quad i \end{array}$ |
| $b \quad (0, \frac{t}{2}, 0)$           | $\begin{array}{c} \{m_{100} \mid 0 \ 0 \ 0\} \\ b_1 \quad -i \\ b_2 \quad i \end{array}$ |
| $c \quad (\frac{1}{2}, \frac{t}{2}, 0)$ | $\begin{array}{c} \{m_{100} \mid 0 \ 0 \ 0\} \\ c_1 \quad -i \\ c_2 \quad i \end{array}$ |
| $d \quad (\frac{t}{2}, \frac{1}{2}, 0)$ | $\begin{array}{c} \{m_{010} \mid 0 \ 0 \ 0\} \\ d_1 \quad -i \\ d_2 \quad i \end{array}$ |

$$\begin{aligned} \mathcal{W}_1^{\text{gapless}} = & \sum_{m=1}^{n_{a_1}} \text{sgn}(v_m^{a_1}) \frac{1 - \text{sgn}(\delta_m^{a_1})}{2} + \sum_{m=1}^{n_{a_2}} \text{sgn}(v_m^{a_2}) \frac{1 - \text{sgn}(\delta_m^{a_2})}{2} - \sum_{m=1}^{n_{b_1}} \text{sgn}(v_m^{b_1}) \frac{1 - \text{sgn}(\delta_m^{b_1})}{2} \\ & - \sum_{m=1}^{n_{b_2}} \text{sgn}(v_m^{b_2}) \frac{1 - \text{sgn}(\delta_m^{b_2})}{2} + \sum_{m=1}^{n_{c_1}} \text{sgn}(v_m^{c_1}) \frac{1 - \text{sgn}(\delta_m^{c_1})}{2} + \sum_{m=1}^{n_{c_2}} \text{sgn}(v_m^{c_2}) \frac{1 - \text{sgn}(\delta_m^{c_2})}{2} \\ & - \sum_{m=1}^{n_{d_1}} \text{sgn}(v_m^{d_1}) \frac{1 - \text{sgn}(\delta_m^{d_1})}{2} - \sum_{m=1}^{n_{d_2}} \text{sgn}(v_m^{d_2}) \frac{1 - \text{sgn}(\delta_m^{d_2})}{2} \end{aligned} \quad (\text{L23.1})$$

$$\mathcal{W}_1^{\text{gapped}} = - \sum_{m=1}^{n_{b_1}} \text{sgn}(v_m^{b_1}) \frac{1 - \text{sgn}(\delta_m^{b_1})}{2} + \sum_{m=1}^{n_{b_2}} \text{sgn}(v_m^{b_2}) \frac{1 - \text{sgn}(\delta_m^{b_2})}{2} \quad (\text{L23.2})$$

$$\mathcal{W}_2^{\text{gapped}} = - \sum_{m=1}^{n_{c_1}} \text{sgn}(v_m^{c_1}) \frac{1 - \text{sgn}(\delta_m^{c_1})}{2} + \sum_{m=1}^{n_{c_2}} \text{sgn}(v_m^{c_2}) \frac{1 - \text{sgn}(\delta_m^{c_2})}{2} \quad (\text{L23.3})$$

$$\begin{aligned} \mathcal{W}_3^{\text{gapped}} = & - \sum_{m=1}^{n_{a_2}} \text{sgn}(v_m^{a_2}) \frac{1 - \text{sgn}(\delta_m^{a_2})}{2} + \sum_{m=1}^{n_{b_1}} \text{sgn}(v_m^{b_1}) \frac{1 - \text{sgn}(\delta_m^{b_1})}{2} - \sum_{m=1}^{n_{c_1}} \text{sgn}(v_m^{c_1}) \frac{1 - \text{sgn}(\delta_m^{c_1})}{2} \\ & + \sum_{m=1}^{n_{d_1}} \text{sgn}(v_m^{d_1}) \frac{1 - \text{sgn}(\delta_m^{d_1})}{2} \end{aligned} \quad (\text{L23.4})$$

$$\begin{aligned} \mathcal{W}_4^{\text{gapped}} = & - \sum_{m=1}^{n_{a_2}} \text{sgn}(v_m^{a_2}) \frac{1 - \text{sgn}(\delta_m^{a_2})}{2} + \sum_{m=1}^{n_{b_1}} \text{sgn}(v_m^{b_1}) \frac{1 - \text{sgn}(\delta_m^{b_1})}{2} - \sum_{m=1}^{n_{c_1}} \text{sgn}(v_m^{c_1}) \frac{1 - \text{sgn}(\delta_m^{c_1})}{2} \\ & + \sum_{m=1}^{n_{d_2}} \text{sgn}(v_m^{d_2}) \frac{1 - \text{sgn}(\delta_m^{d_2})}{2} \end{aligned} \quad (\text{L23.5})$$

#### L24. LAYER GROUP NO. 24

| line segment                            | character of irrep (generators only)                                        |
|-----------------------------------------|-----------------------------------------------------------------------------|
| $a \quad (\frac{t}{2}, 0, 0)$           | $\{m_{010}   \frac{1}{2} \ 0 \ 0 \}$                                        |
|                                         | $a_1 \quad -ie^{-\frac{1}{2}i\pi t}$                                        |
|                                         | $a_2 \quad ie^{-\frac{1}{2}i\pi t}$                                         |
| $b \quad (0, \frac{t}{2}, 0)$           | $\{m_{100}   \frac{1}{2} \ 0 \ 0 \}$                                        |
|                                         | $b_1 \quad -i$<br>$b_2 \quad i$                                             |
| $c \quad (\frac{1}{2}, \frac{t}{2}, 0)$ | $\{m_{100}   \frac{1}{2} \ 0 \ 0 \}$                                        |
|                                         | $c_1 \quad i$<br>$c_2 \quad -i$                                             |
| $d \quad (\frac{t}{2}, \frac{1}{2}, 0)$ | $\{m_{010}   \frac{1}{2} \ 0 \ 0 \}$                                        |
|                                         | $d_1 \quad -ie^{-\frac{1}{2}i\pi t}$<br>$d_2 \quad ie^{-\frac{1}{2}i\pi t}$ |

$$\begin{aligned} \mathcal{W}_1^{\text{gapless}} = & \sum_{m=1}^{n_{a_1}} \text{sgn}(v_m^{a_1}) \frac{1 - \text{sgn}(\delta_m^{a_1})}{2} + \sum_{m=1}^{n_{a_2}} \text{sgn}(v_m^{a_2}) \frac{1 - \text{sgn}(\delta_m^{a_2})}{2} - \sum_{m=1}^{n_{b_1}} \text{sgn}(v_m^{b_1}) \frac{1 - \text{sgn}(\delta_m^{b_1})}{2} - \sum_{m=1}^{n_{b_2}} \text{sgn}(v_m^{b_2}) \frac{1 - \text{sgn}(\delta_m^{b_2})}{2} \\ & + 2 \sum_{m=1}^{n_{c_1}} \text{sgn}(v_m^{c_1}) \frac{1 - \text{sgn}(\delta_m^{c_1})}{2} - \sum_{m=1}^{n_{d_1}} \text{sgn}(v_m^{d_1}) \frac{1 - \text{sgn}(\delta_m^{d_1})}{2} - \sum_{m=1}^{n_{d_2}} \text{sgn}(v_m^{d_2}) \frac{1 - \text{sgn}(\delta_m^{d_2})}{2} \end{aligned} \quad (\text{L24.1})$$

$$\mathcal{W}_1^{\text{gapped}} = \sum_{m=1}^{n_{b_1}} \text{sgn}(v_m^{b_1}) \frac{1 - \text{sgn}(\delta_m^{b_1})}{2} - \sum_{m=1}^{n_{b_2}} \text{sgn}(v_m^{b_2}) \frac{1 - \text{sgn}(\delta_m^{b_2})}{2} \quad (\text{L24.2})$$

$$\mathcal{X}_1 = \sum_{m=1}^{n_{a_2}} \frac{1 - \text{sgn}(\delta_m^{a_2})}{2} + \sum_{m=1}^{n_{b_2}} \frac{1 - \text{sgn}(\delta_m^{b_2})}{2} + \sum_{m=1}^{n_{d_2}} \frac{1 - \text{sgn}(\delta_m^{d_2})}{2} \quad \text{mod } 2 \quad (\text{L24.3})$$

$$\mathcal{X}_2 = \sum_{m=1}^{n_{a_2}} \frac{1 - \text{sgn}(\delta_m^{a_2})}{2} + \sum_{m=1}^{n_{b_2}} \frac{1 - \text{sgn}(\delta_m^{b_2})}{2} + \sum_{m=1}^{n_{d_1}} \frac{1 - \text{sgn}(\delta_m^{d_1})}{2} \mod 2 \quad (\text{L24.4})$$

### L25. LAYER GROUP NO. 25

| line segment                            | character of irrep (generators only)                                                                                         |
|-----------------------------------------|------------------------------------------------------------------------------------------------------------------------------|
| $a \quad (\frac{t}{2}, 0, 0)$           | $\{m_{010}   \frac{1}{2} \frac{1}{2} 0\}$<br>$a_1 \quad -ie^{-\frac{1}{2}i\pi t}$<br>$a_2 \quad ie^{-\frac{1}{2}i\pi t}$     |
| $b \quad (0, \frac{t}{2}, 0)$           | $\{m_{100}   \frac{1}{2} \frac{1}{2} 0\}$<br>$b_1 \quad -ie^{-\frac{1}{2}i\pi t}$<br>$b_2 \quad ie^{-\frac{1}{2}i\pi t}$     |
| $c \quad (\frac{1}{2}, \frac{t}{2}, 0)$ | $\{m_{100}   \frac{1}{2} \frac{1}{2} 0\}$<br>$c_1 \quad -e^{-\frac{1}{2}i\pi(t+1)}$<br>$c_2 \quad e^{-\frac{1}{2}i\pi(t+1)}$ |
| $d \quad (\frac{t}{2}, \frac{1}{2}, 0)$ | $\{m_{010}   \frac{1}{2} \frac{1}{2} 0\}$<br>$d_1 \quad -e^{-\frac{1}{2}i\pi(t+1)}$<br>$d_2 \quad e^{-\frac{1}{2}i\pi(t+1)}$ |

$$\begin{aligned} \mathcal{W}_1^{\text{gapless}} = & \sum_{m=1}^{n_{a_1}} \text{sgn}(v_m^{a_1}) \frac{1 - \text{sgn}(\delta_m^{a_1})}{2} + \sum_{m=1}^{n_{a_2}} \text{sgn}(v_m^{a_2}) \frac{1 - \text{sgn}(\delta_m^{a_2})}{2} - \sum_{m=1}^{n_{b_1}} \text{sgn}(v_m^{b_1}) \frac{1 - \text{sgn}(\delta_m^{b_1})}{2} \\ & - \sum_{m=1}^{n_{b_2}} \text{sgn}(v_m^{b_2}) \frac{1 - \text{sgn}(\delta_m^{b_2})}{2} + 2 \sum_{m=1}^{n_{c_1}} \text{sgn}(v_m^{c_1}) \frac{1 - \text{sgn}(\delta_m^{c_1})}{2} - 2 \sum_{m=1}^{n_{d_1}} \text{sgn}(v_m^{d_1}) \frac{1 - \text{sgn}(\delta_m^{d_1})}{2} \end{aligned} \quad (\text{L25.1})$$

$$\mathcal{X}_1 = \sum_{m=1}^{n_{a_2}} \frac{1 - \text{sgn}(\delta_m^{a_2})}{2} + \sum_{m=1}^{n_{b_1}} \frac{1 - \text{sgn}(\delta_m^{b_1})}{2} \mod 2 \quad (\text{L25.2})$$

$$\begin{aligned} \mathcal{X}_2 = & 2 \sum_{m=1}^{n_{a_2}} \text{sgn}(v_m^{a_2}) \frac{1 - \text{sgn}(\delta_m^{a_2})}{2} - \sum_{m=1}^{n_{b_1}} \text{sgn}(v_m^{b_1}) \frac{1 - \text{sgn}(\delta_m^{b_1})}{2} - \sum_{m=1}^{n_{b_2}} \text{sgn}(v_m^{b_2}) \frac{1 - \text{sgn}(\delta_m^{b_2})}{2} \\ & - 2 \sum_{m=1}^{n_{d_1}} \text{sgn}(v_m^{d_1}) \frac{1 - \text{sgn}(\delta_m^{d_1})}{2} \mod 4 \end{aligned} \quad (\text{L25.3})$$

### L26. LAYER GROUP NO. 26

| line segment        | character of irrep (generators only)                         |
|---------------------|--------------------------------------------------------------|
| $a \quad (t, 0, 0)$ | $\{m_{010}   0 \ 0 \ 0\}$<br>$a_1 \quad -i$<br>$a_2 \quad i$ |
| $b \quad (0, t, 0)$ | $\{m_{100}   0 \ 0 \ 0\}$<br>$b_1 \quad -i$<br>$b_2 \quad i$ |

|                                             |                                                                    |
|---------------------------------------------|--------------------------------------------------------------------|
| $c \quad (\frac{t}{2}, 1 - \frac{t}{2}, 0)$ | $c_1 \quad \begin{array}{c} \{1 \mid 0 \ 0 \ 0\} \\ 1 \end{array}$ |
|---------------------------------------------|--------------------------------------------------------------------|

$$\mathcal{W}_1^{\text{gapless}} = \sum_{m=1}^{n_{a_1}} \text{sgn}(v_m^{a_1}) \frac{1 - \text{sgn}(\delta_m^{a_1})}{2} + \sum_{m=1}^{n_{a_2}} \text{sgn}(v_m^{a_2}) \frac{1 - \text{sgn}(\delta_m^{a_2})}{2} - \sum_{m=1}^{n_{b_1}} \text{sgn}(v_m^{b_1}) \frac{1 - \text{sgn}(\delta_m^{b_1})}{2} - \sum_{m=1}^{n_{b_2}} \text{sgn}(v_m^{b_2}) \frac{1 - \text{sgn}(\delta_m^{b_2})}{2} \quad (\text{L26.1})$$

$$\mathcal{W}_1^{\text{gapped}} = - \sum_{m=1}^{n_{a_2}} \text{sgn}(v_m^{a_2}) \frac{1 - \text{sgn}(\delta_m^{a_2})}{2} + \sum_{m=1}^{n_{b_2}} \text{sgn}(v_m^{b_2}) \frac{1 - \text{sgn}(\delta_m^{b_2})}{2} \quad (\text{L26.2})$$

$$\mathcal{W}_2^{\text{gapped}} = - \sum_{m=1}^{n_{a_2}} \text{sgn}(v_m^{a_2}) \frac{1 - \text{sgn}(\delta_m^{a_2})}{2} + \sum_{m=1}^{n_{b_1}} \text{sgn}(v_m^{b_1}) \frac{1 - \text{sgn}(\delta_m^{b_1})}{2} \quad (\text{L26.3})$$

$$\mathcal{X}_1 = \sum_{m=1}^{n_{c_1}} \frac{1 - \text{sgn}(\delta_m^{c_1})}{2} \quad \text{mod } 2 \quad (\text{L26.4})$$

## L27. LAYER GROUP NO. 27

| line segment                            | character of irrep (generators only)                                                                              |
|-----------------------------------------|-------------------------------------------------------------------------------------------------------------------|
| $a \quad (\frac{t}{2}, 0, 0)$           | $\begin{array}{c} \{m_{001} \mid 0 \ 0 \ 0\} \\ a_1 \quad -i \\ a_2 \quad i \end{array}$                          |
| $b \quad (0, \frac{t}{2}, 0)$           | $\begin{array}{c} \{2_{010} \mid 0 \ 0 \ 0\} \quad \{m_{100} \mid 0 \ 0 \ 0\} \\ b_1 \quad 0 \quad 0 \end{array}$ |
| $c \quad (\frac{1}{2}, \frac{t}{2}, 0)$ | $\begin{array}{c} \{2_{010} \mid 0 \ 0 \ 0\} \quad \{m_{100} \mid 0 \ 0 \ 0\} \\ c_1 \quad 0 \quad 0 \end{array}$ |
| $d \quad (\frac{t}{2}, \frac{1}{2}, 0)$ | $\begin{array}{c} \{m_{001} \mid 0 \ 0 \ 0\} \\ d_1 \quad -i \\ d_2 \quad i \end{array}$                          |

$$\mathcal{W}_1^{\text{gapless}} = \sum_{m=1}^{n_{a_1}} \text{sgn}(v_m^{a_1}) \frac{1 - \text{sgn}(\delta_m^{a_1})}{2} - \sum_{m=1}^{n_{b_1}} \text{sgn}(v_m^{b_1}) \frac{1 - \text{sgn}(\delta_m^{b_1})}{2} + \sum_{m=1}^{n_{c_1}} \text{sgn}(v_m^{c_1}) \frac{1 - \text{sgn}(\delta_m^{c_1})}{2} - \sum_{m=1}^{n_{d_1}} \text{sgn}(v_m^{d_1}) \frac{1 - \text{sgn}(\delta_m^{d_1})}{2} \quad (\text{L27.1})$$

$$\mathcal{W}_2^{\text{gapless}} = \sum_{m=1}^{n_{a_2}} \text{sgn}(v_m^{a_2}) \frac{1 - \text{sgn}(\delta_m^{a_2})}{2} - \sum_{m=1}^{n_{b_1}} \text{sgn}(v_m^{b_1}) \frac{1 - \text{sgn}(\delta_m^{b_1})}{2} + \sum_{m=1}^{n_{c_1}} \text{sgn}(v_m^{c_1}) \frac{1 - \text{sgn}(\delta_m^{c_1})}{2} - \sum_{m=1}^{n_{d_2}} \text{sgn}(v_m^{d_2}) \frac{1 - \text{sgn}(\delta_m^{d_2})}{2} \quad (\text{L27.2})$$

$$\mathcal{W}_1^{\text{gapped}} = - \sum_{m=1}^{n_{d_1}} \text{sgn}(v_m^{d_1}) \frac{1 - \text{sgn}(\delta_m^{d_1})}{2} + \sum_{m=1}^{n_{d_2}} \text{sgn}(v_m^{d_2}) \frac{1 - \text{sgn}(\delta_m^{d_2})}{2} \quad (\text{L27.3})$$

**L28. LAYER GROUP NO. 28**

| line segment                            | character of irrep (generators only) |                                                                                   |
|-----------------------------------------|--------------------------------------|-----------------------------------------------------------------------------------|
| $a \quad (\frac{t}{2}, 0, 0)$           | $a_1$                                | $\{m_{001}   0 \quad \frac{1}{2} \quad 0\}$                                       |
|                                         | $a_2$                                | $\begin{matrix} -i \\ i \end{matrix}$                                             |
| $b \quad (0, \frac{t}{2}, 0)$           | $b_1$                                | $\{2_{010}   0 \quad \frac{1}{2} \quad 0\} \quad \{m_{100}   0 \quad 0 \quad 0\}$ |
|                                         |                                      | $\begin{matrix} 0 \\ 0 \end{matrix}$                                              |
| $c \quad (\frac{1}{2}, \frac{t}{2}, 0)$ | $c_1$                                | $\{2_{010}   0 \quad \frac{1}{2} \quad 0\} \quad \{m_{100}   0 \quad 0 \quad 0\}$ |
|                                         |                                      | $\begin{matrix} 0 \\ 0 \end{matrix}$                                              |
| $d \quad (\frac{t}{2}, \frac{1}{2}, 0)$ | $d_1$                                | $\{m_{001}   0 \quad \frac{1}{2} \quad 0\}$                                       |
|                                         | $d_2$                                | $\begin{matrix} -1 \\ 1 \end{matrix}$                                             |

$$\mathcal{W}_1^{\text{gapless}} = \sum_{m=1}^{n_{a_1}} \text{sgn}(v_m^{a_1}) \frac{1 - \text{sgn}(\delta_m^{a_1})}{2} - \sum_{m=1}^{n_{b_1}} \text{sgn}(v_m^{b_1}) \frac{1 - \text{sgn}(\delta_m^{b_1})}{2} + \sum_{m=1}^{n_{c_1}} \text{sgn}(v_m^{c_1}) \frac{1 - \text{sgn}(\delta_m^{c_1})}{2} - \sum_{m=1}^{n_{d_1}} \text{sgn}(v_m^{d_1}) \frac{1 - \text{sgn}(\delta_m^{d_1})}{2} \quad (\text{L28.1})$$

$$\mathcal{W}_2^{\text{gapless}} = \sum_{m=1}^{n_{a_2}} \text{sgn}(v_m^{a_2}) \frac{1 - \text{sgn}(\delta_m^{a_2})}{2} - \sum_{m=1}^{n_{b_1}} \text{sgn}(v_m^{b_1}) \frac{1 - \text{sgn}(\delta_m^{b_1})}{2} + \sum_{m=1}^{n_{c_1}} \text{sgn}(v_m^{c_1}) \frac{1 - \text{sgn}(\delta_m^{c_1})}{2} - \sum_{m=1}^{n_{d_1}} \text{sgn}(v_m^{d_1}) \frac{1 - \text{sgn}(\delta_m^{d_1})}{2} \quad (\text{L28.2})$$

$$\mathcal{X}_1 = \sum_{m=1}^{n_{d_1}} \frac{1 - \text{sgn}(\delta_m^{d_1})}{2} \quad \text{mod } 2 \quad (\text{L28.3})$$

**L29. LAYER GROUP NO. 29**

| line segment                            | character of irrep (generators only) |                                                                                             |
|-----------------------------------------|--------------------------------------|---------------------------------------------------------------------------------------------|
| $a \quad (\frac{t}{2}, 0, 0)$           | $a_1$                                | $\{m_{001}   0 \quad 0 \quad 0\}$                                                           |
|                                         | $a_2$                                | $\begin{matrix} -i \\ i \end{matrix}$                                                       |
| $b \quad (0, \frac{t}{2}, 0)$           | $b_1$                                | $\{2_{010}   0 \quad \frac{1}{2} \quad 0\} \quad \{m_{100}   0 \quad \frac{1}{2} \quad 0\}$ |
|                                         |                                      | $\begin{matrix} 0 \\ 0 \end{matrix}$                                                        |
| $c \quad (\frac{1}{2}, \frac{t}{2}, 0)$ | $c_1$                                | $\{2_{010}   0 \quad \frac{1}{2} \quad 0\} \quad \{m_{100}   0 \quad \frac{1}{2} \quad 0\}$ |
|                                         |                                      | $\begin{matrix} 0 \\ 0 \end{matrix}$                                                        |
| $d \quad (\frac{t}{2}, \frac{1}{2}, 0)$ | $d_1$                                | $\{m_{001}   0 \quad 0 \quad 0\}$                                                           |
|                                         | $d_2$                                | $\begin{matrix} -i \\ i \end{matrix}$                                                       |

$$\mathcal{W}_1^{\text{gapless}} = \sum_{m=1}^{n_{a_1}} \text{sgn}(v_m^{a_1}) \frac{1 - \text{sgn}(\delta_m^{a_1})}{2} - \sum_{m=1}^{n_{b_1}} \text{sgn}(v_m^{b_1}) \frac{1 - \text{sgn}(\delta_m^{b_1})}{2} + \sum_{m=1}^{n_{c_1}} \text{sgn}(v_m^{c_1}) \frac{1 - \text{sgn}(\delta_m^{c_1})}{2} - 2 \sum_{m=1}^{n_{d_1}} \text{sgn}(v_m^{d_1}) \frac{1 - \text{sgn}(\delta_m^{d_1})}{2} \quad (\text{L29.1})$$

$$\mathcal{W}_2^{\text{gapless}} = \sum_{m=1}^{n_{a_2}} \text{sgn}(v_m^{a_2}) \frac{1 - \text{sgn}(\delta_m^{a_2})}{2} - \sum_{m=1}^{n_{b_1}} \text{sgn}(v_m^{b_1}) \frac{1 - \text{sgn}(\delta_m^{b_1})}{2} + \sum_{m=1}^{n_{c_1}} \text{sgn}(v_m^{c_1}) \frac{1 - \text{sgn}(\delta_m^{c_1})}{2} - 2 \sum_{m=1}^{n_{d_2}} \text{sgn}(v_m^{d_2}) \frac{1 - \text{sgn}(\delta_m^{d_2})}{2} \quad (\text{L29.2})$$

$$\mathcal{W}_1^{\text{gapped}} = - \sum_{m=1}^{n_{d_1}} \text{sgn}(v_m^{d_1}) \frac{1 - \text{sgn}(\delta_m^{d_1})}{2} + \sum_{m=1}^{n_{d_2}} \text{sgn}(v_m^{d_2}) \frac{1 - \text{sgn}(\delta_m^{d_2})}{2} \quad (\text{L29.3})$$

### L30. LAYER GROUP NO. 30

| line segment                            | character of irrep (generators only)                                                                     |
|-----------------------------------------|----------------------------------------------------------------------------------------------------------|
| $a \quad (\frac{t}{2}, 0, 0)$           | $\{m_{001}   0 \quad \frac{1}{2} \quad 0 \}$<br>$a_1 \quad -i$<br>$a_2 \quad i$                          |
| $b \quad (0, \frac{t}{2}, 0)$           | $\{2_{010}   0 \quad 0 \quad 0 \}$ $\{m_{100}   0 \quad \frac{1}{2} \quad 0 \}$<br>$b_1 \quad 0 \quad 0$ |
| $c \quad (\frac{1}{2}, \frac{t}{2}, 0)$ | $\{2_{010}   0 \quad 0 \quad 0 \}$ $\{m_{100}   0 \quad \frac{1}{2} \quad 0 \}$<br>$c_1 \quad 0 \quad 0$ |
| $d \quad (\frac{t}{2}, \frac{1}{2}, 0)$ | $\{m_{001}   0 \quad \frac{1}{2} \quad 0 \}$<br>$d_1 \quad -1$<br>$d_2 \quad 1$                          |

$$\mathcal{W}_1^{\text{gapless}} = \sum_{m=1}^{n_{a_1}} \text{sgn}(v_m^{a_1}) \frac{1 - \text{sgn}(\delta_m^{a_1})}{2} - \sum_{m=1}^{n_{b_1}} \text{sgn}(v_m^{b_1}) \frac{1 - \text{sgn}(\delta_m^{b_1})}{2} + \sum_{m=1}^{n_{c_1}} \text{sgn}(v_m^{c_1}) \frac{1 - \text{sgn}(\delta_m^{c_1})}{2} - \sum_{m=1}^{n_{d_1}} \text{sgn}(v_m^{d_1}) \frac{1 - \text{sgn}(\delta_m^{d_1})}{2} \quad (\text{L30.1})$$

$$\mathcal{W}_2^{\text{gapless}} = \sum_{m=1}^{n_{a_2}} \text{sgn}(v_m^{a_2}) \frac{1 - \text{sgn}(\delta_m^{a_2})}{2} - \sum_{m=1}^{n_{b_1}} \text{sgn}(v_m^{b_1}) \frac{1 - \text{sgn}(\delta_m^{b_1})}{2} + \sum_{m=1}^{n_{c_1}} \text{sgn}(v_m^{c_1}) \frac{1 - \text{sgn}(\delta_m^{c_1})}{2} - \sum_{m=1}^{n_{d_1}} \text{sgn}(v_m^{d_1}) \frac{1 - \text{sgn}(\delta_m^{d_1})}{2} \quad (\text{L30.2})$$

$$\mathcal{X}_1 = \sum_{m=1}^{n_{d_1}} \frac{1 - \text{sgn}(\delta_m^{d_1})}{2} \quad \text{mod } 2 \quad (\text{L30.3})$$

### L31. LAYER GROUP NO. 31

| line segment                            | character of irrep (generators only)                                                                                                                                                    |
|-----------------------------------------|-----------------------------------------------------------------------------------------------------------------------------------------------------------------------------------------|
| $a \quad (\frac{t}{2}, 0, 0)$           | $\{m_{001}   \frac{1}{2} \quad 0 \quad 0 \}$<br>$a_1 \quad -ie^{-\frac{1}{2}i\pi t}$<br>$a_2 \quad ie^{-\frac{1}{2}i\pi t}$                                                             |
| $b \quad (0, \frac{t}{2}, 0)$           | $\{2_{010}   0 \quad 0 \quad 0 \}$ $\{m_{100}   \frac{1}{2} \quad 0 \quad 0 \}$<br>$b_1 \quad 0 \quad 0$                                                                                |
| $c \quad (\frac{1}{2}, \frac{t}{2}, 0)$ | $\{2_{010}   0 \quad 0 \quad 0 \}$ $\{m_{100}   \frac{1}{2} \quad 0 \quad 0 \}$<br>$c_1 \quad -i \quad i$<br>$c_2 \quad -i \quad -i$<br>$c_3 \quad i \quad i$<br>$c_4 \quad i \quad -i$ |
| $d \quad (\frac{t}{2}, \frac{1}{2}, 0)$ | $\{m_{001}   \frac{1}{2} \quad 0 \quad 0 \}$<br>$d_1 \quad -ie^{-\frac{1}{2}i\pi t}$<br>$d_2 \quad ie^{-\frac{1}{2}i\pi t}$                                                             |

$$\begin{aligned} \mathcal{W}_1^{\text{gapless}} = & \sum_{m=1}^{n_{a_1}} \text{sgn}(v_m^{a_1}) \frac{1 - \text{sgn}(\delta_m^{a_1})}{2} - \sum_{m=1}^{n_{b_1}} \text{sgn}(v_m^{b_1}) \frac{1 - \text{sgn}(\delta_m^{b_1})}{2} + \sum_{m=1}^{n_{c_2}} \text{sgn}(v_m^{c_2}) \frac{1 - \text{sgn}(\delta_m^{c_2})}{2} \\ & + \sum_{m=1}^{n_{c_3}} \text{sgn}(v_m^{c_3}) \frac{1 - \text{sgn}(\delta_m^{c_3})}{2} - \sum_{m=1}^{n_{d_1}} \text{sgn}(v_m^{d_1}) \frac{1 - \text{sgn}(\delta_m^{d_1})}{2} \end{aligned} \quad (\text{L31.1})$$

$$\begin{aligned} \mathcal{W}_2^{\text{gapless}} = & \sum_{m=1}^{n_{a_2}} \text{sgn}(v_m^{a_2}) \frac{1 - \text{sgn}(\delta_m^{a_2})}{2} - \sum_{m=1}^{n_{b_1}} \text{sgn}(v_m^{b_1}) \frac{1 - \text{sgn}(\delta_m^{b_1})}{2} + \sum_{m=1}^{n_{c_1}} \text{sgn}(v_m^{c_1}) \frac{1 - \text{sgn}(\delta_m^{c_1})}{2} \\ & + \sum_{m=1}^{n_{c_4}} \text{sgn}(v_m^{c_4}) \frac{1 - \text{sgn}(\delta_m^{c_4})}{2} - \sum_{m=1}^{n_{d_2}} \text{sgn}(v_m^{d_2}) \frac{1 - \text{sgn}(\delta_m^{d_2})}{2} \end{aligned} \quad (\text{L31.2})$$

$$\mathcal{W}_1^{\text{gapped}} = - \sum_{m=1}^{n_{c_2}} \text{sgn}(v_m^{c_2}) \frac{1 - \text{sgn}(\delta_m^{c_2})}{2} + \sum_{m=1}^{n_{c_3}} \text{sgn}(v_m^{c_3}) \frac{1 - \text{sgn}(\delta_m^{c_3})}{2} \quad (\text{L31.3})$$

$$\mathcal{W}_2^{\text{gapped}} = - \sum_{m=1}^{n_{c_1}} \text{sgn}(v_m^{c_1}) \frac{1 - \text{sgn}(\delta_m^{c_1})}{2} + \sum_{m=1}^{n_{c_4}} \text{sgn}(v_m^{c_4}) \frac{1 - \text{sgn}(\delta_m^{c_4})}{2} \quad (\text{L31.4})$$

$$\mathcal{X}_1 = \sum_{m=1}^{n_{d_1}} \frac{1 - \text{sgn}(\delta_m^{d_1})}{2} + \sum_{m=1}^{n_{d_2}} \frac{1 - \text{sgn}(\delta_m^{d_2})}{2} \quad \text{mod } 2 \quad (\text{L31.5})$$

### L32. LAYER GROUP NO. 32

| line segment                            | character of irrep (generators only)                                                                                                                                                                                                                                                                |
|-----------------------------------------|-----------------------------------------------------------------------------------------------------------------------------------------------------------------------------------------------------------------------------------------------------------------------------------------------------|
| $a \quad (\frac{t}{2}, 0, 0)$           | $\{m_{001}   \frac{1}{2} \quad \frac{1}{2} \quad 0\}$<br>$a_1 \quad -ie^{-\frac{1}{2}i\pi t}$<br>$a_2 \quad ie^{-\frac{1}{2}i\pi t}$                                                                                                                                                                |
| $b \quad (0, \frac{t}{2}, 0)$           | $\{2_{010}   \frac{1}{2} \quad \frac{1}{2} \quad 0\} \quad \{m_{100}   0 \quad 0 \quad 0\}$<br>$b_1 \quad 0 \quad 0$                                                                                                                                                                                |
| $c \quad (\frac{1}{2}, \frac{t}{2}, 0)$ | $\{2_{010}   \frac{1}{2} \quad \frac{1}{2} \quad 0\} \quad \{m_{100}   0 \quad 0 \quad 0\}$<br>$c_1 \quad -e^{-\frac{1}{2}i\pi(t+1)} \quad -i$<br>$c_2 \quad -e^{-\frac{1}{2}i\pi(t+1)} \quad i$<br>$c_3 \quad e^{-\frac{1}{2}i\pi(t+1)} \quad -i$<br>$c_4 \quad e^{-\frac{1}{2}i\pi(t+1)} \quad i$ |
| $d \quad (\frac{t}{2}, \frac{1}{2}, 0)$ | $\{m_{001}   \frac{1}{2} \quad \frac{1}{2} \quad 0\}$<br>$d_1 \quad -ie^{-\frac{1}{2}i\pi(t+1)}$<br>$d_2 \quad ie^{-\frac{1}{2}i\pi(t+1)}$                                                                                                                                                          |

$$\begin{aligned} \mathcal{W}_1^{\text{gapless}} = & \sum_{m=1}^{n_{a_1}} \text{sgn}(v_m^{a_1}) \frac{1 - \text{sgn}(\delta_m^{a_1})}{2} - \sum_{m=1}^{n_{b_1}} \text{sgn}(v_m^{b_1}) \frac{1 - \text{sgn}(\delta_m^{b_1})}{2} + \sum_{m=1}^{n_{c_1}} \text{sgn}(v_m^{c_1}) \frac{1 - \text{sgn}(\delta_m^{c_1})}{2} \\ & + \sum_{m=1}^{n_{c_4}} \text{sgn}(v_m^{c_4}) \frac{1 - \text{sgn}(\delta_m^{c_4})}{2} - \sum_{m=1}^{n_{d_1}} \text{sgn}(v_m^{d_1}) \frac{1 - \text{sgn}(\delta_m^{d_1})}{2} \end{aligned} \quad (\text{L32.1})$$

$$\begin{aligned} \mathcal{W}_2^{\text{gapless}} = & \sum_{m=1}^{n_{a_2}} \text{sgn}(v_m^{a_2}) \frac{1 - \text{sgn}(\delta_m^{a_2})}{2} - \sum_{m=1}^{n_{b_1}} \text{sgn}(v_m^{b_1}) \frac{1 - \text{sgn}(\delta_m^{b_1})}{2} + \sum_{m=1}^{n_{c_2}} \text{sgn}(v_m^{c_2}) \frac{1 - \text{sgn}(\delta_m^{c_2})}{2} \\ & + \sum_{m=1}^{n_{c_3}} \text{sgn}(v_m^{c_3}) \frac{1 - \text{sgn}(\delta_m^{c_3})}{2} - \sum_{m=1}^{n_{d_1}} \text{sgn}(v_m^{d_1}) \frac{1 - \text{sgn}(\delta_m^{d_1})}{2} \end{aligned} \quad (\text{L32.2})$$

$$\mathcal{W}_1^{\text{gapped}} = \sum_{m=1}^{n_{c_1}} \text{sgn}(v_m^{c_1}) \frac{1 - \text{sgn}(\delta_m^{c_1})}{2} - \sum_{m=1}^{n_{c_2}} \text{sgn}(v_m^{c_2}) \frac{1 - \text{sgn}(\delta_m^{c_2})}{2} + \sum_{m=1}^{n_{c_3}} \text{sgn}(v_m^{c_3}) \frac{1 - \text{sgn}(\delta_m^{c_3})}{2} - \sum_{m=1}^{n_{c_4}} \text{sgn}(v_m^{c_4}) \frac{1 - \text{sgn}(\delta_m^{c_4})}{2} \quad (\text{L32.3})$$

$$\mathcal{X}_1 = \sum_{m=1}^{n_{c_1}} \frac{1 - \text{sgn}(\delta_m^{c_1})}{2} + \sum_{m=1}^{n_{c_4}} \frac{1 - \text{sgn}(\delta_m^{c_4})}{2} + \sum_{m=1}^{n_{d_1}} \frac{1 - \text{sgn}(\delta_m^{d_1})}{2} \mod 2 \quad (\text{L32.4})$$

### L33. LAYER GROUP NO. 33

| line segment                            | character of irrep (generators only) |                                                                                       |
|-----------------------------------------|--------------------------------------|---------------------------------------------------------------------------------------|
| $a \quad (\frac{t}{2}, 0, 0)$           | $a_1$                                | $\{m_{001}   \frac{1}{2} \ 0 \ 0\}$                                                   |
|                                         |                                      | $-ie^{-\frac{1}{2}i\pi t}$                                                            |
|                                         | $a_2$                                | $ie^{-\frac{1}{2}i\pi t}$                                                             |
| $b \quad (0, \frac{t}{2}, 0)$           | $b_1$                                | $\{2_{010}   0 \ \frac{1}{2} \ 0\} \quad \{m_{100}   \frac{1}{2} \ \frac{1}{2} \ 0\}$ |
|                                         |                                      | $0 \quad 0$                                                                           |
| $c \quad (\frac{1}{2}, \frac{t}{2}, 0)$ | $c_1$                                | $\{2_{010}   0 \ \frac{1}{2} \ 0\} \quad \{m_{100}   \frac{1}{2} \ \frac{1}{2} \ 0\}$ |
|                                         |                                      | $-ie^{-\frac{1}{2}i\pi t} \quad -e^{-\frac{1}{2}i\pi(t+1)}$                           |
|                                         | $c_2$                                | $-ie^{-\frac{1}{2}i\pi t} \quad e^{-\frac{1}{2}i\pi(t+1)}$                            |
|                                         | $c_3$                                | $ie^{-\frac{1}{2}i\pi t} \quad -e^{-\frac{1}{2}i\pi(t+1)}$                            |
| $d \quad (\frac{t}{2}, \frac{1}{2}, 0)$ | $c_4$                                | $ie^{-\frac{1}{2}i\pi t} \quad e^{-\frac{1}{2}i\pi(t+1)}$                             |
|                                         | $d_1$                                | $\{m_{001}   \frac{1}{2} \ 0 \ 0\}$                                                   |
|                                         |                                      | $-ie^{-\frac{1}{2}i\pi t}$                                                            |
|                                         | $d_2$                                | $ie^{-\frac{1}{2}i\pi t}$                                                             |

$$\begin{aligned} \mathcal{W}_1^{\text{gapless}} = & \sum_{m=1}^{n_{a_1}} \text{sgn}(v_m^{a_1}) \frac{1 - \text{sgn}(\delta_m^{a_1})}{2} - \sum_{m=1}^{n_{b_1}} \text{sgn}(v_m^{b_1}) \frac{1 - \text{sgn}(\delta_m^{b_1})}{2} + \sum_{m=1}^{n_{c_2}} \text{sgn}(v_m^{c_2}) \frac{1 - \text{sgn}(\delta_m^{c_2})}{2} \\ & + \sum_{m=1}^{n_{c_3}} \text{sgn}(v_m^{c_3}) \frac{1 - \text{sgn}(\delta_m^{c_3})}{2} - 2 \sum_{m=1}^{n_{d_1}} \text{sgn}(v_m^{d_1}) \frac{1 - \text{sgn}(\delta_m^{d_1})}{2} \end{aligned} \quad (\text{L33.1})$$



$$\begin{aligned} \mathcal{W}_2^{\text{gapless}} = & \sum_{m=1}^{n_{a_2}} \text{sgn}(v_m^{a_2}) \frac{1 - \text{sgn}(\delta_m^{a_2})}{2} - \sum_{m=1}^{n_{b_1}} \text{sgn}(v_m^{b_1}) \frac{1 - \text{sgn}(\delta_m^{b_1})}{2} + \sum_{m=1}^{n_{c_1}} \text{sgn}(v_m^{c_1}) \frac{1 - \text{sgn}(\delta_m^{c_1})}{2} \\ & + \sum_{m=1}^{n_{c_4}} \text{sgn}(v_m^{c_4}) \frac{1 - \text{sgn}(\delta_m^{c_4})}{2} - 2 \sum_{m=1}^{n_{d_2}} \text{sgn}(v_m^{d_2}) \frac{1 - \text{sgn}(\delta_m^{d_2})}{2} \end{aligned} \quad (\text{L33.2})$$

$$\mathcal{X}_1 = \sum_{m=1}^{n_{c_1}} \frac{1 - \text{sgn}(\delta_m^{c_1})}{2} + \sum_{m=1}^{n_{c_4}} \frac{1 - \text{sgn}(\delta_m^{c_4})}{2} \quad \text{mod } 2 \quad (\text{L33.3})$$

$$\begin{aligned} \mathcal{X}_2 = & - \sum_{m=1}^{n_{c_1}} \text{sgn}(v_m^{c_1}) \frac{1 - \text{sgn}(\delta_m^{c_1})}{2} + \sum_{m=1}^{n_{c_2}} \text{sgn}(v_m^{c_2}) \frac{1 - \text{sgn}(\delta_m^{c_2})}{2} - \sum_{m=1}^{n_{c_3}} \text{sgn}(v_m^{c_3}) \frac{1 - \text{sgn}(\delta_m^{c_3})}{2} \\ & + \sum_{m=1}^{n_{c_4}} \text{sgn}(v_m^{c_4}) \frac{1 - \text{sgn}(\delta_m^{c_4})}{2} - 2 \sum_{m=1}^{n_{d_1}} \text{sgn}(v_m^{d_1}) \frac{1 - \text{sgn}(\delta_m^{d_1})}{2} + 2 \sum_{m=1}^{n_{d_2}} \text{sgn}(v_m^{d_2}) \frac{1 - \text{sgn}(\delta_m^{d_2})}{2} \quad \text{mod } 4 \end{aligned} \quad (\text{L33.4})$$

#### L34. LAYER GROUP NO. 34

| line segment                            | character of irrep (generators only) |                                                                                             |
|-----------------------------------------|--------------------------------------|---------------------------------------------------------------------------------------------|
| $a \quad (\frac{t}{2}, 0, 0)$           | $a_1$                                | $\{m_{001}   \frac{1}{2} \quad \frac{1}{2} \quad 0\}$                                       |
|                                         |                                      | $-ie^{-\frac{1}{2}i\pi t}$                                                                  |
|                                         | $a_2$                                | $ie^{-\frac{1}{2}i\pi t}$                                                                   |
| $b \quad (0, \frac{t}{2}, 0)$           | $b_1$                                | $\{2_{010}   0 \quad 0 \quad 0\} \quad \{m_{100}   \frac{1}{2} \quad \frac{1}{2} \quad 0\}$ |
|                                         |                                      | $0 \quad 0$                                                                                 |
| $c \quad (\frac{1}{2}, \frac{t}{2}, 0)$ | $c_1$                                | $\{2_{010}   0 \quad 0 \quad 0\} \quad \{m_{100}   \frac{1}{2} \quad \frac{1}{2} \quad 0\}$ |
|                                         |                                      | $-i \quad -e^{-\frac{1}{2}i\pi(t+1)}$                                                       |
|                                         | $c_2$                                | $-i \quad e^{-\frac{1}{2}i\pi(t+1)}$                                                        |
|                                         | $c_3$                                | $i \quad -e^{-\frac{1}{2}i\pi(t+1)}$                                                        |
| $d \quad (\frac{t}{2}, \frac{1}{2}, 0)$ | $d_1$                                | $\{m_{001}   \frac{1}{2} \quad \frac{1}{2} \quad 0\}$                                       |
|                                         |                                      | $-ie^{-\frac{1}{2}i\pi(t+1)}$                                                               |
|                                         | $d_2$                                | $ie^{-\frac{1}{2}i\pi(t+1)}$                                                                |

$$\begin{aligned} \mathcal{W}_1^{\text{gapless}} = & \sum_{m=1}^{n_{a_1}} \text{sgn}(v_m^{a_1}) \frac{1 - \text{sgn}(\delta_m^{a_1})}{2} - \sum_{m=1}^{n_{b_1}} \text{sgn}(v_m^{b_1}) \frac{1 - \text{sgn}(\delta_m^{b_1})}{2} + \sum_{m=1}^{n_{c_2}} \text{sgn}(v_m^{c_2}) \frac{1 - \text{sgn}(\delta_m^{c_2})}{2} \\ & + \sum_{m=1}^{n_{c_3}} \text{sgn}(v_m^{c_3}) \frac{1 - \text{sgn}(\delta_m^{c_3})}{2} - \sum_{m=1}^{n_{d_1}} \text{sgn}(v_m^{d_1}) \frac{1 - \text{sgn}(\delta_m^{d_1})}{2} \end{aligned} \quad (\text{L34.1})$$

$$\begin{aligned} \mathcal{W}_2^{\text{gapless}} = & \sum_{m=1}^{n_{a_2}} \text{sgn}(v_m^{a_2}) \frac{1 - \text{sgn}(\delta_m^{a_2})}{2} - \sum_{m=1}^{n_{b_1}} \text{sgn}(v_m^{b_1}) \frac{1 - \text{sgn}(\delta_m^{b_1})}{2} + \sum_{m=1}^{n_{c_1}} \text{sgn}(v_m^{c_1}) \frac{1 - \text{sgn}(\delta_m^{c_1})}{2} \\ & + \sum_{m=1}^{n_{c_4}} \text{sgn}(v_m^{c_4}) \frac{1 - \text{sgn}(\delta_m^{c_4})}{2} - \sum_{m=1}^{n_{d_1}} \text{sgn}(v_m^{d_1}) \frac{1 - \text{sgn}(\delta_m^{d_1})}{2} \end{aligned} \quad (\text{L34.2})$$

$$\mathcal{W}_1^{\text{gapped}} = - \sum_{m=1}^{n_{c_1}} \text{sgn}(v_m^{c_1}) \frac{1 - \text{sgn}(\delta_m^{c_1})}{2} - \sum_{m=1}^{n_{c_2}} \text{sgn}(v_m^{c_2}) \frac{1 - \text{sgn}(\delta_m^{c_2})}{2} + \sum_{m=1}^{n_{c_3}} \text{sgn}(v_m^{c_3}) \frac{1 - \text{sgn}(\delta_m^{c_3})}{2} + \sum_{m=1}^{n_{c_4}} \text{sgn}(v_m^{c_4}) \frac{1 - \text{sgn}(\delta_m^{c_4})}{2} \quad (\text{L34.3})$$

$$\mathcal{X}_1 = \sum_{m=1}^{n_{c_1}} \frac{1 - \text{sgn}(\delta_m^{c_1})}{2} + \sum_{m=1}^{n_{c_4}} \frac{1 - \text{sgn}(\delta_m^{c_4})}{2} + \sum_{m=1}^{n_{d_1}} \frac{1 - \text{sgn}(\delta_m^{d_1})}{2} \mod 2 \quad (\text{L34.4})$$

### L35. LAYER GROUP NO. 35

| line segment                            | character of irrep (generators only)                                         |
|-----------------------------------------|------------------------------------------------------------------------------|
| $a \ (t, 0, 0)$                         | $\{m_{001}   0 \ 0 \ 0\}$<br>$a_1 \quad -i$<br>$a_2 \quad i$                 |
| $b \ (0, t, 0)$                         | $\{2_{010}   0 \ 0 \ 0\} \ \{m_{100}   0 \ 0 \ 0\}$<br>$b_1 \quad 0 \quad 0$ |
| $c \ (\frac{t}{2}, 1 - \frac{t}{2}, 0)$ | $\{m_{001}   0 \ 0 \ 0\}$<br>$c_1 \quad -i$<br>$c_2 \quad i$                 |

$$\mathcal{W}_1^{\text{gapless}} = \sum_{m=1}^{n_{a_1}} \text{sgn}(v_m^{a_1}) \frac{1 - \text{sgn}(\delta_m^{a_1})}{2} - \sum_{m=1}^{n_{b_1}} \text{sgn}(v_m^{b_1}) \frac{1 - \text{sgn}(\delta_m^{b_1})}{2} - \sum_{m=1}^{n_{c_1}} \text{sgn}(v_m^{c_1}) \frac{1 - \text{sgn}(\delta_m^{c_1})}{2} + \sum_{m=1}^{n_{c_2}} \text{sgn}(v_m^{c_2}) \frac{1 - \text{sgn}(\delta_m^{c_2})}{2} \quad (\text{L35.1})$$

$$\mathcal{W}_2^{\text{gapless}} = \sum_{m=1}^{n_{a_2}} \text{sgn}(v_m^{a_2}) \frac{1 - \text{sgn}(\delta_m^{a_2})}{2} - \sum_{m=1}^{n_{b_1}} \text{sgn}(v_m^{b_1}) \frac{1 - \text{sgn}(\delta_m^{b_1})}{2} + \sum_{m=1}^{n_{c_1}} \text{sgn}(v_m^{c_1}) \frac{1 - \text{sgn}(\delta_m^{c_1})}{2} - \sum_{m=1}^{n_{c_2}} \text{sgn}(v_m^{c_2}) \frac{1 - \text{sgn}(\delta_m^{c_2})}{2} \quad (\text{L35.2})$$

$$\mathcal{W}_1^{\text{gapped}} = - \sum_{m=1}^{n_{c_1}} \text{sgn}(v_m^{c_1}) \frac{1 - \text{sgn}(\delta_m^{c_1})}{2} + \sum_{m=1}^{n_{c_2}} \text{sgn}(v_m^{c_2}) \frac{1 - \text{sgn}(\delta_m^{c_2})}{2} \quad (\text{L35.3})$$

### L36. LAYER GROUP NO. 36

| line segment                            | character of irrep (generators only)                                                                                     |
|-----------------------------------------|--------------------------------------------------------------------------------------------------------------------------|
| $a \ (t, 0, 0)$                         | $\{m_{001}   0 \ \frac{1}{2} \ 0\}$<br>$a_1 \quad -i$<br>$a_2 \quad i$                                                   |
| $b \ (0, t, 0)$                         | $\{2_{010}   0 \ 0 \ 0\} \ \{m_{100}   0 \ \frac{1}{2} \ 0\}$<br>$b_1 \quad 0 \quad 0$                                   |
| $c \ (\frac{t}{2}, 1 - \frac{t}{2}, 0)$ | $\{m_{001}   0 \ \frac{1}{2} \ 0\}$<br>$c_1 \quad -ie^{-\frac{1}{2}i\pi(2-t)}$<br>$c_2 \quad ie^{-\frac{1}{2}i\pi(2-t)}$ |

$$\mathcal{W}_1^{\text{gapless}} = \sum_{m=1}^{n_{a_1}} \text{sgn}(v_m^{a_1}) \frac{1 - \text{sgn}(\delta_m^{a_1})}{2} - \sum_{m=1}^{n_{b_1}} \text{sgn}(v_m^{b_1}) \frac{1 - \text{sgn}(\delta_m^{b_1})}{2} \quad (\text{L36.1})$$

$$\mathcal{W}_2^{\text{gapless}} = \sum_{m=1}^{n_{a_2}} \text{sgn}(v_m^{a_2}) \frac{1 - \text{sgn}(\delta_m^{a_2})}{2} - \sum_{m=1}^{n_{b_1}} \text{sgn}(v_m^{b_1}) \frac{1 - \text{sgn}(\delta_m^{b_1})}{2} \quad (\text{L36.2})$$

$$\mathcal{X}_1 = \sum_{m=1}^{n_{c_1}} \frac{1 - \text{sgn}(\delta_m^{c_1})}{2} + \sum_{m=1}^{n_{c_2}} \frac{1 - \text{sgn}(\delta_m^{c_2})}{2} \mod 2 \quad (\text{L36.3})$$

### L37. LAYER GROUP NO. 37

| line segment                        | character of irrep (generators only) |                                                                                                                         |
|-------------------------------------|--------------------------------------|-------------------------------------------------------------------------------------------------------------------------|
| $a \ (\frac{t}{2}, 0, 0)$           | $a_1$                                | $\begin{Bmatrix} \{2_{100}  0 & 0 & 0 \} \\ 0 \end{Bmatrix} \begin{Bmatrix} \{m_{010}  0 & 0 & 0 \} \\ 0 \end{Bmatrix}$ |
| $b \ (0, \frac{t}{2}, 0)$           | $b_1$                                | $\begin{Bmatrix} \{2_{010}  0 & 0 & 0 \} \\ 0 \end{Bmatrix} \begin{Bmatrix} \{m_{100}  0 & 0 & 0 \} \\ 0 \end{Bmatrix}$ |
| $c \ (\frac{1}{2}, \frac{t}{2}, 0)$ | $c_1$                                | $\begin{Bmatrix} \{2_{010}  0 & 0 & 0 \} \\ 0 \end{Bmatrix} \begin{Bmatrix} \{m_{100}  0 & 0 & 0 \} \\ 0 \end{Bmatrix}$ |
| $d \ (\frac{t}{2}, \frac{1}{2}, 0)$ | $d_1$                                | $\begin{Bmatrix} \{2_{100}  0 & 0 & 0 \} \\ 0 \end{Bmatrix} \begin{Bmatrix} \{m_{010}  0 & 0 & 0 \} \\ 0 \end{Bmatrix}$ |

$$\mathcal{W}_1^{\text{gapless}} = \sum_{m=1}^{n_{a_1}} \text{sgn}(v_m^{a_1}) \frac{1 - \text{sgn}(\delta_m^{a_1})}{2} - \sum_{m=1}^{n_{b_1}} \text{sgn}(v_m^{b_1}) \frac{1 - \text{sgn}(\delta_m^{b_1})}{2} + \sum_{m=1}^{n_{c_1}} \text{sgn}(v_m^{c_1}) \frac{1 - \text{sgn}(\delta_m^{c_1})}{2} - \sum_{m=1}^{n_{d_1}} \text{sgn}(v_m^{d_1}) \frac{1 - \text{sgn}(\delta_m^{d_1})}{2} \quad (\text{L37.1})$$

### L38. LAYER GROUP NO. 38

| line segment                        | character of irrep (generators only) |                                                                                                                                    |
|-------------------------------------|--------------------------------------|------------------------------------------------------------------------------------------------------------------------------------|
| $a \ (\frac{t}{2}, 0, 0)$           | $a_1$                                | $\begin{Bmatrix} \{2_{100}  0 & 0 & 0 \} \\ 0 \end{Bmatrix} \begin{Bmatrix} \{m_{010}  \frac{1}{2} & 0 & 0 \} \\ 0 \end{Bmatrix}$  |
| $b \ (0, \frac{t}{2}, 0)$           | $b_1$                                | $\begin{Bmatrix} \{2_{010}  \frac{1}{2} & 0 & 0 \} \\ 0 \end{Bmatrix} \begin{Bmatrix} \{m_{100}  0 & 0 & 0 \} \\ 0 \end{Bmatrix}$  |
| $c \ (\frac{1}{2}, \frac{t}{2}, 0)$ | $c_1$                                | $\begin{Bmatrix} \{2_{010}  \frac{1}{2} & 0 & 0 \} \\ i \end{Bmatrix} \begin{Bmatrix} \{m_{100}  0 & 0 & 0 \} \\ -i \end{Bmatrix}$ |
|                                     | $c_2$                                | $\begin{Bmatrix} i \end{Bmatrix} \begin{Bmatrix} i \end{Bmatrix}$                                                                  |
|                                     | $c_3$                                | $\begin{Bmatrix} -i \end{Bmatrix} \begin{Bmatrix} -i \end{Bmatrix}$                                                                |
|                                     | $c_4$                                | $\begin{Bmatrix} -i \end{Bmatrix} \begin{Bmatrix} i \end{Bmatrix}$                                                                 |
| $d \ (\frac{t}{2}, \frac{1}{2}, 0)$ | $d_1$                                | $\begin{Bmatrix} \{2_{100}  0 & 0 & 0 \} \\ 0 \end{Bmatrix} \begin{Bmatrix} \{m_{010}  \frac{1}{2} & 0 & 0 \} \\ 0 \end{Bmatrix}$  |

$$\begin{aligned} \mathcal{W}_1^{\text{gapless}} = & \sum_{m=1}^{n_{a_1}} \text{sgn}(v_m^{a_1}) \frac{1 - \text{sgn}(\delta_m^{a_1})}{2} - \sum_{m=1}^{n_{b_1}} \text{sgn}(v_m^{b_1}) \frac{1 - \text{sgn}(\delta_m^{b_1})}{2} + \sum_{m=1}^{n_{c_1}} \text{sgn}(v_m^{c_1}) \frac{1 - \text{sgn}(\delta_m^{c_1})}{2} \\ & + \sum_{m=1}^{n_{c_3}} \text{sgn}(v_m^{c_3}) \frac{1 - \text{sgn}(\delta_m^{c_3})}{2} - \sum_{m=1}^{n_{d_1}} \text{sgn}(v_m^{d_1}) \frac{1 - \text{sgn}(\delta_m^{d_1})}{2} \end{aligned} \quad (\text{L38.1})$$

$$\mathcal{W}_1^{\text{gapped}} = - \sum_{m=1}^{n_{c_1}} \text{sgn}(v_m^{c_1}) \frac{1 - \text{sgn}(\delta_m^{c_1})}{2} + \sum_{m=1}^{n_{c_3}} \text{sgn}(v_m^{c_3}) \frac{1 - \text{sgn}(\delta_m^{c_3})}{2} \quad (\text{L38.2})$$

### L39. LAYER GROUP NO. 39

| line segment                            | character of irrep (generators only) |                                                                                                           |
|-----------------------------------------|--------------------------------------|-----------------------------------------------------------------------------------------------------------|
| $a \quad (\frac{t}{2}, 0, 0)$           | $a_1$                                | $\{2_{100}   0 \quad \frac{1}{2} \quad 0 \quad \} \quad \{m_{010}   \frac{1}{2} \quad 0 \quad 0 \quad \}$ |
| $b \quad (0, \frac{t}{2}, 0)$           | $b_1$                                | $\{2_{010}   \frac{1}{2} \quad 0 \quad 0 \quad \} \quad \{m_{100}   0 \quad \frac{1}{2} \quad 0 \quad \}$ |
| $c \quad (\frac{1}{2}, \frac{t}{2}, 0)$ | $c_1$                                | $\{2_{010}   \frac{1}{2} \quad 0 \quad 0 \quad \} \quad \{m_{100}   0 \quad \frac{1}{2} \quad 0 \quad \}$ |
|                                         | $c_2$                                | $i \quad -ie^{-\frac{1}{2}i\pi t}$                                                                        |
|                                         | $c_3$                                | $-i \quad ie^{-\frac{1}{2}i\pi t}$                                                                        |
|                                         | $c_4$                                | $-i \quad -ie^{-\frac{1}{2}i\pi t}$                                                                       |
| $d \quad (\frac{t}{2}, \frac{1}{2}, 0)$ | $d_1$                                | $\{2_{100}   0 \quad \frac{1}{2} \quad 0 \quad \} \quad \{m_{010}   \frac{1}{2} \quad 0 \quad 0 \quad \}$ |
|                                         | $d_2$                                | $i \quad -ie^{-\frac{1}{2}i\pi t}$                                                                        |
|                                         | $d_3$                                | $-i \quad ie^{-\frac{1}{2}i\pi t}$                                                                        |
|                                         | $d_4$                                | $-i \quad -ie^{-\frac{1}{2}i\pi t}$                                                                       |

$$\begin{aligned} \mathcal{W}_1^{\text{gapless}} = & \sum_{m=1}^{n_{a_1}} \text{sgn}(v_m^{a_1}) \frac{1 - \text{sgn}(\delta_m^{a_1})}{2} - \sum_{m=1}^{n_{b_1}} \text{sgn}(v_m^{b_1}) \frac{1 - \text{sgn}(\delta_m^{b_1})}{2} + \sum_{m=1}^{n_{c_1}} \text{sgn}(v_m^{c_1}) \frac{1 - \text{sgn}(\delta_m^{c_1})}{2} \\ & + \sum_{m=1}^{n_{c_3}} \text{sgn}(v_m^{c_3}) \frac{1 - \text{sgn}(\delta_m^{c_3})}{2} - \sum_{m=1}^{n_{d_1}} \text{sgn}(v_m^{d_1}) \frac{1 - \text{sgn}(\delta_m^{d_1})}{2} - \sum_{m=1}^{n_{d_3}} \text{sgn}(v_m^{d_3}) \frac{1 - \text{sgn}(\delta_m^{d_3})}{2} \end{aligned} \quad (\text{L39.1})$$

$$\mathcal{W}_1^{\text{gapped}} = - \sum_{m=1}^{n_{c_1}} \text{sgn}(v_m^{c_1}) \frac{1 - \text{sgn}(\delta_m^{c_1})}{2} + \sum_{m=1}^{n_{c_3}} \text{sgn}(v_m^{c_3}) \frac{1 - \text{sgn}(\delta_m^{c_3})}{2} \quad (\text{L39.2})$$

$$\mathcal{W}_2^{\text{gapped}} = - \sum_{m=1}^{n_{d_1}} \text{sgn}(v_m^{d_1}) \frac{1 - \text{sgn}(\delta_m^{d_1})}{2} + \sum_{m=1}^{n_{d_3}} \text{sgn}(v_m^{d_3}) \frac{1 - \text{sgn}(\delta_m^{d_3})}{2} \quad (\text{L39.3})$$

**L40. LAYER GROUP NO. 40**

| line segment                        | character of irrep (generators only)                                                                                                                               |
|-------------------------------------|--------------------------------------------------------------------------------------------------------------------------------------------------------------------|
| $a \ (\frac{t}{2}, 0, 0)$           | $a_1 \ \left\{ \begin{matrix} 2_{100}   \frac{1}{2} & 0 & 0 \\ & 0 & \end{matrix} \right\} \ \left\{ m_{010}   \frac{1}{2} & 0 & 0 \\ & 0 & \end{matrix} \right\}$ |
| $b \ (0, \frac{t}{2}, 0)$           | $b_1 \ \left\{ \begin{matrix} 2_{010}   \frac{1}{2} & 0 & 0 \\ & 0 & \end{matrix} \right\} \ \left\{ m_{100}   \frac{1}{2} & 0 & 0 \\ & 0 & \end{matrix} \right\}$ |
| $c \ (\frac{1}{2}, \frac{t}{2}, 0)$ | $c_1 \ \left\{ \begin{matrix} 2_{010}   \frac{1}{2} & 0 & 0 \\ & 0 & \end{matrix} \right\} \ \left\{ m_{100}   \frac{1}{2} & 0 & 0 \\ & 0 & \end{matrix} \right\}$ |
| $d \ (\frac{t}{2}, \frac{1}{2}, 0)$ | $d_1 \ \left\{ \begin{matrix} 2_{100}   \frac{1}{2} & 0 & 0 \\ & 0 & \end{matrix} \right\} \ \left\{ m_{010}   \frac{1}{2} & 0 & 0 \\ & 0 & \end{matrix} \right\}$ |

$$\mathcal{W}_1^{\text{gapless}} = \sum_{m=1}^{n_{a_1}} \text{sgn}(v_m^{a_1}) \frac{1 - \text{sgn}(\delta_m^{a_1})}{2} - \sum_{m=1}^{n_{b_1}} \text{sgn}(v_m^{b_1}) \frac{1 - \text{sgn}(\delta_m^{b_1})}{2} + 2 \sum_{m=1}^{n_{c_1}} \text{sgn}(v_m^{c_1}) \frac{1 - \text{sgn}(\delta_m^{c_1})}{2} - \sum_{m=1}^{n_{d_1}} \text{sgn}(v_m^{d_1}) \frac{1 - \text{sgn}(\delta_m^{d_1})}{2} \quad (\text{L40.1})$$

**L41. LAYER GROUP NO. 41**

| line segment                        | character of irrep (generators only)                                                                                                                      |
|-------------------------------------|-----------------------------------------------------------------------------------------------------------------------------------------------------------|
| $a \ (\frac{t}{2}, 0, 0)$           | $a_1 \ \left\{ \begin{matrix} 2_{100}   \frac{1}{2} & 0 & 0 \\ & 0 & \end{matrix} \right\} \ \left\{ m_{010}   0 & 0 & 0 \\ & 0 & \end{matrix} \right\}$  |
| $b \ (0, \frac{t}{2}, 0)$           | $b_1 \ \left\{ \begin{matrix} 2_{010}   0 & 0 & 0 \\ & 0 & \end{matrix} \right\} \ \left\{ m_{100}   \frac{1}{2} & 0 & 0 \\ & 0 & \end{matrix} \right\}$  |
| $c \ (\frac{1}{2}, \frac{t}{2}, 0)$ | $c_1 \ \left\{ \begin{matrix} 2_{010}   0 & 0 & 0 \\ & -i & \end{matrix} \right\} \ \left\{ m_{100}   \frac{1}{2} & 0 & 0 \\ & i & \end{matrix} \right\}$ |
|                                     | $c_2 \ \left\{ \begin{matrix} & -i & \\ & & -i \end{matrix} \right\}$                                                                                     |
|                                     | $c_3 \ \left\{ \begin{matrix} & i & \\ & & i \end{matrix} \right\}$                                                                                       |
|                                     | $c_4 \ \left\{ \begin{matrix} & i & \\ & & -i \end{matrix} \right\}$                                                                                      |
| $d \ (\frac{t}{2}, \frac{1}{2}, 0)$ | $d_1 \ \left\{ \begin{matrix} 2_{100}   \frac{1}{2} & 0 & 0 \\ & 0 & \end{matrix} \right\} \ \left\{ m_{010}   0 & 0 & 0 \\ & 0 & \end{matrix} \right\}$  |

$$\begin{aligned} \mathcal{W}_1^{\text{gapless}} = & \sum_{m=1}^{n_{a_1}} \text{sgn}(v_m^{a_1}) \frac{1 - \text{sgn}(\delta_m^{a_1})}{2} - \sum_{m=1}^{n_{b_1}} \text{sgn}(v_m^{b_1}) \frac{1 - \text{sgn}(\delta_m^{b_1})}{2} + \sum_{m=1}^{n_{c_1}} \text{sgn}(v_m^{c_1}) \frac{1 - \text{sgn}(\delta_m^{c_1})}{2} \\ & + \sum_{m=1}^{n_{c_2}} \text{sgn}(v_m^{c_2}) \frac{1 - \text{sgn}(\delta_m^{c_2})}{2} - \sum_{m=1}^{n_{d_1}} \text{sgn}(v_m^{d_1}) \frac{1 - \text{sgn}(\delta_m^{d_1})}{2} \end{aligned} \quad (\text{L41.1})$$

$$\mathcal{W}_1^{\text{gapped}} = - \sum_{m=1}^{n_{c_1}} \text{sgn}(v_m^{c_1}) \frac{1 - \text{sgn}(\delta_m^{c_1})}{2} + \sum_{m=1}^{n_{c_2}} \text{sgn}(v_m^{c_2}) \frac{1 - \text{sgn}(\delta_m^{c_2})}{2} \quad (\text{L41.2})$$

**L42. LAYER GROUP NO. 42**

| line segment | character of irrep (generators only) |
|--------------|--------------------------------------|
|--------------|--------------------------------------|

|                                         |       |                                                                                                                        |
|-----------------------------------------|-------|------------------------------------------------------------------------------------------------------------------------|
| $a \quad (\frac{t}{2}, 0, 0)$           | $a_1$ | $\{2_{100}   0 \ 0 \ 0 \} \quad \{m_{010}   \frac{1}{2} \ \frac{1}{2} \ 0 \}$<br>0                                     |
| $b \quad (0, \frac{t}{2}, 0)$           | $b_1$ | $\{2_{010}   \frac{1}{2} \ \frac{1}{2} \ 0 \} \quad \{m_{100}   0 \ 0 \ 0 \}$<br>0                                     |
| $c \quad (\frac{1}{2}, \frac{t}{2}, 0)$ | $c_1$ | $\{2_{010}   \frac{1}{2} \ \frac{1}{2} \ 0 \} \quad \{m_{100}   0 \ 0 \ 0 \}$<br>$-e^{-\frac{1}{2}i\pi(t+1)} \quad -i$ |
|                                         | $c_2$ | $-e^{-\frac{1}{2}i\pi(t+1)} \quad i$                                                                                   |
|                                         | $c_3$ | $e^{-\frac{1}{2}i\pi(t+1)} \quad -i$                                                                                   |
|                                         | $c_4$ | $e^{-\frac{1}{2}i\pi(t+1)} \quad i$                                                                                    |
| $d \quad (\frac{t}{2}, \frac{1}{2}, 0)$ | $d_1$ | $\{2_{100}   0 \ 0 \ 0 \} \quad \{m_{010}   \frac{1}{2} \ \frac{1}{2} \ 0 \}$<br>$-i \quad -e^{-\frac{1}{2}i\pi(t+1)}$ |
|                                         | $d_2$ | $-i \quad e^{-\frac{1}{2}i\pi(t+1)}$                                                                                   |
|                                         | $d_3$ | $i \quad -e^{-\frac{1}{2}i\pi(t+1)}$                                                                                   |
|                                         | $d_4$ | $i \quad e^{-\frac{1}{2}i\pi(t+1)}$                                                                                    |

$$\begin{aligned} \mathcal{W}_1^{\text{gapless}} = & \sum_{m=1}^{n_{a_1}} \text{sgn}(v_m^{a_1}) \frac{1 - \text{sgn}(\delta_m^{a_1})}{2} - \sum_{m=1}^{n_{b_1}} \text{sgn}(v_m^{b_1}) \frac{1 - \text{sgn}(\delta_m^{b_1})}{2} + \sum_{m=1}^{n_{c_1}} \text{sgn}(v_m^{c_1}) \frac{1 - \text{sgn}(\delta_m^{c_1})}{2} \\ & + \sum_{m=1}^{n_{c_3}} \text{sgn}(v_m^{c_3}) \frac{1 - \text{sgn}(\delta_m^{c_3})}{2} - \sum_{m=1}^{n_{d_1}} \text{sgn}(v_m^{d_1}) \frac{1 - \text{sgn}(\delta_m^{d_1})}{2} - \sum_{m=1}^{n_{d_2}} \text{sgn}(v_m^{d_2}) \frac{1 - \text{sgn}(\delta_m^{d_2})}{2} \end{aligned} \quad (\text{L42.1})$$

$$\mathcal{X}_1 = \sum_{m=1}^{n_{c_1}} \frac{1 - \text{sgn}(\delta_m^{c_1})}{2} + \sum_{m=1}^{n_{c_3}} \frac{1 - \text{sgn}(\delta_m^{c_3})}{2} + \sum_{m=1}^{n_{d_1}} \frac{1 - \text{sgn}(\delta_m^{d_1})}{2} + \sum_{m=1}^{n_{d_2}} \frac{1 - \text{sgn}(\delta_m^{d_2})}{2} \pmod{2} \quad (\text{L42.2})$$

#### L43. LAYER GROUP NO. 43

| line segment                            | character of irrep (generators only) |                                                                                                                                                        |
|-----------------------------------------|--------------------------------------|--------------------------------------------------------------------------------------------------------------------------------------------------------|
| $a \quad (\frac{t}{2}, 0, 0)$           | $a_1$                                | $\{2_{100}   0 \ \frac{1}{2} \ 0 \} \quad \{m_{010}   \frac{1}{2} \ \frac{1}{2} \ 0 \}$<br>0                                                           |
| $b \quad (0, \frac{t}{2}, 0)$           | $b_1$                                | $\{2_{010}   \frac{1}{2} \ \frac{1}{2} \ 0 \} \quad \{m_{100}   0 \ \frac{1}{2} \ 0 \}$<br>0                                                           |
| $c \quad (\frac{1}{2}, \frac{t}{2}, 0)$ | $c_1$                                | $\{2_{010}   \frac{1}{2} \ \frac{1}{2} \ 0 \} \quad \{m_{100}   0 \ \frac{1}{2} \ 0 \}$<br>$-e^{-\frac{1}{2}i\pi(t+1)} \quad -ie^{-\frac{1}{2}i\pi t}$ |
|                                         | $c_2$                                | $-e^{-\frac{1}{2}i\pi(t+1)} \quad ie^{-\frac{1}{2}i\pi t}$                                                                                             |
|                                         | $c_3$                                | $e^{-\frac{1}{2}i\pi(t+1)} \quad -ie^{-\frac{1}{2}i\pi t}$                                                                                             |
|                                         | $c_4$                                | $e^{-\frac{1}{2}i\pi(t+1)} \quad ie^{-\frac{1}{2}i\pi t}$                                                                                              |
| $d \quad (\frac{t}{2}, \frac{1}{2}, 0)$ | $d_1$                                | $\{2_{100}   0 \ \frac{1}{2} \ 0 \} \quad \{m_{010}   \frac{1}{2} \ \frac{1}{2} \ 0 \}$<br>0                                                           |

$$\begin{aligned} \mathcal{W}_1^{\text{gapless}} = & \sum_{m=1}^{n_{a_1}} \text{sgn}(v_m^{a_1}) \frac{1 - \text{sgn}(\delta_m^{a_1})}{2} - \sum_{m=1}^{n_{b_1}} \text{sgn}(v_m^{b_1}) \frac{1 - \text{sgn}(\delta_m^{b_1})}{2} + \sum_{m=1}^{n_{c_1}} \text{sgn}(v_m^{c_1}) \frac{1 - \text{sgn}(\delta_m^{c_1})}{2} \\ & + \sum_{m=1}^{n_{c_3}} \text{sgn}(v_m^{c_3}) \frac{1 - \text{sgn}(\delta_m^{c_3})}{2} - 2 \sum_{m=1}^{n_{d_1}} \text{sgn}(v_m^{d_1}) \frac{1 - \text{sgn}(\delta_m^{d_1})}{2} \end{aligned} \quad (\text{L43.1})$$

$$\mathcal{X}_1 = \sum_{m=1}^{n_{c_1}} \frac{1 - \text{sgn}(\delta_m^{c_1})}{2} + \sum_{m=1}^{n_{c_3}} \frac{1 - \text{sgn}(\delta_m^{c_3})}{2} \pmod{2} \quad (\text{L43.2})$$

**L44. LAYER GROUP NO. 44**

| line segment                            | character of irrep (generators only)                                                                                                                                                            |
|-----------------------------------------|-------------------------------------------------------------------------------------------------------------------------------------------------------------------------------------------------|
| $a \quad (\frac{t}{2}, 0, 0)$           | $a_1 \quad \left\{ \begin{matrix} 2_{100}   \frac{1}{2} & \frac{1}{2} & 0 \\ 0 \end{matrix} \right\} \left\{ \begin{matrix} m_{010}   \frac{1}{2} & \frac{1}{2} & 0 \\ 0 \end{matrix} \right\}$ |
| $b \quad (0, \frac{t}{2}, 0)$           | $b_1 \quad \left\{ \begin{matrix} 2_{010}   \frac{1}{2} & \frac{1}{2} & 0 \\ 0 \end{matrix} \right\} \left\{ \begin{matrix} m_{100}   \frac{1}{2} & \frac{1}{2} & 0 \\ 0 \end{matrix} \right\}$ |
| $c \quad (\frac{1}{2}, \frac{t}{2}, 0)$ | $c_1 \quad \left\{ \begin{matrix} 2_{010}   \frac{1}{2} & \frac{1}{2} & 0 \\ 0 \end{matrix} \right\} \left\{ \begin{matrix} m_{100}   \frac{1}{2} & \frac{1}{2} & 0 \\ 0 \end{matrix} \right\}$ |
| $d \quad (\frac{t}{2}, \frac{1}{2}, 0)$ | $d_1 \quad \left\{ \begin{matrix} 2_{100}   \frac{1}{2} & \frac{1}{2} & 0 \\ 0 \end{matrix} \right\} \left\{ \begin{matrix} m_{010}   \frac{1}{2} & \frac{1}{2} & 0 \\ 0 \end{matrix} \right\}$ |

$$\begin{aligned} \mathcal{W}_1^{\text{gapless}} = & \sum_{m=1}^{n_{a_1}} \text{sgn}(v_m^{a_1}) \frac{1 - \text{sgn}(\delta_m^{a_1})}{2} - \sum_{m=1}^{n_{b_1}} \text{sgn}(v_m^{b_1}) \frac{1 - \text{sgn}(\delta_m^{b_1})}{2} + 2 \sum_{m=1}^{n_{c_1}} \text{sgn}(v_m^{c_1}) \frac{1 - \text{sgn}(\delta_m^{c_1})}{2} \\ & - 2 \sum_{m=1}^{n_{d_1}} \text{sgn}(v_m^{d_1}) \frac{1 - \text{sgn}(\delta_m^{d_1})}{2} \end{aligned} \quad (\text{L44.1})$$

**L45. LAYER GROUP NO. 45**

| line segment                            | character of irrep (generators only)                                                                                                                                                                                                          |
|-----------------------------------------|-----------------------------------------------------------------------------------------------------------------------------------------------------------------------------------------------------------------------------------------------|
| $a \quad (\frac{t}{2}, 0, 0)$           | $a_1 \quad \left\{ \begin{matrix} 2_{100}   \frac{1}{2} & \frac{1}{2} & 0 \\ 0 \end{matrix} \right\} \left\{ \begin{matrix} m_{010}   0 & \frac{1}{2} & 0 \\ 0 \end{matrix} \right\}$                                                         |
| $b \quad (0, \frac{t}{2}, 0)$           | $b_1 \quad \left\{ \begin{matrix} 2_{010}   0 & \frac{1}{2} & 0 \\ 0 \end{matrix} \right\} \left\{ \begin{matrix} m_{100}   \frac{1}{2} & \frac{1}{2} & 0 \\ 0 \end{matrix} \right\}$                                                         |
| $c \quad (\frac{1}{2}, \frac{t}{2}, 0)$ | $c_1 \quad \left\{ \begin{matrix} 2_{010}   0 & \frac{1}{2} & 0 \\ -ie^{-\frac{1}{2}i\pi t} & & -e^{-\frac{1}{2}i\pi(t+1)} \end{matrix} \right\} \left\{ \begin{matrix} m_{100}   \frac{1}{2} & \frac{1}{2} & 0 \\ & & \end{matrix} \right\}$ |
|                                         | $c_2 \quad \left\{ \begin{matrix} & & \\ -ie^{-\frac{1}{2}i\pi t} & & e^{-\frac{1}{2}i\pi(t+1)} \end{matrix} \right\}$                                                                                                                        |
|                                         | $c_3 \quad \left\{ \begin{matrix} & & \\ & & -e^{-\frac{1}{2}i\pi(t+1)} \end{matrix} \right\}$                                                                                                                                                |
|                                         | $c_4 \quad \left\{ \begin{matrix} & & \\ & & e^{-\frac{1}{2}i\pi(t+1)} \end{matrix} \right\}$                                                                                                                                                 |
| $d \quad (\frac{t}{2}, \frac{1}{2}, 0)$ | $d_1 \quad \left\{ \begin{matrix} 2_{100}   \frac{1}{2} & \frac{1}{2} & 0 \\ 0 \end{matrix} \right\} \left\{ \begin{matrix} m_{010}   0 & \frac{1}{2} & 0 \\ 0 \end{matrix} \right\}$                                                         |

$$\begin{aligned} \mathcal{W}_1^{\text{gapless}} = & \sum_{m=1}^{n_{a_1}} \text{sgn}(v_m^{a_1}) \frac{1 - \text{sgn}(\delta_m^{a_1})}{2} - \sum_{m=1}^{n_{b_1}} \text{sgn}(v_m^{b_1}) \frac{1 - \text{sgn}(\delta_m^{b_1})}{2} + \sum_{m=1}^{n_{c_1}} \text{sgn}(v_m^{c_1}) \frac{1 - \text{sgn}(\delta_m^{c_1})}{2} \\ & + \sum_{m=1}^{n_{c_2}} \text{sgn}(v_m^{c_2}) \frac{1 - \text{sgn}(\delta_m^{c_2})}{2} - 2 \sum_{m=1}^{n_{d_1}} \text{sgn}(v_m^{d_1}) \frac{1 - \text{sgn}(\delta_m^{d_1})}{2} \end{aligned} \quad (\text{L45.1})$$

$$\mathcal{X}_1 = \sum_{m=1}^{n_{c_1}} \frac{1 - \text{sgn}(\delta_m^{c_1})}{2} + \sum_{m=1}^{n_{c_2}} \frac{1 - \text{sgn}(\delta_m^{c_2})}{2} \quad \text{mod } 2 \quad (\text{L45.2})$$

**L46. LAYER GROUP NO. 46**

| line segment | character of irrep (generators only) |
|--------------|--------------------------------------|
|--------------|--------------------------------------|

|                                         |       |                                        |                                        |
|-----------------------------------------|-------|----------------------------------------|----------------------------------------|
| $a \quad (\frac{t}{2}, 0, 0)$           | $a_1$ | $\{2_{100}   \frac{1}{2} \ 0 \ 0 \ \}$ | $\{m_{010}   0 \ \frac{1}{2} \ 0 \ \}$ |
| $b \quad (0, \frac{t}{2}, 0)$           | $b_1$ | $\{2_{010}   0 \ \frac{1}{2} \ 0 \ \}$ | $\{m_{100}   \frac{1}{2} \ 0 \ 0 \ \}$ |
| $c \quad (\frac{1}{2}, \frac{t}{2}, 0)$ | $c_1$ | $\{2_{010}   0 \ \frac{1}{2} \ 0 \ \}$ | $\{m_{100}   \frac{1}{2} \ 0 \ 0 \ \}$ |
|                                         |       | $-ie^{-\frac{1}{2}i\pi t}$             | $i$                                    |
|                                         | $c_2$ | $-ie^{-\frac{1}{2}i\pi t}$             | $-i$                                   |
|                                         | $c_3$ | $ie^{-\frac{1}{2}i\pi t}$              | $i$                                    |
| $d \quad (\frac{t}{2}, \frac{1}{2}, 0)$ | $c_4$ | $ie^{-\frac{1}{2}i\pi t}$              | $-i$                                   |
|                                         |       | $\{2_{100}   \frac{1}{2} \ 0 \ 0 \ \}$ | $\{m_{010}   0 \ \frac{1}{2} \ 0 \ \}$ |
|                                         | $d_1$ | $-ie^{-\frac{1}{2}i\pi t}$             | $i$                                    |
|                                         | $d_2$ | $-ie^{-\frac{1}{2}i\pi t}$             | $-i$                                   |
|                                         | $d_3$ | $ie^{-\frac{1}{2}i\pi t}$              | $i$                                    |
|                                         | $d_4$ | $ie^{-\frac{1}{2}i\pi t}$              | $-i$                                   |

$$\begin{aligned} \mathcal{W}_1^{\text{gapless}} = & \sum_{m=1}^{n_{a_1}} \text{sgn}(v_m^{a_1}) \frac{1 - \text{sgn}(\delta_m^{a_1})}{2} - \sum_{m=1}^{n_{b_1}} \text{sgn}(v_m^{b_1}) \frac{1 - \text{sgn}(\delta_m^{b_1})}{2} + \sum_{m=1}^{n_{c_1}} \text{sgn}(v_m^{c_1}) \frac{1 - \text{sgn}(\delta_m^{c_1})}{2} \\ & + \sum_{m=1}^{n_{c_2}} \text{sgn}(v_m^{c_2}) \frac{1 - \text{sgn}(\delta_m^{c_2})}{2} - \sum_{m=1}^{n_{d_1}} \text{sgn}(v_m^{d_1}) \frac{1 - \text{sgn}(\delta_m^{d_1})}{2} - \sum_{m=1}^{n_{d_2}} \text{sgn}(v_m^{d_2}) \frac{1 - \text{sgn}(\delta_m^{d_2})}{2} \end{aligned} \quad (\text{L46.1})$$

$$\mathcal{W}_1^{\text{gapped}} = - \sum_{m=1}^{n_{c_1}} \text{sgn}(v_m^{c_1}) \frac{1 - \text{sgn}(\delta_m^{c_1})}{2} + \sum_{m=1}^{n_{c_2}} \text{sgn}(v_m^{c_2}) \frac{1 - \text{sgn}(\delta_m^{c_2})}{2} \quad (\text{L46.2})$$

$$\mathcal{W}_2^{\text{gapped}} = - \sum_{m=1}^{n_{d_1}} \text{sgn}(v_m^{d_1}) \frac{1 - \text{sgn}(\delta_m^{d_1})}{2} + \sum_{m=1}^{n_{d_2}} \text{sgn}(v_m^{d_2}) \frac{1 - \text{sgn}(\delta_m^{d_2})}{2} \quad (\text{L46.3})$$

#### L47. LAYER GROUP NO. 47

| line segment                                | character of irrep (generators only) |                                                           |
|---------------------------------------------|--------------------------------------|-----------------------------------------------------------|
| $a \quad (t, 0, 0)$                         | $a_1$                                | $\{2_{100}   0 \ 0 \ 0 \ \}$ $\{m_{010}   0 \ 0 \ 0 \ \}$ |
|                                             |                                      | $0$ $0$                                                   |
| $b \quad (0, t, 0)$                         | $b_1$                                | $\{2_{010}   0 \ 0 \ 0 \ \}$ $\{m_{100}   0 \ 0 \ 0 \ \}$ |
|                                             |                                      | $0$ $0$                                                   |
| $c \quad (\frac{t}{2}, 1 - \frac{t}{2}, 0)$ | $c_1$                                | $\{m_{001}   0 \ 0 \ 0 \ \}$                              |
|                                             | $c_2$                                | $-i$                                                      |
|                                             |                                      | $i$                                                       |

$$\mathcal{W}_1^{\text{gapless}} = \sum_{m=1}^{n_{a_1}} \text{sgn}(v_m^{a_1}) \frac{1 - \text{sgn}(\delta_m^{a_1})}{2} - \sum_{m=1}^{n_{b_1}} \text{sgn}(v_m^{b_1}) \frac{1 - \text{sgn}(\delta_m^{b_1})}{2} \quad (\text{L47.1})$$



**L48. LAYER GROUP NO. 48**

| line segment                            | character of irrep (generators only)                                                                                                    |
|-----------------------------------------|-----------------------------------------------------------------------------------------------------------------------------------------|
| $a \ (t, 0, 0)$                         | $a_1 \begin{array}{c} \{2_{100}   0 \ 0 \ 0\} \\ 0 \end{array} \ \{m_{010}   \frac{1}{2} \ 0 \ 0\}$                                     |
| $b \ (0, t, 0)$                         | $b_1 \begin{array}{c} \{2_{010}   \frac{1}{2} \ 0 \ 0\} \\ 0 \end{array} \ \{m_{100}   0 \ 0 \ 0\}$                                     |
| $c \ (\frac{t}{2}, 1 - \frac{t}{2}, 0)$ | $c_1 \begin{array}{c} \{m_{001}   \frac{1}{2} \ 0 \ 0\} \\ -ie^{-\frac{1}{2}i\pi t} \end{array}$<br>$c_2 \quad ie^{-\frac{1}{2}i\pi t}$ |

$$\mathcal{W}_1^{\text{gapless}} = \sum_{m=1}^{n_{a_1}} \text{sgn}(v_m^{a_1}) \frac{1 - \text{sgn}(\delta_m^{a_1})}{2} - \sum_{m=1}^{n_{b_1}} \text{sgn}(v_m^{b_1}) \frac{1 - \text{sgn}(\delta_m^{b_1})}{2} \quad (\text{L48.1})$$

**L49. LAYER GROUP NO. 49**

| line segment                        | character of irrep (generators only)                      |
|-------------------------------------|-----------------------------------------------------------|
| $a \ (\frac{t}{2}, 0, 0)$           | $a_1 \begin{array}{c} \{1   0 \ 0 \ 0\} \\ 1 \end{array}$ |
| $b \ (\frac{1}{2}, \frac{t}{2}, 0)$ | $b_1 \begin{array}{c} \{1   0 \ 0 \ 0\} \\ 1 \end{array}$ |

$$\mathcal{X}_1 = \sum_{m=1}^{n_{a_1}} \frac{1 - \text{sgn}(\delta_m^{a_1})}{2} + \sum_{m=1}^{n_{b_1}} \frac{1 - \text{sgn}(\delta_m^{b_1})}{2} \quad \text{mod } 2 \quad (\text{L49.1})$$

$$\mathcal{X}_2 = \sum_{m=1}^{n_{b_1}} \frac{1 - \text{sgn}(\delta_m^{b_1})}{2} \quad \text{mod } 2 \quad (\text{L49.2})$$

**L50. LAYER GROUP NO. 50**

| line segment                        | character of irrep (generators only)                      |
|-------------------------------------|-----------------------------------------------------------|
| $a \ (\frac{t}{2}, 0, 0)$           | $a_1 \begin{array}{c} \{1   0 \ 0 \ 0\} \\ 1 \end{array}$ |
| $b \ (\frac{1}{2}, \frac{t}{2}, 0)$ | $b_1 \begin{array}{c} \{1   0 \ 0 \ 0\} \\ 1 \end{array}$ |

$$\mathcal{X}_1 = \sum_{m=1}^{n_{a_1}} \frac{1 - \text{sgn}(\delta_m^{a_1})}{2} + \sum_{m=1}^{n_{b_1}} \frac{1 - \text{sgn}(\delta_m^{b_1})}{2} \quad \text{mod } 2 \quad (\text{L50.1})$$

$$\mathcal{X}_2 = \sum_{m=1}^{n_{b_1}} \frac{1 - \text{sgn}(\delta_m^{b_1})}{2} \quad \text{mod } 2 \quad (\text{L50.2})$$

**L51. LAYER GROUP NO. 51**

| line segment                            | character of irrep (generators only)                         |
|-----------------------------------------|--------------------------------------------------------------|
| $a \quad (\frac{t}{2}, 0, 0)$           | $\{m_{001}   0 \ 0 \ 0\}$<br>$a_1 \quad -i$<br>$a_2 \quad i$ |
| $b \quad (\frac{1}{2}, \frac{t}{2}, 0)$ | $\{m_{001}   0 \ 0 \ 0\}$<br>$b_1 \quad -i$<br>$b_2 \quad i$ |

**L52. LAYER GROUP NO. 52**

| line segment                            | character of irrep (generators only)                                                                                               |
|-----------------------------------------|------------------------------------------------------------------------------------------------------------------------------------|
| $a \quad (\frac{t}{2}, 0, 0)$           | $\{m_{001}   \frac{1}{2} \ \frac{1}{2} \ 0\}$<br>$a_1 \quad -ie^{-\frac{1}{2}i\pi t}$<br>$a_2 \quad ie^{-\frac{1}{2}i\pi t}$       |
| $b \quad (\frac{1}{2}, \frac{t}{2}, 0)$ | $\{m_{001}   \frac{1}{2} \ \frac{1}{2} \ 0\}$<br>$b_1 \quad -ie^{-\frac{1}{2}i\pi(t+1)}$<br>$b_2 \quad ie^{-\frac{1}{2}i\pi(t+1)}$ |

$$\mathcal{X}_1 = \sum_{m=1}^{n_{b_1}} \frac{1 - \text{sgn}(\delta_m^{b_1})}{2} \mod 2 \quad (\text{L52.1})$$

**L53. LAYER GROUP NO. 53**

| line segment                              | character of irrep (generators only)                         |
|-------------------------------------------|--------------------------------------------------------------|
| $a \quad (0, \frac{t}{2}, 0)$             | $\{2_{010}   0 \ 0 \ 0\}$<br>$a_1 \quad -i$<br>$a_2 \quad i$ |
| $b \quad (\frac{1-t}{2}, \frac{1}{2}, 0)$ | $\{2_{100}   0 \ 0 \ 0\}$<br>$b_1 \quad -i$<br>$b_2 \quad i$ |
| $c \quad (\frac{t}{2}, \frac{t}{2}, 0)$   | $\{2_{110}   0 \ 0 \ 0\}$<br>$c_1 \quad -i$<br>$c_2 \quad i$ |

$$\begin{aligned} \mathcal{W}_1^{\text{gapless}} = & \sum_{m=1}^{n_{a_1}} \text{sgn}(v_m^{a_1}) \frac{1 - \text{sgn}(\delta_m^{a_1})}{2} + \sum_{m=1}^{n_{a_2}} \text{sgn}(v_m^{a_2}) \frac{1 - \text{sgn}(\delta_m^{a_2})}{2} - \sum_{m=1}^{n_{b_1}} \text{sgn}(v_m^{b_1}) \frac{1 - \text{sgn}(\delta_m^{b_1})}{2} \\ & - \sum_{m=1}^{n_{b_2}} \text{sgn}(v_m^{b_2}) \frac{1 - \text{sgn}(\delta_m^{b_2})}{2} - \sum_{m=1}^{n_{c_1}} \text{sgn}(v_m^{c_1}) \frac{1 - \text{sgn}(\delta_m^{c_1})}{2} - \sum_{m=1}^{n_{c_2}} \text{sgn}(v_m^{c_2}) \frac{1 - \text{sgn}(\delta_m^{c_2})}{2} \end{aligned} \quad (\text{L53.1})$$

$$\mathcal{W}_1^{\text{gapped}} = - \sum_{m=1}^{n_{b_1}} \text{sgn}(v_m^{b_1}) \frac{1 - \text{sgn}(\delta_m^{b_1})}{2} + \sum_{m=1}^{n_{b_2}} \text{sgn}(v_m^{b_2}) \frac{1 - \text{sgn}(\delta_m^{b_2})}{2} \quad (\text{L53.2})$$

$$\mathcal{W}_2^{\text{gapped}} = - \sum_{m=1}^{n_{a_2}} \text{sgn}(v_m^{a_2}) \frac{1 - \text{sgn}(\delta_m^{a_2})}{2} + \sum_{m=1}^{n_{b_1}} \text{sgn}(v_m^{b_1}) \frac{1 - \text{sgn}(\delta_m^{b_1})}{2} + \sum_{m=1}^{n_{c_1}} \text{sgn}(v_m^{c_1}) \frac{1 - \text{sgn}(\delta_m^{c_1})}{2} \quad (\text{L53.3})$$

$$\mathcal{W}_3^{\text{gapped}} = - \sum_{m=1}^{n_{a_2}} \text{sgn}(v_m^{a_2}) \frac{1 - \text{sgn}(\delta_m^{a_2})}{2} + \sum_{m=1}^{n_{b_1}} \text{sgn}(v_m^{b_1}) \frac{1 - \text{sgn}(\delta_m^{b_1})}{2} + \sum_{m=1}^{n_{c_2}} \text{sgn}(v_m^{c_2}) \frac{1 - \text{sgn}(\delta_m^{c_2})}{2} \quad (\text{L53.4})$$

#### L54. LAYER GROUP NO. 54

| line segment                              | character of irrep (generators only)                                                                                         |
|-------------------------------------------|------------------------------------------------------------------------------------------------------------------------------|
| $a \quad (0, \frac{t}{2}, 0)$             | $\{2_{010}   \frac{1}{2} \frac{1}{2} 0\}$<br>$a_1 \quad -ie^{-\frac{1}{2}i\pi t}$<br>$a_2 \quad ie^{-\frac{1}{2}i\pi t}$     |
| $b \quad (\frac{1-t}{2}, \frac{1}{2}, 0)$ | $\{2_{100}   \frac{1}{2} \frac{1}{2} 0\}$<br>$b_1 \quad -e^{-\frac{1}{2}i\pi(2-t)}$<br>$b_2 \quad e^{-\frac{1}{2}i\pi(2-t)}$ |
| $c \quad (\frac{t}{2}, \frac{t}{2}, 0)$   | $\{2_{110}   0 \ 0 \ 0\}$<br>$c_1 \quad -i$<br>$c_2 \quad i$                                                                 |

$$\begin{aligned} \mathcal{W}_1^{\text{gapless}} = & \sum_{m=1}^{n_{a_1}} \text{sgn}(v_m^{a_1}) \frac{1 - \text{sgn}(\delta_m^{a_1})}{2} + \sum_{m=1}^{n_{a_2}} \text{sgn}(v_m^{a_2}) \frac{1 - \text{sgn}(\delta_m^{a_2})}{2} - 2 \sum_{m=1}^{n_{b_1}} \text{sgn}(v_m^{b_1}) \frac{1 - \text{sgn}(\delta_m^{b_1})}{2} \\ & - \sum_{m=1}^{n_{c_1}} \text{sgn}(v_m^{c_1}) \frac{1 - \text{sgn}(\delta_m^{c_1})}{2} - \sum_{m=1}^{n_{c_2}} \text{sgn}(v_m^{c_2}) \frac{1 - \text{sgn}(\delta_m^{c_2})}{2} \end{aligned} \quad (\text{L54.1})$$

$$\mathcal{W}_1^{\text{gapped}} = - \sum_{m=1}^{n_{c_1}} \text{sgn}(v_m^{c_1}) \frac{1 - \text{sgn}(\delta_m^{c_1})}{2} + \sum_{m=1}^{n_{c_2}} \text{sgn}(v_m^{c_2}) \frac{1 - \text{sgn}(\delta_m^{c_2})}{2} \quad (\text{L54.2})$$

$$\mathcal{X}_1 = \sum_{m=1}^{n_{a_2}} \frac{1 - \text{sgn}(\delta_m^{a_2})}{2} + \sum_{m=1}^{n_{c_1}} \frac{1 - \text{sgn}(\delta_m^{c_1})}{2} \quad \text{mod } 2 \quad (\text{L54.3})$$

#### L55. LAYER GROUP NO. 55

| line segment                              | character of irrep (generators only)                          |
|-------------------------------------------|---------------------------------------------------------------|
| $a \quad (0, \frac{t}{2}, 0)$             | $\{m_{100}   0 \ 0 \ 0\}$<br>$a_1 \quad -i$<br>$a_2 \quad i$  |
| $b \quad (\frac{1-t}{2}, \frac{1}{2}, 0)$ | $\{m_{010}   0 \ 0 \ 0\}$<br>$b_1 \quad -i$<br>$b_2 \quad i$  |
| $c \quad (\frac{t}{2}, \frac{t}{2}, 0)$   | $\{m_{1-10}   0 \ 0 \ 0\}$<br>$c_1 \quad -i$<br>$c_2 \quad i$ |

$$\begin{aligned} \mathcal{W}_1^{\text{gapless}} = & \sum_{m=1}^{n_{a_1}} \text{sgn}(v_m^{a_1}) \frac{1 - \text{sgn}(\delta_m^{a_1})}{2} + \sum_{m=1}^{n_{a_2}} \text{sgn}(v_m^{a_2}) \frac{1 - \text{sgn}(\delta_m^{a_2})}{2} - \sum_{m=1}^{n_{b_1}} \text{sgn}(v_m^{b_1}) \frac{1 - \text{sgn}(\delta_m^{b_1})}{2} \\ & - \sum_{m=1}^{n_{b_2}} \text{sgn}(v_m^{b_2}) \frac{1 - \text{sgn}(\delta_m^{b_2})}{2} - \sum_{m=1}^{n_{c_1}} \text{sgn}(v_m^{c_1}) \frac{1 - \text{sgn}(\delta_m^{c_1})}{2} - \sum_{m=1}^{n_{c_2}} \text{sgn}(v_m^{c_2}) \frac{1 - \text{sgn}(\delta_m^{c_2})}{2} \end{aligned} \quad (\text{L55.1})$$

$$\mathcal{W}_1^{\text{gapped}} = - \sum_{m=1}^{n_{b_1}} \text{sgn}(v_m^{b_1}) \frac{1 - \text{sgn}(\delta_m^{b_1})}{2} + \sum_{m=1}^{n_{b_2}} \text{sgn}(v_m^{b_2}) \frac{1 - \text{sgn}(\delta_m^{b_2})}{2} \quad (\text{L55.2})$$

$$\mathcal{W}_2^{\text{gapped}} = - \sum_{m=1}^{n_{a_2}} \text{sgn}(v_m^{a_2}) \frac{1 - \text{sgn}(\delta_m^{a_2})}{2} + \sum_{m=1}^{n_{b_1}} \text{sgn}(v_m^{b_1}) \frac{1 - \text{sgn}(\delta_m^{b_1})}{2} + \sum_{m=1}^{n_{c_1}} \text{sgn}(v_m^{c_1}) \frac{1 - \text{sgn}(\delta_m^{c_1})}{2} \quad (\text{L55.3})$$

$$\mathcal{W}_3^{\text{gapped}} = - \sum_{m=1}^{n_{a_2}} \text{sgn}(v_m^{a_2}) \frac{1 - \text{sgn}(\delta_m^{a_2})}{2} + \sum_{m=1}^{n_{b_1}} \text{sgn}(v_m^{b_1}) \frac{1 - \text{sgn}(\delta_m^{b_1})}{2} + \sum_{m=1}^{n_{c_2}} \text{sgn}(v_m^{c_2}) \frac{1 - \text{sgn}(\delta_m^{c_2})}{2} \quad (\text{L55.4})$$

#### L56. LAYER GROUP NO. 56

| line segment                              | character of irrep (generators only)                                                                                         |
|-------------------------------------------|------------------------------------------------------------------------------------------------------------------------------|
| $a \quad (0, \frac{t}{2}, 0)$             | $\{m_{100}   \frac{1}{2} \frac{1}{2} 0\}$<br>$a_1 \quad -ie^{-\frac{1}{2}i\pi t}$<br>$a_2 \quad ie^{-\frac{1}{2}i\pi t}$     |
| $b \quad (\frac{1-t}{2}, \frac{1}{2}, 0)$ | $\{m_{010}   \frac{1}{2} \frac{1}{2} 0\}$<br>$b_1 \quad -e^{-\frac{1}{2}i\pi(2-t)}$<br>$b_2 \quad e^{-\frac{1}{2}i\pi(2-t)}$ |
| $c \quad (\frac{t}{2}, \frac{t}{2}, 0)$   | $\{m_{1-10}   \frac{1}{2} \frac{1}{2} 0\}$<br>$c_1 \quad -ie^{-i\pi t}$<br>$c_2 \quad ie^{-i\pi t}$                          |

$$\begin{aligned} \mathcal{W}_1^{\text{gapless}} = & \sum_{m=1}^{n_{a_1}} \text{sgn}(v_m^{a_1}) \frac{1 - \text{sgn}(\delta_m^{a_1})}{2} + \sum_{m=1}^{n_{a_2}} \text{sgn}(v_m^{a_2}) \frac{1 - \text{sgn}(\delta_m^{a_2})}{2} - 2 \sum_{m=1}^{n_{b_1}} \text{sgn}(v_m^{b_1}) \frac{1 - \text{sgn}(\delta_m^{b_1})}{2} \\ & - \sum_{m=1}^{n_{c_1}} \text{sgn}(v_m^{c_1}) \frac{1 - \text{sgn}(\delta_m^{c_1})}{2} - \sum_{m=1}^{n_{c_2}} \text{sgn}(v_m^{c_2}) \frac{1 - \text{sgn}(\delta_m^{c_2})}{2} \end{aligned} \quad (\text{L56.1})$$

$$\mathcal{W}_1^{\text{gapped}} = - \sum_{m=1}^{n_{c_1}} \text{sgn}(v_m^{c_1}) \frac{1 - \text{sgn}(\delta_m^{c_1})}{2} + \sum_{m=1}^{n_{c_2}} \text{sgn}(v_m^{c_2}) \frac{1 - \text{sgn}(\delta_m^{c_2})}{2} \quad (\text{L56.2})$$

$$\mathcal{X}_1 = \sum_{m=1}^{n_{a_2}} \frac{1 - \text{sgn}(\delta_m^{a_2})}{2} + \sum_{m=1}^{n_{c_1}} \frac{1 - \text{sgn}(\delta_m^{c_1})}{2} \quad \text{mod } 2 \quad (\text{L56.3})$$

**L57. LAYER GROUP NO. 57**

| line segment                              | character of irrep (generators only)                          |
|-------------------------------------------|---------------------------------------------------------------|
| $a \quad (0, \frac{t}{2}, 0)$             | $\{2_{010}   0 \ 0 \ 0\}$<br>$a_1 \quad -i$<br>$a_2 \quad i$  |
| $b \quad (\frac{1-t}{2}, \frac{1}{2}, 0)$ | $\{2_{100}   0 \ 0 \ 0\}$<br>$b_1 \quad -i$<br>$b_2 \quad i$  |
| $c \quad (\frac{t}{2}, \frac{t}{2}, 0)$   | $\{m_{1-10}   0 \ 0 \ 0\}$<br>$c_1 \quad -i$<br>$c_2 \quad i$ |

$$\begin{aligned} \mathcal{W}_1^{\text{gapless}} = & \sum_{m=1}^{n_{a_1}} \text{sgn}(v_m^{a_1}) \frac{1 - \text{sgn}(\delta_m^{a_1})}{2} + \sum_{m=1}^{n_{a_2}} \text{sgn}(v_m^{a_2}) \frac{1 - \text{sgn}(\delta_m^{a_2})}{2} - \sum_{m=1}^{n_{b_1}} \text{sgn}(v_m^{b_1}) \frac{1 - \text{sgn}(\delta_m^{b_1})}{2} \\ & - \sum_{m=1}^{n_{b_2}} \text{sgn}(v_m^{b_2}) \frac{1 - \text{sgn}(\delta_m^{b_2})}{2} - \sum_{m=1}^{n_{c_1}} \text{sgn}(v_m^{c_1}) \frac{1 - \text{sgn}(\delta_m^{c_1})}{2} - \sum_{m=1}^{n_{c_2}} \text{sgn}(v_m^{c_2}) \frac{1 - \text{sgn}(\delta_m^{c_2})}{2} \end{aligned} \quad (\text{L57.1})$$

$$\mathcal{W}_1^{\text{gapped}} = - \sum_{m=1}^{n_{b_1}} \text{sgn}(v_m^{b_1}) \frac{1 - \text{sgn}(\delta_m^{b_1})}{2} + \sum_{m=1}^{n_{b_2}} \text{sgn}(v_m^{b_2}) \frac{1 - \text{sgn}(\delta_m^{b_2})}{2} \quad (\text{L57.2})$$

$$\mathcal{W}_2^{\text{gapped}} = - \sum_{m=1}^{n_{a_2}} \text{sgn}(v_m^{a_2}) \frac{1 - \text{sgn}(\delta_m^{a_2})}{2} + \sum_{m=1}^{n_{b_1}} \text{sgn}(v_m^{b_1}) \frac{1 - \text{sgn}(\delta_m^{b_1})}{2} + \sum_{m=1}^{n_{c_1}} \text{sgn}(v_m^{c_1}) \frac{1 - \text{sgn}(\delta_m^{c_1})}{2} \quad (\text{L57.3})$$

$$\mathcal{W}_3^{\text{gapped}} = - \sum_{m=1}^{n_{a_2}} \text{sgn}(v_m^{a_2}) \frac{1 - \text{sgn}(\delta_m^{a_2})}{2} + \sum_{m=1}^{n_{b_1}} \text{sgn}(v_m^{b_1}) \frac{1 - \text{sgn}(\delta_m^{b_1})}{2} + \sum_{m=1}^{n_{c_2}} \text{sgn}(v_m^{c_2}) \frac{1 - \text{sgn}(\delta_m^{c_2})}{2} \quad (\text{L57.4})$$

**L58. LAYER GROUP NO. 58**

| line segment                              | character of irrep (generators only)                                                                                             |
|-------------------------------------------|----------------------------------------------------------------------------------------------------------------------------------|
| $a \quad (0, \frac{t}{2}, 0)$             | $\{2_{010}   \frac{1}{2} \ \frac{1}{2} \ 0\}$<br>$a_1 \quad -ie^{-\frac{1}{2}i\pi t}$<br>$a_2 \quad ie^{-\frac{1}{2}i\pi t}$     |
| $b \quad (\frac{1-t}{2}, \frac{1}{2}, 0)$ | $\{2_{100}   \frac{1}{2} \ \frac{1}{2} \ 0\}$<br>$b_1 \quad -e^{-\frac{1}{2}i\pi(2-t)}$<br>$b_2 \quad e^{-\frac{1}{2}i\pi(2-t)}$ |
| $c \quad (\frac{t}{2}, \frac{t}{2}, 0)$   | $\{m_{1-10}   \frac{1}{2} \ \frac{1}{2} \ 0\}$<br>$c_1 \quad -ie^{-i\pi t}$<br>$c_2 \quad ie^{-i\pi t}$                          |

$$\begin{aligned} \mathcal{W}_1^{\text{gapless}} = & \sum_{m=1}^{n_{a_1}} \text{sgn}(v_m^{a_1}) \frac{1 - \text{sgn}(\delta_m^{a_1})}{2} + \sum_{m=1}^{n_{a_2}} \text{sgn}(v_m^{a_2}) \frac{1 - \text{sgn}(\delta_m^{a_2})}{2} - 2 \sum_{m=1}^{n_{b_1}} \text{sgn}(v_m^{b_1}) \frac{1 - \text{sgn}(\delta_m^{b_1})}{2} \\ & - \sum_{m=1}^{n_{c_1}} \text{sgn}(v_m^{c_1}) \frac{1 - \text{sgn}(\delta_m^{c_1})}{2} - \sum_{m=1}^{n_{c_2}} \text{sgn}(v_m^{c_2}) \frac{1 - \text{sgn}(\delta_m^{c_2})}{2} \end{aligned} \quad (\text{L58.1})$$

$$\mathcal{W}_1^{\text{gapped}} = - \sum_{m=1}^{n_{c_1}} \text{sgn}(v_m^{c_1}) \frac{1 - \text{sgn}(\delta_m^{c_1})}{2} + \sum_{m=1}^{n_{c_2}} \text{sgn}(v_m^{c_2}) \frac{1 - \text{sgn}(\delta_m^{c_2})}{2} \quad (\text{L58.2})$$

$$\mathcal{X}_1 = \sum_{m=1}^{n_{a_2}} \frac{1 - \text{sgn}(\delta_m^{a_2})}{2} + \sum_{m=1}^{n_{c_1}} \frac{1 - \text{sgn}(\delta_m^{c_1})}{2} \quad \text{mod } 2 \quad (\text{L58.3})$$

### L59. LAYER GROUP NO. 59

| line segment                              | character of irrep (generators only)                                                  |
|-------------------------------------------|---------------------------------------------------------------------------------------|
| $a \quad (0, \frac{t}{2}, 0)$             | $\begin{array}{c} \{m_{100}   0 \ 0 \ 0\} \\ a_1 \quad -i \\ a_2 \quad i \end{array}$ |
| $b \quad (\frac{1-t}{2}, \frac{1}{2}, 0)$ | $\begin{array}{c} \{m_{010}   0 \ 0 \ 0\} \\ b_1 \quad -i \\ b_2 \quad i \end{array}$ |
| $c \quad (\frac{t}{2}, \frac{t}{2}, 0)$   | $\begin{array}{c} \{2_{110}   0 \ 0 \ 0\} \\ c_1 \quad -i \\ c_2 \quad i \end{array}$ |

$$\begin{aligned} \mathcal{W}_1^{\text{gapless}} = & \sum_{m=1}^{n_{a_1}} \text{sgn}(v_m^{a_1}) \frac{1 - \text{sgn}(\delta_m^{a_1})}{2} + \sum_{m=1}^{n_{a_2}} \text{sgn}(v_m^{a_2}) \frac{1 - \text{sgn}(\delta_m^{a_2})}{2} - \sum_{m=1}^{n_{b_1}} \text{sgn}(v_m^{b_1}) \frac{1 - \text{sgn}(\delta_m^{b_1})}{2} \\ & - \sum_{m=1}^{n_{b_2}} \text{sgn}(v_m^{b_2}) \frac{1 - \text{sgn}(\delta_m^{b_2})}{2} - \sum_{m=1}^{n_{c_1}} \text{sgn}(v_m^{c_1}) \frac{1 - \text{sgn}(\delta_m^{c_1})}{2} - \sum_{m=1}^{n_{c_2}} \text{sgn}(v_m^{c_2}) \frac{1 - \text{sgn}(\delta_m^{c_2})}{2} \end{aligned} \quad (\text{L59.1})$$

$$\mathcal{W}_1^{\text{gapped}} = - \sum_{m=1}^{n_{b_1}} \text{sgn}(v_m^{b_1}) \frac{1 - \text{sgn}(\delta_m^{b_1})}{2} + \sum_{m=1}^{n_{b_2}} \text{sgn}(v_m^{b_2}) \frac{1 - \text{sgn}(\delta_m^{b_2})}{2} \quad (\text{L59.2})$$

$$\mathcal{W}_2^{\text{gapped}} = - \sum_{m=1}^{n_{a_2}} \text{sgn}(v_m^{a_2}) \frac{1 - \text{sgn}(\delta_m^{a_2})}{2} + \sum_{m=1}^{n_{b_1}} \text{sgn}(v_m^{b_1}) \frac{1 - \text{sgn}(\delta_m^{b_1})}{2} + \sum_{m=1}^{n_{c_1}} \text{sgn}(v_m^{c_1}) \frac{1 - \text{sgn}(\delta_m^{c_1})}{2} \quad (\text{L59.3})$$

$$\mathcal{W}_3^{\text{gapped}} = - \sum_{m=1}^{n_{a_2}} \text{sgn}(v_m^{a_2}) \frac{1 - \text{sgn}(\delta_m^{a_2})}{2} + \sum_{m=1}^{n_{b_1}} \text{sgn}(v_m^{b_1}) \frac{1 - \text{sgn}(\delta_m^{b_1})}{2} + \sum_{m=1}^{n_{c_2}} \text{sgn}(v_m^{c_2}) \frac{1 - \text{sgn}(\delta_m^{c_2})}{2} \quad (\text{L59.4})$$

### L60. LAYER GROUP NO. 60

| line segment | character of irrep (generators only) |
|--------------|--------------------------------------|
|--------------|--------------------------------------|

|                                           |                                                                                                                                                      |
|-------------------------------------------|------------------------------------------------------------------------------------------------------------------------------------------------------|
| $a \quad (0, \frac{t}{2}, 0)$             | $\begin{matrix} \{m_{100}   \frac{1}{2} \frac{1}{2} 0\} \\ a_1 \quad -ie^{-\frac{1}{2}i\pi t} \\ a_2 \quad ie^{-\frac{1}{2}i\pi t} \end{matrix}$     |
| $b \quad (\frac{1-t}{2}, \frac{1}{2}, 0)$ | $\begin{matrix} \{m_{010}   \frac{1}{2} \frac{1}{2} 0\} \\ b_1 \quad -e^{-\frac{1}{2}i\pi(2-t)} \\ b_2 \quad e^{-\frac{1}{2}i\pi(2-t)} \end{matrix}$ |
| $c \quad (\frac{t}{2}, \frac{t}{2}, 0)$   | $\begin{matrix} \{2_{110}   \frac{1}{2} \frac{1}{2} 0\} \\ c_1 \quad -ie^{-i\pi t} \\ c_2 \quad ie^{-i\pi t} \end{matrix}$                           |

$$\begin{aligned} \mathcal{W}_1^{\text{gapless}} = & \sum_{m=1}^{n_{a_1}} \text{sgn}(v_m^{a_1}) \frac{1 - \text{sgn}(\delta_m^{a_1})}{2} + \sum_{m=1}^{n_{a_2}} \text{sgn}(v_m^{a_2}) \frac{1 - \text{sgn}(\delta_m^{a_2})}{2} - 2 \sum_{m=1}^{n_{b_1}} \text{sgn}(v_m^{b_1}) \frac{1 - \text{sgn}(\delta_m^{b_1})}{2} \\ & - \sum_{m=1}^{n_{c_1}} \text{sgn}(v_m^{c_1}) \frac{1 - \text{sgn}(\delta_m^{c_1})}{2} - \sum_{m=1}^{n_{c_2}} \text{sgn}(v_m^{c_2}) \frac{1 - \text{sgn}(\delta_m^{c_2})}{2} \end{aligned} \quad (\text{L60.1})$$

$$\mathcal{W}_1^{\text{gapped}} = - \sum_{m=1}^{n_{c_1}} \text{sgn}(v_m^{c_1}) \frac{1 - \text{sgn}(\delta_m^{c_1})}{2} + \sum_{m=1}^{n_{c_2}} \text{sgn}(v_m^{c_2}) \frac{1 - \text{sgn}(\delta_m^{c_2})}{2} \quad (\text{L60.2})$$

$$\mathcal{X}_1 = \sum_{m=1}^{n_{a_2}} \frac{1 - \text{sgn}(\delta_m^{a_2})}{2} + \sum_{m=1}^{n_{c_1}} \frac{1 - \text{sgn}(\delta_m^{c_1})}{2} \quad \text{mod } 2 \quad (\text{L60.3})$$

### L61. LAYER GROUP NO. 61

| line segment                              | character of irrep (generators only)                                                       |
|-------------------------------------------|--------------------------------------------------------------------------------------------|
| $a \quad (0, \frac{t}{2}, 0)$             | $\begin{matrix} \{2_{010}   0 \ 0 \ 0\} & \{m_{100}   0 \ 0 \ 0\} \\ a_1 & 0 \end{matrix}$ |
| $b \quad (\frac{1-t}{2}, \frac{1}{2}, 0)$ | $\begin{matrix} \{2_{100}   0 \ 0 \ 0\} & \{m_{010}   0 \ 0 \ 0\} \\ b_1 & 0 \end{matrix}$ |
| $c \quad (\frac{t}{2}, \frac{t}{2}, 0)$   | $\begin{matrix} \{2_{110}   0 \ 0 \ 0\} & \{m_{001}   0 \ 0 \ 0\} \\ c_1 & 0 \end{matrix}$ |

$$\mathcal{W}_1^{\text{gapless}} = \sum_{m=1}^{n_{a_1}} \text{sgn}(v_m^{a_1}) \frac{1 - \text{sgn}(\delta_m^{a_1})}{2} - \sum_{m=1}^{n_{b_1}} \text{sgn}(v_m^{b_1}) \frac{1 - \text{sgn}(\delta_m^{b_1})}{2} - \sum_{m=1}^{n_{c_1}} \text{sgn}(v_m^{c_1}) \frac{1 - \text{sgn}(\delta_m^{c_1})}{2} \quad (\text{L61.1})$$

### L62. LAYER GROUP NO. 62

| line segment | character of irrep (generators only) |
|--------------|--------------------------------------|
|--------------|--------------------------------------|

|                                           |       |                                      |                                                |
|-------------------------------------------|-------|--------------------------------------|------------------------------------------------|
| $a \quad (0, \frac{t}{2}, 0)$             | $a_1$ | $\{2_{010}   \frac{1}{2} \ 0 \ 0 \}$ | $\{m_{100}   0 \ \frac{1}{2} \ 0 \}$           |
|                                           |       | $0$                                  | $0$                                            |
| $b \quad (\frac{1-t}{2}, \frac{1}{2}, 0)$ | $b_1$ | $\{2_{100}   0 \ \frac{1}{2} \ 0 \}$ | $\{m_{010}   \frac{1}{2} \ 0 \ 0 \}$           |
|                                           |       | $i$                                  | $-ie^{-\frac{1}{2}i\pi(1-t)}$                  |
|                                           | $b_2$ | $i$                                  | $ie^{-\frac{1}{2}i\pi(1-t)}$                   |
|                                           | $b_3$ | $-i$                                 | $-ie^{-\frac{1}{2}i\pi(1-t)}$                  |
|                                           | $b_4$ | $-i$                                 | $ie^{-\frac{1}{2}i\pi(1-t)}$                   |
| $c \quad (\frac{t}{2}, \frac{t}{2}, 0)$   | $c_1$ | $\{2_{110}   0 \ 0 \ 0 \}$           | $\{m_{001}   \frac{1}{2} \ \frac{1}{2} \ 0 \}$ |
|                                           |       | $0$                                  | $0$                                            |

$$\mathcal{W}_1^{\text{gapless}} = \sum_{m=1}^{n_{a_1}} \text{sgn}(v_m^{a_1}) \frac{1 - \text{sgn}(\delta_m^{a_1})}{2} - \sum_{m=1}^{n_{b_1}} \text{sgn}(v_m^{b_1}) \frac{1 - \text{sgn}(\delta_m^{b_1})}{2} - \sum_{m=1}^{n_{b_3}} \text{sgn}(v_m^{b_3}) \frac{1 - \text{sgn}(\delta_m^{b_3})}{2} - \sum_{m=1}^{n_{c_1}} \text{sgn}(v_m^{c_1}) \frac{1 - \text{sgn}(\delta_m^{c_1})}{2} \quad (\text{L62.1})$$

$$\mathcal{W}_1^{\text{gapped}} = \sum_{m=1}^{n_{b_1}} \text{sgn}(v_m^{b_1}) \frac{1 - \text{sgn}(\delta_m^{b_1})}{2} - \sum_{m=1}^{n_{b_3}} \text{sgn}(v_m^{b_3}) \frac{1 - \text{sgn}(\delta_m^{b_3})}{2} \quad (\text{L62.2})$$

### L63. LAYER GROUP NO. 63

| line segment                              | character of irrep (generators only) |                                                |                                                |
|-------------------------------------------|--------------------------------------|------------------------------------------------|------------------------------------------------|
| $a \quad (0, \frac{t}{2}, 0)$             | $a_1$                                | $\{2_{010}   \frac{1}{2} \ \frac{1}{2} \ 0 \}$ | $\{m_{100}   \frac{1}{2} \ \frac{1}{2} \ 0 \}$ |
|                                           |                                      | $0$                                            | $0$                                            |
| $b \quad (\frac{1-t}{2}, \frac{1}{2}, 0)$ | $b_1$                                | $\{2_{100}   \frac{1}{2} \ \frac{1}{2} \ 0 \}$ | $\{m_{010}   \frac{1}{2} \ \frac{1}{2} \ 0 \}$ |
|                                           |                                      | $0$                                            | $0$                                            |
| $c \quad (\frac{t}{2}, \frac{t}{2}, 0)$   | $c_1$                                | $\{2_{110}   \frac{1}{2} \ \frac{1}{2} \ 0 \}$ | $\{m_{001}   0 \ 0 \ 0 \}$                     |
|                                           |                                      | $0$                                            | $0$                                            |

$$\mathcal{W}_1^{\text{gapless}} = \sum_{m=1}^{n_{a_1}} \text{sgn}(v_m^{a_1}) \frac{1 - \text{sgn}(\delta_m^{a_1})}{2} - 2 \sum_{m=1}^{n_{b_1}} \text{sgn}(v_m^{b_1}) \frac{1 - \text{sgn}(\delta_m^{b_1})}{2} - \sum_{m=1}^{n_{c_1}} \text{sgn}(v_m^{c_1}) \frac{1 - \text{sgn}(\delta_m^{c_1})}{2} \quad (\text{L63.1})$$

### L64. LAYER GROUP NO. 64

| line segment                              | character of irrep (generators only) |                                                |                                                |
|-------------------------------------------|--------------------------------------|------------------------------------------------|------------------------------------------------|
| $a \quad (0, \frac{t}{2}, 0)$             | $a_1$                                | $\{2_{010}   0 \ \frac{1}{2} \ 0 \}$           | $\{m_{100}   \frac{1}{2} \ 0 \ 0 \}$           |
|                                           |                                      | $0$                                            | $0$                                            |
| $b \quad (\frac{1-t}{2}, \frac{1}{2}, 0)$ | $b_1$                                | $\{2_{100}   \frac{1}{2} \ 0 \ 0 \}$           | $\{m_{010}   0 \ \frac{1}{2} \ 0 \}$           |
|                                           |                                      | $-ie^{-\frac{1}{2}i\pi(1-t)}$                  | $i$                                            |
|                                           | $b_2$                                | $-ie^{-\frac{1}{2}i\pi(1-t)}$                  | $-i$                                           |
|                                           | $b_3$                                | $ie^{-\frac{1}{2}i\pi(1-t)}$                   | $i$                                            |
|                                           | $b_4$                                | $ie^{-\frac{1}{2}i\pi(1-t)}$                   | $-i$                                           |
| $c \quad (\frac{t}{2}, \frac{t}{2}, 0)$   | $c_1$                                | $\{2_{110}   \frac{1}{2} \ \frac{1}{2} \ 0 \}$ | $\{m_{001}   \frac{1}{2} \ \frac{1}{2} \ 0 \}$ |
|                                           |                                      | $0$                                            | $0$                                            |



---


$$\mathcal{W}_1^{\text{gapless}} = \sum_{m=1}^{n_{a_1}} \text{sgn}(v_m^{a_1}) \frac{1 - \text{sgn}(\delta_m^{a_1})}{2} - \sum_{m=1}^{n_{b_1}} \text{sgn}(v_m^{b_1}) \frac{1 - \text{sgn}(\delta_m^{b_1})}{2} - \sum_{m=1}^{n_{b_2}} \text{sgn}(v_m^{b_2}) \frac{1 - \text{sgn}(\delta_m^{b_2})}{2} - \sum_{m=1}^{n_{c_1}} \text{sgn}(v_m^{c_1}) \frac{1 - \text{sgn}(\delta_m^{c_1})}{2} \quad (\text{L64.1})$$

$$\mathcal{W}_1^{\text{gapped}} = \sum_{m=1}^{n_{b_1}} \text{sgn}(v_m^{b_1}) \frac{1 - \text{sgn}(\delta_m^{b_1})}{2} - \sum_{m=1}^{n_{b_2}} \text{sgn}(v_m^{b_2}) \frac{1 - \text{sgn}(\delta_m^{b_2})}{2} \quad (\text{L64.2})$$

#### L65. LAYER GROUP NO. 65

| line segment                                       | character of irrep (generators only)                            |
|----------------------------------------------------|-----------------------------------------------------------------|
| $a \left( \frac{2t}{3}, -\frac{t}{3}, 0 \right)$   | $\begin{array}{c} \{1  0 \ 0 \ 0 \} \\ a_1 \quad 1 \end{array}$ |
| $b \left( \frac{t+2}{6}, \frac{1-t}{3}, 0 \right)$ | $\begin{array}{c} \{1  0 \ 0 \ 0 \} \\ b_1 \quad 1 \end{array}$ |

$$\mathcal{X}_1 = \sum_{m=1}^{n_{a_1}} \frac{1 - \text{sgn}(\delta_m^{a_1})}{2} + \sum_{m=1}^{n_{b_1}} \frac{1 - \text{sgn}(\delta_m^{b_1})}{2} \quad \text{mod } 2 \quad (\text{L65.1})$$

#### L66. LAYER GROUP NO. 66

| line segment                                       | character of irrep (generators only)                            |
|----------------------------------------------------|-----------------------------------------------------------------|
| $a \left( \frac{2t}{3}, -\frac{t}{3}, 0 \right)$   | $\begin{array}{c} \{1  0 \ 0 \ 0 \} \\ a_1 \quad 1 \end{array}$ |
| $b \left( \frac{t+2}{6}, \frac{1-t}{3}, 0 \right)$ | $\begin{array}{c} \{1  0 \ 0 \ 0 \} \\ b_1 \quad 1 \end{array}$ |

#### L67. LAYER GROUP NO. 67

| line segment                                       | character of irrep (generators only)                                                  |
|----------------------------------------------------|---------------------------------------------------------------------------------------|
| $a \left( \frac{t}{2}, 0, 0 \right)$               | $\begin{array}{c} \{2_{210}  0 \ 0 \ 0 \} \\ a_1 \quad -i \\ a_2 \quad i \end{array}$ |
| $b \left( \frac{t}{3}, \frac{t}{3}, 0 \right)$     | $\begin{array}{c} \{1  0 \ 0 \ 0 \} \\ b_1 \quad 1 \end{array}$                       |
| $c \left( \frac{t+2}{6}, \frac{1-t}{3}, 0 \right)$ | $\begin{array}{c} \{1  0 \ 0 \ 0 \} \\ c_1 \quad 1 \end{array}$                       |

$$\mathcal{W}_1^{\text{gapless}} = \sum_{m=1}^{n_{a_1}} \text{sgn}(v_m^{a_1}) \frac{1 - \text{sgn}(\delta_m^{a_1})}{2} + \sum_{m=1}^{n_{a_2}} \text{sgn}(v_m^{a_2}) \frac{1 - \text{sgn}(\delta_m^{a_2})}{2} - \sum_{m=1}^{n_{b_1}} \text{sgn}(v_m^{b_1}) \frac{1 - \text{sgn}(\delta_m^{b_1})}{2} - \sum_{m=1}^{n_{c_1}} \text{sgn}(v_m^{c_1}) \frac{1 - \text{sgn}(\delta_m^{c_1})}{2} \quad (\text{L67.1})$$

$$\mathcal{W}_1^{\text{gapped}} = -2 \sum_{m=1}^{n_{a_2}} \text{sgn}(v_m^{a_2}) \frac{1 - \text{sgn}(\delta_m^{a_2})}{2} + \sum_{m=1}^{n_{b_1}} \text{sgn}(v_m^{b_1}) \frac{1 - \text{sgn}(\delta_m^{b_1})}{2} + \sum_{m=1}^{n_{c_1}} \text{sgn}(v_m^{c_1}) \frac{1 - \text{sgn}(\delta_m^{c_1})}{2} \quad (\text{L67.2})$$

### L68. LAYER GROUP NO. 68

| line segment                                       | character of irrep (generators only)                                                |
|----------------------------------------------------|-------------------------------------------------------------------------------------|
| $a \left( \frac{t}{2}, 0, 0 \right)$               | $\begin{array}{c} \{1 0 \ 0 \ 0\} \\ a_1 \quad 1 \end{array}$                       |
| $b \left( \frac{t}{3}, \frac{t}{3}, 0 \right)$     | $\begin{array}{c} \{2_{110} 0 \ 0 \ 0\} \\ b_1 \quad -i \\ b_2 \quad i \end{array}$ |
| $c \left( \frac{t+2}{6}, \frac{1-t}{3}, 0 \right)$ | $\begin{array}{c} \{2_{010} 0 \ 0 \ 0\} \\ c_1 \quad -i \\ c_2 \quad i \end{array}$ |

$$\begin{aligned} \mathcal{W}_1^{\text{gapless}} = & \sum_{m=1}^{n_{a_1}} \text{sgn}(v_m^{a_1}) \frac{1 - \text{sgn}(\delta_m^{a_1})}{2} - \sum_{m=1}^{n_{b_1}} \text{sgn}(v_m^{b_1}) \frac{1 - \text{sgn}(\delta_m^{b_1})}{2} - \sum_{m=1}^{n_{b_2}} \text{sgn}(v_m^{b_2}) \frac{1 - \text{sgn}(\delta_m^{b_2})}{2} \\ & - \sum_{m=1}^{n_{c_1}} \text{sgn}(v_m^{c_1}) \frac{1 - \text{sgn}(\delta_m^{c_1})}{2} - \sum_{m=1}^{n_{c_2}} \text{sgn}(v_m^{c_2}) \frac{1 - \text{sgn}(\delta_m^{c_2})}{2} \end{aligned} \quad (\text{L68.1})$$

$$\mathcal{W}_1^{\text{gapped}} = - \sum_{m=1}^{n_{b_1}} \text{sgn}(v_m^{b_1}) \frac{1 - \text{sgn}(\delta_m^{b_1})}{2} + \sum_{m=1}^{n_{b_2}} \text{sgn}(v_m^{b_2}) \frac{1 - \text{sgn}(\delta_m^{b_2})}{2} - \sum_{m=1}^{n_{c_1}} \text{sgn}(v_m^{c_1}) \frac{1 - \text{sgn}(\delta_m^{c_1})}{2} + \sum_{m=1}^{n_{c_2}} \text{sgn}(v_m^{c_2}) \frac{1 - \text{sgn}(\delta_m^{c_2})}{2} \quad (\text{L68.2})$$

### L69. LAYER GROUP NO. 69

| line segment                                       | character of irrep (generators only)                                                |
|----------------------------------------------------|-------------------------------------------------------------------------------------|
| $a \left( \frac{t}{2}, 0, 0 \right)$               | $\begin{array}{c} \{m_{010} 0 \ 0 \ 0\} \\ a_1 \quad -i \\ a_2 \quad i \end{array}$ |
| $b \left( \frac{t}{3}, \frac{t}{3}, 0 \right)$     | $\begin{array}{c} \{1 0 \ 0 \ 0\} \\ b_1 \quad 1 \end{array}$                       |
| $c \left( \frac{t+2}{6}, \frac{1-t}{3}, 0 \right)$ | $\begin{array}{c} \{1 0 \ 0 \ 0\} \\ c_1 \quad 1 \end{array}$                       |

$$\mathcal{W}_1^{\text{gapless}} = \sum_{m=1}^{n_{a_1}} \text{sgn}(v_m^{a_1}) \frac{1 - \text{sgn}(\delta_m^{a_1})}{2} + \sum_{m=1}^{n_{a_2}} \text{sgn}(v_m^{a_2}) \frac{1 - \text{sgn}(\delta_m^{a_2})}{2} - \sum_{m=1}^{n_{b_1}} \text{sgn}(v_m^{b_1}) \frac{1 - \text{sgn}(\delta_m^{b_1})}{2} - \sum_{m=1}^{n_{c_1}} \text{sgn}(v_m^{c_1}) \frac{1 - \text{sgn}(\delta_m^{c_1})}{2} \quad (\text{L69.1})$$

$$\mathcal{W}_1^{\text{gapped}} = -2 \sum_{m=1}^{n_{a_2}} \text{sgn}(v_m^{a_2}) \frac{1 - \text{sgn}(\delta_m^{a_2})}{2} + \sum_{m=1}^{n_{b_1}} \text{sgn}(v_m^{b_1}) \frac{1 - \text{sgn}(\delta_m^{b_1})}{2} + \sum_{m=1}^{n_{c_1}} \text{sgn}(v_m^{c_1}) \frac{1 - \text{sgn}(\delta_m^{c_1})}{2} \quad (\text{L69.2})$$

#### L70. LAYER GROUP NO. 70

| line segment                                       | character of irrep (generators only)                                                   |
|----------------------------------------------------|----------------------------------------------------------------------------------------|
| $a \left( \frac{t}{2}, 0, 0 \right)$               | $\begin{array}{c} \{1  0 \ 0 \ 0 \} \\ a_1 \quad 1 \end{array}$                        |
| $b \left( \frac{t}{3}, \frac{t}{3}, 0 \right)$     | $\begin{array}{c} \{m_{-110}  0 \ 0 \ 0 \} \\ b_1 \quad -i \\ b_2 \quad i \end{array}$ |
| $c \left( \frac{t+2}{6}, \frac{1-t}{3}, 0 \right)$ | $\begin{array}{c} \{m_{210}  0 \ 0 \ 0 \} \\ c_1 \quad -i \\ c_2 \quad i \end{array}$  |

$$\begin{aligned} \mathcal{W}_1^{\text{gapless}} = & \sum_{m=1}^{n_{a_1}} \text{sgn}(v_m^{a_1}) \frac{1 - \text{sgn}(\delta_m^{a_1})}{2} - \sum_{m=1}^{n_{b_1}} \text{sgn}(v_m^{b_1}) \frac{1 - \text{sgn}(\delta_m^{b_1})}{2} - \sum_{m=1}^{n_{b_2}} \text{sgn}(v_m^{b_2}) \frac{1 - \text{sgn}(\delta_m^{b_2})}{2} \\ & - \sum_{m=1}^{n_{c_1}} \text{sgn}(v_m^{c_1}) \frac{1 - \text{sgn}(\delta_m^{c_1})}{2} - \sum_{m=1}^{n_{c_2}} \text{sgn}(v_m^{c_2}) \frac{1 - \text{sgn}(\delta_m^{c_2})}{2} \end{aligned} \quad (\text{L70.1})$$

$$\mathcal{W}_1^{\text{gapped}} = \sum_{m=1}^{n_{b_1}} \text{sgn}(v_m^{b_1}) \frac{1 - \text{sgn}(\delta_m^{b_1})}{2} - \sum_{m=1}^{n_{b_2}} \text{sgn}(v_m^{b_2}) \frac{1 - \text{sgn}(\delta_m^{b_2})}{2} - \sum_{m=1}^{n_{c_1}} \text{sgn}(v_m^{c_1}) \frac{1 - \text{sgn}(\delta_m^{c_1})}{2} + \sum_{m=1}^{n_{c_2}} \text{sgn}(v_m^{c_2}) \frac{1 - \text{sgn}(\delta_m^{c_2})}{2} \quad (\text{L70.2})$$

#### L71. LAYER GROUP NO. 71

| line segment                                       | character of irrep (generators only)                                                   |
|----------------------------------------------------|----------------------------------------------------------------------------------------|
| $a \left( \frac{t}{2}, 0, 0 \right)$               | $\begin{array}{c} \{2_{210}  0 \ 0 \ 0 \} \\ a_1 \quad -i \\ a_2 \quad i \end{array}$  |
| $b \left( \frac{t}{3}, \frac{t}{3}, 0 \right)$     | $\begin{array}{c} \{m_{-110}  0 \ 0 \ 0 \} \\ b_1 \quad -i \\ b_2 \quad i \end{array}$ |
| $c \left( \frac{t+2}{6}, \frac{1-t}{3}, 0 \right)$ | $\begin{array}{c} \{m_{210}  0 \ 0 \ 0 \} \\ c_1 \quad -i \\ c_2 \quad i \end{array}$  |

---


$$\mathcal{W}_1^{\text{gapless}} = \sum_{m=1}^{n_{a_1}} \text{sgn}(v_m^{a_1}) \frac{1 - \text{sgn}(\delta_m^{a_1})}{2} - \sum_{m=1}^{n_{b_1}} \text{sgn}(v_m^{b_1}) \frac{1 - \text{sgn}(\delta_m^{b_1})}{2} - \sum_{m=1}^{n_{c_1}} \text{sgn}(v_m^{c_1}) \frac{1 - \text{sgn}(\delta_m^{c_1})}{2} \quad (\text{L71.1})$$

**L72. LAYER GROUP NO. 72**

| line segment                                       | character of irrep (generators only)                                                  |
|----------------------------------------------------|---------------------------------------------------------------------------------------|
| $a \left( \frac{t}{2}, 0, 0 \right)$               | $\begin{array}{c} \{m_{010}   0 \ 0 \ 0\} \\ a_1 \quad -i \\ a_2 \quad i \end{array}$ |
| $b \left( \frac{t}{3}, \frac{t}{3}, 0 \right)$     | $\begin{array}{c} \{2_{110}   0 \ 0 \ 0\} \\ b_1 \quad -i \\ b_2 \quad i \end{array}$ |
| $c \left( \frac{t+2}{6}, \frac{1-t}{3}, 0 \right)$ | $\begin{array}{c} \{2_{010}   0 \ 0 \ 0\} \\ c_1 \quad -i \\ c_2 \quad i \end{array}$ |

$$\mathcal{W}_1^{\text{gapless}} = \sum_{m=1}^{n_{a_1}} \text{sgn}(v_m^{a_1}) \frac{1 - \text{sgn}(\delta_m^{a_1})}{2} - \sum_{m=1}^{n_{b_1}} \text{sgn}(v_m^{b_1}) \frac{1 - \text{sgn}(\delta_m^{b_1})}{2} - \sum_{m=1}^{n_{c_1}} \text{sgn}(v_m^{c_1}) \frac{1 - \text{sgn}(\delta_m^{c_1})}{2} \quad (\text{L72.1})$$

**L73. LAYER GROUP NO. 73**

| line segment                                       | character of irrep (generators only)                            |
|----------------------------------------------------|-----------------------------------------------------------------|
| $a \left( \frac{2t}{3}, -\frac{t}{3}, 0 \right)$   | $\begin{array}{c} \{1   0 \ 0 \ 0\} \\ a_1 \quad 1 \end{array}$ |
| $b \left( \frac{t+2}{6}, \frac{1-t}{3}, 0 \right)$ | $\begin{array}{c} \{1   0 \ 0 \ 0\} \\ b_1 \quad 1 \end{array}$ |

$$\mathcal{X}_1 = \sum_{m=1}^{n_{a_1}} \frac{1 - \text{sgn}(\delta_m^{a_1})}{2} + \sum_{m=1}^{n_{b_1}} \frac{1 - \text{sgn}(\delta_m^{b_1})}{2} \quad \text{mod } 2 \quad (\text{L73.1})$$

**L74. LAYER GROUP NO. 74**

| line segment                                       | character of irrep (generators only)                                                  |
|----------------------------------------------------|---------------------------------------------------------------------------------------|
| $a \left( \frac{2t}{3}, -\frac{t}{3}, 0 \right)$   | $\begin{array}{c} \{m_{001}   0 \ 0 \ 0\} \\ a_1 \quad -i \\ a_2 \quad i \end{array}$ |
| $b \left( \frac{t+2}{6}, \frac{1-t}{3}, 0 \right)$ | $\begin{array}{c} \{m_{001}   0 \ 0 \ 0\} \\ b_1 \quad -i \\ b_2 \quad i \end{array}$ |

$$\mathcal{W}_1^{\text{gapless}} = \sum_{m=1}^{n_{a_1}} \text{sgn}(v_m^{a_1}) \frac{1 - \text{sgn}(\delta_m^{a_1})}{2} - \sum_{m=1}^{n_{a_2}} \text{sgn}(v_m^{a_2}) \frac{1 - \text{sgn}(\delta_m^{a_2})}{2} - \sum_{m=1}^{n_{b_1}} \text{sgn}(v_m^{b_1}) \frac{1 - \text{sgn}(\delta_m^{b_1})}{2} + \sum_{m=1}^{n_{b_2}} \text{sgn}(v_m^{b_2}) \frac{1 - \text{sgn}(\delta_m^{b_2})}{2} \quad (\text{L74.1})$$

#### L75. LAYER GROUP NO. 75

| line segment                                       | character of irrep (generators only)                                                  |
|----------------------------------------------------|---------------------------------------------------------------------------------------|
| $a \left( \frac{2t}{3}, -\frac{t}{3}, 0 \right)$   | $\begin{array}{c} \{m_{001}   0 \ 0 \ 0\} \\ a_1 \quad -i \\ a_2 \quad i \end{array}$ |
| $b \left( \frac{t+2}{6}, \frac{1-t}{3}, 0 \right)$ | $\begin{array}{c} \{m_{001}   0 \ 0 \ 0\} \\ b_1 \quad -i \\ b_2 \quad i \end{array}$ |

#### L76. LAYER GROUP NO. 76

| line segment                                       | character of irrep (generators only)                                                  |
|----------------------------------------------------|---------------------------------------------------------------------------------------|
| $a \left( \frac{t}{2}, 0, 0 \right)$               | $\begin{array}{c} \{2_{210}   0 \ 0 \ 0\} \\ a_1 \quad -i \\ a_2 \quad i \end{array}$ |
| $b \left( \frac{t}{3}, \frac{t}{3}, 0 \right)$     | $\begin{array}{c} \{2_{110}   0 \ 0 \ 0\} \\ b_1 \quad -i \\ b_2 \quad i \end{array}$ |
| $c \left( \frac{t+2}{6}, \frac{1-t}{3}, 0 \right)$ | $\begin{array}{c} \{2_{010}   0 \ 0 \ 0\} \\ c_1 \quad -i \\ c_2 \quad i \end{array}$ |

$$\begin{aligned} \mathcal{W}_1^{\text{gapless}} = & \sum_{m=1}^{n_{a_1}} \text{sgn}(v_m^{a_1}) \frac{1 - \text{sgn}(\delta_m^{a_1})}{2} + \sum_{m=1}^{n_{a_2}} \text{sgn}(v_m^{a_2}) \frac{1 - \text{sgn}(\delta_m^{a_2})}{2} - \sum_{m=1}^{n_{b_1}} \text{sgn}(v_m^{b_1}) \frac{1 - \text{sgn}(\delta_m^{b_1})}{2} \\ & - \sum_{m=1}^{n_{b_2}} \text{sgn}(v_m^{b_2}) \frac{1 - \text{sgn}(\delta_m^{b_2})}{2} - \sum_{m=1}^{n_{c_1}} \text{sgn}(v_m^{c_1}) \frac{1 - \text{sgn}(\delta_m^{c_1})}{2} - \sum_{m=1}^{n_{c_2}} \text{sgn}(v_m^{c_2}) \frac{1 - \text{sgn}(\delta_m^{c_2})}{2} \end{aligned} \quad (\text{L76.1})$$

$$\mathcal{W}_1^{\text{gapped}} = - \sum_{m=1}^{n_{a_2}} \text{sgn}(v_m^{a_2}) \frac{1 - \text{sgn}(\delta_m^{a_2})}{2} + \sum_{m=1}^{n_{b_1}} \text{sgn}(v_m^{b_1}) \frac{1 - \text{sgn}(\delta_m^{b_1})}{2} + \sum_{m=1}^{n_{c_1}} \text{sgn}(v_m^{c_1}) \frac{1 - \text{sgn}(\delta_m^{c_1})}{2} \quad (\text{L76.2})$$

$$\mathcal{W}_2^{\text{gapped}} = - \sum_{m=1}^{n_{a_2}} \text{sgn}(v_m^{a_2}) \frac{1 - \text{sgn}(\delta_m^{a_2})}{2} + \sum_{m=1}^{n_{b_2}} \text{sgn}(v_m^{b_2}) \frac{1 - \text{sgn}(\delta_m^{b_2})}{2} + \sum_{m=1}^{n_{c_2}} \text{sgn}(v_m^{c_2}) \frac{1 - \text{sgn}(\delta_m^{c_2})}{2} \quad (\text{L76.3})$$

**L77. LAYER GROUP NO. 77**

| line segment                                       | character of irrep (generators only)                                                   |
|----------------------------------------------------|----------------------------------------------------------------------------------------|
| $a \left( \frac{t}{2}, 0, 0 \right)$               | $\begin{array}{c} \{m_{010}   0 \ 0 \ 0\} \\ a_1 \quad -i \\ a_2 \quad i \end{array}$  |
| $b \left( \frac{t}{3}, \frac{t}{3}, 0 \right)$     | $\begin{array}{c} \{m_{-110}   0 \ 0 \ 0\} \\ b_1 \quad -i \\ b_2 \quad i \end{array}$ |
| $c \left( \frac{t+2}{6}, \frac{1-t}{3}, 0 \right)$ | $\begin{array}{c} \{m_{210}   0 \ 0 \ 0\} \\ c_1 \quad -i \\ c_2 \quad i \end{array}$  |

$$\begin{aligned} \mathcal{W}_1^{\text{gapless}} = & \sum_{m=1}^{n_{a_1}} \text{sgn}(v_m^{a_1}) \frac{1 - \text{sgn}(\delta_m^{a_1})}{2} + \sum_{m=1}^{n_{a_2}} \text{sgn}(v_m^{a_2}) \frac{1 - \text{sgn}(\delta_m^{a_2})}{2} - \sum_{m=1}^{n_{b_1}} \text{sgn}(v_m^{b_1}) \frac{1 - \text{sgn}(\delta_m^{b_1})}{2} \\ & - \sum_{m=1}^{n_{b_2}} \text{sgn}(v_m^{b_2}) \frac{1 - \text{sgn}(\delta_m^{b_2})}{2} - \sum_{m=1}^{n_{c_1}} \text{sgn}(v_m^{c_1}) \frac{1 - \text{sgn}(\delta_m^{c_1})}{2} - \sum_{m=1}^{n_{c_2}} \text{sgn}(v_m^{c_2}) \frac{1 - \text{sgn}(\delta_m^{c_2})}{2} \end{aligned} \quad (\text{L77.1})$$

$$\mathcal{W}_1^{\text{gapped}} = - \sum_{m=1}^{n_{a_2}} \text{sgn}(v_m^{a_2}) \frac{1 - \text{sgn}(\delta_m^{a_2})}{2} + \sum_{m=1}^{n_{b_2}} \text{sgn}(v_m^{b_2}) \frac{1 - \text{sgn}(\delta_m^{b_2})}{2} + \sum_{m=1}^{n_{c_1}} \text{sgn}(v_m^{c_1}) \frac{1 - \text{sgn}(\delta_m^{c_1})}{2} \quad (\text{L77.2})$$

$$\mathcal{W}_2^{\text{gapped}} = - \sum_{m=1}^{n_{a_2}} \text{sgn}(v_m^{a_2}) \frac{1 - \text{sgn}(\delta_m^{a_2})}{2} + \sum_{m=1}^{n_{b_1}} \text{sgn}(v_m^{b_1}) \frac{1 - \text{sgn}(\delta_m^{b_1})}{2} + \sum_{m=1}^{n_{c_2}} \text{sgn}(v_m^{c_2}) \frac{1 - \text{sgn}(\delta_m^{c_2})}{2} \quad (\text{L77.3})$$

**L78. LAYER GROUP NO. 78**

| line segment                                       | character of irrep (generators only)                                                                    |
|----------------------------------------------------|---------------------------------------------------------------------------------------------------------|
| $a \left( \frac{t}{2}, 0, 0 \right)$               | $\begin{array}{c} \{2_{210}   0 \ 0 \ 0\} \ \{m_{001}   0 \ 0 \ 0\} \\ a_1 \quad 0 \quad 0 \end{array}$ |
| $b \left( \frac{t}{3}, \frac{t}{3}, 0 \right)$     | $\begin{array}{c} \{m_{001}   0 \ 0 \ 0\} \\ b_1 \quad -i \\ b_2 \quad i \end{array}$                   |
| $c \left( \frac{t+2}{6}, \frac{1-t}{3}, 0 \right)$ | $\begin{array}{c} \{m_{001}   0 \ 0 \ 0\} \\ c_1 \quad -i \\ c_2 \quad i \end{array}$                   |

$$\mathcal{W}_1^{\text{gapless}} = \sum_{m=1}^{n_{a_1}} \text{sgn}(v_m^{a_1}) \frac{1 - \text{sgn}(\delta_m^{a_1})}{2} - \sum_{m=1}^{n_{b_2}} \text{sgn}(v_m^{b_2}) \frac{1 - \text{sgn}(\delta_m^{b_2})}{2} - \sum_{m=1}^{n_{c_2}} \text{sgn}(v_m^{c_2}) \frac{1 - \text{sgn}(\delta_m^{c_2})}{2} \quad (\text{L78.1})$$

$$\mathcal{W}_2^{\text{gapless}} = \sum_{m=1}^{n_{b_1}} \text{sgn}(v_m^{b_1}) \frac{1 - \text{sgn}(\delta_m^{b_1})}{2} - \sum_{m=1}^{n_{b_2}} \text{sgn}(v_m^{b_2}) \frac{1 - \text{sgn}(\delta_m^{b_2})}{2} + \sum_{m=1}^{n_{c_1}} \text{sgn}(v_m^{c_1}) \frac{1 - \text{sgn}(\delta_m^{c_1})}{2} - \sum_{m=1}^{n_{c_2}} \text{sgn}(v_m^{c_2}) \frac{1 - \text{sgn}(\delta_m^{c_2})}{2} \quad (\text{L78.2})$$

**L79. LAYER GROUP NO. 79**

| line segment                                       | character of irrep (generators only)                                                             |
|----------------------------------------------------|--------------------------------------------------------------------------------------------------|
| $a \left( \frac{t}{2}, 0, 0 \right)$               | $\begin{matrix} \{m_{001}  0 & 0 & 0 \} \\ a_1 & -i \\ a_2 & i \end{matrix}$                     |
| $b \left( \frac{t}{3}, \frac{t}{3}, 0 \right)$     | $\begin{matrix} \{2_{110}  0 & 0 & 0 \} & \{m_{001}  0 & 0 & 0 \} \\ b_1 & 0 & & 0 \end{matrix}$ |
| $c \left( \frac{t+2}{6}, \frac{1-t}{3}, 0 \right)$ | $\begin{matrix} \{2_{010}  0 & 0 & 0 \} & \{m_{001}  0 & 0 & 0 \} \\ c_1 & 0 & & 0 \end{matrix}$ |

$$\mathcal{W}_1^{\text{gapless}} = \sum_{m=1}^{n_{a_1}} \text{sgn}(v_m^{a_1}) \frac{1 - \text{sgn}(\delta_m^{a_1})}{2} - \sum_{m=1}^{n_{b_1}} \text{sgn}(v_m^{b_1}) \frac{1 - \text{sgn}(\delta_m^{b_1})}{2} - \sum_{m=1}^{n_{c_1}} \text{sgn}(v_m^{c_1}) \frac{1 - \text{sgn}(\delta_m^{c_1})}{2} \quad (\text{L79.1})$$

$$\mathcal{W}_2^{\text{gapless}} = \sum_{m=1}^{n_{a_2}} \text{sgn}(v_m^{a_2}) \frac{1 - \text{sgn}(\delta_m^{a_2})}{2} - \sum_{m=1}^{n_{b_1}} \text{sgn}(v_m^{b_1}) \frac{1 - \text{sgn}(\delta_m^{b_1})}{2} - \sum_{m=1}^{n_{c_1}} \text{sgn}(v_m^{c_1}) \frac{1 - \text{sgn}(\delta_m^{c_1})}{2} \quad (\text{L79.2})$$

**L80. LAYER GROUP NO. 80**

| line segment                                       | character of irrep (generators only)                                                             |
|----------------------------------------------------|--------------------------------------------------------------------------------------------------|
| $a \left( \frac{t}{2}, 0, 0 \right)$               | $\begin{matrix} \{2_{210}  0 & 0 & 0 \} & \{m_{001}  0 & 0 & 0 \} \\ a_1 & 0 & & 0 \end{matrix}$ |
| $b \left( \frac{t}{3}, \frac{t}{3}, 0 \right)$     | $\begin{matrix} \{2_{110}  0 & 0 & 0 \} & \{m_{001}  0 & 0 & 0 \} \\ b_1 & 0 & & 0 \end{matrix}$ |
| $c \left( \frac{t+2}{6}, \frac{1-t}{3}, 0 \right)$ | $\begin{matrix} \{2_{010}  0 & 0 & 0 \} & \{m_{001}  0 & 0 & 0 \} \\ c_1 & 0 & & 0 \end{matrix}$ |

$$\mathcal{W}_1^{\text{gapless}} = \sum_{m=1}^{n_{a_1}} \text{sgn}(v_m^{a_1}) \frac{1 - \text{sgn}(\delta_m^{a_1})}{2} - \sum_{m=1}^{n_{b_1}} \text{sgn}(v_m^{b_1}) \frac{1 - \text{sgn}(\delta_m^{b_1})}{2} - \sum_{m=1}^{n_{c_1}} \text{sgn}(v_m^{c_1}) \frac{1 - \text{sgn}(\delta_m^{c_1})}{2} \quad (\text{L80.1})$$
